# Supplementary material for: A Zone of Avoidance catalogue of 2MASS bright galaxies. I. Sample description and analysis
Source: arXiv:1811.02773 ancillary file (2018-11-07)
Supplement: Supplementary file 1 [file Aschroeder_supplement.pdf]

**APPENDIX B: ONLINE MATERIAL**

Table B1: a) 2MASX ZoA sample

30

| 2MASX J          | <i>l</i> | <i>b</i> | EBV    | Object | Sample | Disc | 2MRS | Velocity | NIR   | Photom | Ext | <i>K</i> <sub>20</sub> | <i>H-K</i> | <i>J-K</i> | vc   | <i>a</i> | <i>b/a</i> | st.d.  | <i>K</i> <sub>s</sub> <sup>o</sup> | ( <i>H-K</i> ) <sup>o</sup> | ( <i>J-K</i> ) <sup>o</sup> | <i>A<sub>K</sub></i> | <i>a</i> <sub>d</sub> <sup>o</sup> | <i>K</i> <sub>s</sub> <sup>o,d</sup> | ( <i>H-K</i> ) <sup>o,c</sup> | ( <i>J-K</i> ) <sup>o,c</sup> |       |      |      |       |       |       |
|------------------|----------|----------|--------|--------|--------|------|------|----------|-------|--------|-----|------------------------|------------|------------|------|----------|------------|--------|------------------------------------|-----------------------------|-----------------------------|----------------------|------------------------------------|--------------------------------------|-------------------------------|-------------------------------|-------|------|------|-------|-------|-------|
| (1)              | deg      | deg      | mag    | class  | off    | gal  | TF   | obs      | ext'd | type   | Opt | HI                     | mag        | mag        | (17) | (18)     | (19)       | (20)   | mag                                | mag                         | mag                         | mag                  | "                                  | mag                                  | mag                           | mag                           |       |      |      |       |       |       |
| (1)              | (2a)     | (2b)     | (3)    | (4)    | (5)    | (6)  | (7a) | (7c)     | (7d)  | (8)    | (9) | (10a)                  | (10b)      | (11)       | (12) | (13)     | (14)       | (15)   | (16)                               | (17)                        | (18)                        | (19)                 | (20)                               | (21)                                 | (22)                          | (23)                          | (24)  | (25) | (26) | (27)  | (28)  |       |
| 00000637+5319136 | 115.217  | -8.780   | 0.300  | 1      | -      | -    | g    | -        | -     | -      | D4  | c                      | o          | -          | -    | -        | -          | 11.196 | 0.42                               | 1.15                        | 1                           | 35.0                 | 0.90                               | 3.59                                 | 11.084                        | 0.37                          | 1.00  | 0.09 | 35.6 | 11.09 | 0.38  | 1.02  |
| 00000702+6717254 | 117.996  | 4.912    | 10.331 | 9      | -      | -    | -    | -        | -     | -      | -   | -                      | -          | -          | -    | -        | -          | 13.614 | 0.53                               | 1.38                        | -1                          | 11.0                 | 1.00                               | 3.63                                 | 9.765                         | -1.18                         | -3.75 | 3.20 | ...  | ...   | -0.98 | -3.07 |
| 00001859+6716444 | 118.012  | 4.897    | 9.743  | 9      | -      | -    | -    | -        | -     | -      | -   | -                      | -          | -          | -    | -        | -          | 14.306 | 0.36                               | 1.30                        | -1                          | 10.0                 | 1.00                               | 3.63                                 | 10.676                        | -1.26                         | -3.54 | 3.02 | ...  | ...   | -1.06 | -2.89 |
| 00002049+6717044 | 118.016  | 4.902    | 9.880  | 9      | -      | -    | -    | -        | -     | -      | -   | -                      | -          | -          | -    | -        | -          | 13.371 | 0.60                               | 1.61                        | -1                          | 19.4                 | 0.54                               | 3.63                                 | 9.690                         | -1.04                         | -3.30 | 3.06 | ...  | ...   | -0.84 | -2.65 |
| 00003760+6735164 | 118.103  | 5.194    | 4.645  | 8      | -      | -    | -    | -        | -     | -      | -   | -                      | -          | -          | -    | -        | -          | 12.242 | 0.50                               | 1.47                        | -2                          | 22.6                 | 0.34                               | 3.91                                 | 10.511                        | -0.27                         | -0.83 | 1.44 | ...  | ...   | -0.18 | -0.53 |
| 00003769+6710184 | 118.021  | 4.786    | 6.767  | 8      | -      | -    | -    | -        | -     | -      | -   | -                      | -          | -          | -    | -        | -          | 12.635 | 1.11                               | ...                         | 1                           | 37.2                 | 0.46                               | 3.63                                 | 10.114                        | -0.01                         | ...   | 2.10 | ...  | ...   | 0.12  | ...   |
| 00004194+6838344 | 118.318  | 6.227    | 0.957  | 7      | -      | -    | -    | -        | -     | -      | -   | -                      | -          | -          | -    | -        | -          | 9.622  | 1.60                               | 3.34                        | 1                           | 23.2                 | 0.78                               | 3.67                                 | 9.265                         | 1.44                          | 2.87  | 0.30 | ...  | ...   | 1.46  | 2.93  |
| 00004647+6732523 | 118.109  | 5.152    | 6.505  | 8      | -      | -    | -    | -        | -     | -      | -   | -                      | -          | -          | -    | -        | -          | 10.986 | 1.17                               | 3.21                        | 1                           | 42.4                 | 0.62                               | 3.91                                 | 8.562                         | 0.09                          | -0.02 | 2.01 | ...  | ...   | 0.22  | 0.41  |
| 00013723+6436560 | 117.623  | 2.259    | 4.572  | 9      | -      | -    | -    | -        | -     | -      | -   | -                      | -          | -          | -    | -        | -          | 12.737 | 0.35                               | 1.33                        | -2                          | 17.8                 | 0.70                               | 3.94                                 | 11.033                        | -0.41                         | -0.95 | 1.42 | ...  | ...   | -0.32 | -0.64 |
| 00013755+6437360 | 117.626  | 2.270    | 4.633  | 9      | -      | -    | -    | -        | -     | -      | -   | -                      | -          | -          | -    | -        | -          | 11.735 | 0.41                               | 1.23                        | 1                           | 37.2                 | 0.80                               | 3.94                                 | 10.009                        | -0.36                         | -1.08 | 1.44 | ...  | ...   | -0.27 | -0.77 |
| 00014201+6724323 | 118.169  | 4.999    | 7.957  | 8      | -      | -    | -    | -        | -     | -      | -   | -                      | -          | -          | -    | -        | -          | 13.778 | 0.56                               | 1.28                        | -1                          | 13.6                 | 1.00                               | 3.94                                 | 10.813                        | -0.76                         | -2.67 | 2.46 | ...  | ...   | -0.60 | -2.14 |
| 00014668+6708413 | 118.126  | 4.738    | 4.218  | 8      | -      | -    | -    | -        | -     | -      | -   | -                      | -          | -          | -    | -        | -          | 11.590 | 1.18                               | 2.17                        | 1                           | 61.8                 | 0.52                               | 3.79                                 | 10.018                        | 0.48                          | 0.07  | 1.31 | ...  | ...   | 0.57  | 0.35  |
| 00031331+5352149 | 115.783  | -8.330   | 0.299  | 1      | -      | -    | -    | -        | -     | -      | D3  | c                      | o          | -          | -    | -        | -          | 10.252 | 0.37                               | 1.20                        | 1                           | 48.6                 | 0.78                               | 3.57                                 | 10.141                        | 0.32                          | 1.05  | 0.09 | 49.3 | 10.15 | 0.33  | 1.07  |
| 00033726+6919064 | 118.707  | 6.840    | 0.808  | 2      | -      | -    | -    | -        | -     | -      | -   | -                      | -          | -          | -    | -        | -          | 11.480 | 0.40                               | 1.50                        | 1                           | 26.4                 | 0.70                               | 3.60                                 | 11.179                        | 0.27                          | 1.10  | 0.25 | 28.1 | 11.19 | 0.28  | 1.15  |
| 00034142+7036434 | 118.955  | 8.110    | 0.789  | 1      | -      | -    | -    | -        | -     | -      | D4  | c                      | o          | -          | -    | -        | -          | 11.544 | 0.35                               | 1.29                        | 1                           | 36.6                 | 0.68                               | 3.55                                 | 11.250                        | 0.22                          | 0.90  | 0.24 | 39.4 | 11.24 | 0.23  | 0.95  |
| 00040057+6835035 | 118.605  | 6.112    | 3.148  | 9      | -      | -    | -    | -        | -     | -      | -   | -                      | -          | -          | -    | -        | -          | 10.082 | 1.47                               | ...                         | 1                           | 116.4                | 0.66                               | 3.75                                 | 8.909                         | 0.95                          | ...   | 0.98 | ...  | ...   | 1.01  | ...   |
| 00051051+6707589 | 118.449  | 4.665    | 3.076  | 8      | -      | -    | -    | -        | -     | -      | -   | -                      | -          | -          | -    | -        | -          | 11.550 | 1.07                               | 2.33                        | 1                           | 56.0                 | 0.44                               | 3.70                                 | 10.404                        | 0.56                          | 0.81  | 0.95 | ...  | ...   | 0.62  | 1.01  |
| 00053428+5337528 | 116.084  | -8.629   | 0.417  | 1      | -      | -    | -    | -        | -     | -      | D1  | c                      | -          | h          | -    | -        | -          | 10.943 | 0.32                               | 1.16                        | 1                           | 59.2                 | 0.52                               | 3.60                                 | 10.788                        | 0.25                          | 0.95  | 0.13 | 60.8 | 10.80 | 0.26  | 0.98  |
| 00072270+6458025 | 118.290  | 2.494    | 3.690  | 7      | -      | -    | -    | -        | -     | -      | -   | -                      | -          | -          | -    | -        | -          | 11.191 | 0.70                               | 1.83                        | 1                           | 54.2                 | 0.60                               | 3.83                                 | 9.816                         | 0.09                          | -0.00 | 1.14 | ...  | ...   | 0.16  | 0.24  |
| 00083102+5301491 | 116.417  | -9.298   | 0.411  | 1      | -      | -    | -    | -        | -     | -      | D1  | c                      | o          | -          | -    | -        | -          | 11.264 | 0.35                               | 1.15                        | 1                           | 34.8                 | 0.78                               | 3.55                                 | 11.111                        | 0.28                          | 0.95  | 0.13 | 35.7 | 11.12 | 0.29  | 0.98  |
| 00083403+5530408 | 116.844  | -6.853   | 0.432  | 1      | -      | -    | -    | -        | -     | -      | D1  | c                      | o          | h          | -    | -        | -          | 11.294 | 0.33                               | 1.18                        | 1                           | 51.2                 | 0.72                               | 3.64                                 | 11.133                        | 0.26                          | 0.97  | 0.13 | 52.8 | 11.14 | 0.27  | 0.99  |
| 00094437+6520217 | 118.597  | 2.819    | 4.848  | 9      | -      | -    | -    | -        | -     | -      | -   | -                      | -          | -          | -    | -        | -          | 10.060 | 0.63                               | 1.53                        | 1                           | 70.2                 | 0.74                               | 3.83                                 | 8.254                         | -0.17                         | -0.88 | 1.50 | ...  | ...   | -0.07 | -0.56 |
| 00102576+6520598 | 118.670  | 2.818    | 4.552  | 6      | -      | -    | -    | -        | -     | -      | -   | -                      | -          | -          | -    | -        | -          | 12.280 | 0.83                               | 2.42                        | 1                           | 23.2                 | 0.98                               | 3.83                                 | 10.584                        | 0.07                          | 0.16  | 1.41 | ...  | ...   | 0.16  | 0.46  |
| 00103893+5325040 | 116.800  | -8.968   | 0.265  | 1      | -      | -    | -    | -        | -     | -      | D2  | c                      | o          | -          | -    | -        | -          | 10.276 | 0.32                               | 1.10                        | 1                           | 57.4                 | 0.74                               | 3.56                                 | 10.177                        | 0.28                          | 0.97  | 0.08 | 58.2 | 10.19 | 0.29  | 0.99  |
| 00105327+6524463 | 118.727  | 2.873    | 4.866  | 9      | -      | -    | -    | -        | -     | -      | -   | -                      | -          | -          | -    | -        | -          | 10.968 | 0.66                               | 2.05                        | 1                           | 64.2                 | 0.48                               | 3.89                                 | 9.155                         | -0.14                         | -0.37 | 1.51 | ...  | ...   | -0.05 | -0.05 |
| 00105342+6525193 | 118.729  | 2.882    | 4.873  | 9      | -      | -    | -    | -        | -     | -      | -   | -                      | -          | -          | -    | -        | -          | 12.469 | 1.06                               | 1.92                        | 1                           | 27.4                 | 0.84                               | 3.89                                 | 10.653                        | 0.25                          | -0.50 | 1.51 | ...  | ...   | 0.35  | -0.18 |
| 00105581+6528123 | 118.740  | 2.929    | 4.440  | 9      | -      | -    | -    | -        | -     | -      | -   | -                      | -          | -          | -    | -        | -          | 11.875 | 0.94                               | 2.04                        | 1                           | 67.2                 | 0.28                               | 3.76                                 | 10.221                        | 0.20                          | -0.17 | 1.38 | ...  | ...   | 0.29  | 0.13  |
| 00105584+6524083 | 118.730  | 2.862    | 4.731  | 9      | -      | -    | -    | -        | -     | -      | -   | -                      | -          | -          | -    | -        | -          | 11.764 | 0.62                               | 1.83                        | 1                           | 48.8                 | 0.56                               | 3.89                                 | 10.001                        | -0.17                         | -0.52 | 1.47 | ...  | ...   | -0.07 | -0.21 |
| 00110111+6526094 | 118.744  | 2.894    | 4.776  | 7      | -      | -    | -    | -        | -     | -      | -   | -                      | -          | -          | -    | -        | -          | 12.627 | 1.32                               | 2.40                        | -2                          | 20.2                 | 1.00                               | 3.89                                 | 10.847                        | 0.53                          | 0.03  | 1.48 | ...  | ...   | 0.62  | 0.35  |
| 00111787+5849242 | 117.746  | -3.643   | 3.664  | 9      | -      | -    | -    | -        | -     | -      | -   | -                      | -          | -          | -    | -        | -          | 11.453 | 1.14                               | ...                         | 1                           | 57.0                 | 0.58                               | 3.83                                 | 10.088                        | 0.54                          | ...   | 1.13 | ...  | ...   | 0.61  | ...   |
| 00112263+5848542 | 117.755  | -3.653   | 3.621  | 9      | -      | -    | -    | -        | -     | -      | -   | -                      | -          | -          | -    | -        | -          | 11.047 | 1.33                               | ...                         | 1                           | 42.4                 | 1.00                               | 3.83                                 | 9.698                         | 0.73                          | ...   | 1.12 | ...  | ...   | 0.81  | ...   |
| 00112872+5849052 | 117.768  | -3.652   | 3.607  | 9      | -      | -    | -    | -        | -     | -      | -   | -                      | -          | -          | -    | -        | -          | 10.559 | 0.57                               | 1.37                        | 1                           | 112.2                | 0.58                               | 3.74                                 | 9.215                         | -0.03                         | -0.42 | 1.12 | ...  | ...   | 0.04  | -0.18 |
| 00125762+7231261 | 120.012  | 9.871    | 0.391  | 8      | o      | p    | -    | -        | -     | -      | -   | -                      | -          | -          | -    | -        | -          | 8.666  | 1.01                               | 1.21                        | 1                           | 116.4                | 0.66                               | 3.51                                 | 8.520                         | 0.94                          | 1.02  | 1.12 | ...  | ...   | 0.95  | 1.04  |
| 00141253+7036448 | 118.824  | 7.966    | 1.014  | 1      | -      | -    | -    | -        | -     | -      | D1  | e                      | o          | *          | -    | -        | -          | 10.915 | 0.39                               | 1.37                        | 1                           | 53.4                 | 0.70                               | 3.60                                 | 10.537                        | 0.22                          | 0.86  | 0.31 | 58.4 | 10.54 | 0.24  | 0.93  |
| 00142532+6209408 | 118.625  | -0.400   | 1.933  | 7      | -      | -    | -    | -        | -     | -      | -   | -                      | -          | -          | -    | -        | -          | 10.891 | 0.91                               | 2.24                        | 1                           | 54.8                 | 0.36                               | 3.84                                 | 10.171                        | 0.59                          | 1.28  | 0.60 | ...  | ...   | 0.63  | 1.40  |
| 00142832+6428469 | 118.962  | 1.893    | 3.616  | 7      | -      | -    | -    | -        | -     | -      | -   | -                      | -          | -          | -    | -        | -          | 10.572 | 1.03                               | 2.45                        | 1                           | 34.0                 | 0.76                               | 3.85                                 | 9.225                         | 0.44                          | 0.65  | 1.12 | ...  | ...   | 0.51  | 0.89  |
| 00152768+6114161 | 118.617  | -1.332   | 3.965  | 8      | -      | -    | -    | -        | -     | -      | -   | -                      | -          | -          | -    | -        | -          | 9.882  | 1.40                               | 3.11                        | 1                           | 64.2                 | 0.66                               | 3.94                                 | 8.405                         | 0.74                          | 1.14  | 1.23 | ...  | ...   | 0.82  | 1.40  |
| 00153362+6115421 | 118.632  | -1.310   | 3.952  | 9      | -      | -    | -    | -        | -     | -      | -   | -                      | -          | -          | -    | -        | -          | 9.931  | 0.88                               | 2.08                        | 1                           | 94.4                 | 0.88                               | 3.94                                 | 8.458                         | 0.22                          | 0.11  | 1.22 | ...  | ...   | 0.30  | 0.37  |
| 00153433+6114301 | 118.630  | -1.330   | 4.052  | 9      | -      | -    | -    | -        | -     | -      | -   | -                      | -          | -          | -    | -        | -          | 12.234 | 0.57                               | 1.80                        | 1                           | 37.2                 | 0.38                               | 3.94                                 | 10.724                        | -0.10                         | -0.21 | 1.26 | ...  | ...   | -0.02 | 0.06  |
| 00154653+6546142 | 119.280  | 3.152    | 2.153  | 8      | -      | -    | -    | -        | -     | -      | -   | -                      | -          | -          | -    | -        | -          | 10.817 | 0.76                               | 2.21                        | 1                           | 36.6                 | 0.58                               | 3.81                                 | 10.015                        | 0.40                          | 1.14  | 0.67 | ...  | ...   | 0.45  | 1.28  |
| 00161976+7025219 | 119.974  | 7.753    | 1.046  | 2      | o      | -    | -    | -        | -     | -      | D2  | -                      | -          | -          | -    | -        | -          | 11.325 | 0.32                               | 0.99                        | 1                           | 24.2                 | 0.68                               | 3.55                                 | 10.935                        | 0.15                          | 0.47  | 0.32 | 26.4 | 10.95 | 0.17  | 0.54  |
| 00162328+6120128 | 118.741  | -1.249   | 1.814  | 7      | -      | -    | -    | -        | -     | -      | -   | -                      | -          | -          | -    | -        | -          | 10.745 | 0.90                               | 2.10                        | 1                           | 28.4                 | 0.54                               | 3.87                                 | 10.069                        | 0.60                          | 1.19  | 0.56 | ...  | ...   | 0.63  | 1.31  |
| 00165062+6546150 | 119.389  | 3.138    | 2.364  | 6      | -      | -    | -    | -        | -     | -      | -   | -                      | -          | -          | -    | -        | -          | 11.415 | 0.90                               | 2.69                        | 1                           | 25.0                 | 0.86                               | 3.75                                 | 10.534                        | 0.51                          | 1.51  | 0.73 | ...  | ...   | 0.56  | 1.67  |
| 00175637+6550205 | 119.509  | 3.190    | 6.506  | 9      | -      | -    | -    | -        | -     | -      | -   | -                      | -          | -          | -    | -        | -          | 11.250 | 0.67                               | 2.31                        | 1                           | 53.0                 | 0.84                               | 3.82                                 | 8.826                         | -0.40                         | -0.92 | 2.02 | ...  | ...   | -0.28 | -0.49 |
| 00180044+6550475 | 119.517  | 3.197    | 6.797  | 7      | -      | -    | -    | -        | -     | -      | -   | -                      | -          | -          | -    | -        | -          | 11.705 | 1.03                               | 2.52                        | 1                           | 37.8                 | 0.62                               | 3.82                                 | 9.172                         | -0.10                         | -0.86 | 2.11 |      |       |       |       |

Table B1: a) continued.

| 2MASX J          |         | <i>l</i>    | <i>b</i>    | EBV        | Object       | Sample     |             |             |            | Disc        | 2MRS          | Velocity    |     | NIR          | Photom      | Ext          | <i>K</i> <sub>20</sub> | <i>H-K</i>   | <i>J-K</i> | vc          | <i>a</i>    | <i>b/a</i>  | std.d. | <i>K</i> <sub>S</sub> <sup>o</sup> | ( <i>H-K</i> ) <sup>o</sup> | ( <i>J-K</i> ) <sup>o</sup> | <i>A<sub>K</sub></i> | <i>a</i> <sup>d</sup> | <i>K</i> <sub>S</sub> <sup>d,d</sup> | ( <i>H-K</i> ) <sup>o,c</sup> | ( <i>J-K</i> ) <sup>o,c</sup> |             |             |             |       |
|------------------|---------|-------------|-------------|------------|--------------|------------|-------------|-------------|------------|-------------|---------------|-------------|-----|--------------|-------------|--------------|------------------------|--------------|------------|-------------|-------------|-------------|--------|------------------------------------|-----------------------------|-----------------------------|----------------------|-----------------------|--------------------------------------|-------------------------------|-------------------------------|-------------|-------------|-------------|-------|
| (1)              |         | deg<br>(2a) | deg<br>(2b) | mag<br>(3) | class<br>(4) | off<br>(5) | flag<br>(6) | gal<br>(7a) | TF<br>(7b) | obs<br>(7c) | ext'd<br>(7d) | type<br>(8) | (9) | Opt<br>(10a) | HI<br>(10b) | flag<br>(11) | flag<br>(12)           | flag<br>(13) |            | mag<br>(14) | mag<br>(15) | mag<br>(16) | (17)   | "<br>(18)                          | (19)                        | (20)                        | mag<br>(21)          | mag<br>(22)           | mag<br>(23)                          | mag<br>(24)                   | "<br>(25)                     | mag<br>(26) | mag<br>(27) | mag<br>(28) |       |
| 00343086+6257451 | 121.010 | 0.154       | 1.453       | 1          | —            | —          | —           | g           | t          | —           | —             | D1          | —   | —            | —           | —            | —                      | —            | —          | —           | 11.228      | 0.34        | 1.28   | 1                                  | 38.2                        | 0.44                        | 3.88                 | 10.687                | 0.10                                 | 0.56                          | 0.45                          | 44.2        | 10.67       | 0.12        | 0.65  |
| 00343656+6310260 | 121.035 | 0.364       | 1.529       | 1          | —            | —          | —           | g           | t          | —           | —             | D3          | —   | —            | —           | —            | —                      | —            | —          | —           | 11.533      | 0.41        | 1.57   | 1                                  | 25.0                        | 0.74                        | 3.91                 | 10.963                | 0.16                                 | 0.81                          | 0.47                          | 29.2        | 10.95       | 0.19        | 0.91  |
| 00344184+5541240 | 120.556 | -7.104      | 0.395       | 1          | —            | —          | —           | g           | —          | —           | —             | D2          | c   | o            | —           | —            | —                      | —            | —          | —           | 11.157      | 0.34        | 1.15   | 1                                  | 40.6                        | 0.74                        | 3.60                 | 11.010                | 0.28                                 | 0.95                          | 0.12                          | 41.6        | 11.02       | 0.29        | 0.98  |
| 00360774+6614391 | 121.388 | 3.419       | 1.990       | 9          | —            | —          | —           | g           | —          | —           | —             | —           | —   | —            | —           | —            | —                      | —            | —          | —           | 11.487      | 1.95        | —      | 1                                  | 34.8                        | 0.32                        | 3.80                 | 10.746                | 1.62                                 | —                             | 0.62                          | —           | —           | 1.66        | —     |
| 00360888+6319171 | 121.217 | 5.001       | 1.369       | 1          | —            | —          | —           | g           | t          | N           | —             | D1          | —   | —            | —           | —            | —                      | —            | —          | —           | 11.373      | 0.69        | 1.95   | 1                                  | 37.0                        | 0.36                        | 3.92                 | 10.863                | 0.46                                 | 1.27                          | 0.42                          | 42.3        | 10.86       | 0.49        | 1.36  |
| 00360908+5522418 | 120.743 | -7.428      | 0.470       | 1          | —            | —          | —           | g           | t          | —           | —             | D1          | c   | o            | —           | —            | —                      | —            | —          | —           | 11.347      | 0.41        | 1.37   | 1                                  | 42.4                        | 0.36                        | 3.63                 | 11.172                | 0.34                                 | 1.13                          | 0.15                          | 43.7        | 11.18       | 0.34        | 1.16  |
| 00361954+5310405 | 120.636 | -9.626      | 0.215       | 1          | —            | —          | —           | g           | t          | —           | —             | D1          | c   | o            | —           | —            | —                      | —            | —          | —           | 10.961      | 0.43        | 1.19   | 1                                  | 52.0                        | 0.26                        | 3.46                 | 10.881                | 0.40                                 | 1.08                          | 0.07                          | 52.5        | 10.89       | 0.40        | 1.09  |
| 00364076+6328120 | 121.285 | 0.646       | 6.710       | 8          | —            | —          | —           | g           | —          | —           | —             | —           | —   | —            | —           | —            | —                      | —            | —          | —           | 11.225      | —           | —      | —                                  | 58.6                        | 0.52                        | 3.92                 | 8.725                 | —                                    | —                             | 2.08                          | —           | —           | —           | —     |
| 00364164+6329017 | 121.287 | 0.659       | 6.902       | 9          | —            | —          | —           | g           | —          | —           | —             | —           | —   | —            | —           | —            | —                      | —            | —          | —           | 9.182       | 1.05        | 2.92   | 1                                  | 106.0                       | 0.76                        | 3.93                 | 6.610                 | -0.10                                | -0.51                         | 2.14                          | —           | —           | 0.04        | -0.05 |
| 00364675+6329200 | 121.297 | 0.664       | 7.110       | 9          | —            | —          | —           | g           | —          | —           | —             | —           | —   | —            | —           | —            | —                      | —            | —          | —           | 10.664      | 1.37        | 2.47   | 1                                  | 62.2                        | 0.60                        | 3.92                 | 8.015                 | 0.20                                 | -1.06                         | 2.20                          | —           | —           | 0.34        | -0.60 |
| 00364866+6328578 | 121.300 | 0.658       | 6.931       | 9          | —            | —          | —           | g           | —          | —           | —             | —           | —   | —            | —           | —            | —                      | —            | —          | —           | 8.232       | 1.38        | 2.89   | 1                                  | 144.8                       | 0.60                        | 3.93                 | 5.650                 | 0.23                                 | -0.55                         | 2.15                          | —           | —           | 0.37        | -0.10 |
| 00365866+6636218 | 121.494 | 3.775       | 2.598       | 9          | —            | —          | —           | g           | —          | —           | —             | —           | —   | —            | —           | —            | —                      | —            | —          | —           | 12.147      | 1.53        | —      | —                                  | 28.0                        | 0.40                        | 3.82                 | 11.179                | 1.10                                 | —                             | 0.80                          | —           | —           | 1.15        | —     |
| 00372339+6402408 | 121.395 | 1.215       | 2.670       | 9          | —            | —          | —           | g           | —          | —           | —             | —           | —   | —            | —           | —            | —                      | —            | —          | —           | 11.877      | 1.96        | —      | 1                                  | 35.0                        | 0.66                        | 3.89                 | 10.878                | 1.51                                 | —                             | 0.83                          | —           | —           | 1.15        | —     |
| 00384223+6017130 | 121.353 | -2.546      | 0.723       | 1          | —            | —          | —           | g           | —          | N           | —             | D1          | —   | —            | —           | h            | —                      | —            | —          | —           | 10.940      | 0.31        | 1.20   | 1                                  | 50.8                        | 0.74                        | 3.82                 | 10.671                | 0.19                                 | 0.84                          | 0.22                          | 53.9        | 10.67       | 0.21        | 0.89  |
| 00385855+5927568 | 121.347 | -3.367      | 1.041       | 7          | —            | o          | —           | —           | —          | —           | —             | —           | er  | g            | —           | —            | —                      | —            | —          | —           | 11.289      | 0.83        | 1.90   | -2                                 | 35.2                        | 0.80                        | 3.79                 | 10.901                | 0.65                                 | 1.38                          | 0.32                          | —           | —           | 0.68        | 1.45  |
| 00390819+5835378 | 121.326 | -4.239      | 0.488       | 1          | —            | —          | —           | g           | —          | —           | —             | D1          | e   | o            | —           | —            | —                      | —            | —          | —           | 9.413       | 0.41        | 1.28   | 1                                  | 63.4                        | 0.68                        | 3.74                 | 9.231                 | 0.33                                 | 1.04                          | 0.15                          | 65.1        | 9.25        | 0.33        | 1.07  |
| 00394230+5920061 | 121.434 | -3.502      | 0.848       | 1          | —            | —          | —           | g           | —          | —           | —             | D1          | e   | o            | —           | —            | —                      | —            | —          | —           | 11.239      | 0.50        | 1.45   | 1                                  | 29.4                        | 0.72                        | 3.73                 | 10.923                | 0.36                                 | 1.02                          | 0.26                          | 31.6        | 10.93       | 0.38        | 1.08  |
| 00394700+5552521 | 121.286 | -6.953      | 0.664       | 1          | —            | —          | —           | g           | —          | —           | —             | D3          | c   | o            | —           | —            | —                      | —            | —          | —           | 11.396      | 0.45        | 1.26   | 1                                  | 28.6                        | 0.64                        | 3.62                 | 11.149                | 0.34                                 | 0.93                          | 0.21                          | 30.0        | 10.16       | 0.35        | 0.97  |
| 00402126+6732350 | 121.870 | 4.694       | 1.455       | 1          | —            | —          | —           | g           | t          | N           | —             | D1          | —   | —            | —           | —            | —                      | —            | —          | —           | 11.512      | 0.49        | 1.51   | 1                                  | 36.0                        | 0.62                        | 3.78                 | 10.970                | 0.25                                 | 0.78                          | 0.45                          | 41.8        | 10.95       | 0.28        | 0.88  |
| 00402382+6428443 | 121.743 | 1.633       | 1.829       | 1          | —            | —          | —           | g           | t          | N           | —             | D2          | —   | —            | —           | —            | —                      | —            | —          | —           | 11.536      | 0.79        | 2.06   | 1                                  | 32.0                        | 0.38                        | 3.87                 | 10.855                | 0.49                                 | 1.15                          | 0.57                          | 38.9        | 10.83       | 0.52        | 1.27  |
| 00403120+6653492 | 121.859 | 4.048       | 3.496       | 7          | —            | —          | —           | —           | —          | —           | —             | —           | —   | —            | —           | —            | —                      | —            | —          | —           | 12.553      | 1.07        | 2.34   | 1                                  | 20.8                        | 0.60                        | 3.81                 | 11.250                | 0.49                                 | 0.60                          | 1.08                          | —           | —           | 0.56        | 0.83  |
| 00441534+6654411 | 122.226 | 4.050       | 2.563       | 7          | —            | —          | —           | —           | —          | —           | —             | —           | —   | —            | —           | —            | —                      | —            | —          | —           | 10.254      | 0.73        | 1.91   | 1                                  | 47.8                        | 0.70                        | 3.80                 | 9.299                 | 0.31                                 | 0.64                          | 0.79                          | —           | —           | 0.36        | 0.81  |
| 00444994+5546589 | 121.996 | -7.077      | 4.240       | 9          | —            | —          | —           | —           | —          | —           | —             | —           | —   | —            | —           | —            | —                      | —            | —          | —           | 11.208      | 1.33        | 2.71   | 1                                  | 57.6                        | 0.30                        | 3.75                 | 9.628                 | 0.63                                 | 0.60                          | 1.31                          | —           | —           | 0.71        | 0.88  |
| 00445717+5547169 | 122.013 | -7.072      | 4.317       | 9          | —            | —          | —           | —           | —          | —           | —             | —           | —   | —            | —           | —            | —                      | —            | —          | —           | 8.279       | 0.87        | 1.94   | 1                                  | 129.8                       | 0.64                        | 3.75                 | 6.670                 | 0.16                                 | -0.21                         | 1.34                          | —           | —           | 0.24        | 0.88  |
| 00445777+5546219 | 122.014 | -7.087      | 4.055       | 9          | —            | —          | —           | —           | —          | —           | —             | —           | —   | —            | —           | —            | —                      | —            | —          | —           | 12.599      | 1.22        | —      | 1                                  | 29.0                        | 0.44                        | 3.75                 | 11.088                | 0.55                                 | —                             | 1.26                          | —           | —           | 0.63        | —     |
| 00450274+5546498 | 122.026 | -7.080      | 3.836       | 9          | —            | —          | —           | —           | —          | —           | —             | —           | —   | —            | —           | —            | —                      | —            | —          | —           | 11.051      | 0.91        | 1.83   | 1                                  | 67.6                        | 0.46                        | 3.75                 | 9.622                 | 0.27                                 | -0.08                         | 1.19                          | —           | —           | 0.35        | 0.17  |
| 00450298+5547248 | 122.027 | -7.070      | 3.943       | 9          | —            | —          | —           | —           | —          | —           | —             | —           | —   | —            | —           | —            | —                      | —            | —          | —           | 12.662      | 0.37        | 1.45   | -2                                 | 11.6                        | 0.82                        | 3.75                 | 11.193                | -0.28                                | -0.51                         | 1.22                          | —           | —           | -0.20       | -0.25 |
| 00450852+6549280 | 122.287 | 2.961       | 1.600       | 1          | —            | —          | —           | g           | —          | N           | —             | D3          | —   | —            | —           | *            | —                      | —            | —          | —           | 11.818      | 0.52        | 1.80   | 1                                  | 27.8                        | 0.70                        | 3.80                 | 11.222                | 0.26                                 | 1.01                          | 0.50                          | 33.0        | 11.19       | 0.29        | 1.11  |
| 00451532+5534588 | 122.051 | -7.278      | 0.535       | 1          | —            | —          | —           | g           | t          | N           | —             | D1          | c   | o            | —           | —            | —                      | —            | —          | —           | 10.981      | 0.38        | 1.43   | 1                                  | 43.2                        | 0.38                        | 3.59                 | 10.782                | 0.29                                 | 1.17                          | 0.17                          | 44.8        | 10.79       | 0.30        | 1.20  |
| 00453354+5513291 | 122.086 | -7.637      | 0.433       | 1          | —            | —          | —           | g           | —          | N           | —             | D3          | c   | o            | —           | —            | —                      | —            | —          | —           | 11.252      | 0.42        | 1.24   | 1                                  | 36.2                        | 0.70                        | 3.62                 | 11.091                | 0.35                                 | 1.02                          | 0.13                          | 37.3        | 11.10       | 0.36        | 1.05  |
| 00475430+6807433 | 122.602 | 5.259       | 1.143       | 1          | —            | —          | —           | g           | t          | N           | —             | D1          | e   | o            | —           | —            | —                      | —            | —          | —           | 10.857      | 0.50        | 1.42   | 1                                  | 74.0                        | 0.30                        | 3.65                 | 10.431                | 0.31                                 | 0.85                          | 0.35                          | 84.3        | 10.37       | 0.33        | 0.92  |
| 00482304+6430452 | 122.603 | 1.643       | 1.973       | 9          | —            | —          | —           | —           | —          | —           | —             | —           | —   | —            | —           | —            | —                      | —            | —          | —           | 11.625      | 0.89        | 2.17   | 1                                  | 34.0                        | 0.58                        | 3.86                 | 10.890                | 0.56                                 | 1.19                          | 0.61                          | —           | —           | 0.60        | 1.32  |
| 00484648+5609272 | 122.559 | -6.712      | 0.391       | 1          | —            | —          | —           | g           | —          | —           | —             | D2          | c   | o            | —           | —            | —                      | —            | —          | —           | 10.981      | 0.42        | 1.31   | 1                                  | 37.6                        | 0.66                        | 3.64                 | 10.835                | 0.35                                 | 1.12                          | 0.12                          | 38.5        | 10.85       | 0.36        | 1.15  |
| 00492019+5314287 | 122.613 | -9.629      | 0.371       | 1          | —            | —          | —           | g           | —          | —           | —             | D2          | c   | o            | —           | —            | —                      | —            | —          | —           | 11.003      | 0.33        | 1.11   | 1                                  | 34.4                        | 0.94                        | 3.48                 | 10.865                | 0.27                                 | 0.93                          | 0.11                          | 35.2        | 10.88       | 0.28        | 0.95  |
| 00495554+6543396 | 122.776 | 2.857       | 5.300       | 8          | —            | —          | —           | —           | —          | —           | —             | —           | —   | —            | —           | —            | —                      | —            | —          | —           | 9.675       | 1.02        | 2.17   | 1                                  | 76.2                        | 0.84                        | 3.83                 | 7.700                 | 0.14                                 | -0.46                         | 1.64                          | —           | —           | 0.25        | -0.11 |
| 00501956+6702517 | 122.823 | 4.176       | 1.408       | 1          | —            | —          | —           | —           | —          | N           | —             | D1          | —   | —            | —           | —            | —                      | —            | —          | —           | 10.638      | 0.47        | 1.62   | 1                                  | 44.6                        | 0.84                        | 3.77                 | 10.113                | 0.24                                 | 0.92                          | 0.44                          | 50.6        | 10.13       | 0.26        | 1.01  |
| 00503589+5456444 | 122.810 | -7.926      | 0.350       | 1          | —            | —          | —           | g           | —          | —           | —             | D1          | c   | o            | —           | —            | —                      | —            | —          | —           | 11.051      | 0.44        | 1.26   | 1                                  | 36.6                        | 0.82                        | 3.59                 | 10.921                | 0.36                                 | 1.08                          | 0.11                          | 37.4        | 10.93       | 0.37        | 1.11  |
| 00504513+5607464 | 122.836 | -6.742      | 0.339       | 1          | —            | —          | —           | g           | —          | —           | —             | D1          | c   | o            | —           | —            | —                      | —            | —          | —           | 11.362      | 0.42        | 1.33   | 1                                  | 24.0                        | 0.94                        | 3.65                 | 11.236                | 0.38                                 | 1.16                          | 0.11                          | 24.5        | 11.25       | 0.39        | 1.18  |
| 00513443+6548131 | 122.946 | 2.932       | 4.782       | 8          | —            | —          | —           | —           | —          | —           | —             | —           | —   | —            | —           | —            | —                      | —            | —          | —           | 10.569      | 0.82        | 1.89   | 1                                  | 93.4                        | 0.40                        | 3.76                 | 8.787                 | 0.03                                 | -0.49                         | 1.48                          | —           | —           | 0.13        | -0.17 |
| 00521037+5634291 | 123.034 | -6.297      | 6.959       | 9          | —            | —          | —           | —           | —          | —           | —             | —           | —   | —            | —           | —            | —                      | —            | —          | —           | 13.259      | 0.56        | 1.92   | -1                                 | 19.2                        | 0.50                        | 3.82                 | 10.666                | -0.59                                | -1.54                         | 2.16                          | —           | —           | -0.45       | -1.08 |
| 00521171+5633051 | 123.037 | -6.320      | 6.836       | 9          | —            | —          | —           | —           | —          | —           | —             | —           | —   |              |             |              |                        |              |            |             |             |             |        |                                    |                             |                             |                      |                       |                                      |                               |                               |             |             |             |       |

Table B1: a) continued.

| 2MASX J          | <i>l</i> | <i>b</i> | EBV    | Object | Sample | Disc | 2MRS | Velocity | NIR | Photom | Ext  | <i>K</i> <sub>20</sub> | <i>H-K</i> | <i>J-K</i> | vc | <i>a</i> | <i>b/a</i> | st.d. | <i>K</i> <sub>s</sub> <sup>o</sup> | ( <i>H-K</i> ) <sup>o</sup> | ( <i>J-K</i> ) <sup>o</sup> | <i>A<sub>K</sub></i> | <i>a</i> <sub>d</sub> <sup>o</sup> | <i>K</i> <sub>s</sub> <sup>o,d</sup> | ( <i>H-K</i> ) <sup>o,c</sup> | ( <i>J-K</i> ) <sup>o,c</sup> |       |      |      |        |       |        |       |      |       |       |        |
|------------------|----------|----------|--------|--------|--------|------|------|----------|-----|--------|------|------------------------|------------|------------|----|----------|------------|-------|------------------------------------|-----------------------------|-----------------------------|----------------------|------------------------------------|--------------------------------------|-------------------------------|-------------------------------|-------|------|------|--------|-------|--------|-------|------|-------|-------|--------|
| (1)              | deg      | deg      | mag    | class  | off    | flg  | gal  | TF       | obs | ext'd  | type | (8)                    | (9)        | Opt        | HI | (10a)    | (10b)      | (11)  | flg                                | flg                         | flg                         | (13)                 | (14)                               | (15)                                 | (16)                          | (17)                          | (18)  | (19) | (20) | (21)   | (22)  | (23)   | (24)  | (25) | (26)  | (27)  | (28)   |
| 01083403+5900298 | 125.140  | -3.790   | 0.721  | 1      | o      | -    | g    | -        | -   | -      | D2   | e                      | o          | -          | -  | -        | -          | o     | -                                  | -                           | -                           | -                    | 10.228                             | 0.95                                 | 1.37                          | 1                             | 53.0  | 0.84 | 3.64 | 9.959  | 0.83  | 1.01   | 0.22  | 56.7 | 9.94  | 0.84  | 1.06   |
| 01084898+6233597 | 124.932  | -0.237   | 3.008  | 9      | -      | -    | -    | -        | -   | -      | -    | -                      | -          | -          | -  | -        | -          | -     | -                                  | -                           | -                           | -                    | 12.329                             | 0.75                                 | 1.51                          | 1                             | 39.4  | 0.46 | 3.81 | 11.208 | 0.25  | 0.01   | 0.93  | ...  | ...   | 0.31  | 0.21   |
| 01085030+6233197 | 124.935  | -0.248   | 2.909  | 8      | -      | -    | -    | -        | -   | -      | -    | -                      | -          | -          | -  | -        | -          | -     | -                                  | -                           | -                           | -                    | 11.049                             | 0.89                                 | 2.32                          | 1                             | 36.8  | 0.90 | 3.81 | 9.965  | 0.40  | 0.88   | 0.90  | ...  | ...   | 0.46  | 1.07   |
| 01085212+6307177 | 124.901  | 0.317    | 4.947  | 9      | -      | -    | -    | -        | -   | -      | -    | -                      | -          | -          | -  | -        | -          | -     | -                                  | -                           | -                           | -                    | 10.874                             | 1.14                                 | 2.09                          | 1                             | 59.4  | 0.44 | 3.82 | 9.031  | 0.32  | -0.37  | 1.53  | ...  | ...   | 0.41  | -0.04  |
| 01091415+6239489 | 124.974  | -0.137   | 2.718  | 9      | -      | -    | -    | -        | -   | -      | -    | -                      | -          | -          | -  | -        | -          | -     | -                                  | -                           | -                           | -                    | 11.843                             | 0.83                                 | 2.14                          | 1                             | 33.8  | 0.64 | 3.81 | 10.830 | 0.38  | 0.79   | 0.84  | ...  | ...   | 0.43  | 0.97   |
| 01104801+6334101 | 125.085  | 0.779    | 3.324  | 9      | -      | -    | -    | -        | -   | -      | -    | -                      | -          | -          | -  | -        | -          | -     | -                                  | -                           | -                           | -                    | 10.840                             | 1.32                                 | 2.95                          | 1                             | 49.2  | 0.44 | 3.80 | 9.601  | 0.77  | 1.30   | 1.03  | ...  | ...   | 0.84  | 1.52   |
| 01133912+6904309 | 124.925  | 6.290    | 0.936  | 1      | -      | -    | -    | -        | -   | -      | D2   | c                      | o          | -          | -  | -        | -          | -     | -                                  | -                           | -                           | -                    | 11.513                             | 0.37                                 | 1.44                          | 1                             | 32.0  | 0.72 | 3.67 | 11.164 | 0.21  | 0.98   | 0.29  | 34.7 | 11.17 | 0.23  | 1.04   |
| 01135448+6440014 | 125.334  | 1.900    | 1.564  | 1      | o      | -    | -    | -        | -   | -      | D4   | -                      | -          | -          | -  | -        | -          | o     | -                                  | -                           | -                           | -                    | 10.473                             | 0.52                                 | 1.60                          | 1                             | 40.8  | 0.68 | 3.88 | 9.890  | 0.26  | 0.82   | 0.48  | 47.2 | 9.90  | 0.29  | 0.93   |
| 01154030+5653435 | 126.254  | -5.820   | 0.516  | 1      | -      | -    | -    | -        | -   | -      | D1   | c                      | o          | -          | -  | -        | -          | -     | -                                  | -                           | -                           | -                    | 11.105                             | 0.40                                 | 1.27                          | 1                             | 38.2  | 0.48 | 3.68 | 10.913 | 0.31  | 1.01   | 0.16  | 39.5 | 10.93 | 0.32  | 1.05   |
| 01154150+6446421 | 125.513  | 2.028    | 3.019  | 9      | -      | -    | -    | -        | -   | -      | -    | -                      | -          | -          | -  | -        | -          | -     | -                                  | -                           | -                           | -                    | 12.206                             | 0.77                                 | ...                           | 1                             | 29.6  | 1.0  | 3.85 | 11.081 | 0.27  | ...    | 0.94  | ...  | ...   | 0.33  | ...    |
| 01154286+5559475 | 126.345  | -6.714   | 0.451  | 1      | -      | -    | -    | -        | -   | -      | D1   | c                      | o          | -          | -  | -        | -          | -     | -                                  | -                           | -                           | -                    | 11.218                             | 0.35                                 | 1.11                          | 1                             | 44.8  | 0.44 | 3.61 | 11.050 | 0.28  | 0.89   | 0.14  | 46.2 | 11.06 | 0.29  | 0.92   |
| 01154957+6455172 | 125.514  | 2.172    | 3.410  | 7      | -      | -    | -    | -        | -   | -      | -    | -                      | -          | -          | -  | -        | -          | -     | -                                  | -                           | -                           | -                    | 12.043                             | 1.16                                 | 2.84                          | 1                             | 24.4  | 0.76 | 3.85 | 10.772 | 0.59  | 1.14   | 1.06  | ...  | ...   | 0.66  | 1.37   |
| 01161772+6421362 | 125.618  | 1.618    | 1.731  | 7      | -      | -    | -    | -        | -   | -      | -    | -                      | -          | -          | -  | -        | -          | -     | -                                  | -                           | -                           | -                    | 11.262                             | 1.12                                 | 2.47                          | 1                             | 36.6  | 0.52 | 3.78 | 10.617 | 0.83  | 1.61   | 0.54  | ...  | ...   | 0.86  | 1.73   |
| 01163397+6449280 | 125.602  | 2.083    | 5.108  | 9      | -      | -    | -    | -        | -   | -      | -    | -                      | -          | -          | -  | -        | -          | -     | -                                  | -                           | -                           | -                    | 12.914                             | 0.61                                 | 1.75                          | -2                            | 27.8  | 0.30 | 3.85 | 11.011 | -0.24 | -0.79  | 1.58  | ...  | ...   | -0.14 | -0.45  |
| 01163622+6449087 | 125.606  | 2.078    | 5.070  | 7      | -      | -    | -    | -        | -   | -      | -    | -                      | -          | -          | -  | -        | -          | -     | -                                  | -                           | -                           | -                    | 12.945                             | 0.98                                 | 2.40                          | -2                            | 16.0  | 0.60 | 3.86 | 11.056 | 0.14  | -0.12  | 1.57  | ...  | ...   | 0.24  | 0.22   |
| 01163667+6450417 | 125.604  | 2.104    | 5.085  | 8      | -      | -    | -    | -        | -   | -      | -    | -                      | -          | -          | -  | -        | -          | -     | -                                  | -                           | -                           | -                    | 10.474                             | 1.11                                 | 2.44                          | 1                             | 36.0  | 0.60 | 3.86 | 8.579  | 0.27  | -0.09  | 1.58  | ...  | ...   | 0.37  | 0.25   |
| 01164814+6445417 | 125.633  | 2.023    | 3.898  | 7      | -      | -    | -    | -        | -   | -      | -    | -                      | -          | -          | -  | -        | -          | -     | -                                  | -                           | -                           | -                    | 11.233                             | 1.74                                 | 3.42                          | 1                             | 34.6  | 0.70 | 3.86 | 9.781  | 1.09  | 1.48   | 1.21  | ...  | ...   | 1.17  | 1.74   |
| 01173664+5959488 | 126.202  | -2.708   | 0.729  | 1      | -      | -    | -    | -        | -   | -      | D4   | er                     | -          | -          | -  | -        | -          | -     | -                                  | -                           | -                           | -                    | 10.786                             | 0.34                                 | 1.19                          | 1                             | 32.8  | 0.80 | 3.76 | 10.514 | 0.22  | 0.83   | 0.23  | 34.5 | 10.53 | 0.23  | 0.88   |
| 01173679+6426279 | 125.751  | 1.713    | 2.227  | 7      | -      | -    | -    | -        | -   | -      | -    | -                      | -          | -          | -  | -        | -          | -     | -                                  | -                           | -                           | -                    | 11.658                             | 0.75                                 | 1.85                          | 1                             | 22.2  | 0.56 | 3.84 | 10.828 | 0.38  | 0.75   | 0.69  | ...  | ...   | 0.43  | 0.89   |
| 01191564+5610200 | 126.823  | -6.489   | 0.544  | 1      | -      | -    | -    | -        | -   | -      | D1   | c                      | o          | -          | -  | -        | -          | -     | -                                  | -                           | -                           | -                    | 10.994                             | 0.43                                 | 1.20                          | 1                             | 45.8  | 0.58 | 3.60 | 10.791 | 0.34  | 0.93   | 0.17  | 47.6 | 10.80 | 0.35  | 0.97   |
| 01191829+6219297 | 126.161  | -0.372   | 1.236  | 1      | -      | -    | -    | -        | -   | -      | D1   | -                      | -          | -          | -  | -        | -          | h     | -                                  | -                           | -                           | -                    | 10.667                             | 0.52                                 | 1.67                          | 1                             | 62.2  | 0.22 | 3.79 | 10.206 | 0.32  | 1.06   | 0.38  | 69.2 | 10.22 | 0.34  | 1.14   |
| 01192649+6545448 | 125.804  | 3.047    | 1.989  | 8      | -      | -    | -    | -        | -   | -      | -    | -                      | -          | -          | -  | -        | -          | -     | -                                  | -                           | -                           | -                    | 11.249                             | 0.62                                 | 1.62                          | 1                             | 30.0  | 0.78 | 3.79 | 10.508 | 0.29  | 0.63   | 0.62  | ...  | ...   | 0.33  | 0.77   |
| 01192705+5831151 | 126.592  | -4.152   | 0.568  | 1      | -      | -    | -    | -        | -   | -      | D2   | e                      | o          | -          | -  | -        | -          | -     | -                                  | -                           | -                           | -                    | 10.410                             | 0.44                                 | 1.32                          | 1                             | 53.2  | 0.70 | 3.68 | 10.198 | 0.35  | 1.04   | 0.18  | 55.4 | 10.21 | 0.36  | 1.08   |
| 01202398+5801226 | 126.772  | -4.633   | 0.488  | 9      | e      | -    | -    | -        | -   | -      | -    | -                      | -          | -          | -  | -        | -          | o     | -                                  | -                           | -                           | -                    | 9.651                              | 0.41                                 | 1.24                          | -2                            | 105.4 | 0.42 | 3.67 | 9.469  | 0.33  | 1.00   | 0.15  | ...  | ...   | 0.34  | 1.03   |
| 01202409+5801369 | 126.771  | -4.629   | 0.488  | 1      | -      | -    | -    | -        | -   | -      | D4   | e                      | o          | -          | -  | -        | -          | -     | -                                  | -                           | -                           | -                    | 9.640                              | 0.42                                 | 1.27                          | 1                             | 70.6  | 0.74 | ...  | 9.458  | 0.34  | 1.03   | 0.15  | ...  | ...   | 0.35  | 1.06   |
| 01203021+6525055 | 125.951  | 2.717    | 1.276  | 1      | -      | -    | -    | -        | -   | -      | D1   | -                      | -          | -          | -  | -        | -          | -     | -                                  | -                           | -                           | -                    | 9.962                              | 0.45                                 | 1.43                          | 1                             | 80.2  | 0.54 | 3.84 | 9.487  | 0.24  | 0.79   | 0.40  | 91.0 | 9.47  | 0.26  | 0.88   |
| 01214834+6350113 | 126.272  | 1.162    | 1.594  | 1      | -      | -    | -    | -        | -   | -      | D2   | e                      | o          | -          | -  | -        | -          | -     | -                                  | -                           | -                           | -                    | 10.613                             | 0.47                                 | 1.69                          | 1                             | 38.6  | 0.80 | 3.88 | 10.019 | 0.21  | 0.90   | 0.49  | 44.6 | 10.03 | 0.24  | 1.00   |
| 01215577+5601372 | 127.211  | -6.591   | 0.518  | 1      | -      | -    | -    | -        | -   | -      | D3   | c                      | o          | -          | -  | -        | -          | -     | -                                  | -                           | -                           | -                    | 11.368                             | 0.48                                 | 1.32                          | 1                             | 27.4  | 0.84 | 3.58 | 11.175 | 0.40  | 1.06   | 0.16  | 28.4 | 11.19 | 0.41  | 1.10   |
| 01224996+6152268 | 126.623  | -0.772   | 35.776 | 7      | -      | -    | -    | -        | -   | -      | -    | -                      | -          | -          | -  | -        | -          | -     | -                                  | -                           | -                           | -                    | 10.869                             | 1.26                                 | ...                           | 1                             | 82.4  | 0.30 | 3.85 | -2.461 | -4.66 | ...    | 11.08 | ...  | ...   | -3.96 | ...    |
| 01230017+5315438 | 127.706  | -9.317   | 0.412  | 1      | -      | -    | -    | -        | -   | -      | D1   | c                      | o          | -          | -  | -        | -          | -     | -                                  | -                           | -                           | -                    | 10.034                             | 0.33                                 | 1.14                          | 1                             | 55.8  | 0.86 | 3.51 | 9.880  | 0.26  | 0.93   | 0.13  | 57.2 | 9.89  | 0.27  | 0.96   |
| 01230029+6153168 | 126.642  | -0.756   | 36.686 | 8      | -      | -    | -    | -        | -   | -      | -    | -                      | -          | -          | -  | -        | -          | -     | -                                  | -                           | -                           | -                    | 11.799                             | 0.64                                 | 1.90                          | 1                             | 68.2  | 0.26 | 3.85 | -1.870 | -5.43 | -16.32 | 11.36 | ...  | ...   | -4.71 | -13.90 |
| 01230324+6151447 | 126.651  | -0.781   | 37.169 | 9      | -      | -    | -    | -        | -   | -      | -    | -                      | -          | -          | -  | -        | -          | -     | -                                  | -                           | -                           | -                    | 10.456                             | 1.01                                 | 2.05                          | 1                             | 60.4  | 0.60 | 3.85 | -3.393 | -5.14 | -16.42 | 11.51 | ...  | ...   | -4.41 | -13.96 |
| 01230734+6049177 | 126.786  | -1.813   | 0.548  | 1      | o      | -    | -    | -        | -   | -      | D1   | -                      | -          | -          | -  | -        | -          | o     | -                                  | -                           | -                           | -                    | 10.845                             | 0.31                                 | 1.19                          | 1                             | 51.2  | 0.44 | 3.85 | 10.641 | 0.22  | 0.91   | 0.17  | 53.3 | 10.65 | 0.23  | 0.95   |
| 01230804+6151067 | 126.661  | -0.790   | 39.301 | 8      | -      | -    | -    | -        | -   | -      | -    | -                      | -          | -          | -  | -        | -          | -     | -                                  | -                           | -                           | -                    | 13.428                             | ...                                  | 1.42                          | -1                            | 13.2  | 1.00 | 3.85 | -1.216 | ...   | -18.10 | 12.17 | ...  | ...   | ...   | -15.51 |
| 01231656+6153206 | 126.673  | -0.751   | 35.499 | 7      | -      | -    | -    | -        | -   | -      | -    | -                      | -          | -          | -  | -        | -          | -     | -                                  | -                           | -                           | -                    | 12.732                             | ...                                  | ...                           | 1                             | 29.2  | 0.32 | 3.85 | -0.495 | ...   | ...    | 11.00 | ...  | ...   | ...   | ...    |
| 01231968+6153425 | 126.679  | -0.744   | 34.173 | 9      | -      | -    | -    | -        | -   | -      | -    | -                      | -          | -          | -  | -        | -          | -     | -                                  | -                           | -                           | -                    | 11.130                             | 0.86                                 | ...                           | 1                             | 77.0  | 0.26 | 3.88 | -1.603 | -4.80 | ...    | 10.59 | ...  | ...   | -4.13 | ...    |
| 01232352+6152126 | 126.689  | -0.768   | 35.429 | 8      | -      | -    | -    | -        | -   | -      | -    | -                      | -          | -          | -  | -        | -          | -     | -                                  | -                           | -                           | -                    | 11.372                             | 0.88                                 | 2.07                          | 1                             | 38.2  | 0.36 | 3.88 | -1.829 | -4.98 | -15.53 | 10.97 | ...  | ...   | -4.29 | -13.19 |
| 01232749+6150556 | 126.700  | -0.788   | 33.912 | 9      | -      | -    | -    | -        | -   | -      | -    | -                      | -          | -          | -  | -        | -          | -     | -                                  | -                           | -                           | -                    | 13.907                             | 0.51                                 | ...                           | -1                            | 10.0  | 1.00 | 3.88 | 1.271  | -5.11 | ...    | 10.50 | ...  | ...   | -4.44 | ...    |
| 01233032+6149236 | 126.708  | -0.813   | 28.984 | 8      | -      | -    | -    | -        | -   | -      | -    | -                      | -          | -          | -  | -        | -          | -     | -                                  | -                           | -                           | -                    | 11.189                             | 1.13                                 | 2.93                          | 1                             | 36.0  | 0.92 | 3.88 | 0.390  | -3.67 | -11.47 | 8.98  | ...  | ...   | -3.10 | -9.56  |
| 01233315+6148506 | 126.715  | -0.821   | 25.588 | 9      | -      | -    | -    | -        | -   | -      | -    | -                      | -          | -          | -  | -        | -          | -     | -                                  | -                           | -                           | -                    | 8.323                              | 2.11                                 | ...                           | 1                             | 217.0 | 0.26 | 3.88 | -1.211 | -2.13 | ...    | 7.93  | ...  | ...   | -1.63 | ...    |
| 01233499+6148066 | 126.720  | -0.833   | 22.044 | 9      | -      | -    | -    | -        | -   | -      | -    | -                      | -          | -          | -  | -        | -          | -     | -                                  | -                           | -                           | -                    | 9.484                              | 1.86                                 | ...                           | 1                             | 103.6 | 0.72 | 3.88 | 1.270  | -1.79 | ...    | 6.83  | ...  | ...   | -1.35 | ...    |
| 01240480+6151245 | 126.771  | -0.771   | 11.717 | 9      | -      | -    |      |          |     |        |      |                        |            |            |    |          |            |       |                                    |                             |                             |                      |                                    |                                      |                               |                               |       |      |      |        |       |        |       |      |       |       |        |

Table B1: a) continued.

| 2MASX J          | <i>l</i> | <i>b</i> | EBV   | Object |     |     | Sample | Disc | 2MRS  | Velocity | NIR | Photom | Ext   | <i>K</i> <sub>20</sub> | <i>H-K</i> | <i>J-K</i> | vc   | <i>a</i> | <i>b/a</i> | st.d. | <i>K</i> <sub>s</sub> <sup>o</sup> | <i>(H-K)</i> <sup>o</sup> | <i>(J-K)</i> <sup>o</sup> | <i>A<sub>K</sub></i> | <i>a</i> <sub>d</sub> <sup>o</sup> | <i>K</i> <sub>s</sub> <sup>o,d</sup> | <i>(H-K)</i> <sup>o,c</sup> | <i>(J-K)</i> <sup>o,c</sup> |      |      |      |
|------------------|----------|----------|-------|--------|-----|-----|--------|------|-------|----------|-----|--------|-------|------------------------|------------|------------|------|----------|------------|-------|------------------------------------|---------------------------|---------------------------|----------------------|------------------------------------|--------------------------------------|-----------------------------|-----------------------------|------|------|------|
| (1)              | deg      | deg      | (3)   | class  | off | gal | TF     | obs  | ext'd | type     | Opt | HI     | flg   | mag                    | mag        | mag        | (17) | (18)     | (19)       | (20)  | mag                                | mag                       | mag                       | mag                  | (25)                               | mag                                  | mag                         | mag                         |      |      |      |
| (2a)             | (2b)     | (2b)     | (3)   | (4)    | (5) | (6) | (7a)   | (7b) | (7d)  | (8)      | (9) | (10a)  | (10b) | (11)                   | (12)       | (13)       | (14) | (15)     | (16)       | (17)  | (18)                               | (19)                      | (20)                      | (21)                 | (22)                               | (23)                                 | (24)                        | (25)                        | (26) | (27) | (28) |
| 01482037+5318361 | 131.472  | -8.615   | 0.274 | 1      | -   | -   | g      | -    | -     | D3       | c   | o      | -     | 10.835                 | 0.37       | 1.19       | 1    | 38.2     | 0.78       | 3.50  | 10.733                             | 0.32                      | 1.05                      | 0.08                 | 38.7                               | 10.74                                | 0.33                        | 1.07                        |      |      |      |
| 01484462+6050093 | 129.859  | -1.263   | 1.190 | 1      | -   | -   | t      | N    | -     | D1       | e   | o      | -     | 10.612                 | 0.44       | 1.45       | 1    | 41.6     | 0.48       | 3.85  | 10.169                             | 0.24                      | 0.86                      | 0.37                 | 45.9                               | 10.19                                | 0.26                        | 0.94                        |      |      |      |
| 01485859+6045514 | 129.903  | -1.326   | 1.126 | 1      | o   | -   | t      | N    | -     | D1       | -   | -      | o     | 11.035                 | 0.40       | 1.37       | 1    | 45.8     | 0.40       | 3.85  | 10.615                             | 0.21                      | 0.81                      | 0.35                 | 50.8                               | 10.61                                | 0.24                        | 0.88                        |      |      |      |
| 01500012+5354469 | 131.578  | -7.973   | 0.434 | 7      | -   | -   | -      | -    | -     | -        | cr  | -      | -     | 10.544                 | 0.80       | 1.66       | 1    | 57.2     | 0.44       | 3.58  | 10.382                             | 0.73                      | 1.45                      | 0.13                 | ...                                | ...                                  | 0.74                        | 1.48                        |      |      |      |
| 01503879+7054076 | 127.781  | 8.590    | 0.710 | 1      | -   | -   | g      | -    | -     | D1       | c   | o      | o     | 10.915                 | 0.43       | 1.38       | 1    | 35.8     | 0.62       | 3.49  | 10.650                             | 0.31                      | 1.03                      | 0.22                 | 37.6                               | 10.67                                | 0.33                        | 1.08                        |      |      |      |
| 01510698+7118434 | 127.723  | 8.998    | 0.578 | 1      | -   | -   | g      | -    | -     | D1       | c   | o      | o     | 11.395                 | 0.47       | 1.17       | 1    | 29.8     | 0.86       | 3.53  | 11.180                             | 0.37                      | 0.88                      | 0.18                 | 31.2                               | 11.18                                | 0.38                        | 0.92                        |      |      |      |
| 01521830+5948108 | 130.524  | -2.168   | 0.725 | 1      | -   | -   | g      | -    | -     | D2       | e   | o      | o     | 10.910                 | 0.44       | 1.38       | 1    | 36.8     | 0.66       | 3.77  | 10.640                             | 0.32                      | 1.02                      | 0.22                 | 38.7                               | 10.66                                | 0.33                        | 1.07                        |      |      |      |
| 01531023+7111135 | 127.915  | 8.915    | 0.613 | 1      | -   | -   | t      | N    | -     | D1       | e   | o      | o     | 11.108                 | 0.36       | 1.20       | 1    | 34.8     | 0.36       | 3.56  | 10.880                             | 0.26                      | 0.89                      | 0.19                 | 36.3                               | 10.89                                | 0.27                        | 0.93                        |      |      |      |
| 01531807+5915358 | 130.774  | -2.666   | 0.694 | 1      | -   | -   | g      | -    | -     | D1       | c   | o      | o     | 10.963                 | 0.38       | 1.32       | 1    | 35.0     | 0.74       | 3.79  | 10.704                             | 0.26                      | 0.98                      | 0.21                 | 36.8                               | 10.72                                | 0.28                        | 1.02                        |      |      |      |
| 01532586+7115067 | 127.920  | 8.983    | 0.611 | 1      | -   | -   | g      | -    | -     | D3       | c   | o      | o     | 10.017                 | 0.35       | 1.23       | 1    | 54.6     | 0.86       | 3.56  | 9.789                              | 0.24                      | 0.93                      | 0.19                 | 56.8                               | 9.81                                 | 0.26                        | 0.97                        |      |      |      |
| 01543500+5609567 | 131.687  | -5.629   | 0.407 | 1      | -   | -   | t      | N    | -     | D1       | c   | o      | o     | 11.141                 | 0.39       | 1.23       | 1    | 49.6     | 0.30       | 3.58  | 10.989                             | 0.32                      | 1.03                      | 0.13                 | 50.9                               | 11.00                                | 0.33                        | 1.05                        |      |      |      |
| 01551686+7113060 | 128.074  | 8.987    | 0.628 | 1      | -   | -   | t      | N    | -     | D1       | c   | o      | o     | 10.591                 | 0.40       | 1.38       | 1    | 53.2     | 0.42       | 3.47  | 10.357                             | 0.30                      | 1.07                      | 0.19                 | 55.5                               | 10.37                                | 0.31                        | 1.11                        |      |      |      |
| 01561455+5507523 | 132.172  | -6.574   | 0.383 | 1      | -   | -   | t      | N    | -     | D1       | c   | o      | o     | 11.339                 | 0.33       | 1.10       | 1    | 53.8     | 0.32       | 3.63  | 11.196                             | 0.27                      | 0.91                      | 0.12                 | 55.3                               | 11.20                                | 0.28                        | 0.93                        |      |      |      |
| 01562272+7113228 | 128.160  | 9.014    | 0.716 | 1      | -   | -   | g      | -    | -     | D1       | c   | o      | o     | 11.472                 | 0.33       | 1.23       | 1    | 23.6     | 0.80       | 3.56  | 11.205                             | 0.21                      | 0.88                      | 0.22                 | 24.9                               | 11.22                                | 0.22                        | 0.92                        |      |      |      |
| 01572719+6601408 | 129.576  | 4.012    | 1.335 | 1      | -   | -   | g      | -    | -     | D3       | -   | -      | -     | 10.569                 | 0.72       | 2.23       | 1    | 42.4     | 0.62       | 3.76  | 10.072                             | 0.49                      | 1.57                      | 0.41                 | 47.8                               | 10.08                                | 0.52                        | 1.66                        |      |      |      |
| 01573573+6319183 | 130.277  | 1.398    | 1.157 | 8      | -   | p   | -      | -    | -     | -        | -   | -      | -     | 11.052                 | 0.84       | 1.09       | 1    | 20.0     | 0.98       | 3.82  | 10.621                             | 0.65                      | 0.51                      | 0.36                 | ...                                | ...                                  | 0.67                        | 0.59                        |      |      |      |
| 01574159+5457437 | 132.417  | -6.685   | 0.321 | 2      | -   | -   | g      | -    | -     | D3       | c   | o      | o     | 11.333                 | 0.42       | 1.10       | 1    | 29.6     | 0.48       | 3.55  | 11.213                             | 0.36                      | 0.94                      | 0.10                 | 30.1                               | 11.22                                | 0.37                        | 0.96                        |      |      |      |
| 01575361+5843286 | 131.480  | -3.040   | 0.604 | 1      | -   | -   | g      | -    | -     | D1       | e   | o      | o     | 11.338                 | 0.38       | 1.12       | 1    | 39.2     | 0.80       | 3.73  | 11.113                             | 0.28                      | 0.96                      | 0.19                 | 41.0                               | 11.12                                | 0.29                        | 1.00                        |      |      |      |
| 01575530+5726037 | 131.814  | -4.286   | 0.422 | 1      | -   | -   | g      | -    | -     | D2       | e   | o      | o     | 10.199                 | 0.34       | 1.14       | 1    | 51.2     | 0.66       | 3.68  | 10.042                             | 0.27                      | 0.93                      | 0.13                 | 52.4                               | 10.06                                | 0.28                        | 0.96                        |      |      |      |
| 01575636+5726026 | 131.816  | -4.286   | 0.422 | 9      | -   | e   | -      | -    | -     | -        | -   | -      | o     | 9.871                  | 0.29       | 1.08       | 1    | 71.6     | 0.62       | 3.72  | 9.714                              | 0.22                      | 0.88                      | 0.13                 | ...                                | ...                                  | 0.23                        | 0.90                        |      |      |      |
| 01581857+6334035 | 130.292  | 1.656    | 2.380 | 8      | -   | -   | g      | -    | -     | D3       | c   | o      | o     | 10.982                 | 0.65       | 1.58       | -2   | 34.6     | 0.48       | 3.81  | 10.095                             | 0.26                      | 0.39                      | 0.74                 | ...                                | ...                                  | 0.30                        | 0.55                        |      |      |      |
| 01582638+7107081 | 128.350  | 8.956    | 0.733 | 1      | -   | -   | g      | -    | -     | D1       | c   | o      | o     | 9.677                  | 0.42       | 1.40       | 1    | 75.0     | 0.38       | 3.55  | 9.404                              | 0.29                      | 1.04                      | 0.23                 | 78.5                               | 9.43                                 | 0.31                        | 1.08                        |      |      |      |
| 01582742+6744421 | 129.231  | 5.697    | 1.303 | 1      | -   | -   | t      | N    | -     | D3       | e   | o      | o     | 11.618                 | 0.44       | 1.49       | 1    | 26.0     | 0.78       | 3.64  | 11.133                             | 0.23                      | 0.84                      | 0.40                 | 29.6                               | 11.12                                | 0.25                        | 0.93                        |      |      |      |
| 01592028+6512575 | 129.973  | 3.277    | 0.891 | 1      | -   | -   | g      | -    | -     | D2       | e   | o      | o     | 11.357                 | 0.38       | 1.32       | 1    | 29.2     | 0.72       | 3.79  | 11.025                             | 0.23                      | 0.88                      | 0.28                 | 31.3                               | 11.04                                | 0.25                        | 0.94                        |      |      |      |
| 01592758+6606246 | 129.753  | 4.140    | 1.326 | 1      | -   | -   | g      | -    | -     | D1       | e   | o      | o     | 9.727                  | 0.48       | 1.62       | 1    | 72.4     | 0.52       | 3.72  | 9.233                              | 0.26                      | 0.97                      | 0.41                 | 80.4                               | 9.26                                 | 0.28                        | 1.05                        |      |      |      |
| 02002296+6531178 | 129.998  | 3.600    | 0.847 | 1      | -   | -   | g      | -    | -     | D3       | c   | o      | o     | 11.176                 | 0.40       | 1.33       | 1    | 35.0     | 0.90       | 3.77  | 10.860                             | 0.26                      | 0.91                      | 0.26                 | 37.6                               | 10.86                                | 0.28                        | 0.97                        |      |      |      |
| 02005846+5423427 | 133.028  | -7.108   | 0.244 | 1      | -   | -   | g      | -    | -     | D2       | c   | o      | o     | 10.856                 | 0.36       | 1.08       | 1    | 31.6     | 0.56       | 3.55  | 10.765                             | 0.32                      | 0.96                      | 0.08                 | 31.9                               | 10.78                                | 0.33                        | 0.97                        |      |      |      |
| 02010098+6337038 | 130.569  | 1.783    | 1.271 | 7      | -   | -   | g      | -    | -     | D1       | e   | o      | o     | 11.713                 | 1.02       | 2.36       | 1    | 16.4     | 0.84       | 3.82  | 11.239                             | 0.81                      | 1.73                      | 0.39                 | ...                                | ...                                  | 0.84                        | 1.81                        |      |      |      |
| 02013241+6824219 | 129.335  | 6.410    | 1.125 | 1      | -   | -   | g      | -    | -     | D1       | e   | o      | o     | 9.593                  | 0.41       | 1.37       | 1    | 88.8     | 0.88       | 3.62  | 9.174                              | 0.23                      | 0.81                      | 0.35                 | 97.3                               | 9.19                                 | 0.25                        | 0.89                        |      |      |      |
| 02021731+6821460 | 129.414  | 6.387    | 1.128 | 1      | -   | -   | g      | -    | -     | D1       | e   | o      | o     | 9.377                  | 0.40       | 1.34       | 1    | 69.4     | 0.58       | 3.62  | 8.957                              | 0.21                      | 0.78                      | 0.35                 | 75.0                               | 8.99                                 | 0.23                        | 0.85                        |      |      |      |
| 02021798+6721240 | 129.690  | 5.420    | 1.642 | 1      | -   | -   | g      | -    | -     | D1       | e   | o      | o     | 10.819                 | 0.48       | 1.61       | 1    | 54.2     | 0.30       | 3.66  | 10.207                             | 0.21                      | 0.80                      | 0.51                 | 63.9                               | 10.20                                | 0.24                        | 0.90                        |      |      |      |
| 02023124+6008000 | 131.677  | -1.526   | 1.316 | 1      | -   | -   | g      | -    | -     | D1       | e   | o      | o     | 11.315                 | 0.55       | 1.51       | 1    | 52.8     | 0.58       | 3.79  | 10.825                             | 0.33                      | 0.86                      | 0.41                 | 62.1                               | 10.74                                | 0.36                        | 0.95                        |      |      |      |
| 02034595+6650152 | 129.971  | 4.960    | 1.540 | 1      | -   | -   | g      | -    | -     | D1       | e   | o      | o     | 11.532                 | 0.56       | 1.78       | 1    | 35.4     | 0.30       | 3.70  | 10.958                             | 0.30                      | 1.02                      | 0.48                 | 41.4                               | 10.94                                | 0.33                        | 1.12                        |      |      |      |
| 02034762+6843532 | 129.445  | 6.780    | 1.018 | 1      | -   | -   | g      | -    | -     | D1       | e   | o      | o     | 11.266                 | 0.35       | 1.39       | 1    | 39.8     | 0.30       | 3.56  | 10.887                             | 0.18                      | 0.88                      | 0.32                 | 43.5                               | 10.89                                | 0.20                        | 0.95                        |      |      |      |
| 02035883+6737172 | 129.772  | 5.718    | 1.176 | 1      | -   | -   | g      | -    | -     | D1       | e   | o      | o     | 11.594                 | 0.38       | 1.33       | 1    | 29.0     | 0.44       | 3.59  | 11.156                             | 0.19                      | 0.74                      | 0.36                 | 32.5                               | 11.14                                | 0.21                        | 0.82                        |      |      |      |
| 02041880+5808286 | 132.447  | -3.378   | 0.501 | 1      | -   | -   | g      | -    | -     | D2       | e   | o      | o     | 10.128                 | 0.32       | 1.12       | 1    | 52.8     | 0.84       | 3.71  | 9.941                              | 0.24                      | 0.88                      | 0.16                 | 54.5                               | 9.95                                 | 0.25                        | 0.91                        |      |      |      |
| 02055021+6749477 | 129.883  | 5.968    | 1.120 | 1      | -   | -   | g      | -    | -     | D1       | e   | o      | o     | 9.665                  | 0.31       | 1.33       | 1    | 88.6     | 0.58       | 3.66  | 9.248                              | 0.13                      | 0.77                      | 0.35                 | 96.5                               | 9.27                                 | 0.15                        | 0.84                        |      |      |      |
| 02061555+6823324 | 129.759  | 6.518    | 1.108 | 1      | -   | -   | g      | -    | -     | D1       | e   | o      | o     | 11.184                 | 0.44       | 1.42       | 1    | 40.8     | 0.72       | 3.59  | 10.771                             | 0.25                      | 0.87                      | 0.34                 | 45.2                               | 10.77                                | 0.28                        | 0.94                        |      |      |      |
| 02063421+5855125 | 132.510  | -2.547   | 0.788 | 1      | -   | -   | g      | -    | -     | D1       | e   | o      | o     | 10.399                 | 0.39       | 1.23       | 1    | 44.4     | 0.46       | 3.87  | 10.105                             | 0.26                      | 0.83                      | 0.24                 | 46.9                               | 10.13                                | 0.28                        | 0.89                        |      |      |      |
| 02072277+5931285 | 132.434  | -1.939   | 0.985 | 1      | -   | -   | g      | -    | -     | D1       | e   | o      | o     | 11.540                 | 0.44       | 1.33       | 1    | 50.4     | 0.54       | 3.77  | 11.173                             | 0.28                      | 0.84                      | 0.31                 | 56.0                               | 11.13                                | 0.30                        | 0.90                        |      |      |      |
| 02080495+6046006 | 132.157  | -0.725   | 4.362 | 8      | -   | -   | g      | -    | -     | D3       | c   | o      | o     | 8.733                  | 1.29       | 2.50       | 1    | 81.0     | 0.98       | 3.78  | 7.108                              | 0.56                      | 0.33                      | 1.35                 | ...                                | ...                                  | 0.65                        | 0.62                        |      |      |      |
| 02082184+6640353 | 130.453  | 4.935    | 1.193 | 1      | -   | -   | g      | -    | -     | D3       | c   | o      | o     | 11.501                 | ...        | ...        | 1    | 27.8     | 1.00       | 3.67  | 11.056                             | ...                       | ...                       | 0.37                 | 31.0                               | 11.06                                | ...                         | ...                         |      |      |      |
| 02082714+6011497 | 132.367  | -1.256   | 2.124 | 9      | -   | -   | g      | -    | -     | D1       | e   | o      | o     | 11.246                 | 0.76       | 1.55       | 1    | 39.2     | 0.82       | 3.79  | 10.455                             | 0.41                      | 0.50                      | 0.66                 | ...                                | ...                                  | 0.45                        | 0.64                        |      |      |      |
| 02084091+7102087 | 129.180  | 9.107    | 0.806 | 1      | -   | -   | g      | -    | -     | D1       | c   | o      | o     | 10.944                 | 0.44       | 1.25       | 1    | 53.0     | 0.84       | 3.49  | 10.644                             | 0.31                      | 0.85                      | 0.25                 | 56.7                               | 10.65                                | 0.32                        | 0.90                        |      |      |      |
| 02084861+6228485 | 131.736  | 0.939    | 1.151 | 1      | -   | -   | g      | -    | -     | D1       | e   | o      | o     | 11.595                 | 0.41       | 1.49       | 1    | 26.8     | 0.52       | 3.76  | 11.166                             | 0.22                      | 0.92                      | 0.36                 | 29.7                               | 11.17                                | 0.24                        | 1.00                        |      |      |      |
| 02085980+7114029 | 129.145  | 9.304    | 0.718 | 1      | -   | -   | g      | -    | -     | D1       | e   | o      | o     | 11.157                 | ...        | ...        | 1    | 63.6     | 1.00       | 3.50  | 10.889                             | ...                       | ...                       | 0.22                 | 68.3                               | 10.86                                | ...                         | ...                         |      |      |      |
| 02101852+6300516 | 131.741  | 1.500    | 1.411 | 1      | -   | -   | g      | -    | -     | D1       | e   | o      | o     | 11.360                 | 0.52       | 1.58       | 1    | 41.6     | 0.44       | 3.81  | 10.834                             | 0.29                      | 0.88                      |                      |                                    |                                      |                             |                             |      |      |      |

Table B1: a) continued.

| 2MASX J          | <i>l</i> | <i>b</i> | EBV    | Object | Sample | Disc | 2MRS | Velocity | NIR  | Photom | Ext   | <i>K</i> <sub>20</sub> | <i>H-K</i> | <i>J-K</i> | vc    | <i>a</i> | <i>b/a</i> | st.d. | <i>K</i> <sub>s</sub> <sup>o</sup> | ( <i>H-K</i> ) <sup>o</sup> | ( <i>J-K</i> ) <sup>o</sup> | <i>A</i> <sub>K</sub> | <i>a</i> <sub>d</sub> <sup>o</sup> | <i>K</i> <sub>s</sub> <sup>o,d</sup> | ( <i>H-K</i> ) <sup>o,c</sup> | ( <i>J-K</i> ) <sup>o,c</sup> |       |        |       |      |       |       |        |
|------------------|----------|----------|--------|--------|--------|------|------|----------|------|--------|-------|------------------------|------------|------------|-------|----------|------------|-------|------------------------------------|-----------------------------|-----------------------------|-----------------------|------------------------------------|--------------------------------------|-------------------------------|-------------------------------|-------|--------|-------|------|-------|-------|--------|
| (1)              | deg      | deg      | mag    | class  | off    | flag | gal  | TF       | (7b) | (7c)   | ext'd | type                   | Opt        | HI         | (10b) | flag     | flag       | flag  | mag                                | mag                         | mag                         | mag                   | mag                                | mag                                  | mag                           | mag                           | mag   |        |       |      |       |       |        |
| (1)              | (2a)     | (2b)     | (3)    | (4)    | (5)    | (6)  | (7a) | (7b)     | (7c) | (7d)   | (8)   | (9)                    | (10a)      | (10b)      | (17)  | (18)     | (19)       | (20)  | (21)                               | (22)                        | (23)                        | (24)                  | (25)                               | (26)                                 | (27)                          | (28)                          |       |        |       |      |       |       |        |
| 02213358+7038115 | 130.324  | 9.069    | 0.965  | 9      | e      | —    | —    | —        | —    | —      | —     | cr                     | —          | —          | —     | —        | o          | —     | 11.485                             | 0.38                        | 1.26                        | 1                     | 32.0                               | 0.86                                 | 3.49                          | 11.125                        | 0.22  | 0.78   | 0.30  | ...  | ...   | 0.24  | 0.85   |
| 02220408+6500169 | 132.321  | 3.798    | 1.148  | 1      | —      | —    | —    | —        | —    | —      | —     | D1                     | —          | —          | —     | —        | —          | —     | 11.399                             | 0.54                        | 1.53                        | 1                     | 36.6                               | 0.78                                 | 3.68                          | 10.971                        | 0.35  | 0.96   | 0.36  | 40.7 | 10.97 | 0.37  | 1.03   |
| 02230162+6210409 | 133.397  | 1.182    | 1.258  | 9      | —      | —    | —    | —        | —    | —      | —     | —                      | —          | —          | —     | —        | —          | —     | 11.581                             | 0.79                        | 2.12                        | 1                     | 31.4                               | 0.58                                 | 3.71                          | 11.112                        | 0.58  | 1.49   | 0.39  | ...  | ...   | 0.61  | 1.57   |
| 02235399+6337032 | 132.989  | 2.566    | 0.885  | 1      | —      | —    | —    | —        | —    | —      | —     | —                      | —          | *          | —     | —        | —          | —     | 10.973                             | 0.46                        | 1.59                        | 1                     | 38.0                               | 0.70                                 | 3.83                          | 10.643                        | 0.31  | 1.15   | 0.27  | 40.8 | 10.66 | 0.33  | 1.21   |
| 02240808+6458272 | 132.537  | 3.846    | 1.153  | 1      | —      | —    | —    | —        | —    | —      | —     | D2                     | —          | —          | —     | —        | —          | —     | 11.117                             | 0.42                        | 1.45                        | 1                     | 31.2                               | 0.84                                 | 3.72                          | 10.687                        | 0.23  | 0.88   | 0.36  | 34.3 | 10.70 | 0.26  | 0.95   |
| 02243924+5926126 | 134.540  | -1.317   | 1.077  | 1      | —      | —    | —    | —        | —    | —      | —     | D1                     | —          | *          | —     | —        | —          | —     | 11.347                             | 0.46                        | 1.51                        | 1                     | 35.0                               | 0.66                                 | 3.76                          | 10.946                        | 0.28  | 0.98   | 0.33  | 38.5 | 10.95 | 0.30  | 1.05   |
| 02245812+6214020 | 133.589  | 1.313    | 6.653  | 4      | —      | —    | —    | t        | N    | —      | —     | D3                     | —          | —          | —     | —        | —          | e     | 12.768                             | 0.80                        | 2.33                        | 1                     | 20.0                               | 0.62                                 | 3.92                          | 10.289                        | -0.30 | -0.98  | 2.06  | 61.6 | 9.73  | -0.17 | -0.54  |
| 02245872+5201488 | 137.216  | -8.228   | 0.203  | 1      | —      | —    | —    | —        | —    | —      | —     | D1                     | —          | —          | —     | —        | —          | —     | 11.128                             | 0.32                        | 1.10                        | 1                     | 36.0                               | 0.78                                 | 3.52                          | 11.052                        | 0.29  | 1.00   | 0.06  | 36.4 | 11.06 | 0.29  | 1.01   |
| 02250110+6206590 | 133.636  | 1.206    | 34.765 | 9      | —      | —    | —    | —        | —    | —      | —     | —                      | —          | —          | —     | —        | —          | —     | 13.961                             | 0.33                        | 1.10                        | -1                    | 13.0                               | 0.58                                 | 3.92                          | 1.008                         | -5.42 | -16.17 | 10.77 | ...  | ...   | -4.74 | -13.87 |
| 02250182+6207040 | 133.637  | 1.207    | 35.583 | 9      | —      | —    | —    | —        | —    | —      | —     | —                      | —          | —          | —     | —        | —          | —     | 13.311                             | 0.53                        | 1.94                        | -1                    | 10.0                               | 1.00                                 | 3.92                          | 0.053                         | -5.36 | -15.73 | 11.02 | ...  | ...   | -4.66 | -13.39 |
| 02250676+6200570 | 133.682  | 1.115    | 19.624 | 9      | —      | —    | —    | —        | —    | —      | —     | —                      | —          | —          | —     | —        | —          | —     | 13.906                             | 0.63                        | 1.19                        | -1                    | 13.4                               | 1.00                                 | 3.79                          | 6.594                         | -2.62 | -8.56  | 6.08  | ...  | ...   | -2.23 | -7.26  |
| 02250706+6203130 | 133.669  | 1.151    | 30.830 | 9      | —      | —    | —    | —        | —    | —      | —     | —                      | —          | —          | —     | —        | —          | —     | 12.881                             | 0.64                        | ...                         | ...                   | 23.2                               | 1.00                                 | 3.92                          | 1.394                         | -4.47 | ...    | 9.55  | ...  | ...   | -3.86 | ...    |
| 02250934+6203280 | 133.672  | 1.156    | 34.126 | 9      | —      | —    | —    | —        | —    | —      | —     | —                      | —          | —          | —     | —        | —          | —     | 12.888                             | ...                         | ...                         | ...                   | 19.0                               | 1.00                                 | 3.92                          | 0.173                         | ...   | ...    | 10.57 | ...  | ...   | ...   | ...    |
| 02252060+6204279 | 133.687  | 1.180    | 49.619 | 9      | —      | —    | —    | —        | —    | —      | —     | —                      | —          | —          | —     | —        | —          | —     | 12.430                             | 1.07                        | 1.73                        | 1                     | 32.6                               | 0.50                                 | 3.92                          | -6.058                        | -7.14 | -22.92 | 15.37 | ...  | ...   | -6.17 | -19.65 |
| 02252065+6204062 | 133.689  | 1.174    | 46.622 | 8      | —      | —    | —    | —        | —    | —      | —     | —                      | —          | —          | —     | —        | —          | —     | 11.133                             | 1.02                        | 2.53                        | 1                     | 50.2                               | 0.74                                 | 4.14                          | -6.238                        | -6.70 | -20.64 | 14.44 | ...  | ...   | -5.78 | -17.56 |
| 02252235+6207318 | 133.672  | 1.229    | 52.994 | 9      | —      | —    | —    | —        | —    | —      | —     | —                      | —          | —          | —     | —        | —          | —     | 11.405                             | 0.55                        | 2.01                        | 1                     | 39.0                               | 0.80                                 | 3.92                          | -8.341                        | -8.23 | -24.32 | 16.42 | ...  | ...   | -7.19 | -20.82 |
| 02252239+6200308 | 133.713  | 1.119    | 20.569 | 9      | —      | —    | —    | —        | —    | —      | —     | —                      | —          | —          | —     | —        | —          | —     | 11.806                             | 1.93                        | ...                         | ...                   | 48.2                               | 0.32                                 | 3.79                          | 4.142                         | -1.47 | ...    | 6.37  | ...  | ...   | -1.07 | ...    |
| 02252262+6206408 | 133.677  | 1.216    | 57.746 | 9      | —      | —    | —    | —        | —    | —      | —     | —                      | —          | —          | —     | —        | —          | —     | 9.425                              | 0.91                        | 2.67                        | 1                     | 187.4                              | 0.30                                 | 3.92                          | -12.091                       | -8.65 | -26.01 | 17.89 | ...  | ...   | -7.52 | -22.20 |
| 02252323+6159508 | 133.719  | 1.110    | 17.391 | 9      | —      | —    | —    | —        | —    | —      | —     | —                      | —          | —          | —     | —        | —          | —     | 9.205                              | 1.18                        | 1.92                        | 1                     | 182.0                              | 0.26                                 | 3.79                          | 2.725                         | -1.70 | -6.72  | 5.39  | ...  | ...   | -1.35 | -5.57  |
| 02252454+6200152 | 133.719  | 1.117    | 18.821 | 9      | —      | —    | —    | —        | —    | —      | —     | —                      | —          | —          | —     | —        | —          | —     | 8.310                              | 1.24                        | 1.74                        | 1                     | 136.0                              | 0.68                                 | 4.14                          | 1.297                         | -1.88 | -7.61  | 5.83  | ...  | ...   | -1.51 | -6.37  |
| 02252485+6203468 | 133.699  | 1.172    | 45.779 | 9      | —      | —    | —    | —        | —    | —      | —     | —                      | —          | —          | —     | —        | —          | —     | 8.239                              | 1.19                        | 2.32                        | 1                     | 123.8                              | 0.70                                 | 3.92                          | -8.818                        | -6.40 | -20.43 | 14.18 | ...  | ...   | -5.50 | -17.41 |
| 02252690+6204592 | 133.695  | 1.192    | 53.899 | 7      | —      | —    | —    | —        | —    | —      | —     | —                      | —          | —          | —     | —        | —          | —     | 11.543                             | 1.10                        | 2.48                        | 1                     | 25.4                               | 0.74                                 | 4.14                          | -8.540                        | -7.83 | -24.30 | 16.70 | ...  | ...   | -6.77 | -20.74 |
| 02252692+6203342 | 133.704  | 1.170    | 44.492 | 9      | —      | —    | —    | —        | —    | —      | —     | —                      | —          | —          | —     | —        | —          | —     | 8.016                              | 1.25                        | 2.32                        | 1                     | 103.8                              | 0.86                                 | 4.14                          | -8.562                        | -6.12 | -19.78 | 13.78 | ...  | ...   | -5.25 | -16.84 |
| 02253143+6206473 | 133.693  | 1.223    | 62.508 | 9      | —      | —    | —    | —        | —    | —      | —     | —                      | —          | —          | —     | —        | —          | —     | 7.502                              | 1.88                        | 3.80                        | 1                     | 118.0                              | 0.82                                 | 4.14                          | -15.788                       | -8.47 | -27.26 | 19.36 | ...  | ...   | -7.24 | -23.13 |
| 02253231+5049100 | 137.738  | -9.327   | 0.342  | 1      | —      | —    | g    | t        | —    | —      | —     | D1                     | c          | o          | h     | —        | —          | —     | 10.216                             | 0.37                        | 1.22                        | 1                     | 55.0                               | 0.36                                 | 3.42                          | 10.089                        | 0.31  | 1.05   | 0.11  | 56.0 | 10.10 | 0.32  | 1.07   |
| 02253471+6206413 | 133.699  | 1.224    | 61.799 | 9      | —      | —    | —    | —        | —    | —      | —     | —                      | —          | —          | —     | —        | —          | —     | 7.564                              | 1.97                        | 4.01                        | 1                     | 220.0                              | 0.14                                 | 4.14                          | -15.462                       | -8.26 | -26.70 | 19.14 | ...  | ...   | -7.05 | -22.62 |
| 02253659+6203583 | 133.719  | 1.183    | 48.370 | 8      | —      | —    | —    | —        | —    | —      | —     | —                      | —          | —          | —     | —        | —          | —     | 9.481                              | 1.28                        | ...                         | ...                   | 91.6                               | 0.68                                 | 4.14                          | -8.542                        | -6.73 | ...    | 14.98 | ...  | ...   | -5.78 | ...    |
| 02253700+6206003 | 133.708  | 1.215    | 59.582 | 9      | —      | —    | —    | —        | —    | —      | —     | —                      | —          | —          | —     | —        | —          | —     | 7.519                              | 2.99                        | ...                         | ...                   | 193.6                              | 0.50                                 | 4.14                          | -14.681                       | -6.87 | ...    | 18.46 | ...  | ...   | -5.70 | ...    |
| 02253741+6208143 | 133.695  | 1.250    | 58.692 | 7      | —      | —    | —    | —        | —    | —      | —     | —                      | —          | —          | —     | —        | —          | —     | 11.099                             | 0.86                        | 1.69                        | 1                     | 52.4                               | 0.58                                 | 4.14                          | -10.770                       | -8.86 | -27.46 | 18.18 | ...  | ...   | -7.71 | -23.59 |
| 02254384+6206263 | 133.717  | 1.227    | 57.764 | 9      | —      | —    | —    | —        | —    | —      | —     | —                      | —          | —          | —     | —        | —          | —     | 6.408                              | 1.76                        | 3.42                        | 1                     | 157.6                              | 0.74                                 | 4.14                          | -15.115                       | -7.81 | -25.28 | 17.89 | ...  | ...   | -6.67 | -21.46 |
| 02254523+6214494 | 133.670  | 1.358    | 9.510  | 9      | —      | —    | —    | —        | —    | —      | —     | —                      | —          | —          | —     | —        | —          | —     | 13.660                             | 0.57                        | 1.51                        | -1                    | 11.0                               | 0.60                                 | 3.72                          | 10.117                        | -1.01 | -3.21  | 2.95  | ...  | ...   | -0.82 | -2.59  |
| 02254612+6205283 | 133.727  | 1.213    | 55.511 | 9      | —      | —    | —    | —        | —    | —      | —     | —                      | —          | —          | —     | —        | —          | —     | 11.753                             | ...                         | ...                         | ...                   | 29.6                               | 0.52                                 | 4.14                          | -8.930                        | ...   | ...    | 17.19 | ...  | ...   | ...   | ...    |
| 02254669+6203574 | 133.737  | 1.190    | 45.282 | 9      | —      | —    | —    | —        | —    | —      | —     | —                      | —          | —          | —     | —        | —          | —     | 11.334                             | 1.72                        | 2.55                        | 1                     | 46.4                               | 0.40                                 | 4.14                          | -5.538                        | -5.78 | -19.95 | 14.03 | ...  | ...   | -4.90 | -16.96 |
| 02254698+6203323 | 133.740  | 1.184    | 42.325 | 9      | —      | —    | —    | —        | —    | —      | —     | —                      | —          | —          | —     | —        | —          | —     | 8.417                              | 1.34                        | 2.52                        | 1                     | 133.0                              | 0.28                                 | 4.14                          | -7.353                        | -5.67 | -18.51 | 13.11 | ...  | ...   | -4.84 | -15.72 |
| 02255011+6205573 | 133.732  | 1.223    | 53.987 | 9      | —      | —    | —    | —        | —    | —      | —     | —                      | —          | —          | —     | —        | —          | —     | 10.982                             | 2.05                        | ...                         | ...                   | 33.6                               | 0.58                                 | 4.14                          | -9.134                        | -6.89 | ...    | 16.72 | ...  | ...   | -5.83 | ...    |
| 02255039+6205144 | 133.736  | 1.212    | 50.382 | 8      | —      | —    | —    | —        | —    | —      | —     | —                      | —          | —          | —     | —        | —          | —     | 10.663                             | 2.13                        | ...                         | ...                   | 93.0                               | 0.32                                 | 4.14                          | -8.109                        | -6.21 | ...    | 15.61 | ...  | ...   | -5.22 | ...    |
| 02255962+6158223 | 133.794  | 1.112    | 12.820 | 8      | —      | —    | —    | —        | —    | —      | —     | —                      | —          | —          | —     | —        | —          | —     | 10.041                             | 1.20                        | 2.45                        | 1                     | 62.2                               | 0.66                                 | 4.14                          | 5.264                         | -0.92 | -3.91  | 3.97  | ...  | ...   | -0.67 | -3.07  |
| 02261716+6214502 | 133.728  | 1.380    | 8.850  | 9      | —      | —    | —    | —        | —    | —      | —     | —                      | —          | —          | —     | —        | —          | —     | 13.135                             | 0.74                        | 1.38                        | -1                    | 27.2                               | 0.48                                 | 3.72                          | 9.837                         | -0.72 | -3.02  | 2.74  | ...  | ...   | -0.55 | -2.43  |
| 02262230+6157271 | 133.841  | 1.114    | 12.840 | 9      | —      | —    | —    | —        | —    | —      | —     | —                      | —          | —          | —     | —        | —          | —     | 13.919                             | 0.62                        | 1.70                        | -1                    | 10.0                               | 1.00                                 | 3.74                          | 9.135                         | -1.50 | -4.68  | 3.98  | ...  | ...   | -1.25 | -3.83  |
| 02263848+5002423 | 138.189  | -9.985   | 0.226  | 1      | —      | —    | g    | —        | —    | —      | D1    | c                      | o          | —          | —     | —        | —          | —     | 10.336                             | 0.34                        | 1.10                        | 1                     | 60.6                               | 0.82                                 | 3.39                          | 10.252                        | 0.30  | 0.98   | 0.07  | 61.3 | 10.26 | 0.31  | 1.00   |
| 02264122+6215468 | 133.766  | 1.412    | 8.788  | 9      | —      | —    | —    | —        | —    | —      | —     | —                      | —          | —          | —     | —        | —          | —     | 10.851                             | 1.22                        | 2.04                        | 1                     | 43.8                               | 0.66                                 | 3.93                          | 7.577                         | -0.23 | -2.33  | 2.72  | ...  | ...   | -0.06 | -1.75  |
| 02264302+6158538 | 133.870  | 1.151    | 14.250 | 9      | —      | —    | —    | —        | —    | —      | —     | —                      | —          | —          | —     | —        | —          | —     | 13.007                             | 1.00                        | ...                         | ...                   | 22.2                               | 0.36                                 | 4.03                          | 7.697                         | -1.36 | ...    | 4.41  | ...  | ...   | -1.08 | ...    |
| 022              |          |          |        |        |        |      |      |          |      |        |       |                        |            |            |       |          |            |       |                                    |                             |                             |                       |                                    |                                      |                               |                               |       |        |       |      |       |       |        |

Table B1: a) continued.

| 2MASX J          | <i>l</i>    | <i>b</i>    | EBV        | Object       | Sample     | Disc        | 2MRS        | Velocity   | NIR         | Photom        | Ext         | <i>K</i> <sub>20</sub> | <i>H-K</i>   | <i>J-K</i>  | vc          | <i>a</i>    | <i>b/a</i>  | st.d. | <i>K</i> <sub>s</sub> <sup>o</sup> | ( <i>H-K</i> ) <sup>o</sup> | ( <i>J-K</i> ) <sup>o</sup> | <i>A<sub>K</sub></i> | <i>a</i> <sub>d</sub> <sup>o</sup> | <i>K</i> <sub>s</sub> <sup>o,d</sup> | ( <i>H-K</i> ) <sup>o,c</sup> | ( <i>J-K</i> ) <sup>o,c</sup> |             |             |      |             |             |             |      |
|------------------|-------------|-------------|------------|--------------|------------|-------------|-------------|------------|-------------|---------------|-------------|------------------------|--------------|-------------|-------------|-------------|-------------|-------|------------------------------------|-----------------------------|-----------------------------|----------------------|------------------------------------|--------------------------------------|-------------------------------|-------------------------------|-------------|-------------|------|-------------|-------------|-------------|------|
| (1)              | deg<br>(2a) | deg<br>(2b) | mag<br>(3) | class<br>(4) | off<br>(5) | flag<br>(6) | gal<br>(7a) | TF<br>(7b) | obs<br>(7c) | ext'd<br>(7d) | type<br>(8) | (9)                    | Opt<br>(10a) | HI<br>(10b) | flg<br>(11) | flg<br>(12) | flg<br>(13) | (14)  | mag<br>(15)                        | mag<br>(16)                 | (17)                        | (18)                 | (19)                               | (20)                                 | mag<br>(21)                   | mag<br>(22)                   | mag<br>(23) | mag<br>(24) | (25) | mag<br>(26) | mag<br>(27) | mag<br>(28) |      |
| 02295107+6132270 | 134.376     | 0.876       | 2.186      | 8            | —          | —           | —           | —          | —           | —             | —           | —                      | —            | —           | —           | —           | —           | —     | 9.524                              | 0.61                        | 1.58                        | −2                   | 29.6                               | 0.54                                 | 3.79                          | 8.709                         | 0.25        | 0.49        | 0.68 | ...         | ...         | 0.29        | 0.64 |
| 02313335+6800496 | 132.114     | 6.945       | 0.937      | 1            | —          | —           | —           | —          | —           | —             | D3          | —                      | —            | —           | —           | —           | —           | —     | 11.222                             | 0.38                        | 1.32                        | 1                    | 33.4                               | 0.82                                 | 3.54                          | 10.873                        | 0.22        | 0.86        | 0.29 | 36.2        | 10.88       | 0.24        | 0.92 |
| 02313738+6502542 | 133.248     | 4.203       | 1.217      | 1            | —          | —           | —           | —          | —           | —             | D4          | —                      | —            | —           | —           | —           | —           | —     | 10.325                             | 0.43                        | 1.45                        | 1                    | 38.4                               | 0.86                                 | 3.69                          | 9.872                         | 0.22        | 0.85        | 0.38 | 42.3        | 9.90        | 0.25        | 0.93 |
| 02314265+6408193 | 133.601     | 3.364       | 0.961      | 1            | —          | —           | —           | —          | —           | —             | D3          | —                      | —            | —           | —           | —           | —           | —     | 10.130                             | 0.43                        | 1.44                        | 1                    | 44.0                               | 0.86                                 | 3.75                          | 9.772                         | 0.27        | 0.96        | 0.30 | 47.1        | 9.80        | 0.29        | 1.02 |
| 02322165+6454104 | 133.375     | 4.098       | 1.145      | 1            | —          | —           | —           | —          | —           | —             | D1          | —                      | —            | —           | —           | —           | —           | —     | 11.368                             | 0.47                        | 1.49                        | 1                    | 42.0                               | 0.88                                 | 3.68                          | 10.941                        | 0.28        | 0.92        | 0.35 | 47.1        | 10.92       | 0.31        | 0.99 |
| 02324853+6418145 | 133.649     | 3.562       | 0.974      | 1            | —          | —           | —           | —          | —           | —             | D2          | —                      | —            | —           | —           | —           | —           | —     | 10.905                             | 0.43                        | 1.41                        | 1                    | 49.2                               | 0.72                                 | 3.75                          | 10.542                        | 0.26        | 0.93        | 0.30 | 53.4        | 10.55       | 0.28        | 0.99 |
| 02324969+4938202 | 139.282     | −9.987      | 0.278      | 1            | —          | —           | —           | —          | —           | —             | D1          | —                      | —            | —           | —           | —           | —           | —     | 11.145                             | 0.33                        | 1.11                        | 1                    | 38.2                               | 0.78                                 | 3.43                          | 11.041                        | 0.28        | 0.97        | 0.09 | 38.8        | 11.05       | 0.29        | 0.99 |
| 02332153+6009100 | 135.295     | −0.249      | 1.244      | 1            | —          | —           | —           | —          | —           | —             | D1          | —                      | —            | —           | —           | —           | —           | —     | 11.219                             | 0.56                        | 1.84                        | 1                    | 46.8                               | 0.72                                 | 3.84                          | 10.755                        | 0.35        | 1.22        | 0.39 | 53.5        | 10.72       | 0.38        | 1.30 |
| 02334600+6405011 | 133.830     | 3.399       | 0.992      | 1            | —          | —           | —           | —          | —           | —             | D1          | —                      | —            | —           | —           | —           | —           | —     | 10.904                             | 0.48                        | 1.48                        | 1                    | 39.2                               | 0.44                                 | 3.73                          | 10.534                        | 0.32        | 0.99        | 0.31 | 42.8        | 10.53       | 0.34        | 1.05 |
| 02341102+6700106 | 132.738     | 6.108       | 1.301      | 1            | —          | —           | —           | —          | —           | —             | D1          | —                      | —            | —           | —           | —           | —           | —     | 10.627                             | 0.41                        | 1.52                        | 1                    | 43.2                               | 0.90                                 | 3.57                          | 10.142                        | 0.19        | 0.87        | 0.40 | 48.4        | 10.16       | 0.22        | 0.96 |
| 02341282+6802576 | 132.331     | 7.073       | 0.983      | 1            | —          | —           | —           | —          | —           | —             | D4          | —                      | —            | —           | —           | —           | —           | —     | 10.687                             | 0.42                        | 1.45                        | 1                    | 31.8                               | 0.88                                 | 3.60                          | 10.321                        | 0.26        | 0.96        | 0.30 | 34.2        | 10.34       | 0.28        | 1.02 |
| 02343179+6755266 | 132.408     | 6.970       | 1.082      | 1            | —          | —           | —           | —          | —           | —             | D3          | —                      | —            | —           | —           | —           | —           | —     | 10.257                             | 0.38                        | 1.43                        | 1                    | 43.4                               | 0.72                                 | 3.60                          | 9.854                         | 0.20        | 0.89        | 0.34 | 47.2        | 9.87        | 0.23        | 0.96 |
| 02352112+5814384 | 136.268     | −1.911      | 1.041      | 1            | —          | —           | —           | —          | —           | —             | D2          | —                      | —            | —           | —           | —           | —           | —     | 11.201                             | 0.42                        | 1.46                        | 1                    | 37.2                               | 0.72                                 | 3.69                          | 10.813                        | 0.25        | 0.94        | 0.32 | 40.9        | 10.81       | 0.27        | 1.01 |
| 02353356+6656497 | 132.884     | 6.109       | 1.115      | 1            | —          | —           | —           | —          | —           | —             | D1          | —                      | —            | —           | —           | —           | —           | —     | 11.386                             | 0.45                        | 1.50                        | 1                    | 48.8                               | 0.66                                 | 3.55                          | 10.971                        | 0.27        | 0.94        | 0.35 | 55.1        | 10.93       | 0.29        | 1.02 |
| 02361585+6845014 | 132.228     | 7.792       | 1.132      | 1            | —          | —           | —           | —          | —           | —             | D1          | —                      | —            | —           | —           | —           | —           | —     | 11.315                             | 0.43                        | 1.44                        | 1                    | 31.2                               | 0.58                                 | 3.54                          | 10.893                        | 0.24        | 0.88        | 0.35 | 34.7        | 10.89       | 0.26        | 0.95 |
| 02363546+5939165 | 135.862     | −0.551      | 1.164      | 1            | —          | —           | —           | —          | —           | —             | D1          | —                      | —            | —           | —           | —           | —           | —     | 4.749                              | 0.46                        | 1.57                        | 1                    | 470.6                              | 0.79                                 | ...                           | 4.315                         | 0.27        | 0.99        | 0.36 | ...         | ...         | 0.29        | 1.07 |
| 02364998+5410339 | 138.062     | −5.570      | 0.379      | 1            | —          | —           | —           | —          | —           | —             | D4          | —                      | —            | —           | —           | —           | —           | —     | 10.816                             | 0.34                        | 1.17                        | 1                    | 34.6                               | 0.92                                 | 3.57                          | 10.675                        | 0.28        | 0.98        | 0.12 | 35.4        | 10.69       | 0.29        | 1.00 |
| 02365909+5444149 | 137.858     | −5.046      | 0.400      | 1            | —          | —           | —           | —          | —           | —             | D3          | —                      | —            | —           | —           | —           | —           | —     | 10.441                             | 0.33                        | 1.15                        | 1                    | 48.0                               | 0.88                                 | 3.66                          | 10.292                        | 0.27        | 0.96        | 0.12 | 49.1        | 10.30       | 0.27        | 0.98 |
| 02370546+5936210 | 135.939     | −0.571      | 1.038      | 4            | —          | —           | —           | —          | —           | —             | D4          | —                      | —            | —           | —           | —           | —           | —     | 11.123                             | 0.47                        | 1.58                        | −2                   | 24.0                               | 0.92                                 | 3.77                          | 10.736                        | 0.30        | 1.07        | 0.32 | 25.9        | 10.76       | 0.32        | 1.13 |
| 02373382+6440563 | 133.973     | 4.110       | 1.130      | 1            | —          | —           | —           | —          | —           | —             | D1          | —                      | —            | —           | —           | —           | —           | —     | 10.937                             | 0.49                        | 1.42                        | 1                    | 39.4                               | 0.72                                 | 3.71                          | 10.516                        | 0.31        | 0.86        | 0.35 | 43.6        | 10.52       | 0.33        | 0.93 |
| 02380987+6222578 | 134.954     | 2.029       | 0.636      | 1            | —          | —           | —           | —          | —           | —             | D1          | —                      | —            | —           | —           | —           | —           | —     | 11.016                             | 0.48                        | 1.44                        | 1                    | 27.6                               | 0.82                                 | 3.73                          | 10.779                        | 0.38        | 1.13        | 0.20 | 28.8        | 10.80       | 0.39        | 1.17 |
| 02390747+5153273 | 139.303     | −7.525      | 0.311      | 1            | —          | —           | —           | —          | —           | —             | D3          | —                      | —            | —           | —           | —           | —           | —     | 10.917                             | 0.33                        | 1.11                        | 1                    | 33.4                               | 0.96                                 | 3.53                          | 10.801                        | 0.28        | 0.96        | 0.10 | 34.0        | 10.81       | 0.28        | 0.98 |
| 02392731+6431291 | 134.223     | 4.048       | 0.987      | 1            | —          | —           | —           | —          | —           | —             | D1          | —                      | —            | —           | —           | —           | —           | —     | 11.206                             | 0.57                        | 1.61                        | 1                    | 43.4                               | 0.44                                 | 3.75                          | 10.838                        | 0.40        | 1.12        | 0.31 | 47.4        | 10.84       | 0.42        | 1.19 |
| 02403604+5854138 | 136.632     | −1.033      | 1.048      | 2            | —          | —           | —           | —          | —           | —             | D4          | —                      | —            | —           | —           | —           | —           | —     | 11.322                             | 0.49                        | 1.47                        | 1                    | 24.8                               | 0.90                                 | 3.79                          | 10.932                        | 0.32        | 0.95        | 0.32 | 27.0        | 10.95       | 0.34        | 1.02 |
| 02404972+5854097 | 136.660     | −1.022      | 1.056      | 8            | —          | —           | —           | —          | —           | —             | —           | —                      | —            | —           | —           | —           | —           | —     | 11.576                             | 1.01                        | 2.92                        | −2                   | 19.6                               | 0.62                                 | 3.79                          | 11.183                        | 0.84        | 2.40        | 0.33 | ...         | ...         | 0.86        | 2.47 |
| 02415509+5936147 | 136.499     | −0.326      | 2.427      | 1            | —          | s           | —           | —          | —           | —             | D1          | —                      | —            | —           | —           | —           | —           | —     | 5.331                              | 0.52                        | 1.69                        | 1                    | 572.8                              | 0.53                                 | ...                           | 4.427                         | 0.12        | 0.49        | 0.75 | ...         | ...         | 0.17        | 0.65 |
| 02421337+6723309 | 133.298     | 6.777       | 1.173      | 1            | —          | —           | —           | —          | —           | —             | D1          | —                      | —            | —           | —           | —           | —           | —     | 10.368                             | 0.38                        | 1.37                        | 1                    | 72.6                               | 1.18                                 | 3.65                          | 9.931                         | 0.19        | 0.78        | 0.36 | 80.0        | 9.95        | 0.21        | 0.86 |
| 02422187+6254033 | 135.184     | 2.698       | 2.085      | 8            | —          | —           | —           | —          | —           | —             | —           | —                      | —            | —           | —           | —           | —           | —     | 9.343                              | 0.51                        | 1.27                        | −2                   | 108.2                              | 0.62                                 | 3.73                          | 8.566                         | 0.17        | 0.24        | 0.65 | ...         | ...         | 0.21        | 0.37 |
| 02422242+6213323 | 135.465     | 2.084       | 0.525      | 1            | —          | —           | —           | —          | —           | —             | D3          | —                      | —            | —           | —           | —           | —           | —     | 11.445                             | 0.49                        | 1.38                        | 1                    | 23.6                               | 0.82                                 | 3.79                          | 11.249                        | 0.40        | 1.12        | 0.16 | 24.4        | 11.26       | 0.41        | 1.15 |
| 02432862+6257087 | 135.277     | 2.798       | 2.110      | 7            | —          | —           | —           | —          | —           | —             | D1          | —                      | —            | —           | —           | —           | —           | —     | 10.256                             | 1.46                        | 2.94                        | 1                    | 28.6                               | 0.78                                 | 3.76                          | 9.470                         | 1.11        | 1.90        | 0.65 | ...         | ...         | 1.16        | 2.03 |
| 02440181+7005273 | 132.300     | 9.295       | 1.785      | 1            | —          | —           | —           | —          | —           | —             | D1          | —                      | —            | —           | —           | —           | —           | —     | 11.217                             | 0.48                        | 1.54                        | 1                    | 44.4                               | 0.72                                 | 3.39                          | 10.552                        | 0.19        | 0.65        | 0.55 | 55.2        | 10.47       | 0.22        | 0.77 |
| 02442060+6034374 | 136.368     | 0.685       | 2.410      | 7            | —          | —           | —           | —          | —           | —             | D1          | —                      | —            | —           | —           | —           | —           | —     | 11.532                             | 1.32                        | 3.54                        | 1                    | 13.4                               | 0.88                                 | 3.74                          | 10.634                        | 0.92        | 2.34        | 0.75 | ...         | ...         | 0.97        | 2.50 |
| 02442271+5507524 | 138.668     | −4.252      | 0.614      | 1            | —          | —           | —           | —          | —           | —             | D1          | —                      | —            | —           | —           | —           | —           | —     | 11.208                             | 0.40                        | 1.37                        | 1                    | 35.8                               | 0.32                                 | 3.66                          | 10.979                        | 0.30        | 1.07        | 0.19 | 37.3        | 11.00       | 0.31        | 1.11 |
| 02442699+4933031 | 141.063     | −9.301      | 0.321      | 1            | —          | —           | —           | —          | —           | —             | D1          | —                      | —            | —           | —           | —           | —           | —     | 10.912                             | 0.32                        | 1.19                        | 1                    | 53.4                               | 0.56                                 | 3.49                          | 10.792                        | 0.27        | 1.03        | 0.10 | 54.4        | 10.80       | 0.27        | 1.05 |
| 02443634+6059433 | 136.221     | 1.078       | 2.258      | 8            | —          | —           | —           | —          | —           | —             | D1          | —                      | —            | —           | —           | —           | —           | —     | 10.660                             | 0.55                        | 1.51                        | 1                    | 50.6                               | 0.72                                 | 3.83                          | 9.819                         | 0.17        | 0.39        | 0.70 | ...         | ...         | 0.22        | 0.53 |
| 02443854+6100173 | 136.221     | 1.088       | 2.224      | 8            | —          | —           | —           | —          | —           | —             | D1          | —                      | —            | —           | —           | —           | —           | —     | 10.916                             | 1.08                        | 2.50                        | 1                    | 23.4                               | 0.78                                 | 3.83                          | 10.087                        | 0.71        | 1.39        | 0.69 | ...         | ...         | 0.76        | 1.54 |
| 02444352+4936597 | 141.076     | −9.222      | 0.314      | 1            | —          | —           | —           | —          | —           | —             | D2          | —                      | —            | —           | —           | —           | —           | —     | 11.124                             | 0.28                        | 1.09                        | 1                    | 34.8                               | 0.46                                 | 3.54                          | 11.007                        | 0.23        | 0.94        | 0.10 | 35.4        | 11.02       | 0.24        | 0.96 |
| 02451105+6049328 | 136.356     | 0.954       | 2.938      | 9            | —          | —           | —           | —          | —           | —             | D1          | —                      | —            | —           | —           | —           | —           | —     | 11.409                             | 1.27                        | 2.76                        | 1                    | 34.8                               | 0.76                                 | 3.84                          | 10.314                        | 0.79        | 1.30        | 0.91 | ...         | ...         | 0.85        | 1.50 |
| 02455702+5522336 | 138.767     | −3.935      | 0.763      | 1            | —          | —           | —           | —          | —           | —             | D1          | —                      | —            | —           | —           | —           | —           | —     | 11.397                             | 0.49                        | 1.42                        | 1                    | 52.4                               | 0.26                                 | 3.66                          | 11.113                        | 0.36        | 1.04        | 0.24 | 56.0        | 11.11       | 0.38        | 1.09 |
| 02460054+5115142 | 140.552     | −7.655      | 0.329      | 1            | —          | —           | —           | —          | —           | —             | D2          | —                      | —            | —           | —           | —           | —           | —     | 10.733                             | 0.44                        | 1.21                        | 1                    | 34.2                               | 0.92                                 | 3.60                          | 10.610                        | 0.39        | 1.04        | 0.10 | 34.8        | 10.62       | 0.39        | 1.07 |
| 02460356+6455149 | 134.700     | 4.701       | 1.160      | 1            | —          | —           | —           | —          | —           | —             | D1          | —                      | —            | —           | —           | —           | —           | —     | 11.167                             | 0.40                        | 1.39                        | 1                    | 37.2                               | 0.38                                 | 3.67                          | 10.735                        | 0.21        | 0.81        | 0.36 | 41.0        | 10.75       | 0.23        | 0.89 |
| 02460684+6246320 | 135.625</   |             |            |              |            |             |             |            |             |               |             |                        |              |             |             |             |             |       |                                    |                             |                             |                      |                                    |                                      |                               |                               |             |             |      |             |             |             |      |



Table B1: a) continued.

| 2MASS J          |         | $l$    | $b$   | EBV | Object | Sample | Disc | 2MRS | Velocity | NIR | Photom | Ext  | $K_{20}$ | $H-K$ | $J-K$ | vc    | $a$  | $b/a$ | st.d. | $K^o_s$ | $(H-K)^o$ | $(J-K)^o$ | $A_K$ | $a''$ | $K^{o,d}$ | $(H-K)^{o,c}$ | $(J-K)^{o,c}$ |        |       |       |      |      |       |      |     |       |       |      |     |      |     |      |     |      |     |      |
|------------------|---------|--------|-------|-----|--------|--------|------|------|----------|-----|--------|------|----------|-------|-------|-------|------|-------|-------|---------|-----------|-----------|-------|-------|-----------|---------------|---------------|--------|-------|-------|------|------|-------|------|-----|-------|-------|------|-----|------|-----|------|-----|------|-----|------|
| (1)              |         | deg    | deg   | mag | class  | off    | flag | gal  | TF       | obs | ext/d  | type | (9)      | Opt   | HI    | (10b) | (11) | (12)  | flag  | (13)    | mag       | (14)      | mag   | (15)  | mag       | (16)          | (17)          | (18)   | (19)  | (20)  | mag  | (21) | mag   | (22) | mag | (23)  | mag   | (24) | mag | (25) | mag | (26) | mag | (27) | mag | (28) |
| 02513047+6208547 | 136.461 | 2.473  | 1.888 | 9   | -      | -      | -    | -    | -        | -   | -      | -    | -        | -     | -     | -     | -    | -     | -     | -       | 11.810    | 1.25      | 2.63  | 1     | 33.2      | 0.40          | 3.79          | 11.107 | 0.94  | 1.69  | 0.58 | ...  | ...   | ...  | ... | 0.98  | 1.81  |      |     |      |     |      |     |      |     |      |
| 02514925+5049246 | 141.571 | -7.639 | 0.402 | 1   | -      | -      | -    | g    | -        | -   | -      | D2   | c        | o     | -     | -     | -    | -     | -     | -       | 10.689    | 0.30      | 1.10  | 1     | 38.6      | 0.94          | 3.55          | 10.539 | 0.24  | 0.90  | 0.12 | 39.6 | 10.55 | ...  | ... | 0.25  | 0.93  |      |     |      |     |      |     |      |     |      |
| 02515372+6006564 | 137.410 | 0.674  | 1.391 | 8   | -      | -      | -    | -    | -        | -   | -      | -    | -        | -     | -     | -     | -    | -     | -     | -       | 10.447    | 1.33      | 2.65  | 1     | 49.6      | 0.62          | 3.81          | 9.929  | 1.10  | 1.96  | 0.43 | ...  | ...   | ...  | ... | 1.13  | 2.05  |      |     |      |     |      |     |      |     |      |
| 02520392+6235505 | 136.318 | 2.903  | 0.812 | 1   | -      | -      | -    | g    | -        | -   | -      | D1   | e        | o     | -     | *     | -    | -     | -     | -       | 10.890    | 0.40      | 1.36  | 1     | 47.6      | 0.98          | 3.79          | 10.587 | 0.27  | 0.96  | 0.25 | 50.7 | 10.60 | ...  | ... | 0.28  | 1.01  |      |     |      |     |      |     |      |     |      |
| 02521671+5234547 | 140.837 | -6.038 | 0.466 | 1   | -      | -      | -    | g    | -        | -   | -      | D2   | c        | o     | o     | -     | -    | -     | -     | -       | 10.519    | 0.31      | 1.12  | 1     | 38.8      | 0.62          | 3.51          | 10.345 | 0.24  | 0.89  | 0.14 | 39.8 | 10.36 | ...  | ... | 0.24  | 0.92  |      |     |      |     |      |     |      |     |      |
| 02525512+5203283 | 141.163 | -6.461 | 0.440 | 1   | -      | -      | -    | g    | -        | -   | -      | D3   | c        | o     | o     | -     | -    | -     | -     | -       | 11.246    | 0.40      | 1.24  | 1     | 30.2      | 0.72          | 3.57          | 11.082 | 0.33  | 1.02  | 0.14 | 31.0 | 11.09 | ...  | ... | 0.34  | 1.05  |      |     |      |     |      |     |      |     |      |
| 02525589+5220513 | 141.033 | -6.202 | 0.428 | 1   | -      | -      | -    | g    | t        | -   | -      | D1   | c        | o     | -     | -     | -    | -     | -     | -       | 11.225    | 0.45      | 1.30  | 1     | 38.2      | 0.36          | 3.55          | 11.066 | 0.38  | 1.09  | 0.13 | 39.3 | 11.08 | ...  | ... | 0.39  | 1.12  |      |     |      |     |      |     |      |     |      |
| 02530638+6914374 | 133.395 | 8.882  | 3.652 | 8   | -      | -      | -    | g    | -        | -   | -      | -    | -        | -     | -     | -     | -    | -     | -     | -       | 11.743    | 1.89      | 3.66  | 1     | 19.0      | 0.74          | 3.45          | 10.382 | 1.29  | 1.85  | 1.13 | ...  | ...   | ...  | ... | 1.36  | 2.09  |      |     |      |     |      |     |      |     |      |
| 02531475+5528143 | 139.657 | -3.395 | 1.318 | 1   | -      | -      | -    | g    | t        | N   | -      | D1   | e        | o     | -     | h?    | -    | -     | -     | -       | 10.679    | 0.54      | 1.60  | 1     | 64.0      | 0.40          | 3.63          | 10.188 | 0.32  | 0.95  | 0.41 | 72.6 | 10.18 | ...  | ... | 0.35  | 1.03  |      |     |      |     |      |     |      |     |      |
| 02531484+5732583 | 138.718 | -1.540 | 1.335 | 1   | -      | -      | -    | g    | -        | -   | -      | -    | -        | -     | -     | -     | -    | -     | -     | -       | 10.886    | 0.56      | 1.59  | 1     | 41.6      | 0.90          | 3.64          | 10.389 | 0.34  | 0.92  | 0.41 | 47.3 | 10.38 | ...  | ... | 0.37  | 1.0   |      |     |      |     |      |     |      |     |      |
| 02531969+5529140 | 139.660 | -3.375 | 1.307 | 1   | -      | -      | -    | g    | -        | N   | -      | D3   | -        | -     | -     | *     | -    | -     | -     | -       | 10.771    | 0.49      | 1.48  | 1     | 33.2      | 0.58          | 3.65          | 10.284 | 0.28  | 0.83  | 0.40 | 37.1 | 10.30 | ...  | ... | 0.30  | 0.92  |      |     |      |     |      |     |      |     |      |
| 02534352+6229234 | 136.537 | 2.894  | 1.005 | 7   | -      | -      | -    | g    | -        | -   | -      | -    | -        | -     | -     | -     | -    | -     | -     | -       | 9.833     | 1.43      | 3.07  | 1     | 26.2      | 0.72          | 3.78          | 9.459  | 1.26  | 2.57  | 0.31 | ...  | ...   | ...  | ... | 1.28  | 2.64  |      |     |      |     |      |     |      |     |      |
| 02541189+5152046 | 141.427 | -6.540 | 0.431 | 1   | -      | -      | -    | g    | -        | -   | -      | D2   | c        | o     | -     | -     | -    | -     | -     | -       | 10.985    | 0.33      | 1.16  | 1     | 33.4      | 0.88          | 3.53          | 10.824 | 0.25  | 0.94  | 0.13 | 34.2 | 10.84 | ...  | ... | 0.26  | 0.97  |      |     |      |     |      |     |      |     |      |
| 02543223+6923377 | 133.439 | 9.073  | 3.938 | 7   | -      | -      | -    | -    | -        | -   | -      | -    | -        | -     | -     | -     | -    | -     | -     | -       | 12.502    | ...       | ...   | 1     | 47.6      | 0.20          | 3.48          | 11.035 | ...   | ...   | 1.22 | ...  | ...   | ...  | ... | ...   | ...   | ...  | ... | ...  |     |      |     |      |     |      |
| 02543376+6920077 | 133.468 | 9.022  | 3.925 | 9   | -      | -      | -    | -    | -        | -   | -      | -    | -        | -     | -     | -     | -    | -     | -     | -       | 11.883    | 2.61      | ...   | 1     | 22.4      | 0.48          | 3.48          | 10.421 | 1.96  | ...   | ...  | 1.22 | ...   | ...  | ... | 2.04  | ...   | ...  | ... | ...  | ... |      |     |      |     |      |
| 02543754+6919027 | 133.482 | 9.009  | 3.641 | 9   | -      | -      | -    | -    | -        | -   | -      | -    | -        | -     | -     | -     | -    | -     | -     | -       | 11.515    | 1.17      | 2.60  | 1     | 25.2      | 0.80          | 3.48          | 10.158 | 0.57  | 0.79  | 1.13 | ...  | ...   | ...  | ... | 0.64  | 1.03  |      |     |      |     |      |     |      |     |      |
| 02545129+5625144 | 139.426 | -2.447 | 1.296 | 1   | -      | -      | -    | g    | -        | N   | -      | D3   | -        | -     | -     | *     | -    | -     | -     | -       | 11.668    | 0.50      | 1.50  | 1     | 27.2      | 0.64          | 3.73          | 11.185 | 0.29  | 0.86  | 0.40 | 30.8 | 11.18 | ...  | ... | 0.31  | 0.94  |      |     |      |     |      |     |      |     |      |
| 02545182+5720004 | 139.010 | -1.634 | 1.361 | 1   | -      | -      | -    | g    | t        | N   | -      | D1   | -        | -     | -     | -     | -    | -     | -     | -       | 11.457    | 0.50      | 1.53  | 1     | 37.0      | 0.52          | 3.70          | 10.950 | 0.28  | 0.85  | 0.42 | 42.1 | 10.95 | ...  | ... | 0.30  | 0.94  |      |     |      |     |      |     |      |     |      |
| 02545198+5812134 | 138.613 | -0.860 | 1.822 | 1   | -      | -      | -    | g    | t        | N   | -      | D2   | -        | -     | -     | *     | -    | -     | -     | -       | 11.540    | 0.47      | 1.64  | 1     | 30.6      | 0.58          | 3.77          | 10.861 | 0.16  | 0.73  | 0.56 | 37.7 | 10.81 | ...  | ... | 0.20  | 0.85  |      |     |      |     |      |     |      |     |      |
| 02550264+6035457 | 137.540 | 1.279  | 2.060 | 9   | -      | -      | -    | -    | -        | -   | -      | -    | -        | -     | -     | -     | -    | -     | -     | -       | 11.491    | 1.45      | 2.32  | 1     | 39.2      | 0.44          | 3.82          | 10.723 | 1.11  | 1.29  | 0.64 | ...  | ...   | ...  | ... | 1.15  | 1.43  |      |     |      |     |      |     |      |     |      |
| 02550583+6624065 | 134.877 | 6.442  | 1.030 | 1   | -      | -      | -    | g    | -        | N   | -      | D1   | c        | o     | -     | h     | -    | -     | -     | -       | 9.727     | 0.42      | 1.37  | 1     | 70.8      | 0.54          | 3.58          | 9.343  | 0.25  | 0.86  | 0.32 | 77.0 | 9.36  | ...  | ... | 0.27  | 0.93  |      |     |      |     |      |     |      |     |      |
| 02551108+5154257 | 141.545 | -6.436 | 0.437 | 1   | -      | -      | -    | g    | t        | -   | -      | D1   | c        | o     | -     | h     | -    | -     | -     | -       | 9.656     | 0.33      | 1.13  | 1     | 91.0      | 0.38          | ...           | ...    | 9.493 | 0.26  | 0.91 | 0.14 | ...   | ...  | ... | ...   | 0.27  | 0.94 |     |      |     |      |     |      |     |      |
| 02552896+6040057 | 137.555 | 1.368  | 3.099 | 8   | -      | -      | -    | -    | -        | -   | -      | -    | -        | -     | -     | -     | -    | -     | -     | -       | 11.294    | 0.80      | 1.87  | 1     | 23.0      | 0.66          | 3.80          | 10.139 | 0.29  | 0.33  | 0.96 | ...  | ...   | ...  | ... | 0.35  | 0.53  |      |     |      |     |      |     |      |     |      |
| 02554290+5851394 | 138.410 | -0.225 | 1.302 | 1   | -      | -      | -    | g    | -        | -   | -      | D1   | e        | o     | -     | -     | -    | -     | -     | -       | 11.499    | 0.46      | 1.53  | 1     | 48.6      | 0.76          | 3.73          | 11.014 | 0.25  | 0.89  | 0.40 | 57.7 | 10.90 | ...  | ... | 0.27  | 0.97  |      |     |      |     |      |     |      |     |      |
| 02562619+6044597 | 137.621 | 1.494  | 5.284 | 9   | -      | -      | -    | -    | -        | -   | -      | -    | -        | -     | -     | -     | -    | -     | -     | -       | 12.481    | 0.91      | 2.03  | -2    | 25.8      | 0.32          | 3.76          | 10.512 | 0.04  | -0.60 | 1.64 | ...  | ...   | ...  | ... | 0.14  | -0.25 |      |     |      |     |      |     |      |     |      |
| 02562677+6045042 | 137.621 | 1.496  | 5.390 | 8   | -      | -      | -    | -    | -        | -   | -      | -    | -        | -     | -     | -     | -    | -     | -     | -       | 11.518    | 0.88      | 2.18  | 1     | 39.8      | 0.38          | 3.81          | 9.541  | -0.00 | -0.45 | 1.64 | ...  | ...   | ...  | ... | 0.10  | -0.25 |      |     |      |     |      |     |      |     |      |
| 02563463+4841253 | 143.251 | -9.182 | 0.340 | 1   | -      | -      | -    | g    | -        | -   | -      | D4   | c        | o     | -     | -     | -    | -     | -     | -       | 10.400    | 0.29      | 1.06  | 1     | 47.4      | 0.78          | 3.42          | 10.273 | 0.23  | 0.89  | 0.11 | 48.3 | 10.29 | ...  | ... | 0.24  | 0.91  |      |     |      |     |      |     |      |     |      |
| 02564496+5035432 | 142.376 | -7.485 | 0.519 | 1   | -      | -      | -    | g    | t        | -   | -      | D1   | c        | o     | -     | h     | -    | -     | -     | -       | 10.627    | 0.51      | 1.43  | 1     | 62.0      | 0.26          | 3.53          | 10.434 | 0.42  | 1.17  | 0.16 | 64.2 | 10.44 | ...  | ... | 0.26  | 1.21  |      |     |      |     |      |     |      |     |      |
| 02565165+5854416 | 138.518 | -0.111 | 1.464 | 1   | -      | -      | -    | g    | t        | -   | -      | D1   | e        | o     | -     | h     | -    | -     | -     | -       | 9.453     | 0.16      | 1.52  | 1     | 155.0     | 0.40          | ...           | ...    | 8.908 | 0.22  | 0.80 | 0.05 | ...   | ...  | ... | ...   | 0.35  | 0.65 |     |      |     |      |     |      |     |      |
| 02570099+6041103 | 137.713 | 1.470  | 8.511 | 9   | -      | -      | -    | -    | -        | -   | -      | -    | -        | -     | -     | -     | -    | -     | -     | -       | 11.703    | 1.01      | 2.56  | 1     | 21.8      | 0.56          | 3.81          | 8.532  | -0.40 | -1.67 | 2.64 | ...  | ...   | ...  | ... | -0.24 | -1.11 |      |     |      |     |      |     |      |     |      |
| 02570346+5658488 | 139.437 | -1.811 | 1.449 | 1   | -      | -      | -    | g    | t        | N   | -      | -    | -        | -     | -     | *     | -    | -     | -     | -       | 11.444    | 0.43      | 1.52  | 1     | 33.6      | 0.50          | 3.66          | 10.904 | 0.19  | 0.80  | 0.45 | 40.1 | 10.83 | ...  | ... | 0.22  | 0.89  |      |     |      |     |      |     |      |     |      |
| 02570442+6044043 | 137.697 | 1.516  | 9.315 | 9   | -      | -      | -    | -    | -        | -   | -      | -    | -        | -     | -     | -     | -    | -     | -     | -       | 9.823     | 0.64      | 1.19  | 1     | 90.0      | 0.76          | 3.81          | 6.352  | -0.90 | -3.43 | 2.89 | ...  | ...   | ...  | ... | -0.72 | -2.82 |      |     |      |     |      |     |      |     |      |
| 02570681+5032145 | 142.455 | -7.509 | 0.519 | 1   | -      | -      | -    | g    | -        | -   | -      | D1   | c        | o     | -     | -     | -    | -     | -     | -       | 10.295    | 0.34      | 1.16  | 1     | 53.8      | 0.72          | 3.51          | 10.102 | 0.25  | 0.90  | 0.16 | 55.5 | 10.12 | ...  | ... | 0.26  | 0.94  |      |     |      |     |      |     |      |     |      |
| 02572019+6041031 | 137.749 | 1.487  | 8.935 | 7   | -      | -      | -    | -    | -        | -   | -      | -    | -        | -     | -     | -     | -    | -     | -     | -       | 9.822     | 1.15      | 2.71  | 1     | 36.8      | 0.70          | 3.81          | 6.493  | -0.33 | -1.73 | 2.77 | ...  | ...   | ...  | ... | -0.16 | -1.14 |      |     |      |     |      |     |      |     |      |
| 02572253+6038236 | 137.774 | 1.450  | 7.121 | 9   | -      | -      | -    | -    | -        | -   | -      | -    | -        | -     | -     | -     | -    | -     | -     | -       | 13.491    | ...       | ...   | 1     | 16.8      | 0.47          | 3.84          | 10.138 | ...   | ...   | 2.21 | ...  | ...   | ...  | ... | ...   | ...   | ...  | ... |      |     |      |     |      |     |      |
| 02572497+6041380 | 137.753 | 1.500  | 8.939 | 9   | -      | -      | -    | -    | -        | -   | -      | -    | -        | -     | -     | -     | -    | -     | -     | -       | 12.499    | 1.02      | 2.78  | -2    | 11.4      | 0.76          | 3.81          | 9.168  | -0.46 | -1.66 | 2.77 | ...  | ...   | ...  | ... | -0.29 | -1.07 |      |     |      |     |      |     |      |     |      |
| 02572574+6041336 | 137.755 | 1.499  | 8.894 | 9   | -      | -      | -    | -    | -        | -   | -      | -    | -        | -     | -     | -     | -    | -     | -     | -       | 12.287    | 0.92      | 2.16  | 1     | 27.6      | 0.26          | 3.84          | 8.973  | -0.55 | -2.26 | 2.75 | ...  | ...   | ...  | ... | -0.38 | -1.68 |      |     |      |     |      |     |      |     |      |
| 02573053+5825188 | 138.820 | -0.506 | 1.516 | 1   | -      | -      | -    | g    | -        | N   | -      | D3   | -        | -     | -     | -     | -    | -     | -     | -       | 11.795    | 0.76      | 2.06  | 1     | 23.8      | 0.72          | 3.76          | 11.230 | 0.50  | 1.31  | 0.47 | 27.7 | 11.22 | ...  | ... | 0.53  | 1.41  |      |     |      |     |      |     |      |     |      |
| 02573314+6038237 | 137.793 | 1.460  | 6.376 | 9   | -      | -      | -    | -    | -        | -   | -      | -    | -        | -     | -     | -     | -    | -     | -     | -       | 11.759    | 0.62      | 1.40  | 1     | 52.6      | 0.92          | 3.84          | 9.383  | -0.43 | -1.77 | 1.97 | ...  | ...   | ...  | ... | -0.31 | -1.35 |      |     |      |     |      |     |      |     |      |
| 02581379+6220317 | 137.069 | 3.003  | 1.563 | 7   | -      | -      | -    | -    | -        | -   | -      | -    | -        | -     | -     | -     | -    | -     | -     | -       | 11.339    | 1.24      | 2.68  | 1     | 30.4      | 0.66          | 3.72          | 10.757 | 0.99  | 1.90  | 0.48 | ...  | ...   | ...  | ... | 1.02  | 2.00  |      |     |      |     |      |     |      |     |      |
| 02584545+5313540 | 141.408 | -5.011 | 0.730 | 1   | -      | -      | -    | g    | -        | -   | -      | D1   | c        | o     | -     | -     | -    | -     | -     | -       | 11.496    | 0.47      | 1.37  | 1     | 27.4      | 0.70          | 3.64          | 11.224 | 0.35  | 1.00  | 0.23 | 28.9 | 11.24 | ...  | ... | 0.36  | 1.05  |      |     |      |     |      |     |      |     |      |
| 02585431+5950161 | 138.316 | 0.829  | 0.866 | 1   | -      | -      | -    | g    | -        | N</ |        |      |          |       |       |       |      |       |       |         |           |           |       |       |           |               |               |        |       |       |      |      |       |      |     |       |       |      |     |      |     |      |     |      |     |      |



Table B1: a) continued.

| 2MASX J          | <i>l</i> | <i>b</i> | EBV    | Object | Sample  | Disc | 2MRS    | Velocity | NIR   | Photom | Ext | <i>K</i> <sub>20</sub> | <i>H-K</i> | <i>J-K</i> | vc   | <i>a</i> | <i>b/a</i> | st.d.  | <i>K</i> <sub>s</sub> <sup>o</sup> | ( <i>H-K</i> ) <sup>o</sup> | ( <i>J-K</i> ) <sup>o</sup> | <i>A<sub>K</sub></i> | <i>a</i> <sub>d</sub> <sup>o</sup> | <i>K</i> <sub>s</sub> <sup>o,d</sup> | ( <i>H-K</i> ) <sup>o,c</sup> | ( <i>J-K</i> ) <sup>o,c</sup> |       |      |       |       |       |       |
|------------------|----------|----------|--------|--------|---------|------|---------|----------|-------|--------|-----|------------------------|------------|------------|------|----------|------------|--------|------------------------------------|-----------------------------|-----------------------------|----------------------|------------------------------------|--------------------------------------|-------------------------------|-------------------------------|-------|------|-------|-------|-------|-------|
| (1)              | deg      | deg      | mag    | class  | off flg | gal  | TF (7b) | Obs (7c) | ext'd | type   | Opt | HI                     | flg        | flg        | flg  | "        | (19)       | (20)   | mag                                | mag                         | mag                         | mag                  | "                                  | mag                                  | mag                           | mag                           |       |      |       |       |       |       |
| (1)              | (2a)     | (2b)     | (3)    | (4)    | (5)     | (6)  | (7a)    | (7b)     | (7d)  | (8)    | (9) | (10a)                  | (10b)      | (11)       | (12) | (13)     | (14)       | (15)   | (16)                               | (17)                        | (18)                        | (19)                 | (20)                               | (21)                                 | (22)                          | (23)                          | (24)  | (25) | (26)  | (27)  | (28)  |       |
| 03070158+5315165 | 142.482  | -4.391   | 0.833  | 1      | -       | -    | g       | -        | N     | D1     | -   | -                      | -          | U          | -    | -        | -          | 11.104 | 0.43                               | 1.42                        | 1                           | 37.6                 | 0.58                               | 3.63                                 | 10.794                        | 0.29                          | 1.00  | 0.26 | 40.1  | 10.81 | 0.31  | 1.06  |
| 03071054+5517545 | 141.482  | -2.607   | 1.475  | 1      | -       | -    | g       | -        | N     | D1     | -   | -                      | -          | U          | -    | -        | -          | 9.321  | 0.48                               | 1.61                        | 1                           | 71.0                 | 0.72                               | 3.64                                 | 8.771                         | 0.24                          | 0.88  | 0.46 | 79.7  | 8.81  | 0.27  | 0.98  |
| 03071477+5829375 | 139.902  | 0.170    | 9.839  | 8      | -       | -    | g       | -        | -     | -      | -   | -                      | -          | -          | -    | -        | -          | 11.804 | 0.93                               | ...                         | 1                           | 38.6                 | 1.00                               | 3.80                                 | 8.138                         | -0.70                         | ...   | 3.05 | ...   | -0.51 | ...   |       |
| 03072040+5830424 | 139.903  | 0.192    | 10.643 | 9      | e       | -    | g       | -        | -     | -      | -   | -                      | -          | o          | -    | -        | -          | 12.610 | 1.22                               | ...                         | 1                           | 46.2                 | 0.48                               | 3.80                                 | 8.644                         | -0.55                         | ...   | 3.30 | ...   | -0.34 | ...   |       |
| 03072450+5830434 | 139.911  | 0.196    | 11.311 | 8      | -       | -    | g       | -        | -     | -      | -   | -                      | -          | -          | -    | -        | -          | 12.945 | 1.25                               | 2.74                        | 1                           | 88.2                 | 0.76                               | 3.76                                 | 7.331                         | -0.62                         | -2.88 | 3.50 | ...   | -0.40 | -2.14 |       |
| 03072718+5830134 | 139.920  | 0.192    | 11.629 | 9      | -       | -    | g       | -        | -     | -      | -   | -                      | -          | -          | -    | -        | -          | 12.298 | 1.04                               | ...                         | 1                           | 25.6                 | 1.00                               | 3.76                                 | 7.965                         | -0.88                         | ...   | 3.60 | ...   | -0.65 | ...   |       |
| 03073445+5831475 | 139.921  | 0.222    | 10.259 | 9      | -       | -    | g       | -        | -     | -      | -   | -                      | -          | -          | -    | -        | -          | 13.921 | 0.69                               | ...                         | -1                          | 12.8                 | 1.00                               | 3.76                                 | 10.098                        | -1.01                         | ...   | 3.18 | ...   | -0.81 | ...   |       |
| 03073914+5645235 | 140.814  | -1.310   | 3.782  | 1      | -       | -    | g       | -        | N     | -      | -   | -                      | -          | U          | -    | -        | -          | 12.330 | 0.81                               | 2.38                        | 1                           | 23.6                 | 0.86                               | 3.68                                 | 10.921                        | 0.18                          | 0.50  | 1.17 | 39.9  | 10.74 | 0.26  | 0.75  |
| 03074712+6725361 | 135.478  | 7.939    | 0.991  | 1      | -       | -    | g       | -        | -     | D2     | -   | c                      | -          | o          | -    | -        | -          | 11.540 | 0.22                               | 1.19                        | 1                           | 29.2                 | 0.90                               | 3.51                                 | 11.171                        | 0.06                          | 0.69  | 0.31 | 32.1  | 11.16 | 0.08  | 0.76  |
| 03081849+5623343 | 141.074  | -1.580   | 2.366  | 8      | -       | -    | g       | -        | -     | -      | -   | -                      | -          | -          | -    | -        | -          | 10.596 | 1.92                               | 4.11                        | 1                           | 19.8                 | 0.74                               | 3.69                                 | 9.714                         | 1.53                          | 2.93  | 0.73 | ...   | ...   | 1.58  | 3.09  |
| 03082803+5745174 | 140.410  | -0.390   | 1.389  | 1      | -       | -    | g       | -        | t     | D1     | -   | -                      | -          | -          | -    | -        | -          | 10.698 | 0.53                               | 1.74                        | 1                           | 58.4                 | 0.42                               | 3.75                                 | 10.180                        | 0.30                          | 1.05  | 0.43 | 67.2  | 10.16 | 0.32  | 1.14  |
| 03084441+6539435 | 136.457  | 6.463    | 0.888  | 1      | -       | -    | g       | -        | -     | D1     | -   | c                      | -          | o          | -    | -        | -          | 8.852  | 0.37                               | 1.28                        | 1                           | 90.2                 | 0.92                               | 3.57                                 | 8.521                         | 0.22                          | 0.83  | 0.28 | 95.6  | 8.55  | 0.24  | 0.89  |
| 03085635+6839027 | 134.945  | 9.049    | 0.810  | 1      | -       | -    | g       | -        | -     | D1     | -   | -                      | -          | -          | -    | -        | -          | 11.227 | 0.38                               | 1.32                        | 1                           | 32.8                 | 0.82                               | 3.52                                 | 10.925                        | 0.25                          | 0.91  | 0.25 | 34.9  | 10.94 | 0.26  | 0.97  |
| 03092672+5649269 | 140.992  | -1.128   | 6.587  | 9      | -       | -    | g       | -        | -     | -      | -   | -                      | -          | -          | -    | -        | -          | 13.600 | 0.50                               | 1.21                        | -1                          | 15.6                 | 0.46                               | 3.71                                 | 11.146                        | -0.59                         | -2.06 | 2.04 | ...   | ...   | -0.46 | -1.63 |
| 03094303+5650332 | 141.015  | -1.094   | 7.860  | 9      | -       | -    | g       | -        | -     | -      | -   | -                      | -          | U          | -    | -        | -          | 13.475 | 0.51                               | 1.17                        | -1                          | 12.8                 | 0.50                               | 3.69                                 | 10.546                        | -0.79                         | -2.74 | 2.43 | ...   | ...   | -0.64 | -2.22 |
| 03094669+5952577 | 139.486  | 1.534    | 2.856  | 7      | -       | -    | g       | -        | -     | -      | -   | -                      | -          | -          | -    | -        | -          | 11.056 | 0.70                               | 1.78                        | 1                           | 32.6                 | 0.70                               | 3.72                                 | 9.992                         | 0.23                          | 0.36  | 0.88 | ...   | ...   | 0.29  | 0.55  |
| 03095889+5647073 | 141.075  | -1.125   | 7.408  | 2      | -       | -    | g       | -        | -     | D3     | -   | -                      | -          | -          | -    | -        | -          | 12.452 | 0.59                               | 2.14                        | 1                           | 17.2                 | 0.98                               | 3.72                                 | 9.692                         | -0.64                         | -1.55 | 2.29 | 50.9  | 9.36  | -0.49 | -1.06 |
| 03095915+5707553 | 140.900  | -0.825   | 4.163  | 1      | -       | -    | g       | -        | -     | D3     | -   | -                      | -          | -          | -    | -        | -          | 12.251 | 0.82                               | 2.34                        | 1                           | 18.8                 | 0.76                               | 3.72                                 | 10.700                        | 0.13                          | 0.27  | 1.29 | 32.1  | 10.58 | 0.21  | 0.54  |
| 03100983+5747163 | 140.589  | -0.248   | 3.415  | 9      | -       | -    | g       | -        | -     | -      | -   | -                      | -          | -          | -    | -        | -          | 11.361 | 1.16                               | 2.51                        | 1                           | 75.6                 | 0.16                               | 3.65                                 | 10.089                        | 0.60                          | 0.81  | 1.06 | ...   | ...   | 0.66  | 1.04  |
| 03101283+5747343 | 140.592  | -0.240   | 3.453  | 9      | -       | -    | g       | -        | -     | -      | -   | -                      | -          | -          | -    | -        | -          | 12.304 | 1.06                               | ...                         | 1                           | 27.8                 | 0.62                               | 3.65                                 | 11.017                        | 0.49                          | ...   | 1.07 | ...   | ...   | 0.56  | ...   |
| 03101387+5649573 | 141.081  | -1.067   | 10.133 | 9      | -       | -    | g       | -        | -     | -      | -   | -                      | -          | -          | -    | -        | -          | 11.143 | 0.84                               | 2.30                        | 1                           | 80.2                 | 0.38                               | 3.69                                 | 7.367                         | -0.83                         | -2.73 | 3.14 | ...   | ...   | -0.64 | -2.06 |
| 03101644+5656203 | 141.032  | -0.972   | 4.885  | 1      | -       | -    | g       | -        | t     | D1     | -   | -                      | -          | -          | -    | -        | -          | 12.416 | 0.63                               | 2.25                        | 1                           | 22.6                 | 0.48                               | 3.69                                 | 10.596                        | -0.18                         | -0.18 | 1.51 | 45.0  | 10.38 | -0.09 | 0.15  |
| 03102931+5646173 | 141.142  | -1.101   | 5.083  | 1      | -       | -    | g       | -        | -     | D1     | -   | -                      | -          | -          | -    | -        | -          | 12.702 | 0.77                               | 2.09                        | -2                          | 23.0                 | 0.44                               | 3.72                                 | 10.808                        | -0.07                         | -0.43 | 1.57 | 51.2  | 10.44 | 0.03  | -0.10 |
| 03104409+6106477 | 138.963  | 2.655    | 1.264  | 1      | -       | -    | g       | -        | -     | D2     | -   | -                      | -          | -          | -    | -        | -          | 8.081  | 0.48                               | 1.51                        | 1                           | 132.6                | 0.54                               | 3.73                                 | 7.610                         | 0.27                          | 0.88  | 0.39 | 144.8 | 7.65  | 0.29  | 0.97  |
| 03111176+6105047 | 139.026  | 2.658    | 1.230  | 1      | -       | -    | g       | -        | -     | D1     | -   | -                      | -          | -          | -    | -        | -          | 11.460 | 0.48                               | 1.49                        | 1                           | 40.8                 | 0.64                               | 3.71                                 | 11.002                        | 0.27                          | 0.88  | 0.38 | 46.3  | 10.98 | 0.30  | 0.96  |
| 03111754+4720304 | 146.093  | -9.143   | 0.296  | 1      | -       | -    | g       | -        | -     | D4     | -   | -                      | -          | -          | -    | -        | -          | 10.814 | 0.32                               | 1.12                        | 1                           | 29.0                 | 0.94                               | 3.47                                 | 10.704                        | 0.27                          | 0.97  | 0.09 | 29.4  | 10.72 | 0.28  | 0.99  |
| 03113572+6241207 | 138.245  | 4.061    | 1.219  | 1      | o       | -    | g       | -        | -     | D1     | -   | -                      | -          | -          | -    | -        | -          | 11.452 | 0.54                               | 1.55                        | 1                           | 29.2                 | 0.76                               | 3.63                                 | 10.998                        | 0.34                          | 0.95  | 0.38 | 32.0  | 10.97 | 0.37  | 1.03  |
| 03115889+6020491 | 139.486  | 2.074    | 1.369  | 1      | -       | -    | g       | -        | -     | D1     | -   | e                      | -          | -          | -    | -        | -          | 10.969 | 0.34                               | 1.47                        | 1                           | 65.6                 | 0.42                               | 3.65                                 | 10.459                        | 0.11                          | 0.79  | 0.42 | 78.4  | 10.35 | 0.14  | 0.88  |
| 03120931+6724214 | 135.853  | 8.135    | 0.987  | 1      | -       | -    | g       | -        | -     | D1     | -   | e                      | -          | -          | -    | -        | -          | 9.699  | 0.28                               | 1.05                        | 1                           | 80.2                 | 0.54                               | 3.49                                 | 9.331                         | 0.12                          | 0.56  | 0.31 | 89.0  | 9.30  | 0.14  | 0.62  |
| 03121951+6758295 | 135.568  | 8.630    | 1.008  | 1      | -       | -    | g       | -        | -     | D1     | -   | e                      | -          | -          | -    | -        | -          | 11.340 | 0.43                               | 1.33                        | 1                           | 31.6                 | 0.80                               | 3.54                                 | 10.964                        | 0.26                          | 0.83  | 0.31 | 34.4  | 10.97 | 0.28  | 0.90  |
| 03124482+5213500 | 143.752  | -4.835   | 0.724  | 9      | e       | -    | g       | -        | -     | -      | -   | -                      | -          | -          | -    | -        | -          | 11.219 | 0.46                               | 1.36                        | -2                          | 53.4                 | 0.42                               | 3.60                                 | 10.949                        | 0.34                          | 1.00  | 0.22 | ...   | ...   | 0.35  | 1.05  |
| 03124522+5213583 | 143.752  | -4.832   | 0.727  | 1      | -       | -    | g       | -        | -     | D3     | -   | -                      | -          | -          | -    | -        | -          | 11.231 | 0.41                               | 1.30                        | 1                           | 31.0                 | 0.94                               | 3.64                                 | 10.960                        | 0.29                          | 0.94  | 0.23 | 32.7  | 10.97 | 0.31  | 0.99  |
| 03124721+6231391 | 138.446  | 3.993    | 1.323  | 1      | -       | -    | g       | -        | -     | D1     | -   | -                      | -          | -          | -    | -        | -          | 11.689 | 0.55                               | 1.51                        | 1                           | 33.2                 | 0.76                               | 3.61                                 | 11.196                        | 0.33                          | 0.86  | 0.41 | 39.0  | 11.12 | 0.36  | 0.95  |
| 03130062+6752475 | 135.674  | 8.582    | 1.003  | 1      | -       | -    | g       | -        | -     | D1     | -   | e                      | -          | -          | -    | -        | -          | 11.313 | 0.57                               | 1.58                        | 1                           | 58.4                 | 0.18                               | 3.53                                 | 10.939                        | 0.41                          | 1.08  | 0.31 | 64.3  | 10.93 | 0.43  | 1.15  |
| 03132009+6224130 | 138.064  | 3.920    | 1.497  | 1      | -       | -    | g       | -        | -     | D2     | -   | -                      | -          | -          | -    | -        | -          | 10.966 | 0.45                               | 1.51                        | 1                           | 42.6                 | 0.58                               | 3.65                                 | 10.408                        | 0.20                          | 0.77  | 0.46 | 49.2  | 10.41 | 0.23  | 0.87  |
| 03135317+6232589 | 138.543  | 4.078    | 1.221  | 1      | -       | -    | g       | -        | -     | D2     | -   | -                      | -          | -          | -    | -        | -          | 8.732  | 0.43                               | 1.51                        | 1                           | 79.4                 | 0.80                               | 3.66                                 | 8.277                         | 0.23                          | 0.90  | 0.38 | 86.0  | 8.32  | 0.25  | 0.98  |
| 03135517+6233197 | 138.543  | 4.085    | 1.222  | 9      | e       | -    | g       | -        | -     | -      | -   | -                      | -          | -          | -    | -        | -          | 10.083 | 0.44                               | 1.39                        | -2                          | 79.8                 | 0.44                               | 3.69                                 | 9.628                         | 0.23                          | 0.78  | 0.38 | ...   | ...   | 0.26  | 0.86  |
| 03141768+4601520 | 147.232  | -9.992   | 0.283  | 1      | -       | -    | g       | -        | -     | D1     | -   | -                      | -          | -          | -    | -        | -          | 10.439 | 0.41                               | 1.25                        | 1                           | 34.6                 | 0.58                               | 3.37                                 | 10.334                        | 0.36                          | 1.11  | 0.09 | 35.1  | 10.34 | 0.37  | 1.13  |
| 03142355+4610500 | 147.167  | -9.856   | 0.301  | 1      | -       | -    | g       | -        | -     | D1     | -   | c                      | -          | -          | -    | -        | -          | 11.058 | 0.44                               | 1.28                        | 1                           | 32.8                 | 0.84                               | 3.47                                 | 10.946                        | 0.39                          | 1.13  | 0.09 | 33.3  | 10.96 | 0.39  | 1.15  |
| 03144196+5837161 | 140.674  | 0.774    | 2.785  | 7      | -       | -    | g       | -        | -     | D2     | -   | -                      | -          | -          | -    | -        | -          | 10.456 | 0.75                               | 1.43                        | 1                           | 37.4                 | 0.80                               | 3.80                                 | 9.418                         | 0.29                          | 0.05  | 0.86 | ...   | ...   | 0.34  | 0.23  |
| 03161119+6242593 | 138.681  | 4.358    | 1.045  | 1      | -       | -    | g       | -        | -     | D2     | -   | -                      | -          | -          | -    | -        | -          | 11.555 | 0.34                               | 1.34                        | 1                           | 34.0                 | 0.58                               | 3.66                                 | 11.166                        | 0.16                          | 0.82  | 0.32 | 38.1  | 11.13 | 0.18  | 0.89  |
| 03162208+5215460 | 144.209  | -4.518   | 0.908  | 1      | -       | -    | g       | -        | -     | D4     | -   | -                      | -          | -          | -    | -        | -          | 11.388 | 0.47                               | 1.41                        | 1                           | 29.0                 | 0.86                               | 3.51                                 | 11.050                        | 0.32                          | 0.96  | 0.28 | 31.2  | 11.06 | 0.34  | 1.02  |
| 03164400+6501431 | 137.005  | 6.353    | 0.968  | 1      | -       | -    | g       | -        | -     | D3     | -   | -                      | -          | -          | -    | -        | -          | 9.638  | 0.42                               | 1.36                        | 1                           | 90.8                 | 0.36                               | 3.58                                 | 9.277                         | 0.26                          | 0.88  | 0.30 | 97.9  | 9.30  | 0.28  | 0.94  |
| 03164732+4710346 | 146.984  | -8.794   | 0.375  | 1      | -       | -    | g       | -        | -     | D3     | -   | -                      | -          | -          | -    | -        | -          | 11.305 | 0.30                               | 1.13                        | 1                           | 26.0                 | 0.94                               | 3.43                                 | 11.165                        | 0.24                          | 0.95  | 0.12 | 26.6  | 11.18 | 0.25  | 0.97  |
| 03165004         |          |          |        |        |         |      |         |          |       |        |     |                        |            |            |      |          |            |        |                                    |                             |                             |                      |                                    |                                      |                               |                               |       |      |       |       |       |       |

Table B1: a) continued.

| 2MASX J          | <i>l</i> | <i>b</i> | EBV    | Object | Sample | Disc | 2MRS | Velocity | NIR  | Photom | Ext   | <i>K</i> <sub>20</sub> | <i>H-K</i> | <i>J-K</i> | vc   | <i>a</i> | <i>b/a</i> | st.d. | <i>K</i> <sub>s</sub> <sup>o</sup> | ( <i>H-K</i> ) <sup>o</sup> | ( <i>J-K</i> ) <sup>o</sup> | <i>A<sub>K</sub></i> | <i>a</i> <sub>d</sub> <sup>o</sup> | <i>K</i> <sub>s</sub> <sup>o,d</sup> | ( <i>H-K</i> ) <sup>o,c</sup> | ( <i>J-K</i> ) <sup>o,c</sup> |       |       |      |       |       |       |       |
|------------------|----------|----------|--------|--------|--------|------|------|----------|------|--------|-------|------------------------|------------|------------|------|----------|------------|-------|------------------------------------|-----------------------------|-----------------------------|----------------------|------------------------------------|--------------------------------------|-------------------------------|-------------------------------|-------|-------|------|-------|-------|-------|-------|
| (1)              | deg      | deg      | mag    | class  | off    | flg  | gal  | TF       | (7b) | (7c)   | ext'd | type                   | (8)        | (9)        | Opt  | HI       | flg        | flg   | flg                                | flg                         | flg                         | flg                  | flg                                | flg                                  | flg                           | flg                           | flg   |       |      |       |       |       |       |
| (1)              | (2a)     | (2b)     | (3)    | (4)    | (5)    | (6)  | (7a) | (7b)     | (7c) | (7d)   | (8)   | (9)                    | (10a)      | (10b)      | (11) | (12)     | (13)       | (14)  | (15)                               | (16)                        | (17)                        | (18)                 | (19)                               | (20)                                 | (21)                          | (22)                          | (23)  | (24)  | (25) | (26)  | (27)  | (28)  |       |
| 03261404+6635372 | 137.465  | 8.195    | 0.930  | 1      | —      | —    | g    | —        | —    | —      | —     | D1                     | c          | o          | —    | —        | —          | —     | 8.981                              | 0.38                        | 1.23                        | 1                    | 88.0                               | 0.88                                 | 3.51                          | 8.634                         | 0.23  | 0.77  | 0.29 | 93.7  | 8.66  | 0.25  | 0.83  |
| 03264399+5419084 | 144.394  | -1.950   | 1.556  | 1      | —      | —    | t    | N        | —    | —      | —     | D1                     | c          | o          | —    | —        | —          | —     | 11.799                             | 0.54                        | 1.58                        | 1                    | 39.0                               | 0.28                                 | 3.64                          | 11.219                        | 0.28  | 0.80  | 0.48 | 46.9  | 11.15 | 0.31  | 0.91  |
| 03265649+6834523 | 136.385  | 9.874    | 0.766  | 1      | —      | —    | g    | —        | —    | —      | —     | D1                     | c          | o          | —    | —        | —          | —     | 9.972                              | 0.36                        | 1.22                        | 1                    | 92.4                               | 0.64                                 | 3.43                          | 9.687                         | 0.24  | 0.84  | 0.24 | 99.4  | 9.67  | 0.25  | 0.89  |
| 03270534+4657595 | 148.582  | -8.006   | 0.446  | 1      | —      | —    | g    | —        | —    | —      | —     | D1                     | c          | o          | —    | —        | —          | —     | 10.311                             | 0.31                        | 1.17                        | 1                    | 61.6                               | 0.34                                 | 3.53                          | 10.145                        | 0.23  | 0.95  | 0.14 | 63.1  | 10.16 | 0.24  | 0.98  |
| 03272149+5820309 | 142.216  | 1.434    | 5.377  | 9      | —      | —    | g    | —        | —    | —      | —     | —                      | —          | —          | —    | —        | —          | —     | 10.456                             | 1.22                        | 2.69                        | 1                    | 73.0                               | 0.80                                 | 3.62                          | 8.453                         | 0.33  | 0.01  | 1.67 | ...   | ...   | 0.44  | 0.37  |
| 03272168+4959010 | 146.908  | -5.488   | 0.553  | 1      | —      | —    | g    | —        | —    | —      | —     | D1                     | c          | o          | —    | —        | —          | —     | 11.154                             | 0.37                        | 1.20                        | 1                    | 62.2                               | 0.32                                 | 3.56                          | 10.948                        | 0.28  | 0.93  | 0.17 | 64.7  | 10.96 | 0.29  | 0.96  |
| 03273050+5846599 | 141.985  | 1.810    | 10.264 | 9      | —      | —    | g    | —        | —    | —      | —     | —                      | —          | —          | —    | —        | —          | —     | 12.522                             | 1.05                        | ...                         | 1                    | 28.8                               | 0.68                                 | 3.77                          | 8.698                         | -0.65 | ...   | 3.18 | ...   | ...   | -0.45 | ...   |
| 03273140+5819219 | 142.245  | 1.430    | 4.965  | 8      | —      | —    | g    | —        | —    | —      | —     | —                      | —          | —          | —    | —        | —          | —     | 10.545                             | 1.60                        | 3.82                        | 1                    | 46.8                               | 0.74                                 | 3.62                          | 8.695                         | 0.78  | 1.35  | 1.54 | ...   | ...   | 0.88  | 1.68  |
| 03273140+5845240 | 142.002  | 1.789    | 9.702  | 8      | —      | —    | g    | —        | —    | —      | —     | —                      | —          | —          | —    | —        | —          | —     | 12.059                             | 1.33                        | ...                         | 1                    | 32.2                               | 0.48                                 | 3.77                          | 8.444                         | -0.28 | ...   | 3.01 | ...   | ...   | -0.09 | ...   |
| 03273307+5846340 | 141.994  | 1.807    | 10.115 | 9      | —      | —    | g    | —        | —    | —      | —     | —                      | —          | —          | —    | —        | —          | —     | 10.486                             | 1.01                        | 2.47                        | 1                    | 67.0                               | 0.56                                 | 3.77                          | 6.717                         | -0.67 | -2.55 | 3.13 | ...   | ...   | -0.47 | -1.89 |
| 03273397+5847240 | 141.988  | 1.820    | 10.426 | 9      | —      | —    | g    | —        | —    | —      | —     | —                      | —          | —          | —    | —        | —          | —     | 11.439                             | 1.01                        | 2.56                        | 1                    | 43.2                               | 0.34                                 | 3.77                          | 7.554                         | -0.72 | -2.62 | 3.23 | ...   | ...   | -0.52 | -1.93 |
| 03273938+5221060 | 145.611  | -3.503   | 1.054  | 1      | —      | —    | g    | —        | —    | N      | —     | D3                     | c          | o          | —    | —        | —          | —     | 10.778                             | 0.36                        | 1.26                        | 1                    | 33.8                               | 0.62                                 | 3.60                          | 10.385                        | 0.19  | 0.74  | 0.33 | 36.7  | 10.41 | 0.21  | 0.80  |
| 03274465+5847049 | 142.010  | 1.829    | 10.123 | 9      | —      | —    | g    | —        | —    | —      | —     | —                      | —          | —          | —    | —        | —          | —     | 11.174                             | 0.84                        | 2.28                        | -2                   | 68.0                               | 0.62                                 | 3.77                          | 7.402                         | -0.84 | -2.75 | 3.14 | ...   | ...   | -0.64 | -2.08 |
| 03274525+4656102 | 148.694  | -7.967   | 0.438  | 1      | —      | —    | g    | —        | —    | —      | —     | D1                     | c          | o          | —    | —        | —          | —     | 11.159                             | 0.40                        | 1.14                        | 1                    | 34.2                               | 0.72                                 | 3.49                          | 10.996                        | 0.32  | 0.92  | 0.14 | 35.3  | 11.00 | 0.33  | 0.95  |
| 03285780+6656000 | 137.494  | 8.627    | 1.017  | 1      | —      | —    | g    | —        | —    | N      | —     | —                      | —          | —          | —    | —        | —          | —     | 11.119                             | 0.41                        | 1.37                        | 1                    | 35.2                               | 0.74                                 | 3.51                          | 10.740                        | 0.24  | 0.87  | 0.32 | 38.7  | 10.73 | 0.26  | 0.93  |
| 03290640+6458319 | 138.633  | 7.027    | 1.082  | 1      | —      | —    | g    | —        | —    | N      | —     | D1                     | e          | o          | —    | —        | —          | —     | 9.441                              | 0.38                        | 1.34                        | 1                    | 71.0                               | 0.62                                 | 3.54                          | 9.038                         | 0.20  | 0.80  | 0.34 | 76.8  | 9.07  | 0.23  | 0.87  |
| 03292042+6601389 | 138.048  | 7.905    | 1.175  | 1      | —      | —    | t    | N        | —    | —      | —     | D1                     | e          | o          | —    | —        | —          | —     | 9.612                              | 0.40                        | 1.47                        | 1                    | 112.2                              | 0.32                                 | 3.48                          | 9.174                         | 0.21  | 0.88  | 0.36 | 124.8 | 9.18  | 0.23  | 0.96  |
| 03292877+5429573 | 144.623  | -1.577   | 2.087  | 1      | —      | —    | g    | —        | —    | N      | —     | D1                     | e          | o          | —    | —        | —          | —     | 11.476                             | 0.61                        | 1.91                        | 1                    | 42.0                               | 0.44                                 | 3.67                          | 10.698                        | 0.26  | 0.87  | 0.65 | 54.2  | 10.62 | 0.30  | 1.01  |
| 03302327+6110135 | 140.931  | 3.983    | 0.982  | 1      | —      | —    | g    | —        | —    | N      | —     | D1                     | e          | o          | —    | —        | —          | —     | 9.394                              | 0.43                        | 1.49                        | 1                    | 85.8                               | 0.52                                 | 3.63                          | 9.028                         | 0.27  | 1.00  | 0.30 | 92.0  | 9.05  | 0.29  | 1.06  |
| 03302536+5015272 | 147.158  | -4.984   | 0.665  | 1      | —      | —    | g    | —        | —    | N      | —     | D3                     | e          | o          | —    | —        | —          | —     | 11.017                             | 0.32                        | 1.29                        | 1                    | 36.8                               | 0.92                                 | 3.65                          | 10.769                        | 0.21  | 0.96  | 0.21 | 38.6  | 10.78 | 0.22  | 1.00  |
| 03305134+6110207 | 140.977  | 4.017    | 0.993  | 1      | —      | —    | g    | —        | —    | N      | —     | D1                     | e          | o          | —    | —        | —          | —     | 10.435                             | 0.45                        | 1.40                        | 1                    | 51.2                               | 0.58                                 | 3.63                          | 10.065                        | 0.28  | 0.90  | 0.31 | 55.8  | 10.07 | 0.30  | 0.97  |
| 03311276+6630034 | 137.929  | 8.401    | 1.170  | 1      | —      | —    | g    | —        | —    | N      | —     | D1                     | e          | o          | —    | —        | —          | —     | 10.674                             | 0.38                        | 1.44                        | 1                    | 80.8                               | 0.32                                 | 3.42                          | 10.238                        | 0.19  | 0.86  | 0.36 | 92.5  | 10.18 | 0.21  | 0.94  |
| 03311296+6541405 | 138.423  | 7.759    | 1.079  | 1      | —      | —    | g    | —        | —    | N      | —     | D1                     | e          | o          | —    | —        | —          | —     | 11.613                             | 0.51                        | 1.57                        | 1                    | 36.2                               | 0.34                                 | 3.40                          | 11.211                        | 0.33  | 1.04  | 0.33 | 39.9  | 11.21 | 0.35  | 1.11  |
| 03313677+5148312 | 146.421  | -3.605   | 1.019  | 1      | —      | —    | g    | —        | —    | N      | —     | D4                     | e          | o          | —    | —        | —          | —     | 11.615                             | 0.46                        | 1.47                        | 1                    | 23.0                               | 0.86                                 | 3.64                          | 11.235                        | 0.29  | 0.96  | 0.32 | 25.1  | 11.24 | 0.31  | 1.03  |
| 03320341+6822062 | 136.899  | 0.783    | 1      | —      | —      | —    | g    | —        | —    | N      | —     | D1                     | c          | o          | —    | —        | —          | —     | 8.683                              | 0.39                        | 1.30                        | 1                    | 167.4                              | 0.48                                 | ...                           | 8.391                         | 0.26  | 0.91  | 0.24 | ...   | ...   | 0.28  | 0.96  |
| 03320732+4747385 | 148.810  | -6.840   | 0.568  | 1      | —      | —    | g    | —        | —    | N      | —     | D1                     | c          | o          | —    | —        | —          | —     | 10.026                             | 0.25                        | 1.02                        | 1                    | 75.2                               | 0.72                                 | 3.45                          | 9.814                         | 0.16  | 0.74  | 0.18 | 79.0  | 9.80  | 0.17  | 0.78  |
| 03320799+5825273 | 142.685  | 1.856    | 3.269  | 9      | —      | —    | g    | —        | —    | —      | —     | —                      | —          | —          | —    | —        | —          | —     | 12.080                             | 0.33                        | 0.98                        | -2                   | 20.8                               | 0.42                                 | 3.59                          | 10.862                        | -0.21 | -0.64 | 1.01 | ...   | ...   | -0.15 | -0.42 |
| 03323427+4728438 | 149.056  | -7.053   | 0.576  | 1      | —      | —    | g    | —        | —    | N      | —     | D1                     | c          | o          | —    | —        | —          | —     | 10.865                             | 0.40                        | 1.21                        | 1                    | 46.2                               | 0.58                                 | 3.47                          | 10.650                        | 0.30  | 0.93  | 0.18 | 48.2  | 10.66 | 0.32  | 0.96  |
| 03330098+5734131 | 143.273  | 1.226    | 2.543  | 8      | —      | —    | g    | —        | —    | —      | —     | —                      | —          | —          | —    | —        | —          | —     | 10.800                             | 0.98                        | 2.44                        | 1                    | 28.0                               | 0.84                                 | 3.63                          | 9.852                         | 0.56  | 1.18  | 0.79 | ...   | ...   | 0.61  | 1.35  |
| 03331908+6609092 | 138.308  | 8.240    | 1.299  | 1      | —      | —    | g    | —        | —    | N      | —     | D1                     | e          | o          | —    | —        | —          | —     | 10.931                             | 0.48                        | 1.44                        | 1                    | 52.0                               | 0.50                                 | 3.38                          | 10.447                        | 0.26  | 0.80  | 0.40 | 58.7  | 10.45 | 0.29  | 0.88  |
| 03332695+5450231 | 144.899  | -0.969   | 2.183  | 8      | —      | —    | g    | —        | —    | —      | —     | —                      | —          | —          | —    | —        | —          | —     | 12.031                             | 1.33                        | 3.33                        | -2                   | 18.2                               | 0.74                                 | 3.67                          | 11.218                        | 0.97  | 2.24  | 0.68 | ...   | ...   | 1.01  | 2.39  |
| 03333084+4828402 | 148.602  | -6.148   | 0.574  | 1      | —      | —    | g    | —        | —    | N      | —     | D1                     | c          | o          | —    | —        | —          | —     | 11.302                             | 0.39                        | 1.30                        | 1                    | 37.8                               | 0.52                                 | 3.57                          | 11.088                        | 0.30  | 1.02  | 0.18 | 39.4  | 11.10 | 0.31  | 1.06  |
| 03334905+5201071 | 146.578  | -3.237   | 1.151  | 1      | —      | —    | g    | —        | —    | N      | —     | D4                     | e          | o          | —    | —        | —          | —     | 11.279                             | 0.44                        | 1.47                        | 1                    | 30.2                               | 0.94                                 | 3.65                          | 10.850                        | 0.25  | 0.90  | 0.36 | 33.4  | 10.86 | 0.27  | 0.97  |
| 03342260+5730303 | 143.458  | 1.281    | 2.374  | 9      | —      | —    | g    | —        | —    | —      | —     | —                      | —          | —          | —    | —        | —          | —     | 10.753                             | ...                         | 1.31                        | -2                   | 240.0                              | 1.00                                 | 3.69                          | 9.868                         | ...   | 0.13  | 0.74 | ...   | ...   | ...   | 0.29  |
| 03345483+5349073 | 145.665  | -1.677   | 1.737  | 1      | —      | —    | g    | —        | —    | N      | —     | D2                     | e          | o          | —    | —        | —          | —     | 11.849                             | 0.61                        | 1.88                        | 1                    | 28.2                               | 0.66                                 | 3.65                          | 11.202                        | 0.32  | 1.02  | 0.54 | 34.3  | 11.15 | 0.35  | 1.13  |
| 03345508+4551520 | 150.337  | -8.129   | 0.487  | 1      | —      | —    | g    | —        | —    | N      | —     | D3                     | c          | o          | —    | —        | —          | —     | 10.866                             | 0.37                        | 1.23                        | 1                    | 43.2                               | 0.70                                 | 3.49                          | 10.685                        | 0.29  | 0.99  | 0.15 | 44.6  | 10.70 | 0.30  | 1.02  |
| 03351760+4401160 | 151.492  | -9.578   | 0.313  | 1      | —      | —    | t    | N        | —    | —      | —     | D2                     | c          | o          | —    | —        | —          | —     | 11.364                             | 0.33                        | 1.16                        | 1                    | 34.8                               | 0.44                                 | 3.53                          | 11.247                        | 0.28  | 1.00  | 0.10 | 35.4  | 11.26 | 0.28  | 1.02  |
| 03354096+4635530 | 150.009  | -7.458   | 0.601  | 1      | —      | —    | g    | —        | —    | N      | —     | D1                     | c          | o          | —    | —        | —          | —     | 11.226                             | 0.34                        | 1.14                        | 1                    | 38.4                               | 0.52                                 | 3.51                          | 11.002                        | 0.24  | 0.84  | 0.19 | 40.1  | 11.01 | 0.25  | 0.88  |
| 03360608+5416062 | 145.544  | -1.210   | 1.945  | 2      | —      | —    | g    | —        | —    | N      | —     | D1                     | c          | o          | —    | —        | —          | —     | 11.399                             | 0.63                        | 1.65                        | 1                    | 34.8                               | 0.62                                 | 3.67                          | 10.674                        | 0.30  | 0.69  | 0.60 | 42.5  | 10.66 | 0.34  | 0.82  |
| 03361356+6733527 | 137.700  | 9.550    | 0.785  | 1      | —      | —    | g    | —        | —    | —      | —     | D1                     | c          | o          | —    | —        | —          | —     | 9.138                              | 0.39                        | 1.29                        | 1                    | 116.2                              | 0.60                                 | 3.43                          | 8.846                         | 0.26  | 0.90  | 0.24 | 122.3 | 8.87  | 0.28  | 0.95  |
| 03361815+5438151 | 150.670  | -8.169   | 0.590  | 1      | —      | —    | g    | —        | —    | —      | —     | D1                     | c          | o          | —    | —        | —          | —     | 10.386                             | 0.35                        | 1.22                        | 1                    | 46.2                               | 0.90                                 | 3.48                          | 10.166                        | 0.25  | 0.92  | 0.18 | 48.2  | 10.17 | 0.26  | 0.96  |
| 03362290+5048356 | 147.611  | -3.985   | 1.038  | 1      |        |      |      |          |      |        |       |                        |            |            |      |          |            |       |                                    |                             |                             |                      |                                    |                                      |                               |                               |       |       |      |       |       |       |       |

Table B1: a) continued.

| 2MASX J          | <i>l</i> | <i>b</i> | EBV   | Object | Sample | Disc | 2MRS | Velocity | NIR  | Photom | Ext  | <i>K</i> <sub>20</sub> | <i>H-K</i> | <i>J-K</i> | vc   | <i>a</i> | <i>b/a</i> | st.d. | <i>K</i> <sub>s</sub> <sup>o</sup> | ( <i>H-K</i> ) <sup>o</sup> | ( <i>J-K</i> ) <sup>o</sup> | <i>A<sub>K</sub></i> | <i>a</i> <sub>d</sub> <sup>o</sup> | <i>K</i> <sub>s</sub> <sup>o,d</sup> | ( <i>H-K</i> ) <sup>o,c</sup> | ( <i>J-K</i> ) <sup>o,c</sup> |      |      |      |      |       |      |      |
|------------------|----------|----------|-------|--------|--------|------|------|----------|------|--------|------|------------------------|------------|------------|------|----------|------------|-------|------------------------------------|-----------------------------|-----------------------------|----------------------|------------------------------------|--------------------------------------|-------------------------------|-------------------------------|------|------|------|------|-------|------|------|
| (1)              | deg      | deg      | mag   | class  | off    | gal  | TF   | (7b)     | (7c) | ext'd  | type | (8)                    | (9)        | Opt        | HI   | (10a)    | (10b)      | (11)  | mag                                | mag                         | mag                         | mag                  | (25)                               | mag                                  | mag                           | mag                           |      |      |      |      |       |      |      |
| (1)              | (2a)     | (2b)     | (3)   | (4)    | (5)    | (6)  | (7a) | (7b)     | (7c) | (7d)   | (8)  | (9)                    | (10a)      | (10b)      | (11) | (12)     | (13)       | (14)  | (15)                               | (16)                        | (17)                        | (18)                 | (19)                               | (20)                                 | (21)                          | (22)                          | (23) | (24) | (25) | (26) | (27)  | (28) |      |
| 03432258+4609465 | 151.342  | -7.009   | 0.501 | 1      | -      | -    | g    | -        | -    | -      | D1   | c                      | o          | -          | -    | U        | -          | -     | 10.242                             | 0.35                        | 1.18                        | 1                    | 49.0                               | 0.60                                 | 3.52                          | 10.055                        | 0.27 | 0.93 | 0.16 | 50.5 | 10.07 | 0.27 | 0.97 |
| 03433015+5825154 | 143.888  | 2.734    | 1.133 | 1      | -      | -    | t    | N        | -    | -      | D1   | c                      | o          | -          | -    | U        | -          | -     | 11.226                             | 0.49                        | 1.39                        | 1                    | 51.6                               | 0.46                                 | 3.68                          | 10.804                        | 0.31 | 0.83 | 0.35 | 57.6 | 10.79 | 0.33 | 0.90 |
| 03433904+4609196 | 151.384  | -6.986   | 0.492 | 1      | -      | -    | g    | -        | -    | -      | D1   | c                      | o          | -          | -    | U        | -          | -     | 10.390                             | 0.32                        | 1.18                        | 1                    | 52.8                               | 0.74                                 | 3.52                          | 10.207                        | 0.24 | 0.93 | 0.15 | 54.4 | 10.22 | 0.25 | 0.97 |
| 03441400+4606321 | 151.494  | -6.960   | 0.480 | 1      | -      | -    | g    | -        | -    | -      | D1   | c                      | o          | -          | -    | U        | -          | -     | 10.054                             | 0.39                        | 1.20                        | 1                    | 60.4                               | 0.64                                 | 3.57                          | 9.875                         | 0.31 | 0.96 | 0.15 | 62.1 | 9.89  | 0.32 | 0.99 |
| 03441609+4919572 | 149.514  | -4.408   | 0.856 | 1      | -      | -    | g    | -        | -    | -      | D2   | c                      | o          | -          | -    | U        | -          | -     | 11.382                             | 0.44                        | 1.37                        | 1                    | 24.8                               | 0.74                                 | 3.62                          | 11.063                        | 0.30 | 0.95 | 0.27 | 26.5 | 11.08 | 0.32 | 1.00 |
| 03441729+5102202 | 148.473  | -3.055   | 1.236 | 1      | -      | -    | g    | -        | -    | -      | D2   | c                      | o          | -          | -    | U        | -          | -     | 11.233                             | 0.47                        | 1.53                        | 1                    | 39.4                               | 0.58                                 | 3.65                          | 10.772                        | 0.26 | 0.92 | 0.38 | 44.5 | 10.76 | 0.29 | 1.00 |
| 03444001+4337389 | 153.097  | -8.868   | 0.538 | 1      | -      | -    | t    | N        | -    | -      | D1   | c                      | o          | -          | h    | -        | -          | -     | 11.402                             | 0.58                        | 1.56                        | 1                    | 45.4                               | 0.26                                 | 3.46                          | 11.202                        | 0.49 | 1.29 | 0.17 | 47.3 | 11.20 | 0.50 | 1.33 |
| 03445127+4550430 | 151.743  | -7.102   | 0.471 | 1      | -      | -    | t    | N        | -    | -      | D1   | c                      | o          | -          | h    | -        | -          | -     | 10.431                             | 0.36                        | 1.22                        | 1                    | 74.2                               | 0.32                                 | 3.49                          | 10.256                        | 0.28 | 0.99 | 0.15 | 76.5 | 10.27 | 0.29 | 1.02 |
| 03445267+4612070 | 151.525  | -6.819   | 0.473 | 1      | -      | -    | t    | N        | -    | -      | D1   | c                      | o          | -          | h    | -        | -          | -     | 11.324                             | 0.37                        | 1.16                        | 1                    | 51.2                               | 0.36                                 | 3.54                          | 11.148                        | 0.29 | 0.93 | 0.15 | 53.1 | 11.15 | 0.30 | 0.96 |
| 03445333+4620290 | 151.440  | -6.707   | 0.466 | 1      | -      | -    | g    | -        | -    | -      | D1   | c                      | o          | -          | -    | U        | -          | -     | 11.140                             | 0.38                        | 1.17                        | 1                    | 40.0                               | 0.34                                 | 3.54                          | 10.966                        | 0.31 | 0.94 | 0.14 | 41.2 | 10.98 | 0.32 | 0.97 |
| 03445844+4558030 | 151.683  | -6.993   | 0.456 | 1      | -      | -    | g    | -        | -    | -      | D1   | c                      | o          | -          | -    | U        | -          | -     | 9.142                              | 0.36                        | 1.19                        | 1                    | 72.8                               | 0.82                                 | 3.49                          | 8.972                         | 0.29 | 0.96 | 0.14 | 74.5 | 8.99  | 0.30 | 0.99 |
| 03450943+4921435 | 149.611  | -4.296   | 0.917 | 1      | -      | -    | g    | -        | -    | -      | D4   | c                      | o          | -          | -    | U        | -          | -     | 10.958                             | 0.35                        | 1.26                        | 1                    | 30.6                               | 0.78                                 | 3.61                          | 10.616                        | 0.19 | 0.81 | 0.28 | 33.0 | 10.63 | 0.21 | 0.87 |
| 03453291+4451174 | 152.456  | -7.806   | 0.490 | 1      | -      | -    | t    | N        | -    | -      | D1   | c                      | o          | -          | h    | -        | -          | -     | 10.502                             | 0.37                        | 1.22                        | 1                    | 62.0                               | 0.48                                 | 3.51                          | 10.319                        | 0.29 | 0.98 | 0.15 | 64.2 | 10.33 | 0.30 | 1.01 |
| 03453445+4927444 | 149.603  | -4.176   | 1.046 | 1      | -      | -    | g    | -        | -    | -      | D4   | e                      | o          | -          | -    | U        | -          | -     | 10.117                             | 0.40                        | 1.38                        | 1                    | 53.8                               | 0.80                                 | 3.65                          | 9.727                         | 0.22 | 0.86 | 0.32 | 58.2 | 9.75  | 0.24 | 0.93 |
| 03454256+5638563 | 145.206  | 1.511    | 1.433 | 1      | -      | -    | t    | N        | -    | -      | D1   | c                      | o          | -          | h    | -        | -          | -     | 11.720                             | 0.53                        | 1.66                        | 1                    | 28.4                               | 0.60                                 | 3.67                          | 11.186                        | 0.29 | 0.94 | 0.44 | 32.7 | 11.18 | 0.32 | 1.04 |
| 03454377+4640244 | 151.348  | -6.357   | 0.453 | 1      | -      | -    | g    | -        | -    | -      | D1   | c                      | o          | -          | h    | -        | -          | -     | 9.940                              | 0.37                        | 1.20                        | 1                    | 86.2                               | 0.38                                 | 3.51                          | 9.771                         | 0.29 | 0.98 | 0.14 | 88.5 | 9.79  | 0.30 | 1.01 |
| 03460109+4201053 | 154.307  | -9.976   | 0.317 | 1      | -      | -    | g    | -        | -    | -      | D2   | c                      | o          | -          | -    | U        | -          | -     | 11.366                             | 0.31                        | 1.14                        | 1                    | 29.0                               | 0.78                                 | 3.46                          | 11.248                        | 0.26 | 0.99 | 0.10 | 29.5 | 11.26 | 0.26 | 1.01 |
| 03460488+5432382 | 146.540  | -0.118   | 2.297 | 1      | -      | -    | g    | -        | -    | -      | D3   | c                      | o          | -          | -    | U        | -          | -     | 11.630                             | 0.62                        | 1.97                        | 1                    | 20.6                               | 0.84                                 | 3.64                          | 10.774                        | 0.24 | 0.82 | 0.71 | 26.4 | 10.75 | 0.28 | 0.98 |
| 03462398+5430563 | 146.594  | -0.112   | 2.180 | 1      | -      | -    | g    | -        | -    | -      | D2   | c                      | o          | -          | -    | U        | -          | -     | 10.413                             | 0.55                        | 1.79                        | 1                    | 49.8                               | 0.86                                 | 3.67                          | 9.601                         | 0.19 | 0.70 | 0.68 | 63.1 | 9.57  | 0.23 | 0.85 |
| 03462569+4515263 | 152.327  | -7.394   | 0.522 | 1      | -      | -    | g    | -        | -    | -      | D2   | c                      | o          | -          | -    | U        | -          | -     | 10.821                             | 0.31                        | 1.20                        | 1                    | 39.4                               | 0.46                                 | 3.50                          | 10.627                        | 0.22 | 0.94 | 0.16 | 40.7 | 10.64 | 0.23 | 0.97 |
| 03471826+4651245 | 151.447  | -6.046   | 0.510 | 1      | -      | -    | g    | -        | -    | -      | D1   | c                      | o          | -          | h    | -        | -          | -     | 10.972                             | 0.38                        | 1.18                        | 1                    | 30.2                               | 0.74                                 | 3.54                          | 10.782                        | 0.29 | 0.92 | 0.16 | 31.2 | 10.80 | 0.30 | 0.96 |
| 03472283+4558095 | 152.013  | -6.733   | 0.491 | 1      | -      | -    | g    | -        | -    | -      | D1   | c                      | o          | -          | h    | -        | -          | -     | 11.119                             | 0.31                        | 1.16                        | 1                    | 50.0                               | 0.82                                 | 3.52                          | 10.936                        | 0.23 | 0.91 | 0.15 | 52.2 | 10.93 | 0.24 | 0.94 |
| 03474209+4216146 | 154.394  | -9.584   | 0.405 | 1      | -      | -    | g    | -        | -    | -      | D3   | c                      | o          | -          | -    | U        | -          | -     | 10.851                             | 0.36                        | 1.14                        | 1                    | 43.6                               | 0.82                                 | 3.49                          | 10.700                        | 0.29 | 0.94 | 0.13 | 44.7 | 10.71 | 0.30 | 0.97 |
| 03475375+5601049 | 145.834  | 1.202    | 1.615 | 1      | -      | -    | g    | -        | -    | -      | D1   | c                      | o          | -          | -    | U        | -          | -     | 11.432                             | 0.49                        | 1.54                        | 1                    | 28.6                               | 0.68                                 | 3.72                          | 10.830                        | 0.22 | 0.74 | 0.50 | 33.6 | 10.82 | 0.25 | 0.85 |
| 03480684+4955450 | 149.637  | -3.555   | 1.275 | 1      | -      | -    | g    | -        | -    | -      | D1   | c                      | o          | -          | *    | -        | -          | -     | 11.106                             | 0.64                        | 1.67                        | 1                    | 31.0                               | 0.74                                 | 3.65                          | 10.631                        | 0.43 | 1.03 | 0.39 | 34.5 | 10.65 | 0.46 | 1.12 |
| 03480719+4207563 | 154.543  | -9.643   | 0.396 | 1      | -      | -    | g    | -        | -    | -      | D2   | c                      | o          | -          | -    | U        | -          | -     | 11.211                             | 0.33                        | 1.01                        | 1                    | 32.4                               | 0.64                                 | 3.43                          | 11.063                        | 0.27 | 0.82 | 0.12 | 33.2 | 11.08 | 0.28 | 0.84 |
| 03480754+4212483 | 154.492  | -9.579   | 0.421 | 1      | -      | -    | g    | -        | -    | -      | D4   | c                      | o          | -          | -    | U        | -          | -     | 9.548                              | 0.31                        | 1.19                        | 1                    | 59.0                               | 0.82                                 | 3.50                          | 9.391                         | 0.24 | 0.98 | 0.13 | 60.3 | 9.41  | 0.25 | 1.01 |
| 03480963+4955140 | 149.649  | -3.557   | 1.264 | 1      | -      | -    | g    | -        | -    | -      | D2   | c                      | o          | -          | h    | -        | -          | -     | 11.243                             | 0.63                        | 1.63                        | 1                    | 32.2                               | 0.68                                 | 3.65                          | 10.772                        | 0.42 | 1.01 | 0.39 | 36.2 | 10.77 | 0.44 | 1.09 |
| 03481049+5409119 | 147.021  | -0.237   | 2.200 | 1      | -      | -    | t    | N        | -    | -      | D1   | c                      | o          | -          | -    | U        | -          | -     | 11.930                             | 0.79                        | 2.08                        | 1                    | 36.8                               | 0.24                                 | 3.69                          | 11.110                        | 0.42 | 0.99 | 0.68 | 48.1 | 11.03 | 0.46 | 1.13 |
| 03481518+6635025 | 139.247  | 9.491    | 0.762 | 1      | -      | -    | g    | -        | -    | -      | D1   | c                      | o          | -          | h?   | -        | -          | -     | 10.869                             | 0.34                        | 1.25                        | 1                    | 46.6                               | 0.28                                 | 3.47                          | 10.585                        | 0.22 | 0.87 | 0.24 | 49.2 | 10.60 | 0.23 | 0.92 |
| 03481767+5413029 | 146.995  | -0.176   | 2.190 | 1      | -      | -    | g    | -        | -    | -      | D1   | c                      | o          | -          | -    | U        | -          | -     | 11.616                             | 0.54                        | 1.80                        | 1                    | 38.2                               | 0.40                                 | 3.69                          | 10.800                        | 0.18 | 0.71 | 0.68 | 50.1 | 10.71 | 0.22 | 0.85 |
| 03482002+4955207 | 149.669  | -3.538   | 1.254 | 1      | -      | -    | g    | -        | -    | -      | D1   | c                      | o          | -          | -    | U        | -          | -     | 11.715                             | 0.50                        | 1.67                        | 1                    | 38.2                               | 0.64                                 | 3.65                          | 11.248                        | 0.29 | 1.05 | 0.39 | 43.8 | 11.21 | 0.32 | 1.13 |
| 03482003+4156074 | 154.700  | -9.771   | 0.360 | 1      | -      | -    | g    | -        | -    | -      | D1   | c                      | o          | -          | -    | U        | -          | -     | 10.221                             | 0.32                        | 1.12                        | 1                    | 70.0                               | 0.92                                 | 3.43                          | 10.087                        | 0.26 | 0.94 | 0.11 | 71.5 | 10.10 | 0.26 | 0.96 |
| 03484181+5431478 | 146.847  | 0.106    | 2.250 | 9      | -      | -    | g    | -        | -    | -      | D1   | c                      | o          | -          | -    | U        | -          | -     | 11.159                             | 1.38                        | 2.93                        | 1                    | 29.6                               | 0.32                                 | 3.64                          | 10.321                        | 1.01 | 1.82 | 0.70 | ...  | ...   | 1.05 | 1.96 |
| 03484223+4152077 | 154.797  | -9.779   | 0.388 | 1      | -      | -    | g    | -        | -    | -      | D1   | c                      | o          | -          | -    | U        | -          | -     | 10.207                             | 0.33                        | 1.13                        | 1                    | 62.8                               | 0.28                                 | 3.39                          | 10.062                        | 0.26 | 0.93 | 0.12 | 64.1 | 10.08 | 0.27 | 0.96 |
| 03485221+4220375 | 154.517  | -9.391   | 0.425 | 1      | -      | -    | g    | -        | -    | -      | D1   | c                      | o          | -          | -    | U        | -          | -     | 10.717                             | 0.30                        | 1.13                        | 1                    | 63.8                               | 0.26                                 | 3.44                          | 10.559                        | 0.23 | 0.91 | 0.13 | 65.4 | 10.57 | 0.24 | 0.94 |
| 03490015+4219095 | 154.552  | -9.395   | 0.429 | 1      | -      | -    | g    | -        | -    | -      | D1   | c                      | o          | -          | -    | U        | -          | -     | 10.345                             | 0.34                        | 1.17                        | 1                    | 61.8                               | 0.46                                 | 3.44                          | 10.185                        | 0.27 | 0.95 | 0.13 | 63.5 | 10.20 | 0.28 | 0.98 |
| 03492004+4323383 | 153.914  | -8.523   | 0.516 | 1      | -      | -    | g    | -        | -    | -      | D4   | c                      | o          | -          | -    | U        | -          | -     | 10.534                             | 0.38                        | 1.20                        | 1                    | 43.8                               | 0.74                                 | 3.44                          | 10.342                        | 0.30 | 0.94 | 0.16 | 45.2 | 10.36 | 0.31 | 0.98 |
| 03492038+5029171 | 149.442  | -2.995   | 1.434 | 1      | -      | -    | g    | -        | -    | -      | D2   | c                      | o          | -          | -    | U        | -          | -     | 11.474                             | 0.42                        | 1.52                        | 1                    | 28.6                               | 0.74                                 | 3.63                          | 10.940                        | 0.18 | 0.81 | 0.44 | 32.8 | 10.94 | 0.21 | 0.90 |
| 03492373+4924181 | 150.127  | -3.835   | 1.270 | 1      | -      | -    | g    | -        | -    | -      | D1   | c                      | o          | -          | -    | U        | -          | -     | 11.599                             | 0.52                        | 1.57                        | 1                    | 30.2                               | 0.62                                 | 3.54                          | 11.126                        | 0.31 | 0.94 | 0.39 | 34.2 | 11.11 | 0.33 | 1.02 |
| 03500078+4133517 | 155.184  | -9.861   | 0.489 | 1      | -      | -    | g    | -        | -    | -      | D3   | c                      | o          | -          | -    | U        | -          | -     | 11.156                             | 0.39                        | 1.21                        | 1                    | 33.8                               | 0.68                                 | 3.39                          | 10.974                        | 0.31 | 0.97 | 0.15 | 34.9 | 10.99 | 0.32 | 1.00 |
| 03502828+5122423 | 149.024  | -2.189   | 1.856 | 1      | -      | -    | g    | -        | -    | -      | D1   | c                      | o          | -          | h    | -        | -          | -     | 10.082                             | 0.47                        | 1.61                        | 1                    | 56.6                               | 0.68                                 | 3.64                          | 9.390                         | 0.16 | 0.69 | 0.57 | 66.8 | 9.41  | 0.20 | 0.82 |
| 03504786+4216521 | 154.837  |          |       |        |        |      |      |          |      |        |      |                        |            |            |      |          |            |       |                                    |                             |                             |                      |                                    |                                      |                               |                               |      |      |      |      |       |      |      |

Table B1: a) continued.

| 2MASX J          | <i>l</i> | <i>b</i> | EBV    | Object | Sample      | Disc   | 2MRS       | Velocity | NIR  | Photom | Ext | <i>K</i> <sub>20</sub> | <i>H-K</i> | <i>J-K</i> | vc   | <i>a</i> | <i>b/a</i> | st.d. | <i>K</i> <sub>s</sub> <sup>o</sup> | ( <i>H-K</i> ) <sup>o</sup> | ( <i>J-K</i> ) <sup>o</sup> | <i>A<sub>K</sub></i> | <i>a</i> <sub>d</sub> <sup>o</sup> | <i>K</i> <sub>s</sub> <sup>o,d</sup> | ( <i>H-K</i> ) <sup>o,c</sup> | ( <i>J-K</i> ) <sup>o,c</sup> |       |      |      |      |      |      |
|------------------|----------|----------|--------|--------|-------------|--------|------------|----------|------|--------|-----|------------------------|------------|------------|------|----------|------------|-------|------------------------------------|-----------------------------|-----------------------------|----------------------|------------------------------------|--------------------------------------|-------------------------------|-------------------------------|-------|------|------|------|------|------|
| (1)              | deg      | deg      | mag    | class  | off flg gal | TF obs | ext'd type | Opt HI   | flg  | flg    | flg | mag                    | mag        | mag        | (17) | (18)     | (19)       | (20)  | mag                                | mag                         | mag                         | mag                  | (25)                               | mag                                  | mag                           | (28)                          |       |      |      |      |      |      |
| (1)              | (2a)     | (2b)     | (3)    | (4)    | (5)         | (6)    | (7a)       | (7b)     | (7c) | (7d)   | (8) | (9)                    | (10a)      | (10b)      | (11) | (12)     | (13)       | (14)  | (15)                               | (16)                        | (17)                        | (18)                 | (19)                               | (20)                                 | (21)                          | (22)                          | (23)  | (24) | (25) | (26) | (27) | (28) |
| 03593337+4236596 | 155.864  | -7.914   | 0.430  | 1      | -           | -      | g          | -        | -    | -      | -   | -                      | 10.858     | 0.38       | 1.08 | 1        | 52.8       | 0.62  | 3.48                               | 10.698                      | 0.31                        | 0.87                 | 0.13                               | 54.2                                 | 10.71                         | 0.31                          | 0.89  |      |      |      |      |      |
| 03595969+4023423 | 157.408  | -9.529   | 0.769  | 1      | -           | -      | g          | -        | -    | -      | -   | -                      | 11.087     | 0.36       | 1.27 | 1        | 28.8       | 0.60  | 3.40                               | 10.800                      | 0.23                        | 0.88                 | 0.24                               | 30.4                                 | 10.82                         | 0.25                          | 0.93  |      |      |      |      |      |
| 04012052+4250027 | 155.968  | -7.534   | 0.483  | 1      | -           | -      | g          | -        | -    | -      | -   | -                      | 10.582     | 0.41       | 1.24 | 1        | 34.8       | 0.64  | 3.53                               | 10.402                      | 0.33                        | 1.00                 | 0.15                               | 35.9                                 | 10.41                         | 0.34                          | 1.04  |      |      |      |      |      |
| 04012641+5343171 | 148.799  | 0.677    | 1.760  | 8      | -           | -      | -          | -        | -    | -      | -   | -                      | 11.592     | 1.15       | 2.70 | -2       | 23.2       | 0.70  | 3.69                               | 10.936                      | 0.86                        | 1.82                 | 0.55                               | ...                                  | ...                           | 0.90                          | 1.94  |      |      |      |      |      |
| 04014132+5315002 | 149.137  | 0.346    | 2.276  | 1      | -           | -      | -          | -        | -    | -      | -   | -                      | 11.412     | 0.48       | 1.71 | 1        | 23.6       | 0.88  | 3.74                               | 10.564                      | 0.11                        | 0.58                 | 0.71                               | 30.0                                 | 10.55                         | 0.15                          | 0.73  |      |      |      |      |      |
| 04015124+4042146 | 157.468  | -9.064   | 0.915  | 1      | -           | -      | t          | N        | -    | -      | -   | -                      | 11.175     | 0.47       | 1.47 | 1        | 44.0       | 0.22  | 3.49                               | 10.834                      | 0.32                        | 1.01                 | 0.28                               | 47.5                                 | 10.84                         | 0.34                          | 1.07  |      |      |      |      |      |
| 04015541+4924171 | 151.693  | -2.528   | 1.232  | 1      | -           | -      | t          | N        | -    | -      | -   | -                      | 11.230     | 0.47       | 1.53 | 1        | 43.0       | 0.44  | 3.65                               | 10.771                      | 0.27                        | 0.92                 | 0.38                               | 48.2                                 | 10.77                         | 0.29                          | 1.00  |      |      |      |      |      |
| 04020732+5241528 | 149.549  | -0.027   | 1.678  | 1      | -           | -      | t          | N        | -    | -      | -   | -                      | 11.675     | 0.49       | 1.84 | 1        | 26.6       | 0.72  | 3.77                               | 11.050                      | 0.21                        | 1.01                 | 0.52                               | 31.7                                 | 11.03                         | 0.24                          | 1.12  |      |      |      |      |      |
| 04021373+4518315 | 154.440  | -5.572   | 0.524  | 1      | -           | -      | t          | N        | -    | -      | -   | -                      | 11.432     | 0.46       | 1.42 | 1        | 42.0       | 0.36  | 3.56                               | 11.237                      | 0.38                        | 1.16                 | 0.16                               | 43.6                                 | 11.24                         | 0.39                          | 1.20  |      |      |      |      |      |
| 04021796+5226239 | 149.739  | -0.204   | 2.465  | 8      | -           | -      | -          | -        | -    | -      | -   | -                      | 11.508     | 0.83       | 1.39 | 1        | 54.2       | 0.54  | 3.77                               | 10.590                      | 0.42                        | 0.17                 | 0.76                               | ...                                  | ...                           | 0.47                          | 0.33  |      |      |      |      |      |
| 04023369+4242026 | 156.226  | -7.485   | 0.492  | 1      | -           | -      | -          | -        | -    | -      | -   | -                      | 11.345     | 0.38       | 1.23 | 1        | 26.2       | 0.72  | 3.47                               | 11.162                      | 0.30                        | 0.98                 | 0.15                               | 27.0                                 | 11.17                         | 0.31                          | 1.01  |      |      |      |      |      |
| 04024662+4637195 | 153.640  | -4.524   | 0.722  | 1      | -           | -      | -          | -        | -    | -      | -   | -                      | 10.018     | 0.43       | 1.31 | 1        | 57.4       | 0.76  | 3.54                               | 9.749                       | 0.31                        | 0.95                 | 0.22                               | 60.2                                 | 9.77                          | 0.32                          | 1.00  |      |      |      |      |      |
| 04024870+5244088 | 149.602  | 0.070    | 1.676  | 1      | -           | -      | -          | -        | -    | -      | -   | -                      | 11.356     | 0.61       | 1.90 | 1        | 29.0       | 0.76  | 3.72                               | 10.732                      | 0.33                        | 1.07                 | 0.52                               | 34.4                                 | 10.72                         | 0.36                          | 1.18  |      |      |      |      |      |
| 04031107+5118183 | 150.590  | -0.967   | 12.267 | 9      | -           | -      | -          | -        | -    | -      | -   | -                      | 10.832     | 0.89       | 1.49 | 1        | 54.0       | 0.58  | 3.76                               | 6.261                       | -1.14                       | -4.60                | 3.80                               | ...                                  | ...                           | -0.90                         | -3.79 |      |      |      |      |      |
| 04031150+5120103 | 150.571  | -0.942   | 12.970 | 9      | -           | -      | -          | -        | -    | -      | -   | -                      | 11.460     | 1.08       | 2.39 | 1        | 52.0       | 0.46  | 3.76                               | 6.627                       | -1.07                       | -4.05                | 4.02                               | ...                                  | ...                           | -0.82                         | -3.19 |      |      |      |      |      |
| 04031256+5119233 | 150.581  | -0.950   | 13.518 | 9      | -           | -      | -          | -        | -    | -      | -   | -                      | 8.512      | 1.02       | 1.55 | 1        | 219.8      | 0.48  | 3.76                               | 3.475                       | -1.21                       | -5.16                | 4.19                               | ...                                  | ...                           | -0.95                         | -4.27 |      |      |      |      |      |
| 04031470+5118323 | 150.595  | -0.957   | 12.887 | 9      | -           | -      | -          | -        | -    | -      | -   | -                      | 8.754      | 1.00       | 1.33 | 1        | 159.6      | 0.68  | 3.68                               | 3.952                       | -1.13                       | -5.08                | 3.99                               | ...                                  | ...                           | -0.88                         | -4.22 |      |      |      |      |      |
| 04031470+5120293 | 150.573  | -0.933   | 13.143 | 9      | -           | -      | -          | -        | -    | -      | -   | -                      | 9.670      | 0.82       | 1.39 | 1        | 220.0      | 0.36  | 3.76                               | 4.773                       | -1.35                       | -5.13                | 4.07                               | ...                                  | ...                           | -1.10                         | -4.27 |      |      |      |      |      |
| 04031875+5117193 | 150.616  | -0.966   | 11.967 | 9      | -           | -      | -          | -        | -    | -      | -   | -                      | 11.930     | 1.27       | 1.49 | 1        | 62.6       | 0.24  | 3.68                               | 7.471                       | -0.71                       | -4.45                | 3.71                               | ...                                  | ...                           | -0.48                         | -3.66 |      |      |      |      |      |
| 04032768+5114132 | 150.668  | -0.989   | 6.479  | 8      | -           | -      | -          | -        | -    | -      | -   | -                      | 10.728     | 0.92       | 1.90 | -2       | 23.4       | 0.80  | 3.68                               | 8.314                       | -0.15                       | -1.32                | 2.01                               | ...                                  | ...                           | -0.03                         | -0.89 |      |      |      |      |      |
| 04032945+5118386 | 150.622  | -0.931   | 12.557 | 9      | -           | -      | -          | -        | -    | -      | -   | -                      | 13.887     | 0.37       | 0.72 | 2        | 13.2       | 0.66  | 3.62                               | 9.208                       | -1.71                       | -5.52                | 3.89                               | ...                                  | ...                           | -1.47                         | -4.69 |      |      |      |      |      |
| 04033039+6130017 | 143.856  | 6.700    | 0.769  | 1      | -           | -      | t          | N        | -    | -      | -   | -                      | 11.117     | 0.45       | 1.49 | 1        | 62.2       | 0.22  | 3.63                               | 10.830                      | 0.32                        | 1.11                 | 0.24                               | 66.6                                 | 10.82                         | 0.34                          | 1.16  |      |      |      |      |      |
| 04034219+4643428 | 153.688  | -4.339   | 0.717  | 1      | -           | -      | -          | -        | -    | -      | -   | -                      | 9.326      | 0.34       | 1.28 | 1        | 94.0       | 0.26  | 3.61                               | 9.059                       | 0.23                        | 0.92                 | 0.22                               | 98.3                                 | 9.08                          | 0.24                          | 0.97  |      |      |      |      |      |
| 04034964+5100578 | 150.857  | -1.117   | 4.283  | 8      | -           | -      | -          | -        | -    | -      | -   | -                      | 9.478      | 1.05       | 2.13 | 1        | 76.4       | 0.82  | 3.68                               | 7.882                       | 0.34                        | 0.00                 | 1.33                               | ...                                  | ...                           | 0.43                          | 0.28  |      |      |      |      |      |
| 04040031+4613528 | 154.059  | -4.676   | 0.778  | 1      | -           | -      | -          | -        | -    | -      | -   | -                      | 10.775     | 0.41       | 1.27 | 1        | 51.2       | 0.62  | 3.54                               | 10.485                      | 0.28                        | 0.89                 | 0.24                               | 54.5                                 | 10.49                         | 0.30                          | 0.94  |      |      |      |      |      |
| 04040253+5122417 | 150.642  | -0.823   | 6.751  | 8      | -           | -      | -          | -        | -    | -      | -   | -                      | 12.901     | 1.73       | ...  | 1        | 12.8       | 1.00  | 3.72                               | 10.386                      | 0.61                        | ...                  | 2.09                               | ...                                  | ...                           | 0.74                          | ...   |      |      |      |      |      |
| 04040466+5122377 | 150.647  | -0.820   | 6.415  | 8      | -           | -      | -          | -        | -    | -      | -   | -                      | 11.517     | 0.66       | 1.62 | -2       | 25.8       | 0.54  | 3.72                               | 9.127                       | -0.40                       | -1.56                | 1.99                               | ...                                  | ...                           | -0.28                         | -1.14 |      |      |      |      |      |
| 04041342+5122587 | 150.660  | -0.801   | 5.378  | 8      | -           | -      | -          | -        | -    | -      | -   | -                      | 11.092     | 0.84       | 1.63 | -2       | 32.8       | 0.88  | 3.72                               | 9.088                       | -0.05                       | -1.04                | 1.67                               | ...                                  | ...                           | 0.05                          | -0.69 |      |      |      |      |      |
| 04041599+5123146 | 150.662  | -0.793   | 5.197  | 9      | -           | -      | -          | -        | -    | -      | -   | -                      | 12.869     | 1.11       | ...  | 1        | 25.8       | 0.60  | 3.72                               | 10.933                      | 0.25                        | ...                  | 1.61                               | ...                                  | ...                           | 0.36                          | ...   |      |      |      |      |      |
| 04041817+4147204 | 157.082  | -7.949   | 0.704  | 1      | -           | -      | -          | -        | -    | -      | -   | -                      | 11.245     | 0.31       | 1.22 | 1        | 31.8       | 0.82  | 3.51                               | 10.983                      | 0.20                        | 0.87                 | 0.22                               | 33.5                                 | 10.99                         | 0.21                          | 0.92  |      |      |      |      |      |
| 04042013+5123367 | 150.666  | -0.781   | 4.912  | 8      | -           | -      | -          | -        | -    | -      | -   | -                      | 12.899     | 0.86       | 1.99 | -2       | 27.8       | 0.28  | 3.74                               | 11.069                      | 0.05                        | -0.45                | 1.52                               | ...                                  | ...                           | 0.15                          | -0.13 |      |      |      |      |      |
| 04043132+4426000 | 155.330  | -5.957   | 0.523  | 1      | -           | -      | -          | -        | -    | -      | -   | -                      | 10.824     | 0.37       | 1.19 | 1        | 43.2       | 0.76  | 3.47                               | 10.629                      | 0.29                        | 0.93                 | 0.16                               | 44.7                                 | 10.64                         | 0.30                          | 0.97  |      |      |      |      |      |
| 04043687+4151264 | 157.079  | -7.859   | 0.700  | 1      | -           | -      | -          | -        | -    | -      | -   | -                      | 11.296     | 0.33       | 1.18 | 1        | 25.6       | 0.54  | 3.51                               | 11.035                      | 0.21                        | 0.83                 | 0.22                               | 26.9                                 | 11.05                         | 0.23                          | 0.88  |      |      |      |      |      |
| 04045627+6312138 | 142.831  | 8.077    | 0.893  | 1      | -           | -      | -          | -        | -    | -      | -   | -                      | 10.547     | 0.40       | 1.36 | 1        | 39.0       | 0.78  | 3.47                               | 10.214                      | 0.25                        | 0.91                 | 0.28                               | 41.6                                 | 10.24                         | 0.27                          | 0.97  |      |      |      |      |      |
| 04050668+4028583 | 158.083  | -8.814   | 1.076  | 1      | -           | -      | -          | -        | -    | -      | -   | -                      | 11.583     | 0.43       | 1.43 | 1        | 28.6       | 0.58  | 3.40                               | 11.182                      | 0.26                        | 0.89                 | 0.33                               | 31.4                                 | 11.19                         | 0.28                          | 0.96  |      |      |      |      |      |
| 04052574+5445057 | 148.555  | 1.835    | 3.306  | 9      | -           | -      | -          | -        | -    | -      | -   | -                      | 11.219     | 0.93       | 1.86 | 1        | 84.0       | 0.30  | 3.72                               | 9.987                       | 0.39                        | 0.22                 | 1.02                               | ...                                  | ...                           | 0.45                          | 0.43  |      |      |      |      |      |
| 04052826+4938132 | 151.970  | -1.972   | 2.370  | 9      | -           | -      | -          | -        | -    | -      | -   | -                      | 11.016     | 0.94       | 1.85 | 1        | 83.2       | 0.44  | 3.72                               | 10.133                      | 0.55                        | 0.67                 | 0.73                               | ...                                  | ...                           | 0.59                          | 0.83  |      |      |      |      |      |
| 04053024+5445127 | 148.562  | 1.844    | 3.407  | 9      | -           | -      | -          | -        | -    | -      | -   | -                      | 11.921     | 0.74       | 1.66 | 1        | 35.6       | 0.68  | 3.72                               | 10.652                      | 0.18                        | -0.03                | 1.06                               | ...                                  | ...                           | 0.24                          | 0.20  |      |      |      |      |      |
| 04053511+4149351 | 157.236  | -7.761   | 0.713  | 1      | -           | -      | t          | N        | -    | -      | -   | -                      | 11.027     | 0.39       | 1.28 | 1        | 41.0       | 0.28  | 3.49                               | 10.761                      | 0.27                        | 0.92                 | 0.22                               | 43.1                                 | 10.78                         | 0.29                          | 0.97  |      |      |      |      |      |
| 04054076+5454507 | 148.473  | 1.980    | 5.327  | 8      | -           | -      | -          | -        | -    | -      | -   | -                      | 11.426     | 0.94       | 2.33 | -2       | 33.0       | 0.62  | 3.66                               | 9.441                       | 0.06                        | -0.31                | 1.65                               | ...                                  | ...                           | 0.17                          | 0.04  |      |      |      |      |      |
| 04054697+5025041 | 151.486  | -1.357   | 1.596  | 9      | -           | -      | -          | -        | -    | -      | -   | -                      | 11.696     | 1.13       | 2.32 | -2       | 21.2       | 0.48  | 3.73                               | 11.101                      | 0.87                        | 1.52                 | 0.49                               | ...                                  | ...                           | 0.90                          | 1.63  |      |      |      |      |      |
| 04055121+5128262 | 150.789  | -0.564   | 1.817  | 8      | -           | -      | -          | -        | -    | -      | -   | -                      | 10.964     | 1.07       | 2.10 | 1        | 40.2       | 0.86  | 3.77                               | 10.287                      | 0.77                        | 1.20                 | 0.56                               | ...                                  | ...                           | 0.81                          | 1.32  |      |      |      |      |      |
| 04055619+5023102 | 151.526  | -1.365   | 1.537  | 1      | -           | -      | -          | -        | -    | -      | -   | -                      | 11.674     | 0.64       | 1.77 | 1        | 22.8       | 0.72  | 3.73                               | 11.101                      | 0.39                        | 1.00                 | 0.48                               | 26.6                                 | 11.09                         | 0.42                          | 1.11  |      |      |      |      |      |
| 04055657+5127052 | 150.815  | -0.571   | 1.845  | 8      | -           | -      | -          | -        | -    | -      | -   | -                      | 9.263      | 0.81       | 1.93 | -2       | 36.6       | 0.94  | 3.77                               | 8.576                       | 0.51                        | 1.01                 | 0.57                               | ...                                  | ...                           | 0.54                          | 1.13  |      |      |      |      |      |
| 04060596+4020487 | 158.316  | -8.788   | 1.068  | 1      | -           | -      | -          | -        | -    | -      | -   | -                      | 11.182     | 0.52       | 1.52 | 1        | 34.8       | 0.92  | 3.44                               | 10.784                      | 0.34                        | 0.99                 | 0.33                               | 38.3                                 | 10.79                         | 0.36                          | 1.06  |      |      |      |      |      |
| 04062549+5321492 | 149.591  | 0.900    | 1.799  | 8      | -           | -      | -          | -        | -    | -      | -   | -                      | 10.686     | 0.66       | 1.52 | 1        | 54.2       | 0.58  | 3.74                               | 10.016                      | 0.36                        | 0.62                 | 0.56                               | ...                                  | ...                           | 0.39                          | 0.74  |      |      |      |      |      |
| 04065818+6055018 | 144.561  | 6.547    | 0.763  | 8      | -           | p      | -          | -        | -    | -      | -   | -                      | 11.030     | ...        | 1.29 | 1        | 56.8       | 1.00  | 3.56                               | 10.746                      | ...                         | 0.91                 | 0.24                               | ...                                  | ...                           | ...                           | 0.96  |      |      |      |      |      |
| 04070757+5111106 | 151.130  | -0.644   | 2.125  | 8      | -           | -      | -          | -        | -    | -      | -   | -                      | 11.065     | 0.81       | 1.96 | 1        | 26.2       | 0.88  | 3.82                               | 10.273                      | 0.46                        | 0.91                 | 0.66                               | ...                                  | ...                           | 0.50                          | 1.05  |      |      |      |      |      |
| 04071030+5934123 | 145.493  | 5.569    | 0.726  | 1      | -           | -      | t          | N        | -    | -      | -   | -                      | 10.942     | 0.40       | 1.34 | 1        | 38.0       | 0.44  | 3.58                               | 10.671                      | 0.28                        | 0.98                 | 0.22                               | 40.0                                 | 10.69                         | 0.30                          |       |      |      |      |      |      |

Table B1: a) continued.

| 2MASX J          | <i>l</i> | <i>b</i> | EBV    | Object | Sample | Disc | 2MRS | Velocity | NIR  | Photom | Ext   | <i>K</i> <sub>20</sub> | <i>H-K</i> | <i>J-K</i> | vc   | <i>a</i> | <i>b/a</i> | st.d. | <i>K</i> <sub>s</sub> <sup>o</sup> | ( <i>H-K</i> ) <sup>o</sup> | ( <i>J-K</i> ) <sup>o</sup> | <i>A<sub>K</sub></i> | <i>a</i> <sub>d</sub> <sup>o</sup> | <i>K</i> <sub>s</sub> <sup>o,d</sup> | ( <i>H-K</i> ) <sup>o,c</sup> | ( <i>J-K</i> ) <sup>o,c</sup> |      |
|------------------|----------|----------|--------|--------|--------|------|------|----------|------|--------|-------|------------------------|------------|------------|------|----------|------------|-------|------------------------------------|-----------------------------|-----------------------------|----------------------|------------------------------------|--------------------------------------|-------------------------------|-------------------------------|------|
| (1)              | deg      | deg      | mag    | class  | off    | flag | gal  | TF       | (7b) | (7c)   | ext'd | type                   | (8)        | (9)        | Opt  | HI       | (10b)      | (11)  | flag                               | flag                        | flag                        | mag                  | (25)                               | mag                                  | (27)                          | mag                           | (28) |
| (2a)             | (2b)     | (3)      | (4)    | (5)    | (6)    | (7a) | (7b) | (7c)     | (7d) | (7e)   | (7f)  | (7g)                   | (7h)       | (7i)       | (7j) | (7k)     | (7l)       | (7m)  | (7n)                               | (7o)                        | (7p)                        | (7q)                 | (7r)                               | (7s)                                 | (7t)                          | (7u)                          | (7v) |
| 04110989+5110198 | 151.606  | -0.227   | 27.659 | 9      | -      | -    | -    | -        | -    | -      | -     | -                      | -          | -          | -    | -        | -          | -     | -                                  | -                           | -                           | -                    | -                                  | -                                    | -                             | -                             |      |
| 04111032+4710144 | 154.335  | -3.155   | 1.088  | 1      | -      | -    | -    | -        | -    | -      | -     | -                      | -          | -          | -    | -        | -          | -     | -                                  | -                           | -                           | -                    | -                                  | -                                    | -                             | -                             |      |
| 04111245+5110528 | 151.604  | -0.216   | 26.792 | 9      | -      | -    | -    | -        | -    | -      | -     | -                      | -          | -          | -    | -        | -          | -     | -                                  | -                           | -                           | -                    | -                                  | -                                    | -                             | -                             |      |
| 04111287+5109207 | 151.622  | -0.234   | 28.266 | 9      | -      | -    | -    | -        | -    | -      | -     | -                      | -          | -          | -    | -        | -          | -     | -                                  | -                           | -                           | -                    | -                                  | -                                    | -                             | -                             |      |
| 04111563+5109527 | 151.622  | -0.222   | 29.185 | 9      | -      | -    | -    | -        | -    | -      | -     | -                      | -          | -          | -    | -        | -          | -     | -                                  | -                           | -                           | -                    | -                                  | -                                    | -                             | -                             |      |
| 04112872+5518091 | 148.823  | 2.827    | 1.506  | 1      | -      | -    | -    | -        | -    | -      | -     | -                      | -          | -          | -    | -        | -          | -     | -                                  | -                           | -                           | -                    | -                                  | -                                    | -                             | -                             |      |
| 04113162+3914215 | 159.853  | -8.884   | 1.041  | 1      | -      | -    | -    | -        | -    | -      | -     | -                      | -          | -          | -    | -        | -          | -     | -                                  | -                           | -                           | -                    | -                                  | -                                    | -                             | -                             |      |
| 04114143+3841285 | 160.259  | -9.258   | 1.421  | 1      | -      | -    | -    | -        | -    | -      | -     | -                      | -          | -          | -    | -        | -          | -     | -                                  | -                           | -                           | -                    | -                                  | -                                    | -                             | -                             |      |
| 04115648+3930133 | 159.727  | -8.637   | 0.906  | 1      | -      | -    | -    | -        | -    | -      | -     | -                      | -          | -          | -    | -        | -          | -     | -                                  | -                           | -                           | -                    | -                                  | -                                    | -                             | -                             |      |
| 04115755+3838463 | 160.329  | -9.254   | 1.501  | 1      | -      | -    | -    | -        | -    | -      | -     | -                      | -          | -          | -    | -        | -          | -     | -                                  | -                           | -                           | -                    | -                                  | -                                    | -                             | -                             |      |
| 04115864+3842213 | 160.290  | -9.209   | 1.577  | 1      | -      | -    | -    | -        | -    | -      | -     | -                      | -          | -          | -    | -        | -          | -     | -                                  | -                           | -                           | -                    | -                                  | -                                    | -                             | -                             |      |
| 04120068+3846073 | 160.251  | -9.159   | 1.677  | 1      | -      | -    | -    | -        | -    | -      | -     | -                      | -          | -          | -    | -        | -          | -     | -                                  | -                           | -                           | -                    | -                                  | -                                    | -                             | -                             |      |
| 04120222+5555441 | 148.452  | 3.338    | 0.911  | 1      | -      | -    | -    | -        | -    | -      | -     | -                      | -          | -          | -    | -        | -          | -     | -                                  | -                           | -                           | -                    | -                                  | -                                    | -                             | -                             |      |
| 04120378+5457472 | 149.116  | 2.636    | 1.708  | 1      | -      | -    | -    | -        | -    | -      | -     | -                      | -          | -          | -    | -        | -          | -     | -                                  | -                           | -                           | -                    | -                                  | -                                    | -                             | -                             |      |
| 04121283+3842023 | 160.327  | -9.181   | 1.675  | 1      | -      | -    | -    | -        | -    | -      | -     | -                      | -          | -          | -    | -        | -          | -     | -                                  | -                           | -                           | -                    | -                                  | -                                    | -                             | -                             |      |
| 04122913+3838553 | 160.403  | -9.181   | 1.616  | 1      | -      | -    | -    | -        | -    | -      | -     | -                      | -          | -          | -    | -        | -          | -     | -                                  | -                           | -                           | -                    | -                                  | -                                    | -                             | -                             |      |
| 04124119+3843433 | 160.375  | -9.097   | 1.628  | 1      | -      | -    | -    | -        | -    | -      | -     | -                      | -          | -          | -    | -        | -          | -     | -                                  | -                           | -                           | -                    | -                                  | -                                    | -                             | -                             |      |
| 04124692+3835153 | 160.488  | -9.185   | 1.548  | 1      | -      | -    | -    | -        | -    | -      | -     | -                      | -          | -          | -    | -        | -          | -     | -                                  | -                           | -                           | -                    | -                                  | -                                    | -                             | -                             |      |
| 04131274+5020366 | 152.408  | -0.610   | 1.647  | 9      | -      | -    | -    | -        | -    | -      | -     | -                      | -          | -          | -    | -        | -          | -     | -                                  | -                           | -                           | -                    | -                                  | -                                    | -                             | -                             |      |
| 04131504+5656581 | 147.872  | 4.195    | 0.964  | 9      | -      | p    | -    | -        | -    | -      | -     | -                      | -          | -          | -    | -        | -          | -     | -                                  | -                           | -                           | -                    | -                                  | -                                    | -                             | -                             |      |
| 04131853+3819491 | 160.744  | -9.299   | 1.648  | 1      | -      | -    | -    | -        | -    | -      | -     | -                      | -          | -          | -    | -        | -          | -     | -                                  | -                           | -                           | -                    | -                                  | -                                    | -                             | -                             |      |
| 04133389+5041476 | 152.207  | -0.315   | 1.621  | 1      | -      | -    | -    | -        | -    | -      | -     | -                      | -          | -          | -    | -        | -          | -     | -                                  | -                           | -                           | -                    | -                                  | -                                    | -                             | -                             |      |
| 04141562+5037307 | 152.336  | -0.291   | 2.093  | 9      | -      | -    | -    | -        | -    | -      | -     | -                      | -          | -          | -    | -        | -          | -     | -                                  | -                           | -                           | -                    | -                                  | -                                    | -                             | -                             |      |
| 04151246+3840071 | 160.775  | -8.797   | 1.457  | 1      | -      | -    | -    | -        | -    | -      | -     | -                      | -          | -          | -    | -        | -          | -     | -                                  | -                           | -                           | -                    | -                                  | -                                    | -                             | -                             |      |
| 04152200+5034364 | 149.306  | 3.179    | 1.916  | 1      | -      | -    | -    | -        | -    | -      | -     | -                      | -          | -          | -    | -        | -          | -     | -                                  | -                           | -                           | -                    | -                                  | -                                    | -                             | -                             |      |
| 04153820+5513325 | 143.405  | 9.262    | 0.969  | 2      | -      | -    | -    | -        | -    | -      | -     | -                      | -          | -          | -    | -        | -          | -     | -                                  | -                           | -                           | -                    | -                                  | -                                    | -                             | -                             |      |
| 04161343+6338240 | 149.356  | 3.179    | 1.916  | 1      | -      | -    | -    | -        | -    | -      | -     | -                      | -          | -          | -    | -        | -          | -     | -                                  | -                           | -                           | -                    | -                                  | -                                    | -                             | -                             |      |
| 04161779+5034094 | 152.608  | -0.108   | 1.755  | 1      | -      | -    | -    | -        | -    | -      | -     | -                      | -          | -          | -    | -        | -          | -     | -                                  | -                           | -                           | -                    | -                                  | -                                    | -                             | -                             |      |
| 04163977+6055282 | 145.417  | 7.362    | 0.839  | 1      | -      | -    | -    | -        | -    | -      | -     | -                      | -          | -          | -    | -        | -          | -     | -                                  | -                           | -                           | -                    | -                                  | -                                    | -                             | -                             |      |
| 04164549+3925359 | 160.455  | -8.045   | 1.023  | 1      | -      | -    | -    | -        | -    | -      | -     | -                      | -          | -          | -    | -        | -          | -     | -                                  | -                           | -                           | -                    | -                                  | -                                    | -                             | -                             |      |
| 04165899+4437498 | 156.824  | -4.296   | 0.686  | 1      | -      | -    | -    | -        | -    | -      | -     | -                      | -          | -          | -    | -        | -          | -     | -                                  | -                           | -                           | -                    | -                                  | -                                    | -                             | -                             |      |
| 04170636+4910038 | 153.676  | -1.026   | 1.457  | 1      | -      | -    | -    | -        | -    | -      | -     | -                      | -          | -          | -    | -        | -          | -     | -                                  | -                           | -                           | -                    | -                                  | -                                    | -                             | -                             |      |
| 04171667+6111077 | 145.286  | 7.601    | 0.804  | 1      | -      | -    | -    | -        | -    | -      | -     | -                      | -          | -          | -    | -        | -          | -     | -                                  | -                           | -                           | -                    | -                                  | -                                    | -                             | -                             |      |
| 04173955+3745411 | 161.767  | -9.104   | 1.641  | 1      | -      | -    | -    | -        | -    | -      | -     | -                      | -          | -          | -    | -        | -          | -     | -                                  | -                           | -                           | -                    | -                                  | -                                    | -                             | -                             |      |
| 04175296+4911337 | 153.749  | -0.919   | 1.536  | 1      | -      | -    | -    | -        | -    | -      | -     | -                      | -          | -          | -    | -        | -          | -     | -                                  | -                           | -                           | -                    | -                                  | -                                    | -                             | -                             |      |
| 04180187+5828432 | 147.267  | 5.739    | 0.801  | 1      | -      | -    | -    | -        | -    | -      | -     | -                      | -          | -          | -    | -        | -          | -     | -                                  | -                           | -                           | -                    | -                                  | -                                    | -                             | -                             |      |
| 04182123+3801358 | 161.675  | -8.820   | 1.653  | 1      | -      | -    | -    | -        | -    | -      | -     | -                      | -          | -          | -    | -        | -          | -     | -                                  | -                           | -                           | -                    | -                                  | -                                    | -                             | -                             |      |
| 04183258+5326027 | 150.860  | 2.188    | 2.348  | 8      | -      | -    | -    | -        | -    | -      | -     | -                      | -          | -          | -    | -        | -          | -     | -                                  | -                           | -                           | -                    | -                                  | -                                    | -                             | -                             |      |
| 04183887+4528349 | 156.442  | -3.486   | 0.868  | 1      | -      | -    | -    | -        | -    | -      | -     | -                      | -          | -          | -    | -        | -          | -     | -                                  | -                           | -                           | -                    | -                                  | -                                    | -                             | -                             |      |
| 04190951+3927271 | 160.765  | -7.697   | 0.924  | 1      | -      | -    | -    | -        | -    | -      | -     | -                      | -          | -          | -    | -        | -          | -     | -                                  | -                           | -                           | -                    | -                                  | -                                    | -                             | -                             |      |
| 04191179+5552439 | 149.211  | 3.998    | 1.126  | 1      | -      | -    | -    | -        | -    | -      | -     | -                      | -          | -          | -    | -        | -          | -     | -                                  | -                           | -                           | -                    | -                                  | -                                    | -                             | -                             |      |
| 04191224+5552266 | 149.215  | 3.995    | 1.123  | 9      | -      | e    | -    | -        | -    | -      | -     | -                      | -          | -          | -    | -        | -          | -     | -                                  | -                           | -                           | -                    | -                                  | -                                    | -                             | -                             |      |
| 04192537+5257568 | 151.282  | 1.946    | 4.311  | 9      | -      | -    | -    | -        | -    | -      | -     | -                      | -          | -          | -    | -        | -          | -     | -                                  | -                           | -                           | -                    | -                                  | -                                    | -                             | -                             |      |
| 04193291+5258417 | 151.287  | 1.968    | 4.373  | 9      | -      | -    | -    | -        | -    | -      | -     | -                      | -          | -          | -    | -        | -          | -     | -                                  | -                           | -                           | -                    | -                                  | -                                    | -                             | -                             |      |
| 04193292+5251225 | 151.373  | 1.881    | 2.135  | 8      | -      | -    | -    | -        | -    | -      | -     | -                      | -          | -          | -    | -        | -          | -     | -                                  | -                           | -                           | -                    | -                                  | -                                    | -                             | -                             |      |
| 04193391+3616381 | 163.106  | -9.881   | 0.580  | 1      | -      | -    | -    | -        | -    | -      | -     | -                      | -          | -          | -    | -        | -          | -     | -                                  | -                           | -                           | -                    | -                                  | -                                    | -                             | -                             |      |
| 04200181+4203277 | 159.033  | -5.740   | 0.751  | 1      | -      | -    | -    | -        | -    | -      | -     | -                      | -          | -          | -    | -        | -          | -     | -                                  | -                           | -                           | -                    | -                                  | -                                    | -                             | -                             |      |
| 04201232+3608446 | 163.293  | -9.881   | 0.597  | 1      | -      | -    | -    | -        | -    | -      | -     | -                      | -          | -          | -    | -        | -          | -     | -                                  | -                           | -                           | -                    | -                                  | -                                    | -                             | -                             |      |
| 04202172+5810342 | 147.699  | 5.739    | 0.789  | 1      | -      | -    | -    | -        | -    | -      | -     | -                      | -          | -          | -    | -        | -          | -     | -                                  | -                           | -                           | -                    | -                                  | -                                    | -                             | -                             |      |
| 04202281+4535327 | 156.577  | -3.190   | 1.081  | 1      | -      | -    | -    | -        | -    | -      | -     | -                      | -          | -          | -    | -        | -          | -     | -                                  | -                           | -                           | -                    | -                                  | -                                    | -                             | -                             |      |
| 04204654+5237183 | 151.670  | 1.845    | 1.492  | 1      | -      | -    | -    | -        | -    | -      | -     | -                      | -          | -          | -    | -        | -          | -     | -                                  | -                           | -                           | -                    | -                                  | -                                    | -                             | -                             |      |
| 04205271+3659053 | 162.782  | -9.197   | 0.990  | 1      | -      | -    | -    | -        | -    | -      | -     | -                      | -          | -          | -    | -        | -          | -     | -                                  | -                           | -                           | -                    | -                                  | -                                    | -                             | -                             |      |
| 04210089+4042413 | 160.123  | -6.560   | 0.720  | 1      | -      | -    | -    | -        | -    | -      | -     | -                      | -          | -          | -    | -        | -          | -     | -                                  | -                           | -                           | -                    | -                                  | -                                    | -                             | -                             |      |
| 04210584+4830168 | 154.609  | -1.039   | 1.690  | 1      | -      | -    | -    | -        | -    | -      | -     | -                      | -          | -          | -    | -        | -          | -     | -                                  | -                           | -                           | -                    | -                                  | -                                    | -                             | -                             |      |
| 04210637+3704473 | 162.745  | -9.098   | 1.163  | 1      | -      | -    | -    | -        | -    | -      | -     | -                      | -          | -          | -    | -        | -          | -     | -                                  | -                           | -                           | -                    | -                                  | -                                    | -                             | -                             |      |
| 04211418+3555203 | 163.603  | -9.888   | 0.551  | 1      | -      | -    | -    | -        | -    | -      | -     | -                      | -          | -          | -    | -        | -          | -     | -                                  | -                           | -                           | -                    | -                                  | -                                    | -                             | -                             |      |
| 04211472+3710123 | 162.699  | -9.015   | 1.264  | 1      | -      | -    | -    | -        | -    | -      | -     | -                      | -          | -          | -    | -        | -          | -     | -                                  | -                           | -                           | -                    | -                                  | -                                    | -                             | -                             |      |
| 04211998+3645363 | 163.009  | -9.289   | 0.736  | 1      | -      | -    | -    | -        | -    | -      | -     | -                      | -          | -          | -    | -        | -          | -     | -                                  | -                           | -                           | -                    | -                                  | -                                    | -                             | -                             |      |
| 04212943+3656572 | 162.894  | -9.135   | 0.952  | 1      | -      | -    | -    | -        | -    | -      | -     | -                      | -          | -          | -    | -        | -          | -     | -                                  | -                           | -                           | -                    | -                                  | -                                    | -                             | -                             |      |
| 04213887+3734443 | 162.460  | -8.672   | 1.862  | 8      | -      | -    | -    | -        | -    | -      | -     | -                      | -          | -          | -    | -        | -          | -     | -                                  | -                           | -                           | -                    | -                                  | -                                    | -                             | -                             |      |
| 04214005+3643543 | 163.077  | -9.261   | 0.730  | 1      | -      | -    | -    | -        | -    | -      | -     | -                      | -          | -          | -    | -        | -          | -     | -                                  | -                           | -                           | -                    | -                                  | -                                    | -                             | -                             |      |
| 04214920+3652033 | 163.000  | -9.145   | 0.879  | 1      | -      | -    | -    | -        | -    | -      | -     | -                      | -          | -          | -    | -        | -          | -     | -                                  | -                           | -                           | -                    | -                                  | -                                    | -                             | -                             |      |
| 04215207+3607373 | 163.545  | -9.654   | 0.566  | 1      | -      | -    | -    | -        | -    | -      | -     | -                      | -          | -          | -    | -        | -          | -     | -                                  | -                           | -                           | -                    | -                                  | -                                    | -                             | -                             |      |
| 04220023+4302560 | 158.586  | -4.783   | 0.720  | 1      | -      | -    | -    | -        | -    | -      | -     | -                      | -          | -          | -    | -        | -          | -     | -                                  | -                           | -                           | -                    | -                                  | -                                    | -                             | -                             |      |
| 04222603+5150395 | 152.399  | 1.475    | 2.078  | 8      | -      | -    | -    | -        | -    | -      | -     | -                      | -          | -          | -    | -        | -          | -     | -                                  | -                           | -                           | -                    | -                                  | -                                    | -                             | -                             |      |
| 04222946+3707012 | 162.913  | -8.875   | 1.343  | 1      | -      | -    | -    | -        | -    | -      | -     | -                      | -          | -          | -    | -        | -          | -     | -                                  | -                           | -                           | -                    | -                                  | -                                    | -                             | -                             |      |
| 04223304+5150346 | 152.413  | 1.487    | 2.082  | 8      | -      | -    | -    |          |      |        |       |                        |            |            |      |          |            |       |                                    |                             |                             |                      |                                    |                                      |                               |                               |      |



© 2017 RAS, MNRAS 000, 1–133



Table B1: a) continued.

| 2MASX J          | <i>l</i> | <i>b</i> | EBV    | Object |     | Sample | Disc | 2MRS | Velocity | NIR  | Photom | Ext   | <i>K</i> <sub>20</sub> | <i>H-K</i> | <i>J-K</i> | vc   | <i>a</i> | <i>b/a</i> | st.d. | <i>K</i> <sub>s</sub> <sup>o</sup> | ( <i>H-K</i> ) <sup>o</sup> | ( <i>J-K</i> ) <sup>o</sup> | <i>A</i> <sub>K</sub> | <i>a</i> <sub>d</sub> <sup>o</sup> | <i>K</i> <sub>s</sub> <sup>o,d</sup> | ( <i>H-K</i> ) <sup>o,c</sup> | ( <i>J-K</i> ) <sup>o,c</sup> |       |       |      |       |       |       |       |
|------------------|----------|----------|--------|--------|-----|--------|------|------|----------|------|--------|-------|------------------------|------------|------------|------|----------|------------|-------|------------------------------------|-----------------------------|-----------------------------|-----------------------|------------------------------------|--------------------------------------|-------------------------------|-------------------------------|-------|-------|------|-------|-------|-------|-------|
| (1)              | deg      | deg      | mag    | class  | off | gal    | TF   | obs  | ext'd    | type | flag   | flag  | flag                   | mag        | mag        | mag  | "        | "          | "     | mag                                | mag                         | mag                         | mag                   | "                                  | mag                                  | mag                           | mag                           |       |       |      |       |       |       |       |
| (2a)             | (2b)     | (2b)     | (3)    | (4)    | (5) | (6)    | (7a) | (7c) | (7d)     | (8)  | (9)    | (10a) | (10b)                  | (11)       | (12)       | (13) | (14)     | (15)       | (16)  | (17)                               | (18)                        | (19)                        | (20)                  | (21)                               | (22)                                 | (23)                          | (24)                          | (25)  | (26)  | (27) | (28)  |       |       |       |
| 04325689+5946246 | 147.663  | 8.015    | 0.646  | 1      | —   | —      | g    | —    | —        | D2   | c      | o     | h                      | —          | —          | —    | —        | —          | —     | 10.493                             | 0.37                        | 1.26                        | 1                     | 37.2                               | 0.86                                 | 3.47                          | 10.252                        | 0.26  | 0.94  | 0.20 | 38.8  | 10.27 | 0.28  | 0.98  |
| 04332611+5043312 | 154.398  | 1.941    | 2.303  | 9      | —   | —      | —    | —    | —        | D1   | —      | —     | —                      | —          | —          | —    | —        | —          | —     | 10.994                             | 0.75                        | 1.91                        | 1                     | 31.2                               | 0.58                                 | 3.65                          | 10.136                        | 0.37  | 0.77  | 0.71 | ...   | ...   | 0.41  | 0.92  |
| 04333811+4530061 | 158.255  | -1.583   | 1.324  | 1      | —   | —      | —    | —    | —        | D1   | —      | —     | —                      | —          | —          | —    | —        | —          | —     | 9.662                              | 0.48                        | 1.54                        | 1                     | 105.8                              | 0.66                                 | 3.65                          | 9.169                         | 0.26  | 0.89  | 0.41 | 119.2 | 9.18  | 0.29  | 0.97  |
| 04340516+4013021 | 161.608  | -4.555   | 0.628  | 1      | —   | —      | —    | —    | —        | D2   | —      | —     | —                      | —          | —          | —    | —        | —          | —     | 11.304                             | 0.32                        | 1.24                        | 1                     | 34.0                               | 0.66                                 | 3.58                          | 11.070                        | 0.22  | 0.92  | 0.19 | 35.6  | 11.08 | 0.23  | 0.97  |
| 04342620+5527118 | 151.013  | 5.252    | 0.949  | 1      | —   | —      | —    | —    | —        | D1   | c      | o     | o                      | —          | —          | —    | —        | —          | —     | 11.382                             | 0.45                        | 1.27                        | 1                     | 24.6                               | 0.68                                 | 3.46                          | 11.028                        | 0.30  | 0.80  | 0.29 | 26.7  | 11.03 | 0.32  | 0.87  |
| 04343593+4011242 | 162.293  | -5.047   | 0.785  | 1      | —   | —      | —    | —    | —        | D1   | c      | o     | o                      | —          | —          | —    | —        | —          | —     | 10.551                             | 0.35                        | 1.22                        | 1                     | 63.6                               | 0.38                                 | 3.55                          | 10.259                        | 0.22  | 0.83  | 0.24 | 67.4  | 10.27 | 0.23  | 0.88  |
| 04344151+4014219 | 162.268  | -5.001   | 0.772  | 1      | —   | —      | —    | —    | —        | D1   | c      | o     | o                      | —          | —          | —    | —        | —          | —     | 10.564                             | 0.65                        | 1.61                        | 1                     | 31.6                               | 0.78                                 | 3.56                          | 10.276                        | 0.52  | 1.23  | 0.24 | 33.1  | 10.30 | 0.54  | 1.28  |
| 04350092+5939419 | 147.923  | 8.133    | 0.595  | 1      | —   | —      | —    | —    | —        | D1   | c      | o     | o                      | —          | —          | —    | —        | —          | —     | 11.071                             | 0.41                        | 1.41                        | 1                     | 65.4                               | 0.20                                 | 3.49                          | 10.849                        | 0.32  | 1.11  | 0.18 | 68.6  | 10.85 | 0.33  | 1.15  |
| 04352485+5421529 | 151.916  | 4.623    | 1.109  | 1      | —   | —      | —    | —    | —        | D1   | c      | o     | o                      | —          | —          | —    | —        | —          | —     | 11.496                             | 0.46                        | 1.49                        | 1                     | 48.4                               | 0.30                                 | 3.57                          | 11.083                        | 0.27  | 0.94  | 0.34 | 53.6  | 11.08 | 0.30  | 1.01  |
| 04352497+3248050 | 167.945  | -9.867   | 0.734  | 1      | —   | —      | —    | —    | —        | D1   | c      | o     | o                      | —          | —          | —    | —        | —          | —     | 10.931                             | 0.45                        | 1.32                        | 1                     | 36.8                               | 0.86                                 | 3.41                          | 10.658                        | 0.32  | 0.96  | 0.23 | 38.9  | 10.67 | 0.34  | 1.01  |
| 04354370+5201294 | 153.682  | 3.083    | 1.868  | 7      | —   | —      | —    | —    | —        | D1   | c      | o     | o                      | —          | —          | —    | —        | —          | —     | 11.023                             | 1.63                        | 3.34                        | 1                     | 20.0                               | 0.78                                 | 3.70                          | 10.327                        | 1.32  | 2.41  | 0.58 | ...   | ...   | 1.36  | 2.53  |
| 04354851+3552572 | 165.670  | -7.758   | 0.873  | 1      | —   | —      | —    | —    | —        | D1   | c      | o     | o                      | —          | —          | —    | —        | —          | —     | 11.507                             | 0.48                        | 1.55                        | 1                     | 38.0                               | 0.76                                 | 3.40                          | 11.182                        | 0.34  | 1.11  | 0.27 | 40.9  | 11.19 | 0.35  | 1.17  |
| 04360299+5112304 | 154.321  | 2.571    | 8.953  | 9      | —   | —      | —    | —    | —        | —    | —      | —     | —                      | —          | —          | —    | —        | —          | —     | 12.461                             | ...                         | ...                         | 1                     | 30.2                               | 0.48                                 | 3.62                          | 9.125                         | ...   | ...   | 2.77 | ...   | ...   | ...   |       |
| 04360363+4030314 | 162.244  | -4.627   | 0.688  | 1      | —   | —      | —    | —    | —        | D4   | —      | —     | —                      | —          | —          | —    | —        | —          | —     | 11.434                             | 0.44                        | 1.33                        | 1                     | 26.8                               | 0.82                                 | 3.54                          | 11.178                        | 0.32  | 0.98  | 0.21 | 28.3  | 11.19 | 0.34  | 1.03  |
| 04361077+5919153 | 148.279  | 8.016    | 0.594  | 1      | —   | —      | —    | —    | —        | D1   | c      | o     | o                      | —          | —          | —    | —        | —          | —     | 10.278                             | 0.50                        | 1.48                        | 1                     | 47.2                               | 0.56                                 | 3.44                          | 10.057                        | 0.40  | 1.18  | 0.18 | 49.0  | 10.08 | 0.41  | 1.22  |
| 04361212+5111195 | 154.351  | 2.575    | 9.470  | 9      | —   | —      | —    | —    | —        | —    | —      | —     | —                      | —          | —          | —    | —        | —          | —     | 13.345                             | ...                         | ...                         | 1                     | 17.0                               | 0.46                                 | 3.58                          | 9.816                         | ...   | ...   | 2.93 | ...   | ...   | ...   |       |
| 04361318+5111355 | 154.350  | 2.580    | 9.861  | 9      | —   | —      | —    | —    | —        | —    | —      | —     | —                      | —          | —          | —    | —        | —          | —     | 13.246                             | ...                         | ...                         | -1                    | 16.6                               | 1.00                                 | 3.58                          | 9.572                         | ...   | ...   | 3.05 | ...   | ...   | ...   |       |
| 04361434+4500084 | 158.933  | -1.583   | 1.362  | 1      | —   | —      | —    | —    | —        | D1   | —      | —     | —                      | —          | —          | —    | —        | —          | —     | 11.640                             | 0.55                        | 1.61                        | 1                     | 24.8                               | 0.74                                 | 3.69                          | 11.133                        | 0.33  | 0.94  | 0.42 | 28.3  | 11.12 | 0.35  | 1.03  |
| 04361446+5111365 | 154.352  | 2.583    | 9.942  | 8      | —   | —      | —    | —    | —        | —    | —      | —     | —                      | —          | —          | —    | —        | —          | —     | 11.934                             | 1.37                        | ...                         | 1                     | 22.6                               | 0.68                                 | 3.58                          | 8.230                         | -0.28 | ...   | 3.08 | ...   | ...   | -0.09 | ...   |
| 04361587+5108075 | 154.397  | 2.547    | 5.266  | 9      | —   | —      | —    | —    | —        | —    | —      | —     | —                      | —          | —          | —    | —        | —          | —     | 11.794                             | 1.52                        | ...                         | 1                     | 27.0                               | 0.64                                 | 3.58                          | 9.832                         | 0.65  | ...   | 1.63 | ...   | ...   | 0.75  | ...   |
| 04362105+5112546 | 154.347  | 2.610    | 11.714 | 8      | —   | —      | —    | —    | —        | —    | —      | —     | —                      | —          | —          | —    | —        | —          | —     | 8.748                              | 1.07                        | 2.54                        | 1                     | 114.4                              | 0.62                                 | 3.58                          | 4.383                         | -0.87 | -3.28 | 3.63 | ...   | ...   | -0.64 | -2.50 |
| 04362160+5109006 | 154.397  | 2.568    | 6.413  | 9      | —   | —      | —    | —    | —        | —    | —      | —     | —                      | —          | —          | —    | —        | —          | —     | 13.004                             | 1.58                        | ...                         | -1                    | 19.4                               | 0.60                                 | 3.58                          | 10.615                        | 0.51  | ...   | 1.99 | ...   | ...   | 0.64  | ...   |
| 04363002+4426469 | 159.376  | -1.922   | 1.303  | 1      | —   | —      | —    | —    | —        | D1   | —      | —     | —                      | —          | —          | —    | —        | —          | —     | 11.471                             | 0.68                        | 1.79                        | 1                     | 37.4                               | 0.36                                 | 3.68                          | 10.986                        | 0.47  | 1.14  | 0.40 | 42.4  | 10.98 | 0.49  | 1.23  |
| 04363339+5112276 | 154.375  | 2.629    | 8.954  | 9      | —   | —      | —    | —    | —        | —    | —      | —     | —                      | —          | —          | —    | —        | —          | —     | 13.823                             | ...                         | ...                         | -1                    | 12.2                               | 1.00                                 | 3.58                          | 10.487                        | ...   | ...   | 2.77 | ...   | ...   | ...   | ...   |
| 04364790+5052576 | 154.641  | 2.439    | 11.949 | 8      | —   | —      | —    | —    | —        | —    | —      | —     | —                      | —          | —          | —    | —        | —          | —     | 8.874                              | 0.80                        | 1.53                        | 1                     | 171.6                              | 0.64                                 | 3.60                          | 4.422                         | -1.18 | -4.41 | 3.70 | ...   | ...   | -0.95 | -3.62 |
| 04365398+5536579 | 151.126  | 5.620    | 0.882  | 1      | —   | —      | —    | —    | —        | D2   | —      | —     | —                      | —          | —          | —    | —        | —          | —     | 10.856                             | 0.41                        | 1.29                        | 1                     | 45.2                               | 0.44                                 | 3.52                          | 10.527                        | 0.26  | 0.85  | 0.27 | 48.4  | 10.54 | 0.28  | 0.91  |
| 04370228+4356359 | 159.814  | -2.189   | 1.014  | 1      | —   | —      | —    | —    | —        | —    | —      | —     | —                      | —          | —          | —    | —        | —          | —     | 10.187                             | 0.39                        | 1.24                        | 1                     | 59.4                               | 0.42                                 | 3.70                          | 9.809                         | 0.23  | 0.74  | 0.31 | 64.9  | 9.81  | 0.25  | 0.81  |
| 04370607+4355349 | 159.834  | -2.192   | 1.004  | 1      | —   | —      | —    | —    | —        | D1   | —      | —     | —                      | —          | —          | —    | —        | —          | —     | 10.304                             | 0.49                        | 1.43                        | 1                     | 56.2                               | 0.46                                 | 3.70                          | 9.930                         | 0.32  | 0.93  | 0.31 | 60.7  | 9.95  | 0.34  | 0.99  |
| 04371089+5050421 | 154.710  | 2.459    | 6.037  | 9      | —   | —      | —    | —    | —        | —    | —      | —     | —                      | —          | —          | —    | —        | —          | —     | 13.294                             | 0.50                        | 1.31                        | -1                    | 13.6                               | 0.80                                 | 3.69                          | 11.045                        | -0.50 | -1.69 | 1.87 | ...   | ...   | -0.38 | -1.29 |
| 04372043+3534246 | 166.112  | -7.731   | 1.018  | 1      | —   | —      | —    | —    | —        | D2   | —      | —     | —                      | —          | —          | —    | —        | —          | —     | 11.441                             | 0.52                        | 1.59                        | 1                     | 31.6                               | 0.52                                 | 3.40                          | 11.062                        | 0.35  | 1.08  | 0.32 | 34.4  | 11.07 | 0.37  | 1.15  |
| 04372260+5559348 | 150.889  | 5.921    | 0.717  | 1      | —   | —      | —    | —    | —        | —    | —      | —     | —                      | —          | —          | —    | —        | —          | —     | 10.423                             | 0.38                        | 1.27                        | 1                     | 48.6                               | 0.98                                 | 3.54                          | 10.156                        | 0.26  | 0.91  | 0.22 | 51.0  | 10.17 | 0.28  | 0.96  |
| 04373506+5414339 | 152.219  | 4.776    | 1.067  | 1      | —   | —      | —    | —    | —        | D1   | —      | —     | —                      | —          | —          | —    | —        | —          | —     | 10.421                             | 0.31                        | 1.28                        | 1                     | 46.0                               | 0.96                                 | 3.56                          | 10.023                        | 0.14  | 0.75  | 0.33 | 50.1  | 10.04 | 0.16  | 0.82  |
| 04374087+5415389 | 152.215  | 4.799    | 1.066  | 1      | —   | —      | —    | —    | —        | D1   | —      | —     | —                      | —          | —          | —    | —        | —          | —     | 10.833                             | 0.49                        | 1.51                        | 1                     | 43.2                               | 0.38                                 | 3.56                          | 10.436                        | 0.31  | 0.98  | 0.33 | 47.2  | 10.45 | 0.33  | 1.05  |
| 04380428+6040123 | 147.414  | 9.086    | 0.722  | 1      | —   | —      | —    | —    | —        | D1   | —      | —     | —                      | —          | —          | —    | —        | —          | —     | 11.392                             | 0.51                        | 1.49                        | 1                     | 31.2                               | 0.48                                 | 3.41                          | 11.123                        | 0.39  | 1.13  | 0.22 | 33.0  | 11.13 | 0.40  | 1.18  |
| 04381542+4841393 | 156.425  | 1.149    | 1.465  | 1      | —   | —      | —    | —    | —        | D1   | —      | —     | —                      | —          | —          | —    | —        | —          | —     | 10.248                             | 0.53                        | 1.66                        | 1                     | 37.2                               | 0.84                                 | 3.66                          | 9.702                         | 0.29  | 0.94  | 0.45 | 41.9  | 9.73  | 0.31  | 1.03  |
| 04382270+4746546 | 157.118  | 0.554    | 1.548  | 1      | —   | —      | —    | —    | —        | D1   | —      | —     | —                      | —          | —          | —    | —        | —          | —     | 11.802                             | 0.49                        | 1.68                        | 1                     | 36.4                               | 0.50                                 | 3.63                          | 11.225                        | 0.23  | 0.91  | 0.48 | 44.3  | 11.13 | 0.26  | 1.01  |
| 04382564+5533056 | 151.319  | 5.738    | 0.829  | 1      | —   | —      | —    | —    | —        | D2   | —      | —     | —                      | —          | —          | —    | —        | —          | —     | 11.010                             | 0.45                        | 1.44                        | 1                     | 42.0                               | 0.66                                 | 3.51                          | 10.701                        | 0.32  | 1.03  | 0.26 | 44.9  | 10.71 | 0.33  | 1.09  |
| 04382833+4402136 | 159.916  | -1.934   | 0.959  | 1      | —   | —      | —    | —    | —        | D1   | —      | —     | —                      | —          | —          | —    | —        | —          | —     | 9.717                              | 0.39                        | 1.30                        | 1                     | 96.0                               | 0.90                                 | 3.62                          | 9.360                         | 0.23  | 0.82  | 0.30 | 103.6 | 9.37  | 0.25  | 0.88  |
| 04383342+5532126 | 151.342  | 5.742    | 0.837  | 1      | —   | —      | —    | —    | —        | D1   | c      | o     | o                      | —          | —          | —    | —        | —          | —     | 9.778                              | 0.42                        | 1.34                        | 1                     | 61.4                               | 0.80                                 | 3.51                          | 9.466                         | 0.28  | 0.93  | 0.26 | 65.3  | 9.48  | 0.30  | 0.98  |
| 04383916+5154076 | 154.076  | 3.336    | 1.330  | 1      | —   | —      | —    | —    | —        | D3   | —      | —     | —                      | —          | —          | —    | —        | —          | —     | 10.520                             | 0.40                        | 1.42                        | 1                     | 44.0                               | 0.98                                 | 3.63                          | 10.024                        | 0.18  | 0.76  | 0.41 | 49.3  | 10.04 | 0.21  | 0.85  |
| 04385827+3916506 | 163.536  | -5.030   | 0.890  | 1      | —   | —      | —    | —    | —        | D3   | —      | —     | —                      | —          | —          | —    | —        | —          | —     | 9.976                              | 0.36                        | 1.30                        | 1                     | 62.2                               | 0.96                                 |                               |                               |       |       |      |       |       |       |       |

| 2MSS J           |         | <i>l</i> | <i>b</i> | EBV | Object | Sample  | Disc | 2MRS | Velocity | NIR   | Photom | Ext | <i>K</i> <sub>20</sub> | <i>H-K</i> | <i>J-K</i> | vc  | <i>a</i> | <i>b/a</i> | st.d. | <i>K</i> <sub>0</sub> <sup>o</sup> | ( <i>H-K</i> ) <sup>o</sup> | ( <i>J-K</i> ) <sup>o</sup> | <i>A<sub>K</sub></i> | <i>a</i> <sup>d</sup> | <i>K</i> <sub>0</sub> <sup>o,d</sup> | ( <i>H-K</i> ) <sup>o,c</sup> | ( <i>J-K</i> ) <sup>o,c</sup> |        |      |      |      |      |       |      |      |      |     |      |      |     |      |     |      |     |      |
|------------------|---------|----------|----------|-----|--------|---------|------|------|----------|-------|--------|-----|------------------------|------------|------------|-----|----------|------------|-------|------------------------------------|-----------------------------|-----------------------------|----------------------|-----------------------|--------------------------------------|-------------------------------|-------------------------------|--------|------|------|------|------|-------|------|------|------|-----|------|------|-----|------|-----|------|-----|------|
| (1)              |         | deg      | deg      | mag | class  | off flg | gal  | TF   | obs      | ext'd | (type) | (8) | (9)                    | Opt        | HI         | flg | (11)     | (12)       | flg   | (13)                               | mag                         | (14)                        | mag                  | (15)                  | mag                                  | (16)                          | (17)                          | (18)   | (19) | (20) | mag  | (21) | mag   | (22) | mag  | (23) | mag | (24) | (25) | mag | (26) | mag | (27) | mag | (28) |
| 04425353+5114549 | 155.003 | 3.398    | 1.156    | 1   | —      | —       | g    | t    | N        | —     | D1     | —   | —                      | —          | —          | —   | U        | —          | —     | —                                  | 11.334                      | 0.46                        | 1.57                 | 1                     | 42.4                                 | 0.30                          | 3.62                          | 10.903 | 0.27 | 1.00 | 0.36 | 47.1 | 10.91 | 0.29 | 1.07 |      |     |      |      |     |      |     |      |     |      |
| 04425428+4039156 | 162.987 | −3.558   | 0.550    | 1   | —      | —       | g    | —    | —        | —     | D3     | —   | e                      | o          | —          | —   | U        | —          | —     | —                                  | 10.576                      | 0.38                        | 1.23                 | 1                     | 40.8                                 | 0.74                          | 3.58                          | 10.371 | 0.29 | 0.96 | 0.17 | 42.2 | 10.39 | 0.30 | 0.99 |      |     |      |      |     |      |     |      |     |      |
| 04430935+4425043 | 160.199 | −1.053   | 1.236    | 1   | —      | —       | g    | —    | N        | —     | D2     | —   | —                      | —          | —          | —   | U        | —          | —     | —                                  | 11.302                      | 0.48                        | 1.55                 | 1                     | 31.8                                 | 0.64                          | 3.67                          | 10.841 | 0.28 | 0.94 | 0.38 | 55.4 | 10.85 | 0.30 | 1.02 |      |     |      |      |     |      |     |      |     |      |
| 04431593+3850025 | 164.424 | −4.697   | 0.692    | 1   | —      | —       | g    | —    | N        | —     | D1     | —   | —                      | —          | —          | —   | U        | —          | —     | —                                  | 10.201                      | 0.37                        | 1.24                 | 1                     | 48.8                                 | 0.86                          | 3.58                          | 9.943  | 0.26 | 0.89 | 0.21 | 51.1 | 9.96  | 0.27 | 0.94 |      |     |      |      |     |      |     |      |     |      |
| 04431899+4032175 | 163.138 | −3.575   | 0.560    | 1   | —      | —       | g    | —    | N        | —     | D2     | —   | —                      | —          | —          | —   | U        | —          | —     | —                                  | 11.426                      | 0.56                        | 1.46                 | 1                     | 41.2                                 | 0.32                          | 3.65                          | 11.217 | 0.47 | 1.18 | 0.17 | 42.9 | 11.23 | 0.48 | 1.22 |      |     |      |      |     |      |     |      |     |      |
| 04433407+4536452 | 159.333 | −0.214   | 1.516    | 1   | —      | —       | g    | t    | N        | —     | D1     | —   | —                      | —          | —          | —   | U        | —          | —     | —                                  | 11.532                      | 0.44                        | 1.57                 | 1                     | 48.0                                 | 0.20                          | 3.63                          | 10.967 | 0.19 | 0.81 | 0.47 | 55.8 | 10.96 | 0.22 | 0.91 |      |     |      |      |     |      |     |      |     |      |
| 04433437+3812344 | 164.938 | −5.059   | 0.956    | 1   | —      | —       | g    | —    | —        | —     | D3     | —   | —                      | o          | —          | —   | U        | —          | —     | —                                  | 10.005                      | 0.39                        | 1.39                 | 1                     | 48.0                                 | 0.82                          | 3.47                          | 9.649  | 0.23 | 0.91 | 0.30 | 51.4 | 9.67  | 0.25 | 0.98 |      |     |      |      |     |      |     |      |     |      |
| 04434231+5529380 | 151.856 | 6.263    | 0.556    | 1   | —      | —       | g    | —    | —        | —     | D1     | c   | c                      | o          | —          | —   | U        | —          | —     | —                                  | 11.089                      | 0.34                        | 1.20                 | 1                     | 31.8                                 | 0.56                          | 3.51                          | 10.882 | 0.24 | 0.92 | 0.17 | 33.0 | 10.90 | 0.25 | 0.96 |      |     |      |      |     |      |     |      |     |      |
| 04434344+4007040 | 163.507 | −3.791   | 0.655    | 1   | —      | —       | g    | —    | —        | —     | D1     | e   | e                      | —          | —          | h   | U        | —          | —     | —                                  | 10.544                      | 0.43                        | 1.24                 | 1                     | 42.0                                 | 0.76                          | 3.54                          | 10.300 | 0.32 | 0.91 | 0.20 | 44.0 | 10.31 | 0.33 | 0.95 |      |     |      |      |     |      |     |      |     |      |
| 04440562+3853161 | 164.489 | −4.540   | 0.703    | 1   | —      | —       | g    | t    | N        | —     | D1     | —   | —                      | —          | —          | —   | U        | —          | —     | —                                  | 11.092                      | 0.42                        | 1.31                 | 1                     | 52.4                                 | 0.42                          | 3.57                          | 10.830 | 0.30 | 0.96 | 0.22 | 55.7 | 10.82 | 0.31 | 1.01 |      |     |      |      |     |      |     |      |     |      |
| 04441374+3911350 | 164.274 | −4.321   | 0.724    | 1   | —      | —       | g    | —    | N        | —     | D1     | —   | —                      | —          | —          | —   | U        | c          | —     | —                                  | 10.567                      | 0.36                        | 1.23                 | 1                     | 42.0                                 | 0.80                          | 3.56                          | 10.297 | 0.24 | 0.87 | 0.22 | 44.1 | 10.32 | 0.26 | 0.92 |      |     |      |      |     |      |     |      |     |      |
| 04441949+3750057 | 165.320 | −5.191   | 0.921    | 1   | —      | —       | g    | —    | —        | —     | D3     | c   | c                      | o          | —          | —   | U        | —          | —     | —                                  | 11.712                      | 0.31                        | 1.27                 | 1                     | 44.6                                 | 0.72                          | 3.57                          | 10.350 | 0.49 | 0.79 | 0.22 | 48.1 | 10.37 | 0.23 | 0.85 |      |     |      |      |     |      |     |      |     |      |
| 04442990+4429146 | 160.291 | −8.827   | 1.137    | 1   | —      | —       | g    | t    | N        | —     | D1     | —   | —                      | —          | —          | —   | U        | —          | —     | —                                  | 11.576                      | 0.42                        | 1.39                 | 1                     | 46.2                                 | 0.32                          | 3.68                          | 10.576 | 0.30 | 1.02 | 0.35 | 55.8 | 10.58 | 0.36 | 1.10 |      |     |      |      |     |      |     |      |     |      |
| 04443470+5252243 | 153.939 | 4.656    | 1.194    | 1   | —      | —       | g    | —    | —        | —     | D4     | —   | —                      | o          | —          | —   | U        | —          | —     | —                                  | 11.401                      | 0.47                        | 1.53                 | 1                     | 31.2                                 | 0.92                          | 3.59                          | 10.956 | 0.27 | 0.94 | 0.37 | 34.9 | 10.95 | 0.30 | 1.02 |      |     |      |      |     |      |     |      |     |      |
| 04445716+3231058 | 169.489 | −8.531   | 1.157    | 1   | —      | —       | g    | —    | N        | —     | D1     | e   | e                      | o          | —          | —   | U        | —          | —     | —                                  | 11.072                      | 0.43                        | 1.35                 | 1                     | 43.6                                 | 0.88                          | 3.37                          | 10.641 | 0.24 | 0.77 | 0.36 | 49.0 | 10.62 | 0.26 | 0.85 |      |     |      |      |     |      |     |      |     |      |
| 04445949+4533441 | 159.534 | −0.059   | 1.568    | 1   | —      | —       | g    | —    | N        | —     | D3     | —   | —                      | —          | —          | —   | U        | —          | —     | —                                  | 10.941                      | 0.54                        | 1.66                 | 1                     | 35.0                                 | 0.80                          | 3.63                          | 10.357 | 0.28 | 0.88 | 0.49 | 40.5 | 10.36 | 0.31 | 0.99 |      |     |      |      |     |      |     |      |     |      |
| 04450255+3758177 | 165.308 | −4.994   | 0.906    | 1   | —      | —       | g    | —    | N        | —     | D1     | —   | —                      | —          | —          | —   | U        | —          | —     | —                                  | 10.978                      | 0.41                        | 1.31                 | 1                     | 46.0                                 | 0.62                          | 3.50                          | 10.640 | 0.26 | 0.86 | 0.28 | 49.6 | 10.65 | 0.28 | 0.92 |      |     |      |      |     |      |     |      |     |      |
| 04451287+3246507 | 169.322 | −8.320   | 0.846    | 1   | —      | —       | g    | —    | —        | —     | D1     | c   | c                      | o          | —          | —   | U        | —          | —     | —                                  | 11.470                      | 0.51                        | 1.33                 | 1                     | 29.2                                 | 0.76                          | 3.44                          | 11.155 | 0.36 | 0.91 | 0.26 | 31.3 | 11.16 | 0.38 | 0.96 |      |     |      |      |     |      |     |      |     |      |
| 04451775+4049326 | 163.165 | −3.103   | 0.522    | 1   | —      | —       | g    | —    | N        | —     | D3     | —   | —                      | —          | —          | h?  | U        | —          | —     | —                                  | 10.446                      | 0.42                        | 1.32                 | 1                     | 50.6                                 | 0.60                          | 3.57                          | 10.252 | 0.33 | 1.06 | 0.16 | 52.3 | 10.27 | 0.34 | 1.01 |      |     |      |      |     |      |     |      |     |      |
| 04452433+4158496 | 162.300 | −2.336   | 1.341    | 8   | —      | —       | g    | —    | —        | —     | D2     | —   | —                      | —          | —          | —   | U        | —          | —     | —                                  | 10.714                      | 0.84                        | 1.75                 | 1                     | 68.2                                 | 0.64                          | 3.70                          | 10.214 | 0.62 | 1.08 | 0.42 | ...  | ...   | 0.65 | 1.17 |      |     |      |      |     |      |     |      |     |      |
| 04453613+5059042 | 155.482 | 3.548    | 1.116    | 1   | —      | —       | g    | —    | N        | —     | D2     | —   | —                      | —          | —          | —   | U        | —          | —     | —                                  | 11.069                      | 0.48                        | 1.55                 | 1                     | 37.0                                 | 0.54                          | 3.61                          | 10.653 | 0.29 | 0.99 | 0.35 | 40.6 | 10.67 | 0.31 | 1.07 |      |     |      |      |     |      |     |      |     |      |
| 04460579+3122510 | 170.531 | −9.073   | 1.189    | 9   | —      | —       | g    | —    | —        | —     | D1     | —   | e                      | g          | —          | —   | U        | —          | —     | —                                  | 7.740                       | 0.31                        | 1.19                 | 1                     | 130.8                                | 0.88                          | 3.69                          | 7.297  | 0.11 | 0.60 | 0.37 | ...  | ...   | 0.13 | 0.68 |      |     |      |      |     |      |     |      |     |      |
| 04461266+3725188 | 165.879 | −5.174   | 1.061    | 1   | —      | —       | g    | —    | N        | —     | D2     | —   | —                      | —          | —          | —   | U        | —          | —     | —                                  | 10.625                      | 0.49                        | 1.53                 | 1                     | 41.0                                 | 0.70                          | 3.45                          | 10.230 | 0.31 | 1.01 | 0.33 | 44.7 | 10.24 | 0.33 | 1.08 |      |     |      |      |     |      |     |      |     |      |
| 04461371+5510154 | 152.337 | 6.328    | 0.659    | 1   | —      | o       | —    | —    | —        | —     | D1     | e   | c                      | o          | —          | —   | U        | —          | o     | —                                  | 10.992                      | 0.37                        | 1.14                 | 1                     | 44.4                                 | 0.68                          | 3.57                          | 10.746 | 0.26 | 0.82 | 0.20 | 46.8 | 10.75 | 0.28 | 0.86 |      |     |      |      |     |      |     |      |     |      |
| 04463939+4540516 | 159.633 | 0.239    | 1.448    | 1   | —      | —       | g    | t    | N        | —     | D4     | —   | —                      | —          | —          | —   | U        | —          | —     | —                                  | 11.290                      | 0.51                        | 1.55                 | 1                     | 33.0                                 | 0.52                          | 3.66                          | 10.750 | 0.27 | 0.83 | 0.45 | 37.7 | 10.76 | 0.30 | 0.92 |      |     |      |      |     |      |     |      |     |      |
| 04464053+4400413 | 160.906 | −0.840   | 0.816    | 1   | —      | —       | g    | —    | —        | —     | D3     | e   | e                      | o          | —          | —   | U        | —          | —     | —                                  | 10.591                      | 0.40                        | 1.36                 | 1                     | 40.8                                 | 0.68                          | 3.74                          | 10.287 | 0.27 | 0.95 | 0.25 | 43.2 | 10.31 | 0.28 | 1.01 |      |     |      |      |     |      |     |      |     |      |
| 04464159+4943063 | 156.560 | 2.860    | 0.912    | 1   | —      | —       | g    | —    | N        | —     | D1     | —   | —                      | —          | —          | *   | U        | —          | —     | —                                  | 10.999                      | 0.41                        | 1.29                 | 1                     | 69.0                                 | 0.58                          | 3.68                          | 10.659 | 0.26 | 0.83 | 0.28 | 74.4 | 10.67 | 0.28 | 0.90 |      |     |      |      |     |      |     |      |     |      |
| 04464394+3435108 | 168.129 | −6.919   | 1.353    | 1   | —      | —       | g    | —    | N        | —     | D1     | e   | e                      | o          | —          | —   | U        | —          | —     | —                                  | 11.195                      | 0.37                        | 1.39                 | 1                     | 45.2                                 | 0.90                          | 3.46                          | 10.691 | 0.14 | 0.72 | 0.42 | 51.4 | 10.69 | 0.17 | 0.81 |      |     |      |      |     |      |     |      |     |      |
| 04465712+4729304 | 158.286 | 1.451    | 1.093    | 1   | —      | —       | g    | —    | N        | —     | D1     | —   | —                      | —          | —          | —   | U        | —          | —     | —                                  | 11.520                      | 0.46                        | 1.51                 | 1                     | 30.2                                 | 0.80                          | 3.70                          | 11.113 | 0.27 | 0.96 | 0.34 | 33.6 | 11.10 | 0.30 | 1.01 |      |     |      |      |     |      |     |      |     |      |
| 04471937+4417021 | 160.774 | −0.576   | 0.814    | 1   | —      | —       | g    | t    | N        | —     | D3     | —   | —                      | o          | —          | —   | U        | —          | —     | —                                  | 10.908                      | 0.49                        | 1.41                 | 1                     | 36.0                                 | 0.38                          | 3.67                          | 10.605 | 0.35 | 1.01 | 0.25 | 38.3 | 10.62 | 0.37 | 1.06 |      |     |      |      |     |      |     |      |     |      |
| 04472295+4013271 | 163.881 | −3.190   | 0.578    | 1   | —      | —       | g    | —    | N        | —     | D2     | —   | —                      | —          | —          | —   | U        | —          | —     | —                                  | 11.360                      | 0.38                        | 1.28                 | 1                     | 34.2                                 | 0.64                          | 3.58                          | 11.145 | 0.29 | 0.99 | 0.18 | 35.6 | 11.15 | 0.30 | 1.03 |      |     |      |      |     |      |     |      |     |      |
| 04472421+4459281 | 160.244 | −0.107   | 0.984    | 1   | —      | —       | g    | t    | N        | —     | D1     | —   | —                      | o          | —          | —   | U        | —          | —     | —                                  | 11.250                      | 0.42                        | 1.40                 | 1                     | 63.0                                 | 0.22                          | 3.69                          | 10.883 | 0.26 | 0.91 | 0.30 | 68.9 | 10.88 | 0.28 | 0.97 |      |     |      |      |     |      |     |      |     |      |
| 04472448+4854366 | 157.253 | 2.427    | 0.928    | 1   | —      | —       | g    | —    | —        | —     | D1     | —   | —                      | —          | —          | h   | U        | —          | —     | —                                  | 9.721                       | 0.40                        | 1.32                 | 1                     | 67.6                                 | 0.72                          | 3.74                          | 9.375  | 0.25 | 0.86 | 0.29 | 71.9 | 9.41  | 0.27 | 0.93 |      |     |      |      |     |      |     |      |     |      |
| 04473473+4529122 | 159.885 | 0.237    | 1.405    | 1   | —      | —       | g    | t    | N        | —     | D3     | —   | —                      | —          | —          | —   | U        | —          | —     | —                                  | 11.325                      | 0.44                        | 1.41                 | 1                     | 25.6                                 | 0.64                          | 3.61                          | 10.801 | 0.20 | 0.71 | 0.44 | 29.0 | 10.81 | 0.23 | 0.80 |      |     |      |      |     |      |     |      |     |      |
| 04474516+5559249 | 151.844 | 7.018    | 0.509    | 1   | —      | —       | g    | —    | —        | —     | D3     | c   | c                      | o          | —          | —   | U        | —          | —     | —                                  | 10.940                      | 0.37                        | 1.20                 | 1                     | 34.8                                 | 0.82                          | 3.57                          | 10.750 | 0.29 | 0.95 | 0.16 | 36.0 | 10.76 | 0.30 | 0.98 |      |     |      |      |     |      |     |      |     |      |
| 04475352+4432511 | 160.638 | −0.328   | 0.974    | 1   | —      | —       | g    | —    | N        | —     | D1     | —   | —                      | —          | —          | —   | U        | —          | —     | —                                  | 11.518                      | 0.35                        | 1.36                 | 1                     | 26.2                                 | 0.88                          | 3.66                          | 11.155 | 0.19 | 0.88 | 0.30 | 28.4 | 11.16 | 0.21 | 0.94 |      |     |      |      |     |      |     |      |     |      |
| 04475541+3428204 | 168.376 | −6.803   | 1.401    | 1   | —      | —       | g    | —    | N        | —     | D1     | e   | e                      | o          | —          | —   | U        | —          | —     | —                                  | 10.886                      | 0.45                        | 1.45                 | 1                     | 40.0                                 | 0.72                          | 3.41                          | 10.364 | 0.22 | 0.75 | 0.43 | 45.4 | 10.37 | 0.24 | 0.85 |      |     |      |      |     |      |     |      |     |      |
| 04481997+3436502 | 168.320 | −6.648   | 1.562    | 1   | —      | —       | g    | t    | N        | —     | D3     | —   | e                      | o          | —          | —   | U        | —          | —     | —                                  | 10.702                      | 0.54                        | 1.68                 | 1                     | 43.2                                 | 0.58                          | 3.46                          | 10.120 | 0.28 | 0.90 | 0.48 | 49.6 | 10.14 | 0.31 | 1.00 |      |     |      |      |     |      |     |      |     |      |
| 04482813+4952069 | 156.630 | 3.176    | 0.897    | 1   | —      | —       | g    | t    | N        | —     | D3     | —   | —                      | —          | —          | —   | U        | —          | —     | —                                  | 11.511                      | 0.43                        | 1.45                 | 1                     | 46.0                                 | 0.34                          | 3.68                          | 11.177 | 0.28 | 1.01 | 0.28 | 49.8 | 11.18 | 0.30 | 1.06 |      |     |      |      |     |      |     |      |     |      |
| 04483016+4459298 | 160.369 | 0.042    | 1.025    | 1   | —      | —       | g    | —    | —        | —     | D3     | e   | e                      | o          | —          | —   | U        | —          | —     | —                                  | 10.726                      | 0.44                        | 1.48                 | 1                     | 33.4                                 | 0.84                          | 3.71                          | 10.344 | 0.27 | 0.97 | 0.32 | 36.1 | 10.36 | 0.29 | 1.04 |      |     |      |      |     |      |     |      |     |      |

Table B1: a) continued.

| 2MAS J           | <i>l</i><br>deg<br>(2a) | <i>b</i><br>deg<br>(2b) | EBV<br>mag<br>(3) | Object<br>class<br>(4) | off<br>(5) | flg<br>(6) | gal<br>(7a) | TF<br>(7b) | obs<br>(7c) | ext'd<br>(7d) | type<br>(8) | 2MRS<br>(9) | Velocity<br>Opt<br>(10a) | HI<br>(10b) | NIR<br>flg<br>(11) | Photom<br>flg<br>(12) | Ext<br>flg<br>(13) | <i>K</i> <sub>20</sub><br>mag<br>(14) | <i>H-K</i><br>mag<br>(15) | <i>J-K</i><br>mag<br>(16) | vc<br>(17) | <i>a</i><br>" (18) | <i>b/a</i><br>(19) | std.d.<br>(20) | <i>K</i> <sub>S</sub> <sup>o</sup><br>mag<br>(21) | ( <i>H-K</i> ) <sup>o</sup><br>mag<br>(22) | ( <i>J-K</i> ) <sup>o</sup><br>mag<br>(23) | <i>A<sub>K</sub></i><br>mag<br>(24) | <i>a</i> <sup>d</sup><br>" (25) | <i>K</i> <sub>S</sub> <sup>o,d</sup><br>mag<br>(26) | ( <i>H-K</i> ) <sup>o,c</sup><br>mag<br>(27) | ( <i>J-K</i> ) <sup>o,c</sup><br>mag<br>(28) |
|------------------|-------------------------|-------------------------|-------------------|------------------------|------------|------------|-------------|------------|-------------|---------------|-------------|-------------|--------------------------|-------------|--------------------|-----------------------|--------------------|---------------------------------------|---------------------------|---------------------------|------------|--------------------|--------------------|----------------|---------------------------------------------------|--------------------------------------------|--------------------------------------------|-------------------------------------|---------------------------------|-----------------------------------------------------|----------------------------------------------|----------------------------------------------|
| 04522577+4934396 | 157.264                 | 3.483                   | 0.721             | 1                      | —          | —          | g           | —          | —           | —             | D4          | —           | —                        | —           | U                  | —                     | —                  | 11.373                                | 0.38                      | 1.20                      | 1          | 34.6               | 0.96               | 3.66           | 11.104                                            | 0.26                                       | 0.84                                       | 0.22                                | 36.6                            | 11.11                                               | 0.28                                         | 0.88                                         |
| 04523133+4927346 | 157.365                 | 3.420                   | 0.733             | 1                      | —          | —          | g           | t          | N           | —             | D1          | —           | —                        | —           | U                  | —                     | —                  | 11.407                                | 0.45                      | 1.35                      | 1          | 50.4               | 0.38               | 3.66           | 11.134                                            | 0.32                                       | 0.98                                       | 0.23                                | 53.7                            | 11.13                                               | 0.34                                         | 1.03                                         |
| 04523985+5203046 | 155.365                 | 5.075                   | 1.294             | 1                      | —          | o          | —           | —          | —           | —             | D2          | —           | —                        | —           | U                  | o                     | —                  | 11.696                                | 0.47                      | 1.41                      | 1          | 26.6               | 0.56               | 3.66           | 11.214                                            | 0.26                                       | 0.77                                       | 0.40                                | 30.3                            | 11.20                                               | 0.28                                         | 0.85                                         |
| 04524568+4501058 | 160.829                 | 0.638                   | 1.091             | 1                      | —          | —          | g           | —          | N           | —             | D1          | —           | —                        | —           | U                  | —                     | —                  | 11.696                                | 0.45                      | 1.52                      | 1          | 46.6               | 0.56               | 3.68           | 10.157                                            | 0.27                                       | 0.98                                       | 0.34                                | 50.9                            | 10.17                                               | 0.30                                         | 1.05                                         |
| 04524698+5135515 | 155.730                 | 4.803                   | 1.438             | 1                      | —          | —          | g           | t          | N           | —             | D1          | —           | —                        | —           | U                  | —                     | e                  | 11.364                                | 0.56                      | 1.71                      | 1          | 45.8               | 0.42               | 3.45           | 10.828                                            | 0.32                                       | 1.00                                       | 0.45                                | 53.9                            | 10.78                                               | 0.35                                         | 1.09                                         |
| 04525192+4441218 | 161.095                 | 0.443                   | 0.975             | 1                      | —          | —          | g           | t          | N           | —             | D1          | —           | —                        | —           | U                  | —                     | —                  | 11.318                                | 0.47                      | 1.49                      | 1          | 36.8               | 0.40               | 3.64           | 10.955                                            | 0.30                                       | 1.01                                       | 0.30                                | 39.9                            | 10.96                                               | 0.32                                         | 1.07                                         |
| 04525281+5204476 | 155.363                 | 5.119                   | 1.373             | 1                      | —          | —          | g           | —          | N           | —             | D3          | e           | o                        | —           | —                  | —                     | —                  | 10.570                                | 0.48                      | 1.53                      | 1          | 42.6               | 0.74               | 3.54           | 10.058                                            | 0.26                                       | 0.85                                       | 0.43                                | 48.1                            | 10.07                                               | 0.28                                         | 0.94                                         |
| 04525545+5156396 | 155.473                 | 5.039                   | 1.326             | 1                      | —          | —          | g           | t          | N           | —             | D1          | e           | o                        | —           | —                  | —                     | —                  | 11.649                                | 0.50                      | 1.53                      | 1          | 34.4               | 0.34               | 3.54           | 11.155                                            | 0.28                                       | 0.87                                       | 0.41                                | 39.1                            | 11.15                                               | 0.31                                         | 0.96                                         |
| 04525591+3438448 | 168.898                 | −5.896                  | 1.016             | 1                      | —          | —          | g           | t          | N           | —             | D3          | e           | o                        | —           | —                  | —                     | —                  | 11.219                                | 0.39                      | 1.37                      | 1          | 38.0               | 0.50               | 3.37           | 10.840                                            | 0.22                                       | 0.87                                       | 0.31                                | 41.8                            | 10.83                                               | 0.24                                         | 0.93                                         |
| 04531024+3423105 | 169.133                 | −6.021                  | 0.969             | 1                      | —          | o          | —           | —          | —           | —             | D3          | cf          | —                        | h           | —                  | fo                    | —                  | 10.426                                | 0.46                      | 1.48                      | 1          | 84.6               | 0.20               | 3.50           | 10.065                                            | 0.30                                       | 1.00                                       | 0.30                                | 93.0                            | 10.05                                               | 0.32                                         | 1.06                                         |
| 04531459+4402256 | 161.640                 | 0.085                   | 0.702             | 1                      | —          | —          | g           | —          | N           | —             | D1          | e           | o                        | —           | —                  | —                     | —                  | 10.587                                | 0.50                      | 1.43                      | 1          | 47.6               | 0.56               | 3.69           | 10.325                                            | 0.38                                       | 1.08                                       | 0.22                                | 50.1                            | 10.34                                               | 0.40                                         | 1.12                                         |
| 04532075+4603176 | 160.091                 | 1.373                   | 1.020             | 1                      | —          | —          | g           | t          | N           | —             | D3          | —           | —                        | —           | —                  | —                     | —                  | 11.152                                | 0.38                      | 1.28                      | 1          | 38.8               | 0.36               | 3.69           | 10.772                                            | 0.22                                       | 0.77                                       | 0.32                                | 42.2                            | 10.78                                               | 0.24                                         | 0.84                                         |
| 04532441+4511276 | 160.768                 | 0.835                   | 1.127             | 1                      | —          | —          | g           | —          | N           | —             | D3          | —           | —                        | —           | —                  | —                     | —                  | 11.223                                | 0.51                      | 1.38                      | 1          | 34.0               | 0.58               | 3.68           | 10.797                                            | 0.32                                       | 0.88                                       | 0.35                                | 37.4                            | 10.78                                               | 0.25                                         | 0.85                                         |
| 04532674+4419006 | 161.449                 | 0.288                   | 0.811             | 1                      | —          | —          | g           | —          | N           | —             | D4          | —           | —                        | —           | —                  | —                     | —                  | 10.773                                | 0.40                      | 1.31                      | 1          | 35.6               | 0.98               | 3.63           | 10.471                                            | 0.27                                       | 0.90                                       | 0.25                                | 37.9                            | 10.48                                               | 0.28                                         | 0.96                                         |
| 04532922+4152201 | 163.348                 | −1.252                  | 0.721             | 1                      | —          | —          | g           | t          | N           | —             | D1          | —           | —                        | —           | —                  | —                     | —                  | 11.477                                | 0.39                      | 1.28                      | 1          | 38.6               | 0.30               | 3.67           | 11.208                                            | 0.27                                       | 0.92                                       | 0.22                                | 40.7                            | 11.22                                               | 0.28                                         | 0.97                                         |
| 04533259+4532326 | 160.510                 | 1.076                   | 1.150             | 1                      | —          | —          | g           | —          | N           | —             | D1          | —           | —                        | —           | —                  | —                     | —                  | 11.449                                | 0.49                      | 1.50                      | 1          | 26.4               | 0.72               | 3.66           | 11.021                                            | 0.30                                       | 0.93                                       | 0.36                                | 29.3                            | 11.02                                               | 0.32                                         | 1.01                                         |
| 04534624+4507475 | 160.855                 | 0.846                   | 1.111             | 1                      | —          | —          | g           | —          | N           | —             | D1          | —           | —                        | —           | —                  | —                     | —                  | 11.354                                | 0.48                      | 1.49                      | 1          | 39.4               | 0.64               | 3.68           | 10.940                                            | 0.30                                       | 0.94                                       | 0.34                                | 43.9                            | 10.93                                               | 0.32                                         | 1.01                                         |
| 04534877+4218445 | 163.045                 | −0.927                  | 0.665             | 1                      | —          | —          | g           | —          | N           | —             | D1          | —           | o                        | *           | —                  | —                     | —                  | 10.756                                | 0.49                      | 1.46                      | 1          | 62.2               | 0.32               | 3.67           | 10.508                                            | 0.38                                       | 1.12                                       | 0.21                                | 65.6                            | 10.51                                               | 0.39                                         | 1.17                                         |
| 04541186+4127583 | 163.747                 | −1.406                  | 0.773             | 1                      | —          | —          | g           | —          | N           | —             | D4          | —           | —                        | —           | —                  | —                     | —                  | 11.170                                | 0.44                      | 1.44                      | 1          | 34.0               | 0.52               | 3.68           | 10.882                                            | 0.31                                       | 1.05                                       | 0.24                                | 36.0                            | 10.90                                               | 0.33                                         | 1.11                                         |
| 04541490+4503149 | 160.967                 | 0.864                   | 1.080             | 1                      | —          | —          | g           | —          | N           | —             | D1          | —           | —                        | —           | —                  | —                     | —                  | 10.869                                | 0.56                      | 1.43                      | 1          | 51.4               | 0.80               | 3.67           | 10.467                                            | 0.38                                       | 0.89                                       | 0.33                                | 57.0                            | 10.46                                               | 0.40                                         | 0.96                                         |
| 04542558+5203496 | 155.526                 | 5.294                   | 1.617             | 1                      | —          | —          | g           | —          | N           | —             | D3          | —           | —                        | —           | —                  | —                     | —                  | 10.961                                | ...                       | 1.50                      | 1          | 28.6               | 1.00               | 3.52           | 10.359                                            | ...                                        | 0.69                                       | 0.50                                | 33.1                            | 10.37                                               | ...                                          | 0.80                                         |
| 04543180+5240066 | 155.062                 | 5.684                   | 0.947             | 1                      | —          | —          | g           | t          | N           | —             | D1          | c           | o                        | —           | —                  | —                     | —                  | 11.093                                | 0.48                      | 1.52                      | 1          | 45.8               | 0.34               | 3.54           | 10.740                                            | 0.32                                       | 1.05                                       | 0.29                                | 49.4                            | 10.75                                               | 0.34                                         | 1.12                                         |
| 04544599+4620599 | 160.017                 | 1.750                   | 1.008             | 1                      | —          | —          | g           | —          | N           | —             | D1          | —           | —                        | —           | —                  | —                     | —                  | 10.814                                | 0.50                      | 1.70                      | 1          | 48.2               | 0.52               | 3.67           | 10.438                                            | 0.34                                       | 1.20                                       | 0.31                                | 52.5                            | 10.45                                               | 0.36                                         | 1.27                                         |
| 04550178+5159483 | 155.636                 | 5.324                   | 1.671             | 1                      | —          | —          | g           | t          | N           | —             | D1          | —           | —                        | —           | —                  | —                     | —                  | 11.667                                | 0.54                      | 1.79                      | 1          | 38.0               | 0.68               | 3.54           | 11.044                                            | 0.27                                       | 0.96                                       | 0.52                                | 46.0                            | 10.99                                               | 0.30                                         | 1.07                                         |
| 04550702+4559478 | 160.331                 | 1.575                   | 1.016             | 1                      | —          | —          | g           | t          | N           | —             | D3          | —           | —                        | —           | —                  | —                     | —                  | 10.910                                | 0.39                      | 1.40                      | 1          | 42.8               | 0.40               | 3.66           | 10.531                                            | 0.22                                       | 0.89                                       | 0.31                                | 46.4                            | 10.55                                               | 0.24                                         | 0.96                                         |
| 04550828+5116514 | 156.208                 | 4.890                   | 1.216             | 1                      | —          | —          | g           | —          | N           | —             | D1          | e           | o                        | —           | —                  | —                     | —                  | 11.099                                | 0.54                      | 1.54                      | 1          | 39.0               | 0.52               | 3.59           | 10.646                                            | 0.33                                       | 0.93                                       | 0.38                                | 43.4                            | 10.65                                               | 0.36                                         | 1.01                                         |
| 04552286+4546214 | 160.534                 | 1.470                   | 0.991             | 1                      | —          | —          | g           | —          | N           | —             | D2          | —           | —                        | —           | —                  | —                     | —                  | 10.927                                | 0.56                      | 1.66                      | 1          | 45.4               | 0.66               | 3.58           | 10.558                                            | 0.40                                       | 1.17                                       | 0.31                                | 49.4                            | 10.56                                               | 0.42                                         | 1.23                                         |
| 04553812+5218515 | 155.445                 | 5.595                   | 1.038             | 1                      | —          | —          | g           | t          | N           | —             | D2          | e           | o                        | —           | —                  | —                     | —                  | 11.531                                | 0.41                      | 1.39                      | 1          | 31.2               | 0.42               | 3.57           | 11.144                                            | 0.24                                       | 0.88                                       | 0.32                                | 34.4                            | 11.15                                               | 0.26                                         | 0.95                                         |
| 04554245+4402134 | 161.922                 | 0.426                   | 0.816             | 1                      | —          | —          | g           | t          | N           | —             | D1          | —           | —                        | —           | —                  | —                     | —                  | 10.068                                | 0.40                      | 1.35                      | 1          | 69.4               | 0.36               | 3.68           | 9.764                                             | 0.27                                       | 0.94                                       | 0.25                                | 73.7                            | 9.78                                                | 0.29                                         | 1.00                                         |
| 04554990+4533540 | 160.745                 | 1.401                   | 1.031             | 1                      | —          | —          | g           | —          | N           | —             | D1          | —           | —                        | —           | —                  | —                     | —                  | 10.005                                | 0.38                      | 1.36                      | 1          | 61.2               | 0.52               | 3.67           | 9.621                                             | 0.21                                       | 0.84                                       | 0.32                                | 65.8                            | 9.65                                                | 0.23                                         | 0.91                                         |
| 04555788+5113029 | 156.339                 | 4.952                   | 1.309             | 1                      | —          | —          | g           | —          | N           | —             | D4          | e           | o                        | —           | —                  | —                     | —                  | 11.072                                | 0.44                      | 1.45                      | 1          | 28.6               | 0.90               | 3.57           | 10.584                                            | 0.22                                       | 0.80                                       | 0.41                                | 32.1                            | 10.60                                               | 0.25                                         | 0.89                                         |
| 04560341+4722562 | 159.351                 | 2.569                   | 1.435             | 9                      | —          | —          | g           | —          | —           | —             | —           | —           | —                        | —           | —                  | —                     | —                  | 9.904                                 | 0.76                      | 1.78                      | 1          | 82.6               | 0.28               | 3.75           | 8.282                                             | 0.04                                       | −0.39                                      | 1.35                                | ...                             | ...                                                 | −0.10                                        | ...                                          |
| 04561445+5706387 | 151.703                 | 8.632                   | 0.722             | 1                      | —          | —          | g           | t          | —           | —             | D3          | c           | —                        | —           | —                  | —                     | —                  | 11.156                                | 0.44                      | 1.27                      | 1          | 40.0               | 0.52               | 3.44           | 10.887                                            | 0.32                                       | 0.91                                       | 0.22                                | 42.2                            | 10.90                                               | 0.33                                         | 0.96                                         |
| 04561481+3003078 | 172.961                 | −8.206                  | 0.536             | 1                      | —          | —          | g           | t          | —           | —             | D1          | c           | —                        | h           | —                  | —                     | —                  | 9.606                                 | 0.35                      | 1.20                      | 1          | 88.8               | 0.46               | 3.43           | 9.406                                             | 0.26                                       | 0.93                                       | 0.17                                | 92.1                            | 9.42                                                | 0.27                                         | 0.97                                         |
| 04562691+4555425 | 160.529                 | 1.713                   | 1.035             | 1                      | —          | —          | g           | t          | N           | —             | D1          | —           | —                        | —           | —                  | —                     | —                  | 10.208                                | 0.45                      | 1.51                      | 1          | 73.0               | 0.44               | 3.70           | 9.822                                             | 0.28                                       | 0.99                                       | 0.32                                | 80.1                            | 9.82                                                | 0.30                                         | 1.06                                         |
| 04563241+4534186 | 160.817                 | 1.502                   | 1.099             | 1                      | —          | —          | g           | —          | N           | —             | D2          | —           | —                        | —           | —                  | —                     | —                  | 10.407                                | 0.43                      | 1.47                      | 1          | 45.0               | 0.90               | 3.64           | 9.998                                             | 0.25                                       | 0.92                                       | 0.34                                | 49.3                            | 10.01                                               | 0.27                                         | 1.00                                         |
| 04563494+3723521 | 167.208                 | −3.597                  | 0.851             | 1                      | —          | —          | g           | t          | N           | —             | D1          | —           | —                        | *           | —                  | —                     | —                  | 11.549                                | 0.51                      | 1.45                      | 1          | 38.8               | 0.30               | 3.55           | 11.232                                            | 0.37                                       | 1.02                                       | 0.26                                | 41.8                            | 11.23                                               | 0.38                                         | 1.08                                         |
| 04564373+4424037 | 161.752                 | 0.797                   | 0.897             | 1                      | —          | —          | g           | —          | N           | —             | D1          | —           | —                        | —           | —                  | —                     | —                  | 11.517                                | 0.49                      | 1.43                      | 1          | 31.8               | 0.76               | 3.73           | 11.183                                            | 0.35                                       | 0.99                                       | 0.28                                | 34.6                            | 11.17                                               | 0.36                                         | 1.05                                         |
| 04565520+3757166 | 166.814                 | −3.198                  | 1.980             | 8                      | —          | —          | g           | —          | —           | —             | —           | —           | g                        | —           | —                  | —                     | —                  | 10.881                                | 0.72                      | 1.71                      | 1          | 51.4               | 0.56               | 3.61           | 10.143                                            | 0.39                                       | 0.73                                       | 0.61                                | ...                             | ...                                                 | 0.43                                         | 0.86                                         |
| 04565773+4426507 | 161.742                 | 0.858                   | 0.913             | 1                      | —          | —          | g           | —          | N           | —             | D3          | —           | —                        | —           | —                  | —                     | —                  | 11.045                                | 0.45                      | 1.45                      | 1          | 34.2               | 0.82               | 3.73           | 10.705                                            | 0.30                                       | 1.00                                       | 0.28                                | 36.9                            | 10.71                                               | 0.32                                         | 1.06                                         |
| 04570846+4942147 | 157.645                 | 4.157                   | 0.893             | 1                      | —          | —          | g           | t          | N           | —             | D1          | —           | —                        | —           | —                  | —                     | —                  | 11.113                                | 0.37                      | 1.06                      | 1          | 36.2               | 0.38               | 3.61           | 10.780                                            | 0.22                                       | 0.62                                       | 0.28                                | 38.6                            | 10.80                                               | 0.24                                         | 0.68                                         |
| 04571144+4420115 | 161.854                 | 0.821                   | 0.880             | 1                      | —          | —          | g           | t          | N           | —             | D1          | —           | —                        | —           | —                  | —                     | —                  | 11.446                                | 0.37                      | 1.38                      | 1          | 33.2               | 0.36               | 3.57           | 11.118                                            | 0.22                                       | 0.94                                       | 0.27                                | 35.7                            | 11.13                                               | 0.24                                         | 1.00                                         |
| 04574655+4126307 | 164.186                 | −0.898                  | 0.832             | 1                      | —          | —          | g           | —          | N           | —             | D1          | —           | —                        | —           | —                  | —                     | —                  | 11.387                                | 0.49                      | 1.39                      | 1          | 32.2               | 0.54               | 3.67           | 11.077                                            | 0.35                                       | 0.98                                       | 0.26                                |                                 |                                                     |                                              |                                              |

Table B1: a) continued.

| 2MASX J          | <i>l</i>    | <i>b</i>    | EBV        | Object       | Sample     | Disc       | 2MRS        | Velocity   | NIR         | Photom        | Ext         | <i>K</i> <sub>20</sub> | <i>H-K</i>   | <i>J-K</i>  | vc          | <i>a</i>    | <i>b/a</i>  | st.d. | <i>K</i> <sub>s</sub> <sup>o</sup> | ( <i>H-K</i> ) <sup>o</sup> | ( <i>J-K</i> ) <sup>o</sup> | <i>A</i> <sub>K</sub> | <i>a</i> <sub>d</sub> <sup>o</sup> | <i>K</i> <sub>s</sub> <sup>o,d</sup> | ( <i>H-K</i> ) <sup>o,c</sup> | ( <i>J-K</i> ) <sup>o,c</sup> |             |             |      |             |             |             |       |
|------------------|-------------|-------------|------------|--------------|------------|------------|-------------|------------|-------------|---------------|-------------|------------------------|--------------|-------------|-------------|-------------|-------------|-------|------------------------------------|-----------------------------|-----------------------------|-----------------------|------------------------------------|--------------------------------------|-------------------------------|-------------------------------|-------------|-------------|------|-------------|-------------|-------------|-------|
| (1)              | deg<br>(2a) | deg<br>(2b) | mag<br>(3) | class<br>(4) | off<br>(5) | flg<br>(6) | gal<br>(7a) | TF<br>(7b) | obs<br>(7c) | ext'd<br>(7d) | type<br>(8) | (9)                    | Opt<br>(10a) | HI<br>(10b) | flg<br>(11) | flg<br>(12) | flg<br>(13) | (14)  | mag<br>(15)                        | mag<br>(16)                 | (17)                        | (18)                  | (19)                               | (20)                                 | mag<br>(21)                   | mag<br>(22)                   | mag<br>(23) | mag<br>(24) | (25) | mag<br>(26) | mag<br>(27) | mag<br>(28) |       |
| 05035780+5113351 | 157.103     | 5.947       | 0.759      | 1            | —          | —          | g           | —          | —           | —             | D1          | c                      | —            | h           | —           | —           | e           | —     | 10.829                             | 0.49                        | 1.50                        | 1                     | 46.2                               | 0.58                                 | 3.51                          | 10.546                        | 0.37        | 1.12        | 0.24 | 49.4        | 10.54       | 0.38        | 1.17  |
| 05040845+3140333 | 172.703     | -5.874      | 0.803      | 1            | —          | —          | —           | —          | —           | —             | D1          | c                      | o            | *           | —           | —           | —           | —     | 10.388                             | 0.37                        | 1.29                        | 1                     | 66.4                               | 0.74                                 | 3.50                          | 10.089                        | 0.24        | 0.90        | 0.25 | 71.0        | 10.09       | 0.26        | 0.95  |
| 05043136+3731335 | 168.077     | -2.276      | 0.952      | 1            | —          | —          | —           | —          | —           | —             | D1          | c                      | o            | *           | —           | —           | —           | —     | 10.662                             | 0.47                        | 1.38                        | 1                     | 56.6                               | 0.52                                 | 3.65                          | 10.307                        | 0.31        | 0.91        | 0.29 | 61.7        | 10.30       | 0.33        | 0.97  |
| 05050082+2717264 | 176.358     | -8.346      | 0.762      | 1            | —          | —          | —           | —          | —           | —             | D1          | c                      | o            | —           | —           | —           | —           | —     | 11.460                             | 0.45                        | 1.39                        | 1                     | 41.0                               | 0.38                                 | 3.44                          | 11.176                        | 0.33        | 1.01        | 0.24 | 43.7        | 11.18       | 0.34        | 1.06  |
| 05053566+3400344 | 171.016     | -4.226      | 0.617      | 1            | —          | —          | —           | —          | —           | —             | D1          | c                      | o            | h           | —           | —           | —           | —     | 11.329                             | 0.38                        | 1.17                        | 1                     | 46.2                               | 0.84                                 | 3.60                          | 11.099                        | 0.28        | 0.86        | 0.19 | 48.6        | 11.10       | 0.29        | 0.90  |
| 05053748+3230575 | 172.218     | -5.118      | 0.790      | 1            | —          | —          | —           | —          | —           | —             | D1          | c                      | o            | —           | —           | —           | —           | —     | 10.944                             | 0.37                        | 1.31                        | 1                     | 39.2                               | 0.78                                 | 3.49                          | 10.650                        | 0.24        | 0.92        | 0.24 | 41.6        | 10.66       | 0.25        | 0.97  |
| 05055384+4121469 | 165.181     | 0.257       | 0.552      | 1            | —          | —          | t           | —          | N           | —             | D1          | c                      | o            | —           | —           | —           | —           | —     | 11.403                             | 0.38                        | 1.34                        | 1                     | 49.0                               | 0.40                                 | 3.71                          | 11.197                        | 0.29        | 1.06        | 0.17 | 51.2        | 11.20       | 0.30        | 1.10  |
| 05060225+5149180 | 156.818     | 6.562       | 0.626      | 1            | —          | —          | —           | —          | —           | —             | D1          | c                      | o            | —           | —           | —           | —           | —     | 11.441                             | 0.41                        | 1.35                        | 1                     | 26.6                               | 0.88                                 | 3.51                          | 11.208                        | 0.30        | 1.04        | 0.19 | 27.8        | 11.22       | 0.31        | 1.08  |
| 05062070+5050310 | 157.638     | 6.016       | 0.632      | 1            | —          | —          | t           | —          | —           | —             | D1          | c                      | o            | —           | —           | —           | —           | —     | 10.844                             | 0.48                        | 1.57                        | 1                     | 56.6                               | 0.24                                 | 3.53                          | 10.609                        | 0.38        | 1.26        | 0.20 | 59.2        | 10.62       | 0.39        | 1.30  |
| 05062450+3535105 | 169.854     | -3.144      | 0.706      | 1            | —          | —          | —           | —          | N           | —             | D1          | c                      | o            | —           | —           | —           | —           | —     | 11.396                             | 0.42                        | 1.35                        | 1                     | 32.8                               | 0.64                                 | 3.57                          | 11.133                        | 0.31        | 1.00        | 0.22 | 34.7        | 11.14       | 0.32        | 1.04  |
| 05062761+2805178 | 175.902     | -7.615      | 0.889      | 1            | —          | —          | —           | —          | —           | —             | D1          | c                      | o            | h           | —           | —           | —           | —     | 11.482                             | 0.43                        | 1.38                        | 1                     | 27.6                               | 0.70                                 | 3.52                          | 11.151                        | 0.29        | 0.94        | 0.28 | 29.8        | 11.15       | 0.30        | 1.00  |
| 05063010+4512499 | 162.173     | 2.665       | 1.052      | 1            | —          | —          | —           | —          | N           | —             | D1          | c                      | o            | —           | —           | —           | —           | —     | 11.554                             | 0.43                        | 1.46                        | 1                     | 29.4                               | 0.54                                 | 3.63                          | 11.162                        | 0.26        | 0.94        | 0.33 | 32.4        | 11.16       | 0.28        | 1.01  |
| 05063335+4417469 | 162.913     | 2.121       | 0.822      | 1            | —          | —          | t           | —          | N           | —             | D1          | c                      | o            | —           | —           | —           | —           | —     | 11.260                             | 0.45                        | 1.41                        | 1                     | 40.0                               | 0.36                                 | 3.63                          | 10.954                        | 0.32        | 1.00        | 0.25 | 42.8        | 10.96       | 0.33        | 1.05  |
| 05064627+2512511 | 178.289     | -9.255      | 0.768      | 1            | —          | —          | —           | —          | —           | —             | D1          | c                      | o            | h           | —           | —           | —           | —     | 11.534                             | 0.46                        | 1.15                        | 1                     | 44.2                               | 0.60                                 | 3.42                          | 11.248                        | 0.34        | 0.77        | 0.24 | 47.7        | 11.22       | 0.35        | 0.82  |
| 05065081+5021579 | 158.070     | 5.796       | 0.590      | 1            | —          | —          | —           | —          | —           | —             | D1          | c                      | o            | —           | —           | —           | —           | —     | 10.786                             | 0.35                        | 1.18                        | 1                     | 39.0                               | 0.62                                 | 3.54                          | 10.566                        | 0.26        | 0.89        | 0.18 | 40.5        | 10.58       | 0.27        | 0.93  |
| 05072947+4723396 | 160.527     | 4.108       | 0.607      | 1            | —          | —          | —           | —          | N           | —             | D2          | —                      | —            | —           | —           | —           | —           | —     | 11.437                             | 0.51                        | 1.53                        | 1                     | 34.8                               | 0.78                                 | 3.63                          | 11.211                        | 0.41        | 1.23        | 0.19 | 36.5        | 11.22       | 0.42        | 1.27  |
| 05082986+4420513 | 163.080     | 2.429       | 0.743      | 1            | —          | —          | —           | —          | —           | —             | D1          | e                      | o            | h           | —           | —           | e           | —     | 9.295                              | 0.40                        | 1.29                        | 1                     | 88.8                               | 0.68                                 | 3.64                          | 9.018                         | 0.27        | 0.92        | 0.23 | 93.2        | 9.04        | 0.29        | 0.97  |
| 05084540+3116199 | 173.619     | -5.326      | 0.700      | 1            | —          | —          | —           | —          | —           | —             | D2          | —                      | —            | —           | —           | —           | —           | —     | 10.105                             | 0.33                        | 1.22                        | 1                     | 59.8                               | 0.90                                 | 3.53                          | 9.844                         | 0.21        | 0.87        | 0.22 | 62.7        | 9.86        | 0.23        | 0.92  |
| 05084571+3116380 | 173.615     | -5.322      | 0.702      | 9            | e          | —          | —           | —          | —           | —             | cr          | —                      | —            | h           | —           | o           | —           | —     | 10.319                             | 0.36                        | 1.24                        | -2                    | 63.0                               | 0.44                                 | 3.52                          | 10.057                        | 0.25        | 0.89        | 0.22 | ...         | ...         | 0.26        | 0.94  |
| 05092334+5218430 | 156.727     | 7.267       | 0.486      | 1            | —          | —          | t           | —          | —           | —             | D1          | c                      | o            | *           | —           | —           | —           | —     | 10.970                             | 0.35                        | 1.15                        | 1                     | 57.8                               | 0.32                                 | 3.53                          | 10.789                        | 0.27        | 0.91        | 0.15 | 59.8        | 10.80       | 0.28        | 0.94  |
| 05095533+4436308 | 163.021     | 2.789       | 0.677      | 1            | —          | —          | —           | —          | N           | —             | D1          | c                      | o            | —           | —           | —           | —           | —     | 10.878                             | 0.43                        | 1.27                        | 1                     | 53.6                               | 0.34                                 | 3.66                          | 10.626                        | 0.32        | 0.94        | 0.21 | 56.6        | 10.63       | 0.33        | 0.98  |
| 05101563+4039582 | 166.232     | 0.499       | 0.531      | 7            | —          | —          | —           | —          | —           | —             | D1          | c                      | o            | —           | —           | —           | —           | —     | 10.684                             | 0.65                        | 1.40                        | 1                     | 57.4                               | 0.60                                 | 3.69                          | 10.486                        | 0.56        | 1.14        | 0.16 | ...         | ...         | 0.57        | 1.17  |
| 05104461+5045270 | 158.120     | 6.527       | 0.395      | 1            | —          | —          | —           | —          | —           | —             | D1          | c                      | o            | —           | —           | —           | —           | —     | 11.187                             | 0.37                        | 1.07                        | 1                     | 42.6                               | 0.68                                 | 3.59                          | 11.040                        | 0.30        | 0.87        | 0.12 | 43.6        | 11.05       | 0.31        | 0.90  |
| 05105986+3759269 | 168.471     | -0.973      | 4.279      | 8            | —          | —          | —           | —          | —           | —             | —           | —                      | —            | —           | —           | —           | —           | —     | 9.229                              | 0.78                        | 1.51                        | 1                     | 136.4                              | 0.78                                 | 3.68                          | 7.635                         | 0.07        | -0.62       | 1.33 | ...         | ...         | 0.15        | -0.34 |
| 05111982+5132030 | 157.539     | 7.055       | 0.356      | 1            | —          | —          | —           | —          | —           | —             | D1          | c                      | o            | —           | —           | —           | —           | —     | 11.245                             | 0.40                        | 1.17                        | 1                     | 43.6                               | 0.58                                 | 3.48                          | 11.112                        | 0.35        | 0.99        | 0.11 | 44.7        | 11.11       | 0.35        | 1.01  |
| 05112466+2709083 | 177.315     | -7.277      | 0.943      | 1            | —          | —          | —           | —          | —           | —             | D4          | c                      | o            | —           | —           | —           | —           | —     | 11.441                             | 0.50                        | 1.48                        | 1                     | 33.2                               | 0.74                                 | 3.51                          | 11.090                        | 0.35        | 1.01        | 0.29 | 36.1        | 11.09       | 0.36        | 1.07  |
| 05112587+2445183 | 179.290     | -8.664      | 0.488      | 1            | —          | —          | t           | —          | —           | —             | D1          | c                      | o            | h           | —           | —           | —           | —     | 11.026                             | 0.48                        | 1.34                        | 1                     | 31.0                               | 0.48                                 | 3.37                          | 10.844                        | 0.40        | 1.10        | 0.15 | 31.9        | 10.86       | 0.41        | 1.13  |
| 05112697+3752378 | 168.616     | -0.968      | 1.902      | 8            | —          | —          | —           | —          | —           | —             | D1          | c                      | o            | —           | —           | —           | —           | —     | 11.240                             | 1.08                        | 2.21                        | -2                    | 31.2                               | 0.70                                 | 3.65                          | 10.531                        | 0.76        | 1.27        | 0.59 | ...         | ...         | 0.80        | 1.39  |
| 05114743+5359159 | 155.563     | 8.536       | 0.476      | 1            | —          | —          | —           | —          | —           | —             | D1          | c                      | o            | —           | —           | —           | —           | —     | 11.081                             | 0.42                        | 1.17                        | 1                     | 41.4                               | 0.74                                 | 3.47                          | 10.904                        | 0.34        | 0.93        | 0.15 | 42.8        | 10.91       | 0.35        | 0.96  |
| 05115105+3131317 | 173.804     | -4.643      | 0.666      | 1            | —          | —          | t           | —          | N           | —             | D2          | —                      | —            | —           | —           | —           | —           | —     | 10.859                             | 0.36                        | 1.22                        | 1                     | 37.0                               | 0.46                                 | 3.55                          | 10.611                        | 0.25        | 0.89        | 0.21 | 38.7        | 10.63       | 0.27        | 0.93  |
| 05115386+4537142 | 162.409     | 3.668       | 0.555      | 1            | —          | —          | —           | —          | —           | —             | D1          | c                      | o            | h           | —           | —           | —           | —     | 10.627                             | 0.42                        | 1.32                        | 1                     | 51.4                               | 0.44                                 | 3.63                          | 10.420                        | 0.33        | 1.05        | 0.17 | 53.4        | 10.43       | 0.34        | 1.08  |
| 05122582+4519525 | 162.699     | 3.574       | 0.611      | 1            | —          | —          | —           | —          | —           | —             | D1          | c                      | o            | h           | —           | —           | —           | —     | 10.777                             | 0.33                        | 1.27                        | 1                     | 46.6                               | 0.66                                 | 3.67                          | 10.549                        | 0.23        | 0.96        | 0.19 | 48.6        | 10.56       | 0.24        | 1.00  |
| 05122970+5117149 | 157.848     | 7.059       | 0.331      | 1            | —          | —          | —           | —          | —           | —             | D1          | c                      | o            | —           | —           | —           | —           | —     | 9.849                              | 0.37                        | 1.19                        | 1                     | 64.6                               | 0.34                                 | 3.57                          | 9.726                         | 0.32        | 1.03        | 0.10 | 65.7        | 9.74        | 0.33        | 1.05  |
| 05123258+4426135 | 163.436     | 3.065       | 0.716      | 1            | —          | —          | —           | —          | N           | —             | D1          | c                      | o            | —           | —           | —           | —           | —     | 11.264                             | 0.42                        | 1.32                        | 1                     | 29.2                               | 0.54                                 | 3.66                          | 10.997                        | 0.30        | 0.97        | 0.22 | 30.7        | 11.01       | 0.31        | 1.01  |
| 05130361+5213479 | 157.124     | 7.676       | 0.334      | 1            | —          | —          | —           | —          | —           | —             | D1          | c                      | o            | —           | —           | —           | —           | —     | 10.552                             | 0.32                        | 1.10                        | 1                     | 48.6                               | 0.76                                 | 3.48                          | 10.428                        | 0.26        | 0.93        | 0.10 | 49.5        | 10.44       | 0.27        | 0.95  |
| 05131664+5119537 | 157.883     | 7.185       | 0.333      | 1            | —          | —          | —           | —          | —           | —             | D1          | c                      | o            | —           | —           | —           | —           | —     | 11.008                             | 0.40                        | 1.15                        | 1                     | 42.0                               | 0.70                                 | 3.50                          | 10.884                        | 0.34        | 0.99        | 0.10 | 42.8        | 10.89       | 0.35        | 1.01  |
| 05132138+2509501 | 179.207     | -8.072      | 0.617      | 1            | —          | —          | —           | —          | —           | —             | D1          | c                      | o            | —           | —           | —           | —           | —     | 11.377                             | 0.37                        | 1.22                        | 1                     | 36.6                               | 0.90                                 | 3.45                          | 11.147                        | 0.27        | 0.91        | 0.19 | 38.3        | 11.16       | 0.28        | 0.95  |
| 05132469+3727108 | 169.187     | -0.904      | 8.053      | 8            | —          | —          | —           | —          | —           | —             | —           | —                      | —            | —           | —           | —           | —           | —     | 8.184                              | 0.96                        | 1.69                        | 1                     | 154.4                              | 0.62                                 | 3.78                          | 5.183                         | -0.38       | -2.31       | 2.49 | ...         | ...         | -0.22       | -1.78 |
| 05132533+2442504 | 179.587     | -8.318      | 0.550      | 1            | —          | —          | t           | —          | —           | —             | D1          | c                      | o            | h           | —           | —           | —           | —     | 11.073                             | 0.35                        | 1.24                        | 1                     | 39.4                               | 0.42                                 | 3.48                          | 10.868                        | 0.26        | 0.97        | 0.17 | 40.9        | 10.88       | 0.27        | 1.00  |
| 05132637+3727458 | 169.183     | -0.894      | 8.139      | 9            | —          | —          | —           | —          | —           | —             | —           | —                      | —            | —           | —           | —           | —           | —     | 12.055                             | 1.05                        | 1.95                        | 1                     | 41.2                               | 0.36                                 | 3.78                          | 9.022                         | -0.30       | -2.10       | 2.52 | ...         | ...         | -0.14       | -1.56 |
| 05132830+3726188 | 169.206     | -0.903      | 7.225      | 9            | —          | —          | —           | —          | —           | —             | —           | —                      | —            | —           | —           | —           | —           | —     | 10.369                             | 0.78                        | 1.31                        | 1                     | 96.4                               | 0.60                                 | 3.78                          | 7.677                         | -0.41       | -2.28       | 2.24 | ...         | ...         | -0.27       | -1.80 |
| 05133015+3726568 | 169.201     | -0.891      | 7.48       |              |            |            |             |            |             |               |             |                        |              |             |             |             |             |       |                                    |                             |                             |                       |                                    |                                      |                               |                               |             |             |      |             |             |             |       |

Table B1: a) continued.

| 2MASX J          | <i>l</i> | <i>b</i> | EBV   | Object | Sample | Disc | 2MRS | Velocity | NIR  | Photom | Ext   | <i>K</i> <sub>20</sub> | <i>H-K</i> | <i>J-K</i> | vc    | <i>a</i> | <i>b/a</i> | st.d. | <i>K</i> <sub>s</sub> <sup>o</sup> | ( <i>H-K</i> ) <sup>o</sup> | ( <i>J-K</i> ) <sup>o</sup> | <i>A<sub>K</sub></i> | <i>a</i> <sub>d</sub> <sup>o</sup> | <i>K</i> <sub>s</sub> <sup>o,d</sup> | ( <i>H-K</i> ) <sup>o,c</sup> | ( <i>J-K</i> ) <sup>o,c</sup> |       |       |      |      |       |       |       |
|------------------|----------|----------|-------|--------|--------|------|------|----------|------|--------|-------|------------------------|------------|------------|-------|----------|------------|-------|------------------------------------|-----------------------------|-----------------------------|----------------------|------------------------------------|--------------------------------------|-------------------------------|-------------------------------|-------|-------|------|------|-------|-------|-------|
| (1)              | deg      | deg      | mag   | class  | off    | flag | gal  | TF       | (7b) | (7c)   | ext'd | type                   | (8)        | (9)        | Opt   | HI       | (10b)      | (11)  | flag                               | flag                        | flag                        | mag                  | (25)                               | mag                                  | (26)                          | mag                           | (28)  |       |      |      |       |       |       |
| (1)              | (2a)     | (2b)     | (3)   | (4)    | (5)    | (6)  | (7a) | (7b)     | (7c) | (7d)   | (7e)  | (8)                    | (9)        | (10a)      | (10b) | (11)     | (12)       | (13)  | (14)                               | (15)                        | (16)                        | (17)                 | (18)                               | (19)                                 | (20)                          | (21)                          | (22)  | (23)  | (24) | (25) | (26)  | (27)  | (28)  |
| 05200820+3901546 | 168.665  | 1.087    | 2.497 | 9      | —      | —    | —    | —        | —    | —      | —     | D2                     | —          | —          | —     | —        | —          | —     | 11.355                             | 0.68                        | 1.61                        | 1                    | 49.6                               | 0.88                                 | 3.73                          | 10.425                        | 0.27  | 0.37  | 0.77 | ...  | ...   | 0.32  | 0.53  |
| 05200866+4314313 | 165.206  | 3.492    | 0.611 | 1      | —      | —    | —    | —        | —    | —      | —     | D1                     | —          | —          | —     | —        | —          | —     | 10.666                             | 0.29                        | 1.11                        | 1                    | 34.8                               | 0.92                                 | 3.60                          | 10.438                        | 0.19  | 0.81  | 0.19 | 36.3 | 10.45 | 0.20  | 0.85  |
| 05201415+4318214 | 165.163  | 3.542    | 0.618 | 1      | —      | —    | —    | —        | —    | —      | —     | D1                     | —          | —          | —     | —        | —          | —     | 9.943                              | 0.38                        | 1.13                        | 1                    | 51.6                               | 0.72                                 | 3.60                          | 9.713                         | 0.28  | 0.82  | 0.19 | 53.8 | 9.73  | 0.29  | 0.86  |
| 05201442+3637045 | 170.657  | -0.276   | 3.888 | 8      | —      | —    | —    | —        | —    | —      | —     | —                      | —          | —          | —     | —        | —          | —     | 11.661                             | 0.95                        | 2.35                        | 1                    | 12.8                               | 0.84                                 | 3.66                          | 10.212                        | 0.31  | 0.41  | 1.20 | ...  | ...   | 0.39  | 0.67  |
| 05201660+3637034 | 170.662  | -0.271   | 4.049 | 9      | —      | —    | —    | —        | —    | —      | —     | —                      | —          | —          | —     | —        | —          | —     | 12.108                             | 0.83                        | 2.14                        | 1                    | 19.4                               | 0.54                                 | 3.65                          | 10.599                        | 0.16  | 0.13  | 1.25 | ...  | ...   | 0.23  | 0.39  |
| 05201718+3637384 | 170.655  | -0.263   | 4.271 | 7      | o      | —    | —    | —        | —    | —      | —     | —                      | —          | —          | —     | —        | —          | —     | 11.208                             | 0.31                        | 1.13                        | 1                    | 74.2                               | 0.80                                 | 3.65                          | 9.617                         | -0.40 | -0.99 | 1.32 | ...  | ...   | -0.32 | -0.71 |
| 05202100+3637595 | 170.657  | -0.250   | 4.654 | 8      | —      | —    | —    | —        | —    | —      | —     | —                      | —          | —          | —     | —        | —          | —     | 10.766                             | 1.05                        | 2.47                        | 1                    | 63.4                               | 0.58                                 | 3.65                          | 9.032                         | 0.28  | 0.16  | 1.44 | ...  | ...   | 0.37  | 0.47  |
| 05202170+4537453 | 163.259  | 4.881    | 0.676 | 1      | —      | —    | —    | —        | —    | —      | —     | D4                     | —          | —          | —     | —        | —          | —     | 11.294                             | 0.38                        | 1.35                        | 1                    | 31.4                               | 0.72                                 | 3.57                          | 11.042                        | 0.27  | 1.01  | 0.21 | 33.0 | 11.05 | 0.28  | 1.06  |
| 05205668+3638294 | 170.719  | -0.147   | 1.732 | 7      | —      | —    | —    | —        | —    | —      | —     | —                      | —          | —          | —     | —        | —          | —     | 11.681                             | 1.19                        | 3.18                        | 1                    | 19.0                               | 0.64                                 | 3.65                          | 11.036                        | 0.90  | 2.32  | 0.54 | ...  | ...   | 0.94  | 2.43  |
| 05205769+2340308 | 181.435  | -7.492   | 0.916 | 1      | —      | —    | —    | —        | —    | —      | —     | D4                     | —          | —          | —     | —        | —          | —     | 11.497                             | 0.48                        | 1.37                        | 1                    | 31.6                               | 0.96                                 | 3.39                          | 11.156                        | 0.33  | 0.91  | 0.28 | 34.3 | 11.15 | 0.35  | 0.98  |
| 05210581+3639365 | 170.721  | -0.111   | 1.449 | 8      | —      | —    | —    | —        | —    | —      | —     | —                      | —          | —          | —     | —        | —          | —     | 10.998                             | 1.45                        | 3.33                        | 1                    | 20.8                               | 0.58                                 | 3.65                          | 10.458                        | 1.21  | 2.61  | 0.45 | ...  | ...   | 1.24  | 2.71  |
| 05211998+5143491 | 158.268  | 8.443    | 0.384 | 1      | —      | —    | —    | —        | —    | —      | —     | D1                     | —          | —          | —     | —        | —          | —     | 11.159                             | 0.41                        | 1.21                        | 1                    | 44.0                               | 0.72                                 | 3.37                          | 11.016                        | 0.35  | 1.02  | 0.12 | 45.2 | 11.02 | 0.35  | 1.04  |
| 05214064+4907191 | 160.484  | 7.033    | 0.367 | 1      | —      | —    | —    | —        | —    | —      | —     | D1                     | —          | —          | —     | —        | —          | —     | 10.145                             | 0.39                        | 1.23                        | 1                    | 59.2                               | 0.60                                 | 3.56                          | 10.008                        | 0.33  | 1.05  | 0.11 | 60.3 | 10.02 | 0.34  | 1.07  |
| 05215254+3750551 | 169.831  | 0.693    | 1.216 | 8      | —      | —    | —    | —        | —    | —      | —     | —                      | —          | —          | —     | —        | —          | —     | 11.543                             | 0.68                        | 1.65                        | 1                    | 14.8                               | 0.78                                 | 3.68                          | 11.090                        | 0.48  | 1.05  | 0.38 | ...  | ...   | 0.51  | 1.13  |
| 05215822+4058480 | 167.263  | 2.485    | 0.908 | 1      | —      | —    | —    | —        | —    | —      | —     | D1                     | —          | —          | —     | —        | —          | —     | 11.283                             | 0.44                        | 1.43                        | 1                    | 37.4                               | 0.56                                 | 3.62                          | 10.945                        | 0.29  | 0.98  | 0.28 | 40.4 | 10.95 | 0.31  | 1.04  |
| 05220064+4005407 | 167.997  | 1.989    | 1.362 | 7      | —      | —    | —    | —        | —    | —      | —     | —                      | —          | —          | —     | —        | —          | —     | 10.282                             | 1.11                        | 2.35                        | 1                    | 35.0                               | 0.80                                 | 3.61                          | 9.775                         | 0.89  | 1.67  | 0.42 | ...  | ...   | 0.91  | 1.76  |
| 05221454+3826469 | 169.380  | 1.091    | 0.788 | 1      | —      | —    | —    | —        | —    | —      | —     | D1                     | —          | —          | —     | —        | —          | —     | 10.978                             | 0.54                        | 1.61                        | 1                    | 56.4                               | 0.22                                 | 3.68                          | 10.684                        | 0.41  | 1.21  | 0.24 | 60.4 | 10.68 | 0.43  | 1.27  |
| 05221961+2150424 | 183.147  | -8.250   | 1.012 | 1      | —      | —    | —    | —        | —    | —      | —     | D4                     | —          | —          | —     | —        | —          | —     | 11.337                             | 0.47                        | 1.41                        | 1                    | 24.4                               | 0.76                                 | 3.35                          | 10.960                        | 0.30  | 0.91  | 0.31 | 26.6 | 10.97 | 0.32  | 0.97  |
| 05222630+5110419 | 158.829  | 8.279    | 0.365 | 1      | —      | —    | —    | —        | —    | —      | —     | D1                     | —          | —          | —     | —        | —          | —     | 11.217                             | 0.30                        | 1.10                        | 1                    | 32.8                               | 0.66                                 | 3.46                          | 11.081                        | 0.24  | 0.92  | 0.11 | 33.5 | 11.09 | 0.25  | 0.94  |
| 05224663+5112476 | 158.829  | 8.343    | 0.368 | 1      | —      | —    | —    | —        | —    | —      | —     | D1                     | —          | —          | —     | —        | —          | —     | 11.340                             | 0.35                        | 1.14                        | 1                    | 37.2                               | 0.58                                 | 3.52                          | 11.203                        | 0.29  | 0.95  | 0.11 | 38.0 | 11.21 | 0.29  | 0.98  |
| 05225518+3331318 | 173.513  | -1.584   | 2.446 | 8      | —      | —    | —    | —        | —    | —      | —     | —                      | —          | —          | —     | —        | —          | —     | 12.058                             | 0.91                        | 1.73                        | -2                   | 32.6                               | 0.60                                 | 3.93                          | 11.147                        | 0.50  | 0.51  | 0.76 | ...  | ...   | 0.55  | 0.67  |
| 05225606+3331488 | 173.511  | -1.579   | 2.425 | 9      | —      | —    | —    | —        | —    | —      | —     | —                      | —          | —          | —     | —        | —          | —     | 10.776                             | 0.98                        | 1.63                        | -2                   | 63.2                               | 0.24                                 | 3.93                          | 9.872                         | 0.58  | 0.42  | 0.75 | ...  | ...   | 0.63  | 0.58  |
| 05230354+3358258 | 173.160  | -1.307   | 3.863 | 9      | —      | —    | —    | —        | —    | —      | —     | —                      | —          | —          | —     | —        | —          | —     | 9.168                              | 1.07                        | 2.07                        | 1                    | 107.6                              | 0.72                                 | 3.69                          | 7.729                         | 0.43  | 0.16  | 1.20 | ...  | ...   | 0.51  | 0.41  |
| 05230829+3328378 | 173.579  | -1.574   | 2.065 | 8      | —      | —    | —    | —        | —    | —      | —     | —                      | —          | —          | —     | —        | —          | —     | 8.578                              | 0.61                        | 1.31                        | 1                    | 83.0                               | 0.72                                 | 3.93                          | 7.809                         | 0.26  | 0.29  | 0.64 | ...  | ...   | 0.30  | 0.42  |
| 05231061+3357547 | 173.181  | -1.291   | 3.906 | 8      | —      | —    | —    | —        | —    | —      | —     | —                      | —          | —          | —     | —        | —          | —     | 12.029                             | 0.85                        | 1.67                        | -2                   | 31.2                               | 0.80                                 | 3.69                          | 10.574                        | 0.20  | -0.27 | 1.21 | ...  | ...   | 0.28  | -0.01 |
| 05231096+4822525 | 161.243  | 6.825    | 0.425 | 1      | —      | —    | —    | —        | —    | —      | —     | D2                     | —          | —          | —     | —        | —          | —     | 11.070                             | 0.33                        | 1.20                        | 1                    | 33.0                               | 0.74                                 | 3.56                          | 10.912                        | 0.26  | 0.98  | 0.13 | 33.9 | 10.92 | 0.27  | 1.01  |
| 05231302+5112435 | 158.869  | 8.400    | 0.389 | 1      | —      | —    | —    | —        | —    | —      | —     | D1                     | —          | —          | —     | —        | —          | —     | 11.389                             | 0.31                        | 1.19                        | 1                    | 31.0                               | 0.90                                 | 3.52                          | 11.244                        | 0.25  | 1.00  | 0.12 | 31.8 | 11.25 | 0.26  | 1.02  |
| 05231868+3918221 | 168.789  | 1.749    | 0.703 | 8      | —      | —    | —    | —        | —    | —      | —     | —                      | —          | —          | —     | —        | —          | —     | 10.346                             | 0.95                        | 2.16                        | 1                    | 25.6                               | 0.80                                 | 3.64                          | 10.084                        | 0.84  | 1.82  | 0.22 | ...  | ...   | 0.85  | 1.86  |
| 05232341+4633162 | 162.788  | 5.836    | 0.624 | 1      | —      | —    | —    | —        | —    | —      | —     | D1                     | —          | —          | —     | —        | —          | —     | 10.747                             | 0.41                        | 1.27                        | 1                    | 77.4                               | 0.28                                 | 3.58                          | 10.514                        | 0.30  | 0.96  | 0.19 | 81.0 | 10.53 | 0.31  | 1.00  |
| 05232875+4333332 | 165.287  | 4.171    | 0.649 | 1      | —      | —    | —    | —        | —    | —      | —     | D4                     | —          | —          | —     | —        | —          | —     | 11.239                             | 0.41                        | 1.31                        | 1                    | 40.6                               | 0.74                                 | 3.64                          | 10.997                        | 0.30  | 0.99  | 0.20 | 42.9 | 10.99 | 0.31  | 1.03  |
| 05233237+5116160 | 158.847  | 8.474    | 0.390 | 1      | —      | —    | —    | —        | —    | —      | —     | D1                     | —          | —          | —     | —        | —          | —     | 10.741                             | 0.36                        | 1.17                        | 1                    | 37.8                               | 0.82                                 | 3.51                          | 10.596                        | 0.30  | 0.97  | 0.12 | 38.6 | 10.61 | 0.31  | 1.00  |
| 05235899+2128531 | 183.668  | -8.130   | 0.740 | 1      | —      | —    | —    | —        | —    | —      | —     | D1                     | —          | —          | —     | —        | —          | —     | 11.037                             | 0.46                        | 1.36                        | 1                    | 28.6                               | 0.88                                 | 3.47                          | 10.761                        | 0.34  | 0.99  | 0.23 | 30.4 | 10.76 | 0.35  | 1.04  |
| 05240487+3205564 | 174.829  | -2.187   | 1.131 | 1      | —      | —    | —    | —        | —    | —      | —     | D1                     | —          | —          | —     | —        | —          | —     | 11.199                             | 0.43                        | 1.49                        | 1                    | 45.8                               | 0.34                                 | 3.62                          | 10.778                        | 0.25  | 0.93  | 0.35 | 51.3 | 10.76 | 0.27  | 1.00  |
| 05242849+4840568 | 161.110  | 7.171    | 0.439 | 1      | —      | —    | —    | —        | —    | —      | —     | D3                     | —          | —          | —     | —        | —          | —     | 11.208                             | 0.38                        | 1.22                        | 1                    | 31.6                               | 0.90                                 | 3.56                          | 11.044                        | 0.31  | 1.01  | 0.14 | 32.4 | 11.06 | 0.32  | 1.04  |
| 05245544+5001060 | 160.026  | 7.968    | 0.473 | 1      | —      | —    | —    | —        | —    | —      | —     | D3                     | —          | —          | —     | —        | —          | —     | 11.208                             | 0.31                        | 1.25                        | 1                    | 32.0                               | 0.56                                 | 3.55                          | 11.032                        | 0.23  | 1.01  | 0.15 | 33.0 | 11.04 | 0.24  | 1.04  |
| 05250816+3221028 | 174.746  | -1.861   | 0.811 | 1      | —      | —    | —    | —        | —    | —      | —     | D3                     | —          | —          | —     | —        | —          | —     | 10.654                             | 0.39                        | 1.41                        | 1                    | 41.6                               | 0.94                                 | 3.61                          | 10.352                        | 0.26  | 1.00  | 0.25 | 44.2 | 10.37 | 0.27  | 1.06  |
| 05251873+3212438 | 174.882  | -1.908   | 0.887 | 1      | —      | —    | —    | —        | —    | —      | —     | D3                     | —          | —          | —     | —        | —          | —     | 10.762                             | 0.46                        | 1.45                        | 1                    | 39.8                               | 0.80                                 | 3.66                          | 10.432                        | 0.32  | 1.01  | 0.27 | 42.6 | 10.45 | 0.33  | 1.07  |
| 05252022+4953221 | 160.172  | 7.953    | 0.424 | 1      | —      | —    | —    | —        | —    | —      | —     | D1                     | —          | —          | —     | —        | —          | —     | 11.355                             | 0.43                        | 1.33                        | 1                    | 29.0                               | 0.72                                 | 3.47                          | 11.197                        | 0.36  | 1.11  | 0.13 | 29.8 | 11.21 | 0.37  | 1.14  |
| 05252560+2443418 | 181.125  | -6.059   | 1.268 | 1      | —      | —    | —    | —        | —    | —      | —     | D1                     | —          | —          | —     | —        | —          | —     | 11.610                             | 0.44                        | 1.63                        | 1                    | 30.4                               | 0.72                                 | 3.44                          | 11.138                        | 0.23  | 1.00  | 0.39 | 34.5 | 11.12 | 0.25  | 1.09  |
| 05252929+2151220 | 183.546  | -7.632   | 0.595 | 1      | —      | —    | —    | —        | —    | —      | —     | D1                     | —          | —          | —     | —        | —          | —     | 11.456                             | 0.29                        | 1.12                        | 1                    | 37.4                               | 0.60                                 | 3.47                          | 11.234                        | 0.19  | 0.82  | 0.18 | 39.4 | 11.23 | 0.20  | 0.86  |
| 05253552+3221283 | 174.794  | -1.777   | 0.807 | 1      | —      | —    | —    | —        | —    | —      | —     | D3                     | —          | —          | —     | —        | —          | —     | 10.593                             | 0.43                        | 1.36                        | 1                    | 38.2                               | 0.86                                 | 3.59                          | 10.292                        | 0.30  | 0.96  | 0.25 | 40.5 | 10.31 | 0.32  | 1.02  |



48

A. C. Schröder et al.



Table B1: a) continued.

| 2MASX J          | <i>l</i> | <i>b</i> | EBV    | Object | Sample | Disc | 2MRS | Velocity | NIR  | Photom | Ext   | <i>K</i> <sub>20</sub> | <i>H-K</i> | <i>J-K</i> | vc   | <i>a</i> | <i>b/a</i> | st.d. | <i>K</i> <sub>s</sub> <sup>o</sup> | ( <i>H-K</i> ) <sup>o</sup> | ( <i>J-K</i> ) <sup>o</sup> | <i>A<sub>K</sub></i> | <i>a</i> <sub>d</sub> <sup>o</sup> | <i>K</i> <sub>s</sub> <sup>o,d</sup> | ( <i>H-K</i> ) <sup>o,c</sup> | ( <i>J-K</i> ) <sup>o,c</sup> |       |     |      |      |     |      |     |      |     |      |
|------------------|----------|----------|--------|--------|--------|------|------|----------|------|--------|-------|------------------------|------------|------------|------|----------|------------|-------|------------------------------------|-----------------------------|-----------------------------|----------------------|------------------------------------|--------------------------------------|-------------------------------|-------------------------------|-------|-----|------|------|-----|------|-----|------|-----|------|
| (1)              | deg      | deg      | mag    | class  | off    | flag | gal  | TF       | (7b) | (7c)   | ext'd | type                   | (8)        | (9)        | Opt  | HI       | (10b)      | (11)  | flag                               | flag                        | flag                        | mag                  | (21)                               | mag                                  | (22)                          | mag                           | (23)  | mag | (24) | (25) | mag | (26) | mag | (27) | mag | (28) |
| 05385067+3041392 | 177.731  | -0.322   | 10.110 | 9      | -      | -    | -    | -        | -    | -      | -     | -                      | 12.034     | 1.11       | 2.13 | 1        | 54.4       | 0.52  | 3.73                               | 8.267                       | -0.57                       | -2.89                | 3.13                               | ...                                  | ...                           | -0.37                         | -2.22 |     |      |      |     |      |     |      |     |      |
| 05385507+3337492 | 175.256  | 1.258    | 0.885  | 1      | -      | -    | -    | -        | -    | -      | -     | -                      | 11.564     | 0.52       | 1.62 | 1        | 27.8       | 0.48  | 3.69                               | 11.234                      | 0.37                        | 1.18                 | 0.27                               | 30.0                                 | 11.24                         | 0.39                          | 1.24  |     |      |      |     |      |     |      |     |      |
| 05390248+2020199 | 186.546  | -5.783   | 0.488  | 1      | -      | -    | -    | -        | -    | -      | -     | -                      | 10.200     | 0.35       | 1.20 | 1        | 61.0       | 0.76  | 3.52                               | 10.018                      | 0.27                        | 0.96                 | 0.15                               | 62.9                                 | 10.03                         | 0.28                          | 0.99  |     |      |      |     |      |     |      |     |      |
| 05390339+1534316 | 190.639  | -8.270   | 0.484  | 1      | -      | -    | -    | -        | -    | -      | -     | -                      | 10.244     | 0.40       | 1.30 | 1        | 78.0       | 0.26  | 3.40                               | 10.064                      | 0.32                        | 1.06                 | 0.15                               | 80.4                                 | 10.08                         | 0.33                          | 1.09  |     |      |      |     |      |     |      |     |      |
| 05390365+3041148 | 177.762  | -0.286   | 6.667  | 7      | -      | -    | -    | -        | -    | -      | -     | -                      | 12.228     | 1.29       | 3.20 | -2       | 18.8       | 0.74  | 3.68                               | 9.744                       | 0.18                        | -0.12                | 2.07                               | ...                                  | ...                           | 0.31                          | 0.32  |     |      |      |     |      |     |      |     |      |
| 05390889+3545058 | 173.485  | 2.428    | 8.321  | 8      | -      | -    | -    | -        | -    | -      | -     | -                      | 11.596     | 0.75       | 1.92 | -2       | 48.8       | 0.46  | 3.68                               | 8.496                       | -0.63                       | -2.22                | 2.58                               | ...                                  | ...                           | -0.47                         | -1.67 |     |      |      |     |      |     |      |     |      |
| 05390994+2731585 | 180.444  | -1.947   | 1.382  | 8      | -      | -    | -    | -        | -    | -      | -     | -                      | 11.586     | 0.88       | 2.20 | 1        | 19.2       | 0.54  | 3.60                               | 11.071                      | 0.65                        | 1.52                 | 0.43                               | ...                                  | ...                           | 0.67                          | 1.61  |     |      |      |     |      |     |      |     |      |
| 05391037+3545038 | 173.488  | 2.432    | 8.171  | 9      | -      | -    | -    | -        | -    | -      | -     | -                      | 11.135     | 0.78       | 2.04 | -2       | 38.6       | 0.52  | 3.68                               | 8.090                       | -0.58                       | -2.02                | 2.53                               | ...                                  | ...                           | -0.42                         | -1.48 |     |      |      |     |      |     |      |     |      |
| 05391349+3545538 | 173.482  | 2.448    | 8.569  | 8      | -      | -    | -    | -        | -    | -      | -     | -                      | 9.293      | 2.16       | ...  | 1        | 92.4       | 0.56  | 3.68                               | 6.100                       | 0.74                        | ...                  | 2.65                               | ...                                  | ...                           | 0.91                          | ...   |     |      |      |     |      |     |      |     |      |
| 05392433+3541118 | 173.568  | 2.437    | 3.284  | 7      | -      | -    | -    | -        | -    | -      | -     | -                      | 12.242     | 0.96       | 2.51 | -2       | 24.8       | 0.64  | 3.57                               | 11.018                      | 0.42                        | 0.88                 | 1.02                               | ...                                  | ...                           | 0.48                          | 1.09  |     |      |      |     |      |     |      |     |      |
| 05392840+2456298 | 182.679  | -3.266   | 0.973  | 8      | -      | -    | -    | -        | -    | -      | -     | -                      | 11.472     | 1.05       | 2.42 | 1        | 16.4       | 0.74  | 3.57                               | 11.109                      | 0.88                        | 1.94                 | 0.30                               | ...                                  | ...                           | 0.90                          | 2.00  |     |      |      |     |      |     |      |     |      |
| 05393522+2841388 | 179.510  | -1.251   | 1.543  | 1      | -      | -    | -    | -        | -    | -      | -     | -                      | 11.237     | 0.57       | 1.72 | 1        | 40.8       | 0.26  | 3.62                               | 10.662                      | 0.32                        | 0.96                 | 0.48                               | 48.1                                 | 10.63                         | 0.35                          | 1.06  |     |      |      |     |      |     |      |     |      |
| 05395434+2656147 | 181.036  | -2.124   | 1.224  | 1      | -      | -    | -    | -        | -    | -      | -     | -                      | 11.558     | 0.51       | 1.57 | 1        | 34.4       | 0.64  | 3.61                               | 11.102                      | 0.31                        | 0.96                 | 0.38                               | 39.0                                 | 11.08                         | 0.33                          | 1.04  |     |      |      |     |      |     |      |     |      |
| 05401954+2352033 | 183.694  | -3.669   | 3.745  | 8      | -      | -    | -    | -        | -    | -      | -     | -                      | 11.961     | 1.95       | ...  | 1        | 18.0       | 0.86  | 3.49                               | 10.566                      | 1.33                        | ...                  | 1.16                               | ...                                  | ...                           | 1.41                          | ...   |     |      |      |     |      |     |      |     |      |
| 05402025+2500485 | 182.721  | -3.061   | 0.868  | 8      | -      | -    | -    | -        | -    | -      | -     | -                      | 11.222     | 1.51       | 3.11 | -2       | 15.6       | 0.68  | 3.56                               | 10.899                      | 1.36                        | 2.68                 | 0.27                               | ...                                  | ...                           | 1.38                          | 2.74  |     |      |      |     |      |     |      |     |      |
| 05402311+2350550 | 183.718  | -3.668   | 3.934  | 9      | -      | -    | -    | -        | -    | -      | -     | -                      | 12.394     | 1.17       | 2.89 | 1        | 22.4       | 0.34  | 3.56                               | 10.928                      | 0.52                        | 0.94                 | 1.22                               | ...                                  | ...                           | 0.60                          | 1.20  |     |      |      |     |      |     |      |     |      |
| 05402435+3311311 | 175.793  | 1.288    | 0.795  | 1      | -      | -    | -    | -        | -    | -      | -     | -                      | 10.932     | 0.47       | 1.46 | 1        | 45.2       | 0.82  | 3.72                               | 10.636                      | 0.34                        | 1.06                 | 0.25                               | 48.1                                 | 10.64                         | 0.35                          | 1.11  |     |      |      |     |      |     |      |     |      |
| 05402818+3313361 | 175.770  | 1.317    | 0.805  | 1      | -      | -    | -    | -        | -    | -      | -     | -                      | 11.223     | 0.49       | 1.49 | 1        | 30.8       | 0.72  | 3.72                               | 10.923                      | 0.36                        | 1.09                 | 0.25                               | 32.8                                 | 10.94                         | 0.38                          | 1.14  |     |      |      |     |      |     |      |     |      |
| 05402865+2352300 | 183.706  | -3.636   | 3.548  | 8      | -      | -    | -    | -        | -    | -      | -     | -                      | 11.400     | 1.22       | 2.95 | 1        | 26.4       | 0.80  | 3.56                               | 10.078                      | 0.63                        | 1.18                 | 1.10                               | ...                                  | ...                           | 0.70                          | 1.42  |     |      |      |     |      |     |      |     |      |
| 05402955+1609559 | 190.310  | -7.669   | 0.439  | 1      | -      | -    | -    | -        | -    | -      | -     | -                      | 10.577     | 0.32       | 1.13 | 1        | 36.0       | 0.74  | 3.43                               | 10.413                      | 0.24                        | 0.91                 | 0.14                               | 36.9                                 | 10.43                         | 0.25                          | 0.94  |     |      |      |     |      |     |      |     |      |
| 05403032+1806560 | 188.633  | -6.653   | 0.398  | 1      | -      | -    | -    | -        | -    | -      | -     | -                      | 11.169     | 0.45       | 1.31 | 1        | 41.8       | 0.54  | 3.54                               | 11.021                      | 0.39                        | 1.11                 | 0.12                               | 42.9                                 | 11.03                         | 0.40                          | 1.13  |     |      |      |     |      |     |      |     |      |
| 05403099+3550411 | 174.593  | 2.712    | 11.485 | 9      | -      | -    | -    | -        | -    | -      | -     | -                      | 13.458     | 0.53       | 1.52 | -1       | 13.6       | 0.78  | 3.61                               | 9.179                       | -1.37                       | -4.19                | 3.56                               | ...                                  | ...                           | -1.15                         | -3.43 |     |      |      |     |      |     |      |     |      |
| 05403530+4612227 | 166.650  | 8.150    | 0.368  | 1      | -      | -    | -    | -        | -    | -      | -     | -                      | 10.918     | 0.34       | 1.14 | 1        | 36.8       | 0.88  | 3.48                               | 10.781                      | 0.28                        | 0.95                 | 0.11                               | 37.6                                 | 10.79                         | 0.29                          | 0.98  |     |      |      |     |      |     |      |     |      |
| 05403952+3545460 | 173.638  | 2.693    | 13.314 | 9      | -      | -    | -    | -        | -    | -      | -     | -                      | 13.382     | 1.29       | ...  | 1        | 14.0       | 0.46  | 3.61                               | 8.421                       | -0.91                       | ...                  | 4.12                               | ...                                  | ...                           | -0.65                         | ...   |     |      |      |     |      |     |      |     |      |
| 05403994+1627400 | 190.077  | -7.480   | 0.447  | 1      | -      | -    | -    | -        | -    | -      | -     | -                      | 11.242     | 0.35       | 1.08 | 1        | 44.8       | 0.66  | 3.48                               | 11.075                      | 0.27                        | 0.86                 | 0.14                               | 46.6                                 | 11.06                         | 0.28                          | 0.89  |     |      |      |     |      |     |      |     |      |
| 05404131+3555218 | 173.505  | 2.783    | 12.786 | 7      | -      | -    | -    | -        | -    | -      | -     | -                      | 11.974     | 1.35       | 3.51 | -2       | 20.0       | 0.46  | 3.71                               | 7.210                       | -0.77                       | -2.84                | 3.96                               | ...                                  | ...                           | -0.52                         | -2.00 |     |      |      |     |      |     |      |     |      |
| 05404371+4941415 | 161.669  | 9.958    | 0.301  | 1      | -      | -    | -    | -        | -    | -      | -     | -                      | 10.152     | 0.52       | 1.38 | 1        | 48.8       | 0.94  | 3.32                               | 10.040                      | 0.47                        | 1.23                 | 0.09                               | 49.5                                 | 10.05                         | 0.48                          | 1.25  |     |      |      |     |      |     |      |     |      |
| 05404756+3538148 | 173.759  | 2.650    | 11.558 | 9      | -      | -    | -    | -        | -    | -      | -     | -                      | 10.543     | 1.14       | 2.55 | 1        | 87.0       | 0.26  | 3.91                               | 6.236                       | -0.78                       | -3.19                | 3.58                               | ...                                  | ...                           | -0.55                         | -2.43 |     |      |      |     |      |     |      |     |      |
| 05404901+3402088 | 175.122  | 1.807    | 0.782  | 8      | -      | -    | -    | -        | -    | -      | -     | -                      | 11.399     | 1.09       | 2.49 | -2       | 34.4       | 0.34  | 3.67                               | 11.108                      | 0.96                        | 2.11                 | 0.24                               | ...                                  | ...                           | 0.98                          | 2.16  |     |      |      |     |      |     |      |     |      |
| 05404954+2400305 | 183.635  | -3.498   | 1.299  | 1      | -      | -    | -    | -        | -    | -      | -     | -                      | 10.516     | 0.44       | 1.46 | 1        | 43.8       | 0.88  | 3.52                               | 10.032                      | 0.23                        | 0.82                 | 0.40                               | 49.0                                 | 10.05                         | 0.25                          | 0.90  |     |      |      |     |      |     |      |     |      |
| 05404994+3539028 | 173.752  | 2.664    | 13.378 | 9      | -      | -    | -    | -        | -    | -      | -     | -                      | 12.643     | 0.89       | 2.04 | 1        | 37.6       | 0.14  | 3.91                               | 7.658                       | -1.33                       | -4.61                | 4.14                               | ...                                  | ...                           | -1.07                         | -3.72 |     |      |      |     |      |     |      |     |      |
| 05405141+3541228 | 173.722  | 2.689    | 18.674 | 9      | -      | -    | -    | -        | -    | -      | -     | -                      | 11.530     | 0.95       | 1.98 | 1        | 45.2       | 0.40  | 3.91                               | 4.572                       | -2.14                       | -7.29                | 5.78                               | ...                                  | ...                           | -1.77                         | -6.06 |     |      |      |     |      |     |      |     |      |
| 05405149+3538118 | 173.767  | 2.661    | 11.352 | 9      | -      | -    | -    | -        | -    | -      | -     | -                      | 9.191      | 1.29       | 2.90 | 1        | 102.4      | 0.52  | 3.91                               | 4.961                       | -0.59                       | -2.74                | 3.52                               | ...                                  | ...                           | -0.36                         | -1.99 |     |      |      |     |      |     |      |     |      |
| 05405264+3539298 | 173.750  | 2.676    | 14.668 | 9      | -      | -    | -    | -        | -    | -      | -     | -                      | 10.293     | 1.13       | 2.97 | -2       | 54.8       | 0.64  | 3.91                               | 4.828                       | -1.30                       | -4.32                | 4.54                               | ...                                  | ...                           | -1.01                         | -3.35 |     |      |      |     |      |     |      |     |      |
| 05405273+3542188 | 173.711  | 2.701    | 18.377 | 9      | -      | -    | -    | -        | -    | -      | -     | -                      | 7.604      | 1.09       | 2.42 | 1        | 142.2      | 0.86  | 3.91                               | 0.757                       | -1.96                       | -6.71                | 5.69                               | ...                                  | ...                           | -1.60                         | -5.50 |     |      |      |     |      |     |      |     |      |
| 05405281+3540148 | 173.740  | 2.683    | 16.683 | 9      | -      | -    | -    | -        | -    | -      | -     | -                      | 12.473     | 0.87       | 2.64 | -2       | 32.2       | 0.80  | 3.91                               | 6.257                       | -1.89                       | -5.65                | 5.17                               | ...                                  | ...                           | -1.56                         | -4.55 |     |      |      |     |      |     |      |     |      |
| 05405404+3539598 | 173.746  | 2.684    | 15.933 | 9      | -      | -    | -    | -        | -    | -      | -     | -                      | 13.030     | 1.13       | 2.74 | 1        | 10.0       | 0.36  | 3.91                               | 7.093                       | -1.51                       | -5.18                | 4.94                               | ...                                  | ...                           | -1.20                         | -4.13 |     |      |      |     |      |     |      |     |      |
| 05405453+3544088 | 173.688  | 2.722    | 18.403 | 8      | -      | -    | -    | -        | -    | -      | -     | -                      | 9.175      | 1.08       | 2.54 | 1        | 75.8       | 0.68  | 3.91                               | 2.318                       | -1.97                       | -6.61                | 5.70                               | ...                                  | ...                           | -1.61                         | -5.39 |     |      |      |     |      |     |      |     |      |
| 05405494+3541258 | 173.727  | 2.699    | 18.288 | 9      | -      | -    | -    | -        | -    | -      | -     | -                      | 11.485     | 1.05       | 2.23 | -2       | 37.8       | 0.56  | 3.91                               | 4.671                       | -1.98                       | -6.86                | 5.66                               | ...                                  | ...                           | -1.62                         | -5.65 |     |      |      |     |      |     |      |     |      |
| 05405882+3159438 | 176.872  | 0.756    | 1.085  | 1      | -      | -    | -    | -        | -    | -      | -     | -                      | 11.508     | 0.58       | 1.37 | 1        | 28.0       | 0.84  | 3.66                               | 11.104                      | 0.40                        | 0.83                 | 0.34                               | 30.8                                 | 11.11                         | 0.43                          | 0.90  |     |      |      |     |      |     |      |     |      |
| 05410391+3549537 | 173.623  | 2.800    | 23.042 | 9      | -      | -    | -    | -        | -    | -      | -     | -                      | 11.393     | 1.31       | 2.59 | -2       | 54.6       | 0.30  | 3.83                               | 2.808                       | -2.51                       | -8.86                | 7.14                               | ...                                  | ...                           | -2.06                         | -7.34 |     |      |      |     |      |     |      |     |      |
| 05410433+3552137 | 173.591  | 2.821    | 23.841 | 9      | -      | -    | -    | -        | -    | -      | -     | -                      | 10.671     | 1.02       | 1.90 | 1        | 93.8       | 0.38  | 3.83                               | 1.788                       | -2.93                       | -9.95                | 7.38                               | ...                                  | ...                           | -2.46                         | -8.37 |     |      |      |     |      |     |      |     |      |
| 05410516+2930260 | 178.995  | -0.542   | 1.712  | 8      | -      | -    | -    | -        | -    | -      | -     | -                      | 11.541     | 0.94       | 2.24 | 1        | 34.4       | 0.64  | 3.63                               | 10.903                      | 0.66                        | 1.39                 | 0.53                               | ...                                  | ...                           | 0.70                          | 1.51  |     |      |      |     |      |     |      |     |      |
| 05410633+3608571 | 173.357  | 2.974    | 1.986  | 8      | -      | -    | -    | -        | -    | -      | -     | -                      | 11.760     | 0.94       | 2.44 | -2       | 24.2       | 0.72  | 3.59                               | 11.020                      | 0.61                        | 1.45                 | 0.62                               | ...                                  | ...                           | 0.65                          | 1.58  |     |      |      |     |      |     |      |     |      |
| 05410635+3552081 | 173.596  | 2.826    | 23.211 | 9      | -      | -    | -    | -        | -    | -      | -     | -                      | 12.187     | 0.91       | 2.14 | 1        | 64.8       | 0.14  | 3.71                               | 3.539                       | -2.94                       | -9.39                | 7.19                               | ...                                  | ...                           | -2.48                         | -7.86 |     |      |      |     |      |     |      |     |      |
| 05410687+3549287 | 173.634  | 2.804    | 22.216 | 8      | -      | -    | -    | -        | -    | -      | -     | -                      | 7.482      | 1.82       | 3.79 | 1        | 96.8       | 0.54  | 3.83                               | -0.796                      | -1.86                       | -7.25                | 6.88                               | ...                                  | ...                           | -1.43                         | -5.78 |     |      |      |     |      |     |      |     |      |
| 05410933+3549277 | 173.639  | 2.811    | 21.486 | 9      | -      | -    | -    | -        | -    | -      | -     | -                      | 11.213     | 1.45       | 4.68 | -2       | 29.2       | 0.44  | 3.83                               | 3.207                       | -2.11                       | -6.00                | 6.66                               | ...                                  | ...                           | -1.68                         | -4.58 |     |      |      |     |      |     |      |     |      |
| 05411459+3550019 | 173.640  | 2.831    | 20.921 | 9      | -      | -    | -    | -        | -    | -      | -     | -                      | 12.495     | 1.19       | 3.16 | 1        | 21.0       | 0.32  | 3.77                               | 4.700                       | -2.28                       | -7.23                | 6.48                               | ...                                  | ...                           | -1.87                         | -5.85 |     |      |      |     |      |     |      |     |      |
| 05411499+3552119 | 173.610  | 2.852    | 19.518 | 8      | -      | -    | -    | -        | -    | -      | -     | -                      | 13.941     | ...        | 2.03 | 1        | 11.4       | 1.00  | 3.77                               | 6.669                       | ...                         | -7.66                | 6.05                               | ...                                  | ...                           | ...                           | -6.38 |     |      |      |     |      |     |      |     |      |
| 05411739+3553320 | 173.596  | 2.870    | 16.579 | 9      | -      | -    | -    | -        | -    | -      | -     | -                      | 14.265     | ...        | 1.53 | -1       | 10.0       | 1.00  | 3.65                               | 8.088                       | ...                         | -6.70                | 5.14                               | ...                                  | ...                           | ...                           | -5.61 |     |      |      |     |      |     |      |     |      |
| 05411745+3440059 | 174.637  | 2.225    | 1.339  | 1</    |        |      |      |          |      |        |       |                        |            |            |      |          |            |       |                                    |                             |                             |                      |                                    |                                      |                               |                               |       |     |      |      |     |      |     |      |     |      |

Table B1: a) continued.

| 2MASX J          | <i>l</i> | <i>b</i> | EBV   | Object | Sample | Disc | 2MRS | Velocity | NIR   | Photom | Ext | <i>K</i> <sub>20</sub> | <i>H-K</i> | <i>J-K</i> | vc   | <i>a</i> | <i>b/a</i> | st.d. | <i>K</i> <sub>s</sub> <sup>o</sup> | ( <i>H-K</i> ) <sup>o</sup> | ( <i>J-K</i> ) <sup>o</sup> | <i>A<sub>K</sub></i> | <i>a</i> <sub>d</sub> <sup>o</sup> | <i>K</i> <sub>s</sub> <sup>o,d</sup> | ( <i>H-K</i> ) <sup>o,c</sup> | ( <i>J-K</i> ) <sup>o,c</sup> |      |      |       |      |      |
|------------------|----------|----------|-------|--------|--------|------|------|----------|-------|--------|-----|------------------------|------------|------------|------|----------|------------|-------|------------------------------------|-----------------------------|-----------------------------|----------------------|------------------------------------|--------------------------------------|-------------------------------|-------------------------------|------|------|-------|------|------|
| (1)              | deg      | deg      | mag   | class  | off    | gal  | TF   | obs      | ext'd | type   | Opt | HI                     | mag        | mag        | (17) | "        | (19)       | (20)  | mag                                | mag                         | mag                         | mag                  | "                                  | mag                                  | mag                           | mag                           |      |      |       |      |      |
| (1)              | (2a)     | (2b)     | (3)   | (4)    | (5)    | (6)  | (7a) | (7c)     | (7d)  | (8)    | (9) | (10a)                  | (10b)      | (11)       | (12) | (13)     | (14)       | (15)  | (16)                               | (17)                        | (18)                        | (19)                 | (20)                               | (21)                                 | (22)                          | (23)                          | (24) | (25) | (26)  | (27) | (28) |
| 05430220+2801422 | 180.477  | -0.959   | 1.255 | 1      | --     | g    |      |          |       | D1     | e   | --                     | h          | U          | --   | --       | 11.024     | 0.51  | 1.60                               | 1                           | 32.6                        | 0.58                 | 3.65                               | 10.556                               | 0.31                          | 0.98                          | 0.39 | 36.9 | 10.54 | 0.33 | 1.06 |
| 05430236+1620591 | 190.470  | -7.050   | 0.485 | 1      | --     | g    |      |          |       | D2     | e   | --                     | h:         | U          | --   | --       | 10.894     | 0.34  | 1.16                               | 1                           | 40.2                        | 0.62                 | 3.48                               | 10.713                               | 0.26                          | 0.92                          | 0.15 | 41.4 | 10.73 | 0.27 | 0.95 |
| 05431777+3138489 | 177.427  | 0.991    | 1.172 | 1      | --     | g    |      | N        | --    | D1     | c   | o                      | --         | U          | --   | --       | 11.411     | 0.47  | 1.54                               | 1                           | 39.6                        | 0.70                 | 3.65                               | 10.974                               | 0.28                          | 0.96                          | 0.36 | 44.5 | 10.96 | 0.30 | 1.04 |
| 05432166+1639543 | 190.238  | -6.822   | 0.423 | 1      | --     | g    |      |          |       | D2     | c   | o                      | --         | U          | --   | --       | 11.348     | 0.34  | 1.13                               | 1                           | 25.8                        | 0.56                 | 3.47                               | 11.190                               | 0.26                          | 0.92                          | 0.13 | 26.5 | 11.20 | 0.27 | 0.95 |
| 05433099+4009019 | 170.187  | 5.472    | 0.480 | 1      | --     | g    |      |          |       | D4     | c   | o                      | --         | U          | --   | --       | 11.059     | 0.31  | 1.17                               | 1                           | 30.0                        | 0.94                 | 3.51                               | 10.880                               | 0.23                          | 0.93                          | 0.15 | 30.9 | 10.89 | 0.23 | 0.96 |
| 05434263+3516031 | 174.387  | 2.961    | 0.976 | 1      | --     | g    |      | N        | --    | D3     | --  | --                     | --         | U          | --   | --       | 11.128     | 0.59  | 1.63                               | 1                           | 38.2                        | 0.90                 | 3.62                               | 10.764                               | 0.43                          | 1.15                          | 0.30 | 41.6 | 10.77 | 0.44 | 1.21 |
| 05434892+3056391 | 178.084  | 0.716    | 2.036 | 1      | --     | s?   |      |          |       | D2     | --  | --                     | --         | U          | --   | s?       | 11.622     | 0.58  | 1.58                               | 1                           | 29.8                        | 0.92                 | 3.64                               | 10.863                               | 0.24                          | 0.57                          | 0.63 | 37.1 | 10.84 | 0.28 | 0.71 |
| 05441004+1653210 | 190.144  | -6.541   | 0.392 | 1      | --     | g    |      |          |       | D1     | c   | o                      | --         | U          | --   | --       | 10.928     | 0.36  | 1.16                               | 1                           | 42.0                        | 0.68                 | 3.51                               | 10.782                               | 0.30                          | 0.96                          | 0.12 | 43.0 | 10.79 | 0.31 | 0.99 |
| 05443764+4159369 | 168.708  | 6.602    | 0.389 | 1      | --     | g    |      |          |       | D4     | c   | o                      | --         | U          | --   | --       | 10.777     | 0.33  | 1.20                               | 1                           | 36.6                        | 0.78                 | 3.56                               | 10.632                               | 0.26                          | 1.00                          | 0.12 | 37.5 | 10.64 | 0.27 | 1.03 |
| 05444298+1652221 | 190.226  | -6.437   | 0.389 | 1      | --     | g    |      |          |       | D3     | c   | o                      | --         | U          | --   | --       | 11.166     | 0.41  | 1.24                               | 1                           | 28.2                        | 0.78                 | 3.55                               | 11.021                               | 0.34                          | 1.04                          | 0.12 | 28.8 | 11.03 | 0.35 | 1.07 |
| 05444416+1648501 | 190.280  | -6.463   | 0.394 | 1      | --     | g    |      |          |       | D4     | c   | o                      | --         | U          | --   | --       | 9.898      | 0.32  | 1.13                               | 1                           | 53.4                        | 0.90                 | 3.55                               | 9.751                                | 0.25                          | 0.93                          | 0.12 | 54.5 | 9.77  | 0.26 | 0.96 |
| 05444886+1646263 | 190.324  | -6.468   | 0.394 | 1      | --     | g    |      | N        | --    | D1     | c   | o                      | --         | h          | U    | --       | 10.942     | 0.30  | 1.12                               | 1                           | 49.0                        | 0.48                 | 3.50                               | 10.795                               | 0.23                          | 0.92                          | 0.12 | 50.3 | 10.80 | 0.24 | 0.95 |
| 05450906+1736351 | 189.644  | -5.969   | 0.536 | 1      | --     | g    |      |          |       | D1     | c   | o                      | --         | U          | --   | --       | 11.317     | 0.44  | 1.46                               | 1                           | 47.4                        | 0.26                 | 3.51                               | 11.117                               | 0.36                          | 1.20                          | 0.17 | 49.3 | 11.12 | 0.37 | 1.23 |
| 05451158+2115474 | 186.508  | -4.074   | 0.755 | 1      | --     | g    |      |          |       | D2     | e   | --                     | --         | U          | --   | --       | 11.133     | 0.35  | 1.30                               | 1                           | 32.0                        | 0.64                 | 3.56                               | 10.852                               | 0.22                          | 0.92                          | 0.23 | 33.8 | 10.87 | 0.24 | 0.97 |
| 05452012+1447335 | 192.103  | -7.374   | 0.447 | 1      | --     | g    |      |          |       | D1     | c   | o                      | --         | U          | --   | --       | 11.155     | 0.40  | 1.30                               | 1                           | 55.4                        | 0.22                 | 3.51                               | 10.988                               | 0.33                          | 1.08                          | 0.14 | 57.1 | 11.00 | 0.34 | 1.11 |
| 05452013+3649316 | 173.225  | 4.052    | 0.659 | 1      | o      | g    |      | N        | --    | D1     | --  | --                     | --         | o          | --   | --       | 11.198     | 0.40  | 1.27                               | 1                           | 37.2                        | 0.68                 | 3.63                               | 10.952                               | 0.29                          | 0.95                          | 0.20 | 39.2 | 10.96 | 0.31 | 0.99 |
| 05452124+2321174 | 184.736  | -2.957   | 1.328 | 1      | --     | g    |      |          |       | D1     | --  | --                     | --         | U          | --   | --       | 11.633     | 0.48  | 1.66                               | 1                           | 36.4                        | 0.32                 | 3.57                               | 11.138                               | 0.26                          | 1.00                          | 0.41 | 41.2 | 11.14 | 0.29 | 1.08 |
| 05453448+1453595 | 192.040  | -7.269   | 0.439 | 1      | --     | g    |      |          |       | D3     | c   | o                      | --         | U          | --   | --       | 9.813      | 0.35  | 1.17                               | 1                           | 58.6                        | 0.78                 | 3.53                               | 9.649                                | 0.27                          | 0.95                          | 0.14 | 60.0 | 9.67  | 0.28 | 0.98 |
| 05454087+2813165 | 180.617  | -0.361   | 1.288 | 1      | --     | g    |      | N        | --    | D2     | e   | --                     | --         | U          | --   | e?       | 10.994     | 0.54  | 1.57                               | 1                           | 35.2                        | 0.88                 | 3.61                               | 10.514                               | 0.32                          | 0.93                          | 0.40 | 39.7 | 10.51 | 0.35 | 1.01 |
| 05454092+1306184 | 193.613  | -8.158   | 0.507 | 1      | --     | g    |      |          | *     | D1     | c   | --                     | --         | U          | --   | --       | 11.431     | 0.34  | 1.22                               | 1                           | 34.0                        | 0.32                 | 3.43                               | 11.242                               | 0.26                          | 0.97                          | 0.16 | 35.2 | 11.25 | 0.27 | 1.00 |
| 05462224+3155264 | 177.532  | 1.692    | 0.690 | 1      | --     | g    |      |          |       | D1     | c   | o                      | --         | h          | U    | --       | 11.126     | 0.46  | 1.28                               | 1                           | 38.2                        | 0.76                 | 3.59                               | 10.869                               | 0.35                          | 0.94                          | 0.21 | 40.2 | 10.88 | 0.36 | 0.98 |
| 05462465+1505201 | 191.980  | -6.999   | 0.385 | 1      | --     | g    |      |          |       | D4     | c   | o                      | --         | U          | --   | --       | 11.111     | 0.31  | 1.15                               | 1                           | 26.4                        | 0.64                 | 3.53                               | 10.968                               | 0.25                          | 0.96                          | 0.12 | 27.0 | 10.98 | 0.25 | 0.99 |
| 05463922+1858511 | 188.647  | -4.958   | 0.525 | 1      | --     | g    |      |          |       | D1     | c   | o                      | --         | U          | --   | --       | 10.349     | 0.37  | 1.28                               | 1                           | 48.8                        | 0.74                 | 3.48                               | 10.153                               | 0.29                          | 1.02                          | 0.16 | 50.4 | 10.17 | 0.30 | 1.05 |
| 05465108+2503459 | 183.452  | -1.779   | 1.617 | 9      | --     | g    |      |          |       | --     | --  | --                     | --         | U          | --   | --       | 9.638      | 1.62  | 2.91                               | 1                           | 56.8                        | 0.28                 | 3.62                               | 9.036                                | 1.35                          | 2.10                          | 0.50 | ...  | ...   | 1.38 | 2.21 |
| 05465770+3152089 | 177.644  | 1.771    | 0.643 | 1      | --     | g    |      |          |       | D2     | e   | o                      | --         | U          | --   | --       | 10.971     | 0.39  | 1.24                               | 1                           | 30.4                        | 0.92                 | 3.63                               | 10.731                               | 0.28                          | 0.92                          | 0.20 | 31.8 | 10.75 | 0.30 | 0.97 |
| 05470483+2531192 | 183.086  | -1.496   | 1.169 | 1      | --     | g    |      | t        | --    | D1     | e   | --                     | h          | U          | --   | --       | 11.457     | 0.53  | 1.54                               | 1                           | 36.0                        | 0.36                 | 3.63                               | 11.021                               | 0.33                          | 0.96                          | 0.36 | 40.1 | 11.02 | 0.36 | 1.04 |
| 05470571+1733127 | 189.931  | -5.600   | 0.392 | 1      | --     | g    |      |          |       | D1     | c   | --                     | h          | U          | --   | --       | 11.277     | 0.32  | 1.12                               | 1                           | 49.0                        | 0.88                 | 3.53                               | 11.131                               | 0.26                          | 0.93                          | 0.12 | 50.3 | 11.14 | 0.27 | 0.95 |
| 05471117+1733467 | 189.934  | -5.577   | 0.392 | 1      | --     | g    |      | N        | --    | D1     | c   | --                     | *          | U          | --   | --       | 10.746     | 0.46  | 1.32                               | 1                           | 36.2                        | 0.64                 | 3.53                               | 10.600                               | 0.40                          | 1.13                          | 0.12 | 36.9 | 10.62 | 0.40 | 1.16 |
| 05471129+3036369 | 178.746  | 1.161    | 2.771 | 9      | --     | g    |      |          |       | --     | --  | --                     | --         | U          | --   | --       | 10.548     | 1.18  | 1.35                               | -2                          | 240.0                       | 1.00                 | 3.68                               | 9.516                                | 0.72                          | -0.03                         | 0.86 | ...  | ...   | 0.78 | 0.15 |
| 05471330+3036099 | 178.756  | 1.163    | 2.740 | 8      | --     | g    |      |          |       | --     | --  | --                     | --         | U          | --   | --       | 10.450     | 1.02  | 1.91                               | 1                           | 53.6                        | 0.88                 | 3.70                               | 9.429                                | 0.57                          | 0.55                          | 0.85 | ...  | ...   | 0.62 | 0.73 |
| 05471940+2444422 | 183.780  | -1.852   | 1.030 | 1      | --     | g    |      | N        | --    | D1     | e   | --                     | --         | U          | --   | --       | 11.296     | 0.49  | 1.55                               | 1                           | 37.8                        | 0.28                 | 3.67                               | 10.912                               | 0.32                          | 1.03                          | 0.32 | 41.3 | 10.92 | 0.34 | 1.10 |
| 05474966+2529148 | 183.203  | -1.370   | 0.935 | 1      | --     | g    |      | t        | --    | D1     | e   | --                     | h          | U          | --   | --       | 11.176     | 0.39  | 1.39                               | 1                           | 48.2                        | 0.32                 | 3.66                               | 10.828                               | 0.24                          | 0.93                          | 0.29 | 52.2 | 10.83 | 0.26 | 0.99 |
| 05480756+2141579 | 186.487  | -3.265   | 0.579 | 1      | --     | g    |      | N        | --    | D1     | e   | o                      | --         | U          | --   | --       | 10.445     | 0.47  | 1.38                               | 1                           | 61.4                        | 0.30                 | 3.66                               | 10.229                               | 0.37                          | 1.09                          | 0.18 | 63.7 | 10.25 | 0.38 | 1.13 |
| 05481285+3153223 | 177.764  | 2.009    | 0.573 | 1      | --     | g    |      |          |       | D2     | c   | o                      | --         | U          | --   | --       | 10.500     | 0.37  | 1.22                               | 1                           | 41.2                        | 0.80                 | 3.66                               | 10.286                               | 0.28                          | 0.93                          | 0.18 | 42.7 | 10.30 | 0.29 | 0.97 |
| 05481986+4144473 | 169.275  | 7.069    | 0.390 | 1      | --     | g    |      |          |       | D3     | e   | o                      | --         | U          | --   | --       | 10.999     | 0.35  | 1.16                               | 1                           | 36.8                        | 0.68                 | 3.49                               | 10.854                               | 0.29                          | 0.97                          | 0.12 | 37.6 | 10.87 | 0.30 | 0.99 |
| 05482218+3841373 | 171.926  | 5.527    | 0.501 | 1      | o      | g    |      |          |       | D1     | c   | --                     | --         | o          | --   | --       | 10.323     | 0.35  | 1.22                               | 1                           | 48.2                        | 0.66                 | 3.55                               | 10.136                               | 0.27                          | 0.97                          | 0.16 | 50.4 | 10.12 | 0.28 | 1.00 |
| 05482421+1403238 | 193.122  | -7.107   | 0.460 | 1      | --     | g    |      |          |       | D1     | c   | --                     | h          | U          | --   | --       | 11.132     | 0.28  | 1.17                               | 1                           | 38.8                        | 0.88                 | 3.50                               | 10.961                               | 0.20                          | 0.94                          | 0.14 | 40.1 | 10.96 | 0.21 | 0.97 |
| 05491821+1947083 | 188.275  | -4.009   | 0.822 | 1      | --     | g    |      | N        | --    | D4     | --  | --                     | --         | U          | --   | --       | 10.548     | 0.44  | 1.43                               | 1                           | 44.4                        | 0.90                 | 3.60                               | 10.242                               | 0.31                          | 1.03                          | 0.25 | 47.3 | 10.26 | 0.32 | 1.08 |
| 05492111+1750279 | 189.958  | -4.991   | 0.364 | 1      | --     | g    |      |          |       | D1     | e   | --                     | h          | U          | --   | --       | 10.752     | 0.46  | 1.24                               | 1                           | 56.6                        | 0.56                 | 3.64                               | 10.616                               | 0.40                          | 1.06                          | 0.11 | 57.9 | 10.63 | 0.41 | 1.09 |
| 05492365+3149150 | 177.952  | 2.189    | 0.506 | 1      | --     | g    |      |          |       | D1     | e   | o                      | --         | U          | --   | --       | 11.294     | 0.57  | 1.24                               | 1                           | 36.0                        | 0.72                 | 3.64                               | 11.105                               | 0.49                          | 0.99                          | 0.16 | 37.4 | 11.11 | 0.50 | 1.03 |
| 05493145+1738569 | 190.145  | -5.054   | 0.354 | 1      | --     | g    |      |          |       | D1     | c   | o                      | --         | h          | U    | --       | 9.976      | 0.42  | 1.30                               | 1                           | 69.4                        | 0.32                 | 3.61                               | 9.844                                | 0.36                          | 1.12                          | 0.11 | 70.7 | 9.86  | 0.37 | 1.14 |
| 05493153+1741079 | 190.114  | -5.035   | 0.353 | 1      | --     | g    |      |          |       | D1     | c   | o?                     | --         | U          | --   | --       | 9.773      | 0.31  | 1.09                               | 1                           | 57.8                        | 0.52                 | 3.61                               | 9.641                                | 0.25                          | 0.91                          | 0.11 | 58.8 | 9.66  | 0.26 | 0.94 |
| 05493394+1836051 | 189.328  | -4.560   | 0.509 | 1      | --     | g    |      |          |       | D2     | e   | o                      | --         | U          | --   | --       | 11.405     | 0.28  | 1.21                               | 1                           | 31.6                        | 0.76                 | 3.63                               | 11.215                               | 0.20                          | 0.96                          | 0.16 | 32.7 | 11.23 | 0.21 | 0.99 |
| 05495856+1501098 | 192.479  | -6.292   | 0.341 | 1      | --     | g    |      | N        | --    | D1     | c   | --                     | --         | U          | --   | --       | 11.239     | 0.32  | 1.08                               | 1                           | 42.4                        | 0.44                 | 3.57                               | 11.112                               | 0.27                          | 0.91                          | 0.11 | 43.3 | 11.12 | 0.28 | 0.93 |
| 05500286+4246578 | 168.533  | 7.865    | 0.296 | 1      | --     | g    |      |          |       | D3     |     |                        |            |            |      |          |            |       |                                    |                             |                             |                      |                                    |                                      |                               |                               |      |      |       |      |      |

Table B1: a) continued.

| 2MASX J          | <i>l</i> | <i>b</i> | EBV    | Object |     | Sample | Disc | 2MRS | Velocity | NIR   | Photom | Ext | <i>K</i> <sub>20</sub> | <i>H-K</i> | <i>J-K</i> | vc   | <i>a</i> | <i>b/a</i> | st.d. | <i>K</i> <sub>s</sub> <sup>o</sup> | ( <i>H-K</i> ) <sup>o</sup> | ( <i>J-K</i> ) <sup>o</sup> | <i>A<sub>K</sub></i> | <i>a</i> <sub>d</sub> <sup>o</sup> | <i>K</i> <sub>s</sub> <sup>o,d</sup> | ( <i>H-K</i> ) <sup>o,c</sup> | ( <i>J-K</i> ) <sup>o,c</sup> |      |      |      |      |      |
|------------------|----------|----------|--------|--------|-----|--------|------|------|----------|-------|--------|-----|------------------------|------------|------------|------|----------|------------|-------|------------------------------------|-----------------------------|-----------------------------|----------------------|------------------------------------|--------------------------------------|-------------------------------|-------------------------------|------|------|------|------|------|
| (1)              | deg      | deg      | mag    | class  | off | flag   | gal  | TF   | obs      | ext'd | type   |     | (14)                   | mag        | mag        | (17) | "        | (19)       | (20)  | mag                                | mag                         | mag                         | mag                  | "                                  | mag                                  | mag                           | mag                           |      |      |      |      |      |
| (2a)             | (2b)     | (2b)     | (3)    | (4)    | (5) | (6)    | (7a) | (7b) | (7c)     | (7d)  | (8)    | (9) | (10a)                  | (10b)      | (11)       | (12) | (13)     | (14)       | (15)  | (16)                               | (17)                        | (18)                        | (19)                 | (20)                               | (21)                                 | (22)                          | (23)                          | (24) | (25) | (26) | (27) | (28) |
| 05521130+2700317 | 182.399  | 0.250    | 13.786 | 8      | –   | –      | –    | –    | –        | –     | –      | –   | 9.463                  | 1.74       | 4.08       | 1    | 62.0     | 0.68       | 3.71  | 4.326                              | −0.54                       | −2.77                       | 4.27                 | ...                                | ...                                  | −0.27                         | −1.86                         |      |      |      |      |      |
| 05521244+2659595 | 182.409  | 0.249    | 13.017 | 9      | –   | –      | –    | –    | –        | –     | –      | –   | 13.171                 | 1.20       | ...        | −1   | 17.4     | 1.00       | 3.72  | 8.321                              | −0.95                       | ...                         | 4.03                 | ...                                | ...                                  | −0.70                         | ...                           |      |      |      |      |      |
| 05521278+3344455 | 176.596  | 3.680    | 0.715  | 1      | –   | –      | –    | –    | –        | –     | –      | –   | 10.191                 | 0.38       | 1.22       | 1    | 70.0     | 0.72       | 3.62  | 9.925                              | 0.26                        | 0.87                        | 0.22                 | 74.1                               | 9.93                                 | 0.28                          | 0.92                          |      |      |      |      |      |
| 05521304+2659175 | 182.420  | 0.245    | 12.108 | 8      | –   | –      | –    | –    | –        | –     | –      | –   | 12.154                 | 1.57       | 2.72       | −2   | 33.4     | 0.76       | 3.72  | 7.643                              | −0.43                       | −3.30                       | 3.75                 | ...                                | ...                                  | −0.20                         | −2.50                         |      |      |      |      |      |
| 05521551+2659085 | 182.427  | 0.252    | 11.711 | 9      | –   | –      | –    | –    | –        | –     | –      | –   | 12.183                 | 1.08       | 2.61       | −2   | 14.0     | 0.58       | 3.72  | 7.819                              | −0.86                       | −3.20                       | 3.63                 | ...                                | ...                                  | −0.63                         | −2.43                         |      |      |      |      |      |
| 05521581+2659305 | 182.422  | 0.256    | 12.203 | 9      | –   | –      | –    | –    | –        | –     | –      | –   | 11.952                 | 0.92       | 1.72       | −2   | 33.8     | 0.78       | 3.72  | 7.405                              | −1.10                       | −4.34                       | 3.78                 | ...                                | ...                                  | −0.87                         | −3.54                         |      |      |      |      |      |
| 05521648+3750158 | 173.057  | 5.755    | 0.619  | 1      | –   | –      | –    | –    | –        | –     | –      | –   | 11.426                 | 0.46       | 1.29       | 1    | 44.8     | 0.54       | 3.51  | 11.195                             | 0.36                        | 0.98                        | 0.19                 | 47.1                               | 11.20                                | 0.37                          | 1.02                          |      |      |      |      |      |
| 05524113+3056577 | 179.061  | 2.348    | 0.481  | 1      | –   | –      | –    | –    | –        | –     | –      | –   | 11.183                 | 0.49       | 1.44       | 1    | 47.4     | 0.30       | 3.63  | 11.004                             | 0.41                        | 1.20                        | 0.15                 | 49.0                               | 11.01                                | 0.42                          | 1.23                          |      |      |      |      |      |
| 05531219+2144149 | 187.057  | −2.231   | 0.852  | 1      | –   | –      | –    | –    | –        | –     | –      | –   | 11.373                 | 0.38       | 1.07       | 1    | 35.2     | 0.64       | 3.69  | 11.056                             | 0.23                        | 0.64                        | 0.26                 | 37.7                               | 11.07                                | 0.25                          | 0.70                          |      |      |      |      |      |
| 05531423+3622021 | 174.432  | 5.183    | 0.543  | 1      | –   | –      | –    | –    | –        | –     | –      | –   | 11.246                 | 0.33       | 1.14       | 1    | 38.8     | 0.70       | 3.57  | 11.044                             | 0.24                        | 0.88                        | 0.17                 | 40.3                               | 11.06                                | 0.25                          | 0.91                          |      |      |      |      |      |
| 05534271+2414540 | 184.951  | −0.857   | 2.265  | 8      | –   | –      | –    | –    | –        | –     | –      | –   | 9.987                  | 0.99       | 2.75       | 1    | 71.4     | 0.58       | 3.62  | 9.143                              | 0.61                        | 1.62                        | 0.70                 | ...                                | ...                                  | 0.66                          | 1.77                          |      |      |      |      |      |
| 05534910+3106555 | 179.040  | 2.642    | 0.570  | 1      | –   | –      | –    | –    | –        | –     | –      | –   | 10.520                 | 0.35       | 1.25       | 1    | 35.0     | 0.80       | 3.62  | 10.308                             | 0.25                        | 0.96                        | 0.18                 | 36.3                               | 10.33                                | 0.27                          | 1.00                          |      |      |      |      |      |
| 05540495+3127485 | 178.768  | 2.866    | 0.492  | 1      | –   | –      | –    | –    | –        | –     | –      | –   | 11.422                 | 0.44       | 1.31       | 1    | 25.0     | 0.72       | 3.68  | 11.239                             | 0.36                        | 1.07                        | 0.15                 | 25.8                               | 11.25                                | 0.37                          | 1.10                          |      |      |      |      |      |
| 05540715+1759352 | 190.402  | −3.936   | 0.721  | 1      | –   | –      | –    | –    | –        | –     | –      | –   | 10.499                 | 0.38       | 1.31       | 1    | 40.6     | 0.82       | 3.63  | 10.230                             | 0.26                        | 0.96                        | 0.22                 | 42.7                               | 10.25                                | 0.27                          | 1.00                          |      |      |      |      |      |
| 05540813+0948493 | 197.538  | −8.005   | 0.595  | 1      | –   | –      | –    | –    | –        | –     | –      | –   | 11.296                 | 0.40       | 1.27       | 1    | 35.8     | 0.40       | 3.42  | 11.074                             | 0.30                        | 0.98                        | 0.18                 | 37.4                               | 11.08                                | 0.31                          | 1.02                          |      |      |      |      |      |
| 05541029+1758346 | 190.423  | −3.934   | 0.744  | 1      | –   | –      | –    | –    | –        | –     | –      | –   | 9.752                  | 0.35       | 1.24       | 1    | 64.0     | 0.76       | 3.58  | 9.475                              | 0.23                        | 0.87                        | 0.23                 | 67.2                               | 9.50                                 | 0.24                          | 0.92                          |      |      |      |      |      |
| 05544072+1510134 | 192.920  | −5.235   | 0.319  | 1      | –   | –      | –    | –    | –        | –     | –      | –   | 11.313                 | 0.28       | 0.96       | 1    | 52.6     | 0.50       | 3.53  | 11.194                             | 0.23                        | 0.80                        | 0.10                 | 53.8                               | 11.20                                | 0.24                          | 0.83                          |      |      |      |      |      |
| 05544721+3133030 | 178.768  | 3.040    | 0.466  | 1      | –   | –      | –    | –    | –        | –     | –      | –   | 10.699                 | 0.37       | 1.22       | 1    | 43.6     | 0.74       | 3.61  | 10.525                             | 0.29                        | 0.99                        | 0.14                 | 44.9                               | 10.54                                | 0.30                          | 1.02                          |      |      |      |      |      |
| 05545873+3905337 | 172.228  | 6.839    | 0.496  | 1      | –   | –      | –    | –    | –        | –     | –      | –   | 11.262                 | 0.45       | 1.30       | 1    | 33.8     | 0.56       | 3.48  | 11.077                             | 0.37                        | 1.05                        | 0.15                 | 35.0                               | 11.08                                | 0.38                          | 1.09                          |      |      |      |      |      |
| 05545521+1503265 | 193.149  | −5.066   | 0.339  | 1      | –   | –      | –    | –    | –        | –     | –      | –   | 10.869                 | 0.32       | 1.14       | 1    | 33.4     | 0.80       | 3.57  | 10.743                             | 0.27                        | 0.98                        | 0.11                 | 34.0                               | 10.75                                | 0.28                          | 1.00                          |      |      |      |      |      |
| 05555495+0919112 | 198.190  | −7.865   | 0.574  | 1      | –   | –      | –    | –    | –        | –     | –      | –   | 11.409                 | 0.39       | 1.33       | 1    | 30.0     | 0.90       | 3.53  | 11.195                             | 0.30                        | 1.05                        | 0.18                 | 31.2                               | 11.21                                | 0.31                          | 1.08                          |      |      |      |      |      |
| 05561062+4100185 | 170.662  | 7.979    | 0.344  | 1      | –   | –      | –    | –    | –        | –     | –      | –   | 11.372                 | 0.41       | 1.20       | 1    | 39.2     | 0.66       | 3.44  | 11.244                             | 0.36                        | 1.03                        | 0.11                 | 40.0                               | 11.25                                | 0.36                          | 1.05                          |      |      |      |      |      |
| 05562235+0749432 | 199.561  | −8.494   | 0.467  | 5      | –   | –      | –    | –    | –        | –     | –      | –   | 11.130                 | 0.42       | 1.14       | 1    | 31.8     | 0.54       | 3.50  | 10.956                             | 0.34                        | 0.91                        | 0.14                 | 32.7                               | 10.97                                | 0.35                          | 0.94                          |      |      |      |      |      |
| 05563208+1331376 | 194.577  | −5.662   | 0.287  | 1      | –   | –      | –    | –    | –        | –     | –      | –   | 11.234                 | 0.32       | 1.09       | 1    | 35.6     | 0.82       | 3.60  | 11.127                             | 0.28                        | 0.95                        | 0.09                 | 36.2                               | 11.13                                | 0.28                          | 0.97                          |      |      |      |      |      |
| 05565742+1149306 | 196.116  | −6.413   | 0.325  | 1      | –   | –      | –    | –    | –        | –     | –      | –   | 11.336                 | 0.35       | 1.21       | 1    | 44.6     | 0.30       | 3.57  | 11.215                             | 0.29                        | 1.05                        | 0.10                 | 45.5                               | 11.22                                | 0.30                          | 1.07                          |      |      |      |      |      |
| 05570273+1333516 | 194.606  | −5.535   | 0.293  | 1      | –   | –      | –    | –    | –        | –     | –      | –   | 10.827                 | 0.32       | 1.10       | 1    | 44.2     | 0.58       | 3.59  | 10.718                             | 0.27                        | 0.95                        | 0.09                 | 44.9                               | 10.73                                | 0.28                          | 0.97                          |      |      |      |      |      |
| 05572695+1156572 | 196.067  | −6.247   | 0.329  | 1      | –   | –      | –    | –    | –        | –     | –      | –   | 9.022                  | 0.31       | 1.09       | 1    | 91.4     | 0.70       | 3.63  | 8.899                              | 0.25                        | 0.92                        | 0.10                 | 92.8                               | 8.91                                 | 0.26                          | 0.94                          |      |      |      |      |      |
| 05572787+1521162 | 193.096  | −4.560   | 0.404  | 1      | –   | –      | –    | –    | –        | –     | –      | –   | 11.037                 | 0.37       | 1.17       | 1    | 35.0     | 0.66       | 3.58  | 10.886                             | 0.31                        | 0.97                        | 0.13                 | 35.9                               | 10.90                                | 0.31                          | 1.00                          |      |      |      |      |      |
| 05573375+4054266 | 170.877  | 8.160    | 0.329  | 1      | –   | –      | –    | –    | –        | –     | –      | –   | 11.264                 | 0.41       | 1.28       | 1    | 57.6     | 0.28       | 3.48  | 11.141                             | 0.35                        | 1.12                        | 0.10                 | 58.8                               | 11.15                                | 0.36                          | 1.14                          |      |      |      |      |      |
| 05575173+2233406 | 186.888  | −0.884   | 1.219  | 1      | –   | –      | –    | –    | –        | –     | –      | –   | 11.480                 | 0.57       | 1.59       | 1    | 31.0     | 0.64       | 3.68  | 11.026                             | 0.37                        | 0.98                        | 0.38                 | 34.8                               | 11.02                                | 0.39                          | 1.06                          |      |      |      |      |      |
| 05581153+1632196 | 192.152  | −3.821   | 5.863  | 8      | –   | –      | –    | –    | –        | –     | –      | –   | 12.397                 | 1.18       | 2.50       | 1    | 30.8     | 0.54       | 3.65  | 10.212                             | 0.21                        | −0.42                       | 1.82                 | ...                                | ...                                  | 0.32                          | −0.03                         |      |      |      |      |      |
| 05581194+1632546 | 192.144  | −3.814   | 5.852  | 9      | –   | –      | –    | –    | –        | –     | –      | –   | 11.444                 | 1.16       | 2.05       | 1    | 64.2     | 0.42       | 3.65  | 9.264                              | 0.19                        | −0.86                       | 1.81                 | ...                                | ...                                  | 0.31                          | −0.47                         |      |      |      |      |      |
| 05581389+1631566 | 192.162  | −3.816   | 5.604  | 9      | –   | –      | –    | –    | –        | –     | –      | –   | 9.554                  | 1.78       | 3.53       | 1    | 54.4     | 0.32       | 3.65  | 7.466                              | 0.86                        | 0.75                        | 1.74                 | ...                                | ...                                  | 0.97                          | 1.12                          |      |      |      |      |      |
| 05581473+1631066 | 192.176  | −3.820   | 5.073  | 8      | –   | –      | –    | –    | –        | –     | –      | –   | 8.865                  | 1.66       | 3.76       | 1    | 38.2     | 0.82       | 3.65  | 6.975                              | 0.82                        | 1.24                        | 1.57                 | ...                                | ...                                  | 0.92                          | 1.58                          |      |      |      |      |      |
| 05581521+1631136 | 192.175  | −3.817   | 5.147  | 9      | –   | –      | –    | –    | –        | –     | –      | –   | 12.108                 | 0.76       | 1.73       | 1    | 38.8     | 0.50       | 3.65  | 10.190                             | −0.09                       | −0.83                       | 1.59                 | ...                                | ...                                  | 0.01                          | −0.49                         |      |      |      |      |      |
| 05581570+1632296 | 192.158  | −3.805   | 5.991  | 8      | –   | –      | –    | –    | –        | –     | –      | –   | 12.429                 | 1.03       | 2.70       | 1    | 18.8     | 0.66       | 3.65  | 10.197                             | 0.03                        | −0.27                       | 1.86                 | ...                                | ...                                  | 0.15                          | 0.12                          |      |      |      |      |      |
| 05581625+0548287 | 201.581  | −9.057   | 0.695  | 1      | –   | –      | –    | –    | –        | –     | –      | –   | 11.438                 | 0.42       | 1.20       | 1    | 24.4     | 0.92       | 3.44  | 11.179                             | 0.30                        | 0.86                        | 0.22                 | 25.7                               | 11.19                                | 0.32                          | 0.91                          |      |      |      |      |      |
| 05582189+1100258 | 197.004  | −6.514   | 0.407  | 1      | –   | –      | –    | –    | –        | –     | –      | –   | 11.222                 | 0.23       | 1.04       | 1    | 36.4     | 0.84       | 3.55  | 11.070                             | 0.16                        | 0.84                        | 0.13                 | 37.3                               | 11.08                                | 0.17                          | 0.86                          |      |      |      |      |      |
| 05582445+2013570 | 188.970  | −1.938   | 6.466  | 8      | –   | –      | –    | –    | –        | –     | –      | –   | 9.622                  | 1.66       | 3.50       | 1    | 58.4     | 0.66       | 3.68  | 7.213                              | 0.59                        | 0.29                        | 2.00                 | ...                                | ...                                  | 0.71                          | 0.72                          |      |      |      |      |      |
| 05583106+2642132 | 183.375  | 1.315    | 1.604  | 9      | –   | –      | –    | –    | –        | –     | –      | –   | 11.266                 | 1.35       | 2.71       | 1    | 32.2     | 0.46       | 3.68  | 10.668                             | 1.08                        | 1.91                        | 0.50                 | ...                                | ...                                  | 1.11                          | 2.02                          |      |      |      |      |      |
| 05583132+4031028 | 171.310  | 8.130    | 0.367  | 1      | –   | –      | –    | –    | –        | –     | –      | –   | 11.169                 | 0.45       | 1.23       | 1    | 57.0     | 0.50       | 3.44  | 11.032                             | 0.39                        | 1.05                        | 0.11                 | 58.2                               | 11.04                                | 0.39                          | 1.07                          |      |      |      |      |      |
| 05583187+2244210 | 186.811  | −0.662   | 1.329  | 1      | –   | –      | –    | –    | –        | –     | –      | –   | 10.962                 | 0.59       | 1.67       | 1    | 41.6     | 0.54       | 3.68  | 10.467                             | 0.37                        | 1.01                        | 0.41                 | 47.5                               | 10.45                                | 0.40                          | 1.10                          |      |      |      |      |      |
| 05583483+1754200 | 191.010  | −3.061   | 1.192  | 1      | –   | –      | –    | –    | –        | –     | –      | –   | 10.978                 | 0.42       | 1.36       | 1    | 51.0     | 0.58       | 3.58  | 10.534                             | 0.22                        | 0.76                        | 0.37                 | 57.5                               | 10.52                                | 0.24                          | 0.84                          |      |      |      |      |      |
| 05583605+4031118 | 171.315  | 8.144    | 0.367  | 1      | –   | –      | –    | –    | –        | –     | –      | –   | 10.630                 | 0.33       | 1.12       | 1    | 45.0     | 0.68       | 3.44  | 10.493                             | 0.27                        | 0.93                        | 0.11                 | 45.9                               | 10.51                                | 0.27                          | 0.96                          |      |      |      |      |      |
| 05583756+0823278 | 199.338  | −7.733   | 0.479  | 1      | –   | –      | –    | –    | –        | –     | –      | –   | 10.994                 | 0.38       | 1.25       | 1    | 35.0     | 0.72       | 3.55  | 10.816                             | 0.30                        | 1.01                        | 0.15                 | 36.1                               | 10.83                                | 0.31                          | 1.04                          |      |      |      |      |      |
| 05584006+1018118 | 197.659  | −6.793   | 0.397  | 1      | –   | –      | –    | –    | –        | –     | –      | –   | 10.032                 | 0.34       | 1.20       | 1    | 66.4     | 0.76       | 3.48  | 9.884                              | 0.28                        | 1.00                        | 0.12                 | 67.9                               | 9.90                                 | 0.28                          | 1.03                          |      |      |      |      |      |
| 05585447+1759445 | 190.970  | −2.949   | 1.339  | 1      | –   | –      | –    | –    | –        | –     | –      | –   | 11.372                 | 0.49       | 1.70       | 1    | 27.2     | 0.62       | 3.60  | 10.873                             | 0.27                        |                             |                      |                                    |                                      |                               |                               |      |      |      |      |      |

Table B1: a) continued.

| 2MASX J          | <i>l</i> | <i>b</i> | EBV   | Object | Sample | Disc | 2MRS | Velocity | NIR  | Photom | Ext   | <i>K</i> <sub>20</sub> | <i>H-K</i> | <i>J-K</i> | vc   | <i>a</i> | <i>b/a</i> | st.d. | <i>K</i> <sub>s</sub> <sup>o</sup> | ( <i>H-K</i> ) <sup>o</sup> | ( <i>J-K</i> ) <sup>o</sup> | <i>A<sub>K</sub></i> | <i>a</i> <sub>d</sub> <sup>o</sup> | <i>K</i> <sub>s</sub> <sup>o,d</sup> | ( <i>H-K</i> ) <sup>o,c</sup> | ( <i>J-K</i> ) <sup>o,c</sup> |       |       |      |      |       |       |       |
|------------------|----------|----------|-------|--------|--------|------|------|----------|------|--------|-------|------------------------|------------|------------|------|----------|------------|-------|------------------------------------|-----------------------------|-----------------------------|----------------------|------------------------------------|--------------------------------------|-------------------------------|-------------------------------|-------|-------|------|------|-------|-------|-------|
| (1)              | deg      | deg      | mag   | class  | off    | flg  | gal  | TF       | (7b) | (7c)   | ext'd | type                   | (8)        | (9)        | Opt  | HI       | (10b)      | flg   | flg                                | flg                         | flg                         | mag                  | mag                                | mag                                  | mag                           | mag                           | mag   |       |      |      |       |       |       |
| (1)              | (2a)     | (2b)     | (3)   | (4)    | (5)    | (6)  | (7a) | (7b)     | (7c) | (7d)   | (8)   | (9)                    | (10a)      | (10b)      | (11) | (12)     | (13)       | (14)  | (15)                               | (16)                        | (17)                        | (18)                 | (19)                               | (20)                                 | (21)                          | (22)                          | (23)  | (24)  | (25) | (26) | (27)  | (28)  |       |
| 06024206+0914215 | 199.081  | -6.441   | 0.382 | 1      | -      | -    | g    | -        | -    | -      | -     | D2                     | c          | o          | -    | -        | -          | -     | 11.344                             | 0.35                        | 1.18                        | 1                    | 33.0                               | 0.68                                 | 3.54                          | 11.202                        | 0.28  | 0.99  | 0.12 | 33.7 | 11.21 | 0.29  | 1.02  |
| 06030431+0641304 | 201.376  | -7.587   | 0.418 | 1      | o      | -    | -    | -        | P    | -      | -     | D1                     | cp         | o          | -    | -        | po         | -     | 11.324                             | 0.33                        | 1.00                        | 1                    | 26.2                               | 0.56                                 | 3.51                          | 11.168                        | 0.26  | 0.80  | 0.13 | 26.9 | 11.18 | 0.27  | 0.82  |
| 06031133+0749374 | 200.386  | -7.016   | 0.419 | 1      | -      | -    | g    | -        | -    | -      | -     | D1                     | c          | o          | -    | -        | -          | -     | 10.697                             | 0.38                        | 1.15                        | 1                    | 36.8                               | 0.76                                 | 3.53                          | 10.541                        | 0.31  | 0.94  | 0.13 | 37.6 | 10.56 | 0.32  | 0.97  |
| 06031802+1847563 | 190.787  | -1.646   | 1.537 | 1      | -      | -    | -    | t        | N    | -      | -     | D2                     | -          | -          | -    | -        | -          | -     | 11.702                             | 0.47                        | 1.54                        | 1                    | 23.4                               | 0.44                                 | 3.55                          | 11.129                        | 0.21  | 0.78  | 0.48 | 27.1 | 11.13 | 0.24  | 0.88  |
| 06032163+3014084 | 180.826  | 3.985    | 3.274 | 9      | -      | -    | -    | -        | -    | -      | -     | -                      | -          | -          | -    | -        | -          | -     | 9.762                              | 0.66                        | 1.45                        | 1                    | 125.2                              | 0.88                                 | 3.68                          | 8.542                         | 0.12  | -0.18 | 1.01 | ...  | ...   | 0.18  | 0.04  |
| 06033527+2941442 | 181.323  | 3.764    | 0.695 | 1      | -      | -    | g    | -        | -    | -      | -     | D2                     | e          | o          | -    | -        | -          | -     | 10.184                             | 0.38                        | 1.36                        | 1                    | 57.6                               | 0.88                                 | 3.66                          | 9.925                         | 0.26  | 1.02  | 0.22 | 60.7 | 9.94  | 0.28  | 1.06  |
| 06033565+0747075 | 200.471  | -6.948   | 0.432 | 1      | -      | -    | -    | t        | N    | -      | -     | D1                     | -          | -          | -    | -        | -          | -     | 10.529                             | 0.35                        | 1.19                        | 1                    | 55.8                               | 0.32                                 | 3.61                          | 10.368                        | 0.28  | 0.98  | 0.13 | 57.1 | 10.38 | 0.29  | 1.00  |
| 06034202+3013317 | 180.871  | 4.044    | 5.309 | 9      | -      | -    | g    | -        | -    | -      | -     | -                      | -          | -          | -    | -        | -          | -     | 12.971                             | 0.91                        | 2.13                        | -2                   | 22.0                               | 0.44                                 | 3.76                          | 10.993                        | 0.03  | -0.51 | 1.64 | ...  | ...   | 0.13  | -0.16 |
| 06034287+3013287 | 180.873  | 4.046    | 5.315 | 8      | -      | -    | g    | -        | -    | -      | -     | -                      | -          | -          | -    | -        | c          | -     | 11.958                             | 1.10                        | 2.69                        | 1                    | 22.0                               | 0.52                                 | 3.76                          | 9.978                         | 0.22  | 0.05  | 1.65 | ...  | ...   | 0.32  | 0.40  |
| 06034588+1812362 | 191.354  | -1.839   | 2.235 | 1      | -      | -    | g    | -        | -    | -      | -     | D1                     | -          | -          | -    | -        | -          | -     | 11.849                             | 0.66                        | 2.02                        | 1                    | 31.6                               | 0.38                                 | 3.62                          | 11.016                        | 0.29  | 0.91  | 0.69 | 41.1 | 10.95 | 0.34  | 1.06  |
| 06034709+2937302 | 181.405  | 3.767    | 0.663 | 1      | -      | -    | g    | -        | -    | -      | -     | D2                     | e          | o          | -    | -        | -          | -     | 11.432                             | 0.40                        | 1.30                        | 1                    | 25.0                               | 0.56                                 | 3.66                          | 11.185                        | 0.29  | 0.97  | 0.21 | 26.2 | 11.20 | 0.30  | 1.01  |
| 06035264+2942134 | 181.346  | 3.823    | 0.751 | 1      | -      | -    | -    | -        | -    | -      | -     | D4                     | e          | o          | -    | -        | -          | -     | 10.993                             | 0.44                        | 1.47                        | 1                    | 27.4                               | 0.86                                 | 3.62                          | 10.713                        | 0.32  | 1.09  | 0.23 | 28.9 | 10.73 | 0.34  | 1.14  |
| 06035375+3014457 | 180.874  | 4.091    | 6.787 | 8      | -      | -    | g    | -        | -    | -      | -     | -                      | -          | -          | -    | -        | -          | -     | 9.553                              | 1.24                        | 2.47                        | 1                    | 97.2                               | 0.42                                 | 3.76                          | 7.024                         | 0.11  | -0.90 | 2.10 | ...  | ...   | 0.25  | -0.45 |
| 06035490+3015257 | 180.866  | 4.100    | 6.985 | 9      | -      | -    | g    | -        | -    | -      | -     | -                      | -          | -          | -    | -        | -          | -     | 13.390                             | 0.51                        | 1.36                        | 1                    | 15.6                               | 1.00                                 | 3.76                          | 10.787                        | -0.65 | -2.11 | 2.16 | ...  | ...   | -0.51 | -1.65 |
| 06035621+3014327 | 180.881  | 4.097    | 6.535 | 9      | -      | -    | g    | -        | -    | -      | -     | -                      | -          | -          | -    | -        | -          | -     | 12.780                             | 0.78                        | 1.39                        | 1                    | 24.8                               | 0.58                                 | 3.76                          | 10.345                        | -0.30 | -1.86 | 2.02 | ...  | ...   | -0.17 | -1.43 |
| 06035830+3015327 | 180.870  | 4.112    | 6.777 | 9      | -      | -    | g    | -        | -    | -      | -     | -                      | -          | -          | -    | -        | -          | -     | 11.811                             | 0.61                        | 1.45                        | 1                    | 41.4                               | 0.58                                 | 3.76                          | 9.286                         | -0.51 | -1.92 | 2.10 | ...  | ...   | -0.38 | -1.47 |
| 06035853+3015097 | 180.876  | 4.109    | 6.643 | 9      | -      | -    | g    | -        | -    | -      | -     | -                      | -          | -          | -    | -        | -          | -     | 12.482                             | 0.49                        | 0.94                        | 1                    | 53.6                               | 0.20                                 | 3.76                          | 10.007                        | -0.61 | -2.36 | 2.06 | ...  | ...   | -0.48 | -1.92 |
| 06035892+3016147 | 180.861  | 4.119    | 6.918 | 9      | -      | -    | g    | -        | -    | -      | -     | -                      | -          | -          | -    | -        | -          | -     | 12.380                             | 0.39                        | 1.23                        | 1                    | 25.6                               | 0.54                                 | 3.76                          | 9.802                         | -0.76 | -2.21 | 2.14 | ...  | ...   | -0.62 | -1.75 |
| 06035923+3016317 | 180.858  | 4.123    | 6.930 | 9      | -      | -    | g    | -        | -    | -      | -     | -                      | -          | -          | -    | -        | -          | -     | 11.214                             | 0.86                        | 2.01                        | 1                    | 44.4                               | 0.86                                 | 3.76                          | 8.632                         | -0.28 | -1.43 | 2.15 | ...  | ...   | -0.15 | -0.98 |
| 06041012+3020237 | 180.820  | 4.188    | 3.825 | 8      | -      | -    | g    | -        | -    | -      | -     | -                      | -          | -          | -    | -        | -          | -     | 12.053                             | 1.06                        | 2.74                        | 1                    | 14.0                               | 0.90                                 | 3.76                          | 10.628                        | 0.43  | 0.84  | 1.18 | ...  | ...   | 0.50  | 1.09  |
| 06041049+3129322 | 179.811  | 4.750    | 0.803 | 9      | -      | -    | g    | -        | -    | -      | -     | -                      | -          | -          | -    | -        | -          | -     | 11.265                             | 0.43                        | 1.33                        | 1                    | 55.6                               | 0.80                                 | 3.71                          | 10.966                        | 0.30  | 0.93  | 0.25 | ...  | ...   | 0.31  | 0.99  |
| 06041759+0946030 | 198.807  | -5.843   | 0.436 | 1      | -      | -    | g    | -        | -    | -      | -     | D3                     | c          | o          | -    | -        | -          | -     | 11.412                             | 0.42                        | 1.30                        | 1                    | 35.2                               | 0.82                                 | 3.60                          | 11.250                        | 0.35  | 1.08  | 0.14 | 36.3 | 11.26 | 0.36  | 1.11  |
| 06042948+4130325 | 170.970  | 9.592    | 0.262 | 1      | -      | -    | g    | -        | -    | -      | -     | D4                     | c          | o          | -    | -        | -          | -     | 11.160                             | 0.38                        | 1.12                        | 1                    | 33.0                               | 0.80                                 | 3.40                          | 11.062                        | 0.34  | 0.99  | 0.08 | 33.4 | 11.07 | 0.35  | 1.01  |
| 06043221+3055063 | 180.352  | 4.539    | 0.682 | 1      | -      | -    | g    | -        | -    | -      | -     | D1                     | e          | o          | -    | -        | -          | -     | 11.188                             | 0.37                        | 1.31                        | 1                    | 39.6                               | 0.44                                 | 3.57                          | 10.934                        | 0.26  | 0.97  | 0.21 | 41.6 | 10.95 | 0.27  | 1.02  |
| 06043266+3031093 | 180.703  | 4.346    | 8.311 | 9      | -      | -    | g    | -        | -    | -      | -     | -                      | -          | -          | -    | -        | -          | -     | 11.034                             | 1.04                        | 2.44                        | 1                    | 89.4                               | 0.10                                 | 3.69                          | 7.937                         | -0.33 | -1.69 | 2.57 | ...  | ...   | -0.17 | -1.14 |
| 06043474+3028313 | 180.745  | 4.331    | 6.949 | 4      | -      | -    | g    | -        | -    | N      | -     | D1                     | -          | -          | -    | -        | -          | -     | 13.592                             | 0.76                        | 1.99                        | -1                   | 10.6                               | 1.00                                 | 3.69                          | 11.003                        | -0.39 | -1.47 | 2.15 | 34.5 | 10.42 | -0.26 | -1.01 |
| 06043652+3030533 | 180.713  | 4.356    | 8.695 | 9      | -      | -    | g    | -        | -    | -      | -     | -                      | -          | -          | -    | -        | -          | -     | 8.455                              | 1.16                        | 2.26                        | 1                    | 219.8                              | 0.50                                 | 3.69                          | 5.215                         | -0.28 | -2.06 | 2.69 | ...  | ...   | -0.11 | -1.49 |
| 06043691+3031513 | 180.700  | 4.365    | 8.109 | 9      | -      | -    | g    | -        | -    | -      | -     | -                      | -          | -          | -    | -        | -          | -     | 12.072                             | ...                         | 1.44                        | -2                   | 34.6                               | 1.00                                 | 3.69                          | 9.051                         | ...   | -2.59 | 2.51 | ...  | ...   | ...   | -2.05 |
| 06043722+3030253 | 180.721  | 4.355    | 8.453 | 9      | -      | -    | g    | -        | -    | -      | -     | -                      | -          | -          | -    | -        | -          | -     | 9.640                              | 1.12                        | 2.67                        | 1                    | 182.4                              | 0.10                                 | 3.69                          | 6.490                         | -0.28 | -1.53 | 2.62 | ...  | ...   | -0.12 | -0.97 |
| 06043745+3029533 | 180.730  | 4.351    | 8.094 | 9      | -      | -    | g    | -        | -    | -      | -     | -                      | -          | -          | -    | -        | -          | -     | 12.472                             | 1.11                        | ...                         | 1                    | 37.4                               | 0.46                                 | 3.69                          | 9.456                         | -0.23 | ...   | 2.51 | ...  | ...   | -0.07 | ...   |
| 06044670+3013571 | 180.979  | 4.251    | 1.515 | 9      | -      | -    | g    | -        | -    | -      | -     | -                      | -          | -          | -    | -        | -          | -     | 11.589                             | 0.43                        | 1.10                        | -2                   | 41.2                               | 0.60                                 | 3.62                          | 11.025                        | 0.18  | 0.35  | 0.47 | ...  | ...   | 0.21  | 0.45  |
| 06045193+0656185 | 201.372  | -7.077   | 0.434 | 1      | -      | -    | g    | -        | -    | -      | -     | D3                     | c          | o          | -    | -        | -          | -     | 10.631                             | 0.36                        | 1.25                        | 1                    | 41.2                               | 0.76                                 | 3.52                          | 10.469                        | 0.29  | 1.03  | 0.13 | 42.2 | 10.48 | 0.29  | 1.06  |
| 06045592+2201120 | 188.168  | 0.269    | 1.035 | 1      | -      | -    | g    | -        | -    | -      | -     | D1                     | c          | o          | -    | -        | -          | -     | 11.132                             | 0.51                        | 1.46                        | 1                    | 43.2                               | 0.52                                 | 3.65                          | 10.746                        | 0.34  | 0.94  | 0.32 | 47.3 | 10.75 | 0.36  | 1.01  |
| 06051202+3201231 | 179.451  | 5.198    | 0.836 | 1      | -      | -    | g    | -        | -    | -      | -     | D1                     | c          | o          | -    | -        | -          | -     | 11.164                             | 0.53                        | 1.43                        | 1                    | 40.8                               | 0.50                                 | 3.52                          | 10.853                        | 0.39  | 1.02  | 0.26 | 43.8 | 10.86 | 0.40  | 1.07  |
| 06051457+3047491 | 180.532  | 4.612    | 0.869 | 8      | -      | -    | g    | -        | -    | -      | -     | -                      | -          | -          | -    | -        | -          | -     | 10.599                             | 1.28                        | 2.50                        | 1                    | 38.4                               | 0.60                                 | 3.54                          | 10.275                        | 1.14  | 2.07  | 0.27 | ...  | ...   | 1.16  | 2.13  |
| 06051642+0535242 | 202.616  | -7.631   | 0.442 | 1      | -      | -    | g    | -        | -    | -      | -     | D1                     | c          | o          | -    | -        | -          | -     | 11.415                             | 0.38                        | 1.22                        | 1                    | 45.4                               | 0.50                                 | 3.52                          | 11.250                        | 0.31  | 1.00  | 0.14 | 46.9 | 11.25 | 0.32  | 1.03  |
| 06052948+0940512 | 199.026  | -5.626   | 0.445 | 1      | -      | -    | g    | -        | -    | -      | -     | D1                     | c          | o          | -    | -        | -          | -     | 10.830                             | 0.38                        | 1.32                        | 1                    | 51.4                               | 0.30                                 | 3.52                          | 10.664                        | 0.31  | 1.10  | 0.14 | 52.8 | 10.68 | 0.32  | 1.13  |
| 06053254+2941454 | 181.530  | 4.135    | 1.001 | 2      | o      | -    | -    | -        | N    | -      | -     | D4                     | e          | o          | -    | -        | o          | -     | 11.066                             | 0.50                        | 1.50                        | -2                   | 52.2                               | 0.48                                 | 3.45                          | 10.693                        | 0.33  | 1.00  | 0.31 | 59.0 | 10.61 | 0.35  | 1.06  |
| 06055381+2807514 | 182.938  | 3.443    | 0.355 | 1      | -      | -    | g    | -        | -    | -      | -     | D1                     | c          | o          | -    | -        | -          | -     | 11.042                             | 0.34                        | 1.16                        | 1                    | 54.8                               | 0.28                                 | 3.63                          | 10.910                        | 0.28  | 0.98  | 0.11 | 56.0 | 10.92 | 0.29  | 1.01  |
| 06060282+3003307 | 181.265  | 4.406    | 0.873 | 1      | -      | -    | g    | -        | -    | N      | -     | D2                     | e          | o          | -    | -        | -          | -     | 10.818                             | 0.64                        | 1.93                        | 1                    | 46.4                               | 0.60                                 | 3.53                          | 10.493                        | 0.49  | 1.50  | 0.27 | 50.1 | 10.49 | 0.51  | 1.56  |
| 06061308+3102377 | 180.417  | 4.915    | 0.789 | 1      | -      | -    | g    | -        | -    | -      | -     | D2                     | e          | o          | -    | -        | -          | -     | 11.428                             | 0.50                        | 1.51                        | 1                    | 33.8                               | 0.64                                 | 3.55                          | 11.134                        | 0.37  | 1.12  | 0.24 | 36.0 | 11.14 | 0.39  | 1.17  |
| 06062432+3147327 | 179.778  | 5.310    | 0.790 | 1      | -      | -    | g    | -        | -    | -      | -     | D2                     | c          | o          | -    | -        | -          | -     | 10.301                             | 0.40                        | 1.40                        | 1                    | 47.8                               | 0.92                                 | 3.55                          | 10.007                        | 0.27  | 1.01  | 0.24 | 50.6 | 10.03 | 0.29  | 1.06  |
| 06063865+2839196 | 182.559  | 3.841    | 0.555 | 1      | -      | -    | g    | -        | -    | -      | -     | D1                     | e          | o          | -    | -        | -          | -     | 11.211                             | 0.36                        | 1.24                        | 1                    | 38.4                               | 0.98                                 | 3.46                          | 11.004                        | 0.27  | 0.97  | 0.17 | 39.9 | 11.01 | 0.28  | 1.01  |
| 06064363+1820200 | 191.586  |          |       |        |        |      |      |          |      |        |       |                        |            |            |      |          |            |       |                                    |                             |                             |                      |                                    |                                      |                               |                               |       |       |      |      |       |       |       |

Table B1: a) continued.

| 2MASX J          | <i>l</i>    | <i>b</i>    | EBV        | Object       | Sample     | Disc        | 2MRS        | Velocity   | NIR         | Photom        | Ext         | <i>K</i> <sub>20</sub> | <i>H-K</i>   | <i>J-K</i>  | <i>vc</i>    | <i>a</i>     | <i>b/a</i>   | std. | <i>K</i> <sub>s</sub> <sup>o</sup> | ( <i>H-K</i> ) <sup>o</sup> | ( <i>J-K</i> ) <sup>o</sup> | <i>A<sub>K</sub></i> | <i>a</i> <sup>d</sup> | <i>K</i> <sub>s</sub> <sup>o,d</sup> | ( <i>H-K</i> ) <sup>o,c</sup> | ( <i>J-K</i> ) <sup>o,c</sup> |             |             |           |             |             |             |       |
|------------------|-------------|-------------|------------|--------------|------------|-------------|-------------|------------|-------------|---------------|-------------|------------------------|--------------|-------------|--------------|--------------|--------------|------|------------------------------------|-----------------------------|-----------------------------|----------------------|-----------------------|--------------------------------------|-------------------------------|-------------------------------|-------------|-------------|-----------|-------------|-------------|-------------|-------|
| (1)              | deg<br>(2a) | deg<br>(2b) | mag<br>(3) | class<br>(4) | off<br>(5) | flag<br>(6) | gal<br>(7a) | TF<br>(7b) | obs<br>(7c) | ext'd<br>(7d) | type<br>(8) | (9)                    | Opt<br>(10a) | HI<br>(10b) | flag<br>(11) | flag<br>(12) | flag<br>(13) | (14) | (15)                               | (16)                        | (17)                        | (18)                 | (19)                  | (20)                                 | mag<br>(21)                   | mag<br>(22)                   | mag<br>(23) | mag<br>(24) | "<br>(25) | mag<br>(26) | mag<br>(27) | mag<br>(28) |       |
| 06085119+2138157 | 188.945     | 0.877       | 17.590     | 9            | -          | -           | -           | -          | -           | -             | -           | -                      | -            | -           | -            | -            | -            | -    | 11.393                             | ...                         | ...                         | 1                    | 56.2                  | 1.00                                 | 3.76                          | 8.239                         | ...         | ...         | 5.45      | ...         | ...         | ...         |       |
| 06085126+2029257 | 189.949     | 0.321       | 10.911     | 9            | -          | -           | -           | -          | -           | -             | -           | -                      | -            | -           | -            | -            | -            | -    | 12.126                             | 2.08                        | ...                         | 1                    | 15.4                  | 0.54                                 | 3.86                          | 8.061                         | 0.27        | ...         | 3.38      | ...         | ...         | 0.49        |       |
| 06085134+2139117 | 188.932     | 0.885       | 17.853     | 9            | -          | -           | -           | -          | -           | -             | -           | -                      | -            | -           | -            | -            | -            | -    | 12.637                             | 1.24                        | 2.72                        | 1                    | 27.6                  | 0.54                                 | 3.76                          | 5.985                         | -1.72       | -6.15       | 5.53      | ...         | ...         | -4.97       |       |
| 06085162+2030347 | 189.933     | 0.332       | 12.229     | 9            | -          | -           | -           | -          | -           | -             | -           | -                      | -            | -           | -            | -            | -            | -    | 13.644                             | 1.15                        | ...                         | -1                   | 10.0                  | 1.00                                 | 3.86                          | 9.087                         | -0.88       | ...         | 3.79      | ...         | ...         | -0.64       |       |
| 06085300+2142427 | 188.884     | 0.919       | 9.720      | 9            | -          | -           | -           | -          | -           | -             | -           | -                      | -            | -           | -            | -            | -            | -    | 14.180                             | ...                         | ...                         | -1                   | 10.0                  | 1.00                                 | 3.76                          | 10.558                        | ...         | ...         | 3.01      | ...         | ...         | ...         |       |
| 06085342+2138277 | 188.947     | 0.886       | 16.941     | 9            | -          | -           | -           | -          | -           | -             | -           | -                      | -            | -           | -            | -            | -            | -    | 7.250                              | 1.37                        | 2.89                        | 1                    | 194.8                 | 0.40                                 | 3.76                          | 0.938                         | -1.44       | -5.53       | 5.25      | ...         | ...         | -1.10       | -4.41 |
| 06085476+1654420 | 193.087     | -1.401      | 2.839      | 9            | -          | -           | -           | -          | -           | -             | -           | -                      | -            | -           | -            | -            | -            | -    | 12.152                             | 0.62                        | 1.42                        | 1                    | 12.2                  | 0.58                                 | 3.57                          | 11.094                        | 0.15        | 0.01        | 0.88      | ...         | ...         | 0.20        | 0.20  |
| 06085585+2136487 | 188.975     | 0.881       | 16.143     | 9            | -          | -           | -           | -          | -           | -             | -           | -                      | -            | -           | -            | -            | -            | -    | 14.132                             | 0.59                        | 1.63                        | -1                   | 10.0                  | 1.00                                 | 3.76                          | 8.117                         | -2.08       | -6.39       | 5.00      | ...         | ...         | -1.77       | -5.33 |
| 06085642+3147243 | 180.039     | 5.782       | 0.665      | 1            | -          | -           | g           | -          | -           | -             | D2          | c                      | o            | -           | -            | -            | -            | -    | 11.291                             | 0.49                        | 1.49                        | 1                    | 37.6                  | 0.54                                 | 3.57                          | 11.043                        | 0.38        | 1.16        | 0.21      | 39.5        | 11.05       | 0.39        | 1.21  |
| 06085658+2138307 | 188.952     | 0.897       | 15.496     | 9            | -          | -           | -           | -          | -           | -             | -           | -                      | -            | -           | -            | -            | -            | -    | 9.642                              | 1.43                        | 3.14                        | 1                    | 84.4                  | 0.74                                 | 3.76                          | 3.868                         | -1.14       | -4.56       | 4.80      | ...         | ...         | -0.84       | -3.54 |
| 06085882+2138463 | 188.952     | 0.907       | 14.497     | 9            | -          | -           | -           | -          | -           | -             | -           | -                      | -            | -           | -            | -            | -            | -    | 12.122                             | 1.58                        | ...                         | 1                    | 58.8                  | 0.24                                 | 3.66                          | 6.720                         | -0.82       | ...         | 4.49      | ...         | ...         | -0.54       | ...   |
| 06085995+1543230 | 194.137     | -1.958      | 6.630      | 2            | -          | -           | g           | t          | N           | -             | n           | -                      | -            | -           | U            | -            | e            | -    | 12.300                             | 0.55                        | 2.05                        | -2                   | 34.4                  | 0.56                                 | 3.58                          | 10.947                        | -0.06       | 0.24        | 1.12      | 59.3        | 10.69       | 0.02        | 0.48  |
| 06090147+2137393 | 188.970     | 0.907       | 12.705     | 9            | -          | -           | -           | -          | -           | -             | -           | -                      | -            | -           | U            | -            | -            | -    | 14.170                             | ...                         | ...                         | -1                   | 10.0                  | 1.00                                 | 3.66                          | 9.436                         | ...         | ...         | 3.94      | ...         | ...         | ...         |       |
| 06090334+2137313 | 188.979     | 0.912       | 11.646     | 9            | -          | -           | -           | -          | -           | -             | -           | -                      | -            | -           | -            | -            | -            | -    | 13.032                             | 1.27                        | ...                         | 1                    | 14.4                  | 0.64                                 | 3.66                          | 8.693                         | -0.66       | ...         | 3.61      | ...         | ...         | -0.43       | ...   |
| 06090459+2039063 | 189.833     | 0.445       | 19.420     | 9            | -          | -           | -           | -          | -           | -             | -           | -                      | -            | -           | -            | -            | -            | -    | 14.238                             | 0.49                        | 0.98                        | -1                   | 10.0                  | 1.00                                 | 3.85                          | 7.002                         | -2.72       | -8.67       | 6.02      | ...         | ...         | -2.34       | -7.39 |
| 06090545+2029293 | 189.975     | 0.370       | 11.095     | 9            | -          | -           | -           | -          | -           | -             | -           | -                      | -            | -           | U            | -            | -            | -    | 12.324                             | 1.07                        | 2.19                        | 1                    | 38.6                  | 0.26                                 | 3.72                          | 8.190                         | -0.77       | -3.32       | 3.44      | ...         | ...         | -0.55       | -2.59 |
| 06090615+2042143 | 189.790     | 0.476       | 15.925     | 8            | -          | -           | -           | -          | -           | -             | -           | -                      | -            | -           | -            | -            | -            | -    | 12.572                             | 0.96                        | 2.84                        | 1                    | 22.2                  | 0.68                                 | 3.85                          | 6.638                         | -1.67       | -5.07       | 4.93      | ...         | ...         | -1.36       | -4.02 |
| 06090637+2029483 | 189.972     | 0.376       | 11.196     | 9            | -          | -           | -           | -          | -           | -             | -           | -                      | -            | -           | -            | -            | -            | -    | 13.031                             | 0.67                        | 1.97                        | -1                   | 20.0                  | 0.40                                 | 3.72                          | 8.859                         | -1.18       | -3.60       | 3.47      | ...         | ...         | -0.96       | -2.86 |
| 06090714+2150343 | 188.796     | 1.030       | 9.751      | 9            | -          | -           | -           | -          | -           | -             | -           | -                      | -            | -           | -            | -            | -            | -    | 8.624                              | 1.38                        | 3.11                        | 1                    | 95.8                  | 0.58                                 | 3.75                          | 4.991                         | -0.23       | -1.73       | 3.02      | ...         | ...         | -0.04       | -1.09 |
| 06090758+2029173 | 189.982     | 0.376       | 10.748     | 9            | -          | -           | -           | -          | -           | -             | -           | -                      | -            | -           | -            | -            | -            | -    | 13.411                             | 0.83                        | 1.66                        | -1                   | 14.8                  | 0.40                                 | 3.72                          | 9.406                         | -0.95       | -3.68       | 3.33      | ...         | ...         | -0.74       | -2.97 |
| 06090908+2150563 | 188.794     | 1.040       | 10.266     | 9            | -          | -           | -           | -          | -           | -             | -           | -                      | -            | -           | -            | -            | -            | -    | 12.260                             | ...                         | ...                         | 1                    | 29.4                  | 1.0                                  | 3.75                          | 8.435                         | ...         | ...         | 3.18      | ...         | ...         | ...         | ...   |
| 06091137+2150523 | 188.799     | 1.047       | 9.653      | 9            | -          | -           | -           | -          | -           | -             | -           | -                      | -            | -           | -            | -            | -            | -    | 13.217                             | 0.59                        | 2.29                        | 1                    | 14.6                  | 0.64                                 | 3.75                          | 9.620                         | -1.01       | -2.50       | 2.99      | ...         | ...         | -0.82       | -1.86 |
| 06091178+2026533 | 190.025     | 0.371       | 8.784      | 8            | -          | -           | -           | -          | -           | -             | -           | -                      | -            | -           | -            | -            | -            | -    | 13.270                             | 0.70                        | 1.80                        | 2                    | 23.2                  | 0.42                                 | 3.72                          | 9.997                         | -0.76       | -2.56       | 2.72      | ...         | ...         | -0.59       | -1.99 |
| 06091777+2039203 | 189.855     | 0.492       | 19.859     | 9            | -          | -           | -           | -          | -           | -             | -           | -                      | -            | -           | -            | -            | -            | -    | 11.276                             | 0.62                        | 1.77                        | 1                    | 45.8                  | 0.86                                 | 3.85                          | 3.877                         | -2.67       | -8.09       | 6.15      | ...         | ...         | -2.28       | -6.78 |
| 06091791+2150493 | 188.812     | 1.069       | 7.531      | 9            | -          | -           | -           | -          | -           | -             | -           | -                      | -            | -           | -            | -            | -            | -    | 11.152                             | 1.34                        | 2.91                        | 1                    | 38.8                  | 0.76                                 | 3.75                          | 8.346                         | 0.10        | -0.83       | 2.33      | ...         | ...         | 0.24        | -0.34 |
| 06091877+2039443 | 189.851     | 0.498       | 20.185     | 9            | -          | -           | -           | -          | -           | -             | -           | -                      | -            | -           | -            | -            | -            | -    | 9.562                              | 0.87                        | 1.97                        | 1                    | 102.4                 | 0.22                                 | 3.85                          | 2.041                         | -2.47       | -8.06       | 6.25      | ...         | ...         | -2.07       | -6.73 |
| 06092083+2038453 | 189.869     | 0.497       | 19.546     | 9            | -          | -           | -           | -          | -           | -             | -           | -                      | -            | -           | -            | -            | -            | -    | 8.015                              | 0.95                        | 2.09                        | 1                    | 231.4                 | 0.74                                 | 3.85                          | 0.732                         | -2.28       | -7.63       | 6.05      | ...         | ...         | -1.90       | -6.34 |
| 06092161+2123213 | 189.220     | 0.860       | 2.023      | 8            | -          | -           | -           | -          | -           | -             | -           | -                      | -            | -           | U            | -            | -            | -    | 11.734                             | 1.15                        | 2.53                        | 1                    | 17.4                  | 0.46                                 | 3.66                          | 10.980                        | 0.81        | 1.53        | 0.63      | ...         | ...         | 0.85        | 1.66  |
| 06092397+2039163 | 189.867     | 0.512       | 20.266     | 9            | -          | -           | -           | -          | -           | -             | -           | -                      | -            | -           | -            | -            | -            | -    | 8.501                              | 1.00                        | 2.14                        | 1                    | 168.6                 | 0.62                                 | 3.85                          | 0.950                         | -2.36       | -7.92       | 6.28      | ...         | ...         | -1.96       | -6.59 |
| 06092468+2040113 | 189.855     | 0.522       | 20.568     | 9            | -          | -           | -           | -          | -           | -             | -           | -                      | -            | -           | -            | -            | -            | -    | 8.765                              | 1.10                        | 2.22                        | 1                    | 1220.0                | 0.32                                 | 3.85                          | 1.101                         | -2.30       | -8.00       | 6.37      | ...         | ...         | -1.90       | -6.64 |
| 06092756+1338133 | 196.020     | -2.868      | 2.935      | 1            | -          | -           | g           | -          | -           | -             | D3          | -                      | -            | -           | -            | e?           | -            | -    | 12.290                             | 0.57                        | 1.72                        | 1                    | 19.4                  | 0.80                                 | 3.63                          | 11.196                        | 0.08        | 0.26        | 0.91      | 28.0        | 11.10       | 0.14        | 0.46  |
| 06093663+0729211 | 201.450     | -5.780      | 0.455      | 1            | -          | -           | -           | -          | -           | -             | D3          | c                      | o            | -           | -            | -            | -            | -    | 10.928                             | 0.45                        | 1.30                        | 1                    | 42.8                  | 0.82                                 | 3.56                          | 10.758                        | 0.37        | 1.07        | 0.14      | 44.0        | 10.77       | 0.38        | 1.10  |
| 06093817+2037172 | 189.923     | 0.545       | 12.468     | 9            | -          | -           | g           | -          | -           | -             | -           | -                      | -            | -           | -            | -            | -            | -    | 13.817                             | 0.84                        | 1.91                        | -1                   | 13.0                  | 1.00                                 | 3.88                          | 9.171                         | -1.23       | -4.28       | 3.86      | ...         | ...         | -0.98       | -3.46 |
| 06094969+2138111 | 189.056     | 1.075       | 2.399      | 9            | -          | -           | -           | -          | -           | -             | -           | -                      | -            | -           | -            | -            | -            | -    | 11.461                             | 1.60                        | ...                         | 1                    | 48.0                  | 0.62                                 | 3.71                          | 10.570                        | 1.21        | ...         | 0.74      | ...         | ...         | 1.26        | ...   |
| 06095101+1839501 | 191.661     | -0.358      | 1.819      | 1            | -          | -           | g           | t          | N           | -             | -           | -                      | -            | -           | U            | -            | -            | -    | 11.693                             | 0.75                        | 2.23                        | 1                    | 24.8                  | 0.56                                 | 3.62                          | 11.015                        | 0.45        | 1.33        | 0.56      | 30.1        | 10.99       | 0.49        | 1.45  |
| 06095168+2030061 | 190.053     | 0.533       | 12.507     | 9            | -          | -           | -           | -          | -           | -             | -           | -                      | -            | -           | -            | -            | -            | -    | 8.121                              | 0.91                        | 1.83                        | 1                    | 141.2                 | 0.70                                 | 3.88                          | 3.461                         | -1.16       | -4.39       | 3.87      | ...         | ...         | -0.92       | -3.56 |
| 06095325+2030471 | 190.046     | 0.544       | 12.821     | 9            | -          | -           | -           | -          | -           | -             | -           | -                      | -            | -           | -            | -            | -            | -    | 9.754                              | 0.78                        | 1.85                        | 1                    | 70.0                  | 0.64                                 | 3.88                          | 4.977                         | -1.35       | -4.52       | 3.97      | ...         | ...         | -1.09       | -3.68 |
| 06095948+1910113 | 191.234     | -0.084      | 1.572      | 1            | -          | -           | g           | t          | N           | -             | D3          | -                      | -            | -           | U            | -            | -            | -    | 10.923                             | 0.61                        | 1.89                        | 1                    | 38.4                  | 0.58                                 | 3.63                          | 10.337                        | 0.35        | 1.11        | 0.49      | 44.3        | 10.35       | 0.38        | 1.21  |
| 06100449+2029063 | 190.092     | 0.569       | 9.322      | 2            | -          | -           | g           | t          | N           | -             | D1          | -                      | -            | -           | -            | e            | -            | -    | 13.588                             | 0.68                        | ...                         | -1                   | 17.8                  | 0.58                                 | 3.64                          | 10.115                        | -0.87       | ...         | 2.89      | 104.2       | 9.09        | -0.69       | ...   |
| 06100794+2018075 | 199.030     | -4.325      | 0.600      | 1            | -          | -           | g           | t          | N           | -             | D1          | e                      | o            | -           | -            | -            | -            | -    | 10.937                             | 0.40                        | 1.27                        | 1                    | 42.8                  | 0.44                                 | 3.61                          | 10.713                        | 0.30        | 0.97        | 0.19      | 44.5        | 10.73       | 0.32        | 1.01  |
| 06101251+1248483 | 196.830     | -3.104      | 5.131      | 8            | -          | -           | g           | t          | -           | -             | -           | -                      | -            | -           | -            | -            | -            | -    | 8.692                              | 0.75                        | 1.75                        | 1                    | 89.6                  | 0.90                                 | 3.73                          | 6.780                         | -0.10       | -0.80       | 1.59      | ...         | ...         | -0.00       | -0.46 |
| 06101533+1641123 | 193.439     | -1.228      | 3.113      | 9            | -          | -           | -           | -          | -           | -             | -           | -                      | -            | -           | U            | -            | -            | -    | 12.157                             | 1.11                        | 2.55                        | 1                    | 22.2                  | 0.64                                 | 3.70                          | 10.997                        | 0.59        | 1.00        | 0.96      | ...         | ...         | 0.65        | 1.21  |
| 06101886+3227276 | 179.587     | 6.355       | 0.626      | 1            | -          | -           | g           | t          | N           | -             | D1          | c                      | o            | -           | -            | -            | -            | -    | 11.090                             | 0.37                        | 1.24                        | 1                    | 45.0                  | 0.40                                 | 3.56                          | 10.857                        | 0.27        | 0.93        | 0.19      | 47.3        | 10.86       | 0.28        | 0.97  |
| 06102125+1642343 | 193.430     | -1.196      | 3.599      | 7            | -          | -           | -           | -          | -           | -             | -           | -                      | -            | -           | U            | -            | -            | -    | 11.794                             | 1.50                        | 3.23                        | 1                    | 18.0                  | 0.78                                 | 3.70                          | 10.453                        | 0.90        | 1.44        | 1.11      | ...         | ...         | 0.97        | 1.68  |
| 06102428+2033462 | 190.061     | 0.674       | 5.525      | 8            | -          | -           | -           | -          | -           | -             | -           | -                      | -            | -           | U            | -            | -            | -    | 12.816                             | 1.45                        | ...                         | 1                    | 11.6                  | 1.00                                 | 3.64                          | 10.757                        | 0.53        | ...         | 1.71      | ...         | ...         | 0.64        | ...   |
| 06102654+1643213 | 193.429     | -1.172      | 3.874      | 9            | -          | -           | -           | -          | -           | -             | -           | -                      | -            | -           | U            |              |              |      |                                    |                             |                             |                      |                       |                                      |                               |                               |             |             |           |             |             |             |       |

2M-ZoA galaxy catalogue description and analysis 53

Table B1: a) continued.

[illegible]



Table B1: a) continued.

| 2MASX J          |         | <i>l</i>    | <i>b</i>    | EBV        | Object       | Sample     |            |             |            | Disc        | 2MRS          | Velocity    |     | NIR          | Photom      | Ext         | <i>K</i> <sub>20</sub> | <i>H-K</i>  | <i>J-K</i>  | <i>vc</i>   | <i>a</i>    | <i>b/a</i> | std.d.    | <i>K</i> <sub>S</sub> <sup>o</sup> | ( <i>H-K</i> ) <sup>o</sup> | ( <i>J-K</i> ) <sup>o</sup> | <i>A<sub>K</sub></i> | <i>a</i> <sup>d</sup> | <i>K</i> <sub>S</sub> <sup>o,d</sup> | ( <i>H-K</i> ) <sup>o,c</sup> | ( <i>J-K</i> ) <sup>o,c</sup> |             |             |
|------------------|---------|-------------|-------------|------------|--------------|------------|------------|-------------|------------|-------------|---------------|-------------|-----|--------------|-------------|-------------|------------------------|-------------|-------------|-------------|-------------|------------|-----------|------------------------------------|-----------------------------|-----------------------------|----------------------|-----------------------|--------------------------------------|-------------------------------|-------------------------------|-------------|-------------|
| (1)              | (2)     | deg<br>(2a) | deg<br>(2b) | mag<br>(3) | class<br>(4) | off<br>(5) | flg<br>(6) | gal<br>(7a) | TF<br>(7b) | obs<br>(7c) | ext'd<br>(7d) | type<br>(8) | (9) | Opt<br>(10a) | HI<br>(10b) | flg<br>(11) | flg<br>(12)            | flg<br>(13) | mag<br>(14) | mag<br>(15) | mag<br>(16) | (17)       | "<br>(18) | (19)                               | (20)                        | mag<br>(21)                 | mag<br>(22)          | mag<br>(23)           | mag<br>(24)                          | "<br>(25)                     | mag<br>(26)                   | mag<br>(27) | mag<br>(28) |
| 06153508+1417047 | 196.163 | -1.253      | 4.006       | 8          | -            | -          | -          | -           | -          | -           | -             | -           | -   | -            | -           | U           | -                      | -           | 10.522      | 1.48        | 2.91        | 1          | 38.2      | 0.74                               | 3.71                        | 9.029                       | 0.82                 | 0.92                  | 1.24                                 | ...                           | ...                           | 0.90        | 1.18        |
| 06160217+2439014 | 187.089 | 0.788       | 3.769       | 1          | -            | -          | -          | g           | -          | -           | -             | -           | -   | -            | -           | U           | -                      | -           | 11.479      | 0.43        | 1.35        | 1          | 24.6      | 0.94                               | 3.58                        | 11.185                      | 0.30                 | 0.96                  | 0.24                                 | 26.1                          | 11.20                         | 0.31        | 1.01        |
| 06160639+1659496 | 193.838 | 0.149       | 1.481       | 1          | -            | -          | -          | g           | -          | -           | -             | -           | -   | -            | -           | U           | -                      | -           | 10.744      | 0.50        | 1.69        | 1          | 37.4      | 0.84                               | 3.62                        | 10.192                      | 0.25                 | 0.96                  | 0.46                                 | 42.6                          | 10.21                         | 0.28        | 1.05        |
| 06162063+0717492 | 202.413 | -4.401      | 1.501       | 1          | -            | -          | -          | g           | -          | N           | -             | -           | -   | -            | -           | U           | -                      | -           | 9.020       | 0.36        | 1.24        | 1          | 96.0      | 0.42                               | 3.59                        | 8.833                       | 0.28                 | 0.99                  | 0.16                                 | 98.5                          | 8.86                          | 0.29        | 1.03        |
| 06162384+2418084 | 187.436 | 3.677       | 1.046       | 8          | -            | -          | -          | g           | -          | -           | -             | -           | -   | -            | -           | U           | -                      | -           | 11.359      | 0.59        | 1.03        | 1          | 50.8      | 0.72                               | 3.62                        | 10.969                      | 0.42                 | 0.51                  | 0.32                                 | ...                           | ...                           | 0.44        | 0.58        |
| 06162583+1654326 | 193.952 | 0.176       | 1.534       | 1          | -            | -          | -          | g           | -          | t           | N             | -           | -   | -            | -           | U           | -                      | -           | 11.588      | 0.53        | 1.60        | 1          | 37.6      | 0.60                               | 3.66                        | 11.016                      | 0.28                 | 0.83                  | 0.48                                 | 44.9                          | 10.96                         | 0.31        | 0.93        |
| 06163176+2347234 | 187.902 | 3.461       | 0.846       | 8          | -            | -          | -          | g           | -          | -           | -             | -           | -   | -            | -           | U           | -                      | -           | 10.154      | 1.65        | 3.19        | 1          | 28.6      | 0.82                               | 3.61                        | 9.839                       | 1.51                 | 2.77                  | 0.26                                 | ...                           | ...                           | 1.53        | 2.83        |
| 06163296+2434424 | 187.208 | 3.838       | 0.831       | 1          | -            | -          | -          | g           | -          | -           | -             | -           | -   | -            | -           | U           | -                      | -           | 10.799      | 0.44        | 1.33        | 1          | 44.0      | 0.82                               | 3.59                        | 10.489                      | 0.30                 | 0.92                  | 0.26                                 | 47.0                          | 10.50                         | 0.32        | 0.97        |
| 06163504+2231504 | 189.020 | 2.877       | 2.093       | 9          | -            | -          | -          | g           | -          | -           | -             | -           | -   | -            | -           | U           | -                      | -           | 10.645      | 1.99        | 2.91        | 1          | 72.8      | 0.50                               | 3.62                        | 9.865                       | 1.65                 | 1.87                  | 0.65                                 | ...                           | ...                           | 1.69        | 2.01        |
| 06163615+1058407 | 199.193 | -2.605      | 0.700       | 1          | -            | -          | -          | g           | -          | N           | -             | -           | -   | -            | -           | U           | -                      | -           | 9.355       | 0.48        | 1.42        | 1          | 72.4      | 0.64                               | 3.64                        | 9.094                       | 0.37                 | 1.07                  | 0.22                                 | 75.5                          | 9.12                          | 0.38        | 1.12        |
| 06164227+2233596 | 189.001 | 2.918       | 2.140       | 9          | -            | -          | -          | g           | -          | -           | -             | -           | -   | -            | -           | U           | -                      | -           | 11.815      | 1.68        | 2.34        | 1          | 42.4      | 0.42                               | 3.78                        | 11.018                      | 1.33                 | 1.27                  | 0.66                                 | ...                           | ...                           | 1.37        | 1.41        |
| 06164249+2232056 | 189.029 | 2.904       | 2.061       | 9          | -            | -          | -          | g           | -          | -           | -             | -           | -   | -            | -           | U           | -                      | -           | 9.656       | 2.32        | 3.57        | 1          | 78.8      | 0.44                               | 3.78                        | 8.888                       | 1.98                 | 2.55                  | 0.64                                 | ...                           | ...                           | 2.02        | 2.69        |
| 06164401+2232466 | 189.023 | 2.915       | 2.087       | 9          | -            | -          | -          | g           | -          | -           | -             | -           | -   | -            | -           | U           | -                      | -           | 11.523      | 2.42        | 3.55        | 1          | 114.2     | 0.52                               | 3.78                        | 8.128                       | 2.08                 | 2.51                  | 0.65                                 | ...                           | ...                           | 2.12        | 2.65        |
| 06164445+2232176 | 189.133 | 2.957       | 2.129       | 9          | -            | -          | -          | g           | -          | -           | -             | -           | -   | -            | -           | U           | -                      | -           | 11.523      | ...         | ...         | ...        | ...       | ...                                | ...                         | ...                         | ...                  | ...                   | ...                                  | ...                           | ...                           | ...         |             |
| 06164487+2234106 | 189.003 | 2.929       | 2.101       | 9          | -            | -          | -          | g           | -          | -           | -             | -           | -   | -            | -           | U           | -                      | -           | 9.252       | 1.92        | 2.79        | 1          | 164.8     | 0.34                               | 3.78                        | 8.469                       | 1.57                 | 1.74                  | 0.65                                 | ...                           | ...                           | 1.61        | 1.88        |
| 06164597+2226096 | 189.123 | 2.869       | 2.100       | 9          | -            | -          | -          | g           | -          | -           | -             | -           | -   | -            | -           | U           | -                      | -           | 10.946      | 2.22        | ...         | 1          | 34.4      | 0.82                               | 3.78                        | 10.164                      | 1.88                 | ...                   | 0.65                                 | ...                           | ...                           | 1.92        | ...         |
| 06165042+3358015 | 178.880 | 8.266       | 0.413       | 1          | -            | -          | -          | g           | -          | -           | -             | -           | -   | -            | -           | U           | -                      | -           | 11.287      | 0.32        | 1.10        | 1          | 25.6      | 0.88                               | 3.41                        | 11.133                      | 0.25                 | 0.89                  | 0.13                                 | 26.2                          | 11.15                         | 0.26        | 0.92        |
| 06165058+2235367 | 188.992 | 2.959       | 1.897       | 9          | -            | -          | -          | g           | -          | -           | -             | -           | -   | -            | -           | U           | -                      | -           | 11.656      | ...         | ...         | 1          | 61.0      | 1.10                               | 3.78                        | 10.949                      | ...                  | ...                   | 0.59                                 | ...                           | ...                           | ...         | ...         |
| 06165419+2225237 | 189.186 | 2.871       | 2.064       | 9          | -            | -          | -          | g           | -          | -           | -             | -           | -   | -            | -           | U           | -                      | -           | 11.302      | ...         | 2.99        | 1          | 94.8      | 0.40                               | 3.78                        | 10.533                      | ...                  | 1.96                  | 0.64                                 | ...                           | ...                           | ...         | 2.10        |
| 06165700+2224087 | 189.173 | 2.891       | 2.078       | 9          | -            | -          | -          | g           | -          | -           | -             | -           | -   | -            | -           | U           | -                      | -           | 10.543      | ...         | ...         | 1          | 94.0      | 1.0                                | 3.78                        | 9.769                       | ...                  | ...                   | 0.64                                 | ...                           | ...                           | ...         | ...         |
| 06170032+2224207 | 189.176 | 2.903       | 2.043       | 9          | -            | -          | -          | g           | -          | -           | -             | -           | -   | -            | -           | U           | -                      | -           | 10.897      | ...         | ...         | 1          | 48.6      | 1.0                                | 3.78                        | 10.136                      | ...                  | ...                   | 0.63                                 | ...                           | ...                           | ...         | ...         |
| 06170474+1437545 | 196.030 | -0.769      | 1.485       | 8          | -            | -          | -          | g           | -          | -           | -             | -           | -   | -            | -           | U           | -                      | -           | 11.089      | 0.68        | 1.44        | -2         | 32.6      | 0.82                               | 3.72                        | 10.536                      | 0.43                 | 0.70                  | 0.46                                 | ...                           | ...                           | 0.46        | 0.80        |
| 06170666+2225286 | 189.171 | 2.934       | 1.946       | 9          | -            | -          | -          | g           | -          | -           | -             | -           | -   | -            | -           | U           | -                      | -           | 10.041      | 2.42        | 3.48        | 1          | 114.0     | 0.42                               | 3.78                        | 9.316                       | 2.10                 | 2.51                  | 0.60                                 | ...                           | ...                           | 2.14        | 2.64        |
| 06170773+2225344 | 189.171 | 2.938       | 1.930       | 9          | -            | -          | -          | g           | -          | -           | -             | -           | -   | -            | -           | U           | -                      | -           | 10.252      | 2.21        | 3.46        | 1          | 82.4      | 0.66                               | 3.78                        | 9.533                       | 1.89                 | 2.50                  | 0.60                                 | ...                           | ...                           | 1.93        | 2.63        |
| 06171364+2223215 | 189.215 | 2.941       | 1.912       | 9          | -            | -          | -          | g           | -          | -           | -             | -           | -   | -            | -           | U           | -                      | -           | 10.005      | ...         | 3.06        | 1          | 90.6      | 0.68                               | 3.78                        | 9.293                       | ...                  | 2.11                  | 0.59                                 | ...                           | ...                           | ...         | 2.24        |
| 06171616+1655575 | 194.027 | 0.363       | 1.386       | 1          | -            | -          | -          | g           | -          | N           | -             | -           | -   | -            | -           | U           | -                      | -           | 10.948      | 0.43        | 1.49        | 1          | 33.4      | 0.76                               | 3.62                        | 10.432                      | 0.20                 | 0.81                  | 0.43                                 | 38.2                          | 10.43                         | 0.23        | 0.90        |
| 06171638+2225165 | 189.191 | 2.965       | 1.909       | 9          | -            | -          | -          | g           | -          | -           | -             | -           | -   | -            | -           | U           | -                      | -           | 11.325      | ...         | ...         | 1          | 62.6      | 0.52                               | 3.78                        | 10.614                      | ...                  | ...                   | 0.59                                 | ...                           | ...                           | ...         | ...         |
| 06172392+1454325 | 195.822 | -0.570      | 1.726       | 8          | -            | -          | -          | g           | -          | -           | -             | -           | -   | -            | -           | U           | -                      | -           | 11.037      | 0.68        | 1.72        | 1          | 47.2      | 0.86                               | 3.68                        | 10.394                      | 0.39                 | 0.86                  | 0.53                                 | ...                           | ...                           | 0.43        | 0.97        |
| 06172785+2224405 | 189.221 | 2.999       | 2.001       | 9          | -            | -          | -          | g           | -          | -           | -             | -           | -   | -            | -           | U           | -                      | -           | 10.997      | ...         | ...         | 1          | 53.6      | 0.62                               | 3.78                        | 10.251                      | ...                  | ...                   | 0.62                                 | ...                           | ...                           | ...         | ...         |
| 06173746+2220244 | 189.301 | 2.999       | 1.766       | 9          | -            | -          | -          | g           | -          | -           | -             | -           | -   | -            | -           | U           | -                      | -           | 11.404      | ...         | ...         | 1          | 68.6      | 0.52                               | 3.70                        | 10.746                      | ...                  | ...                   | 0.55                                 | ...                           | ...                           | ...         | ...         |
| 06173772+2220105 | 189.305 | 2.998       | 1.714       | 9          | -            | -          | -          | g           | -          | -           | -             | -           | -   | -            | -           | U           | -                      | -           | 11.298      | 1.81        | 2.50        | 1          | 64.0      | 0.44                               | 3.78                        | 10.659                      | 1.52                 | 1.65                  | 0.53                                 | ...                           | ...                           | 1.56        | 1.76        |
| 06173991+2221184 | 189.293 | 3.014       | 1.926       | 9          | -            | -          | -          | g           | -          | -           | -             | -           | -   | -            | -           | U           | -                      | -           | 11.159      | ...         | ...         | 1          | 50.8      | 0.70                               | 3.70                        | 10.441                      | ...                  | ...                   | 0.60                                 | ...                           | ...                           | ...         | ...         |
| 06174380+2221164 | 189.300 | 3.027       | 1.905       | 9          | -            | -          | -          | g           | -          | -           | -             | -           | -   | -            | -           | U           | -                      | -           | 9.579       | 2.13        | 3.13        | 1          | 111.4     | 0.30                               | 3.70                        | 8.869                       | 1.81                 | 2.18                  | 0.59                                 | ...                           | ...                           | 1.85        | 2.31        |
| 06174489+2222314 | 189.284 | 3.040       | 2.129       | 9          | -            | -          | -          | g           | -          | -           | -             | -           | -   | -            | -           | U           | -                      | -           | 10.226      | 1.91        | 2.85        | 1          | 98.6      | 0.44                               | 3.70                        | 9.433                       | 1.55                 | 1.79                  | 0.66                                 | ...                           | ...                           | 1.60        | 1.93        |
| 06174676+2222524 | 189.282 | 3.050       | 2.170       | 9          | -            | -          | -          | g           | -          | -           | -             | -           | -   | -            | -           | U           | -                      | -           | 12.049      | ...         | ...         | 1          | 55.0      | 0.42                               | 3.78                        | 11.240                      | ...                  | ...                   | 0.67                                 | ...                           | ...                           | ...         | ...         |
| 06175231+2222524 | 189.292 | 3.068       | 2.102       | 9          | -            | -          | -          | g           | -          | -           | -             | -           | -   | -            | -           | U           | -                      | -           | 11.119      | 1.57        | 2.42        | 1          | 44.8      | 0.58                               | 3.78                        | 10.336                      | 1.22                 | 1.38                  | 0.65                                 | ...                           | ...                           | 1.26        | 1.51        |
| 06175498+2223254 | 189.289 | 3.082       | 2.128       | 9          | -            | -          | -          | g           | -          | -           | -             | -           | -   | -            | -           | U           | -                      | -           | 11.178      | ...         | ...         | -2         | 70.6      | 0.44                               | 3.78                        | 10.385                      | ...                  | ...                   | 0.66                                 | ...                           | ...                           | ...         | ...         |
| 06175915-0137555 | 210.651 | -8.185      | 0.355       | 1          | -            | -          | -          | g           | -          | -           | -             | -           | -   | -            | -           | U           | -                      | -           | 10.945      | 0.28        | 1.07        | 1          | 37.2      | 0.96                               | 3.49                        | 10.813                      | 0.22                 | 0.89                  | 0.11                                 | 38.0                          | 10.82                         | 0.23        | 0.92        |
| 06180039+2224144 | 189.287 | 3.107       | 2.121       | 9          | -            | -          | -          | g           | -          | -           | -             | -           | -   | -            | -           | U           | -                      | -           | 11.203      | ...         | ...         | 1          | 52.6      | 1.00                               | 3.78                        | 10.413                      | ...                  | ...                   | 0.66                                 | ...                           | ...                           | ...         | ...         |
| 06180420+2319144 | 188.484 | 3.551       | 2.657       | 8          | -            | -          | -          | g           | -          | -           | -             | -           | -   | -            | -           | U           | -                      | -           | 10.981      | 1.06        | 2.36        | -2         | 31.6      | 0.64                               | 3.64                        | 9.991                       | 0.62                 | 1.04                  | 0.82                                 | ...                           | ...                           | 0.67        | 1.21        |
| 06180507+2225014 | 189.284 | 3.129       | 2.021       | 9          | -            | -          | -          | g           | -          | -           | -             | -           | -   | -            | -           | U           | -                      | -           | 11.025      | 1.84        | 2.71        | 1          | 52.0      | 0.74                               | 3.78                        | 10.272                      | 1.51                 | 1.71                  | 0.63                                 | ...                           | ...                           | 1.55        | 1.84        |
| 06180746+2227344 | 189.251 | 3.157       | 2.038       | 8          | -            | -          | -          | g           | -          | -           | -             | -           | -   | -            | -           | U           | -                      | -           | 10.719      | 2.07        | 2.96        | 1          | 91.6      | 0.34                               | 3.78                        | 9.960                       | 1.73                 | 1.95                  | 0.63                                 | ...                           | ...                           | 1.77        | 2.08        |
| 06180811+2228094 | 189.243 | 3.164       | 2.055       | 9          | -            | -          | -          | g           | -          | -           | -             | -           | -   | -            | -           | U           | -                      | -           | 11.922      | 1.63        | 2.13        | 1          | 40.8      | 0.48                               | 3.78                        | 11.156                      | 1.29                 | 1.11                  | 0.64                                 | ...                           | ...                           | 1.33        | 1.24        |
| 06181144+1500129 | 195.830 | -0.357      | 1.136       | 7          | -            | -          | -          | g           | -          | -           | -             | -           | -   | -            | -           | U           | -                      | -           | 11.429      | 0.71        | 1.62        | -2         | 22.0      | 0.72                               | 3.68                        | 11.066                      | 0.52                 | 1.05                  | 0.35                                 | ...                           | ...                           | 0.55        | 1.13        |
| 06181338+2844455 | 183.687 | 6.120       | 0.566       | 1          | -            | -          | -          | g           | -          | -           | -             | -           | -   | -            | -           | U           | -                      | -           | 11.455      | 0.42        | 1.28        | 1          | 26.6      | 0.56                               | 3.46                        | 11.244                      | 0.33                 | 1.00                  | 0.18                                 | 27.6                          | 11.26                         | 0.34        | 1.04        |
| 06181475+2232109 | 189.196 | 3.218       | 1.969       | 9          | -            | -          | -          | g           | -          | -           | -             | -           | -   | -            | -           | U           | -                      | -           | 11.92       |             |             |            |           |                                    |                             |                             |                      |                       |                                      |                               |                               |             |             |

Table B1: a) continued.

| 2MASX J          | <i>l</i> | <i>b</i> | EBV   | Object | Sample | Disc | 2MRS | Velocity | NIR  | Photom | Ext  | <i>K</i> <sub>20</sub> | <i>H-K</i> | <i>J-K</i> | vc   | <i>a</i> | <i>b/a</i> | st.d.  | <i>K</i> <sub>s</sub> <sup>o</sup> | ( <i>H-K</i> ) <sup>o</sup> | ( <i>J-K</i> ) <sup>o</sup> | <i>A</i> <sub>K</sub> | <i>a</i> <sub>d</sub> <sup>o</sup> | <i>K</i> <sub>s</sub> <sup>o,d</sup> | ( <i>H-K</i> ) <sup>o,c</sup> | ( <i>J-K</i> ) <sup>o,c</sup> |      |      |      |       |      |      |
|------------------|----------|----------|-------|--------|--------|------|------|----------|------|--------|------|------------------------|------------|------------|------|----------|------------|--------|------------------------------------|-----------------------------|-----------------------------|-----------------------|------------------------------------|--------------------------------------|-------------------------------|-------------------------------|------|------|------|-------|------|------|
| (1)              | deg      | deg      | mag   | class  | off    | flg  | gal  | TF       | obs  | ext'd  | type | (9)                    | Opt        | HI         | vc   | "        | (19)       | (20)   | mag                                | mag                         | mag                         | mag                   | "                                  | mag                                  | mag                           | mag                           |      |      |      |       |      |      |
| (1)              | (2a)     | (2b)     | (3)   | (4)    | (5)    | (6)  | (7a) | (7b)     | (7c) | (7d)   | (8)  | (9)                    | (10a)      | (10b)      | (11) | (12)     | (13)       | (14)   | (15)                               | (16)                        | (17)                        | (18)                  | (19)                               | (20)                                 | (21)                          | (22)                          | (23) | (24) | (25) | (26)  | (27) | (28) |
| 06201733+2511389 | 187.061  | 4.875    | 0.570 | 1      | —      | —    | g    | t        | —    | —      | D1   | e                      | o          | h          | —    | —        | —          | 11.414 | 0.45                               | 1.44                        | 1                           | 36.8                  | 0.36                               | 3.50                                 | 11.202                        | 0.35                          | 1.16 | 0.18 | 38.4 | 11.21 | 0.37 | 1.19 |
| 06203402+2758426 | 184.612  | 6.222    | 0.373 | 1      | —      | —    | —    | —        | —    | —      | D1   | c                      | e          | h          | —    | —        | —          | 10.136 | 0.36                               | 1.13                        | 1                           | 70.0                  | 0.56                               | 3.45                                 | 9.997                         | 0.30                          | 0.94 | 0.12 | 71.5 | 10.01 | 0.31 | 0.97 |
| 06205756+1343537 | 197.268  | −0.366   | 0.897 | 1      | —      | —    | —    | —        | —    | —      | D1   | e                      | o          | —          | —    | —        | —          | 11.071 | 0.41                               | 1.40                        | 1                           | 31.8                  | 0.74                               | 3.63                                 | 10.737                        | 0.27                          | 0.96 | 0.28 | 34.1 | 10.75 | 0.28 | 1.02 |
| 06210911+2255353 | 189.166  | 3.992    | 1.565 | 1      | —      | —    | —    | —        | —    | —      | D1   | —                      | —          | h          | —    | e        | —          | 10.633 | 0.63                               | 1.95                        | 1                           | 52.8                  | 0.34                               | 3.56                                 | 10.050                        | 0.37                          | 1.17 | 0.48 | 61.5 | 10.05 | 0.40 | 1.27 |
| 06211266+2751224 | 184.787  | 6.291    | 0.352 | 1      | —      | —    | —    | —        | —    | —      | D1   | c                      | —          | h          | —    | —        | —          | 10.634 | 0.38                               | 1.15                        | 1                           | 46.6                  | 0.54                               | 3.44                                 | 10.503                        | 0.32                          | 0.98 | 0.11 | 47.5 | 10.51 | 0.33 | 1.00 |
| 06214768+1039233 | 200.078  | −1.633   | 2.018 | 8      | o      | —    | —    | —        | N    | —      | —    | —                      | —          | —          | —    | —        | —          | 11.381 | 0.63                               | 1.90                        | 1                           | 41.2                  | 0.48                               | 3.65                                 | 10.629                        | 0.29                          | 0.90 | 0.63 | ...  | ...   | 0.33 | 1.03 |
| 06215050+0021581 | 209.216  | −6.413   | 0.598 | 1      | —      | —    | —    | —        | —    | —      | D1   | c                      | o          | h          | —    | —        | —          | 8.361  | 0.38                               | 1.25                        | 1                           | 94.2                  | 0.72                               | 3.59                                 | 8.138                         | 0.28                          | 0.95 | 0.19 | 97.0 | 8.17  | 0.29 | 0.99 |
| 06215783+1907436 | 192.616  | 2.383    | 0.607 | 1      | —      | —    | —    | t        | —    | —      | D1   | —                      | —          | h          | —    | —        | —          | 11.174 | 0.56                               | 1.40                        | 1                           | 60.2                  | 0.30                               | 3.64                                 | 10.948                        | 0.46                          | 1.10 | 0.19 | 63.2 | 10.95 | 0.47 | 1.14 |
| 06220599+1646075 | 194.717  | 1.305    | 0.934 | 1      | —      | —    | —    | —        | N    | —      | D4   | er                     | —          | —          | —    | —        | —          | 11.243 | 0.35                               | 1.32                        | 1                           | 35.8                  | 0.78                               | 3.61                                 | 10.895                        | 0.20                          | 0.85 | 0.29 | 38.7 | 10.90 | 0.22 | 0.92 |
| 06221502+1359475 | 197.181  | 0.035    | 0.756 | 1      | —      | —    | —    | —        | —    | —      | D1   | e                      | o          | h          | —    | —        | —          | 11.044 | 0.42                               | 1.24                        | 1                           | 47.2                  | 0.54                               | 3.71                                 | 10.762                        | 0.29                          | 0.87 | 0.23 | 50.3 | 10.76 | 0.31 | 0.92 |
| 06222633+0431236 | 205.582  | −4.359   | 0.603 | 1      | —      | —    | —    | —        | —    | —      | D1   | e                      | o          | h          | —    | —        | —          | 10.249 | 0.39                               | 1.35                        | 1                           | 58.0                  | 0.40                               | 3.61                                 | 10.024                        | 0.29                          | 1.05 | 0.19 | 60.7 | 10.03 | 0.30 | 1.09 |
| 06222939+1358391 | 197.225  | 0.077    | 0.729 | 1      | —      | —    | —    | —        | —    | —      | D1   | —                      | —          | —          | —    | —        | —          | 11.389 | 0.48                               | 1.40                        | 1                           | 34.0                  | 0.52                               | 3.65                                 | 11.117                        | 0.36                          | 1.04 | 0.23 | 36.0 | 11.13 | 0.37 | 1.09 |
| 06222944+1027158 | 200.337  | −1.576   | 0.804 | 1      | —      | —    | —    | —        | N    | —      | D3   | —                      | —          | —          | —    | —        | —          | 11.183 | 0.50                               | 1.59                        | 1                           | 34.4                  | 0.86                               | 3.70                                 | 10.883                        | 0.36                          | 1.19 | 0.25 | 36.8 | 10.89 | 0.38 | 1.25 |
| 06224972+2921577 | 183.599  | 7.299    | 0.300 | 1      | —      | —    | —    | t        | N    | —      | D1   | c                      | o          | —          | *    | —        | —          | 11.242 | 0.50                               | 1.38                        | 1                           | 43.0                  | 0.42                               | 3.51                                 | 11.130                        | 0.45                          | 1.23 | 0.09 | 43.7 | 11.14 | 0.45 | 1.25 |
| 06224986+2439027 | 187.813  | 5.134    | 0.480 | 1      | —      | —    | —    | —        | —    | —      | D1   | c                      | o          | h          | —    | —        | —          | 10.690 | 0.43                               | 1.34                        | 1                           | 44.0                  | 0.40                               | 3.54                                 | 10.511                        | 0.35                          | 1.10 | 0.15 | 45.2 | 10.53 | 0.36 | 1.13 |
| 06225815+1108312 | 199.784  | −1.150   | 1.059 | 1      | —      | —    | —    | —        | N    | —      | D1   | —                      | —          | h          | —    | —        | —          | 11.145 | 0.57                               | 1.56                        | 1                           | 52.8                  | 0.44                               | 3.69                                 | 10.750                        | 0.40                          | 1.04 | 0.33 | 58.3 | 10.74 | 0.42 | 1.11 |
| 06230531+0607132 | 215.192  | −9.079   | 0.483 | 1      | —      | —    | —    | —        | —    | —      | D1   | c                      | o          | —          | —    | —        | —          | 11.391 | 0.38                               | 1.22                        | 1                           | 30.0                  | 0.58                               | 3.41                                 | 11.211                        | 0.30                          | 0.98 | 0.15 | 30.9 | 11.22 | 0.31 | 1.01 |
| 06231132+1443129 | 196.649  | 0.575    | 0.895 | 1      | —      | —    | —    | —        | —    | —      | D1   | e                      | —          | h          | —    | —        | —          | 10.388 | 0.39                               | 1.34                        | 1                           | 62.2                  | 0.82                               | 3.68                                 | 10.055                        | 0.24                          | 0.89 | 0.28 | 66.7 | 10.07 | 0.26 | 0.95 |
| 06233428+0956192 | 200.917  | −1.583   | 0.641 | 8      | —      | —    | —    | —        | —    | —      | D1   | e                      | —          | h          | —    | —        | —          | 10.067 | 0.92                               | 1.99                        | 1                           | 53.0                  | 0.76                               | 3.67                                 | 9.828                         | 0.82                          | 1.68 | 0.20 | ...  | ...   | 0.83 | 1.72 |
| 06235989+0442387 | 205.597  | −3.928   | 0.553 | 1      | —      | —    | —    | —        | —    | —      | D1   | e                      | —          | h          | —    | —        | —          | 10.123 | 0.40                               | 1.27                        | 1                           | 70.8                  | 0.58                               | 3.66                                 | 9.917                         | 0.31                          | 1.00 | 0.17 | 73.8 | 9.92  | 0.32 | 1.03 |
| 06241605+0825453 | 202.333  | −2.137   | 0.494 | 8      | —      | —    | —    | —        | —    | —      | D1   | e                      | o          | —          | —    | —        | —          | 10.850 | 1.19                               | 2.58                        | −2                          | 18.0                  | 0.74                               | 3.73                                 | 10.666                        | 1.10                          | 2.33 | 0.15 | ...  | ...   | 1.11 | 2.36 |
| 06243012+1749352 | 194.050  | 2.306    | 0.781 | 1      | —      | —    | —    | —        | —    | —      | D1   | e                      | o          | h          | —    | —        | —          | 10.963 | 0.50                               | 1.34                        | 1                           | 50.2                  | 0.68                               | 3.55                                 | 10.672                        | 0.37                          | 0.95 | 0.24 | 53.6 | 10.67 | 0.38 | 1.00 |
| 06244655+1558061 | 195.725  | 1.497    | 0.693 | 1      | —      | —    | —    | —        | —    | —      | D1   | e                      | o          | h          | —    | —        | —          | 10.956 | 0.41                               | 1.29                        | 1                           | 78.2                  | 0.20                               | 3.64                                 | 10.698                        | 0.29                          | 0.95 | 0.21 | 82.6 | 10.70 | 0.31 | 0.99 |
| 06244711+1558451 | 195.716  | 1.504    | 0.692 | 1      | —      | —    | —    | t        | —    | —      | D1   | e                      | o          | h          | —    | —        | —          | 10.843 | 0.41                               | 1.24                        | 1                           | 49.0                  | 0.14                               | 3.64                                 | 10.585                        | 0.29                          | 0.90 | 0.21 | 51.4 | 10.60 | 0.31 | 0.95 |
| 06245794+1458369 | 196.623  | 1.075    | 0.881 | 1      | —      | —    | —    | —        | N    | —      | D1   | —                      | —          | —          | —    | —        | —          | 10.797 | 0.39                               | 1.30                        | 1                           | 41.8                  | 0.92                               | 3.62                                 | 10.469                        | 0.24                          | 0.86 | 0.27 | 45.0 | 10.47 | 0.26 | 0.92 |
| 06245891+2502014 | 187.697  | 5.743    | 0.431 | 1      | —      | —    | —    | —        | —    | —      | D2   | c                      | o          | —          | —    | —        | —          | 11.324 | 0.35                               | 1.25                        | 1                           | 32.2                  | 0.60                               | 3.49                                 | 11.163                        | 0.28                          | 1.04 | 0.13 | 33.1 | 11.17 | 0.29 | 1.07 |
| 06251411+1505346 | 196.551  | 1.186    | 0.867 | 1      | —      | —    | —    | —        | —    | —      | D4   | c                      | o          | —          | —    | —        | —          | 11.252 | 0.47                               | 1.40                        | 1                           | 25.0                  | 0.82                               | 3.67                                 | 10.929                        | 0.33                          | 0.97 | 0.27 | 26.7 | 10.94 | 0.34 | 1.03 |
| 06254194+3039226 | 182.720  | 8.436    | 0.264 | 1      | —      | —    | —    | —        | —    | —      | D1   | e                      | o          | h          | —    | —        | —          | 10.317 | 0.38                               | 1.12                        | 1                           | 57.0                  | 0.60                               | 3.46                                 | 10.219                        | 0.34                          | 0.99 | 0.08 | 57.7 | 10.23 | 0.34 | 1.01 |
| 06254269+1700046 | 194.915  | 2.177    | 0.564 | 1      | —      | —    | —    | —        | —    | —      | D2   | c                      | o          | —          | —    | —        | —          | 11.428 | 0.46                               | 1.27                        | 1                           | 27.8                  | 0.68                               | 3.68                                 | 11.218                        | 0.37                          | 0.99 | 0.17 | 28.9 | 11.23 | 0.38 | 1.03 |
| 06255436+0632286 | 204.194  | −2.657   | 0.778 | 1      | —      | —    | —    | —        | N    | —      | D1   | —                      | —          | —          | —    | —        | —          | 11.520 | 0.50                               | 1.52                        | 1                           | 23.6                  | 0.56                               | 3.64                                 | 11.230                        | 0.37                          | 1.13 | 0.24 | 25.1 | 11.24 | 0.38 | 1.18 |
| 06255723+1747275 | 194.242  | 2.596    | 0.521 | 8      | —      | p    | —    | —        | —    | —      | D1   | e                      | o          | —          | —    | —        | —          | 10.144 | 1.11                               | 1.46                        | 1                           | 25.4                  | 0.74                               | 3.66                                 | 9.950                         | 1.02                          | 1.20 | 0.16 | ...  | ...   | 1.03 | 1.24 |
| 06260540+1644287 | 195.188  | 2.136    | 0.534 | 1      | —      | —    | —    | —        | —    | —      | D1   | e                      | o          | —          | —    | —        | —          | 10.305 | 0.31                               | 1.15                        | 1                           | 49.0                  | 0.68                               | 3.63                                 | 10.106                        | 0.22                          | 0.89 | 0.17 | 50.6 | 10.12 | 0.23 | 0.92 |
| 06262702+0727287 | 203.445  | −2.111   | 0.662 | 1      | —      | —    | —    | —        | N    | —      | D1   | —                      | —          | —          | —    | —        | —          | 11.063 | 0.52                               | 1.43                        | 1                           | 50.6                  | 0.64                               | 3.63                                 | 10.816                        | 0.41                          | 1.10 | 0.21 | 53.3 | 10.82 | 0.42 | 1.14 |
| 06263895+1601067 | 195.890  | 1.919    | 0.552 | 1      | —      | —    | —    | —        | N    | —      | D1   | —                      | —          | —          | —    | —        | —          | 11.164 | 0.34                               | 1.18                        | 1                           | 30.2                  | 0.52                               | 3.61                                 | 10.958                        | 0.25                          | 0.91 | 0.17 | 31.4 | 10.97 | 0.26 | 0.95 |
| 06265626+1006451 | 219.250  | −9.994   | 1.074 | 7      | o      | —    | —    | —        | —    | —      | D1   | —                      | —          | —          | —    | —        | —          | 11.414 | 1.21                               | 2.91                        | 1                           | 28.4                  | 0.44                               | 3.45                                 | 11.014                        | 1.03                          | 2.38 | 0.33 | ...  | ...   | 1.05 | 2.45 |
| 06270279+0334227 | 206.960  | −3.781   | 0.798 | 8      | —      | —    | —    | —        | —    | —      | D1   | —                      | —          | —          | —    | —        | —          | 11.333 | 1.80                               | 3.24                        | 1                           | 20.0                  | 0.86                               | 3.54                                 | 11.036                        | 1.66                          | 2.84 | 0.25 | ...  | ...   | 1.68 | 2.90 |
| 06271546+1010081 | 219.336  | −9.948   | 1.046 | 9      | —      | —    | —    | —        | —    | —      | D1   | —                      | —          | —          | —    | —        | —          | 11.363 | 1.41                               | ...                         | 1                           | 52.0                  | 0.48                               | 3.53                                 | 10.973                        | 1.24                          | ...  | ...  | ...  | ...   | 1.26 | ...  |
| 06271830+1009342 | 219.333  | −9.934   | 1.043 | 8      | —      | —    | —    | —        | —    | —      | D1   | —                      | —          | —          | —    | —        | —          | 8.360  | 1.68                               | 3.23                        | 1                           | 105.6                 | 0.56                               | 3.53                                 | 7.971                         | 1.51                          | 2.71 | 0.32 | ...  | ...   | 1.53 | 2.78 |
| 06274112+1004479 | 219.302  | −9.815   | 1.093 | 7      | —      | —    | —    | —        | —    | —      | D1   | —                      | —          | —          | —    | —        | —          | 9.942  | 1.68                               | 3.36                        | 1                           | 28.4                  | 0.72                               | 3.45                                 | 9.535                         | 1.50                          | 2.82 | 0.34 | ...  | ...   | 1.52 | 2.89 |
| 06281852+2417350 | 188.707  | 6.077    | 0.366 | 1      | —      | —    | —    | —        | —    | —      | D1   | c                      | o          | —          | —    | —        | —          | 11.222 | 0.44                               | 1.30                        | 1                           | 31.0                  | 0.90                               | 3.51                                 | 11.086                        | 0.38                          | 1.12 | 0.11 | 31.7 | 11.10 | 0.38 | 1.14 |
| 06282347+2337294 | 189.314  | 5.790    | 0.332 | 1      | —      | —    | —    | —        | —    | —      | D2   | c                      | o          | —          | —    | —        | —          | 10.878 | 0.40                               | 1.24                        | 1                           | 39.2                  | 0.98                               | 3.55                                 | 10.754                        | 0.34                          | 1.08 | 0.10 | 40.0 | 10.76 | 0.35 | 1.10 |
| 06283061+2132595 | 191.180  | 4.865    | 0.394 | 1      | —      | —    | —    | —        | —    | —      | D3   | e                      | o          | —          | —    | —        | —          | 9.290  | 0.34                               | 1.18                        | 1                           | 76.2                  | 0.96                               | 3.54                                 | 9.143                         | 0.28                          | 0.99 | 0.12 |      |       |      |      |

Table B1: a) continued.

| 2MASX J           | <i>l</i> | <i>b</i> | EBV   | Object | Sample | Disc | 2MRS | Velocity | NIR   | Photom | Ext | <i>K</i> <sub>20</sub> | <i>H-K</i> | <i>J-K</i> | vc    | <i>a</i> | <i>b/a</i> | st.d. | <i>K</i> <sub>s</sub> <sup>o</sup> | ( <i>H-K</i> ) <sup>o</sup> | ( <i>J-K</i> ) <sup>o</sup> | <i>A<sub>K</sub></i> | <i>a</i> <sup>d</sup> | <i>K</i> <sub>s</sub> <sup>o,d</sup> | ( <i>H-K</i> ) <sup>o,c</sup> | ( <i>J-K</i> ) <sup>o,c</sup> |        |       |       |      |      |       |       |       |
|-------------------|----------|----------|-------|--------|--------|------|------|----------|-------|--------|-----|------------------------|------------|------------|-------|----------|------------|-------|------------------------------------|-----------------------------|-----------------------------|----------------------|-----------------------|--------------------------------------|-------------------------------|-------------------------------|--------|-------|-------|------|------|-------|-------|-------|
| (1)               | deg      | deg      | mag   | class  | off    | gal  | TF   | obs      | ext'd | type   |     |                        | mag        | mag        |       | "        |            |       | mag                                | mag                         | mag                         | mag                  | "                     | mag                                  | mag                           | mag                           |        |       |       |      |      |       |       |       |
| (2a)              | (2b)     | (3)      | (4)   | (5)    | (6)    | (7a) | (7b) | (7c)     | (7d)  | (8)    | (9) | Opt                    | HI         | (10a)      | (10b) | (11)     | (12)       | (13)  | (14)                               | (15)                        | (16)                        | (17)                 | (18)                  | (19)                                 | (20)                          | (21)                          | (22)   | (23)  | (24)  | (25) | (26) | (27)  | (28)  |       |
| 063332957+0913524 | 202.680  | 0.254    | 0.766 | 1      | —      | —    | g    | —        | —     | D1     | e   | o                      | —          | —          | —     | U        | —          | —     | —                                  | 11.476                      | 0.35                        | 1.13                 | 1                     | 31.4                                 | 0.54                          | 3.67                          | 11.191 | 0.22  | 0.75  | 0.24 | 33.3 | 11.20 | 0.23  | 0.80  |
| 063333089+2804280 | 185.825  | 8.815    | 0.244 | 1      | —      | —    | g    | —        | —     | D1     | c   | —                      | —          | —          | —     | —        | —          | —     | —                                  | 11.006                      | 0.27                        | 1.09                 | 1                     | 39.2                                 | 0.78                          | 3.34                          | 10.915 | 0.23  | 0.97  | 0.08 | 39.7 | 10.92 | 0.23  | 0.99  |
| 063333198+0400236 | 207.322  | -2.145   | 7.767 | 9      | —      | —    | —    | —        | —     | —      | —   | —                      | —          | —          | —     | —        | —          | —     | —                                  | 8.675                       | 1.35                        | 3.00                 | 1                     | 108.6                                | 0.78                          | 3.73                          | 5.781  | 0.06  | -0.85 | 2.41 | ...  | ...   | 0.21  | -0.34 |
| 063333350+2102135 | 192.176  | 5.679    | 0.324 | 1      | —      | —    | g    | —        | —     | D1     | c   | —                      | h          | —          | —     | —        | —          | —     | —                                  | 10.331                      | 0.47                        | 1.44                 | 1                     | 74.6                                 | 0.22                          | ...                           | 10.210 | 0.42  | 1.28  | 0.10 | ...  | ...   | 0.43  | 1.31  |
| 06333627+0723201  | 217.518  | -7.311   | 0.733 | 1      | —      | —    | —    | —        | —     | D1     | c   | o                      | —          | —          | —     | —        | —          | —     | —                                  | 11.099                      | 0.33                        | 1.20                 | 1                     | 39.6                                 | 0.34                          | 3.54                          | 10.826 | 0.21  | 0.84  | 0.23 | 41.7 | 10.84 | 0.22  | 0.89  |
| 06335224+0843222  | 218.752  | -7.846   | 0.558 | 5      | —      | —    | p    | —        | —     | —      | n   | c                      | o?         | —          | —     | —        | —          | —     | —                                  | 11.355                      | 1.37                        | 2.99                 | -2                    | 16.8                                 | 0.80                          | 3.48                          | 11.147 | 1.28  | 2.71  | 0.17 | 17.3 | 11.17 | 1.29  | 2.75  |
| 06340572+0425126  | 207.019  | -1.830   | 6.825 | 9      | —      | —    | —    | —        | —     | —      | —   | —                      | —          | —          | —     | —        | —          | —     | —                                  | 11.639                      | 1.05                        | ...                  | 1                     | 74.2                                 | 0.22                          | 3.89                          | 9.096  | -0.08 | ...   | 2.11 | ...  | ...   | 0.06  | ...   |
| 06340645+0424396  | 207.029  | -1.832   | 6.778 | 9      | —      | —    | —    | —        | —     | —      | —   | —                      | —          | —          | —     | —        | —          | —     | —                                  | 12.511                      | 1.30                        | ...                  | 1                     | 39.0                                 | 0.36                          | 3.89                          | 9.986  | 0.17  | ...   | 2.10 | ...  | ...   | 0.31  | ...   |
| 06340979+0426376  | 207.006  | -1.804   | 6.871 | 9      | —      | —    | —    | —        | —     | —      | —   | —                      | —          | —          | —     | —        | —          | —     | —                                  | 12.171                      | 1.74                        | ...                  | 1                     | 17.6                                 | 0.44                          | 3.89                          | 9.611  | 0.60  | ...   | 2.13 | ...  | ...   | 0.74  | ...   |
| 06340985+2131565  | 191.796  | 6.028    | 0.236 | 1      | —      | —    | g    | —        | —     | D1     | c   | —                      | o          | —          | —     | —        | —          | —     | —                                  | 11.124                      | 0.47                        | 1.25                 | 1                     | 34.6                                 | 0.70                          | 3.51                          | 11.036 | 0.43  | 1.13  | 0.07 | 35.0 | 11.04 | 0.43  | 1.15  |
| 06341652+0758280  | 203.884  | -0.154   | 0.966 | 1      | —      | —    | g    | —        | —     | D1     | c   | —                      | —          | —          | —     | —        | —          | —     | —                                  | 11.290                      | 0.46                        | 1.52                 | 1                     | 59.8                                 | 0.42                          | 3.73                          | 10.930 | 0.30  | 1.04  | 0.30 | 65.3 | 10.92 | 0.32  | 1.10  |
| 06341661+0418436  | 207.136  | -1.840   | 6.059 | 9      | —      | —    | —    | —        | —     | —      | —   | —                      | —          | —          | —     | —        | —          | —     | —                                  | 11.751                      | 1.76                        | ...                  | 1                     | 26.8                                 | 0.92                          | 3.69                          | 9.493  | 0.76  | ...   | 1.88 | ...  | ...   | 0.88  | ...   |
| 06341666+0915552  | 219.288  | -7.997   | 0.832 | 6      | —      | —    | p?   | —        | —     | —      | cn  | —                      | —          | —          | —     | —        | —          | —     | —                                  | 10.916                      | 1.53                        | 3.36                 | -2                    | 22.6                                 | 0.68                          | 3.54                          | 10.606 | 1.40  | 2.95  | 0.26 | ...  | ...   | 1.41  | 3.00  |
| 06341942+0421326  | 207.100  | -1.808   | 6.328 | 9      | —      | —    | —    | —        | —     | —      | —   | —                      | —          | —          | —     | —        | —          | —     | —                                  | 13.175                      | 0.95                        | 2.23                 | 1                     | 15.0                                 | 1.00                          | 3.89                          | 10.817 | -0.10 | -0.92 | 1.96 | ...  | ...   | 0.03  | -0.50 |
| 06342716+0414464  | 207.215  | -1.831   | 7.189 | 8      | —      | —    | o    | —        | —     | —      | —   | —                      | —          | —          | —     | —        | —          | —     | —                                  | 13.257                      | 1.01                        | ...                  | -1                    | 17.2                                 | 0.74                          | 3.67                          | 10.578 | -0.18 | ...   | 2.23 | ...  | ...   | -0.04 | ...   |
| 06343138+0904375  | 202.934  | 0.409    | 0.750 | 1      | —      | —    | g    | —        | —     | D2     | —   | —                      | —          | —          | —     | —        | —          | —     | —                                  | 8.929                       | 0.28                        | 1.06                 | 1                     | 84.8                                 | 0.88                          | 3.66                          | 8.650  | 0.15  | 0.69  | 0.23 | 89.0 | 8.67  | 0.17  | 0.74  |
| 06343258+0417444  | 207.181  | -1.788   | 6.218 | 9      | —      | —    | —    | —        | —     | —      | —   | —                      | —          | —          | —     | —        | —          | —     | —                                  | 11.355                      | ...                         | ...                  | 1                     | 64.6                                 | 0.50                          | 3.80                          | 9.038  | ...   | ...   | 1.93 | ...  | ...   | ...   | ...   |
| 06343565+0412454  | 207.261  | -1.815   | 7.840 | 8      | —      | —    | —    | —        | —     | —      | —   | —                      | —          | —          | —     | —        | —          | —     | —                                  | 9.183                       | 1.23                        | 2.45                 | 1                     | 57.6                                 | 0.76                          | 3.67                          | 6.262  | -0.07 | -1.44 | 2.43 | ...  | ...   | 0.08  | -0.93 |
| 06343673+0238144  | 208.663  | -2.535   | 2.959 | 1      | —      | —    | —    | —        | —     | D3     | —   | —                      | —          | —          | —     | —        | —          | —     | —                                  | 11.861                      | 0.61                        | 1.73                 | 1                     | 23.2                                 | 0.94                          | 3.62                          | 10.758 | 0.12  | 0.26  | 0.92 | 33.1 | 10.69 | 0.18  | 0.46  |
| 06343706+0413054  | 207.259  | -1.808   | 7.792 | 9      | —      | —    | —    | —        | —     | —      | —   | —                      | —          | —          | —     | —        | —          | —     | —                                  | 10.200                      | 0.76                        | 2.18                 | 1                     | 84.6                                 | 0.82                          | 3.67                          | 7.297  | -0.53 | -1.69 | 2.41 | ...  | ...   | -0.38 | -1.18 |
| 06343906+0436144  | 206.920  | -1.623   | 4.216 | 7      | —      | —    | —    | —        | —     | —      | —   | —                      | —          | —          | —     | —        | —          | —     | —                                  | 9.889                       | 1.39                        | 3.11                 | 1                     | 22.2                                 | 0.78                          | 3.59                          | 8.318  | 0.69  | 1.02  | 1.31 | ...  | ...   | 0.77  | 1.30  |
| 06344020+0139344  | 209.540  | -2.971   | 1.304 | 1      | —      | —    | g    | —        | —     | D3     | —   | —                      | —          | —          | —     | —        | —          | —     | —                                  | 11.355                      | 0.41                        | 1.52                 | 1                     | 39.6                                 | 0.54                          | 3.67                          | 10.869 | 0.20  | 0.88  | 0.40 | 44.4 | 10.88 | 0.22  | 0.96  |
| 06344281+0445594  | 206.782  | -1.534   | 2.810 | 1      | —      | —    | g    | —        | —     | D1     | —   | —                      | —          | —          | —     | —        | —          | e     | —                                  | 11.071                      | 0.76                        | 2.10                 | 1                     | 61.6                                 | 0.28                          | 3.59                          | 10.024 | 0.30  | 0.71  | 0.87 | 87.0 | 9.94  | 0.35  | 0.89  |
| 06344614+1712496  | 195.725  | 4.196    | 0.509 | 1      | —      | —    | g    | —        | —     | D2     | e   | o                      | —          | —          | —     | —        | —          | —     | —                                  | 11.290                      | 0.43                        | 1.30                 | 1                     | 33.2                                 | 0.94                          | 3.52                          | 11.100 | 0.34  | 1.05  | 0.16 | 34.4 | 11.11 | 0.35  | 1.08  |
| 06344840+0942038  | 219.741  | -8.073   | 0.667 | 1      | —      | —    | —    | —        | —     | D3     | —   | —                      | —          | —          | —     | —        | —          | —     | —                                  | 10.912                      | 0.40                        | 1.23                 | 1                     | 38.4                                 | 0.84                          | 3.52                          | 10.663 | 0.29  | 0.90  | 0.21 | 40.3 | 10.68 | 0.31  | 0.94  |
| 06345236+0347024  | 207.674  | -1.951   | 2.326 | 8      | —      | —    | —    | —        | —     | —      | —   | —                      | —          | —          | —     | —        | —          | —     | —                                  | 12.050                      | 1.32                        | 3.32                 | 1                     | 17.2                                 | 0.84                          | 3.61                          | 11.183 | 0.94  | 2.16  | 0.72 | ...  | ...   | 0.98  | 2.31  |
| 06345637+2440474  | 189.043  | 7.599    | 0.284 | 1      | —      | —    | g    | —        | —     | D1     | e   | o                      | —          | —          | —     | —        | —          | —     | —                                  | 11.189                      | 0.30                        | 1.10                 | 1                     | 37.4                                 | 0.84                          | 3.33                          | 11.083 | 0.25  | 0.96  | 0.09 | 38.0 | 11.09 | 0.26  | 0.98  |
| 06345941+0653184  | 204.930  | -0.497   | 0.926 | 1      | —      | —    | g    | —        | —     | D2     | —   | —                      | h          | —          | —     | —        | —          | —     | —                                  | 9.261                       | 0.41                        | 1.39                 | 1                     | 89.8                                 | 0.48                          | 3.74                          | 8.916  | 0.26  | 0.93  | 0.29 | 95.8 | 8.94  | 0.27  | 0.99  |
| 06350343+2231160  | 191.001  | 6.658    | 0.208 | 1      | —      | —    | g    | —        | —     | D1     | cp  | o?                     | —          | —          | —     | —        | p          | —     | —                                  | 10.730                      | 0.37                        | 1.15                 | 1                     | 69.2                                 | 0.52                          | 3.54                          | 10.652 | 0.33  | 1.05  | 0.06 | 70.0 | 10.66 | 0.34  | 1.06  |
| 06350718+1842450  | 194.424  | 4.952    | 0.466 | 1      | —      | —    | g    | —        | —     | D2     | e   | —                      | —          | —          | —     | —        | —          | —     | —                                  | 11.293                      | 0.43                        | 1.27                 | 1                     | 39.0                                 | 0.60                          | 3.56                          | 11.119 | 0.35  | 1.04  | 0.14 | 40.3 | 11.13 | 0.36  | 1.07  |
| 06350768+0351539  | 207.631  | -1.857   | 2.461 | 8      | —      | —    | o    | —        | —     | —      | —   | —                      | —          | —          | —     | —        | —          | —     | —                                  | 11.731                      | 0.90                        | 1.88                 | -2                    | 48.6                                 | 0.62                          | 3.60                          | 10.814 | 0.50  | 0.66  | 0.76 | ...  | ...   | 0.55  | 0.82  |
| 06350929+0351279  | 207.640  | -1.854   | 2.474 | 8      | —      | —    | —    | —        | —     | —      | —   | —                      | —          | —          | —     | —        | —          | —     | —                                  | 12.071                      | 1.10                        | 2.15                 | 1                     | 40.2                                 | 0.54                          | 3.60                          | 11.149 | 0.69  | 0.92  | 0.77 | ...  | ...   | 0.73  | 1.08  |
| 06351067+2627524  | 187.451  | 8.437    | 0.211 | 1      | —      | —    | g    | —        | —     | D1     | e   | o                      | —          | —          | —     | —        | —          | —     | —                                  | 11.252                      | 0.33                        | 1.10                 | 1                     | 33.0                                 | 0.84                          | 3.41                          | 11.173 | 0.29  | 1.00  | 0.07 | 33.4 | 11.18 | 0.30  | 1.01  |
| 06352031+1458436  | 197.780  | 3.297    | 0.522 | 1      | —      | —    | g    | —        | —     | D1     | —   | —                      | —          | —          | —     | —        | —          | —     | —                                  | 10.659                      | 0.44                        | 1.34                 | 1                     | 68.2                                 | 0.26                          | 3.56                          | 10.465 | 0.35  | 1.08  | 0.16 | 70.8 | 10.47 | 0.36  | 1.12  |
| 06352675+0230578  | 208.867  | -2.406   | 1.958 | 1      | —      | —    | g    | —        | —     | D3     | —   | —                      | —          | —          | —     | —        | e          | —     | —                                  | 11.114                      | 0.55                        | 1.87                 | 1                     | 34.6                                 | 0.84                          | 3.67                          | 10.384 | 0.23  | 0.90  | 0.61 | 42.3 | 10.37 | 0.26  | 1.03  |
| 06353594+2616376  | 187.663  | 8.439    | 0.207 | 1      | —      | —    | g    | —        | —     | D3     | —   | —                      | —          | —          | —     | —        | —          | —     | —                                  | 11.189                      | 0.31                        | 1.12                 | 1                     | 35.2                                 | 0.88                          | 3.48                          | 11.112 | 0.28  | 1.02  | 0.06 | 35.6 | 11.12 | 0.28  | 1.04  |
| 06353794+0022498  | 210.789  | -3.342   | 1.585 | 1      | —      | —    | g    | —        | —     | D1     | —   | —                      | —          | —          | —     | —        | —          | —     | —                                  | 10.857                      | 0.51                        | 1.60                 | 1                     | 30.4                                 | 0.50                          | 3.57                          | 10.266 | 0.25  | 0.81  | 0.49 | 35.2 | 10.27 | 0.28  | 0.91  |
| 06354230+0226468  | 208.958  | -2.380   | 1.812 | 1      | —      | —    | g    | —        | —     | D3     | —   | —                      | —          | —          | —     | —        | e          | —     | —                                  | 10.778                      | 0.61                        | 1.90                 | 1                     | 60.4                                 | 0.26                          | 3.67                          | 10.103 | 0.31  | 1.00  | 0.56 | 72.7 | 10.09 | 0.35  | 1.12  |
| 06354472+0125487  | 212.416  | -4.143   | 0.966 | 1      | —      | —    | p?   | —        | —     | D1     | e   | o                      | —          | —          | —     | —        | —          | —     | —                                  | 10.126                      | 0.45                        | 1.40                 | 1                     | 58.0                                 | 0.72                          | 3.65                          | 9.766  | 0.29  | 0.92  | 0.30 | 62.1 | 9.79  | 0.30  | 0.98  |
| 06354512+0005377  | 211.225  | -3.532   | 1.354 | 7      | —      | —    | p?   | —        | —     | —      | —   | —                      | —          | —          | —     | —        | —          | —     | —                                  | 10.292                      | 1.18                        | 1.78                 | 1                     | 18.8                                 | 0.90                          | 3.64                          | 9.787  | 0.96  | 1.11  | 0.42 | ...  | ...   | 0.99  | 1.19  |
| 06354846+1115047  | 201.149  | 1.690    | 0.989 | 1      | —      | —    | g    | —        | —     | D1     | —   | —                      | —          | —          | —     | —        | o          | —     | —                                  | 11.161                      | 0.35                        | 1.36                 | 1                     | 51.0                                 | 0.44                          | 3.62                          |        |       |       |      |      |       |       |       |

Table B1: a) continued.

| 2MASX J          |         | <i>l</i>    | <i>b</i>    | EBV        | Object       |            |            | Sample      |            |             | Disc          | 2MRS        | Velocity |              | NIR         | Photom      | Ext         | <i>K</i> <sub>20</sub> | <i>H-K</i>  | <i>J-K</i>  | <i>vc</i>   | <i>a</i> | <i>b/a</i> | st.d. | <i>K</i> <sub>s</sub> <sup>o</sup> | ( <i>H-K</i> ) <sup>o</sup> | ( <i>J-K</i> ) <sup>c</sup> | <i>A<sub>K</sub></i> | <i>a</i> <sup>d</sup> | <i>K</i> <sub>s</sub> <sup>o,d</sup> | ( <i>H-K</i> ) <sup>o,c</sup> | ( <i>J-K</i> ) <sup>o,c</sup> |             |
|------------------|---------|-------------|-------------|------------|--------------|------------|------------|-------------|------------|-------------|---------------|-------------|----------|--------------|-------------|-------------|-------------|------------------------|-------------|-------------|-------------|----------|------------|-------|------------------------------------|-----------------------------|-----------------------------|----------------------|-----------------------|--------------------------------------|-------------------------------|-------------------------------|-------------|
| (1)              |         | deg<br>(2a) | deg<br>(2b) | mag<br>(3) | class<br>(4) | off<br>(5) | flg<br>(6) | gal<br>(7a) | TF<br>(7b) | obs<br>(7c) | ext'd<br>(7d) | type<br>(8) | (9)      | Opt<br>(10a) | HI<br>(10b) | flg<br>(11) | flg<br>(12) | flg<br>(13)            | mag<br>(14) | mag<br>(15) | mag<br>(16) | (17)     | (18)       | (19)  | (20)                               | mag<br>(21)                 | mag<br>(22)                 | mag<br>(23)          | mag<br>(24)           | (25)                                 | mag<br>(26)                   | mag<br>(27)                   | mag<br>(28) |
| 06410261+1015070 | 202.627 | 2.376       | 2.368       | 9          | -            | -          | -          | -           | -          | -           | -             | -           | -        | -            | -           | -           | -           | -                      | 10.776      | 1.52        | 2.94        | 1        | 51.2       | 0.58  | 3.63                               | 9.894                       | 1.12                        | 1.77                 | 0.73                  | ...                                  | ...                           | 1.17                          | 1.92        |
| 06410544+0934091 | 203.240 | 2.074       | 12.903      | 9          | -            | -          | -          | -           | -          | -           | -             | -           | -        | -            | -           | -           | -           | -                      | 11.155      | 1.41        | 3.03        | 1        | 32.8       | 0.84  | 3.90                               | 6.347                       | -0.73                       | -3.38                | 4.00                  | ...                                  | ...                           | -0.47                         | -2.53       |
| 06410605+0934460 | 203.232 | 2.081       | 12.416      | 8          | -            | -          | -          | -           | -          | -           | -             | -           | -        | -            | -           | U           | -           | -                      | 11.444      | 1.38        | 3.48        | 1        | 20.4       | 0.50  | 3.90                               | 6.818                       | -0.68                       | -2.69                | 3.85                  | ...                                  | ...                           | -0.44                         | -1.87       |
| 06410754+0930000 | 203.305 | 2.050       | 15.243      | 9          | -            | -          | -          | -           | -          | -           | -             | -           | -        | -            | -           | -           | -           | -                      | 8.925       | 0.86        | 2.19        | 1        | 102.0      | 0.70  | 3.90                               | 3.245                       | -1.67                       | -5.38                | 4.72                  | ...                                  | ...                           | -1.37                         | -4.38       |
| 06410774+0929150 | 203.317 | 2.045       | 14.294      | 9          | -            | -          | -          | -           | -          | -           | -             | -           | -        | -            | -           | -           | -           | -                      | 10.502      | 0.84        | 1.95        | 1        | 57.4       | 0.64  | 3.90                               | 5.176                       | -1.53                       | -5.15                | 4.43                  | ...                                  | ...                           | -1.25                         | -4.21       |
| 06411044+0934180 | 203.247 | 2.094       | 11.474      | 9          | -            | -          | -          | -           | -          | -           | -             | -           | -        | -            | -           | -           | -           | -                      | 11.709      | 1.84        | ...         | 1        | 15.8       | 0.44  | 3.90                               | 7.434                       | -0.06                       | ...                  | 3.55                  | ...                                  | ...                           | 0.17                          | ...         |
| 06411196+0929087 | 203.326 | 2.060       | 15.370      | 9          | -            | -          | -          | -           | -          | -           | -             | -           | -        | -            | -           | -           | -           | -                      | 9.244       | 2.02        | ...         | 1        | 208.0      | 1.00  | 3.76                               | 3.517                       | -0.53                       | ...                  | 4.76                  | ...                                  | ...                           | -0.22                         | ...         |
| 06411202+0935317 | 203.232 | 2.109       | 10.469      | 9          | -            | -          | -          | -           | -          | -           | -             | -           | -        | -            | -           | -           | -           | -                      | 10.782      | 1.85        | ...         | 1        | 52.4       | 0.52  | 3.74                               | 6.881                       | 0.11                        | ...                  | 3.74                  | ...                                  | ...                           | 0.32                          | ...         |
| 06411311+0925577 | 203.376 | 8.175       | 8           | 8          | -            | -          | -          | -           | -          | -           | -             | -           | -        | -            | -           | U           | o           | -                      | 11.842      | 0.69        | 1.04        | 1        | 32.2       | 0.82  | 3.66                               | 8.796                       | -0.67                       | -3.02                | 2.53                  | ...                                  | ...                           | -0.51                         | -2.48       |
| 06411331+0930117 | 203.313 | 2.073       | 16.205      | 8          | -            | -          | -          | -           | -          | -           | -             | -           | -        | -            | -           | U           | -           | -                      | 11.659      | 1.05        | 2.99        | 1        | 22.0       | 0.76  | 3.74                               | 5.621                       | -1.64                       | -5.06                | 5.02                  | ...                                  | ...                           | -1.32                         | -3.99       |
| 06411487+0925548 | 203.383 | 7.882       | 8           | 8          | -            | -          | -          | -           | -          | -           | -             | -           | -        | -            | -           | U           | -           | -                      | 13.521      | 0.67        | 1.81        | -1       | 10.0       | 1.00  | 3.68                               | 10.584                      | -0.63                       | -2.81                | 2.44                  | ...                                  | ...                           | -0.48                         | -1.58       |
| 06414659+0147270 | 210.236 | -1.333      | 1.165       | 8          | -            | -          | -          | -           | -          | -           | -             | -           | -        | -            | -           | U           | c           | -                      | 11.203      | 0.67        | 1.40        | 1        | 34.0       | 0.58  | 3.66                               | 10.754                      | 0.42                        | 0.80                 | 1.03                  | ...                                  | ...                           | 0.45                          | 0.83        |
| 06414770+1102252 | 202.008 | 2.892       | 8.818       | 8          | -            | -          | -          | -           | -          | -           | -             | D4          | -        | -            | -           | -           | -           | e                      | 11.289      | 1.52        | 1.43        | 1        | 30.2       | 0.94  | 3.56                               | 10.384                      | 0.38                        | 1.01                 | 25.5                  | 32.1                                 | 11.00                         | 1.06                          | ...         |
| 06421440+2603013 | 188.528 | 8.892       | 0.112       | 1          | -            | -          | -          | g           | -          | t           | N             | D1          | c        | o            | -           | -           | -           | -                      | 10.802      | 0.28        | 0.4         | 1        | 50.4       | 0.32  | 3.56                               | 10.760                      | 0.27                        | 0.99                 | 0.03                  | 50.6                                 | 10.77                         | 0.27                          | 0.99        |
| 06443350+0210256 | 110.102 | -0.755      | 1.320       | 8          | -            | -          | -          | g           | -          | -           | -             | -           | -        | -            | -           | -           | -           | -                      | 11.128      | 1.15        | 2.23        | 1        | 25.8       | 0.72  | 3.76                               | 10.636                      | 0.93                        | 1.58                 | 0.41                  | ...                                  | ...                           | 0.96                          | 1.66        |
| 06433846+0107470 | 213.049 | -2.250      | 5.495       | 8          | -            | -          | -          | -           | -          | -           | -             | -           | er       | g            | -           | -           | -           | -                      | 12.048      | 0.46        | 1.13        | -2       | 22.2       | 0.68  | 3.76                               | 10.001                      | -0.45                       | -1.60                | 1.70                  | ...                                  | ...                           | -0.34                         | -1.24       |
| 06434846+0108200 | 213.076 | -2.217      | 6.558       | 7          | -            | -          | -          | -           | -          | -           | -             | -           | -        | -            | -           | -           | -           | -                      | 8.468       | 1.05        | 1.91        | 1        | 80.4       | 0.86  | 3.76                               | 6.024                       | -0.03                       | -1.35                | 2.03                  | ...                                  | ...                           | 0.09                          | -0.92       |
| 06435110+2550328 | 188.877 | 9.919       | 0.107       | 1          | -            | -          | -          | g           | -          | -           | -             | D1          | c        | o            | -           | -           | -           | -                      | 10.968      | 0.37        | 1.01        | 1        | 37.4       | 0.96  | 3.31                               | 10.928                      | 0.35                        | 1.01                 | 0.03                  | 37.6                                 | 10.93                         | 0.35                          | 1.02        |
| 06440058+1224067 | 201.040 | 4.500       | 0.438       | 1          | -            | -          | -          | g           | -          | -           | -             | D1          | e        | o            | -           | -           | -           | -                      | 10.009      | 0.32        | 1.17        | 1        | 68.4       | 0.38  | 3.53                               | 9.846                       | 0.25                        | 0.95                 | 0.14                  | 70.1                                 | 9.86                          | 0.26                          | 0.98        |
| 06442769+1755566 | 228.269 | -9.665      | 0.416       | 1          | -            | -          | -          | g           | -          | t           | -             | D1          | c        | o            | -           | h           | -           | -                      | 11.154      | 0.15        | 0.92        | 1        | 88.0       | 0.26  | 3.47                               | 10.999                      | 0.09                        | 0.71                 | 0.13                  | 91.4                                 | 10.91                         | 0.09                          | 0.74        |
| 06443785+1235048 | 223.426 | -7.189      | 0.555       | 1          | -            | -          | -          | -           | -          | -           | -             | D1          | c        | o            | -           | -           | -           | -                      | 11.302      | 0.35        | 1.24        | 1        | 28.4       | 0.80  | 3.63                               | 11.095                      | 0.26                        | 0.97                 | 0.17                  | 29.5                                 | 11.10                         | 0.27                          | 1.00        |
| 06444284+0013432 | 211.962 | -1.392      | 1.727       | 7          | -            | -          | -          | -           | -          | -           | -             | -           | -        | -            | -           | -           | -           | -                      | 11.838      | 1.23        | 0.97        | 1        | 20.0       | 0.52  | 3.78                               | 11.195                      | 0.95                        | 2.12                 | 0.53                  | ...                                  | ...                           | 0.98                          | 2.23        |
| 06445738+1317198 | 224.098 | -7.429      | 0.444       | 1          | -            | -          | -          | g           | -          | -           | -             | D2          | c        | o            | -           | -           | -           | -                      | 10.407      | 0.27        | 1.08        | 1        | 42.0       | 0.92  | 3.66                               | 10.242                      | 0.20                        | 0.86                 | 0.14                  | 43.1                                 | 10.26                         | 0.21                          | 0.89        |
| 06445958+0020511 | 211.888 | -1.275      | 3.226       | 7          | -            | -          | -          | -           | -          | -           | -             | -           | -        | -            | -           | -           | -           | -                      | 11.414      | 1.50        | 2.97        | 1        | 19.6       | 0.60  | 3.78                               | 10.212                      | 0.97                        | 1.37                 | 1.00                  | ...                                  | ...                           | 1.03                          | 1.58        |
| 06451445+0025131 | 211.851 | -1.187      | 4.514       | 8          | -            | -          | -          | -           | -          | -           | -             | -           | -        | -            | -           | -           | -           | -                      | 11.136      | 1.16        | 2.96        | 1        | 34.4       | 0.50  | 3.78                               | 9.454                       | 0.42                        | 0.72                 | 1.40                  | ...                                  | ...                           | 0.51                          | 1.02        |
| 06451612+0022241 | 211.896 | -1.202      | 4.144       | 7          | -            | -          | -          | -           | -          | -           | -             | -           | -        | -            | -           | -           | -           | -                      | 10.855      | 1.32        | 2.72        | 1        | 34.8       | 0.70  | 3.78                               | 9.311                       | 0.64                        | 0.66                 | 1.28                  | ...                                  | ...                           | 0.72                          | 0.93        |
| 06452386+0301101 | 214.933 | -2.719      | 1.783       | 9          | -            | -          | -          | -           | -          | -           | -             | -           | -        | -            | -           | -           | -           | -                      | 11.846      | 0.56        | 1.32        | -2       | 41.0       | 0.66  | 3.67                               | 11.182                      | 0.26                        | 0.43                 | 0.55                  | ...                                  | ...                           | 0.30                          | 0.55        |
| 06453206+0006198 | 212.165 | -1.265      | 2.210       | 9          | -            | -          | -          | -           | -          | -           | -             | -           | -        | -            | -           | -           | -           | -                      | 12.071      | 1.21        | 2.34        | 1        | 23.4       | 0.64  | 3.70                               | 11.248                      | 0.84                        | 1.24                 | 0.68                  | ...                                  | ...                           | 0.89                          | 1.38        |
| 06453740+0019493 | 211.975 | -1.143      | 3.102       | 8          | -            | -          | -          | -           | -          | -           | -             | -           | -        | -            | -           | U           | -           | -                      | 11.466      | 0.74        | 1.84        | -2       | 22.2       | 0.82  | 3.77                               | 10.310                      | 0.23                        | 0.29                 | 0.96                  | ...                                  | ...                           | 0.29                          | 0.50        |
| 06454086+0022253 | 211.943 | -1.110      | 3.441       | 8          | -            | -          | -          | -           | -          | -           | -             | -           | -        | -            | -           | -           | -           | -                      | 11.104      | 1.36        | 2.75        | 1        | 27.8       | 0.78  | 3.77                               | 9.822                       | 0.79                        | 1.04                 | 1.07                  | ...                                  | ...                           | 0.86                          | 1.27        |
| 06454358+1411382 | 225.000 | -7.661      | 0.469       | 1          | -            | -          | -          | g           | -          | -           | -             | D4          | c        | o            | -           | -           | -           | -                      | 11.267      | 0.39        | 1.34        | 1        | 29.8       | 0.86  | 3.59                               | 11.092                      | 0.32                        | 1.11                 | 0.55                  | 30.7                                 | 11.10                         | 0.32                          | 1.14        |
| 06455204+1811513 | 228.658 | -9.378      | 0.383       | 9          | -            | e          | -          | -           | -          | -           | -             | -           | cr       | o            | -           | -           | -           | o                      | 11.189      | 0.25        | 0.97        | -2       | 73.4       | 0.62  | 3.46                               | 11.046                      | 0.18                        | 0.60                 | 0.12                  | ...                                  | ...                           | 0.19                          | 0.62        |
| 06455492+1812493 | 228.677 | -9.375      | 0.384       | 1          | -            | o          | -          | g           | -          | -           | N             | D1          | ca       | -            | -           | h           | -           | ao                     | 10.121      | -0.03       | 0.69        | -2       | 82.8       | 1.00  | 3.46                               | 9.978                       | -0.10                       | 0.50                 | 0.12                  | 85.4                                 | 9.97                          | -0.09                         | 0.52        |
| 06461612+0006204 | 212.249 | -1.102      | 3.113       | 8          | -            | -          | -          | -           | -          | -           | -             | -           | -        | -            | -           | -           | -           | -                      | 9.844       | 1.22        | 2.28        | 1        | 111.4      | 0.68  | 3.74                               | 8.684                       | 0.70                        | 0.74                 | 0.96                  | ...                                  | ...                           | 0.77                          | 0.94        |
| 06465145+0120261 | 211.217 | -0.407      | 6.210       | 9          | -            | -          | -          | -           | -          | -           | -             | -           | -        | -            | -           | -           | -           | -                      | 12.921      | ...         | 1.68        | -2       | 22.0       | 1.00  | 3.81                               | 10.607                      | ...                         | -1.40                | 1.92                  | ...                                  | ...                           | ...                           | -0.99       |
| 06465228+0118164 | 211.250 | -0.421      | 6.638       | 9          | -            | -          | -          | -           | -          | -           | -             | -           | -        | -            | -           | -           | -           | -                      | 13.331      | 0.49        | 1.76        | -2       | 17.4       | 0.80  | 3.82                               | 10.858                      | -0.61                       | -1.54                | 2.06                  | ...                                  | ...                           | -0.47                         | -1.10       |
| 06465294+0118564 | 211.242 | -0.413      | 6.639       | 9          | -            | -          | -          | -           | -          | -           | -             | -           | -        | -            | -           | -           | -           | -                      | 11.672      | 0.62        | 1.67        | 1        | 38.2       | 1.00  | 3.82                               | 9.198                       | -0.48                       | -1.62                | 2.06                  | ...                                  | ...                           | -0.35                         | -1.19       |
| 06465339+0120021 | 211.226 | -0.403      | 6.257       | 9          | -            | -          | -          | -           | -          | -           | -             | -           | -        | -            | -           | -           | -           | -                      | 12.408      | 0.59        | 1.58        | -2       | 24.2       | 0.52  | 3.81                               | 10.077                      | -0.45                       | -1.53                | 1.94                  | ...                                  | ...                           | -0.32                         | -1.12       |
| 06465405+0118401 | 211.248 | -0.411      | 6.706       | 9          | -            | -          | -          | -           | -          | -           | -             | -           | -        | -            | -           | -           | -           | -                      | 11.241      | 0.81        | 2.20        | 1        | 62.8       | 0.90  | 3.81                               | 8.742                       | -0.30                       | -1.13                | 2.08                  | ...                                  | ...                           | -0.16                         | -0.69       |
| 06465617+0117059 | 211.275 | -0.415      | 5.418       | 8          | -            | o          | -          | -           | -          | -           | -             | -           | -        | -            | -           | -           | -           | -                      | 11.213      | 0.13        | 1.17        | 1        | 41.8       | 0.74  | 3.81                               | 9.194                       | -0.77                       | -1.52                | 1.68                  | ...                                  | ...                           | -0.66                         | -1.17       |
| 06470937+1057266 | 202.680 | 4.034       | 0.444       | 1          | -            | -          | -          | g           | -          | t           | N             | D1          | e        | o            | -           | -           | -           | -                      | 10.874      | 0.32        | 1.17        | 1        | 46.4       | 0.46  | 3.62                               | 10.709                      | 0.24                        | 0.95                 | 0.14                  | 47.6                                 | 10.72                         | 0.25                          | 0.98        |
| 06471340+0026072 | 212.064 | -0.739      | 3.101       | 7          | -            | -          | -          | -           | -          | -           | -             | -           | -        | -            | -           | -           | -           | -                      | 8.987       | 1.52        | 3.35        | 1        | 65.6       | 0.54  | 3.76                               | 7.832                       | 1.01                        | 1.81                 | 0.96                  | ...                                  | ...                           | 1.07                          | 2.02        |
| 06473023+0540270 | 207.433 | 1.712       | 0.762       | 8          | -            | -          | -          | -           | -          | -           | -             | -           | -        | -            | -           | -           | -           | -                      | 10.618      | 0.61        | 1.53        | 1        | 58.0       | 0.46  | 3.73                               | 10.334                      | 0.48                        | 1.15                 | 0.24                  | ...                                  | ...                           | 0.50                          | 1.20        |
| 06473511+1203159 | 201.746 | 4.623       | 0.338       | 1          | -            | -          | -          | g           | -          | -           | -             | D1          | e        | o            | -           | -           | -           | -                      | 11.240      | 0.42        | 1.25        | 1        | 35.0       | 0.72  | 3.60                               | 11.114                      | 0.37                        | 1.08                 | 0.10                  | 35.7                                 | 11.13                         | 0.37                          | 1.10        |
| 06473930+0000098 | 212.503 | -0.843      | 0.982       | 1          | -            | -          | -          | g           | -          | t           | N             | D1          | e        | o            | -           | -           | -           | -                      | 11.081      | 0.50        | 1.67        | 1        |            |       |                                    |                             |                             |                      |                       |                                      |                               |                               |             |

Table B1: a) continued.

| 2MASX J          | <i>l</i>    | <i>b</i>    | EBV        | Object       | Sample     | Disc        | 2MRS        | Velocity   | NIR         | Photom        | Ext         | <i>K</i> <sub>20</sub> | <i>H-K</i>   | <i>J-K</i>  | <i>vc</i>    | <i>a</i>     | <i>b/a</i>   | std.d. | <i>K</i> <sub>S</sub> <sup>o</sup> | ( <i>H-K</i> ) <sup>o</sup> | ( <i>J-K</i> ) <sup>o</sup> | <i>A</i> <sub>K</sub> | <i>a</i> <sup>d</sup> | <i>K</i> <sub>S</sub> <sup>o,d</sup> | ( <i>H-K</i> ) <sup>o,c</sup> | ( <i>J-K</i> ) <sup>o,c</sup> |             |             |           |             |             |             |       |
|------------------|-------------|-------------|------------|--------------|------------|-------------|-------------|------------|-------------|---------------|-------------|------------------------|--------------|-------------|--------------|--------------|--------------|--------|------------------------------------|-----------------------------|-----------------------------|-----------------------|-----------------------|--------------------------------------|-------------------------------|-------------------------------|-------------|-------------|-----------|-------------|-------------|-------------|-------|
| (1)              | deg<br>(2a) | deg<br>(2b) | mag<br>(3) | class<br>(4) | off<br>(5) | flag<br>(6) | gal<br>(7a) | TF<br>(7b) | obs<br>(7c) | ext'd<br>(7d) | type<br>(8) | (9)                    | Opt<br>(10a) | HI<br>(10b) | flag<br>(11) | flag<br>(12) | flag<br>(13) | (14)   | mag<br>(15)                        | mag<br>(16)                 | (17)                        | "<br>(18)             | (19)                  | (20)                                 | mag<br>(21)                   | mag<br>(22)                   | mag<br>(23) | mag<br>(24) | "<br>(25) | mag<br>(26) | mag<br>(27) | mag<br>(28) |       |
| 06533601-2123207 | 232.370     | -9.119      | 0.290      | 1            | -          | -           | g           | -          | -           | -             | D3          | c                      | -            | -           | -            | -            | -            | -      | 10.561                             | 0.34                        | 1.13                        | 1                     | 49.4                  | 0.90                                 | 3.49                          | 10.453                        | 0.29        | 0.98        | 0.09      | 50.1        | 10.46       | 0.30        | 1.00  |
| 06535387-0337410 | 216.441     | -1.107      | 0.920      | 1            | -          | -           | g           | t          | N           | -             | D1          | c                      | -            | -           | h            | -            | -            | -      | 10.799                             | 0.57                        | 1.61                        | 1                     | 63.2                  | 0.20                                 | 3.74                          | 10.456                        | 0.42        | 1.16        | 0.28      | 68.5        | 10.46       | 0.43        | 1.22  |
| 06545485+1917587 | 195.878     | 9.194       | 0.094      | 1            | -          | -           | g           | t          | -           | -             | D1          | c                      | -            | -           | -            | -            | -            | -      | 11.131                             | 0.23                        | 0.89                        | 1                     | 61.6                  | 0.48                                 | 3.41                          | 11.096                        | 0.21        | 0.84        | 0.03      | 61.9        | 11.10       | 0.21        | 0.85  |
| 06541017-2006209 | 231.259     | -8.441      | 0.332      | 1            | -          | -           | g           | -          | -           | -             | D1          | c                      | -            | -           | -            | -            | -            | -      | 11.296                             | 0.33                        | 1.14                        | 1                     | 41.8                  | 0.30                                 | 3.59                          | 11.172                        | 0.28        | 0.97        | 0.10      | 42.6        | 11.18       | 0.29        | 0.99  |
| 06541984-1208232 | 224.088     | -4.871      | 0.773      | 1            | -          | -           | g           | -          | N           | -             | D2          | c                      | -            | -           | *            | -            | -            | -      | 11.129                             | 0.33                        | 1.17                        | 1                     | 33.8                  | 0.52                                 | 3.72                          | 10.841                        | 0.20        | 0.79        | 0.24      | 35.8        | 10.86       | 0.21        | 0.84  |
| 06543456+0703194 | 206.999     | 3.905       | 0.275      | 1            | -          | -           | g           | -          | -           | -             | D1          | e                      | -            | -           | -            | -            | -            | -      | 10.559                             | 0.52                        | 1.31                        | 1                     | 34.2                  | 0.84                                 | 3.62                          | 10.129                        | 0.48        | 1.18        | 0.09      | 34.8        | 10.46       | 0.48        | 1.19  |
| 06543530-0432170 | 217.330     | -1.368      | 4.781      | 1            | -          | -           | g           | -          | -           | -             | -           | -                      | -            | -           | -            | -            | -            | -      | 11.910                             | 1.28                        | 2.65                        | 1                     | 39.2                  | 0.88                                 | 3.70                          | 10.429                        | 0.48        | 0.27        | 1.48      | ...         | ...         | 0.58        | 0.59  |
| 06544554-0354210 | 216.787     | -1.042      | 2.158      | 7            | -          | -           | -           | -          | -           | -             | -           | -                      | -            | -           | -            | -            | -            | -      | 10.572                             | 0.93                        | 2.65                        | 1                     | 32.8                  | 0.78                                 | 3.72                          | 9.768                         | 0.58        | 1.18        | 0.67      | ...         | ...         | 0.62        | 1.32  |
| 06551779-0031145 | 213.835     | 0.621       | 3.286      | 9            | -          | -           | -           | -          | -           | -             | -           | -                      | -            | -           | -            | -            | -            | -      | 10.751                             | 0.94                        | 1.60                        | 1                     | 80.2                  | 0.64                                 | 3.74                          | 9.527                         | 0.40        | -0.03       | 1.02      | ...         | ...         | 0.47        | 0.18  |
| 06552670-0411095 | 217.114     | -1.018      | 1.289      | 1            | -          | -           | g           | -          | N           | -             | D1          | -                      | -            | -           | *            | -            | -            | -      | 11.460                             | 0.52                        | 1.55                        | 1                     | 40.8                  | 0.76                                 | 3.66                          | 10.980                        | 0.31        | 0.91        | 0.40      | 46.9        | 10.94       | 0.33        | 1.00  |
| 06560633+0033477 | 212.963     | 1.295       | 1.123      | 8            | -          | -           | -           | -          | -           | -             | -           | -                      | -            | -           | -            | -            | -            | -      | 10.002                             | 1.57                        | 2.90                        | 1                     | 43.4                  | 0.52                                 | 3.73                          | 9.584                         | 1.38        | 2.35        | 0.35      | ...         | ...         | 1.41        | 2.42  |
| 06562110+0600057 | 208.141     | 3.822       | 0.360      | 1            | -          | -           | g           | -          | -           | -             | D3          | e                      | -            | -           | h            | -            | -            | -      | 11.206                             | 0.33                        | 1.03                        | 1                     | 34.6                  | 0.92                                 | 3.57                          | 11.072                        | 0.27        | 0.86        | 0.11      | 35.5        | 11.08       | 0.27        | 0.88  |
| 06562641-0300515 | 216.183     | -0.266      | 1.678      | 1            | -          | -           | g           | -          | N           | -             | D3          | -                      | -            | -           | -            | -            | -            | -      | 11.677                             | 0.58                        | 1.78                        | 1                     | 27.0                  | 0.70                                 | 3.68                          | 11.067                        | 0.31        | 0.95        | 0.52      | 32.2        | 11.04       | 0.34        | 1.06  |
| 06563214+0612076 | 207.983     | 3.953       | 0.317      | 1            | -          | -           | g           | -          | -           | -             | D4          | e                      | -            | -           | -            | -            | -            | -      | 11.006                             | 0.30                        | 1.10                        | 1                     | 28.0                  | 0.86                                 | 3.57                          | 10.888                        | 0.25        | 0.94        | 0.10      | 28.5        | 10.90       | 0.25        | 0.96  |
| 06563505-1920335 | 230.819     | -7.595      | 0.319      | 1            | -          | -           | g           | t          | N           | -             | D1          | c                      | -            | -           | -            | -            | -            | -      | 10.598                             | 0.30                        | 1.11                        | 1                     | 41.8                  | 0.38                                 | 3.56                          | 10.479                        | 0.25        | 0.95        | 0.10      | 42.5        | 10.49       | 0.26        | 0.97  |
| 06570322-0501137 | 218.040     | -1.042      | 1.101      | 1            | -          | -           | g           | -          | -           | -             | D1          | c                      | -            | -           | -            | -            | -            | -      | 11.542                             | 0.36                        | 1.10                        | 1                     | 54.2                  | 0.26                                 | 3.74                          | 11.132                        | 0.18        | 0.55        | 0.34      | 60.0        | 11.13       | 0.20        | 0.62  |
| 06570782-0811036 | 220.866     | -2.467      | 7.984      | 9            | -          | -           | -           | -          | -           | -             | -           | -                      | -            | -           | -            | -            | -            | -      | 12.053                             | ...                         | 1.23                        | -2                    | 32.0                  | 1.0                                  | 3.78                          | 9.078                         | ...         | -2.74       | 2.47      | ...         | ...         | ...         | -2.21 |
| 06571091-0810386 | 220.866     | -2.452      | 7.692      | 9            | -          | -           | -           | -          | -           | -             | -           | -                      | -            | -           | -            | -            | -            | -      | 9.883                              | 1.93                        | ...                         | 1                     | 94.6                  | 1.00                                 | 3.78                          | 7.017                         | 0.65        | ...         | 2.38      | ...         | ...         | 0.80        | ...   |
| 06571428-0819446 | 221.007     | -2.509      | 6.150      | 8            | -          | -           | -           | -          | -           | -             | -           | -                      | -            | -           | -            | -            | -            | -      | 8.422                              | 0.86                        | 1.94                        | 1                     | 76.2                  | 0.46                                 | 3.75                          | 6.131                         | -0.16       | -1.12       | 1.90      | ...         | ...         | -0.04       | -0.71 |
| 06571604-0819466 | 221.011     | -2.502      | 6.031      | 9            | -          | -           | -           | -          | -           | -             | -           | -                      | -            | -           | -            | -            | -            | -      | 13.384                             | ...                         | ...                         | -1                    | 19.0                  | 1.00                                 | 3.75                          | 11.137                        | ...         | ...         | 1.87      | ...         | ...         | ...         | ...   |
| 06571729-0109507 | 214.635     | 0.771       | 2.951      | 7            | -          | -           | -           | -          | -           | -             | -           | -                      | -            | -           | -            | -            | -            | -      | 10.208                             | 1.44                        | 3.09                        | 1                     | 33.6                  | 0.76                                 | 3.70                          | 9.108                         | 0.96        | 1.63        | 0.91      | ...         | ...         | 1.01        | 1.82  |
| 06572149-0508597 | 218.189     | -1.033      | 1.143      | 1            | -          | -           | g           | t          | N           | -             | D1          | -                      | -            | -           | h            | -            | -            | -      | 11.000                             | 0.42                        | 1.48                        | 1                     | 83.6                  | 0.26                                 | 3.74                          | 10.574                        | 0.23        | 0.91        | 0.35      | 95.2        | 10.52       | 0.25        | 0.99  |
| 06572470-2443369 | 235.806     | -9.768      | 0.236      | 1            | -          | -           | g           | -          | -           | -             | D2          | c                      | -            | -           | h            | -            | -            | -      | 10.136                             | 0.32                        | 1.12                        | 1                     | 77.4                  | 0.26                                 | 3.54                          | 10.048                        | 0.28        | 1.01        | 0.07      | 78.3        | 10.06       | 0.28        | 1.02  |
| 06572487-2456229 | 236.001     | -9.859      | 0.264      | 1            | -          | -           | g           | -          | -           | -             | D1          | c                      | -            | -           | -            | -            | -            | -      | 10.544                             | 0.26                        | 1.01                        | 1                     | 49.4                  | 0.68                                 | 3.49                          | 10.446                        | 0.22        | 0.88        | 0.08      | 50.0        | 10.46       | 0.23        | 0.89  |
| 06573331+1103141 | 203.744     | 6.358       | 0.141      | 1            | -          | -           | g           | -          | -           | -             | D2          | c                      | -            | -           | h            | -            | -            | -      | 11.203                             | 0.38                        | 1.12                        | 1                     | 29.2                  | 0.72                                 | 3.58                          | 11.150                        | 0.36        | 1.05        | 0.04      | 29.4        | 11.16       | 0.36        | 1.06  |
| 06573486-0952230 | 222.423     | -3.135      | 1.643      | 8            | -          | -           | -           | -          | -           | -             | -           | -                      | -            | -           | -            | -            | -            | -      | 11.060                             | 0.84                        | 2.25                        | 1                     | 36.4                  | 0.56                                 | 3.71                          | 10.448                        | 0.57        | 1.43        | 0.51      | ...         | ...         | 0.60        | 1.54  |
| 06580164+1240017 | 202.340     | 7.178       | 0.134      | 1            | -          | -           | g           | -          | -           | -             | D2          | c                      | -            | -           | h            | -            | -            | -      | 10.164                             | 0.37                        | 1.08                        | 1                     | 35.4                  | 0.88                                 | 3.52                          | 10.114                        | 0.35        | 1.01        | 0.04      | 35.6        | 10.12       | 0.35        | 1.02  |
| 06580289-0520410 | 218.441     | -0.969      | 1.282      | 1            | -          | -           | g           | -          | -           | -             | D1          | c                      | -            | -           | h            | -            | -            | -      | 10.245                             | 0.49                        | 1.51                        | 1                     | 49.6                  | 0.96                                 | 3.70                          | 9.767                         | 0.27        | 0.87        | 0.40      | 56.0        | 9.76        | 0.30        | 0.96  |
| 06582558-0138254 | 215.189     | 0.806       | 1.261      | 9            | -          | -           | -           | -          | -           | -             | -           | -                      | -            | -           | -            | -            | -            | -      | 10.730                             | 0.81                        | 1.82                        | 1                     | 53.8                  | 0.44                                 | 3.72                          | 10.260                        | 0.60        | 1.19        | 0.39      | ...         | ...         | 0.62        | 1.27  |
| 06583710+1240008 | 202.405     | 7.307       | 0.120      | 1            | -          | -           | g           | -          | -           | -             | D1          | c                      | -            | -           | h            | -            | -            | -      | 10.665                             | 0.36                        | 1.08                        | 1                     | 40.8                  | 0.82                                 | 3.40                          | 10.620                        | 0.34        | 1.02        | 0.04      | 41.0        | 10.63       | 0.34        | 1.03  |
| 06584227-0456074 | 218.152     | -0.637      | 3.779      | 9            | -          | -           | -           | -          | -           | -             | -           | -                      | -            | -           | -            | -            | -            | -      | 10.865                             | 0.85                        | 2.35                        | 1                     | 62.2                  | 0.30                                 | 3.76                          | 9.457                         | 0.22        | 0.47        | 1.17      | ...         | ...         | 0.30        | 0.72  |
| 06584549-0341214 | 217.049     | -0.056      | 1.972      | 8            | -          | -           | g           | -          | -           | -             | -           | -                      | -            | -           | -            | -            | -            | -      | 11.174                             | 0.65                        | 1.37                        | 1                     | 61.4                  | 0.40                                 | 3.72                          | 10.439                        | 0.32        | 0.39        | 0.61      | ...         | ...         | 0.36        | 0.52  |
| 06585638-0453441 | 218.143     | -0.567      | 3.923      | 8            | -          | -           | g           | -          | -           | -             | -           | -                      | -            | -           | -            | -            | -            | -      | 11.903                             | 1.15                        | 2.44                        | 1                     | 44.6                  | 0.36                                 | 3.78                          | 10.441                        | 0.50        | 0.49        | 1.22      | ...         | ...         | 0.57        | 0.75  |
| 06590153+0634579 | 207.922     | 4.677       | 0.262      | 1            | -          | -           | g           | t          | N           | -             | D1          | e                      | -            | -           | h            | -            | -            | -      | 11.085                             | 0.30                        | 1.04                        | 1                     | 59.8                  | 0.36                                 | 3.44                          | 10.987                        | 0.26        | 0.91        | 0.08      | 60.8        | 10.99       | 0.26        | 0.93  |
| 06590970-0249301 | 216.327     | 0.428       | 1.274      | 1            | -          | -           | g           | -          | N           | -             | D2          | -                      | -            | -           | -            | -            | -            | -      | 11.389                             | 0.64                        | 1.78                        | 1                     | 42.8                  | 0.80                                 | 3.75                          | 10.914                        | 0.43        | 1.15        | 0.39      | 49.1        | 10.88       | 0.45        | 1.24  |
| 06591297-0354541 | 217.302     | -0.058      | 6.505      | 8            | -          | -           | -           | -          | -           | -             | -           | -                      | -            | -           | -            | -            | -            | -      | 9.237                              | 1.23                        | 2.95                        | 1                     | 72.8                  | 0.84                                 | 3.79                          | 6.813                         | 0.16        | -0.28       | 2.01      | ...         | ...         | 0.28        | 0.15  |
| 06591376+0614318 | 208.250     | 4.569       | 0.276      | 1            | -          | -           | g           | t          | N           | -             | D1          | e                      | -            | -           | -            | -            | -            | -      | 10.876                             | 0.40                        | 1.24                        | 1                     | 54.0                  | 0.28                                 | 3.51                          | 10.773                        | 0.36        | 1.10        | 0.09      | 54.8        | 10.78       | 0.36        | 1.12  |
| 06591437-0351441 | 217.258     | -0.028      | 3.596      | 8            | -          | -           | g           | -          | -           | -             | -           | -                      | -            | -           | -            | -            | -            | -      | 11.551                             | 1.00                        | 2.19                        | 1                     | 42.4                  | 0.68                                 | 3.70                          | 10.211                        | 0.40        | 0.41        | 1.11      | ...         | ...         | 0.47        | 0.64  |
| 06591578-0359361 | 217.377     | -0.083      | 9.908      | 8            | -          | -           | -           | -          | -           | -             | -           | -                      | -            | -           | -            | -            | -            | -      | 8.332                              | 0.99                        | 2.17                        | 1                     | 100.4                 | 0.72                                 | 3.79                          | 4.640                         | -0.65       | -2.75       | 3.07      | ...         | ...         | -0.45       | -2.10 |
| 06591689-0359510 | 217.383     | -0.081      | 9.740      | 9            | -          | -           | -           | -          | -           | -             | -           | -                      | -            | -           | -            | -            | -            | -      | 9.902                              | 0.93                        | 1.85                        | 1                     | 79.8                  | 0.52                                 | 3.77                          | 6.273                         | -0.68       | -2.98       | 3.02      | ...         | ...         | -0.49       | -2.34 |
| 06591745-0354371 | 217.307     | -0.039      | 6.061      | 9            | -          | -           | -           | -          | -           | -             | -           | -                      | -            | -           | -            | -            | -            | -      | 11.772                             | 1.01                        | 2.24                        | 1                     | 38.2                  | 0.74                                 | 3.79                          | 9.514                         | 0.00        | -0.77       | 1.88      | ...         | ...         | 0.12        | -0.37 |
| 06591950-0358580 | 217.375     | -0.064      | 10.216     | 9            | -          | -           | -           | -          | -           | -             | -           | -                      | -            | -           | -            | -            | -            | -      | 10.520                             | 1.32                        | 3.17                        | 1                     | 43.6                  | 0.80                                 | 3.77                          | 6.714                         | -0.37       | -1.91       | 3.16      | ...         | ...         | -0.17       | -1.23 |
| 06592134-2553589 | 237.072     | -9.876      | 0.250      | 1            | -          | -           | g           | t          | -           | -             | D1          | c                      | -            | -           | h            | -            | -            | -      | 10.144                             | 0.29                        | 1.01                        | 1                     | 80.4                  | 0.44                                 | 3.48                          | 10.051                        | 0.24        | 0.88        | 0.08      | 81.4        | 10.06       | 0.25        | 0.90  |
| 06592209-0415410 | 217.628     | -0.182      | 4.880      | 9            | -          | -           | g           | -          | -           | -             | -           | -                      | -            | -           | -            | -            | -            | -      | 9.647                              | 1.05                        | 2.14                        | 1                     | 110.0                 | 0.44                                 | 3.79                          | 7.829                         | 0.24        | -0.29       | 1.51      | ...         | ...         | 0.34        | 0.04  |
| 06593186-0405420 | 217.498     | -0.070      | 3.020      |              |            |             |             |            |             |               |             |                        |              |             |              |              |              |        |                                    |                             |                             |                       |                       |                                      |                               |                               |             |             |           |             |             |             |       |

Table B1: a) continued.

[illegible]



Table B1: a) continued.

| 2MASX J          | <i>l</i> | <i>b</i> | EBV   | Object |     | Sample | Disc | 2MRS | Velocity | NIR  | Photom | Ext   | <i>K</i> <sub>20</sub> | <i>H-K</i> | <i>J-K</i> | vc   | <i>a</i> | <i>b/a</i> | st.d. | <i>K</i> <sub>s</sub> <sup>o</sup> | ( <i>H-K</i> ) <sup>o</sup> | ( <i>J-K</i> ) <sup>o</sup> | <i>A<sub>K</sub></i> | <i>a</i> <sub>d</sub> <sup>o</sup> | <i>K</i> <sub>s</sub> <sup>o,d</sup> | ( <i>H-K</i> ) <sup>o,c</sup> | ( <i>J-K</i> ) <sup>o,c</sup> |       |      |      |      |
|------------------|----------|----------|-------|--------|-----|--------|------|------|----------|------|--------|-------|------------------------|------------|------------|------|----------|------------|-------|------------------------------------|-----------------------------|-----------------------------|----------------------|------------------------------------|--------------------------------------|-------------------------------|-------------------------------|-------|------|------|------|
| (1)              | deg      | deg      | (3)   | class  | off | gal    | TF   | obs  | ext'd    | type | flag   | flag  | flag                   | mag        | mag        | (17) | "        | (19)       | (20)  | mag                                | mag                         | mag                         | mag                  | "                                  | mag                                  | mag                           | mag                           |       |      |      |      |
| (1)              | (2a)     | (2b)     | (3)   | (4)    | (5) | (6)    | (7a) | (7c) | (7d)     | (8)  | (9)    | (10a) | (10b)                  | (11)       | (12)       | (13) | (14)     | (15)       | (16)  | (17)                               | (18)                        | (19)                        | (20)                 | (21)                               | (22)                                 | (23)                          | (24)                          | (25)  | (26) | (27) | (28) |
| 07134001+0612196 | 209.906  | 7.757    | 0.140 | 1      | —   | —      | g    | —    | —        | D2   | c      | o     | —                      | 10.775     | 0.27       | 0.99 | 1        | 46.8       | 0.68  | 3.53                               | 10.723                      | 0.24                        | 0.92                 | 0.04                               | 47.1                                 | 10.73                         | 0.25                          | 0.93  |      |      |      |
| 07140158–2511463 | 237.911  | –6.597   | 0.417 | 1      | —   | —      | g    | —    | —        | D2   | c      | o     | —                      | 11.379     | 0.36       | 1.21 | 1        | 33.8       | 0.52  | 3.67                               | 11.224                      | 0.29                        | 1.00                 | 0.13                               | 34.7                                 | 11.23                         | 0.30                          | 1.03  |      |      |      |
| 07141558–1155193 | 226.124  | –0.437   | 2.273 | 9      | —   | —      | g    | —    | —        | —    | c      | o     | —                      | 11.553     | 0.64       | 1.91 | 1        | 28.2       | 0.68  | 3.68                               | 10.706                      | 0.26                        | 0.78                 | 0.70                               | —                                    | —                             | 0.30                          | 0.93  |      |      |      |
| 07141582–3133587 | 243.688  | –9.399   | 0.145 | 1      | —   | —      | g    | —    | —        | D2   | c      | o     | —                      | 11.146     | 0.31       | 1.00 | 1        | 32.4       | 0.82  | 3.61                               | 11.092                      | 0.29                        | 0.93                 | 0.04                               | 32.6                                 | 11.10                         | 0.29                          | 0.94  |      |      |      |
| 07141736–1216244 | 226.439  | –0.594   | 2.689 | 8      | —   | —      | g    | —    | —        | —    | c      | o     | —                      | 10.539     | 1.51       | 3.74 | 1        | 58.0       | 0.52  | 3.81                               | 9.537                       | 1.06                        | 2.40                 | 0.83                               | —                                    | —                             | 1.11                          | 2.58  |      |      |      |
| 07142169+0504531 | 210.998  | 7.407    | 0.144 | 1      | —   | —      | g    | —    | —        | D4   | c      | o     | —                      | 10.093     | 0.30       | 1.02 | 1        | 54.8       | 0.96  | 3.52                               | 10.039                      | 0.28                        | 0.95                 | 0.04                               | 55.1                                 | 10.05                         | 0.28                          | 0.96  |      |      |      |
| 07142493–1207024 | 226.315  | –0.494   | 2.042 | 8      | —   | —      | g    | —    | —        | —    | c      | o     | —                      | 11.898     | 1.32       | 2.78 | 1        | 34.0       | 0.62  | 3.78                               | 11.137                      | 0.98                        | 1.76                 | 0.63                               | —                                    | —                             | 1.02                          | 1.90  |      |      |      |
| 07143332–1152395 | 226.118  | –0.352   | 2.244 | 8      | —   | —      | g    | —    | —        | —    | c      | o     | —                      | 11.147     | 1.72       | 3.41 | 1        | 27.6       | 0.72  | 3.68                               | 10.311                      | 1.34                        | 2.30                 | 0.70                               | —                                    | —                             | 1.39                          | 2.45  |      |      |      |
| 07143364–2538052 | 238.359  | –6.688   | 0.378 | 1      | —   | —      | g    | —    | —        | D1   | c      | o     | —                      | 11.015     | 0.38       | 1.20 | 1        | 38.0       | 0.78  | 3.71                               | 10.874                      | 0.32                        | 1.01                 | 0.12                               | 38.8                                 | 10.89                         | 0.32                          | 1.03  |      |      |      |
| 07143453–2601312 | 238.712  | –6.861   | 0.405 | 1      | —   | —      | g    | —    | —        | D3   | c      | o     | —                      | 10.407     | 0.41       | 1.28 | 1        | 48.2       | 0.70  | 3.70                               | 10.256                      | 0.35                        | 1.07                 | 0.13                               | 49.3                                 | 10.27                         | 0.36                          | 1.10  |      |      |      |
| 07143575+0533011 | 210.602  | 7.670    | 0.126 | 1      | —   | —      | g    | —    | —        | D2   | c      | o     | —                      | 10.970     | 0.34       | 1.08 | 1        | 38.6       | 0.58  | 3.47                               | 10.923                      | 0.32                        | 1.02                 | 0.04                               | 38.8                                 | 10.93                         | 0.32                          | 1.03  |      |      |      |
| 07143657–1857385 | 232.405  | –3.624   | 1.682 | 1      | —   | —      | g    | —    | —        | D3   | c      | o     | —                      | 10.979     | 0.66       | 1.76 | 1        | 29.4       | 0.68  | 3.71                               | 10.352                      | 0.38                        | 0.93                 | 0.52                               | 34.3                                 | 10.37                         | 0.41                          | 1.04  |      |      |      |
| 07143807–1003285 | 224.516  | 0.510    | 0.737 | 1      | —   | —      | g    | —    | —        | D1   | c      | o     | —                      | 11.497     | 0.33       | 1.24 | 1        | 34.8       | 0.50  | 3.68                               | 11.222                      | 0.20                        | 0.88                 | 0.23                               | 37.0                                 | 11.22                         | 0.22                          | 0.93  |      |      |      |
| 07144680–2945103 | 242.093  | –8.495   | 0.175 | 1      | —   | —      | g    | —    | —        | D1   | c      | o     | —                      | 11.280     | 0.33       | 1.11 | 1        | 61.8       | 0.24  | 3.64                               | 11.215                      | 0.30                        | 1.02                 | 0.05                               | 62.4                                 | 11.22                         | 0.31                          | 1.03  |      |      |      |
| 07145413+0635440 | 209.693  | 8.206    | 0.087 | 1      | —   | —      | g    | —    | —        | D1   | c      | o     | —                      | 10.522     | 0.30       | 1.09 | 1        | 58.8       | 0.34  | 3.43                               | 10.490                      | 0.29                        | 1.05                 | 0.03                               | 59.0                                 | 10.49                         | 0.29                          | 1.05  |      |      |      |
| 07145463–2647543 | 239.441  | –7.144   | 0.440 | 1      | —   | —      | g    | —    | —        | D1   | c      | o     | —                      | 10.266     | 0.46       | 1.41 | 1        | 78.6       | 0.20  | 3.66                               | 10.102                      | 0.38                        | 1.19                 | 0.14                               | 80.7                                 | 10.12                         | 0.39                          | 1.22  |      |      |      |
| 07151092–2758194 | 240.524  | –7.619   | 0.244 | 1      | —   | —      | g    | —    | —        | D2   | c      | o     | —                      | 10.301     | 0.32       | 1.10 | 1        | 69.0       | 0.62  | 3.61                               | 10.210                      | 0.28                        | 0.98                 | 0.08                               | 69.8                                 | 10.22                         | 0.28                          | 1.00  |      |      |      |
| 07151559–2916534 | 241.714  | –8.191   | 0.188 | 1      | —   | —      | g    | —    | —        | D1   | c      | o     | —                      | 10.923     | 0.30       | 1.07 | 1        | 75.4       | 0.28  | 3.62                               | 10.853                      | 0.27                        | 0.98                 | 0.06                               | 76.2                                 | 10.86                         | 0.27                          | 0.99  |      |      |      |
| 07153127–2921324 | 241.809  | –8.175   | 0.187 | 1      | —   | —      | g    | —    | —        | D4   | c      | o     | —                      | 8.714      | 0.26       | 0.99 | 1        | 78.0       | 0.86  | 3.62                               | 8.644                       | 0.23                        | 0.90                 | 0.06                               | 78.5                                 | 8.65                          | 0.24                          | 0.91  |      |      |      |
| 07154219–0152439 | 217.382  | 4.534    | 0.144 | 9      | —   | p?     | g    | —    | —        | D1   | c      | o     | —                      | 11.298     | –0.07      | 0.44 | 1        | 29.8       | 0.44  | 3.58                               | 11.244                      | –0.09                       | 0.37                 | 0.04                               | —                                    | —                             | –0.09                         | 0.38  |      |      |      |
| 07154670+0446228 | 211.436  | 7.583    | 0.157 | 1      | —   | —      | g    | —    | —        | D4   | c      | o     | —                      | 10.783     | 0.28       | 1.04 | 1        | 37.0       | 0.96  | 3.46                               | 10.725                      | 0.25                        | 0.96                 | 0.05                               | 37.2                                 | 10.73                         | 0.26                          | 0.97  |      |      |      |
| 07160927–1950273 | 233.356  | –3.707   | 1.089 | 1      | —   | —      | g    | —    | —        | D1   | c      | o     | —                      | 11.004     | 0.48       | 1.44 | 1        | 41.2       | 0.50  | 3.74                               | 10.598                      | 0.30                        | 0.90                 | 0.34                               | 45.4                                 | 10.60                         | 0.32                          | 0.97  |      |      |      |
| 07161385–2703250 | 239.807  | –6.998   | 0.416 | 1      | —   | —      | g    | —    | —        | D4   | c      | o     | —                      | 11.400     | 0.38       | 1.27 | 1        | 26.6       | 0.84  | 3.68                               | 11.245                      | 0.31                        | 1.06                 | 0.13                               | 27.3                                 | 11.26                         | 0.32                          | 1.09  |      |      |      |
| 07161634–2820340 | 240.967  | –7.571   | 0.212 | 1      | —   | —      | g    | —    | —        | D1   | c      | o     | —                      | 10.815     | 0.32       | 1.09 | 1        | 35.6       | 0.68  | 3.62                               | 10.736                      | 0.29                        | 0.99                 | 0.07                               | 36.0                                 | 10.74                         | 0.29                          | 1.00  |      |      |      |
| 07162633–2937150 | 242.136  | –8.114   | 0.202 | 1      | —   | —      | g    | —    | —        | D1   | c      | o     | —                      | 10.568     | 0.33       | 1.12 | 1        | 46.8       | 0.46  | 3.56                               | 10.493                      | 0.30                        | 1.02                 | 0.06                               | 47.2                                 | 10.50                         | 0.30                          | 1.03  |      |      |      |
| 07163123–2919290 | 241.877  | –7.965   | 0.196 | 1      | —   | —      | g    | —    | —        | D1   | c      | o     | —                      | 8.859      | 0.30       | 1.04 | 1        | 95.6       | 0.60  | 3.64                               | 8.786                       | 0.27                        | 0.94                 | 0.06                               | 96.2                                 | 8.80                          | 0.27                          | 0.96  |      |      |      |
| 07163390–0925241 | 224.176  | 1.227    | 4.466 | 9      | —   | —      | g    | —    | —        | —    | c      | o     | —                      | 11.638     | 0.63       | 1.88 | 1        | 34.6       | 0.44  | 3.74                               | 9.974                       | –0.11                       | –0.34                | 1.38                               | —                                    | —                             | –0.02                         | –0.05 |      |      |      |
| 07163843–0925391 | 224.188  | 1.241    | 4.328 | 9      | —   | —      | g    | —    | —        | D1   | c      | o     | —                      | 11.111     | 1.34       | —    | 1        | 51.2       | 0.42  | 3.74                               | 9.498                       | 0.62                        | —                    | 1.34                               | —                                    | —                             | 0.71                          | —     |      |      |      |
| 07164720+0350518 | 212.383  | 7.390    | 0.347 | 1      | —   | —      | g    | —    | —        | D1   | c      | o     | —                      | 10.988     | 0.33       | 1.14 | 1        | 46.6       | 0.80  | 3.48                               | 10.859                      | 0.27                        | 0.97                 | 0.11                               | 47.6                                 | 10.87                         | 0.28                          | 0.99  |      |      |      |
| 07165094–1852251 | 232.573  | –3.114   | 1.778 | 1      | —   | —      | g    | —    | —        | D2   | c      | o     | —                      | 11.200     | 0.60       | 1.88 | 1        | 95.6       | 0.12  | 3.83                               | 10.538                      | 0.30                        | 1.00                 | 0.55                               | 120.7                                | 10.42                         | 0.34                          | 1.12  |      |      |      |
| 07165183+0746253 | 208.845  | 9.167    | 0.079 | 1      | —   | —      | g    | —    | —        | D1   | c      | o     | —                      | 10.941     | 0.31       | 1.02 | 1        | 40.0       | 0.44  | 3.48                               | 10.912                      | 0.30                        | 0.98                 | 0.02                               | 40.1                                 | 10.92                         | 0.30                          | 0.98  |      |      |      |
| 07165193–1852341 | 232.577  | –3.112   | 1.785 | 9      | —   | e      | g    | —    | —        | D1   | c      | o     | —                      | 11.500     | 0.69       | 2.01 | 1        | 60.4       | 0.30  | 3.73                               | 10.835                      | 0.39                        | 1.12                 | 0.55                               | —                                    | —                             | 0.42                          | 1.24  |      |      |      |
| 07171347–2819137 | 241.043  | –7.374   | 0.234 | 1      | —   | —      | g    | —    | —        | D1   | c      | o     | —                      | 11.175     | 0.34       | 1.08 | 1        | 46.6       | 0.64  | 3.70                               | 11.088                      | 0.31                        | 0.96                 | 0.07                               | 47.2                                 | 11.09                         | 0.31                          | 0.98  |      |      |      |
| 07171375–2855007 | 241.580  | –7.643   | 0.226 | 1      | —   | —      | g    | —    | —        | D1   | c      | o     | —                      | 11.148     | 0.33       | 1.10 | 1        | 61.8       | 0.26  | 3.63                               | 11.064                      | 0.29                        | 0.99                 | 0.07                               | 62.7                                 | 11.07                         | 0.30                          | 1.00  |      |      |      |
| 07172784+0320028 | 212.922  | 7.308    | 0.231 | 1      | —   | —      | g    | —    | —        | D1   | c      | o     | —                      | 11.096     | 0.33       | 1.12 | 1        | 44.2       | 0.30  | 3.50                               | 11.010                      | 0.29                        | 1.01                 | 0.07                               | 44.7                                 | 11.02                         | 0.30                          | 1.03  |      |      |      |
| 07174056–2803388 | 240.855  | –7.168   | 0.239 | 1      | —   | —      | g    | —    | —        | D1   | c      | o     | —                      | 10.496     | 0.33       | 1.11 | 1        | 43.0       | 0.78  | 3.69                               | 10.407                      | 0.29                        | 0.99                 | 0.07                               | 43.5                                 | 10.42                         | 0.29                          | 1.01  |      |      |      |
| 07174505+0017504 | 215.674  | 5.988    | 0.196 | 1      | —   | —      | g    | —    | —        | D1   | c      | o     | —                      | 11.279     | 0.36       | 1.20 | 1        | 30.0       | 0.60  | 3.53                               | 11.206                      | 0.33                        | 1.10                 | 0.06                               | 30.3                                 | 11.21                         | 0.33                          | 1.11  |      |      |      |
| 07174645+0757128 | 208.783  | 9.449    | 0.075 | 1      | —   | —      | g    | —    | —        | D1   | c      | o     | —                      | 10.014     | 0.27       | 0.97 | 1        | 66.2       | 0.58  | 3.42                               | 9.986                       | 0.26                        | 0.93                 | 0.02                               | 66.4                                 | 9.99                          | 0.26                          | 0.94  |      |      |      |
| 07182618–2206067 | 235.612  | –4.281   | 1.221 | 7      | —   | —      | g    | —    | —        | —    | c      | o     | —                      | 11.520     | 1.49       | 3.25 | 1        | 14.6       | 1.00  | 3.82                               | 11.065                      | 1.29                        | 2.64                 | 0.38                               | —                                    | —                             | 1.31                          | 2.72  |      |      |      |
| 07184092–2935463 | 242.336  | –7.668   | 0.170 | 1      | —   | —      | g    | —    | —        | D1   | c      | o     | —                      | 10.934     | 0.31       | 1.02 | 1        | 42.2       | 0.40  | 3.67                               | 10.871                      | 0.29                        | 0.94                 | 0.05                               | 42.5                                 | 10.88                         | 0.29                          | 0.95  |      |      |      |
| 07185096–1822067 | 232.347  | –2.459   | 1.821 | 7      | —   | —      | g    | —    | —        | —    | c      | o     | —                      | 10.504     | 0.80       | 2.27 | 1        | 37.0       | 0.84  | 3.80                               | 9.825                       | 0.50                        | 1.36                 | 0.56                               | —                                    | —                             | 0.53                          | 1.48  |      |      |      |
| 07185104–1822174 | 232.349  | –2.460   | 1.825 | 9      | —   | —      | g    | —    | —        | —    | c      | o     | —                      | 9.776      | 1.13       | 2.42 | 1        | 59.0       | 0.56  | 3.77                               | 9.096                       | 0.83                        | 1.51                 | 0.57                               | —                                    | —                             | 0.86                          | 1.63  |      |      |      |
| 07185825–2201195 | 235.599  | –4.134   | 1.526 | 8      | —   | —      | g    | —    | —        | —    | c      | o     | —                      | 11.206     | 0.87       | 1.80 | –2       | 25.2       | 0.84  | 3.79                               | 10.637                      | 0.61                        | 1.04                 | 0.47                               | —                                    | —                             | 0.64                          | 1.14  |      |      |      |
| 07191037–1749270 | 231.901  | –2.137   | 2.878 | 7      | —   | o      | g    | —    | —        | —    | c      | o     | —                      | 10.438     | 1.60       | 3.63 | 1        | 46.0       | 0.48  | 3.77                               | 9.366                       | 1.12                        | 2.20                 | 0.89                               | —                                    | —                             | 1.17                          | 2.39  |      |      |      |
| 07191802+0422375 | 212.192  | 8.188    | 0.252 | 1      | —   | —      | g    | —    | —        | D1   | c      | o     | —                      | 11.331     | 0.30       | 1.07 | 1        | 43.4       | 0.50  | 3.49                               | 11.237                      | 0.26                        | 0.94                 | 0.08                               | 44.0                                 | 11.24                         | 0.26                          | 0.96  |      |      |      |
| 07192746–1752171 | 231.974  | –2.099   | 3.890 | 8      | —   | —      | g    | —    | —        | —    | c      | o     | —                      | 11.366     | 1.27       | 2.73 | 1        | 18.4       | 0.52  | 3.77                               | 9.917                       | 0.62                        | 0.79</               |                                    |                                      |                               |                               |       |      |      |      |

Table B1: a) continued.

| 2MASX J          | <i>l</i>    | <i>b</i>    | EBV        | Object       | Sample         | Disc        | 2MRS       | Velocity    | NIR           | Photom      | Ext | <i>K</i> <sub>20</sub> | <i>H-K</i>  | <i>J-K</i>  | vc          | <i>a</i>    | <i>b/a</i> | st.d.       | <i>K</i> <sub>s</sub> <sup>o</sup> | ( <i>H-K</i> ) <sup>o</sup> | ( <i>J-K</i> ) <sup>o</sup> | <i>A</i> <sub>K</sub> | <i>a</i> <sub>d</sub> <sup>h</sup> | <i>K</i> <sub>s</sub> <sup>o,d</sup> | ( <i>H-K</i> ) <sup>o,c</sup> | ( <i>J-K</i> ) <sup>o,c</sup> |             |       |             |             |             |      |      |
|------------------|-------------|-------------|------------|--------------|----------------|-------------|------------|-------------|---------------|-------------|-----|------------------------|-------------|-------------|-------------|-------------|------------|-------------|------------------------------------|-----------------------------|-----------------------------|-----------------------|------------------------------------|--------------------------------------|-------------------------------|-------------------------------|-------------|-------|-------------|-------------|-------------|------|------|
| (1)              | deg<br>(2a) | deg<br>(2b) | mag<br>(3) | class<br>(4) | off flg<br>(5) | gal<br>(7a) | TF<br>(7b) | obs<br>(7c) | ext'd<br>(7d) | type<br>(8) | (9) | Opt<br>(10a)           | HI<br>(10b) | flg<br>(11) | flg<br>(12) | flg<br>(13) | (14)       | mag<br>(15) | mag<br>(16)                        | (17)                        | (18)                        | (19)                  | (20)                               | mag<br>(21)                          | mag<br>(22)                   | mag<br>(23)                   | mag<br>(24) | (25)  | mag<br>(26) | mag<br>(27) | mag<br>(28) |      |      |
| 07234591+0431102 | 212.571     | 9.245       | 0.112      | 1            | —              | —           | g          | t           | N             | —           | D1  | c                      | o           | —           | —           | —           | —          | —           | 11.205                             | 0.40                        | 1.13                        | 1                     | 28.2                               | 0.48                                 | 3.40                          | 11.163                        | 0.38        | 1.07  | 0.03        | 28.3        | 11.17       | 0.38 | 1.08 |
| 07235168+1053287 | 226.315     | 1.225       | 0.471      | 1            | —              | —           | g          | —           | N             | —           | D2  | —                      | —           | —           | U           | —           | —          | —           | 11.026                             | 0.31                        | 1.15                        | 1                     | 39.4                               | 0.68                                 | 3.72                          | 10.851                        | 0.23        | 0.91  | 0.15        | 40.5        | 10.87       | 0.24 | 0.94 |
| 07235474+2731446 | 241.017     | -5.699      | 0.307      | 1            | —              | —           | g          | —           | —             | —           | D4  | c                      | o           | —           | —           | —           | —          | —           | 7.601                              | 0.30                        | 1.03                        | 1                     | 143.0                              | 0.92                                 | ...                           | 7.487                         | 0.25        | 0.88  | 0.10        | ...         | 0.26        | 0.90 |      |
| 07235484+3553169 | 248.517     | -9.524      | 0.290      | 1            | —              | —           | g          | t           | —             | —           | D1  | c                      | —           | h           | —           | —           | —          | —           | 10.314                             | 0.30                        | 1.12                        | 1                     | 69.2                               | 0.34                                 | 3.57                          | 10.206                        | 0.25        | 0.98  | 0.09        | 70.3        | 10.22       | 0.26 | 1.00 |
| 07235850+2553267 | 239.568     | -4.923      | 3.164      | 7            | —              | —           | —          | —           | —             | —           | —   | —                      | —           | —           | —           | —           | —          | —           | 11.327                             | 0.76                        | 1.52                        | -2                    | 43.8                               | 0.68                                 | 3.84                          | 10.148                        | 0.24        | -0.06 | 0.98        | ...         | 0.30        | 0.15 |      |
| 07240520+2554059 | 239.589     | -4.906      | 3.134      | 9            | —              | —           | —          | —           | —             | —           | —   | —                      | —           | —           | —           | —           | —          | —           | 12.406                             | 0.90                        | 1.88                        | -2                    | 41.0                               | 0.18                                 | 3.77                          | 11.238                        | 0.38        | 0.32  | 0.97        | ...         | 0.44        | 0.53 |      |
| 07240918+3645540 | 249.334     | -9.875      | 0.346      | 1            | —              | —           | g          | —           | —             | —           | D1  | c                      | o           | —           | —           | —           | —          | —           | 11.292                             | 0.31                        | 1.04                        | 1                     | 50.8                               | 0.52                                 | 3.42                          | 11.163                        | 0.25        | 0.87  | 0.11        | 52.0        | 11.17       | 0.26 | 0.89 |
| 07241262+2549239 | 239.533     | -4.845      | 2.705      | 9            | o              | —           | —          | —           | —             | —           | —   | —                      | —           | —           | o           | —           | —          | —           | 11.881                             | 1.70                        | ...                         | 1                     | 32.0                               | 0.56                                 | 3.77                          | 10.873                        | 1.25        | ...   | 0.84        | ...         | 1.31        | ...  |      |
| 07241276+3648420 | 249.382     | -9.885      | 0.339      | 1            | —              | —           | g          | —           | —             | —           | D4  | c                      | o           | —           | —           | —           | —          | —           | 9.900                              | 0.29                        | 1.06                        | 1                     | 54.8                               | 0.86                                 | 3.42                          | 9.774                         | 0.23        | 0.89  | 0.11        | 55.7        | 9.79        | 0.24 | 0.91 |
| 07241306+2553259 | 239.593     | -4.875      | 3.117      | 7            | —              | —           | —          | —           | —             | —           | —   | —                      | —           | —           | c           | —           | —          | —           | 11.843                             | 1.51                        | 2.99                        | 1                     | 17.0                               | 0.62                                 | 3.77                          | 10.682                        | 1.00        | 1.45  | 0.97        | ...         | 1.06        | 1.65 |      |
| 07241313+2550099 | 239.545     | -4.849      | 2.770      | 8            | —              | —           | —          | —           | —             | —           | —   | —                      | —           | —           | —           | —           | —          | —           | 9.603                              | 0.66                        | 1.67                        | 1                     | 62.8                               | 0.46                                 | 3.77                          | 8.571                         | 0.20        | 0.30  | 0.86        | ...         | 0.25        | 0.48 |      |
| 07241487+2923269 | 242.710     | -6.497      | 0.246      | 1            | —              | —           | g          | —           | —             | —           | —   | —                      | —           | —           | —           | —           | —          | —           | 9.984                              | 0.29                        | 1.06                        | 1                     | 52.0                               | 0.72                                 | 3.71                          | 9.892                         | 0.25        | 0.94  | 0.08        | 52.6        | 9.90        | 0.25 | 0.95 |
| 07242543+3152131 | 244.945     | -7.605      | 0.190      | 1            | —              | —           | g          | t           | —             | —           | D1  | c                      | o           | —           | —           | —           | —          | —           | 11.186                             | 0.31                        | 1.14                        | 1                     | 45.4                               | 0.28                                 | 3.71                          | 11.115                        | 0.28        | 1.04  | 0.06        | 45.8        | 11.12       | 0.28 | 1.06 |
| 07244054+2434247 | 238.474     | -4.166      | 1.782      | 8            | —              | —           | —          | —           | —             | —           | —   | —                      | —           | —           | —           | —           | —          | —           | 9.978                              | 0.89                        | 2.02                        | 1                     | 36.4                               | 0.74                                 | 3.84                          | 9.314                         | 0.60        | 1.13  | 0.55        | ...         | 0.63        | 1.25 |      |
| 07244364+2419277 | 238.259     | -4.039      | 1.520      | 7            | —              | —           | —          | —           | —             | —           | —   | —                      | —           | —           | —           | —           | —          | —           | 11.790                             | 1.44                        | 3.47                        | 1                     | 17.4                               | 0.78                                 | 3.74                          | 11.224                        | 1.19        | 2.72  | 0.47        | ...         | 1.22        | 2.82 |      |
| 07245535+2430057 | 238.437     | -4.083      | 1.563      | 1            | —              | —           | g          | —           | N             | —           | D3  | c                      | —           | h           | —           | —           | —          | —           | 11.134                             | 0.43                        | 1.55                        | 1                     | 32.8                               | 0.92                                 | 3.84                          | 10.552                        | 0.17        | 0.77  | 0.48        | 38.4        | 10.54       | 0.20 | 0.87 |
| 07245681+0939336 | 225.354     | 2.941       | 0.341      | 1            | —              | —           | g          | —           | —             | —           | D1  | e                      | o           | —           | —           | —           | —          | —           | 9.123                              | 0.35                        | 1.10                        | 1                     | 96.6                               | 0.76                                 | 3.63                          | 8.996                         | 0.29        | 0.93  | 0.11        | 98.3        | 9.01        | 0.30 | 0.95 |
| 07245743+2715167 | 240.882     | -5.366      | 0.365      | 1            | —              | —           | g          | —           | —             | —           | D1  | c                      | —           | h           | —           | —           | —          | —           | 11.002                             | 0.44                        | 1.02                        | 1                     | 36.6                               | 0.86                                 | 3.81                          | 10.866                        | 0.38        | 0.83  | 0.11        | 37.5        | 10.87       | 0.38 | 0.86 |
| 07250156+3229565 | 245.568     | -7.780      | 0.237      | 1            | —              | —           | g          | t           | —             | —           | D1  | c                      | —           | h           | —           | —           | —          | —           | 10.224                             | 0.28                        | 1.09                        | 1                     | 111.8                              | 0.18                                 | ...                           | 10.136                        | 0.24        | 0.97  | 0.07        | ...         | 0.24        | 0.99 |      |
| 07251259+2658574 | 240.666     | -5.189      | 0.420      | 1            | —              | —           | g          | —           | —             | —           | D1  | c                      | —           | h           | —           | —           | —          | —           | 11.091                             | 0.49                        | 1.21                        | 1                     | 57.2                               | 0.38                                 | 3.76                          | 10.935                        | 0.42        | 1.00  | 0.13        | 59.0        | 10.94       | 0.43 | 1.03 |
| 07251471+2645054 | 240.465     | -5.074      | 0.490      | 1            | —              | —           | g          | t           | N             | —           | D1  | c                      | —           | h           | —           | —           | —          | —           | 11.347                             | 0.47                        | 1.43                        | 1                     | 53.8                               | 0.22                                 | 3.70                          | 11.164                        | 0.39        | 1.18  | 0.15        | 55.6        | 11.17       | 0.40 | 1.22 |
| 07252097+2428114 | 238.455     | -3.982      | 1.413      | 1            | o              | —           | —          | —           | —             | —           | D1  | c                      | —           | h           | —           | —           | —          | —           | 11.273                             | 0.46                        | 1.26                        | 1                     | 92.6                               | 1.00                                 | 3.71                          | 10.747                        | 0.22        | 0.56  | 0.44        | 112.5       | 10.61       | 0.25 | 0.65 |
| 07252625+0914177 | 238.039     | 3.247       | 0.329      | 1            | —              | —           | g          | —           | —             | —           | D2  | e                      | o           | —           | —           | —           | —          | —           | 11.238                             | 0.41                        | 1.18                        | 1                     | 36.4                               | 0.56                                 | 3.67                          | 11.115                        | 0.36        | 1.02  | 0.10        | 37.1        | 11.13       | 0.37 | 1.04 |
| 07254066+3024166 | 243.759     | -6.691      | 0.262      | 1            | —              | —           | g          | —           | —             | —           | D1  | c                      | —           | h           | —           | —           | —          | —           | 9.835                              | 0.25                        | 0.99                        | 1                     | 88.2                               | 0.90                                 | 3.68                          | 9.737                         | 0.21        | 0.86  | 0.08        | 89.5        | 9.74        | 0.21 | 0.87 |
| 07254536+1752531 | 232.689     | -0.782      | 1.383      | 1            | —              | —           | g          | —           | —             | —           | D1  | c                      | —           | h           | —           | —           | —          | —           | 10.493                             | 0.49                        | 1.60                        | 1                     | 48.8                               | 0.82                                 | 3.68                          | 9.978                         | 0.27        | 0.92  | 0.43        | 56.0        | 9.96        | 0.29 | 1.01 |
| 07254650+3426426 | 247.389     | -8.532      | 0.267      | 1            | —              | —           | g          | —           | —             | —           | D3  | c                      | o           | —           | —           | —           | —          | —           | 11.098                             | 0.26                        | 1.06                        | 1                     | 32.0                               | 0.76                                 | 3.49                          | 10.999                        | 0.21        | 0.93  | 0.08        | 32.4        | 11.01       | 0.22 | 0.94 |
| 07260165+2637519 | 240.440     | -4.863      | 0.579      | 1            | —              | —           | g          | —           | —             | —           | D1  | c                      | —           | h           | —           | —           | —          | —           | 11.271                             | 0.38                        | 1.20                        | 1                     | 38.8                               | 0.62                                 | 3.75                          | 11.055                        | 0.29        | 0.92  | 0.18        | 40.5        | 11.06       | 0.30 | 0.95 |
| 07260863+0159013 | 215.131     | 8.625       | 0.142      | 1            | —              | —           | g          | —           | —             | —           | D2  | c                      | —           | h           | —           | —           | —          | —           | 10.154                             | 0.31                        | 1.01                        | 1                     | 48.4                               | 0.78                                 | 3.40                          | 10.101                        | 0.28        | 0.94  | 0.04        | 48.7        | 10.11       | 0.29 | 0.94 |
| 07261948+3519474 | 248.237     | -8.835      | 0.411      | 1            | —              | —           | g          | —           | —             | —           | D1  | c                      | —           | h           | —           | —           | —          | —           | 10.882                             | 0.27                        | 1.04                        | 1                     | 41.8                               | 0.78                                 | 3.56                          | 10.729                        | 0.20        | 0.84  | 0.13        | 43.0        | 10.74       | 0.21 | 0.86 |
| 07262635+3554214 | 248.767     | -9.076      | 0.393      | 1            | —              | —           | g          | —           | —             | —           | D2  | c                      | —           | h           | —           | —           | —          | —           | 9.999                              | 0.38                        | 1.21                        | 1                     | 54.4                               | 0.76                                 | 3.54                          | 9.853                         | 0.32        | 1.01  | 0.12        | 55.5        | 9.87        | 0.33 | 1.04 |
| 07263535+1531546 | 230.717     | 0.510       | 1.936      | 7            | —              | —           | —          | —           | —             | —           | —   | —                      | —           | —           | —           | —           | —          | —           | 8.831                              | 1.27                        | 2.64                        | 1                     | 57.6                               | 0.72                                 | 3.74                          | 8.110                         | 0.95        | 1.68  | 0.60        | ...         | 0.98        | 1.81 |      |
| 07264061+1524416 | 230.621     | 0.586       | 1.581      | 8            | —              | —           | —          | —           | —             | —           | —   | —                      | —           | —           | —           | —           | —          | —           | 10.550                             | 0.95                        | 2.08                        | 1                     | 54.0                               | 0.40                                 | 3.74                          | 9.961                         | 0.69        | 1.29  | 0.49        | ...         | 0.72        | 1.40 |      |
| 07264631+2351096 | 238.063     | -3.405      | 1.188      | 1            | —              | —           | g          | —           | N             | —           | D2  | c                      | —           | h           | —           | —           | —          | —           | 10.645                             | 0.50                        | 1.55                        | 1                     | 44.6                               | 0.72                                 | 3.75                          | 10.202                        | 0.30        | 0.96  | 0.37        | 49.5        | 10.21       | 0.32 | 1.04 |
| 07265062+0138508 | 215.514     | 8.627       | 0.165      | 1            | —              | —           | g          | —           | —             | —           | D1  | c                      | —           | h           | —           | —           | —          | —           | 10.359                             | 0.37                        | 1.10                        | 1                     | 55.0                               | 0.56                                 | 3.46                          | 10.298                        | 0.34        | 1.02  | 0.05        | 55.4        | 10.31       | 0.34 | 1.03 |
| 07265314+3519437 | 248.289     | -8.733      | 0.378      | 1            | —              | —           | g          | —           | —             | —           | D3  | c                      | —           | h           | —           | —           | —          | —           | 11.235                             | 0.34                        | 1.17                        | 1                     | 30.4                               | 0.84                                 | 3.54                          | 11.094                        | 0.28        | 0.98  | 0.12        | 31.1        | 11.10       | 0.28 | 1.01 |
| 07265364+0732511 | 223.715     | 4.362       | 0.246      | 1            | —              | —           | g          | —           | —             | —           | D1  | e                      | —           | h           | —           | —           | —          | —           | 10.083                             | 0.28                        | 1.01                        | 1                     | 64.8                               | 0.88                                 | 3.60                          | 9.991                         | 0.24        | 0.89  | 0.08        | 65.8        | 10.00       | 0.24 | 0.91 |
| 07272918+2357333 | 238.235     | -3.312      | 1.112      | 1            | —              | —           | g          | t           | —             | —           | D1  | e                      | —           | h           | —           | —           | —          | —           | 10.532                             | 0.51                        | 1.56                        | 1                     | 67.6                               | 0.30                                 | 3.88                          | 10.118                        | 0.33        | 1.01  | 0.34        | 74.7        | 10.12       | 0.35 | 1.08 |
| 07273064+1308046 | 228.715     | 1.847       | 0.510      | 1            | —              | —           | g          | —           | N             | —           | D3  | c                      | —           | h           | —           | —           | —          | —           | 11.196                             | 0.37                        | 1.25                        | 1                     | 35.0                               | 0.64                                 | 3.70                          | 11.006                        | 0.28        | 1.00  | 0.16        | 36.2        | 11.02       | 0.29 | 1.03 |
| 07273273+2319396 | 237.684     | -3.000      | 1.569      | 1            | —              | —           | g          | —           | N             | —           | D4  | —                      | —           | —           | —           | —           | —          | —           | 11.093                             | 0.56                        | 1.72                        | 1                     | 23.6                               | 0.86                                 | 3.70                          | 10.508                        | 0.30        | 0.94  | 0.49        | 27.2        | 10.52       | 0.33 | 1.05 |
| 07273400+1308106 | 228.722     | 1.858       | 0.509      | 1            | —              | —           | g          | —           | N             | —           | D2  | —                      | —           | —           | —           | —           | —          | —           | 10.683                             | 0.48                        | 1.30                        | 1                     | 51.0                               | 0.76                                 | 3.70                          | 10.493                        | 0.40        | 1.05  | 0.16        | 52.7        | 10.51       | 0.41 | 1.08 |
| 07274286+2018487 | 235.049     | -1.532      | 1.798      | 7            | —              | —           | —          | —           | —             | —           | —   | —                      | —           | —           | —           | —           | —          | —           | 11.197                             | 0.88                        | 2.33                        | 1                     | 38.2                               | 0.88                                 | 3.78                          | 10.527                        | 0.59        | 1.43  | 0.56        | ...         | 0.62        | 1.55 |      |
| 07275638+2040077 | 235.387     | -1.655      | 1.549      | 8            | —              | —           | —          | —           | —             | —           | —   | —                      | —           | —           | —           | —           | —          | —           | 11.614                             | 0.80                        | 1.47                        | 1                     |                                    |                                      |                               |                               |             |       |             |             |             |      |      |

Table B1: a) continued.

[illegible]

| 2MASX J          |         | <i>l</i>    | <i>b</i>    | EBV        | Object       |            |             | Sample      |            |             | Disc          | 2MRS | Velocity |              | NIR         | Photom      | Ext         | <i>K</i> <sub>20</sub> | <i>H-K</i>  | <i>J-K</i>  | vc          | <i>a</i> | <i>b/a</i> | st.d. | <i>K</i> <sub>0</sub> <sup>o</sup> | <i>(H-K)</i> <sup>o</sup> | <i>(J-K)</i> <sup>o</sup> | <i>A<sub>K</sub></i> | <i>a</i> <sup>d</sup> | <i>K</i> <sub>0</sub> <sup>o,d</sup> | <i>(H-K)</i> <sup>o,c</sup> | <i>(J-K)</i> <sup>o,c</sup> |             |
|------------------|---------|-------------|-------------|------------|--------------|------------|-------------|-------------|------------|-------------|---------------|------|----------|--------------|-------------|-------------|-------------|------------------------|-------------|-------------|-------------|----------|------------|-------|------------------------------------|---------------------------|---------------------------|----------------------|-----------------------|--------------------------------------|-----------------------------|-----------------------------|-------------|
| (1)              |         | deg<br>(2a) | deg<br>(2b) | mag<br>(3) | class<br>(4) | off<br>(5) | flag<br>(6) | gal<br>(7a) | TF<br>(7b) | obs<br>(7c) | ext'd<br>(7d) | (8)  | (9)      | Opt<br>(10a) | HI<br>(10b) | flg<br>(11) | flg<br>(12) | flg<br>(13)            | mag<br>(14) | mag<br>(15) | mag<br>(16) | (17)     | (18)       | (19)  | (20)                               | mag<br>(21)               | mag<br>(22)               | mag<br>(23)          | mag<br>(24)           | (25)                                 | mag<br>(26)                 | mag<br>(27)                 | mag<br>(28) |
| 07415021-0241130 | 221.167 | 9.936       | 0.097       | 1          | -            | -          | -           | g           | t          | -           | -             | D1   | c        | o            | h           | V           | -           | -                      | 10.911      | 0.49        | 1.14        | 1        | 73.6       | 0.30  | 3.34                               | 10.875                    | 0.47                      | 1.09                 | 0.03                  | 73.9                                 | 10.88                       | 0.47                        | 1.10        |
| 07415613-1812215 | 234.837 | 2.425       | 0.613       | 8          | -            | -          | -           | g           | -          | -           | -             | D1   | -        | -            | -           | -           | o           | -                      | 9.527       | 0.75        | 0.78        | 1        | 73.0       | 0.34  | 3.71                               | 9.299                     | 0.65                      | 0.47                 | 0.19                  | ...                                  | ...                         | 0.66                        | 0.51        |
| 07421777-2422528 | 240.243 | -0.563      | 0.606       | 1          | -            | -          | -           | g           | -          | -           | -             | D1   | -        | -            | -           | -           | -           | -                      | 10.957      | 0.47        | 1.25        | 1        | 43.8       | 0.66  | 3.77                               | 10.731                    | 0.37                      | 0.95                 | 0.19                  | 45.9                                 | 10.73                       | 0.38                        | 0.99        |
| 07422118-2742508 | 243.145 | -2.204      | 0.769       | 1          | -            | -          | -           | g           | -          | N           | -             | D2   | e        | o            | h           | -           | o           | -                      | 11.258      | 0.34        | 1.20        | 1        | 28.2       | 0.86  | 3.86                               | 10.971                    | 0.21                      | 0.82                 | 0.24                  | 30.0                                 | 10.98                       | 0.23                        | 0.87        |
| 07423793-3438274 | 249.216 | -5.566      | 1.359       | 1          | -            | -          | -           | g           | -          | -           | -             | D1   | e        | -            | -           | -           | -           | -                      | 10.498      | 0.50        | 1.56        | 1        | 55.8       | 0.86  | 3.75                               | 9.992                     | 0.27                      | 0.88                 | 0.42                  | 79.6                                 | 9.96                        | 0.30                        | 0.97        |
| 07425207-1530591 | 246.932 | -4.225      | 0.829       | 1          | -            | -          | -           | g           | -          | -           | -             | D1   | e        | -            | -           | -           | -           | -                      | 9.970       | 0.36        | 1.23        | 1        | 65.6       | 0.48  | 3.75                               | 9.661                     | 0.22                      | 0.82                 | 0.26                  | 58.9                                 | 9.68                        | 0.24                        | 0.87        |
| 07425342-1951306 | 236.429 | 1.778       | 0.712       | 1          | -            | -          | -           | g           | t          | -           | -             | D3   | -        | -            | -           | -           | -           | -                      | 10.391      | 0.42        | 1.28        | 1        | 30.8       | 0.88  | 3.76                               | 10.928                    | 0.30                      | 0.93                 | 0.22                  | 32.5                                 | 10.94                       | 0.32                        | 0.98        |
| 07431309-2958362 | 245.207 | -3.160      | 0.596       | 1          | -            | -          | -           | g           | -          | N           | -             | D1   | e        | o            | -           | -           | -           | -                      | 11.193      | 0.42        | 1.28        | 1        | 49.4       | 0.62  | 3.81                               | 10.169                    | 0.23                      | 0.85                 | 0.18                  | 51.3                                 | 10.19                       | 0.24                        | 0.89        |
| 07431472-2545501 | 241.550 | -1.063      | 0.718       | 1          | -            | -          | -           | g           | -          | -           | -             | D1   | -        | o            | -           | h           | -           | -                      | 10.887      | 0.62        | 1.49        | 1        | 43.0       | 0.84  | 3.81                               | 10.619                    | 0.50                      | 1.13                 | 0.22                  | 45.1                                 | 10.64                       | 0.51                        | 1.18        |
| 07431751-3333172 | 248.333 | -4.914      | 1.444       | 1          | -            | -          | -           | g           | -          | N           | -             | D3   | -        | -            | -           | -           | -           | -                      | 10.607      | 0.53        | 1.69        | 1        | 41.8       | 0.78  | 3.74                               | 10.069                    | 0.29                      | 0.98                 | 0.45                  | 47.2                                 | 10.09                       | 0.32                        | 1.05        |
| 07431853-2006196 | 236.648 | 1.765       | 0.787       | 1          | -            | -          | -           | g           | -          | N           | -             | D3   | -        | -            | -           | -           | -           | -                      | 11.439      | 0.46        | 1.39        | 1        | 36.6       | 0.72  | 3.78                               | 11.146                    | 0.33                      | 1.00                 | 0.24                  | 39.1                                 | 11.15                       | 0.34                        | 1.05        |
| 07432302-2912591 | 244.563 | 0.636       | 1           | -          | -            | -          | -           | g           | t          | N           | -             | D2   | -        | o            | *           | -           | -           | -                      | 9.731       | 0.40        | 1.20        | 1        | 87.8       | 0.44  | 3.81                               | 9.493                     | 0.29                      | 0.98                 | 0.15                  | 9.51                                 | 10.30                       | 0.93                        | 0.93        |
| 07434049-3802129 | 252.301 | -7.041      | 0.666       | 1          | -            | -          | -           | g           | -          | -           | -             | D2   | c        | o            | -           | -           | -           | -                      | 10.761      | 0.31        | 1.27        | 1        | 38.4       | 0.60  | 3.67                               | 10.628                    | 0.21                      | 0.94                 | 0.21                  | 44.1                                 | 10.63                       | 0.22                        | 0.99        |
| 07435826-3834009 | 252.796 | -7.248      | 0.668       | 1          | -            | -          | -           | g           | t          | -           | -             | D1   | c        | o            | -           | -           | -           | -                      | 9.937       | 0.35        | 1.20        | 1        | 74.2       | 0.42  | 3.69                               | 9.688                     | 0.24                      | 0.86                 | 0.21                  | 77.7                                 | 9.70                        | 0.25                        | 0.91        |
| 07440227-2721456 | 243.025 | -1.705      | 0.746       | 1          | -            | -          | -           | g           | -          | N           | -             | D1   | -        | o            | *           | -           | -           | -                      | 11.248      | 0.47        | 1.33        | 1        | 41.6       | 0.74  | 3.81                               | 10.970                    | 0.34                      | 0.96                 | 0.23                  | 44.6                                 | 10.96                       | 0.36                        | 1.01        |
| 07441185-3548317 | 250.397 | -5.860      | 0.947       | 1          | -            | -          | -           | g           | -          | -           | -             | D1   | -        | -            | -           | -           | -           | -                      | 11.230      | 0.53        | 1.72        | 1        | 59.6       | 0.24  | 3.67                               | 10.877                    | 0.38                      | 1.25                 | 0.29                  | 64.9                                 | 10.87                       | 0.40                        | 1.31        |
| 07442148-2602486 | 241.920 | -0.987      | 1.004       | 1          | -            | -          | -           | g           | t          | -           | -             | D1   | c        | -            | -           | -           | -           | -                      | 10.903      | 0.42        | 1.41        | 1        | 60.0       | 0.54  | 3.82                               | 10.529                    | 0.25                      | 0.91                 | 0.31                  | 66.4                                 | 10.50                       | 0.27                        | 0.97        |
| 07442386-2600016 | 241.884 | -0.956      | 0.995       | 1          | -            | -          | -           | g           | -          | -           | -             | D2   | -        | -            | -           | -           | -           | -                      | 10.966      | 0.54        | 1.60        | 1        | 30.6       | 0.56  | 3.82                               | 10.595                    | 0.37                      | 1.10                 | 0.31                  | 33.0                                 | 10.61                       | 0.39                        | 1.17        |
| 07442784-1820196 | 235.250 | 2.880       | 0.573       | 1          | -            | -          | -           | g           | -          | N           | -             | D2   | -        | -            | -           | -           | -           | -                      | 11.445      | 0.39        | 1.29        | 1        | 30.6       | 0.54  | 3.74                               | 11.231                    | 0.29                      | 1.00                 | 0.18                  | 31.8                                 | 11.24                       | 0.30                        | 1.04        |
| 07442813-2008316 | 236.816 | 1.983       | 0.839       | 7          | -            | -          | -           | g           | -          | -           | -             | -    | -        | -            | -           | -           | -           | -                      | 9.172       | 2.02        | 4.23        | 1        | 46.0       | 0.68  | 3.73                               | 8.859                     | 1.88                      | 3.81                 | 0.26                  | ...                                  | ...                         | 1.89                        | 3.87        |
| 07443885-2007426 | 236.825 | 2.026       | 0.832       | 7          | -            | -          | -           | g           | -          | -           | -             | -    | -        | -            | -           | -           | -           | -                      | 10.576      | 2.08        | 4.42        | 1        | 30.0       | 0.78  | 3.73                               | 10.266                    | 1.95                      | 4.01                 | 0.26                  | ...                                  | ...                         | 1.96                        | 4.06        |
| 07444712-2408268 | 240.317 | 0.049       | 7.022       | 9          | -            | -          | -           | g           | -          | -           | -             | -    | -        | -            | -           | -           | -           | -                      | 13.030      | 0.92        | 1.83        | -2       | 18.6       | 0.44  | 3.86                               | 10.414                    | -0.24                     | -1.66                | 2.18                  | ...                                  | ...                         | -0.11                       | -1.20       |
| 07445216-2407358 | 240.315 | 0.073       | 7.301       | 8          | -            | -          | -           | g           | -          | -           | -             | -    | -        | -            | -           | -           | -           | -                      | 8.835       | 1.24        | 2.51        | 1        | 90.0       | 0.72  | 3.86                               | 6.115                     | 0.03                      | -1.12                | 2.26                  | ...                                  | ...                         | 0.18                        | -0.63       |
| 07445637-2530598 | 241.526 | -0.609      | 4.787       | 7          | -            | -          | -           | g           | -          | -           | -             | -    | -        | -            | -           | -           | -           | -                      | 12.319      | 0.48        | 1.48        | -2       | 18.0       | 0.22  | 3.86                               | 10.535                    | -0.31                     | -0.90                | 1.46                  | ...                                  | ...                         | -0.22                       | -0.58       |
| 07445755-2531018 | 241.529 | -0.605      | 4.831       | 9          | -            | -          | -           | g           | -          | -           | -             | -    | -        | -            | -           | -           | -           | -                      | 12.335      | 1.30        | 2.24        | 1        | 38.4       | 0.50  | 3.86                               | 10.535                    | 0.50                      | -0.16                | 1.50                  | ...                                  | ...                         | 0.60                        | 0.15        |
| 07450046-4108069 | 255.160 | -8.320      | 0.308       | 1          | -            | -          | -           | g           | -          | -           | -             | D3   | c        | o            | -           | -           | -           | -                      | 11.310      | 0.41        | 1.18        | 1        | 31.0       | 0.96  | 3.60                               | 11.195                    | 0.36                      | 1.02                 | 0.10                  | 31.5                                 | 11.20                       | 0.36                        | 1.05        |
| 07450390-2531299 | 241.548 | -0.588      | 5.326       | 9          | -            | -          | -           | g           | -          | -           | -             | -    | -        | -            | -           | -           | -           | -                      | 11.374      | 0.92        | 1.58        | 1        | 59.8       | 0.44  | 3.86                               | 9.390                     | 0.04                      | -1.07                | 1.65                  | ...                                  | ...                         | 0.14                        | -0.72       |
| 07450649-2531529 | 241.558 | -0.583      | 5.263       | 9          | -            | -          | -           | g           | -          | -           | -             | -    | -        | -            | -           | -           | -           | -                      | 11.225      | 0.82        | 1.49        | 1        | 64.8       | 0.24  | 3.86                               | 9.264                     | -0.05                     | -1.13                | 1.63                  | ...                                  | ...                         | 0.05                        | -0.78       |
| 07451544-3845199 | 253.057 | -7.104      | 0.630       | 1          | -            | -          | -           | g           | -          | -           | -             | D2   | c        | o            | -           | -           | -           | -                      | 10.196      | 0.34        | 1.18        | 1        | 41.2       | 0.94  | 3.66                               | 9.961                     | 0.23                      | 0.86                 | 0.20                  | 42.9                                 | 9.98                        | 0.24                        | 0.90        |
| 07451604-1719400 | 234.467 | 3.549       | 0.294       | 1          | -            | -          | -           | g           | -          | -           | -             | D1   | e        | o            | h           | -           | -           | -                      | 11.085      | 0.44        | 1.23        | 1        | 24.4       | 0.82  | 3.64                               | 10.975                    | 0.39                      | 1.08                 | 0.09                  | 24.8                                 | 10.98                       | 0.40                        | 1.10        |
| 07451725-3413310 | 249.124 | -4.885      | 1.490       | 1          | -            | -          | -           | g           | t          | N           | -             | D2   | -        | -            | -           | -           | -           | -                      | 11.760      | 0.60        | 1.65        | 1        | 30.4       | 0.62  | 3.84                               | 11.205                    | 0.35                      | 0.91                 | 0.46                  | 35.6                                 | 11.17                       | 0.38                        | 1.01        |
| 07451863-3231000 | 247.638 | -4.033      | 1.518       | 1          | -            | -          | -           | g           | t          | N           | -             | D1   | e        | o            | -           | -           | -           | -                      | 8.709       | 0.46        | 1.56        | 1        | 106.6      | 0.48  | 3.75                               | 8.143                     | 0.20                      | 0.81                 | 0.47                  | 119.9                                | 8.18                        | 0.23                        | 0.91        |
| 07452996-2715311 | 243.097 | -1.372      | 0.841       | 1          | -            | -          | -           | g           | t          | N           | -             | D1   | -        | -            | -           | -           | -           | -                      | 11.275      | 0.49        | 1.36        | 1        | 62.6       | 0.22  | 3.83                               | 10.962                    | 0.35                      | 0.95                 | 0.26                  | 67.6                                 | 10.95                       | 0.37                        | 1.00        |
| 07453012-2049594 | 237.536 | 1.847       | 2.727       | 9          | -            | -          | -           | g           | -          | -           | -             | -    | -        | -            | -           | -           | -           | -                      | 10.289      | ...         | ...         | 1        | 81.8       | 1.00  | 3.74                               | 9.273                     | ...                       | ...                  | 0.84                  | ...                                  | ...                         | ...                         | ...         |
| 07461220-4108531 | 255.282 | -8.130      | 0.332       | 1          | -            | -          | -           | g           | t          | -           | -             | D1   | c        | o            | -           | -           | -           | -                      | 10.435      | 0.34        | 1.14        | 1        | 61.6       | 0.32  | 3.61                               | 10.311                    | 0.28                      | 0.97                 | 0.10                  | 62.7                                 | 10.32                       | 0.29                        | 0.99        |
| 07462535-1832493 | 235.663 | 3.179       | 0.465       | 1          | -            | -          | -           | g           | t          | -           | -             | D1   | e        | o            | h           | -           | -           | -                      | 10.272      | 0.43        | 1.27        | 1        | 75.2       | 0.34  | 3.72                               | 10.099                    | 0.35                      | 1.04                 | 0.14                  | 77.6                                 | 10.11                       | 0.36                        | 1.07        |
| 07462675-3736461 | 252.199 | -6.356      | 0.626       | 1          | -            | -          | -           | g           | -          | -           | -             | D1   | c        | o            | h           | -           | -           | -                      | 10.109      | 0.39        | 1.27        | 1        | 58.0       | 0.96  | 3.68                               | 9.876                     | 0.29                      | 0.96                 | 0.19                  | 60.6                                 | 9.89                        | 0.30                        | 1.01        |
| 07465428-3818121 | 252.848 | -6.618      | 0.675       | 1          | -            | -          | -           | g           | -          | N           | -             | D1   | c        | o            | h           | -           | o           | -                      | 10.216      | 0.47        | 1.25        | 1        | 69.4       | 0.68  | 3.67                               | 9.964                     | 0.36                      | 0.91                 | 0.21                  | 74.2                                 | 9.94                        | 0.37                        | 0.96        |
| 07465855-2915253 | 244.990 | -2.093      | 0.942       | 3          | -            | -          | -           | g           | -          | N           | -             | n    | -        | -            | -           | -           | -           | -                      | 11.251      | 0.62        | 1.53        | 1        | 35.0       | 0.64  | 3.78                               | 10.900                    | 0.46                      | 1.07                 | 0.29                  | 37.8                                 | 10.91                       | 0.48                        | 1.13        |
| 07471332-2617423 | 242.457 | -0.556      | 0.636       | 1          | -            | -          | -           | g           | -          | -           | -             | D2   | -        | -            | -           | -           | -           | -                      | 10.993      | ...         | ...         | 1        | 61.2       | 1.00  | 3.79                               | 10.756                    | ...                       | ...                  | 0.20                  | 64.7                                 | 10.75                       | ...                         | ...         |
| 07471479-3049352 | 246.378 | -2.831      | 0.820       | 1          | -            | -          | -           | g           | -          | N           | -             | D2   | -        | -            | -           | -           | -           | -                      | 10.587      | 0.39        | 1.23        | 1        | 44.0       | 0.58  | 3.84                               | 10.281                    | 0.26                      | 0.82                 | 0.25                  | 46.9                                 | 10.29                       | 0.27                        | 0.88        |
| 07472637-2720023 | 243.379 | -1.037      | 1.088       | 8          | -            | -          | -           | g           | -          | o           | p             | -    | -        | -            | -           | -           | o           | -                      | 11.622      | 0.66        | 0.86        | 1        | 33.6       | 0.72  | 3.83                               | 11.217                    | 0.48                      | 0.31                 | 0.34                  | ...                                  | ...                         | 0.50                        | 0.39        |
| 07473405-4127077 | 255.676 | -8.055      | 0.368       | 1          | -            | -          | -           | g           | t          | -           | -             | D1   | c        | o            | h           | -           | -           | -                      | 7.941       | 0.26        | 1.05        | 1        | 191.4      | 0.24  | ...                                | 7.804                     | 0.20                      | 0.87                 | 0.11                  | ...                                  | ...                         | 0.21                        | 0.89        |
| 07473672-2101573 | 237.956 | 2.173       | 0.534       | 1          | -            | -          | -           | g           | -          | N           | -             | D3   | -        | -            | -           | -           | -           | -                      | 11.406      | 0.36        | 1.17        | 1        | 29.2       | 0.76  | 3.75                               | 11.207                    | 0.27                      |                      |                       |                                      |                             |                             |             |

Table B1: a) continued.

| 2MASX J          | <i>l</i> | <i>b</i> | EBV   | Object | Sample | Disc | 2MRS | Velocity | NIR   | Photom | Ext | <i>K</i> <sub>20</sub> | <i>H-K</i> | <i>J-K</i> | vc   | <i>a</i> | <i>b/a</i> | st.d. | <i>K</i> <sub>s</sub> <sup>o</sup> | ( <i>H-K</i> ) <sup>o</sup> | ( <i>J-K</i> ) <sup>o</sup> | <i>A<sub>K</sub></i> | <i>a</i> <sub>d</sub> <sup>o</sup> | <i>K</i> <sub>s</sub> <sup>o,d</sup> | ( <i>H-K</i> ) <sup>o,c</sup> | ( <i>J-K</i> ) <sup>o,c</sup> |       |       |      |       |       |       |       |
|------------------|----------|----------|-------|--------|--------|------|------|----------|-------|--------|-----|------------------------|------------|------------|------|----------|------------|-------|------------------------------------|-----------------------------|-----------------------------|----------------------|------------------------------------|--------------------------------------|-------------------------------|-------------------------------|-------|-------|------|-------|-------|-------|-------|
| (1)              | deg      | deg      | mag   | class  | off    | gal  | TF   | Obs      | ext'd | type   |     | (14)                   | mag        | mag        | (17) | "        | (19)       | (20)  | mag                                | mag                         | mag                         | mag                  | "                                  | mag                                  | mag                           | mag                           |       |       |      |       |       |       |       |
| (1)              | (2a)     | (2b)     | (3)   | (4)    | (5)    | (6)  | (7a) | (7b)     | (7c)  | (7d)   | (8) | (9)                    | (10a)      | (10b)      | (11) | (12)     | (13)       | (14)  | (15)                               | (16)                        | (17)                        | (18)                 | (19)                               | (20)                                 | (21)                          | (22)                          | (23)  | (24)  | (25) | (26)  | (27)  | (28)  |       |
| 07501898–2630208 | 242.990  | −0.065   | 0.423 | 1      | –      | –    | g    | t        | –     | –      | D1  | e                      | –          | h          | –    | –        | –          | –     | 10.252                             | 0.42                        | 1.37                        | 1                    | 54.8                               | 0.38                                 | 3.82                          | 10.094                        | 0.35  | 1.16  | 0.13 | 56.1  | 10.11 | 0.35  | 1.19  |
| 07502465–3106347 | 246.965  | −2.389   | 1.038 | 1      | –      | –    | g    | t        | N     | –      | D1  | –                      | –          | *          | –    | –        | –          | –     | 11.550                             | 0.73                        | 1.51                        | 1                    | 40.8                               | 0.32                                 | 3.82                          | 11.163                        | 0.56  | 1.00  | 0.32 | 45.0  | 11.15 | 0.58  | 1.07  |
| 07504533–2949184 | 245.894  | −1.670   | 0.958 | 1      | –      | –    | g    | t        | N     | –      | D2  | e                      | o          | –          | –    | –        | –          | –     | 10.034                             | 0.41                        | 1.35                        | 1                    | 58.0                               | 0.44                                 | 3.88                          | 9.677                         | 0.25  | 0.87  | 0.30 | 62.0  | 9.71  | 0.27  | 0.93  |
| 07505059–3053204 | 246.822  | −2.197   | 1.080 | 1      | o      | –    | g    | t        | N     | –      | D2  | –                      | –          | –          | –    | o        | –          | –     | 10.845                             | 0.38                        | 1.24                        | 1                    | 42.4                               | 0.50                                 | 3.80                          | 10.443                        | 0.20  | 0.71  | 0.33 | 46.3  | 10.46 | 0.22  | 0.78  |
| 07510101–3821434 | 253.304  | −5.948   | 0.636 | 1      | –      | –    | g    | t        | –     | –      | D2  | c                      | o          | –          | –    | –        | –          | –     | 11.396                             | 0.44                        | 1.27                        | 1                    | 34.2                               | 0.60                                 | 3.85                          | 11.159                        | 0.34  | 0.95  | 0.20 | 35.8  | 11.17 | 0.35  | 0.99  |
| 07512791–2938273 | 245.816  | −1.445   | 0.744 | 1      | –      | –    | g    | t        | N     | –      | D1  | e                      | o          | h          | –    | –        | –          | –     | 10.656                             | 0.52                        | 1.55                        | 1                    | 67.2                               | 0.20                                 | 3.82                          | 10.379                        | 0.40  | 1.18  | 0.23 | 71.2  | 10.39 | 0.41  | 1.23  |
| 07513733–3845050 | 253.702  | −6.041   | 0.776 | 1      | –      | –    | g    | t        | –     | –      | D1  | c                      | o          | –          | –    | –        | –          | –     | 10.748                             | 0.48                        | 1.39                        | 1                    | 79.8                               | 0.18                                 | 4.07                          | 10.459                        | 0.35  | 1.00  | 0.24 | 85.5  | 10.45 | 0.37  | 1.06  |
| 07515109–2523545 | 242.214  | 0.797    | 0.421 | 1      | –      | –    | g    | t        | N     | –      | D1  | –                      | –          | –          | –    | –        | –          | –     | 11.185                             | 0.36                        | 1.16                        | 1                    | 30.8                               | 0.52                                 | 3.83                          | 11.028                        | 0.29  | 0.95  | 0.13 | 31.6  | 11.04 | 0.30  | 0.98  |
| 07515161–3314133 | 248.955  | −3.207   | 2.414 | 8      | –      | –    | g    | t        | –     | –      | –   | –                      | –          | –          | –    | –        | –          | –     | 11.803                             | 0.83                        | 2.61                        | 1                    | 12.4                               | 0.98                                 | 3.78                          | 10.904                        | 0.43  | 1.41  | 0.75 | ...   | ...   | 0.48  | 1.57  |
| 07515273–3314454 | 248.965  | −3.208   | 2.395 | 8      | –      | –    | g    | t        | –     | –      | –   | –                      | –          | –          | –    | –        | –          | –     | 11.976                             | 2.11                        | ...                         | 1                    | 20.8                               | 0.40                                 | 3.78                          | 11.084                        | 1.72  | ...   | 0.74 | ...   | ...   | 1.76  | ...   |
| 07521098–2100174 | 238.473  | 3.107    | 0.335 | 1      | –      | –    | g    | t        | N     | –      | D2  | –                      | –          | –          | –    | –        | –          | –     | 11.035                             | 0.35                        | 1.19                        | 1                    | 35.6                               | 0.86                                 | 3.69                          | 10.910                        | 0.29  | 1.02  | 0.10 | 36.3  | 10.92 | 0.30  | 1.04  |
| 07521744–2627205 | 243.172  | 0.341    | 8.313 | 8      | –      | –    | g    | t        | –     | –      | –   | –                      | –          | –          | –    | –        | –          | –     | 9.593                              | 0.84                        | 1.20                        | 1                    | 178.4                              | 0.38                                 | 3.98                          | 6.496                         | −0.54 | −2.93 | 2.57 | ...   | ...   | −0.38 | −2.38 |
| 07522033–3721154 | 252.561  | −5.214   | 0.964 | 1      | –      | –    | g    | t        | –     | –      | D1  | c                      | o          | –          | –    | –        | –          | –     | 10.742                             | 0.43                        | 1.38                        | 1                    | 45.0                               | 0.96                                 | 3.71                          | 10.383                        | 0.27  | 0.90  | 0.30 | 48.7  | 10.39 | 0.28  | 0.97  |
| 07522034–2627536 | 243.186  | 0.345    | 7.758 | 9      | –      | –    | g    | t        | –     | –      | –   | –                      | –          | –          | –    | –        | –          | –     | 10.392                             | 0.80                        | 1.15                        | 1                    | 59.0                               | 0.66                                 | 3.98                          | 7.501                         | −0.49 | −2.70 | 2.40 | ...   | ...   | −0.33 | −2.19 |
| 07522062–2508405 | 242.052  | 1.022    | 0.378 | 1      | –      | –    | g    | t        | N     | –      | D1  | e                      | o          | h          | –    | –        | –          | –     | 9.842                              | 0.34                        | 1.13                        | 1                    | 56.2                               | 0.52                                 | 3.81                          | 9.701                         | 0.28  | 0.94  | 0.12 | 57.4  | 9.72  | 0.29  | 0.97  |
| 07523434–2626276 | 243.192  | 0.402    | 9.428 | 9      | –      | –    | g    | t        | –     | –      | –   | –                      | –          | –          | –    | –        | –          | –     | 12.944                             | 0.75                        | 1.48                        | 1                    | 21.6                               | 0.54                                 | 3.98                          | 9.431                         | −0.81 | −3.20 | 2.92 | ...   | ...   | −0.62 | −2.58 |
| 07523883–3224563 | 248.333  | −2.645   | 1.507 | 1      | –      | –    | g    | t        | N     | –      | D2  | –                      | –          | –          | –    | –        | –          | –     | 11.520                             | 0.51                        | 1.66                        | 1                    | 40.0                               | 0.66                                 | 3.81                          | 10.958                        | 0.26  | 0.91  | 0.47 | 46.8  | 10.94 | 0.29  | 1.01  |
| 07524324–2431356 | 241.565  | 1.413    | 0.464 | 1      | –      | –    | g    | t        | N     | –      | D1  | –                      | –          | –          | –    | –        | –          | –     | 11.277                             | 0.38                        | 1.28                        | 1                    | 54.8                               | 0.26                                 | 3.78                          | 11.104                        | 0.30  | 1.05  | 0.14 | 56.6  | 11.11 | 0.31  | 1.08  |
| 07524364–2624206 | 243.180  | 0.450    | 9.026 | 9      | –      | –    | g    | t        | –     | –      | –   | –                      | –          | –          | –    | –        | –          | –     | 9.840                              | 0.90                        | 1.91                        | 1                    | 102.6                              | 0.86                                 | 3.98                          | 6.477                         | −0.59 | −2.57 | 2.80 | ...   | ...   | −0.42 | −1.98 |
| 07524709–2624407 | 243.191  | 0.458    | 7.934 | 9      | –      | –    | g    | t        | –     | –      | –   | –                      | –          | –          | –    | –        | –          | –     | 12.030                             | 1.20                        | ...                         | 1                    | 27.8                               | 0.82                                 | 3.90                          | 9.074                         | −0.11 | ...   | 2.46 | ...   | ...   | 0.04  | ...   |
| 07524726–2616167 | 243.071  | 0.531    | 4.763 | 9      | –      | –    | g    | t        | –     | –      | –   | –                      | –          | –          | –    | –        | –          | –     | 12.181                             | 0.20                        | 0.78                        | 1                    | 62.0                               | 0.30                                 | 3.88                          | 10.406                        | −0.59 | −1.58 | 1.48 | ...   | ...   | −0.50 | −1.27 |
| 07530159–2158341 | 239.410  | 2.779    | 0.543 | 1      | –      | –    | g    | t        | N     | –      | D2  | –                      | –          | –          | –    | –        | –          | –     | 10.474                             | 0.40                        | 1.28                        | 1                    | 37.2                               | 0.84                                 | 3.68                          | 10.272                        | 0.31  | 1.01  | 0.17 | 38.6  | 10.28 | 0.32  | 1.05  |
| 07530935–2825588 | 244.968  | −0.509   | 1.010 | 1      | –      | –    | g    | t        | –     | –      | D2  | e                      | o          | –          | –    | –        | –          | –     | 9.339                              | 0.38                        | 1.35                        | 1                    | 71.2                               | 0.82                                 | 3.86                          | 8.963                         | 0.22  | 0.84  | 0.31 | 76.3  | 8.99  | 0.24  | 0.91  |
| 07531125–2217385 | 239.702  | 2.649    | 0.492 | 1      | –      | –    | g    | t        | –     | –      | D2  | –                      | –          | h          | –    | –        | –          | –     | 10.848                             | 0.48                        | 1.37                        | 1                    | 44.0                               | 0.50                                 | 3.76                          | 10.665                        | 0.40  | 1.13  | 0.15 | 45.6  | 10.67 | 0.41  | 1.16  |
| 07531836–3611492 | 251.660  | −4.459   | 1.746 | 1      | –      | –    | g    | t        | N     | –      | D2  | –                      | –          | –          | –    | –        | –          | –     | 11.248                             | 0.52                        | 1.77                        | 1                    | 40.0                               | 0.50                                 | 3.75                          | 10.597                        | 0.23  | 0.91  | 0.54 | 48.3  | 10.57 | 0.26  | 1.02  |
| 07533288–2129485 | 239.059  | 3.129    | 0.425 | 1      | –      | –    | g    | t        | N     | –      | D1  | –                      | –          | *          | –    | –        | –          | –     | 10.740                             | 0.38                        | 1.17                        | 1                    | 53.6                               | 0.36                                 | 3.71                          | 10.582                        | 0.31  | 0.96  | 0.13 | 55.2  | 10.59 | 0.31  | 0.99  |
| 07535089–3849350 | 253.987  | −5.705   | 0.803 | 1      | –      | –    | g    | t        | –     | –      | D2  | c                      | o          | –          | –    | –        | –          | –     | 10.292                             | 0.47                        | 1.37                        | 1                    | 50.4                               | 0.76                                 | 3.78                          | 9.993                         | 0.34  | 0.97  | 0.25 | 53.5  | 10.01 | 0.35  | 1.02  |
| 07535256–3412293 | 250.006  | −3.343   | 1.720 | 6      | –      | –    | g    | t        | –     | –      | –   | –                      | –          | –          | –    | –        | –          | –     | 10.452                             | 1.06                        | 2.45                        | 1                    | 25.0                               | 0.62                                 | 3.78                          | 9.811                         | 0.77  | 1.59  | 0.53 | ...   | ...   | 0.80  | 1.71  |
| 07541170–2423209 | 241.620  | 1.771    | 0.392 | 1      | –      | –    | g    | t        | N     | –      | D1  | –                      | –          | –          | –    | –        | –          | –     | 10.717                             | 0.36                        | 1.21                        | 1                    | 47.4                               | 0.52                                 | 3.81                          | 10.571                        | 0.30  | 1.01  | 0.12 | 48.5  | 10.58 | 0.31  | 1.04  |
| 07543034–3524203 | 251.103  | −3.846   | 1.464 | 1      | –      | –    | g    | t        | N     | –      | D1  | –                      | –          | –          | –    | –        | –          | –     | 11.630                             | 0.48                        | 1.50                        | 1                    | 42.0                               | 0.50                                 | 3.80                          | 11.085                        | 0.23  | 0.77  | 0.45 | 49.1  | 11.05 | 0.26  | 0.87  |
| 07543584–3454472 | 250.689  | −3.577   | 2.380 | 7      | –      | –    | g    | t        | –     | –      | –   | –                      | –          | –          | –    | –        | –          | –     | 11.505                             | 0.80                        | 1.97                        | 1                    | 38.6                               | 0.50                                 | 3.85                          | 10.618                        | 0.40  | 0.78  | 0.74 | ...   | ...   | 0.45  | 0.94  |
| 07545226–2434463 | 241.862  | 1.805    | 0.339 | 1      | –      | –    | g    | t        | –     | –      | D1  | e                      | o          | h          | –    | –        | –          | –     | 11.105                             | 0.34                        | 1.16                        | 1                    | 64.2                               | 0.68                                 | 3.76                          | 10.979                        | 0.29  | 0.99  | 0.11 | 65.8  | 10.98 | 0.29  | 1.01  |
| 07545229–2756453 | 244.745  | 0.066    | 0.767 | 1      | –      | –    | g    | t        | –     | –      | D2  | –                      | –          | –          | –    | –        | –          | –     | 11.185                             | 0.41                        | 1.32                        | 1                    | 26.8                               | 0.94                                 | 3.89                          | 10.899                        | 0.28  | 0.94  | 0.24 | 28.4  | 10.91 | 0.30  | 0.99  |
| 07545280–3318173 | 249.337  | −2.699   | 1.279 | 1      | –      | –    | g    | t        | –     | –      | D1  | –                      | –          | o          | h    | –        | –          | –     | 11.074                             | 0.44                        | 1.50                        | 1                    | 44.6                               | 0.60                                 | 3.83                          | 10.597                        | 0.23  | 0.86  | 0.40 | 50.9  | 10.57 | 0.25  | 0.95  |
| 07545608–3449383 | 250.651  | −3.473   | 3.809 | 8      | –      | s?   | g    | t        | –     | –      | –   | –                      | –          | –          | –    | –        | –          | –     | 10.532                             | 0.89                        | 2.11                        | 1                    | 39.4                               | 0.88                                 | 3.85                          | 9.113                         | 0.26  | 0.21  | 1.18 | ...   | ...   | 0.33  | 0.46  |
| 07551072–2341325 | 241.138  | 2.323    | 0.413 | 1      | –      | –    | g    | t        | –     | –      | D4  | e                      | o          | –          | –    | –        | –          | –     | 9.473                              | 0.32                        | 1.17                        | 1                    | 67.2                               | 0.92                                 | 3.71                          | 9.319                         | 0.26  | 0.97  | 0.13 | 68.7  | 9.33  | 0.26  | 0.99  |
| 07551240–2809554 | 244.972  | 0.016    | 0.889 | 1      | –      | s?   | g    | t        | –     | –      | D1  | e                      | o          | h          | –    | –        | –          | –     | 9.693                              | 0.35                        | 1.23                        | 1                    | 144.6                              | 0.44                                 | 3.88                          | 9.362                         | 0.20  | 0.79  | 0.28 | 155.5 | 9.37  | 0.22  | 0.85  |
| 07553013–2243466 | 240.351  | 2.883    | 0.460 | 1      | o      | –    | g    | t        | N     | –      | D1  | –                      | –          | o          | h    | –        | –          | –     | 10.105                             | 0.41                        | 1.27                        | 1                    | 76.6                               | 0.30                                 | 3.72                          | 9.934                         | 0.33  | 1.04  | 0.14 | 79.2  | 9.94  | 0.34  | 1.07  |
| 07554671–2716477 | 244.280  | 0.582    | 0.796 | 1      | –      | –    | g    | t        | –     | –      | D1  | e                      | o          | –          | –    | –        | –          | –     | 11.237                             | 0.42                        | 1.42                        | 1                    | 30.2                               | 0.92                                 | 3.81                          | 10.940                        | 0.29  | 1.02  | 0.25 | 32.1  | 10.95 | 0.30  | 1.08  |
| 07561560–3656270 | 252.605  | −4.331   | 1.428 | 1      | –      | –    | g    | t        | –     | –      | D3  | –                      | –          | *          | –    | –        | –          | –     | 10.798                             | 0.46                        | 1.59                        | 1                    | 33.6                               | 0.74                                 | 3.79                          | 10.266                        | 0.23  | 0.88  | 0.44 | 38.1  | 10.28 | 0.25  | 0.97  |
| 07561963–4137420 | 256.656  | −6.723   | 0.772 | 1      | –      | –    | g    | t        | –     | –      | D1  | c                      | o          | –          | –    | –        | –          | –     | 10.247                             | 0.53                        | 1.44                        | 1                    | 42.6                               | 0.64                                 | 3.69                          | 9.959                         | 0.40  | 1.06  | 0.24 | 44.7  | 9.99  | 0.42  | 1.11  |
| 07563338–2150060 | 239.710  | 3.554    | 0.287 |        |        |      |      |          |       |        |     |                        |            |            |      |          |            |       |                                    |                             |                             |                      |                                    |                                      |                               |                               |       |       |      |       |       |       |       |

Table B1: a) continued.

| 2MASX J          | <i>l</i>    | <i>b</i>    | EBV        | Object       | Sample     | Disc        | 2MRS        | Velocity   | NIR         | Photom        | Ext         | <i>K</i> <sub>20</sub> | <i>H-K</i>   | <i>J-K</i>  | vc          | <i>a</i>    | <i>b/a</i>  | st.d. | <i>K</i> <sub>s</sub> <sup>o</sup> | ( <i>H-K</i> ) <sup>o</sup> | ( <i>J-K</i> ) <sup>o</sup> | <i>A</i> <sub>K</sub> | <i>a</i> <sub>d</sub> <sup>o</sup> | <i>K</i> <sub>s</sub> <sup>o,d</sup> | ( <i>H-K</i> ) <sup>o,c</sup> | ( <i>J-K</i> ) <sup>o,c</sup> |             |             |      |             |             |             |       |
|------------------|-------------|-------------|------------|--------------|------------|-------------|-------------|------------|-------------|---------------|-------------|------------------------|--------------|-------------|-------------|-------------|-------------|-------|------------------------------------|-----------------------------|-----------------------------|-----------------------|------------------------------------|--------------------------------------|-------------------------------|-------------------------------|-------------|-------------|------|-------------|-------------|-------------|-------|
| (1)              | deg<br>(2a) | deg<br>(2b) | mag<br>(3) | class<br>(4) | off<br>(5) | flag<br>(6) | gal<br>(7a) | TF<br>(7b) | obs<br>(7c) | ext'd<br>(7d) | type<br>(8) | (9)                    | Opt<br>(10a) | HI<br>(10b) | flg<br>(11) | flg<br>(12) | flg<br>(13) | (14)  | mag<br>(15)                        | mag<br>(16)                 | (17)                        | (18)                  | (19)                               | (20)                                 | mag<br>(21)                   | mag<br>(22)                   | mag<br>(23) | mag<br>(24) | (25) | mag<br>(26) | mag<br>(27) | mag<br>(28) |       |
| 08053136−2449022 | 243.336     | 3.739       | 0.199      | 9            | e          | −           | −           | −          | −           | −             | −           | −                      | −            | −           | −           | o           | −           | −     | 10.835                             | 0.26                        | 1.11                        | −2                    | 51.8                               | 0.56                                 | 3.68                          | 10.761                        | 0.23        | 1.01        | 0.06 | ...         | ...         | 0.23        | 1.03  |
| 08053248−2448519 | 243.336     | 3.744       | 0.199      | 1            | −          | −           | −           | −          | −           | −             | −           | −                      | −            | −           | −           | −           | −           | −     | 9.592                              | 0.33                        | 1.07                        | 1                     | 104.4                              | 0.36                                 | 3.72                          | 9.518                         | 0.30        | 0.97        | 0.06 | 105.3       | 9.53        | 0.30        | 0.98  |
| 08055070−2558480 | 244.360     | 3.179       | 0.213      | 1            | −          | −           | −           | −          | −           | −             | −           | −                      | −            | −           | −           | −           | −           | −     | 10.789                             | 0.37                        | 1.09                        | 1                     | 44.6                               | 0.56                                 | 3.72                          | 10.710                        | 0.34        | 0.99        | 0.07 | 45.0        | 10.72       | 0.34        | 1.00  |
| 08055927−2723510 | 245.575     | 2.447       | 0.409      | 1            | −          | −           | −           | −          | −           | −             | −           | −                      | −            | −           | −           | −           | −           | −     | 8.478                              | 0.31                        | 1.07                        | 1                     | 130.0                              | 0.54                                 | 3.76                          | 8.326                         | 0.24        | 0.87        | 0.13 | 132.5       | 8.34        | 0.25        | 0.90  |
| 08060089−2723541 | 245.579     | 2.452       | 0.410      | 9            | e          | −           | −           | −          | −           | −             | −           | −                      | −            | −           | −           | o           | −           | −     | 9.346                              | 0.29                        | 0.98                        | −2                    | 82.6                               | 0.68                                 | 3.77                          | 9.193                         | 0.22        | 0.77        | 0.13 | ...         | ...         | 0.23        | 0.80  |
| 08060746−2233492 | 241.498     | 5.057       | 0.195      | 1            | −          | −           | −           | −          | −           | −             | −           | −                      | −            | −           | −           | −           | −           | −     | 9.553                              | 0.29                        | 1.04                        | 1                     | 65.8                               | 0.70                                 | 3.63                          | 9.480                         | 0.26        | 0.94        | 0.06 | 66.3        | 9.49        | 0.26        | 0.95  |
| 08061109−2731422 | 245.709     | 2.414       | 0.421      | 1            | −          | −           | −           | −          | −           | −             | −           | −                      | −            | −           | −           | −           | −           | −     | 8.259                              | 0.32                        | 1.05                        | 1                     | 203.4                              | 0.51                                 | ...                           | 8.102                         | 0.25        | 0.84        | 0.13 | ...         | ...         | 0.26        | 0.87  |
| 08062059−3825366 | 254.923     | −3.415      | 2.360      | 9            | −          | −           | −           | −          | −           | −             | −           | −                      | −            | −           | −           | −           | −           | −     | 11.581                             | 0.69                        | 1.48                        | 1                     | 42.2                               | 0.68                                 | 3.82                          | 10.702                        | 0.30        | 0.30        | 0.73 | ...         | ...         | 0.35        | 0.46  |
| 08063182−3730059 | 254.161     | −2.887      | 1.401      | 9            | −          | −           | −           | −          | −           | −             | −           | −                      | −            | −           | −           | −           | −           | −     | 10.545                             | 0.72                        | 1.48                        | 1                     | 52.6                               | 0.54                                 | 3.82                          | 10.023                        | 0.48        | 0.78        | 0.43 | ...         | ...         | 0.51        | 0.87  |
| 08063858−2559092 | 244.461     | 3.328       | 0.216      | 1            | −          | −           | −           | −          | −           | −             | −           | −                      | −            | −           | −           | −           | −           | −     | 10.171                             | 0.31                        | 1.06                        | 1                     | 61.0                               | 0.46                                 | 3.74                          | 10.091                        | 0.28        | 0.95        | 0.07 | 61.6        | 10.10       | 0.28        | 0.97  |
| 08063924−4356568 | 259.642     | −6.311      | 0.405      | 1            | −          | −           | −           | −          | −           | −             | −           | −                      | −            | −           | −           | −           | −           | −     | 10.826                             | 0.35                        | 1.12                        | 1                     | 43.2                               | 0.46                                 | 3.84                          | 10.675                        | 0.28        | 0.92        | 0.13 | 44.2        | 10.69       | 0.29        | 0.95  |
| 08064256−2254184 | 241.860     | 4.989       | 0.253      | 1            | −          | −           | −           | −          | −           | −             | −           | −                      | −            | −           | −           | −           | −           | −     | 9.828                              | 0.36                        | 1.15                        | 1                     | 71.6                               | 0.38                                 | 3.60                          | 9.734                         | 0.32        | 1.02        | 0.08 | 72.4        | 9.74        | 0.33        | 1.04  |
| 08070708−2803182 | 246.265     | 2.305       | 0.458      | 9            | e          | −           | −           | −          | −           | −             | −           | −                      | −            | −           | −           | o           | −           | −     | 11.354                             | 0.30                        | 1.13                        | −2                    | 95.4                               | 0.58                                 | 3.75                          | 11.183                        | 0.22        | 0.90        | 0.14 | ...         | ...         | 0.23        | 0.93  |
| 08070860−2803084 | 246.266     | 2.311       | 0.457      | 1            | −          | −           | −           | −          | −           | −             | −           | −                      | −            | −           | −           | −           | −           | −     | 9.625                              | 0.28                        | 1.04                        | 1                     | 136.2                              | 0.42                                 | 3.71                          | 9.455                         | 0.21        | 0.81        | 0.14 | 141.2       | 9.45        | 0.22        | 0.84  |
| 08070978−2231450 | 241.597     | 5.278       | 0.172      | 1            | −          | −           | −           | −          | −           | −             | −           | −                      | −            | −           | −           | −           | −           | −     | 11.210                             | 0.26                        | 1.09                        | 1                     | 34.0                               | 0.78                                 | 3.53                          | 11.146                        | 0.23        | 1.01        | 0.05 | 34.3        | 11.15       | 0.23        | 1.02  |
| 08072860−2233050 | 241.654     | 5.328       | 0.199      | 1            | −          | −           | −           | −          | −           | −             | −           | −                      | −            | −           | −           | −           | −           | −     | 10.180                             | 0.27                        | 0.99                        | 1                     | 54.4                               | 0.84                                 | 3.58                          | 10.106                        | 0.24        | 0.90        | 0.06 | 54.9        | 10.11       | 0.24        | 0.91  |
| 08073242−3522489 | 252.481     | −1.574      | 1.984      | 7            | −          | −           | −           | −          | −           | −             | −           | −                      | −            | −           | −           | −           | −           | −     | 10.669                             | 1.31                        | ...                         | 1                     | 52.8                               | 0.42                                 | 3.88                          | 9.930                         | 0.98        | ...         | 0.61 | ...         | ...         | 1.02        | ...   |
| 08074237−3544499 | 252.808     | −1.744      | 1.547      | 1            | −          | −           | −           | −          | −           | −             | −           | −                      | −            | −           | −           | −           | −           | −     | 10.330                             | 0.49                        | 1.61                        | 1                     | 47.2                               | 0.84                                 | 3.79                          | 9.754                         | 0.23        | 0.85        | 0.48 | 54.1        | 9.77        | 0.26        | 0.95  |
| 08074946−2557173 | 244.578     | 3.568       | 0.227      | 1            | −          | −           | −           | −          | −           | −             | −           | −                      | −            | −           | −           | −           | −           | −     | 11.080                             | 0.37                        | 1.19                        | 1                     | 63.2                               | 0.20                                 | 3.66                          | 10.995                        | 0.33        | 1.08        | 0.07 | 64.0        | 11.00       | 0.33        | 1.09  |
| 08080036−5104311 | 265.885     | −9.868      | 0.653      | 1            | −          | −           | −           | −          | −           | −             | −           | −                      | −            | −           | −           | −           | −           | −     | 10.840                             | 0.47                        | 1.14                        | 1                     | 57.4                               | 0.78                                 | 3.59                          | 10.597                        | 0.36        | 0.81        | 0.20 | 60.2        | 10.61       | 0.37        | 0.86  |
| 08080066−3558243 | 253.032     | −1.814      | 1.802      | 1            | −          | −           | −           | −          | −           | −             | −           | −                      | −            | −           | −           | −           | −           | −     | 10.408                             | 0.29                        | 0.78                        | 1                     | 41.0                               | 0.54                                 | 3.88                          | 9.737                         | −0.01       | −0.12       | 0.56 | 49.8        | 9.71        | 0.02        | −0.00 |
| 08080435−1534427 | 235.768     | 9.143       | 0.068      | 1            | −          | −           | −           | −          | −           | −             | −           | −                      | −            | −           | −           | −           | −           | −     | 11.132                             | 0.26                        | 0.94                        | 1                     | 29.6                               | 0.90                                 | 3.33                          | 11.107                        | 0.24        | 0.91        | 0.02 | 29.7        | 11.11       | 0.25        | 0.91  |
| 08080461−1452387 | 235.163     | 9.511       | 0.069      | 1            | −          | −           | −           | −          | −           | −             | −           | −                      | −            | −           | −           | −           | −           | −     | 10.687                             | 0.36                        | 1.17                        | 1                     | 69.8                               | 0.22                                 | 3.47                          | 10.661                        | 0.34        | 1.14        | 0.02 | 70.0        | 10.66       | 0.35        | 1.14  |
| 08081083−2225256 | 241.634     | 5.533       | 0.201      | 1            | −          | −           | −           | −          | −           | −             | −           | −                      | −            | −           | −           | −           | −           | −     | 10.620                             | 0.25                        | 1.01                        | 1                     | 44.2                               | 0.68                                 | 3.53                          | 10.545                        | 0.21        | 0.91        | 0.06 | 44.6        | 10.55       | 0.22        | 0.92  |
| 08084087−1841386 | 238.521     | 7.622       | 0.101      | 1            | −          | −           | −           | −          | −           | −             | −           | −                      | −            | −           | −           | −           | −           | −     | 10.884                             | 0.34                        | 1.00                        | 1                     | 39.0                               | 0.70                                 | 3.53                          | 10.846                        | 0.32        | 0.95        | 0.03 | 39.1        | 10.85       | 0.33        | 0.96  |
| 08085396−5105056 | 265.967     | −9.754      | 0.717      | 1            | −          | −           | −           | −          | −           | −             | −           | −                      | −            | −           | −           | −           | −           | −     | 10.224                             | 0.40                        | 1.30                        | 1                     | 48.2                               | 0.90                                 | 3.62                          | 9.957                         | 0.28        | 0.94        | 0.22 | 50.6        | 9.98        | 0.29        | 0.99  |
| 08090254−2427021 | 243.456     | 4.611       | 0.205      | 1            | −          | −           | −           | −          | −           | −             | −           | −                      | −            | −           | −           | −           | −           | −     | 11.105                             | 0.38                        | 1.24                        | 1                     | 31.8                               | 0.88                                 | 3.71                          | 11.029                        | 0.34        | 1.14        | 0.06 | 32.1        | 11.04       | 0.35        | 1.16  |
| 08091411−1841421 | 238.592     | 7.733       | 0.107      | 1            | −          | −           | −           | −          | −           | −             | −           | −                      | −            | −           | −           | −           | −           | −     | 10.733                             | 0.37                        | 1.07                        | 1                     | 43.8                               | 0.82                                 | 3.55                          | 10.693                        | 0.36        | 1.02        | 0.03 | 44.0        | 10.70       | 0.36        | 1.02  |
| 08091516−1839531 | 238.568     | 7.752       | 0.107      | 1            | −          | −           | −           | −          | −           | −             | −           | −                      | −            | −           | −           | −           | −           | −     | 11.225                             | 0.39                        | 1.13                        | 1                     | 44.0                               | 0.66                                 | 3.55                          | 11.185                        | 0.37        | 1.08        | 0.03 | 44.2        | 11.19       | 0.37        | 1.09  |
| 08092197−1756223 | 237.962     | 8.160       | 0.114      | 1            | −          | −           | −           | −          | −           | −             | −           | −                      | −            | −           | −           | −           | −           | −     | 11.098                             | 0.43                        | 1.26                        | 1                     | 57.4                               | 0.32                                 | 3.48                          | 11.056                        | 0.41        | 1.20        | 0.04 | 57.7        | 11.06       | 0.41        | 1.21  |
| 08093283−3604559 | 253.292     | −1.612      | 1.802      | 8            | −          | −           | −           | −          | −           | −             | −           | −                      | −            | −           | −           | −           | −           | −     | 11.178                             | 1.15                        | 2.17                        | 1                     | 29.2                               | 0.54                                 | 3.86                          | 10.507                        | 0.85        | 1.27        | 0.56 | ...         | ...         | 0.89        | 1.39  |
| 08093338−4105369 | 257.509     | −4.330      | 1.220      | 1            | −          | −           | −           | −          | −           | −             | −           | −                      | −            | −           | −           | −           | −           | −     | 11.440                             | 0.47                        | 1.49                        | 1                     | 31.4                               | 0.46                                 | 3.81                          | 10.985                        | 0.27        | 0.88        | 0.38 | 35.1        | 10.99       | 0.30        | 0.96  |
| 08094340−4337479 | 259.669     | −5.672      | 0.560      | 1            | −          | −           | −           | −          | −           | −             | −           | −                      | −            | −           | −           | −           | −           | −     | 10.519                             | 0.41                        | 1.27                        | 1                     | 39.0                               | 0.90                                 | 3.78                          | 10.310                        | 0.32        | 0.99        | 0.17 | 40.4        | 10.33       | 0.33        | 1.03  |
| 08095370−4141379 | 258.050     | −4.601      | 1.198      | 1            | −          | −           | −           | −          | −           | −             | −           | −                      | −            | −           | −           | −           | −           | −     | 10.023                             | 0.57                        | 1.69                        | 1                     | 134.6                              | 0.18                                 | 3.81                          | 9.577                         | 0.37        | 1.10        | 0.37 | 152.7       | 9.54        | 0.39        | 1.18  |
| 08102288−2218546 | 241.816     | 6.021       | 0.159      | 1            | −          | −           | −           | −          | −           | −             | −           | −                      | −            | −           | −           | −           | −           | −     | 10.629                             | 0.29                        | 0.96                        | 1                     | 45.4                               | 0.82                                 | 3.59                          | 10.570                        | 0.26        | 0.88        | 0.05 | 45.7        | 10.58       | 0.27        | 0.89  |
| 08103485−2242340 | 242.175     | 5.847       | 0.163      | 1            | −          | −           | −           | −          | −           | −             | −           | −                      | −            | −           | −           | −           | −           | −     | 10.283                             | 0.30                        | 1.07                        | 1                     | 55.0                               | 0.56                                 | 3.60                          | 10.222                        | 0.27        | 0.99        | 0.05 | 55.3        | 10.23       | 0.27        | 1.00  |
| 08104071−3602536 | 253.388     | −1.402      | 2.809      | 8            | −          | −           | −           | −          | −           | −             | −           | −                      | −            | −           | −           | −           | −           | −     | 9.944                              | 1.25                        | 3.07                        | 1                     | 70.0                               | 0.22                                 | 3.85                          | 8.897                         | 0.79        | 1.67        | 0.87 | ...         | ...         | 0.84        | 1.86  |
| 08104263−4923538 | 264.671     | −8.617      | 0.370      | 1            | −          | −           | −           | −          | −           | −             | −           | −                      | −            | −           | −           | −           | −           | −     | 11.131                             | 0.35                        | 1.17                        | 1                     | 42.8                               | 0.78                                 | 3.77                          | 10.993                        | 0.29        | 0.98        | 0.11 | 43.8        | 11.00       | 0.30        | 1.01  |
| 08104351−3603196 | 253.399     | −1.398      | 2.832      | 9            | −          | −           | −           | −          | −           | −             | −           | −                      | −            | −           | −           | −           | −           | −     | 11.351                             | 1.64                        | ...                         | 1                     | 36.4                               | 0.22                                 | 3.85                          | 10.296                        | 1.17        | ...         | 0.88 | ...         | ...         | 1.22        | ...   |
| 08105503−3051287 | 249.069     | 1.478       | 0.628      | 1            | −          | −           | −           | −          | −           | −             | −           | −                      | −            | −           | −           | −           | −           | −     | 11.342                             | 0.48                        | 1.38                        | 1                     | 43.0                               | 0.40                                 | 3.78                          | 11.108                        | 0.38        | 1.07        | 0.19 | 45.1        | 11.12       | 0.39        | 1.11  |
| 08105951−3604517 | 253.450     | −1.367      | 2.131      | 8            | −          | −           | −           | −          | −           | −             | −           | −                      | −            | −           | −           | −           | −           | −     | 10.524                             | 1.47                        | 3.46                        | 1                     | 25.4                               | 0.70                                 | 3.86                          | 9.730                         | 1.11        | 2.40        | 0.66 | ...         | ...         | 1.15        | 2.54  |
| 08110108−3605007 | 253.455     | −1.364      | 2.         |              |            |             |             |            |             |               |             |                        |              |             |             |             |             |       |                                    |                             |                             |                       |                                    |                                      |                               |                               |             |             |      |             |             |             |       |



Table B1: a) continued.

| 2MASX J          | <i>l</i>    | <i>b</i>    | EBV        | Object       | Sample     | Disc        | 2MRS       | Velocity    | NIR           | Photom      | Ext | <i>K</i> <sub>20</sub> | <i>H-K</i>  | <i>J-K</i>  | vc          | <i>a</i>    | <i>b/a</i> | st.d.       | <i>K</i> <sub>s</sub> <sup>o</sup> | ( <i>H-K</i> ) <sup>o</sup> | ( <i>J-K</i> ) <sup>o</sup> | <i>A<sub>K</sub></i> | <i>a</i> <sub>d</sub> <sup>o</sup> | <i>K</i> <sub>s</sub> <sup>o,d</sup> | ( <i>H-K</i> ) <sup>o,c</sup> | ( <i>J-K</i> ) <sup>o,c</sup> |             |      |             |             |             |       |
|------------------|-------------|-------------|------------|--------------|------------|-------------|------------|-------------|---------------|-------------|-----|------------------------|-------------|-------------|-------------|-------------|------------|-------------|------------------------------------|-----------------------------|-----------------------------|----------------------|------------------------------------|--------------------------------------|-------------------------------|-------------------------------|-------------|------|-------------|-------------|-------------|-------|
| (1)              | deg<br>(2a) | deg<br>(2b) | mag<br>(3) | class<br>(4) | off<br>(5) | gal<br>(7a) | TF<br>(7b) | obs<br>(7c) | ext'd<br>(7d) | type<br>(8) | (9) | Opt<br>(10a)           | HI<br>(10b) | flg<br>(11) | flg<br>(12) | flg<br>(13) | (14)       | mag<br>(15) | mag<br>(16)                        | (17)                        | (18)                        | (19)                 | (20)                               | mag<br>(21)                          | mag<br>(22)                   | mag<br>(23)                   | mag<br>(24) | (25) | mag<br>(26) | mag<br>(27) | mag<br>(28) |       |
| 08165172–4750417 | 263.908     | −6.922      | 0.680      | 1            | —          | —           | —          | —           | —             | D3          | c   | o                      | —           | —           | —           | —           | —          | 10.831      | 0.39                               | 1.30                        | 1                           | 37.8                 | 0.62                               | 3.71                                 | 10.578                        | 0.28                          | 0.96        | 0.21 | 39.6        | 10.60       | 0.29        | 1.00  |
| 08170147–3410277 | 252.545     | 0.716       | 0.483      | 1            | —          | —           | —          | —           | —             | D1          | —   | —                      | —           | —           | —           | —           | —          | 10.735      | 0.50                               | 1.46                        | 1                           | 78.4                 | 0.18                               | 3.84                                 | 10.555                        | 0.42                          | 1.22        | 0.15 | 81.0        | 10.56       | 0.43        | 1.25  |
| 08170607–2727209 | 246.974     | 4.481       | 0.219      | 1            | —          | —           | —          | —           | —             | D1          | e   | o                      | h           | —           | —           | —           | —          | 7.495       | 0.30                               | 1.01                        | 1                           | 189.4                | 0.54                               | ...                                  | 7.413                         | 0.27                          | 0.91        | 0.07 | ...         | ...         | 0.27        | 0.92  |
| 08172690–2440519 | 244.699     | 6.086       | 0.165      | 1            | —          | —           | —          | —           | —             | D2          | c   | o                      | —           | —           | V           | —           | —          | 10.168      | 0.33                               | 1.05                        | 1                           | 66.6                 | 0.46                               | 3.59                                 | 10.107                        | 0.31                          | 0.96        | 0.05 | 67.1        | 10.11       | 0.31        | 0.97  |
| 08172741–2759259 | 247.463     | 4.249       | 0.290      | 1            | —          | —           | —          | —           | —             | D3          | —   | —                      | —           | —           | —           | —           | —          | 11.042      | 0.44                               | 1.25                        | 1                           | 21.4                 | 0.92                               | 3.65                                 | 10.934                        | 0.39                          | 1.11        | 0.09 | 21.7        | 10.95       | 0.40        | 1.13  |
| 08173227–4537124 | 262.107     | −5.596      | 0.806      | 1            | o          | —           | —          | —           | —             | D1          | ca  | —                      | h           | —           | —           | ao          | —          | 10.707      | 0.39                               | 1.13                        | 1                           | 48.0                 | 0.60                               | 3.80                                 | 10.407                        | 0.26                          | 0.73        | 0.25 | 51.7        | 10.39       | 0.28        | 0.79  |
| 08173846–2943505 | 248.933     | 3.311       | 0.332      | 1            | —          | —           | —          | —           | —             | D1          | e   | o                      | —           | —           | —           | —           | —          | 9.824       | 0.29                               | 1.04                        | 1                           | 75.2                 | 1.00                               | ...                                  | 9.700                         | 0.23                          | 0.88        | 0.10 | ...         | ...         | 0.24        | 0.90  |
| 08174326–3007501 | 249.274     | 3.101       | 0.395      | 1            | —          | —           | —          | —           | —             | D1          | e   | —                      | h           | —           | —           | —           | —          | 9.579       | 0.28                               | 1.00                        | 1                           | 124.2                | 0.54                               | ...                                  | 9.432                         | 0.21                          | 0.80        | 0.12 | ...         | ...         | 0.22        | 0.83  |
| 08175193–3827281 | 256.187     | −1.545      | 2.640      | 6            | —          | —           | —          | —           | —             | —           | —   | —                      | —           | —           | —           | —           | —          | 11.111      | 0.90                               | 2.09                        | 1                           | 45.6                 | 0.52                               | 3.90                                 | 10.127                        | 0.46                          | 0.78        | 0.82 | ...         | ...         | 0.51        | 0.95  |
| 08175237–3552503 | 254.055     | −0.097      | 3.572      | 7            | —          | —           | —          | —           | —             | —           | —   | —                      | —           | —           | —           | —           | —          | 8.262       | 1.08                               | 2.38                        | 1                           | 97.4                 | 0.52                               | 3.87                                 | 6.931                         | 0.48                          | 0.60        | 1.11 | ...         | ...         | 0.55        | 0.84  |
| 08175393–4139481 | 258.848     | −3.336      | 2.238      | 9            | —          | —           | —          | —           | —             | —           | —   | —                      | —           | —           | —           | —           | —          | 11.386      | 0.33                               | 1.13                        | 2                           | 31.8                 | ...                                | 3.99                                 | ...                           | −0.04                         | 0.02        | 0.69 | ...         | ...         | ...         | ...   |
| 08182775–3547298 | 254.049     | 0.052       | 2.101      | 7            | —          | —           | —          | —           | —             | —           | —   | —                      | —           | —           | —           | —           | —          | 9.945       | 0.75                               | 1.86                        | 1                           | 34.8                 | 0.90                               | 3.90                                 | 9.162                         | 0.40                          | 0.81        | 0.65 | ...         | ...         | 0.44        | 0.95  |
| 08183000–2148580 | 242.428     | 7.870       | 0.114      | 1            | —          | —           | —          | —           | —             | D4          | c   | o                      | —           | —           | V           | —           | —          | 9.841       | 0.25                               | 0.98                        | 1                           | 55.8                 | 0.74                               | 3.52                                 | 9.799                         | 0.23                          | 0.93        | 0.04 | 56.0        | 9.80        | 0.24        | 0.93  |
| 08183025–2524391 | 245.443     | 5.879       | 0.147      | 1            | —          | —           | —          | —           | —             | D2          | c   | —                      | —           | —           | V           | —           | —          | 10.554      | 0.20                               | 0.97                        | 1                           | 54.0                 | 0.46                               | 3.54                                 | 10.499                        | 0.18                          | 0.90        | 0.05 | 54.3        | 10.51       | 0.18        | 0.91  |
| 08184004–3956567 | 257.509     | −2.254      | 3.209      | 6            | —          | —           | —          | —           | —             | —           | —   | —                      | —           | —           | —           | —           | —          | 12.055      | 1.52                               | ...                         | 1                           | 23.6                 | 0.76                               | 3.80                                 | 10.859                        | 0.99                          | ...         | 0.99 | ...         | ...         | 1.06        | ...   |
| 08184560–2529582 | 245.449     | 5.878       | 0.144      | 1            | —          | —           | —          | —           | —             | D1          | c   | —                      | h           | —           | V           | —           | —          | 7.919       | 0.29                               | 0.99                        | 1                           | 180.4                | 0.56                               | ...                                  | 7.865                         | 0.27                          | 0.92        | 0.04 | ...         | ...         | 0.27        | 0.93  |
| 08184597–2522111 | 245.442     | 5.952       | 0.144      | 1            | —          | —           | —          | —           | —             | D4          | c   | o                      | —           | —           | V           | —           | —          | 8.414       | 0.25                               | 0.97                        | 1                           | 84.8                 | 0.96                               | 3.54                                 | 8.360                         | 0.22                          | 0.90        | 0.04 | 85.2        | 8.37        | 0.22        | 0.91  |
| 08190358–3703594 | 255.170     | −0.567      | 1.057      | 7            | —          | —           | —          | —           | —             | —           | —   | —                      | —           | —           | —           | —           | —          | 11.262      | 0.89                               | 1.94                        | 1                           | 29.4                 | 0.68                               | 3.89                                 | 10.868                        | 0.72                          | 1.42        | 0.33 | ...         | ...         | 0.74        | 1.49  |
| 08190586–4008354 | 257.716     | −2.295      | 3.731      | 1            | —          | —           | —          | —           | —             | D3          | —   | —                      | —           | —           | —           | —           | —          | 11.602      | 0.82                               | 2.79                        | 1                           | 22.6                 | 0.82                               | 3.80                                 | 10.212                        | 0.21                          | 0.94        | 1.16 | 35.8        | 10.12       | 0.28        | 1.18  |
| 08191136–3833104 | 256.412     | −1.384      | 1.549      | 1            | —          | —           | —          | —           | —             | D2          | —   | —                      | —           | —           | —           | —           | —          | 10.885      | 0.55                               | 1.68                        | 1                           | 24.6                 | 0.94                               | 3.90                                 | 10.308                        | 0.30                          | 0.91        | 0.48 | 28.2        | 10.33       | 0.33        | 1.01  |
| 08191474–2511170 | 245.351     | 6.143       | 0.142      | 1            | —          | —           | —          | —           | —             | D1          | c   | o                      | h           | —           | V           | —           | —          | 9.713       | 0.34                               | 1.08                        | 1                           | 53.8                 | 0.96                               | 3.56                                 | 9.660                         | 0.31                          | 1.01        | 0.04 | 54.0        | 9.67        | 0.32        | 1.02  |
| 08192425–2447083 | 245.035     | 6.397       | 0.139      | 1            | —          | —           | —          | —           | —             | D1          | c   | o                      | h           | —           | V           | —           | —          | 10.728      | 0.15                               | 0.95                        | 1                           | 72.4                 | 0.44                               | 3.56                                 | 10.676                        | 0.12                          | 0.88        | 0.04 | 72.9        | 10.68       | 0.13        | 0.89  |
| 08192544–5331401 | 268.934     | −9.702      | 0.414      | 1            | —          | —           | —          | —           | —             | D2          | c   | o                      | —           | —           | —           | —           | —          | 10.854      | 0.43                               | 1.26                        | 1                           | 36.2                 | 0.72                               | 3.57                                 | 10.700                        | 0.36                          | 1.05        | 0.13 | 37.1        | 10.71       | 0.37        | 1.08  |
| 08201972–5025202 | 266.390     | −7.874      | 1.008      | 1            | —          | —           | —          | —           | —             | D3          | e   | o                      | —           | —           | —           | —           | —          | 11.313      | 0.40                               | 1.44                        | 1                           | 30.0                 | 0.54                               | 3.64                                 | 10.937                        | 0.23                          | 0.94        | 0.31 | 32.6        | 10.95       | 0.25        | 1.00  |
| 08203279–3540352 | 254.193     | 0.466       | 0.948      | 7            | —          | —           | —          | —           | —             | —           | —   | —                      | —           | —           | —           | —           | —          | 10.917      | 1.48                               | 3.24                        | 1                           | 20.2                 | 0.68                               | 3.82                                 | 10.564                        | 1.32                          | 2.77        | 0.29 | ...         | ...         | 1.34        | 2.83  |
| 08204759–3613189 | 254.670     | 0.197       | 11.010     | 9            | —          | —           | —          | —           | —             | —           | —   | —                      | —           | —           | —           | —           | —          | 10.295      | 0.99                               | 1.59                        | 1                           | 123.0                | 0.60                               | 3.89                                 | 6.193                         | −0.84                         | −3.88       | 3.41 | ...         | ...         | −0.62       | −3.16 |
| 08205164–3613339 | 254.681     | 0.206       | 11.400     | 9            | —          | —           | —          | —           | —             | —           | —   | —                      | —           | —           | —           | —           | —          | 9.892       | 1.22                               | 1.73                        | 1                           | 94.4                 | 1.00                               | 3.89                                 | 5.644                         | −0.67                         | −3.94       | 3.53 | ...         | ...         | −0.44       | −3.18 |
| 08205536–3613122 | 254.683     | 0.220       | 12.526     | 8            | —          | —           | —          | —           | —             | —           | —   | —                      | —           | —           | —           | —           | —          | 8.283       | 1.20                               | 2.02                        | 1                           | 75.6                 | 0.60                               | 3.89                                 | 3.616                         | −0.88                         | −4.20       | 3.88 | ...         | ...         | −0.63       | −3.38 |
| 08205823–4822250 | 264.734     | −6.645      | 0.741      | 1            | —          | —           | —          | —           | —             | D3          | c   | o                      | —           | —           | —           | —           | —          | 10.829      | 0.34                               | 1.35                        | 1                           | 33.6                 | 0.88                               | 3.70                                 | 10.553                        | 0.22                          | 0.98        | 0.23 | 35.5        | 10.57       | 0.23        | 1.03  |
| 08205860–4934442 | 265.742     | −7.318      | 1.624      | 8            | o          | —           | —          | —           | —             | —           | —   | —                      | —           | —           | —           | —           | —          | 10.109      | 0.99                               | 2.26                        | 1                           | 71.0                 | 0.56                               | 3.66                                 | 9.504                         | 0.72                          | 1.45        | 0.50 | ...         | ...         | 0.75        | 1.56  |
| 08210598–4940511 | 265.838     | −7.359      | 1.714      | 8            | —          | —           | —          | —           | —             | —           | —   | —                      | —           | —           | —           | —           | —          | 10.710      | 1.14                               | 2.48                        | 1                           | 51.8                 | 0.38                               | 3.62                                 | 10.071                        | 0.86                          | 1.63        | 0.53 | ...         | ...         | 0.89        | 1.74  |
| 08210735–4321103 | 260.583     | −3.796      | 2.109      | 1            | —          | —           | —          | —           | —             | D2          | —   | —                      | —           | —           | —           | —           | —          | 12.016      | 0.72                               | 1.87                        | 1                           | 30.4                 | 0.66                               | 3.86                                 | 11.230                        | 0.37                          | 0.82        | 0.65 | 39.5        | 11.14       | 0.41        | 0.96  |
| 08212494–5301582 | 268.681     | −9.181      | 0.465      | 1            | —          | —           | —          | —           | —             | D2          | c   | o                      | —           | —           | —           | —           | —          | 10.377      | 0.38                               | 1.20                        | 1                           | 49.0                 | 0.86                               | 3.64                                 | 10.204                        | 0.30                          | 0.97        | 0.14 | 50.5        | 10.22       | 0.31        | 1.00  |
| 08212649–5301162 | 268.674     | −9.171      | 0.469      | 1            | —          | —           | —          | —           | —             | D1          | c   | —                      | —           | —           | —           | —           | —          | 11.116      | 0.45                               | 1.25                        | 1                           | 55.6                 | 0.40                               | 3.64                                 | 10.941                        | 0.37                          | 1.01        | 0.15 | 57.4        | 10.95       | 0.38        | 1.04  |
| 08213966–3903268 | 257.100     | −1.274      | 2.127      | 2            | —          | —           | —          | —           | —             | D3          | —   | —                      | h           | —           | —           | —           | —          | 11.931      | 0.57                               | 1.81                        | 1                           | 22.4                 | 0.62                               | 3.89                                 | 11.138                        | 0.22                          | 0.75        | 0.66 | 28.2        | 11.11       | 0.26        | 0.89  |
| 08221941–4206459 | 259.685     | −2.910      | 7.476      | 9            | —          | —           | —          | —           | —             | —           | —   | —                      | —           | —           | —           | —           | —          | 13.594      | 0.47                               | 1.20                        | −1                          | 14.0                 | 0.58                               | 3.91                                 | 10.808                        | −0.77                         | −2.51       | 2.32 | ...         | ...         | −0.63       | −2.02 |
| 08224226–3240398 | 251.980     | 2.539       | 0.360      | 1            | —          | —           | —          | —           | —             | D3          | —   | —                      | —           | —           | —           | —           | —          | 11.027      | 0.33                               | 1.15                        | 1                           | 32.2                 | 0.84                               | 3.81                                 | 10.893                        | 0.27                          | 0.97        | 0.11 | 32.9        | 10.90       | 0.28        | 0.99  |
| 08225239–4208018 | 259.761     | −2.838      | 12.828     | 8            | —          | —           | —          | —           | —             | —           | —   | —                      | —           | —           | —           | —           | —          | 8.373       | 0.93                               | 2.44                        | 1                           | 110.4                | 0.78                               | 3.92                                 | 3.593                         | −1.19                         | −3.94       | 3.97 | ...         | ...         | −0.94       | −3.09 |
| 08230395–4155551 | 259.615     | −2.694      | 6.114      | 8            | —          | —           | —          | —           | —             | —           | —   | —                      | —           | —           | —           | —           | —          | 9.910       | 1.34                               | 3.05                        | 1                           | 58.4                 | 0.60                               | 3.86                                 | 7.632                         | 0.33                          | 0.01        | 1.89 | ...         | ...         | 0.45        | 0.42  |
| 08231438–4146314 | 259.505     | −2.578      | 4.517      | 9            | —          | —           | —          | —           | —             | —           | —   | —                      | —           | —           | —           | —           | —          | 12.331      | 1.01                               | ...                         | 1                           | 32.0                 | 0.44                               | 3.87                                 | 10.648                        | 0.26                          | ...         | 1.40 | ...         | ...         | 0.35        | ...   |
| 08231546–4146064 | 259.502     | −2.571      | 4.498      | 8            | —          | —           | —          | —           | —             | —           | —   | —                      | —           | —           | —           | —           | —          | 11.620      | 0.89                               | 2.31                        | 1                           | 39.8                 | 0.48                               | 3.87                                 | 9.944                         | 0.15                          | 0.07        | 1.39 | ...         | ...         | 0.24        | 0.37  |
| 08231909–2611495 | 246.709     | 6.335       | 0.177      | 1            | —          | —           | —          | —           | —             | D1          | c   | —                      | h           | —           | V           | —           | —          | 10.242      | 0.22                               | 0.92                        | 1                           | 70.0                 | 0.88                               | 3.56                                 | 10.176                        | 0.19                          | 0.83        | 0.05 | 70.7        | 10.18       | 0.20        | 0.84  |
| 08232452–4836112 | 265.154     | −6.440      | 0.791      | 1            | —          | —           | —          | —           | —             | D3          | c   | o                      | —           | —           | —           | —           | —          | 11.197      | 0.43                               | 1.20</                      |                             |                      |                                    |                                      |                               |                               |             |      |             |             |             |       |

Table B1: a) continued.

| 2MASX J          | <i>l</i> | <i>b</i> | EBV    | Object | Sample | Disc | 2MRS | Velocity | NIR  | Photom | Ext  | <i>K</i> <sub>20</sub> | <i>H-K</i> | <i>J-K</i> | vc   | <i>a</i> | <i>b/a</i> | st.d. | <i>K</i> <sub>s</sub> <sup>o</sup> | ( <i>H-K</i> ) <sup>o</sup> | ( <i>J-K</i> ) <sup>o</sup> | <i>A</i> <sub>K</sub> | <i>a</i> <sub>d</sub> <sup>o</sup> | <i>K</i> <sub>s</sub> <sup>o,d</sup> | ( <i>H-K</i> ) <sup>o,c</sup> | ( <i>J-K</i> ) <sup>o,c</sup> |       |       |      |      |       |       |       |
|------------------|----------|----------|--------|--------|--------|------|------|----------|------|--------|------|------------------------|------------|------------|------|----------|------------|-------|------------------------------------|-----------------------------|-----------------------------|-----------------------|------------------------------------|--------------------------------------|-------------------------------|-------------------------------|-------|-------|------|------|-------|-------|-------|
| (1)              | deg      | deg      | mag    | class  | off    | flag | gal  | TF       | obs  | ext'd  | type | (9)                    | Opt        | HI         | flag | flag     | flag       | flag  | mag                                | mag                         | mag                         | mag                   | mag                                | mag                                  | mag                           | mag                           |       |       |      |      |       |       |       |
| (1)              | (2a)     | (2b)     | (3)    | (4)    | (5)    | (6)  | (7a) | (7b)     | (7c) | (7d)   | (8)  | (9)                    | (10a)      | (10b)      | (11) | (12)     | (13)       | (14)  | (15)                               | (16)                        | (17)                        | (18)                  | (19)                               | (20)                                 | (21)                          | (22)                          | (23)  | (24)  | (25) | (26) | (27)  | (28)  |       |
| 08290990-4109311 | 259.645  | -1.316   | 5.700  | 8      | -      | -    | -    | -        | -    | -      | -    | -                      | -          | -          | -    | -        | -          | -     | 12.872                             | 1.13                        | ...                         | -2                    | 23.2                               | 0.54                                 | 3.94                          | 10.748                        | 0.18  | ...   | 1.77 | ...  | ...   | 0.30  | ...   |
| 08291388-4110501 | 259.670  | -1.318   | 5.877  | 8      | -      | -    | -    | -        | -    | -      | -    | -                      | -          | -          | -    | -        | -          | -     | 11.027                             | 1.19                        | 2.92                        | 1                     | 50.6                               | 0.30                                 | 3.94                          | 8.837                         | 0.22  | -0.00 | 1.82 | ...  | ...   | 0.34  | 0.39  |
| 08293151-4111092 | 259.707  | -1.277   | 5.516  | 9      | -      | -    | -    | -        | -    | -      | -    | -                      | -          | -          | -    | -        | -          | -     | 12.900                             | 0.64                        | 1.79                        | 1                     | 23.2                               | 0.58                                 | 3.94                          | 10.845                        | -0.28 | -0.95 | 1.71 | ...  | ...   | -0.17 | -0.59 |
| 08293319-4111052 | 259.709  | -1.272   | 5.429  | 9      | -      | -    | -    | -        | -    | -      | -    | -                      | -          | -          | -    | -        | -          | -     | 13.116                             | ...                         | ...                         | 1                     | 13.4                               | 1.00                                 | 3.94                          | 11.093                        | ...   | ...   | 1.68 | ...  | ...   | ...   | ...   |
| 08293905-3526048 | 255.063  | 2.118    | 0.763  | 1      | -      | -    | g    | -        | N    | -      | D3   | -                      | -          | -          | -    | -        | -          | -     | 10.447                             | 0.44                        | 1.35                        | 1                     | 45.2                               | 0.68                                 | 3.80                          | 10.163                        | 0.31  | 0.97  | 0.24 | 47.7 | 10.18 | 0.32  | 1.02  |
| 08295316-4555092 | 263.585  | -3.997   | 1.603  | 7      | -      | -    | -    | -        | -    | -      | -    | -                      | -          | -          | -    | -        | -          | -     | 10.153                             | 1.43                        | 3.21                        | 1                     | 29.8                               | 0.86                                 | 3.92                          | 9.556                         | 1.16  | 2.41  | 0.50 | ...  | ...   | 1.19  | 2.52  |
| 08300716-4427323 | 262.424  | -3.108   | 2.684  | 8      | -      | -    | -    | -        | -    | -      | -    | -                      | -          | -          | -    | -        | -          | -     | 11.923                             | 0.69                        | 1.95                        | 1                     | 29.0                               | 0.82                                 | 3.92                          | 10.923                        | 0.24  | 0.62  | 0.83 | ...  | ...   | 0.30  | 0.79  |
| 08301024-4429123 | 262.451  | -3.117   | 2.593  | 8      | -      | -    | -    | -        | -    | -      | -    | -                      | -          | -          | -    | -        | -          | -     | 11.412                             | 0.57                        | 1.69                        | -2                    | 28.4                               | 0.54                                 | 3.92                          | 10.446                        | 0.15  | 0.40  | 0.80 | ...  | ...   | 0.20  | 0.58  |
| 08302510-4427093 | 262.450  | -3.062   | 2.586  | 8      | -      | -    | -    | -        | -    | -      | -    | -                      | -          | -          | -    | -        | -          | -     | 11.511                             | 1.23                        | 2.87                        | 1                     | 16.8                               | 0.86                                 | 3.92                          | 10.547                        | 0.81  | 1.59  | 0.80 | ...  | ...   | 0.86  | 1.76  |
| 08303660-4051390 | 259.564  | -0.920   | 4.433  | 7      | -      | -    | -    | -        | -    | -      | -    | -                      | -          | -          | -    | -        | -          | -     | 9.975                              | 1.02                        | 2.32                        | 1                     | 72.6                               | 0.60                                 | 3.94                          | 8.323                         | 0.29  | 0.11  | 1.37 | ...  | ...   | 0.37  | 0.41  |
| 08305941-3249032 | 253.105  | 3.879    | 0.369  | 1      | -      | -    | g    | -        | N    | -      | D2   | -                      | -          | -          | -    | -        | -          | -     | 11.166                             | 0.33                        | 1.16                        | 1                     | 38.0                               | 0.62                                 | 3.78                          | 11.029                        | 0.26  | 0.97  | 0.11 | 38.8 | 11.04 | 0.27  | 1.00  |
| 08312668-4434583 | 262.663  | -2.990   | 1.610  | 1      | -      | -    | g    | -        | t    | P      | D1   | -                      | -          | -          | -    | -        | -          | -     | 11.296                             | 0.53                        | 1.53                        | 1                     | 35.2                               | 0.38                                 | 3.96                          | 10.696                        | 0.26  | 0.73  | 0.50 | 40.9 | 10.70 | 0.29  | 0.84  |
| 08313400-4228094 | 260.969  | -1.725   | 2.733  | 2      | -      | -    | g    | -        | t    | -      | D1   | -                      | -          | h          | -    | -        | e          | -     | 12.113                             | 0.79                        | 2.63                        | 1                     | 26.0                               | 0.48                                 | 3.93                          | 11.095                        | 0.33  | 1.27  | 0.85 | 37.2 | 10.97 | 0.39  | 1.45  |
| 08314334-2607132 | 247.735  | 7.924    | 0.088  | 1      | -      | -    | -    | -        | -    | -      | D1   | c                      | o          | -          | -    | -        | -          | -     | 10.471                             | 0.30                        | 1.03                        | 1                     | 50.4                               | 0.62                                 | 3.56                          | 10.438                        | 0.29  | 0.98  | 0.03 | 50.6 | 10.44 | 0.29  | 0.99  |
| 08315860-4200381 | 260.643  | -1.392   | 2.755  | 7      | -      | -    | -    | -        | -    | -      | -    | -                      | -          | -          | -    | -        | -          | -     | 12.155                             | 0.97                        | ...                         | -2                    | 38.8                               | 0.30                                 | 4.01                          | 11.128                        | 0.51  | ...   | 0.85 | ...  | ...   | 0.57  | ...   |
| 08320488-4310262 | 261.593  | -2.065   | 9.496  | 9      | -      | -    | -    | -        | -    | -      | -    | -                      | -          | -          | -    | -        | -          | -     | 13.736                             | 0.53                        | 1.26                        | -1                    | 10.0                               | 1.00                                 | 3.92                          | 10.198                        | -1.05 | -3.46 | 2.94 | ...  | ...   | -0.86 | -2.83 |
| 08320506-4310322 | 261.595  | -2.066   | 9.690  | 7      | -      | -    | -    | -        | -    | -      | -    | -                      | -          | -          | -    | -        | -          | -     | 13.386                             | 1.07                        | ...                         | -1                    | 12.6                               | 1.00                                 | 3.92                          | 9.776                         | -0.53 | ...   | 3.00 | ...  | ...   | -0.34 | ...   |
| 08320586-4202462 | 260.685  | -1.395   | 3.157  | 7      | -      | -    | -    | -        | -    | -      | -    | -                      | -          | -          | -    | -        | -          | -     | 10.059                             | 1.73                        | 3.61                        | 1                     | 23.6                               | 0.82                                 | 4.01                          | 8.883                         | 1.21  | 2.04  | 0.98 | ...  | ...   | 1.27  | 2.25  |
| 08320685-4202502 | 260.688  | -1.393   | 3.176  | 9      | -      | -    | -    | -        | -    | -      | -    | -                      | -          | -          | -    | -        | -          | -     | 11.998                             | ...                         | ...                         | 1                     | 34.8                               | 1.00                                 | 4.01                          | 10.815                        | ...   | ...   | 0.98 | ...  | ...   | ...   | ...   |
| 08320715-4313362 | 261.640  | -2.091   | 10.959 | 9      | -      | -    | -    | -        | -    | -      | -    | -                      | -          | -          | -    | -        | -          | -     | 9.730                              | 1.77                        | 3.58                        | 1                     | 91.4                               | 0.36                                 | 3.92                          | 5.647                         | -0.05 | -1.87 | 3.39 | ...  | ...   | 0.17  | -1.14 |
| 08321296-4204252 | 260.721  | -1.394   | 3.197  | 7      | -      | -    | -    | -        | -    | -      | -    | -                      | -          | -          | -    | -        | -          | -     | 10.821                             | 0.81                        | 1.84                        | 1                     | 49.4                               | 0.60                                 | 3.97                          | 9.630                         | 0.28  | 0.25  | 0.99 | ...  | ...   | 0.34  | 0.46  |
| 08324115-2402317 | 246.151  | 9.307    | 0.107  | 1      | -      | -    | -    | -        | -    | -      | -    | -                      | -          | -          | -    | -        | -          | -     | 10.745                             | 0.37                        | 1.10                        | 1                     | 42.4                               | 0.70                                 | 3.50                          | 10.705                        | 0.35  | 1.04  | 0.03 | 42.6 | 10.71 | 0.35  | 1.05  |
| 08324123-5113345 | 268.178  | -6.730   | 0.959  | 1      | -      | -    | g    | -        | -    | -      | D1   | c                      | cn         | *          | o    | -        | -          | -     | 11.334                             | 0.47                        | 1.60                        | 1                     | 35.0                               | 0.72                                 | 3.72                          | 10.977                        | 0.31  | 1.12  | 0.30 | 38.1 | 10.97 | 0.33  | 1.18  |
| 08342434-3149197 | 252.726  | 5.049    | 0.216  | 1      | -      | -    | g    | -        | t    | -      | D1   | c                      | o          | -          | h    | -        | -          | -     | 10.491                             | 0.23                        | 0.94                        | 1                     | 54.4                               | 0.50                                 | 3.73                          | 10.411                        | 0.20  | 0.83  | 0.07 | 55.0 | 10.42 | 0.20  | 0.84  |
| 08342749-4334516 | 262.177  | -1.960   | 3.380  | 7      | -      | -    | -    | -        | -    | -      | -    | -                      | -          | -          | -    | -        | -          | -     | 11.081                             | 0.92                        | 2.35                        | 1                     | 42.2                               | 0.66                                 | 3.89                          | 9.822                         | 0.36  | 0.68  | 1.05 | ...  | ...   | 0.43  | 0.90  |
| 08343306-4324345 | 262.050  | -1.844   | 3.856  | 8      | -      | -    | -    | -        | -    | -      | -    | -                      | -          | -          | -    | -        | -          | -     | 8.976                              | 1.57                        | 3.49                        | 1                     | 39.2                               | 0.80                                 | 3.90                          | 7.539                         | 0.93  | 1.58  | 1.19 | ...  | ...   | 1.00  | 1.83  |
| 08343417-4324347 | 262.052  | -1.842   | 3.870  | 8      | -      | -    | -    | -        | -    | -      | -    | -                      | -          | -          | -    | -        | -          | -     | 12.269                             | 1.09                        | ...                         | 1                     | 25.8                               | 0.66                                 | 3.90                          | 10.827                        | 0.45  | ...   | 1.20 | ...  | ...   | 0.53  | ...   |
| 08343529-4232037 | 261.352  | -1.316   | 2.965  | 8      | -      | -    | -    | -        | -    | -      | -    | -                      | -          | -          | -    | -        | -          | -     | 11.360                             | 1.33                        | 2.90                        | 1                     | 26.8                               | 0.36                                 | 3.95                          | 10.255                        | 0.84  | 1.43  | 0.92 | ...  | ...   | 0.90  | 1.63  |
| 08344652-5503416 | 271.499  | -8.725   | 0.371  | 1      | -      | -    | g    | -        | -    | -      | D1   | c                      | o          | o          | -    | -        | -          | e?    | 10.463                             | 0.29                        | 1.02                        | 1                     | 46.8                               | 0.88                                 | 3.62                          | 10.325                        | 0.23  | 0.84  | 0.11 | 47.8 | 10.34 | 0.24  | 0.86  |
| 08350348-4926103 | 266.950  | -5.368   | 1.217  | 1      | -      | -    | g    | -        | t    | -      | D1   | c                      | o          | o          | -    | -        | -          | -     | 11.062                             | 0.54                        | 1.48                        | 1                     | 38.8                               | 0.50                                 | 3.78                          | 10.609                        | 0.34  | 0.87  | 0.38 | 42.9 | 10.63 | 0.37  | 0.95  |
| 08350801-2505383 | 247.346  | 9.147    | 0.116  | 1      | -      | -    | g    | -        | -    | -      | D4   | c                      | o          | o          | -    | -        | -          | -     | 11.017                             | 0.34                        | 1.03                        | 1                     | 37.2                               | 0.86                                 | 3.47                          | 10.974                        | 0.32  | 0.98  | 0.04 | 37.4 | 10.98 | 0.32  | 0.98  |
| 08352642-4040437 | 259.962  | -0.077   | 17.569 | 9      | -      | -    | -    | -        | -    | -      | -    | -                      | -          | -          | -    | -        | -          | -     | 9.153                              | 0.84                        | 2.11                        | 1                     | 128.2                              | 0.44                                 | 3.99                          | 2.607                         | -2.07 | -6.62 | 5.44 | ...  | ...   | -1.72 | -5.46 |
| 08352888-4040057 | 259.958  | -0.064   | 19.306 | 8      | -      | -    | -    | -        | -    | -      | -    | -                      | -          | -          | -    | -        | -          | -     | 12.862                             | 0.82                        | 1.61                        | -2                    | 19.2                               | 1.00                                 | 3.99                          | 5.669                         | -2.38 | -7.98 | 5.98 | ...  | ...   | -2.00 | -6.71 |
| 08352952-2420449 | 246.779  | 9.651    | 0.096  | 1      | -      | -    | g    | -        | -    | -      | D2   | c                      | o          | o          | -    | -        | -          | -     | 11.253                             | 0.29                        | 1.00                        | 1                     | 30.0                               | 0.88                                 | 3.50                          | 11.217                        | 0.28  | 0.95  | 0.03 | 30.1 | 11.22 | 0.28  | 0.95  |
| 08353082-4038417 | 259.943  | -0.045   | 18.294 | 9      | -      | -    | -    | -        | -    | -      | -    | -                      | -          | -          | -    | -        | -          | -     | 8.253                              | 1.38                        | 3.46                        | 1                     | 149.2                              | 0.48                                 | 3.99                          | 1.437                         | -1.65 | -5.63 | 5.67 | ...  | ...   | -1.29 | -4.42 |
| 08353425-4042387 | 260.002  | -0.076   | 13.285 | 9      | -      | -    | -    | -        | -    | -      | -    | -                      | -          | -          | -    | -        | -          | -     | 13.619                             | 0.48                        | 1.44                        | -1                    | 19.0                               | 0.44                                 | 3.85                          | 8.669                         | -1.72 | -5.16 | 4.12 | ...  | ...   | -1.46 | -4.28 |
| 08353469-4046217 | 260.052  | -0.112   | 5.811  | 8      | -      | -    | -    | -        | -    | -      | -    | -                      | -          | -          | -    | -        | -          | -     | 12.584                             | 0.64                        | 2.35                        | -2                    | 18.8                               | 0.50                                 | 3.85                          | 10.419                        | -0.32 | -0.53 | 1.80 | ...  | ...   | -0.20 | -0.15 |
| 08354492-4119116 | 260.509  | -0.415   | 2.247  | 1      | -      | -    | g    | -        | t    | P      | D3   | -                      | -          | -          | -    | -        | -          | -     | 10.635                             | 0.59                        | 1.84                        | 1                     | 45.6                               | 0.64                                 | 3.88                          | 9.798                         | 0.21  | 0.72  | 0.70 | 57.8 | 9.78  | 0.26  | 0.87  |
| 08354888-4208138 | 261.170  | -0.896   | 3.596  | 9      | -      | -    | -    | -        | -    | -      | -    | -                      | -          | -          | -    | -        | -          | -     | 12.179                             | 1.52                        | ...                         | 1                     | 24.2                               | 0.80                                 | 3.95                          | 10.839                        | 0.93  | ...   | 1.11 | ...  | ...   | 1.00  | ...   |
| 08361519-2624336 | 248.573  | 8.578    | 0.112  | 1      | -      | -    | g    | -        | -    | -      | D2   | c                      | o          | o          | h    | -        | -          | -     | 9.091                              | 0.27                        | 0.91                        | 1                     | 72.0                               | 0.76                                 | 3.52                          | 9.049                         | 0.25  | 0.86  | 0.03 | 72.2 | 9.06  | 0.25  | 0.86  |
| 08362259-5719336 | 273.491  | -9.871   | 0.184  | 1      | -      | -    | g    | -        | -    | -      | D2   | c                      | o          | o          | -    | -        | -          | -     | 11.152                             | 0.26                        | 1.01                        | 1                     | 34.4                               | 0.66                                 | 3.64                          | 11.083                        | 0.23  | 0.92  | 0.06 | 34.7 | 11.09 | 0.23  | 0.93  |
| 08363186-4306116 | 262.021  | -1.372   | 2.534  | 1      | -      | -    | -    | -        | -    | -      | D1   | -                      | -          | -          | -    | -        | -          | -     | 11.069                             | 0.57                        | 1.82                        | 1                     | 49.4                               | 0.68                                 | 3.99                          | 10.125                        | 0.15  | 0.57  | 0.78 | 67.4 | 10.04 | 0.20  | 0.73  |
| 08363600-4337556 | 262.451  | -1.681   | 2.142  | 1      | -      | -    | -    | -        | -    | -      | D1   | -                      | -          | *          | -    | -        | -          | -     | 11.449                             | 0.63                        | 1.98                        | 1                     | 27.8                               | 0.82                                 | 3.96                          | 10.651                        | 0.27  | 0.92  | 0.66 | 35.2 | 10.61 | 0.31  | 1.06  |
| 08365157-4337407 | 262.476  | -1.641   | 2.208  | 1      | -      | -    | -    | -        | -    | -      | D1   | e                      | -          | -          | h    | -        | -          | -     | 11.181                             | 0.63                        | 2.07                        | 1                     | 35.6                               | 0.40                                 | 3.96                          | 10.358                        | 0.27  | 0.97  | 0.68 | 45.  |       |       |       |

Table B1: a) continued.

| 2MASX J          | <i>l</i>    | <i>b</i>    | EBV        | Object       | Sample     | Disc        | 2MRS        | Velocity   | NIR         | Photom        | Ext         | <i>K</i> <sub>20</sub> | <i>H-K</i>   | <i>J-K</i>  | <i>vc</i>    | <i>a</i>     | <i>b/a</i>   | std.d. | <i>K</i> <sub>S</sub> <sup>o</sup> | ( <i>H-K</i> ) <sup>o</sup> | ( <i>J-K</i> ) <sup>o</sup> | <i>A<sub>K</sub></i> | <i>a</i> <sup>d</sup> | <i>K</i> <sub>S</sub> <sup>d,d</sup> | ( <i>H-K</i> ) <sup>o,c</sup> | ( <i>J-K</i> ) <sup>o,c</sup> |             |             |           |             |             |             |       |
|------------------|-------------|-------------|------------|--------------|------------|-------------|-------------|------------|-------------|---------------|-------------|------------------------|--------------|-------------|--------------|--------------|--------------|--------|------------------------------------|-----------------------------|-----------------------------|----------------------|-----------------------|--------------------------------------|-------------------------------|-------------------------------|-------------|-------------|-----------|-------------|-------------|-------------|-------|
| (1)              | deg<br>(2a) | deg<br>(2b) | mag<br>(3) | class<br>(4) | off<br>(5) | flag<br>(6) | gal<br>(7a) | TF<br>(7b) | obs<br>(7c) | ext'd<br>(7d) | type<br>(8) | (9)                    | Opt<br>(10a) | HI<br>(10b) | flag<br>(11) | flag<br>(12) | flag<br>(13) | (14)   | mag<br>(15)                        | mag<br>(16)                 | (17)                        | (18)                 | (19)                  | (20)                                 | mag<br>(21)                   | mag<br>(22)                   | mag<br>(23) | mag<br>(24) | "<br>(25) | mag<br>(26) | mag<br>(27) | mag<br>(28) |       |
| 08433295-4050420 | 261.029     | 1.040       | 3.835      | 9            | -          | -           | -           | -          | -           | -             | -           | -                      | -            | -           | -            | -            | -            | -      | 12.152                             | 1.66                        | ...                         | 1                    | 31.4                  | 0.78                                 | 3.80                          | 10.723                        | 1.02        | ...         | 1.19      | ...         | ...         | 1.10        | ...   |
| 08433358-4823085 | 266.960     | -3.621      | 1.209      | 3            | -          | -           | g           | t          | P           | -             | n           | -                      | -            | -           | -            | -            | -            | -      | 11.671                             | 0.44                        | 1.29                        | 1                    | 35.2                  | 0.42                                 | 3.99                          | 11.221                        | 0.24        | 0.69        | 0.37      | 39.3        | 11.22       | 0.27        | 0.77  |
| 08435200-4242339 | 262.530     | -0.068      | 2.942      | 9            | -          | -           | -           | -          | -           | -             | -           | -                      | -            | -           | -            | -            | -            | -      | 12.262                             | 0.80                        | 2.29                        | 2                    | 15.2                  | ...                                  | 3.91                          | ...                           | 0.31        | 0.83        | 0.91      | ...         | ...         | ...         |       |
| 08435749-4338260 | 263.271     | -0.632      | 2.951      | 1            | -          | -           | g           | -          | P           | -             | D1          | -                      | -            | -           | -            | -            | e?           | 11.907 | 0.68                               | 1.19                        | 1                           | 12.8                 | 0.82                  | 3.93                                 | 10.807                        | 0.19                          | 0.73        | 0.91        | 18.6      | 10.70       | ...         | 0.25        | 0.92  |
| 08440059-4116412 | 261.423     | 0.840       | 13.050     | 8            | -          | -           | -           | -          | -           | -             | -           | -                      | -            | -           | -            | -            | -            | -      | 11.576                             | 1.30                        | 3.27                        | 1                    | 23.2                  | 0.54                                 | 3.86                          | 6.714                         | -0.86       | -3.22       | 4.04      | ...         | ...         | -0.61       | -2.36 |
| 08440269-4059382 | 261.204     | 1.021       | 7.999      | 9            | -          | -           | -           | -          | -           | -             | -           | -                      | -            | -           | -            | -            | -            | -      | 13.190                             | 0.69                        | 1.93                        | -1                   | 16.8                  | 1.00                                 | 3.81                          | 10.210                        | -0.64       | -2.04       | 2.48      | ...         | ...         | -0.48       | -1.52 |
| 08440715-4116212 | 261.431     | 0.859       | 12.682     | 8            | -          | -           | -           | -          | -           | -             | -           | -                      | -            | -           | -            | -            | -            | -      | 11.526                             | 1.13                        | 2.35                        | -2                   | 43.0                  | 0.72                                 | 3.86                          | 6.801                         | -0.97       | -3.95       | 3.93      | ...         | ...         | -0.72       | -3.12 |
| 08440766-4135302 | 261.683     | 0.663       | 5.353      | 3            | -          | -           | g           | t          | P           | -             | D3          | -                      | -            | -           | e            | -            | -            | -      | 12.701                             | 0.86                        | 2.35                        | -1                   | 18.0                  | 0.46                                 | 3.81                          | 10.706                        | -0.03       | -0.32       | 1.66      | 40.9        | 10.37       | 0.07        | 0.03  |
| 08440895-4116162 | 261.434     | 0.865       | 12.518     | 9            | -          | -           | -           | -          | -           | -             | -           | -                      | -            | -           | -            | -            | -            | -      | 11.242                             | 0.91                        | 1.95                        | -2                   | 50.0                  | 0.64                                 | 4.10                          | 6.578                         | -1.17       | -4.27       | 3.88      | ...         | ...         | -0.92       | -3.45 |
| 08441071-4117212 | 261.451     | 0.858       | 11.828     | 9            | -          | -           | -           | -          | -           | -             | -           | -                      | -            | -           | -            | -            | -            | -      | 12.937                             | 1.09                        | ...                         | 1                    | 19.8                  | 1.00                                 | 3.86                          | 8.530                         | -0.87       | ...         | 3.66      | ...         | ...         | -0.64       | ...   |
| 08441291-3612532 | 257.407     | 4.005       | 0.506      | 1            | -          | -           | g           | t          | N           | -             | D1          | -                      | -            | -           | -            | -            | -            | -      | 11.147                             | 0.39                        | 1.26                        | 1                    | 45.0                  | 0.40                                 | 3.70                          | 10.958                        | 0.30        | 1.01        | 0.16      | 46.7        | 10.96       | 0.31        | 1.04  |
| 08441299-5112594 | 269.262     | -5.282      | 0.943      | 1            | -          | -           | g           | -          | P           | -             | D1          | c                      | o            | -           | -            | -            | -            | -      | 11.547                             | 0.44                        | 1.42                        | 1                    | 35.0                  | 0.72                                 | 3.88                          | 11.196                        | 0.28        | 0.95        | 0.29      | 38.3        | 11.18       | 0.30        | 1.01  |
| 08442202-3441387 | 256.286     | 4.969       | 0.352      | 1            | -          | -           | g           | -          | -           | -             | D1          | c                      | o            | h           | -            | -            | V            | -      | 10.512                             | 0.36                        | 1.19                        | 1                    | 38.4                  | 0.58                                 | 3.67                          | 10.381                        | 0.30        | 1.01        | 0.11      | 39.1        | 10.39       | 0.31        | 1.03  |
| 08442894-3141307 | 253.922     | 6.835       | 0.257      | 1            | -          | -           | g           | -          | -           | -             | D2          | cp                     | o            | -           | -            | -            | V            | p      | 6.756                              | 0.57                        | 1.11                        | 1                    | 78.0                  | 0.76                                 | 3.54                          | 6.660                         | 0.53        | 0.98        | 0.08      | 78.8        | 6.67        | 0.54        | 1.00  |
| 08444188-4311480 | 263.006     | -0.251      | 3.241      | 8            | -          | -           | -           | -          | -           | -             | -           | -                      | -            | -           | -            | -            | -            | -      | 11.962                             | 1.43                        | 2.86                        | 1                    | 16.8                  | 0.62                                 | 3.93                          | 10.754                        | 0.89        | 1.25        | 1.00      | ...         | ...         | 0.96        | 1.46  |
| 08444203-5704363 | 273.971     | -8.819      | 0.205      | 1            | -          | -           | g           | t          | N           | -             | D3          | c                      | o            | -           | -            | -            | -            | -      | 11.243                             | 0.33                        | 1.10                        | 1                    | 33.2                  | 0.86                                 | 3.66                          | 11.167                        | 0.30        | 0.99        | 0.06      | 33.5        | 11.17       | 0.30        | 1.01  |
| 08450592-3120222 | 253.723     | 7.155       | 0.254      | 1            | -          | -           | g           | t          | P           | -             | D1          | c                      | o            | *           | -            | -            | V            | -      | 10.560                             | 0.23                        | 0.95                        | 1                    | 63.4                  | 0.48                                 | 3.50                          | 10.465                        | 0.18        | 0.82        | 0.08      | 64.2        | 10.47       | 0.19        | 0.84  |
| 08450680-4302101 | 262.928     | -0.092      | 2.760      | 1            | o          | -           | g           | t          | P           | -             | D1          | c                      | o            | -           | -            | -            | o            | e      | 11.864                             | 0.75                        | 2.15                        | 1                    | 41.4                  | 0.36                                 | 3.86                          | 10.836                        | 0.29        | 0.78        | 0.85      | 60.2        | 10.68       | 0.35        | 0.96  |
| 08450824-3347411 | 255.674     | 5.649       | 0.360      | 1            | -          | -           | g           | -          | -           | -             | D3          | c                      | o            | -           | -            | -            | V            | -      | 6.921                              | 0.30                        | 1.05                        | 1                    | 210.8                 | 0.77                                 | ...                           | 6.787                         | 0.24        | 0.87        | 0.11      | ...         | ...         | 0.25        | 0.90  |
| 08451082-3354402 | 255.772     | 5.584       | 0.341      | 1            | -          | -           | g           | -          | -           | -             | D4          | c                      | o            | -           | -            | -            | V            | -      | 11.110                             | 0.30                        | 1.01                        | 1                    | 42.8                  | 0.54                                 | 3.64                          | 10.983                        | 0.24        | 0.84        | 0.11      | 43.7        | 10.99       | 0.25        | 0.86  |
| 08451761-4535292 | 264.948     | -1.657      | 1.661      | 1            | -          | -           | g           | t          | P           | -             | D1          | -                      | -            | -           | -            | -            | e?           | 11.371 | 0.49                               | 1.64                        | 1                           | 50.8                 | 0.34                  | 4.02                                 | 10.752                        | 0.21                          | 0.82        | 0.51        | 59.9      | 10.75       | 0.24        | 0.93        |       |
| 08452081-4114551 | 261.556     | 1.055       | 8.201      | 8            | -          | -           | -           | -          | -           | -             | -           | -                      | -            | -           | -            | -            | -            | -      | 10.571                             | 1.07                        | 2.62                        | 1                    | 55.6                  | 0.34                                 | 3.94                          | 7.515                         | -0.28       | -1.82       | 2.54      | ...         | ...         | -0.12       | -1.28 |
| 08452168-4218462 | 262.390     | 0.394       | 3.101      | 1            | -          | -           | g           | -          | -           | -             | D1          | -                      | -            | -           | h            | -            | e            | 9.705  | 0.50                               | 2.45                        | 1                           | 86.0                 | 0.84                  | 3.82                                 | 8.550                         | -0.01                         | 0.91        | 0.96        | 129.2     | 8.42        | 0.05        | 1.12        |       |
| 08452198-4114467 | 261.556     | 1.059       | 8.341      | 8            | -          | -           | -           | -          | -           | -             | -           | -                      | -            | -           | -            | -            | -            | -      | 9.985                              | 0.99                        | 2.08                        | 1                    | 78.6                  | 0.60                                 | 3.91                          | 6.877                         | -0.39       | -2.06       | 2.58      | ...         | ...         | -0.22       | -1.51 |
| 08452391-4115061 | 261.564     | 1.061       | 8.262      | 8            | -          | -           | -           | -          | -           | -             | -           | -                      | -            | -           | -            | -            | -            | -      | 11.590                             | 1.08                        | 2.73                        | 1                    | 25.6                  | 0.82                                 | 4.05                          | 8.512                         | -0.29       | -1.38       | 2.56      | ...         | ...         | -0.13       | -0.83 |
| 08452535-4114428 | 261.562     | 1.068       | 8.544      | 8            | -          | -           | -           | -          | -           | -             | -           | -                      | -            | -           | -            | -            | -            | -      | 11.274                             | 1.55                        | 3.30                        | 1                    | 25.2                  | 0.74                                 | 3.91                          | 8.091                         | 0.14        | -0.95       | 2.65      | ...         | ...         | 0.30        | -0.38 |
| 08452558-3942278 | 260.359     | 2.026       | 1.840      | 1            | -          | -           | g           | -          | P           | -             | D3          | -                      | -            | -           | -            | -            | -            | -      | 11.490                             | 0.55                        | 1.85                        | 1                    | 25.6                  | 0.88                                 | 3.81                          | 10.804                        | 0.25        | 0.93        | 0.57      | 30.9        | 10.79       | 0.28        | 1.05  |
| 08453348-4350561 | 263.614     | -0.535      | 14.211     | 9            | -          | -           | -           | -          | -           | -             | -           | -                      | -            | -           | -            | -            | -            | -      | 9.605                              | 1.20                        | 2.39                        | 1                    | 116.4                 | 0.26                                 | 3.99                          | 4.310                         | -1.15       | -4.67       | 4.40      | ...         | ...         | -0.87       | -3.73 |
| 08453358-4352241 | 263.633     | -0.550      | 12.260     | 8            | -          | -           | -           | -          | -           | -             | -           | -                      | -            | -           | -            | -            | -            | -      | 11.059                             | 1.31                        | 3.52                        | 1                    | 28.6                  | 0.68                                 | 3.99                          | 6.491                         | -0.72       | -2.57       | 3.80      | ...         | ...         | -0.48       | -1.77 |
| 08453403-4350191 | 263.607     | -0.527      | 13.815     | 9            | -          | -           | -           | -          | -           | -             | -           | -                      | -            | -           | -            | -            | -            | -      | 9.105                              | 1.02                        | ...                         | 1                    | 219.4                 | 0.58                                 | 3.99                          | 3.958                         | -1.27       | ...         | 4.28      | ...         | ...         | -1.00       | ...   |
| 08453663-4353091 | 263.649     | -0.551      | 9.880      | 9            | -          | -           | -           | -          | -           | -             | -           | -                      | -            | -           | -            | -            | -            | -      | 12.551                             | 0.91                        | ...                         | -2                   | 16.8                  | 1.00                                 | 3.99                          | 8.870                         | -0.72       | ...         | 3.06      | ...         | ...         | -0.53       | ...   |
| 08453718-4351421 | 263.631     | -0.534      | 13.083     | 9            | -          | -           | -           | -          | -           | -             | -           | -                      | -            | -           | -            | -            | -            | -      | 11.488                             | 1.35                        | 2.88                        | 1                    | 45.2                  | 0.58                                 | 3.99                          | 6.613                         | -0.82       | -3.62       | 4.05      | ...         | ...         | -0.56       | -2.76 |
| 08453742-5101365 | 269.249     | -4.991      | 1.123      | 1            | -          | -           | g           | t          | P           | -             | D1          | -                      | -            | -           | -            | -            | -            | -      | 11.545                             | 0.56                        | 1.61                        | 1                    | 30.8                  | 0.48                                 | 3.87                          | 11.127                        | 0.37        | 1.05        | 0.35      | 34.0        | 11.13       | 0.39        | 1.13  |
| 08453957-4350584 | 263.626     | -0.521      | 14.177     | 9            | -          | -           | -           | -          | -           | -             | -           | -                      | -            | -           | -            | -            | -            | -      | 9.291                              | 1.05                        | 1.74                        | 1                    | 138.2                 | 0.48                                 | 3.99                          | 4.009                         | -1.30       | -5.30       | 4.39      | ...         | ...         | -1.02       | -4.37 |
| 08454014-4351001 | 263.627     | -0.520      | 14.066     | 9            | -          | -           | -           | -          | -           | -             | -           | -                      | -            | -           | -            | -            | -            | -      | 9.351                              | 1.56                        | 2.19                        | 1                    | 89.2                  | 0.92                                 | 3.99                          | 4.110                         | -0.77       | -4.80       | 4.36      | ...         | ...         | -0.50       | -3.87 |
| 08454917-4353185 | 263.674     | -0.523      | 9.154      | 9            | -          | -           | -           | -          | -           | -             | -           | -                      | -            | -           | -            | -            | -            | -      | 13.199                             | ...                         | ...                         | 1                    | 18.6                  | 0.38                                 | 3.99                          | 9.788                         | ...         | ...         | 2.84      | ...         | ...         | ...         | ...   |
| 08460211-4109109 | 261.562     | 1.216       | 7.044      | 8            | -          | -           | -           | -          | -           | -             | -           | -                      | -            | -           | -            | -            | -            | -      | 13.651                             | ...                         | ...                         | -1                   | 11.6                  | 1.00                                 | 3.78                          | 11.026                        | ...         | ...         | 2.18      | ...         | ...         | ...         | ...   |
| 08461212-4323086 | 263.325     | -0.155      | 3.975      | 9            | -          | -           | -           | -          | -           | -             | -           | -                      | -            | -           | -            | -            | -            | -      | 9.822                              | 2.08                        | 4.28                        | 1                    | 29.2                  | 0.74                                 | 3.80                          | 8.341                         | 1.42        | 2.30        | 2.13      | ...         | ...         | 1.50        | 2.57  |
| 08462640-4342405 | 263.606     | -0.325      | 3.500      | 7            | -          | -           | -           | -          | -           | -             | -           | -                      | -            | -           | -            | -            | -            | -      | 11.439                             | 1.06                        | 2.65                        | 1                    | 36.2                  | 0.78                                 | 4.00                          | 10.135                        | 0.48        | 0.91        | 1.08      | ...         | ...         | 0.55        | 1.14  |
| 08463458-4354265 | 263.774     | -0.428      | 8.527      | 8            | -          | -           | -           | -          | -           | -             | -           | -                      | -            | -           | -            | -            | -            | -      | 8.187                              | 1.60                        | 3.34                        | 1                    | 91.6                  | 0.82                                 | 4.00                          | 5.010                         | 0.19        | -0.89       | 2.64      | ...         | ...         | 0.36        | -0.33 |
| 08463875-4353196 | 263.768     | -0.407      | 8.698      | 9            | -          | -           | -           | -          | -           | -             | -           | -                      | -            | -           | -            | -            | -            | -      | 10.434                             | 0.91                        | 2.42                        | -2                   | 73.0                  | 0.66                                 | 4.00                          | 7.193                         | -0.53       | -1.91       | 2.69      | ...         | ...         | -0.36       | -1.33 |
| 08470542-3345507 | 255.903     | 5.986       | 0.388      | 1            | -          | -           | g           | -          | -           | -             | D1          | c                      | o            | h           | -            | -            | V            | -      | 8.338                              | 0.29                        | 1.05                        | 1                    | 219.8                 | 0.60                                 | 3.56                          | 8.193                         | 0.22        | 0.86        | 0.12      | 224.4       | 8.21        | 0.23        | 0.88  |
| 08471717-4253030 | 263.058     | 0.314       | 2.088      | 8            | -          | -           | -           | -          | -           | -             | -           | -                      | -            | -           | -            | -            | -            | -      | 12.019                             | 0.46                        | 1.78                        | -2                   | 15.6                  | 0.72                                 | 3.86                          | 11.241                        | 0.12        | 0.75        | 0.65      | ...         | ...         | 0.16        | 0.88  |
| 08471978-3320011 | 255.595     | 6.293       | 0.354      | 1            | o          | -           | g           | t          | N           | -             | D3          | c                      | o            | -           | -            | -            | V            | o      | 10.581                             | 0.35                        | 1.68                        | -2                   | 96.8                  | 0.38                                 | 3.62                          | 10.449                        | 0.29        | 1.50        | 0.11      | 99.6        | 10.44       | 0.30        | 1.53  |
| 08472534-4348560 | 263.798     | -0.252      | 4.046      | 8            | -          | -           | -           | -          | -           | -             | -           | -                      | -            | -           | -            | -            | -            | -      | 11.827                             | 1.45                        | ...                         | 1                    | 12.6                  | 0.56                                 | 3.96                          | 10.319                        | 0.78</      |             |           |             |             |             |       |

Table B1: a) continued.

70

| 2MASX J          | <i>l</i> | <i>b</i> | EBV    | Object | Sample | Disc | 2MRS | Velocity | NIR  | Photom | Ext  | <i>K</i> <sub>20</sub> | <i>H-K</i> | <i>J-K</i> | vc   | <i>a</i> | <i>b/a</i> | st.d. | <i>K</i> <sub>s</sub> <sup>o</sup> | ( <i>H-K</i> ) <sup>o</sup> | ( <i>J-K</i> ) <sup>o</sup> | <i>A</i> <sub>K</sub> | <i>a</i> <sub>d</sub> <sup>o</sup> | <i>K</i> <sub>s</sub> <sup>o,d</sup> | ( <i>H-K</i> ) <sup>o,c</sup> | ( <i>J-K</i> ) <sup>o,c</sup> |       |       |      |       |       |       |       |
|------------------|----------|----------|--------|--------|--------|------|------|----------|------|--------|------|------------------------|------------|------------|------|----------|------------|-------|------------------------------------|-----------------------------|-----------------------------|-----------------------|------------------------------------|--------------------------------------|-------------------------------|-------------------------------|-------|-------|------|-------|-------|-------|-------|
| (1)              | deg      | deg      | mag    | class  | off    | flag | gal  | TF       | obs  | ext'd  | type | (8)                    | (9)        | Opt        | HI   | (10b)    | flag       | flag  | flag                               | mag                         | mag                         | mag                   | mag                                | mag                                  | mag                           | mag                           | mag   |       |      |       |       |       |       |
| (1)              | (2a)     | (2b)     | (3)    | (4)    | (5)    | (6)  | (7a) | (7b)     | (7c) | (7d)   | (8)  | (9)                    | (10a)      | (10b)      | (11) | (12)     | (13)       | (14)  | (15)                               | (16)                        | (17)                        | (18)                  | (19)                               | (20)                                 | (21)                          | (22)                          | (23)  | (24)  | (25) | (26)  | (27)  | (28)  |       |
| 08504233-4906408 | 268.265  | -3.155   | 2.953  | 8      | -      | -    | -    | -        | -    | -      | -    | -                      | -          | -          | -    | -        | -          | -     | 12.239                             | 1.53                        | ...                         | 1                     | 27.4                               | 0.26                                 | 4.01                          | 11.139                        | 1.05  | ...   | 0.91 | ...   | ...   | 1.10  | ...   |
| 08505602-3432152 | 257.010  | 6.122    | 0.329  | 1      | -      | -    | -    | -        | -    | -      | -    | -                      | -          | -          | -    | -        | -          | -     | 9.130                              | 0.30                        | 1.01                        | 1                     | 164.6                              | 0.24                                 | 3.61                          | 9.007                         | 0.24  | 0.84  | 0.10 | 168.1 | 9.01  | 0.25  | 0.87  |
| 08510132-4128318 | 262.403  | 1.740    | 1.653  | 1      | -      | -    | -    | -        | -    | -      | -    | -                      | -          | -          | -    | -        | -          | -     | 11.408                             | 0.48                        | 1.58                        | 1                     | 35.2                               | 0.38                                 | 3.89                          | 10.792                        | 0.21  | 0.75  | 0.51 | 41.6  | 10.78 | 0.24  | 0.86  |
| 08510970-3505361 | 257.473  | 5.808    | 0.378  | 1      | -      | -    | -    | -        | -    | -      | -    | -                      | -          | -          | -    | -        | -          | -     | 10.887                             | 0.23                        | 0.96                        | 1                     | 40.2                               | 0.68                                 | 3.61                          | 10.746                        | 0.16  | 0.77  | 0.12 | 41.0  | 10.76 | 0.17  | 0.80  |
| 08511339-4146478 | 262.661  | 1.575    | 1.729  | 1      | -      | -    | -    | -        | -    | -      | -    | -                      | -          | -          | -    | -        | -          | -     | 10.426                             | 0.55                        | 1.67                        | 1                     | 44.2                               | 0.80                                 | 3.93                          | 9.782                         | 0.26  | 0.81  | 0.54 | 51.8  | 9.80  | 0.30  | 0.92  |
| 08512388-4250218 | 263.499  | 0.926    | 4.092  | 8      | -      | -    | -    | -        | -    | -      | -    | -                      | -          | -          | -    | -        | -          | -     | 12.084                             | 1.35                        | 2.64                        | -2                    | 27.8                               | 1.00                                 | 3.94                          | 10.559                        | 0.67  | 0.61  | 1.27 | ...   | ...   | 0.75  | 0.88  |
| 08512406-4250078 | 263.497  | 0.929    | 4.100  | 7      | -      | -    | -    | -        | -    | -      | -    | -                      | -          | -          | -    | -        | -          | -     | 12.032                             | 1.20                        | ...                         | 1                     | 25.8                               | 0.66                                 | 3.94                          | 10.504                        | 0.53  | ...   | 1.27 | ...   | ...   | 0.61  | ...   |
| 08512960-4833077 | 267.915  | -2.700   | 0.729  | 1      | -      | -    | -    | -        | -    | -      | -    | -                      | -          | -          | -    | -        | -          | -     | 10.851                             | 0.58                        | 1.63                        | 1                     | 53.2                               | 0.32                                 | 4.06                          | 10.579                        | 0.46  | 1.27  | 0.23 | 56.1  | 10.59 | 0.47  | 1.32  |
| 08513903-4628040 | 266.324  | -1.352   | 1.923  | 2      | -      | -    | -    | -        | -    | -      | -    | -                      | -          | -          | -    | -        | -          | -     | 11.622                             | 0.50                        | 1.79                        | 1                     | 26.4                               | 0.60                                 | 4.08                          | 10.905                        | 0.18  | 0.83  | 0.60 | 32.1  | 10.90 | 0.22  | 0.96  |
| 08514922-4305300 | 263.743  | 0.824    | 2.559  | 7      | -      | -    | -    | -        | -    | -      | -    | -                      | -          | -          | -    | -        | -          | -     | 11.075                             | 0.89                        | 1.94                        | 1                     | 38.2                               | 0.72                                 | 3.89                          | 10.122                        | 0.46  | 0.67  | 0.79 | ...   | ...   | 0.51  | 0.84  |
| 08515810-4625361 | 266.328  | -1.284   | 1.904  | 1      | -      | -    | -    | -        | -    | -      | -    | -                      | -          | -          | -    | -        | -          | -     | 10.117                             | 0.52                        | 1.65                        | 1                     | 57.6                               | 0.62                                 | 4.08                          | 9.408                         | 0.20  | 0.71  | 0.59 | 68.0  | 9.44  | 0.24  | 0.83  |
| 08521238-3040129 | 254.149  | 8.764    | 0.258  | 1      | -      | -    | -    | -        | -    | -      | -    | -                      | -          | -          | -    | -        | -          | -     | 11.233                             | 0.30                        | 1.16                        | 1                     | 32.0                               | 0.76                                 | 3.50                          | 11.137                        | 0.26  | 1.03  | 0.08 | 32.4  | 11.15 | 0.26  | 1.05  |
| 08522514-4846090 | 268.180  | -2.720   | 2.885  | 8      | -      | -    | -    | -        | -    | -      | -    | -                      | -          | -          | -    | -        | -          | -     | 11.966                             | 0.73                        | 2.25                        | -2                    | 33.8                               | 0.64                                 | 4.02                          | 10.891                        | 0.26  | 0.82  | 0.89 | ...   | ...   | 0.31  | 1.01  |
| 08522527-3926038 | 260.997  | 3.245    | 0.973  | 1      | -      | -    | -    | -        | -    | -      | -    | -                      | -          | -          | -    | -        | -          | -     | 10.977                             | 0.53                        | 1.54                        | 1                     | 42.6                               | 0.54                                 | 3.80                          | 10.614                        | 0.37  | 1.06  | 0.30 | 46.6  | 10.61 | 0.39  | 1.12  |
| 08523283-4850530 | 268.255  | -2.755   | 2.111  | 7      | o      | -    | -    | -        | -    | -      | -    | -                      | -          | -          | -    | -        | -          | -     | 11.657                             | 0.99                        | 2.13                        | 1                     | 30.4                               | 0.68                                 | 4.02                          | 10.870                        | 0.64  | 1.09  | 0.65 | ...   | ...   | 0.68  | 1.22  |
| 08525391-4413031 | 264.733  | 0.255    | 5.012  | 9      | -      | -    | -    | -        | -    | -      | -    | -                      | -          | -          | -    | -        | -          | -     | 12.396                             | 0.67                        | 1.56                        | -2                    | 24.4                               | 1.00                                 | 3.99                          | 10.529                        | -0.16 | -0.93 | 1.55 | ...   | ...   | -0.06 | -0.60 |
| 08525604-4412402 | 264.733  | 0.264    | 5.042  | 9      | -      | -    | -    | -        | -    | -      | -    | -                      | -          | -          | -    | -        | -          | -     | 12.195                             | 0.64                        | 1.56                        | -2                    | 36.2                               | 0.70                                 | 3.99                          | 10.316                        | -0.20 | -0.94 | 1.56 | ...   | ...   | -0.10 | -0.61 |
| 08525870-5032384 | 269.606  | -3.784   | 1.745  | 7      | -      | -    | -    | -        | -    | -      | -    | -                      | -          | -          | -    | -        | -          | -     | 11.161                             | 1.49                        | 3.16                        | 1                     | 21.8                               | 0.84                                 | 3.95                          | 10.511                        | 1.20  | 2.29  | 0.54 | ...   | ...   | 1.24  | 2.41  |
| 08530933-4213052 | 263.228  | 1.572    | 6.038  | 9      | -      | -    | -    | -        | -    | -      | -    | -                      | -          | -          | -    | -        | -          | -     | 9.483                              | 1.33                        | 2.59                        | 1                     | 73.6                               | 0.66                                 | 3.83                          | 7.233                         | 0.33  | -0.41 | 1.87 | ...   | ...   | 0.45  | -0.01 |
| 08530969-4213342 | 263.235  | 1.567    | 5.796  | 8      | -      | -    | -    | -        | -    | -      | -    | -                      | -          | -          | -    | -        | -          | -     | 10.699                             | 1.19                        | 2.93                        | 1                     | 41.6                               | 0.16                                 | 3.83                          | 8.539                         | 0.23  | 0.05  | 1.80 | ...   | ...   | 0.35  | 0.43  |
| 08531045-4544263 | 265.934  | -0.684   | 2.669  | 2      | -      | -    | -    | -        | -    | -      | -    | -                      | -          | -          | -    | -        | -          | -     | 12.197                             | 0.91                        | 2.37                        | 1                     | 27.4                               | 0.46                                 | 3.99                          | 11.203                        | 0.47  | 1.05  | 0.83 | 39.1  | 11.07 | 0.52  | 1.23  |
| 08531482-4214333 | 263.258  | 1.569    | 5.273  | 9      | -      | -    | -    | -        | -    | -      | -    | -                      | -          | -          | -    | -        | -          | -     | 10.322                             | 0.82                        | 2.10                        | 1                     | 56.8                               | 0.84                                 | 3.83                          | 8.357                         | -0.06 | -0.52 | 1.63 | ...   | ...   | 0.05  | -0.17 |
| 08532482-4215292 | 263.289  | 1.583    | 4.352  | 8      | -      | -    | -    | -        | -    | -      | -    | -                      | -          | -          | -    | -        | -          | -     | 11.645                             | 2.08                        | ...                         | 1                     | 28.8                               | 0.34                                 | 3.83                          | 10.023                        | 1.36  | ...   | 1.35 | ...   | ...   | 1.45  | ...   |
| 08532984-5913016 | 276.400  | -9.234   | 0.276  | 1      | -      | -    | -    | -        | -    | -      | -    | -                      | -          | -          | -    | -        | -          | -     | 8.916                              | 0.28                        | 1.05                        | 1                     | 84.2                               | 0.92                                 | 3.70                          | 8.813                         | 0.23  | 0.91  | 0.09 | 85.2  | 8.83  | 0.24  | 0.93  |
| 08533113-4003487 | 261.617  | 3.005    | 1.523  | 9      | o      | p?   | -    | -        | -    | -      | -    | -                      | -          | -          | -    | -        | -          | -     | 11.172                             | 1.02                        | 1.50                        | 1                     | 37.4                               | 0.54                                 | 3.76                          | 10.605                        | 0.77  | 0.74  | 0.47 | ...   | ...   | 0.80  | 0.84  |
| 08533724-4217109 | 263.336  | 1.594    | 2.945  | 8      | -      | -    | -    | -        | -    | -      | -    | -                      | -          | -          | -    | -        | -          | -     | 11.199                             | 1.50                        | 3.29                        | 1                     | 34.8                               | 0.40                                 | 3.79                          | 10.102                        | 1.01  | 1.83  | 0.91 | ...   | ...   | 1.07  | 2.02  |
| 08534593-4424110 | 264.975  | 0.255    | 3.085  | 9      | -      | -    | -    | -        | -    | -      | -    | -                      | -          | -          | -    | -        | -          | -     | 11.422                             | 0.62                        | 1.75                        | -2                    | 54.2                               | 0.86                                 | 3.93                          | 10.273                        | 0.11  | 0.22  | 0.96 | ...   | ...   | 0.17  | 0.42  |
| 08541840-5032231 | 269.738  | -3.619   | 1.361  | 9      | -      | p    | -    | -        | -    | -      | -    | -                      | -          | -          | -    | -        | -          | -     | 11.661                             | 0.93                        | 1.12                        | 1                     | 14.0                               | 0.96                                 | 4.01                          | 11.154                        | 0.70  | 0.44  | 0.42 | ...   | ...   | 0.73  | 0.53  |
| 08541996-4057473 | 262.407  | 2.546    | 1.249  | 2      | -      | -    | -    | -        | -    | -      | -    | -                      | -          | -          | -    | -        | -          | -     | 11.691                             | 0.49                        | 1.55                        | 1                     | 22.2                               | 0.96                                 | 3.80                          | 11.226                        | 0.28  | 0.93  | 0.39 | 25.0  | 11.22 | 0.31  | 1.01  |
| 08543250-3256149 | 256.241  | 7.716    | 0.309  | 1      | -      | -    | -    | -        | -    | -      | -    | -                      | -          | -          | -    | -        | -          | -     | 8.712                              | 0.29                        | 1.05                        | 1                     | 131.8                              | 0.32                                 | ...                           | 8.597                         | 0.24  | 0.90  | 0.10 | ...   | ...   | 0.24  | 0.92  |
| 08544096-5156462 | 270.857  | -4.477   | 1.755  | 3      | -      | -    | -    | -        | -    | -      | -    | -                      | -          | -          | -    | -        | -          | -     | 11.882                             | 0.68                        | 1.46                        | 1                     | 25.2                               | 0.58                                 | 3.91                          | 11.228                        | 0.39  | 0.59  | 0.54 | 31.4  | 11.14 | 0.42  | 0.70  |
| 08545131-4206151 | 263.343  | 1.886    | 1.609  | 1      | -      | -    | -    | -        | -    | -      | -    | -                      | -          | -          | -    | -        | -          | -     | 11.741                             | 0.52                        | 1.66                        | 1                     | 31.0                               | 0.40                                 | 3.83                          | 11.141                        | 0.26  | 0.86  | 0.50 | 37.0  | 11.10 | 0.29  | 0.97  |
| 08545431-5143502 | 270.714  | -4.312   | 1.641  | 1      | -      | -    | -    | -        | -    | -      | -    | -                      | -          | -          | -    | -        | -          | -     | 10.933                             | 0.52                        | 1.73                        | 1                     | 41.4                               | 0.78                                 | 3.92                          | 10.322                        | 0.24  | 0.92  | 0.51 | 48.6  | 10.32 | 0.28  | 1.03  |
| 08545445-4609091 | 266.443  | -0.718   | 2.251  | 9      | -      | -    | -    | -        | -    | -      | -    | -                      | -          | -          | -    | -        | -          | -     | 11.657                             | 1.63                        | ...                         | 1                     | 50.8                               | 0.84                                 | 3.91                          | 10.818                        | 1.26  | ...   | 0.70 | ...   | ...   | 1.30  | ...   |
| 08545724-5855087 | 276.286  | -8.900   | 0.305  | 1      | -      | -    | -    | -        | -    | -      | -    | -                      | -          | -          | -    | -        | -          | -     | 10.849                             | 0.27                        | 1.06                        | 1                     | 48.2                               | 0.62                                 | 3.68                          | 10.735                        | 0.22  | 0.91  | 0.09 | 49.0  | 10.74 | 0.23  | 0.93  |
| 08545840-5143461 | 270.720  | -4.304   | 1.640  | 1      | -      | -    | -    | -        | -    | -      | -    | -                      | -          | -          | -    | -        | -          | -     | 11.424                             | 0.44                        | 1.67                        | 1                     | 31.2                               | 0.82                                 | 3.92                          | 10.813                        | 0.17  | 0.85  | 0.51 | 36.6  | 10.81 | 0.20  | 0.96  |
| 08550711-4429242 | 265.197  | 0.383    | 2.548  | 7      | -      | -    | -    | -        | -    | -      | -    | -                      | -          | -          | -    | -        | -          | -     | 11.694                             | 0.93                        | 2.23                        | 1                     | 44.0                               | 0.60                                 | 3.90                          | 10.745                        | 0.51  | 0.96  | 0.79 | ...   | ...   | 0.56  | 1.13  |
| 08551298-4313052 | 264.238  | 1.218    | 1.986  | 8      | -      | -    | -    | -        | -    | -      | -    | -                      | -          | -          | -    | -        | -          | -     | 11.946                             | 1.11                        | 2.44                        | 1                     | 48.8                               | 0.80                                 | 3.86                          | 11.206                        | 0.78  | 1.45  | 0.62 | ...   | ...   | 0.82  | 1.58  |
| 08551578-3202478 | 255.645  | 8.400    | 0.341  | 1      | -      | -    | -    | -        | -    | -      | -    | -                      | -          | -          | -    | -        | -          | -     | 9.999                              | 0.27                        | 1.03                        | 1                     | 93.2                               | 0.34                                 | 3.49                          | 9.872                         | 0.22  | 0.86  | 0.11 | 94.9  | 9.88  | 0.22  | 0.88  |
| 08554336-4443569 | 265.452  | 0.309    | 2.475  | 7      | -      | -    | -    | -        | -    | -      | -    | -                      | -          | -          | -    | -        | -          | -     | 11.849                             | 1.64                        | 3.53                        | 1                     | 18.8                               | 0.80                                 | 3.88                          | 10.927                        | 1.23  | 2.30  | 0.77 | ...   | ...   | 1.28  | 2.46  |
| 08554652-4145496 | 263.194  | 2.237    | 1.512  | 1      | -      | -    | -    | -        | -    | -      | -    | -                      | -          | -          | -    | -        | -          | -     | 11.346                             | 0.55                        | 1.59                        | 1                     | 34.6                               | 0.62                                 | 3.87                          | 10.783                        | 0.30  | 0.83  | 0.47 | 40.3  | 10.77 | 0.33  | 0.93  |
| 08555714-4631289 | 266.844  | -0.821   | 1.781  | 6      | -      | -    | -    | -        | -    | -      | -    | -                      | -          | -          | -    | -        | -          | -     | 11.432                             | 1.13                        | 3.05                        | 1                     | 19.2                               | 0.52                                 | 3.93                          | 10.768                        | 0.84  | 2.16  | 0.55 | ...   | ...   | 0.87  | 2.28  |
| 08561258-4306346 | 264.272  | 1.426    | 15.324 | 9      | -      | -    | -    | -        | -    | -      | -    | -                      | -          | -          | -    | -        | -          | -     | 13.629                             | 0.52                        | 1.54                        | -1                    | 13.4                               | 1.00                                 | 3.98                          | 7.919                         | -2.02 | -6.07 | 4.75 | ...   | ...   | -1.72 | -5.06 |
| 08562107-4307066 | 264.296  | 1.440    | 18.267 | 9      | -      | -    | -    | -        | -    | -      | -    | -                      | -          | -          | -    | -        | -          | -     | 11.120                             | 0.75                        | 2.03                        | 1                     | 58.6                               | 0.54                                 | 3.98                          | 4.314</                       |       |       |      |       |       |       |       |

Table B1: a) continued.

| 2MASX J          | <i>l</i> | <i>b</i> | EBV    | Object | Sample | Disc | 2MRS | Velocity | NIR  | Photom | Ext  | <i>K</i> <sub>20</sub> | <i>H-K</i> | <i>J-K</i> | vc   | <i>a</i> | <i>b/a</i> | st.d. | <i>K</i> <sub>s</sub> <sup>o</sup> | ( <i>H-K</i> ) <sup>o</sup> | ( <i>J-K</i> ) <sup>o</sup> | <i>A<sub>K</sub></i> | <i>a</i> <sub>d</sub> <sup>o</sup> | <i>K</i> <sub>s</sub> <sup>o,d</sup> | ( <i>H-K</i> ) <sup>o,c</sup> | ( <i>J-K</i> ) <sup>o,c</sup> |        |        |       |       |        |        |      |
|------------------|----------|----------|--------|--------|--------|------|------|----------|------|--------|------|------------------------|------------|------------|------|----------|------------|-------|------------------------------------|-----------------------------|-----------------------------|----------------------|------------------------------------|--------------------------------------|-------------------------------|-------------------------------|--------|--------|-------|-------|--------|--------|------|
| (1)              | deg      | deg      | mag    | class  | off    | flag | gal  | TF       | obs  | ext'd  | type | (9)                    | Opt        | HI         | flag | flag     | flag       | flag  | mag                                | mag                         | mag                         | mag                  | mag                                | mag                                  | mag                           | mag                           |        |        |       |       |        |        |      |
| (2a)             | (2b)     | (3)      | (4)    | (5)    | (6)    | (7a) | (7b) | (7c)     | (7d) | (8)    | (9)  | (10a)                  | (10b)      | (11)       | (12) | (13)     | (14)       | (15)  | (16)                               | (17)                        | (18)                        | (19)                 | (20)                               | (21)                                 | (22)                          | (23)                          | (24)   | (25)   | (26)  | (27)  | (28)   |        |      |
| 08582872–4516317 | 266.181  | 0.325    | 3.581  | 1      | –      | –    | g    | –        | –    | –      | D1   | –                      | –          | h          | –    | –        | –          | –     | 10.206                             | 0.77                        | 2.32                        | 1                    | 73.8                               | 0.70                                 | 3.92                          | 8.872                         | 0.18   | 0.54   | 1.11  | 121.0 | 8.70   | 0.25   | 0.78 |
| 08583875–4231577 | 264.125  | 2.141    | 4.252  | 1      | –      | –    | g    | –        | –    | –      | D2   | –                      | –          | h          | –    | –        | –          | –     | 9.270                              | 0.79                        | 2.52                        | 1                    | 70.8                               | 0.52                                 | 3.82                          | 7.686                         | 0.09   | 0.40   | 1.32  | 109.9 | 7.71   | 0.17   | 0.68 |
| 08585293–4733088 | 267.949  | –1.112   | 39.253 | 9      | –      | –    | –    | –        | –    | –      | –    | –                      | –          | –          | –    | –        | –          | –     | 9.563                              | 1.27                        | 2.30                        | 1                    | 152.2                              | 0.30                                 | 4.14                          | –5.063                        | –5.23  | –17.20 | 12.16 | ...   | –4.46  | –14.61 |      |
| 08585343–4732068 | 267.937  | –1.099   | 46.496 | 9      | –      | –    | –    | –        | –    | –      | –    | –                      | –          | –          | –    | –        | –          | –     | 10.522                             | ...                         | ...                         | 1                    | 48.2                               | 0.32                                 | 4.14                          | –6.802                        | ...    | ...    | 14.40 | ...   | ...    | ...    |      |
| 08585423–4729498 | 267.910  | –1.073   | 59.731 | 9      | –      | –    | –    | –        | –    | –      | –    | –                      | –          | –          | –    | –        | –          | –     | 1.68                               | ...                         | ...                         | 1                    | 143.4                              | 1.00                                 | 4.17                          | –14.628                       | –8.21  | ...    | 18.50 | ...   | –7.04  | ...    |      |
| 08585440–4609438 | 266.901  | –0.198   | 2.729  | 8      | –      | –    | –    | –        | –    | –      | –    | –                      | –          | –          | –    | –        | –          | –     | 12.095                             | 0.81                        | 1.98                        | –2                   | 23.6                               | 0.58                                 | 3.98                          | 11.078                        | 0.36   | 0.62   | 0.85  | ...   | 0.42   | 0.80   |      |
| 08585500–4345408 | 265.087  | 1.375    | 33.136 | 9      | –      | –    | –    | –        | –    | –      | –    | –                      | –          | –          | –    | –        | –          | –     | 12.046                             | 0.97                        | 2.27                        | 1                    | 41.6                               | 0.50                                 | 3.91                          | –0.300                        | –4.51  | –14.19 | 10.26 | ...   | –3.86  | –12.00 |      |
| 08585521–4731548 | 267.938  | –1.093   | 50.348 | 9      | –      | –    | –    | –        | –    | –      | –    | –                      | –          | –          | –    | –        | –          | –     | 10.306                             | 1.60                        | 2.98                        | 1                    | 81.0                               | 0.22                                 | 4.14                          | –8.454                        | –6.73  | –22.04 | 15.60 | ...   | –5.75  | –18.71 |      |
| 08585731–4722478 | 267.827  | –0.989   | 20.910 | 8      | –      | –    | –    | –        | –    | –      | –    | –                      | –          | –          | –    | –        | –          | –     | 10.109                             | 1.11                        | ...                         | 1                    | 93.2                               | 0.92                                 | 4.17                          | 2.318                         | –2.35  | ...    | 6.48  | ...   | –1.94  | ...    |      |
| 08585749–4728408 | 267.901  | –1.053   | 60.394 | 9      | –      | –    | –    | –        | –    | –      | –    | –                      | –          | –          | –    | –        | –          | –     | 8.390                              | 1.47                        | 2.39                        | 1                    | 72.2                               | 0.76                                 | 4.17                          | –14.113                       | –8.53  | –27.61 | 18.71 | ...   | –7.35  | –23.63 |      |
| 08585788–4731219 | 267.936  | –1.082   | 57.063 | 9      | –      | –    | –    | –        | –    | –      | –    | –                      | –          | –          | –    | –        | –          | –     | 1.36                               | ...                         | ...                         | 1                    | 134.0                              | 0.38                                 | 4.14                          | –13.684                       | –8.09  | ...    | 17.68 | ...   | –6.97  | ...    |      |
| 08585808–4730198 | 267.923  | –1.070   | 63.232 | 9      | –      | –    | –    | –        | –    | –      | –    | –                      | –          | –          | –    | –        | –          | –     | 6.226                              | 1.40                        | 2.63                        | 1                    | 233.0                              | 0.66                                 | 4.17                          | –17.334                       | –9.07  | –28.79 | 19.59 | ...   | –7.83  | –24.61 |      |
| 08585827–4732578 | 267.956  | –1.098   | 46.974 | 9      | –      | –    | –    | –        | –    | –      | –    | –                      | –          | –          | –    | –        | –          | –     | 10.305                             | 1.47                        | 2.87                        | 1                    | 45.4                               | 0.56                                 | 4.14                          | –7.198                        | –6.31  | –20.47 | 14.55 | ...   | –5.38  | –17.37 |      |
| 08585828–4727279 | 267.887  | –1.038   | 52.703 | 9      | –      | –    | –    | –        | –    | –      | –    | –                      | –          | –          | –    | –        | –          | –     | 9.614                              | 1.13                        | 2.51                        | 1                    | 75.2                               | 0.52                                 | 4.17                          | –10.023                       | –7.60  | –23.67 | 16.33 | ...   | –6.56  | –20.19 |      |
| 08585956–4729299 | 267.915  | –1.058   | 62.821 | 9      | –      | –    | –    | –        | –    | –      | –    | –                      | –          | –          | –    | –        | –          | –     | 6.856                              | 1.33                        | 2.24                        | 1                    | 219.8                              | 0.11                                 | 4.17                          | –16.551                       | –9.07  | –28.97 | 19.46 | ...   | –7.84  | –24.83 |      |
| 08590034–4735059 | 267.987  | –1.117   | 28.036 | 9      | –      | –    | –    | –        | –    | –      | –    | –                      | –          | –          | –    | –        | –          | –     | 9.443                              | 0.96                        | 1.58                        | 1                    | 150.2                              | 0.40                                 | 4.14                          | –1.003                        | –3.68  | –12.35 | 8.68  | ...   | –3.13  | –10.50 |      |
| 08590162–4732109 | 267.953  | –1.083   | 57.453 | 9      | –      | –    | –    | –        | –    | –      | –    | –                      | –          | –          | –    | –        | –          | –     | 7.424                              | 2.94                        | ...                         | 1                    | 174.2                              | 0.82                                 | 4.14                          | –13.983                       | –6.57  | ...    | 17.80 | ...   | –5.44  | ...    |      |
| 08590203–4728189 | 267.905  | –1.039   | 58.902 | 9      | –      | –    | –    | –        | –    | –      | –    | –                      | –          | –          | –    | –        | –          | –     | 8.505                              | 1.18                        | 2.35                        | 1                    | 131.0                              | 0.62                                 | 4.17                          | –13.442                       | –8.58  | –26.91 | 18.25 | ...   | –7.42  | –23.02 |      |
| 08590262–4729599 | 267.927  | –1.057   | 63.824 | 9      | –      | –    | –    | –        | –    | –      | –    | –                      | –          | –          | –    | –        | –          | –     | 6.889                              | 1.08                        | 2.75                        | 1                    | 104.6                              | 0.66                                 | 4.17                          | –16.892                       | –9.49  | –28.96 | 19.77 | ...   | –8.24  | –24.74 |      |
| 08590291–4730539 | 267.939  | –1.066   | 65.273 | 9      | –      | –    | –    | –        | –    | –      | –    | –                      | –          | –          | –    | –        | –          | –     | 7.121                              | ...                         | 2.08                        | 1                    | 41.2                               | 1.00                                 | 4.17                          | –17.200                       | ...    | –30.35 | 20.22 | ...   | ...    | –26.04 |      |
| 08590325–5314504 | 272.284  | –4.813   | 0.783  | 1      | –      | –    | –    | –        | P    | –      | D3   | –                      | –          | –          | –    | –        | –          | –     | 10.591                             | 0.52                        | 1.45                        | 1                    | 49.6                               | 0.96                                 | 3.96                          | 10.299                        | 0.39   | 1.06   | 0.24  | 52.6  | 10.31  | 0.40   | 1.11 |
| 08590528–4729429 | 267.928  | –1.048   | 62.775 | 9      | –      | –    | –    | –        | –    | –      | –    | –                      | –          | –          | –    | –        | –          | –     | 5.303                              | 1.62                        | 3.00                        | 1                    | 154.2                              | 0.46                                 | 4.17                          | –18.087                       | –8.77  | –28.19 | 19.44 | ...   | –7.54  | –24.04 |      |
| 08590637–4729099 | 267.923  | –1.040   | 61.958 | 9      | –      | –    | –    | –        | –    | –      | –    | –                      | –          | –          | –    | –        | –          | –     | 6.561                              | 1.59                        | 2.94                        | 1                    | 168.2                              | 0.66                                 | 4.17                          | –16.525                       | –8.67  | –27.84 | 19.19 | ...   | –7.45  | –23.75 |      |
| 08590647–4732549 | 267.971  | –1.080   | 51.898 | 9      | –      | –    | –    | –        | –    | –      | –    | –                      | –          | –          | –    | –        | –          | –     | 10.727                             | 1.86                        | ...                         | 1                    | 47.6                               | 0.52                                 | 4.14                          | –8.610                        | –6.73  | ...    | 16.08 | ...   | –5.72  | ...    |      |
| 08590755–4734379 | 267.995  | –1.097   | 33.007 | 9      | –      | –    | –    | –        | –    | –      | –    | –                      | –          | –          | –    | –        | –          | –     | 9.434                              | 0.97                        | 1.10                        | 1                    | 114.4                              | 0.16                                 | 4.14                          | –2.864                        | –4.49  | –15.29 | 10.22 | ...   | –3.85  | –13.12 |      |
| 08590795–4730599 | 267.949  | –1.056   | 63.340 | 9      | –      | –    | –    | –        | –    | –      | –    | –                      | –          | –          | –    | –        | –          | –     | 5.541                              | ...                         | 2.79                        | 1                    | 217.8                              | 1.00                                 | 4.14                          | –18.059                       | ...    | –28.68 | 19.62 | ...   | ...    | –24.50 |      |
| 08590913–4730499 | 267.950  | –1.052   | 62.411 | 9      | –      | –    | –    | –        | –    | –      | –    | –                      | –          | –          | –    | –        | –          | –     | 6.275                              | 1.85                        | 4.05                        | 1                    | 220.0                              | 0.46                                 | 4.17                          | –16.979                       | –8.48  | –26.96 | 19.33 | ...   | –7.26  | –22.84 |      |
| 08590913–4734049 | 267.991  | –1.087   | 38.833 | 9      | –      | –    | –    | –        | –    | –      | –    | –                      | –          | –          | –    | –        | –          | –     | 10.333                             | 0.87                        | 1.24                        | 1                    | 97.4                               | 0.28                                 | 4.14                          | –4.136                        | –5.56  | –18.06 | 12.03 | ...   | –4.80  | –15.49 |      |
| 08590963–4733199 | 267.982  | –1.078   | 47.894 | 9      | –      | –    | –    | –        | –    | –      | –    | –                      | –          | –          | –    | –        | –          | –     | 10.178                             | 1.05                        | 1.33                        | 1                    | 102.0                              | 0.22                                 | 4.14                          | –7.667                        | –6.88  | –22.46 | 14.84 | ...   | –5.94  | –19.30 |      |
| 08591002–4729409 | 267.937  | –1.037   | 60.552 | 9      | –      | –    | –    | –        | –    | –      | –    | –                      | –          | –          | –    | –        | –          | –     | 8.720                              | 2.02                        | ...                         | 1                    | 62.0                               | 0.82                                 | 4.17                          | –13.842                       | –8.01  | ...    | 18.76 | ...   | –6.82  | ...    |      |
| 08591044–5156174 | 271.301  | –3.945   | 1.476  | 1      | –      | –    | –    | –        | P    | –      | D1   | –                      | –          | –          | –    | –        | –          | –     | 11.524                             | 0.51                        | 1.57                        | 1                    | 33.2                               | 0.70                                 | 3.99                          | 10.974                        | 0.26   | 0.84   | 0.46  | 38.6  | 10.95  | 0.29   | 0.93 |
| 08591058–5002204 | 269.862  | –2.702   | 1.442  | 2      | –      | –    | –    | –        | t    | –      | D3   | –                      | –          | –          | –    | –        | –          | –     | 11.050                             | 0.48                        | 1.61                        | 1                    | 35.4                               | 0.56                                 | 4.04                          | 10.513                        | 0.24   | 0.90   | 0.45  | 40.3  | 10.52  | 0.27   | 0.99 |
| 08591448–4347449 | 265.151  | 1.397    | 64.791 | 9      | –      | –    | –    | –        | –    | –      | –    | –                      | –          | –          | –    | –        | –          | –     | 12.390                             | 1.14                        | 2.57                        | –2                   | 28.4                               | 1.00                                 | 3.91                          | –11.751                       | –9.59  | –29.62 | 20.07 | ...   | –8.32  | –25.34 |      |
| 08591466–4730569 | 267.961  | –1.041   | 56.714 | 9      | –      | –    | –    | –        | –    | –      | –    | –                      | –          | –          | –    | –        | –          | –     | 9.620                              | 2.50                        | ...                         | 1                    | 72.6                               | 0.44                                 | 4.17                          | –11.512                       | –6.89  | ...    | 17.57 | ...   | –5.78  | ...    |      |
| 08591718–4018341 | 262.519  | 3.685    | 0.895  | 1      | –      | –    | –    | –        | t    | –      | D1   | –                      | –          | o          | –    | –        | –          | –     | 10.681                             | 0.51                        | 1.56                        | 1                    | 45.0                               | 0.40                                 | 3.74                          | 10.348                        | 0.36   | 1.11   | 0.28  | 48.1  | 10.37  | 0.38   | 1.17 |
| 08591751–4341539 | 265.084  | 1.467    | 68.423 | 9      | –      | –    | –    | –        | –    | –      | –    | –                      | –          | –          | –    | –        | –          | –     | 12.149                             | 1.08                        | 2.51                        | 1                    | 39.4                               | 0.58                                 | 3.77                          | –13.345                       | –10.25 | –31.48 | 21.19 | ...   | –8.91  | –26.97 |      |
| 08591770–4535269 | 266.513  | 0.227    | 7.450  | 8      | –      | –    | –    | –        | –    | –      | –    | –                      | –          | –          | –    | –        | –          | –     | 8.951                              | ...                         | 2.75                        | 1                    | 102.0                              | 1.00                                 | 3.95                          | 6.175                         | ...    | –0.96  | 2.31  | ...   | ...    | –0.46  |      |
| 08591827–4536259 | 266.527  | 0.218    | 7.418  | 9      | –      | –    | –    | –        | –    | –      | –    | –                      | –          | –          | –    | –        | –          | –     | 12.910                             | 1.03                        | 2.26                        | –2                   | 26.2                               | 0.48                                 | 3.95                          | 10.146                        | –0.19  | –1.43  | 2.30  | ...   | –0.05  | –0.94  |      |
| 08591900–4732248 | 267.988  | –1.048   | 45.803 | 9      | –      | –    | –    | –        | –    | –      | –    | –                      | –          | –          | –    | –        | –          | –     | 9.749                              | ...                         | ...                         | 1                    | 203.2                              | 0.18                                 | 4.14                          | –7.317                        | ...    | ...    | 14.19 | ...   | ...    | ...    |      |
| 08591982–4342049 | 265.090  | 1.471    | 73.215 | 9      | –      | –    | –    | –        | –    | –      | –    | –                      | –          | –          | –    | –        | –          | –     | 9.414                              | 1.22                        | ...                         | 1                    | 101.6                              | 0.18                                 | 3.77                          | –17.866                       | –10.91 | ...    | 22.68 | ...   | –9.47  | ...    |      |
| 08591983–4344339 | 265.122  | 1.443    | 93.465 | 9      | –      | –    | –    | –        | –    | –      | –    | –                      | –          | –          | –    | –        | –          | –     | 8.900                              | 2.51                        | 5.37                        | 1                    | 219.8                              | 0.24                                 | 3.77                          | –25.925                       | –12.97 | –41.07 | 28.95 | ...   | –11.14 | –34.90 |      |
| 08592020–4346459 | 265.150  | 1.420    | 80.574 | 9      | –      | –    | –    | –        | –    | –      | –    | –                      | –          | –          | –    | –        | –          | –     | 7.994                              | 1.92                        | 3.89                        | 1                    | 219.6                              | 0.24                                 | 3.91                          | –22.028                       | –11.42 | –36.14 | 24.96 | ...   | –9.84  | –30.82 |      |
| 08592058–4729309 |          |          |        |        |        |      |      |          |      |        |      |                        |            |            |      |          |            |       |                                    |                             |                             |                      |                                    |                                      |                               |                               |        |        |       |       |        |        |      |

72

A. C. Schröder et al.



Table B1: a) continued.

| 2MASX J          |         | <i>l</i>    | <i>b</i>    | EBV        | Object       |            |             | Sample      |            |             | Disc          | 2MRS        | Velocity | NIR          | Photom      | Ext          | <i>K</i> <sub>20</sub> | <i>H-K</i>   | <i>J-K</i> | <i>vc</i>   | <i>a</i>    | <i>b/a</i>  | std.d. | <i>K</i> <sub>S</sub> <sup>o</sup> | ( <i>H-K</i> ) <sup>o</sup> | ( <i>J-K</i> ) <sup>o</sup> | <i>A<sub>K</sub></i> | <i>a</i> <sup>d</sup> | <i>K</i> <sub>S</sub> <sup>o,d</sup> | ( <i>H-K</i> ) <sup>o,c</sup> | ( <i>J-K</i> ) <sup>o,c</sup> |             |             |             |
|------------------|---------|-------------|-------------|------------|--------------|------------|-------------|-------------|------------|-------------|---------------|-------------|----------|--------------|-------------|--------------|------------------------|--------------|------------|-------------|-------------|-------------|--------|------------------------------------|-----------------------------|-----------------------------|----------------------|-----------------------|--------------------------------------|-------------------------------|-------------------------------|-------------|-------------|-------------|
| (1)              |         | deg<br>(2a) | deg<br>(2b) | mag<br>(3) | class<br>(4) | off<br>(5) | flag<br>(6) | gal<br>(7a) | TF<br>(7b) | obs<br>(7c) | ext'd<br>(7d) | type<br>(8) | (9)      | Opt<br>(10a) | HI<br>(10b) | flag<br>(11) | flag<br>(12)           | flag<br>(13) |            | mag<br>(14) | mag<br>(15) | mag<br>(16) | (17)   | "<br>(18)                          | (19)                        | (20)                        | mag<br>(21)          | mag<br>(22)           | mag<br>(23)                          | mag<br>(24)                   | "<br>(25)                     | mag<br>(26) | mag<br>(27) | mag<br>(28) |
| 09033747-4827470 | 269.157 | -1.117      | 26.965      | 9          | -            | -          | -           | -           | -          | -           | -             | -           | -        | -            | -           | -            | -                      | -            | -          | 12.099      | ...         | ...         | 1      | 28.8                               | 0.36                        | 4.04                        | 2.052                | ...                   | ...                                  | 8.35                          | ...                           | ...         | ...         | ...         |
| 09034400-4828291 | 269.177 | -1.111      | 22.125      | 9          | -            | -          | -           | -           | -          | -           | -             | -           | -        | -            | -           | -            | -                      | -            | -          | 9.583       | 1.47        | ...         | 1      | 130.0                              | 0.64                        | 3.95                        | 1.339                | -2.19                 | ...                                  | 6.85                          | ...                           | ...         | -1.76       | ...         |
| 09035422-5229302 | 272.197 | -3.765      | 1.562       | 2          | -            | -          | -           | g           | -          | +           | -             | n           | -        | -            | -           | -            | -                      | -            | -          | 11.801      | 0.43        | 1.41        | 1      | 24.4                               | 0.98                        | 4.03                        | 11.234               | 0.17                  | 0.65                                 | 0.47                          | 28.9                          | 11.19       | 0.20        | 0.75        |
| 09042214-4854212 | 269.569 | -1.321      | 4.862       | 9          | -            | -          | -           | -           | -          | -           | -             | -           | -        | -            | -           | -            | -                      | -            | -          | 9.710       | 1.40        | ...         | 1      | 80.2                               | 0.64                        | 3.98                        | 7.898                | 0.59                  | ...                                  | 1.51                          | ...                           | ...         | 0.69        | ...         |
| 09043141-4849356 | 269.527 | -1.249      | 4.422       | 7          | -            | -          | -           | -           | -          | -           | -             | -           | -        | -            | -           | -            | -                      | -            | -          | 11.211      | 0.97        | 2.55        | 1      | 33.4                               | 0.72                        | 3.98                        | 9.377                | 0.16                  | 0.10                                 | 1.52                          | ...                           | ...         | 0.26        | 0.43        |
| 09043331-3829221 | 261.818 | 5.650       | 4.942       | 1          | -            | -          | -           | g           | -          | -           | -             | D1          | c        | o            | -           | V            | -                      | -            | -          | 10.230      | 0.48        | 1.35        | 1      | 44.6                               | 0.54                        | 3.62                        | 10.065               | 0.41                  | 1.13                                 | 0.14                          | 45.6                          | 10.08       | 0.41        | 1.15        |
| 09050037-3416059 | 258.691 | 8.513       | 0.372       | 1          | -            | -          | -           | g           | -          | -           | -             | D4          | c        | o            | -           | V            | -                      | -            | -          | 11.094      | 0.35        | 1.18        | 1      | 28.6                               | 0.84                        | 3.58                        | 10.955               | 0.29                  | 0.99                                 | 0.12                          | 29.2                          | 10.97       | 0.30        | 1.02        |
| 09050958-4930222 | 270.102 | -1.626      | 5.908       | 9          | -            | -          | -           | -           | -          | -           | -             | -           | -        | -            | -           | -            | -                      | -            | -          | 12.901      | 0.90        | ...         | 1      | 19.4                               | 0.62                        | 3.99                        | 10.700               | -0.07                 | ...                                  | 1.83                          | ...                           | ...         | 0.04        | ...         |
| 09051061-4930042 | 270.100 | -1.620      | 5.962       | 7          | -            | -          | -           | -           | -          | -           | -             | -           | -        | -            | -           | -            | -                      | -            | -          | 12.595      | 1.41        | ...         | 1      | 21.0                               | 0.56                        | 3.99                        | 10.374               | 0.42                  | ...                                  | 1.85                          | ...                           | ...         | 0.54        | ...         |
| 09051403-4615033 | 267.692 | 0.563       | 1.457       | 1          | -            | -          | -           | g           | -          | -           | -             | D1          | c        | o            | h           | -            | -                      | -            | -          | 10.886      | 0.59        | 1.95        | 1      | 35.2                               | 0.82                        | 3.95                        | 10.343               | 0.35                  | 1.22                                 | 0.45                          | 40.6                          | 10.34       | 0.38        | 1.32        |
| 09060422-3436000 | 259.089 | 8.459       | 0.436       | 1          | -            | -          | -           | g           | t          | -           | -             | D1          | c        | o            | -           | V            | -                      | -            | -          | 11.289      | 0.40        | 1.27        | 1      | 46.4                               | 0.50                        | 3.54                        | 11.127               | 0.33                  | 1.05                                 | 0.14                          | 47.9                          | 11.13       | 0.34        | 1.08        |
| 09064483-4229388 | 265.086 | 3.284       | 0.943       | 1          | -            | -          | -           | g           | -          | P           | -             | D3          | c        | o            | -           | -            | -                      | -            | -          | 10.460      | 0.38        | 1.33        | 1      | 35.8                               | 0.88                        | 3.82                        | 10.029               | 0.22                  | 0.86                                 | 0.29                          | 38.3                          | 10.08       | 0.24        | 0.92        |
| 09065346-4146560 | 264.576 | 3.783       | 0.737       | 1          | -            | -          | -           | g           | -          | P           | -             | D3          | c        | o            | -           | -            | -                      | -            | -          | 11.066      | 0.25        | 1.14        | 1      | 52.2                               | 0.58                        | 3.77                        | 10.791               | 0.17                  | 0.78                                 | 0.23                          |                               |             |             |             |

2M-ZoA galaxy catalogue description and analysis 73

| 2MASX J          | <i>l</i><br>deg<br>(2a) | <i>b</i><br>deg<br>(2b) | EBV<br>mag<br>(3) | Object<br>class off flg<br>(4) (5) (6) | Sample<br>gal TF obs<br>(7a) (7b) (7c) | Disc<br>ext'd<br>(7d) | 2MRS<br>type<br>(8) | Velocity<br>Opt HI<br>(10a) (10b) | NIR<br>flg<br>(11) | Photom<br>flg<br>(12) | Ext<br>flg<br>(13) | <i>K</i> <sub>20</sub><br>mag<br>(14) | <i>H-K</i><br>mag<br>(15) | <i>J-K</i><br>mag<br>(16) | vc<br>(17) | <i>a</i><br>" (18) | <i>b/a</i><br>(19) | st.d.<br>(20) | <i>K</i> <sub>0</sub><br>mag<br>(21) | ( <i>H-K</i> ) <sup>o</sup><br>mag<br>(22) | ( <i>J-K</i> ) <sup>a</sup><br>mag<br>(23) | <i>A<sub>K</sub></i><br>mag<br>(24) | <i>a</i> <sup>d</sup><br>" (25) | <i>K</i> <sub>0</sub> <sup>d</sup><br>mag<br>(26) | ( <i>H-K</i> ) <sup>o,c</sup><br>mag<br>(27) | ( <i>J-K</i> ) <sup>o,c</sup><br>mag<br>(28) |
|------------------|-------------------------|-------------------------|-------------------|----------------------------------------|----------------------------------------|-----------------------|---------------------|-----------------------------------|--------------------|-----------------------|--------------------|---------------------------------------|---------------------------|---------------------------|------------|--------------------|--------------------|---------------|--------------------------------------|--------------------------------------------|--------------------------------------------|-------------------------------------|---------------------------------|---------------------------------------------------|----------------------------------------------|----------------------------------------------|
| 09173325-4748538 | 270.269                 | 1.024                   | 7.500             | 9                                      | -                                      | -                     | -                   | -                                 | -                  | -                     | -                  | 13.728                                | 0.48                      | 1.19                      | -1         | 13.2               | 0.46               | 3.84          | 10.934                               | -0.76                                      | -2.53                                      | 2.32                                | ...                             | ...                                               | -0.61                                        | -2.04                                        |
| 09175436-4827194 | 270.768                 | 0.618                   | 5.687             | 9                                      | -                                      | -                     | -                   | -                                 | -                  | -                     | -                  | 11.812                                | 1.34                      | ...                       | 1          | 37.8               | 1.00               | 3.92          | 9.693                                | 0.39                                       | ...                                        | 1.76                                | ...                             | ...                                               | 0.50                                         | -2.04                                        |
| 09175521-5024184 | 272.162                 | -0.745                  | 2.301             | 3                                      | -                                      | -                     | -                   | -                                 | -                  | -                     | -                  | 12.097                                | 0.75                      | 2.15                      | 1          | 16.4               | 0.76               | 4.08          | 11.240                               | 0.36                                       | 1.01                                       | 0.71                                | 21.5                            | 11.18                                             | 0.41                                         | 1.16                                         |
| 09180214-4810564 | 270.588                 | 0.824                   | 4.505             | 7                                      | -                                      | g                     | -                   | P                                 | -                  | -                     | e                  | 10.008                                | 1.47                      | 3.32                      | 1          | 40.2               | 0.74               | 3.89          | 8.329                                | 0.73                                       | 1.08                                       | 1.40                                | ...                             | 11.18                                             | 0.81                                         | 1.38                                         |
| 09180961-4823313 | 270.752                 | 0.692                   | 5.561             | 9                                      | -                                      | -                     | -                   | -                                 | -                  | -                     | -                  | 12.577                                | 1.88                      | ...                       | 1          | 18.2               | 0.44               | 3.92          | 10.505                               | 0.96                                       | ...                                        | 1.72                                | ...                             | ...                                               | 1.07                                         | -                                            |
| 09181946-4826450 | 270.810                 | 0.674                   | 6.746             | 9                                      | -                                      | -                     | -                   | -                                 | -                  | -                     | -                  | 10.535                                | 1.50                      | 3.62                      | 1          | 49.8               | 0.80               | 3.92          | 8.021                                | 0.39                                       | 0.26                                       | 2.09                                | ...                             | ...                                               | 0.52                                         | 0.71                                         |
| 09182399-4826260 | 270.815                 | 0.687                   | 6.910             | 9                                      | -                                      | -                     | -                   | -                                 | -                  | -                     | -                  | 12.158                                | 1.07                      | 2.20                      | 1          | 52.4               | 0.18               | 3.92          | 8.023                                | -0.07                                      | -1.23                                      | 2.14                                | ...                             | ...                                               | 0.07                                         | -0.77                                        |
| 09182511-3917188 | 264.253                 | 7.086                   | 0.298             | 9                                      | e                                      | -                     | -                   | -                                 | -                  | -                     | -                  | 11.334                                | 0.32                      | 1.12                      | -2         | 33.2               | 0.72               | 3.66          | 11.223                               | 0.27                                       | 0.98                                       | 0.09                                | ...                             | ...                                               | 0.28                                         | 1.00                                         |
| 09182611-3917123 | 264.254                 | 7.089                   | 0.298             | 1                                      | -                                      | -                     | -                   | -                                 | -                  | -                     | -                  | 10.164                                | 0.35                      | 1.15                      | 1          | 76.4               | 0.40               | 3.68          | 10.053                               | 0.30                                       | 1.00                                       | 0.09                                | 77.6                            | 10.06                                             | 0.31                                         | 1.03                                         |
| 09183669-3800363 | 263.352                 | 8.001                   | 0.237             | 1                                      | -                                      | g                     | t                   | -                                 | -                  | -                     | -                  | 8.364                                 | 0.28                      | 1.04                      | 1          | 126.2              | 0.64               | 3.54          | 8.276                                | 0.24                                       | 0.92                                       | 0.07                                | 127.4                           | 8.29                                              | 0.25                                         | 0.93                                         |
| 09183969-4517537 | 268.603                 | 2.921                   | 1.176             | 2                                      | -                                      | -                     | -                   | -                                 | -                  | -                     | -                  | 11.480                                | 0.52                      | 1.41                      | 1          | 28.2               | 0.64               | 3.87          | 11.042                               | 0.33                                       | 0.83                                       | 0.36                                | 31.5                            | 11.04                                             | 0.35                                         | 0.91                                         |
| 09185135-3845073 | 263.924                 | 7.520                   | 0.230             | 1                                      | -                                      | g                     | -                   | -                                 | -                  | -                     | -                  | 10.025                                | 0.28                      | 1.02                      | 1          | 65.8               | 0.92               | 3.64          | 9.937                                | 0.24                                       | 0.92                                       | 0.09                                | 66.5                            | 9.95                                              | 0.24                                         | 0.92                                         |
| 09192603-5934249 | 278.883                 | 7.003                   | 0.317             | 1                                      | -                                      | g                     | -                   | -                                 | -                  | -                     | -                  | 11.186                                | 0.38                      | 1.10                      | 1          | 37.2               | 0.78               | 3.81          | 11.068                               | 0.25                                       | 0.94                                       | 0.10                                | 37.8                            | 11.08                                             | 0.26                                         | 0.97                                         |
| 09195905-3910294 | 264.384                 | 7.382                   | 0.286             | 1                                      | -                                      | g                     | t                   | -                                 | -                  | -                     | -                  | 11.163                                | 0.22                      | 1.00                      | 1          | 41.0               | 0.36               | 3.61          | 11.056                               | 0.17                                       | 0.86                                       | 0.09                                | 41.6                            | 11.07                                             | 0.18                                         | 0.88                                         |
| 09200635-4842183 | 271.201                 | 0.701                   | 3.021             | 6                                      | -                                      | -                     | -                   | -                                 | -                  | -                     | -                  | 11.217                                | 1.26                      | 3.13                      | 1          | 15.6               | 0.84               | 3.93          | 10.091                               | 0.76                                       | 1.63                                       | 0.94                                | ...                             | ...                                               | 0.82                                         | 1.83                                         |
| 09212497-5818422 | 278.159                 | -5.937                  | 0.423             | 9                                      | -                                      | p                     | -                   | -                                 | -                  | -                     | -                  | 10.782                                | 0.87                      | 0.88                      |            |                    |                    |               |                                      |                                            |                                            |                                     |                                 |                                                   |                                              |                                              |

Table B1: a) continued.

| 2MASX J          | <i>l</i> | <i>b</i> | EBV   | Object |     | Sample | Disc | 2MRS | Velocity | NIR   | Photom | Ext  | <i>K</i> <sub>20</sub> | <i>H-K</i> | <i>J-K</i> | vc   | <i>a</i> | <i>b/a</i> | st.d. | <i>K</i> <sub>s</sub> <sup>o</sup> | ( <i>H-K</i> ) <sup>o</sup> | ( <i>J-K</i> ) <sup>o</sup> | <i>A<sub>K</sub></i> | <i>a</i> <sub>d</sub> <sup>o</sup> | <i>K</i> <sub>s</sub> <sup>o,d</sup> | ( <i>H-K</i> ) <sup>o,c</sup> | ( <i>J-K</i> ) <sup>o,c</sup> |
|------------------|----------|----------|-------|--------|-----|--------|------|------|----------|-------|--------|------|------------------------|------------|------------|------|----------|------------|-------|------------------------------------|-----------------------------|-----------------------------|----------------------|------------------------------------|--------------------------------------|-------------------------------|-------------------------------|
| (1)              | deg      | deg      | mag   | class  | off | gal    | TF   | Obs  | type     | Opt   | HI     | flag | <i>K</i> <sub>20</sub> | mag        | mag        | (17) | "        | (19)       | (20)  | mag                                | mag                         | mag                         | mag                  | "                                  | mag                                  | mag                           | mag                           |
| (2a)             | (2b)     | (3)      | (4)   | (5)    | (6) | (7a)   | (7b) | (7c) | (7d)     | (10a) | (10b)  | (11) | (14)                   | (15)       | (16)       | (17) | (18)     | (19)       | (20)  | (21)                               | (22)                        | (23)                        | (24)                 | (25)                               | (26)                                 | (27)                          | (28)                          |
| 09292924−4341001 | 268.847  | 5.426    | 0.828 | 1      | −   | −      | g    | −    | D4       | c     | o      | −    | 11.169                 | 0.53       | 1.41       | 1    | 34.8     | 0.80       | 3.74  | 10.860                             | 0.40                        | 0.99                        | 0.26                 | 37.2                               | 10.87                                | 0.41                          | 1.05                          |
| 09293943−5317341 | 275.479  | −1.535   | 1.922 | 2      | −   | −      | g    | −    | D1       | −     | −      | −    | 11.045                 | 0.50       | 1.75       | 1    | 31.6     | 0.82       | 4.17  | 10.329                             | 0.18                        | 0.79                        | 0.60                 | 38.2                               | 10.33                                | 0.22                          | 0.92                          |
| 09294384−5718019 | 278.244  | −4.440   | 0.960 | 1      | −   | −      | g    | −    | D1       | −     | −      | −    | 10.935                 | 0.37       | 1.35       | 1    | 39.8     | 0.66       | 4.04  | 10.577                             | 0.22                        | 0.88                        | 0.30                 | 43.5                               | 10.57                                | 0.23                          | 0.94                          |
| 09295846−6210599 | 281.656  | −7.954   | 0.314 | 1      | −   | −      | g    | −    | D1       | c     | o      | h    | 8.459                  | 0.28       | 1.09       | 1    | 109.2    | 0.60       | 3.83  | 8.342                              | 0.23                        | 0.93                        | 0.10                 | 110.7                              | 8.36                                 | 0.24                          | 0.95                          |
| 09300273−5738080 | 278.506  | −4.654   | 0.862 | 1      | −   | −      | g    | +    | D4       | −     | −      | −    | 11.542                 | 0.43       | 1.46       | 1    | 24.8     | 0.74       | 3.99  | 11.221                             | 0.29                        | 1.03                        | 0.27                 | 26.5                               | 11.23                                | 0.30                          | 1.08                          |
| 09300712−4325114 | 268.748  | 5.696    | 0.771 | 1      | −   | −      | g    | t    | D1       | c     | o      | −    | 11.465                 | 0.38       | 1.18       | 1    | 43.6     | 0.44       | 3.72  | 11.178                             | 0.25                        | 0.79                        | 0.24                 | 46.9                               | 11.16                                | 0.27                          | 0.84                          |
| 09300865−4211544 | 267.905  | 6.584    | 0.586 | 1      | −   | −      | g    | −    | D1       | c     | o      | −    | 10.833                 | 0.43       | 1.25       | 1    | 52.4     | 0.42       | 3.66  | 10.615                             | 0.34                        | 0.95                        | 0.18                 | 54.5                               | 10.63                                | 0.35                          | 0.99                          |
| 09302571−6502042 | 283.694  | −9.973   | 0.251 | 1      | −   | −      | g    | t    | D2       | c     | o      | −    | 11.234                 | 0.37       | 1.23       | 1    | 30.4     | 0.34       | 3.66  | 11.140                             | 0.33                        | 1.10                        | 0.08                 | 30.8                               | 11.15                                | 0.34                          | 1.12                          |
| 09310533−4214227 | 268.061  | 6.675    | 0.625 | 1      | −   | −      | g    | −    | D1       | c     | o      | −    | 11.048                 | 0.37       | 1.29       | 1    | 22.6     | 0.62       | 3.66  | 10.815                             | 0.27                        | 0.98                        | 0.19                 | 23.5                               | 10.83                                | 0.28                          | 1.02                          |
| 09311940−5232594 | 275.154  | −0.822   | 2.419 | 6      | −   | −      | g    | −    | −        | −     | −      | −    | 11.619                 | 1.16       | ...        | 1    | 22.2     | 0.60       | 4.19  | 10.718                             | 0.76                        | ...                         | 0.75                 | ...                                | ...                                  | 0.81                          | ...                           |
| 09314183−6135385 | 281.394  | −7.387   | 0.306 | 1      | −   | −      | g    | t    | D1       | c     | o      | −    | 11.238                 | 0.43       | 1.32       | 1    | 34.2     | 0.42       | 3.91  | 11.124                             | 0.38                        | 1.16                        | 0.09                 | 34.8                               | 11.13                                | 0.38                          | 1.18                          |
| 09314617−5149345 | 274.710  | −0.246   | 1.670 | 1      | o   | −      | g    | t    | D1       | −     | −      | o    | 11.661                 | 0.38       | 1.23       | 1    | 28.6     | 0.52       | 4.18  | 11.039                             | 0.11                        | 0.40                        | 0.52                 | 33.7                               | 11.03                                | 0.14                          | 0.51                          |
| 09330225−3954037 | 266.711  | 8.628    | 0.459 | 1      | −   | −      | g    | −    | D1       | c     | o      | −    | 11.323                 | 0.51       | 1.19       | 1    | 34.2     | 0.68       | 3.56  | 11.152                             | 0.44                        | 0.96                        | 0.14                 | 35.3                               | 11.16                                | 0.45                          | 0.99                          |
| 09331565−4353278 | 269.488  | 5.741    | 0.700 | 1      | −   | −      | g    | −    | D3       | c     | o      | −    | 10.970                 | 0.30       | 1.16       | 1    | 30.0     | 0.94       | 3.67  | 10.709                             | 0.19                        | 0.81                        | 0.22                 | 31.5                               | 10.73                                | 0.20                          | 0.86                          |
| 09332667−5130242 | 274.684  | 0.165    | 2.594 | 8      | o   | −      | g    | −    | −        | −     | −      | o    | 8.534                  | 2.81       | 4.79       | −2   | 49.6     | 0.42       | 4.04  | 7.567                              | 2.38                        | 3.50                        | 0.80                 | ...                                | ...                                  | 2.44                          | 3.67                          |
| 09333076−5900273 | 279.781  | −5.344   | 0.602 | 1      | −   | −      | g    | −    | D1       | c     | o      | −    | 11.275                 | 0.28       | 1.10       | 1    | 32.0     | 0.76       | 3.96  | 11.051                             | 0.18                        | 0.80                        | 0.19                 | 33.4                               | 11.06                                | 0.19                          | 0.84                          |
| 09334264−3852177 | 266.092  | 9.466    | 0.406 | 1      | −   | −      | g    | −    | D1       | c     | o      | −    | 11.246                 | 0.41       | 1.17       | 1    | 27.0     | 0.80       | 3.48  | 11.095                             | 0.34                        | 0.97                        | 0.13                 | 27.7                               | 11.11                                | 0.35                          | 0.99                          |
| 09344668−6037123 | 280.999  | −6.421   | 0.349 | 1      | −   | −      | g    | t    | D1       | c     | o      | −    | 11.062                 | 0.36       | 1.16       | 1    | 51.6     | 0.34       | 3.94  | 10.932                             | 0.30                        | 0.98                        | 0.11                 | 52.8                               | 10.94                                | 0.31                          | 1.01                          |
| 09345810−5646361 | 278.410  | −3.571   | 1.456 | 1      | −   | −      | g    | −    | D1       | c     | o      | −    | 11.784                 | 0.47       | 1.43       | 1    | 29.8     | 0.70       | 4.08  | 11.241                             | 0.23                        | 0.70                        | 0.45                 | 35.0                               | 11.20                                | 0.26                          | 0.80                          |
| 09350321−5822051 | 279.494  | −4.738   | 0.727 | 1      | −   | −      | g    | t    | D1       | c     | o      | −    | 10.987                 | 0.41       | 1.16       | 1    | 38.2     | 0.48       | 3.99  | 10.716                             | 0.29                        | 0.80                        | 0.23                 | 40.2                               | 10.73                                | 0.30                          | 0.85                          |
| 09351238−4148163 | 268.325  | 7.515    | 0.567 | 1      | −   | −      | g    | −    | D1       | c     | o      | −    | 10.553                 | 0.36       | 1.18       | 1    | 61.0     | 0.50       | 3.53  | 10.342                             | 0.27                        | 0.90                        | 0.18                 | 63.3                               | 10.36                                | 0.28                          | 0.94                          |
| 09353312−3856164 | 266.403  | 9.663    | 0.403 | 1      | −   | −      | g    | −    | D4       | c     | o      | −    | 11.160                 | 0.36       | 1.22       | 1    | 44.2     | 0.54       | 3.48  | 11.010                             | 0.29                        | 1.02                        | 0.12                 | 45.4                               | 11.02                                | 0.30                          | 1.05                          |
| 09354870−5022312 | 274.197  | 1.252    | 1.355 | 1      | −   | −      | g    | −    | D3       | c     | o      | −    | 10.479                 | 0.47       | 1.64       | 1    | 44.4     | 0.72       | 4.06  | 9.974                              | 0.25                        | 0.97                        | 0.42                 | 50.0                               | 9.99                                 | 0.28                          | 1.06                          |
| 09363028−6205576 | 282.160  | −7.371   | 0.361 | 1      | −   | −      | g    | −    | D4       | c     | o      | −    | 9.462                  | 0.31       | 1.11       | 1    | 60.0     | 0.94       | 3.86  | 9.327                              | 0.26                        | 0.93                        | 0.11                 | 61.0                               | 9.34                                 | 0.26                          | 0.95                          |
| 09363929−5437078 | 277.135  | −1.813   | 1.899 | 1      | −   | −      | g    | −    | −        | −     | h      | −    | 11.478                 | 0.50       | 1.59       | 1    | 29.4     | 0.84       | 4.22  | 10.770                             | 0.19                        | 0.64                        | 0.59                 | 37.1                               | 10.69                                | 0.23                          | 0.77                          |
| 09370080−6055596 | 281.414  | −6.468   | 0.386 | 1      | −   | −      | g    | t    | D1       | c     | o      | h    | 10.754                 | 0.30       | 1.04       | 1    | 71.8     | 0.46       | 3.93  | 10.610                             | 0.24                        | 0.85                        | 0.12                 | 73.9                               | 10.61                                | 0.24                          | 0.88                          |
| 09371614−5602089 | 278.148  | −2.808   | 1.492 | 1      | −   | −      | g    | t    | D1       | c     | o      | −    | 11.631                 | 0.53       | 1.79       | 1    | 30.0     | 0.60       | 4.19  | 11.075                             | 0.28                        | 1.05                        | 0.46                 | 34.7                               | 11.07                                | 0.31                          | 1.15                          |
| 09372430−5025244 | 274.418  | 1.387    | 1.378 | 1      | −   | −      | g    | t    | D1       | c     | o      | −    | 10.626                 | 0.51       | 1.55       | 1    | 53.6     | 0.58       | 4.02  | 10.113                             | 0.28                        | 0.87                        | 0.43                 | 60.7                               | 10.12                                | 0.31                          | 0.96                          |
| 09375125−6209039 | 282.312  | −7.303   | 0.379 | 1      | −   | −      | g    | −    | D3       | c     | o      | −    | 9.063                  | 0.35       | 1.14       | 1    | 135.0    | 0.28       | 3.88  | 8.922                              | 0.29                        | 0.96                        | 0.12                 | 138.0                              | 8.93                                 | 0.29                          | 0.98                          |
| 09375988−6032179 | 281.237  | −6.094   | 0.375 | 1      | −   | −      | g    | −    | D1       | c     | o      | −    | 11.250                 | 0.38       | 1.27       | 1    | 41.4     | 0.86       | 3.97  | 11.110                             | 0.31                        | 1.08                        | 0.12                 | 42.4                               | 11.12                                | 0.32                          | 1.11                          |
| 09381025−4221020 | 269.106  | 7.482    | 0.541 | 1      | −   | −      | g    | t    | D1       | c     | o      | −    | 11.394                 | 0.51       | 1.27       | 1    | 47.6     | 0.28       | 3.55  | 11.192                             | 0.42                        | 1.00                        | 0.17                 | 49.7                               | 11.19                                | 0.43                          | 1.03                          |
| 09381364−6329113 | 283.249  | −8.265   | 0.227 | 1      | −   | −      | g    | t    | D1       | c     | o      | h    | 9.749                  | 0.34       | 1.13       | 1    | 84.2     | 0.30       | 3.76  | 9.664                              | 0.30                        | 1.02                        | 0.07                 | 85.1                               | 9.67                                 | 0.31                          | 1.03                          |
| 09382912−6149464 | 282.151  | −7.015   | 0.337 | 1      | −   | −      | g    | −    | D1       | c     | o      | −    | 9.880                  | 0.26       | 1.02       | 1    | 70.6     | 0.60       | 3.88  | 9.754                              | 0.20                        | 0.85                        | 0.10                 | 71.9                               | 9.77                                 | 0.21                          | 0.87                          |
| 09383171−6356004 | 283.577  | −8.573   | 0.260 | 1      | −   | −      | g    | −    | −        | −     | h      | −    | 9.913                  | 0.26       | 1.05       | 1    | 77.4     | 0.64       | 3.74  | 9.816                              | 0.21                        | 0.92                        | 0.08                 | 78.4                               | 9.83                                 | 0.22                          | 0.93                          |
| 09383352−6144185 | 282.096  | −6.941   | 0.345 | 1      | −   | −      | g    | −    | D3       | c     | o      | h    | 9.439                  | 0.32       | 1.10       | 1    | 62.8     | 0.72       | 3.88  | 9.310                              | 0.27                        | 0.93                        | 0.11                 | 63.7                               | 9.33                                 | 0.27                          | 0.96                          |
| 09384714−6005305 | 281.011  | −5.697   | 0.456 | 9      | −   | p?     | g    | −    | D1       | c     | o      | −    | 9.270                  | 1.02       | 1.21       | 1    | 32.0     | 0.76       | 3.97  | 9.100                              | 0.94                        | 0.98                        | 0.14                 | ...                                | ...                                  | 0.95                          | 1.01                          |
| 09404610−4112329 | 268.700  | 8.655    | 0.454 | 3      | −   | +      | g    | −    | D3       | cr    | −      | −    | 10.547                 | 0.60       | 1.40       | −2   | 193.4    | 1.00       | 3.53  | 10.378                             | 0.52                        | 1.17                        | 0.14                 | 200.5                              | 10.37                                | 0.53                          | 1.20                          |
| 09412450−5716276 | 279.396  | −3.359   | 1.001 | 7      | −   | −      | g    | −    | −        | −     | h      | −    | 11.068                 | 0.37       | 1.10       | −2   | 26.2     | 0.66       | 4.18  | 10.695                             | 0.21                        | 0.60                        | 0.31                 | ...                                | ...                                  | 0.23                          | 0.67                          |
| 09414364−6047560 | 281.755  | −5.986   | 0.455 | 1      | −   | −      | g    | −    | D1       | c     | o      | h    | 11.132                 | 0.26       | 1.09       | 1    | 35.2     | 0.56       | 3.92  | 10.962                             | 0.18                        | 0.86                        | 0.14                 | 36.4                               | 10.97                                | 0.19                          | 0.89                          |
| 09415565−4205567 | 269.460  | 8.133    | 0.547 | 1      | −   | −      | g    | −    | D1       | c     | o      | −    | 11.375                 | 0.33       | 1.26       | 1    | 32.0     | 0.66       | 3.58  | 11.171                             | 0.24                        | 0.98                        | 0.17                 | 33.3                               | 11.18                                | 0.25                          | 1.02                          |
| 09422208−4148573 | 269.333  | 8.400    | 0.569 | 1      | −   | −      | g    | t    | D1       | c     | o      | −    | 9.796                  | 0.45       | 1.44       | 1    | 84.4     | 0.22       | 3.54  | 9.584                              | 0.35                        | 1.16                        | 0.18                 | 87.4                               | 9.60                                 | 0.36                          | 1.19                          |
| 09423087−5225450 | 276.341  | 0.406    | 2.093 | 9      | −   | −      | g    | −    | −        | −     | −      | −    | 10.743                 | 0.31       | 1.55       | −2   | 77.0     | 0.40       | 4.14  | 9.963                              | −0.04                       | 0.51                        | 0.65                 | ...                                | ...                                  | 0.00                          | 0.64                          |
| 09424851−4203213 | 269.555  | 8.273    | 0.535 | 1      | −   | −      | g    | −    | D1       | c     | o      | h    | 10.901                 | 0.40       | 1.19       | 1    | 42.2     | 0.58       | 3.62  | 10.702                             | 0.31                        | 0.92                        | 0.17                 | 43.9                               | 10.71                                | 0.32                          | 0.96                          |
| 09425161−6529243 | 284.977  | −9.426   | 0.265 | 1      | −   | −      | g    | −    | D4       | c     | o      | −    | 10.913                 | 0.30       | 1.06       | 1    | 41.4     | 0.82       | 3.61  | 10.814                             | 0.26                        | 0.93                        | 0.08                 | 41.9                               | 10.83                                | 0.26                          | 0.95                          |
| 09432153−5701146 | 279.430  | −2.994   | 1.142 | 2      | −   | +      | g    | −    | n        | −     | −      | −    | 10.995                 | 0.48       | 1.48       | 1    | 41.0     | 0.50       | 4.17  | 10.569                             | 0.29                        | 0.92                        | 0.35                 | 45.1                               | 10.58                                | 0.32                          | 0.99                          |
| 09462280−4144586 | 269.860  | 8.940    | 0.455 | 1      | −   | −      | g    | −    | D1       | c     | o      | −    | 10.935                 | 0.29       | 1.12       | 1    | 43.2     | 0.64       | 3.57  | 10.765                             | 0.21                        | 0.90                        | 0.14                 | 44.5                               | 10.78                                | 0.22                          | 0.93                          |
| 09462882−4129396 | 269.706  | 9.146    | 0.479 | 1      | −   | −      | g    | −    | D1       | c     | o      | −    | 11.347                 | 0.48       | 1.18       | 1    | 32.2     | 0.78       | 3.57  | 11.169                             | 0.40                        | 0.94                        | 0.15                 | 33.3                               |                                      |                               |                               |

76

A. C. Schröder et al.

Table B1: a) continued.

| 2MASX J          | <i>l</i> | <i>b</i> | EBV    | Object |     | Sample | Disc | 2MRS | Velocity | NIR   | Photom | Ext | <i>K</i> <sub>20</sub> | <i>H-K</i> | <i>J-K</i> | vc   | <i>a</i> | <i>b/a</i> | st.d.  | <i>K</i> <sub>s</sub> <sup>o</sup> | ( <i>H-K</i> ) <sup>o</sup> | ( <i>J-K</i> ) <sup>o</sup> | <i>A<sub>K</sub></i> | <i>a</i> <sub>d</sub> <sup>o</sup> | <i>K</i> <sub>s</sub> <sup>o,d</sup> | ( <i>H-K</i> ) <sup>o,c</sup> | ( <i>J-K</i> ) <sup>o,c</sup> |      |      |       |       |      |      |
|------------------|----------|----------|--------|--------|-----|--------|------|------|----------|-------|--------|-----|------------------------|------------|------------|------|----------|------------|--------|------------------------------------|-----------------------------|-----------------------------|----------------------|------------------------------------|--------------------------------------|-------------------------------|-------------------------------|------|------|-------|-------|------|------|
| (1)              | deg      | deg      | mag    | class  | off | flag   | gal  | TF   | obs      | ext'd | type   |     | (14)                   | mag        | mag        | (17) | "        | (19)       | (20)   | mag                                | mag                         | mag                         | mag                  | "                                  | mag                                  | mag                           | mag                           |      |      |       |       |      |      |
| (2a)             | (2b)     | (2b)     | (3)    | (4)    | (5) | (6)    | (7a) | (7b) | (7c)     | (7d)  | (8)    | (9) | (10a)                  | (10b)      | (11)       | (12) | (13)     | (14)       | (15)   | (16)                               | (17)                        | (18)                        | (19)                 | (20)                               | (21)                                 | (22)                          | (23)                          | (24) | (25) | (26)  | (27)  | (28) |      |
| 10114466–5743082 | 282.883  | –1.202   | 5.025  | 9      | –   | –      | –    | –    | –        | –     | –      | –   | 12.636                 | ...        | ...        | –2   | 18.0     | 0.34       | 4.29   | 10.764                             | ...                         | ...                         | 1.56                 | ...                                | ...                                  | ...                           | ...                           | ...  | ...  | ...   | ...   |      |      |
| 10120401–5721284 | 282.712  | –0.881   | 8.141  | 9      | –   | –      | –    | –    | –        | –     | –      | –   | 10.179                 | 0.91       | 2.44       | 1    | 56.0     | 0.78       | 4.28   | 7.146                              | –0.44                       | –1.61                       | 2.52                 | ...                                | ...                                  | –0.28                         | –1.07                         | ...  | ...  | ...   | ...   |      |      |
| 10121187–6232002 | 285.685  | –5.121   | 0.291  | 1      | –   | –      | –    | –    | –        | –     | D1     | c   | o                      | h          | –          | –    | –        | –          | 9.538  | 0.39                               | 1.10                        | 1                           | 70.8                 | 0.46                               | 4.00                                 | 9.430                         | 0.34                          | 0.96 | 0.09 | 71.9  | 9.44  | 0.35 | 0.98 |
| 10121985–4717415 | 276.983  | 7.401    | 0.191  | 1      | –   | –      | –    | –    | –        | –     | D1     | c   | –                      | h          | V          | –    | –        | –          | 9.385  | 0.38                               | 1.41                        | 1                           | 219.8                | 0.12                               | 3.64                                 | 9.314                         | 0.35                          | 1.32 | 0.06 | 221.9 | 9.32  | 0.35 | 1.33 |
| 10122126–5734144 | 282.865  | –1.034   | 6.424  | 9      | –   | –      | –    | –    | –        | –     | –      | –   | 11.043                 | ...        | ...        | 1    | 50.8     | 0.38       | 4.25   | 8.649                              | ...                         | ...                         | 1.99                 | ...                                | ...                                  | ...                           | ...                           | ...  | ...  | ...   | ...   |      |      |
| 10122974–5300193 | 280.282  | 2.731    | 0.708  | 1      | –   | –      | –    | –    | –        | –     | D3     | –   | –                      | –          | –          | –    | –        | –          | 11.282 | 0.37                               | 1.19                        | 1                           | 24.6                 | 0.82                               | 4.03                                 | 11.018                        | 0.25                          | 0.84 | 0.22 | 25.8  | 11.04 | 0.27 | 0.89 |
| 10124021–6401533 | 286.590  | –6.319   | 0.289  | 1      | –   | –      | –    | –    | –        | –     | D1     | c   | o                      | –          | –          | –    | –        | –          | 11.096 | 0.40                               | 1.29                        | 1                           | 34.0                 | 0.42                               | 3.93                                 | 10.988                        | 0.35                          | 1.15 | 0.09 | 34.5  | 11.00 | 0.36 | 1.17 |
| 10124289–4547531 | 276.169  | 8.665    | 0.167  | 1      | –   | –      | –    | –    | –        | –     | D3     | c   | o                      | –          | V          | –    | –        | –          | 11.210 | 0.38                               | 1.09                        | 1                           | 36.8                 | 0.64                               | 3.54                                 | 11.148                        | 0.36                          | 1.01 | 0.05 | 37.1  | 11.15 | 0.36 | 1.02 |
| 10131037–6216544 | 285.634  | –4.850   | 0.341  | 1      | –   | –      | –    | –    | –        | –     | D3     | e   | o                      | h          | –          | –    | –        | –          | 9.662  | 0.29                               | 1.07                        | 1                           | 61.4                 | 0.72                               | 4.09                                 | 9.535                         | 0.23                          | 0.90 | 0.11 | 62.4  | 9.55  | 0.24 | 0.93 |
| 10132507–5231223 | 280.123  | 3.207    | 0.571  | 1      | –   | –      | –    | –    | –        | –     | D1     | e   | o                      | h          | –          | –    | –        | –          | 11.213 | 0.39                               | 1.17                        | 1                           | 31.4                 | 0.56                               | 3.98                                 | 11.000                        | 0.30                          | 0.89 | 0.18 | 32.7  | 11.01 | 0.31 | 0.92 |
| 10132903–5802524 | 283.260  | –1.341   | 4.034  | 9      | –   | –      | –    | –    | –        | –     | –      | –   | 10.432                 | 0.76       | 1.74       | 1    | 46.8     | 0.90       | 4.31   | 8.929                              | 0.09                        | –0.27                       | 1.25                 | ...                                | ...                                  | ...                           | ...                           | ...  | ...  | 0.17  | 0.00  |      |      |
| 10133504–5652235 | 282.607  | –0.365   | 2.107  | 4      | –   | –      | –    | –    | –        | –     | –      | n   | –                      | –          | –          | –    | –        | –          | 11.923 | 0.60                               | 1.70                        | –2                          | 24.8                 | 0.58                               | 4.27                                 | 11.138                        | 0.25                          | 0.66 | 0.65 | 31.7  | 11.08 | 0.29 | 0.80 |
| 10134565–5217134 | 280.032  | 3.431    | 0.503  | 1      | –   | –      | –    | –    | –        | –     | D1     | e   | o                      | h          | –          | –    | –        | –          | 11.012 | 0.34                               | 1.13                        | 1                           | 60.2                 | 0.66                               | 3.96                                 | 10.825                        | 0.26                          | 0.88 | 0.16 | 62.8  | 10.82 | 0.27 | 0.91 |
| 10140153–5741065 | 283.115  | –1.001   | 12.812 | 9      | –   | –      | –    | –    | –        | –     | –      | –   | 12.085                 | 1.02       | ...        | –2   | 25.8     | 0.20       | 4.27   | 7.311                              | –1.10                       | ...                         | 3.97                 | ...                                | ...                                  | –0.85                         | ...                           | ...  | ...  | ...   | ...   |      |      |
| 10141616–5743204 | 283.163  | –1.014   | 14.503 | 9      | –   | –      | –    | –    | –        | –     | –      | –   | 10.352                 | ...        | ...        | 1    | 50.0     | 1.00       | 4.29   | 4.948                              | ...                         | ...                         | 4.49                 | ...                                | ...                                  | ...                           | ...                           | ...  | ...  | ...   | ...   |      |      |
| 10141880–6454226 | 287.239  | –6.937   | 0.264  | 1      | –   | –      | –    | –    | –        | –     | D1     | c   | o                      | h          | –          | –    | –        | –          | 11.172 | 0.26                               | 1.04                        | 1                           | 40.2                 | 0.56                               | 3.91                                 | 11.074                        | 0.22                          | 0.91 | 0.08 | 40.8  | 11.08 | 0.23 | 0.93 |
| 10143327–5742405 | 283.188  | –0.983   | 13.313 | 9      | –   | –      | –    | –    | –        | –     | –      | –   | 11.239                 | ...        | ...        | 1    | 124.6    | 0.28       | 4.29   | 6.279                              | ...                         | ...                         | 4.12                 | ...                                | ...                                  | ...                           | ...                           | ...  | ...  | ...   | ...   |      |      |
| 10144180–4451158 | 275.911  | 9.638    | 0.211  | 1      | –   | –      | –    | –    | –        | –     | D1     | c   | o                      | h          | V          | –    | –        | –          | 10.848 | 0.29                               | 0.92                        | 1                           | 89.2                 | 0.48                               | 3.54                                 | 10.769                        | 0.25                          | 0.81 | 0.07 | 90.4  | 10.77 | 0.26 | 0.83 |
| 10144575–5818145 | 283.544  | –1.458   | 3.621  | 7      | –   | –      | –    | –    | –        | –     | –      | –   | 10.372                 | 1.35       | 3.23       | 1    | 33.0     | 0.76       | 4.34   | 9.023                              | 0.75                        | 1.43                        | 1.12                 | ...                                | ...                                  | ...                           | ...                           | ...  | ...  | 0.82  | 1.67  |      |      |
| 10145984–5741384 | 283.227  | –0.936   | 11.007 | 7      | –   | –      | –    | –    | –        | –     | –      | –   | 10.762                 | 1.44       | ...        | 1    | 28.8     | 0.72       | 4.29   | 6.661                              | –0.38                       | ...                         | 3.41                 | ...                                | ...                                  | –0.17                         | ...                           | ...  | ...  | ...   | ...   |      |      |
| 10150518–5751066 | 283.325  | –1.060   | 11.140 | 9      | –   | –      | –    | –    | –        | –     | –      | –   | 10.982                 | 0.92       | ...        | 1    | 45.6     | 1.00       | 4.34   | 6.831                              | –0.92                       | ...                         | 3.45                 | ...                                | ...                                  | –0.70                         | ...                           | ...  | ...  | ...   | ...   |      |      |
| 10153337–4507580 | 276.198  | 9.495    | 0.202  | 1      | –   | –      | –    | –    | –        | –     | D1     | c   | o                      | V          | –          | –    | –        | –          | 10.231 | 0.26                               | 1.02                        | 1                           | 71.2                 | 0.42                               | 3.58                                 | 10.156                        | 0.23                          | 0.92 | 0.06 | 71.8  | 10.17 | 0.23 | 0.93 |
| 10153482–5851107 | 283.941  | –1.852   | 1.863  | 9      | –   | –      | –    | –    | –        | –     | –      | –   | 11.539                 | ...        | ...        | 1    | 31.0     | 0.68       | 4.35   | 10.845                             | ...                         | ...                         | 0.78                 | 0.58                               | ...                                  | ...                           | ...                           | ...  | ...  | ...   | 0.91  |      |      |
| 10154951–5723486 | 283.152  | –0.627   | 8.752  | 9      | –   | –      | –    | –    | –        | –     | –      | –   | 9.831                  | ...        | ...        | 1    | 88.8     | 1.00       | 4.30   | 6.570                              | ...                         | ...                         | 2.47                 | 2.71                               | ...                                  | ...                           | ...                           | ...  | ...  | ...   | –1.90 |      |      |
| 10155260–5723576 | 283.160  | –0.625   | 8.874  | 9      | –   | –      | –    | –    | –        | –     | –      | –   | 10.171                 | 0.64       | 2.05       | 1    | 81.8     | 0.74       | 4.30   | 6.865                              | –0.83                       | –2.36                       | 2.75                 | ...                                | ...                                  | –0.65                         | –1.77                         | ...  | ...  | ...   | ...   |      |      |
| 10162006–6224183 | 286.008  | –4.745   | 0.386  | 1      | –   | –      | –    | –    | –        | –     | D3     | –   | –                      | –          | –          | –    | –        | –          | 11.310 | 0.31                               | 1.13                        | 1                           | 33.2                 | 0.62                               | 4.06                                 | 11.166                        | 0.24                          | 0.94 | 0.12 | 34.0  | 11.18 | 0.25 | 0.96 |
| 10165552–4852518 | 278.525  | 6.529    | 0.213  | 1      | –   | –      | –    | –    | –        | –     | D1     | c   | o                      | h          | V          | –    | –        | –          | 8.879  | 0.36                               | 1.02                        | 1                           | 153.0                | 0.47                               | ...                                  | 8.800                         | 0.32                          | 0.91 | 0.07 | ...   | ...   | 0.32 | 0.93 |
| 10165553–6050532 | 285.196  | –3.413   | 0.763  | 3      | o   | –      | –    | –    | –        | –     | D2     | –   | –                      | –          | o          | –    | –        | –          | 10.824 | 0.33                               | 1.17                        | 1                           | 30.4                 | 0.54                               | 4.20                                 | 10.540                        | 0.20                          | 0.79 | 0.24 | 32.0  | 10.56 | 0.22 | 0.84 |
| 10170533–5024469 | 279.407  | 5.273    | 0.292  | 1      | –   | –      | –    | –    | –        | –     | D3     | c   | o                      | –          | V          | –    | –        | –          | 11.298 | 0.41                               | 1.23                        | 1                           | 34.6                 | 0.68                               | 3.82                                 | 11.189                        | 0.36                          | 1.08 | 0.09 | 35.2  | 11.20 | 0.37 | 1.10 |
| 10172807–5819397 | 283.852  | –1.279   | 3.273  | 9      | –   | –      | –    | –    | –        | –     | –      | –   | 9.247                  | 0.87       | 2.05       | 1    | 101.0    | 0.62       | 4.37   | 8.027                              | 0.33                        | 0.42                        | 1.01                 | ...                                | ...                                  | ...                           | ...                           | ...  | ...  | 0.39  | 0.64  |      |      |
| 10174918–6832243 | 289.600  | –9.742   | 0.180  | 1      | o   | –      | –    | –    | –        | –     | D1     | c   | o                      | –          | –          | o    | –        | –          | 10.884 | 0.35                               | 1.05                        | 1                           | 62.4                 | 0.24                               | 3.72                                 | 10.817                        | 0.32                          | 0.96 | 0.06 | 63.0  | 10.82 | 0.32 | 0.97 |
| 10181253–4657433 | 277.625  | 8.242    | 0.237  | 1      | –   | –      | –    | –    | –        | –     | D3     | c   | o                      | –          | V          | –    | –        | –          | 10.990 | 0.35                               | 1.23                        | 1                           | 34.8                 | 0.80                               | 3.66                                 | 10.902                        | 0.31                          | 1.11 | 0.07 | 35.2  | 10.91 | 0.31 | 1.12 |
| 10185021–5810126 | 283.915  | –1.048   | 7.276  | 9      | –   | –      | –    | –    | –        | –     | –      | –   | 11.266                 | ...        | ...        | 1    | 29.6     | 0.62       | 4.39   | 8.555                              | ...                         | ...                         | 2.25                 | ...                                | ...                                  | ...                           | ...                           | ...  | ...  | ...   | ...   |      |      |
| 10185690–5809026 | 283.917  | –1.024   | 7.719  | 7      | –   | –      | –    | –    | –        | –     | –      | –   | 9.928                  | 1.77       | ...        | 1    | 54.0     | 0.60       | 4.39   | 7.052                              | 0.49                        | ...                         | 2.39                 | ...                                | ...                                  | ...                           | ...                           | ...  | ...  | 0.64  | ...   |      |      |
| 10190461–4807014 | 278.395  | 7.363    | 0.154  | 1      | –   | –      | –    | –    | –        | –     | D1     | c   | o                      | –          | V          | –    | –        | –          | 11.156 | 0.38                               | 1.22                        | 1                           | 29.0                 | 0.84                               | 3.71                                 | 11.099                        | 0.35                          | 1.15 | 0.05 | 29.2  | 11.11 | 0.36 | 1.16 |
| 10191121–5802124 | 283.881  | –0.911   | 7.932  | 9      | –   | –      | –    | –    | –        | –     | –      | –   | 8.713                  | 0.51       | 1.56       | 1    | 111.6    | 0.58       | 4.36   | 5.758                              | –0.80                       | –2.39                       | 2.46                 | ...                                | ...                                  | –0.65                         | –1.86                         | ...  | ...  | ...   | ...   |      |      |
| 10193250–6013294 | 285.120  | –2.716   | 1.588  | 8      | –   | –      | –    | –    | –        | –     | D2     | –   | –                      | –          | –          | –    | –        | –          | 8.862  | 1.28                               | 2.14                        | –2                          | 26.4                 | 0.80                               | 4.26                                 | 8.270                         | 1.02                          | 1.35 | 0.49 | ...   | ...   | 1.05 | 1.45 |
| 10193893–6255244 | 286.614  | –4.965   | 0.365  | 1      | –   | –      | –    | –    | –        | –     | D1     | –   | –                      | –          | –          | –    | –        | –          | 11.316 | 0.35                               | 1.12                        | 1                           | 26.6                 | 0.68                               | 4.03                                 | 11.180                        | 0.29                          | 0.94 | 0.11 | 27.2  | 11.19 | 0.29 | 0.96 |
| 10194125–5403325 | 281.759  | 2.454    | 0.786  | 1      | –   | –      | –    | –    | –        | –     | D2     | –   | –                      | –          | –          | –    | –        | –          | 11.360 | 0.48                               | 1.30                        | 1                           | 43.0                 | 0.84                               | 4.06                                 | 11.067                        | 0.35                          | 0.91 | 0.24 | 46.3  | 11.05 | 0.37 | 0.97 |
| 10200614–5806124 | 284.019  | –0.901   | 14.582 | 9      | –   | –      | –    | –    | –        | –     | –      | –   | 11.065                 | 1.43       | ...        | 1    | 24.6     | 0.96       | 4.38   | 5.632                              | –0.98                       | ...                         | 4.52                 | ...                                | ...                                  | –0.70                         | ...                           | ...  | ...  | ...   | ...   |      |      |
| 10201127–6401008 | 287.268  | –5.846   | 0.356  | 1      | –   | –      | –    | –    | –        | –     | D3     | c   | o                      | –          | –          | –    | –        | –          | 10.458 | 0.32                               | 1.16                        | 1                           | 42.8                 | 0.64                               | 3.95                                 | 10.325                        | 0.26                          | 0.98 | 0.11 | 43.6  | 10.34 | 0.27 | 1.00 |
| 10201360–5803065 | 284.004  | –0.849   | 18.204 | 9      | –   | –      | –    | –    | –        | –     | –      | –   | 9.417                  | ...        | ...        | 1    | 119.2    | 0.32       | 4.38   | 2.634                              | ...                         | ...                         | 5.64                 | ...                                | ...                                  | ...                           | ...                           | ...  | ...  | ...   | ...   |      |      |
| 10201447–5805165 | 284.025  | –0.878   | 16.259 | 9      | –   | –      | –    | –    | –        | –     | –      | –   | 10.722                 | ...        | ...        | 1    | 55.2     | 0.68       | 4.38   | 4.664                              | ...                         | ...                         | 5.04                 | ...                                | ...                                  | ...                           | ...                           | ...  | ...  | ...   | ...   |      |      |
| 10201611–5803565 | 284.016  | –0.857   | 17.350 | 9      |     |        |      |      |          |       |        |     |                        |            |            |      |          |            |        |                                    |                             |                             |                      |                                    |                                      |                               |                               |      |      |       |       |      |      |

Table B1: a) continued.

| 2MASX J          | <i>l</i> | <i>b</i> | EBV    | Object | Sample | Disc | 2MRS | Velocity | NIR  | Photom | Ext   | <i>K</i> <sub>20</sub> | <i>H-K</i> | <i>J-K</i> | vc  | <i>a</i> | <i>b/a</i> | st.d. | <i>K</i> <sub>s</sub> <sup>o</sup> | ( <i>H-K</i> ) <sup>o</sup> | ( <i>J-K</i> ) <sup>o</sup> | <i>A</i> <sub>K</sub> | <i>a</i> <sub>d</sub> <sup>o</sup> | <i>K</i> <sub>s</sub> <sup>o,d</sup> | ( <i>H-K</i> ) <sup>o,c</sup> | ( <i>J-K</i> ) <sup>o,c</sup> |       |      |      |         |       |        |       |      |       |       |        |
|------------------|----------|----------|--------|--------|--------|------|------|----------|------|--------|-------|------------------------|------------|------------|-----|----------|------------|-------|------------------------------------|-----------------------------|-----------------------------|-----------------------|------------------------------------|--------------------------------------|-------------------------------|-------------------------------|-------|------|------|---------|-------|--------|-------|------|-------|-------|--------|
| (1)              | deg      | deg      | mag    | class  | off    | flg  | gal  | TF       | (7b) | (7c)   | ext'd | type                   | (8)        | (9)        | Opt | HI       | (10b)      | (11)  | flg                                | (12)                        | flg                         | (13)                  | (14)                               | (15)                                 | (16)                          | (17)                          | (18)  | (19) | (20) | (21)    | (22)  | (23)   | (24)  | (25) | (26)  | (27)  | (28)   |
| 10252710-5335392 | 282.225  | 3.304    | 0.481  | 1      | o      | -    | g    | -        | P    | -      | -     | D1                     | -          | -          | -   | -        | -          | -     | o                                  | -                           | -                           | -                     | 11.263                             | 0.42                                 | 1.21                          | 1                             | 33.2  | 0.60 | 4.04 | 11.084  | 0.34  | 0.98   | 0.15  | 34.5 | 11.08 | 0.35  | 1.01   |
| 10252831-5158022 | 281.362  | 4.685    | 0.421  | 1      | -      | -    | g    | -        | t    | -      | -     | D2                     | -          | e          | o   | -        | -          | -     | -                                  | -                           | -                           | -                     | 11.218                             | 0.41                                 | 1.26                          | 1                             | 40.6  | 0.42 | 3.89 | 11.061  | 0.34  | 1.05   | 0.13  | 41.7 | 11.07 | 0.35  | 1.08   |
| 10254085-5805574 | 284.638  | -0.501   | 4.578  | 8      | -      | -    | -    | -        | -    | -      | -     | -                      | -          | -          | -   | -        | -          | -     | -                                  | -                           | -                           | -                     | 10.491                             | 0.62                                 | 1.56                          | 1                             | 56.6  | 0.68 | 4.39 | 8.785   | -0.14 | -0.71  | 1.42  | ...  | ...   | -0.05 | -0.41  |
| 10260284-5347429 | 282.407  | 3.180    | 0.519  | 1      | -      | -    | g    | -        | -    | -      | -     | D3                     | -          | -          | -   | -        | -          | -     | -                                  | -                           | -                           | -                     | 10.539                             | 0.30                                 | 1.12                          | 1                             | 42.0  | 0.76 | 4.09 | 10.346  | 0.22  | 0.86   | 0.16  | 43.4 | 10.36 | 0.23  | 0.89   |
| 10261040-5346519 | 282.415  | 3.202    | 0.508  | 1      | -      | -    | -    | -        | P    | -      | -     | D1                     | -          | -          | -   | -        | -          | -     | -                                  | -                           | -                           | -                     | 10.850                             | 0.37                                 | 1.21                          | 1                             | 42.2  | 0.78 | 4.09 | 10.661  | 0.29  | 0.96   | 0.16  | 43.7 | 10.67 | 0.30  | 1.00   |
| 10262979-5354426 | 282.525  | 3.116    | 0.558  | 1      | -      | -    | g    | -        | -    | -      | -     | D3                     | -          | -          | -   | -        | -          | -     | -                                  | -                           | -                           | -                     | 11.276                             | 0.23                                 | 1.04                          | 1                             | 25.0  | 0.72 | 4.02 | 11.068  | 0.14  | 0.76   | 0.17  | 25.9 | 11.08 | 0.15  | 0.80   |
| 10263655-5800395 | 284.696  | -0.362   | 3.652  | 7      | -      | -    | -    | -        | -    | -      | -     | -                      | -          | -          | -   | -        | -          | -     | -                                  | -                           | -                           | -                     | 10.104                             | 1.95                                 | ...                           | 1                             | 31.6  | 0.38 | 4.39 | 8.743   | 1.34  | ...    | 1.13  | ...  | ...   | 1.42  | ...    |
| 10271754-4907397 | 280.098  | 7.247    | 0.297  | 1      | -      | -    | g    | -        | -    | -      | -     | D2                     | -          | c          | o   | -        | -          | -     | -                                  | -                           | -                           | -                     | 11.049                             | 0.24                                 | 0.99                          | 1                             | 32.6  | 0.86 | 3.65 | 10.938  | 0.20  | 0.85   | 0.09  | 33.1 | 10.95 | 0.20  | 0.87   |
| 10271968-4906597 | 280.097  | 7.259    | 0.300  | 1      | o      | -    | g    | -        | t    | -      | -     | D1                     | -          | c          | o   | -        | h          | V     | o                                  | -                           | -                           | -                     | 10.644                             | 0.24                                 | 1.03                          | 1                             | 51.4  | 0.40 | 3.65 | 10.532  | 0.19  | 0.88   | 0.09  | 52.2 | 10.54 | 0.19  | 0.90   |
| 10280884-5938402 | 285.720  | -1.649   | 2.388  | 9      | -      | -    | -    | -        | -    | -      | -     | -                      | -          | -          | -   | -        | -          | -     | -                                  | -                           | -                           | -                     | 11.567                             | ...                                  | ...                           | 1                             | 34.6  | 0.56 | 4.40 | 10.677  | ...   | ...    | 0.74  | ...  | ...   | ...   | ...    |
| 10282509-5041312 | 281.080  | 6.011    | 0.295  | 1      | -      | -    | -    | -        | -    | -      | -     | D1                     | -          | c          | o   | -        | h          | V     | -                                  | -                           | -                           | -                     | 10.452                             | 0.27                                 | 0.93                          | 1                             | 59.0  | 0.54 | 3.78 | 10.342  | 0.22  | 0.78   | 0.09  | 60.1 | 10.35 | 0.23  | 0.80   |
| 10284393-5058150 | 281.269  | 5.799    | 0.345  | 1      | -      | -    | g    | -        | t    | -      | -     | D1                     | -          | c          | o   | -        | -          | V     | -                                  | -                           | -                           | -                     | 10.692                             | 0.38                                 | 1.26                          | 1                             | 67.8  | 0.28 | 3.82 | 10.563  | 0.32  | 1.09   | 0.11  | 69.3 | 10.57 | 0.33  | 1.11   |
| 10284788-5041570 | 281.136  | 6.036    | 0.290  | 1      | -      | -    | g    | -        | -    | -      | -     | D1                     | -          | c          | o   | -        | -          | V     | -                                  | -                           | -                           | -                     | 9.998                              | 0.33                                 | 1.12                          | 1                             | 61.0  | 0.58 | 3.77 | 9.890   | 0.28  | 0.98   | 0.09  | 61.9 | 9.90  | 0.29  | 1.00   |
| 10285821-6730517 | 289.924  | -8.315   | 0.245  | 1      | -      | -    | -    | -        | t    | -      | -     | D1                     | -          | -          | -   | -        | -          | -     | -                                  | -                           | -                           | -                     | 11.141                             | 0.36                                 | 1.05                          | 1                             | 38.2  | 0.40 | 3.77 | 11.050  | 0.32  | 0.93   | 0.08  | 38.7 | 11.06 | 0.33  | 0.95   |
| 10290304-5804156 | 285.003  | -0.244   | 3.655  | 9      | -      | -    | -    | -        | -    | -      | -     | -                      | -          | -          | -   | -        | -          | -     | -                                  | -                           | -                           | -                     | 11.100                             | ...                                  | ...                           | 1                             | 44.2  | 0.84 | 4.35 | 9.738   | ...   | ...    | 1.13  | ...  | ...   | ...   | ...    |
| 10292660-5726430 | 284.724  | 0.318    | 5.419  | 9      | -      | -    | -    | -        | -    | -      | -     | -                      | -          | -          | -   | -        | -          | -     | -                                  | -                           | -                           | -                     | 8.527                              | 1.15                                 | ...                           | 1                             | 191.8 | 1.00 | 4.32 | 6.508   | 0.25  | ...    | 1.68  | ...  | ...   | 0.36  | ...    |
| 10293082-5726149 | 284.728  | 0.330    | 5.295  | 9      | -      | -    | -    | -        | -    | -      | -     | -                      | -          | -          | -   | -        | -          | -     | -                                  | -                           | -                           | -                     | 8.250                              | 1.23                                 | 2.34                          | 1                             | 185.0 | 0.42 | 4.32 | 6.277   | 0.36  | -0.29  | 1.64  | ...  | ...   | 0.46  | 0.06   |
| 10293422-5745539 | 284.903  | 0.053    | 3.732  | 8      | -      | -    | -    | -        | -    | -      | -     | -                      | -          | -          | -   | -        | -          | -     | -                                  | -                           | -                           | -                     | 9.606                              | 1.20                                 | 2.82                          | 1                             | 75.8  | 0.72 | 4.33 | 8.215   | 0.58  | 0.96   | 1.16  | ...  | ...   | 0.66  | 1.21   |
| 10294819-5958395 | 286.071  | -1.826   | 2.550  | 8      | -      | -    | -    | -        | -    | -      | -     | -                      | -          | -          | -   | -        | -          | -     | -                                  | -                           | -                           | -                     | 11.218                             | 0.83                                 | ...                           | 1                             | 35.4  | 0.48 | 4.38 | 10.268  | 0.41  | ...    | 0.79  | ...  | ...   | 0.46  | ...    |
| 10303330-5853523 | 285.597  | -0.851   | 4.472  | 8      | -      | -    | -    | -        | -    | -      | -     | -                      | -          | -          | -   | -        | -          | -     | -                                  | -                           | -                           | -                     | 10.745                             | ...                                  | ...                           | 1                             | 44.0  | 0.84 | 4.38 | 9.079   | ...   | ...    | 1.39  | ...  | ...   | ...   | ...    |
| 10310139-4902491 | 280.580  | 7.634    | 0.330  | 1      | -      | -    | g    | -        | t    | -      | -     | D1                     | -          | c          | o   | -        | h          | V     | -                                  | -                           | -                           | -                     | 10.469                             | 0.36                                 | 1.14                          | 1                             | 70.0  | 0.40 | 3.68 | 10.346  | 0.30  | 0.98   | 0.10  | 71.5 | 10.35 | 0.31  | 1.00   |
| 10310231-5749330 | 285.102  | 0.102    | 4.257  | 9      | -      | -    | -    | -        | -    | -      | -     | -                      | -          | -          | -   | -        | -          | -     | -                                  | -                           | -                           | -                     | 11.899                             | ...                                  | ...                           | 1                             | 26.8  | 0.44 | 4.29 | 10.313  | ...   | ...    | 1.32  | ...  | ...   | ...   | ...    |
| 10312483-5802300 | 285.256  | -0.058   | 49.532 | 9      | -      | -    | -    | -        | -    | -      | -     | -                      | -          | -          | -   | -        | -          | -     | -                                  | -                           | -                           | -                     | 9.632                              | 1.13                                 | 2.18                          | 1                             | 33.4  | 0.40 | 4.35 | -8.824  | -7.07 | -22.42 | 15.34 | ...  | ...   | -6.10 | -19.15 |
| 10312546-5803040 | 285.262  | -0.066   | 49.842 | 9      | -      | -    | -    | -        | -    | -      | -     | -                      | -          | -          | -   | -        | -          | -     | -                                  | -                           | -                           | -                     | 7.655                              | 1.46                                 | ...                           | 1                             | 146.6 | 0.68 | 4.35 | -10.916 | -6.79 | ...    | 15.44 | ...  | ...   | -5.82 | ...    |
| 10312772-5802444 | 285.263  | -0.059   | 49.544 | 9      | -      | -    | -    | -        | -    | -      | -     | -                      | -          | -          | -   | -        | -          | -     | -                                  | -                           | -                           | -                     | 8.094                              | 1.43                                 | ...                           | 1                             | 88.0  | 0.62 | 4.33 | -10.366 | -6.78 | ...    | 15.35 | ...  | ...   | -5.80 | ...    |
| 10312774-5801244 | 285.252  | -0.039   | 49.171 | 9      | -      | -    | -    | -        | -    | -      | -     | -                      | -          | -          | -   | -        | -          | -     | -                                  | -                           | -                           | -                     | 8.202                              | 0.99                                 | 1.68                          | 1                             | 220.4 | 0.14 | 4.33 | -10.119 | -7.15 | -22.75 | 15.23 | ...  | ...   | -6.19 | -19.50 |
| 10312872-5801429 | 285.256  | -0.043   | 48.994 | 9      | -      | -    | -    | -        | -    | -      | -     | -                      | -          | -          | -   | -        | -          | -     | -                                  | -                           | -                           | -                     | 7.063                              | 1.13                                 | 2.08                          | 1                             | 219.4 | 0.54 | 4.35 | -11.192 | -6.98 | -22.26 | 15.18 | ...  | ...   | -6.02 | -19.02 |
| 10313314-5802229 | 285.270  | -0.047   | 48.764 | 9      | -      | -    | -    | -        | -    | -      | -     | -                      | -          | -          | -   | -        | -          | -     | -                                  | -                           | -                           | -                     | 8.113                              | 1.31                                 | 2.10                          | 1                             | 123.8 | 0.86 | 4.35 | -10.056 | -6.77 | -22.13 | 15.10 | ...  | ...   | -5.81 | -18.91 |
| 10313731-5800355 | 285.263  | -0.017   | 46.566 | 9      | -      | -    | -    | -        | -    | -      | -     | -                      | -          | -          | -   | -        | -          | -     | -                                  | -                           | -                           | -                     | 9.568                              | 1.31                                 | 2.39                          | 1                             | 181.4 | 0.28 | 4.33 | -7.782  | -6.40 | -20.74 | 14.42 | ...  | ...   | -5.48 | -17.67 |
| 10313766-5804585 | 285.301  | -0.079   | 35.931 | 9      | -      | -    | -    | -        | -    | -      | -     | -                      | -          | -          | -   | -        | -          | -     | -                                  | -                           | -                           | -                     | 9.717                              | 1.28                                 | 2.68                          | 1                             | 74.4  | 0.66 | 4.33 | -3.671  | -4.67 | -15.17 | 11.13 | ...  | ...   | -3.97 | -12.80 |
| 10314587-5801225 | 285.286  | -0.019   | 42.573 | 9      | -      | -    | -    | -        | -    | -      | -     | -                      | -          | -          | -   | -        | -          | -     | -                                  | -                           | -                           | -                     | 9.384                              | 1.67                                 | ...                           | 1                             | 104.2 | 0.84 | 4.33 | -6.479  | -5.38 | ...    | 13.19 | ...  | ...   | -4.54 | ...    |
| 10315722-6342306 | 288.208  | -4.898   | 0.476  | 1      | -      | -    | -    | -        | -    | -      | -     | D1                     | -          | e          | o   | -        | h          | -     | -                                  | -                           | -                           | -                     | 10.651                             | 0.28                                 | 1.10                          | 1                             | 56.2  | 0.58 | 4.07 | 10.474  | 0.20  | 0.86   | 0.15  | 58.1 | 10.48 | 0.21  | 0.89   |
| 10321588-5802152 | 285.350  | 0.002    | 15.381 | 9      | -      | -    | -    | -        | -    | -      | -     | -                      | -          | -          | -   | -        | -          | -     | -                                  | -                           | -                           | -                     | 9.896                              | ...                                  | ...                           | 1                             | 65.8  | 0.62 | 4.34 | 4.165   | ...   | ...    | 4.76  | ...  | ...   | ...   | ...    |
| 10322642-4726285 | 279.949  | 9.132    | 0.211  | 1      | -      | -    | -    | -        | -    | -      | -     | D4                     | -          | c          | o   | -        | -          | V     | -                                  | -                           | -                           | -                     | 11.092                             | 0.30                                 | 1.05                          | 1                             | 29.2  | 0.88 | 3.61 | 11.013  | 0.27  | 0.94   | 0.07  | 29.5 | 11.02 | 0.27  | 0.96   |
| 10324357-6137201 | 287.220  | -3.057   | 3.098  | 9      | -      | -    | -    | -        | -    | -      | -     | -                      | -          | -          | -   | -        | -          | -     | -                                  | -                           | -                           | -                     | 9.064                              | 0.78                                 | 1.66                          | 1                             | 220.4 | 0.28 | 4.25 | 7.910   | 0.27  | 0.12   | 0.96  | ...  | ...   | 0.33  | 0.32   |
| 10333601-5951227 | 286.419  | -1.479   | 4.374  | 7      | o      | -    | -    | -        | -    | -      | -     | -                      | -          | -          | -   | -        | -          | -     | -                                  | -                           | -                           | -                     | 10.316                             | ...                                  | ...                           | 1                             | 72.0  | 0.68 | 4.39 | 8.686   | ...   | ...    | 1.35  | ...  | ...   | ...   | ...    |
| 10333933-5952177 | 286.433  | -1.489   | 4.250  | 8      | -      | -    | -    | -        | -    | -      | -     | -                      | -          | -          | -   | -        | -          | -     | -                                  | -                           | -                           | -                     | 10.822                             | 0.83                                 | ...                           | 1                             | 43.0  | 0.84 | 4.39 | 9.238   | 0.13  | ...    | 1.32  | ...  | ...   | 0.21  | ...    |
| 10335438-5809389 | 285.600  | 0.006    | 4.146  | 8      | -      | -    | -    | -        | -    | -      | -     | -                      | -          | -          | -   | -        | -          | -     | -                                  | -                           | -                           | -                     | 11.015                             | 1.57                                 | ...                           | -2                            | 30.8  | 0.90 | 4.34 | 9.470   | 0.88  | ...    | 1.28  | ...  | ...   | 0.96  | ...    |
| 10335650-5943596 | 286.394  | -1.351   | 5.678  | 9      | -      | -    | -    | -        | -    | -      | -     | -                      | -          | -          | -   | -        | -          | -     | -                                  | -                           | -                           | -                     | 9.657                              | ...                                  | ...                           | 1                             | 201.6 | 0.34 | 4.39 | 7.541   | ...   | ...    | 1.76  | ...  | ...   | ...   | ...    |
| 10342471-5741491 | 285.425  | 0.441    | 2.166  | 4      | -      | -    | g    | -        | t    | +      | -     | -                      | -          | n          | -   | -        | -          | -     | e                                  | -                           | -                           | -                     | 11.933                             | 0.63                                 | 1.77                          | 1                             | 19.4  | 0.54 | 4.30 | 11.126  | 0.27  | 0.70   | 0.67  | 24.6 | 11.10 | 0.31  | 0.84   |
| 10345664-6743206 | 290.525  | -8.201   | 0.278  | 1      | -      | -    | g    | -        | -    | -      | -     | D1                     | -          | c          | o   | -        | h          | -     | -                                  | -                           | -                           | -                     | 11.299                             | 0.28                                 | 0.90                          | 1                             | 34.0  | 0.80 | 3.78 | 11.195  | 0.23  | 0.76   | 0.09  | 34.6 | 11.20 | 0.24  | 0.78   |
| 10353918-6356009 | 288.675  | -4.887   | 0.649  | 1      | -      | -    | g    | -        | -    | -      | -     | D3                     | -          | -          | -   | -        | h          | -     | -                                  | -                           | -                           | -                     | 11.080                             | 0.30                                 | 1.16                          |                               |       |      |      |         |       |        |       |      |       |       |        |



Table B1: a) continued.

| 2MASX J          |         | <i>l</i>    | <i>b</i>    | EBV        | Object       | Sample     |             |             |            | Disc        | 2MRS          | Velocity    |     | NIR          | Photom      | Ext          | <i>K</i> <sub>20</sub> | <i>H-K</i>   | <i>J-K</i> | <i>vc</i> | <i>a</i> | <i>b/a</i> | std.d. | <i>K</i> <sub>S</sub> <sup>o</sup> | ( <i>H-K</i> ) <sup>o</sup> | ( <i>J-K</i> ) <sup>o</sup> | <i>A<sub>K</sub></i> | <i>a</i> <sup>d</sup> | <i>K</i> <sub>S</sub> <sup>d,d</sup> | ( <i>H-K</i> ) <sup>o,c</sup> | ( <i>J-K</i> ) <sup>o,c</sup> |       |       |      |       |       |       |       |
|------------------|---------|-------------|-------------|------------|--------------|------------|-------------|-------------|------------|-------------|---------------|-------------|-----|--------------|-------------|--------------|------------------------|--------------|------------|-----------|----------|------------|--------|------------------------------------|-----------------------------|-----------------------------|----------------------|-----------------------|--------------------------------------|-------------------------------|-------------------------------|-------|-------|------|-------|-------|-------|-------|
| (1)              |         | deg<br>(2a) | deg<br>(2b) | mag<br>(3) | class<br>(4) | off<br>(5) | flag<br>(6) | gal<br>(7a) | TF<br>(7b) | obs<br>(7c) | ext'd<br>(7d) | type<br>(8) | (9) | Opt<br>(10a) | HI<br>(10b) | flag<br>(11) | flag<br>(12)           | flag<br>(13) |            |           | "        | (19)       | (20)   | mag<br>(21)                        | mag<br>(22)                 | mag<br>(23)                 | mag<br>(24)          | "                     | mag<br>(26)                          | mag<br>(27)                   | mag<br>(28)                   |       |       |      |       |       |       |       |
| 10443827-5937335 | 287.523 | -0.603      | 17.500      | 9          | -            | -          | -           | -           | -          | -           | -             | -           | -   | -            | -           | -            | -                      | -            | -          | -         | -        | -          | -      | 9.126                              | ...                         | 1.07                        | 1                    | 100.6                 | 0.22                                 | 4.50                          | 2.606                         | ...   | -7.62 | 5.42 | ...   | ...   | ...   | -6.47 |
| 10444166-5939426 | 287.546 | -0.631      | 16.928      | 9          | -            | -          | -           | -           | -          | -           | -             | -           | -   | -            | -           | -            | -                      | -            | -          | -         | -        | -          | -      | 7.243                              | 1.21                        | 1.43                        | 1                    | 149.6                 | 0.24                                 | 4.50                          | 0.936                         | -1.60 | -6.98 | 5.24 | ...   | ...   | -1.27 | -5.86 |
| 10450517-6403498 | 289.646 | -4.501      | 0.691       | 2          | -            | -          | -           | -           | -          | -           | -             | -           | -   | -            | -           | -            | -                      | -            | -          | -         | -        | -          | -      | 11.299                             | 0.44                        | 1.29                        | 1                    | 67.6                  | 0.56                                 | 4.10                          | 11.042                        | 0.33  | 0.95  | 0.21 | 72.6  | 11.01 | 0.34  | 1.00  |
| 10450780-5938118 | 287.582 | -0.583      | 15.467      | 9          | -            | -          | -           | g           | -          | -           | -             | -           | -   | -            | -           | -            | -                      | -            | -          | -         | -        | -          | -      | 7.208                              | 1.26                        | ...                         | 1                    | 108.0                 | 1.00                                 | 4.50                          | 1.445                         | -1.30 | ...   | 4.79 | ...   | ...   | -1.00 | ...   |
| 10455200-5956430 | 287.808 | -0.813      | 9.776       | 9          | -            | -          | -           | -           | -          | -           | -             | -           | -   | -            | -           | -            | -                      | -            | -          | -         | -        | -          | -      | 8.632                              | 1.02                        | ...                         | 1                    | 142.6                 | 0.16                                 | 4.50                          | 4.989                         | -0.60 | ...   | 3.03 | ...   | ...   | -0.41 | ...   |
| 10455227-5957030 | 287.811 | -0.818      | 9.677       | 9          | -            | -          | -           | -           | -          | -           | -             | -           | -   | -            | -           | -            | -                      | -            | -          | -         | -        | -          | -      | 8.335                              | 0.92                        | 1.84                        | 1                    | 107.6                 | 0.88                                 | 4.50                          | 4.729                         | -0.68 | -2.96 | 3.00 | ...   | ...   | -0.49 | -2.32 |
| 10455475-5956544 | 287.815 | -0.813      | 9.617       | 9          | -            | -          | -           | -           | -          | -           | -             | -           | -   | -            | -           | -            | -                      | -            | -          | -         | -        | -          | -      | 7.579                              | ...                         | 1.82                        | 1                    | 94.0                  | 1.00                                 | 4.50                          | 3.996                         | ...   | -2.96 | 2.98 | ...   | ...   | -2.33 | ...   |
| 10460008-6005119 | 287.888 | -0.931      | 8.079       | 7          | -            | -          | -           | -           | -          | -           | -             | -           | -   | -            | -           | -            | -                      | -            | -          | -         | -        | -          | -      | 9.896                              | 0.41                        | 1.04                        | 1                    | 38.4                  | 0.84                                 | 4.50                          | 6.886                         | -0.93 | -2.97 | 2.50 | ...   | ...   | -0.77 | -2.44 |
| 10472672-5915035 | 287.605 | -0.105      | 2.525       | 4          | -            | -          | -           | g           | -          | +           | -             | -           | -   | -            | -           | -            | -                      | -            | -          | -         | -        | -          | -      | 11.450                             | ...                         | ...                         | 1                    | 42.0                  | 0.80                                 | 4.40                          | 10.509                        | ...   | ...   | 0.78 | 57.8  | 10.41 | ...   | ...   |
| 10481009-6519282 | 290.525 | -5.466      | 0.524       | 1          | -            | -          | -           | -           | -          | -           | -             | -           | -   | -            | -           | -            | -                      | -            | -          | -         | -        | -          | -      | 10.993                             | 0.40                        | 1.22                        | 1                    | 34.8                  | 0.68                                 | 4.00                          | 10.798                        | 0.32  | 0.96  | 0.16 | 36.1  | 10.81 | 0.33  | 0.99  |
| 10481396-5318058 | 285.036 | 5.235       | 0.494       | 1          | -            | -          | -           | g           | -          | -           | -             | -           | -   | -            | -           | -            | -                      | -            | -          | -         | -        | -          | -      | 10.476                             | 0.34                        | 1.19                        | 1                    | 69.4                  | 0.34                                 | 3.84                          | 10.292                        | 0.26  | 0.94  | 0.15 | 71.7  | 10.30 | 0.26  | 0.97  |
| 10504178-6510408 | 290.695 | -5.215      | 0.569       | 1          | -            | -          | -           | g           | t          | -           | -             | -           | -   | -            | -           | -            | -                      | -            | -          | -         | -        | -          | -      | 10.808                             | 0.40                        | 1.35                        | 1                    | 57.8                  | 0.30                                 | 4.08                          | 10.596                        | 0.31  | 1.07  | 0.18 | 60.1  | 10.61 | 0.32  | 1.10  |
| 10506219-5611581 | 286.836 | -2.895      | 3.061       | 8          | -            | -          | -           | -           | -          | -           | -             | -           | -   | -            | -           | -            | -                      | -            | -          | -         | -        | -          | -      | 12.287                             | 1.00                        | ...                         | 1                    | 14.2                  | 0.64                                 | 4.12                          | 11.146                        | 0.95  | ...   | 0.95 | ...   | ...   | 1.01  | ...   |
| 10521528-5612424 | 286.869 | -2.897      | 3.357       | 8          | -            | -          | -           | -           | -          | -           | -             | -           | -   | -            | -           | -            | -                      | -            | -          | -         | -        | -          | -      | 9.488                              | 1.00                        | ...                         | 1                    | 92.6                  | 1.00                                 | 4.10                          | 8.237                         | 0.45  | ...   | 1.04 | ...   | ...   | 0.51  | ...   |
| 10534560-6250026 | 289.955 | -2.966      | 0.857       | 2          | -            | -          | -           | g           | -          | -           | -             | -           | -   | -            | -           | -            | -                      | -            | -          | -         | -        | -          | -      | 10.196                             | 0.43                        | 1.53                        | 1                    | 97.2                  | 0.54                                 | 4.27                          | 9.877                         | 0.29  | 1.10  | 0.27 | 105.3 | 9.86  | 0.30  | 1.16  |
| 10542476-5738299 | 287.762 | 1.742       | 0.828       | 1          | -            | -          | -           | g           | -          | -           | P             | -           | -   | -            | -           | -            | -                      | -            | -          | -         | -        | -          | -      | 10.702                             | 0.42                        | 1.44                        | 1                    | 45.4                  | 0.58                                 | 4.25                          | 10.393                        | 0.28  | 1.02  | 0.26 | 48.4  | 10.41 | 0.30  | 1.08  |
| 10543287-5939178 | 288.653 | -0.064      | 4.262       | 6          | -            | -          | -           | g           | -          | -           | -             | -           | -   | -            | -           | -            | -                      | -            | -          | -         | -        | -          | -      | 10.468                             | ...                         | ...                         | 1                    | 55.2                  | 1.00                                 | 4.40                          | 8.880                         | ...   | ...   | 1.32 | ...   | ...   | ...   | ...   |
| 10561182-6012555 | 289.081 | -0.480      | 7.601       | 7          | -            | -          | -           | -           | -          | -           | -             | -           | -   | -            | -           | -            | -                      | -            | -          | -         | -        | -          | -      | 10.979                             | 0.91                        | ...                         | 1                    | 20.6                  | 0.82                                 | 4.48                          | 8.147                         | -0.35 | ...   | 2.35 | ...   | ...   | -0.20 | ...   |
| 10562081-5033367 | 284.935 | 8.246       | 0.299       | 1          | -            | -          | -           | g           | t          | -           | -             | -           | -   | -            | -           | -            | -                      | -            | -          | -         | -        | -          | -      | 8.737                              | 0.33                        | 1.08                        | 1                    | 94.0                  | 0.50                                 | 3.66                          | 8.626                         | 0.28  | 0.93  | 0.09 | 95.2  | 8.64  | 0.29  | 0.95  |
| 10562669-6008575 | 289.081 | -0.407      | 16.224      | 9          | -            | -          | -           | -           | -          | -           | -             | -           | -   | -            | -           | -            | -                      | -            | -          | -         | -        | -          | -      | 11.524                             | ...                         | ...                         | 1                    | 23.4                  | 0.36                                 | 4.48                          | 5.479                         | ...   | ...   | 5.03 | ...   | ...   | ...   | ...   |
| 10562790-6009194 | 289.086 | -0.411      | 15.479      | 9          | -            | -          | -           | -           | -          | -           | -             | -           | -   | -            | -           | -            | -                      | -            | -          | -         | -        | -          | -      | 11.197                             | ...                         | ...                         | 1                    | 34.4                  | 0.32                                 | 4.48                          | 5.430                         | ...   | ...   | 4.79 | ...   | ...   | ...   | ...   |
| 10563215-6006074 | 289.071 | -0.359      | 21.007      | 8          | -            | -          | -           | -           | -          | -           | -             | -           | -   | -            | -           | -            | -                      | -            | -          | -         | -        | -          | -      | 9.573                              | ...                         | ...                         | -2                   | 88.6                  | 0.52                                 | 4.48                          | 1.746                         | ...   | ...   | 6.51 | ...   | ...   | ...   | ...   |
| 10563522-6005184 | 289.071 | -0.344      | 20.495      | 8          | -            | -          | -           | -           | -          | -           | -             | -           | -   | -            | -           | -            | -                      | -            | -          | -         | -        | -          | -      | 8.001                              | 0.71                        | ...                         | 1                    | 182.6                 | 0.72                                 | 4.48                          | 0.365                         | -2.68 | ...   | 6.35 | ...   | ...   | -2.28 | ...   |
| 10564154-5838289 | 288.464 | 0.970       | 3.413       | 8          | -            | -          | -           | -           | -          | -           | -             | -           | -   | -            | -           | -            | -                      | -            | -          | -         | -        | -          | -      | 10.244                             | 0.92                        | 1.96                        | 1                    | 54.2                  | 0.88                                 | 4.33                          | 8.972                         | 0.35  | 0.26  | 1.06 | ...   | ...   | 0.42  | 0.49  |
| 10565639-5836539 | 288.482 | 1.007       | 3.669       | 8          | -            | -          | -           | -           | -          | -           | -             | -           | -   | -            | -           | -            | -                      | -            | -          | -         | -        | -          | -      | 9.782                              | 0.76                        | 1.70                        | 1                    | 87.6                  | 0.52                                 | 4.33                          | 8.415                         | 0.15  | -0.12 | 1.14 | ...   | ...   | 0.22  | 0.12  |
| 10565727-5000028 | 284.779 | 8.792       | 0.316       | 1          | -            | -          | -           | g           | -          | -           | -             | -           | -   | -            | -           | -            | -                      | -            | -          | -         | -        | -          | -      | 10.978                             | 0.31                        | 1.15                        | 1                    | 34.4                  | 0.72                                 | 3.59                          | 10.860                        | 0.26  | 0.99  | 0.10 | 35.1  | 10.87 | 0.26  | 1.01  |
| 10570368-5901494 | 288.674 | 0.638       | 1.748       | 8          | -            | -          | -           | -           | -          | -           | -             | -           | -   | -            | -           | -            | -                      | -            | -          | -         | -        | -          | -      | 11.335                             | ...                         | ...                         | 1                    | 45.0                  | 0.28                                 | 4.37                          | 10.684                        | ...   | ...   | 0.54 | ...   | ...   | ...   | ...   |
| 10570410-5902028 | 288.676 | 0.635       | 1.737       | 8          | -            | -          | -           | -           | -          | -           | -             | -           | -   | -            | -           | -            | -                      | -            | -          | -         | -        | -          | -      | 10.457                             | 0.81                        | 1.71                        | 1                    | 57.0                  | 0.48                                 | 4.39                          | 9.810                         | 0.52  | 0.85  | 0.54 | ...   | ...   | 0.55  | 0.96  |
| 10570730-6007128 | 289.145 | -0.345      | 11.827      | 7          | -            | -          | -           | -           | -          | -           | -             | -           | -   | -            | -           | -            | -                      | -            | -          | -         | -        | -          | -      | 10.954                             | 0.85                        | ...                         | 1                    | 30.6                  | 0.76                                 | 4.45                          | 6.547                         | -1.11 | ...   | 3.66 | ...   | ...   | -0.88 | ...   |
| 10571761-5015269 | 284.940 | 8.584       | 0.283       | 1          | -            | -          | -           | g           | -          | -           | -             | -           | -   | -            | -           | -            | -                      | -            | -          | -         | -        | -          | -      | 10.456                             | 0.28                        | 0.89                        | 1                    | 40.2                  | 0.82                                 | 3.60                          | 10.351                        | 0.23  | 0.75  | 0.09 | 40.7  | 10.36 | 0.24  | 0.77  |
| 10572544-6253028 | 290.354 | -2.831      | 2.392       | 8          | -            | -          | -           | -           | -          | -           | -             | -           | -   | -            | -           | -            | -                      | -            | -          | -         | -        | -          | -      | 10.046                             | 0.91                        | 2.12                        | 1                    | 60.0                  | 0.66                                 | 4.28                          | 9.155                         | 0.51  | 0.93  | 0.74 | ...   | ...   | 0.56  | 1.09  |
| 10573282-6258508 | 290.407 | -2.912      | 3.223       | 8          | -            | -          | -           | -           | -          | -           | -             | -           | -   | -            | -           | -            | -                      | -            | -          | -         | -        | -          | -      | 10.299                             | 0.83                        | 1.60                        | -2                   | 57.0                  | 0.62                                 | 4.28                          | 9.098                         | 0.30  | -0.01 | 1.00 | ...   | ...   | 0.36  | 0.21  |
| 10573752-6005347 | 289.190 | -0.293      | 8.110       | 8          | -            | -          | -           | -           | -          | -           | -             | -           | -   | -            | -           | -            | -                      | -            | -          | -         | -        | -          | -      | 10.754                             | ...                         | ...                         | 1                    | 43.6                  | 0.56                                 | 4.45                          | 7.732                         | ...   | ...   | 2.51 | ...   | ...   | ...   | ...   |
| 10580539-5030289 | 285.165 | 8.412       | 0.311       | 1          | -            | -          | -           | g           | -          | -           | -             | -           | -   | -            | -           | -            | -                      | -            | -          | -         | -        | -          | -      | 9.605                              | 0.26                        | 0.95                        | 1                    | 52.2                  | 0.56                                 | 3.64                          | 9.489                         | 0.21  | 0.80  | 0.10 | 52.9  | 9.50  | 0.21  | 0.82  |
| 10581260-5026359 | 285.154 | 8.479       | 0.287       | 1          | -            | -          | -           | -           | -          | -           | -             | -           | -   | -            | -           | -            | -                      | -            | -          | -         | -        | -          | -      | 9.723                              | 0.25                        | 1.04                        | 1                    | 80.8                  | 0.58                                 | 3.65                          | 9.616                         | 0.20  | 0.89  | 0.09 | 82.0  | 9.63  | 0.21  | 0.91  |
| 10581325-5026492 | 285.157 | 8.476       | 0.288       | 9          | -            | -          | -           | e           | -          | -           | -             | -           | -   | -            | -           | -            | -                      | -            | -          | -         | -        | -          | -      | 10.131                             | 0.25                        | 1.03                        | 1                    | 87.4                  | 0.52                                 | 3.64                          | 10.024                        | 0.20  | 0.89  | 0.09 | ...   | ...   | 0.21  | 0.91  |
| 10581534-4925258 | 284.720 | 9.404       | 0.339       | 1          | -            | -          | -           | g           | -          | -           | -             | -           | -   | -            | -           | -            | -                      | -            | -          | -         | -        | -          | -      | 9.665                              | 0.29                        | 1.10                        | 1                    | 52.0                  | 0.86                                 | 3.56                          | 9.539                         | 0.24  | 0.94  | 0.11 | 52.8  | 9.55  | 0.25  | 0.96  |
| 10581564-5046208 | 285.303 | 8.185       | 0.352       | 1          | -            | -          | -           | g           | -          | -           | -             | -           | -   | -            | -           | -            | -                      | -            | -          | -         | -        | -          | -      | 11.008                             | 0.29                        | 1.09                        | 1                    | 41.2                  | 0.66                                 | 3.73                          | 10.877                        | 0.23  | 0.91  | 0.11 | 42.1  | 10.88 | 0.23  | 0.94  |
| 10582296-5015353 | 285.100 | 8.657       | 0.278       | 1          | -            | -          | -           | g           | -          | -           | -             | -           | -   | -            | -           | -            | -                      | -            | -          | -         | -        | -          | -      | 11.015                             | 0.30                        | 1.09                        | 1                    | 30.2                  | 0.74                                 | 3.66                          | 10.911                        | 0.25  | 0.96  | 0.09 | 30.6  | 10.92 | 0.26  | 0.97  |
| 10583884-6450448 | 291.309 | -4.551      | 0.625       | 1          | -            | -          | -           | g           | -          | -           | -             | -           | -   | -            | -           | -            | -                      | -            | -          | -         | -        | -          | -      | 10.279                             | 0.37                        | 1.29                        | 1                    | 43.6                  | 0.64                                 | 4.14                          | 10.046                        | 0.27  | 0.98  | 0.19 | 45.4  | 10.06 | 0.28  | 1.02  |
| 10584051-6111078 | 289.768 | -1.229      | 11.686      | 8          | -            | -          | -           | -           | -          | -           | -             | -           | -   | -            | -           | -            | -                      | -            | -          | -         | -        | -          | -      | 8.772                              | 0.37                        | 1.05                        | 1                    | 135.8                 | 0.66                                 | 4.48                          | 4.418                         | -1.57 | -4.76 | 3.62 | ...   | ...   | -1.34 | -3.99 |
| 10584287-5019294 | 285.177 | 8.620       | 0.285       | 1          | -            | -          | -           | g           | t          | -           | -             | -           | -   | -            | -           | -            | -                      | -            | -          | -         | -        | -          | -      | 10.036                             | 0.37                        | 1.27                        |                      |                       |                                      |                               |                               |       |       |      |       |       |       |       |

Table B1: a) continued.

| 2MASX J          | <i>l</i> | <i>b</i> | EBV    | Object | Sample | Disc | 2MRS | Velocity | NIR  | Photom | Ext  | <i>K</i> <sub>20</sub> | <i>H-K</i> | <i>J-K</i> | vc   | <i>a</i> | <i>b/a</i> | st.d. | <i>K</i> <sub>s</sub> <sup>o</sup> | ( <i>H-K</i> ) <sup>o</sup> | ( <i>J-K</i> ) <sup>o</sup> | <i>A</i> <sub>K</sub> | <i>a</i> <sub>d</sub> <sup>o</sup> | <i>K</i> <sub>s</sub> <sup>o,d</sup> | ( <i>H-K</i> ) <sup>o,c</sup> | ( <i>J-K</i> ) <sup>o,c</sup> |       |        |       |       |       |       |        |
|------------------|----------|----------|--------|--------|--------|------|------|----------|------|--------|------|------------------------|------------|------------|------|----------|------------|-------|------------------------------------|-----------------------------|-----------------------------|-----------------------|------------------------------------|--------------------------------------|-------------------------------|-------------------------------|-------|--------|-------|-------|-------|-------|--------|
| (1)              | deg      | deg      | mag    | class  | off    | flag | gal  | TF       | obs  | ext'd  | type | (9)                    | Opt        | HI         | flg  | flg      | flg        | flg   | mag                                | mag                         | mag                         | mag                   | mag                                | mag                                  | mag                           | mag                           | mag   |        |       |       |       |       |        |
| (1)              | (2a)     | (2b)     | (3)    | (4)    | (5)    | (6)  | (7a) | (7b)     | (7c) | (7d)   | (8)  | (9)                    | (10a)      | (10b)      | (11) | (12)     | (13)       | (14)  | (15)                               | (16)                        | (17)                        | (18)                  | (19)                               | (20)                                 | (21)                          | (22)                          | (23)  | (24)   | (25)  | (26)  | (27)  | (28)  |        |
| 11121313-6116497 | 291.301  | -0.669   | 44.852 | 9      | -      | -    | -    | -        | -    | -      | -    | -                      | -          | -          | -    | -        | -          | -     | 7.798                              | 1.20                        | 1.66                        | 1                     | 219.8                              | 0.38                                 | 4.52                          | -8.914                        | -6.23 | -20.62 | 13.89 | ...   | ...   | -5.35 | -17.66 |
| 11121544-6116387 | 291.304  | -0.665   | 42.183 | 9      | -      | -    | -    | -        | -    | -      | -    | -                      | -          | -          | -    | -        | -          | -     | 8.094                              | 1.29                        | 1.90                        | 1                     | 144.8                              | 0.68                                 | 4.46                          | -7.623                        | -5.70 | -19.06 | 13.07 | ...   | ...   | -4.87 | -16.27 |
| 11121717-5846307 | 290.374  | 1.658    | 4.986  | 8      | -      | -    | -    | -        | -    | -      | -    | -                      | -          | -          | -    | -        | -          | -     | 7.915                              | 0.77                        | 1.73                        | 1                     | 129.6                              | 0.56                                 | 4.35                          | 6.057                         | -0.06 | -0.74  | 1.54  | ...   | ...   | 0.04  | -0.41  |
| 11122130-6053218 | 291.170  | -0.301   | 6.313  | 9      | -      | -    | -    | -        | -    | -      | -    | -                      | -          | -          | -    | -        | -          | -     | 11.074                             | ...                         | ...                         | 1                     | 31.4                               | 0.80                                 | 4.55                          | 8.722                         | ...   | ...    | 1.96  | ...   | ...   | ...   | ...    |
| 11122885-6121409 | 294.378  | -8.039   | 19.188 | 9      | -      | -    | -    | -        | -    | -      | -    | -                      | -          | -          | -    | -        | -          | -     | 8.893                              | 0.87                        | 1.47                        | 1                     | 175.0                              | 0.20                                 | 4.46                          | 1.744                         | -2.31 | -8.07  | 5.94  | ...   | ...   | -1.93 | -6.80  |
| 11122969-6120319 | 291.355  | -0.714   | 24.384 | 9      | -      | -    | -    | -        | -    | -      | -    | -                      | -          | -          | -    | -        | -          | -     | 8.564                              | ...                         | 1.43                        | 1                     | 192.0                              | 0.14                                 | 4.46                          | -0.521                        | ...   | -10.68 | 7.55  | ...   | ...   | ...   | -9.07  |
| 11130773-6915419 | 294.378  | -8.039   | 0.223  | 1      | o      | -    | -    | -        | -    | -      | D1   | c                      | o          | h          | -    | o        | -          | -     | 10.878                             | 0.13                        | 0.85                        | 1                     | 50.8                               | 1.00                                 | 3.81                          | 10.795                        | 0.10  | 0.74   | 0.07  | 51.6  | 10.79 | 0.10  | 0.76   |
| 11131304-6732029 | 293.736  | -6.433   | 0.328  | 1      | -      | -    | -    | -        | -    | -      | D1   | c                      | o          | -          | -    | -        | -          | -     | 10.901                             | 0.32                        | 1.16                        | 1                     | 37.2                               | 0.70                                 | 3.95                          | 10.779                        | 0.26  | 1.00   | 0.10  | 37.9  | 10.79 | 0.27  | 1.02   |
| 11144901-6152080 | 291.806  | -1.102   | 2.475  | 9      | -      | -    | -    | -        | -    | -      | -    | -                      | -          | -          | -    | -        | -          | -     | 11.535                             | ...                         | ...                         | 1                     | 24.6                               | 0.34                                 | 4.45                          | 10.613                        | ...   | ...    | 0.77  | ...   | ...   | ...   | ...    |
| 11145099-6117060 | 291.597  | -0.557   | 47.392 | 9      | -      | -    | -    | -        | -    | -      | -    | -                      | -          | -          | -    | -        | -          | -     | 7.800                              | 1.17                        | 1.56                        | 1                     | 113.4                              | 0.56                                 | 4.58                          | -9.858                        | -6.68 | -21.99 | 14.68 | ...   | ...   | -5.75 | -18.86 |
| 11145278-6115160 | 291.589  | -0.527   | 54.189 | 9      | -      | -    | -    | -        | -    | -      | -    | -                      | -          | -          | -    | -        | -          | -     | 6.887                              | 1.09                        | 1.60                        | 1                     | 219.8                              | 0.46                                 | 4.58                          | -13.304                       | -7.89 | -25.32 | 16.79 | ...   | ...   | -6.82 | -21.75 |
| 11145568-6114010 | 291.587  | -0.506   | 53.293 | 9      | -      | -    | -    | -        | -    | -      | -    | -                      | -          | -          | -    | -        | -          | -     | 6.309                              | 1.48                        | 2.89                        | 1                     | 113.8                              | 0.84                                 | 4.58                          | -13.548                       | -7.35 | -23.58 | 16.51 | ...   | ...   | -6.30 | -20.07 |
| 11145678-6112570 | 291.582  | -0.488   | 51.446 | 9      | -      | -    | -    | -        | -    | -      | -    | -                      | -          | -          | -    | -        | -          | -     | 8.679                              | ...                         | ...                         | 1                     | 50.4                               | 0.32                                 | 4.58                          | -10.490                       | ...   | ...    | 15.94 | ...   | ...   | ...   | ...    |
| 11145954-6111409 | 291.580  | -0.467   | 47.739 | 9      | -      | -    | -    | -        | -    | -      | -    | -                      | -          | -          | -    | -        | -          | -     | 7.645                              | 1.33                        | 2.69                        | 1                     | 216.4                              | 0.48                                 | 4.49                          | -10.143                       | -6.57 | -21.03 | 14.79 | ...   | ...   | -5.63 | -17.88 |
| 11150063-6108239 | 291.562  | -0.415   | 30.707 | 9      | -      | -    | -    | -        | -    | -      | -    | -                      | -          | -          | -    | -        | -          | -     | 9.778                              | ...                         | ...                         | 1                     | 48.6                               | 0.66                                 | 4.49                          | -1.663                        | ...   | ...    | 9.51  | ...   | ...   | ...   | ...    |
| 11150083-6115539 | 291.608  | -0.531   | 56.620 | 9      | -      | -    | -    | -        | -    | -      | -    | -                      | -          | -          | -    | -        | -          | -     | 7.414                              | 0.93                        | 1.41                        | 1                     | 101.2                              | 0.30                                 | 4.58                          | -13.683                       | -8.45 | -26.72 | 17.54 | ...   | ...   | -7.34 | -22.98 |
| 11150125-6116439 | 291.613  | -0.544   | 54.010 | 9      | -      | -    | -    | -        | -    | -      | -    | -                      | -          | -          | -    | -        | -          | -     | 6.473                              | 1.07                        | 1.64                        | 1                     | 159.0                              | 0.80                                 | 4.58                          | -13.651                       | -7.88 | -25.19 | 16.73 | ...   | ...   | -6.82 | -21.63 |
| 11150292-6117399 | 291.622  | -0.557   | 52.388 | 9      | -      | -    | -    | -        | -    | -      | -    | -                      | -          | -          | -    | -        | -          | -     | 7.269                              | ...                         | ...                         | 1                     | 188.2                              | 0.40                                 | 4.58                          | -12.251                       | ...   | ...    | 16.23 | ...   | ...   | ...   | ...    |
| 11150301-6112229 | 291.590  | -0.475   | 51.326 | 9      | -      | -    | -    | -        | -    | -      | -    | -                      | -          | -          | -    | -        | -          | -     | 8.157                              | 1.54                        | ...                         | 1                     | 118.6                              | 0.44                                 | 4.49                          | -10.967                       | -6.96 | ...    | 15.90 | ...   | ...   | -5.95 | ...    |
| 11150441-6113369 | 291.600  | -0.493   | 54.957 | 9      | -      | -    | -    | -        | -    | -      | -    | -                      | -          | -          | -    | -        | -          | -     | 6.872                              | 1.35                        | 2.43                        | 1                     | 220.0                              | 0.30                                 | 4.58                          | -13.605                       | -7.75 | -24.87 | 17.02 | ...   | ...   | -6.67 | -21.25 |
| 11150567-6115129 | 291.613  | -0.517   | 58.094 | 9      | -      | -    | -    | -        | -    | -      | -    | -                      | -          | -          | -    | -        | -          | -     | 8.055                              | 0.83                        | ...                         | 1                     | 101.8                              | 1.00                                 | 4.58                          | -13.591                       | -8.79 | ...    | 17.99 | ...   | ...   | -7.65 | ...    |
| 11150769-6114357 | 291.613  | -0.506   | 57.871 | 9      | -      | -    | -    | -        | -    | -      | -    | -                      | -          | -          | -    | -        | -          | -     | 7.246                              | 1.23                        | 2.35                        | 1                     | 145.2                              | 0.82                                 | 4.57                          | -14.317                       | -8.35 | -26.40 | 17.93 | ...   | ...   | -7.22 | -22.58 |
| 11151028-6117368 | 291.636  | -0.551   | 55.904 | 9      | -      | -    | -    | -        | -    | -      | -    | -                      | -          | -          | -    | -        | -          | -     | 7.533                              | ...                         | ...                         | 1                     | 94.0                               | 1.00                                 | 4.58                          | -13.297                       | ...   | ...    | 17.32 | ...   | ...   | ...   | ...    |
| 11151056-6116197 | 291.628  | -0.531   | 56.270 | 9      | -      | -    | -    | -        | -    | -      | -    | -                      | -          | -          | -    | -        | -          | -     | 5.545                              | 0.92                        | 1.57                        | 1                     | 149.8                              | 0.92                                 | 4.57                          | -15.421                       | -8.40 | -26.38 | 17.43 | ...   | ...   | -7.30 | -22.67 |
| 11151111-6117117 | 291.635  | -0.544   | 56.247 | 9      | -      | -    | -    | -        | -    | -      | -    | -                      | -          | -          | -    | -        | -          | -     | 6.825                              | 1.36                        | 2.22                        | 1                     | 118.6                              | 0.44                                 | 4.57                          | -14.133                       | -7.95 | -25.72 | 17.42 | ...   | ...   | -6.85 | -22.01 |
| 11153026-6116469 | 291.668  | -0.524   | 46.414 | 9      | -      | -    | -    | -        | -    | -      | -    | -                      | -          | -          | -    | -        | -          | -     | 9.375                              | 0.76                        | 1.20                        | 1                     | 51.0                               | 0.76                                 | 4.57                          | -7.919                        | -6.92 | -21.86 | 14.38 | ...   | ...   | -6.01 | -18.80 |
| 11160973-5534122 | 289.685  | 4.832    | 0.635  | 1      | -      | -    | -    | -        | -    | -      | D4   | -                      | -          | -          | -    | -        | -          | -     | 11.271                             | 0.48                        | 1.32                        | 1                     | 27.8                               | 0.84                                 | 3.94                          | 11.034                        | 0.37  | 1.01   | 0.20  | 29.1  | 11.05 | 0.38  | 1.05   |
| 11163055-6129363 | 291.857  | -0.680   | 4.539  | 9      | -      | -    | -    | -        | -    | -      | -    | -                      | -          | -          | -    | -        | -          | -     | 8.262                              | ...                         | 1.68                        | 1                     | 133.4                              | 1.00                                 | 4.50                          | 6.571                         | ...   | -0.57  | 1.41  | ...   | ...   | ...   | -0.27  |
| 11163348-6130193 | 291.867  | -0.689   | 3.992  | 9      | -      | -    | -    | -        | -    | -      | -    | -                      | -          | -          | -    | -        | -          | -     | 8.810                              | 1.27                        | ...                         | 1                     | 107.6                              | 0.28                                 | 4.50                          | 7.323                         | 0.60  | ...    | 1.24  | ...   | ...   | 0.68  | ...    |
| 11163530-6129503 | 291.867  | -0.680   | 4.216  | 9      | -      | -    | -    | -        | -    | -      | -    | -                      | -          | -          | -    | -        | -          | -     | 11.452                             | ...                         | ...                         | 1                     | 37.0                               | 0.12                                 | 4.50                          | 9.881                         | ...   | ...    | 1.31  | ...   | ...   | ...   | ...    |
| 11171671-6040432 | 291.653  | 0.115    | 0.204  | 3      | -      | -    | -    | -        | -    | -      | -    | n                      | -          | -          | -    | -        | -          | -     | 10.803                             | 0.73                        | ...                         | 1                     | 38.6                               | 0.86                                 | 4.49                          | 10.727                        | 0.70  | ...    | 0.06  | 39.0  | 10.74 | 0.71  | ...    |
| 11192831-5222177 | 288.997  | 7.994    | 0.267  | 1      | -      | -    | -    | -        | -    | -      | D1   | c                      | o          | -          | -    | -        | -          | -     | 9.596                              | 0.29                        | 1.05                        | 1                     | 101.2                              | 0.42                                 | 3.65                          | 9.497                         | 0.25  | 0.92   | 0.08  | 102.4 | 9.51  | 0.26  | 0.93   |
| 11210707-5959443 | 291.860  | 0.920    | 0.663  | 8      | -      | -    | -    | -        | -    | -      | -    | c                      | o          | -          | -    | -        | -          | -     | 11.059                             | 0.37                        | 1.14                        | 1                     | 21.2                               | 0.54                                 | 4.40                          | 10.812                        | 0.26  | 0.81   | 0.21  | ...   | ...   | 0.27  | 0.85   |
| 11211523-5030020 | 288.601  | 9.845    | 0.235  | 1      | -      | -    | -    | -        | -    | -      | D1   | c                      | o          | -          | -    | -        | -          | -     | 11.237                             | 0.28                        | 1.00                        | 1                     | 30.6                               | 0.48                                 | 3.58                          | 11.149                        | 0.24  | 0.88   | 0.07  | 31.0  | 11.16 | 0.25  | 0.89   |
| 11235407-6221537 | 292.974  | -1.198   | 3.874  | 9      | -      | -    | -    | -        | -    | -      | -    | -                      | -          | -          | -    | -        | -          | -     | 7.848                              | 1.54                        | ...                         | -2                    | 44.6                               | 0.38                                 | 3.44                          | 6.405                         | 0.90  | ...    | 1.20  | ...   | ...   | 0.98  | ...    |
| 11240570-6443368 | 293.779  | -3.419   | 1.445  | 1      | -      | -    | -    | -        | -    | -      | D2   | -                      | -          | -          | -    | -        | -          | -     | 10.104                             | 0.44                        | 1.53                        | 1                     | 38.0                               | 0.92                                 | 4.24                          | 9.566                         | 0.20  | 0.81   | 0.45  | 42.8  | 9.59  | 0.23  | 0.91   |
| 11240763-6121528 | 292.668  | -0.245   | 3.367  | 2      | -      | -    | -    | -        | -    | -      | D1   | -                      | -          | -          | h    | -        | -          | -     | 10.406                             | 0.72                        | ...                         | 1                     | 56.4                               | 0.46                                 | 4.52                          | 9.151                         | 0.16  | ...    | 1.04  | 84.1  | 9.09  | 0.23  | ...    |
| 11241726-6204009 | 292.918  | -0.902   | 6.550  | 7      | -      | -    | -    | -        | -    | -      | -    | -                      | -          | -          | -    | -        | -          | -     | 10.482                             | 1.41                        | ...                         | 1                     | 40.0                               | 0.44                                 | 4.44                          | 8.041                         | 0.33  | ...    | 2.03  | ...   | ...   | 0.46  | ...    |
| 11241873-5842533 | 291.813  | 2.263    | 0.847  | 1      | -      | -    | -    | -        | -    | -      | D1   | -                      | -          | -          | -    | -        | -          | -     | 10.945                             | 0.44                        | 1.37                        | 1                     | 50.2                               | 0.52                                 | 4.28                          | 10.629                        | 0.30  | 0.95   | 0.26  | 53.9  | 10.63 | 0.32  | 1.01   |
| 11244274-5856439 | 291.938  | 2.063    | 2.311  | 9      | -      | -    | -    | -        | -    | -      | -    | -                      | -          | -          | -    | -        | -          | -     | 10.982                             | 0.91                        | ...                         | 1                     | 54.8                               | 0.34                                 | 4.29                          | 10.121                        | 0.53  | ...    | 0.72  | ...   | ...   | 0.57  | ...    |
| 11244871-6213267 | 293.028  | -1.030   | 10.468 | 9      | -      | -    | -    | -        | -    | -      | -    | -                      | -          | -          | -    | -        | -          | -     | 9.362                              | 1.63                        | ...                         | 1                     | 121.2                              | 0.50                                 | 4.44                          | 5.462                         | -0.11 | ...    | 3.24  | ...   | ...   | 0.10  | ...    |
| 11253134-6326121 | 293.501  | -2.149   | 2.551  | 9      | -      | -    | -    | -        | -    | -      | -    | -                      | -          | -          | -    | -        | -          | -     | 11.891                             | ...                         | ...                         | -2                    | 36.4                               | 0.36                                 | 4.34                          | 10.940                        | ...   | ...    | 0.79  | ...   | ...   | ...   | ...    |
| 11260854-5414089 | 290.579  | 6.577    | 0.271  | 1      | -      | -    | -    | -        | -    | -      | D1   | c                      | o          | h          | -    | -        | -          | -     | 9.942                              | 0.28                        | 1.03                        | 1                     | 84.0                               | 0.36                                 | 3.79                          | 9.841                         | 0.24  | 0.89   | 0.08  | 85.2  | 9.85  | 0.24  | 0.91   |
| 11263836-6820380 | 295.209  | -6.753   | 0.414  | 1      | -      | -    | -    | -        | -    | -      | D1   | c                      | o          | -          | -    | -        | -          | -     | 11.384                             | 0.33                        | 1.08                        | 1                     | 24.2                               | 0.86                                 | 3.93                          | 11.230                        | 0.26  | 0.88   | 0.13  | 24.9  | 11.23 | 0.27  | 0.90   |
| 11264117-5415209 | 290.661  | 6.584    | 0.273  | 1      | -      | -    | -    | -        | -    | -      | D1   | c                      | o          | h          | -    | -        | -          | -     | 10.584                             | 0.39                        | 1.26                        | 1                     |                                    |                                      |                               |                               |       |        |       |       |       |       |        |

Table B1: a) continued.

| 2MASX J          |         | <i>l</i>    | <i>b</i>    | EBV        | Object       |            |             | Sample      |            |             | Disc          | 2MRS        | Velocity |              | NIR         | Photom       | Ext          | <i>K</i> <sub>20</sub> | <i>H-K</i>  | <i>J-K</i>  | <i>vc</i>   | <i>a</i> | <i>b/a</i> | std. | <i>K</i> <sub>S</sub> <sup>o</sup> | <i>(H-K)</i> <sup>o</sup> | <i>(J-K)</i> <sup>o</sup> | <i>A<sub>K</sub></i> | <i>a</i> <sup>d</sup> | <i>K</i> <sub>S</sub> <sup>o,d</sup> | <i>(H-K)</i> <sup>o,c</sup> | <i>(J-K)</i> <sup>o,c</sup> |             |
|------------------|---------|-------------|-------------|------------|--------------|------------|-------------|-------------|------------|-------------|---------------|-------------|----------|--------------|-------------|--------------|--------------|------------------------|-------------|-------------|-------------|----------|------------|------|------------------------------------|---------------------------|---------------------------|----------------------|-----------------------|--------------------------------------|-----------------------------|-----------------------------|-------------|
| (1)              |         | deg<br>(2a) | deg<br>(2b) | mag<br>(3) | class<br>(4) | off<br>(5) | flag<br>(6) | gal<br>(7a) | TF<br>(7b) | obs<br>(7c) | ext'd<br>(7d) | type<br>(8) | (9)      | Opt<br>(10a) | HI<br>(10b) | flag<br>(11) | flag<br>(12) | flag<br>(13)           | mag<br>(14) | mag<br>(15) | mag<br>(16) | (17)     | "<br>(18)  | (19) | (20)                               | mag<br>(21)               | mag<br>(22)               | mag<br>(23)          | mag<br>(24)           | "<br>(25)                            | mag<br>(26)                 | mag<br>(27)                 | mag<br>(28) |
| 11391307-6329013 | 294.975 | -1.733      | 19.883      | 9          | -            | -          | -           | -           | -          | -           | -             | -           | -        | -            | -           | -            | -            | -                      | 9.903       | 1.43        | ...         | 1        | 51.6       | 0.70 | 4.51                               | 2.495                     | -1.86                     | ...                  | 6.16                  | ...                                  | ...                         | -1.47                       | ...         |
| 11391632-5333132 | 292.229 | 7.812       | 0.223       | 1          | -            | -          | -           | g           | t          | -           | -             | D1          | c        | -            | h           | V            | -            | -                      | 11.169      | 0.49        | 1.44        | 1        | 42.6       | 0.32 | 3.76                               | 11.086                    | 0.45                      | 1.33                 | 0.07                  | 43.1                                 | 11.09                       | 0.46                        | 1.35        |
| 11392277-6328212 | 294.989 | -1.718      | 19.408      | 9          | -            | -          | -           | g           | -          | -           | -             | D3          | c        | o            | -           | -            | -            | -                      | 9.741       | ...         | ...         | 1        | 54.6       | 0.46 | 4.51                               | 2.510                     | ...                       | ...                  | 6.01                  | ...                                  | ...                         | ...                         | ...         |
| 11400676-5141418 | 291.832 | 9.633       | 0.223       | 1          | -            | -          | -           | g           | -          | -           | -             | D3          | c        | o            | -           | -            | -            | -                      | 11.54       | 0.33        | 1.05        | 1        | 40.6       | 0.92 | 3.65                               | 11.071                    | 0.29                      | 0.94                 | 0.07                  | 41.1                                 | 11.08                       | 0.30                        | 0.95        |
| 11402953-6327520 | 295.107 | -1.676      | 11.920      | 9          | -            | -          | -           | g           | -          | -           | -             | D1          | c        | o            | -           | -            | -            | -                      | 9.025       | 1.31        | ...         | 1        | 102.0      | 0.40 | 4.45                               | 4.584                     | -0.67                     | ...                  | 3.69                  | ...                                  | ...                         | -0.43                       | ...         |
| 11403915-5552004 | 293.063 | 5.643       | 0.475       | 1          | -            | o          | -           | g           | -          | -           | -             | D1          | c        | o            | -           | -            | -            | -                      | 11.277      | 0.30        | 1.07        | 1        | 25.6       | 0.90 | 3.91                               | 11.100                    | 0.22                      | 0.84                 | 0.15                  | 26.4                                 | 11.11                       | 0.23                        | 0.87        |
| 11404801-6907434 | 296.679 | -7.119      | 0.359       | 1          | -            | -          | -           | g           | t          | -           | -             | D1          | c        | o            | -           | -            | -            | -                      | 11.191      | 0.33        | 1.16        | 1        | 39.8       | 0.28 | 3.86                               | 11.057                    | 0.27                      | 0.98                 | 0.11                  | 40.6                                 | 11.07                       | 0.28                        | 1.00        |
| 11412204-5130349 | 291.971 | 9.865       | 0.182       | 1          | -            | -          | -           | g           | -          | -           | -             | D4          | c        | o            | -           | -            | -            | -                      | 11.111      | 0.36        | 1.15        | 1        | 39.0       | 0.70 | 3.62                               | 11.043                    | 0.33                      | 1.06                 | 0.06                  | 39.3                                 | 11.05                       | 0.34                        | 1.07        |
| 11430594-5146599 | 292.308 | 9.673       | 0.204       | 1          | -            | -          | -           | g           | -          | -           | -             | D1          | c        | o            | -           | -            | -            | -                      | 11.175      | 0.29        | 1.15        | 1        | 33.0       | 0.58 | 3.63                               | 11.099                    | 0.26                      | 1.05                 | 0.06                  | 33.3                                 | 11.11                       | 0.26                        | 1.06        |
| 11434131-5223539 | 292.561 | 9.104       | 0.177       | 1          | -            | -          | -           | g           | -          | -           | -             | D1          | c        | o            | -           | -            | -            | -                      | 11.081      | 0.57        | ...         | 1        | 50.6       | 1.00 | 3.64                               | 11.015                    | 0.54                      | ...                  | 0.05                  | 51.0                                 | 11.02                       | 0.54                        | ...         |
| 11443956-5902024 | 294.422 | 2.730       | 1.020       | 1          | -            | -          | -           | g           | -          | P           | -             | D3          | c        | o            | -           | -            | -            | -                      | 11.478      | 0.44        | 1.38        | 1        | 30.0       | 0.64 | 4.21                               | 11.098                    | 0.27                      | 0.87                 | 0.32                  | 32.7                                 | 11.11                       | 0.29                        | 0.94        |
| 11445527-5154206 | 292.616 | 9.629       | 0.208       | 1          | -            | -          | -           | g           | t          | -           | -             | D1          | c        | o            | -           | -            | -            | -                      | 10.232      | 0.33        | 1.05        | 1        | 76.6       | 0.32 | 3.63                               | 10.154                    | 0.30                      | 0.95                 | 0.06                  | 77.4                                 | 10.16                       | 0.30                        | 0.96        |
| 11450474-6317459 | 295.558 | -1.378      | 4.770       | 8          | -            | -          | -           | g           | -          | -           | -             | D3          | c        | o            | -           | -            | -            | -                      | 8.997       | 1.33        | ...         | 1        | 79.0       | 0.66 | 4.54                               | 7.216                     | 0.54                      | ...                  | 1.48                  | ...                                  | ...                         | 0.38                        | ...         |
| 11452197-5411386 | 293.275 | 7.434       | 0.280       | 1          | -            | -          | -           | g           | -          | -           | -             | D4          | c        | o            | -           | -            | -            | -                      | 11.219      | 0.36        | 1.13        | 1        | 31.4       | 0.84 | 3.80                               | 11.115                    | 0.32                      | 0.99                 | 0.09                  | 31.9                                 | 11.12                       | 0.32                        | 1.01        |
| 11453425-6532575 | 296.181 | -3.545      | 4.387       | 8          | -            | -          | -           | -           | -          | -           | -             | -           | -        | -            | -           | -            | -            | -                      | 8.455       | 0.84        | 1.89        | 1        | 90.2       | 0.88 | 4.25                               | 6.820                     | 0.11                      | -0.29                | 1.36                  | ...                                  | ...                         | 0.20                        | -0.00       |
| 11460182-5622504 | 293.925 | 5.343       | 0.387       | 9          | -            | -          | -           | -           | -          | -           | -             | cr          | ca       | o            | -           | -            | -            | -                      | 11.175      | 0.50        | 1.20        | 1        | 47.8       | 0.66 | 3.91                               | 11.031                    | 0.44                      | 1.00                 | 0.12                  | ...                                  | ...                         | 0.44                        | 1.03        |
| 11460639-5623274 | 293.938 | 5.336       | 0.386       | 1          | -            | -          | -           | g           | -          | -           | -             | D1          | c        | o            | h           | -            | -            | a                      | 8.374       | 0.41        | 1.14        | 1        | 158.8      | 0.60 | 3.91                               | 8.230                     | 0.35                      | 0.95                 | 0.12                  | 162.4                                | 8.24                        | 0.36                        | 0.97        |
| 11462422-5502144 | 293.637 | 6.056       | 0.391       | 1          | -            | -          | -           | g           | -          | -           | -             | D2          | c        | o            | -           | -            | -            | -                      | 10.992      | 0.47        | 1.29        | 1        | 37.2       | 0.56 | 3.84                               | 10.846                    | 0.40                      | 1.09                 | 0.12                  | 38.1                                 | 10.86                       | 0.41                        | 1.12        |
| 11480232-5225056 | 293.216 | 9.253       | 0.183       | 1          | -            | -          | -           | g           | -          | -           | -             | D1          | c        | o            | -           | -            | -            | -                      | 10.754      | 0.31        | 1.02        | 1        | 36.6       | 0.76 | 3.65                               | 10.686                    | 0.28                      | 0.93                 | 0.06                  | 36.9                                 | 10.69                       | 0.28                        | 0.94        |
| 11485605-6947361 | 297.547 | -7.578      | 0.358       | 1          | -            | -          | -           | g           | -          | -           | -             | D1          | c        | o            | -           | -            | -            | -                      | 11.375      | 0.40        | 1.21        | 1        | 48.8       | 0.22 | 3.84                               | 11.242                    | 0.34                      | 1.03                 | 0.11                  | 50.0                                 | 10.25                       | 0.35                        | 1.06        |
| 11492716-6841379 | 297.325 | -6.500      | 0.298       | 1          | -            | -          | -           | g           | t          | -           | -             | D1          | c        | o            | -           | -            | -            | -                      | 11.201      | 0.52        | 1.31        | 1        | 50.6       | 0.20 | 3.97                               | 11.090                    | 0.47                      | 1.16                 | 0.09                  | 51.5                                 | 11.10                       | 0.48                        | 1.18        |
| 11493660-5251587 | 293.560 | 8.877       | 0.170       | 1          | -            | -          | -           | g           | -          | -           | -             | D1          | c        | o            | -           | -            | -            | -                      | 11.207      | 0.49        | 1.16        | 1        | 43.6       | 0.32 | 3.72                               | 11.144                    | 0.46                      | 1.07                 | 0.05                  | 44.0                                 | 11.15                       | 0.47                        | 1.08        |
| 11494338-6848457 | 297.377 | -6.609      | 0.315       | 1          | -            | -          | -           | g           | -          | -           | -             | D2          | c        | o            | -           | -            | -            | -                      | 10.744      | 0.25        | 0.96        | 1        | 42.4       | 0.70 | 3.95                               | 10.627                    | 0.20                      | 0.81                 | 0.10                  | 43.1                                 | 10.64                       | 0.21                        | 0.83        |
| 11494658-5207198 | 293.404 | 9.605       | 0.175       | 1          | -            | -          | -           | g           | t          | -           | -             | D1          | c        | o            | -           | -            | -            | -                      | 11.004      | 0.39        | 1.14        | 1        | 54.6       | 0.24 | 3.69                               | 10.939                    | 0.36                      | 1.05                 | 0.05                  | 55.1                                 | 10.94                       | 0.37                        | 1.06        |
| 11494881-6400073 | 296.241 | -1.934      | 2.449       | 1          | -            | -          | -           | g           | t          | -           | -             | D1          | -        | -            | h           | V            | -            | -                      | 9.529       | 0.60        | ...         | 1        | 97.0       | 0.44 | 4.51                               | 8.617                     | 0.20                      | ...                  | 0.76                  | 126.9                                | 8.59                        | 0.24                        | ...         |
| 11501351-6452222 | 296.490 | -2.769      | 5.674       | 9          | -            | -          | -           | -           | -          | -           | -             | -           | -        | -            | -           | -            | -            | -                      | 9.965       | 0.77        | 1.68        | 1        | 105.8      | 0.28 | 4.35                               | 7.851                     | -0.17                     | -1.14                | 1.76                  | ...                                  | ...                         | -0.06                       | -0.76       |
| 11510294-6532041 | 296.729 | -3.393      | 0.956       | 1          | -            | -          | -           | g           | t          | P           | -             | D1          | -        | -            | -           | -            | -            | -                      | 11.238      | 0.37        | 1.41        | 1        | 28.4       | 0.50 | 4.23                               | 10.882                    | 0.22                      | 0.93                 | 0.30                  | 30.7                                 | 10.89                       | 0.23                        | 1.00        |
| 11515143-5201565 | 293.698 | 9.768       | 0.148       | 1          | -            | -          | -           | g           | -          | -           | -             | D1          | c        | o            | -           | -            | -            | -                      | 11.258      | 0.32        | 1.10        | 1        | 40.4       | 0.86 | 3.57                               | 11.203                    | 0.30                      | 1.03                 | 0.05                  | 40.7                                 | 11.21                       | 0.30                        | 1.04        |
| 11520923-6153348 | 296.010 | 0.179       | 2.125       | 9          | -            | -          | -           | -           | -          | -           | -             | -           | -        | -            | -           | -            | -            | -                      | 7.576       | ...         | ...         | -2       | 48.6       | 0.26 | 4.57                               | 6.784                     | ...                       | ...                  | 0.66                  | ...                                  | ...                         | ...                         | ...         |
| 11523245-5950248 | 295.590 | 2.189       | 1.638       | 1          | -            | -          | -           | g           | t          | -           | -             | D1          | -        | -            | h           | V            | -            | -                      | 11.504      | 0.60        | ...         | 1        | 48.0       | 0.36 | 4.26                               | 10.894                    | 0.33                      | ...                  | 0.51                  | 58.4                                 | 10.82                       | 0.36                        | ...         |
| 11523284-5900598 | 295.404 | 2.992       | 0.900       | 1          | -            | -          | -           | g           | t          | P           | -             | D1          | -        | -            | -           | -            | -            | -                      | 11.536      | 0.43        | 1.50        | 1        | 33.6       | 0.50 | 4.18                               | 11.201                    | 0.28                      | 1.05                 | 0.28                  | 36.3                                 | 11.20                       | 0.30                        | 1.11        |
| 11523666-5717128 | 295.020 | 4.678       | 0.425       | 1          | -            | -          | -           | g           | -          | -           | -             | D1          | e        | o            | -           | -            | -            | -                      | 10.242      | 0.33        | 1.09        | 1        | 45.0       | 0.84 | 3.97                               | 10.084                    | 0.26                      | 0.88                 | 0.13                  | 46.1                                 | 10.10                       | 0.26                        | 0.91        |
| 11530961-6836321 | 297.635 | -6.339      | 0.280       | 1          | -            | -          | -           | g           | t          | -           | -             | D1          | c        | o            | -           | -            | -            | -                      | 10.083      | 0.31        | 1.11        | 1        | 83.4       | 0.30 | 3.95                               | 9.979                     | 0.26                      | 0.97                 | 0.09                  | 84.5                                 | 9.99                        | 0.26                        | 0.99        |
| 11532440-5336532 | 294.295 | 8.281       | 0.202       | 1          | -            | -          | -           | g           | -          | -           | -             | D1          | c        | o            | -           | -            | -            | -                      | 10.894      | 0.39        | 1.11        | 1        | 37.2       | 0.68 | 3.67                               | 10.819                    | 0.36                      | 1.01                 | 0.06                  | 37.6                                 | 10.83                       | 0.36                        | 1.02        |
| 11534248-5406175 | 294.450 | 7.813       | 0.267       | 1          | -            | -          | -           | g           | t          | -           | -             | D1          | c        | o            | h           | V            | -            | -                      | 11.142      | 0.28        | 1.10        | 1        | 43.8       | 0.46 | 3.73                               | 11.043                    | 0.23                      | 0.97                 | 0.08                  | 44.5                                 | 11.05                       | 0.24                        | 0.99        |
| 11535055-6420218 | 296.746 | -2.162      | 3.015       | 8          | -            | -          | -           | -           | -          | -           | -             | -           | -        | -            | -           | -            | -            | -                      | 10.412      | 0.19        | ...         | -2       | 28.4       | 0.36 | 4.47                               | 9.289                     | 0.69                      | ...                  | 0.93                  | ...                                  | ...                         | 0.75                        | ...         |
| 11550129-5712316 | 295.321 | 4.827       | 0.477       | 1          | -            | -          | -           | g           | t          | P           | -             | D1          | -        | -            | -           | -            | -            | -                      | 10.986      | 0.43        | 1.36        | 1        | 33.6       | 0.40 | 3.98                               | 10.808                    | 0.35                      | 1.12                 | 0.15                  | 34.6                                 | 10.82                       | 0.36                        | 1.15        |
| 11551431-6750328 | 297.654 | -5.548      | 0.342       | 2          | -            | -          | -           | g           | -          | P           | -             | D3          | -        | -            | -           | -            | -            | -                      | 11.312      | 0.29        | 1.02        | -2       | 30.6       | 0.68 | 4.07                               | 11.185                    | 0.23                      | 0.85                 | 0.11                  | 31.2                                 | 10.20                       | 0.24                        | 0.87        |
| 11555240-5939413 | 295.960 | 2.456       | 1.125       | 2          | -            | -          | -           | g           | -          | +           | P             | n           | -        | -            | -           | -            | -            | -                      | 11.596      | 0.31        | 1.26        | 1        | 32.6       | 0.56 | 4.25                               | 11.177                    | 0.12                      | 0.70                 | 0.35                  | 36.3                                 | 11.17                       | 0.14                        | 0.77        |
| 11565971-6019148 | 296.237 | 1.841       | 0.993       | 1          | o            | -          | -           | g           | -          | -           | -             | D1          | -        | -            | -           | V            | o            | -                      | 10.957      | 0.31        | 1.15        | 1        | 30.2       | 0.74 | 4.37                               | 10.587                    | 0.15                      | 0.66                 | 0.31                  | 33.0                                 | 10.59                       | 0.17                        | 0.72        |
| 11582367-7223193 | 298.892 | -9.934      | 0.318       | 1          | -            | -          | -           | g           | t          | -           | -             | D1          | c        | o            | -           | -            | -            | -                      | 10.597      | 0.34        | 1.11        | 1        | 56.4       | 0.44 | 3.74                               | 10.479                    | 0.29                      | 0.96                 | 0.10                  | 57.4                                 | 10.49                       | 0.30                        | 0.98        |
| 11585505-6337470 | 297.139 | -1.350      | 7.762       | 7          | -            | -          | -           | -           | -          | -           | -             | -           | -        | -            | -           | V            | -            | -                      | 11.086      | ...         | ...         | 1        | 20.6       | 0.78 | 4.55                               | 8.194                     | ...                       | ...                  | 2.40                  | ...                                  | ...                         | ...                         | ...         |
| 11590274-6839513 | 298.174 | -6.278      | 0.276       | 1          | -            | -          | -           | g           | -          | -           | -             | D3          | c        | o            | -           | -            | -            | -                      | 11.163      | 0.24        | 1.06        | 1        | 27.8       | 0.86 | 3.95                               | 11.060                    | 0.19                      | 0.92                 | 0.09                  | 28.2                                 | 11.07                       | 0.20                        | 0.94        |
| 11590953-5324325 | 295.095 | 8.665       | 0.186       | 1          | -            | -          | -           | g           | -          | -           | -             | D3          | c        | o            | -           | -            | -            | -                      | 9.172       | 0.30        | 1.04        | 1        | 88.6       | 0.70 | 3.76                               | 9.103                     | 0.27                      | 0.95                 | 0.06                  | 89.2                                 | 9.11                        | 0.27                        | 0.96        |

2M-ZoA galaxy catalogue description and analysis 81

Table B1: a) continued.

| 2MASX J          | <i>l</i>    | <i>b</i>    | EBV        | Object       | Sample         | Disc        | 2MRS       | Velocity    | NIR           | Photom      | Ext | <i>K</i> <sub>20</sub> | <i>H-K</i>  | <i>J-K</i>  | vc          | <i>a</i>    | <i>b/a</i> | st.d.       | <i>K</i> <sub>s</sub> <sup>o</sup> | ( <i>H-K</i> ) <sup>o</sup> | ( <i>J-K</i> ) <sup>o</sup> | <i>A<sub>K</sub></i> | <i>a</i> <sub>d</sub> <sup>o</sup> | <i>K</i> <sub>s</sub> <sup>o,d</sup> | ( <i>H-K</i> ) <sup>o,c</sup> | ( <i>J-K</i> ) <sup>o,c</sup> |             |        |             |             |             |        |        |
|------------------|-------------|-------------|------------|--------------|----------------|-------------|------------|-------------|---------------|-------------|-----|------------------------|-------------|-------------|-------------|-------------|------------|-------------|------------------------------------|-----------------------------|-----------------------------|----------------------|------------------------------------|--------------------------------------|-------------------------------|-------------------------------|-------------|--------|-------------|-------------|-------------|--------|--------|
| (1)              | deg<br>(2a) | deg<br>(2b) | mag<br>(3) | class<br>(4) | off flg<br>(5) | gal<br>(7a) | TF<br>(7b) | obs<br>(7c) | ext'd<br>(7d) | type<br>(8) | (9) | Opt<br>(10a)           | HI<br>(10b) | flg<br>(11) | flg<br>(12) | flg<br>(13) | (14)       | mag<br>(15) | mag<br>(16)                        | (17)                        | (18)                        | (19)                 | (20)                               | mag<br>(21)                          | mag<br>(22)                   | mag<br>(23)                   | mag<br>(24) | (25)   | mag<br>(26) | mag<br>(27) | mag<br>(28) |        |        |
| 12174466–5837222 | 298.547     | 3.962       | 0.623      | 2            | –              | –           | g          | t           | +             | –           | n   | –                      | –           | –           | –           | –           | –          | –           | 11.450                             | 0.35                        | 1.16                        | 1                    | 32.0                               | 0.42                                 | 4.11                          | 11.218                        | 0.25        | 0.85   | 0.19        | 33.5        | 11.23       | 0.26   | 0.89   |
| 12180926–5644271 | 298.356     | 5.835       | 0.525      | 1            | –              | –           | g          | –           | –             | D1          | c   | o                      | –           | –           | V           | –           | –          | –           | 10.461                             | 0.40                        | 1.27                        | 1                    | 55.8                               | 0.74                                 | 3.84                          | 10.265                        | 0.31        | 1.01   | 0.16        | 57.7        | 10.28       | 0.32   | 1.04   |
| 12193360–5619287 | 298.496     | 6.272       | 0.489      | 1            | –              | –           | g          | –           | –             | D1          | c   | o                      | –           | –           | V           | –           | –          | –           | 11.213                             | 0.36                        | 1.22                        | 1                    | 36.0                               | 0.84                                 | 3.88                          | 11.031                        | 0.28        | 0.98   | 0.15        | 37.2        | 11.04       | 0.29   | 1.01   |
| 12194313–5335100 | 298.176     | 8.992       | 0.186      | 1            | –              | –           | g          | –           | –             | D2          | c   | o                      | –           | –           | V           | –           | –          | –           | 10.955                             | 0.29                        | 1.02                        | 1                    | 37.2                               | 0.70                                 | 3.70                          | 10.886                        | 0.26        | 0.92   | 0.06        | 37.5        | 10.89       | 0.26   | 0.94   |
| 12204537–6310426 | 299.479     | –0.513      | 3.437      | 9            | –              | –           | g          | –           | –             | –           | –   | –                      | –           | –           | –           | –           | –          | –           | 7.731                              | 1.04                        | 3.03                        | –2                   | 39.6                               | 0.36                                 | 4.60                          | 6.450                         | 0.47        | 1.32   | 1.06        | ...         | ...         | 0.54   | 1.55   |
| 12220996–5501199 | 298.707     | 7.609       | 0.297      | 1            | –              | –           | g          | –           | –             | D2          | c   | o                      | –           | –           | V           | –           | –          | –           | 11.130                             | 0.34                        | 1.11                        | 1                    | 33.2                               | 0.94                                 | 3.81                          | 11.019                        | 0.29        | 0.96   | 0.09        | 33.7        | 11.03       | 0.29   | 0.98   |
| 12223838–5836598 | 299.181     | 4.045       | 0.581      | 1            | –              | –           | g          | t           | –             | D1          | c   | o                      | –           | –           | –           | –           | –          | –           | 8.392                              | 0.29                        | 1.11                        | 1                    | 124.4                              | 0.36                                 | 4.15                          | 8.176                         | 0.19        | 0.82   | 0.18        | 128.3       | 8.20        | 0.21   | 0.86   |
| 12224995–6830165 | 300.304     | –5.779      | 0.336      | 1            | –              | –           | g          | –           | –             | D1          | c   | o                      | –           | –           | –           | –           | –          | –           | 11.184                             | 0.38                        | 1.14                        | 1                    | 37.8                               | 0.52                                 | 4.05                          | 11.059                        | 0.33        | 0.97   | 0.10        | 38.6        | 11.06       | 0.33   | 0.99   |
| 12234861–5956414 | 299.475     | 2.741       | 1.208      | 1            | –              | –           | g          | t           | P             | D1          | –   | –                      | –           | –           | –           | –           | –          | –           | 10.715                             | 0.40                        | 1.53                        | 1                    | 54.8                               | 0.26                                 | 4.28                          | 10.265                        | 0.20        | 0.93   | 0.37        | 61.0        | 10.27       | 0.23   | 1.01   |
| 12263910–7240018 | 301.062     | –9.886      | 0.551      | 7            | –              | –           | g          | –           | –             | –           | –   | –                      | –           | –           | –           | –           | –          | –           | 9.507                              | –0.12                       | 0.60                        | –2                   | 129.2                              | 0.88                                 | 4.08                          | 9.302                         | –0.22       | 0.33   | 0.17        | ...         | ...         | –0.21  | 0.36   |
| 12264272–6020043 | 299.874     | 2.390       | 1.405      | 1            | –              | –           | g          | t           | P             | D1          | –   | –                      | –           | –           | –           | –           | –          | –           | 11.395                             | 0.48                        | 1.42                        | 1                    | 32.6                               | 0.60                                 | 4.35                          | 10.871                        | 0.25        | 0.72   | 0.44        | 37.3        | 10.87       | 0.27   | 0.81   |
| 12265379–7237587 | 301.077     | –9.850      | 0.565      | 8            | –              | –           | g          | –           | –             | D1          | c   | o                      | –           | –           | V           | –           | –          | –           | 9.416                              | –0.32                       | 0.68                        | –2                   | 148.0                              | 0.48                                 | 4.08                          | 9.205                         | –0.41       | 0.40   | 0.18        | ...         | ...         | –0.40  | 0.43   |
| 12272397–5628104 | 299.577     | 6.246       | 0.578      | 1            | –              | –           | g          | t           | –             | D1          | c   | o                      | –           | –           | –           | –           | –          | –           | 11.032                             | 0.40                        | 1.31                        | 1                    | 37.0                               | 0.42                                 | 3.87                          | 10.817                        | 0.30        | 1.02   | 0.18        | 38.4        | 10.83       | 0.31   | 1.06   |
| 12274739–5314446 | 299.350     | 9.461       | 0.171      | 1            | –              | –           | g          | –           | –             | D1          | c   | o                      | –           | –           | V           | –           | –          | –           | 10.895                             | 0.32                        | 0.99                        | –2                   | 63.4                               | 0.48                                 | 3.66                          | 10.831                        | 0.29        | 0.91   | 0.05        | 64.1        | 10.83       | 0.29   | 0.92   |
| 12280968–6054558 | 300.106     | 1.828       | 1.737      | 1            | –              | –           | g          | t           | P             | D1          | –   | –                      | –           | –           | –           | –           | –          | –           | 11.370                             | ...                         | ...                         | –                    | 40.4                               | 0.48                                 | 4.47                          | 10.723                        | ...         | ...    | 0.54        | 48.9        | 10.69       | ...    | ...    |
| 12285595–5805496 | 299.952     | 4.644       | 1.061      | 1            | –              | –           | g          | t           | P             | D1          | –   | –                      | –           | –           | V           | –           | –          | –           | 11.606                             | 0.57                        | 1.78                        | 1                    | 45.2                               | 0.22                                 | 4.05                          | 11.211                        | 0.39        | 1.25   | 0.33        | 50.3        | 11.19       | 0.41   | 1.32   |
| 12290692–5957596 | 300.139     | 2.784       | 1.066      | 1            | –              | –           | g          | –           | –             | D1          | –   | –                      | –           | –           | –           | –           | –          | –           | 10.209                             | 0.43                        | 1.42                        | 1                    | 44.6                               | 0.80                                 | 4.30                          | 9.812                         | 0.25        | 0.89   | 0.33        | 48.4        | 9.83        | 0.27   | 0.96   |
| 12292688–6003366 | 300.188     | 2.694       | 1.091      | 1            | –              | –           | g          | –           | –             | D2          | –   | –                      | –           | –           | –           | –           | –          | –           | 10.146                             | 0.47                        | 1.39                        | 1                    | 53.2                               | 0.74                                 | 4.34                          | 9.739                         | 0.28        | 0.85   | 0.34        | 57.9        | 9.76        | 0.31   | 0.92   |
| 12292900–5955556 | 300.182     | 2.822       | 1.016      | 2            | –              | –           | g          | P           | –             | D2          | –   | –                      | –           | –           | –           | –           | –          | –           | 10.882                             | 0.27                        | 1.23                        | 1                    | 33.2                               | 0.58                                 | 4.34                          | 10.503                        | 0.10        | 0.72   | 0.31        | 36.1        | 10.52       | 0.12   | 0.79   |
| 12294170–6213085 | 300.401     | 0.546       | 5.493      | 9            | –              | –           | g          | –           | –             | –           | –   | –                      | –           | –           | –           | –           | –          | –           | 11.128                             | ...                         | ...                         | 1                    | 29.4                               | 0.80                                 | 4.59                          | 9.081                         | ...         | ...    | 1.70        | ...         | ...         | ...    | ...    |
| 12294797–5421487 | 299.749     | 8.374       | 0.240      | 1            | –              | –           | g          | t           | –             | D1          | c   | o                      | –           | –           | V           | –           | –          | –           | 10.600                             | 0.33                        | 1.16                        | 1                    | 51.4                               | 0.32                                 | 3.74                          | 10.511                        | 0.29        | 1.04   | 0.07        | 52.0        | 10.52       | 0.30   | 1.06   |
| 12294880–6107045 | 300.323     | 1.644       | 1.950      | 1            | –              | –           | g          | t           | –             | D1          | –   | –                      | –           | –           | V           | –           | –          | –           | 10.437                             | 0.51                        | ...                         | 1                    | 35.4                               | 0.62                                 | 4.49                          | 9.710                         | 0.18        | ...    | 0.60        | 43.6        | 9.69        | 0.22   | ...    |
| 12300399–6256387 | 300.505     | –0.173      | 16.982     | 9            | –              | –           | g          | –           | –             | –           | –   | –                      | –           | –           | –           | –           | –          | –           | 9.453                              | ...                         | ...                         | 1                    | 66.0                               | 0.76                                 | 4.65                          | 3.126                         | ...         | ...    | 5.26        | ...         | ...         | ...    | ...    |
| 12305461–5933581 | 300.331     | 3.202       | 0.853      | 1            | –              | –           | g          | –           | –             | D3          | –   | –                      | –           | –           | –           | –           | –          | –           | 10.687                             | 0.42                        | 1.38                        | 1                    | 49.4                               | 0.70                                 | 4.24                          | 10.369                        | 0.28        | 0.96   | 0.26        | 52.7        | 10.38       | 0.29   | 1.02   |
| 12315756–5950587 | 300.485     | 2.930       | 0.926      | 1            | –              | –           | g          | P           | –             | D3          | –   | –                      | –           | –           | –           | –           | –          | –           | 10.017                             | ...                         | 1.31                        | 1                    | 63.2                               | 1.00                                 | 4.29                          | 9.672                         | ...         | 0.85   | 0.29        | 68.0        | 9.69        | ...    | 0.91   |
| 12320090–5951163 | 300.492     | 2.925       | 0.923      | 1            | –              | –           | g          | P           | –             | D3          | –   | –                      | –           | –           | –           | –           | –          | –           | 10.449                             | 0.55                        | 1.36                        | –2                   | 70.4                               | 0.88                                 | 4.29                          | 10.105                        | 0.40        | 0.90   | 0.29        | 75.8        | 10.12       | 0.42   | 0.97   |
| 12320218–5947566 | 300.491     | 2.981       | 0.893      | 2            | –              | –           | g          | +           | –             | n           | –   | –                      | –           | –           | –           | –           | –          | –           | 11.304                             | 0.30                        | 1.28                        | 1                    | 30.2                               | 0.70                                 | 4.29                          | 10.971                        | 0.15        | 0.83   | 0.28        | 32.5        | 10.98       | 0.17   | 0.89   |
| 12321185–5952122 | 300.517     | 2.911       | 0.910      | 1            | –              | –           | g          | t           | P             | D1          | –   | –                      | –           | –           | –           | –           | –          | –           | 11.065                             | 0.38                        | 1.38                        | 1                    | 39.4                               | 0.42                                 | 4.30                          | 10.726                        | 0.23        | 0.93   | 0.28        | 42.4        | 10.74       | 0.25   | 0.99   |
| 12322646–6820115 | 301.172     | –5.530      | 0.335      | 1            | –              | –           | g          | –           | –             | D1          | c   | o                      | –           | –           | –           | –           | –          | –           | 10.427                             | 0.43                        | 1.13                        | 1                    | 66.0                               | 0.52                                 | 4.07                          | 10.302                        | 0.38        | 0.96   | 0.10        | 67.2        | 10.31       | 0.38   | 0.99   |
| 12323349–6832200 | 301.198     | –5.731      | 0.283      | 1            | –              | –           | g          | –           | –             | D2          | c   | o                      | –           | –           | –           | –           | –          | –           | 9.839                              | 0.32                        | 1.08                        | 1                    | 64.4                               | 0.64                                 | 4.06                          | 9.734                         | 0.27        | 0.94   | 0.09        | 65.3        | 9.74        | 0.28   | 0.95   |
| 12324972–6135310 | 300.720     | 1.200       | 4.410      | 9            | –              | –           | g          | –           | –             | –           | –   | –                      | –           | –           | –           | –           | –          | –           | 10.679                             | ...                         | ...                         | 1                    | 53.8                               | 0.26                                 | 4.47                          | 9.036                         | ...         | ...    | 1.37        | ...         | ...         | ...    | ...    |
| 12325467–5959231 | 300.615     | 2.799       | 0.923      | 1            | –              | –           | g          | –           | –             | D3          | –   | –                      | –           | –           | –           | –           | –          | –           | 10.325                             | 0.46                        | 1.41                        | 1                    | 46.0                               | 0.84                                 | 4.27                          | 9.981                         | 0.31        | 0.95   | 0.29        | 49.2        | 10.00       | 0.32   | 1.01   |
| 12331117–5913436 | 300.595     | 3.560       | 1.198      | 1            | –              | –           | g          | –           | –             | D1          | –   | –                      | –           | –           | –           | –           | –          | –           | 11.348                             | 0.40                        | 1.33                        | 1                    | 45.0                               | 0.82                                 | 4.15                          | 10.902                        | 0.20        | 0.73   | 0.37        | 50.8        | 10.88       | 0.22   | 0.81   |
| 12335345–5950041 | 300.726     | 2.962       | 0.904      | 1            | –              | –           | g          | –           | –             | D1          | –   | –                      | –           | –           | –           | –           | –          | –           | 10.967                             | 0.41                        | 1.16                        | 1                    | 41.4                               | 0.74                                 | 4.27                          | 10.630                        | 0.26        | 0.72   | 0.28        | 45.0        | 10.62       | 0.28   | 0.78   |
| 12341389–5958544 | 300.779     | 2.818       | 0.942      | 1            | –              | –           | g          | –           | –             | D1          | –   | –                      | –           | –           | –           | –           | –          | –           | 10.412                             | 0.33                        | 1.17                        | 1                    | 64.8                               | 0.52                                 | 4.29                          | 10.061                        | 0.18        | 0.71   | 0.29        | 70.2        | 10.07       | 0.19   | 0.77   |
| 12343220–5943464 | 300.800     | 3.072       | 0.862      | 2            | –              | –           | g          | –           | –             | D3          | –   | –                      | –           | –           | –           | –           | –          | –           | 10.992                             | 0.32                        | 1.25                        | 1                    | 38.0                               | 0.78                                 | 4.22                          | 10.671                        | 0.18        | 0.82   | 0.27        | 40.6        | 10.68       | 0.19   | 0.88   |
| 12344923–6139290 | 300.961     | 1.150       | 39.761     | 9            | –              | –           | g          | –           | –             | –           | –   | –                      | –           | –           | –           | –           | –          | –           | 7.310                              | ...                         | 1.61                        | 1                    | 219.4                              | 1.00                                 | 4.48                          | –7.505                        | ...         | –18.15 | 12.32       | ...         | ...         | –15.52 | ...    |
| 12345078–6139070 | 300.963     | 1.156       | 39.263     | 9            | –              | –           | g          | –           | –             | –           | –   | –                      | –           | –           | –           | –           | –          | –           | 6.910                              | 0.97                        | 1.73                        | 1                    | 143.8                              | 0.76                                 | 4.48                          | –7.719                        | –5.54       | –17.78 | 12.16       | ...         | ...         | –4.77  | –15.18 |
| 12345259–6140190 | 300.968     | 1.137       | 38.190     | 9            | –              | –           | g          | –           | –             | –           | –   | –                      | –           | –           | –           | –           | –          | –           | 9.661                              | 0.86                        | 2.08                        | 1                    | 57.4                               | 0.64                                 | 4.48                          | –4.569                        | –5.46       | –16.90 | 11.83       | ...         | ...         | –4.71  | –14.38 |
| 12345752–6139401 | 300.977     | 1.148       | 38.315     | 9            | –              | –           | g          | –           | –             | –           | –   | –                      | –           | –           | –           | –           | –          | –           | 7.604                              | 1.07                        | 2.16                        | 1                    | 196.0                              | 0.46                                 | 4.48                          | –6.672                        | –5.27       | –16.87 | 11.87       | ...         | ...         | –4.52  | –14.34 |
| 12350355–6141451 | 300.991     | 1.114       | 27.247     | 9            | –              | –           | g          | –           | –             | –           | –   | –                      | –           | –           | –           | –           | –          | –           | 8.978                              | 0.80                        | ...                         | 1                    | 125.4                              | 0.30                                 | 4.44                          | –1.174                        | –3.71       | ...    | 8.44        | ...         | ...         | –3.18  | ...    |
| 12352170–5947185 | 300.908     | 3.020       | 0.802      | 1            | –              | –           | g          | +           | –             | n           | –   | –                      | –           | –           | –           | –           | –          | –           | 11.425                             | 0.32                        | 1.21                        | 1                    | 28.2                               |                                      |                               |                               |             |        |             |             |             |        |        |

Table B1: a) continued.

| 2MASX J          | <i>l</i> | <i>b</i> | EBV    | Object | Sample | Disc | 2MRS | Velocity | NIR  | Photom | Ext  | <i>K</i> <sub>20</sub> | <i>H-K</i> | <i>J-K</i> | vc    | <i>a</i> | <i>b/a</i> | st.d. | <i>K</i> <sub>s</sub> <sup>o</sup> | <i>(H-K)</i> <sup>o</sup> | <i>(J-K)</i> <sup>o</sup> | <i>A<sub>K</sub></i> | <i>a</i> <sub>d</sub> <sup>o</sup> | <i>K</i> <sub>s</sub> <sup>o,d</sup> | <i>(H-K)</i> <sup>o,c</sup> | <i>(J-K)</i> <sup>o,c</sup> |       |      |       |      |       |      |      |
|------------------|----------|----------|--------|--------|--------|------|------|----------|------|--------|------|------------------------|------------|------------|-------|----------|------------|-------|------------------------------------|---------------------------|---------------------------|----------------------|------------------------------------|--------------------------------------|-----------------------------|-----------------------------|-------|------|-------|------|-------|------|------|
| (1)              | deg      | deg      | mag    | class  | off    | flag | gal  | TF       | obs  | ext'd  | type | (9)                    | Opt        | HI         | (10b) | (11)     | flag       | flag  | mag                                | mag                       | mag                       | mag                  | mag                                | mag                                  | mag                         | mag                         | mag   |      |       |      |       |      |      |
| (2a)             | (2b)     | (3)      | (4)    | (5)    | (6)    | (7a) | (7b) | (7c)     | (7d) | (8)    | (9)  | (10a)                  | (10b)      | (11)       | (12)  | (13)     | (14)       | (15)  | (16)                               | (17)                      | (18)                      | (19)                 | (20)                               | (21)                                 | (22)                        | (23)                        | (24)  | (25) | (26)  | (27) | (28)  |      |      |
| 13033543–5305280 | 304.783  | 9.737    | 0.394  | 1      | –      | –    | g    | –        | –    | –      | D1   | c                      | o          | –          | –     | –        | –          | –     | 10.712                             | 0.25                      | 1.10                      | 1                    | 53.6                               | 0.76                                 | 3.64                        | 10.565                      | 0.18  | 0.90 | 0.12  | 54.8 | 10.58 | 0.19 | 0.93 |
| 13035049–7207229 | 303.896  | –9.275   | 0.287  | 1      | –      | –    | g    | –        | –    | –      | D1   | c                      | o          | –          | –     | –        | –          | –     | 11.089                             | 0.25                      | 1.07                      | 1                    | 28.6                               | 0.62                                 | 3.82                        | 10.982                      | 0.20  | 0.93 | 0.09  | 29.1 | 10.99 | 0.21 | 0.95 |
| 13050567–5728451 | 304.775  | 5.344    | 0.385  | 1      | –      | –    | g    | –        | –    | –      | D4   | c                      | o          | –          | –     | –        | –          | –     | 10.610                             | 0.28                      | 1.02                      | 1                    | 32.0                               | 0.76                                 | 4.05                        | 10.467                      | 0.22  | 0.83 | 0.12  | 32.6 | 10.48 | 0.22 | 0.86 |
| 13061289–5733224 | 304.921  | 5.258    | 0.358  | 1      | –      | –    | g    | –        | –    | –      | D1   | c                      | o          | –          | –     | –        | –          | –     | 10.548                             | 0.33                      | 1.11                      | 1                    | 54.0                               | 0.80                                 | 4.05                        | 10.415                      | 0.27  | 0.93 | 0.11  | 55.2 | 10.42 | 0.27 | 0.96 |
| 13065923–5713382 | 305.045  | 5.581    | 0.383  | 1      | o      | –    | g    | –        | –    | –      | D4   | c                      | cf         | –          | –     | –        | –          | –     | 10.033                             | 0.37                      | 1.18                      | 1                    | 56.6                               | 0.52                                 | 4.02                        | 9.890                       | 0.31  | 0.99 | 0.12  | 58.3 | 9.89  | 0.32 | 1.01 |
| 13070255–5714292 | 305.052  | 5.566    | 0.384  | 1      | –      | –    | g    | –        | –    | –      | D2   | c                      | o          | –          | –     | –        | –          | –     | 10.607                             | 0.35                      | 1.16                      | 1                    | 38.6                               | 0.80                                 | 4.02                        | 10.464                      | 0.29  | 0.97 | 0.12  | 39.4 | 10.48 | 0.29 | 0.99 |
| 13071466–5546353 | 305.170  | 7.027    | 0.380  | 1      | –      | –    | g    | –        | –    | –      | D1   | c                      | o          | –          | –     | –        | –          | –     | 10.837                             | 0.42                      | 1.31                      | 1                    | 54.0                               | 0.34                                 | 3.90                        | 10.695                      | 0.36  | 1.12 | 0.12  | 55.3 | 10.71 | 0.37 | 1.15 |
| 13071779–5407352 | 305.281  | 8.673    | 0.381  | 1      | –      | –    | g    | –        | –    | –      | D1   | c                      | o          | –          | –     | –        | –          | –     | 11.371                             | 0.30                      | 1.12                      | 1                    | 39.2                               | 0.46                                 | 3.81                        | 11.229                      | 0.23  | 0.93 | 0.12  | 40.2 | 11.24 | 0.24 | 0.96 |
| 13072063–5606592 | 305.163  | 6.686    | 0.421  | 1      | –      | –    | g    | –        | –    | –      | D3   | c                      | o          | –          | –     | –        | –          | –     | 10.671                             | 0.31                      | 1.16                      | 1                    | 40.2                               | 0.82                                 | 3.90                        | 10.514                      | 0.25  | 0.95 | 0.13  | 41.2 | 10.53 | 0.25 | 0.98 |
| 13072260–5706182 | 305.106  | 5.699    | 0.353  | 1      | –      | –    | g    | –        | –    | –      | D1   | c                      | o          | –          | –     | –        | –          | –     | 11.323                             | 0.29                      | 1.09                      | 1                    | 26.6                               | 0.68                                 | 4.02                        | 11.191                      | 0.23  | 0.91 | 0.11  | 27.2 | 11.20 | 0.24 | 0.94 |
| 13073640–5704259 | 305.139  | 5.729    | 0.349  | 1      | –      | –    | g    | –        | –    | –      | D2   | c                      | o          | –          | –     | –        | –          | –     | 10.796                             | 0.36                      | 1.14                      | 1                    | 37.8                               | 0.86                                 | 4.03                        | 10.666                      | 0.31  | 0.96 | 0.11  | 38.5 | 10.68 | 0.31 | 0.98 |
| 13075558–5613271 | 305.237  | 6.574    | 0.458  | 1      | –      | –    | g    | –        | –    | –      | D2   | c                      | o          | –          | –     | –        | –          | –     | 11.138                             | 0.31                      | 1.17                      | 1                    | 36.8                               | 0.70                                 | 3.91                        | 10.967                      | 0.24  | 0.95 | 0.14  | 37.8 | 10.98 | 0.25 | 0.98 |
| 13081287–5744181 | 305.178  | 5.060    | 0.372  | 1      | –      | –    | g    | –        | –    | –      | D1   | c                      | o          | –          | –     | –        | –          | –     | 11.044                             | 0.29                      | 1.08                      | 1                    | 40.4                               | 0.54                                 | 4.10                        | 10.905                      | 0.23  | 0.90 | 0.12  | 41.4 | 10.91 | 0.24 | 0.92 |
| 13081875–5727300 | 305.210  | 5.339    | 0.397  | 1      | –      | –    | g    | –        | –    | –      | D2   | c                      | o          | –          | –     | –        | –          | –     | 10.588                             | 0.41                      | 1.20                      | 1                    | 45.4                               | 0.76                                 | 4.07                        | 10.440                      | 0.34  | 1.01 | 0.12  | 46.5 | 10.45 | 0.35 | 1.03 |
| 13083302–6214482 | 304.923  | 0.559    | 17.330 | 9      | –      | –    | g    | –        | –    | –      | –    | –                      | –          | –          | –     | –        | –          | –     | 7.983                              | ...                       | ...                       | 1                    | 116.4                              | 1.00                                 | 4.59                        | 1.526                       | ...   | ...  | 5.37  | ...  | ...   | ...  |      |
| 13084090–6215161 | 304.938  | 0.550    | 17.057 | 9      | –      | –    | g    | –        | –    | –      | –    | –                      | –          | –          | –     | –        | –          | –     | 7.710                              | 1.25                      | ...                       | 1                    | 219.8                              | 3.38                                 | 4.59                        | 1.355                       | –1.57 | ...  | 5.28  | ...  | –1.24 | ...  |      |
| 13093047–5728160 | 305.370  | 5.315    | 0.456  | 1      | –      | –    | g    | –        | –    | –      | D1   | c                      | o          | –          | –     | –        | –          | –     | 11.095                             | 0.34                      | 1.25                      | 1                    | 36.2                               | 0.42                                 | 4.02                        | 10.925                      | 0.27  | 1.02 | 0.14  | 37.3 | 10.94 | 0.28 | 1.05 |
| 13102904–5618221 | 305.588  | 6.467    | 0.592  | 1      | o      | –    | g    | –        | –    | –      | P    | –                      | –          | –          | –     | –        | –          | –     | 11.376                             | 0.29                      | 1.02                      | –2                   | 64.2                               | 0.34                                 | 3.97                        | 11.155                      | 0.19  | 0.73 | 0.18  | 67.0 | 11.17 | 0.20 | 0.77 |
| 13103369–5800211 | 305.472  | 4.772    | 0.484  | 1      | –      | –    | g    | –        | –    | –      | D3   | c                      | ep         | –          | –     | –        | –          | –     | 9.306                              | 0.32                      | 1.14                      | 1                    | 77.6                               | 0.70                                 | 4.08                        | 9.126                       | 0.24  | 0.90 | 0.15  | 79.7 | 9.14  | 0.25 | 0.94 |
| 13104702–5746550 | 305.518  | 4.993    | 0.438  | 1      | –      | –    | g    | –        | –    | –      | D2   | c                      | o          | –          | –     | –        | –          | –     | 10.826                             | 0.58                      | 1.00                      | –2                   | 50.2                               | 0.72                                 | 4.06                        | 10.663                      | 0.51  | 0.78 | 0.14  | 51.6 | 10.67 | 0.52 | 0.81 |
| 13105341–5758079 | 305.518  | 4.805    | 0.471  | 1      | –      | –    | g    | –        | –    | –      | D1   | c                      | o          | –          | –     | –        | –          | –     | 10.852                             | 0.24                      | 1.05                      | 1                    | 51.2                               | 0.54                                 | 4.08                        | 10.677                      | 0.17  | 0.82 | 0.15  | 52.7 | 10.69 | 0.18 | 0.85 |
| 13110442–5816311 | 305.519  | 4.498    | 0.599  | 1      | –      | –    | g    | –        | –    | –      | D1   | c                      | o          | –          | –     | –        | –          | –     | 11.166                             | 0.53                      | 1.53                      | 1                    | 34.4                               | 0.42                                 | 4.13                        | 10.943                      | 0.43  | 1.23 | 0.19  | 35.9 | 10.96 | 0.44 | 1.27 |
| 13110865–6234415 | 305.199  | 0.207    | 58.315 | 9      | –      | –    | g    | –        | –    | –      | –    | –                      | –          | –          | –     | –        | –          | –     | 8.997                              | 1.34                      | ...                       | 1                    | 55.0                               | 0.60                                 | 4.62                        | –12.731                     | –8.32 | ...  | 18.06 | ...  | –7.18 | ...  |      |
| 13111431–6245005 | 305.196  | 0.035    | 50.662 | 9      | –      | –    | g    | –        | –    | –      | –    | –                      | –          | –          | –     | –        | –          | –     | 8.539                              | ...                       | ...                       | 1                    | 94.8                               | 0.68                                 | 4.62                        | –10.338                     | ...   | ...  | 15.69 | ...  | ...   | ...  |      |
| 13111621–6245505 | 305.199  | 0.020    | 51.603 | 9      | –      | –    | g    | –        | –    | –      | –    | –                      | –          | –          | –     | –        | –          | –     | 8.446                              | 1.31                      | ...                       | 1                    | 66.6                               | 0.84                                 | 4.57                        | –10.781                     | –7.24 | ...  | 15.98 | ...  | –6.22 | ...  |      |
| 13115832–5831276 | 305.617  | 4.240    | 0.733  | 1      | –      | –    | g    | –        | –    | –      | D3   | c                      | o          | –          | –     | –        | –          | –     | 10.223                             | 0.37                      | 1.30                      | 1                    | 49.2                               | 0.82                                 | 4.17                        | 9.950                       | 0.25  | 0.93 | 0.23  | 51.6 | 9.97  | 0.26 | 0.98 |
| 13121738–6242198 | 305.320  | 0.070    | 34.312 | 9      | –      | –    | g    | –        | –    | –      | –    | –                      | –          | –          | –     | –        | –          | –     | 6.787                              | 1.45                      | ...                       | 1                    | 170.6                              | 1.00                                 | 4.68                        | –5.998                      | –4.23 | ...  | 10.63 | ...  | –3.56 | ...  |      |
| 13122717–6233047 | 305.351  | 0.222    | 65.790 | 9      | –      | –    | g    | –        | –    | –      | –    | –                      | –          | –          | –     | –        | –          | –     | 9.418                              | ...                       | ...                       | 1                    | 74.4                               | 0.40                                 | 4.64                        | –15.095                     | ...   | ...  | 20.38 | ...  | ...   | ...  |      |
| 13122869–5829295 | 305.686  | 4.268    | 0.719  | 2      | –      | –    | g    | –        | –    | –      | n    | –                      | –          | –          | –     | –        | –          | –     | 11.397                             | 0.28                      | 1.26                      | 1                    | 33.0                               | 0.64                                 | 4.17                        | 11.129                      | 0.16  | 0.91 | 0.22  | 34.9 | 11.14 | 0.18 | 0.95 |
| 13123666–5827039 | 305.707  | 4.307    | 0.705  | 1      | –      | –    | g    | –        | –    | –      | P    | –                      | –          | –          | –     | –        | –          | –     | 10.674                             | 0.36                      | 1.23                      | 1                    | 53.2                               | 0.38                                 | 4.21                        | 10.411                      | 0.24  | 0.88 | 0.22  | 55.9 | 10.43 | 0.25 | 0.93 |
| 13132590–5716339 | 305.915  | 5.468    | 0.513  | 1      | –      | –    | g    | –        | –    | –      | D1   | c                      | o          | –          | –     | –        | –          | –     | 10.569                             | 0.30                      | 1.12                      | 1                    | 33.2                               | 0.70                                 | 4.04                        | 10.378                      | 0.21  | 0.86 | 0.16  | 34.2 | 10.40 | 0.22 | 0.90 |
| 13140807–5832409 | 305.897  | 4.196    | 0.795  | 1      | –      | –    | g    | –        | –    | –      | D1   | e                      | o          | –          | –     | –        | –          | –     | 9.041                              | 0.34                      | 1.21                      | 1                    | 87.6                               | 0.64                                 | 4.21                        | 8.745                       | 0.21  | 0.82 | 0.25  | 92.3 | 8.77  | 0.23 | 0.87 |
| 13142096–6244230 | 305.552  | 0.015    | 37.046 | 9      | –      | –    | g    | –        | –    | –      | –    | –                      | –          | –          | –     | –        | –          | –     | 8.619                              | ...                       | ...                       | 1                    | 85.2                               | 1.00                                 | 4.66                        | –5.184                      | ...   | ...  | 11.48 | ...  | ...   | ...  |      |
| 13142635–6244309 | 305.562  | 0.012    | 37.352 | 9      | –      | –    | g    | –        | –    | –      | –    | –                      | –          | –          | –     | –        | –          | –     | 7.795                              | 1.85                      | ...                       | 1                    | 141.2                              | 0.50                                 | 4.66                        | –6.122                      | –4.34 | ...  | 11.57 | ...  | –3.61 | ...  |      |
| 13144834–5522235 | 306.275  | 7.347    | 0.427  | 1      | –      | –    | g    | –        | –    | –      | D4   | c                      | o          | –          | –     | –        | –          | –     | 11.098                             | 0.31                      | 1.10                      | 1                    | 35.6                               | 0.76                                 | 3.80                        | 10.939                      | 0.24  | 0.88 | 0.13  | 36.6 | 10.95 | 0.25 | 0.91 |
| 13150638–5509225 | 306.338  | 7.559    | 0.391  | 1      | –      | –    | g    | –        | –    | –      | D1   | c                      | o          | –          | –     | –        | –          | –     | 10.228                             | 0.66                      | 1.65                      | 1                    | 29.2                               | 0.98                                 | 3.83                        | 10.082                      | 0.59  | 1.45 | 0.12  | 29.7 | 10.10 | 0.60 | 1.48 |
| 13150989–5856116 | 306.995  | 3.794    | 0.907  | 1      | –      | –    | g    | –        | –    | –      | D1   | e                      | o          | –          | –     | –        | –          | –     | 10.915                             | 0.35                      | 1.21                      | 1                    | 40.2                               | 0.66                                 | 4.23                        | 10.577                      | 0.20  | 0.76 | 0.28  | 44.0 | 10.55 | 0.22 | 0.82 |
| 13154453–5311486 | 306.618  | 9.501    | 0.445  | 1      | –      | –    | g    | –        | –    | –      | D2   | c                      | o          | –          | –     | –        | –          | –     | 10.305                             | 0.28                      | 1.11                      | 1                    | 51.4                               | 0.62                                 | 3.70                        | 10.139                      | 0.21  | 0.89 | 0.14  | 52.7 | 10.15 | 0.22 | 0.92 |
| 13162860–5834549 | 306.199  | 4.131    | 0.854  | 1      | –      | –    | g    | –        | –    | –      | P    | –                      | –          | –          | –     | –        | –          | –     | 11.198                             | 0.46                      | 1.37                      | 1                    | 55.0                               | 0.28                                 | 4.19                        | 10.880                      | 0.32  | 0.94 | 0.26  | 59.9 | 10.85 | 0.33 | 1.00 |
| 13183230–5832091 | 306.472  | 4.149    | 0.768  | 1      | –      | –    | g    | –        | –    | –      | P    | –                      | –          | –          | –     | –        | –          | –     | 10.189                             | 0.32                      | 1.19                      | 1                    | 44.4                               | 0.82                                 | 4.23                        | 9.903                       | 0.19  | 0.81 | 0.24  | 46.7 | 9.93  | 0.21 | 0.86 |
| 13184507–5803262 | 306.550  | 4.622    | 0.669  | 1      | –      | –    | g    | –        | –    | –      | P    | –                      | –          | –          | –     | –        | –          | –     | 10.927                             | 0.35                      | 1.23                      | 1                    | 41.0                               | 0.94                                 | 4.14                        | 10.678                      | 0.24  | 0.90 | 0.21  | 43.1 | 10.69 | 0.25 | 0.94 |
| 13190643–5744311 | 306.631  | 4.931    | 0.735  | 1      | –      | –    | g    | –        | –    | –      | D1   | c                      | o          | –          | –     | –        | –          | –     | 11.413                             | 0.39                      | 1.24                      |                      |                                    |                                      |                             |                             |       |      |       |      |       |      |      |

Table B1: a) continued.

| 2MASX J          | <i>l</i>    | <i>b</i>    | EBV        | Object       | Sample     | Disc       | 2MRS        | Velocity   | NIR         | Photom        | Ext         | <i>K</i> <sub>20</sub> | <i>H-K</i>   | <i>J-K</i>  | vc          | <i>a</i>    | <i>b/a</i>  | st.d. | <i>K</i> <sub>s</sub> <sup>o</sup> | ( <i>H-K</i> ) <sup>o</sup> | ( <i>J-K</i> ) <sup>o</sup> | <i>A</i> <sub>K</sub> | <i>a</i> <sub>d</sub> <sup>o</sup> | <i>K</i> <sub>s</sub> <sup>o,d</sup> | ( <i>H-K</i> ) <sup>o,c</sup> | ( <i>J-K</i> ) <sup>o,c</sup> |             |             |       |             |             |             |        |
|------------------|-------------|-------------|------------|--------------|------------|------------|-------------|------------|-------------|---------------|-------------|------------------------|--------------|-------------|-------------|-------------|-------------|-------|------------------------------------|-----------------------------|-----------------------------|-----------------------|------------------------------------|--------------------------------------|-------------------------------|-------------------------------|-------------|-------------|-------|-------------|-------------|-------------|--------|
| (1)              | deg<br>(2a) | deg<br>(2b) | mag<br>(3) | class<br>(4) | off<br>(5) | flg<br>(6) | gal<br>(7a) | TF<br>(7b) | obs<br>(7c) | ext'd<br>(7d) | type<br>(8) | (9)                    | Opt<br>(10a) | HI<br>(10b) | flg<br>(11) | flg<br>(12) | flg<br>(13) | (14)  | mag<br>(15)                        | mag<br>(16)                 | (17)                        | (18)                  | (19)                               | (20)                                 | mag<br>(21)                   | mag<br>(22)                   | mag<br>(23) | mag<br>(24) | (25)  | mag<br>(26) | mag<br>(27) | mag<br>(28) |        |
| 13283697–5742188 | 307.900     | 4.807       | 0.703      | 1            | –          | –          | g           | –          | –           | –             | D2          | –                      | o            | –           | –           | –           | –           | –     | 10.746                             | 0.33                        | 1.15                        | 1                     | 46.4                               | 0.70                                 | 4.12                          | 10.484                        | 0.21        | 0.80        | 0.22  | 48.8        | 10.50       | 0.23        | 0.85   |
| 13291753–5756032 | 307.956     | 4.568       | 0.658      | 1            | –          | –          | g           | –          | –           | –             | D1          | –                      | o            | –           | –           | –           | –           | –     | 11.166                             | 0.31                        | 1.22                        | 1                     | 31.6                               | 0.40                                 | 4.19                          | 10.921                        | 0.20        | 0.89        | 0.20  | 33.0        | 10.94       | 0.21        | 0.93   |
| 13293316–5850552 | 307.855     | 3.658       | 0.725      | 1            | –          | –          | g           | –          | –           | –             | D1          | –                      | –            | h           | –           | –           | –           | –     | 10.894                             | 0.38                        | 1.21                        | 1                     | 57.2                               | 0.64                                 | 4.27                          | 10.624                        | 0.26        | 0.85        | 0.22  | 60.9        | 10.62       | 0.28        | 0.90   |
| 13295188–6827036 | 306.465     | –5.843      | 0.470      | 1            | –          | –          | g           | –          | –           | –             | D2          | c                      | o            | –           | –           | –           | –           | –     | 10.949                             | 0.34                        | 1.19                        | 1                     | 40.8                               | 0.68                                 | 4.05                          | 10.774                        | 0.27        | 0.96        | 0.15  | 42.0        | 10.79       | 0.28        | 0.99   |
| 13295273–5732075 | 308.093     | 4.951       | 0.814      | 2            | –          | –          | g           | –          | –           | –             | D2          | –                      | –            | –           | –           | –           | –           | –     | 11.490                             | 0.49                        | 1.47                        | 1                     | 35.4                               | 0.38                                 | 4.12                          | 11.187                        | 0.36        | 1.06        | 0.25  | 37.8        | 11.19       | 0.37        | 1.12   |
| 13295575–5439406 | 308.532     | 7.791       | 0.433      | 1            | –          | –          | g           | –          | –           | –             | D1          | c                      | o            | o           | h           | V           | –           | –     | 11.360                             | 0.33                        | 0.99                        | 1                     | 41.8                               | 0.80                                 | 3.88                          | 11.199                        | 0.26        | 0.77        | 0.13  | 43.3        | 11.19       | 0.26        | 0.80   |
| 13300509–5534147 | 308.417     | 6.889       | 0.510      | 1            | –          | –          | g           | –          | –           | –             | D1          | c                      | o            | o           | h           | V           | –           | –     | 10.620                             | 0.20                        | 0.95                        | 1                     | 62.4                               | 0.84                                 | 3.91                          | 10.430                        | 0.11        | 0.70        | 0.16  | 65.0        | 10.43       | 0.12        | 0.73   |
| 13310962–5809453 | 308.166     | 4.305       | 0.666      | 2            | –          | –          | g           | –          | –           | –             | n           | –                      | –            | –           | –           | –           | –           | –     | 11.396                             | 0.40                        | 1.23                        | 1                     | 24.0                               | 0.80                                 | 4.25                          | 11.148                        | 0.29        | 0.90        | 0.21  | 25.2        | 11.16       | 0.30        | 0.95   |
| 13313318–5750054 | 308.269     | 4.621       | 0.647      | 1            | –          | –          | g           | –          | –           | –             | D1          | –                      | –            | –           | –           | –           | –           | –     | 10.514                             | 0.39                        | 1.30                        | 1                     | 53.0                               | 0.40                                 | 4.11                          | 10.273                        | 0.29        | 0.98        | 0.20  | 55.4        | 10.29       | 0.30        | 1.02   |
| 13314368–5753125 | 308.284     | 4.566       | 0.676      | 1            | –          | –          | g           | –          | –           | –             | D3          | e                      | o            | –           | –           | –           | –           | –     | 10.702                             | 0.35                        | 1.21                        | 1                     | 29.2                               | 0.80                                 | 4.11                          | 10.450                        | 0.24        | 0.87        | 0.21  | 30.5        | 10.47       | 0.25        | 0.92   |
| 13314873–6516385 | 307.140     | –2.736      | 1.264      | 1            | –          | –          | g           | –          | –           | –             | D1          | e                      | –            | –           | h           | –           | –           | –     | 10.387                             | 0.39                        | 1.51                        | 1                     | 45.6                               | 0.80                                 | 4.45                          | 9.916                         | 0.19        | 0.89        | 0.39  | 51.2        | 9.92        | 0.21        | 0.97   |
| 13324576–6026565 | 308.010     | 2.015       | 4.960      | 9            | –          | –          | g           | –          | –           | –             | –           | –                      | –            | –           | –           | –           | –           | –     | 8.905                              | ...                         | ...                         | 1                     | 120.0                              | 0.76                                 | 4.51                          | 7.057                         | ...         | ...         | 1.54  | ...         | ...         | ...         |        |
| 13331968–5321170 | 309.238     | 9.003       | 0.299      | 1            | –          | –          | g           | –          | –           | –             | D1          | c                      | o            | –           | –           | V           | –           | –     | 9.801                              | 0.20                        | 0.95                        | 1                     | 96.0                               | 0.44                                 | 3.77                          | 9.690                         | 0.15        | 0.80        | 0.09  | 97.5        | 9.70        | 0.16        | 0.82   |
| 13333914–5747422 | 308.552     | 4.615       | 0.677      | 1            | –          | –          | g           | –          | –           | –             | D2          | e                      | –            | –           | –           | –           | –           | –     | 10.459                             | 0.33                        | 1.18                        | 1                     | 35.6                               | 0.88                                 | 4.11                          | 10.207                        | 0.22        | 0.84        | 0.21  | 37.3        | 10.22       | 0.23        | 0.89   |
| 13361064–5632237 | 309.103     | 5.795       | 0.700      | 1            | o          | –          | g           | –          | –           | –             | D1          | c                      | o            | –           | h           | V           | o           | –     | 10.658                             | 0.41                        | 0.94                        | 1                     | 112.2                              | 0.34                                 | 4.02                          | 10.397                        | 0.29        | 0.59        | 0.22  | 120.6       | 10.36       | 0.31        | 0.63   |
| 13362981–5504481 | 309.404     | 7.225       | 0.549      | 1            | –          | –          | g           | –          | –           | –             | D1          | c                      | o            | o           | h           | V           | –           | –     | 10.645                             | 0.40                        | 1.23                        | 1                     | 61.6                               | 0.92                                 | 3.89                          | 10.440                        | 0.31        | 0.95        | 0.17  | 53.7        | 10.45       | 0.32        | 0.99   |
| 13363492–5720032 | 309.019     | 5.003       | 0.677      | 1            | o          | –          | g           | –          | –           | –             | D1          | c                      | o            | –           | –           | o           | –           | –     | 11.100                             | 0.48                        | 1.26                        | 1                     | 52.6                               | 0.48                                 | 4.12                          | 10.848                        | 0.36        | 0.92        | 0.21  | 66.7        | 10.83       | 0.38        | 0.97   |
| 13363595–5455552 | 309.445     | 7.368       | 0.557      | 1            | –          | –          | g           | –          | –           | –             | D1          | c                      | o            | o           | h           | V           | –           | –     | 11.125                             | 0.27                        | 1.15                        | 1                     | 52.8                               | 0.52                                 | 3.89                          | 10.917                        | 0.18        | 0.87        | 0.17  | 55.0        | 10.93       | 0.19        | 0.91   |
| 13371698–5504342 | 309.516     | 7.208       | 0.567      | 1            | –          | –          | g           | –          | –           | –             | D1          | c                      | o            | –           | h           | V           | –           | –     | 11.361                             | 0.37                        | 1.19                        | 1                     | 45.8                               | 0.46                                 | 3.89                          | 11.150                        | 0.27        | 0.91        | 0.18  | 48.0        | 11.15       | 0.28        | 0.95   |
| 13372458–5852216 | 308.855     | 3.469       | 1.091      | 1            | –          | –          | g           | –          | –           | –             | D1          | –                      | –            | –           | h           | –           | –           | –     | 10.028                             | 0.34                        | 1.24                        | 1                     | 69.4                               | 0.26                                 | 4.31                          | 9.621                         | 0.16        | 0.70        | 0.34  | 75.3        | 9.65        | 0.18        | 0.77   |
| 13373282–5854136 | 308.867     | 3.436       | 1.092      | 1            | –          | –          | g           | –          | –           | –             | D1          | –                      | –            | –           | h           | –           | –           | –     | 9.669                              | 0.48                        | 1.40                        | 1                     | 96.8                               | 0.46                                 | 4.31                          | 9.262                         | 0.30        | 0.86        | 0.34  | 104.9       | 9.29        | 0.32        | 0.93   |
| 13375912–5830556 | 308.992     | 3.808       | 1.127      | 1            | –          | –          | g           | –          | –           | –             | n           | –                      | –            | –           | –           | –           | –           | –     | 11.189                             | 0.61                        | 1.58                        | 1                     | 33.0                               | 0.60                                 | 4.28                          | 10.769                        | 0.42        | 1.02        | 0.35  | 36.7        | 10.76       | 0.44        | 1.10   |
| 13380855–5845197 | 308.969     | 3.568       | 0.997      | 2            | –          | –          | g           | –          | –           | –             | D3          | –                      | –            | –           | –           | –           | –           | –     | 10.926                             | 0.36                        | 1.39                        | 1                     | 25.8                               | 0.86                                 | 4.30                          | 10.555                        | 0.19        | 0.89        | 0.31  | 27.8        | 10.58       | 0.21        | 0.96   |
| 13402175–7107449 | 306.906     | –8.636      | 0.424      | 1            | –          | –          | g           | –          | –           | –             | D1          | c                      | o            | –           | h           | –           | –           | –     | 10.346                             | 0.39                        | 1.27                        | 1                     | 61.6                               | 0.42                                 | 3.79                          | 10.188                        | 0.32        | 1.06        | 0.13  | 63.3        | 10.20       | 0.33        | 1.09   |
| 13405761–6145447 | 308.754     | 0.548       | 27.394     | 9            | –          | –          | g           | –          | –           | –             | –           | –                      | –            | –           | –           | –           | –           | –     | 8.217                              | ...                         | ...                         | 1                     | 233.2                              | 0.36                                 | 4.71                          | –1.990                        | ...         | ...         | 8.49  | ...         | ...         | ...         |        |
| 13440358–6019350 | 309.405     | 1.882       | 2.509      | 1            | –          | –          | g           | –          | –           | –             | D2          | –                      | –            | –           | –           | V           | –           | –     | 10.281                             | 0.55                        | ...                         | 1                     | 44.4                               | 0.88                                 | 4.50                          | 9.346                         | 0.14        | ...         | 0.78  | 57.3        | 9.35        | 0.18        | ...    |
| 13442388–5222099 | 311.087     | 9.662       | 0.449      | 1            | –          | –          | g           | –          | –           | –             | D1          | c                      | o            | –           | h           | V           | –           | –     | 10.050                             | 0.32                        | 1.27                        | 1                     | 102.4                              | 0.26                                 | 3.74                          | 9.883                         | 0.25        | 1.05        | 0.14  | 105.6       | 9.89        | 0.26        | 1.08   |
| 13445626–6540515 | 308.408     | –3.380      | 0.891      | 1            | –          | –          | g           | –          | –           | –             | D1          | e                      | o            | –           | h           | –           | –           | –     | 9.755                              | 0.40                        | 1.33                        | 1                     | 78.8                               | 0.46                                 | 4.40                          | 9.423                         | 0.26        | 0.89        | 0.28  | 83.8        | 9.45        | 0.27        | 0.95   |
| 13453054–7118422 | 307.280     | –8.898      | 0.364      | 1            | –          | –          | g           | –          | –           | –             | D1          | c                      | o            | –           | –           | –           | –           | –     | 10.733                             | 0.39                        | 1.22                        | 1                     | 44.8                               | 0.52                                 | 3.75                          | 10.597                        | 0.33        | 1.04        | 0.11  | 45.8        | 10.61       | 0.33        | 1.06   |
| 13455154–6009067 | 309.659     | 2.007       | 1.989      | 1            | o          | –          | g           | –          | –           | –             | D2          | –                      | –            | –           | –           | o           | –           | –     | 10.635                             | 0.42                        | ...                         | –2                    | 48.6                               | 0.56                                 | 4.54                          | 9.894                         | 0.09        | ...         | 0.62  | 60.7        | 9.85        | 0.13        | ...    |
| 13462058–6247597 | 309.159     | –0.594      | 13.835     | 8            | –          | –          | g           | –          | –           | –             | –           | –                      | –            | –           | V           | –           | –           | –     | 8.827                              | 1.43                        | 3.39                        | 1                     | 51.2                               | 0.54                                 | 4.72                          | 3.672                         | –0.86       | –3.49       | 4.29  | ...         | ...         | –0.59       | –2.57  |
| 13463702–6239303 | 309.220     | –0.462      | 27.021     | 8            | –          | –          | g           | –          | –           | –             | –           | –                      | –            | –           | –           | –           | –           | –     | 6.780                              | ...                         | ...                         | 1                     | 64.0                               | 0.20                                 | 4.67                          | –3.288                        | ...         | ...         | 8.37  | ...         | ...         | ...         |        |
| 13464910–6024299 | 309.722     | 1.731       | 2.971      | 1            | –          | –          | g           | –          | –           | –             | D2          | e                      | o            | –           | –           | V           | –           | –     | 8.719                              | 0.65                        | 2.15                        | 1                     | 99.6                               | 0.80                                 | ...                           | 7.612                         | 0.16        | 0.67        | 0.92  | ...         | ...         | 0.22        | 0.87   |
| 13471848–6034133 | 309.746     | 1.560       | 2.949      | 1            | –          | –          | g           | –          | –           | –             | D1          | –                      | –            | –           | –           | V           | –           | –     | 9.743                              | 0.70                        | ...                         | 1                     | 93.6                               | 0.22                                 | 4.55                          | 8.644                         | 0.21        | ...         | 0.91  | 131.5       | 8.60        | 0.27        | ...    |
| 13502487–6005380 | 310.226     | 1.940       | 2.314      | 1            | –          | –          | g           | –          | –           | –             | D1          | –                      | –            | –           | –           | V           | –           | –     | 11.354                             | 0.44                        | ...                         | 1                     | 29.2                               | 0.66                                 | 4.50                          | 10.492                        | 0.05        | ...         | 0.72  | 37.5        | 10.47       | 0.10        | ...    |
| 13502826–5239385 | 311.936     | 9.176       | 0.397      | 1            | –          | –          | g           | –          | –           | –             | D1          | c                      | o            | –           | h           | V           | –           | –     | 9.810                              | 0.34                        | 1.10                        | 1                     | 72.6                               | 0.64                                 | 3.73                          | 9.662                         | 0.28        | 0.90        | 0.12  | 74.5        | 9.67        | 0.29        | 0.92   |
| 13502912–5256475 | 311.872     | 8.897       | 0.413      | 1            | –          | –          | g           | –          | –           | –             | D1          | c                      | o            | –           | h           | V           | –           | –     | 11.110                             | 0.23                        | 1.08                        | 1                     | 50.0                               | 0.84                                 | 3.80                          | 10.956                        | 0.16        | 0.87        | 0.13  | 51.6        | 10.95       | 0.17        | 0.90   |
| 13503488–6140199 | 309.888     | 0.398       | 34.416     | 9            | –          | –          | g           | –          | –           | –             | –           | –                      | –            | –           | –           | –           | –           | –     | 7.963                              | 1.47                        | 3.10                        | 1                     | 118.4                              | 0.76                                 | 4.60                          | –4.860                        | –4.23       | –14.00      | 10.66 | ...         | ...         | –3.56       | –11.73 |
| 13504691–5923083 | 310.432     | 2.619       | 1.462      | 2            | –          | –          | g           | –          | –           | –             | D3          | –                      | –            | –           | –           | –           | –           | –     | 11.338                             | 0.49                        | ...                         | 1                     | 32.0                               | 0.76                                 | 4.47                          | 10.793                        | 0.25        | ...         | 0.45  | 36.9        | 10.79       | 0.28        | ...    |
| 13510266–6130150 | 309.980     | 0.549       | 18.597     | 8            | –          | –          | g           | –          | –           | –             | –           | –                      | –            | –           | V           | –           | –           | –     | 9.037                              | 1.99                        | ...                         | 1                     | 57.2                               | 0.58                                 | 4.60                          | 2.108                         | –1.09       | ...         | 5.76  | ...         | ...         | –0.73       |        |
| 13513072–5255237 | 312.030     | 0.393       | 1          | –            | –          | –          | g           | –          | –           | –             | D1          | c                      | o            | –           | h           | V           | –           | –     | 10.746                             | 0.29                        | 1.07                        | 1                     | 47.4                               | 0.74                                 | 3.80                          | 10.600                        | 0.23        | 0.87        | 0.12  | 48.8        | 10.60       | 0.23        | 0.90   |
| 13513848–5835153 | 310.724     | 3.370       | 0.996      | 1            | –          | –          | g           | –          | –           | –             | D2          | e                      | o            | –           | h           | –           | –           | –     | 8.577                              | 0.41                        | 1.34                        | 1                     | 94.4                               | 0.58</                               |                               |                               |             |             |       |             |             |             |        |



Table B1: a) continued.

| 2MASX J          | <i>l</i>    | <i>b</i>    | EBV        | Object       | Sample     | Disc        | 2MRS        | Velocity   | NIR         | Photom        | Ext         | <i>K</i> <sub>20</sub> | <i>H-K</i>   | <i>J-K</i>  | vc           | <i>a</i>     | <i>b/a</i>   | st.d. | <i>K</i> <sub>s</sub> <sup>o</sup> | ( <i>H-K</i> ) <sup>o</sup> | ( <i>J-K</i> ) <sup>o</sup> | <i>A<sub>K</sub></i> | <i>a</i> <sub>d</sub> <sup>o</sup> | <i>K</i> <sub>s</sub> <sup>o,d</sup> | ( <i>H-K</i> ) <sup>o,c</sup> | ( <i>J-K</i> ) <sup>o,c</sup> |             |             |      |             |             |             |       |       |
|------------------|-------------|-------------|------------|--------------|------------|-------------|-------------|------------|-------------|---------------|-------------|------------------------|--------------|-------------|--------------|--------------|--------------|-------|------------------------------------|-----------------------------|-----------------------------|----------------------|------------------------------------|--------------------------------------|-------------------------------|-------------------------------|-------------|-------------|------|-------------|-------------|-------------|-------|-------|
| (1)              | deg<br>(2a) | deg<br>(2b) | mag<br>(3) | class<br>(4) | off<br>(5) | flag<br>(6) | gal<br>(7a) | TF<br>(7b) | obs<br>(7c) | ext'd<br>(7d) | type<br>(8) | (9)                    | Opt<br>(10a) | HI<br>(10b) | flag<br>(11) | flag<br>(12) | flag<br>(13) | (14)  | mag<br>(15)                        | mag<br>(16)                 | (17)                        | (18)                 | (19)                               | (20)                                 | mag<br>(21)                   | mag<br>(22)                   | mag<br>(23) | mag<br>(24) | (25) | mag<br>(26) | mag<br>(27) | mag<br>(28) |       |       |
| 14103615–6534583 | 310.997     | –3.958      | 0.608      | 1            | –          | –           | g           | –          | –           | –             | D1          | e                      | o            | –           | –            | –            | –            | –     | 8.764                              | 0.33                        | 1.17                        | 1                    | 115.0                              | 0.52                                 | 4.34                          | 8.537                         | 0.23        | 0.86        | 0.19 | 119.1       | 8.56        | 0.24        | 0.90  |       |
| 14103702–5206059 | 315.087     | 8.892       | 0.500      | 1            | –          | –           | –           | –          | –           | –             | D4          | c                      | o            | –           | –            | –            | –            | –     | 10.723                             | 0.31                        | 1.17                        | 1                    | 33.4                               | 0.88                                 | 3.80                          | 10.537                        | 0.23        | 0.92        | 0.15 | 34.4        | 10.55       | 0.24        | 0.95  |       |
| 14103822–6534568 | 311.001     | –3.959      | 0.607      | 9            | e          | –           | –           | –          | –           | –             | –           | –                      | –            | –           | –            | –            | –            | –     | 9.845                              | 0.26                        | 1.11                        | 1                    | 66.8                               | 0.80                                 | 4.36                          | 9.619                         | 0.16        | 0.81        | 0.19 | –           | –           | 0.17        | 0.85  |       |
| 14104114–5211029 | 315.071     | 8.810       | 0.482      | 1            | –          | –           | g           | –          | –           | –             | D1          | c                      | o            | –           | –            | –            | –            | –     | 10.848                             | 0.40                        | 1.22                        | 1                    | 60.0                               | 0.30                                 | 3.79                          | 10.668                        | 0.32        | 0.98        | 0.15 | 62.2        | 10.67       | 0.33        | 1.01  |       |
| 14123376–5634412 | 313.974     | 4.544       | 0.660      | 1            | o          | –           | –           | –          | –           | –             | D1          | c                      | o            | –           | –            | –            | –            | –     | 10.340                             | 0.29                        | 1.03                        | 1                    | 100.2                              | 0.48                                 | 4.24                          | 10.094                        | 0.18        | 0.71        | 0.20 | 105.2       | 10.11       | 0.19        | 0.75  |       |
| 14123838–5550342 | 314.213     | 5.240       | 0.531      | 1            | –          | –           | –           | –          | –           | –             | D4          | c                      | o            | –           | –            | –            | –            | –     | 10.889                             | 0.32                        | 1.22                        | 1                    | 30.6                               | 0.78                                 | 4.13                          | 10.691                        | 0.23        | 0.95        | 0.16 | 31.7        | 10.71       | 0.24        | 0.99  |       |
| 14130990–6520204 | 311.326     | –3.808      | 1.456      | 1            | –          | –           | –           | –          | –           | –             | D1          | e                      | o            | –           | –            | –            | –            | –     | 5.039                              | 0.38                        | 1.27                        | 1                    | 519.0                              | 0.41                                 | –                             | 4.496                         | 0.13        | 0.55        | 0.45 | –           | –           | 0.16        | 0.64  |       |
| 14143959–6222433 | 312.412     | –1.049      | 6.906      | 9            | –          | –           | –           | –          | –           | –             | –           | –                      | –            | –           | –            | –            | –            | –     | 10.615                             | –                           | –                           | –2                   | 35.2                               | 0.86                                 | 4.72                          | 8.042                         | –           | –           | –    | 2.14        | –           | –           | –     |       |
| 14151775–5419457 | 315.055     | 6.557       | 0.580      | 1            | –          | –           | –           | –          | –           | –             | D1          | c                      | o            | –           | –            | –            | –            | –     | 11.289                             | 0.43                        | 1.21                        | 1                    | 34.4                               | 0.62                                 | 3.97                          | 11.073                        | 0.33        | 0.93        | 0.18 | 35.9        | 11.08       | 0.34        | 0.96  |       |
| 14154417–5719118 | 314.151     | 3.704       | 1.259      | 2            | –          | –           | –           | –          | –           | –             | D3          | –                      | –            | –           | –            | –            | –            | –     | 10.874                             | 0.39                        | 1.47                        | 1                    | 38.4                               | 0.78                                 | 4.27                          | 10.405                        | 0.18        | 0.84        | 0.39 | 42.6        | 10.42       | 0.21        | 0.93  |       |
| 14155209–5855348 | 313.652     | 2.177       | 2.112      | 1            | –          | –           | –           | –          | –           | –             | D1          | c                      | o            | –           | –            | –            | –            | –     | 10.859                             | 0.65                        | –                           | 1                    | 40.4                               | 0.54                                 | 4.50                          | 10.072                        | 0.30        | –           | 0.65 | 50.1        | 10.07       | 0.35        | –     |       |
| 14155392–5200405 | 315.895     | 8.722       | 0.423      | 1            | –          | –           | –           | –          | –           | –             | D1          | c                      | o            | –           | –            | –            | –            | –     | 10.044                             | 0.40                        | 1.24                        | 1                    | 39.0                               | 0.74                                 | 3.74                          | 9.886                         | 0.33        | 1.03        | 0.13 | 40.0        | 9.90        | 0.34        | 1.06  |       |
| 14160206–5342595 | 315.357     | 7.102       | 0.577      | 1            | –          | –           | –           | –          | –           | –             | D1          | c                      | o            | –           | –            | –            | –            | –     | 10.257                             | 0.33                        | 1.21                        | 1                    | 54.4                               | 0.92                                 | 3.96                          | 10.042                        | 0.24        | 0.93        | 0.18 | 56.4        | 10.06       | 0.25        | 0.97  |       |
| 14160447–5236315 | 315.725     | 8.148       | 0.436      | 1            | –          | –           | –           | –          | –           | –             | D1          | c                      | o            | –           | –            | –            | –            | –     | 9.303                              | 0.30                        | 1.10                        | 1                    | 95.2                               | 0.30                                 | 3.87                          | 9.141                         | 0.22        | 0.88        | 0.14 | 97.4        | 9.16        | 0.23        | 0.91  |       |
| 14171004–5532394 | 314.915     | 5.320       | 0.622      | 1            | –          | –           | –           | –          | –           | –             | D1          | c                      | o            | –           | –            | –            | –            | –     | 9.764                              | 0.47                        | 1.47                        | 1                    | 117.6                              | 0.18                                 | 4.04                          | 9.532                         | 0.37        | 1.16        | 0.19 | 123.0       | 9.54        | 0.38        | 1.20  |       |
| 14181728–5633251 | 314.730     | 4.312       | 0.903      | 2            | –          | –           | –           | –          | –           | –             | D3          | –                      | –            | –           | –            | –            | –            | –     | 11.496                             | 0.44                        | 1.28                        | 1                    | 38.8                               | 0.60                                 | 4.22                          | 11.160                        | 0.29        | 0.84        | 0.28 | 42.1        | 11.16       | 0.31        | 0.89  |       |
| 14182995–6432216 | 312.119     | –3.232      | 0.926      | 1            | –          | –           | –           | –          | –           | –             | D1          | c                      | o            | –           | –            | –            | –            | –     | 11.477                             | –                           | –                           | –                    | 31.6                               | 0.52                                 | 4.43                          | 11.132                        | –           | –           | 0.29 | 34.4        | 11.13       | –           | –     |       |
| 14190092–5447141 | 315.417     | 5.948       | 0.573      | 1            | –          | –           | –           | –          | –           | –             | D1          | c                      | o            | –           | –            | –            | –            | –     | 10.715                             | 0.33                        | 1.24                        | 1                    | 48.8                               | 0.66                                 | 4.02                          | 10.502                        | 0.23        | 0.95        | 0.18 | 50.7        | 10.52       | 0.24        | 0.99  |       |
| 14191556–5728491 | 314.548     | 3.397       | 1.802      | 2            | –          | –           | –           | –          | –           | –             | D3          | –                      | –            | –           | –            | –            | –            | –     | 11.704                             | 0.41                        | 1.60                        | 1                    | 34.2                               | 0.48                                 | 4.29                          | 11.033                        | 0.11        | 0.70        | 0.56 | 42.3        | 10.97       | 0.15        | 0.82  |       |
| 14192257–5710270 | 314.665     | 3.681       | 1.121      | 1            | –          | –           | –           | –          | –           | –             | D1          | c                      | o            | –           | –            | –            | –            | –     | 11.637                             | 0.44                        | 1.53                        | 1                    | 26.8                               | 0.50                                 | 4.29                          | 11.219                        | 0.25        | 0.97        | 0.35 | 29.6        | 11.22       | 0.28        | 1.05  |       |
| 14193375–5808521 | 314.363     | 2.755       | 1.553      | 1            | –          | –           | –           | –          | –           | –             | D1          | –                      | –            | –           | –            | –            | –            | –     | 9.646                              | 0.23                        | 1.37                        | 1                    | 232.8                              | 0.46                                 | 4.44                          | 9.067                         | –0.02       | 0.59        | 0.48 | 273.4       | 9.05        | 0.01        | 0.70  |       |
| 14201249–6821595 | 310.995     | –6.896      | 0.513      | 4            | –          | –           | –           | –          | –           | –             | D4          | cr                     | o            | –           | –            | –            | –            | –     | 10.754                             | 0.32                        | 1.12                        | 1                    | 42.4                               | 0.66                                 | 3.99                          | 10.563                        | 0.23        | 0.87        | 0.16 | 43.8        | 10.58       | 0.24        | 0.90  |       |
| 14202352–5504074 | 315.509     | 5.616       | 0.604      | 1            | –          | –           | –           | –          | –           | –             | D1          | c                      | o            | –           | –            | –            | –            | –     | 10.668                             | 0.40                        | 1.12                        | 1                    | 45.8                               | 0.70                                 | 4.07                          | 10.443                        | 0.30        | 0.82        | 0.19 | 48.2        | 10.44       | 0.32        | 0.86  |       |
| 14204296–5806485 | 314.518     | 2.736       | 1.576      | 2            | –          | –           | –           | –          | –           | –             | D2          | c                      | o            | –           | –            | –            | –            | –     | 11.421                             | 0.39                        | –                           | 1                    | 24.4                               | 0.82                                 | 4.46                          | 10.834                        | 0.13        | –           | 0.49 | 28.8        | 10.81       | 0.16        | –     |       |
| 14231328–5017506 | 317.578     | 9.946       | 0.387      | 1            | –          | –           | –           | –          | –           | –             | D1          | c                      | o            | –           | –            | –            | –            | –     | 10.948                             | 0.33                        | 1.24                        | 1                    | 43.4                               | 0.36                                 | 3.76                          | 10.804                        | 0.26        | 1.04        | 0.12 | 44.4        | 10.82       | 0.27        | 1.07  |       |
| 14242344–6205208 | 313.577     | –1.154      | 9.821      | 9            | –          | –           | –           | –          | –           | –             | –           | –                      | –            | –           | –            | –            | –            | –     | 9.628                              | –                           | –                           | –                    | 68.0                               | 0.54                                 | 4.72                          | 5.969                         | –           | –           | –    | 3.04        | –           | –           | –     |       |
| 14242759–5808510 | 314.971     | 2.533       | 2.034      | 3            | –          | –           | –           | –          | –           | –             | –           | –                      | –            | –           | –            | –            | –            | –     | 10.866                             | 0.54                        | 1.71                        | 1                    | 37.4                               | 0.90                                 | 4.47                          | 10.108                        | 0.21        | 0.70        | 0.63 | 46.3        | 10.09       | 0.25        | 0.83  |       |
| 14243655–6358490 | 312.935     | –2.933      | 1.224      | 3            | –          | –           | –           | –          | –           | –             | –           | –                      | –            | –           | –            | –            | –            | –     | 10.803                             | 0.41                        | 1.43                        | 1                    | 34.6                               | 0.80                                 | 4.48                          | 10.347                        | 0.21        | 0.83        | 0.38 | 38.0        | 10.38       | 0.23        | 0.91  |       |
| 14245658–6144520 | 313.758     | –0.857      | 9.881      | 9            | –          | –           | –           | –          | –           | –             | –           | –                      | –            | –           | –            | –            | –            | –     | 8.138                              | 1.34                        | 3.12                        | 1                    | 158.2                              | 0.30                                 | 4.72                          | 4.456                         | –0.29       | –           | 1.78 | 3.06        | –           | –           | –0.10 | –1.13 |
| 14251293–5243085 | 317.002     | 7.572       | 0.553      | 1            | –          | –           | –           | –          | –           | –             | D1          | c                      | o            | –           | –            | –            | –            | –     | 10.999                             | 0.36                        | 1.32                        | 1                    | 37.6                               | 0.62                                 | 3.93                          | 10.793                        | 0.27        | 1.05        | 0.17 | 39.0        | 10.81       | 0.28        | 1.08  |       |
| 14260346–5547190 | 316.014     | 4.661       | 0.842      | 1            | –          | –           | –           | –          | –           | –             | D4          | c                      | o            | –           | –            | –            | –            | –     | 10.781                             | 0.49                        | 1.46                        | 1                    | 37.4                               | 0.92                                 | 4.15                          | 10.467                        | 0.35        | 1.04        | 0.26 | 39.8        | 10.48       | 0.37        | 1.10  |       |
| 14263054–5422051 | 316.587     | 5.964       | 0.774      | 1            | o          | –           | –           | –          | –           | –             | D1          | c                      | o            | –           | –            | –            | –            | –     | 11.287                             | 0.43                        | 1.30                        | 1                    | 56.6                               | 0.28                                 | 4.03                          | 10.999                        | 0.30        | 0.91        | 0.24 | 61.2        | 10.97       | 0.31        | 0.97  |       |
| 14263555–5244028 | 317.193     | 7.483       | 0.558      | 1            | –          | –           | –           | –          | –           | –             | D1          | c                      | o            | –           | –            | –            | –            | –     | 10.764                             | 0.45                        | 1.28                        | 1                    | 56.2                               | 0.40                                 | 3.92                          | 10.556                        | 0.36        | 1.00        | 0.17 | 58.4        | 10.57       | 0.37        | 1.04  |       |
| 14275344–5844595 | 315.174     | 1.810       | 3.855      | 8            | –          | –           | –           | –          | –           | –             | D1          | c                      | o            | –           | –            | –            | –            | –     | 7.994                              | 0.71                        | 2.34                        | –2                   | 29.4                               | 0.56                                 | 4.58                          | 6.558                         | 0.07        | 0.43        | 1.19 | –           | –           | 0.15        | 0.68  |       |
| 14282893–5303195 | 317.342     | 7.080       | 0.586      | 1            | o          | –           | –           | –          | –           | –             | D1          | c                      | o            | –           | –            | –            | –            | –     | 11.207                             | 0.32                        | 1.17                        | 1                    | 34.0                               | 0.54                                 | 3.98                          | 10.989                        | 0.22        | 0.88        | 0.18 | 35.5        | 11.00       | 0.23        | 0.92  |       |
| 14293735–5221012 | 317.768     | 7.670       | 0.533      | 1            | –          | –           | –           | –          | –           | –             | D2          | c                      | o            | –           | –            | –            | –            | –     | 10.974                             | 0.36                        | 1.29                        | 1                    | 34.8                               | 0.86                                 | 3.90                          | 10.775                        | 0.27        | 1.02        | 0.17 | 36.1        | 10.79       | 0.28        | 1.06  |       |
| 14294859–6447544 | 313.163     | –3.899      | 0.609      | 3            | –          | –           | –           | –          | –           | –             | D2          | –                      | –            | –           | –            | –            | –            | –     | 11.465                             | 0.62                        | –                           | 1                    | 40.0                               | 1.00                                 | 4.29                          | 11.238                        | 0.52        | –           | 0.19 | 42.0        | 11.24       | 0.53        | –     |       |
| 14295032–6451414 | 313.142     | –3.959      | 0.577      | 2            | –          | –           | –           | –          | –           | –             | –           | –                      | –            | –           | –            | –            | –            | –     | 11.316                             | 0.40                        | 1.19                        | 1                    | 27.0                               | 0.78                                 | 4.29                          | 11.101                        | 0.31        | 0.90        | 0.18 | 28.1        | 11.11       | 0.32        | 0.94  |       |
| 14304210–5228415 | 317.873     | 7.490       | 0.565      | 1            | –          | –           | –           | –          | –           | –             | D3          | c                      | o            | –           | –            | –            | –            | –     | 11.385                             | 0.32                        | 1.14                        | 1                    | 28.0                               | 0.88                                 | 3.88                          | 11.174                        | 0.22        | 0.85        | 0.18 | 29.1        | 11.19       | 0.23        | 0.89  |       |
| 14315026–5256068 | 317.859     | 7.002       | 0.796      | 1            | –          | –           | –           | –          | –           | –             | D2          | c                      | o            | –           | –            | –            | –            | –     | 10.595                             | 0.45                        | 1.39                        | 1                    | 53.8                               | 0.92                                 | 3.97                          | 10.298                        | 0.32        | 1.00        | 0.25 | 57.1        | 10.31       | 0.34        | 1.05  |       |
| 14315310–5443499 | 317.180     | 5.339       | 0.730      | 1            | –          | –           | –           | –          | –           | –             | D2          | cn                     | o            | –           | –            | –            | –            | –     | 11.472                             | 0.46                        | 1.50                        | 1                    | 32.8                               | 0.66                                 | 4.11                          | 11.200                        | 0.34        | 1.14        | 0.23 | 34.7        | 11.21       | 0.36        | 1.19  |       |
| 14315891–5528000 | 316.912     | 4.652       | 0.861      | 1            | –          | –           | –           | –          | –           |               |             |                        |              |             |              |              |              |       |                                    |                             |                             |                      |                                    |                                      |                               |                               |             |             |      |             |             |             |       |       |

Table B1: a) continued.

| 2MASX J          | <i>l</i> | <i>b</i> | EBV    | Object | Sample | Disc | 2MRS | Velocity | NIR  | Photom | Ext  | <i>K</i> <sub>20</sub> | <i>H-K</i> | <i>J-K</i> | vc   | <i>a</i> | <i>b/a</i> | st.d. | <i>K</i> <sub>s</sub> <sup>o</sup> | ( <i>H-K</i> ) <sup>o</sup> | ( <i>J-K</i> ) <sup>o</sup> | <i>A</i> <sub>K</sub> | <i>a</i> <sub>d</sub> <sup>o</sup> | <i>K</i> <sub>s</sub> <sup>o,d</sup> | ( <i>H-K</i> ) <sup>o,c</sup> | ( <i>J-K</i> ) <sup>o,c</sup> |       |       |      |       |       |       |      |
|------------------|----------|----------|--------|--------|--------|------|------|----------|------|--------|------|------------------------|------------|------------|------|----------|------------|-------|------------------------------------|-----------------------------|-----------------------------|-----------------------|------------------------------------|--------------------------------------|-------------------------------|-------------------------------|-------|-------|------|-------|-------|-------|------|
| (1)              | deg      | deg      | mag    | class  | off    | flag | gal  | TF       | obs  | ext'd  | type | (9)                    | Opt        | HI         | vc   | (18)     | (19)       | (20)  | mag                                | mag                         | mag                         | mag                   | (25)                               | mag                                  | mag                           | mag                           |       |       |      |       |       |       |      |
| (1)              | (2a)     | (2b)     | (3)    | (4)    | (5)    | (6)  | (7a) | (7b)     | (7c) | (7d)   | (8)  | (9)                    | (10a)      | (10b)      | (17) | (18)     | (19)       | (20)  | (21)                               | (22)                        | (23)                        | (24)                  | (25)                               | (26)                                 | (27)                          | (28)                          |       |       |      |       |       |       |      |
| 14513316–5540388 | 319.350  | 3.318    | 1.131  | 1      | –      | –    | g    | t        | –    | –      | D2   | –                      | o          | –          | –    | –        | –          | –     | 9.828                              | 0.34                        | 1.34                        | 1                     | 55.2                               | 0.50                                 | 4.37                          | 9.407                         | 0.16  | 0.78  | 0.35 | 60.0  | 9.44  | 0.18  | 0.85 |
| 14523435–5501089 | 319.775  | 3.842    | 0.943  | 2      | –      | –    | g    | –        | –    | –      | D2   | –                      | –          | h          | –    | –        | –          | –     | 11.435                             | 0.41                        | 1.30                        | 1                     | 31.4                               | 0.88                                 | 4.32                          | 11.084                        | 0.25  | 0.83  | 0.29 | 34.2  | 11.08 | 0.27  | 0.89 |
| 14531172–5254404 | 320.812  | 5.681    | 0.653  | 1      | –      | –    | g    | –        | –    | –      | D2   | c                      | o          | –          | –    | –        | –          | –     | 10.786                             | 0.36                        | 1.22                        | 1                     | 36.4                               | 0.80                                 | 4.09                          | 10.543                        | 0.25  | 0.90  | 0.20 | 38.1  | 10.56 | 0.27  | 0.94 |
| 14533680–5630468 | 319.231  | 2.442    | 1.505  | 1      | –      | –    | g    | t        | P    | –      | D3   | –                      | –          | –          | –    | –        | –          | –     | 10.273                             | 0.54                        | 1.66                        | 1                     | 52.2                               | 0.60                                 | 4.50                          | 9.712                         | 0.29  | 0.91  | 0.47 | 59.2  | 9.74  | 0.32  | 1.01 |
| 14535709–7015561 | 312.987  | –9.824   | 0.180  | 1      | –      | –    | g    | –        | –    | –      | D2   | c                      | o          | –          | –    | –        | –          | –     | 10.878                             | 0.31                        | 1.07                        | 1                     | 35.6                               | 0.80                                 | 3.78                          | 10.811                        | 0.28  | 0.98  | 0.06 | 35.9  | 10.82 | 0.28  | 0.99 |
| 14551586–5213460 | 321.407  | 6.144    | 0.621  | 1      | –      | –    | g    | –        | P    | –      | D2   | –                      | –          | *          | –    | –        | –          | –     | 11.373                             | ...                         | 1.37                        | 1                     | 30.4                               | 1.00                                 | 4.04                          | 11.142                        | ...   | 1.06  | 0.19 | 31.8  | 11.15 | ...   | 1.10 |
| 14551742–5134150 | 321.715  | 6.727    | 0.669  | 1      | –      | –    | g    | –        | –    | –      | D1   | c                      | o          | –          | –    | –        | –          | –     | 10.484                             | 0.43                        | 1.29                        | 1                     | 41.6                               | 0.80                                 | 3.98                          | 10.235                        | 0.32  | 0.95  | 0.21 | 43.5  | 10.25 | 0.34  | 1.00 |
| 14553197–5446291 | 320.267  | 3.866    | 1.009  | 2      | –      | –    | g    | –        | P    | –      | D2   | –                      | –          | –          | –    | –        | –          | –     | 11.467                             | 0.40                        | 1.41                        | 1                     | 26.6                               | 0.58                                 | 4.30                          | 11.091                        | 0.24  | 0.91  | 0.31 | 28.9  | 11.10 | 0.26  | 0.97 |
| 14553218–5209040 | 321.480  | 6.194    | 0.638  | 1      | –      | –    | g    | t        | –    | –      | D1   | cn                     | –          | h          | –    | –        | –          | –     | 11.353                             | 0.38                        | 1.27                        | 1                     | 39.8                               | 0.42                                 | 4.06                          | 11.115                        | 0.28  | 0.96  | 0.20 | 41.8  | 11.12 | 0.29  | 1.00 |
| 14555389–5200450 | 321.594  | 6.292    | 0.617  | 1      | –      | –    | g    | –        | –    | –      | D3   | c                      | o          | –          | –    | –        | –          | –     | 10.300                             | 0.32                        | 1.24                        | 1                     | 43.4                               | 0.90                                 | 4.06                          | 10.070                        | 0.21  | 0.93  | 0.19 | 45.2  | 10.09 | 0.23  | 0.97 |
| 14555704–5106480 | 322.021  | 7.085    | 0.658  | 1      | –      | –    | g    | –        | –    | –      | D2   | c                      | o          | –          | –    | –        | –          | –     | 11.114                             | 0.33                        | 1.22                        | 1                     | 29.6                               | 0.70                                 | 3.96                          | 10.869                        | 0.23  | 0.89  | 0.20 | 31.0  | 10.88 | 0.24  | 0.93 |
| 14561716–5201347 | 321.641  | 6.252    | 0.610  | 1      | –      | –    | g    | –        | –    | –      | D4   | c                      | o          | –          | –    | –        | –          | –     | 10.345                             | 0.34                        | 1.18                        | 1                     | 42.2                               | 0.80                                 | 4.07                          | 10.218                        | 0.23  | 0.88  | 0.19 | 43.9  | 10.14 | 0.25  | 0.92 |
| 14571003–5423318 | 320.654  | 4.095    | 0.848  | 1      | –      | –    | g    | –        | –    | –      | D1   | e                      | o          | h          | –    | –        | –          | –     | 8.532                              | 0.37                        | 1.33                        | 1                     | 111.8                              | 0.48                                 | 4.25                          | 8.116                         | 0.23  | 0.90  | 0.26 | 117.8 | 8.25  | 0.24  | 0.96 |
| 14573760–5212141 | 321.741  | 5.999    | 0.599  | 1      | –      | –    | g    | –        | –    | –      | D1   | c                      | o          | –          | –    | –        | –          | –     | 10.951                             | 0.40                        | 1.31                        | 1                     | 46.6                               | 0.36                                 | 4.10                          | 10.728                        | 0.30  | 1.01  | 0.19 | 48.6  | 10.74 | 0.31  | 1.05 |
| 14574749–6437005 | 315.958  | –4.990   | 0.768  | 1      | –      | –    | g    | –        | P    | –      | D1   | c                      | o          | –          | –    | –        | –          | –     | 11.287                             | ...                         | 1.41                        | 1                     | 44.6                               | 1.00                                 | 4.20                          | 11.001                        | ...   | 1.03  | 0.24 | 47.4  | 11.01 | ...   | 1.08 |
| 14574927–5158162 | 321.877  | 6.190    | 0.599  | 1      | –      | –    | g    | t        | –    | –      | D1   | c                      | o          | h          | –    | –        | –          | –     | 9.555                              | 0.46                        | 1.35                        | 1                     | 97.2                               | 0.40                                 | 4.08                          | 9.332                         | 0.36  | 1.06  | 0.19 | 101.1 | 9.35  | 0.37  | 1.10 |
| 14575314–5551067 | 320.064  | 2.756    | 1.524  | 3      | –      | –    | g    | –        | P    | –      | D2   | –                      | –          | –          | –    | –        | –          | –     | 11.701                             | ...                         | ...                         | 1                     | 17.6                               | 0.90                                 | 4.45                          | 11.133                        | ...   | ...   | 0.47 | 20.2  | 11.14 | ...   | ...  |
| 14581431–5511360 | 320.416  | 3.315    | 0.887  | 1      | –      | –    | g    | –        | –    | –      | D1   | –                      | –          | h          | –    | –        | –          | –     | 10.790                             | 0.43                        | ...                         | 1                     | 46.0                               | 0.66                                 | 4.39                          | 10.460                        | 0.28  | ...   | 0.27 | 50.2  | 10.44 | 0.30  | ...  |
| 14583037–7471561 | 324.013  | 9.904    | 0.306  | 1      | –      | –    | g    | –        | –    | –      | D1   | c                      | o          | –          | –    | –        | –          | –     | 10.233                             | 0.19                        | 0.91                        | 1                     | 82.0                               | 0.82                                 | 3.78                          | 10.119                        | 0.14  | 0.76  | 0.09 | 84.0  | 10.11 | 0.14  | 0.78 |
| 14583208–5157150 | 321.983  | 6.154    | 0.606  | 1      | –      | –    | g    | –        | –    | –      | D3   | c                      | o          | –          | –    | –        | –          | –     | 11.295                             | 0.38                        | 1.31                        | 1                     | 41.6                               | 0.38                                 | 4.12                          | 11.069                        | 0.28  | 1.01  | 0.19 | 43.6  | 11.07 | 0.29  | 1.05 |
| 14583230–6628452 | 315.147  | –6.670   | 0.367  | 1      | –      | –    | g    | –        | –    | –      | D1   | c                      | o          | –          | –    | –        | –          | –     | 10.803                             | 0.40                        | 1.16                        | 1                     | 40.4                               | 0.90                                 | 4.02                          | 10.666                        | 0.33  | 0.98  | 0.11 | 41.3  | 10.68 | 0.34  | 1.00 |
| 14592915–5820102 | 319.089  | 0.460    | 7.368  | 7      | –      | –    | g    | –        | –    | –      | –    | –                      | –          | –          | –    | –        | –          | –     | 9.559                              | ...                         | ...                         | 1                     | 61.8                               | 0.58                                 | 4.76                          | 6.814                         | ...   | ...   | 2.28 | ...   | ...   | ...   |      |
| 14593166–5749002 | 319.339  | 0.916    | 4.384  | 9      | –      | –    | g    | –        | –    | –      | –    | –                      | –          | –          | –    | –        | –          | –     | 10.250                             | ...                         | ...                         | 1                     | 43.0                               | 0.24                                 | 4.59                          | 8.617                         | ...   | ...   | 1.36 | ...   | ...   | ...   |      |
| 14593308–5154213 | 322.144  | 6.122    | 0.584  | 2      | –      | –    | g    | –        | –    | –      | D4   | cn                     | –          | –          | –    | –        | –          | –     | 11.329                             | 0.38                        | 1.29                        | 1                     | 37.2                               | 0.78                                 | 4.10                          | 11.111                        | 0.29  | 1.00  | 0.18 | 38.8  | 11.12 | 0.30  | 1.04 |
| 14593546–6407233 | 316.364  | –4.646   | 0.840  | 1      | –      | –    | g    | –        | P    | –      | n    | –                      | –          | –          | –    | –        | –          | –     | 10.873                             | 0.36                        | 1.32                        | 1                     | 28.0                               | 0.92                                 | 4.21                          | 10.560                        | 0.22  | 0.90  | 0.26 | 29.8  | 10.58 | 0.24  | 0.96 |
| 14594019–5543272 | 320.345  | 2.751    | 1.537  | 2      | –      | –    | g    | t        | P    | –      | D2   | –                      | –          | –          | –    | –        | –          | –     | 11.095                             | 0.33                        | ...                         | 1                     | 36.8                               | 0.66                                 | 4.46                          | 10.522                        | 0.07  | ...   | 0.48 | 43.1  | 10.50 | 0.10  | ...  |
| 15002253–5211571 | 322.116  | 5.804    | 0.795  | 1      | –      | –    | g    | –        | –    | –      | D2   | c                      | o          | –          | –    | –        | –          | –     | 11.045                             | 0.35                        | 1.35                        | 1                     | 32.2                               | 0.62                                 | 4.06                          | 10.749                        | 0.22  | 0.96  | 0.25 | 34.1  | 10.77 | 0.23  | 1.01 |
| 15002412–5924522 | 318.683  | –0.545   | 7.266  | 8      | –      | –    | g    | –        | –    | –      | –    | –                      | –          | –          | –    | –        | –          | –     | 10.667                             | 0.74                        | ...                         | –2                    | 15.8                               | 0.90                                 | 4.71                          | 7.960                         | –0.46 | ...   | 2.25 | ...   | ...   | –0.32 |      |
| 15003503–5858101 | 318.915  | –0.165   | 19.683 | 9      | –      | –    | g    | –        | –    | –      | –    | –                      | –          | –          | –    | –        | –          | –     | 10.525                             | ...                         | ...                         | 1                     | 28.6                               | 0.62                                 | 4.69                          | 3.191                         | ...   | ...   | 6.10 | ...   | ...   | ...   |      |
| 15004300–4802523 | 324.173  | 9.420    | 0.249  | 1      | –      | –    | g    | –        | –    | –      | D1   | c                      | o          | –          | –    | –        | –          | –     | 11.153                             | 0.40                        | 1.22                        | 1                     | 40.0                               | 0.50                                 | 3.84                          | 11.060                        | 0.36  | 1.10  | 0.08 | 40.5  | 11.07 | 0.36  | 1.11 |
| 15004836–5144203 | 322.396  | 6.176    | 0.585  | 1      | –      | –    | g    | –        | –    | –      | D2   | c                      | o          | –          | –    | –        | –          | –     | 11.098                             | 0.23                        | 1.13                        | 1                     | 40.0                               | 0.28                                 | 4.04                          | 10.880                        | 0.13  | 0.84  | 0.18 | 41.7  | 10.89 | 0.15  | 0.88 |
| 15005020–5134043 | 322.482  | 6.324    | 0.581  | 1      | –      | –    | g    | –        | –    | –      | D3   | c                      | o          | –          | –    | –        | –          | –     | 9.985                              | 0.39                        | 1.25                        | 1                     | 66.2                               | 0.80                                 | 4.06                          | 9.769                         | 0.29  | 0.96  | 0.18 | 68.8  | 9.78  | 0.30  | 1.00 |
| 15005787–5114123 | 322.660  | 6.605    | 0.528  | 1      | –      | –    | g    | –        | –    | –      | D2   | c                      | o          | –          | –    | –        | –          | –     | 11.195                             | 0.39                        | 1.18                        | 1                     | 33.8                               | 0.58                                 | 4.05                          | 10.998                        | 0.31  | 0.92  | 0.16 | 35.0  | 11.01 | 0.32  | 0.96 |
| 15010019–6413090 | 316.454  | –4.804   | 0.860  | 1      | –      | –    | g    | –        | P    | –      | D3   | –                      | –          | –          | –    | –        | –          | –     | 11.396                             | 0.37                        | 1.40                        | 1                     | 23.6                               | 0.90                                 | 4.22                          | 11.076                        | 0.23  | 0.97  | 0.27 | 25.3  | 11.09 | 0.25  | 1.03 |
| 15011381–4759122 | 324.280  | 9.432    | 0.243  | 1      | –      | –    | g    | –        | –    | –      | D2   | c                      | o          | –          | –    | –        | –          | –     | 11.163                             | 0.33                        | 1.15                        | 1                     | 26.4                               | 0.78                                 | 3.85                          | 11.072                        | 0.29  | 1.03  | 0.08 | 26.7  | 11.08 | 0.30  | 1.05 |
| 15015394–6425283 | 316.440  | –5.030   | 0.924  | 2      | –      | –    | g    | –        | –    | –      | n    | –                      | –          | –          | –    | –        | –          | –     | 10.759                             | 0.36                        | 1.15                        | 1                     | 69.4                               | 0.54                                 | 4.21                          | 10.415                        | 0.21  | 0.69  | 0.29 | 75.0  | 10.42 | 0.23  | 0.75 |
| 15020535–5122531 | 322.745  | 6.394    | 0.586  | 1      | –      | –    | g    | –        | –    | –      | D3   | c                      | o          | –          | –    | –        | –          | –     | 11.007                             | 0.28                        | 1.22                        | 1                     | 36.0                               | 0.86                                 | 4.05                          | 10.789                        | 0.18  | 0.92  | 0.18 | 37.5  | 10.80 | 0.19  | 0.96 |
| 15031365–5904294 | 319.163  | –0.421   | 27.730 | 8      | –      | –    | g    | –        | –    | –      | –    | –                      | –          | –          | –    | –        | –          | –     | 9.687                              | ...                         | ...                         | 1                     | 31.8                               | 0.68                                 | 4.81                          | –0.645                        | ...   | ...   | 8.59 | ...   | ...   | ...   |      |
| 15034121–5835075 | 319.452  | –0.021   | 24.232 | 9      | –      | –    | g    | –        | –    | –      | –    | –                      | –          | –          | –    | –        | –          | –     | 8.716                              | ...                         | ...                         | –2                    | 95.4                               | 0.18                                 | 4.79                          | –0.313                        | ...   | ...   | 7.51 | ...   | ...   | ...   |      |
| 15034869–5309147 | 322.112  | 4.716    | 0.699  | 1      | –      | –    | g    | t        | –    | –      | D1   | e                      | o          | h          | –    | –        | –          | –     | 9.965                              | 0.36                        | 1.24                        | 1                     | 95.6                               | 0.24                                 | 4.18                          | 9.705                         | 0.24  | 0.89  | 0.22 | 100.4 | 9.72  | 0.26  | 0.94 |
| 15044535–5449534 | 321.411  | 3.185    | 1.231  | 2      | –      | –    | g    | –        | P    | –      | D2   | –                      | –          | –          | –    | –        | –          | –     | 11.159                             | 0.31                        | ...                         | 1                     | 31.8                               | 0.62                                 | 4.41                          | 10.700                        | 0.11  | ...   | 0.38 | 36.0  | 10.68 | 0.13  | ...  |
| 15051680–5731176 | 320.156  | 0.804    | 29.399 | 9      | –      | –    | g    | –        | –    | –      | –    | –                      | –          | –          | –    | –        | –          | –     | 6.579                              | 1.10                        | 2.09                        | 1                     | 183.2                              | 0.66                                 | 4.69                          | –4.375                        | –3.77 | –12.5 |      |       |       |       |      |

Table B1: a) continued.

| 2MASX J          | <i>l</i>    | <i>b</i>    | EBV        | Object       |            | Sample      | Disc        | 2MRS       | Velocity    | NIR           | Photom      | Ext | <i>K</i> <sub>20</sub> | <i>H-K</i>  | <i>J-K</i>   | vc           | <i>a</i>     | <i>b/a</i> | st.d.       | <i>K</i> <sub>s</sub> <sup>o</sup> | ( <i>H-K</i> ) <sup>o</sup> | ( <i>J-K</i> ) <sup>o</sup> | <i>A<sub>K</sub></i> | <i>a</i> <sup>d</sup> | <i>K</i> <sub>s</sub> <sup>o,d</sup> | ( <i>H-K</i> ) <sup>o,c</sup> | ( <i>J-K</i> ) <sup>o,c</sup> |             |       |             |             |             |      |
|------------------|-------------|-------------|------------|--------------|------------|-------------|-------------|------------|-------------|---------------|-------------|-----|------------------------|-------------|--------------|--------------|--------------|------------|-------------|------------------------------------|-----------------------------|-----------------------------|----------------------|-----------------------|--------------------------------------|-------------------------------|-------------------------------|-------------|-------|-------------|-------------|-------------|------|
| (1)              | deg<br>(2a) | deg<br>(2b) | mag<br>(3) | class<br>(4) | off<br>(5) | flag<br>(6) | gal<br>(7a) | TF<br>(7b) | obs<br>(7c) | ext'd<br>(7d) | type<br>(8) | (9) | Opt<br>(10a)           | HI<br>(10b) | flag<br>(11) | flag<br>(12) | flag<br>(13) | (14)       | mag<br>(15) | mag<br>(16)                        | (17)                        | (18)                        | (19)                 | (20)                  | mag<br>(21)                          | mag<br>(22)                   | mag<br>(23)                   | mag<br>(24) | (25)  | mag<br>(26) | mag<br>(27) | mag<br>(28) |      |
| 15273504–6410154 | 318.957     | –6.272      | 0.293      | 1            | –          | –           | g           | –          | –           | –             | D1          | c   | o                      | h           | –            | –            | –            | –          | 8.684       | 0.28                               | 1.03                        | 1                           | 136.0                | 0.64                  | ...                                  | 8.575                         | 0.23                          | 0.89        | 0.09  | ...         | ...         | 0.23        | 0.91 |
| 15280035–5040163 | 326.604     | 4.862       | 0.511      | 9            | –          | –           | –           | –          | –           | –             | –           | –   | g                      | –           | –            | –            | –            | –          | 7.090       | 0.24                               | 0.84                        | 1                           | 46.6                 | 0.11                  | 4.46                                 | 6.900                         | 0.16                          | 0.58        | 0.16  | ...         | ...         | 0.17        | 0.61 |
| 15280246–5039453 | 326.614     | 4.866       | 0.510      | 9            | –          | –           | –           | –          | –           | –             | –           | –   | –                      | –           | –            | –            | –            | –          | 6.379       | 0.17                               | 0.69                        | 1                           | 138.4                | 0.66                  | 4.46                                 | 6.189                         | 0.08                          | 0.43        | 0.16  | ...         | ...         | 0.09        | 0.47 |
| 15280329–5040333 | 326.608     | 4.854       | 0.515      | 9            | –          | –           | –           | –          | –           | –             | –           | –   | –                      | –           | –            | –            | –            | –          | 5.452       | 0.18                               | 0.68                        | 1                           | 232.6                | 0.62                  | 4.46                                 | 5.260                         | 0.10                          | 0.42        | 0.16  | ...         | ...         | 0.11        | 0.46 |
| 15281022–4646448 | 328.843     | 8.056       | 0.397      | 1            | –          | –           | –           | –          | –           | –             | D3          | c   | o                      | –           | –            | V            | –            | –          | 10.132      | 0.35                               | 1.13                        | 1                           | 53.0                 | 0.90                  | 3.94                                 | 9.984                         | 0.29                          | 0.93        | 0.12  | 54.2        | 10.00       | 0.29        | 0.96 |
| 15281344–6752201 | 316.893     | –9.358      | 0.131      | 1            | –          | –           | –           | –          | –           | –             | D1          | c   | o                      | –           | –            | –            | –            | –          | 10.475      | 0.28                               | 1.02                        | 1                           | 60.4                 | 0.54                  | 3.84                                 | 10.426                        | 0.26                          | 0.95        | 0.04  | 60.7        | 10.43       | 0.26        | 0.96 |
| 15303848–4737494 | 328.700     | 7.117       | 0.428      | 1            | –          | –           | –           | –          | –           | –             | D1          | c   | o                      | –           | –            | V            | –            | –          | 10.972      | 0.37                               | 1.21                        | 1                           | 31.2                 | 0.50                  | 4.06                                 | 10.813                        | 0.30                          | 1.00        | 0.13  | 31.9        | 10.83       | 0.31        | 1.03 |
| 15303997–4438044 | 330.448     | 9.564       | 0.275      | 2            | –          | –           | –           | –          | –           | –             | D2          | cp  | –                      | –           | –            | –            | p            | –          | 9.372       | 0.15                               | 0.75                        | –2                          | 40.8                 | 0.50                  | 3.83                                 | 9.270                         | 0.11                          | 0.62        | 0.09  | 41.5        | 9.27        | 0.11        | 0.63 |
| 15311475–4635264 | 329.389     | 7.908       | 0.341      | 1            | –          | –           | –           | –          | –           | –             | D1          | c   | o                      | –           | –            | V            | –            | –          | 11.221      | 0.36                               | 1.06                        | 1                           | 30.0                 | 0.80                  | 3.96                                 | 11.094                        | 0.31                          | 0.89        | 0.11  | 30.6        | 11.10       | 0.31        | 0.91 |
| 15312308–4641444 | 329.347     | 7.809       | 0.319      | 1            | –          | –           | –           | –          | –           | –             | D3          | c   | o                      | –           | –            | V            | –            | –          | 11.261      | 0.41                               | 1.24                        | 1                           | 27.0                 | 0.84                  | 3.98                                 | 11.142                        | 0.36                          | 1.09        | 0.10  | 27.5        | 11.15       | 0.37        | 1.11 |
| 15315422–4957230 | 327.527     | 5.095       | 0.559      | 2            | –          | –           | –           | –          | –           | –             | D1          | c   | o                      | –           | –            | V            | –            | –          | 11.450      | 0.35                               | 1.26                        | 1                           | 24.0                 | 0.74                  | 4.21                                 | 11.242                        | 0.26                          | 0.98        | 0.17  | 24.9        | 11.25       | 0.27        | 1.02 |
| 15323066–4657343 | 329.352     | 7.482       | 0.400      | 1            | –          | –           | –           | –          | –           | –             | D3          | c   | o                      | –           | –            | V            | –            | –          | 11.242      | 0.30                               | 1.04                        | 1                           | 27.2                 | 0.78                  | 4.00                                 | 10.993                        | 0.23                          | 0.85        | 0.12  | 27.9        | 11.10       | 0.24        | 0.87 |
| 15325252–4650139 | 329.474     | 7.546       | 0.396      | 1            | –          | –           | –           | –          | –           | –             | D3          | c   | o                      | –           | –            | V            | –            | –          | 11.067      | 0.30                               | 1.11                        | 1                           | 31.0                 | 0.80                  | 3.95                                 | 10.919                        | 0.23                          | 0.92        | 0.12  | 31.7        | 10.93       | 0.24        | 0.94 |
| 15325265–5556106 | 324.199     | 0.121       | 39.439     | 9            | –          | –           | –           | –          | –           | –             | –           | –   | –                      | –           | –            | –            | –            | –          | 8.316       | ...                                | ...                         | 1                           | 145.0                | 0.34                  | 4.78                                 | –6.379                        | ...                           | ...         | 12.22 | ...         | ...         | ...         |      |
| 15331139–4703438 | 329.386     | 7.332       | 0.407      | 1            | –          | –           | –           | –          | –           | –             | D3          | c   | o                      | –           | –            | V            | –            | –          | 11.058      | 0.34                               | 1.20                        | 1                           | 33.6                 | 0.84                  | 3.99                                 | 10.906                        | 0.27                          | 0.99        | 0.13  | 34.4        | 10.92       | 0.28        | 1.02 |
| 15333008–6021434 | 321.709     | –3.540      | 0.827      | 2            | o          | –           | –           | –          | –           | –             | D1          | c   | o                      | –           | –            | –            | o            | –          | 11.254      | 0.29                               | 1.03                        | 1                           | 35.2                 | 0.48                  | 4.45                                 | 10.946                        | 0.16                          | 0.62        | 0.26  | 37.8        | 10.95       | 0.17        | 0.67 |
| 15334921–4701429 | 329.494     | 7.296       | 0.440      | 1            | –          | –           | –           | –          | –           | –             | D1          | c   | o                      | –           | –            | V            | –            | –          | 10.268      | 0.35                               | 1.21                        | 1                           | 57.6                 | 0.76                  | 4.02                                 | 10.104                        | 0.28                          | 0.99        | 0.14  | 59.2        | 10.12       | 0.28        | 1.02 |
| 15335919–4432525 | 330.986     | 9.290       | 0.297      | 1            | –          | –           | –           | –          | –           | –             | D1          | c   | o                      | –           | –            | V            | –            | –          | 11.124      | 0.34                               | 1.16                        | 1                           | 30.8                 | 0.50                  | 3.90                                 | 10.103                        | 0.30                          | 1.01        | 0.09  | 31.3        | 11.02       | 0.30        | 1.03 |
| 15343955–4700447 | 329.621     | 7.226       | 0.471      | 1            | –          | –           | –           | –          | –           | –             | D4          | c   | o                      | –           | –            | V            | –            | –          | 11.358      | 0.38                               | 1.24                        | 1                           | 27.2                 | 0.72                  | 3.98                                 | 11.183                        | 0.30                          | 1.00        | 0.15  | 28.0        | 11.20       | 0.31        | 1.04 |
| 15350250–5156363 | 326.776     | 3.189       | 1.036      | 1            | –          | –           | –           | –          | –           | –             | D3          | c   | o                      | –           | –            | –            | –            | –          | 10.864      | 0.37                               | ...                         | 1                           | 41.4                 | 1.00                  | 4.47                                 | 10.478                        | 0.19                          | ...         | 0.32  | 45.2        | 10.49       | 0.21        | ...  |
| 15351196–4657242 | 329.729     | 7.217       | 0.438      | 1            | –          | –           | –           | –          | –           | –             | D2          | c   | o                      | –           | –            | V            | –            | –          | 10.630      | 0.31                               | 1.16                        | 1                           | 49.4                 | 0.60                  | 4.00                                 | 10.467                        | 0.24                          | 0.94        | 0.14  | 50.7        | 10.48       | 0.25        | 0.97 |
| 15352343–5039195 | 327.574     | 4.202       | 0.713      | 9            | –          | –           | –           | –          | –           | –             | –           | –   | –                      | –           | –            | –            | –            | –          | 9.851       | 0.14                               | 0.61                        | 1                           | 85.6                 | 0.88                  | 4.35                                 | 9.585                         | 0.02                          | 0.25        | 0.22  | ...         | ...         | 0.04        | 0.30 |
| 15352479–5040035 | 327.570     | 4.190       | 0.711      | 9            | –          | –           | –           | –          | –           | –             | –           | –   | –                      | –           | –            | –            | –            | –          | 10.315      | 0.12                               | 0.67                        | 1                           | 48.4                 | 0.54                  | 4.35                                 | 10.050                        | 0.00                          | 0.32        | 0.22  | ...         | ...         | 0.01        | 0.37 |
| 15352688–5136475 | 327.020     | 3.420       | 0.993      | 2            | –          | –           | –           | –          | –           | –             | D3          | c   | o                      | –           | –            | –            | –            | –          | 11.469      | 0.45                               | 1.37                        | 1                           | 23.2                 | 0.84                  | 4.41                                 | 11.099                        | 0.29                          | 0.88        | 0.31  | 25.3        | 11.10       | 0.31        | 0.94 |
| 15352973–5039315 | 327.586     | 4.190       | 0.726      | 9            | –          | –           | –           | –          | –           | –             | –           | –   | –                      | –           | –            | –            | –            | –          | 6.673       | 0.15                               | 0.76                        | 1                           | 207.8                | 0.74                  | 4.35                                 | 6.402                         | 0.03                          | 0.40        | 0.22  | ...         | ...         | 0.04        | 0.45 |
| 15360225–5944487 | 322.326     | –3.224      | 0.975      | 2            | o          | –           | –           | –          | –           | –             | D1          | c   | o                      | –           | –            | –            | o            | –          | 9.068       | 0.42                               | 0.61                        | 1                           | 60.2                 | 0.42                  | 4.48                                 | 8.705                         | 0.25                          | 0.13        | 0.30  | 65.7        | 8.70        | 0.27        | 0.19 |
| 15362082–5939014 | 322.414     | –3.169      | 0.899      | 2            | –          | –           | –           | –          | –           | –             | D2          | c   | o                      | –           | –            | –            | –            | –          | 11.020      | 0.37                               | ...                         | 1                           | 46.6                 | 0.28                  | 4.47                                 | 10.685                        | 0.22                          | ...         | 0.28  | 50.1        | 10.70       | 0.24        | ...  |
| 15362626–6651350 | 318.141     | –8.995      | 0.155      | 1            | –          | –           | –           | –          | –           | –             | D1          | c   | o                      | –           | –            | h            | –            | –          | 8.488       | 0.23                               | 0.95                        | 1                           | 135.0                | 0.69                  | ...                                  | 8.430                         | 0.20                          | 0.87        | 0.05  | ...         | ...         | 0.21        | 0.88 |
| 15362964–5149582 | 327.022     | 3.147       | 1.022      | 1            | –          | –           | –           | –          | –           | –             | D2          | c   | o                      | –           | –            | –            | –            | –          | 11.419      | ...                                | ...                         | 1                           | 33.2                 | 0.72                  | 4.45                                 | 11.038                        | ...                           | ...         | 0.32  | 36.4        | 11.03       | ...         | ...  |
| 15363909–6241456 | 320.645     | –5.653      | 0.452      | 1            | –          | –           | –           | –          | –           | –             | D2          | c   | o                      | –           | –            | –            | –            | –          | 10.488      | 0.38                               | 1.12                        | 1                           | 50.2                 | 0.82                  | 4.15                                 | 10.320                        | 0.31                          | 0.90        | 0.14  | 51.6        | 10.33       | 0.32        | 0.93 |
| 15364755–5859334 | 320.645     | –2.670      | 2.227      | 1            | –          | –           | –           | –          | –           | –             | D2          | c   | o                      | –           | –            | –            | –            | –          | 10.725      | 0.55                               | ...                         | 1                           | 28.6                 | 0.56                  | 4.58                                 | 9.895                         | 0.18                          | ...         | 0.69  | 35.5        | 9.91        | 0.23        | ...  |
| 15370333–5500156 | 325.224     | 0.533       | 8.589      | 8            | –          | –           | –           | –          | –           | –             | –           | –   | –                      | –           | –            | –            | –            | –          | 9.114       | ...                                | ...                         | –2                          | 40.4                 | 0.58                  | 4.79                                 | 5.914                         | ...                           | ...         | 2.66  | ...         | ...         | ...         |      |
| 15371385–6316563 | 320.350     | –6.164      | 0.315      | 2            | –          | –           | –           | –          | –           | –             | D1          | c   | o                      | –           | –            | –            | –            | –          | 11.300      | 0.37                               | 1.06                        | –2                          | 23.2                 | 0.98                  | 4.14                                 | 11.183                        | 0.32                          | 0.91        | 0.10  | 23.6        | 11.19       | 0.32        | 0.93 |
| 15373137–6018424 | 322.142     | –3.790      | 0.719      | 2            | –          | –           | –           | –          | –           | –             | –           | –   | –                      | –           | –            | –            | –            | –          | 11.422      | 0.41                               | 1.22                        | 1                           | 32.0                 | 0.74                  | 4.42                                 | 11.154                        | 0.29                          | 0.86        | 0.22  | 33.9        | 11.16       | 0.30        | 0.91 |
| 15373472–5534467 | 324.945     | 0.025       | 12.853     | 9            | –          | –           | –           | –          | –           | –             | –           | –   | –                      | –           | –            | –            | –            | –          | 8.865       | 1.42                               | ...                         | –2                          | 24.8                 | 0.30                  | 4.82                                 | 4.076                         | –0.70                         | ...         | 3.98  | ...         | ...         | –0.45       | ...  |
| 15374801–4436465 | 331.501     | 8.835       | 0.319      | 1            | –          | –           | –           | –          | –           | –             | D2          | c   | o                      | –           | –            | V            | –            | –          | 10.318      | 0.27                               | 1.12                        | 1                           | 53.8                 | 0.84                  | 3.92                                 | 10.199                        | 0.22                          | 0.97        | 0.10  | 54.8        | 10.21       | 0.23        | 0.99 |
| 15380529–5947130 | 322.511     | –3.409      | 1.021      | 1            | –          | –           | –           | –          | –           | –             | D1          | c   | o                      | –           | –            | –            | –            | –          | 9.147       | 0.38                               | 1.36                        | 1                           | 70.8                 | 0.66                  | 4.46                                 | 8.767                         | 0.21                          | 0.86        | 0.32  | 75.9        | 8.80        | 0.23        | 0.92 |
| 15381595–4424397 | 331.690     | 8.947       | 0.322      | 1            | o          | –           | –           | –          | –           | –             | D1          | c   | o                      | –           | –            | h            | –            | –          | 11.345      | 0.31                               | 0.95                        | 1                           | 55.8                 | 0.78                  | 3.82                                 | 11.225                        | 0.25                          | 0.79        | 0.10  | 57.3        | 11.22       | 0.26        | 0.81 |
| 15382201–4427568 | 331.672     | 8.893       | 0.305      | 1            | –          | –           | –           | –          | –           | –             | D1          | c   | o                      | –           | –            | V            | –            | –          | 10.675      | 0.37                               | 1.17                        | 1                           | 45.4                 | 0.62                  | 3.82                                 | 10.561                        | 0.32                          | 1.02        | 0.09  | 46.1        | 10.57       | 0.33        | 1.04 |
| 15385974–5950277 | 322.570     | –3.520      | 0.997      | 1            | –          | –           | –           | –          | –           | –             | D3          | c   | o                      | –           | –            | –            | –            | –          | 11.102      | 0.46                               | 1.51                        | 1                           | 28.2                 | 0.64                  | 4.43                                 | 10.731                        | 0.29                          | 1.01        | 0.31  | 30.4        | 10.75       | 0.31        | 1.08 |
| 15385976–4424076 | 331.801     | 8.876       | 0.327      | 1            | –          | –           | –           | –          | –           | –             | D2          | c   | o                      | –           | –            | V            | –            | –          | 10.200      | 0.34                               | 1.12                        | 1                           | 49.4                 | 0.72                  | 3.85                                 | 10.078                        | 0.28                          | 0.95        | 0.10  | 50.2        | 10.09       | 0.29        | 0.98 |
| 15393154–5934382 | 322.782     | –3.348      | 0.977      | 2            | –          | –           | –           | –          | –           | –             | D1          | c   | o                      | –           | –            | h            | –            | –          | 10.668      | 0.41                               | 1.30                        | 1                           | 57.8                 | 0.46                  | 4.49                                 | 10.304                        | 0.25                          | 0.          |       |             |             |             |      |

Table B1: a) continued.

| 2MASX J          | <i>l</i> | <i>b</i> | EBV     | Object | Sample | Disc | 2MRS | Velocity | NIR  | Photom | Ext   | <i>K</i> <sub>20</sub> | <i>H-K</i> | <i>J-K</i> | vc   | <i>a</i> | <i>b/a</i> | st.d. | <i>K</i> <sub>s</sub> <sup>o</sup> | ( <i>H-K</i> ) <sup>o</sup> | ( <i>J-K</i> ) <sup>o</sup> | <i>A</i> <sub>K</sub> | <i>a</i> <sub>d</sub> <sup>o</sup> | <i>K</i> <sub>s</sub> <sup>o,d</sup> | ( <i>H-K</i> ) <sup>o,c</sup> | ( <i>J-K</i> ) <sup>o,c</sup> |     |
|------------------|----------|----------|---------|--------|--------|------|------|----------|------|--------|-------|------------------------|------------|------------|------|----------|------------|-------|------------------------------------|-----------------------------|-----------------------------|-----------------------|------------------------------------|--------------------------------------|-------------------------------|-------------------------------|-----|
| (1)              | deg      | deg      | mag     | class  | off    | flg  | gal  | TF       | (7b) | (7c)   | ext'd | type                   | (8)        | (9)        | Opt  | HI       | (10b)      | flg   | flg                                | flg                         | flg                         | mag                   | mag                                | mag                                  | mag                           | mag                           | mag |
| (1)              | (2a)     | (2b)     | (3)     | (4)    | (5)    | (6)  | (7a) | (7b)     | (7c) | (7d)   | (8)   | (9)                    | (10a)      | (10b)      | (17) | (18)     | (19)       | (20)  | (21)                               | (22)                        | (23)                        | (24)                  | (25)                               | (26)                                 | (27)                          | (28)                          |     |
| 15485359–4809228 | 330.845  | 4.862    | 1.052   | 1      | –      | –    | g    | t        | P    | –      | –     | D2                     | –          | –          | –    | –        | –          | –     | –                                  | –                           | –                           | –                     | –                                  | –                                    | –                             | –                             |     |
| 15491367–5015556 | 329.568  | 3.181    | 1.490   | 2      | –      | –    | g    | t        | +    | –      | –     | n                      | –          | –          | –    | –        | –          | –     | –                                  | –                           | –                           | –                     | –                                  | –                                    | –                             | –                             |     |
| 15491423–5836352 | 324.363  | –3.344   | 0.673   | 1      | –      | –    | g    | t        | –    | –      | –     | D3                     | e          | o          | –    | –        | –          | –     | –                                  | –                           | –                           | –                     | –                                  | –                                    | –                             | –                             |     |
| 15491623–5425461 | 326.975  | –0.079   | 27.234  | 8      | –      | –    | g    | t        | –    | –      | –     | n                      | –          | –          | –    | –        | –          | –     | –                                  | –                           | –                           | –                     | –                                  | –                                    | –                             | –                             |     |
| 15492477–5836052 | 324.386  | –3.351   | 0.678   | 1      | –      | –    | g    | t        | –    | –      | –     | n                      | e          | o          | –    | –        | –          | –     | –                                  | –                           | –                           | –                     | –                                  | –                                    | –                             | –                             |     |
| 15492921–5839533 | 324.354  | –3.407   | 0.661   | 1      | –      | –    | g    | t        | –    | –      | –     | D2                     | e          | o          | –    | –        | –          | –     | –                                  | –                           | –                           | –                     | –                                  | –                                    | –                             | –                             |     |
| 15494968–5938514 | 323.771  | –4.201   | 0.559   | 1      | –      | –    | g    | t        | –    | –      | –     | D1                     | e          | o          | *    | –        | –          | –     | –                                  | –                           | –                           | –                     | –                                  | –                                    | –                             | –                             |     |
| 15495241–5842564 | 324.361  | –3.478   | 0.632   | 1      | –      | –    | g    | t        | –    | –      | –     | D1                     | e          | o          | –    | –        | –          | –     | –                                  | –                           | –                           | –                     | –                                  | –                                    | –                             | –                             |     |
| 15495333–5900594 | 324.174  | –3.714   | 0.633   | 1      | –      | –    | g    | t        | –    | –      | –     | D3                     | e          | o          | –    | –        | –          | –     | –                                  | –                           | –                           | –                     | –                                  | –                                    | –                             | –                             |     |
| 15500315–5403503 | 327.292  | 0.135    | 14.559  | 9      | –      | –    | g    | t        | –    | –      | –     | D1                     | e          | o          | –    | –        | –          | –     | –                                  | –                           | –                           | –                     | –                                  | –                                    | –                             | –                             |     |
| 15501876–6057431 | 322.990  | –5.262   | 0.465   | 1      | –      | –    | g    | t        | –    | –      | –     | D1                     | c          | o          | –    | –        | –          | –     | –                                  | –                           | –                           | –                     | –                                  | –                                    | –                             | –                             |     |
| 15502283–5822355 | 324.626  | –3.255   | 0.780   | 1      | –      | –    | g    | t        | –    | –      | –     | D1                     | e          | o          | h?   | –        | –          | –     | –                                  | –                           | –                           | –                     | –                                  | –                                    | –                             | –                             |     |
| 15502513–5838386 | 324.461  | –3.467   | 0.619   | 1      | –      | –    | g    | t        | –    | –      | –     | D3                     | e          | o          | –    | –        | –          | –     | –                                  | –                           | –                           | –                     | –                                  | –                                    | –                             | –                             |     |
| 15513886–6046289 | 323.236  | –5.219   | 0.446   | 1      | –      | –    | g    | t        | –    | –      | –     | D1                     | c          | o          | –    | –        | –          | –     | –                                  | –                           | –                           | –                     | –                                  | –                                    | –                             | –                             |     |
| 15513960–6342089 | 321.369  | –7.484   | 0.286   | 1      | –      | –    | g    | t        | –    | –      | –     | D1                     | c          | o          | –    | –        | –          | –     | –                                  | –                           | –                           | –                     | –                                  | –                                    | –                             | –                             |     |
| 15521978–6248365 | 322.000  | –6.844   | 0.273   | 1      | –      | –    | g    | t        | –    | –      | –     | D1                     | c          | o          | h    | –        | –          | –     | –                                  | –                           | –                           | –                     | –                                  | –                                    | –                             | –                             |     |
| 15522989–6038084 | 323.405  | –5.177   | 0.417   | 1      | –      | –    | g    | t        | –    | –      | –     | D1                     | c          | o          | h    | –        | –          | –     | –                                  | –                           | –                           | –                     | –                                  | –                                    | –                             | –                             |     |
| 15523425–5015107 | 329.992  | 2.854    | 1.754   | 2      | –      | –    | g    | t        | –    | –      | –     | D3                     | e          | o          | –    | –        | –          | –     | –                                  | –                           | –                           | –                     | –                                  | –                                    | –                             | –                             |     |
| 15523438–5823397 | 324.838  | –3.450   | 0.739   | 1      | –      | –    | g    | t        | –    | –      | –     | D1                     | e          | o          | h    | –        | –          | –     | –                                  | –                           | –                           | –                     | –                                  | –                                    | –                             | –                             |     |
| 15523567–6534183 | 320.243  | –8.988   | 0.129   | 1      | –      | –    | g    | t        | –    | –      | –     | D3                     | c          | o          | –    | –        | –          | –     | –                                  | –                           | –                           | –                     | –                                  | –                                    | –                             | –                             |     |
| 15523875–4927266 | 330.506  | 3.462    | 1.152   | 2      | –      | –    | g    | t        | –    | –      | –     | D2                     | e          | o          | –    | –        | –          | –     | –                                  | –                           | –                           | –                     | –                                  | –                                    | –                             | –                             |     |
| 15524737–4426593 | 333.723  | 7.312    | 0.411   | 2      | –      | –    | g    | t        | –    | –      | –     | n                      | e          | o          | –    | –        | –          | –     | –                                  | –                           | –                           | –                     | –                                  | –                                    | –                             | –                             |     |
| 15530050–5434515 | 327.302  | –0.538   | 110.698 | 9      | –      | –    | g    | t        | –    | –      | –     | D1                     | e          | o          | –    | –        | –          | –     | –                                  | –                           | –                           | –                     | –                                  | –                                    | –                             | –                             |     |
| 15530199–5435425 | 327.295  | –0.551   | 105.622 | 9      | –      | –    | g    | t        | –    | –      | –     | n                      | e          | o          | –    | –        | –          | –     | –                                  | –                           | –                           | –                     | –                                  | –                                    | –                             | –                             |     |
| 15530579–5435206 | 327.306  | –0.552   | 108.185 | 9      | –      | –    | g    | t        | –    | –      | –     | n                      | e          | o          | –    | –        | –          | –     | –                                  | –                           | –                           | –                     | –                                  | –                                    | –                             | –                             |     |
| 15530848–5916595 | 324.329  | –4.184   | 0.488   | 1      | –      | –    | g    | t        | –    | –      | –     | D2                     | e          | o          | –    | –        | –          | –     | –                                  | –                           | –                           | –                     | –                                  | –                                    | –                             | –                             |     |
| 15531882–6108136 | 323.161  | –5.627   | 0.400   | 1      | –      | –    | g    | t        | –    | –      | –     | D1                     | c          | o          | h    | –        | –          | –     | –                                  | –                           | –                           | –                     | –                                  | –                                    | –                             | –                             |     |
| 15532578–5018180 | 330.065  | 2.727    | 1.617   | 1      | –      | –    | g    | t        | –    | –      | –     | D2                     | e          | o          | –    | –        | –          | –     | –                                  | –                           | –                           | –                     | –                                  | –                                    | –                             | –                             |     |
| 15532684–5001330 | 330.244  | 2.941    | 1.537   | 2      | –      | –    | g    | t        | –    | –      | –     | n                      | e          | o          | –    | –        | –          | –     | –                                  | –                           | –                           | –                     | –                                  | –                                    | –                             | –                             |     |
| 15533351–4210521 | 335.299  | 8.965    | 0.420   | 1      | –      | –    | g    | t        | –    | –      | –     | D1                     | c          | o          | *    | –        | –          | –     | –                                  | –                           | –                           | –                     | –                                  | –                                    | –                             | –                             |     |
| 15533419–4944041 | 330.445  | 3.153    | 1.405   | 2      | –      | –    | g    | t        | –    | –      | –     | D2                     | e          | o          | –    | –        | –          | –     | –                                  | –                           | –                           | –                     | –                                  | –                                    | –                             | –                             |     |
| 15533528–6140584 | 322.837  | –6.068   | 0.337   | 1      | –      | –    | g    | t        | –    | –      | –     | D1                     | c          | o          | h    | –        | –          | –     | –                                  | –                           | –                           | –                     | –                                  | –                                    | –                             | –                             |     |
| 15533781–5841294 | 324.755  | –3.767   | 0.747   | 1      | –      | –    | g    | t        | –    | –      | –     | D1                     | e          | o          | –    | –        | –          | –     | –                                  | –                           | –                           | –                     | –                                  | –                                    | –                             | –                             |     |
| 15534427–5002132 | 330.273  | 2.902    | 1.497   | 1      | –      | –    | g    | t        | –    | –      | –     | D3                     | e          | o          | –    | –        | –          | –     | –                                  | –                           | –                           | –                     | –                                  | –                                    | –                             | –                             |     |
| 15534458–5000182 | 330.294  | 2.927    | 1.505   | 1      | –      | –    | g    | t        | –    | –      | –     | D2                     | e          | o          | –    | –        | –          | –     | –                                  | –                           | –                           | –                     | –                                  | –                                    | –                             | –                             |     |
| 15535656–5015312 | 330.157  | 2.711    | 1.472   | 2      | –      | –    | g    | t        | –    | –      | –     | D2                     | e          | o          | –    | –        | –          | –     | –                                  | –                           | –                           | –                     | –                                  | –                                    | –                             | –                             |     |
| 15540626–5311391 | 328.307  | 0.431    | 60.715  | 9      | –      | –    | g    | t        | –    | –      | –     | n                      | e          | o          | –    | –        | –          | –     | –                                  | –                           | –                           | –                     | –                                  | –                                    | –                             | –                             |     |
| 15540750–5323442 | 328.181  | 0.274    | 25.341  | 9      | –      | –    | g    | t        | –    | –      | –     | n                      | e          | o          | –    | –        | –          | –     | –                                  | –                           | –                           | –                     | –                                  | –                                    | –                             | –                             |     |
| 15542315–6120239 | 323.131  | –5.866   | 0.405   | 1      | –      | –    | g    | t        | –    | –      | –     | D1                     | c          | o          | h    | –        | –          | –     | –                                  | –                           | –                           | –                     | –                                  | –                                    | –                             | –                             |     |
| 15544486–6056065 | 323.425  | –5.583   | 0.485   | 1      | –      | –    | g    | t        | –    | –      | –     | D1                     | c          | o          | h    | –        | –          | –     | –                                  | –                           | –                           | –                     | –                                  | –                                    | –                             | –                             |     |
| 15545900–6224285 | 322.495  | –6.730   | 0.252   | 1      | –      | –    | g    | t        | –    | –      | –     | D2                     | e          | o          | –    | –        | –          | –     | –                                  | –                           | –                           | –                     | –                                  | –                                    | –                             | –                             |     |
| 15550161–6218126 | 322.567  | –6.653   | 0.274   | 1      | –      | –    | g    | t        | –    | –      | –     | D2                     | e          | o          | –    | –        | –          | –     | –                                  | –                           | –                           | –                     | –                                  | –                                    | –                             | –                             |     |
| 15550346–5007406 | 330.379  | 2.697    | 1.481   | 6      | –      | –    | g    | t        | –    | –      | –     | n                      | e          | o          | –    | –        | –          | –     | –                                  | –                           | –                           | –                     | –                                  | –                                    | –                             | –                             |     |
| 15550554–4049191 | 336.411  | 9.817    | 0.373   | 1      | –      | –    | g    | t        | –    | –      | –     | D1                     | c          | o          | –    | –        | –          | –     | –                                  | –                           | –                           | –                     | –                                  | –                                    | –                             | –                             |     |
| 15551868–6122575 | 323.189  | –5.970   | 0.416   | 1      | –      | –    | g    | t        | –    | –      | –     | D1                     | c          | o          | –    | –        | –          | –     | –                                  | –                           | –                           | –                     | –                                  | –                                    | –                             | –                             |     |
| 15552400–5814306 | 325.222  | –3.569   | 0.734   | 1      | –      | –    | g    | t        | –    | –      | –     | D1                     | e          | o          | *    | –        | –          | –     | –                                  | –                           | –                           | –                     | –                                  | –                                    | –                             | –                             |     |
| 15553600–6056279 | 323.501  | –5.654   | 0.499   | 1      | –      | –    | g    | t        | –    | –      | –     | D2                     | c          | o          | –    | –        | –          | –     | –                                  | –                           | –                           | –                     | –                                  | –                                    | –                             | –                             |     |
| 15555386–4701506 | 332.478  | 4.983    | 1.408   | 1      | –      | –    | g    | t        | –    | –      | –     | D2                     | e          | o          | –    | –        | –          | –     | –                                  | –                           | –                           | –                     | –                                  | –                                    | –                             | –                             |     |
| 15560795–5419395 | 327.813  | –0.632   | 19.718  | 7      | –      | –    | g    | t        | –    | –      | –     | n                      | e          | o          | –    | –        | –          | –     | –                                  | –                           | –                           | –                     | –                                  | –                                    | –                             | –                             |     |
| 15563299–6130461 | 323.218  | –6.165   | 0.439   | 1      | –      | –    | g    | t        | –    | –      | –     | D1                     | c          | o          | –    | –        | –          | –     | –                                  | –                           | –                           | –                     | –                                  | –                                    | –                             | –                             |     |
| 15571651–6216243 | 322.787  | –6.799   | 0.516   | 1      | –      | –    | g    | t        | –    | –      | –     | D1                     | c          | o          | –    | –        | –          | –     | –                                  | –                           | –                           | –                     | –                                  | –                                    | –                             | –                             |     |
| 15572693–5857203 | 324.965  | –4.287   | 0.508   | 1      | –      | –    | g    | t        | –    | –      | –     | D3                     | e          | o          | –    | –        | –          | –     | –                                  | –                           | –                           | –                     | –                                  | –                                    | –                             | –                             |     |
| 15573343–5901083 | 324.935  | –4.344   | 0.518   | 1      | –      | –    | g    | t        | –    | –      | –     | D1                     | e          | o          | –    | –        | –          | –     | –                                  | –                           | –                           | –                     | –                                  | –                                    | –                             | –                             |     |
| 15575303–5402134 | 328.196  | –0.575   | 44.101  | 9      | –      | –    | g    | t        | –    | –      | –     | n                      | e          | o          | –    | –        | –          | –     | –                                  | –                           | –                           | –                     | –                                  | –                                    | –                             | –                             |     |
| 15580608–4610134 | 333.326  | 5.394    | 1.355   | 1      | –      | –    | g    | t        | –    | –      | –     | D1                     | e          | o          | –    | –        | –          | –     | –                                  | –                           | –                           | –                     | –                                  | –                                    | –                             | –                             |     |
| 15580927–4322374 | 335.165  | 7.507    | 0.532   | 1      | –      | –    | g    | t        | –    | –      | –     | D1                     | e          | o          | –    | –        | –          | –     | –                                  | –                           | –                           | –                     | –                                  | –                                    | –                             | –                             |     |
| 15581341–6253139 | 322.468  | –7.336   | 0.344   | 1      | –      | –    | g    | t        | –    | –      | –     | D1                     | e          | o          | –    | –        | –          | –     | –                                  | –                           | –                           | –                     | –                                  | –                                    | –                             | –                             |     |
| 15581658–5207370 | 329.477  | 0.843    | 16.321  | 8      | –      | –    | g    | t        | –    | –      | –     | n                      | e          | o          | –    | –        | –          | –     | –                                  | –                           | –                           | –                     | –                                  | –                                    | –                             | –                             |     |
| 15582254–5917484 | 324.834  | –4.624   | 0.469   | 1      | –      | –    | g    | t        | –    | –      | –     | D1                     | e          | o          | –    | –        | –          | –     | –                                  | –                           | –                           | –                     | –                                  | –                                    | –                             | –                             |     |
| 15592196–6001218 | 324.454  | –5.256   | 0.377   | 1      | –      | –    | g    | t        | –    | –      | –     | D1                     | c          | o          | –    |          |            |       |                                    |                             |                             |                       |                                    |                                      |                               |                               |     |

Table B1: a) continued.

| 2MASX J          | <i>l</i>    | <i>b</i>    | EBV        | Object       | Sample     | Disc       | 2MRS        | Velocity   | NIR         | Photom        | Ext         | <i>K</i> <sub>20</sub> | <i>H-K</i>   | <i>J-K</i>  | vc          | <i>a</i>    | <i>b/a</i>  | st.d. | <i>K</i> <sub>s</sub> <sup>o</sup> | <i>(H-K)</i> <sup>o</sup> | <i>(J-K)</i> <sup>o</sup> | <i>A<sub>K</sub></i> | <i>a</i> <sub>d</sub> <sup>o</sup> | <i>K</i> <sub>s</sub> <sup>o,d</sup> | <i>(H-K)</i> <sup>o,c</sup> | <i>(J-K)</i> <sup>o,c</sup> |      |      |       |       |       |      |      |
|------------------|-------------|-------------|------------|--------------|------------|------------|-------------|------------|-------------|---------------|-------------|------------------------|--------------|-------------|-------------|-------------|-------------|-------|------------------------------------|---------------------------|---------------------------|----------------------|------------------------------------|--------------------------------------|-----------------------------|-----------------------------|------|------|-------|-------|-------|------|------|
| (1)              | deg<br>(2a) | deg<br>(2b) | mag<br>(3) | class<br>(4) | off<br>(5) | flg<br>(6) | gal<br>(7a) | TF<br>(7b) | obs<br>(7c) | ext'd<br>(7d) | type<br>(8) | (9)                    | Opt<br>(10a) | HI<br>(10b) | flg<br>(11) | flg<br>(12) | flg<br>(13) | (14)  | mag<br>(21)                        | mag<br>(22)               | mag<br>(23)               | mag<br>(24)          | (25)                               | mag<br>(26)                          | mag<br>(27)                 | mag<br>(28)                 |      |      |       |       |       |      |      |
| 16010518–6106506 | 323.895     | –6.218      | 0.352      | 1            | –          | –          | g           | –          | –           | –             | D3          | c                      | o            | –           | –           | –           | –           | –     | 10.758                             | 0.25                      | 1.06                      | 1                    | 32.6                               | 0.80                                 | 4.15                        | 10.627                      | 0.20 | 0.88 | 0.11  | 33.2  | 10.64 | 0.20 | 0.90 |
| 16010640–4835261 | 332.127     | 3.230       | 1.872      | 2            | –          | –          | g           | t          | P           | –             | D2          | –                      | –            | –           | –           | –           | –           | –     | 11.716                             | 0.46                      | ...                       | 1                    | 31.8                               | 0.48                                 | 4.47                        | 11.018                      | 0.15 | ...  | 0.58  | 39.0  | 10.98 | 0.18 | ...  |
| 16011281–5842435 | 325.495     | –4.420      | 0.566      | 1            | –          | –          | g           | –          | –           | –             | D1          | e                      | o            | –           | –           | –           | –           | –     | 9.594                              | 0.28                      | 1.11                      | 1                    | 60.0                               | 0.72                                 | 4.34                        | 9.383                       | 0.19 | 0.83 | 0.18  | 62.2  | 9.40  | 0.20 | 0.86 |
| 16011315–5234360 | 329.525     | 0.209       | 38.903     | 9            | –          | –          | g           | –          | –           | –             | –           | –                      | –            | –           | –           | –           | –           | –     | 9.111                              | ...                       | ...                       | 1                    | 28.4                               | 0.38                                 | 4.78                        | –5.384                      | ...  | ...  | 12.05 | ...   | ...   | ...  |      |
| 16013110–4916046 | 331.733     | 2.674       | 2.345      | 7            | –          | –          | g           | –          | –           | –             | –           | –                      | –            | –           | –           | –           | –           | –     | 9.608                              | 0.71                      | 2.35                      | 1                    | 44.0                               | 0.64                                 | 4.55                        | 8.734                       | 0.32 | 1.18 | 0.73  | ...   | ...   | 0.36 | 1.34 |
| 16013673–5904444 | 325.291     | –4.731      | 0.369      | 1            | –          | –          | g           | –          | P           | –             | D1          | –                      | –            | –           | –           | –           | –           | –     | 11.076                             | 0.36                      | 1.10                      | 1                    | 38.2                               | 0.72                                 | 4.31                        | 10.939                      | 0.30 | 0.92 | 0.11  | 39.1  | 10.95 | 0.31 | 0.94 |
| 16014957–4428214 | 334.942     | 6.247       | 0.941      | 1            | –          | –          | g           | –          | –           | –             | D1          | e                      | o            | –           | –           | –           | –           | –     | 11.546                             | 0.52                      | 1.48                      | 1                    | 34.8                               | 0.78                                 | 4.11                        | 11.195                      | 0.37 | 1.01 | 0.29  | 38.4  | 11.16 | 0.39 | 1.07 |
| 16015300–5356196 | 328.706     | –0.884      | 7.315      | 7            | –          | –          | g           | –          | –           | –             | –           | –                      | –            | –           | –           | –           | –           | –     | 9.481                              | ...                       | ...                       | 1                    | 41.0                               | 0.82                                 | 4.84                        | 6.755                       | ...  | ...  | 2.27  | ...   | ...   | ...  |      |
| 16015527–4835426 | 332.226     | 3.138       | 1.901      | 3            | –          | –          | g           | –          | P           | –             | D2          | –                      | –            | –           | –           | –           | –           | –     | 11.283                             | 0.49                      | ...                       | 1                    | 34.0                               | 0.84                                 | 4.48                        | 10.575                      | 0.18 | ...  | 0.59  | 41.4  | 10.56 | 0.22 | ...  |
| 16020678–4820457 | 332.414     | 3.304       | 1.691      | 2            | –          | –          | g           | –          | +           | –             | n           | –                      | –            | –           | –           | –           | –           | –     | 11.117                             | 0.39                      | 1.56                      | 1                    | 31.4                               | 0.90                                 | 4.47                        | 10.487                      | 0.11 | 0.72 | 0.52  | 37.1  | 10.48 | 0.14 | 0.84 |
| 16022512–4801267 | 332.665     | 3.513       | 1.619      | 2            | –          | –          | g           | –          | –           | –             | D1          | –                      | –            | –           | –           | –           | –           | –     | 11.417                             | 0.58                      | 1.78                      | 1                    | 28.4                               | 0.78                                 | 4.39                        | 10.814                      | 0.31 | 0.98 | 0.50  | 33.5  | 10.80 | 0.34 | 1.08 |
| 16023547–6146281 | 323.591     | –6.832      | 0.284      | 1            | –          | –          | g           | –          | –           | –             | D1          | c                      | o            | –           | –           | –           | –           | –     | 10.789                             | 0.34                      | 0.99                      | 1                    | 49.2                               | 0.72                                 | 4.09                        | 10.683                      | 0.29 | 0.85 | 0.09  | 50.1  | 10.69 | 0.30 | 0.87 |
| 16030281–6145432 | 323.640     | –6.859      | 0.291      | 1            | –          | –          | g           | –          | –           | –             | D1          | c                      | o            | –           | –           | –           | –           | –     | 10.861                             | 0.33                      | 1.16                      | 1                    | 35.2                               | 0.58                                 | 4.09                        | 10.753                      | 0.28 | 1.02 | 0.09  | 35.7  | 10.76 | 0.29 | 1.04 |
| 16031236–6406551 | 322.070     | –8.625      | 0.192      | 1            | –          | –          | g           | –          | –           | –             | D1          | c                      | o            | –           | –           | –           | –           | –     | 10.829                             | 0.31                      | 1.08                      | –2                   | 60.4                               | 0.92                                 | 3.95                        | 10.757                      | 0.28 | 0.98 | 0.06  | 61.0  | 10.76 | 0.29 | 1.00 |
| 16032935–5939476 | 325.083     | –5.327      | 0.346      | 1            | –          | –          | g           | t          | –           | –             | D1          | c                      | o            | –           | –           | –           | –           | –     | 11.252                             | 0.23                      | 0.97                      | 1                    | 59.4                               | 0.30                                 | 4.27                        | 11.123                      | 0.17 | 0.80 | 0.11  | 60.7  | 11.13 | 0.18 | 0.82 |
| 16032964–4745126 | 332.980     | 3.596       | 1.523      | 2            | –          | –          | g           | t          | P           | –             | D3          | –                      | –            | –           | –           | –           | –           | –     | 11.587                             | 0.52                      | ...                       | 1                    | 27.8                               | 0.64                                 | 4.44                        | 11.020                      | 0.26 | ...  | 0.47  | 32.6  | 10.99 | 0.29 | ...  |
| 16033562–6009011 | 324.768     | –5.699      | 0.338      | 1            | o          | –          | g           | –          | –           | –             | D4          | c                      | o            | –           | –           | –           | –           | –     | 9.313                              | 0.26                      | 1.05                      | 1                    | 75.2                               | 0.70                                 | 4.17                        | 9.187                       | 0.20 | 0.89 | 0.10  | 76.4  | 9.20  | 0.21 | 0.91 |
| 16034282–4814023 | 332.689     | 3.212       | 1.638      | 4            | –          | –          | g           | t          | +           | –             | n           | –                      | –            | –           | –           | –           | –           | –     | 11.740                             | ...                       | ...                       | 1                    | 22.4                               | 0.46                                 | 4.47                        | 11.130                      | ...  | ...  | 0.51  | 26.7  | 11.10 | ...  | ...  |
| 16034796–4737236 | 333.105     | 3.660       | 1.546      | 2            | –          | –          | g           | +          | –           | –             | n           | –                      | –            | –           | –           | –           | –           | –     | 11.320                             | 0.58                      | 1.69                      | 1                    | 23.4                               | 0.82                                 | 4.39                        | 10.744                      | 0.33 | 0.93 | 0.48  | 27.0  | 10.75 | 0.36 | 1.03 |
| 16034826–4738466 | 333.091     | 3.642       | 1.555      | 1            | –          | –          | g           | –          | P           | –             | D2          | –                      | –            | –           | –           | –           | –           | –     | 9.776                              | 0.63                      | 1.70                      | 1                    | 66.8                               | 0.96                                 | 4.39                        | 9.197                       | 0.38 | 0.93 | 0.48  | 76.5  | 9.22  | 0.41 | 1.03 |
| 16034846–5908466 | 325.459     | –4.967      | 0.319      | 1            | –          | –          | g           | –          | –           | –             | D1          | e                      | o            | –           | –           | –           | –           | –     | 11.316                             | 0.27                      | 1.16                      | 1                    | 24.8                               | 0.62                                 | 4.29                        | 11.197                      | 0.22 | 1.00 | 0.10  | 25.2  | 11.21 | 0.22 | 1.02 |
| 16034936–6058402 | 324.235     | –6.336      | 0.320      | 1            | –          | –          | g           | –          | –           | –             | D1          | c                      | o            | –           | –           | –           | –           | –     | 9.406                              | 0.36                      | 1.17                      | 1                    | 124.8                              | 0.22                                 | 4.08                        | 9.287                       | 0.30 | 1.01 | 0.10  | 126.9 | 9.30  | 0.31 | 1.03 |
| 16035124–4842493 | 332.387     | 2.838       | 2.288      | 3            | –          | –          | g           | t          | +           | –             | n           | –                      | –            | –           | –           | –           | –           | –     | 10.924                             | 0.64                      | ...                       | 1                    | 49.2                               | 0.42                                 | 4.49                        | 10.071                      | 0.26 | ...  | 0.71  | 63.3  | 10.04 | 0.30 | ...  |
| 16042503–6044147 | 324.450     | –6.205      | 0.317      | 1            | –          | –          | g           | –          | –           | –             | D1          | c                      | o            | –           | –           | –           | –           | –     | 9.621                              | 0.27                      | 1.08                      | 1                    | 82.6                               | 0.36                                 | 4.15                        | 9.503                       | 0.22 | 0.92 | 0.10  | 83.8  | 9.52  | 0.23 | 0.94 |
| 16042665–6033547 | 324.569     | –6.079      | 0.347      | 1            | –          | –          | g           | –          | –           | –             | D1          | c                      | o            | –           | –           | –           | –           | –     | 10.225                             | 0.28                      | 1.08                      | 1                    | 44.0                               | 0.72                                 | 4.14                        | 10.096                      | 0.22 | 0.91 | 0.11  | 44.7  | 10.11 | 0.23 | 0.93 |
| 16042704–6229477 | 323.268     | –7.515      | 0.241      | 1            | –          | –          | g           | –          | –           | –             | D4          | c                      | o            | –           | –           | –           | –           | –     | 11.095                             | 0.45                      | 1.17                      | 1                    | 36.8                               | 0.88                                 | 4.00                        | 11.005                      | 0.41 | 1.05 | 0.07  | 37.2  | 11.01 | 0.42 | 1.06 |
| 16043756–6046318 | 324.444     | –6.250      | 0.301      | 1            | –          | –          | g           | t          | –           | –             | D1          | c                      | o            | –           | –           | –           | –           | –     | 10.845                             | 0.32                      | 1.16                      | 1                    | 55.6                               | 0.30                                 | 4.15                        | 10.733                      | 0.28 | 1.01 | 0.09  | 56.6  | 10.74 | 0.28 | 1.03 |
| 16044114–4139472 | 337.221     | 7.995       | 0.643      | 1            | –          | –          | g           | –          | –           | –             | D1          | e                      | o            | –           | –           | –           | –           | –     | 10.060                             | 0.31                      | 1.17                      | 1                    | 65.0                               | 0.66                                 | 3.98                        | 9.820                       | 0.20 | 0.85 | 0.20  | 68.2  | 9.83  | 0.22 | 0.89 |
| 16044954–4143012 | 337.204     | 7.937       | 0.645      | 1            | –          | –          | g           | t          | –           | –             | D1          | e                      | o            | –           | –           | –           | –           | –     | 10.300                             | 0.30                      | 1.19                      | 1                    | 85.8                               | 0.48                                 | 3.98                        | 10.060                      | 0.19 | 0.87 | 0.20  | 90.1  | 10.07 | 0.21 | 0.92 |
| 16045039–5958558 | 324.997     | –5.678      | 0.332      | 1            | –          | –          | g           | –          | –           | –             | D1          | c                      | o            | –           | –           | –           | –           | –     | 10.328                             | 0.27                      | 1.04                      | 1                    | 66.8                               | 0.56                                 | 4.17                        | 10.204                      | 0.22 | 0.88 | 0.10  | 68.0  | 10.22 | 0.22 | 0.90 |
| 16054881–6008450 | 324.977     | –5.881      | 0.297      | 1            | –          | –          | g           | t          | –           | –             | D1          | c                      | o            | –           | –           | –           | –           | –     | 10.740                             | 0.21                      | 0.91                      | 1                    | 43.0                               | 0.36                                 | 4.15                        | 10.629                      | 0.16 | 0.76 | 0.09  | 43.7  | 10.64 | 0.16 | 0.78 |
| 16055177–5048136 | 331.238     | 1.062       | 18.027     | 8            | –          | –          | g           | –          | –           | –             | –           | –                      | –            | –           | –           | –           | –           | –     | 8.127                              | ...                       | ...                       | 1                    | 128.8                              | 0.80                                 | 4.73                        | 1.410                       | ...  | ...  | 5.58  | ...   | ...   | ...  |      |
| 16061387–6010169 | 324.999     | –5.934      | 0.292      | 1            | –          | –          | g           | –          | –           | –             | D1          | c                      | o            | –           | –           | –           | –           | –     | 10.311                             | 0.26                      | 1.05                      | 1                    | 41.4                               | 0.54                                 | 4.15                        | 10.202                      | 0.21 | 0.90 | 0.09  | 42.0  | 10.22 | 0.22 | 0.92 |
| 16061400–6111289 | 324.309     | –6.689      | 0.260      | 1            | –          | –          | g           | –          | –           | –             | D2          | –                      | –            | –           | –           | –           | –           | –     | 10.293                             | 0.35                      | 1.11                      | 1                    | 40.4                               | 0.90                                 | 4.12                        | 10.196                      | 0.31 | 0.98 | 0.08  | 40.9  | 10.21 | 0.32 | 1.00 |
| 16062307–5043275 | 331.352     | 1.066       | 29.584     | 9            | –          | –          | g           | –          | –           | –             | –           | –                      | –            | –           | –           | –           | –           | –     | 8.021                              | ...                       | ...                       | 1                    | 220.0                              | 0.46                                 | 4.73                        | –3.002                      | ...  | ...  | 9.16  | ...   | ...   | ...  |      |
| 16062383–6346520 | 322.559     | –8.613      | 0.205      | 1            | –          | –          | g           | t          | –           | –             | D1          | c                      | o            | –           | –           | –           | –           | –     | 11.279                             | 0.32                      | 1.08                      | 1                    | 36.2                               | 0.46                                 | 3.91                        | 11.203                      | 0.28 | 0.97 | 0.06  | 36.6  | 11.21 | 0.29 | 0.99 |
| 16062662–5043302 | 331.359     | 1.059       | 28.005     | 9            | –          | –          | g           | –          | –           | –             | –           | –                      | –            | –           | –           | –           | –           | –     | 7.718                              | ...                       | ...                       | 1                    | 163.0                              | 0.46                                 | 4.75                        | –2.717                      | ...  | ...  | 8.67  | ...   | ...   | ...  |      |
| 16062738–6354130 | 322.480     | –8.708      | 0.188      | 1            | –          | –          | g           | –          | –           | –             | D1          | c                      | o            | –           | –           | –           | –           | –     | 10.502                             | 0.28                      | 1.04                      | 1                    | 43.6                               | 0.44                                 | 3.93                        | 10.432                      | 0.25 | 0.94 | 0.06  | 44.0  | 10.44 | 0.25 | 0.96 |
| 16062746–5733496 | 326.778     | –4.022      | 0.579      | 1            | –          | –          | g           | t          | –           | –             | D1          | c                      | o            | –           | –           | –           | –           | –     | 11.304                             | 0.27                      | 1.31                      | 1                    | 27.0                               | 0.70                                 | 4.38                        | 11.088                      | 0.18 | 1.02 | 0.18  | 28.2  | 11.10 | 0.19 | 1.06 |
| 16063004–4751020 | 333.292     | 3.187       | 1.371      | 2            | –          | –          | g           | t          | P           | –             | D2          | –                      | –            | –           | –           | –           | –           | –     | 11.392                             | ...                       | ...                       | 1                    | 38.4                               | 0.60                                 | 4.48                        | 10.881                      | ...  | ...  | 0.42  | 44.1  | 10.87 | ...  | ...  |
| 16063031–6125160 | 324.177     | –6.881      | 0.255      | 1            | –          | –          | g           | –          | –           | –             | D4          | c                      | o            | –           | –           | –           | –           | –     | 9.945                              | 0.28                      | 1.02                      | 1                    | 49.8                               | 0.82                                 | 4.06                        | 9.850                       | 0.24 | 0.89 | 0.08  | 50.4  | 9.86  | 0.25 | 0.91 |
| 16071460–6044502 | 324.701     | –6.444      | 0.288      | 1            | –          | –          | g           | –          | –           | –             | D1          | c                      | o            | –           | –           | –           | –           | –     | 10.759                             | 0.25                      | 0.95                      | 1                    | 57.0                               | 0.76                                 | 4.11                        | 10.652                      | 0.20 | 0.81 | 0.09  | 57.9  | 10.66 | 0.21 | 0.83 |
| 16071765–6040492 | 324.751     | –6.399      |            |              |            |            |             |            |             |               |             |                        |              |             |             |             |             |       |                                    |                           |                           |                      |                                    |                                      |                             |                             |      |      |       |       |       |      |      |

Table B1: a) continued.

| 2MASX J          | <i>l</i> | <i>b</i> | EBV    | Object | Sample | Disc | 2MRS | Velocity | NIR  | Photom | Ext   | <i>K</i> <sub>20</sub> | <i>H-K</i> | <i>J-K</i> | vc   | <i>a</i> | <i>b/a</i> | st.d. | <i>K</i> <sub>s</sub> <sup>o</sup> | ( <i>H-K</i> ) <sup>o</sup> | ( <i>J-K</i> ) <sup>o</sup> | <i>A<sub>K</sub></i> | <i>a</i> <sub>d</sub> <sup>o</sup> | <i>K</i> <sub>s</sub> <sup>o,d</sup> | ( <i>H-K</i> ) <sup>o,c</sup> | ( <i>J-K</i> ) <sup>o,c</sup> |        |       |        |       |       |       |       |       |     |
|------------------|----------|----------|--------|--------|--------|------|------|----------|------|--------|-------|------------------------|------------|------------|------|----------|------------|-------|------------------------------------|-----------------------------|-----------------------------|----------------------|------------------------------------|--------------------------------------|-------------------------------|-------------------------------|--------|-------|--------|-------|-------|-------|-------|-------|-----|
| (1)              | deg      | deg      | mag    | class  | off    | flag | gal  | TF       | (7b) | (7c)   | ext'd | type                   | (8)        | (9)        | Opt  | HI       | (10b)      | flag  | flag                               | flag                        | mag                         | mag                  | mag                                | mag                                  | mag                           | mag                           | mag    |       |        |       |       |       |       |       |     |
| (1)              | (2a)     | (2b)     | (3)    | (4)    | (5)    | (7a) | (7a) | (7b)     | (7c) | (7d)   | (8)   | (9)                    | (10a)      | (10b)      | (17) | (18)     | (19)       | (20)  | (21)                               | (22)                        | (23)                        | (24)                 | (25)                               | (26)                                 | (27)                          | (28)                          |        |       |        |       |       |       |       |       |     |
| 16122275-4624177 | 335.010  | 3.572    | 1.687  | 1      | -      | -    | g    | -        | P    | -      | -     | D3                     | -          | -          | -    | -        | -          | -     | e?                                 | 10.841                      | 0.55                        | 1.79                 | 1                                  | 37.8                                 | 0.82                          | 4.43                          | 10.212 | 0.27  | 0.95   | 0.52  | 44.6  | 10.21 | 0.30  | 1.06  |     |
| 16122291-5556102 | 328.482  | -3.376   | 0.721  | 1      | -      | -    | g    | -        | P    | -      | -     | D2                     | -          | -          | -    | -        | -          | -     | -                                  | 11.150                      | 0.43                        | ...                  | 1                                  | 29.2                                 | 0.84                          | 4.51                          | 10.881 | 0.31  | ...    | 0.22  | 30.8  | 10.89 | 0.32  | ...   |     |
| 16124178-5914342 | 326.234  | -5.809   | 0.286  | 1      | -      | -    | g    | -        | -    | -      | -     | D4                     | c          | o          | -    | -        | -          | -     | -                                  | 9.320                       | 0.26                        | 1.03                 | 1                                  | 75.6                                 | 0.82                          | 4.17                          | 9.213  | 0.21  | 0.89   | 0.09  | 76.5  | 9.23  | 0.22  | 0.90  |     |
| 16124234-5145015 | 331.386  | -0.359   | 39.097 | 8      | -      | -    | g    | -        | -    | -      | -     | -                      | -          | -          | -    | -        | -          | V     | -                                  | 8.294                       | 1.09                        | ...                  | 1                                  | 105.8                                | 0.68                          | 4.75                          | -6.274 | -5.38 | ...    | 12.11 | ...   | ...   | -4.61 | ...   |     |
| 16125677-6101040 | 325.025  | -7.116   | 0.213  | 1      | -      | -    | g    | -        | t    | -      | -     | D1                     | c          | o          | -    | -        | -          | -     | -                                  | 10.560                      | 0.25                        | 0.91                 | 1                                  | 62.2                                 | 0.68                          | 4.04                          | 10.481 | 0.21  | 0.80   | 0.07  | 62.8  | 10.49 | 0.22  | 0.82  |     |
| 16130681-5955262 | 325.801  | -6.339   | 0.275  | 1      | -      | -    | g    | -        | -    | -      | -     | D2                     | c          | o          | -    | -        | -          | -     | -                                  | 10.756                      | 0.24                        | 0.97                 | 1                                  | 43.0                                 | 0.70                          | 4.13                          | 10.654 | 0.19  | 0.83   | 0.09  | 43.6  | 10.66 | 0.20  | 0.85  |     |
| 16131977-5623491 | 328.261  | -3.802   | 0.556  | 1      | -      | -    | g    | -        | -    | -      | -     | D1                     | -          | -          | h    | -        | -          | -     | -                                  | 9.833                       | 0.33                        | 1.12                 | 1                                  | 79.4                                 | 0.56                          | 4.44                          | 9.626  | 0.24  | 0.85   | 0.17  | 82.3  | 9.64  | 0.25  | 0.88  |     |
| 16132454-4512439 | 335.962  | 4.316    | 1.335  | 1      | -      | -    | g    | -        | P    | -      | -     | D2                     | -          | -          | -    | -        | -          | V     | -                                  | 11.428                      | 0.49                        | 1.53                 | 1                                  | 31.2                                 | 0.88                          | 4.37                          | 10.931 | 0.27  | 0.87   | 0.41  | 35.5  | 10.92 | 0.30  | 0.96  |     |
| 16133209-6100225 | 325.085  | -7.157   | 0.209  | 1      | -      | -    | g    | -        | -    | -      | -     | D4                     | c          | o          | -    | -        | -          | -     | -                                  | 10.352                      | 0.26                        | 1.03                 | 1                                  | 43.4                                 | 0.90                          | 4.04                          | 10.274 | 0.23  | 0.92   | 0.06  | 43.8  | 10.28 | 0.23  | 0.94  |     |
| 16133290-6049236 | 325.214  | -7.026   | 0.204  | 1      | -      | -    | g    | -        | -    | -      | -     | D4                     | c          | o          | -    | -        | -          | -     | -                                  | 10.366                      | 0.27                        | 1.01                 | 1                                  | 40.2                                 | 0.90                          | 4.04                          | 10.290 | 0.24  | 0.91   | 0.06  | 40.5  | 10.30 | 0.24  | 0.93  |     |
| 16133565-6051545 | 325.189  | -7.060   | 0.200  | 1      | -      | -    | g    | -        | t    | -      | -     | D1                     | c          | o          | -    | -        | -          | -     | -                                  | 9.745                       | 0.33                        | 1.08                 | 1                                  | 82.8                                 | 0.30                          | 4.04                          | 9.670  | 0.30  | 0.98   | 0.06  | 83.5  | 9.68  | 0.30  | 0.99  |     |
| 16133938-6059555 | 325.101  | -7.161   | 0.208  | 1      | -      | -    | g    | -        | -    | -      | -     | D1                     | c          | o          | -    | -        | -          | -     | -                                  | 10.850                      | 0.32                        | 0.93                 | 1                                  | 38.6                                 | 0.66                          | 4.04                          | 10.773 | 0.29  | 0.82   | 0.06  | 39.0  | 10.78 | 0.29  | 0.84  |     |
| 16134504-6324295 | 323.420  | -8.903   | 0.139  | 1      | -      | -    | g    | -        | t    | -      | -     | D4                     | c          | o          | -    | h        | -          | -     | -                                  | 10.886                      | 0.36                        | 1.11                 | 1                                  | 55.8                                 | 0.28                          | 3.93                          | 10.834 | 0.33  | 1.04   | 0.04  | 56.2  | 10.84 | 0.33  | 1.05  |     |
| 16134598-6100295 | 325.104  | -7.177   | 0.210  | 1      | -      | -    | g    | -        | -    | -      | -     | D1                     | c          | o          | -    | -        | -          | -     | -                                  | 10.057                      | 0.27                        | 1.00                 | 1                                  | 67.2                                 | 0.38                          | 4.04                          | 9.979  | 0.24  | 0.90   | 0.07  | 67.8  | 9.99  | 0.24  | 0.91  |     |
| 16135372-6052014 | 325.214  | -7.086   | 0.202  | 1      | -      | -    | g    | -        | t    | -      | -     | D1                     | c          | o          | -    | -        | -          | -     | -                                  | 10.676                      | 0.29                        | 0.99                 | 1                                  | 49.2                                 | 0.36                          | 4.04                          | 10.601 | 0.26  | 0.89   | 0.06  | 49.6  | 10.61 | 0.26  | 0.90  |     |
| 16135616-6100414 | 325.117  | -7.194   | 0.211  | 1      | -      | -    | g    | -        | -    | -      | -     | D4                     | c          | o          | -    | -        | -          | -     | -                                  | 9.512                       | 0.29                        | 1.01                 | 1                                  | 65.4                                 | 0.84                          | 4.04                          | 9.433  | 0.25  | 0.91   | 0.07  | 65.9  | 9.44  | 0.26  | 0.92  |     |
| 16135748-6056244 | 325.169  | -7.144   | 0.201  | 1      | -      | -    | g    | -        | t    | -      | -     | D4                     | c          | o          | -    | -        | -          | -     | -                                  | 10.359                      | 0.27                        | 1.04                 | 1                                  | 48.0                                 | 0.36                          | 4.04                          | 10.284 | 0.24  | 0.94   | 0.06  | 48.4  | 10.29 | 0.25  | 0.96  |     |
| 16140096-6059273 | 325.138  | -7.186   | 0.206  | 1      | -      | -    | g    | -        | -    | -      | -     | D2                     | c          | o          | -    | -        | -          | -     | -                                  | 10.268                      | 0.27                        | 1.00                 | 1                                  | 46.8                                 | 0.68                          | 4.04                          | 10.191 | 0.23  | 0.89   | 0.06  | 47.2  | 10.20 | 0.24  | 0.91  |     |
| 16140287-6029406 | 325.488  | -6.831   | 0.216  | 1      | -      | -    | g    | -        | -    | -      | -     | D4                     | c          | o          | -    | -        | -          | -     | -                                  | 10.887                      | 0.30                        | 1.01                 | 1                                  | 44.6                                 | 0.82                          | 4.09                          | 10.807 | 0.26  | 0.90   | 0.07  | 45.1  | 10.81 | 0.27  | 0.91  |     |
| 16140865-6124527 | 324.853  | -7.502   | 0.182  | 1      | -      | -    | g    | -        | -    | -      | -     | D1                     | c          | o          | -    | -        | -          | -     | -                                  | 11.250                      | 0.29                        | 1.01                 | 1                                  | 39.4                                 | 0.60                          | 4.02                          | 11.182 | 0.26  | 0.92   | 0.06  | 39.8  | 11.19 | 0.26  | 0.93  |     |
| 16142265-6108378 | 325.063  | -7.326   | 0.225  | 1      | -      | -    | g    | -        | -    | -      | -     | D4                     | c          | o          | -    | -        | -          | -     | -                                  | 11.101                      | 0.28                        | 1.02                 | 1                                  | 31.6                                 | 0.76                          | 4.07                          | 11.017 | 0.24  | 0.91   | 0.07  | 32.0  | 11.03 | 0.25  | 0.93  |     |
| 16142542-6103398 | 325.125  | -7.271   | 0.217  | 1      | -      | -    | g    | -        | t    | -      | -     | D1                     | c          | o          | -    | -        | -          | -     | -                                  | 10.605                      | 0.32                        | 1.01                 | 1                                  | 62.4                                 | 0.50                          | 4.07                          | 10.524 | 0.29  | 0.90   | 0.07  | 63.0  | 10.53 | 0.29  | 0.91  |     |
| 16142579-6124308 | 324.882  | -7.521   | 0.188  | 1      | -      | -    | g    | -        | -    | -      | -     | D2                     | c          | o          | -    | -        | -          | -     | -                                  | 11.101                      | 0.29                        | 1.01                 | 1                                  | 37.2                                 | 0.58                          | 4.02                          | 11.031 | 0.26  | 0.92   | 0.06  | 37.5  | 11.04 | 0.26  | 0.93  |     |
| 16144524-6101507 | 325.175  | -7.277   | 0.209  | 1      | -      | -    | g    | -        | -    | -      | -     | D2                     | c          | o          | -    | -        | -          | -     | -                                  | 10.604                      | 0.29                        | 1.03                 | 1                                  | 38.2                                 | 0.52                          | 4.07                          | 10.526 | 0.26  | 0.92   | 0.06  | 38.5  | 10.54 | 0.26  | 0.94  |     |
| 16150065-4950392 | 332.961  | 0.774    | 27.886 | 9      | -      | -    | g    | -        | -    | -      | -     | -                      | -          | -          | -    | -        | -          | -     | -                                  | 7.234                       | 1.40                        | 2.68                 | 1                                  | 219.6                                | 0.56                          | 4.68                          | -3.156 | -3.22 | -11.17 | 8.64  | ...   | ...   | -2.67 | -9.33 |     |
| 16150386-6054261 | 325.289  | -7.214   | 0.195  | 1      | -      | -    | g    | -        | -    | -      | -     | D4                     | c          | o          | -    | -        | -          | -     | -                                  | 8.339                       | 0.32                        | 1.07                 | 1                                  | 110.0                                | 0.78                          | 4.04                          | 8.266  | 0.29  | 0.98   | 0.06  | 110.8 | 8.28  | 0.29  | 0.99  |     |
| 16150990-6053282 | 325.309  | -7.211   | 0.196  | 1      | -      | -    | g    | -        | -    | -      | -     | D1                     | c          | o          | -    | -        | -          | -     | -                                  | 10.850                      | 0.24                        | 0.98                 | 1                                  | 39.0                                 | 0.54                          | 4.04                          | 10.777 | 0.21  | 0.89   | 0.06  | 39.4  | 10.78 | 0.21  | 0.90  |     |
| 16151362-4948505 | 333.007  | 0.772    | 29.552 | 9      | -      | -    | g    | -        | -    | -      | -     | -                      | -          | -          | -    | -        | -          | -     | -                                  | 8.042                       | ...                         | ...                  | 1                                  | 187.8                                | 0.62                          | 4.71                          | -2.969 | ...   | ...    | 9.15  | ...   | ...   | ...   |       |     |
| 16151482-6035312 | 325.527  | -7.003   | 0.245  | 1      | -      | -    | g    | -        | -    | -      | -     | D1                     | c          | o          | -    | -        | -          | -     | -                                  | 10.701                      | 0.23                        | 0.95                 | 1                                  | 46.8                                 | 0.64                          | 4.10                          | 10.610 | 0.19  | 0.83   | 0.08  | 47.4  | 10.62 | 0.20  | 0.84  |     |
| 16151536-6056152 | 325.285  | -7.252   | 0.194  | 1      | -      | -    | g    | -        | -    | -      | -     | D4                     | c          | o          | -    | -        | -          | -     | -                                  | 11.164                      | 0.26                        | 1.03                 | 1                                  | 24.4                                 | 0.84                          | 3.99                          | 11.092 | 0.23  | 0.94   | 0.06  | 24.6  | 11.10 | 0.23  | 0.95  |     |
| 16151598-6107582 | 325.148  | -7.393   | 0.212  | 1      | -      | -    | g    | -        | t    | -      | -     | D1                     | c          | o          | -    | -        | -          | -     | -                                  | 10.905                      | 0.27                        | 0.94                 | 1                                  | 48.2                                 | 0.32                          | 3.99                          | 10.826 | 0.23  | 0.83   | 0.07  | 48.7  | 10.83 | 0.24  | 0.85  |     |
| 16151868-4948535 | 333.017  | 0.762    | 26.148 | 9      | -      | -    | g    | -        | -    | -      | -     | -                      | -          | -          | -    | -        | -          | -     | -                                  | 9.258                       | 1.50                        | ...                  | 1                                  | 68.4                                 | 0.26                          | 4.71                          | -0.485 | -2.83 | ...    | 8.10  | ...   | ...   | -2.32 | ...   |     |
| 16152012-4913215 | 333.429  | 1.187    | 4.727  | 9      | -      | p    | g    | -        | -    | -      | -     | -                      | -          | -          | -    | -        | -          | -     | -                                  | 10.442                      | ...                         | 1.25                 | 1                                  | 19.8                                 | 0.86                          | 4.79                          | 8.681  | ...   | ...    | -1.10 | 1.46  | ...   | ...   | -0.79 | ... |
| 16153118-6232282 | 324.177  | -8.422   | 0.132  | 1      | -      | -    | g    | -        | -    | -      | -     | D2                     | c          | o          | -    | -        | -          | -     | -                                  | 11.282                      | 0.34                        | 1.07                 | 1                                  | 30.0                                 | 0.84                          | 3.97                          | 11.233 | 0.32  | 1.00   | 0.04  | 30.2  | 11.24 | 0.32  | 1.01  |     |
| 16153255-6205222 | 324.498  | -8.101   | 0.144  | 1      | -      | -    | g    | -        | t    | -      | -     | D1                     | c          | o          | -    | -        | -          | -     | -                                  | 10.929                      | 0.28                        | 0.99                 | 1                                  | 49.4                                 | 0.32                          | 3.99                          | 10.875 | 0.26  | 0.92   | 0.04  | 49.7  | 10.88 | 0.26  | 0.93  |     |
| 16153288-6039552 | 325.502  | -7.082   | 0.261  | 1      | -      | -    | g    | -        | -    | -      | -     | D4                     | c          | o          | -    | -        | -          | -     | -                                  | 9.159                       | 0.26                        | 1.03                 | 1                                  | 76.6                                 | 0.84                          | 4.10                          | 9.062  | 0.22  | 0.90   | 0.08  | 77.5  | 9.07  | 0.22  | 0.92  |     |
| 16154609-6055071 | 325.343  | -7.282   | 0.194  | 1      | -      | -    | g    | -        | -    | -      | -     | D4                     | c          | o          | -    | -        | -          | -     | -                                  | 8.315                       | 0.26                        | 0.96                 | 1                                  | 116.4                                | 0.88                          | 4.04                          | 8.243  | 0.23  | 0.87   | 0.06  | 117.2 | 8.25  | 0.24  | 0.88  |     |
| 16155013-6048111 | 325.430  | -7.205   | 0.237  | 1      | -      | -    | g    | -        | -    | -      | -     | D4                     | c          | o          | -    | -        | -          | -     | -                                  | 8.612                       | 0.26                        | 1.00                 | 1                                  | 110.8                                | 0.84                          | 4.04                          | 8.524  | 0.22  | 0.88   | 0.07  | 112.0 | 8.53  | 0.23  | 0.90  |     |
| 16155290-6050571 | 325.402  | -7.242   | 0.214  | 1      | -      | -    | g    | -        | -    | -      | -     | D4                     | c          | o          | -    | -        | -          | -     | -                                  | 10.582                      | 0.28                        | 1.03                 | 1                                  | 68.2                                 | 0.42                          | 4.04                          | 10.502 | 0.24  | 0.92   | 0.07  | 68.9  | 10.51 | 0.25  | 0.93  |     |
| 16160007-3730193 | 341.713  | 9.517    | 1.212  | 1      | -      | -    | g    | -        | -    | N      | -     | D2                     | c          | o          | -    | -        | -          | -     | -                                  | 11.359                      | 0.41                        | 1.43                 | 1                                  | 31.0                                 | 0.56                          | 3.91                          | 10.907 | 0.21  | 0.83   | 0.38  | 34.5  | 10.91 | 0.24  | 0.91  |     |
| 16160871-6102357 | 325.288  | -7.403   | 0.199  | 1      | -      | -    | g    | -        | -    | -      | -     | D2                     | c          | o          | -    | -        | -          | -     | -                                  | 11.314                      | 0.34                        | 1.07                 | 1                                  | 29.0                                 | 0.54                          | 4.06                          | 11.240 | 0.31  | 0.97   | 0.06  | 29.3  | 11.25 | 0.31  | 0.98  |     |
| 16161676-4003142 | 339.945  | 7.662    | 0.995  | 1      | -      | -    | g    | -        | -    | -      | -     | D1                     | -          | -          | h    | -        | -          | -     | -                                  | 10.835                      | 0.33                        | 1.33                 | 1                                  | 55.2                                 | 0.42                          | 4.00                          | 10.464 | 0.17  | 0.83   | 0.31  | 60.8  | 10.45 | 0.18  | 0.90  |     |
| 16161892-6057237 | 325.364  | -7.35    |        |        |        |      |      |          |      |        |       |                        |            |            |      |          |            |       |                                    |                             |                             |                      |                                    |                                      |                               |                               |        |       |        |       |       |       |       |       |     |



Table B1: a) continued.

| 2MASX J          | <i>l</i>    | <i>b</i>    | EBV        | Object       | Sample     | Disc        | 2MRS        | Velocity   | NIR         | Photom        | Ext         | <i>K</i> <sub>20</sub> | <i>H-K</i>   | <i>J-K</i>  | vc           | <i>a</i>     | <i>b/a</i>   | st.d. | <i>K</i> <sub>s</sub> <sup>o</sup> | ( <i>H-K</i> ) <sup>o</sup> | ( <i>J-K</i> ) <sup>o</sup> | <i>A<sub>K</sub></i> | <i>a</i> <sub>d</sub> <sup>o</sup> | <i>K</i> <sub>s</sub> <sup>o,d</sup> | ( <i>H-K</i> ) <sup>o,c</sup> | ( <i>J-K</i> ) <sup>o,c</sup> |             |             |       |             |             |             |        |
|------------------|-------------|-------------|------------|--------------|------------|-------------|-------------|------------|-------------|---------------|-------------|------------------------|--------------|-------------|--------------|--------------|--------------|-------|------------------------------------|-----------------------------|-----------------------------|----------------------|------------------------------------|--------------------------------------|-------------------------------|-------------------------------|-------------|-------------|-------|-------------|-------------|-------------|--------|
| (1)              | deg<br>(2a) | deg<br>(2b) | mag<br>(3) | class<br>(4) | off<br>(5) | flag<br>(6) | gal<br>(7a) | TF<br>(7b) | obs<br>(7c) | ext'd<br>(7d) | type<br>(8) | (9)                    | Opt<br>(10a) | HI<br>(10b) | flag<br>(11) | flag<br>(12) | flag<br>(13) | (14)  | mag<br>(15)                        | mag<br>(16)                 | (17)                        | (18)                 | (19)                               | (20)                                 | mag<br>(21)                   | mag<br>(22)                   | mag<br>(23) | mag<br>(24) | (25)  | mag<br>(26) | mag<br>(27) | mag<br>(28) |        |
| 16201048–5053291 | 332.822     | −0.551      | 52.109     | 9            | –          | –           | –           | –          | –           | –             | D3          | –                      | –            | –           | –            | –            | –            | –     | 8.952                              | ...                         | ...                         | 1                    | 63.0                               | 0.50                                 | 4.83                          | −10.464                       | ...         | ...         | 16.14 | ...         | ...         | ...         |        |
| 16201509–6100450 | 325.666     | −7.732      | 0.218      | 1            | –          | –           | –           | –          | –           | –             | D1          | c                      | o            | –           | –            | –            | –            | –     | 11.072                             | 0.23                        | 0.95                        | 1                    | 36.8                               | 0.56                                 | 4.03                          | 10.991                        | 0.19        | 0.84        | 0.07  | 37.2        | 11.00       | 0.20        | 0.85   |
| 16201973–4231341 | 338.740     | 5.370       | 0.873      | 1            | –          | –           | –           | –          | –           | –             | D1          | c                      | o            | –           | –            | –            | –            | –     | 11.013                             | 0.43                        | 1.26                        | 1                    | 37.0                               | 0.66                                 | 4.24                          | 10.688                        | 0.29        | 0.83        | 0.27  | 39.6        | 10.70       | 0.31        | 0.88   |
| 16203332–5040423 | 333.015     | −0.442      | 80.299     | 9            | –          | –           | –           | –          | –           | –             | –           | –                      | –            | –           | –            | –            | –            | –     | 7.292                              | ...                         | ...                         | 1                    | 115.4                              | 0.80                                 | 4.74                          | −22.627                       | ...         | ...         | 24.87 | ...         | ...         | ...         |        |
| 16203357–4428001 | 337.394     | 3.966       | 1.331      | 2            | –          | –           | –           | –          | +           | –             | n           | –                      | –            | –           | –            | –            | –            | –     | 10.616                             | 0.31                        | 1.07                        | 1                    | 51.0                               | 0.84                                 | 4.37                          | 10.120                        | 0.09        | 0.40        | 0.41  | 58.4        | 10.10       | 0.11        | 0.49   |
| 16204949–6024173 | 326.151     | −7.353      | 0.245      | 1            | –          | –           | –           | –          | –           | –             | D1          | c                      | o            | –           | –            | –            | –            | –     | 10.422                             | 0.30                        | 1.11                        | 1                    | 49.4                               | 0.58                                 | 3.99                          | 10.331                        | 0.26        | 0.99        | 0.08  | 50.0        | 10.34       | 0.27        | 1.00   |
| 16205221–6105164 | 325.665     | −7.838      | 0.204      | 1            | –          | –           | –           | –          | –           | –             | D2          | c                      | o            | –           | –            | –            | –            | –     | 10.469                             | 0.21                        | 0.96                        | 1                    | 47.2                               | 0.74                                 | 4.03                          | 10.393                        | 0.18        | 0.85        | 0.06  | 47.6        | 10.40       | 0.18        | 0.87   |
| 16205835–6029274 | 326.102     | −7.427      | 0.245      | 1            | –          | o           | –           | –          | –           | –             | D1          | c                      | –            | –           | h            | –            | o            | –     | 10.506                             | 0.19                        | 0.83                        | 1                    | 81.2                               | 0.36                                 | 3.99                          | 10.415                        | 0.15        | 0.71        | 0.08  | 82.5        | 10.42       | 0.16        | 0.72   |
| 16205968–5035141 | 333.128     | −0.426      | 94.843     | 9            | –          | –           | –           | –          | –           | –             | –           | –                      | –            | –           | –            | –            | –            | –     | 8.529                              | ...                         | ...                         | 1                    | 79.2                               | 1.00                                 | 4.74                          | −26.810                       | ...         | ...         | 29.38 | ...         | ...         | ...         |        |
| 16210034–5036143 | 333.118     | −0.439      | 102.805    | 9            | –          | –           | –           | –          | –           | –             | –           | –                      | –            | –           | –            | –            | –            | –     | 8.000                              | ...                         | ...                         | 1                    | 218.6                              | 0.62                                 | 4.75                          | −30.305                       | ...         | ...         | 31.84 | ...         | ...         | ...         |        |
| 16210050–5035089 | 333.131     | −0.427      | 93.697     | 9            | –          | –           | –           | –          | –           | –             | –           | –                      | –            | –           | –            | –            | –            | –     | 7.306                              | ...                         | ...                         | 1                    | 159.2                              | 1.00                                 | 4.75                          | −27.605                       | ...         | ...         | 29.02 | ...         | ...         | ...         |        |
| 16210166–3608318 | 343.413     | 9.765       | 0.711      | 1            | –          | –           | –           | –          | –           | –             | D1          | c                      | –            | –           | h            | –            | –            | –     | 9.588                              | 0.33                        | 1.18                        | 1                    | 79.6                               | 0.48                                 | 3.89                          | 9.323                         | 0.21        | 0.82        | 0.22  | 83.3        | 9.35        | 0.23        | 0.87   |
| 16210615–6037085 | 326.022     | −7.528      | 0.219      | 1            | –          | –           | –           | –          | –           | –             | D3          | c                      | o            | –           | –            | –            | –            | –     | 10.297                             | 0.38                        | 1.13                        | 1                    | 41.6                               | 0.88                                 | 3.99                          | 10.215                        | 0.34        | 1.03        | 0.07  | 42.0        | 10.23       | 0.35        | 1.04   |
| 16210829–6118175 | 325.532     | −8.013      | 0.203      | 1            | –          | –           | –           | –          | –           | –             | D1          | c                      | o            | –           | –            | –            | –            | –     | 11.316                             | 0.23                        | 0.99                        | 1                    | 25.4                               | 0.88                                 | 3.99                          | 11.240                        | 0.20        | 0.89        | 0.06  | 25.6        | 11.25       | 0.20        | 0.90   |
| 16211112–6059065 | 325.766     | −7.793      | 0.231      | 1            | –          | –           | –           | –          | –           | –             | D1          | c                      | o            | –           | –            | –            | –            | –     | 10.270                             | 0.36                        | 1.04                        | 1                    | 51.6                               | 0.80                                 | 4.03                          | 10.184                        | 0.32        | 0.92        | 0.07  | 52.1        | 10.19       | 0.32        | 0.94   |
| 16211990–6046585 | 325.924     | −7.663      | 0.215      | 1            | –          | –           | –           | –          | –           | –             | D3          | c                      | –            | –           | –            | –            | –            | –     | 9.107                              | 0.29                        | 1.03                        | 1                    | 75.2                               | 0.76                                 | 4.00                          | 9.027                         | 0.25        | 0.92        | 0.07  | 75.9        | 9.04        | 0.25        | 0.93   |
| 16213188–5025042 | 333.308     | −0.366      | 79.638     | 9            | –          | –           | –           | –          | –           | –             | –           | –                      | –            | –           | –            | –            | –            | –     | 6.812                              | 2.02                        | ...                         | 1                    | 178.6                              | 0.94                                 | 4.72                          | −22.861                       | −11.17      | ...         | 24.67 | ...         | ...         | −9.61       | ...    |
| 16214525–6110483 | 325.674     | −7.978      | 0.206      | 1            | –          | –           | –           | –          | –           | –             | D1          | c                      | –            | –           | –            | –            | –            | –     | 10.637                             | 0.30                        | 1.03                        | 1                    | 46.0                               | 0.74                                 | 4.03                          | 10.560                        | 0.27        | 0.93        | 0.06  | 46.4        | 10.57       | 0.27        | 0.95   |
| 16214686–6125313 | 325.500     | −8.153      | 0.195      | 1            | –          | –           | –           | –          | –           | –             | D1          | c                      | o            | –           | –            | –            | –            | –     | 10.950                             | 0.32                        | 1.09                        | 1                    | 33.6                               | 0.50                                 | 3.99                          | 10.877                        | 0.29        | 0.99        | 0.06  | 33.9        | 10.89       | 0.29        | 1.01   |
| 16215494–6040087 | 326.056     | −7.635      | 0.214      | 1            | –          | –           | –           | –          | –           | –             | D1          | c                      | –            | –           | –            | –            | –            | –     | 8.855                              | 0.25                        | 0.99                        | 1                    | 95.4                               | 0.42                                 | 4.00                          | 8.775                         | 0.21        | 0.88        | 0.07  | 96.2        | 8.79        | 0.22        | 0.89   |
| 16220379–3811082 | 342.080     | 8.189       | 1.027      | 1            | –          | –           | –           | –          | –           | –             | D2          | c                      | –            | –           | –            | –            | –            | –     | 10.758                             | 0.40                        | 1.40                        | 1                    | 38.6                               | 0.90                                 | 3.99                          | 10.375                        | 0.23        | 0.89        | 0.32  | 41.9        | 10.39       | 0.25        | 0.96   |
| 16220862–5005405 | 333.606     | −0.207      | 96.267     | 9            | –          | –           | –           | –          | –           | –             | –           | –                      | –            | –           | –            | –            | –            | –     | 6.137                              | ...                         | ...                         | 1                    | 164.0                              | 1.00                                 | 4.72                          | −29.732                       | ...         | ...         | 29.82 | ...         | ...         | ...         | ...    |
| 16221035–5006168 | 333.602     | −0.217      | 91.800     | 9            | –          | –           | –           | –          | –           | –             | –           | –                      | –            | –           | –            | –            | –            | –     | 5.775                              | 1.54                        | 2.83                        | 1                    | 233.0                              | 0.70                                 | 4.72                          | −28.430                       | −13.67      | −42.78      | 28.44 | ...         | ...         | −11.86      | −36.72 |
| 16221294–6333019 | 323.995     | −9.672      | 0.129      | 1            | –          | –           | –           | –          | –           | –             | D1          | c                      | –            | –           | –            | –            | –            | –     | 10.727                             | 0.35                        | 1.09                        | 1                    | 42.4                               | 0.56                                 | 3.91                          | 10.679                        | 0.33        | 1.03        | 0.04  | 42.6        | 10.69       | 0.33        | 1.04   |
| 16221431–3809491 | 342.120     | 8.180       | 1.046      | 1            | –          | –           | –           | –          | –           | –             | D3          | c                      | –            | –           | –            | –            | –            | –     | 11.636                             | 0.40                        | 1.34                        | 1                    | 19.2                               | 0.58                                 | 3.99                          | 11.246                        | 0.23        | 0.82        | 0.32  | 20.9        | 11.26       | 0.25        | 0.89   |
| 16222962–4444511 | 337.439     | 3.524       | 1.150      | 2            | –          | –           | –           | –          | –           | –             | D2          | c                      | –            | –           | h            | –            | –            | –     | 11.615                             | 0.40                        | ...                         | 1                    | 18.2                               | 0.80                                 | 4.47                          | 11.187                        | 0.21        | ...         | 0.36  | 20.3        | 11.18       | 0.23        | ...    |
| 16223484–6102138 | 325.848     | −7.950      | 0.239      | 1            | –          | –           | –           | –          | –           | –             | D4          | c                      | –            | –           | –            | –            | –            | –     | 10.649                             | 0.31                        | 1.08                        | 1                    | 38.4                               | 0.98                                 | 4.00                          | 10.560                        | 0.27        | 0.96        | 0.07  | 38.8        | 10.57       | 0.28        | 0.98   |
| 16225317–5048489 | 333.180     | −0.798      | 7.304      | 8            | –          | –           | –           | –          | –           | –             | –           | –                      | –            | –           | –            | –            | –            | –     | 8.658                              | 0.83                        | ...                         | −2                   | 76.4                               | 1.00                                 | 4.85                          | 5.937                         | −0.38       | ...         | 2.26  | ...         | ...         | −0.24       | ...    |
| 16230766–3739356 | 342.608     | 8.406       | 1.418      | 1            | –          | –           | –           | –          | –           | –             | D1          | c                      | –            | –           | –            | –            | –            | –     | 11.519                             | 0.47                        | 1.63                        | 1                    | 38.4                               | 0.92                                 | 3.93                          | 10.991                        | 0.23        | 0.93        | 0.44  | 44.5        | 10.96       | 0.26        | 1.02   |
| 16233614–6142283 | 325.448     | −8.505      | 0.170      | 1            | –          | –           | –           | –          | –           | –             | D1          | c                      | –            | –           | –            | –            | –            | –     | 10.209                             | 0.28                        | 0.91                        | 1                    | 57.2                               | 0.38                                 | 3.95                          | 10.146                        | 0.25        | 0.83        | 0.05  | 57.6        | 10.15       | 0.26        | 0.84   |
| 16241101–4356519 | 338.222     | 3.871       | 1.157      | 4            | –          | –           | –           | –          | –           | –             | D4          | c                      | –            | –           | –            | –            | –            | –     | 11.528                             | 0.34                        | 1.34                        | −2                   | 20.2                               | 0.86                                 | 4.42                          | 11.097                        | 0.15        | 0.76        | 0.36  | 22.3        | 11.11       | 0.17        | 0.84   |
| 16241246–6018415 | 326.513     | −7.587      | 0.231      | 1            | –          | –           | –           | –          | –           | –             | D1          | c                      | –            | –           | –            | –            | –            | –     | 10.487                             | 0.19                        | 0.90                        | 1                    | 58.8                               | 0.48                                 | 4.02                          | 10.401                        | 0.15        | 0.78        | 0.07  | 59.5        | 10.41       | 0.15        | 0.80   |
| 16241496–6105415 | 325.948     | −8.135      | 0.222      | 1            | –          | –           | –           | –          | –           | –             | D1          | c                      | o            | –           | –            | –            | –            | –     | 10.312                             | 0.31                        | 1.03                        | 1                    | 44.8                               | 0.58                                 | 3.96                          | 10.229                        | 0.28        | 0.92        | 0.07  | 45.2        | 10.24       | 0.28        | 0.94   |
| 16243987–6113104 | 325.892     | −8.257      | 0.212      | 1            | –          | –           | –           | –          | –           | –             | D1          | c                      | –            | –           | –            | –            | –            | –     | 10.315                             | 0.25                        | 0.97                        | 1                    | 46.4                               | 0.88                                 | 3.96                          | 10.236                        | 0.21        | 0.86        | 0.07  | 46.8        | 10.25       | 0.22        | 0.87   |
| 16252396–6238169 | 324.915     | −9.300      | 0.165      | 1            | –          | –           | –           | –          | –           | –             | D3          | c                      | –            | –           | –            | –            | –            | –     | 9.285                              | 0.24                        | 0.97                        | 1                    | 88.2                               | 0.48                                 | 3.91                          | 9.224                         | 0.22        | 0.88        | 0.05  | 88.7        | 9.23        | 0.22        | 0.89   |
| 16252989–5402389 | 331.154     | −3.347      | 0.790      | 4            | –          | –           | –           | –          | –           | –             | t           | +                      | n            | –           | –            | –            | –            | –     | 9.872                              | 0.36                        | 1.33                        | −2                   | 41.6                               | 0.30                                 | 4.53                          | 9.578                         | 0.23        | 0.94        | 0.24  | 44.3        | 9.59        | 0.25        | 0.99   |
| 16254669–3707583 | 343.361     | 8.392       | 0.982      | 1            | –          | –           | –           | –          | –           | –             | D1          | c                      | –            | –           | –            | –            | –            | –     | 11.107                             | 0.48                        | 1.62                        | 1                    | 37.6                               | 0.36                                 | 3.98                          | 10.741                        | 0.32        | 1.14        | 0.30  | 40.7        | 10.75       | 0.34        | 1.20   |
| 16255024–6045092 | 326.333     | −8.037      | 0.192      | 1            | –          | –           | –           | –          | –           | –             | D3          | c                      | –            | –           | –            | –            | –            | –     | 9.107                              | 0.24                        | 1.02                        | 1                    | 82.4                               | 0.90                                 | 4.00                          | 9.035                         | 0.21        | 0.92        | 0.06  | 83.0        | 9.04        | 0.21        | 0.93   |
| 16255621–6257533 | 324.718     | −9.569      | 0.190      | 1            | –          | –           | –           | –          | –           | –             | D1          | c                      | –            | –           | –            | –            | –            | –     | 10.561                             | 0.28                        | 0.97                        | 1                    | 42.2                               | 0.54                                 | 3.83                          | 10.490                        | 0.24        | 0.87        | 0.06  | 42.5        | 10.50       | 0.25        | 0.89   |
| 16260518–6031363 | 326.519     | −7.903      | 0.204      | 1            | –          | –           | –           | –          | –           | –             | D1          | c                      | –            | –           | –            | –            | –            | –     | 9.882                              | 0.26                        | 1.05                        | 1                    | 68.0                               | 0.38                                 | 4.04                          | 9.806                         | 0.23        | 0.95        | 0.06  | 68.6        | 9.81        | 0.23        | 0.97   |
| 16260948–6139433 | 325.694     | −8.692      | 0.184      | 1            | –          | –           | –           | –          | –           | –             | D1          | c                      | –            | –           | –            | –            | –            | –     | 9.709                              | 0.31                        | 0.99                        | 1                    | 65.2                               | 0.46                                 | 3.92                          | 9.640                         | 0.28        | 0.90        | 0.06  | 65.7        | 9.65        | 0.29        | 0.91   |
| 16263569–6311462 | 324.599     | −9.782      | 0.165      | 1            | –          | –           | –           | –          | –           | –             | D1          | c                      | –            | –           | h            | –            | –            | –     | 9.608                              | 0.29                        | 0.98                        | 1                    | 89.0                               | 0.56                                 | 3.89                          | 9.547                         |             |             |       |             |             |             |        |

Table B1: a) continued.

| 2MASX J          | <i>l</i>    | <i>b</i>    | EBV        | Object       | Sample     | Disc       | 2MRS        | Velocity   | NIR         | Photom        | Ext         | <i>K</i> <sub>20</sub> | <i>H-K</i>   | <i>J-K</i>  | vc          | <i>a</i>    | <i>b/a</i>  | st.d.  | <i>K</i> <sub>s</sub> <sup>o</sup> | ( <i>H-K</i> ) <sup>o</sup> | ( <i>J-K</i> ) <sup>o</sup> | <i>A<sub>K</sub></i> | <i>a</i> <sub>d</sub> <sup>o</sup> | <i>K</i> <sub>s</sub> <sup>o,d</sup> | ( <i>H-K</i> ) <sup>o,c</sup> | ( <i>J-K</i> ) <sup>o,c</sup> |             |             |       |             |             |             |
|------------------|-------------|-------------|------------|--------------|------------|------------|-------------|------------|-------------|---------------|-------------|------------------------|--------------|-------------|-------------|-------------|-------------|--------|------------------------------------|-----------------------------|-----------------------------|----------------------|------------------------------------|--------------------------------------|-------------------------------|-------------------------------|-------------|-------------|-------|-------------|-------------|-------------|
| (1)              | deg<br>(2a) | deg<br>(2b) | mag<br>(3) | class<br>(4) | off<br>(5) | flg<br>(6) | gal<br>(7a) | TF<br>(7b) | obs<br>(7c) | ext'd<br>(7d) | type<br>(8) | (9)                    | Opt<br>(10a) | HI<br>(10b) | flg<br>(11) | flg<br>(12) | flg<br>(13) | (14)   | mag<br>(15)                        | mag<br>(16)                 | (17)                        | (18)                 | (19)                               | (20)                                 | mag<br>(21)                   | mag<br>(22)                   | mag<br>(23) | mag<br>(24) | (25)  | mag<br>(26) | mag<br>(27) | mag<br>(28) |
| 16332520-6145145 | 326.216     | -9.387      | 0.392      | 1            | -          | -          | g           | -          | -           | -             | D2          | c                      | o            | -           | -           | -           | e           | 10.709 | 0.31                               | 1.15                        | 1                           | 51.2                 | 0.74                               | 3.94                                 | 10.563                        | 0.25                          | 0.96        | 0.12        | 52.4  | 10.58       | 0.26        | 0.98        |
| 16334670-5732425 | 329.397     | -6.594      | 0.434      | 1            | -          | -          | g           | -          | -           | -             | D3          | c                      | o            | -           | -           | -           | e           | 11.263 | 0.33                               | 1.14                        | 1                           | 24.4                 | 0.76                               | 4.12                                 | 11.101                        | 0.26                          | 0.92        | 0.13        | 25.0  | 11.11       | 0.27        | 0.95        |
| 16340733-6137462 | 326.367     | -9.365      | 0.266      | 1            | -          | -          | g           | -          | -           | -             | D1          | c                      | o            | -           | -           | -           | e?          | 11.236 | 0.47                               | 1.29                        | 1                           | 27.6                 | 0.60                               | 3.92                                 | 11.137                        | 0.42                          | 1.16        | 0.08        | 28.0  | 11.15       | 0.43        | 1.18        |
| 16342643-5833520 | 328.696     | -7.344      | 0.312      | 1            | -          | -          | g           | -          | -           | -             | D4          | c                      | o            | -           | -           | -           | -           | 11.059 | 0.34                               | 1.12                        | 1                           | 34.0                 | 0.78                               | 4.06                                 | 10.943                        | 0.29                          | 0.97        | 0.10        | 34.6  | 10.95       | 0.30        | 0.99        |
| 16342689-3856119 | 343.204     | 5.913       | 0.838      | 1            | -          | -          | g           | -          | -           | -             | D3          | c                      | o            | -           | -           | V           | -           | 10.526 | 0.37                               | 1.20                        | 1                           | 47.0                 | 0.86                               | 4.22                                 | 10.214                        | 0.24                          | 0.78        | 0.26        | 49.9  | 10.23       | 0.25        | 0.84        |
| 16342826-3857439 | 343.188     | 5.893       | 0.852      | 1            | -          | -          | g           | -          | N           | -             | D1          | c                      | o            | -           | -           | V           | -           | 11.336 | 0.28                               | 1.15                        | 1                           | 27.0                 | 0.70                               | 4.22                                 | 11.019                        | 0.14                          | 0.72        | 0.26        | 29.0  | 11.02       | 0.15        | 0.78        |
| 16343783-3335383 | 347.233     | 9.463       | 0.546      | 1            | -          | -          | g           | -          | -           | -             | D1          | c                      | o            | -           | -           | V           | -           | 11.355 | 0.36                               | 1.16                        | 1                           | 33.4                 | 0.60                               | 3.96                                 | 11.152                        | 0.27                          | 0.89        | 0.17        | 34.7  | 11.16       | 0.28        | 0.92        |
| 16344705-3909459 | 343.080     | 5.713       | 1.147      | 1            | -          | -          | g           | -          | N           | -             | D1          | c                      | o            | -           | -           | V           | -           | 10.607 | 0.38                               | 1.38                        | 1                           | 47.2                 | 0.44                               | 4.25                                 | 10.180                        | 0.19                          | 0.81        | 0.36        | 51.9  | 10.20       | 0.22        | 0.88        |
| 16345255-6037075 | 327.191     | -8.759      | 0.172      | 1            | -          | -          | g           | -          | -           | -             | D1          | c                      | o            | -           | -           | h           | -           | 8.777  | 0.32                               | 1.03                        | 1                           | 94.8                 | 0.82                               | 3.98                                 | 8.713                         | 0.29                          | 0.95        | 0.05        | 95.4  | 8.72        | 0.29        | 0.96        |
| 16351411-5804481 | 329.129     | -7.097      | 0.335      | 1            | -          | -          | g           | -          | -           | -             | D1          | c                      | o            | -           | -           | h           | -           | 8.362  | 0.29                               | 0.98                        | 1                           | 112.0                | 0.87                               | ...                                  | 8.237                         | 0.24                          | 0.82        | 0.10        | ...   | ...         | 0.24        | 0.84        |
| 16351643-6123364 | 326.638     | -9.311      | 0.255      | 1            | -          | -          | g           | -          | -           | -             | D1          | c                      | o            | -           | -           | h           | -           | 10.653 | 0.31                               | 1.04                        | 1                           | 57.6                 | 0.34                               | 3.92                                 | 10.558                        | 0.27                          | 0.91        | 0.08        | 58.3  | 10.57       | 0.27        | 0.93        |
| 16351917-5813077 | 329.033     | -7.198      | 0.319      | 1            | -          | -          | g           | -          | -           | -             | D2          | c                      | o            | -           | -           | h           | -           | 9.612  | 0.24                               | 0.97                        | 1                           | 77.4                 | 0.62                               | 4.05                                 | 9.493                         | 0.19                          | 0.81        | 0.10        | 78.7  | 9.51        | 0.20        | 0.83        |
| 16354738-5529558 | 331.108     | -5.424      | 0.428      | 1            | -          | -          | g           | -          | -           | -             | D3          | c                      | o            | -           | -           | h           | -           | 11.401 | 0.39                               | 1.22                        | 1                           | 30.8                 | 0.84                               | 4.24                                 | 11.242                        | 0.32                          | 1.01        | 0.13        | 31.7  | 11.25       | 0.33        | 1.04        |
| 16355086-6128002 | 326.628     | -9.411      | 0.246      | 1            | -          | -          | g           | -          | -           | -             | D1          | c                      | o            | -           | -           | h           | -           | 9.681  | 0.33                               | 0.99                        | 1                           | 83.6                 | 0.40                               | 3.91                                 | 9.589                         | 0.29                          | 0.87        | 0.08        | 84.6  | 9.60        | 0.30        | 0.89        |
| 16361692-4213242 | 340.997     | 3.445       | 1.946      | 1            | -          | -          | g           | -          | P           | -             | D1          | c                      | o            | -           | -           | h           | -           | 9.920  | 0.51                               | 1.48                        | 1                           | 62.4                 | 0.82                               | 4.49                                 | 9.195                         | 0.19                          | 0.51        | 0.60        | 74.5  | 9.22        | 0.23        | 0.64        |
| 16365206-6016347 | 327.615     | -8.715      | 0.231      | 1            | -          | -          | g           | -          | -           | -             | D1          | c                      | o            | -           | -           | h           | -           | 10.654 | 0.32                               | 0.97                        | 1                           | 48.8                 | 0.68                               | 3.96                                 | 10.568                        | 0.28                          | 0.85        | 0.07        | 49.4  | 10.58       | 0.29        | 0.87        |
| 16365352-6101397 | 327.046     | -9.214      | 0.258      | 1            | -          | -          | g           | -          | -           | -             | D2          | c                      | o            | -           | -           | h           | -           | 9.877  | 0.21                               | 0.92                        | 1                           | 66.0                 | 0.38                               | 3.92                                 | 9.781                         | 0.17                          | 0.79        | 0.08        | 66.8  | 9.79        | 0.18        | 0.81        |
| 16380086-3605570 | 345.806     | 7.281       | 0.802      | 1            | -          | -          | g           | -          | N           | -             | D1          | c                      | o            | -           | -           | h           | -           | 9.437  | 0.38                               | 1.26                        | 1                           | 74.0                 | 0.44                               | 4.12                                 | 9.138                         | 0.25                          | 0.86        | 0.25        | 78.1  | 9.16        | 0.26        | 0.91        |
| 16380546-6106465 | 327.078     | -9.379      | 0.278      | 1            | -          | -          | g           | -          | -           | -             | D2          | c                      | o            | -           | -           | h           | -           | 10.719 | 0.26                               | 1.04                        | 1                           | 40.4                 | 0.46                               | 3.92                                 | 10.615                        | 0.21                          | 0.90        | 0.09        | 41.0  | 10.63       | 0.22        | 0.92        |
| 16385274-4125075 | 341.921     | 3.623       | 0.959      | 6            | -          | -          | g           | -          | -           | -             | D1          | c                      | o            | -           | -           | h           | -           | 11.419 | 0.42                               | 1.39                        | 1                           | 20.6                 | 0.72                               | 4.48                                 | 11.062                        | 0.26                          | 0.91        | 0.30        | ...   | ...         | 0.28        | 0.98        |
| 16391837-5953106 | 328.114     | -8.687      | 0.281      | 1            | -          | -          | g           | -          | -           | -             | D1          | c                      | o            | -           | -           | h           | -           | 10.529 | 0.23                               | 1.04                        | 1                           | 56.0                 | 0.28                               | 3.95                                 | 10.424                        | 0.19                          | 0.90        | 0.09        | 56.8  | 10.44       | 0.19        | 0.92        |
| 16395987-4851524 | 336.489     | -1.476      | 36.081     | 9            | -          | -          | g           | -          | -           | -             | D1          | c                      | o            | -           | -           | h           | -           | 6.723  | 1.23                               | 2.56                        | 1                           | 113.8                | 0.88                               | 4.82                                 | -6.721                        | -4.74                         | -15.37      | 11.18       | ...   | ...         | -4.04       | -12.99      |
| 16400714-3806551 | 344.562     | 5.634       | 0.663      | 1            | -          | -          | g           | -          | -           | -             | D2          | e                      | o            | -           | -           | V           | -           | 11.036 | 0.43                               | 1.31                        | 1                           | 38.8                 | 0.58                               | 4.31                                 | 10.789                        | 0.32                          | 0.98        | 0.21        | 40.6  | 10.81       | 0.33        | 1.02        |
| 16402196-5240403 | 333.668     | -4.046      | 0.654      | 2            | -          | -          | g           | -          | +           | -             | n           | c                      | o            | -           | -           | h           | -           | 10.492 | 0.38                               | 1.20                        | 1                           | 41.2                 | 0.62                               | 4.44                                 | 10.248                        | 0.27                          | 0.88        | 0.20        | 43.3  | 10.26       | 0.29        | 0.92        |
| 16405260-6023395 | 327.854     | -9.167      | 0.246      | 1            | -          | -          | g           | -          | -           | -             | D1          | c                      | o            | -           | -           | h           | -           | 9.831  | 0.33                               | 1.04                        | 1                           | 66.2                 | 0.58                               | 3.94                                 | 9.739                         | 0.29                          | 0.91        | 0.08        | 67.0  | 9.75        | 0.29        | 0.93        |
| 16405900-4707080 | 337.906     | -0.442      | 53.393     | 9            | -          | -          | g           | -          | -           | -             | D1          | c                      | o            | -           | -           | h           | -           | 9.050  | ...                                | ...                         | 1                           | 56.0                 | 0.42                               | 4.83                                 | -10.844                       | ...                           | ...         | 16.54       | ...   | ...         | ...         | ...         |
| 16410186-6138515 | 326.900     | -9.995      | 0.292      | 1            | -          | -          | g           | -          | -           | -             | D1          | c                      | o            | -           | -           | h           | -           | 10.945 | 0.34                               | 1.05                        | 1                           | 45.2                 | 0.54                               | 3.88                                 | 10.836                        | 0.29                          | 0.90        | 0.09        | 45.9  | 10.85       | 0.30        | 0.92        |
| 16410569-4707383 | 337.912     | -0.462      | 54.151     | 9            | -          | -          | g           | -          | -           | -             | D1          | c                      | o            | -           | -           | h           | -           | 7.219  | 1.41                               | 2.84                        | 1                           | 83.4                 | 0.68                               | 4.81                                 | -12.958                       | -7.56                         | -24.06      | 16.77       | ...   | ...         | -6.49       | -20.49      |
| 16410805-4706463 | 337.927     | -0.457      | 61.494     | 9            | -          | -          | g           | -          | -           | -             | D1          | c                      | o            | -           | -           | h           | -           | 6.287  | 1.31                               | 2.76                        | 1                           | 232.6                | 0.34                               | 4.81                                 | -16.626                       | -8.87                         | -27.79      | 19.05       | ...   | ...         | -7.66       | -23.73      |
| 16410990-4708074 | 337.914     | -0.476      | 53.498     | 9            | -          | -          | g           | -          | -           | -             | D1          | c                      | o            | -           | -           | h           | -           | 6.431  | ...                                | ...                         | 1                           | 161.4                | 0.56                               | 4.81                                 | -13.502                       | ...                           | ...         | 16.57       | ...   | ...         | ...         | ...         |
| 16412624-5448360 | 332.164     | -5.571      | 0.373      | 1            | -          | -          | g           | -          | -           | -             | D2          | e                      | o            | -           | -           | V           | -           | 8.714  | 0.32                               | 1.02                        | 1                           | 98.8                 | 0.70                               | 4.26                                 | 8.575                         | 0.26                          | 0.84        | 0.12        | 100.6 | 8.59        | 0.26        | 0.86        |
| 16414244-3620078 | 346.120     | 6.565       | 1.055      | 9            | -          | -          | g           | -          | e           | -             | D1          | c                      | o            | -           | -           | h           | -           | 11.270 | 0.18                               | 1.08                        | -2                          | 53.0                 | 0.64                               | 4.21                                 | 10.877                        | 0.00                          | 0.55        | 0.33        | ...   | ...         | 0.02        | 0.62        |
| 16414252-3619588 | 346.122     | 6.566       | 1.053      | 1            | -          | -          | g           | -          | -           | -             | D1          | e                      | o            | -           | -           | V           | -           | 10.455 | 0.36                               | 1.29                        | 1                           | 53.6                 | 0.44                               | 4.17                                 | 10.063                        | 0.19                          | 0.77        | 0.33        | 57.9  | 10.09       | 0.21        | 0.84        |
| 16422261-5556008 | 331.398     | -6.407      | 0.291      | 1            | -          | -          | g           | -          | -           | -             | D4          | e                      | o            | -           | -           | h           | -           | 9.108  | 0.27                               | 1.01                        | 1                           | 74.0                 | 0.84                               | 4.16                                 | 9.000                         | 0.22                          | 0.87        | 0.09        | 74.9  | 9.01        | 0.23        | 0.89        |
| 16424985-6105257 | 327.473     | -9.799      | 0.298      | 1            | -          | -          | g           | -          | -           | -             | D1          | c                      | o            | -           | -           | h           | -           | 11.234 | 0.35                               | 1.26                        | 1                           | 80.4                 | 0.14                               | 3.89                                 | 11.123                        | 0.30                          | 1.11        | 0.09        | 82.0  | 11.13       | 0.30        | 1.13        |
| 16431182-3055328 | 350.482     | 9.841       | 0.428      | 1            | -          | -          | g           | -          | -           | -             | D1          | c                      | o            | -           | -           | h           | -           | 10.743 | 0.29                               | 1.11                        | 1                           | 47.6                 | 0.94                               | 3.97                                 | 10.584                        | 0.22                          | 0.90        | 0.13        | 49.0  | 10.59       | 0.23        | 0.92        |
| 16431592-4605409 | 338.934     | -0.062      | 28.212     | 8            | -          | -          | g           | -          | -           | -             | D1          | c                      | o            | -           | -           | h           | -           | 8.370  | ...                                | ...                         | 1                           | 81.8                 | 0.62                               | 4.80                                 | -2.142                        | ...                           | ...         | 8.74        | ...   | ...         | ...         | ...         |
| 16434955-3705384 | 345.821     | 5.748       | 1.031      | 1            | -          | -          | g           | -          | N           | -             | D2          | e                      | o            | -           | -           | V           | -           | 9.516  | 0.37                               | 1.37                        | 1                           | 68.8                 | 0.76                               | 4.25                                 | 9.132                         | 0.20                          | 0.86        | 0.32        | 74.5  | 9.15        | 0.22        | 0.93        |
| 16442139-5529372 | 331.916     | -6.333      | 0.351      | 1            | -          | -          | g           | -          | -           | -             | D1          | c                      | o            | -           | -           | h           | -           | 10.593 | 0.40                               | 1.21                        | 1                           | 42.4                 | 0.52                               | 4.15                                 | 10.462                        | 0.34                          | 1.03        | 0.11        | 43.3  | 10.47       | 0.34        | 1.06        |
| 16443791-6051053 | 327.802     | -9.813      | 0.257      | 1            | -          | -          | g           | -          | -           | -             | D1          | c                      | o            | -           | -           | h           | -           | 10.757 | 0.31                               | 1.09                        | 1                           | 59.6                 | 0.30                               | 3.92                                 | 10.661                        | 0.27                          | 0.96        | 0.08        | 60.5  | 10.67       | 0.27        | 0.98        |
| 16452293-5955252 | 328.585     | -9.291      | 0.188      | 1            | -          | -          | g           | -          | -           | -             | D1          | c                      | o            | -           | -           | h           | -           | 10.468 | 0.35                               | 1.11                        | 1                           | 61.8                 | 0.50                               | 3.99                                 | 10.398                        | 0.32                          | 1.01        | 0.06        | 62.3  | 10.41       | 0.32        | 1.03        |
| 16463421-3903086 | 344.676     | 4.067       | 1.002      | 1            | -          | -          | g           | -          | N           | -             | D1          | c                      | o            | -           | -           | h           | -           | 10.842 | 0.38                               | 1.40                        | 1                           | 34.8                 | 0.78                               | 4.46                                 | 10.469                        | 0.21                          | 0.90        | 0.31        | 38.0  | 10.47       | 0.23        | 0.97        |
| 16463543-3135214 | 350.436     | 8.859       | 0.432      | 1            | -          | -          | g           | -          | -           | -             | D1          | c                      | o            | -           | -           | V           | -           | 11.011 | 0.39                               | 1.24                        | 1                           | 42.8                 | 0.60                               | 4.10                                 | 10.850                        | 0.32                          | 1.03        | 0.13        | 44.2  | 10.85       | 0.33        | 1.05        |
| 16465670-3721166 | 346.025     | 5.106       | 0.940      | 1            | -          | -          | g           | -          | N           | -             | D2          | ea                     | o            | -           | -           | V           | -           | 10.402 | 0.45                               | 1.21                        | 1                           | 45.0                 | 0.60                               | 4.34                                 | 10.052                        | 0.29                          | 0.74        | 0.29        | 48.2  | 10.08       | 0.3         |             |

Table B1: a) continued.

| 2MASX J          |         | <i>l</i>    | <i>b</i>    | EBV        | Object       |            |            | Sample      |            |             | Disc 2MRS     |             | Velocity |              | NIR         | Photom      | Ext         | <i>K</i> <sub>20</sub> | <i>H-K</i>  | <i>J-K</i>  | <i>vc</i>   | <i>a</i> | <i>b/a</i> | std. | <i>K</i> <sub>S</sub> <sup>o</sup> | ( <i>H-K</i> ) <sup>o</sup> | ( <i>J-K</i> ) <sup>o</sup> | <i>A</i> <sub>K</sub> | <i>a</i> <sup>d</sup> | <i>K</i> <sub>S</sub> <sup>o,d</sup> | ( <i>H-K</i> ) <sup>o,c</sup> | ( <i>J-K</i> ) <sup>o,c</sup> |             |
|------------------|---------|-------------|-------------|------------|--------------|------------|------------|-------------|------------|-------------|---------------|-------------|----------|--------------|-------------|-------------|-------------|------------------------|-------------|-------------|-------------|----------|------------|------|------------------------------------|-----------------------------|-----------------------------|-----------------------|-----------------------|--------------------------------------|-------------------------------|-------------------------------|-------------|
| (1)              |         | deg<br>(2a) | deg<br>(2b) | mag<br>(3) | class<br>(4) | off<br>(5) | flg<br>(6) | gal<br>(7a) | TF<br>(7b) | obs<br>(7c) | ext'd<br>(7d) | type<br>(8) | (9)      | Opt<br>(10a) | HI<br>(10b) | flg<br>(11) | flg<br>(12) | flg<br>(13)            | mag<br>(14) | mag<br>(15) | mag<br>(16) | (17)     | (18)       | (19) | (20)                               | mag<br>(21)                 | mag<br>(22)                 | mag<br>(23)           | mag<br>(24)           | "<br>(25)                            | mag<br>(26)                   | mag<br>(27)                   | mag<br>(28) |
| 16541312-3227598 | 350.778 | 7.051       | -0.459      | 1          | -            | -          | -          | g           | -          | -           | -             | D2          | e        | o            | -           | V           | -           | -                      | 11.167      | 0.31        | 1.06        | 1        | 29.6       | 0.86 | 4.32                               | 10.996                      | 0.24                        | 0.83                  | 0.14                  | 30.4                                 | 11.01                         | 0.25                          | 0.86        |
| 16541460-4517282 | 340.783 | -1.012      | 50.119      | 9          | -            | -          | -          | -           | -          | -           | -             | -           | -        | -            | -           | -           | -           | -                      | 7.236       | ...         | ...         | 1        | 219.4      | 0.36 | 4.75                               | -11.438                     | ...                         | ...                   | ...                   | ...                                  | ...                           | ...                           |             |
| 16541902-4519002 | 340.766 | -1.032      | 42.994      | 9          | -            | -          | -          | -           | -          | -           | -             | -           | -        | -            | -           | -           | -           | -                      | 9.158       | ...         | ...         | 1        | 96.8       | 0.86 | 4.78                               | -6.862                      | ...                         | ...                   | 15.52                 | ...                                  | ...                           | ...                           |             |
| 16541764-4517122 | 340.792 | -1.016      | 52.104      | 9          | -            | -          | -          | -           | -          | -           | -             | -           | -        | -            | -           | -           | -           | -                      | 8.522       | ...         | ...         | 1        | 104.6      | 0.10 | 4.75                               | -10.892                     | ...                         | ...                   | 13.32                 | ...                                  | ...                           | ...                           |             |
| 16553517-3532460 | 348.535 | -0.808      | 1.909       | 1          | -            | -          | -          | -           | -          | N           | -             | D1          | -        | -            | -           | -           | -           | -                      | 11.304      | 0.39        | 1.29        | 1        | 27.8       | 0.52 | 4.45                               | 11.003                      | 0.25                        | 0.89                  | 0.25                  | 29.6                                 | 11.02                         | 0.27                          | 0.94        |
| 16560261-4304439 | 342.707 | 0.127       | 26.714      | 9          | -            | -          | -          | g           | -          | -           | -             | D1          | -        | -            | -           | -           | -           | -                      | 9.408       | ...         | ...         | 1        | 63.6       | 0.74 | 4.77                               | -0.546                      | ...                         | ...                   | 8.27                  | ...                                  | ...                           | ...                           |             |
| 16561212-2902288 | 353.761 | 8.836       | 0.219       | 1          | -            | -          | -          | g           | -          | P           | -             | D1          | ca       | -            | -           | -           | a           | -                      | 11.261      | 0.49        | 1.30        | 1        | 69.2       | 0.70 | 4.19                               | 11.179                      | 0.46                        | 1.19                  | 0.07                  | 70.1                                 | 11.18                         | 0.46                          | 1.21        |
| 16563986-4013290 | 345.006 | 1.822       | 26.222      | 9          | -            | -          | -          | -           | -          | -           | -             | -           | -        | -            | -           | -           | -           | -                      | 9.725       | ...         | ...         | 1        | 45.6       | 0.46 | 4.59                               | -0.045                      | ...                         | ...                   | 8.12                  | ...                                  | ...                           | ...                           |             |
| 16564248-3137161 | 351.776 | 7.161       | 0.326       | 1          | -            | -          | -          | g           | t          | -           | -             | D1          | e        | o            | h           | V           | -           | -                      | 9.500       | 0.28        | 1.02        | 1        | 90.2       | 0.44 | 4.35                               | 9.379                       | 0.23                        | 0.86                  | 0.10                  | 91.6                                 | 9.39                          | 0.24                          | 0.88        |
| 16564527-4014280 | 345.004 | 1.798       | 28.353      | 9          | -            | -          | -          | -           | -          | -           | -             | -           | -        | -            | -           | -           | -           | -                      | 9.794       | ...         | ...         | 1        | 48.8       | 0.60 | 4.59                               | -0.770                      | ...                         | ...                   | 8.78                  | ...                                  | ...                           | ...                           |             |
| 16565885-3443206 | 349.360 | 5.198       | 0.785       | 1          | -            | -          | -          | -           | -          | N           | -             | D1          | e        | o            | h           | V           | -           | -                      | 10.362      | 0.67        | 1.38        | 1        | 48.6       | 0.58 | 4.48                               | 10.070                      | 0.54                        | 0.99                  | 0.24                  | 51.5                                 | 10.08                         | 0.55                          | 1.04        |
| 16572692-3053505 | 352.449 | 7.482       | 0.385       | 1          | -            | -          | -          | g           | -          | -           | -             | D3          | e        | o            | -           | V           | -           | -                      | 11.109      | 0.29        | 1.11        | 1        | 30.2       | 0.72 | 4.32                               | 10.966                      | 0.22                        | 0.92                  | 0.12                  | 30.9                                 | 10.98                         | 0.23                          | 0.94        |
| 16574847-3438179 | 349.532 | 5.116       | 0.924       | 1          | -            | -          | -          | g           | -          | N           | -             | D2          | -        | -            | -           | -           | V           | -                      | 11.132      | 0.34        | 1.26        | 1        | 29.8       | 0.86 | 4.46                               | 10.781                      | 0.18                        | 0.80                  | 0.29                  | 32.1                                 | 10.79                         | 0.20                          | 0.86        |
| 16574897-4034050 | 344.875 | 1.436       | 12.470      | 9          | -            | -          | -          | -           | -          | -           | -             | -           | -        | -            | -           | -           | -           | -                      | 9.518       | ...         | ...         | 1        | 57.4       | 0.46 | 4.67                               | 4.872                       | ...                         | ...                   | 3.86                  | ...                                  | ...                           | ...                           |             |
| 16583028-2829088 | 354.518 | 8.776       | 0.268       | 1          | -            | -          | -          | g           | -          | N           | -             | D1          | c        | o            | h           | -           | -           | -                      | 10.158      | 0.29        | 1.03        | 1        | 63.8       | 0.56 | 4.25                               | 10.058                      | 0.25                        | 0.80                  | 0.08                  | 64.6                                 | 10.07                         | 0.25                          | 0.92        |
| 16592078-4232376 | 343.502 | -0.014      | 76.442      | 9          | -            | -          | -          | -           | -          | -           | -             | -           | -        | -            | -           | -           | -           | -                      | 8.693       | 1.48        | 3.18        | 1        | 44.2       | 0.54 | 4.78                               | -19.789                     | -11.18                      | -34.79                | 23.68                 | ...                                  | ...                           | -9.68                         | -29.75      |
| 16593051-4010419 | 345.380 | 1.425       | 50.156      | 9          | -            | -          | -          | -           | -          | -           | -             | -           | -        | -            | -           | -           | -           | -                      | 8.807       | ...         | ...         | 1        | 126.2      | 0.46 | 4.69                               | -9.881                      | ...                         | ...                   | 15.54                 | ...                                  | ...                           | ...                           |             |
| 16593198-3707279 | 347.788 | 3.306       | 1.699       | 9          | -            | -          | -          | -           | -          | -           | -             | -           | -        | -            | -           | -           | -           | -                      | 7.399       | 0.21        | 0.97        | 1        | 155.6      | 0.76 | 4.58                               | 6.766                       | -0.07                       | 0.12                  | 0.53                  | ...                                  | ...                           | -0.04                         | 0.24        |
| 16593668-4003251 | 345.488 | 1.484       | 47.446      | 9          | -            | -          | -          | -           | -          | -           | -             | -           | -        | -            | -           | -           | -           | -                      | 8.772       | 1.69        | 3.35        | 1        | 112.4      | 0.66 | 4.56                               | -8.906                      | -6.17                       | -20.22                | 14.70                 | ...                                  | ...                           | -5.24                         | -17.09      |
| 16593754-4005271 | 345.463 | 1.461       | 47.196      | 9          | -            | -          | -          | -           | -          | -           | -             | -           | -        | -            | -           | -           | -           | -                      | 8.756       | 1.54        | 2.69        | 1        | 133.8      | 0.70 | 4.56                               | -8.829                      | -6.27                       | -20.76                | 14.62                 | ...                                  | ...                           | -5.35                         | -17.64      |
| 16594225-4003451 | 345.494 | 1.467       | 47.737      | 9          | -            | -          | -          | -           | -          | -           | -             | -           | -        | -            | -           | -           | -           | -                      | 7.354       | 2.35        | ...         | 1        | 208.2      | 0.78 | 4.56                               | -10.433                     | -5.56                       | ...                   | 14.79                 | ...                                  | ...                           | -4.62                         | ...         |
| 16594625-4004141 | 345.496 | 1.452       | 48.513      | 9          | -            | -          | -          | -           | -          | -           | -             | -           | -        | -            | -           | -           | -           | -                      | 9.120       | ...         | ...         | 1        | 109.8      | 0.30 | 4.56                               | -8.956                      | ...                         | ...                   | 15.03                 | ...                                  | ...                           | ...                           | ...         |
| 17000638-3152265 | 352.021 | 6.436       | 0.514       | 1          | -            | -          | -          | g           | -          | -           | -             | D3          | e        | o            | -           | V           | -           | -                      | 10.346      | 0.32        | 1.11        | 1        | 53.0       | 0.68 | 4.46                               | 10.154                      | 0.24                        | 0.85                  | 0.16                  | 54.7                                 | 10.17                         | 0.25                          | 0.88        |
| 17000944-4922154 | 338.210 | -4.336      | 0.891       | 3          | -            | -          | -          | g           | -          | P           | -             | D3          | -        | -            | -           | -           | -           | -                      | 10.800      | 0.70        | 1.36        | 1        | 29.8       | 0.78 | 4.45                               | 10.468                      | 0.55                        | 0.92                  | 0.28                  | 31.8                                 | 10.49                         | 0.57                          | 0.98        |
| 17003381-4034210 | 345.194 | 1.023       | 34.112      | 9          | -            | -          | -          | -           | -          | -           | -             | -           | -        | -            | -           | -           | -           | -                      | 7.956       | 1.29        | 3.17        | 1        | 219.6      | 0.14 | 4.63                               | -4.754                      | -4.36                       | -13.78                | 10.57                 | ...                                  | ...                           | -3.69                         | -11.53      |
| 17003600-4033300 | 345.209 | 1.027       | 38.399      | 9          | -            | -          | -          | -           | -          | -           | -             | -           | -        | -            | -           | -           | -           | -                      | 6.755       | 1.49        | 3.30        | 1        | 116.4      | 0.84 | 4.63                               | -7.552                      | -4.86                       | -15.78                | 11.89                 | ...                                  | ...                           | -4.11                         | -13.24      |
| 17003615-2826461 | 354.833 | 8.434       | 0.294       | 2          | -            | -          | -          | g           | -          | -           | -             | n           | c        | o            | -           | -           | -           | -                      | 11.298      | 0.38        | 1.08        | 1        | 28.6       | 0.68 | 4.29                               | 11.188                      | 0.33                        | 0.94                  | 0.09                  | 29.1                                 | 11.20                         | 0.33                          | 0.96        |
| 17003811-4032379 | 345.225 | 1.030       | 43.257      | 9          | -            | -          | -          | -           | -          | -           | -             | -           | -        | -            | -           | -           | -           | -                      | 7.708       | 1.45        | 3.32        | 1        | 105.2      | 0.78 | 4.63                               | -8.410                      | -5.72                       | -18.17                | 13.40                 | ...                                  | ...                           | -4.87                         | -15.31      |
| 17005453-2839511 | 354.698 | 8.248       | 0.297       | 1          | -            | -          | -          | g           | -          | -           | -             | n           | c        | o            | -           | -           | -           | -                      | 10.552      | 0.35        | 1.05        | 1        | 42.0       | 0.90 | 4.29                               | 10.441                      | 0.30                        | 0.90                  | 0.09                  | 42.6                                 | 10.45                         | 0.30                          | 0.92        |
| 17010271-2606596 | 356.776 | 7.758       | 0.305       | 1          | -            | -          | -          | g           | t          | -           | -             | D1          | c        | o            | h           | V           | -           | -                      | 10.650      | 0.30        | 1.05        | 1        | 68.8       | 0.24 | 4.12                               | 10.536                      | 0.25                        | 0.90                  | 0.09                  | 70.0                                 | 10.54                         | 0.26                          | 0.92        |
| 17010747-3006484 | 353.562 | 7.334       | 0.451       | 9          | -            | -          | -          | -           | -          | -           | -             | -           | -        | -            | -           | -           | -           | -                      | 7.712       | ...         | ...         | 1        | 85.6       | 1.00 | 4.55                               | 7.544                       | ...                         | ...                   | 0.14                  | ...                                  | ...                           | ...                           |             |
| 17010783-2804046 | 355.208 | 8.569       | 0.293       | 1          | -            | -          | -          | g           | t          | N           | -             | D1          | c        | o            | h?          | -           | -           | -                      | 10.647      | 0.31        | 1.11        | 1        | 54.2       | 0.42 | 4.28                               | 10.538                      | 0.27                        | 0.96                  | 0.09                  | 55.0                                 | 10.55                         | 0.27                          | 0.98        |
| 17011125-3006494 | 353.570 | 7.323       | 0.457       | 9          | -            | -          | -          | -           | -          | -           | -             | -           | -        | -            | -           | -           | -           | -                      | 7.653       | 0.23        | 1.06        | 1        | 10.0       | 0.92 | 4.55                               | 7.483                       | 0.16                        | 0.83                  | 0.14                  | ...                                  | ...                           | 0.17                          | 0.86        |
| 17011171-3007364 | 353.561 | 7.313       | 0.465       | 9          | -            | -          | -          | -           | -          | -           | -             | -           | -        | -            | -           | -           | -           | -                      | 5.971       | 0.23        | 0.61        | 1        | 219.2      | 0.70 | 4.55                               | 5.798                       | 0.16                        | 0.38                  | 0.14                  | ...                                  | ...                           | 0.17                          | 0.41        |
| 17011456-3006224 | 353.884 | 7.318       | 0.458       | 9          | -            | -          | -          | -           | -          | -           | -             | -           | -        | -            | -           | -           | -           | -                      | 5.132       | 0.46        | 0.92        | 1        | 218.6      | 0.86 | 4.55                               | 4.961                       | 0.38                        | 0.70                  | 0.14                  | ...                                  | ...                           | 0.39                          | 0.73        |
| 17012142-2834026 | 354.586 | 8.228       | 0.304       | 1          | -            | -          | -          | g           | -          | -           | -             | n           | c        | o            | -           | -           | -           | -                      | 10.453      | 0.35        | 1.03        | 1        | 44.0       | 0.82 | 4.31                               | 10.340                      | 0.30                        | 0.88                  | 0.09                  | 44.7                                 | 10.35                         | 0.30                          | 0.90        |
| 17014392-2834388 | 354.878 | 8.156       | 0.331       | 2          | -            | -          | -          | g           | -          | -           | -             | n           | c        | o            | -           | -           | -           | -                      | 11.181      | 0.28        | 1.03        | 1        | 32.0       | 0.82 | 4.32                               | 11.058                      | 0.22                        | 0.86                  | 0.10                  | 32.6                                 | 11.07                         | 0.23                          | 0.88        |
| 17022242-4831436 | 339.102 | -4.109      | 0.954       | 2          | -            | -          | -          | g           | +          | -           | -             | -           | -        | -            | -           | -           | -           | -                      | 11.382      | 0.39        | ...         | 1        | 32.8       | 0.68 | 4.47                               | 11.027                      | 0.23                        | ...                   | 0.30                  | 35.5                                 | 11.04                         | 0.25                          | ...         |
| 17023725-2615554 | 356.870 | 9.386       | 0.313       | 9          | -            | -          | -          | -           | -          | -           | -             | -           | -        | -            | -           | -           | -           | -                      | 5.507       | 0.16        | 0.81        | 1        | 62.0       | 0.9  | 4.35                               | 5.390                       | 0.11                        | 0.66                  | 0.10                  | ...                                  | ...                           | 0.12                          | 0.68        |
| 17023762-2616264 | 356.864 | 9.379       | 0.313       | 9          | -            | -          | -          | -           | -          | -           | -             | -           | -        | -            | -           | -           | -           | -                      | 5.843       | 0.16        | 0.76        | 1        | 65.6       | 0.11 | 4.35                               | 5.726                       | 0.11                        | 0.61                  | 0.10                  | ...                                  | ...                           | 0.11                          | 0.63        |
| 17024267-2616414 | 356.872 | 9.362       | 0.319       | 9          | -            | -          | -          | -           | -          | -           | -             | -           | -        | -            | -           | -           | -           | -                      | 8.576       | 0.19        | 0.69        | 1        | 57.8       | 0.54 | 4.35                               | 8.457                       | 0.13                        | 0.53                  | 0.10                  | ...                                  | ...                           | 0.14                          | 0.55        |
| 17024654-3405128 | 350.600 | 4.644       | 0.623       | 2          | -            | -          | -          | g           | -          | N           | -             | D2          | -        | -            | -           | V           | -           | -                      | 10.995      | ...         | ...         | 1        | 27.2       | 0.80 | 4.62                               | 10.763                      | ...                         | ...                   | 0.19                  | 28.4                                 | 10.78                         | ...                           | ...         |
| 17024728-2616174 | 356.887 | 9.352       | 0.325       | 9          | -            | -          | -          | -           | -          | -           | -             | -           | -        | -            | -           | -           | -           | -                      | 9.902       | 0.13        | 0.51        | 1        | 96.0       | 0.78 | 4.35                               | 9.781                       | 0.07                        | 0.35                  | 0.10                  | ...                                  | ...                           | 0.08                          | 0.37        |
| 17025135-5247076 | 335.748 | -6.751      | 0.377       | 1          | -            | -          | -          | g           | -          | -           | -             | D2          | e        | o            | -           | V           | -           | -                      | 10.857      | 0.38        | 1.23        | 1        | 36.2       | 0.88 | 4.14                               | 10.717                      | 0.32                        | 1.04                  | 0.12                  | 37.0                                 | 10.73                         | 0.33                          | 1.07        |
| 17032172-2920268 | 354.479 | 7.412       | 0.296       | 1          | -            | -          | -          | g           | -          | D1          | e             | o           | -        | -            | -           | -           | -           | -                      | 11.154      | 0.31        | 1.13        | 1        | 36.6       | 0.54 | 4.43                               | 11.044                      | 0.26                        | 0.98                  | 0.09                  | 37.2                                 | 11.05                         | 0.27                          | 1.00        |
| 17033276-2905047 | 354.710 | 7.534       | 0.280       | 1          | -            | -          | -</        |             |            |             |               |             |          |              |             |             |             |                        |             |             |             |          |            |      |                                    |                             |                             |                       |                       |                                      |                               |                               |             |

Table B1: a) continued.

| 2MASX J          | <i>l</i> | <i>b</i> | EBV   | Object | Sample | Disc | 2MRS | Velocity | NIR  | Photom | Ext   | <i>K</i> <sub>20</sub> | <i>H-K</i> | <i>J-K</i> | vc   | <i>a</i> | <i>b/a</i> | st.d. | <i>K</i> <sub>s</sub> <sup>o</sup> | ( <i>H-K</i> ) <sup>o</sup> | ( <i>J-K</i> ) <sup>o</sup> | <i>A</i> <sub>K</sub> | <i>a</i> <sub>d</sub> <sup>o</sup> | <i>K</i> <sub>s</sub> <sup>o,d</sup> | ( <i>H-K</i> ) <sup>o,c</sup> | ( <i>J-K</i> ) <sup>o,c</sup> |       |       |      |       |       |      |       |
|------------------|----------|----------|-------|--------|--------|------|------|----------|------|--------|-------|------------------------|------------|------------|------|----------|------------|-------|------------------------------------|-----------------------------|-----------------------------|-----------------------|------------------------------------|--------------------------------------|-------------------------------|-------------------------------|-------|-------|------|-------|-------|------|-------|
| (1)              | deg      | deg      | mag   | class  | off    | flg  | gal  | TF       | (7b) | (7c)   | ext'd | type                   | Opt        | HI         | vc   | "        | "          | "     | mag                                | mag                         | mag                         | mag                   | "                                  | mag                                  | mag                           | mag                           |       |       |      |       |       |      |       |
| (1)              | (2a)     | (2b)     | (3)   | (4)    | (5)    | (6)  | (7a) | (7b)     | (7c) | (7d)   | (8)   | (9)                    | (10a)      | (10b)      | (17) | (18)     | (19)       | (20)  | (21)                               | (22)                        | (23)                        | (24)                  | (25)                               | (26)                                 | (27)                          | (28)                          |       |       |      |       |       |      |       |
| 17101163−4705168 | 341.047  | −4.295   | 1.238 | 1      | —      | —    | g    | t        | P    | —      | —     | D1                     | —          | —          | *    | —        | —          | —     | 11.248                             | 0.48                        | ...                         | 1                     | 36.6                               | 0.42                                 | 4.41                          | 10.787                        | 0.28  | ...   | 0.38 | 41.1  | 10.78 | 0.30 | ...   |
| 17110675−4552503 | 342.118  | −3.710   | 5.964 | 9      | —      | —    | —    | —        | —    | —      | —     | —                      | —          | —          | —    | —        | —          | —     | 9.014                              | 1.76                        | ...                         | 1                     | 104.8                              | 0.58                                 | 4.44                          | 6.792                         | 0.77  | ...   | 1.85 | ...   | ...   | 0.89 | ...   |
| 17112078−2234457 | 1.080    | 9.934    | 0.710 | 1      | —      | —    | —    | —        | —    | —      | —     | D4                     | c          | o          | —    | —        | —          | —     | 10.553                             | 0.41                        | 1.26                        | 1                     | 42.8                               | 0.90                                 | 4.09                          | 10.288                        | 0.30  | 0.91  | 0.22 | 44.9  | 10.31 | 0.31 | 0.95  |
| 17112119−2318497 | 0.471    | 9.510    | 0.608 | 1      | —      | —    | —    | —        | —    | —      | —     | D1                     | c          | o          | —    | —        | —          | —     | 10.725                             | 0.38                        | 1.20                        | 1                     | 46.0                               | 0.46                                 | 4.19                          | 10.498                        | 0.28  | 0.89  | 0.19 | 47.9  | 10.51 | 0.29 | 0.94  |
| 17112442−2452438 | 359.184  | 8.597    | 0.801 | 1      | —      | —    | —    | —        | —    | —      | —     | D3                     | c          | o          | —    | —        | —          | V     | 11.385                             | 0.40                        | 1.35                        | 1                     | 24.4                               | 0.74                                 | 4.26                          | 11.087                        | 0.27  | 0.95  | 0.25 | 25.9  | 11.10 | 0.28 | 1.00  |
| 17113574−2413554 | 359.744  | 8.936    | 0.627 | 1      | —      | —    | —    | —        | —    | —      | —     | D4                     | c          | o          | —    | —        | —          | —     | 11.067                             | 0.39                        | 1.28                        | 1                     | 25.2                               | 0.62                                 | 4.24                          | 10.833                        | 0.29  | 0.96  | 0.19 | 26.3  | 10.85 | 0.30 | 1.01  |
| 17113598−2303057 | 0.722    | 9.615    | 0.649 | 1      | —      | —    | —    | —        | —    | —      | —     | D1                     | c          | o          | —    | —        | —          | —     | 11.345                             | 0.34                        | 1.19                        | 1                     | 40.0                               | 0.60                                 | 4.16                          | 11.103                        | 0.24  | 0.86  | 0.20 | 42.1  | 11.11 | 0.25 | 0.91  |
| 17113750−2258457 | 0.785    | 9.652    | 0.619 | 2      | —      | —    | —    | —        | —    | —      | —     | D3                     | c          | o          | —    | —        | —          | —     | 11.229                             | 0.42                        | 1.22                        | 1                     | 32.0                               | 0.54                                 | 4.16                          | 10.998                        | 0.32  | 0.91  | 0.19 | 33.4  | 11.01 | 0.33 | 0.95  |
| 17114071−3210252 | 353.256  | 4.292    | 0.855 | 1      | —      | —    | —    | N        | —    | —      | —     | D3                     | c          | o          | —    | —        | —          | V     | 9.763                              | 0.32                        | ...                         | 1                     | 52.8                               | 0.94                                 | 4.81                          | 9.444                         | 0.18  | ...   | 0.26 | 56.1  | 9.47  | 0.19 | ...   |
| 17114409−2303397 | 0.732    | 9.584    | 0.653 | 1      | —      | —    | —    | —        | —    | —      | —     | D2                     | c          | o          | —    | —        | —          | —     | 10.705                             | 0.35                        | 1.14                        | 1                     | 42.8                               | 0.82                                 | 4.16                          | 10.462                        | 0.24  | 0.82  | 0.20 | 44.8  | 10.48 | 0.26 | 0.86  |
| 17114504−2544504 | 358.514  | 8.031    | 0.494 | 1      | —      | —    | —    | t        | —    | —      | —     | D1                     | c          | o          | —    | —        | —          | V     | 10.454                             | 0.39                        | 1.24                        | 1                     | 82.4                               | 0.22                                 | 4.40                          | 10.270                        | 0.31  | 1.00  | 0.15 | 85.2  | 10.28 | 0.32 | 1.03  |
| 17114534−2308447 | 0.665    | 9.531    | 0.639 | 2      | —      | —    | —    | —        | —    | —      | —     | n                      | c          | o          | —    | —        | —          | —     | 11.370                             | 0.35                        | 1.20                        | 1                     | 20.8                               | 0.58                                 | 4.16                          | 11.132                        | 0.25  | 0.88  | 0.20 | 21.7  | 11.15 | 0.26 | 0.93  |
| 17115130−2301363 | 0.777    | 9.581    | 0.629 | 1      | —      | —    | —    | —        | —    | —      | —     | D4                     | c          | o          | —    | —        | —          | —     | 10.905                             | 0.32                        | 1.20                        | 1                     | 30.8                               | 0.92                                 | 4.21                          | 10.671                        | 0.21  | 0.89  | 0.19 | 32.1  | 10.69 | 0.23 | 0.93  |
| 17115542−2309423 | 0.674    | 9.491    | 0.649 | 1      | —      | —    | —    | —        | —    | —      | —     | D3                     | c          | o          | —    | —        | —          | —     | 10.754                             | 0.34                        | 1.22                        | 1                     | 46.2                               | 0.60                                 | 4.21                          | 10.512                        | 0.23  | 0.90  | 0.20 | 48.4  | 10.52 | 0.25 | 0.94  |
| 17115724−2302113 | 0.782    | 9.557    | 0.634 | 1      | —      | —    | —    | —        | —    | —      | —     | D4                     | c          | o          | —    | —        | —          | —     | 10.826                             | 0.32                        | 1.18                        | 1                     | 29.6                               | 0.96                                 | 4.21                          | 10.590                        | 0.22  | 0.87  | 0.20 | 30.9  | 10.61 | 0.23 | 0.91  |
| 17115865−2438004 | 359.463  | 8.633    | 0.686 | 1      | —      | —    | —    | —        | —    | —      | —     | D4                     | c          | o          | —    | —        | —          | —     | 11.092                             | 0.36                        | 1.25                        | 1                     | 26.2                               | 1.00                                 | 4.29                          | 10.836                        | 0.25  | 0.91  | 0.21 | 27.5  | 10.85 | 0.26 | 0.95  |
| 17121895−2322192 | 0.552    | 9.296    | 0.595 | 2      | —      | —    | —    | —        | —    | —      | —     | n                      | c          | o          | —    | —        | —          | —     | 11.344                             | 0.30                        | 1.19                        | 1                     | 22.6                               | 0.82                                 | 4.23                          | 11.122                        | 0.20  | 0.89  | 0.18 | 23.5  | 11.14 | 0.21 | 0.93  |
| 17121976−2315418 | 0.645    | 9.357    | 0.573 | 2      | —      | —    | —    | —        | —    | —      | —     | n                      | c          | o          | —    | —        | —          | —     | 11.368                             | 0.34                        | 1.16                        | 1                     | 24.4                               | 0.96                                 | 4.26                          | 11.155                        | 0.24  | 0.88  | 0.18 | 25.4  | 11.17 | 0.25 | 0.91  |
| 17121989−2324187 | 0.526    | 9.274    | 0.595 | 1      | —      | —    | —    | —        | —    | —      | —     | D3                     | c          | o          | —    | —        | —          | —     | 11.167                             | 0.33                        | 1.21                        | 1                     | 33.0                               | 0.64                                 | 4.26                          | 10.945                        | 0.23  | 0.92  | 0.18 | 34.4  | 10.96 | 0.24 | 0.96  |
| 17122070−2318318 | 0.608    | 9.327    | 0.581 | 1      | —      | —    | —    | —        | —    | —      | —     | n                      | c          | o          | —    | —        | —          | —     | 11.012                             | 0.36                        | 1.19                        | 1                     | 31.6                               | 0.82                                 | 4.26                          | 10.796                        | 0.26  | 0.91  | 0.18 | 32.8  | 10.81 | 0.27 | 0.94  |
| 17122085−2310048 | 0.725    | 9.407    | 0.624 | 1      | —      | —    | —    | t        | —    | —      | —     | D2                     | c          | o          | —    | —        | —          | —     | 11.330                             | 0.42                        | 1.24                        | 1                     | 35.8                               | 0.42                                 | 4.22                          | 11.097                        | 0.32  | 0.93  | 0.19 | 37.5  | 11.11 | 0.33 | 0.98  |
| 17122113−2329568 | 0.451    | 9.216    | 0.592 | 2      | —      | —    | —    | —        | —    | —      | —     | n                      | c          | o          | —    | —        | —          | —     | 11.244                             | 0.44                        | 1.20                        | 1                     | 26.8                               | 0.86                                 | 4.26                          | 11.023                        | 0.34  | 0.91  | 0.18 | 27.9  | 11.04 | 0.35 | 0.94  |
| 17122214−2326048 | 0.507    | 9.250    | 0.592 | 1      | —      | —    | —    | —        | —    | —      | —     | D2                     | c          | o          | —    | —        | —          | —     | 11.100                             | 0.39                        | 1.21                        | 1                     | 29.8                               | 0.56                                 | 4.26                          | 10.879                        | 0.29  | 0.91  | 0.18 | 31.0  | 10.89 | 0.30 | 0.95  |
| 17122357−2447566 | 359.381  | 8.461    | 0.791 | 1      | —      | —    | —    | t        | N    | —      | —     | D1                     | c          | o          | —    | —        | —          | V     | 11.291                             | 0.47                        | 1.41                        | 1                     | 43.8                               | 0.34                                 | 4.32                          | 10.996                        | 0.34  | 1.01  | 0.25 | 46.7  | 11.00 | 0.35 | 1.07  |
| 17122774−2322108 | 0.573    | 9.270    | 0.592 | 1      | —      | —    | —    | —        | —    | —      | —     | D1                     | c          | o          | —    | —        | —          | —     | 9.146                              | 0.34                        | 1.11                        | 1                     | 100.8                              | 0.70                                 | 4.26                          | 8.925                         | 0.24  | 0.81  | 0.18 | 105.5 | 8.93  | 0.25 | 0.85  |
| 17123170−2512066 | 359.066  | 8.203    | 0.718 | 1      | —      | —    | —    | —        | —    | —      | —     | D2                     | c          | o          | —    | —        | —          | V     | 11.380                             | 0.41                        | 1.31                        | 1                     | 33.4                               | 0.76                                 | 4.37                          | 11.112                        | 0.29  | 0.96  | 0.22 | 35.3  | 11.12 | 0.30 | 1.00  |
| 17123325−2307348 | 0.788    | 9.392    | 0.631 | 1      | —      | —    | —    | —        | —    | —      | —     | D1                     | c          | o          | —    | —        | —          | —     | 10.892                             | 0.32                        | 1.14                        | 1                     | 44.0                               | 0.82                                 | 4.22                          | 10.657                        | 0.22  | 0.82  | 0.20 | 46.1  | 10.67 | 0.23 | 0.87  |
| 17123572−2548136 | 358.579  | 7.843    | 0.573 | 1      | —      | —    | —    | t        | N    | —      | —     | D1                     | e          | o          | —    | —        | —          | —     | 10.957                             | 0.34                        | 1.17                        | 1                     | 34.8                               | 0.46                                 | 4.42                          | 10.743                        | 0.25  | 0.89  | 0.18 | 36.1  | 10.76 | 0.26 | 0.93  |
| 17123633−2506425 | 359.151  | 8.241    | 0.803 | 1      | —      | —    | —    | —        | —    | —      | —     | D1                     | e          | o          | —    | —        | —          | V     | 10.797                             | 0.18                        | 1.13                        | 1                     | 52.4                               | 0.58                                 | 4.33                          | 10.498                        | 0.05  | 0.73  | 0.25 | 56.2  | 10.49 | 0.07 | 0.79  |
| 17124256−2324167 | 0.577    | 9.203    | 0.579 | 2      | —      | —    | —    | —        | —    | —      | —     | D3                     | c          | o          | —    | —        | —          | —     | 11.116                             | 0.39                        | 1.20                        | 1                     | 23.4                               | 0.74                                 | 4.26                          | 10.900                        | 0.29  | 0.91  | 0.18 | 24.3  | 10.92 | 0.30 | 0.95  |
| 17124278−2435477 | 359.590  | 8.518    | 0.684 | 1      | —      | —    | —    | —        | —    | —      | —     | D1                     | c          | o          | —    | —        | —          | —     | 9.977                              | 0.34                        | 1.13                        | 1                     | 57.8                               | 0.94                                 | 4.25                          | 9.722                         | 0.23  | 0.79  | 0.21 | 60.6  | 9.74  | 0.24 | 0.84  |
| 17124957−2307207 | 0.827    | 9.343    | 0.602 | 2      | —      | —    | —    | —        | —    | —      | —     | n                      | c          | o          | —    | —        | —          | —     | 11.082                             | 0.43                        | 1.26                        | 1                     | 27.2                               | 0.74                                 | 4.22                          | 10.858                        | 0.33  | 0.96  | 0.19 | 28.3  | 10.87 | 0.34 | 1.00  |
| 17125134−2415096 | 359.894  | 8.689    | 0.659 | 1      | —      | —    | —    | —        | —    | —      | —     | D3                     | c          | o          | —    | —        | —          | —     | 10.962                             | 0.37                        | 1.26                        | 1                     | 34.4                               | 0.74                                 | 4.25                          | 10.716                        | 0.26  | 0.93  | 0.20 | 36.0  | 10.73 | 0.27 | 0.97  |
| 17125506−2257000 | 0.983    | 9.425    | 0.612 | 1      | —      | —    | —    | t        | —    | —      | —     | D1                     | c          | o          | —    | —        | —          | —     | 11.415                             | 0.46                        | 1.30                        | 1                     | 45.8                               | 0.28                                 | 4.21                          | 11.187                        | 0.36  | 0.99  | 0.19 | 48.1  | 11.19 | 0.37 | 1.03  |
| 17131541−2502266 | 359.295  | 8.161    | 0.760 | 1      | —      | —    | —    | —        | —    | —      | —     | D3                     | c          | o          | —    | —        | —          | V     | 10.261                             | 0.34                        | 1.26                        | 1                     | 45.8                               | 0.96                                 | 4.33                          | 9.978                         | 0.22  | 0.88  | 0.24 | 48.3  | 10.00 | 0.23 | 0.93  |
| 17131749−2334290 | 0.514    | 8.997    | 0.532 | 1      | —      | —    | —    | —        | —    | —      | —     | D4                     | c          | o          | —    | —        | —          | —     | 10.719                             | 0.35                        | 1.14                        | 1                     | 46.8                               | 0.58                                 | 4.26                          | 10.521                        | 0.26  | 0.88  | 0.16 | 48.4  | 10.54 | 0.27 | 0.91  |
| 17132420−2339146 | 0.463    | 8.930    | 0.551 | 2      | —      | —    | —    | —        | —    | —      | —     | n                      | c          | o          | —    | —        | —          | —     | 11.345                             | 0.34                        | 1.19                        | 1                     | 24.8                               | 0.58                                 | 4.26                          | 11.140                        | 0.25  | 0.92  | 0.17 | 25.7  | 11.15 | 0.26 | 0.95  |
| 17134463−3706111 | 349.509  | 1.055    | 5.424 | 8      | —      | —    | p?   | —        | —    | —      | —     | —                      | —          | —          | —    | —        | —          | —     | 7.644                              | 0.83                        | 1.22                        | 1                     | 110.6                              | 0.72                                 | 4.88                          | 5.623                         | −0.07 | −1.47 | 1.68 | ...   | ...   | 0.04 | −1.12 |
| 17140156−2448551 | 359.583  | 8.148    | 0.809 | 1      | —      | —    | —    | —        | —    | —      | —     | D3                     | c          | o          | —    | —        | —          | U     | 10.677                             | 0.35                        | 1.13                        | 1                     | 42.8                               | 0.58                                 | 4.31                          | 10.376                        | 0.21  | 0.73  | 0.25 | 45.6  | 10.39 | 0.23 | 0.78  |
| 17140172−2313026 | 0.908    | 9.062    | 0.519 | 1      | —      | —    | —    | —        | —    | —      | —     | n                      | c          | o          | —    | —        | —          | —     | 10.856                             | 0.39                        | 1.14                        | 1                     | 36.4                               | 0.74                                 | 4.29                          | 10.663                        | 0.31  | 0.89  | 0.16 | 37.6  | 10.68 | 0.32 | 0.92  |
| 17140971−2331536 | 0.665    | 8.858    | 0.589 | 1      | —      | —    | —    | t        | —    | —      | —     | D1                     | c          | o          | —    | —        | —          | h     | 10.554                             | 0.39                        | 1.29                        | 1                     | 71.4                               | 0.28                                 | 4.30                          | 10.335                        | 0.29  | 1.00  | 0.18 | 74.2  | 10.35 | 0.30 | 1.04  |
| 17142031−2134406 | 2.317    | 9.936    | 0.973 | 1      | —      | —    | —    | —        | —    | —      | —     | D1                     | c          |            |      |          |            |       |                                    |                             |                             |                       |                                    |                                      |                               |                               |       |       |      |       |       |      |       |

Table B1: a) continued.

| 2MASX J          | <i>l</i>    | <i>b</i>    | EBV        | Object       | Sample     | Disc        | 2MRS        | Velocity   | NIR         | Photom        | Ext         | <i>K</i> <sub>20</sub> | <i>H-K</i>   | <i>J-K</i>  | vc           | <i>a</i>     | <i>b/a</i>   | st.d. | <i>K</i> <sub>s</sub> <sup>o</sup> | ( <i>H-K</i> ) <sup>o</sup> | ( <i>J-K</i> ) <sup>o</sup> | <i>A</i> <sub>K</sub> | <i>a</i> <sub>d</sub> <sup>o</sup> | <i>K</i> <sub>s</sub> <sup>o,d</sup> | ( <i>H-K</i> ) <sup>o,c</sup> | ( <i>J-K</i> ) <sup>o,c</sup> |             |             |       |             |             |             |        |
|------------------|-------------|-------------|------------|--------------|------------|-------------|-------------|------------|-------------|---------------|-------------|------------------------|--------------|-------------|--------------|--------------|--------------|-------|------------------------------------|-----------------------------|-----------------------------|-----------------------|------------------------------------|--------------------------------------|-------------------------------|-------------------------------|-------------|-------------|-------|-------------|-------------|-------------|--------|
| (1)              | deg<br>(2a) | deg<br>(2b) | mag<br>(3) | class<br>(4) | off<br>(5) | flag<br>(6) | gal<br>(7a) | TF<br>(7b) | obs<br>(7c) | ext'd<br>(7d) | type<br>(8) | (9)                    | Opt<br>(10a) | HI<br>(10b) | flag<br>(11) | flag<br>(12) | flag<br>(13) | (14)  | mag<br>(15)                        | mag<br>(16)                 | (17)                        | (18)                  | (19)                               | (20)                                 | mag<br>(21)                   | mag<br>(22)                   | mag<br>(23) | mag<br>(24) | (25)  | mag<br>(26) | mag<br>(27) | mag<br>(28) |        |
| 17184154–2750144 | 357.688     | 5.563       | 1.213      | 1            | –          | –           | g           | –          | N           | –             | D2          | –                      | o            | *           | –            | –            | –            | –     | 10.392                             | ...                         | ...                         | 1                     | 41.8                               | 0.66                                 | 4.80                          | 9.940                         | ...         | ...         | 0.38  | 46.2        | 9.96        | ...         | ...    |
| 17191552–3904324 | 348.531     | –0.972      | 19.057     | 8            | –          | –           | –           | –          | –           | –             | –           | –                      | –            | –           | –            | –            | –            | –     | 8.795                              | 1.42                        | ...                         | 1                     | 70.0                               | 0.74                                 | 4.77                          | 1.694                         | –1.73       | ...         | 5.90  | ...         | ...         | –1.36       | ...    |
| 17192058–3903543 | 348.549     | –0.980      | 20.727     | 8            | –          | –           | –           | –          | –           | –             | –           | –                      | –            | –           | –            | –            | –            | –     | 9.536                              | ...                         | ...                         | 1                     | 36.4                               | 0.40                                 | 4.77                          | 1.813                         | ...         | ...         | 6.42  | ...         | ...         | ...         | ...    |
| 17192369–4555271 | 342.919     | –4.910      | 0.594      | 1            | –          | –           | g           | t          | –           | –             | D1          | –                      | o            | h           | –            | –            | –            | –     | 10.429                             | 0.30                        | 1.19                        | 1                     | 61.6                               | 0.46                                 | 4.43                          | 10.208                        | 0.20        | 0.90        | 0.18  | 64.2        | 10.22       | 0.21        | 0.94   |
| 17194814–2528040 | 359.792     | 6.702       | 0.963      | 1            | –          | –           | g           | t          | N           | –             | D1          | e                      | o            | –           | –            | –            | –            | –     | 11.140                             | 0.81                        | ...                         | 1                     | 28.6                               | 0.50                                 | 4.61                          | 10.781                        | 0.15        | ...         | 0.30  | 31.0        | 10.79       | 0.17        | ...    |
| 17195582–3900424 | 348.658     | –1.043      | 44.397     | 8            | –          | –           | –           | –          | –           | –             | –           | –                      | –            | –           | –            | –            | –            | –     | 9.141                              | 0.97                        | 2.19                        | 1                     | 69.2                               | 0.74                                 | 4.74                          | –7.401                        | –6.38       | –19.87      | 13.75 | ...         | ...         | –5.51       | –16.94 |
| 17200115–3558069 | 351.164     | 0.684       | 87.080     | 9            | –          | –           | –           | –          | –           | –             | –           | –                      | –            | –           | –            | –            | –            | –     | 7.057                              | 1.26                        | ...                         | –2                    | 164.0                              | 0.36                                 | 4.68                          | –25.389                       | –13.16      | ...         | 26.97 | ...         | ...         | –11.45      | ...    |
| 17200305–3556019 | 351.196     | 0.699       | 99.441     | 9            | –          | –           | –           | –          | –           | –             | –           | –                      | –            | –           | –            | –            | –            | –     | 6.551                              | 1.33                        | 2.74                        | 1                     | 218.4                              | 0.40                                 | 4.68                          | –30.501                       | –15.14      | –46.66      | 30.80 | ...         | ...         | –13.19      | –40.10 |
| 17200331–3858039 | 348.708     | –1.037      | 67.355     | 9            | –          | –           | –           | –          | –           | –             | –           | –                      | –            | –           | –            | –            | –            | –     | 7.171                              | 1.29                        | 2.26                        | 1                     | 112.4                              | 0.66                                 | 4.71                          | –17.925                       | –9.87       | –31.20      | 20.86 | ...         | ...         | –8.55       | –26.75 |
| 17200631–3615129 | 350.940     | 0.507       | 15.039     | 9            | –          | –           | –           | –          | –           | –             | –           | –                      | –            | –           | –            | –            | –            | –     | 9.165                              | 1.60                        | ...                         | –2                    | 25.6                               | 0.76                                 | 4.75                          | 3.561                         | –0.89       | ...         | 4.66  | ...         | ...         | –0.60       | ...    |
| 17200631–3858379 | 348.706     | –1.051      | 62.341     | 9            | –          | –           | –           | –          | –           | –             | –           | –                      | –            | –           | –            | –            | –            | –     | 7.698                              | ...                         | ...                         | 1                     | 74.4                               | 0.48                                 | 4.71                          | –15.530                       | ...         | ...         | 19.31 | ...         | ...         | ...         | ...    |
| 17200691–3859539 | 348.690     | –1.064      | 53.535     | 9            | –          | –           | –           | –          | –           | –             | –           | –                      | –            | –           | –            | –            | –            | –     | 9.810                              | ...                         | ...                         | 1                     | 50.0                               | 0.40                                 | 4.71                          | –10.137                       | ...         | ...         | 16.58 | ...         | ...         | ...         | ...    |
| 17201806–3554178 | 351.249     | 0.674       | 98.685     | 9            | –          | –           | –           | –          | –           | –             | –           | –                      | –            | –           | –            | –            | –            | –     | 8.228                              | ...                         | ...                         | 1                     | 70.2                               | 0.54                                 | 4.75                          | –28.542                       | ...         | ...         | 30.57 | ...         | ...         | ...         | ...    |
| 17201844–3554149 | 351.251     | 0.673       | 99.152     | 9            | –          | –           | –           | –          | –           | –             | –           | –                      | –            | –           | –            | –            | –            | –     | 7.808                              | 1.69                        | 3.33                        | 1                     | 98.6                               | 0.88                                 | 4.68                          | –29.136                       | –14.73      | –45.93      | 30.71 | ...         | ...         | –12.78      | –39.38 |
| 17203029–3551218 | 351.313     | 0.668       | 104.943    | 9            | –          | –           | –           | –          | –           | –             | –           | –                      | –            | –           | –            | –            | –            | –     | 6.344                              | 1.73                        | 2.90                        | 1                     | 145.4                              | 0.60                                 | 4.68                          | –32.758                       | –15.65      | –49.23      | 32.51 | ...         | ...         | –13.59      | –42.31 |
| 17203210–3551290 | 351.315     | 0.662       | 102.008    | 9            | –          | –           | –           | –          | –           | –             | –           | –                      | –            | –           | –            | –            | –            | –     | 5.950                              | 1.33                        | 2.28                        | 1                     | 156.0                              | 0.56                                 | 4.71                          | –32.058                       | –15.56      | –48.40      | 31.60 | ...         | ...         | –13.56      | –41.66 |
| 17203254–3551237 | 351.317     | 0.661       | 101.689    | 9            | –          | –           | –           | –          | –           | –             | –           | –                      | –            | –           | –            | –            | –            | –     | 6.112                              | 1.32                        | 2.33                        | 1                     | 135.4                              | 0.72                                 | 4.75                          | –31.777                       | –15.52      | –48.18      | 31.50 | ...         | ...         | –13.53      | –41.47 |
| 17203465–3550400 | 351.331     | 0.663       | 104.321    | 9            | –          | –           | –           | –          | –           | –             | –           | –                      | –            | –           | –            | –            | –            | –     | 6.853                              | 1.38                        | 2.40                        | 1                     | 141.0                              | 0.86                                 | 4.71                          | –32.017                       | –15.89      | –49.43      | 32.31 | ...         | ...         | –13.85      | –42.54 |
| 17204420–3549371 | 351.364     | 0.646       | 101.910    | 9            | –          | –           | –           | –          | –           | –             | –           | –                      | –            | –           | –            | –            | –            | –     | 6.085                              | 1.60                        | 2.89                        | 1                     | 162.6                              | 0.30                                 | 4.71                          | –31.887                       | –15.28      | –47.74      | 31.57 | ...         | ...         | –13.28      | –41.01 |
| 17204716–3549151 | 351.374     | 0.641       | 100.011    | 9            | –          | –           | –           | –          | –           | –             | –           | –                      | –            | –           | –            | –            | –            | –     | 5.905                              | 1.45                        | 2.67                        | 1                     | 163.6                              | 0.70                                 | 4.71                          | –31.359                       | –15.11      | –47.01      | 30.98 | ...         | ...         | –13.15      | –40.41 |
| 17204864–3548261 | 351.388     | 0.645       | 104.943    | 9            | –          | –           | –           | –          | –           | –             | –           | –                      | –            | –           | –            | –            | –            | –     | 6.550                              | 1.36                        | 2.74                        | 1                     | 201.0                              | 0.56                                 | 4.71                          | –32.552                       | –16.01      | –49.40      | 32.51 | ...         | ...         | –13.96      | –42.47 |
| 17210024–2348567 | 1.323       | 7.405       | 0.845      | 1            | –          | –           | g           | t          | –           | –             | D1          | e                      | o            | –           | –            | –            | –            | –     | 11.526                             | 0.42                        | ...                         | 1                     | 43.8                               | 0.32                                 | 4.47                          | 11.211                        | 0.28        | ...         | 0.26  | 47.1        | 11.21       | 0.29        | ...    |
| 17211081–1935200 | 4.899       | 9.722       | 0.534      | 9            | –          | –           | –           | –          | –           | –             | –           | –                      | –            | –           | –            | –            | –            | –     | 8.699                              | 0.12                        | 0.91                        | 1                     | 27.8                               | 0.72                                 | 4.28                          | 8.500                         | 0.03        | 0.65        | 0.17  | ...         | ...         | 0.04        | 0.68   |
| 17211102–1934220 | 4.913       | 9.730       | 0.549      | 9            | –          | –           | –           | –          | –           | –             | –           | –                      | –            | –           | –            | –            | –            | –     | 11.000                             | 0.11                        | 0.60                        | 1                     | 65.0                               | 0.52                                 | 4.28                          | 10.795                        | 0.02        | 0.33        | 0.17  | ...         | ...         | 0.03        | 0.37   |
| 17212074–2331390 | 1.608       | 7.501       | 0.758      | 1            | –          | –           | g           | t          | N           | –             | D1          | e                      | o            | –           | –            | –            | –            | –     | 10.987                             | 0.44                        | 1.39                        | 1                     | 44.2                               | 0.26                                 | 4.49                          | 10.705                        | 0.31        | 1.01        | 0.23  | 46.9        | 10.71       | 0.33        | 1.06   |
| 17221086–2721389 | 358.522     | 5.195       | 1.291      | 9            | –          | –           | –           | –          | –           | –             | –           | –                      | –            | –           | –            | –            | –            | –     | 7.584                              | 1.55                        | 3.73                        | –2                    | 55.0                               | 0.46                                 | 4.87                          | 7.103                         | 1.34        | 3.09        | 0.40  | ...         | ...         | 1.36        | 3.17   |
| 17223473–5242027 | 337.557     | –9.139      | 0.228      | 1            | –          | –           | g           | –          | –           | –             | D1          | c                      | o            | –           | –            | –            | –            | –     | 10.504                             | 0.46                        | 1.34                        | 1                     | 45.6                               | 0.36                                 | 3.98                          | 10.419                        | 0.42        | 1.23        | 0.07  | 46.1        | 10.43       | 0.43        | 1.25   |
| 17223539–2352338 | 1.477       | 7.071       | 0.926      | 2            | –          | –           | –           | –          | –           | –             | D2          | e                      | o            | –           | –            | –            | e            | –     | 10.548                             | 0.38                        | 1.31                        | 1                     | 40.4                               | 0.72                                 | 4.56                          | 10.203                        | 0.23        | 0.85        | 0.29  | 43.3        | 10.22       | 0.24        | 0.91   |
| 17224092–1833400 | 5.968       | 9.991       | 0.574      | 1            | –          | –           | g           | –          | –           | –             | D2          | c                      | o            | –           | –            | –            | –            | –     | 10.464                             | 0.29                        | 1.13                        | 1                     | 49.8                               | 0.80                                 | 4.16                          | 10.250                        | 0.20        | 0.85        | 0.18  | 51.9        | 10.26       | 0.21        | 0.88   |
| 17225871–4522586 | 343.723     | –5.120      | 0.503      | 1            | –          | –           | –           | –          | –           | –             | D2          | e                      | o            | –           | –            | –            | –            | –     | 9.991                              | 0.35                        | 1.23                        | 1                     | 49.4                               | 0.78                                 | 4.41                          | 9.804                         | 0.27        | 0.98        | 0.16  | 50.8        | 9.82        | 0.28        | 1.01   |
| 17230386–2945162 | 356.477     | 3.687       | 1.311      | 9            | –          | –           | –           | –          | –           | –             | –           | –                      | –            | –           | –            | –            | –            | –     | 7.667                              | 1.70                        | ...                         | –2                    | 46.8                               | 0.34                                 | 4.96                          | 7.179                         | 1.48        | ...         | 0.41  | ...         | 1.50        | ...         |        |
| 17230425–3555161 | 351.555     | 0.203       | 30.612     | 8            | –          | –           | –           | –          | –           | –             | –           | –                      | –            | –           | –            | –            | –            | –     | 8.165                              | ...                         | ...                         | 1                     | 101.4                              | 0.82                                 | 4.92                          | –3.241                        | ...         | ...         | 9.48  | ...         | ...         | ...         | ...    |
| 17230761–1849383 | 5.801       | 9.757       | 0.674      | 1            | o          | –           | g           | t          | N           | –             | D1          | cf                     | o            | –           | –            | –            | –            | –     | 10.621                             | 0.39                        | 1.22                        | 1                     | 64.2                               | 0.34                                 | 4.18                          | 10.370                        | 0.28        | 0.89        | 0.21  | 67.7        | 10.37       | 0.29        | 0.93   |
| 17232296–3553436 | 351.612     | 0.166       | 37.177     | 8            | –          | –           | –           | –          | –           | –             | –           | –                      | –            | –           | –            | –            | –            | –     | 7.428                              | ...                         | ...                         | 1                     | 129.8                              | 0.78                                 | 4.91                          | –6.424                        | ...         | ...         | 11.52 | ...         | ...         | ...         | ...    |
| 17235817–2621060 | 359.585     | 5.430       | 1.193      | 9            | –          | –           | –           | –          | –           | –             | –           | –                      | –            | –           | –            | –            | –            | –     | 6.937                              | 0.22                        | 0.88                        | 1                     | 118.8                              | 0.94                                 | 4.74                          | 6.492                         | 0.02        | 0.29        | 0.37  | ...         | ...         | 0.04        | 0.37   |
| 17244259–3410190 | 353.189     | 0.913       | 57.071     | 9            | –          | –           | –           | –          | –           | –             | –           | –                      | –            | –           | –            | –            | –            | –     | 5.412                              | ...                         | 2.47                        | 1                     | 163.2                              | 0.50                                 | 4.88                          | –15.853                       | ...         | –25.88      | 17.68 | ...         | ...         | –22.12      | ...    |
| 17244364–3409430 | 353.199     | 0.915       | 60.678     | 9            | –          | –           | –           | –          | –           | –             | –           | –                      | –            | –           | –            | –            | –            | –     | 5.387                              | ...                         | 2.78                        | 1                     | 152.6                              | 0.18                                 | 4.87                          | –17.222                       | ...         | –27.36      | 18.80 | ...         | ...         | –23.36      | ...    |
| 17244573–3411070 | 353.184     | 0.896       | 54.666     | 9            | –          | –           | –           | –          | –           | –             | –           | –                      | –            | –           | –            | –            | –            | –     | 5.016                              | 1.31                        | 2.05                        | 1                     | 217.4                              | 0.82                                 | 4.88                          | –15.353                       | –7.75       | –25.11      | 16.93 | ...         | ...         | –6.67       | –21.50 |
| 17244582–3410000 | 353.199     | 0.906       | 61.963     | 9            | –          | –           | –           | –          | –           | –             | –           | –                      | –            | –           | –            | –            | –            | –     | 5.566                              | ...                         | ...                         | 1                     | 184.8                              | 1.0                                  | 4.88                          | –17.521                       | ...         | ...         | 19.19 | ...         | ...         | ...         | ...    |
| 17244791–3409160 | 353.213     | 0.907       | 63.542     | 9            | –          | –           | –           | –          | –           | –             | –           | –                      | –            | –           | –            | –            | –            | –     | 5.817                              | ...                         | 2.53                        | 1                     | 152.6                              | 1.0                                  | 4.87                          | –17.859                       | ...         | –29.04      | 19.68 | ...         | ...         | –24.85      | ...    |
| 17253053–4510279 | 344.146     | –5.373      | 0.477      | 1            | –          | –           | g           | –          | –           | –             | D2          | e                      | o            | –           | –            | –            | –            | –     | 10.573                             | 0.39                        | 1.25                        | 1                     | 34.6                               | 0.74                                 | 4.41                          | 10.395                        | 0.31        | 1.01        | 0.15  | 35.6        | 10.41       | 0.32        | 1.04   |
| 17260894–3715202 | 350.799     | –1.058      | 5.821      | 9            | –          | –           | –           | –          | –           | –             | –           | –                      | –            | –           | –            | –            | –            | –     | 8.731                              | 0.72                        | 2.33                        | –2                    | 39.8                               | 0.54                                 | 4.85                          | 6.562                         | –0.24       | –0.56       | 1.80  | ...         | ...         | –0.13       | –0.17  |
| 17262425–3501418 | 352.675     | 0.144       | 15.771     | 9            | –          | –           | p?          | –          | –           | –             | –           |                        |              |             |              |              |              |       |                                    |                             |                             |                       |                                    |                                      |                               |                               |             |             |       |             |             |             |        |

Table B1: a) continued.

| 2MASX J          | <i>l</i> | <i>b</i> | EBV    | Object | Sample | Disc | 2MRS | Velocity | NIR | Photom | Ext  | <i>K</i> <sub>20</sub> | <i>H-K</i> | <i>J-K</i> | vc   | <i>a</i> | <i>b/a</i> | st.d. | <i>K</i> <sub>s</sub> <sup>o</sup> | ( <i>H-K</i> ) <sup>o</sup> | ( <i>J-K</i> ) <sup>o</sup> | <i>A</i> <sub>K</sub> | <i>a</i> <sub>d</sub> <sup>u</sup> | <i>K</i> <sub>s</sub> <sup>o,d</sup> | ( <i>H-K</i> ) <sup>o,c</sup> | ( <i>J-K</i> ) <sup>o,c</sup> |       |      |      |       |       |      |      |     |      |     |      |
|------------------|----------|----------|--------|--------|--------|------|------|----------|-----|--------|------|------------------------|------------|------------|------|----------|------------|-------|------------------------------------|-----------------------------|-----------------------------|-----------------------|------------------------------------|--------------------------------------|-------------------------------|-------------------------------|-------|------|------|-------|-------|------|------|-----|------|-----|------|
| (1)              | deg      | deg      | mag    | class  | off    | flag | gal  | TF       | obs | ext'd  | type | (8)                    | (9)        | Opt        | HI   | (10a)    | (10b)      | flag  | flag                               | flag                        | flag                        | mag                   | (21)                               | mag                                  | (22)                          | mag                           | (23)  | mag  | (24) | mag   | (25)  | mag  | (26) | mag | (27) | mag | (28) |
| 17403470–2503169 | 2.715    | 2.994    | 1.708  | 9      | –      | –    | –    | –        | –   | –      | –    | –                      | 9.065      | 0.53       | ...  | –2       | 46.6       | 0.16  | 4.94                               | 8.429                       | 0.24                        | ...                   | 0.53                               | ...                                  | ...                           | 0.28                          | ...   | ...  | ...  | ...   | ...   | ...  | ...  | ... | ...  | ... |      |
| 17403580–4042494 | 349.413  | –5.291   | 0.492  | 1      | –      | –    | g    | –        | –   | –      | D2   | e                      | o          | –          | –    | –        | –          | –     | 10.084                             | 0.28                        | 1.16                        | 1                     | 50.8                               | 0.96                                 | 4.51                          | 9.901                         | 0.19  | 0.92 | 0.15 | 52.3  | 9.92  | 0.20 | 0.95 | ... | ...  |     |      |
| 17404833–1750547 | 8.900    | 6.731    | 0.523  | 1      | –      | –    | g    | t        | N   | –      | D2   | ea                     | o          | –          | –    | –        | –          | V     | 8.186                              | 0.39                        | ...                         | 1                     | 65.0                               | 0.44                                 | 4.52                          | 7.991                         | 0.30  | ...  | 0.16 | 67.3  | 8.00  | 0.31 | ...  | ... | ...  |     |      |
| 17412069–3036350 | 358.089  | –0.089   | 19.477 | 9      | –      | –    | –    | –        | –   | –      | –    | –                      | 6.437      | 1.16       | 2.63 | –2       | 112.6      | 0.72  | 4.87                               | –0.820                      | –2.06                       | –7.05                 | 6.03                               | ...                                  | –1.68                         | –5.76                         | ...   | ...  | ...  | ...   | ...   | ...  | ...  | ... |      |     |      |
| 17423620–3854340 | 351.159  | –4.675   | 0.838  | 1      | –      | –    | g    | t        | N   | –      | D4   | –                      | –          | –          | –    | –        | –          | V     | 9.344                              | 0.26                        | 1.20                        | 1                     | 126.0                              | 0.40                                 | 4.66                          | 9.032                         | 0.12  | 0.78 | 0.26 | 133.3 | 9.06  | 0.13 | 0.84 | ... | ...  |     |      |
| 17432726–1930135 | 7.805    | 5.335    | 0.812  | 9      | –      | –    | –    | –        | –   | –      | –    | –                      | 10.993     | ...        | ...  | –2       | 18.2       | 0.56  | 4.71                               | 10.690                      | ...                         | ...                   | 0.25                               | ...                                  | ...                           | ...                           | ...   | ...  | ...  | ...   | ...   | ...  | ...  | ... | ...  |     |      |
| 17444121–4050325 | 349.707  | –6.019   | 0.437  | 2      | –      | –    | g    | t        | –   | –      | D3   | e                      | o          | –          | –    | –        | –          | –     | 11.301                             | 0.22                        | 0.96                        | 1                     | 32.4                               | 0.44                                 | 4.42                          | 11.138                        | 0.14  | 0.74 | 0.14 | 33.3  | 11.15 | 0.15 | 0.77 | ... | ...  |     |      |
| 17451726–1430457 | 12.340   | 7.526    | 0.582  | 1      | –      | –    | g    | –        | –   | –      | –    | –                      | 10.804     | 0.33       | 1.26 | 1        | 35.0       | 0.84  | 4.24                               | 10.587                      | 0.23                        | 0.97                  | 0.18                               | 36.4                                 | 10.60                         | 0.24                          | 1.00  | ...  | ...  | ...   | ...   | ...  | ...  | ... | ...  |     |      |
| 17453525–4009391 | 350.383  | –5.816   | 0.548  | 1      | –      | –    | g    | t        | –   | –      | D1   | e                      | o          | –          | –    | –        | –          | V     | 11.283                             | 0.44                        | ...                         | 1                     | 49.0                               | 0.40                                 | 4.46                          | 11.079                        | 0.35  | ...  | 0.17 | 51.0  | 11.09 | 0.36 | ...  | ... | ...  |     |      |
| 17453533–4605233 | 345.238  | –8.835   | 0.189  | 8      | –      | p?   | –    | –        | –   | –      | –    | –                      | 9.208      | 0.90       | 1.21 | 1        | 33.8       | 0.90  | 4.10                               | 9.138                       | 0.87                        | 1.12                  | 0.06                               | ...                                  | ...                           | 0.88                          | 1.13  | ...  | ...  | ...   | ...   | ...  | ...  | ... | ...  |     |      |
| 17453592–2900532 | 359.930  | –0.037   | 97.885 | 9      | –      | –    | –    | –        | –   | –      | –    | –                      | 5.715      | ...        | ...  | 1        | 59.6       | 0.48  | 5.09                               | –30.757                     | ...                         | ...                   | 30.32                              | ...                                  | ...                           | ...                           | ...   | ...  | ...  | ...   | ...   | ...  | ...  | ... | ...  | ... |      |
| 17454133–2900082 | 359.951  | –0.047   | 97.639 | 9      | –      | –    | –    | –        | –   | –      | –    | –                      | 3.336      | ...        | ...  | 1        | 154.0      | 0.62  | 5.09                               | –33.044                     | ...                         | ...                   | 30.24                              | ...                                  | ...                           | ...                           | ...   | ...  | ...  | ...   | ...   | ...  | ...  | ... | ...  | ... |      |
| 17454438–2859112 | 359.971  | –0.049   | 97.631 | 9      | –      | –    | –    | –        | –   | –      | –    | –                      | 4.741      | 2.04       | ...  | 1        | 220.0      | 0.18  | 5.09                               | –31.636                     | –14.13                      | ...                   | 30.24                              | ...                                  | ...                           | –12.21                        | ...   | ...  | ...  | ...   | ...   | ...  | ...  | ... | ...  | ... |      |
| 17454632–2228191 | 5.542    | 3.333    | 1.017  | 8      | –      | –    | –    | –        | –   | –      | –    | –                      | 7.349      | 0.51       | 1.43 | 1        | 122.2      | 0.28  | 4.92                               | 6.970                       | 0.34                        | 0.92                  | 0.32                               | ...                                  | ...                           | 0.36                          | 0.99  | ...  | ...  | ...   | ...   | ...  | ...  | ... | ...  |     |      |
| 17461635–3322279 | 356.280  | –2.427   | 2.185  | 8      | –      | –    | –    | –        | –   | –      | –    | –                      | 7.006      | 0.77       | 1.89 | –2       | 95.0       | 0.40  | 4.94                               | 6.192                       | 0.41                        | 0.80                  | 0.68                               | ...                                  | ...                           | 0.45                          | 0.95  | ...  | ...  | ...   | ...   | ...  | ...  | ... | ...  |     |      |
| 17473612–2848224 | 0.336    | –0.303   | 27.795 | 9      | –      | –    | –    | –        | –   | –      | –    | –                      | 7.603      | ...        | ...  | –2       | 94.8       | 0.52  | 4.87                               | –2.753                      | ...                         | ...                   | 8.61                               | ...                                  | ...                           | ...                           | ...   | ...  | ...  | ...   | ...   | ...  | ...  | ... | ...  | ... |      |
| 17474365–4322487 | 347.796  | –7.798   | 0.312  | 1      | –      | –    | g    | –        | –   | –      | D1   | e                      | o          | –          | –    | –        | –          | V     | 11.152                             | 0.37                        | 1.14                        | 1                     | 45.4                               | 0.34                                 | 4.21                          | 11.036                        | 0.32  | 0.99 | 0.10 | 46.3  | 11.04 | 0.33 | 1.01 | ... | ...  | ... | ...  |
| 17480455–2446441 | 3.839    | 1.688    | 4.234  | 9      | –      | –    | –    | –        | –   | –      | –    | –                      | 3.323      | 0.55       | 1.96 | 1        | 182.2      | 0.84  | 4.86                               | 1.745                       | –0.15                       | –0.15                 | 1.31                               | ...                                  | ...                           | –0.07                         | 0.13  | ...  | ...  | ...   | ...   | ...  | ...  | ... | ...  |     |      |
| 17480925–2447241 | 3.839    | 1.667    | 4.292  | 9      | –      | –    | –    | –        | –   | –      | –    | –                      | 8.124      | 0.59       | ...  | –2       | 42.4       | 1.00  | 4.86                               | 6.525                       | –0.12                       | ...                   | 1.33                               | ...                                  | ...                           | –0.04                         | ...   | ...  | ...  | ...   | ...   | ...  | ...  | ... | ...  |     |      |
| 17481868–1449499 | 12.438   | 6.735    | 0.700  | 1      | –      | –    | –    | –        | –   | –      | D2   | e                      | o          | –          | –    | –        | –          | V     | 11.212                             | 0.40                        | 1.26                        | 1                     | 25.8                               | 0.64                                 | 4.36                          | 10.951                        | 0.29  | 0.91 | 0.22 | 27.1  | 10.97 | 0.30 | 0.96 | ... | ...  | ... | ...  |
| 17485084–2021159 | 7.730    | 3.811    | 1.137  | 9      | –      | –    | –    | –        | –   | –      | –    | –                      | 6.666      | 0.26       | 1.00 | 1        | 111.8      | 0.90  | 4.88                               | 6.242                       | 0.07                        | 0.43                  | 0.35                               | ...                                  | ...                           | 0.09                          | 0.51  | ...  | ...  | ...   | ...   | ...  | ...  | ... | ...  |     |      |
| 17485332–2021469 | 7.727    | 3.798    | 1.138  | 9      | –      | –    | –    | –        | –   | –      | –    | –                      | 4.350      | 0.29       | 1.26 | 1        | 161.0      | 0.82  | 4.88                               | 3.926                       | 0.10                        | 0.70                  | 0.35                               | ...                                  | ...                           | 0.12                          | 0.77  | ...  | ...  | ...   | ...   | ...  | ...  | ... | ...  |     |      |
| 17501031–3703366 | 353.520  | –5.002   | 0.620  | 9      | –      | –    | –    | –        | –   | –      | –    | –                      | 6.725      | 0.15       | 0.64 | 1        | 115.2      | 0.88  | 4.75                               | 6.494                       | 0.04                        | 0.33                  | 0.19                               | ...                                  | ...                           | 0.06                          | 0.37  | ...  | ...  | ...   | ...   | ...  | ...  | ... | ...  |     |      |
| 17501048–3702206 | 353.539  | –4.992   | 0.605  | 9      | –      | –    | –    | –        | –   | –      | –    | –                      | 6.209      | 0.14       | 0.67 | 1        | 219.2      | 0.30  | 4.75                               | 5.984                       | 0.04                        | 0.37                  | 0.19                               | ...                                  | ...                           | 0.06                          | 0.41  | ...  | ...  | ...   | ...   | ...  | ...  | ... | ...  |     |      |
| 17501357–3703076 | 353.532  | –5.008   | 0.614  | 9      | –      | –    | –    | –        | –   | –      | –    | –                      | 4.058      | 0.18       | 0.87 | 1        | 152.2      | 0.86  | 4.75                               | 3.829                       | 0.08                        | 0.57                  | 0.19                               | ...                                  | ...                           | 0.09                          | 0.61  | ...  | ...  | ...   | ...   | ...  | ...  | ... | ...  |     |      |
| 17501591–3703506 | 353.526  | –5.020   | 0.622  | 9      | –      | –    | –    | –        | –   | –      | –    | –                      | 6.478      | 0.16       | 0.75 | 1        | 219.4      | 0.84  | 4.75                               | 6.246                       | 0.05                        | 0.44                  | 0.19                               | ...                                  | ...                           | 0.07                          | 0.49  | ...  | ...  | ...   | ...   | ...  | ...  | ... | ...  |     |      |
| 17504702–3116296 | 358.573  | –2.163   | 2.634  | 8      | –      | –    | –    | –        | –   | –      | –    | –                      | 6.497      | 0.42       | 1.68 | 1        | 130.8      | 0.94  | 4.91                               | 5.516                       | –0.01                       | 0.37                  | 0.82                               | ...                                  | ...                           | 0.04                          | 0.55  | ...  | ...  | ...   | ...   | ...  | ...  | ... | ...  |     |      |
| 17505167–3435596 | 355.717  | –3.873   | 0.664  | 9      | –      | –    | –    | –        | –   | –      | –    | –                      | 6.210      | 0.19       | 0.82 | 1        | 166.2      | 0.76  | 4.84                               | 5.963                       | 0.08                        | 0.49                  | 0.21                               | ...                                  | ...                           | 0.09                          | 0.54  | ...  | ...  | ...   | ...   | ...  | ...  | ... | ...  |     |      |
| 17510451–1614023 | 11.559   | 5.451    | 0.668  | 1      | –      | –    | g    | –        | –   | –      | D2   | e                      | o          | –          | –    | –        | –          | V     | 11.353                             | 0.38                        | ...                         | 1                     | 26.2                               | 0.92                                 | 4.52                          | 11.104                        | 0.27  | ...  | 0.21 | 27.5  | 11.12 | 0.28 | ...  | ... | ...  | ... |      |
| 17521905–1517459 | 12.524   | 5.665    | 0.715  | 1      | –      | –    | –    | –        | –   | –      | D3   | –                      | –          | –          | –    | –        | –          | –     | 11.020                             | 0.25                        | ...                         | –2                    | 39.8                               | 1.00                                 | 4.46                          | 10.754                        | 0.14  | ...  | 0.22 | 42.0  | 10.76 | 0.15 | ...  | ... | ...  | ... |      |
| 17523736–3332225 | 356.818  | –3.649   | 1.011  | 8      | o      | –    | –    | –        | –   | –      | –    | –                      | 7.517      | ...        | ...  | –2       | 61.0       | 0.30  | 4.96                               | 7.140                       | ...                         | ...                   | 0.31                               | ...                                  | ...                           | ...                           | ...   | ...  | ...  | ...   | ...   | ...  | ...  | ... | ...  | ... |      |
| 17541141–4106159 | 350.389  | –7.701   | 0.248  | 1      | –      | –    | –    | –        | –   | –      | D1   | e                      | o          | –          | –    | –        | –          | V     | 11.256                             | 0.28                        | 1.08                        | 1                     | 30.2                               | 0.54                                 | 4.23                          | 11.164                        | 0.24  | 0.95 | 0.08 | 30.6  | 11.17 | 0.25 | 0.97 | ... | ...  | ... | ...  |
| 17542696–2408460 | 5.124    | 0.764    | 6.542  | 9      | –      | –    | –    | –        | –   | –      | –    | –                      | 5.007      | 0.63       | 2.20 | 1        | 143.2      | 0.82  | 4.90                               | 2.569                       | –0.45                       | –1.05                 | 2.03                               | ...                                  | ...                           | –0.32                         | –0.92 | ...  | ...  | ...   | ...   | ...  | ...  | ... | ...  |     |      |
| 17543142–4115049 | 350.291  | –7.828   | 0.236  | 2      | –      | –    | –    | –        | –   | –      | D1   | e                      | o          | –          | –    | –        | –          | V     | 11.320                             | 0.37                        | 1.13                        | 1                     | 25.8                               | 0.80                                 | 4.20                          | 11.232                        | 0.33  | 1.01 | 0.07 | 26.1  | 11.24 | 0.33 | 1.03 | ... | ...  | ... | ...  |
| 17545985–2137147 | 7.368    | 1.931    | 1.819  | 9      | –      | –    | –    | –        | –   | –      | –    | –                      | 6.517      | 1.28       | 2.70 | 1        | 81.0       | 0.40  | 4.94                               | 5.839                       | 0.98                        | 1.80                  | 0.56                               | ...                                  | ...                           | 1.02                          | 1.92  | ...  | ...  | ...   | ...   | ...  | ...  | ... | ...  |     |      |
| 17552396–3912415 | 352.164  | –6.969   | 0.326  | 1      | –      | –    | –    | –        | –   | –      | D1   | e                      | o          | –          | –    | –        | –          | V     | 10.523                             | 0.31                        | 1.00                        | 1                     | 52.4                               | 0.62                                 | 4.40                          | 10.402                        | 0.25  | 0.84 | 0.10 | 53.4  | 10.41 | 0.26 | 0.86 | ... | ...  | ... | ...  |
| 17561497–4243159 | 349.153  | –8.825   | 0.176  | 1      | –      | –    | –    | –        | –   | –      | D1   | c                      | o          | –          | –    | –        | –          | V     | 10.510                             | 0.28                        | 1.08                        | 1                     | 54.8                               | 0.68                                 | 4.09                          | 10.444                        | 0.25  | 1.00 | 0.05 | 55.3  | 10.45 | 0.26 | 1.01 | ... | ...  | ... | ...  |
| 17575504–1138276 | 16.394   | 6.299    | 1.089  | 1      | –      | –    | –    | –        | –   | –      | D3   | –                      | –          | –          | –    | –        | –          | V     | 10.836                             | 0.45                        | 1.45                        | 1                     | 44.2                               | 0.72                                 | 4.28                          | 10.430                        | 0.27  | 0.91 | 0.34 | 48.5  | 10.44 | 0.30 | 0.98 | ... | ...  | ... | ...  |
| 17581377–1241453 | 15.508   | 5.713    | 1.226  | 2      | –      | –    | –    | –        | –   | –      | D3   | –                      | –          | –          | –    | –        | –          | V     | 11.537                             | 0.51                        | 1.52                        | –2                    | 19.4                               | 0.84                                 | 4.32                          | 11.080                        | 0.31  | 0.91 | 0.38 | 21.6  | 11.09 | 0.33 | 1.00 | ... | ...  | ... | ...  |
| 17582147–1137141 | 16.465   | 6.215    | 1.036  | 1      | –      | –    | –    | –        | –   | –      | D1   | –                      | –          | –          | –    | –        | –          | V     | 11.589                             | 0.50                        | 1.43                        | 1                     | 32.2                               | 0.38                                 | 4.28                          | 11.203                        | 0.33  | 0.91 | 0.32 | 35.2  | 11.21 | 0.35 | 0.98 | ... | ...  | ... | ...  |
| 17585198–4415565 | 348.010  | –9.983   | 0.245  | 9      | –      | –    | –    | –        | –   | –      | –    | –                      | 8.703      | –0.19      | 0.24 | –2       | 187.4      | 0.92  | 4.12                               | 8.612                       | –0.23                       | 0.12                  | 0.08                               | ...                                  | ...                           | –0.23                         | 0.14  | ...  | ...  | ...   | ...   | ...  | ...  | ... | ...  |     |      |
| 17585394–4415085 | 348.025  | –9.982   | 0.244  | 9      |        |      |      |          |     |        |      |                        |            |            |      |          |            |       |                                    |                             |                             |                       |                                    |                                      |                               |                               |       |      |      |       |       |      |      |     |      |     |      |



Table B1: a) continued.

| 2MASX J          | <i>l</i>    | <i>b</i>    | EBV        | Object       | Sample     | Disc        | 2MRS        | Velocity   | NIR         | Photom        | Ext         | <i>K</i> <sub>20</sub> | <i>H-K</i>   | <i>J-K</i>  | vc           | <i>a</i>     | <i>b/a</i>   | st.d. | <i>K</i> <sub>s</sub> <sup>o</sup> | ( <i>H-K</i> ) <sup>o</sup> | ( <i>J-K</i> ) <sup>o</sup> | <i>A<sub>K</sub></i> | <i>a</i> <sub>d</sub> <sup>o</sup> | <i>K</i> <sub>s</sub> <sup>o,d</sup> | ( <i>H-K</i> ) <sup>o,c</sup> | ( <i>J-K</i> ) <sup>o,c</sup> |             |             |      |             |             |             |      |
|------------------|-------------|-------------|------------|--------------|------------|-------------|-------------|------------|-------------|---------------|-------------|------------------------|--------------|-------------|--------------|--------------|--------------|-------|------------------------------------|-----------------------------|-----------------------------|----------------------|------------------------------------|--------------------------------------|-------------------------------|-------------------------------|-------------|-------------|------|-------------|-------------|-------------|------|
| (1)              | deg<br>(2a) | deg<br>(2b) | mag<br>(3) | class<br>(4) | off<br>(5) | flag<br>(6) | gal<br>(7a) | TF<br>(7b) | obs<br>(7c) | ext'd<br>(7d) | type<br>(8) | (9)                    | Opt<br>(10a) | HI<br>(10b) | flag<br>(11) | flag<br>(12) | flag<br>(13) | (14)  | mag<br>(15)                        | mag<br>(16)                 | (17)                        | (18)                 | (19)                               | (20)                                 | mag<br>(21)                   | mag<br>(22)                   | mag<br>(23) | mag<br>(24) | (25) | mag<br>(26) | mag<br>(27) | mag<br>(28) |      |
| 18045461−0736191 | 20.788      | 6.749       | 1.097      | 9            | —          | —           | —           | —          | —           | —             | —           | —                      | 8.727        | 0.39        | 0.95         | 1            | 206.0        | 0.44  | 4.39                               | 8.318                       | 0.21                        | 0.41                 | 0.34                               | ...                                  | ...                           | 0.23                          | 0.48        |             |      |             |             |             |      |
| 18045529−0734521 | 20.810      | 6.758       | 1.092      | 9            | —          | —           | —           | —          | —           | —             | —           | —                      | 9.189        | 0.66        | 0.79         | 1            | 131.6        | 0.74  | 4.39                               | 8.782                       | 0.48                        | 0.25                 | 0.34                               | ...                                  | ...                           | 0.50                          | 0.32        |             |      |             |             |             |      |
| 18045876−4139491 | 350.875     | −9.745      | 0.151      | 1            | —          | —           | —           | —          | —           | —             | D1          | c                      | o            | —           | —            | V            | —            | —     | 10.272                             | 0.36                        | 1.10                        | 1                    | 54.0                               | 0.32                                 | 4.03                          | 10.216                        | 0.33        | 1.02        | 0.05 | 54.3        | 10.22       | 0.33        | 1.03 |
| 18051311−1950348 | 10.099      | 0.739       | 6.675      | 8            | —          | p           | —           | —          | —           | —             | —           | —                      | 9.196        | 0.98        | 1.39         | 1            | 36.2         | 0.72  | 4.81                               | 6.709                       | −0.12                       | −1.92                | 2.07                               | ...                                  | ...                           | 0.01                          | −1.48       |             |      |             |             |             |      |
| 18055139−0436219 | 23.560      | 7.970       | 2.760      | 2            | —          | —           | —           | —          | N           | —             | D2          | —                      | —            | —           | —            | V            | —            | —     | 11.695                             | 0.73                        | 2.27                        | 1                    | 22.2                               | 0.90                                 | 3.83                          | 10.667                        | 0.27        | 0.90        | 0.85 | 30.8        | 10.61       | 0.33        | 1.08 |
| 18062037−0751501 | 20.730      | 6.314       | 1.230      | 1            | —          | —           | —           | —          | N           | —             | D2          | —                      | —            | —           | —            | V            | —            | —     | 10.473                             | 0.40                        | 1.54                        | 1                    | 52.0                               | 0.64                                 | 4.16                          | 10.015                        | 0.19        | 0.92        | 0.38 | 57.9        | 10.02       | 0.22        | 1.01 |
| 18063559−3541277 | 356.352     | −7.209      | 0.300      | 2            | —          | —           | —           | —          | —           | —             | D2          | e                      | o            | —           | —            | —            | —            | —     | 10.961                             | 0.28                        | ...                         | 1                    | 36.6                               | 0.96                                 | 4.56                          | 10.849                        | 0.23        | ...         | 0.09 | 37.2        | 10.86       | 0.23        | ...  |
| 18070109−1017198 | 18.672      | 5.004       | 0.932      | 2            | —          | —           | —           | —          | N           | —             | D3          | —                      | —            | —           | —            | V            | —            | —     | 11.159                             | 0.35                        | 1.28                        | 1                    | 26.2                               | 0.74                                 | 4.37                          | 10.812                        | 0.20        | 0.82        | 0.29 | 28.4        | 10.81       | 0.21        | 0.88 |
| 18071027−0249517 | 25.298      | 8.517       | 1.612      | 1            | —          | —           | —           | —          | —           | —             | D1          | e                      | —            | h           | —            | V            | —            | —     | 10.271                             | 0.40                        | 1.38                        | 1                    | 73.0                               | 0.80                                 | 3.91                          | 9.670                         | 0.14        | 0.58        | 0.50 | 88.9        | 9.59        | 0.17        | 0.68 |
| 18071996−2459542 | 5.836       | −2.202      | 1.795      | 9            | —          | —           | —           | —          | —           | —             | —           | —                      | 5.368        | 0.33        | 0.98         | 1            | 71.4         | 0.82  | 4.85                               | 4.699                       | 0.03                        | 0.09                 | 0.56                               | ...                                  | ...                           | 0.06                          | 0.21        |             |      |             |             |             |      |
| 18072115−2151261 | 8.584       | −0.679      | 10.986     | 9            | —          | —           | —           | —          | —           | —             | D2          | —                      | —            | —           | —            | —            | —            | —     | 6.470                              | 1.54                        | ...                         | 1                    | 72.0                               | 0.36                                 | 4.85                          | 2.377                         | −0.28       | ...         | 3.40 | ...         | ...         | −0.07       | ...  |
| 18072606−0905469 | 19.772      | 5.486       | 1.383      | 1            | —          | —           | —           | —          | t           | N             | D2          | —                      | —            | —           | —            | V            | —            | —     | 11.025                             | 0.50                        | 1.74                        | 1                    | 38.0                               | 0.68                                 | 4.29                          | 10.510                        | 0.27        | 1.05        | 0.43 | 43.3        | 10.51       | 0.30        | 1.15 |
| 18073208−0909508 | 19.724      | 5.432       | 1.390      | 1            | —          | —           | —           | —          | —           | —             | D2          | —                      | —            | —           | —            | V            | —            | —     | 10.065                             | 0.56                        | 1.69                        | 1                    | 52.4                               | 0.90                                 | 4.29                          | 9.547                         | 0.33        | 1.00        | 0.43 | 59.6        | 9.55        | 0.35        | 1.10 |
| 18073511−0901148 | 19.857      | 5.490       | 1.413      | 2            | —          | —           | —           | —          | —           | —             | D2          | —                      | —            | —           | —            | V            | —            | —     | 11.516                             | 0.50                        | 1.53                        | 1                    | 27.6                               | 0.76                                 | 4.26                          | 10.990                        | 0.26        | 0.83        | 0.44 | 31.7        | 10.98       | 0.29        | 0.92 |
| 18073699−0850329 | 20.018      | 5.568       | 1.446      | 1            | —          | —           | —           | —          | t           | N             | D2          | —                      | —            | —           | —            | V            | —            | —     | 10.945                             | 1.08                        | ...                         | 1                    | 38.2                               | 1.00                                 | 4.30                          | 10.406                        | 0.84        | ...         | 0.45 | 44.1        | 10.39       | 0.87        | ...  |
| 18074654−3745046 | 354.631     | −8.390      | 0.148      | 1            | —          | —           | —           | —          | —           | —             | D1          | c                      | o            | —           | —            | V            | —            | —     | 10.433                             | 0.26                        | 0.99                        | 1                    | 65.0                               | 0.46                                 | 4.33                          | 10.378                        | 0.24        | 0.92        | 0.05 | 65.4        | 10.38       | 0.24        | 0.93 |
| 18085372−3705543 | 355.319     | −8.281      | 0.165      | 1            | —          | —           | —           | —          | —           | —             | D4          | c                      | —            | —           | —            | V            | —            | —     | 9.288                              | 0.25                        | 0.91                        | 1                    | 83.2                               | 0.90                                 | 4.32                          | 9.227                         | 0.22        | 0.83        | 0.05 | 83.7        | 9.23        | 0.22        | 0.84 |
| 18090034−2005040 | 10.321      | −0.155      | 65.157     | 9            | —          | —           | —           | —          | —           | —             | —           | —                      | 6.989        | ...         | ...          | 1            | 188.0        | 0.46  | 4.78                               | −17.288                     | ...                         | ...                  | 20.18                              | ...                                  | ...                           | ...                           | ...         | ...         | ...  | ...         | ...         | ...         |      |
| 18091483−2554067 | 5.254       | −3.017      | 1.375      | 9            | —          | —           | —           | —          | —           | —             | —           | —                      | 5.261        | 0.29        | 1.16         | 1            | 127.2        | 0.64  | 4.70                               | 4.749                       | 0.06                        | 0.48                 | 0.43                               | ...                                  | ...                           | 0.09                          | 0.57        |             |      |             |             |             |      |
| 18091691−2554447 | 5.248       | −3.029      | 1.374      | 9            | —          | —           | —           | —          | —           | —             | —           | —                      | 4.281        | 0.31        | 1.11         | 1            | 182.2        | 0.62  | 4.70                               | 3.769                       | 0.08                        | 0.43                 | 0.43                               | ...                                  | ...                           | 0.11                          | 0.52        |             |      |             |             |             |      |
| 18092009−2554427 | 5.255       | −3.039      | 1.361      | 9            | —          | —           | —           | —          | —           | —             | —           | —                      | 4.798        | 0.28        | 1.07         | 1            | 183.6        | 0.60  | 4.70                               | 4.291                       | 0.05                        | 0.39                 | 0.42                               | ...                                  | ...                           | 0.08                          | 0.48        |             |      |             |             |             |      |
| 18092698−2019470 | 10.157      | −0.365      | 103.918    | 9            | —          | —           | —           | —          | —           | —             | —           | —                      | 6.355        | ...         | ...          | 1            | 219.4        | 0.30  | 4.82                               | −32.365                     | ...                         | ...                  | 32.19                              | ...                                  | ...                           | ...                           | ...         | ...         | ...  | ...         | ...         | ...         |      |
| 18092846−2019199 | 10.167      | −0.367      | 106.361    | 9            | —          | —           | —           | —          | —           | —             | —           | —                      | 6.530        | ...         | ...          | 1            | 126.8        | 1.00  | 4.84                               | −33.100                     | ...                         | ...                  | 32.95                              | ...                                  | ...                           | ...                           | ...         | ...         | ...  | ...         | ...         | ...         |      |
| 18092888−0038358 | 27.529      | 9.027       | 0.960      | 1            | —          | —           | —           | —          | t           | N             | D1          | c                      | —            | *           | —            | V            | —            | —     | 11.053                             | 0.44                        | 1.54                        | 1                    | 45.8                               | 0.38                                 | 3.87                          | 10.695                        | 0.28        | 1.06        | 0.30 | 49.6        | 10.70       | 0.30        | 1.12 |
| 18093621−2046199 | 9.787       | −0.611      | 9.937      | 9            | —          | —           | —           | —          | —           | —             | —           | —                      | 7.477        | ...         | ...          | 1            | 103.6        | 0.42  | 4.90                               | 3.774                       | ...                         | ...                  | 3.08                               | ...                                  | ...                           | ...                           | ...         | ...         | ...  | ...         | ...         | ...         |      |
| 18100236−0043306 | 27.521      | 8.865       | 1.039      | 1            | —          | —           | —           | —          | —           | —             | D1          | —                      | —            | *           | —            | V            | o            | —     | 10.930                             | 0.50                        | 1.36                        | 1                    | 45.0                               | 0.50                                 | 3.86                          | 10.543                        | 0.33        | 0.84        | 0.32 | 49.3        | 10.55       | 0.35        | 0.91 |
| 18100993−0010196 | 28.032      | 9.093       | 0.652      | 1            | o          | —           | —           | —          | t           | N             | D1          | c                      | —            | —           | —            | V            | o            | —     | 10.462                             | 0.25                        | 1.06                        | 1                    | 74.0                               | 0.48                                 | 3.87                          | 10.219                        | 0.14        | 0.74        | 0.20 | 77.8        | 10.23       | 0.15        | 0.78 |
| 18103194−0652259 | 22.103      | 5.872       | 1.232      | 1            | —          | —           | —           | —          | —           | —             | D3          | —                      | —            | —           | —            | V            | —            | —     | 11.645                             | 0.59                        | 1.88                        | 1                    | 21.4                               | 0.76                                 | 4.18                          | 11.186                        | 0.38        | 1.27        | 0.38 | 23.9        | 11.19       | 0.41        | 1.35 |
| 18104013−0712369 | 21.821      | 5.682       | 1.399      | 9            | —          | —           | —           | —          | —           | —             | —           | —                      | 10.536       | ...         | 0.94         | 1            | 44.2         | 1.00  | 4.46                               | 10.015                      | ...                         | ...                  | 0.24                               | 0.43                                 | ...                           | ...                           | ...         | ...         | ...  | ...         | ...         | 0.34        |      |
| 18104651−0712469 | 21.832      | 5.658       | 1.398      | 9            | —          | —           | —           | —          | —           | —             | —           | —                      | 8.101        | 0.08        | ...          | 1            | 174.4        | 1.00  | 4.46                               | 7.580                       | −0.15                       | ...                  | 0.43                               | ...                                  | ...                           | −0.13                         | ...         | ...         | ...  | ...         | ...         | ...         |      |
| 18113842+0131397 | 29.733      | 9.548       | 0.531      | 2            | —          | —           | —           | —          | —           | —             | D2          | c                      | —            | —           | —            | —            | —            | —     | 10.970                             | 0.59                        | 1.47                        | 1                    | 23.2                               | 0.82                                 | 3.87                          | 10.772                        | 0.51        | 1.21        | 0.16 | 24.0        | 10.79       | 0.52        | 1.24 |
| 18121459−2244365 | 8.354       | −2.097      | 2.926      | 9            | —          | —           | —           | —          | —           | —             | —           | —                      | 7.149        | 0.36        | ...          | 1            | 80.6         | 0.62  | 4.91                               | 6.059                       | −0.12                       | ...                  | 0.91                               | ...                                  | ...                           | −0.06                         | ...         | ...         | ...  | ...         | ...         | ...         |      |
| 18122468−1307308 | 16.814      | 2.484       | 3.061      | 9            | —          | —           | —           | —          | —           | —             | —           | —                      | 10.551       | ...         | ...          | 1            | 24.2         | 0.48  | 4.67                               | 9.410                       | ...                         | ...                  | 0.95                               | ...                                  | ...                           | ...                           | ...         | ...         | ...  | ...         | ...         | ...         |      |
| 18122631−3434558 | 357.905     | −7.743      | 0.231      | 1            | —          | —           | —           | —          | —           | —             | D3          | e                      | —            | *           | —            | V            | —            | —     | 10.900                             | 0.25                        | 0.95                        | 1                    | 38.2                               | 0.58                                 | 4.49                          | 10.814                        | 0.21        | 0.83        | 0.07 | 38.6        | 10.82       | 0.21        | 0.85 |
| 18122673−3851070 | 354.072     | −9.712      | 0.113      | 1            | —          | —           | —           | —          | t           | N             | D1          | c                      | —            | —           | —            | V            | —            | —     | 11.207                             | 0.37                        | 1.13                        | 1                    | 42.4                               | 0.26                                 | 4.12                          | 11.165                        | 0.35        | 1.08        | 0.04 | 42.6        | 11.17       | 0.35        | 1.08 |
| 18130421−3740314 | 355.190     | −9.283      | 0.148      | 1            | —          | —           | —           | —          | —           | —             | D4          | c                      | —            | —           | —            | V            | —            | —     | 9.610                              | 0.28                        | 1.04                        | 1                    | 69.4                               | 0.56                                 | 4.23                          | 9.555                         | 0.26        | 0.97        | 0.05 | 69.8        | 9.56        | 0.26        | 0.98 |
| 18131474−3740354 | 355.205     | −9.315      | 0.153      | 1            | —          | —           | —           | —          | —           | —             | D1          | c                      | —            | —           | —            | V            | —            | —     | 10.671                             | 0.33                        | 1.09                        | 1                    | 52.4                               | 0.70                                 | 4.23                          | 10.614                        | 0.31        | 1.01        | 0.05 | 52.7        | 10.62       | 0.31        | 1.02 |
| 18131758−0113069 | 27.460      | 7.916       | 1.375      | 1            | —          | —           | —           | —          | —           | —             | D2          | e                      | —            | —           | —            | V            | e            | —     | 10.929                             | 0.45                        | 1.56                        | 1                    | 34.8                               | 0.64                                 | 3.92                          | 10.417                        | 0.22        | 0.88        | 0.43 | 39.2        | 10.43       | 0.25        | 0.97 |
| 18131810−0041379 | 27.930      | 8.157       | 1.060      | 1            | —          | —           | —           | —          | t           | N             | D1          | e                      | —            | —           | —            | V            | —            | —     | 11.388                             | 0.58                        | 1.71                        | 1                    | 38.0                               | 0.32                                 | 3.94                          | 10.993                        | 0.40        | 1.18        | 0.33 | 41.7        | 11.00       | 0.42        | 1.25 |
| 18133867−3149395 | 0.480       | −6.681      | 0.429      | 9            | —          | —           | —           | —          | —           | —             | —           | —                      | 5.977        | 0.14        | 0.79         | 1            | 162.0        | 0.76  | 4.63                               | 5.817                       | 0.07                        | 0.58                 | 0.13                               | ...                                  | ...                           | 0.08                          | 0.61        |             |      |             |             |             |      |
| 18134117−3442225 | 357.915     | −8.027      | 0.203      | 1            | —          | —           | —           | —          | —           | —             | D4          | c                      | —            | —           | —            | V            | —            | —     | 10.406                             | 0.21                        | 1.03                        | 1                    | 36.6                               | 0.92                                 | 4.45                          | 10.330                        | 0.18        | 0.93        | 0.06 | 36.9        | 10.34       | 0.18        | 0.95 |
| 18134954−3414326 | 358.343     | −7.838      | 0.225      | 2            | —          | —           | —           | —          | n           | —             | D3          | e                      | —            | —           | —            | V            | —            | —     | 10.954                             | 0.31                        | ...                         | 1                    | 47.4                               | 0.52                                 | 4.47                          | 10.870                        | 0.28        | ...         | 0.07 | 48.0        | 10.88       | 0.28        | ...  |
| 18140441−0822089 | 21.198      | 4.390       | 1.682      | 1            | —          | —           | —           | —          | t           | N             | D1          | c                      | —            | —           | —            | V            | c            | —     | 11.055                             | 0.49                        | 1.70                        | 1                    | 61.4                               | 0.54                                 | 4.34                          | 10.428                        | 0.21        | 0.86        | 0.52 | 72.1        | 10.43       | 0.24        | 0.97 |
| 18140664−1756061 | 12.786      | −0.178      | 130.932    | 8            | —          | —           | —           | —          | —           | —             | —           | —                      | 8.852        | 1.48        | 2.95         | 1            | 80.6         | 0.66  | 4.70                               | −39.933                     | −20.20                      | −6                   |                                    |                                      |                               |                               |             |             |      |             |             |             |      |

Table B1: a) continued.

| 2MASX J          | <i>l</i>    | <i>b</i>    | EBV        | Object       | Sample         | Disc        | 2MRS       | Velocity    | NIR           | Photom      | Ext | <i>K</i> <sub>20</sub> | <i>H-K</i>  | <i>J-K</i>  | vc          | <i>a</i>    | <i>b/a</i> | st.d.       | <i>K</i> <sub>s</sub> <sup>o</sup> | ( <i>H-K</i> ) <sup>o</sup> | ( <i>J-K</i> ) <sup>o</sup> | <i>A<sub>K</sub></i> | <i>a</i> <sub>d</sub> <sup>o</sup> | <i>K</i> <sub>s</sub> <sup>o,d</sup> | ( <i>H-K</i> ) <sup>o,c</sup> | ( <i>J-K</i> ) <sup>o,c</sup> |             |       |             |             |             |        |
|------------------|-------------|-------------|------------|--------------|----------------|-------------|------------|-------------|---------------|-------------|-----|------------------------|-------------|-------------|-------------|-------------|------------|-------------|------------------------------------|-----------------------------|-----------------------------|----------------------|------------------------------------|--------------------------------------|-------------------------------|-------------------------------|-------------|-------|-------------|-------------|-------------|--------|
| (1)              | deg<br>(2a) | deg<br>(2b) | mag<br>(3) | class<br>(4) | off flg<br>(5) | gal<br>(7a) | TF<br>(7b) | obs<br>(7c) | ext'd<br>(7d) | type<br>(8) | (9) | Opt<br>(10a)           | HI<br>(10b) | flg<br>(11) | flg<br>(12) | flg<br>(13) | (14)       | mag<br>(15) | mag<br>(16)                        | (17)                        | (18)                        | (19)                 | (20)                               | mag<br>(21)                          | mag<br>(22)                   | mag<br>(23)                   | mag<br>(24) | (25)  | mag<br>(26) | mag<br>(27) | mag<br>(28) |        |
| 18202335−0117447 | 28.217      | 6.307       | 1.587      | 1            | −              | −           | g          | t           | N             | −           | D1  | −                      | −           | −           | V           | −           | −          | 11.472      | 0.51                               | 1.69                        | 1                           | 52.6                 | 0.20                               | 4.04                                 | 10.881                        | 0.25                          | 0.90        | 0.49  | 63.6        | 10.81       | 0.28        | 1.00   |
| 18202669−1611186 | 15.042      | −0.682      | 107.301    | 9            | −              | −           | −          | −           | −             | −           | −   | −                      | −           | −           | −           | −           | −          | 4.449       | 1.34                               | 2.36                        | 1                           | 151.6                | 0.42                               | 4.68                                 | −35.531                       | −16.43                        | −50.94      | 33.24 | ...         | ...         | −14.32      | −43.86 |
| 18202863−1612116 | 15.033      | −0.695      | 102.589    | 9            | −              | −           | −          | −           | −             | −           | −   | −                      | −           | −           | −           | −           | −          | 6.786       | ...                                | ...                         | 1                           | 45.0                 | 1.00                               | 4.68                                 | −31.439                       | ...                           | ...         | 31.78 | ...         | ...         | ...         | ...    |
| 18202912−1613396 | 15.012      | −0.709      | 93.620     | 9            | −              | −           | −          | −           | −             | −           | −   | −                      | −           | −           | −           | −           | −          | 5.057       | 1.37                               | 2.24                        | 1                           | 135.6                | 0.64                               | 4.68                                 | −29.826                       | −14.14                        | −44.27      | 29.00 | ...         | ...         | −12.30      | −38.09 |
| 18203316−0121387 | 28.178      | 6.241       | 1.634      | 1            | −              | −           | g          | −           | N             | −           | D2  | −                      | −           | −           | V           | −           | −          | 10.150      | 0.48                               | 1.62                        | 1                           | 47.0                 | 0.88                               | 4.04                                 | 9.541                         | 0.21                          | 0.81        | 0.51  | 54.5        | 9.55        | 0.25        | 0.91   |
| 18203384−1615226 | 14.996      | −0.739      | 79.916     | 8            | −              | −           | −          | −           | −             | −           | −   | −                      | −           | −           | U           | −           | −          | 8.302       | ...                                | ...                         | 1                           | 41.4                 | 0.20                               | 4.68                                 | −21.475                       | ...                           | ...         | 24.75 | ...         | ...         | ...         | ...    |
| 18203391−1608106 | 15.102      | −0.682      | 104.518    | 9            | −              | −           | −          | −           | −             | −           | −   | −                      | −           | −           | −           | −           | −          | 4.639       | 1.12                               | 1.81                        | 1                           | 216.4                | 0.38                               | 4.60                                 | −34.304                       | −16.19                        | −50.12      | 32.37 | ...         | ...         | −14.14      | −43.22 |
| 18203766−1608306 | 15.104      | −0.698      | 97.562     | 9            | −              | −           | −          | −           | −             | −           | −   | −                      | −           | −           | −           | −           | −          | 5.390       | 1.08                               | 1.63                        | 1                           | 109.8                | 0.58                               | 4.60                                 | −30.962                       | −15.07                        | −46.84      | 30.22 | ...         | ...         | −13.16      | −40.40 |
| 18204092−1609406 | 15.093      | −0.719      | 91.481     | 9            | −              | −           | −          | −           | −             | −           | −   | −                      | −           | −           | −           | −           | −          | 5.214       | 1.00                               | 1.43                        | 1                           | 110.2                | 0.58                               | 4.60                                 | −28.872                       | −14.14                        | −44.02      | 28.34 | ...         | ...         | −12.35      | −37.98 |
| 18204395−1609120 | 15.106      | −0.726      | 85.620     | 9            | −              | −           | −          | −           | −             | −           | −   | −                      | −           | −           | −           | −           | −          | 5.662       | ...                                | 1.80                        | 1                           | 141.2                | 0.74                               | 4.84                                 | −26.240                       | ...                           | −40.73      | 26.52 | ...         | ...         | ...         | −35.08 |
| 18204506−1609580 | 15.096      | −0.736      | 83.120     | 9            | −              | −           | −          | −           | −             | −           | −   | −                      | −           | −           | −           | −           | −          | 5.532       | 1.03                               | 1.40                        | 1                           | 124.2                | 0.68                               | 4.84                                 | −25.439                       | −12.73                        | −39.89      | 25.75 | ...         | ...         | −11.10      | −34.41 |
| 18212385−0601552 | 24.123      | 3.886       | 1.200      | 8            | −              | −           | p          | −           | −             | −           | −   | −                      | −           | −           | U           | −           | −          | 11.526      | ...                                | 1.12                        | 1                           | 16.0                 | 0.94                               | 4.46                                 | 11.079                        | ...                           | 0.52        | 0.37  | ...         | ...         | ...         | 0.60   |
| 18215137+0621323 | 35.270      | 9.460       | 0.311      | 1            | −              | −           | g          | −           | −             | −           | D1  | c                      | o           | −           | −           | −           | −          | 10.134      | 0.32                               | 1.02                        | 1                           | 69.4                 | 0.60                               | 3.82                                 | 10.018                        | 0.26                          | 0.86        | 0.10  | 70.5        | 10.03       | 0.27        | 0.88   |
| 18215540−0238478 | 27.191      | 5.343       | 2.094      | 1            | −              | −           | g          | −           | N             | −           | n   | −                      | −           | −           | U           | −           | −          | 11.649      | 0.63                               | 1.86                        | 1                           | 24.4                 | 0.74                               | 4.19                                 | 10.869                        | 0.28                          | 0.82        | 0.65  | 30.4        | 10.85       | 0.33        | 0.96   |
| 18221558−0705051 | 23.290      | 3.205       | 1.455      | 1            | −              | −           | g          | −           | N             | −           | d3  | −                      | −           | −           | −           | −           | −          | 10.833      | ...                                | ...                         | 1                           | 32.0                 | 0.86                               | 4.55                                 | 10.291                        | ...                           | ...         | 0.45  | 36.6        | 10.30       | ...         | ...    |
| 18221913−0449343 | 25.299      | 4.245       | 1.634      | 1            | −              | −           | g          | −           | N             | −           | D1  | −                      | −           | −           | U           | −           | −          | 11.495      | 0.59                               | 1.76                        | 1                           | 31.2                 | 0.70                               | 4.37                                 | 10.886                        | 0.32                          | 0.95        | 0.51  | 37.7        | 10.83       | 0.36        | 1.05   |
| 18222131−0156593 | 27.862      | 5.570       | 1.821      | 9            | −              | −           | −          | −           | −             | −           | −   | −                      | −           | −           | −           | −           | −          | 10.157      | 0.93                               | ...                         | 1                           | 92.4                 | 0.22                               | 4.14                                 | 9.478                         | 0.63                          | ...         | 0.56  | ...         | ...         | 0.66        | ...    |
| 18223005−0232323 | 27.353      | 5.265       | 1.883      | 1            | −              | −           | g          | t           | N             | −           | D1  | −                      | −           | −           | U           | −           | −          | 10.650      | 0.48                               | 1.52                        | 1                           | 56.2                 | 0.32                               | 4.17                                 | 9.948                         | 0.17                          | 0.59        | 0.58  | 68.2        | 9.94        | 0.20        | 0.71   |
| 18234211−3022092 | 2.784       | −7.922      | 0.267      | 9            | −              | −           | −          | −           | −             | −           | −   | −                      | −           | −           | −           | −           | −          | 7.494       | 0.15                               | 0.57                        | 1                           | 202.0                | 0.10                               | 4.50                                 | 7.395                         | 0.11                          | 0.43        | 0.08  | ...         | ...         | 0.12        | 0.45   |
| 18235170−3112061 | 2.049       | −8.328      | 0.232      | 2            | −              | −           | g          | −           | −             | −           | n   | c                      | o           | −           | V           | −           | −          | 11.216      | 0.40                               | 1.02                        | 1                           | 34.2                 | 0.92                               | 4.41                                 | 11.130                        | 0.36                          | 0.91        | 0.07  | 34.6        | 11.14       | 0.36        | 0.92   |
| 18242335−3410546 | 359.398     | −9.758      | 0.130      | 1            | −              | −           | g          | −           | −             | −           | d1  | c                      | o           | h           | V           | −           | −          | 10.068      | 0.27                               | 1.02                        | 1                           | 47.8                 | 0.68                               | 4.20                                 | 10.020                        | 0.25                          | 0.95        | 0.04  | 48.0        | 10.03       | 0.25        | 0.96   |
| 18243232−2452325 | 7.792       | −5.581      | 0.488      | 9            | −              | −           | g          | −           | −             | −           | −   | −                      | −           | −           | −           | −           | −          | 6.674       | 0.13                               | 0.73                        | 1                           | 52.2                 | 0.40                               | 4.73                                 | 6.492                         | 0.05                          | 0.49        | 0.15  | ...         | ...         | 0.06        | 0.52   |
| 18243841+0149078 | 31.494      | 6.791       | 1.222      | 1            | −              | −           | g          | t           | N             | −           | D1  | e                      | o           | h           | −           | −           | −          | 10.145      | 0.41                               | 1.42                        | 1                           | 72.8                 | 0.42                               | 3.99                                 | 9.690                         | 0.21                          | 0.82        | 0.38  | 80.2        | 9.71        | 0.23        | 0.90   |
| 18244489−1808155 | 13.802      | −2.503      | 1.127      | 8            | −              | −           | −          | −           | −             | −           | −   | −                      | −           | −           | −           | −           | −          | 7.293       | 0.70                               | 1.52                        | −2                          | 52.2                 | 0.34                               | 4.80                                 | 6.873                         | 0.51                          | 0.96        | 0.35  | ...         | ...         | 0.53        | 1.03   |
| 18251151+0201241 | 31.740      | 6.762       | 1.057      | 1            | −              | −           | g          | t           | N             | −           | D1  | e                      | o           | −           | −           | −           | −          | 9.781       | 0.39                               | 1.39                        | 1                           | 88.6                 | 0.26                               | 4.03                                 | 9.387                         | 0.22                          | 0.86        | 0.33  | 95.9        | 9.41        | 0.24        | 0.93   |
| 18252596−3030448 | 2.824       | −8.320      | 0.306      | 2            | −              | −           | −          | −           | −             | −           | D4  | c                      | o           | −           | V           | −           | −          | 10.705      | 0.38                               | 1.11                        | 1                           | 41.4                 | 0.86                               | 4.44                                 | 10.591                        | 0.33                          | 0.96        | 0.09  | 42.1        | 10.60       | 0.33        | 0.98   |
| 18254229−1310191 | 18.303      | −0.390      | 28.735     | 8            | −              | −           | −          | −           | −             | −           | −   | −                      | −           | −           | −           | −           | −          | 8.260       | ...                                | ...                         | 1                           | 66.0                 | 0.74                               | 4.86                                 | −2.447                        | ...                           | ...         | 8.90  | ...         | ...         | ...         | ...    |
| 18254245−2312102 | 9.407       | −5.059      | 0.647      | 8            | −              | −           | p          | −           | −             | −           | −   | −                      | −           | −           | V           | −           | −          | 9.616       | 0.63                               | 0.81                        | 1                           | 29.2                 | 0.88                               | 4.66                                 | 9.375                         | 0.52                          | 0.49        | 0.20  | ...         | ...         | 0.53        | 0.53   |
| 18260722−1209120 | 19.251      | −0.005      | 21.052     | 9            | −              | −           | −          | −           | −             | −           | −   | −                      | −           | −           | −           | −           | −          | 7.364       | 0.77                               | ...                         | 2                           | 113.2                | 0.58                               | 4.87                                 | −0.480                        | −2.71                         | ...         | 6.52  | ...         | ...         | −2.30       | ...    |
| 18261102+0058105 | 30.910      | 6.060       | 1.600      | 1            | −              | −           | g          | t           | N             | −           | D2  | e                      | o           | −           | −           | −           | −          | 11.842      | 0.39                               | 1.51                        | 1                           | 22.6                 | 0.70                               | 4.04                                 | 11.246                        | 0.13                          | 0.71        | 0.50  | 26.3        | 11.25       | 0.16        | 0.82   |
| 18262863−3132588 | 1.986       | −8.983      | 0.257      | 1            | −              | −           | g          | t           | N             | −           | D1  | e                      | o           | h           | V           | −           | −          | 10.498      | 0.40                               | 1.15                        | 1                           | 58.0                 | 0.50                               | 4.34                                 | 10.402                        | 0.36                          | 1.03        | 0.08  | 58.8        | 10.41       | 0.37        | 1.04   |
| 18263588+0221130 | 32.197      | 6.599       | 1.038      | 1            | −              | −           | g          | t           | N             | −           | D1  | e                      | o           | −           | −           | −           | −          | 11.317      | 0.52                               | 1.68                        | 1                           | 32.2                 | 0.36                               | 4.00                                 | 10.930                        | 0.35                          | 1.17        | 0.32  | 35.3        | 10.93       | 0.37        | 1.23   |
| 18273375−0348416 | 26.808      | 3.557       | 20.210     | 9            | −              | −           | g          | −           | −             | −           | −   | −                      | −           | −           | −           | −           | −          | 11.882      | ...                                | ...                         | 1                           | 36.2                 | 0.74                               | 4.12                                 | 4.352                         | ...                           | ...         | 6.26  | ...         | ...         | ...         | ...    |
| 18273481−0350226 | 26.785      | 3.540       | 19.290     | 9            | −              | −           | g          | −           | −             | −           | −   | −                      | −           | −           | −           | −           | −          | 10.153      | 1.10                               | 2.00                        | 1                           | 65.2                 | 0.60                               | 4.12                                 | 2.966                         | −2.10                         | −7.58       | 5.98  | ...         | ...         | −1.72       | −6.31  |
| 18273769−0348176 | 26.821      | 3.545       | 22.023     | 9            | −              | −           | g          | −           | −             | −           | −   | −                      | −           | −           | −           | −           | −          | 9.527       | ...                                | ...                         | 1                           | 109.8                | 0.56                               | 4.12                                 | 1.321                         | ...                           | ...         | 6.82  | ...         | ...         | ...         | ...    |
| 18275944+0031420 | 30.723      | 5.457       | 2.011      | 1            | −              | −           | g          | t           | N             | −           | D1  | −                      | −           | −           | −           | −           | −          | 11.577      | 0.68                               | 1.89                        | 1                           | 38.8                 | 0.54                               | 4.10                                 | 10.828                        | 0.34                          | 0.89        | 0.62  | 49.2        | 10.76       | 0.38        | 1.03   |
| 18282690+0032151 | 30.784      | 5.359       | 2.316      | 1            | −              | −           | g          | t           | N             | −           | D3  | −                      | −           | −           | U           | −           | −          | 12.019      | 0.95                               | ...                         | 1                           | 21.8                 | 0.82                               | 4.00                                 | 11.156                        | 0.57                          | ...         | 0.72  | 28.8        | 11.08       | 0.61        | ...    |
| 18282772−0307325 | 27.521      | 3.674       | 2.756      | 1            | o              | −           | −          | −           | −             | −           | D1  | −                      | −           | −           | o           | e?          | −          | 12.100      | 0.71                               | ...                         | 1                           | 23.4                 | 0.58                               | 4.34                                 | 11.073                        | 0.25                          | ...         | 0.85  | 33.4        | 10.96       | 0.30        | ...    |
| 18285975+0648277 | 36.478      | 8.074       | 0.299      | 1            | −              | −           | g          | −           | −             | −           | D4  | c                      | o           | −           | −           | −           | −          | 9.588       | 0.28                               | 1.03                        | 1                           | 58.2                 | 0.68                               | 3.94                                 | 9.477                         | 0.23                          | 0.88        | 0.09  | 59.0        | 9.49        | 0.23        | 0.90   |
| 18290219+0029401 | 30.813      | 5.209       | 2.401      | 8            | −              | −           | −          | −           | −             | −           | −   | −                      | −           | −           | U           | −           | −          | 10.125      | 0.57                               | 1.50                        | 1                           | 115.2                | 0.84                               | 3.94                                 | 9.230                         | 0.17                          | 0.31        | 0.74  | ...         | ...         | 0.22        | 0.46   |
| 18290286+0030091 | 30.822      | 5.210       | 2.403      | 8            | −              | −           | −          | −           | −             | −           | −   | −                      | −           | −           | U           | −           | −          | 10.212      | 0.76                               | 1.77                        | 1                           | 73.0                 | 0.38                               | 3.94                                 | 9.317                         | 0.36                          | 0.57        | 0.74  | ...         | ...         | 0.41        | 0.73   |
| 18293900−0151067 | 28.792      | 3.997       | 1.705      | 9            | −              | −           | −          | −           | −             | −           | −   | −                      | −           | −           | −           | −           | −          | 10.900      | 2.09                               | ...                         | 1                           | 38.4                 | 0.76                               | 3.90                                 | 10.265                        | 1.81                          | ...         | 0.53  | ...         | ...         | 1.85        | ...    |
| 18294926+0116257 | 31.599      | 5.390       | 8.037      | 9            | −              | −           | −          | −           | −             | −           | −   | −                      | −           | −           | −           | −           | −          | 12.441      | ...                                | ...                         | 1                           | 20.8                 | 1.0                                | 3.94                                 | 9.446                         | ...                           | ...         | 2.49  | ...         | ...         | ...         | ...    |
| 18295106+0116397 | 31.606      | 5.385       | 8.029      | 8            | −              | −           | −          | −           | −             |             |     |                        |             |             |             |             |            |             |                                    |                             |                             |                      |                                    |                                      |                               |                               |             |       |             |             |             |        |

Table B1: a) continued.

[illegible]

Table B1: a) continued.

| 2MASX J          | $l$    | $b$    | EBV     | Object | Sample | Disc | 2MRS | Velocity | NIR   | Photom | Ext | $K_{20}$ | $H-K$ | $J-K$ | vc    | $a$   | $b/a$ | st.d. | $K_s^o$ | $(H-K)^o$ | $(J-K)^o$ | $A_K$ | $a_d^H$ | $K_s^{o,d}$ | $(H-K)^{o,c}$ | $(J-K)^{o,c}$ |       |        |       |      |       |      |       |       |        |      |
|------------------|--------|--------|---------|--------|--------|------|------|----------|-------|--------|-----|----------|-------|-------|-------|-------|-------|-------|---------|-----------|-----------|-------|---------|-------------|---------------|---------------|-------|--------|-------|------|-------|------|-------|-------|--------|------|
| (1)              | deg    | deg    | mag     | class  | off    | gal  | TF   | Obs      | ext'd | type   |     |          | mag   | mag   |       | "     |       |       | mag     | mag       | mag       | mag   | "       | mag         | mag           | mag           |       |        |       |      |       |      |       |       |        |      |
| (1)              | (2a)   | (2b)   | (3)     | (4)    | (5)    | (6)  | (7a) | (7b)     | (7c)  | (7d)   | (8) | (9)      | Opt   | HI    | (10a) | (10b) | (11)  | flag  | flag    | flag      | (13)      | (14)  | (15)    | (16)        | (17)          | (18)          | (19)  | (20)   | (21)  | (22) | (23)  | (24) | (25)  | (26)  | (27)   | (28) |
| 18524710+0939480 | 41.699 | 4.094  | 0.928   | 1      | —      | —    | g    | —        | N     | —      | D3  | —        | —     | —     | —     | —     | —     | —     | 11.344  | 0.48      | 1.29      | 1     | 37.8    | 0.84        | 4.27          | 10.998        | 0.33  | 0.82   | 0.29  | 41.0 | 11.00 | 0.35 | 0.89  | ...   | ...    |      |
| 18525037+0055264 | 33.914 | 0.110  | 31.750  | 8      | —      | —    | —    | —        | —     | —      | —   | —        | —     | —     | —     | —     | —     | —     | 9.264   | ...       | ...       | 1     | 68.0    | 0.76        | 4.77          | —2.566        | ...   | ...    | 9.83  | ...  | ...   | ...  | ...   | ...   | ...    | ...  |
| 18531497+0623155 | 27.446 | −3.309 | 0.641   | 2      | o      | —    | —    | —        | N     | —      | D1  | —        | —     | —     | —     | —     | —     | —     | 11.053  | 0.27      | 0.89      | 2     | 30.4    | 0.62        | 4.56          | 10.814        | 0.16  | 0.57   | 0.20  | 31.7 | 10.83 | 0.17 | 0.61  | ...   | ...    |      |
| 18532004+0114452 | 34.257 | 0.146  | 132.575 | 9      | —      | —    | —    | —        | —     | —      | —   | —        | —     | —     | —     | —     | —     | —     | 7.265   | ...       | ...       | 1     | 182.8   | 0.74        | 4.64          | −42.132       | ...   | ...    | 41.07 | ...  | ...   | ...  | ...   | ...   | ...    | ...  |
| 18532144+0113502 | 34.246 | 0.134  | 117.519 | 9      | —      | —    | —    | —        | —     | —      | —   | —        | —     | —     | —     | —     | —     | —     | 8.173   | ...       | ...       | 1     | 220.0   | 1.00        | 4.64          | −35.615       | ...   | ...    | 36.40 | ...  | ...   | ...  | ...   | ...   | ...    | ...  |
| 18534771+0951131 | 41.982 | 3.957  | 0.899   | 2      | o      | —    | —    | —        | —     | —      | D1  | —        | —     | *     | —     | —     | —     | —     | 11.095  | 0.25      | 1.14      | −2    | 51.2    | 0.60        | 4.33          | 10.760        | 0.10  | 0.70   | 0.28  | 55.8 | 10.75 | 0.12 | 0.75  | ...   | ...    |      |
| 18535531+0203574 | 35.054 | 0.390  | 26.233  | 9      | —      | —    | —    | —        | —     | —      | —   | —        | —     | —     | —     | —     | —     | —     | 8.880   | 1.57      | ...       | −2    | 90.0    | 0.50        | 4.51          | −0.894        | −2.77 | ...    | 8.13  | ...  | ...   | ...  | ...   | −2.25 | ...    |      |
| 18543884−1447321 | 20.052 | −7.381 | 0.442   | 1      | —      | —    | —    | —        | —     | —      | D1  | e        | o     | —     | —     | —     | —     | —     | 10.686  | 0.21      | 1.02      | 1     | 40.8    | 0.84        | 4.10          | 10.521        | 0.13  | 0.80   | 0.14  | 42.0 | 10.53 | 0.14 | 0.83  | ...   | ...    |      |
| 18545455−0834368 | 25.675 | −4.665 | 0.376   | 1      | —      | —    | —    | —        | —     | —      | D1  | e        | o     | —     | —     | —     | —     | —     | 11.079  | 0.29      | 1.10      | 1     | 22.4    | 0.82        | 4.41          | 10.939        | 0.23  | 0.91   | 0.12  | 22.9 | 10.95 | 0.24 | 0.93  | ...   | ...    |      |
| 18550002−0849098 | 25.468 | −4.794 | 0.353   | 1      | —      | —    | —    | —        | —     | —      | D3  | e        | o     | —     | —     | —     | —     | —     | 11.095  | 0.21      | 0.90      | 1     | 37.8    | 0.80        | 4.39          | 10.963        | 0.15  | 0.73   | 0.11  | 38.6 | 10.97 | 0.16 | 0.75  | ...   | ...    |      |
| 18552042−1146309 | 22.851 | −6.194 | 0.680   | 1      | —      | —    | —    | —        | —     | —      | D1  | e        | o     | —     | —     | —     | —     | —     | 11.332  | 0.53      | 1.41      | 1     | 32.8    | 0.62        | 4.21          | 11.079        | 0.42  | 1.07   | 0.21  | 34.7 | 11.08 | 0.43 | 1.12  | ...   | ...    |      |
| 18553355−1926100 | 15.923 | −9.603 | 0.243   | 1      | —      | —    | —    | —        | —     | —      | D1  | c        | o     | —     | —     | —     | —     | —     | 11.310  | 0.42      | 1.07      | 1     | 31.6    | 0.68        | 4.05          | 11.219        | 0.38  | 0.95   | 0.08  | 32.0 | 11.23 | 0.38 | 0.97  | ...   | ...    |      |
| 18560437+0757147 | 40.542 | 2.595  | 41.918  | 8      | —      | —    | —    | —        | —     | —      | —   | —        | —     | —     | —     | —     | —     | —     | 9.692   | 1.86      | ...       | 1     | 35.0    | 0.50        | 4.37          | −5.927        | −5.08 | ...    | 12.98 | ...  | ...   | ...  | ...   | −4.26 | ...    |      |
| 18560565+0757447 | 40.551 | 2.594  | 40.580  | 9      | —      | —    | —    | —        | —     | —      | —   | —        | —     | —     | —     | —     | —     | —     | 9.695   | ...       | ...       | 1     | 102.0   | 1.00        | 4.37          | −5.425        | ...   | ...    | 12.57 | ...  | ...   | ...  | ...   | ...   | ...    |      |
| 18561144+0754107 | 40.509 | 2.546  | 46.172  | 9      | —      | —    | —    | —        | —     | —      | —   | —        | —     | —     | —     | —     | —     | —     | 9.838   | 1.96      | ...       | 1     | 92.6    | 0.50        | 4.37          | −7.366        | −5.69 | ...    | 14.30 | ...  | ...   | ...  | ...   | −4.78 | ...    |      |
| 18561150+0753147 | 40.496 | 2.539  | 43.792  | 9      | —      | —    | —    | —        | —     | —      | —   | —        | —     | —     | —     | —     | —     | —     | 9.799   | 1.64      | 3.49      | 1     | 85.4    | 0.68        | 4.37          | −8.338        | −5.61 | −18.26 | 13.56 | ...  | ...   | ...  | ...   | −4.75 | −15.37 |      |
| 18561816+0707258 | 39.828 | 2.167  | 4.390   | 8      | —      | p    | —    | —        | —     | —      | —   | —        | —     | —     | —     | —     | —     | —     | 9.599   | 1.22      | 1.91      | 1     | 79.0    | 0.92        | 4.52          | 7.963         | 0.49  | −0.27  | 1.36  | ...  | ...   | ...  | ...   | 0.58  | 0.01   |      |
| 18565611−0613346 | 28.006 | −4.053 | 0.454   | 1      | —      | —    | —    | —        | N     | —      | D1  | —        | —     | —     | —     | —     | —     | —     | 10.205  | 0.35      | 1.18      | 1     | 42.2    | 0.88        | 4.44          | 10.036        | 0.27  | 0.95   | 0.14  | 43.3 | 10.05 | 0.28 | 0.98  | ...   | ...    |      |
| 18565657+1757433 | 49.608 | 6.909  | 0.487   | 1      | —      | —    | t    | —        | —     | —      | D1  | c        | —     | h     | —     | —     | —     | —     | 11.327  | 0.29      | 1.01      | 1     | 51.8    | 0.46        | 3.90          | 11.146        | 0.21  | 0.77   | 0.15  | 53.8 | 11.14 | 0.22 | 0.80  | ...   | ...    |      |
| 18573128−0436546 | 29.512 | −3.453 | 0.716   | 1      | —      | —    | —    | —        | N     | —      | D3  | —        | —     | —     | —     | —     | —     | —     | 11.267  | 0.49      | ...       | 1     | 27.8    | 0.74        | 4.52          | 11.000        | 0.37  | ...    | 0.22  | 29.3 | 11.01 | 0.38 | ...   | ...   | ...    | ...  |
| 18573773+0203396 | 35.472 | −0.437 | 11.378  | 8      | —      | p?   | —    | —        | —     | —      | —   | —        | —     | —     | —     | —     | —     | —     | 9.782   | 1.28      | 2.61      | 1     | 33.6    | 0.62        | 4.83          | 5.543         | −0.61 | −3.04  | 3.52  | ...  | ...   | ...  | ...   | −0.38 | −2.29  |      |
| 18581124+0136580 | 35.140 | −0.764 | 28.374  | 9      | —      | —    | —    | —        | —     | —      | —   | —        | —     | —     | —     | —     | —     | —     | 8.278   | 1.48      | 2.82      | 1     | 145.2   | 0.60        | 4.58          | −2.294        | −3.22 | −11.27 | 8.79  | ...  | ...   | ...  | ...   | −2.66 | −9.40  |      |
| 18581256+0140260 | 35.194 | −0.743 | 28.351  | 8      | —      | —    | —    | —        | —     | —      | —   | —        | —     | —     | —     | —     | —     | —     | 8.368   | ...       | ...       | 1     | 159.2   | 0.18        | 4.58          | −2.196        | ...   | ...    | 8.78  | ...  | ...   | ...  | ...   | ...   | ...    | ...  |
| 18582963−0933358 | 25.192 | −5.897 | 0.339   | 1      | —      | —    | —    | —        | —     | —      | D1  | e        | o     | —     | —     | —     | —     | —     | 10.681  | 0.36      | 1.09      | 1     | 48.2    | 0.56        | 4.27          | 10.555        | 0.30  | 0.92   | 0.11  | 49.1 | 10.57 | 0.31 | 0.94  | ...   | ...    |      |
| 18583627+1137375 | 44.103 | 3.707  | 0.898   | 1      | —      | —    | —    | —        | N     | —      | D1  | —        | —     | —     | —     | —     | —     | —     | 10.771  | 0.40      | 1.33      | 1     | 36.6    | 0.88        | 4.32          | 10.436        | 0.25  | 0.88   | 0.28  | 39.3 | 10.45 | 0.27 | 0.94  | ...   | ...    |      |
| 18590713+0702589 | 40.080 | 1.511  | 12.921  | 8      | —      | —    | —    | —        | —     | —      | —   | —        | —     | —     | —     | —     | —     | —     | 10.313  | 1.28      | ...       | 1     | 41.8    | 0.42        | 4.58          | 5.499         | −0.86 | ...    | 4.00  | ...  | ...   | ...  | ...   | −0.60 | ...    |      |
| 18591407+0704485 | 40.120 | 1.499  | 15.456  | 7      | —      | —    | —    | —        | —     | —      | —   | —        | —     | —     | —     | —     | —     | —     | 9.215   | 1.59      | ...       | 1     | 51.2    | 0.72        | 4.55          | 3.456         | −0.97 | ...    | 4.79  | ...  | ...   | ...  | ...   | −0.67 | ...    |      |
| 18591639+1919573 | 51.092 | 7.022  | 0.510   | 1      | —      | —    | t    | —        | —     | —      | D1  | c        | o     | —     | h     | *     | —     | —     | 10.631  | 0.43      | 1.29      | 1     | 59.8    | 0.46        | 3.90          | 10.441        | 0.34  | 1.03   | 0.16  | 62.2 | 10.44 | 0.35 | 1.07  | ...   | ...    |      |
| 18591780+1316371 | 45.654 | 4.303  | 0.919   | 1      | —      | —    | —    | —        | —     | —      | D1  | c        | o     | —     | —     | —     | —     | —     | 10.470  | 0.39      | 1.30      | 1     | 33.0    | 0.80        | 4.16          | 10.128        | 0.24  | 0.84   | 0.28  | 35.4 | 10.15 | 0.25 | 0.91  | ...   | ...    |      |
| 18593477+1906217 | 50.920 | 6.857  | 0.593   | 1      | —      | —    | —    | —        | —     | —      | D2  | c        | o     | —     | —     | —     | —     | —     | 9.155   | 0.30      | 1.16      | 1     | 81.2    | 0.70        | 3.91          | 8.934         | 0.21  | 0.87   | 0.18  | 84.0 | 8.96  | 0.22 | 0.91  | ...   | ...    |      |
| 18593645+1925387 | 51.213 | 6.993  | 0.529   | 1      | —      | —    | —    | —        | —     | —      | D1  | c        | o     | —     | h     | —     | —     | —     | 10.352  | 0.29      | 1.05      | 1     | 64.4    | 0.70        | 3.90          | 10.155        | 0.20  | 0.79   | 0.16  | 67.2 | 10.15 | 0.21 | 0.83  | ...   | ...    |      |
| 18594719+1849497 | 50.693 | 6.690  | 0.621   | 1      | —      | —    | t    | —        | —     | —      | D1  | c        | o     | —     | h     | —     | —     | —     | 9.868   | 0.33      | 1.19      | 1     | 91.0    | 0.24        | 3.93          | 9.637         | 0.22  | 0.88   | 0.19  | 94.9 | 9.65  | 0.24 | 0.92  | ...   | ...    |      |
| 18595195−0928549 | 25.414 | −6.165 | 0.401   | 1      | —      | —    | —    | —        | —     | —      | D2  | c        | o     | —     | —     | —     | —     | —     | 10.823  | 0.33      | 1.06      | 1     | 38.4    | 0.86        | 4.21          | 10.674        | 0.26  | 0.86   | 0.12  | 39.3 | 10.69 | 0.27 | 0.89  | ...   | ...    |      |
| 19001580−1412185 | 21.188 | −8.344 | 0.333   | 1      | —      | —    | —    | —        | —     | —      | D1  | c        | o     | —     | —     | —     | —     | —     | 11.332  | 0.39      | 1.11      | 1     | 37.0    | 0.64        | 4.07          | 11.208        | 0.34  | 0.94   | 0.10  | 37.8 | 11.21 | 0.34 | 0.96  | ...   | ...    |      |
| 19004514+1741359 | 49.773 | 5.977  | 0.624   | 1      | —      | —    | t    | N        | —     | —      | cp  | —        | —     | —     | —     | —     | —     | —     | 11.469  | 0.47      | 1.57      | 1     | 56.8    | 0.14        | 3.99          | 11.236        | 0.37  | 1.26   | 0.19  | 60.0 | 11.23 | 0.38 | 1.30  | ...   | ...    |      |
| 19004973−0322063 | 31.000 | −3.623 | 0.961   | 1      | —      | —    | —    | —        | N     | —      | D1  | —        | —     | —     | —     | —     | —     | —     | 11.281  | 0.42      | 1.41      | 1     | 23.6    | 0.76        | 4.42          | 10.923        | 0.26  | 0.93   | 0.30  | 25.4 | 10.94 | 0.28 | 0.99  | ...   | ...    |      |
| 19005281+0643153 | 39.987 | 0.972  | 5.698   | 8      | —      | —    | —    | —        | —     | —      | —   | —        | —     | —     | —     | —     | —     | —     | 9.488   | 0.92      | ...       | 1     | 24.0    | 0.38        | 4.74          | 7.365         | −0.02 | ...    | 1.76  | ...  | ...   | ...  | 0.09  | ...   |        |      |
| 19014208+0113308 | 35.193 | −1.724 | 64.284  | 8      | —      | —    | —    | —        | —     | —      | —   | —        | —     | —     | —     | —     | —     | —     | 10.704  | 1.60      | ...       | 1     | 22.4    | 0.70        | 4.52          | −13.248       | −9.04 | ...    | 19.91 | ...  | ...   | ...  | −7.78 | ...   |        |      |
| 19014488+0112488 | 35.188 | −1.739 | 63.806  | 9      | —      | —    | —    | —        | —     | —      | —   | —        | —     | —     | —     | —     | —     | —     | 9.059   | 1.78      | ...       | 1     | 72.2    | 0.32        | 4.52          | −14.715       | −8.78 | ...    | 19.76 | ...  | ...   | ...  | −7.53 | ...   |        |      |
| 19014668+0113228 | 35.200 | −1.742 | 69.414  | 8      | —      | —    | —    | —        | —     | —      | —   | —        | —     | —     | —     | —     | —     | —     | 8.862   | 2.18      | ...       | 1     | 45.6    | 0.42        | 4.52          | −17.002       | −9.31 | ...    | 21.50 | ...  | ...   | ...  | −7.95 | ...   |        |      |
| 19014715+0112468 | 35.192 | −1.748 | 64.584  | 9      | —      | —    | —    | —        | —     | —      | —   | —        | —     | —     | —     | —     | —     | —     | 8.361   | ...       | ...       | 1     | 123.6   | 0.22        | 4.52          | −15.703       | ...   | ...    | 20.01 | ...  | ...   | ...  | ...   | ...</ |        |      |

Table B1: a) continued.

| 2MASX J          | <i>l</i> | <i>b</i> | EBV    | Object | Sample | Disc | 2MRS | Velocity | NIR   | Photom | Ext   | <i>K</i> <sub>20</sub> | <i>H-K</i> | <i>J-K</i> | vc   | <i>a</i> | <i>b/a</i> | st.d. | <i>K</i> <sub>s</sub> <sup>o</sup> | ( <i>H-K</i> ) <sup>o</sup> | ( <i>J-K</i> ) <sup>o</sup> | <i>A<sub>K</sub></i> | <i>a</i> <sub>d</sub> <sup>o</sup> | <i>K</i> <sub>s</sub> <sup>o,d</sup> | ( <i>H-K</i> ) <sup>o,c</sup> | ( <i>J-K</i> ) <sup>o,c</sup> |       |        |       |       |       |       |        |
|------------------|----------|----------|--------|--------|--------|------|------|----------|-------|--------|-------|------------------------|------------|------------|------|----------|------------|-------|------------------------------------|-----------------------------|-----------------------------|----------------------|------------------------------------|--------------------------------------|-------------------------------|-------------------------------|-------|--------|-------|-------|-------|-------|--------|
| (1)              | deg      | deg      | mag    | class  | off    | gal  | TF   | obs      | ext'd | type   | Opt   | HI                     | mag        | mag        | (17) | (18)     | (19)       | (20)  | mag                                | mag                         | mag                         | mag                  | (25)                               | mag                                  | mag                           | mag                           |       |        |       |       |       |       |        |
| (2a)             | (2b)     | (3)      | (4)    | (5)    | (6)    | (7a) | (7b) | (7c)     | (7d)  | (8)    | (10a) | (10b)                  | (11)       | (12)       | (13) | (14)     | (15)       | (16)  | (17)                               | (18)                        | (19)                        | (20)                 | (21)                               | (22)                                 | (23)                          | (24)                          | (28)  |        |       |       |       |       |        |
| 19113555+2352023 | 56.466   | 6.489    | 0.689  | 1      | –      | –    | –    | –        | –     | D1     | c     | o                      | –          | –          | –    | –        | –          | –     | 10.884                             | 0.35                        | 1.22                        | 1                    | 38.4                               | 0.64                                 | 3.92                          | 10.627                        | 0.24  | 0.88   | 0.21  | 40.4  | 10.64 | 0.25  | 0.93   |
| 19115165+0949402 | 43.995   | −0.012   | 13.214 | 7      | –      | –    | –    | –        | –     | –      | –     | –                      | –          | –          | –    | –        | –          | –     | 8.651                              | 2.08                        | ...                         | 1                    | 70.8                               | 0.50                                 | 4.70                          | 3.727                         | −0.11 | ...    | 4.09  | ...   | 0.15  | ...   |        |
| 19120105+2043284 | 53.696   | 4.975    | 1.090  | 1      | –      | –    | –    | –        | –     | D3     | –     | –                      | –          | –          | –    | –        | –          | –     | 11.467                             | 0.44                        | 1.40                        | 1                    | 36.6                               | 0.52                                 | 4.07                          | 11.061                        | 0.26  | 0.86   | 0.34  | 40.5  | 11.06 | 0.29  | 0.93   |
| 19121114+0852222 | 43.186   | −0.525   | 14.115 | 8      | –      | –    | –    | –        | –     | –      | –     | –                      | –          | –          | –    | –        | –          | –     | 9.816                              | ...                         | ...                         | 1                    | 60.4                               | 0.88                                 | 4.62                          | 4.557                         | ...   | ...    | 4.37  | ...   | ...   | ...   |        |
| 19123868+2228570 | 55.334   | 5.646    | 0.765  | 1      | –      | –    | –    | –        | –     | D1     | c     | o                      | –          | –          | –    | –        | –          | –     | 10.770                             | 0.40                        | 1.26                        | 1                    | 36.4                               | 0.86                                 | 4.03                          | 10.485                        | 0.27  | 0.88   | 0.24  | 38.5  | 10.50 | 0.29  | 0.93   |
| 19123993+1728258 | 50.870   | 3.348    | 1.521  | 1      | –      | –    | –    | –        | –     | D1     | –     | –                      | –          | –          | –    | –        | –          | –     | 11.317                             | 0.38                        | 1.34                        | 1                    | 23.6                               | 0.84                                 | 4.29                          | 10.750                        | 0.13  | 0.59   | 0.47  | 27.4  | 10.74 | 0.15  | 0.69   |
| 19124311−0356087 | 31.841   | −6.524   | 0.702  | 1      | –      | –    | –    | –        | –     | D1     | c     | o                      | –          | –          | –    | –        | –          | –     | 10.500                             | 0.40                        | 1.19                        | 1                    | 53.2                               | 0.90                                 | 4.05                          | 10.238                        | 0.29  | 0.84   | 0.22  | 56.4  | 10.24 | 0.30  | 0.89   |
| 19124699+0256056 | 37.985   | −3.400   | 0.919  | 1      | –      | –    | –    | –        | –     | D1     | –     | –                      | –          | –          | –    | –        | –          | –     | 10.790                             | 0.36                        | ...                         | 1                    | 52.0                               | 0.64                                 | 4.43                          | 10.448                        | 0.21  | ...    | 0.28  | 56.7  | 10.43 | 0.22  | ...    |
| 19132691+1054273 | 45.133   | 0.142    | 49.918 | 9      | –      | –    | –    | –        | –     | –      | –     | –                      | –          | –          | –    | –        | –          | –     | 7.661                              | 1.43                        | 2.84                        | 1                    | 142.8                              | 0.80                                 | 4.69                          | −10.938                       | −6.84 | −21.95 | 15.46 | ...   | ...   | −5.86 | −18.66 |
| 19135226+1655279 | 50.515   | 2.839    | 2.321  | 1      | –      | –    | –    | –        | –     | D1     | –     | –                      | –          | –          | –    | –        | –          | –     | 10.105                             | 0.65                        | 1.78                        | 1                    | 108.0                              | 0.16                                 | 4.44                          | 9.240                         | 0.26  | 0.63   | 0.72  | 141.1 | 9.19  | 0.31  | 0.78   |
| 19140875+1112237 | 45.477   | 0.130    | 54.997 | 9      | –      | –    | –    | –        | –     | –      | –     | –                      | –          | –          | –    | –        | –          | –     | 8.107                              | ...                         | ...                         | 1                    | 132.2                              | 0.40                                 | 4.67                          | −12.385                       | ...   | ...    | 17.04 | ...   | ...   | ...   | ...    |
| 19142126+1929285 | 52.849   | 3.922    | 1.430  | 1      | –      | –    | –    | –        | –     | D1     | e     | –                      | –          | –          | –    | –        | –          | –     | 11.067                             | 0.43                        | 1.42                        | 1                    | 28.4                               | 0.86                                 | 4.20                          | 10.534                        | 0.19  | 0.71   | 0.44  | 32.5  | 10.53 | 0.22  | 0.81   |
| 19142128+1109117 | 45.454   | 0.059    | 65.033 | 8      | –      | –    | –    | –        | –     | –      | –     | –                      | –          | –          | –    | –        | –          | –     | 7.753                              | 1.69                        | ...                         | 1                    | 140.2                              | 0.58                                 | 4.66                          | −16.478                       | −9.08 | ...    | 20.14 | ...   | ...   | −7.80 | ...    |
| 19142607+0922347 | 43.889   | −0.783   | 13.039 | 7      | –      | –    | –    | –        | –     | –      | –     | –                      | –          | –          | –    | –        | –          | –     | 10.677                             | ...                         | ...                         | 1                    | 40.2                               | 1.00                                 | 4.61                          | 5.229                         | ...   | ...    | 4.04  | ...   | ...   | ...   | ...    |
| 19150245+2010197 | 53.530   | 4.092    | 1.571  | 1      | –      | –    | –    | –        | –     | D1     | –     | –                      | –          | –          | –    | –        | –          | –     | 9.679                              | 0.42                        | 1.44                        | 1                    | 77.2                               | 0.58                                 | 4.16                          | 9.094                         | 0.16  | 0.65   | 0.49  | 89.6  | 9.10  | 0.19  | 0.76   |
| 19151500+0434501 | 39.732   | −3.187   | 1.522  | 1      | –      | –    | –    | –        | –     | D2     | –     | –                      | –          | –          | –    | –        | –          | –     | 11.240                             | 0.38                        | 1.40                        | 1                    | 32.4                               | 0.44                                 | 4.39                          | 10.673                        | 0.12  | 0.64   | 0.47  | 37.3  | 10.68 | 0.15  | 0.74   |
| 19151937+1013060 | 44.737   | −0.586   | 13.396 | 8      | –      | –    | –    | –        | –     | –      | –     | –                      | –          | –          | –    | –        | –          | –     | 10.991                             | ...                         | ...                         | −2                   | 24.2                               | 0.66                                 | 4.60                          | 6.000                         | ...   | ...    | 4.15  | ...   | ...   | ...   | ...    |
| 19152093+2254593 | 56.008   | 5.289    | 0.837  | 1      | –      | –    | –    | –        | –     | D1     | cp    | –                      | –          | –          | –    | –        | –          | –     | 11.386                             | 0.34                        | 1.31                        | 1                    | 56.6                               | 0.28                                 | 4.05                          | 11.074                        | 0.20  | 0.89   | 0.26  | 61.4  | 11.05 | 0.21  | 0.95   |
| 19152537+1655187 | 50.685   | 2.509    | 3.057  | 1      | –      | –    | –    | –        | –     | D1     | e     | –                      | –          | –          | –    | –        | –          | –     | 11.210                             | 0.67                        | ...                         | 1                    | 34.2                               | 0.60                                 | 4.45                          | 10.071                        | 0.16  | ...    | 0.95  | 49.9  | 9.98  | 0.22  | ...    |
| 19160922−0047090 | 35.056   | −5.856   | 0.558  | 1      | –      | –    | –    | –        | –     | D1     | –     | –                      | –          | –          | –    | –        | –          | –     | 10.962                             | 0.42                        | 1.39                        | 1                    | 52.8                               | 0.30                                 | 4.13                          | 10.754                        | 0.33  | 1.12   | 0.17  | 54.9  | 10.76 | 0.34  | 1.15   |
| 19161856+1119129 | 45.825   | −0.287   | 21.881 | 8      | –      | –    | –    | –        | –     | –      | –     | –                      | –          | –          | –    | –        | –          | –     | 8.894                              | 1.49                        | ...                         | 1                    | 108.0                              | 0.56                                 | 4.55                          | 0.741                         | −2.13 | ...    | 6.78  | ...   | ...   | −1.70 | ...    |
| 19170089+1044398 | 45.396   | −0.709   | 10.961 | 8      | –      | –    | –    | –        | –     | –      | –     | –                      | –          | –          | –    | –        | –          | –     | 9.926                              | 0.89                        | ...                         | −2                   | 63.2                               | 0.90                                 | 4.61                          | 5.842                         | −0.93 | ...    | 3.40  | ...   | ...   | −0.71 | ...    |
| 19170381−0142148 | 34.338   | −6.478   | 0.417  | 1      | –      | –    | –    | –        | –     | D2     | c     | o                      | –          | –          | –    | –        | –          | –     | 10.950                             | 0.29                        | 1.01                        | 1                    | 34.2                               | 0.90                                 | 4.07                          | 10.795                        | 0.22  | 0.80   | 0.13  | 35.1  | 10.81 | 0.23  | 0.83   |
| 19171703+3325309 | 65.665   | 9.648    | 0.151  | 1      | –      | –    | –    | –        | –     | D1     | c     | o                      | –          | –          | –    | –        | –          | –     | 10.822                             | 0.42                        | 1.25                        | 1                    | 36.4                               | 0.54                                 | 3.67                          | 10.766                        | 0.39  | 1.17   | 0.05  | 36.6  | 10.77 | 0.40  | 1.18   |
| 19172078+0243008 | 38.317   | −4.512   | 0.795  | 1      | –      | –    | –    | –        | –     | D2     | c     | o                      | –          | –          | –    | –        | –          | –     | 10.291                             | 0.33                        | 1.19                        | 1                    | 78.0                               | 0.32                                 | 4.24                          | 9.995                         | 0.19  | 0.80   | 0.25  | 82.6  | 10.01 | 0.21  | 0.85   |
| 19172690−0146412 | 34.316   | −6.597   | 0.373  | 1      | –      | –    | –    | –        | –     | D1     | c     | o                      | –          | –          | –    | –        | –          | –     | 11.116                             | 0.27                        | 1.05                        | 1                    | 33.0                               | 0.38                                 | 4.04                          | 10.977                        | 0.21  | 0.87   | 0.12  | 33.7  | 10.99 | 0.22  | 0.89   |
| 19173203−0145442 | 34.340   | −6.609   | 0.369  | 1      | –      | –    | –    | –        | –     | D2     | c     | o                      | –          | –          | –    | –        | –          | –     | 10.510                             | 0.25                        | 1.06                        | 1                    | 40.4                               | 0.78                                 | 4.04                          | 10.373                        | 0.19  | 0.88   | 0.11  | 41.3  | 10.38 | 0.20  | 0.90   |
| 19173769+0426248 | 39.882   | −3.777   | 0.991  | 1      | –      | –    | –    | –        | –     | D1     | –     | –                      | –          | –          | –    | –        | –          | –     | 10.605                             | 0.53                        | 1.50                        | 1                    | 47.8                               | 0.50                                 | 4.34                          | 10.236                        | 0.37  | 1.01   | 0.31  | 51.5  | 10.26 | 0.39  | 1.07   |
| 19174536+0140198 | 37.435   | −5.085   | 0.463  | 1      | –      | –    | –    | –        | –     | D1     | c     | o                      | –          | –          | –    | –        | –          | –     | 10.286                             | 0.33                        | 1.21                        | 1                    | 56.8                               | 0.54                                 | 4.25                          | 10.113                        | 0.25  | 0.98   | 0.14  | 58.4  | 10.13 | 0.26  | 1.01   |
| 19175996+1834568 | 52.442   | 2.737    | 2.042  | 9      | –      | –    | –    | –        | –     | –      | –     | –                      | –          | –          | –    | –        | –          | –     | 9.060                              | 0.15                        | 1.12                        | 1                    | 220.4                              | 0.32                                 | 4.47                          | 8.299                         | −0.19 | 0.10   | 0.63  | ...   | ...   | −0.15 | 0.24   |
| 19180012−0519102 | 31.194   | −8.323   | 0.530  | 1      | –      | –    | –    | –        | –     | D2     | c     | o                      | –          | –          | –    | –        | –          | –     | 11.286                             | 0.43                        | 1.23                        | 1                    | 32.8                               | 0.70                                 | 3.94                          | 11.089                        | 0.34  | 0.97   | 0.16  | 34.0  | 11.10 | 0.35  | 1.00   |
| 19180235+1834588 | 52.447   | 2.729    | 2.039  | 9      | –      | –    | –    | –        | –     | –      | –     | –                      | –          | –          | –    | –        | –          | –     | 9.016                              | 0.14                        | ...                         | 1                    | 141.0                              | 1.00                                 | 4.47                          | 8.256                         | −0.20 | ...    | 0.63  | ...   | ...   | −0.16 | ...    |
| 19180320+1834048 | 52.435   | 2.719    | 2.057  | 9      | –      | –    | –    | –        | –     | –      | –     | –                      | –          | –          | –    | –        | –          | –     | 7.249                              | 0.32                        | 1.30                        | 1                    | 163.8                              | 0.50                                 | 4.47                          | 6.483                         | −0.02 | 0.28   | 0.64  | ...   | ...   | 0.02  | 0.41   |
| 19182469+0631536 | 41.828   | −2.978   | 1.608  | 9      | –      | –    | –    | –        | –     | –      | –     | –                      | –          | –          | –    | –        | –          | –     | 9.722                              | ...                         | ...                         | 1                    | 90.8                               | 0.66                                 | 4.43                          | 9.123                         | ...   | ...    | 0.50  | ...   | ...   | ...   | ...    |
| 19182469+0632186 | 41.834   | −2.975   | 1.626  | 9      | –      | –    | –    | –        | –     | –      | –     | –                      | –          | –          | –    | –        | –          | –     | 9.150                              | ...                         | ...                         | 1                    | 219.6                              | 0.36                                 | 4.41                          | 8.544                         | ...   | ...    | 0.50  | ...   | ...   | ...   | ...    |
| 19182520−0135489 | 34.590   | −6.731   | 0.457  | 9      | –      | –    | –    | –        | –     | –      | –     | –                      | –          | –          | –    | –        | –          | –     | 11.192                             | 0.86                        | 0.86                        | 1                    | 33.6                               | 0.72                                 | 4.03                          | 11.022                        | 0.79  | 0.63   | 0.14  | ...   | ...   | 0.80  | 0.66   |
| 19182744+0631266 | 41.827   | −2.992   | 1.609  | 9      | –      | –    | –    | –        | –     | –      | –     | –                      | –          | –          | –    | –        | –          | –     | 10.169                             | ...                         | ...                         | 1                    | 96.4                               | 0.60                                 | 4.43                          | 9.569                         | ...   | ...    | 0.50  | ...   | ...   | ...   | ...    |
| 19183173+0632146 | 41.847   | −3.001   | 1.604  | 9      | –      | –    | –    | –        | –     | –      | –     | –                      | –          | –          | –    | –        | –          | –     | 9.544                              | ...                         | ...                         | 1                    | 142.6                              | 0.28                                 | 4.41                          | 8.946                         | ...   | ...    | 0.50  | ...   | ...   | ...   | ...    |
| 19194212+0721408 | 42.712   | −2.875   | 1.527  | 1      | –      | –    | –    | –        | –     | D1     | –     | –                      | –          | –          | –    | –        | –          | –     | 11.096                             | 0.54                        | 1.68                        | 1                    | 39.4                               | 0.70                                 | 4.40                          | 10.527                        | 0.29  | 0.92   | 0.47  | 46.3  | 10.50 | 0.32  | 1.02   |
| 19202854+3049317 | 63.619   | 7.879    | 0.228  | 1      | –      | –    | –    | –        | –     | D1     | c     | o                      | –          | –          | –    | –        | –          | –     | 10.378                             | 0.36                        | 0.98                        | 1                    | 59.6                               | 0.94                                 | 3.78                          | 10.293                        | 0.32  | 0.87   | 0.07  | 60.4  | 10.30 | 0.32  | 0.88   |
| 19203114+1355279 | 48.607   | 0.024    | 30.418 | 8      | –      | –    | –    | –        | –     | –      | –     | –                      | –          | –          | –    | –        | –          | –     | 8.977                              | ...                         | ...                         | 1                    | 171.2                              | 0.40                                 | 4.64                          | −2.357                        | ...   | ...    | 9.42  | ...   | ...   | ...   | ...    |
| 19203180+0836246 | 43.911   | −2.474   | 1.372  | 1      | –      | –    | –    | –        | –     | D1     | –     | –                      | –          | –          | –    | –        | –          | –     | 11.442                             | 0.36                        | ...                         | 1                    | 38.0                               | 0.28                                 | 4.46                          | 10.931                        | 0.13  | ...    | 0.42  | 43.5  | 10.92 | 0.16  | ...    |
| 19205612+1841331 | 52.865   | 2.174    | 2.697  | 1      | –      | –    | –    | –        | –     | D1     | –     | –                      | –          | –</        |      |          |            |       |                                    |                             |                             |                      |                                    |                                      |                               |                               |       |        |       |       |       |       |        |

Table B1: a) continued.

| 2MASX J          | <i>l</i> | <i>b</i> | EBV    | Object | Sample | Disc | 2MRS | Velocity | NIR   | Photom | Ext  | <i>K</i> <sub>20</sub> | <i>H-K</i> | <i>J-K</i> | vc   | <i>a</i> | <i>b/a</i> | st.d. | <i>K</i> <sub>s</sub> <sup>o</sup> | ( <i>H-K</i> ) <sup>o</sup> | ( <i>J-K</i> ) <sup>o</sup> | <i>A<sub>K</sub></i> | <i>a</i> <sub>d</sub> <sup>o</sup> | <i>K</i> <sub>s</sub> <sup>o,d</sup> | ( <i>H-K</i> ) <sup>o,c</sup> | ( <i>J-K</i> ) <sup>o,c</sup> |       |       |       |      |       |       |       |
|------------------|----------|----------|--------|--------|--------|------|------|----------|-------|--------|------|------------------------|------------|------------|------|----------|------------|-------|------------------------------------|-----------------------------|-----------------------------|----------------------|------------------------------------|--------------------------------------|-------------------------------|-------------------------------|-------|-------|-------|------|-------|-------|-------|
| (1)              | deg      | deg      | mag    | class  | off    | gal  | TF   | obs      | ext'd | type   | Opt  | HI                     | mag        | mag        | (17) | (18)     | (19)       | (20)  | mag                                | mag                         | mag                         | mag                  | (25)                               | mag                                  | mag                           | mag                           |       |       |       |      |       |       |       |
| (1)              | (2a)     | (2b)     | (3)    | (4)    | (5)    | (6)  | (7a) | (7c)     | (7d)  | (8)    | (9a) | (10a)                  | (11)       | (12)       | (13) | (14)     | (15)       | (16)  | (17)                               | (18)                        | (19)                        | (20)                 | (21)                               | (22)                                 | (23)                          | (24)                          | (25)  | (26)  | (27)  | (28) |       |       |       |
| 19235006+3447422 | 67.521   | 9.047    | 0.155  | 1      | o      | —    | g    | t        | —     | D1     | c    | —                      | h          | —          | —    | —        | —          | —     | 11.290                             | 0.36                        | 1.05                        | 1                    | 59.4                               | 0.24                                 | 3.70                          | 11.232                        | 0.34  | 0.98  | 0.05  | 59.9 | 11.23 | 0.34  | 0.99  |
| 19235128+1432508 | 49.537   | −0.396   | 95.530 | 9      | —      | —    | —    | —        | —     | —      | —    | —                      | —          | —          | —    | —        | —          | —     | 8.073                              | ...                         | ...                         | 1                    | 178.4                              | 1.00                                 | 4.64                          | −27.521                       | ...   | ...   | 29.59 | ...  | ...   | ...   |       |
| 19240313+1428339 | 49.497   | −0.472   | 49.619 | 8      | —      | —    | —    | —        | —     | —      | —    | —                      | —          | —          | —    | —        | —          | —     | 10.495                             | ...                         | ...                         | −2                   | 40.0                               | 0.92                                 | 4.55                          | −7.993                        | ...   | ...   | 15.37 | ...  | ...   | ...   |       |
| 19241113+2208141 | 56.267   | 3.120    | 1.404  | 1      | —      | —    | —    | —        | —     | —      | —    | —                      | —          | —          | —    | —        | —          | —     | 11.660                             | 0.48                        | 1.35                        | −2                   | 24.0                               | 0.68                                 | 4.35                          | 11.137                        | 0.25  | 0.65  | 0.43  | 27.5 | 11.13 | 0.28  | 0.74  |
| 19241426+2047311 | 55.085   | 2.476    | 2.901  | 1      | o      | s    | —    | N        | —     | D3     | —    | —                      | —          | —          | —    | —        | —          | —     | 10.971                             | 0.55                        | 1.61                        | −2                   | 34.4                               | 0.72                                 | 4.38                          | 8.890                         | 0.07  | 0.17  | 0.90  | 47.5 | 9.86  | 0.13  | 0.36  |
| 19242966+2047391 | 55.115   | 2.424    | 3.729  | 9      | —      | —    | —    | —        | —     | —      | —    | —                      | —          | —          | —    | —        | —          | —     | 9.914                              | 0.64                        | 1.34                        | 1                    | 86.8                               | 0.70                                 | 4.38                          | 8.525                         | 0.02  | −0.51 | 1.16  | ...  | ...   | 0.09  | −0.26 |
| 19243023+2047111 | 55.109   | 2.418    | 3.681  | 9      | —      | —    | —    | —        | —     | —      | —    | —                      | —          | —          | —    | —        | —          | —     | 9.436                              | 0.81                        | 1.61                        | 1                    | 80.8                               | 0.64                                 | 4.43                          | 8.064                         | 0.20  | −0.22 | 1.14  | ...  | ...   | 0.28  | 0.03  |
| 19244095+0225142 | 38.905   | −6.273   | 0.384  | 1      | —      | —    | —    | —        | —     | D2     | c    | o                      | —          | —          | —    | —        | —          | —     | 10.527                             | 0.40                        | 1.16                        | 1                    | 50.4                               | 0.54                                 | 4.07                          | 10.384                        | 0.34  | 0.97  | 0.12  | 51.5 | 10.40 | 0.35  | 1.00  |
| 19244319+0025092 | 37.122   | −7.207   | 0.442  | 1      | —      | —    | —    | —        | —     | D1     | c    | o                      | h          | —          | —    | —        | —          | —     | 10.482                             | 0.39                        | 1.31                        | 1                    | 39.4                               | 0.82                                 | 3.98                          | 10.317                        | 0.32  | 1.10  | 0.14  | 40.4 | 10.33 | 0.33  | 1.12  |
| 19250012+1729004 | 52.254   | 0.752    | 20.769 | 9      | —      | —    | —    | —        | —     | —      | —    | —                      | —          | —          | —    | —        | —          | —     | 10.394                             | 0.56                        | 1.84                        | −2                   | 27.4                               | 0.76                                 | 4.64                          | 2.655                         | −2.88 | −8.47 | 6.43  | ...  | ...   | −2.47 | −7.10 |
| 19250068+1725254 | 52.202   | 0.721    | 19.189 | 7      | —      | —    | —    | —        | —     | —      | —    | —                      | —          | —          | —    | —        | —          | —     | 10.308                             | ...                         | ...                         | 1                    | 42.4                               | 0.80                                 | 4.62                          | 3.158                         | ...   | ...   | 5.94  | ...  | ...   | ...   |       |
| 19250524+1205438 | 47.519   | −1.820   | 3.034  | 9      | —      | —    | —    | —        | —     | —      | —    | —                      | —          | —          | —    | —        | —          | —     | 11.497                             | ...                         | ...                         | −2                   | 31.6                               | 1.00                                 | 4.52                          | 10.367                        | ...   | ...   | 0.94  | ...  | ...   | ...   |       |
| 19250621+2515073 | 59.121   | 4.399    | 0.764  | 1      | o      | —    | —    | —        | —     | D1     | e    | o                      | —          | —          | —    | —        | —          | —     | 11.108                             | 0.39                        | 1.26                        | 1                    | 27.8                               | 0.74                                 | 4.13                          | 10.823                        | 0.26  | 0.88  | 0.24  | 29.6 | 10.83 | 0.28  | 0.93  |
| 19250658−0107245 | 35.785   | −8.002   | 0.288  | 1      | —      | —    | —    | —        | —     | D1     | c    | o                      | —          | —          | —    | —        | —          | —     | 11.295                             | 0.29                        | 1.06                        | 1                    | 35.2                               | 0.90                                 | 3.95                          | 11.083                        | 0.25  | 0.92  | 0.09  | 35.8 | 11.20 | 0.25  | 0.94  |
| 19251779+1512247 | 50.283   | −0.390   | 12.521 | 7      | —      | —    | —    | —        | —     | —      | —    | —                      | —          | —          | —    | —        | —          | —     | 9.698                              | ...                         | ...                         | 1                    | 47.6                               | 0.60                                 | 4.47                          | 5.033                         | ...   | ...   | 3.88  | ...  | ...   | ...   |       |
| 19252052−0008175 | 36.695   | −7.601   | 0.325  | 1      | —      | —    | —    | —        | —     | D1     | c    | —                      | h          | —          | —    | —        | —          | —     | 11.047                             | 0.22                        | 1.06                        | 1                    | 51.2                               | 0.58                                 | 3.99                          | 10.926                        | 0.17  | 0.90  | 0.10  | 52.2 | 10.93 | 0.17  | 0.92  |
| 19255793+1503017 | 50.222   | −0.607   | 8.189  | 8      | —      | —    | —    | —        | —     | —      | —    | —                      | —          | —          | —    | —        | —          | —     | 8.918                              | 1.95                        | ...                         | 1                    | 41.0                               | 0.52                                 | 4.57                          | 5.867                         | 0.59  | ...   | 2.54  | ...  | ...   | 0.75  |       |
| 19255928+2100385 | 55.471   | 2.219    | 2.008  | 1      | —      | —    | —    | t        | N     | D1     | —    | —                      | —          | —          | —    | —        | —          | —     | 11.546                             | 0.45                        | ...                         | −2                   | 20.0                               | 0.66                                 | 4.51                          | 10.798                        | 0.12  | ...   | 0.62  | 24.6 | 10.79 | 0.16  | ...   |
| 19260399+1620457 | 51.373   | −0.012   | 26.528 | 9      | —      | —    | —    | —        | —     | —      | —    | —                      | —          | —          | —    | —        | —          | —     | 10.062                             | ...                         | ...                         | 1                    | 84.2                               | 1.00                                 | 4.60                          | 0.178                         | ...   | ...   | 8.22  | ...  | ...   | ...   |       |
| 19265425+2104568 | 55.636   | 2.065    | 2.561  | 1      | —      | —    | —    | t        | N     | D2     | —    | —                      | —          | —          | —    | —        | —          | —     | 11.014                             | ...                         | ...                         | 1                    | 37.4                               | 0.50                                 | 4.48                          | 10.060                        | ...   | ...   | 0.79  | 51.1 | 9.98  | ...   | ...   |
| 19271138+2121295 | 55.910   | 2.137    | 2.507  | 1      | —      | —    | —    | t        | N     | D1     | —    | —                      | —          | —          | e    | —        | —          | —     | 11.686                             | ...                         | ...                         | 1                    | 32.8                               | 0.66                                 | 4.42                          | 10.752                        | ...   | ...   | 0.78  | 43.9 | 10.70 | ...   | ...   |
| 19273202+1743256 | 52.752   | 0.335    | 9.045  | 8      | —      | —    | —    | —        | —     | —      | —    | —                      | —          | —          | —    | —        | —          | —     | 10.304                             | ...                         | ...                         | 1                    | 35.6                               | 0.54                                 | 4.63                          | 6.934                         | ...   | ...   | 2.80  | ...  | ...   | ...   |       |
| 19273482+1754366 | 52.921   | 0.414    | 7.877  | 8      | —      | —    | —    | —        | —     | —      | —    | —                      | —          | —          | —    | —        | —          | —     | 10.808                             | ...                         | ...                         | 1                    | 29.4                               | 0.52                                 | 4.59                          | 7.873                         | ...   | ...   | 2.44  | ...  | ...   | ...   |       |
| 19275896+3445205 | 67.878   | 8.270    | 0.169  | 1      | —      | —    | —    | t        | N     | D2     | c    | o                      | —          | —          | —    | —        | —          | —     | 11.221                             | 0.37                        | 1.19                        | 1                    | 38.4                               | 0.40                                 | 3.73                          | 11.158                        | 0.34  | 1.10  | 0.05  | 38.7 | 11.16 | 0.35  | 1.11  |
| 19282817+1930293 | 54.426   | 0.992    | 9.767  | 8      | o      | —    | —    | —        | —     | —      | —    | —                      | —          | —          | —    | —        | —          | —     | 9.879                              | 0.91                        | 2.12                        | 1                    | 59.6                               | 0.78                                 | 4.58                          | 6.240                         | −0.71 | −2.74 | 3.03  | ...  | ...   | −0.52 | −2.09 |
| 19285189+1307064 | 48.857   | −2.145   | 1.503  | 1      | —      | —    | —    | t        | N     | D1     | —    | —                      | —          | —          | —    | —        | —          | —     | 11.046                             | 0.61                        | ...                         | 1                    | 33.6                               | 0.68                                 | 4.43                          | 10.486                        | 0.36  | ...   | 0.47  | 38.6 | 10.50 | 0.39  | ...   |
| 19290252+1239344 | 48.474   | −2.402   | 1.598  | 1      | —      | —    | —    | —        | —     | D2     | n    | —                      | —          | —          | —    | —        | —          | —     | 11.156                             | 0.51                        | 1.59                        | 1                    | 26.0                               | 0.92                                 | 4.42                          | 10.561                        | 0.24  | 0.79  | 0.49  | 30.3 | 10.56 | 0.27  | 0.90  |
| 19290539+0116083 | 38.391   | −7.783   | 0.369  | 1      | —      | —    | —    | —        | —     | D1     | c    | o                      | —          | —          | —    | —        | —          | —     | 10.385                             | 0.35                        | 1.11                        | 1                    | 46.4                               | 0.88                                 | 3.94                          | 10.248                        | 0.29  | 0.92  | 0.11  | 47.3 | 10.26 | 0.30  | 0.95  |
| 19291755+1756206 | 53.141   | 0.070    | 16.870 | 8      | —      | —    | —    | —        | —     | —      | —    | —                      | —          | —          | —    | —        | —          | —     | 9.451                              | 2.37                        | ...                         | 1                    | 36.6                               | 0.70                                 | 4.53                          | 3.165                         | −0.43 | ...   | 5.23  | ...  | ...   | −0.09 | ...   |
| 19291770+1756136 | 53.140   | 0.069    | 16.739 | 8      | —      | —    | —    | —        | —     | —      | —    | —                      | —          | —          | —    | —        | —          | —     | 9.852                              | ...                         | ...                         | 1                    | 50.2                               | 0.80                                 | 4.52                          | 3.615                         | ...   | ...   | 5.18  | ...  | ...   | ...   |       |
| 19292085+1757146 | 53.161   | 0.066    | 16.677 | 8      | —      | —    | —    | —        | —     | —      | —    | —                      | —          | —          | —    | —        | —          | —     | 11.292                             | ...                         | ...                         | 1                    | 21.2                               | 0.80                                 | 4.52                          | 5.078                         | ...   | ...   | 5.17  | ...  | ...   | ...   |       |
| 19293185+1759456 | 53.218   | 0.048    | 13.572 | 8      | —      | —    | —    | —        | —     | —      | —    | —                      | —          | —          | —    | —        | —          | —     | 9.758                              | ...                         | 3.54                        | 1                    | 35.6                               | 1.00                                 | 4.52                          | 4.701                         | ...   | −3.20 | 4.20  | ...  | ...   | −2.30 | ...   |
| 19294865+3540551 | 68.883   | 8.366    | 0.128  | 1      | —      | —    | —    | t        | N     | D1     | c    | o                      | —          | —          | —    | —        | —          | —     | 10.079                             | 0.37                        | 1.16                        | 1                    | 50.0                               | 0.48                                 | 3.78                          | 10.031                        | 0.35  | 1.10  | 0.04  | 50.2 | 10.04 | 0.35  | 1.10  |
| 19302260+1802224 | 53.616   | 0.036    | 32.778 | 8      | —      | —    | —    | —        | —     | —      | —    | —                      | —          | —          | —    | —        | —          | —     | 9.463                              | ...                         | ...                         | 1                    | 145.6                              | 0.58                                 | 4.63                          | −2.750                        | ...   | ...   | 10.15 | ...  | ...   | ...   |       |
| 19303004−0028146 | 36.997   | −8.899   | 0.320  | 1      | —      | —    | —    | —        | —     | D3     | c    | o                      | —          | —          | —    | —        | —          | —     | 10.676                             | 0.32                        | 1.11                        | 1                    | 42.0                               | 0.84                                 | 3.86                          | 10.557                        | 0.26  | 0.95  | 0.10  | 42.7 | 10.57 | 0.27  | 0.97  |
| 19305286−0037278 | 36.903   | −9.054   | 0.293  | 1      | —      | —    | —    | —        | —     | D4     | c    | o                      | —          | —          | —    | —        | —          | —     | 11.170                             | 0.32                        | 1.12                        | 1                    | 26.6                               | 0.68                                 | 3.88                          | 11.061                        | 0.27  | 0.97  | 0.09  | 27.0 | 11.07 | 0.28  | 0.99  |
| 19305289+3547067 | 69.077   | 8.221    | 0.129  | 1      | —      | —    | —    | —        | —     | D1     | c    | o                      | h          | —          | —    | —        | —          | —     | 10.443                             | 0.26                        | 0.92                        | 1                    | 54.6                               | 0.72                                 | 3.74                          | 10.395                        | 0.24  | 0.85  | 0.04  | 54.9 | 10.40 | 0.24  | 0.86  |
| 19305466+1728435 | 52.922   | −0.489   | 12.753 | 8      | —      | —    | —    | —        | —     | —      | —    | —                      | —          | —          | —    | —        | —          | —     | 10.330                             | ...                         | ...                         | 1                    | 32.6                               | 0.36                                 | 4.61                          | 5.578                         | ...   | ...   | 3.95  | ...  | ...   | ...   |       |
| 19312276+3702213 | 70.247   | 8.713    | 0.181  | 1      | —      | —    | —    | —        | —     | D1     | c    | o                      | —          | —          | —    | —        | —          | —     | 10.776                             | 0.24                        | 0.96                        | 1                    | 44.4                               | 0.68                                 | 3.67                          | 10.709                        | 0.21  | 0.87  | 0.06  | 44.8 | 10.71 | 0.22  | 0.89  |
| 19312354+2632370 | 60.933   | 3.765    | 0.865  | 1      | —      | —    | —    | —        | —     | D4     | —    | —                      | —          | —          | —    | —        | —          | —     | 11.367                             | 0.32                        | 1.25                        | 1                    | 29.6                               | 0.82                                 | 4.24                          | 11.045                        | 0.17  | 0.82  | 0.27  | 31.7 | 11.05 | 0.19  | 0.88  |
| 19313005+3552358 | 69.217   | 8.152    | 0.109  | 1      | —      | —    | —    | —        | —     | D1     | c    | o                      | h          | —          | —    | —        | —          | —     | 10.527                             | 0.37                        | 1.00                        | 1                    | 55.6                               | 0.82                                 | 3.69                          | 10.486                        | 0.35  | 0.95  | 0.03  | 55.9 | 10.49 | 0.36  | 0.96  |
| 19314991+1643330 | 52.368   | −1.044   | 7.679  | 8      | —      | —    | —    | —        | —     | —      | —    | —                      | —          | —          | —    | —        | —          | —     | 9.860                              | ...                         | ...                         | 1                    | 76.2                               | 0.78                                 | 4.50                          | 6.999                         | ...   | ...   | 2.38  | ...  | ...   | ...   |       |
| 19315025+2543597 | 60.268   | 3.290    | 1.083  | 1      | —      | —    | —    | —        | —     | D3     | —    | —                      | —          | —          | —    | —        | —          | —     | 10.835                             | 0.42                        | 1.51                        | 1                    | 41.8                               | 0.66                                 | 4.34                          | 10.431                        | 0.24  | 0.97  | 0.34  | 45.7 | 10.45 | 0.26  | 1.04  |
| 19320659+0624059 | 43.315   | −6.044   | 0.374  | 1      | —      | —    | —    | —</      |       |        |      |                        |            |            |      |          |            |       |                                    |                             |                             |                      |                                    |                                      |                               |                               |       |       |       |      |       |       |       |



Table B1: a) continued.

| 2MASX J          | <i>l</i> | <i>b</i> | EBV    | Object | Sample | Disc | 2MRS | Velocity | NIR   | Photom | Ext | <i>K</i> <sub>20</sub> | <i>H-K</i> | <i>J-K</i> | vc   | <i>a</i> | <i>b/a</i> | st.d. | <i>K</i> <sub>s</sub> <sup>o</sup> | ( <i>H-K</i> ) <sup>o</sup> | ( <i>J-K</i> ) <sup>o</sup> | <i>A<sub>K</sub></i> | <i>a</i> <sub>d</sub> <sup>o</sup> | <i>K</i> <sub>s</sub> <sup>o,d</sup> | ( <i>H-K</i> ) <sup>o,c</sup> | ( <i>J-K</i> ) <sup>o,c</sup> |       |        |       |      |       |        |       |
|------------------|----------|----------|--------|--------|--------|------|------|----------|-------|--------|-----|------------------------|------------|------------|------|----------|------------|-------|------------------------------------|-----------------------------|-----------------------------|----------------------|------------------------------------|--------------------------------------|-------------------------------|-------------------------------|-------|--------|-------|------|-------|--------|-------|
| (1)              | deg      | deg      | mag    | class  | off    | gal  | TF   | (7b)     | ext'd | type   |     | (14)                   | mag        | mag        | (17) | "        | (19)       | (20)  | mag                                | mag                         | mag                         | mag                  | "                                  | mag                                  | mag                           | mag                           |       |        |       |      |       |        |       |
| (2a)             | (2b)     | (3)      | (4)    | (5)    | (6)    | (7a) | (7b) | (7c)     | (7d)  | (8)    | (9) | (10a)                  | (10b)      | (11)       | (12) | (13)     | (14)       | (15)  | (16)                               | (17)                        | (18)                        | (19)                 | (20)                               | (21)                                 | (22)                          | (23)                          | (24)  | (25)   | (26)  | (27) | (28)  |        |       |
| 19390547+2856372 | 63.863   | 3.434    | 0.792  | 1      | —      | —    | g    | —        | N     | —      | —   | D1                     | —          | —          | —    | U        | —          | —     | 11.506                             | 0.39                        | 1.35                        | 1                    | 29.6                               | 0.94                                 | 4.29                          | 11.211                        | 0.25  | 0.95   | 0.25  | 31.6 | 11.21 | 0.27   | 1.00  |
| 19390892+0848372 | 46.282   | −6.426   | 0.365  | 1      | —      | —    | g    | —        | t     | —      | —   | D1                     | —          | —          | —    | h        | —          | —     | 10.668                             | 0.37                        | 1.20                        | 1                    | 91.6                               | 0.16                                 | 3.99                          | 10.532                        | 0.31  | 1.02   | 0.11  | 94.0 | 10.53 | 0.32   | 1.04  |
| 19391152+2511102 | 60.595   | 1.573    | 3.221  | 7      | —      | —    | g    | —        | —     | —      | —   | —                      | —          | —          | —    | —        | —          | —     | 10.005                             | 0.87                        | 1.77                        | 1                    | 60.0                               | 0.92                                 | 4.48                          | 8.805                         | 0.34  | 0.17   | 1.00  | ...  | ...   | 0.40   | 0.38  |
| 19391650+3357478 | 68.282   | 5.842    | 0.245  | 1      | —      | —    | g    | —        | —     | —      | —   | D2                     | —          | —          | —    | —        | —          | —     | 10.259                             | 0.29                        | 0.99                        | 1                    | 53.8                               | 0.56                                 | 3.98                          | 10.168                        | 0.25  | 0.86   | 0.08  | 54.4 | 10.18 | 0.25   | 0.88  |
| 19392360+0200362 | 40.269   | −9.716   | 0.377  | 1      | —      | —    | g    | —        | —     | —      | —   | D3                     | —          | —          | —    | —        | —          | —     | 10.936                             | 0.54                        | 1.27                        | 1                    | 41.2                               | 0.64                                 | 3.79                          | 10.796                        | 0.47  | 1.08   | 0.12  | 42.2 | 10.80 | 0.48   | 1.10  |
| 19392920+0620543 | 44.146   | −7.681   | 0.278  | 1      | o      | —    | g    | —        | —     | —      | —   | D1                     | —          | —          | —    | h        | —          | —     | 10.734                             | 0.25                        | 0.96                        | −2                   | 46.6                               | 0.60                                 | 3.95                          | 10.630                        | 0.20  | 0.82   | 0.09  | 47.2 | 10.64 | 0.21   | 0.84  |
| 19393271+2605247 | 61.422   | 1.948    | 3.032  | 8      | —      | —    | g    | —        | —     | —      | —   | —                      | —          | —          | —    | —        | —          | —     | 10.736                             | ...                         | ...                         | 1                    | 46.4                               | 0.72                                 | 4.42                          | 9.606                         | ...   | ...    | 0.94  | ...  | ...   | ...    | ...   |
| 19393445+2400197 | 59.610   | 0.917    | 7.886  | 7      | —      | —    | g    | —        | —     | —      | —   | —                      | —          | —          | —    | —        | —          | —     | 10.235                             | ...                         | ...                         | 1                    | 69.4                               | 0.74                                 | 4.51                          | 7.297                         | ...   | ...    | 2.44  | ...  | ...   | ...    | ...   |
| 19400578+2941390 | 64.626   | 3.610    | 0.641  | 2      | —      | —    | g    | —        | —     | —      | —   | D2                     | —          | —          | —    | —        | —          | —     | 11.136                             | 0.44                        | 1.26                        | 1                    | 30.8                               | 0.60                                 | 4.22                          | 10.897                        | 0.34  | 0.94   | 0.20  | 32.2 | 10.91 | 0.35   | 0.98  |
| 19401121+2916559 | 64.276   | 3.391    | 0.725  | 1      | —      | —    | g    | —        | —     | —      | —   | D1                     | —          | —          | —    | —        | —          | —     | 10.881                             | 0.38                        | 1.15                        | 1                    | 46.6                               | 0.78                                 | 4.25                          | 10.611                        | 0.26  | 0.79   | 0.22  | 49.4 | 10.62 | 0.27   | 0.84  |
| 19401784+3047414 | 65.609   | 4.111    | 0.496  | 1      | —      | —    | g    | —        | —     | —      | —   | D3                     | —          | —          | —    | —        | —          | —     | 10.367                             | 0.35                        | 1.11                        | 1                    | 50.8                               | 0.80                                 | 4.17                          | 10.182                        | 0.27  | 0.86   | 0.15  | 52.4 | 10.20 | 0.28   | 0.90  |
| 19402310+2718188 | 62.573   | 2.382    | 4.328  | 8      | o      | —    | g    | —        | —     | —      | —   | —                      | —          | —          | —    | —        | —          | —     | 9.630                              | 0.70                        | 1.39                        | 1                    | 101.2                              | 0.66                                 | 4.33                          | 8.017                         | −0.01 | −0.76  | 1.34  | ...  | ...   | 0.07   | −0.47 |
| 19402868+4113089 | 74.822   | 9.109    | 0.198  | 1      | —      | —    | g    | —        | —     | —      | —   | D3                     | —          | —          | —    | —        | —          | —     | 11.217                             | 0.42                        | 1.12                        | 1                    | 34.0                               | 0.76                                 | 3.61                          | 11.143                        | 0.38  | 1.02   | 0.06  | 34.3 | 11.15 | 0.39   | 1.04  |
| 19403458+2634148 | 61.955   | 1.983    | 1.989  | 8      | —      | —    | g    | —        | —     | —      | —   | —                      | —          | —          | —    | —        | —          | —     | 11.729                             | ...                         | ...                         | 1                    | 26.8                               | 0.72                                 | 4.41                          | 10.988                        | ...   | ...    | 0.62  | ...  | ...   | ...    | ...   |
| 19404833+2705117 | 62.429   | 2.193    | 2.184  | 8      | —      | —    | g    | —        | —     | —      | —   | D2                     | —          | —          | —    | —        | —          | —     | 11.267                             | 1.24                        | ...                         | 1                    | 21.0                               | 0.72                                 | 4.37                          | 10.453                        | 0.88  | ...    | 0.68  | ...  | ...   | 0.93   | ...   |
| 19410154+2638147 | 62.062   | 1.929    | 2.113  | 1      | —      | —    | g    | —        | N     | —      | —   | —                      | —          | —          | —    | —        | —          | —     | 10.156                             | 0.36                        | 1.34                        | −2                   | 51.4                               | 0.96                                 | 4.37                          | 9.369                         | 0.01  | 0.29   | 0.65  | 64.4 | 9.35  | 0.05   | 0.43  |
| 19411540+4102439 | 74.738   | 8.898    | 0.238  | 1      | —      | —    | g    | —        | —     | —      | —   | D3                     | —          | —          | —    | —        | —          | —     | 11.013                             | 0.33                        | 1.04                        | 1                    | 35.4                               | 0.62                                 | 3.66                          | 10.924                        | 0.29  | 0.92   | 0.07  | 35.8 | 10.93 | 0.29   | 0.94  |
| 19412030+2603236 | 61.592   | 1.581    | 1.924  | 9      | —      | —    | g    | —        | —     | —      | —   | —                      | —          | —          | —    | —        | —          | —     | 11.736                             | 0.19                        | 1.03                        | −2                   | 15.6                               | 0.90                                 | 4.45                          | 11.019                        | −0.13 | 0.07   | 0.60  | ...  | ...   | −0.09  | 0.20  |
| 19413492+0339064 | 41.999   | −9.424   | 0.326  | 1      | —      | —    | g    | —        | —     | —      | —   | D2                     | —          | —          | —    | —        | —          | —     | 10.967                             | 0.33                        | 1.09                        | 1                    | 34.8                               | 0.70                                 | 3.81                          | 10.846                        | 0.28  | 0.93   | 0.10  | 35.4 | 10.86 | 0.28   | 0.95  |
| 19413829+4237210 | 76.178   | 9.583    | 0.192  | 1      | —      | —    | g    | —        | —     | —      | —   | D3                     | —          | —          | —    | —        | —          | —     | 10.699                             | 0.42                        | 1.15                        | 1                    | 47.4                               | 0.76                                 | 3.66                          | 10.627                        | 0.39  | 1.06   | 0.06  | 47.8 | 10.63 | 0.39   | 1.07  |
| 19422860+2305059 | 59.138   | −0.117   | 12.031 | 8      | —      | —    | g    | —        | —     | —      | —   | —                      | —          | —          | —    | —        | —          | —     | 9.773                              | ...                         | ...                         | 1                    | 74.6                               | 0.52                                 | 4.56                          | 5.290                         | ...   | ...    | 3.73  | ...  | ...   | ...    | ...   |
| 19423541+4247305 | 76.414   | 9.509    | 0.214  | 1      | —      | —    | g    | —        | —     | —      | —   | D1                     | —          | —          | —    | —        | —          | —     | 11.195                             | 0.37                        | 1.13                        | 1                    | 35.0                               | 0.74                                 | 3.64                          | 11.115                        | 0.33  | 1.03   | 0.07  | 35.4 | 11.12 | 0.34   | 1.04  |
| 19424363+2340330 | 59.680   | 0.127    | 8.592  | 9      | —      | —    | g    | —        | —     | —      | —   | —                      | —          | —          | —    | —        | —          | —     | 11.092                             | ...                         | ...                         | 1                    | 28.8                               | 0.64                                 | 4.57                          | 7.891                         | ...   | ...    | 2.66  | ...  | ...   | ...    | ...   |
| 19425998+4012114 | 74.150   | 8.204    | 0.245  | 1      | o      | —    | g    | —        | t     | —      | —   | D2                     | —          | —          | —    | —        | —          | —     | 11.327                             | 0.30                        | 1.06                        | 1                    | 29.2                               | 0.46                                 | 3.73                          | 11.236                        | 0.26  | 0.94   | 0.08  | 29.6 | 11.24 | 0.27   | 0.96  |
| 19431085+2344046 | 59.782   | 0.066    | 19.625 | 9      | —      | —    | g    | —        | —     | —      | —   | —                      | —          | —          | —    | —        | —          | —     | 9.129                              | ...                         | ...                         | 1                    | 41.4                               | 0.46                                 | 4.54                          | 1.817                         | ...   | ...    | 6.08  | ...  | ...   | ...    | ...   |
| 19432494+4156280 | 75.730   | 8.970    | 0.244  | 1      | —      | —    | g    | —        | —     | —      | —   | D1                     | —          | —          | —    | h        | —          | —     | 10.384                             | 0.32                        | 1.00                        | 1                    | 54.2                               | 0.74                                 | 3.67                          | 10.293                        | 0.28  | 0.88   | 0.08  | 54.9 | 10.30 | 0.29   | 0.89  |
| 19432669+4139340 | 75.482   | 8.830    | 0.205  | 1      | o      | —    | g    | —        | t     | —      | —   | D4                     | —          | —          | —    | —        | —          | —     | 10.406                             | 0.26                        | 0.96                        | 1                    | 70.2                               | 0.40                                 | 3.72                          | 10.330                        | 0.23  | 0.86   | 0.06  | 71.3 | 10.32 | 0.23   | 0.88  |
| 19434848+2329189 | 59.641   | −0.181   | 15.526 | 7      | —      | —    | g    | —        | —     | —      | —   | —                      | —          | —          | —    | —        | —          | —     | 10.449                             | ...                         | ...                         | −2                   | 27.6                               | 0.80                                 | 4.54                          | 4.664                         | ...   | ...    | 4.81  | ...  | ...   | ...    | ...   |
| 19440453+0752137 | 46.045   | −7.947   | 0.362  | 1      | —      | —    | g    | —        | —     | —      | —   | D1                     | —          | —          | —    | —        | —          | —     | 11.241                             | 0.34                        | 1.12                        | 1                    | 32.0                               | 0.88                                 | 3.87                          | 11.106                        | 0.28  | 0.94   | 0.11  | 32.7 | 11.12 | 0.29   | 0.96  |
| 19440465+0819397 | 46.449   | −7.726   | 0.540  | 1      | —      | —    | g    | —        | t     | —      | —   | D1                     | —          | —          | —    | h        | —          | —     | 11.314                             | 0.33                        | 1.23                        | 1                    | 43.6                               | 0.42                                 | 3.86                          | 11.113                        | 0.24  | 0.96   | 0.17  | 45.3 | 11.12 | 0.26   | 1.00  |
| 19441883+1815302 | 55.163   | −2.889   | 0.781  | 1      | —      | —    | g    | —        | —     | —      | —   | D1                     | —          | —          | —    | —        | —          | —     | 10.825                             | 0.47                        | 1.43                        | 1                    | 31.4                               | 0.62                                 | 4.29                          | 10.534                        | 0.34  | 1.04   | 0.24  | 33.1 | 10.56 | 0.36   | 1.09  |
| 19441905+4410002 | 77.792   | 9.887    | 0.206  | 1      | —      | —    | g    | —        | —     | —      | —   | D1                     | —          | —          | —    | —        | —          | —     | 11.181                             | 0.37                        | 1.09                        | 1                    | 36.8                               | 0.78                                 | 3.62                          | 11.104                        | 0.33  | 0.99   | 0.06  | 37.2 | 11.11 | 0.34   | 1.00  |
| 19442348+2548415 | 61.720   | 0.863    | 4.807  | 8      | —      | —    | g    | —        | —     | —      | —   | —                      | —          | —          | —    | —        | —          | —     | 10.934                             | 0.85                        | ...                         | 1                    | 19.4                               | 0.74                                 | 4.55                          | 9.143                         | 0.05  | ...    | 1.49  | ...  | ...   | 0.15   | ...   |
| 19445550+2614437 | 62.156   | 0.976    | 4.464  | 8      | —      | —    | g    | —        | —     | —      | —   | —                      | —          | —          | —    | —        | —          | —     | 11.069                             | ...                         | ...                         | 1                    | 36.2                               | 0.68                                 | 4.48                          | 9.406                         | ...   | ...    | 1.38  | ...  | ...   | ...    | ...   |
| 19452425+2750589 | 63.599   | 1.686    | 2.388  | 8      | —      | —    | g    | —        | —     | —      | —   | —                      | —          | —          | —    | —        | —          | —     | 9.149                              | 1.04                        | 2.40                        | 1                    | 79.6                               | 0.56                                 | 4.42                          | 8.259                         | 0.64  | 1.22   | 0.74  | ...  | ...   | 0.69   | 1.38  |
| 19453068+0549454 | 44.411   | −9.245   | 0.187  | 1      | —      | —    | g    | —        | —     | —      | —   | D4                     | —          | —          | —    | —        | —          | —     | 11.297                             | 0.36                        | 1.08                        | 1                    | 31.8                               | 0.68                                 | 3.83                          | 11.227                        | 0.33  | 0.99   | 0.06  | 32.1 | 11.23 | 0.33   | 1.00  |
| 19453186+4308260 | 76.985   | 9.204    | 0.207  | 1      | —      | —    | g    | —        | —     | —      | —   | D1                     | —          | —          | —    | h        | —          | —     | 10.955                             | 0.25                        | 0.93                        | 1                    | 55.6                               | 0.66                                 | 3.71                          | 10.878                        | 0.22  | 0.83   | 0.06  | 56.3 | 10.88 | 0.22   | 0.84  |
| 19455247+2417420 | 60.575   | −0.187   | 5.381  | 8      | —      | —    | g    | —        | —     | —      | —   | —                      | —          | —          | —    | —        | —          | —     | 10.429                             | ...                         | ...                         | 1                    | 35.8                               | 0.52                                 | 4.60                          | 8.424                         | ...   | ...    | 1.67  | ...  | ...   | ...    | ...   |
| 19461952+2435245 | 60.882   | −0.127   | 35.778 | 9      | —      | —    | g    | —        | —     | —      | —   | —                      | —          | —          | —    | —        | —          | —     | 7.602                              | 1.30                        | 2.55                        | 1                    | 162.2                              | 0.48                                 | 4.57                          | −5.729                        | −4.63 | −15.22 | 11.08 | ...  | −3.92 | −12.86 |       |
| 19464385+4216114 | 76.321   | 8.590    | 0.268  | 1      | —      | —    | g    | —        | —     | —      | —   | D3                     | —          | —          | —    | —        | —          | —     | 11.050                             | 0.34                        | 1.10                        | 1                    | 36.0                               | 0.68                                 | 3.75                          | 10.950                        | 0.29  | 0.96   | 0.08  | 36.5 | 10.96 | 0.30   | 0.98  |
| 19464467+2513186 | 61.476   | 0.108    | 70.918 | 9      | —      | —    | g    | —        | —     | —      | —   | —                      | —          | —          | —    | —        | —          | —     | 9.785                              | ...                         | ...                         | 1                    | 76.8                               | 0.40                                 | 4.53                          | −16.639                       | ...   | ...    | 21.97 | ...  | ...   | ...    | ...   |
| 19464489+2512076 | 61.459   | 0.098    | 67.489 | 9      | —      | —    | g    | —        | —     | —      | —   | —                      | —          | —          | —    | —        | —          | —     | 7.894                              | 1.50                        | ...                         | 1                    | 202.8                              | 0.22                                 | 4.53                          | −17.252                       | −9.68 | ...    | 20.91 | ...  | ...   | −8.35  | ...   |
| 19464732+2512456 | 61.473   | 0.095    | 67.328 | 9      |        |      |      |          |       |        |     |                        |            |            |      |          |            |       |                                    |                             |                             |                      |                                    |                                      |                               |                               |       |        |       |      |       |        |       |

Table B1: a) continued.

| 2MASX J          | <i>l</i> | <i>b</i> | EBV    | Object | Sample | Disc | 2MRS | Velocity | NIR  | Photom | Ext  | <i>K</i> <sub>20</sub> | <i>H-K</i> | <i>J-K</i> | vc   | <i>a</i> | <i>b/a</i> | st.d.  | <i>K</i> <sub>s</sub> <sup>o</sup> | ( <i>H-K</i> ) <sup>o</sup> | ( <i>J-K</i> ) <sup>o</sup> | <i>A</i> <sub>K</sub> | <i>a</i> <sub>d</sub> <sup>o</sup> | <i>K</i> <sub>s</sub> <sup>o,d</sup> | ( <i>H-K</i> ) <sup>o,c</sup> | ( <i>J-K</i> ) <sup>o,c</sup> |        |       |      |       |       |        |       |
|------------------|----------|----------|--------|--------|--------|------|------|----------|------|--------|------|------------------------|------------|------------|------|----------|------------|--------|------------------------------------|-----------------------------|-----------------------------|-----------------------|------------------------------------|--------------------------------------|-------------------------------|-------------------------------|--------|-------|------|-------|-------|--------|-------|
| (1)              | deg      | deg      | mag    | class  | off    | flag | gal  | TF       | obs  | ext'd  | type | (9)                    | Opt        | HI         | (11) | flag     | flag       | flag   | mag                                | mag                         | mag                         | mag                   | mag                                | mag                                  | mag                           | mag                           | mag    |       |      |       |       |        |       |
| (1)              | (2a)     | (2b)     | (3)    | (4)    | (5)    | (6)  | (7a) | (7b)     | (7c) | (7d)   | (8)  | (9)                    | (10a)      | (10b)      | (11) | (12)     | (13)       | (14)   | (15)                               | (16)                        | (17)                        | (18)                  | (19)                               | (20)                                 | (21)                          | (22)                          | (23)   | (24)  | (25) | (26)  | (27)  | (28)   |       |
| 19580314+3144069 | 68.342   | 1.314    | 4.281  | 7      | —      | —    | —    | —        | —    | —      | —    | —                      | —          | —          | U    | —        | —          | —      | 10.756                             | 1.23                        | 2.36                        | −2                    | 27.0                               | 0.84                                 | 4.38                          | 9.161                         | 0.53   | 0.24  | 1.33 | ...   | ...   | 0.61   | 0.52  |
| 19582178+3123060 | 68.078   | 1.074    | 5.013  | 7      | —      | —    | —    | —        | —    | —      | —    | —                      | —          | —          | U    | —        | —          | —      | 11.915                             | ...                         | ...                         | ...                   | 18.8                               | 0.80                                 | 4.41                          | 10.047                        | ...    | ...   | 1.55 | ...   | ...   | ...    |       |
| 19582351+3122170 | 68.069   | 1.062    | 5.064  | 8      | —      | —    | —    | —        | —    | —      | —    | —                      | —          | —          | U    | —        | —          | —      | 10.506                             | 0.99                        | 2.13                        | −2                    | 39.6                               | 0.80                                 | 4.41                          | 8.619                         | 0.15   | −0.38 | 1.57 | ...   | ...   | 0.25   | −0.05 |
| 19585050+4052424 | 76.252   | 5.932    | 0.329  | 1      | —      | —    | g    | t        | —    | —      | D1   | c                      | o          | —          | —    | —        | —          | 10.894 | 0.41                               | 1.12                        | 1                           | 36.6                  | 0.44                               | 3.99                                 | 10.771                        | 0.36                          | 0.95   | 0.10  | 37.4 | 10.78 | 0.36  | 0.98   |       |
| 19590886+3121505 | 68.147   | 0.921    | 6.604  | 7      | —      | —    | —    | —        | —    | —      | —    | —                      | —          | —          | U    | —        | —          | —      | 9.506                              | ...                         | ...                         | 1                     | 181.2                              | 0.24                                 | 4.49                          | 7.045                         | ...    | ...   | 2.05 | ...   | ...   | ...    |       |
| 19592833+4044022 | 76.190   | 5.756    | 0.375  | 1      | —      | —    | g    | —        | —    | —      | D1   | c                      | o          | —          | —    | —        | e          | 10.552 | 0.37                               | 1.21                        | 1                           | 52.2                  | 0.84                               | 3.98                                 | 10.412                        | 0.31                          | 1.02   | 0.12  | 53.6 | 10.42 | 0.32  | 1.05   |       |
| 19592944+2242257 | 60.810   | −3.681   | 1.478  | 9      | —      | —    | —    | —        | —    | —      | —    | —                      | —          | —          | —    | —        | —          | 10.744 | 1.28                               | 1.61                        | 1                           | 80.8                  | 0.34                               | 4.16                                 | 10.193                        | 1.04                          | 0.87   | 0.46  | ...  | ...   | 1.07  | 0.97   |       |
| 19593637+2243157 | 60.836   | −3.696   | 1.544  | 9      | —      | —    | —    | —        | —    | —      | —    | —                      | —          | —          | —    | —        | —          | 10.609 | ...                                | 1.18                        | 1                           | 95.0                  | 1.00                               | 4.16                                 | 10.034                        | ...                           | 0.41   | 0.48  | ...  | ...   | ...   | 0.51   |       |
| 19593645+2244077 | 60.849   | −3.689   | 1.557  | 9      | —      | —    | —    | —        | —    | —      | —    | —                      | —          | —          | —    | —        | —          | 9.709  | 0.68                               | 1.10                        | 1                           | 116.0                 | 0.60                               | 4.16                                 | 9.129                         | 0.43                          | 0.33   | 0.48  | ...  | ...   | 0.46  | 0.43   |       |
| 19594376+1445555 | 54.010   | −7.842   | 0.271  | 1      | —      | —    | g    | —        | —    | —      | D1   | c                      | o          | h          | —    | —        | —          | 10.916 | 0.25                               | 0.94                        | 1                           | 50.2                  | 0.62                               | 3.84                                 | 10.815                        | 0.20                          | 0.80   | 0.08  | 51.0 | 10.82 | 0.21  | 0.82   |       |
| 19595504+4233309 | 77.804   | 6.628    | 0.392  | 1      | —      | —    | —    | t        | —    | —      | D1   | c                      | o          | —          | —    | —        | e          | 10.418 | 0.31                               | 1.11                        | 1                           | 55.4                  | 0.38                               | 3.92                                 | 10.272                        | 0.24                          | 0.92   | 0.12  | 56.6 | 10.29 | 0.25  | 0.95   |       |
| 19595530+4045194 | 76.253   | 5.694    | 0.391  | 1      | —      | —    | g    | —        | —    | —      | D3   | c                      | o          | —          | —    | —        | e?         | 11.278 | 0.45                               | 1.28                        | 1                           | 30.2                  | 0.80                               | 3.98                                 | 11.132                        | 0.38                          | 1.08   | 0.12  | 30.9 | 11.14 | 0.39  | 1.11   |       |
| 20000622+1827566 | 57.251   | −6.011   | 0.519  | 1      | —      | —    | g    | t        | —    | —      | D1   | c                      | o          | h          | —    | —        | —          | 9.972  | 0.37                               | 1.28                        | 1                           | 80.6                  | 0.26                               | 3.99                                 | 9.779                         | 0.28                          | 1.03   | 0.16  | 83.2 | 9.79  | 0.29  | 1.06   |       |
| 20000736+2601248 | 63.714   | −2.066   | 1.973  | 9      | —      | —    | —    | —        | —    | —      | —    | —                      | —          | —          | —    | —        | —          | 9.638  | 1.49                               | ...                         | −2                          | 51.0                  | 0.56                               | 4.27                                 | 8.903                         | 1.16                          | ...    | 0.61  | ...  | ...   | 1.20  | ...    |       |
| 20000942+4321590 | 78.523   | 7.008    | 0.429  | 1      | —      | —    | g    | t        | N    | —      | D3   | e                      | o          | —          | —    | —        | e?         | 11.157 | ...                                | 1.33                        | 1                           | 35.8                  | 1.00                               | 3.87                                 | 10.997                        | ...                           | 1.11   | 0.13  | 36.8 | 11.01 | ...   | 1.14   |       |
| 20000957+2201495 | 60.313   | −4.166   | 0.729  | 1      | —      | —    | —    | —        | —    | —      | D1   | e                      | o          | *          | —    | —        | —          | 11.087 | 0.40                               | 1.20                        | 1                           | 40.6                  | 0.50                               | 4.11                                 | 10.815                        | 0.28                          | 0.83   | 0.23  | 43.2 | 10.81 | 0.29  | 0.88   |       |
| 20003365+2552400 | 63.642   | −2.226   | 2.574  | 9      | —      | —    | —    | —        | —    | —      | —    | —                      | —          | —          | —    | —        | —          | 11.985 | ...                                | ...                         | 1                           | 42.0                  | 0.22                               | 4.25                                 | 11.026                        | ...                           | ...    | 0.80  | ...  | ...   | ...   | ...    |       |
| 20005548+3329255 | 70.154   | 1.719    | 7.630  | 9      | —      | —    | —    | —        | —    | —      | —    | —                      | —          | —          | —    | —        | —          | 10.145 | 0.62                               | 1.02                        | 1                           | 203.6                 | 0.14                               | 4.39                                 | 7.302                         | −0.64                         | −2.77  | 2.36  | ...  | ...   | −0.49 | −2.26  |       |
| 20010747+3311446 | 69.925   | 1.529    | 9.737  | 9      | —      | —    | —    | —        | —    | —      | —    | —                      | —          | —          | —    | —        | —          | 9.335  | ...                                | ...                         | 1                           | 88.8                  | 0.26                               | 4.43                                 | 5.707                         | ...                           | ...    | 3.02  | ...  | ...   | ...   | ...    |       |
| 20010969+2655338 | 64.604   | −1.788   | 2.314  | 1      | o      | —    | g    | —        | t    | N      | D1   | e                      | o          | —          | —    | o        | —          | 11.593 | 0.50                               | 1.62                        | 1                           | 32.6                  | 0.34                               | 4.31                                 | 10.731                        | 0.11                          | 0.47   | 0.72  | 42.9 | 10.66 | 0.16  | 0.63   |       |
| 20011090+3311056 | 69.923   | 1.513    | 9.238  | 9      | —      | —    | —    | —        | —    | —      | —    | —                      | —          | —          | —    | —        | —          | 7.613  | 1.21                               | 2.32                        | 1                           | 216.4                 | 0.54                               | 4.43                                 | 4.171                         | −0.32                         | −2.27  | 2.86  | ...  | ...   | −0.14 | −1.66  |       |
| 20012343+3331561 | 70.241   | 1.659    | 22.181 | 8      | —      | —    | —    | —        | —    | —      | —    | —                      | —          | —          | —    | —        | —          | 12.481 | ...                                | ...                         | −2                          | 25.4                  | 0.60                               | 4.35                                 | 4.216                         | ...                           | ...    | 6.87  | ...  | ...   | ...   | ...    |       |
| 20012791+2957418 | 67.218   | −0.242   | 2.767  | 9      | —      | —    | —    | —        | —    | —      | —    | —                      | —          | —          | —    | —        | —          | 10.521 | 0.56                               | ...                         | −2                          | 26.4                  | 0.38                               | 4.51                                 | 9.490                         | 0.10                          | ...    | 0.86  | ...  | ...   | 0.15  | ...    |       |
| 20013735+3335282 | 70.316   | 1.649    | 42.325 | 8      | —      | —    | —    | —        | —    | —      | —    | —                      | —          | —          | —    | —        | —          | 9.725  | 0.89                               | 2.04                        | 1                           | 64.8                  | 0.76                               | 4.40                                 | −6.045                        | −6.12                         | −18.98 | 13.11 | ...  | ...   | −5.29 | −16.19 |       |
| 20014495+3335502 | 70.335   | 1.630    | 40.882 | 8      | —      | —    | —    | —        | —    | —      | —    | —                      | —          | —          | —    | —        | —          | 11.384 | ...                                | ...                         | −2                          | 43.8                  | 0.80                               | 4.40                                 | −3.849                        | ...                           | ...    | 12.66 | ...  | ...   | ...   | ...    |       |
| 20014511+3333152 | 70.299   | 1.607    | 45.592 | 9      | —      | —    | —    | —        | —    | —      | —    | —                      | —          | —          | —    | —        | —          | 10.176 | 1.08                               | 1.95                        | 1                           | 92.2                  | 0.22                               | 4.35                                 | −6.812                        | −6.47                         | −20.71 | 14.12 | ...  | ...   | −5.58 | −17.70 |       |
| 20014694+3331342 | 70.279   | 1.586    | 35.188 | 9      | —      | —    | —    | —        | —    | —      | —    | —                      | —          | —          | —    | —        | —          | 7.147  | 1.02                               | 1.68                        | 1                           | 107.6                 | 0.74                               | 4.35                                 | −5.964                        | −4.80                         | −15.81 | 10.90 | ...  | ...   | −4.11 | −13.48 |       |
| 20014831+3332552 | 70.300   | 1.594    | 42.901 | 9      | —      | —    | —    | —        | —    | —      | —    | —                      | —          | —          | —    | —        | —          | 6.612  | 0.98                               | 1.78                        | 1                           | 230.0                 | 0.68                               | 4.35                                 | −9.373                        | −6.13                         | −19.53 | 13.29 | ...  | ...   | −5.28 | −16.70 |       |
| 20015506+3334200 | 70.333   | 1.587    | 40.968 | 8      | —      | —    | —    | —        | —    | —      | —    | —                      | —          | —          | —    | —        | —          | 8.872  | 1.38                               | ...                         | 1                           | 87.8                  | 0.80                               | 4.35                                 | −6.393                        | −5.40                         | ...    | 12.69 | ...  | ...   | −4.60 | ...    |       |
| 20020150+4300073 | 78.387   | 6.528    | 0.900  | 1      | —      | —    | g    | t        | —    | —      | D1   | c                      | o          | —          | —    | —        | e          | 11.060 | 0.55                               | 1.55                        | 1                           | 50.6                  | 0.30                               | 3.87                                 | 10.725                        | 0.40                          | 1.10   | 0.28  | 54.9 | 10.72 | 0.42  | 1.16   |       |
| 20020228+3726080 | 73.630   | 3.607    | 0.757  | 1      | —      | —    | g    | —        | N    | —      | D1   | e                      | o          | —          | —    | —        | —          | 10.242 | 0.51                               | 1.50                        | 1                           | 49.6                  | 0.42                               | 4.20                                 | 9.960                         | 0.38                          | 1.12   | 0.23  | 52.5 | 9.97  | 0.40  | 1.17   |       |
| 20021437+3404421 | 70.798   | 1.798    | 2.569  | 8      | —      | —    | —    | —        | —    | —      | —    | —                      | —          | —          | —    | —        | —          | 11.918 | ...                                | ...                         | 1                           | 27.0                  | 0.46                               | 4.40                                 | 10.961                        | ...                           | ...    | 0.80  | ...  | ...   | ...   | ...    |       |
| 20021959+4307366 | 78.523   | 6.546    | 0.948  | 1      | —      | —    | g    | —        | —    | —      | D1   | c                      | o          | —          | —    | —        | e?         | 9.674  | 0.42                               | 1.32                        | 1                           | 69.4                  | 0.76                               | 3.86                                 | 9.321                         | 0.26                          | 0.85   | 0.29  | 74.5 | 9.34  | 0.28  | 0.91   |       |
| 20022276+3937370 | 75.533   | 4.704    | 0.408  | 1      | —      | —    | —    | —        | —    | —      | D3   | e                      | o          | —          | —    | —        | —          | 11.047 | 0.51                               | 1.28                        | 1                           | 35.2                  | 0.84                               | 4.08                                 | 10.895                        | 0.44                          | 1.08   | 0.13  | 36.1 | 10.91 | 0.45  | 1.11   |       |
| 20022818+4934006 | 84.110   | 9.848    | 0.175  | 1      | —      | —    | —    | —        | —    | —      | D1   | c                      | o          | —          | —    | —        | —          | 10.877 | 0.24                               | 0.90                        | 1                           | 27.6                  | 0.88                               | 3.63                                 | 10.812                        | 0.21                          | 0.81   | 0.05  | 27.8 | 10.82 | 0.21  | 0.82   |       |
| 20023820+3304002 | 69.984   | 1.192    | 2.565  | 9      | —      | —    | —    | —        | —    | —      | —    | —                      | —          | —          | —    | —        | —          | 11.729 | ...                                | ...                         | −2                          | 20.8                  | 0.58                               | 4.40                                 | 10.773                        | ...                           | ...    | 0.79  | ...  | ...   | ...   | ...    |       |
| 20024988+4919112 | 83.925   | 9.671    | 0.194  | 1      | —      | —    | —    | —        | —    | —      | D4   | c                      | o          | —          | —    | —        | —          | 10.072 | 0.33                               | 1.06                        | 1                           | 44.6                  | 0.84                               | 3.70                                 | 10.000                        | 0.30                          | 0.96   | 0.06  | 45.0 | 10.01 | 0.30  | 0.97   |       |
| 20030728+3157588 | 69.106   | 0.521    | 3.208  | 9      | —      | —    | —    | —        | —    | —      | —    | —                      | —          | —          | —    | —        | —          | 11.093 | 0.68                               | 1.08                        | 1                           | 37.6                  | 0.62                               | 4.42                                 | 9.898                         | 0.15                          | −0.51  | 0.99  | ...  | ...   | 0.21  | −0.30  |       |
| 20040030+3516101 | 72.000   | 2.123    | 2.657  | 9      | —      | —    | —    | —        | —    | —      | —    | —                      | —          | —          | —    | —        | —          | 11.668 | ...                                | ...                         | 1                           | 52.0                  | 0.26                               | 4.31                                 | 10.678                        | ...                           | ...    | 0.82  | ...  | ...   | ...   | ...    |       |
| 20043355+3439122 | 71.540   | 1.699    | 2.934  | 9      | —      | —    | —    | —        | —    | —      | —    | —                      | —          | —          | —    | —        | —          | 12.234 | ...                                | ...                         | −2                          | 25.8                  | 0.44                               | 4.39                                 | 11.141                        | ...                           | ...    | 0.91  | ...  | ...   | ...   | ...    |       |
| 20043453+1244218 | 52.861   | −9.892   | 0.134  | 1      | —      | —    | g    | t        | —    | —      | D1   | c                      | o          | h          | —    | —        | —          | 9.970  | 0.27                               | 1.05                        | 1                           | 71.6                  | 0.36                               | 3.77                                 | 9.920                         | 0.25                          | 0.98   | 0.04  | 72.0 | 9.93  | 0.26  | 0.99   |       |
| 20044538+2915033 | 66.996   | −1.225   | 14.209 | 8      | —      | —    | —    | —        | —    | —      | —    | —                      | —          | —          | —    | —        | —          | 9.235  | 0.57                               | 1.14                        | 1                           | 50.0                  | 0.62                               | 4.36                                 | 3.941                         | −1.79                         | −5.92  | 4.40  | ...  | ...   | −1.51 | −4.98  |       |
| 20044736+2914143 | 66.988   | −1.239   | 16.212 | 9      | —      | —    | —    | —        | —    | —      | —    | —                      | —          | —          | —    | —        | —          | 9.551  | ...                                | ...                         | 1                           | 99.6                  | 1.00                               | 4.36                                 | 3.510                         | ...                           | ...    | 5.02  | ...  | ...   | ...   | ...    |       |
| 20045280+2911433 | 66.964   | −1.278   | 17.459 | 8      | —      | —    | —    | —        | —    | —      | —    | —                      | —          | —          | —    | —        | —          | 7.887  | 0.88                               | 1.84                        | −2                          | 121.6                 | 0.                                 |                                      |                               |                               |        |       |      |       |       |        |       |

Table B1: a) continued.

| 2MASX J          | <i>l</i>    | <i>b</i>    | EBV        | Object       |            | Sample     | Disc        | 2MRS       | Velocity    | NIR           | Photom      | Ext | <i>K</i> <sub>20</sub> | <i>H-K</i>  | <i>J-K</i>  | vc          | <i>a</i>    | <i>b/a</i> | st.d.       | <i>K</i> <sub>s</sub> <sup>o</sup> | ( <i>H-K</i> ) <sup>o</sup> | ( <i>J-K</i> ) <sup>o</sup> | <i>A<sub>K</sub></i> | <i>a</i> <sub>d</sub> <sup>o</sup> | <i>K</i> <sub>s</sub> <sup>o,d</sup> | ( <i>H-K</i> ) <sup>o,c</sup> | ( <i>J-K</i> ) <sup>o,c</sup> |             |      |             |             |             |       |
|------------------|-------------|-------------|------------|--------------|------------|------------|-------------|------------|-------------|---------------|-------------|-----|------------------------|-------------|-------------|-------------|-------------|------------|-------------|------------------------------------|-----------------------------|-----------------------------|----------------------|------------------------------------|--------------------------------------|-------------------------------|-------------------------------|-------------|------|-------------|-------------|-------------|-------|
| (1)              | deg<br>(2a) | deg<br>(2b) | mag<br>(3) | class<br>(4) | off<br>(5) | flg<br>(6) | gal<br>(7a) | TF<br>(7b) | obs<br>(7c) | ext'd<br>(7d) | type<br>(8) | (9) | Opt<br>(10a)           | HI<br>(10b) | flg<br>(11) | flg<br>(12) | flg<br>(13) | (14)       | mag<br>(15) | mag<br>(16)                        | (17)                        | (18)                        | (19)                 | (20)                               | mag<br>(21)                          | mag<br>(22)                   | mag<br>(23)                   | mag<br>(24) | (25) | mag<br>(26) | mag<br>(27) | mag<br>(28) |       |
| 20100506+2557368 | 64.857      | -3.993      | 1.702      | 1            | -          | -          | g           | -          | N           | -             | D1          | -   | -                      | -           | -           | -           | -           | -          | 11.867      | 0.53                               | 1.71                        | 1                           | 19.0                 | 0.90                               | 3.97                                 | 11.233                        | 0.25                          | 0.87        | 0.53 | 22.6        | 11.22       | 0.28        | 0.98  |
| 20100779+3131381 | 69.538      | -0.971      | 21.460     | 8            | -          | -          | -           | -          | -           | -             | -           | -   | -                      | -           | -           | -           | -           | -          | 9.844       | ...                                | ...                         | 1                           | 82.6                 | 0.36                               | 4.30                                 | 1.848                         | ...                           | ...         | 6.65 | ...         | ...         | ...         |       |
| 20100954+2728258 | 66.140      | -3.185      | 18.357     | 9            | -          | -          | -           | -          | -           | -             | -           | -   | -                      | -           | -           | -           | -           | -          | 12.737      | 0.97                               | ...                         | 1                           | 16.8                 | 1.00                               | 4.03                                 | 5.897                         | -2.07                         | ...         | 5.69 | ...         | ...         | -1.71       | ...   |
| 20101074+2729398 | 66.160      | -3.177      | 19.684     | 9            | -          | -          | -           | -          | -           | -             | -           | -   | -                      | -           | -           | -           | -           | -          | 8.367       | 1.18                               | 2.67                        | -2                          | 219.2                | 0.64                               | 4.03                                 | 1.033                         | -2.08                         | -7.11       | 6.10 | ...         | ...         | -1.69       | -5.81 |
| 20101270+2728558 | 66.153      | -3.190      | 19.077     | 9            | -          | -          | -           | -          | -           | -             | -           | -   | -                      | -           | -           | -           | -           | -          | 9.007       | 1.21                               | ...                         | 1                           | 212.0                | 0.20                               | 4.03                                 | 1.899                         | -1.95                         | ...         | 5.91 | ...         | ...         | -1.58       | ...   |
| 20101324+2850488 | 67.301      | -2.449      | 2.085      | 1            | -          | -          | h           | t          | N           | -             | D3          | -   | -                      | -           | -           | -           | -           | -          | 11.982      | 0.50                               | 1.69                        | 1                           | 23.4                 | 0.58                               | 4.13                                 | 11.205                        | 0.15                          | 0.66        | 0.65 | 29.9        | 11.14       | 0.19        | 0.80  |
| 20101871+2723438 | 66.093      | -3.256      | 8.266      | 9            | -          | -          | -           | -          | -           | -             | -           | -   | -                      | -           | -           | -           | -           | -          | 13.636      | 0.20                               | ...                         | -1                          | 10.0                 | 1.00                               | 4.03                                 | 10.556                        | -1.17                         | ...         | 2.56 | ...         | ...         | -1.01       | ...   |
| 20102369+4627398 | 82.136      | 7.094       | 0.605      | 8            | -          | p          | -           | -          | -           | -             | -           | cr  | -                      | -           | -           | -           | -           | -          | 10.384      | 0.80                               | 0.94                        | -2                          | 15.4                 | 0.52                               | 3.80                                 | 10.159                        | 0.70                          | 0.64        | 0.19 | ...         | ...         | 0.71        | 0.68  |
| 20103216+2730128 | 66.210      | -3.239      | 8.534      | 9            | -          | -          | -           | -          | -           | -             | -           | -   | -                      | -           | -           | -           | -           | -          | 13.524      | 0.77                               | ...                         | -1                          | 16.2                 | 0.44                               | 4.03                                 | 10.344                        | -0.64                         | ...         | 2.64 | ...         | ...         | -0.48       | ...   |
| 20104485+1744189 | 57.967      | -8.545      | 0.345      | 1            | -          | -          | h           | -          | -           | -             | -           | -   | -                      | -           | -           | -           | -           | -          | 11.223      | 0.37                               | 1.22                        | 1                           | 33.2                 | 0.82                               | 3.80                                 | 11.094                        | 0.31                          | 1.05        | 0.11 | 33.9        | 11.10       | 0.32        | 1.07  |
| 20105438+4701439 | 82.666      | 7.324       | 0.544      | 1            | -          | -          | h           | t          | -           | -             | D4          | -   | -                      | -           | -           | -           | -           | -          | 11.222      | 0.22                               | 0.65                        | -2                          | 30.0                 | 0.36                               | 3.79                                 | 11.019                        | 0.13                          | 0.38        | 0.17 | 31.2        | 11.03       | 0.14        | 0.42  |
| 20110038+3300518 | 70.885      | -0.314      | 4.180      | 8            | -          | -          | -           | -          | -           | -             | -           | -   | -                      | -           | -           | -           | -           | -          | 11.949      | 0.48                               | 2.07                        | 1                           | 16.8                 | 0.60                               | 4.28                                 | 10.392                        | -0.21                         | -0.01       | 1.29 | ...         | ...         | -0.13       | 0.27  |
| 20113049+4209265 | 78.603      | 4.600       | 1.250      | 1            | -          | -          | h           | t          | N           | -             | D1          | -   | -                      | -           | -           | -           | e           | -          | 11.682      | 0.61                               | 1.68                        | 1                           | 37.8                 | 0.36                               | 3.96                                 | 11.216                        | 0.41                          | 1.05        | 0.39 | 43.0        | 11.19       | 0.43        | 1.14  |
| 20113888+5028553 | 85.681      | 9.066       | 0.254      | 1            | -          | -          | -           | -          | -           | -             | D1          | -   | -                      | -           | -           | -           | -           | -          | 11.043      | 0.32                               | 1.04                        | 1                           | 42.8                 | 0.66                               | 3.76                                 | 10.948                        | 0.28                          | 0.91        | 0.08 | 43.4        | 10.96       | 0.28        | 0.93  |
| 20114417+2743549 | 66.547      | -3.337      | 2.634      | 1            | -          | -          | h           | t          | N           | -             | D2          | -   | -                      | -           | -           | -           | -           | -          | 11.760      | 0.74                               | 1.94                        | 1                           | 30.4                 | 0.50                               | 4.01                                 | 10.779                        | 0.31                          | 0.63        | 0.82 | 42.0        | 10.70       | 0.36        | 0.80  |
| 20114644+3649348 | 74.160      | 1.643       | 3.990      | 7            | -          | -          | -           | -          | -           | -             | -           | -   | -                      | -           | -           | -           | -           | -          | 10.092      | 0.80                               | 1.90                        | 1                           | 51.2                 | 0.82                               | 4.34                                 | 8.605                         | 0.14                          | -0.08       | 1.24 | ...         | ...         | 0.22        | 0.19  |
| 20114990+3424196 | 72.142      | 0.305       | 3.412      | 9            | -          | -          | -           | -          | -           | -             | -           | -   | -                      | -           | -           | -           | -           | -          | 11.961      | 0.29                               | ...                         | -2                          | 27.0                 | 0.54                               | 4.36                                 | 10.690                        | -0.27                         | ...         | 1.06 | ...         | ...         | -0.21       | ...   |
| 20115360+3652298 | 74.214      | 1.650       | 3.822      | 9            | -          | -          | -           | -          | -           | -             | -           | -   | -                      | -           | -           | -           | -           | -          | 11.255      | ...                                | ...                         | 1                           | 48.4                 | 0.18                               | 4.34                                 | 9.831                         | ...                           | ...         | 1.18 | ...         | ...         | ...         | ...   |
| 20115745+5141133 | 86.742      | 9.666       | 0.191      | 1            | -          | -          | h           | -          | -           | -             | D3          | -   | -                      | -           | -           | -           | -           | -          | 11.210      | 0.24                               | 0.97                        | 1                           | 34.6                 | 0.60                               | 3.61                                 | 11.139                        | 0.21                          | 0.88        | 0.06 | 34.9        | 11.15       | 0.21        | 0.89  |
| 20121513+3642546 | 74.120      | 1.502       | 3.734      | 7            | -          | -          | -           | -          | -           | -             | -           | -   | -                      | -           | -           | -           | -           | -          | 11.802      | ...                                | ...                         | 1                           | 22.2                 | 0.64                               | 4.38                                 | 10.411                        | ...                           | ...         | 1.16 | ...         | ...         | ...         | ...   |
| 20122414+1917287 | 59.504      | -8.046      | 0.267      | 1            | -          | -          | h           | t          | -           | -             | D1          | -   | -                      | -           | -           | -           | -           | -          | 10.407      | 0.39                               | 1.19                        | 1                           | 57.8                 | 0.40                               | 3.82                                 | 10.308                        | 0.34                          | 1.06        | 0.08 | 58.7        | 10.32       | 0.35        | 1.08  |
| 20123332+3555517 | 73.498      | 1.020       | 3.999      | 9            | -          | -          | -           | -          | -           | -             | -           | -   | -                      | -           | -           | -           | -           | -          | 10.731      | ...                                | ...                         | 1                           | 58.4                 | 0.46                               | 4.39                                 | 9.241                         | ...                           | ...         | 1.24 | ...         | ...         | ...         | ...   |
| 20123340+4048047 | 77.572      | 3.695       | 1.092      | 7            | -          | -          | -           | -          | -           | -             | -           | -   | -                      | -           | -           | -           | -           | -          | 11.076      | 0.89                               | 1.94                        | 1                           | 61.0                 | 0.72                               | 4.10                                 | 10.669                        | 0.71                          | 1.39        | 0.34 | ...         | ...         | 0.73        | 1.47  |
| 20124772+3420327 | 72.199      | 0.104       | 2.120      | 9            | -          | p?         | -           | -          | -           | -             | -           | -   | -                      | -           | -           | -           | -           | -          | 11.809      | ...                                | ...                         | -2                          | 15.8                 | 1.00                               | 4.40                                 | 10.019                        | ...                           | ...         | 0.66 | ...         | ...         | ...         | ...   |
| 20125530+4310184 | 79.599      | 4.936       | 1.621      | 1            | -          | -          | h           | t          | N           | -             | D1          | -   | -                      | -           | -           | -           | -           | -          | 11.447      | 0.39                               | 1.42                        | 1                           | 48.8                 | 0.62                               | 3.96                                 | 10.843                        | 0.12                          | 0.61        | 0.50 | 58.4        | 10.80       | 0.16        | 0.72  |
| 20133266+3123053 | 69.819      | -1.658      | 3.322      | 9            | -          | -          | -           | -          | -           | -             | -           | -   | -                      | -           | -           | -           | -           | -          | 11.863      | 1.40                               | ...                         | 1                           | 27.8                 | 0.34                               | 4.17                                 | 10.625                        | 0.84                          | ...         | 1.03 | ...         | ...         | 0.91        | ...   |
| 20133421+3614597 | 73.877      | 1.025       | 4.593      | 7            | -          | -          | -           | -          | -           | -             | -           | -   | -                      | -           | -           | -           | -           | -          | 9.637       | 1.00                               | 2.45                        | 1                           | 40.4                 | 0.84                               | 4.36                                 | 7.926                         | 0.24                          | 0.16        | 1.42 | ...         | ...         | 0.33        | 0.47  |
| 20133996+3314015 | 71.375      | -0.658      | 2.598      | 3            | -          | o          | -           | -          | t           | N             | D1          | -   | -                      | -           | -           | -           | -           | -          | 11.405      | 0.63                               | ...                         | -2                          | 44.4                 | 0.64                               | 4.37                                 | 10.437                        | 0.20                          | ...         | 0.80 | 61.2        | 10.35       | 0.25        | ...   |
| 20135618+4443093 | 81.000      | 5.629       | 1.303      | 1            | -          | -          | h           | t          | N           | -             | D1          | -   | -                      | -           | -           | -           | -           | -          | 11.286      | 0.50                               | 1.52                        | 1                           | 44.8                 | 0.42                               | 3.92                                 | 10.801                        | 0.29                          | 0.87        | 0.40 | 51.0        | 10.79       | 0.31        | 0.96  |
| 20135690+2902036 | 67.905      | -3.028      | 1.614      | 1            | -          | -          | -           | -          | t           | N             | D1          | -   | -                      | -           | -           | -           | -           | -          | 10.912      | 0.53                               | 1.61                        | 1                           | 53.8                 | 0.66                               | 4.13                                 | 10.311                        | 0.27                          | 0.81        | 0.50 | 64.6        | 10.26       | 0.30        | 0.92  |
| 20135750+3716099 | 74.770      | 1.524       | 2.242      | 7            | -          | -          | -           | -          | -           | -             | -           | -   | -                      | -           | -           | -           | -           | -          | 10.082      | 1.88                               | ...                         | 1                           | 22.4                 | 0.36                               | 4.32                                 | 9.247                         | 1.51                          | ...         | 0.69 | ...         | ...         | 1.55        | ...   |
| 20141998+3732490 | 75.043      | 1.615       | 2.284      | 1            | -          | o          | -           | -          | -           | -             | D1          | -   | -                      | -           | -           | -           | -           | -          | 10.889      | 0.78                               | ...                         | 1                           | 61.6                 | 0.20                               | 4.29                                 | 10.038                        | 0.40                          | ...         | 0.71 | 81.2        | 9.96        | 0.44        | ...   |
| 20142587+4113370 | 78.123      | 3.634       | 4.449      | 8            | -          | -          | h           | -          | -           | -             | -           | -   | -                      | -           | -           | -           | -           | -          | 9.467       | 2.13                               | 3.78                        | 1                           | 51.2                 | 0.30                               | 4.09                                 | 7.809                         | 1.39                          | 1.57        | 1.38 | ...         | ...         | 1.48        | 1.86  |
| 20145323+3603032 | 73.859      | 0.693       | 3.576      | 9            | -          | -          | -           | -          | -           | -             | -           | -   | -                      | -           | -           | -           | -           | -          | 11.977      | ...                                | ...                         | 1                           | 25.6                 | 1.00                               | 4.33                                 | 10.645                        | ...                           | ...         | 1.11 | ...         | ...         | ...         | ...   |
| 20150392+3645527 | 74.473      | 1.060       | 4.344      | 9            | -          | -          | -           | -          | -           | -             | D2          | -   | -                      | -           | -           | -           | -           | -          | 11.908      | ...                                | ...                         | 1                           | 19.2                 | 0.68                               | 4.37                                 | 10.289                        | ...                           | ...         | 1.35 | ...         | ...         | ...         | ...   |
| 20152415+5007412 | 85.705      | 8.371       | 0.368      | 1            | -          | -          | h           | -          | -           | -             | D2          | -   | -                      | -           | -           | -           | -           | -          | 11.348      | 0.31                               | 1.09                        | 1                           | 29.6                 | 0.64                               | 3.80                                 | 11.211                        | 0.25                          | 0.90        | 0.11 | 30.2        | 11.22       | 0.26        | 0.93  |
| 20160867+2251076 | 62.998      | -6.845      | 0.627      | 1            | -          | -          | -           | -          | c           | -             | D1          | -   | -                      | -           | -           | -           | -           | -          | 11.147      | 0.31                               | 1.18                        | 1                           | 27.4                 | 0.90                               | 3.78                                 | 10.913                        | 0.21                          | 0.87        | 0.19 | 28.7        | 10.93       | 0.22        | 0.91  |
| 20161122+3423227 | 72.627      | -0.452      | 3.213      | 9            | -          | -          | -           | -          | -           | -             | -           | -   | -                      | -           | -           | -           | -           | -          | 7.830       | ...                                | ...                         | -2                          | 34.0                 | 1.00                               | 4.35                                 | 6.633                         | ...                           | ...         | 1.00 | ...         | ...         | ...         | ...   |
| 20162742+3654543 | 74.753      | 0.912       | 3.747      | 8            | -          | o          | -           | -          | -           | -             | -           | -   | -                      | -           | -           | -           | -           | -          | 11.497      | ...                                | ...                         | 1                           | 33.2                 | 0.56                               | 4.33                                 | 10.101                        | ...                           | ...         | 1.16 | ...         | ...         | ...         | ...   |
| 20164862+3906203 | 76.609      | 2.078       | 3.002      | 8            | -          | -          | -           | -          | -           | -             | -           | -   | -                      | -           | -           | -           | -           | -          | 11.063      | 0.63                               | 1.61                        | -2                          | 36.0                 | 0.76                               | 4.25                                 | 9.944                         | 0.13                          | 0.12        | 0.93 | ...         | ...         | 0.19        | 0.32  |
| 20165034+3449467 | 73.067      | -0.317      | 5.779      | 8            | -          | -          | -           | -          | -           | -             | -           | -   | -                      | -           | -           | -           | -           | -          | 9.517       | 0.89                               | 2.00                        | -2                          | 83.8                 | 0.52                               | 4.33                                 | 7.364                         | -0.06                         | -0.87       | 1.79 | ...         | ...         | 0.05        | -0.49 |
| 20165717+4411158 | 80.853      | 4.887       | 2.333      | 9            | -          | -          | -           | -          | -           | -             | -           | -   | -                      | -           | -           | -           | -           | -          | 11.332      | 2.42                               | ...                         | 1                           | 25.4                 | 0.46                               | 3.98                                 | 10.463                        | 2.03                          | ...         | 0.72 | ...         | ...         | 2.08        | ...   |
| 20165918+3630203 | 74.472      | 0.596       | 3.451      | 8            | -          | -          | -           | -          | -           | -             | -           | -   | -                      | -           | -           | -           | -           | -          | 12.221      | 0.71                               | ...                         | 1                           | 23.6                 | 0.36                               | 4.34                                 | 10.935                        | 0.14                          | ...         | 1.07 | ...         | ...         | 0.21        | ...   |
| 20165949+3929513 | 76.954      | 2.268       | 4.150      | 8            | -          | -          | -           | -          | -           | -             | -           | -   | -                      | -           | -           | -           | -           | -          | 11.798      | 1.23                               | ...                         | 1                           | 26.8                 | 0.36                               | 4.20                                 | 10.252                        | 0.55                          | ...         | 1.29 | ...         | ...         | 0.63        | ...   |
| 20170253+3150065 | 70.607      | -2.027      | 2.592      | 1            | -          | o          | -           | -          | t           | N             | D1          | -   | -                      | -           | -           | -           | -           | -          | 10.253      | 0.65                               | 1.99                        | 1                           | 74.8                 | 0.34                               | 4.19                                 | 9.287                         | 0.22                          | 0.70        | 0.80 | 106.5       | 9.13        | 0.27        | 0.87  |
| 20171300+4341267 | 80.465      | 4.572       | 1.178      | 1            | -          | o          |             |            |             |               |             |     |                        |             |             |             |             |            |             |                                    |                             |                             |                      |                                    |                                      |                               |                               |             |      |             |             |             |       |

Table B1: a) continued.

| 2MASX J          | <i>l</i>    | <i>b</i>    | EBV        | Object       | Sample     | Disc        | 2MRS        | Velocity   | NIR         | Photom        | Ext         | <i>K</i> <sub>20</sub> | <i>H-K</i>   | <i>J-K</i>  | vc          | <i>a</i>    | <i>b/a</i>  | st.d. | <i>K</i> <sub>s</sub> <sup>o</sup> | ( <i>H-K</i> ) <sup>o</sup> | ( <i>J-K</i> ) <sup>o</sup> | <i>A</i> <sub>K</sub> | <i>a</i> <sub>d</sub> <sup>o</sup> | <i>K</i> <sub>s</sub> <sup>o,d</sup> | ( <i>H-K</i> ) <sup>o,c</sup> | ( <i>J-K</i> ) <sup>o,c</sup> |             |             |       |             |             |             |        |
|------------------|-------------|-------------|------------|--------------|------------|-------------|-------------|------------|-------------|---------------|-------------|------------------------|--------------|-------------|-------------|-------------|-------------|-------|------------------------------------|-----------------------------|-----------------------------|-----------------------|------------------------------------|--------------------------------------|-------------------------------|-------------------------------|-------------|-------------|-------|-------------|-------------|-------------|--------|
| (1)              | deg<br>(2a) | deg<br>(2b) | mag<br>(3) | class<br>(4) | off<br>(5) | flag<br>(6) | gal<br>(7a) | TF<br>(7b) | obs<br>(7c) | ext'd<br>(7d) | type<br>(8) | (9)                    | Opt<br>(10a) | HI<br>(10b) | flg<br>(11) | flg<br>(12) | flg<br>(13) | (14)  | mag<br>(15)                        | mag<br>(16)                 | (17)                        | (18)                  | (19)                               | (20)                                 | mag<br>(21)                   | mag<br>(22)                   | mag<br>(23) | mag<br>(24) | (25)  | mag<br>(26) | mag<br>(27) | mag<br>(28) |        |
| 20210368+3733236 | 75.799      | 0.517       | 8.784      | 8            | —          | —           | —           | —          | —           | —             | —           | —                      | U            | —           | —           | —           | —           | —     | 11.459                             | 1.09                        | ...                         | 1                     | 38.0                               | 0.28                                 | 4.28                          | 8.186                         | -0.36       | ...         | 2.72  | ...         | ...         | -0.19       | ...    |
| 20211725+4002112 | 77.865      | 1.890       | 6.829      | 9            | —          | —           | —           | —          | —           | —             | —           | —                      | —            | —           | —           | —           | —           | —     | 13.159                             | 0.51                        | 1.64                        | -1                    | 17.2                               | 0.52                                 | 4.17                          | 10.615                        | -0.62       | -1.75       | 2.12  | ...         | ...         | -0.49       | -1.30  |
| 20212069+2230211 | 63.376      | -8.036      | 0.497      | 2            | —          | —           | g           | —          | t           | —             | n           | cp                     | o            | —           | —           | —           | p           | —     | 10.923                             | 0.14                        | 0.28                        | 1                     | 37.4                               | 0.40                                 | 3.78                          | 10.738                        | 0.05        | 0.03        | 0.15  | 39.0        | 10.73       | 0.06        | 0.06   |
| 20212173+3729362 | 75.781      | 0.432       | 30.950     | 8            | —          | —           | —           | —          | —           | —             | —           | —                      | —            | —           | —           | —           | —           | —     | 10.295                             | 1.18                        | ...                         | 1                     | 61.2                               | 0.66                                 | 4.30                          | -1.237                        | -3.94       | ...         | 9.59  | ...         | ...         | -3.34       | ...    |
| 20212592+4438079 | 81.675      | 4.476       | 2.719      | 1            | —          | —           | g           | —          | —           | N             | —           | D1                     | —            | —           | —           | —           | e           | —     | 10.841                             | 0.59                        | 2.05                        | 1                     | 36.2                               | 0.90                                 | 4.02                          | 9.828                         | 0.14        | 0.70        | 0.84  | 48.8        | 9.80        | 0.19        | 0.88   |
| 20213489+3724417 | 75.738      | 0.349       | 36.065     | 9            | —          | —           | —           | —          | —           | —             | —           | —                      | —            | —           | —           | —           | —           | —     | 10.690                             | ...                         | ...                         | -2                    | 49.2                               | 1.00                                 | 4.26                          | -2.748                        | ...         | ...         | 11.17 | ...         | ...         | ...         | ...    |
| 20213785+3725362 | 75.756      | 0.350       | 43.180     | 9            | —          | —           | —           | —          | —           | —             | —           | —                      | —            | —           | —           | —           | —           | —     | 10.284                             | 1.09                        | 2.05                        | 1                     | 53.6                               | 0.56                                 | 4.26                          | -5.805                        | -6.06       | -19.40      | 13.38 | ...         | ...         | -5.21       | -16.55 |
| 20214050+3726203 | 75.771      | 0.350       | 48.407     | 9            | —          | —           | —           | —          | —           | —             | —           | —                      | —            | —           | —           | —           | —           | —     | 9.075                              | ...                         | ...                         | 1                     | 81.4                               | 1.00                                 | 4.30                          | -8.961                        | ...         | ...         | 14.99 | ...         | ...         | ...         | ...    |
| 20214095+3726122 | 75.770      | 0.347       | 47.821     | 9            | —          | —           | —           | —          | —           | —             | —           | —                      | —            | —           | —           | —           | —           | —     | 7.529                              | 1.50                        | 2.98                        | 1                     | 218.8                              | 0.42                                 | 4.26                          | -10.289                       | -6.42       | -20.78      | 14.81 | ...         | ...         | -5.48       | -17.63 |
| 20214160+3725313 | 75.762      | 0.339       | 43.893     | 9            | —          | —           | —           | —          | —           | —             | —           | —                      | —            | —           | —           | —           | —           | —     | 7.373                              | 1.65                        | ...                         | 1                     | 105.8                              | 0.44                                 | 4.30                          | -8.982                        | -5.62       | ...         | 13.60 | ...         | ...         | -4.76       | ...    |
| 20214907+4400399 | 81.198      | 4.065       | 1.321      | 1            | —          | —           | g           | —          | —           | N             | —           | D1                     | —            | —           | —           | —           | e           | —     | 11.200                             | 0.55                        | 1.67                        | 1                     | 36.6                               | 0.68                                 | 4.08                          | 10.708                        | 0.33        | 1.01        | 0.41  | 41.4        | 10.71       | 0.36        | 1.10   |
| 20215381+5224323 | 88.197      | 8.775       | 0.256      | 1            | —          | —           | g           | —          | t           | —             | D1          | c                      | o            | h           | —           | —           | —           | —     | 10.943                             | 0.37                        | 1.13                        | 1                     | 48.2                               | 0.26                                 | 3.72                          | 10.848                        | 0.32        | 1.00        | 0.08  | 48.9        | 10.85       | 0.33        | 1.02   |
| 20215509+3959455 | 77.900      | 1.767       | 9.867      | 8            | —          | —           | —           | —          | —           | —             | —           | —                      | —            | —           | —           | —           | —           | —     | 8.920                              | 1.84                        | 4.10                        | 1                     | 93.6                               | 0.80                                 | 4.10                          | 5.244                         | 0.21        | -0.80       | 3.06  | ...         | ...         | 0.40        | -0.15  |
| 20215739+4013235 | 78.091      | 1.891       | 7.062      | 7            | —          | —           | —           | —          | —           | —             | —           | —                      | —            | —           | —           | —           | —           | —     | 11.600                             | 0.84                        | 2.41                        | -2                    | 13.6                               | 0.98                                 | 4.17                          | 8.969                         | -0.33       | -1.10       | 2.19  | ...         | ...         | -0.19       | -0.64  |
| 20215769+3733075 | 75.897      | 0.367       | 21.669     | 9            | —          | —           | —           | —          | —           | —             | —           | —                      | —            | —           | —           | —           | —           | —     | 11.060                             | 0.05                        | 2.12                        | -2                    | 51.8                               | 0.86                                 | 4.30                          | 2.986                         | -3.54       | -8.64       | 6.71  | ...         | ...         | -3.12       | -7.21  |
| 20220701+3957296 | 77.891      | 1.715       | 10.233     | 8            | —          | —           | —           | —          | —           | —             | —           | —                      | —            | —           | —           | —           | —           | —     | 12.479                             | 1.19                        | ...                         | 1                     | 28.4                               | 0.44                                 | 4.10                          | 8.666                         | -0.50       | ...         | 3.17  | ...         | ...         | -0.30       | ...    |
| 20220719+3957586 | 77.898      | 1.719       | 10.422     | 3            | —          | —           | g           | —          | —           | N             | —           | D3                     | —            | —           | —           | —           | e           | —     | 12.554                             | 1.01                        | 2.40                        | -2                    | 15.4                               | 1.00                                 | 4.10                          | 8.671                         | -0.71       | -2.78       | 3.23  | 68.4        | 8.31        | -0.51       | -2.09  |
| 20220805+4006396 | 78.019      | 1.799       | 9.485      | 7            | o          | —           | —           | —          | —           | —             | —           | —                      | —            | —           | —           | —           | —           | —     | 12.837                             | 1.07                        | ...                         | 1                     | 13.6                               | 0.82                                 | 4.10                          | 9.303                         | -0.50       | ...         | 2.94  | ...         | ...         | -0.31       | ...    |
| 20220989+2459351 | 65.560      | -6.799      | 0.539      | 2            | —          | —           | g           | —          | —           | —             | n           | c                      | o            | —           | —           | —           | —           | —     | 11.150                             | 0.40                        | 1.12                        | 1                     | 30.2                               | 0.76                                 | 3.79                          | 10.949                        | 0.31        | 0.85        | 0.17  | 31.3        | 10.96       | 0.32        | 0.88   |
| 20221606+3956236 | 77.893      | 1.680       | 9.536      | 9            | —          | —           | —           | —          | —           | —             | —           | —                      | —            | —           | —           | —           | —           | —     | 13.489                             | 0.44                        | 1.65                        | -1                    | 10.4                               | 0.62                                 | 4.10                          | 9.936                         | -1.13       | -3.09       | 2.95  | ...         | ...         | -0.95       | -2.46  |
| 20222222+3957557 | 77.925      | 1.679       | 10.135     | 8            | —          | —           | —           | —          | —           | —             | —           | —                      | —            | —           | —           | —           | —           | —     | 8.820                              | 1.33                        | 3.26                        | 1                     | 142.0                              | 0.82                                 | 4.15                          | 5.044                         | -0.35       | -1.78       | 3.14  | ...         | ...         | -0.15       | -1.11  |
| 20223164+4012478 | 78.145      | 1.796       | 10.180     | 9            | —          | —           | —           | —          | —           | —             | —           | —                      | —            | —           | —           | —           | —           | —     | 10.895                             | 0.72                        | 1.40                        | 1                     | 53.4                               | 0.40                                 | 4.23                          | 7.102                         | -0.97       | -3.66       | 3.15  | ...         | ...         | -0.77       | -2.98  |
| 20223320+4014118 | 78.167      | 1.805       | 9.339      | 9            | —          | —           | —           | —          | —           | —             | —           | —                      | —            | —           | —           | —           | —           | —     | 12.698                             | 0.17                        | 1.40                        | -2                    | 19.0                               | 0.52                                 | 4.23                          | 9.218                         | -1.37       | -3.24       | 2.89  | ...         | ...         | -1.19       | -2.62  |
| 20224366+3921289 | 77.465      | 1.275       | 3.251      | 9            | —          | —           | —           | —          | —           | —             | —           | —                      | —            | —           | —           | —           | —           | —     | 11.799                             | 0.48                        | 1.41                        | -2                    | 15.6                               | 0.76                                 | 4.31                          | 10.588                        | -0.06       | -0.21       | 1.01  | ...         | ...         | 0.01        | 0.01   |
| 20225406+4159049 | 79.641      | 2.749       | 5.718      | 9            | —          | —           | —           | —          | —           | —             | —           | —                      | —            | —           | —           | —           | —           | —     | 13.239                             | 0.61                        | 1.62                        | -1                    | 10.6                               | 1.00                                 | 4.07                          | 11.108                        | -0.34       | -1.22       | 1.77  | ...         | ...         | -0.23       | -0.84  |
| 20231262+3925015 | 77.567      | 1.233       | 2.453      | 7            | —          | p?          | —           | —          | —           | N             | —           | —                      | —            | —           | —           | —           | —           | —     | 10.062                             | 1.42                        | 3.35                        | 1                     | 37.6                               | 0.46                                 | 4.33                          | 9.148                         | 1.01        | 2.13        | 0.76  | ...         | ...         | 1.06        | 2.29   |
| 20232385+4117404 | 79.127      | 2.279       | 7.406      | 8            | —          | —           | —           | —          | —           | —             | —           | —                      | —            | —           | —           | —           | —           | —     | 8.826                              | 1.88                        | 4.26                        | 1                     | 68.6                               | 0.56                                 | 4.05                          | 6.067                         | 0.66        | 0.58        | 2.29  | ...         | ...         | 0.80        | 1.07   |
| 20232447+3652534 | 75.511      | -0.252      | 3.987      | 9            | —          | —           | —           | —          | —           | —             | —           | —                      | —            | —           | —           | —           | —           | —     | 12.602                             | 0.62                        | 1.88                        | 1                     | 12.8                               | 0.60                                 | 4.25                          | 11.116                        | -0.04       | -0.10       | 1.23  | ...         | ...         | 0.04        | 0.16   |
| 20232714+3734504 | 76.089      | 0.141       | 4.163      | 8            | o          | —           | —           | —          | —           | —             | —           | —                      | —            | —           | —           | o           | —           | —     | 11.005                             | 2.08                        | ...                         | 1                     | 32.4                               | 0.58                                 | 4.19                          | 9.454                         | 1.39        | ...         | 1.29  | ...         | ...         | 1.48        | ...    |
| 20232734+3734572 | 76.091      | 0.142       | 4.204      | 8            | o          | —           | —           | —          | —           | —             | —           | —                      | —            | —           | —           | o           | —           | —     | 10.664                             | 1.96                        | ...                         | 1                     | 41.8                               | 0.50                                 | 4.26                          | 9.098                         | 1.27        | ...         | 1.30  | ...         | ...         | 1.35        | ...    |
| 20234437+4117013 | 79.155      | 2.220       | 8.792      | 8            | —          | —           | —           | —          | —           | —             | —           | —                      | —            | —           | —           | —           | —           | —     | 11.778                             | ...                         | ...                         | 1                     | 30.4                               | 0.56                                 | 4.05                          | 8.502                         | ...         | ...         | 2.72  | ...         | ...         | ...         | ...    |
| 20234472+3541201 | 74.573      | -0.992      | 4.306      | 7            | —          | —           | —           | —          | —           | —             | —           | D2                     | c            | o           | —           | —           | —           | —     | 11.055                             | 1.37                        | ...                         | -2                    | 25.8                               | 0.76                                 | 4.26                          | 9.451                         | 0.66        | ...         | 1.33  | ...         | ...         | 0.74        | ...    |
| 20235668+2542038 | 66.377      | -6.732      | 0.397      | 1            | —          | —           | g           | —          | —           | —             | —           | —                      | —            | —           | —           | —           | —           | —     | 11.050                             | 0.38                        | 1.18                        | 1                     | 32.4                               | 0.94                                 | 3.81                          | 10.902                        | 0.31        | 0.99        | 0.12  | 33.2        | 10.91       | 0.32        | 1.01   |
| 20240016+3736523 | 76.179      | 0.072       | 9.251      | 9            | —          | —           | —           | —          | —           | —             | —           | —                      | —            | —           | —           | —           | —           | —     | 7.624                              | 1.64                        | ...                         | 1                     | 57.0                               | 0.64                                 | 4.26                          | 4.177                         | 0.11        | ...         | 2.87  | ...         | ...         | 0.29        | ...    |
| 20240508+4126022 | 79.316      | 2.253       | 8.537      | 8            | —          | —           | —           | —          | —           | —             | —           | —                      | —            | —           | —           | —           | —           | —     | 12.491                             | 0.74                        | 2.31                        | -2                    | 15.6                               | 0.64                                 | 4.05                          | 9.310                         | -0.67       | -1.94       | 2.64  | ...         | ...         | -0.50       | -1.37  |
| 20241125+3551304 | 74.764      | -0.968      | 5.695      | 8            | —          | —           | —           | —          | —           | —             | e           | g                      | —            | —           | —           | —           | —           | —     | 9.916                              | 0.80                        | 2.00                        | 1                     | 89.8                               | 0.44                                 | 4.25                          | 7.794                         | -0.14       | -0.83       | 1.76  | ...         | ...         | -0.03       | -0.45  |
| 20241257+3551382 | 74.768      | -0.971      | 5.755      | 8            | —          | —           | —           | —          | —           | —             | —           | —                      | —            | —           | —           | —           | —           | —     | 9.955                              | 0.90                        | 2.16                        | 1                     | 142.4                              | 0.24                                 | 4.28                          | 7.811                         | -0.06       | -0.70       | 1.78  | ...         | ...         | 0.06        | -0.32  |
| 20242022+2703499 | 67.557      | -6.031      | 0.600      | 1            | —          | —           | g           | —          | —           | —             | D1          | c                      | o            | —           | —           | —           | —           | —     | 9.898                              | 0.33                        | 1.16                        | 1                     | 75.4                               | 0.64                                 | 3.89                          | 9.674                         | 0.23        | 0.87        | 0.19  | 78.3        | 9.69        | 0.24        | 0.91   |
| 20242063+4215497 | 80.024      | 2.690       | 5.672      | 9            | —          | —           | —           | —          | —           | —             | —           | —                      | —            | —           | —           | —           | —           | —     | 9.046                              | 1.88                        | ...                         | 1                     | 99.0                               | 0.50                                 | 4.05                          | 6.933                         | 0.94        | ...         | 1.76  | ...         | ...         | 1.05        | ...    |
| 20242961+4203579 | 79.878      | 2.553       | 5.925      | 9            | —          | —           | —           | —          | —           | —             | —           | —                      | —            | —           | —           | —           | —           | —     | 12.805                             | 1.09                        | ...                         | -2                    | 29.8                               | 0.42                                 | 3.99                          | 10.597                        | 0.11        | ...         | 1.84  | ...         | ...         | 0.23        | ...    |
| 20244119+4207520 | 79.951      | 2.561       | 6.455      | 9            | —          | —           | —           | —          | —           | —             | —           | —                      | —            | —           | —           | —           | —           | —     | 13.149                             | ...                         | ...                         | 1                     | 22.8                               | 0.30                                 | 3.99                          | 10.744                        | ...         | ...         | 2.00  | ...         | ...         | ...         | ...    |
| 20244243+4003353 | 78.259      | 1.366       | 8.723      | 9            | —          | —           | —           | —          | —           | —             | —           | —                      | —            | —           | —           | —           | —           | —     | 13.187                             | 0.74                        | ...                         | -1                    | 10.0                               | 1.00                                 | 4.11                          | 9.937                         | -0.71       | ...         | 2.70  | ...         | ...         | -0.54       | ...    |
| 20244437+4231440 | 80.283      | 2.782       | 5.528      | 9            | —          | —           | —           | —          | —           | —             | —           | —                      | —            | —           | —           | —           | —           | —     | 13.128                             | ...                         | ...                         | 1                     | 21.2                               | 0.36                                 | 4.15                          | 11.068                        | ...         | ...         | 1.71  | ...         | ...         | ...         | ...    |
| 20245239+4040249 | 78.779      | 1.694       | 2.427      | 8            | —          | —           | —           | —          |             |               |             |                        |              |             |             |             |             |       |                                    |                             |                             |                       |                                    |                                      |                               |                               |             |             |       |             |             |             |        |

Table B1: a) continued.

| 2MASX J          | <i>l</i>    | <i>b</i>    | EBV        | Object       |            | Sample     | Disc        | 2MRS       | Velocity    | NIR           | Photom      | Ext | <i>K</i> <sub>20</sub> | <i>H-K</i>  | <i>J-K</i>  | vc          | <i>a</i>    | <i>b/a</i> | st.d.       | <i>K</i> <sub>s</sub> <sup>o</sup> | ( <i>H-K</i> ) <sup>o</sup> | ( <i>J-K</i> ) <sup>o</sup> | <i>A</i> <sub>K</sub> | <i>a</i> <sub>d</sub> <sup>o</sup> | <i>K</i> <sub>s</sub> <sup>o,d</sup> | ( <i>H-K</i> ) <sup>o,c</sup> | ( <i>J-K</i> ) <sup>o,c</sup> |             |       |             |             |             |       |       |
|------------------|-------------|-------------|------------|--------------|------------|------------|-------------|------------|-------------|---------------|-------------|-----|------------------------|-------------|-------------|-------------|-------------|------------|-------------|------------------------------------|-----------------------------|-----------------------------|-----------------------|------------------------------------|--------------------------------------|-------------------------------|-------------------------------|-------------|-------|-------------|-------------|-------------|-------|-------|
| (1)              | deg<br>(2a) | deg<br>(2b) | mag<br>(3) | class<br>(4) | off<br>(5) | flg<br>(6) | gal<br>(7a) | TF<br>(7b) | obs<br>(7c) | ext'd<br>(7d) | type<br>(8) | (9) | Opt<br>(10a)           | HI<br>(10b) | flg<br>(11) | flg<br>(12) | flg<br>(13) | (14)       | mag<br>(15) | mag<br>(16)                        | (17)                        | (18)                        | (19)                  | (20)                               | mag<br>(21)                          | mag<br>(22)                   | mag<br>(23)                   | mag<br>(24) | (25)  | mag<br>(26) | mag<br>(27) | mag<br>(28) |       |       |
| 20280687+4051016 | 79.279      | 1.296       | 17.603     | 9            | —          | —          | —           | —          | —           | —             | —           | —   | —                      | —           | —           | —           | —           | —          | —           | 10.090                             | 1.96                        | ...                         | 1                     | 61.0                               | 1.00                                 | 4.19                          | 3.531                         | −0.96       | ...   | 5.45        | ...         | ...         | −0.61 | ...   |
| 20280916+4051506 | 79.294      | 1.298       | 20.095     | 9            | —          | —          | —           | —          | —           | —             | —           | —   | —                      | —           | —           | —           | —           | —          | —           | 7.770                              | 1.42                        | 3.29                        | 1                     | 219.0                              | 0.54                                 | 4.19                          | 0.283                         | −1.90       | −6.69 | 6.22        | ...         | ...         | −1.51 | −5.37 |
| 20280978+4052446 | 79.308      | 1.306       | 22.163     | 8            | —          | —          | —           | —          | —           | —             | —           | —   | —                      | —           | —           | —           | —           | —          | —           | 7.564                              | 1.37                        | 2.84                        | 1                     | 232.8                              | 0.48                                 | 4.19                          | −0.694                        | −2.30       | −8.17 | 6.87        | ...         | ...         | −1.86 | −6.71 |
| 20281331+4051576 | 79.303      | 1.289       | 20.527     | 9            | —          | —          | —           | —          | —           | —             | —           | —   | —                      | —           | —           | —           | —           | —          | —           | 11.130                             | 0.97                        | 2.80                        | −2                    | 30.0                               | 0.64                                 | 4.19                          | 3.482                         | −2.43       | −7.40 | 6.36        | ...         | ...         | −2.03 | −6.04 |
| 20281622+4053026 | 79.323      | 1.292       | 21.043     | 9            | —          | —          | —           | —          | —           | —             | —           | —   | —                      | —           | —           | —           | —           | —          | —           | 9.481                              | ...                         | ...                         | 1                     | 86.6                               | 0.56                                 | 4.19                          | 1.640                         | ...         | ...   | 6.52        | ...         | ...         | ...   | ...   |
| 20281822+4056451 | 79.377      | 1.323       | 17.571     | 8            | —          | —          | —           | —          | —           | —             | —           | —   | —                      | —           | —           | —           | —           | —          | —           | 11.781                             | ...                         | ...                         | 1                     | 33.0                               | 0.70                                 | 4.18                          | 5.234                         | ...         | ...   | 5.44        | ...         | ...         | ...   | ...   |
| 20282044+4052591 | 79.330      | 1.281       | 19.188     | 8            | —          | —          | —           | —          | —           | —             | —           | —   | —                      | —           | —           | —           | —           | —          | —           | 11.520                             | 1.59                        | ...                         | 1                     | 30.8                               | 0.84                                 | 4.18                          | 4.371                         | −1.59       | ...   | 5.94        | ...         | ...         | −1.21 | ...   |
| 20282133+4049281 | 79.284      | 1.244       | 12.895     | 8            | —          | —          | —           | —          | —           | —             | —           | —   | —                      | —           | —           | —           | —           | —          | —           | 12.763                             | ...                         | ...                         | −2                    | 19.0                               | 1.00                                 | 4.18                          | 7.958                         | ...         | ...   | 3.99        | ...         | ...         | ...   | ...   |
| 20282650+4100401 | 79.446      | 1.340       | 8.411      | 9            | —          | —          | —           | —          | —           | —             | —           | —   | —                      | —           | —           | —           | —           | —          | —           | 13.850                             | ...                         | ...                         | −2                    | 13.8                               | 0.26                                 | 4.12                          | 10.716                        | ...         | ...   | 2.61        | ...         | ...         | ...   | ...   |
| 20282884+2543241 | 66.983      | −7.558      | 0.443      | 1            | —          | —          | —           | —          | —           | —             | —           | —   | —                      | —           | —           | —           | —           | —          | —           | 8.868                              | 0.36                        | 1.18                        | 1                     | 72.0                               | 0.40                                 | 3.74                          | 8.703                         | 0.29        | 0.96  | 0.14        | 73.5        | 8.72        | 0.30  | 0.99  |
| 20283445+3554282 | 75.319      | −1.664      | 3.981      | 8            | —          | —          | —           | —          | —           | —             | —           | —   | —                      | —           | —           | —           | —           | —          | —           | 10.742                             | 1.05                        | 2.87                        | 1                     | 36.6                               | 0.86                                 | 4.16                          | 9.259                         | 0.39        | 0.89  | 1.23        | ...         | ...         | 0.46  | 1.15  |
| 20283506+2544001 | 67.005      | −7.572      | 0.443      | 1            | —          | —          | —           | —          | —           | —             | —           | —   | —                      | —           | —           | —           | —           | —          | —           | 9.926                              | 0.46                        | 1.39                        | 1                     | 58.6                               | 0.44                                 | 3.74                          | 9.761                         | 0.39        | 1.17  | 0.14        | 60.0        | 9.78        | 0.40  | 1.20  |
| 20290447+4032102 | 79.130      | 0.965       | 5.637      | 8            | —          | —          | —           | —          | —           | —             | —           | —   | —                      | —           | —           | —           | —           | —          | —           | 8.401                              | 1.23                        | 2.88                        | 1                     | 73.8                               | 0.54                                 | 4.27                          | 6.301                         | 0.30        | 0.08  | 1.75        | ...         | ...         | 0.41  | 0.45  |
| 20290596+2442225 | 66.224      | −8.257      | 0.414      | 1            | —          | —          | —           | —          | —           | —             | —           | —   | —                      | —           | —           | —           | —           | —          | —           | 11.297                             | 0.40                        | 1.17                        | 1                     | 32.0                               | 0.56                                 | 3.73                          | 11.143                        | 0.33        | 0.97  | 0.13        | 32.8        | 11.15       | 0.34  | 0.99  |
| 20292220+4131443 | 79.968      | 1.502       | 6.797      | 8            | —          | —          | —           | —          | —           | —             | —           | —   | —                      | —           | —           | —           | —           | —          | —           | 12.639                             | 0.61                        | 1.75                        | −2                    | 16.2                               | 0.66                                 | 4.21                          | 10.106                        | −0.52       | −1.62 | 2.11        | ...         | ...         | −0.38 | −1.17 |
| 20292312+4010563 | 78.878      | 0.710       | 13.329     | 9            | —          | —          | —           | —          | —           | —             | —           | —   | —                      | —           | —           | —           | —           | —          | —           | 10.241                             | 1.31                        | 2.87                        | 1                     | 42.8                               | 0.30                                 | 4.22                          | 5.275                         | −0.90       | −3.75 | 4.13        | ...         | ...         | −0.63 | −2.87 |
| 20292828+4011133 | 78.892      | 0.699       | 13.704     | 8            | —          | —          | —           | —          | —           | —             | —           | —   | —                      | —           | —           | —           | —           | —          | —           | 10.228                             | 1.58                        | ...                         | 1                     | 68.0                               | 0.92                                 | 4.21                          | 5.122                         | −0.69       | ...   | 4.24        | ...         | ...         | −0.42 | ...   |
| 20293179+3901203 | 77.955      | 0.007       | 14.928     | 8            | —          | —          | —           | —          | —           | —             | —           | —   | —                      | —           | —           | —           | —           | —          | —           | 9.344                              | 1.41                        | 3.00                        | 1                     | 98.0                               | 0.48                                 | 4.18                          | 3.782                         | −1.06       | −4.41 | 4.62        | ...         | ...         | −0.77 | −3.43 |
| 20293650+3902274 | 77.979      | 0.005       | 16.160     | 9            | —          | —          | —           | —          | —           | —             | —           | —   | —                      | —           | —           | —           | —           | —          | —           | 11.194                             | 1.26                        | ...                         | 1                     | 38.0                               | 0.64                                 | 4.18                          | 5.173                         | −1.42       | ...   | 5.01        | ...         | ...         | −1.10 | ...   |
| 20293694+3901224 | 77.965      | −0.007      | 15.703     | 8            | —          | —          | —           | —          | —           | —             | —           | —   | —                      | —           | —           | —           | —           | —          | —           | 8.851                              | 1.31                        | 2.62                        | 1                     | 55.6                               | 0.46                                 | 4.18                          | 3.000                         | −1.29       | −5.18 | 4.86        | ...         | ...         | −0.98 | −4.15 |
| 20294054+3900234 | 77.959      | −0.026      | 15.120     | 8            | —          | —          | —           | —          | —           | —             | —           | —   | —                      | —           | —           | —           | —           | —          | —           | 11.257                             | 1.35                        | 3.34                        | 1                     | 46.8                               | 0.56                                 | 4.18                          | 5.623                         | −1.16       | −4.17 | 4.68        | ...         | ...         | −0.86 | −3.18 |
| 20294585+3558464 | 75.518      | −1.817      | 2.708      | 8            | —          | —          | —           | —          | —           | —             | —           | —   | —                      | —           | —           | —           | —           | —          | —           | 11.243                             | 1.11                        | 2.77                        | 1                     | 24.8                               | 0.88                                 | 4.19                          | 10.234                        | 0.66        | 1.43  | 0.84        | ...         | ...         | 0.71  | 1.60  |
| 20294683+3531424 | 75.155      | −2.084      | 3.277      | 8            | —          | —          | —           | —          | —           | —             | —           | —   | —                      | —           | —           | —           | —           | —          | —           | 9.579                              | 0.91                        | 1.91                        | 1                     | 60.8                               | 0.66                                 | 4.14                          | 8.358                         | 0.37        | 0.28  | 1.02        | ...         | ...         | 0.44  | 0.49  |
| 20295076+3852534 | 77.877      | −0.126      | 6.248      | 9            | —          | —          | —           | —          | —           | —             | —           | —   | —                      | —           | —           | —           | —           | —          | —           | 12.769                             | 0.71                        | 1.98                        | −2                    | 16.0                               | 0.70                                 | 4.18                          | 10.441                        | −0.32       | −1.13 | 1.94        | ...         | ...         | −0.20 | −0.71 |
| 20295210+4208124 | 80.515      | 1.783       | 5.705      | 9            | —          | —          | —           | —          | —           | —             | —           | —   | —                      | —           | —           | —           | —           | —          | —           | 12.834                             | 1.11                        | ...                         | 1                     | 16.6                               | 0.38                                 | 4.15                          | 10.708                        | 0.17        | ...   | 1.77        | ...         | ...         | 0.28  | ...   |
| 20300351+4002064 | 78.835      | 0.519       | 5.576      | 8            | —          | —          | —           | —          | —           | —             | —           | —   | —                      | —           | —           | —           | —           | —          | —           | 12.929                             | 0.71                        | 1.76                        | −2                    | 14.4                               | 0.60                                 | 4.22                          | 10.851                        | −0.21       | −1.01 | 1.73        | ...         | ...         | −0.10 | −0.64 |
| 20300373+3849551 | 77.862      | −0.189      | 5.788      | 9            | —          | —          | —           | —          | —           | —             | —           | —   | —                      | —           | —           | —           | —           | —          | —           | 13.216                             | 0.50                        | 1.57                        | −1                    | 16.0                               | 0.80                                 | 4.14                          | 11.059                        | −0.46       | −1.30 | 1.79        | ...         | ...         | −0.34 | −0.92 |
| 20300478+4109181 | 79.743      | 1.174       | 7.537      | 9            | —          | —          | —           | —          | —           | —             | —           | —   | —                      | —           | —           | —           | —           | —          | —           | 12.789                             | ...                         | ...                         | 1                     | 15.0                               | 0.64                                 | 4.16                          | 9.981                         | ...         | ...   | 2.33        | ...         | ...         | ...   | ...   |
| 20302211+4020062 | 79.112      | 0.648       | 5.747      | 7            | —          | —          | —           | —          | —           | —             | —           | —   | —                      | —           | —           | —           | —           | —          | —           | 12.797                             | 0.94                        | ...                         | 1                     | 21.6                               | 0.80                                 | 4.11                          | 10.656                        | −0.01       | ...   | 1.78        | ...         | ...         | 0.11  | ...   |
| 20302719+4116012 | 79.875      | 1.183       | 9.789      | 8            | —          | —          | —           | —          | —           | —             | —           | —   | —                      | —           | —           | —           | —           | —          | —           | 9.941                              | 1.39                        | ...                         | 1                     | 70.2                               | 0.56                                 | 4.21                          | 6.294                         | −0.23       | ...   | 3.03        | ...         | ...         | −0.04 | ...   |
| 20303558+3853102 | 77.967      | −0.241      | 7.006      | 9            | —          | —          | —           | —          | —           | —             | —           | —   | —                      | —           | —           | —           | —           | —          | —           | 13.514                             | 0.66                        | ...                         | −1                    | 13.2                               | 0.38                                 | 4.14                          | 10.904                        | −0.50       | ...   | 2.17        | ...         | ...         | −0.36 | ...   |
| 20304165+4006171 | 78.963      | 0.462       | 6.124      | 8            | —          | —          | —           | —          | —           | —             | —           | —   | —                      | —           | —           | —           | —           | —          | —           | 13.312                             | ...                         | ...                         | −1                    | 20.0                               | 1.00                                 | 4.07                          | 11.030                        | ...         | ...   | 1.90        | ...         | ...         | ...   | ...   |
| 20304522+4021501 | 79.179      | 0.605       | 5.552      | 7            | —          | —          | —           | —          | —           | —             | —           | —   | —                      | —           | —           | —           | —           | —          | —           | 11.523                             | 1.84                        | ...                         | 1                     | 32.4                               | 0.46                                 | 4.07                          | 9.454                         | 0.92        | ...   | 1.72        | ...         | ...         | 1.03  | ...   |
| 20305093+4102302 | 79.737      | 0.990       | 6.715      | 8            | —          | —          | —           | —          | —           | —             | —           | —   | —                      | —           | —           | —           | —           | —          | —           | 12.439                             | ...                         | ...                         | 1                     | 17.6                               | 0.60                                 | 4.19                          | 9.937                         | ...         | ...   | 2.08        | ...         | ...         | ...   | ...   |
| 20305320+4109172 | 79.832      | 1.051       | 6.416      | 9            | —          | —          | —           | —          | —           | —             | —           | —   | —                      | —           | —           | —           | —           | —          | —           | 12.985                             | 0.88                        | ...                         | 1                     | 20.6                               | 0.44                                 | 4.19                          | 10.594                        | −0.19       | ...   | 1.99        | ...         | ...         | −0.06 | ...   |
| 20305540+3942062 | 78.663      | 0.189       | 4.946      | 9            | —          | —          | —           | —          | —           | —             | —           | —   | —                      | —           | —           | —           | —           | —          | —           | 11.458                             | ...                         | ...                         | 1                     | 41.4                               | 0.48                                 | 4.12                          | 9.615                         | ...         | ...   | 1.53        | ...         | ...         | ...   | ...   |
| 20310684+4017313 | 79.161      | 0.507       | 7.207      | 9            | —          | —          | —           | —          | —           | —             | —           | —   | —                      | —           | —           | —           | —           | —          | —           | 10.708                             | 1.34                        | 4.79                        | 1                     | 62.4                               | 0.48                                 | 4.07                          | 8.023                         | 0.15        | 1.21  | 2.23        | ...         | ...         | 0.29  | 1.69  |
| 20310849+4002463 | 78.966      | 0.358       | 6.542      | 9            | —          | —          | —           | —          | —           | —             | —           | —   | —                      | —           | —           | —           | —           | —          | —           | 11.587                             | 1.92                        | ...                         | 1                     | 28.0                               | 0.46                                 | 4.07                          | 9.149                         | 0.83        | ...   | 2.03        | ...         | ...         | 0.96  | ...   |
| 20311250+4003193 | 78.981      | 0.353       | 6.729      | 9            | —          | —          | —           | —          | —           | —             | —           | —   | —                      | —           | —           | —           | —           | —          | —           | 9.420                              | 1.54                        | 3.11                        | 1                     | 95.8                               | 0.62                                 | 4.07                          | 6.913                         | 0.43        | −0.23 | 2.08        | ...         | ...         | 0.56  | 0.21  |
| 20311323+4124232 | 80.073      | 1.149       | 3.030      | 9            | —          | —          | —           | —          | —           | —             | —           | —   | —                      | —           | —           | —           | —           | —          | —           | 11.977                             | 0.50                        | 1.52                        | −2                    | 17.6                               | 0.74                                 | 4.24                          | 10.848                        | −0.00       | 0.02  | 0.94        | ...         | ...         | 0.05  | 0.22  |
| 20311591+3845173 | 77.938      | −0.424      | 7.267      | 8            | —          | —          | —           | —          | —           | —             | —           | —   | —                      | —           | —           | —           | —           | —          | —           | 13.538                             | ...                         | ...                         | −1                    | 10.8                               | 1.00                                 | 4.11                          | 10.830                        | ...         | ...   | 2.25        | ...         | ...         | ...   | ...   |
| 20311851+2436031 | 66.429      | −8.728      | 0.327      | 1            | —          | —          | —           | —          | —           | —             | —           | —   | —                      | —           | —           | —           | —           | —          | —           | 11.237                             | 0.34                        | 1.09                        | 1                     | 29.2                               | 0.64                                 | 3.73                          | 11.115                        | 0.29        | 0.93  | 0.10        | 29.7        | 11.13       | 0.29  | 0.95  |
| 20313241+4359529 | 82.200      | 2.632       | 4.963      | 9            | —          |            |             |            |             |               |             |     |                        |             |             |             |             |            |             |                                    |                             |                             |                       |                                    |                                      |                               |                               |             |       |             |             |             |       |       |

Table B1: a) continued.

| 2MASX J          | <i>l</i> | <i>b</i> | EBV    | Object | Sample | Disc | 2MRS | Velocity | NIR  | Photom | Ext  | <i>K</i> <sub>20</sub> | <i>H-K</i> | <i>J-K</i> | vc   | <i>a</i> | <i>b/a</i> | st.d. | <i>K</i> <sub>s</sub> <sup>o</sup> | ( <i>H-K</i> ) <sup>o</sup> | ( <i>J-K</i> ) <sup>o</sup> | <i>A<sub>K</sub></i> | <i>a</i> <sub>d</sub> <sup>d</sup> | <i>K</i> <sub>s</sub> <sup>o,d</sup> | ( <i>H-K</i> ) <sup>o,c</sup> | ( <i>J-K</i> ) <sup>o,c</sup> |       |        |       |      |      |       |        |
|------------------|----------|----------|--------|--------|--------|------|------|----------|------|--------|------|------------------------|------------|------------|------|----------|------------|-------|------------------------------------|-----------------------------|-----------------------------|----------------------|------------------------------------|--------------------------------------|-------------------------------|-------------------------------|-------|--------|-------|------|------|-------|--------|
| (1)              | deg      | deg      | mag    | class  | off    | flag | gal  | TF       | obs  | ext'd  | type | (9)                    | Opt        | HI         | flag | flag     | flag       | flag  | mag                                | mag                         | mag                         | mag                  | mag                                | mag                                  | mag                           | mag                           |       |        |       |      |      |       |        |
| (1)              | (2a)     | (2b)     | (3)    | (4)    | (5)    | (6)  | (7a) | (7b)     | (7c) | (7d)   | (8)  | (9)                    | (10a)      | (10b)      | (11) | (12)     | (13)       | (14)  | (15)                               | (16)                        | (17)                        | (18)                 | (19)                               | (20)                                 | (21)                          | (22)                          | (23)  | (24)   | (25)  | (26) | (27) | (28)  |        |
| 20323106+4016502 | 79.310   | 0.285    | 39.970 | 9      | —      | —    | —    | —        | —    | —      | —    | —                      | —          | —          | —    | —        | —          | —     | 6.784                              | 1.46                        | 3.19                        | 1                    | 219.2                              | 0.86                                 | 4.21                          | −8.109                        | −5.16 | −16.66 | 12.38 | ...  | ...  | −4.37 | −14.03 |
| 20323158+4017412 | 79.323   | 0.292    | 40.415 | 9      | —      | —    | —    | —        | —    | —      | —    | —                      | —          | —          | —    | —        | —          | —     | 8.927                              | 3.04                        | 2.92                        | −2                   | 184.4                              | 0.44                                 | 4.21                          | −6.132                        | −3.65 | −17.16 | 12.52 | ...  | ...  | −2.86 | −14.49 |
| 20323290+4016042 | 79.303   | 0.273    | 37.935 | 9      | —      | —    | —    | —        | —    | —      | —    | —                      | —          | —          | —    | —        | —          | —     | 9.871                              | 1.73                        | 3.26                        | 1                    | 31.4                               | 0.70                                 | 4.21                          | −4.264                        | −4.55 | −15.58 | 11.75 | ...  | ...  | −3.81 | −13.08 |
| 20323596+4015212 | 79.300   | 0.258    | 32.845 | 9      | —      | —    | —    | —        | —    | —      | —    | —                      | —          | —          | —    | —        | —          | —     | 9.423                              | 1.32                        | ...                         | 1                    | 112.8                              | 1.00                                 | 4.21                          | −2.815                        | −4.12 | ...    | 10.17 | ...  | ...  | −3.48 | ...    |
| 20323683+4016152 | 79.313   | 0.264    | 35.870 | 9      | —      | —    | —    | —        | —    | —      | —    | —                      | —          | —          | —    | —        | —          | —     | 8.462                              | ...                         | ...                         | 1                    | 131.0                              | 1.00                                 | 4.21                          | −4.903                        | ...   | ...    | 11.11 | ...  | ...  | ...   | ...    |
| 20324124+3846103 | 78.114   | −0.638   | 9.406  | 9      | —      | —    | —    | —        | —    | —      | —    | —                      | —          | —          | —    | —        | —          | —     | 10.647                             | ...                         | ...                         | 1                    | 56.8                               | 0.54                                 | 4.08                          | 7.142                         | ...   | ...    | 2.91  | ...  | ...  | ...   | ...    |
| 20324149+3846153 | 78.115   | −0.638   | 9.431  | 9      | —      | —    | —    | —        | —    | —      | —    | —                      | —          | —          | —    | —        | —          | —     | 10.957                             | ...                         | ...                         | 1                    | 79.8                               | 1.00                                 | 4.08                          | 7.443                         | ...   | ...    | 2.92  | ...  | ...  | ...   | ...    |
| 20325004+4312064 | 81.697   | 1.972    | 5.888  | 9      | —      | —    | —    | —        | —    | —      | —    | —                      | —          | —          | —    | —        | —          | —     | 12.901                             | ...                         | ...                         | −2                   | 23.6                               | 0.10                                 | 4.11                          | 10.707                        | ...   | ...    | 1.82  | ...  | ...  | ...   | ...    |
| 20325247+3751313 | 77.403   | −1.209   | 3.676  | 9      | —      | —    | —    | —        | —    | —      | —    | —                      | —          | —          | —    | —        | —          | —     | 11.996                             | ...                         | ...                         | 1                    | 42.0                               | 0.34                                 | 4.20                          | 10.626                        | ...   | ...    | 1.14  | ...  | ...  | ...   | ...    |
| 20325336+3924203 | 78.649   | −0.292   | 8.945  | 9      | —      | —    | —    | —        | —    | —      | —    | —                      | —          | —          | —    | —        | —          | —     | 13.108                             | 0.85                        | 1.94                        | −1                   | 24.2                               | 0.52                                 | 4.03                          | 9.775                         | −0.63 | −2.50  | 2.77  | ...  | ...  | −0.46 | −1.91  |
| 20325594+5430316 | 90.889   | 8.618    | 0.369  | 1      | —      | —    | g    | —        | N    | —      | D2   | c                      | —          | h          | —    | —        | —          | —     | 9.592                              | 0.28                        | 1.03                        | 1                    | 61.6                               | 0.52                                 | 3.73                          | 9.455                         | 0.22  | 0.85   | 0.11  | 62.7 | 9.47 | 0.23  | 0.88   |
| 20325868+3844443 | 78.128   | −0.698   | 7.009  | 9      | —      | —    | —    | —        | —    | —      | —    | —                      | —          | —          | —    | —        | —          | —     | 12.751                             | 0.77                        | 2.58                        | 1                    | 10.4                               | 1.00                                 | 4.08                          | 10.139                        | −0.39 | −0.90  | 2.17  | ...  | ...  | −0.26 | −0.44  |
| 20331636+4311256 | 81.735   | 1.901    | 6.594  | 9      | —      | —    | —    | —        | —    | —      | —    | —                      | —          | —          | —    | —        | —          | —     | 13.126                             | 0.81                        | 1.76                        | −1                   | 11.0                               | 1.00                                 | 4.04                          | 10.669                        | −0.28 | −1.52  | 2.04  | ...  | ...  | −0.15 | −1.08  |
| 20332123+3834486 | 78.039   | −0.856   | 5.634  | 7      | o      | —    | —    | —        | —    | —      | —    | —                      | —          | —          | —    | o        | —          | —     | 12.121                             | 1.42                        | 3.34                        | 1                    | 18.8                               | 0.36                                 | 4.01                          | 10.022                        | 0.49  | 0.55   | 1.75  | ...  | ...  | 0.60  | 0.92   |
| 20332126+4013156 | 79.357   | 0.121    | 5.725  | 9      | —      | —    | —    | —        | —    | —      | —    | —                      | —          | —          | —    | —        | —          | —     | 13.217                             | ...                         | ...                         | −1                   | 16.8                               | 1.00                                 | 4.17                          | 11.084                        | ...   | ...    | 1.77  | ...  | ...  | ...   | ...    |
| 20332200+3834596 | 78.043   | −0.856   | 5.647  | 9      | —      | —    | —    | —        | —    | —      | —    | —                      | —          | —          | —    | —        | —          | —     | 12.594                             | 1.24                        | 2.75                        | 1                    | 14.6                               | 0.64                                 | 4.01                          | 10.490                        | 0.31  | −0.06  | 1.75  | ...  | ...  | 0.42  | 0.32   |
| 20332683+3945196 | 78.994   | −0.170   | 8.334  | 9      | —      | —    | —    | —        | —    | —      | —    | —                      | —          | —          | —    | —        | —          | —     | 12.856                             | 1.44                        | ...                         | 1                    | 11.0                               | 1.00                                 | 3.98                          | 9.751                         | 0.06  | ...    | 2.58  | ...  | ...  | 0.22  | ...    |
| 20332857+3949105 | 79.049   | −0.137   | 7.337  | 9      | —      | —    | —    | —        | —    | —      | —    | —                      | —          | —          | —    | —        | —          | —     | 13.002                             | 0.66                        | 1.94                        | −2                   | 15.4                               | 0.54                                 | 3.98                          | 10.268                        | −0.55 | −1.70  | 2.27  | ...  | ...  | −0.41 | −1.22  |
| 20332890+3941185 | 78.944   | −0.216   | 8.242  | 9      | —      | —    | —    | —        | —    | —      | —    | —                      | —          | —          | —    | —        | —          | —     | 13.697                             | ...                         | ...                         | −1                   | 16.2                               | 0.32                                 | 3.98                          | 10.626                        | ...   | ...    | 2.55  | ...  | ...  | ...   | ...    |
| 20333346+3848115 | 78.242   | −0.755   | 6.364  | 8      | —      | —    | —    | —        | —    | —      | —    | —                      | —          | —          | —    | —        | —          | —     | 13.434                             | 0.77                        | ...                         | −1                   | 10.4                               | 1.00                                 | 4.01                          | 11.063                        | −0.28 | ...    | 1.97  | ...  | ...  | −0.15 | ...    |
| 20333414+3848575 | 78.253   | −0.749   | 6.465  | 6      | —      | —    | —    | —        | N    | —      | —    | —                      | —          | —          | —    | —        | —          | —     | 13.156                             | 1.20                        | ...                         | −1                   | 14.0                               | 1.00                                 | 4.01                          | 10.747                        | 0.13  | ...    | 2.00  | ...  | ...  | 0.26  | ...    |
| 20333468+4404536 | 82.485   | 2.386    | 7.030  | 8      | —      | —    | —    | —        | —    | —      | —    | —                      | —          | —          | —    | —        | —          | —     | 12.366                             | ...                         | ...                         | −2                   | 27.4                               | 0.76                                 | 4.13                          | 9.747                         | ...   | ...    | 2.18  | ...  | ...  | ...   | ...    |
| 20333535+4535376 | 83.703   | 3.284    | 10.966 | 9      | —      | —    | —    | —        | —    | —      | —    | —                      | —          | —          | —    | —        | —          | —     | 8.681                              | 1.21                        | ...                         | 1                    | 167.4                              | 0.34                                 | 4.17                          | 4.595                         | −0.61 | ...    | 3.40  | ...  | ...  | −0.39 | ...    |
| 20333798+3936205 | 78.895   | −0.288   | 8.762  | 9      | —      | —    | —    | —        | —    | —      | —    | —                      | —          | —          | —    | —        | —          | —     | 13.716                             | 0.43                        | 1.45                        | −1                   | 11.4                               | 0.54                                 | 3.96                          | 10.451                        | −1.02 | −2.90  | 2.71  | ...  | ...  | −0.85 | −2.32  |
| 20333926+4537140 | 83.732   | 3.290    | 14.353 | 8      | —      | —    | —    | —        | —    | —      | —    | —                      | —          | —          | —    | —        | —          | —     | 10.743                             | 1.02                        | 2.11                        | 1                    | 63.8                               | 0.92                                 | 4.12                          | 5.395                         | −1.35 | −5.02  | 4.45  | ...  | ...  | −1.07 | −4.07  |
| 20334102+3856365 | 78.369   | −0.691   | 6.926  | 9      | —      | —    | —    | —        | —    | —      | —    | —                      | —          | —          | —    | —        | —          | —     | 13.648                             | 0.76                        | ...                         | −1                   | 10.6                               | 1.00                                 | 4.01                          | 11.067                        | −0.38 | ...    | 2.15  | ...  | ...  | −0.25 | ...    |
| 20334308+4536241 | 83.727   | 3.273    | 12.126 | 9      | —      | —    | —    | —        | —    | —      | —    | —                      | —          | —          | —    | —        | —          | —     | 10.745                             | 0.88                        | 1.64                        | 1                    | 87.0                               | 0.42                                 | 4.12                          | 6.227                         | −1.13 | −4.38  | 3.76  | ...  | ...  | −0.89 | −3.58  |
| 20334726+4511401 | 83.403   | 3.018    | 1.976  | 1      | —      | —    | g    | —        | t    | N      | —    | D1                     | —          | —          | —    | —        | —          | —     | 10.598                             | 0.45                        | 1.48                        | 1                    | 58.0                               | 0.50                                 | 4.17                          | 9.862                         | 0.12  | 0.50   | 0.61  | 71.5 | 9.84 | 0.16  | 0.63   |
| 20334811+4540531 | 83.796   | 3.306    | 14.877 | 8      | —      | —    | —    | —        | —    | —      | —    | —                      | —          | —          | —    | —        | —          | —     | 10.660                             | 1.16                        | 3.05                        | 1                    | 36.0                               | 0.46                                 | 4.15                          | 5.117                         | −1.31 | −4.34  | 4.61  | ...  | ...  | −1.02 | −3.36  |
| 20334889+4008353 | 79.347   | 0.004    | 7.229  | 8      | —      | —    | —    | —        | —    | —      | —    | —                      | —          | —          | —    | —        | —          | —     | 7.629                              | 0.99                        | 2.17                        | 1                    | 167.4                              | 0.56                                 | 4.17                          | 4.935                         | −0.21 | −1.42  | 2.24  | ...  | ...  | −0.07 | −0.94  |
| 20335124+4009183 | 79.361   | 0.005    | 6.917  | 9      | —      | —    | —    | —        | —    | —      | —    | —                      | —          | —          | —    | —        | —          | —     | 10.474                             | 0.88                        | 2.30                        | 1                    | 66.6                               | 0.66                                 | 4.17                          | 7.897                         | −0.26 | −1.14  | 2.14  | ...  | ...  | −0.13 | −0.68  |
| 20335345+4337071 | 82.146   | 2.065    | 3.899  | 8      | —      | —    | —    | —        | —    | —      | —    | —                      | —          | —          | —    | —        | —          | —     | 12.260                             | ...                         | ...                         | 1                    | 21.8                               | 0.46                                 | 4.13                          | 10.807                        | ...   | ...    | 1.21  | ...  | ...  | ...   | ...    |
| 20335597+3956533 | 79.204   | −0.130   | 6.511  | 9      | —      | —    | —    | —        | —    | —      | —    | —                      | —          | —          | —    | —        | —          | —     | 13.500                             | ...                         | ...                         | −1                   | 11.8                               | 1.00                                 | 4.05                          | 11.074                        | ...   | ...    | 2.02  | ...  | ...  | ...   | ...    |
| 20340183+4654511 | 84.813   | 4.007    | 5.905  | 8      | —      | —    | —    | —        | —    | —      | —    | —                      | —          | —          | —    | —        | —          | —     | 13.055                             | 0.70                        | ...                         | 2                    | 15.2                               | 0.68                                 | 4.00                          | 10.855                        | −0.28 | ...    | 1.83  | ...  | ...  | −0.16 | ...    |
| 20340806+4649371 | 84.753   | 3.941    | 6.347  | 8      | —      | —    | —    | —        | —    | —      | —    | —                      | —          | —          | —    | —        | —          | —     | 13.475                             | 0.28                        | 0.98                        | 2                    | 11.8                               | 0.74                                 | 4.00                          | 11.110                        | −0.77 | −2.18  | 1.97  | ...  | ...  | −0.64 | −1.76  |
| 20341174+3919443 | 78.738   | −0.541   | 7.604  | 9      | —      | —    | —    | —        | —    | —      | —    | —                      | —          | —          | —    | —        | —          | —     | 13.688                             | 0.36                        | 1.39                        | −1                   | 10.0                               | 1.00                                 | 3.98                          | 10.855                        | −0.90 | −2.38  | 2.36  | ...  | ...  | −0.75 | −1.88  |
| 20341242+4658296 | 84.880   | 4.019    | 5.608  | 1      | —      | —    | g    | —        | t    | N      | —    | D1                     | —          | —          | —    | —        | —          | —     | 11.294                             | 0.77                        | 2.45                        | 1                    | 41.0                               | 0.56                                 | 4.08                          | 9.204                         | −0.16 | −0.34  | 1.74  | 90.1 | 8.98 | −0.05 | 0.03   |
| 20341660+4001043 | 79.299   | −0.142   | 5.706  | 9      | —      | —    | —    | —        | —    | —      | —    | —                      | —          | —          | —    | —        | —          | —     | 12.414                             | 1.30                        | ...                         | 1                    | 15.2                               | 0.46                                 | 4.05                          | 10.288                        | 0.35  | ...    | 1.77  | ...  | ...  | 0.46  | ...    |
| 20341800+3902302 | 78.519   | −0.728   | 6.197  | 9      | —      | —    | —    | —        | —    | —      | —    | —                      | —          | —          | —    | —        | —          | —     | 13.127                             | ...                         | ...                         | −1                   | 14.6                               | 1.00                                 | 4.06                          | 10.818                        | ...   | ...    | 1.92  | ...  | ...  | ...   | ...    |
| 20342791+3843573 | 78.291   | −0.939   | 7.753  | 9      | —      | —    | —    | —        | —    | —      | —    | —                      | —          | —          | —    | —        | —          | —     | 13.483                             | 0.73                        | ...                         | −1                   | 10.0                               | 1.00                                 | 3.99                          | 10.594                        | −0.55 | ...    | 2.40  | ...  | ...  | −0.40 | ...    |
| 20342807+3849103 | 78.361   | −0.887   | 7.699  | 9      | —      | —    | —    | —        | —    | —      | —    | —                      | —          | —          | —    | —        | —          | —     | 13.394                             | ...                         | ...                         | −1                   | 10.2                               | 1.00                                 | 3.99                          | 10.525                        | ...   | ...    | 2.38  | ...  | ...  | ...   | ...    |
| 20342918+4130593 | 80.525   | 0.722    | 5.675  | 9      | —      | —    | —    | —        | —    | —      | —    | —                      | —          | —          | —    | —        | —          | —     | 11.379                             | 1.38                        | 2.86                        | 1                    | 38.0                               | 0.76                                 | 4.19                          | 9.264                         | 0.44  | 0.04   | 1.76  | ...  | ...  | 0.55  | 0.42   |
| 20343007+4130213 | 80.518   | 0.714    | 5.742  | 9      | —      | —    | —    | —        | —    | —      | —    | —                      | —          | —          | —    | —        | —          | —     | 10.078                             | 1.43                        | ...                         | 1                    | 72.2                               | 1.00                                 | 4.25                          | 7.939                         | 0.48  | ...    | 1.78  | ...  | ...  | 0.59  | ...    |
| 20343158+4704397 | 84.995   | 4.036    | 5.419  | 8      | —      |      |      |          |      |        |      |                        |            |            |      |          |            |       |                                    |                             |                             |                      |                                    |                                      |                               |                               |       |        |       |      |      |       |        |



|   |   |   |        |
|---|---|---|--------|
| U | — | — | 12.967 |
| U | — | — | 11.970 |
| — | — | — | 13.210 |

2M-ZoA galaxy catalogue description and analysis 109

Table B1: a) continued.

| 2MASX J          | $l$    | $b$    | EBV    | Object | Sample | Disc | 2MRS | Velocity | NIR  | Photom | Ext  | $K_{20}$ | $H-K$ | $J-K$ | vc    | $a$  | $b/a$ | st.d. | $K_s^o$ | $(H-K)^o$ | $(J-K)^o$ | $A_K$ | $a_d^o$ | $K_s^{o,d}$ | $(H-K)^{o,c}$ | $(J-K)^{o,c}$ |       |       |      |      |       |       |       |
|------------------|--------|--------|--------|--------|--------|------|------|----------|------|--------|------|----------|-------|-------|-------|------|-------|-------|---------|-----------|-----------|-------|---------|-------------|---------------|---------------|-------|-------|------|------|-------|-------|-------|
| (1)              | deg    | deg    | mag    | class  | off    | flag | gal  | TF       | obs  | ext'd  | type | (9)      | Opt   | HI    | (10b) | (11) | flag  | flag  | mag     | mag       | mag       | mag   | mag     | mag         | mag           | mag           |       |       |      |      |       |       |       |
| (1)              | (2a)   | (2b)   | (3)    | (4)    | (5)    | (6)  | (7a) | (7b)     | (7c) | (7d)   | (8)  | (9)      | (10a) | (10b) | (11)  | (12) | (13)  | (14)  | (15)    | (16)      | (17)      | (18)  | (19)    | (20)        | (21)          | (22)          | (23)  | (24)  | (25) | (26) | (27)  | (28)  |       |
| 20410777+4102153 | 80.899 | -0.561 | 3.390  | 9      | -      | -    | -    | -        | -    | -      | -    | -        | -     | -     | -     | -    | -     | -     | 12.316  | 0.78      | 2.12      | 1     | 20.6    | 0.56        | 4.03          | 11.053        | 0.22  | 0.44  | 1.05 | ...  | ...   | 0.29  | 0.66  |
| 20411108+4151233 | 81.552 | -0.067 | 14.652 | 9      | -      | -    | -    | -        | -    | -      | -    | -        | -     | -     | -     | -    | -     | -     | 13.136  | ...       | ...       | -1    | 21.2    | 0.34        | 4.11          | 7.677         | ...   | ...   | 4.54 | ...  | ...   | ...   |       |
| 20411215+4151483 | 81.560 | -0.065 | 14.539 | 8      | -      | -    | -    | -        | -    | -      | -    | -        | -     | -     | -     | -    | -     | -     | 13.092  | 0.89      | ...       | 1     | 11.0    | 1.00        | 4.11          | 7.675         | -1.51 | ...   | ...  | 4.50 | ...   | ...   | -1.23 |
| 20411305+3442467 | 75.903 | -4.446 | 0.742  | 1      | -      | -    | -    | -        | -    | -      | -    | -        | -     | -     | -     | -    | -     | -     | 11.175  | 0.40      | 1.37      | 1     | 43.0    | 0.48        | 4.38          | 10.899        | 0.28  | 1.00  | 0.23 | 45.7 | 10.90 | 0.29  | 1.05  |
| 20411689+4152173 | 81.575 | -0.072 | 14.660 | 8      | -      | -    | -    | -        | -    | -      | -    | -        | -     | -     | -     | -    | -     | -     | 12.339  | 1.28      | ...       | 1     | 17.8    | 0.78        | 4.11          | 6.877         | -1.15 | ...   | ...  | 4.54 | ...   | ...   | -0.86 |
| 20412222+5054235 | 88.740 | 5.446  | 1.386  | 1      | -      | -    | -    | -        | -    | -      | -    | -        | -     | -     | -     | -    | -     | -     | 10.500  | 0.53      | 1.53      | 1     | 42.0    | 0.90        | 3.91          | 9.984         | 0.30  | 0.85  | 0.43 | 47.2 | 10.00 | 0.33  | 0.94  |
| 20412600+2626054 | 69.292 | -9.496 | 0.286  | 1      | -      | -    | -    | -        | -    | -      | -    | -        | -     | -     | -     | -    | -     | -     | 11.033  | 0.47      | 1.43      | 1     | 52.2    | 0.26        | 3.67          | 10.926        | 0.43  | 1.29  | 0.09 | 53.0 | 10.94 | 0.43  | 1.31  |
| 20413936+4450026 | 83.956 | 1.693  | 3.321  | 1      | o      | -    | -    | -        | -    | -      | -    | -        | -     | -     | -     | -    | -     | -     | 12.146  | 0.87      | ...       | 1     | 32.6    | 0.44        | 4.19          | 10.909        | 0.32  | ...   | 1.03 | 52.9 | 10.68 | 0.39  | ...   |
| 20414210+5541532 | 92.608 | 8.313  | 0.659  | 1      | -      | -    | -    | -        | -    | -      | -    | -        | -     | -     | -     | -    | -     | -     | 10.416  | 0.35      | 1.19      | 1     | 63.8    | 0.44        | 3.69          | 10.170        | 0.25  | 0.86  | 0.20 | 67.3 | 10.17 | 0.26  | 0.90  |
| 20414647+4228256 | 82.107 | 0.226  | 6.156  | 9      | -      | -    | -    | -        | -    | -      | -    | -        | -     | -     | -     | -    | -     | -     | 13.432  | ...       | ...       | -1    | 11.6    | 1.00        | 4.12          | 11.138        | ...   | ...   | 1.91 | ...  | ...   | ...   |       |
| 20415341+4515456 | 84.320 | 1.923  | 4.077  | 9      | -      | -    | -    | -        | -    | -      | -    | -        | -     | -     | -     | -    | -     | -     | 12.575  | 0.55      | ...       | -2    | 17.2    | 0.74        | 4.22          | 11.056        | -0.13 | ...   | ...  | 1.26 | ...   | ...   | -0.05 |
| 20415353+4531596 | 84.534 | 2.089  | 3.724  | 8      | -      | -    | -    | -        | -    | -      | -    | -        | -     | -     | -     | -    | -     | -     | 11.159  | 0.97      | 1.97      | 1     | 32.4    | 0.78        | 4.24          | 9.771         | 0.36  | 0.12  | 1.15 | ...  | ...   | 0.43  | 0.36  |
| 20415515+4532386 | 84.546 | 2.092  | 3.666  | 8      | -      | -    | -    | -        | -    | -      | -    | -        | -     | -     | -     | -    | -     | -     | 11.357  | 1.17      | ...       | 1     | 26.2    | 0.68        | 4.24          | 9.991         | 0.56  | ...   | 1.14 | ...  | ...   | 0.63  | ...   |
| 20420536+4225174 | 82.101 | 0.148  | 6.761  | 9      | -      | -    | -    | -        | -    | -      | -    | -        | -     | -     | -     | -    | -     | -     | 13.590  | ...       | ...       | -1    | 10.8    | 1.00        | 4.05          | 11.071        | ...   | ...   | 2.09 | ...  | ...   | ...   | ...   |
| 20420550+4636124 | 85.401 | 2.719  | 3.035  | 1      | -      | -    | -    | -        | -    | -      | -    | -        | -     | -     | -     | -    | -     | -     | 10.826  | 0.88      | 2.74      | 1     | 35.4    | 0.86        | 4.12          | 9.695         | 0.37  | 1.23  | 0.94 | 49.6 | 9.67  | 0.43  | 1.43  |
| 20421491+4237225 | 82.278 | 0.249  | 5.409  | 9      | -      | -    | -    | -        | -    | -      | -    | -        | -     | -     | -     | -    | -     | -     | 12.839  | ...       | ...       | 1     | 21.8    | 0.38        | 4.13          | 10.824        | ...   | ...   | 1.68 | ...  | ...   | ...   | ...   |
| 20422120+4605455 | 85.028 | 2.372  | 5.334  | 8      | -      | -    | -    | -        | -    | -      | -    | -        | -     | -     | -     | -    | -     | -     | 9.285   | 1.07      | 2.45      | 1     | 90.0    | 0.78        | 4.22          | 7.298         | 0.19  | -0.20 | 1.65 | ...  | ...   | 0.29  | 0.15  |
| 20423202+4256315 | 82.562 | 0.404  | 15.590 | 9      | -      | -    | -    | -        | -    | -      | -    | -        | -     | -     | -     | -    | -     | -     | 10.071  | 0.91      | 1.83      | -2    | 77.4    | 0.88        | 4.27          | 4.262         | -1.67 | -5.92 | 4.83 | ...  | ...   | -1.36 | -4.89 |
| 20423268+4852093 | 87.239 | 4.050  | 2.908  | 8      | -      | -    | -    | -        | -    | -      | -    | -        | -     | -     | -     | -    | -     | -     | 11.587  | 1.67      | ...       | 1     | 29.6    | 0.62        | 3.99          | 10.503        | 1.19  | ...   | 0.90 | ...  | ...   | 1.24  | ...   |
| 20423725+4226094 | 82.173 | 0.079  | 6.310  | 7      | -      | -    | -    | -        | -    | -      | -    | -        | -     | -     | -     | -    | -     | -     | 9.775   | 1.16      | 2.83      | 1     | 33.2    | 0.82        | 4.05          | 7.424         | 0.11  | -0.31 | 1.95 | ...  | ...   | 0.24  | 0.11  |
| 20423755+4853413 | 87.267 | 4.056  | 2.894  | 9      | -      | -    | -    | -        | -    | -      | -    | -        | -     | -     | -     | -    | -     | -     | 11.607  | 1.61      | ...       | 1     | 43.0    | 0.48        | 4.02          | 10.529        | 1.13  | ...   | 0.90 | ...  | ...   | 1.19  | ...   |
| 20425453+5453261 | 92.065 | 7.687  | 0.535  | 1      | -      | -    | -    | -        | -    | -      | -    | -        | -     | -     | -     | -    | -     | -     | 10.619  | 0.30      | 1.13      | 1     | 54.4    | 0.46        | 3.73          | 10.420        | 0.21  | 0.86  | 0.17 | 56.2 | 10.44 | 0.22  | 0.90  |
| 20432804+4249579 | 82.581 | 0.202  | 4.888  | 8      | -      | -    | -    | -        | -    | -      | -    | -        | -     | -     | -     | -    | -     | -     | 10.938  | 1.73      | 3.75      | 1     | 26.6    | 0.74        | 4.11          | 9.117         | 0.92  | 1.32  | 1.51 | ...  | ...   | 1.01  | 1.64  |
| 20433669+4451540 | 84.194 | 1.439  | 6.475  | 8      | -      | -    | -    | -        | -    | -      | -    | -        | -     | -     | -     | -    | -     | -     | 8.997   | 1.24      | 2.74      | 1     | 153.6   | 0.36        | 4.26          | 6.584         | 0.17  | -0.48 | 2.01 | ...  | ...   | 0.30  | -0.05 |
| 20433966+5736291 | 94.313 | 9.253  | 0.681  | 1      | -      | -    | -    | -        | -    | -      | -    | -        | -     | -     | -     | -    | -     | -     | 11.373  | 0.40      | 1.27      | 1     | 30.0    | 0.62        | 3.54          | 11.119        | 0.29  | 0.93  | 0.21 | 31.5 | 11.13 | 0.31  | 0.97  |
| 20435702+5032583 | 88.708 | 4.905  | 1.407  | 1      | -      | -    | -    | -        | -    | -      | -    | -        | -     | -     | -     | -    | -     | -     | 10.570  | 0.44      | 1.43      | 1     | 63.6    | 0.48        | 3.91          | 10.046        | 0.20  | 0.73  | 0.44 | 74.2 | 10.00 | 0.23  | 0.83  |
| 20440027+4143156 | 81.770 | -0.564 | 2.018  | 1      | -      | -    | -    | -        | -    | -      | -    | -        | -     | -     | -     | -    | -     | -     | 10.662  | 0.94      | 2.89      | 1     | 53.0    | 0.56        | 4.05          | 9.910         | 0.61  | 1.89  | 0.63 | 65.3 | 9.90  | 0.65  | 2.02  |
| 20440241+5043362 | 88.857 | 5.002  | 1.425  | 1      | -      | -    | -    | -        | -    | -      | -    | -        | -     | -     | -     | -    | -     | -     | 10.641  | 0.45      | 1.56      | 1     | 65.4    | 0.34        | 3.91          | 10.110        | 0.21  | 0.85  | 0.44 | 75.9 | 10.09 | 0.24  | 0.94  |
| 20441259+4940566 | 88.049 | 4.337  | 1.759  | 1      | -      | -    | -    | -        | -    | -      | -    | -        | -     | -     | -     | -    | -     | -     | 11.826  | 0.48      | 1.77      | 1     | 24.2    | 0.52        | 4.02          | 11.171        | 0.19  | 0.89  | 0.54 | 29.5 | 11.12 | 0.23  | 1.01  |
| 20441866+3627187 | 77.668 | -3.872 | 0.944  | 1      | -      | -    | -    | -        | -    | -      | -    | -        | -     | -     | -     | -    | -     | -     | 11.427  | 0.39      | 1.29      | 1     | 26.2    | 0.98        | 3.95          | 11.075        | 0.23  | 0.82  | 0.29 | 28.4 | 11.08 | 0.25  | 0.89  |
| 20443279+4526350 | 84.751 | 1.667  | 4.387  | 8      | -      | -    | -    | -        | -    | -      | -    | -        | -     | -     | -     | -    | -     | -     | 10.851  | 1.22      | ...       | 1     | 43.6    | 0.72        | 4.24          | 9.216         | 0.49  | ...   | 1.36 | ...  | ...   | 0.58  | ...   |
| 20450499+4319010 | 93.144 | 0.271  | 3.866  | 8      | -      | -    | -    | -        | -    | -      | -    | -        | -     | -     | -     | -    | -     | -     | 11.661  | 0.93      | 2.23      | 1     | 33.8    | 0.46        | 4.22          | 10.221        | 0.29  | 0.31  | 1.20 | ...  | ...   | 0.37  | 0.57  |
| 20450632+5842171 | 85.314 | 9.767  | 0.655  | 1      | -      | -    | -    | -        | -    | -      | -    | -        | -     | -     | -     | -    | -     | -     | 10.981  | 0.39      | 1.27      | 1     | 40.6    | 0.70        | 3.62          | 10.737        | 0.29  | 0.94  | 0.20 | 42.7 | 10.74 | 0.30  | 0.98  |
| 20451603+3628482 | 77.807 | -4.007 | 0.701  | 1      | -      | -    | -    | -        | -    | -      | -    | -        | -     | -     | -     | -    | -     | -     | 10.493  | 0.33      | 1.25      | 1     | 38.4    | 0.84        | 3.98          | 10.232        | 0.21  | 0.90  | 0.22 | 40.3 | 10.25 | 0.23  | 0.95  |
| 20452664+3626122 | 77.795 | -4.062 | 0.640  | 1      | -      | -    | -    | -        | -    | -      | -    | -        | -     | -     | -     | -    | -     | -     | 10.643  | 0.34      | 1.17      | 1     | 47.2    | 0.66        | 3.98          | 10.405        | 0.23  | 0.85  | 0.20 | 49.3 | 10.42 | 0.24  | 0.89  |
| 20453536+4441192 | 84.274 | 1.054  | 4.308  | 9      | -      | -    | -    | -        | -    | -      | -    | -        | -     | -     | -     | -    | -     | -     | 12.255  | 0.76      | 1.77      | 1     | 19.8    | 0.90        | 4.23          | 10.650        | 0.04  | -0.37 | 1.33 | ...  | ...   | 0.13  | -0.09 |
| 20453614+4415042 | 83.934 | 0.780  | 16.684 | 8      | -      | -    | -    | -        | -    | -      | -    | -        | -     | -     | -     | -    | -     | -     | 7.163   | ...       | ...       | 1     | 162.0   | 1.00        | 4.20          | 0.947         | ...   | ...   | 5.17 | ...  | ...   | ...   | ...   |
| 20453697+5733282 | 94.434 | 9.015  | 0.671  | 1      | -      | -    | -    | -        | -    | -      | -    | -        | -     | -     | -     | -    | -     | -     | 11.452  | 0.46      | 1.26      | 1     | 31.4    | 0.90        | 3.66          | 11.202        | 0.35  | 0.92  | 0.21 | 33.0 | 11.21 | 0.36  | 0.97  |
| 20453717+4046002 | 81.211 | -1.395 | 2.119  | 1      | o      | -    | -    | -        | -    | -      | -    | -        | -     | -     | -     | -    | -     | -     | 11.955  | 0.60      | 1.77      | 1     | 18.2    | 0.64        | 4.15          | 11.165        | 0.25  | 0.71  | 0.66 | 23.1 | 11.12 | 0.29  | 0.85  |
| 20454042+4414242 | 83.933 | 0.763  | 14.834 | 9      | -      | -    | -    | -        | -    | -      | -    | -        | -     | -     | -     | -    | -     | -     | 9.506   | 1.16      | 2.55      | 1     | 121.4   | 0.26        | 4.20          | 3.979         | -1.30 | -4.82 | 4.59 | ...  | ...   | -1.01 | -3.84 |
| 20454080+4415572 | 83.954 | 0.778  | 16.684 | 9      | -      | -    | -    | -        | -    | -      | -    | -        | -     | -     | -     | -    | -     | -     | 9.901   | 1.22      | 2.63      | 1     | 127.4   | 0.62        | 4.20          | 3.685         | -1.55 | -5.66 | 5.17 | ...  | ...   | -1.22 | -4.56 |
| 20454256+4415082 | 83.946 | 0.765  | 16.271 | 9      | -      | -    | -    | -        | -    | -      | -    | -        | -     | -     | -     | -    | -     | -     | 9.044   | 1.47      | 2.40      | 1     | 154.2   | 0.26        | 4.20          | 2.981         | -1.23 | -5.68 | 5.04 | ...  | ...   | -0.91 | -4.61 |
| 20455694+2831560 | 71.597 | -9.022 | 0.270  | 1      | -      | -    | -    | -        | -    | -      | -    | -        | -     | -     | -     | -    | -     | -     | 11.158  | 0.43      | 1.17      | 1     | 51.2    | 0.58        | 3.72          | 11.057        | 0.38  | 1.04  | 0.08 | 52.0 | 11.06 | 0.39  | 1.06  |
| 20460831+4640399 | 85.890 | 2.220  | 4.162  | 8      | -      | -    | -    | -        | -    | -      | -    | -        | -     | -     | -     | -    | -     | -     | 9.404   | 0.92      | 2.01      | 1     | 71.0    | 0.70        | 4.20          | 7.853         | 0.23  | -0.06 | 1.29 | ...  | ...   | 0.31  | 0.22  |
| 20461490+4447129 | 84.424 | 1.024  | 4.836  | 8      | -      | -    | -    | -        | -    | -      | -    | -        | -     | -     | -     | -    | -     | -     | 10.638  | 1.19      | ...       | 1     | 48.4    | 0.34        | 4.21          | 8.836         | 0.39  | ...   | 1.50 | ...  | ...   | 0.48  | ...</ |

Table B1: a) continued.

| 2MASX J          |        | <i>l</i>    | <i>b</i>    | EBV        | Object       |            |             | Sample      |            |             | Disc 2MRS     |             | Velocity |              | NIR         | Photom       | Ext          | <i>K</i> <sub>20</sub> | <i>H-K</i>  | <i>J-K</i>  | <i>vc</i>   | <i>a</i> | <i>b/a</i> | std.d. | <i>K</i> <sub>S</sub> <sup>o</sup> | ( <i>H-K</i> ) <sup>o</sup> | ( <i>J-K</i> ) <sup>o</sup> | <i>A<sub>K</sub></i> | <i>a</i> <sup>d</sup> | <i>K</i> <sub>S</sub> <sup>d,d</sup> | ( <i>H-K</i> ) <sup>o,c</sup> | ( <i>J-K</i> ) <sup>o,c</sup> |             |       |
|------------------|--------|-------------|-------------|------------|--------------|------------|-------------|-------------|------------|-------------|---------------|-------------|----------|--------------|-------------|--------------|--------------|------------------------|-------------|-------------|-------------|----------|------------|--------|------------------------------------|-----------------------------|-----------------------------|----------------------|-----------------------|--------------------------------------|-------------------------------|-------------------------------|-------------|-------|
| (1)              |        | deg<br>(2a) | deg<br>(2b) | mag<br>(3) | class<br>(4) | off<br>(5) | flag<br>(6) | gal<br>(7a) | TF<br>(7b) | obs<br>(7c) | ext'd<br>(7d) | type<br>(8) | (9)      | Opt<br>(10a) | HI<br>(10b) | flag<br>(11) | flag<br>(12) | flag<br>(13)           | mag<br>(14) | mag<br>(15) | mag<br>(16) | (17)     | "<br>(18)  | (19)   | (20)                               | mag<br>(21)                 | mag<br>(22)                 | mag<br>(23)          | mag<br>(24)           | "<br>(25)                            | mag<br>(26)                   | mag<br>(27)                   | mag<br>(28) |       |
| 20514516+4349023 | 84.294 | -0.352      | 4.811       | 7          | -            | -          | -           | -           | -          | -           | -             | -           | -        | -            | -           | -            | U            | -                      | -           | 10.081      | 1.13        | 2.68     | 1          | 26.2   | 0.82                               | 4.19                        | 8.288                       | 0.33                 | 0.29                  | 1.49                                 | ...                           | 0.42                          | 0.61        |       |
| 20514892+5132328 | 90.261 | 4.561       | 2.010       | 1          | -            | -          | -           | g           | -          | N           | -             | D3          | -        | -            | -           | -            | U            | -                      | -           | 11.938      | 0.51        | 1.69     | 1          | 26.6   | 0.82                               | 3.94                        | 11.189                      | 0.18                 | 0.69                  | 0.62                                 | 33.4                          | 11.14                         | 0.22        | 0.82  |
| 20520738+4951290 | 88.990 | 3.452       | 2.990       | 8          | -            | -          | -           | -           | -          | -           | -             | -           | -        | -            | -           | -            | U            | -                      | -           | 12.058      | 1.29        | ...      | 1          | 18.2   | 0.84                               | 4.03                        | 10.944                      | 0.80                 | ...                   | 0.93                                 | ...                           | 0.86                          | ...         |       |
| 20520777+5224130 | 90.960 | 5.071       | 2.920       | 2          | -            | o          | -           | g           | -          | N           | -             | D1          | e        | o            | -           | -            | U            | o                      | -           | 10.628      | 0.37        | 1.47     | 1          | 36.2   | 0.78                               | 3.93                        | 10.730                      | 0.03                 | 0.47                  | 0.63                                 | 44.7                          | 9.86                          | 0.07        | 0.60  |
| 20525281+4131331 | 82.663 | -1.975      | 3.380       | 7          | -            | -          | -           | -           | -          | -           | -             | -           | -        | -            | -           | -            | U            | -                      | -           | 11.989      | 2.00        | ...      | 1          | 10.4   | 0.62                               | 3.97                        | 10.875                      | 1.44                 | ...                   | 1.05                                 | ...                           | 1.50                          | ...         |       |
| 20525943+5311105 | 91.649 | 5.468       | 1.663       | 1          | -            | -          | -           | g           | t          | N           | -             | D1          | e        | -            | *           | -            | -            | -                      | -           | 11.621      | 0.53        | 1.69     | 1          | 34.0   | 0.46                               | 3.89                        | 11.001                      | 0.25                 | 0.87                  | 0.52                                 | 40.7                          | 10.97                         | 0.29        | 0.98  |
| 20533478+4447263 | 85.251 | 0.020       | 9.602       | 9          | -            | -          | -           | -           | -          | -           | -             | -           | -        | -            | -           | -            | -            | -                      | -           | 9.548       | 0.84        | ...      | 1          | 131.0  | 0.82                               | 4.24                        | 5.970                       | -0.75                | ...                   | 2.97                                 | ...                           | ...                           | -0.57       | ...   |
| 20533486+4432463 | 85.064 | -0.137      | 14.065      | 8          | -            | -          | -           | -           | -          | -           | -             | -           | -        | -            | -           | -            | U            | -                      | -           | 11.476      | ...         | ...      | 1          | 41.0   | 0.60                               | 4.13                        | 6.235                       | ...                  | ...                   | 4.36                                 | ...                           | ...                           | ...         | ...   |
| 20533911+4447112 | 85.256 | 0.007       | 9.105       | 9          | -            | -          | -           | -           | -          | -           | -             | -           | -        | -            | -           | -            | -            | -                      | -           | 9.891       | 1.02        | 2.08     | 1          | 98.6   | 0.54                               | 4.24                        | 6.498                       | -0.49                | -2.45                 | 2.82                                 | ...                           | ...                           | -0.31       | -1.84 |
| 20534150+4431502 | 85.065 | -0.162      | 15.566      | 9          | -            | -          | -           | -           | -          | -           | -             | -           | -        | -            | -           | -            | -            | -                      | -           | 8.845       | 1.25        | 3.25     | 1          | 126.2  | 0.50                               | 4.13                        | 3.045                       | -1.33                | -4.48                 | 4.82                                 | ...                           | ...                           | -1.02       | -3.45 |
| 20534552+4431142 | 85.065 | -0.178      | 14.138      | 9          | -            | -          | -           | -           | -          | -           | -             | -           | -        | -            | -           | -            | -            | -                      | -           | 10.804      | 1.27        | ...      | 1          | 53.6   | 0.50                               | 4.13                        | 5.536                       | -1.07                | ...                   | 4.38                                 | ...                           | ...                           | -0.79       | ...   |
| 20535370+5012580 | 89.448 | 3.462       | 3.060       | 1          | -            | -          | -           | g           | -          | -           | -             | D1          | -        | -            | -           | -            | U            | -                      | -           | 12.341      | 1.09        | ...      | 1          | 31.0   | 0.72                               | 4.06                        | 11.201                      | 0.58                 | ...                   | 0.95                                 | 50.6                          | 10.89                         | 0.64        | ...   |
| 20540327+4402466 | 84.735 | -0.523      | 4.550       | 1          | -            | -          | -           | -           | -          | -           | -             | -           | -        | -            | -           | -            | -            | -                      | -           | 8.188       | 1.59        | 4.03     | -2         | 41.4   | 0.44                               | 4.06                        | 6.511                       | 0.81                 | 1.79                  | 1.39                                 | ...                           | ...                           | 0.63        | 2.09  |
| 20540380+5422258 | 92.671 | 6.10        |             |            |              |            |             |             |            |             |               |             |          |              |             |              |              |                        |             |             |             |          |            |        |                                    |                             |                             |                      |                       |                                      |                               |                               |             |       |

2M-ZoA galaxy catalogue description and analysis III

Table B1: a) continued.

| 2MASX J          | <i>l</i> | <i>b</i> | EBV    | Object | Sample | Disc | 2MRS | Velocity | NIR  | Photom | Ext   | <i>K</i> <sub>20</sub> | <i>H-K</i> | <i>J-K</i> | vc   | <i>a</i> | <i>b/a</i> | st.d. | <i>K</i> <sub>s</sub> <sup>o</sup> | ( <i>H-K</i> ) <sup>o</sup> | ( <i>J-K</i> ) <sup>o</sup> | <i>A<sub>K</sub></i> | <i>a</i> <sub>d</sub> <sup>o</sup> | <i>K</i> <sub>s</sub> <sup>o,d</sup> | ( <i>H-K</i> ) <sup>o,c</sup> | ( <i>J-K</i> ) <sup>o,c</sup> |        |     |      |     |      |     |      |     |      |      |      |
|------------------|----------|----------|--------|--------|--------|------|------|----------|------|--------|-------|------------------------|------------|------------|------|----------|------------|-------|------------------------------------|-----------------------------|-----------------------------|----------------------|------------------------------------|--------------------------------------|-------------------------------|-------------------------------|--------|-----|------|-----|------|-----|------|-----|------|------|------|
| (1)              | deg      | deg      | mag    | class  | off    | flag | gal  | TF       | (7b) | (7c)   | ext'd | type                   | (8)        | (9)        | Opt  | HI       | (10b)      | flg   | flg                                | flg                         | flg                         | mag                  | (21)                               | mag                                  | (22)                          | mag                           | (23)   | mag | (24) | mag | (25) | mag | (26) | mag | (27) | mag  | (28) |
| 21061494+5122043 | 91.601   | 2.745    | 9.772  | 9      | —      | —    | —    | —        | —    | —      | —     | —                      | 10.458     | 1.09       | ...  | 1        | 74.6       | 0.12  | 4.08                               | 6.817                       | -0.53                       | ...                  | 3.03                               | ...                                  | ...                           | -0.34                         | ...    | ... | ...  | ... | ...  | ... | ...  | ... | ...  | ...  |      |
| 21061631+4503203 | 86.927   | -1.499   | 1.178  | 1      | —      | —    | —    | —        | —    | —      | —     | D1                     | —          | —          | —    | —        | —          | —     | —                                  | —                           | —                           | —                    | —                                  | —                                    | —                             | —                             | —      | —   | —    | —   | —    | —   | —    | —   | —    | 0.19 | 0.75 |
| 21061823+4751071 | 89.001   | 0.376    | 2.754  | 8      | —      | p?   | —    | —        | —    | —      | —     | —                      | 10.161     | 0.75       | 0.78 | 1        | 49.4       | 0.64  | 4.22                               | 9.135                       | 0.30                        | -0.59                | 0.85                               | ...                                  | ...                           | 0.35                          | -0.41  | ... | ...  | ... | ...  | ... | ...  | ... | ...  | ...  |      |
| 21061846+5122113 | 91.608   | 2.739    | 9.460  | 9      | —      | —    | —    | —        | —    | —      | —     | —                      | 11.784     | 1.01       | 2.04 | 1        | 36.2       | 0.28  | 4.08                               | 8.259                       | -0.56                       | -2.66                | 2.93                               | ...                                  | ...                           | -0.37                         | -2.04  | ... | ...  | ... | ...  | ... | ...  | ... | ...  | ...  |      |
| 21061891+4751074 | 89.003   | 0.375    | 2.756  | 8      | —      | p?   | —    | —        | —    | —      | —     | —                      | 9.744      | 0.55       | 0.77 | 1        | 65.6       | 0.68  | 4.17                               | 8.717                       | 0.09                        | -0.60                | 0.85                               | ...                                  | ...                           | 0.15                          | -0.42  | ... | ...  | ... | ...  | ... | ...  | ... | ...  | ...  |      |
| 21063587+4923012 | 90.168   | 1.370    | 2.705  | 1      | o      | —    | —    | t        | N    | —      | —     | D1                     | 11.927     | 0.39       | 1.54 | 1        | 40.4       | 0.38  | 4.22                               | 10.919                      | -0.06                       | 0.20                 | 0.84                               | 59.0                                 | 10.74                         | -0.01                         | 0.38   | ... | ...  | ... | ...  | ... | ...  | ... | ...  | ...  |      |
| 21064188+4525375 | 87.253   | -1.305   | 1.090  | 1      | —      | —    | —    | —        | —    | —      | —     | D1                     | 11.573     | 0.52       | 1.61 | 1        | 31.2       | 0.58  | 4.16                               | 11.167                      | 0.34                        | 1.07                 | 0.34                               | 34.5                                 | 11.16                         | 0.36                          | 1.14   | ... | ...  | ... | ...  | ... | ...  | ... | ...  | ...  |      |
| 21064324+4741525 | 88.935   | 0.221    | 2.421  | 1      | —      | —    | —    | —        | —    | —      | —     | D2                     | 10.887     | 0.59       | 1.81 | 1        | 29.6       | 0.80  | 4.26                               | 9.985                       | 0.19                        | 0.61                 | 0.75                               | 37.8                                 | 9.99                          | 0.24                          | 0.77   | ... | ...  | ... | ...  | ... | ...  | ... | ...  | ...  |      |
| 21064553+5211569 | 92.271   | 3.245    | 3.677  | 9      | —      | —    | —    | —        | —    | —      | —     | —                      | 11.951     | 0.44       | 1.25 | -2       | 18.4       | 0.54  | 3.99                               | 10.581                      | -0.17                       | -0.57                | 1.14                               | ...                                  | ...                           | -0.09                         | -0.33  | ... | ...  | ... | ...  | ... | ...  | ... | ...  | ...  |      |
| 21064766+4302585 | 85.504   | -2.917   | 1.141  | 1      | —      | —    | —    | —        | —    | —      | —     | D1                     | 10.729     | 0.36       | 1.25 | 1        | 39.6       | 0.54  | 4.04                               | 10.304                      | 0.18                        | 0.68                 | 0.35                               | 43.7                                 | 10.31                         | 0.20                          | 0.76   | ... | ...  | ... | ...  | ... | ...  | ... | ...  | ...  |      |
| 21065986+3942532 | 83.053   | -5.185   | 0.644  | 1      | o      | —    | —    | —        | —    | —      | —     | D1                     | 11.342     | 0.37       | 1.09 | 1        | 41.8       | 0.84  | 3.88                               | 11.102                      | 0.26                        | 0.77                 | 0.20                               | 44.4                                 | 11.09                         | 0.27                          | 0.81   | ... | ...  | ... | ...  | ... | ...  | ... | ...  | ...  |      |
| 21070267+4214098 | 84.932   | -3.499   | 1.226  | 8      | o      | —    | —    | —        | —    | —      | —     | —                      | 6.492      | 0.94       | 1.30 | -2       | 72.6       | 0.66  | 3.97                               | 6.035                       | 0.74                        | 0.69                 | 0.38                               | ...                                  | ...                           | 0.77                          | 0.77   | ... | ...  | ... | ...  | ... | ...  | ... | ...  | ...  |      |
| 21070600+3707023 | 81.126   | -6.939   | 0.257  | 1      | —      | —    | —    | —        | —    | —      | —     | D1                     | 11.095     | 0.36       | 1.07 | 1        | 39.4       | 0.64  | 3.78                               | 10.999                      | 0.32                        | 0.94                 | 0.08                               | 40.0                                 | 11.01                         | 0.32                          | 0.96   | ... | ...  | ... | ...  | ... | ...  | ... | ...  | ...  |      |
| 21071353+4456529 | 86.961   | -1.697   | 1.306  | 1      | —      | —    | —    | —        | —    | —      | —     | D2                     | 10.338     | 0.45       | 1.58 | 1        | 50.4       | 0.90  | 4.11                               | 9.851                       | 0.24                        | 0.93                 | 0.40                               | 56.5                                 | 9.86                          | 0.26                          | 1.01   | ... | ...  | ... | ...  | ... | ...  | ... | ...  | ...  |      |
| 21071744+3706509 | 81.149   | -6.969   | 0.259  | 1      | —      | —    | —    | t        | N    | —      | —     | D1                     | 11.194     | 0.45       | 1.31 | 1        | 44.0       | 0.24  | 3.71                               | 11.097                      | 0.41                        | 1.18                 | 0.08                               | 44.6                                 | 11.10                         | 0.41                          | 1.20   | ... | ...  | ... | ...  | ... | ...  | ... | ...  | ...  |      |
| 21072604+5612009 | 95.311   | 5.859    | 1.361  | 8      | —      | —    | —    | —        | —    | —      | —     | —                      | 11.736     | 1.32       | 2.95 | 1        | 18.4       | 0.78  | 3.88                               | 11.229                      | 1.10                        | 2.27                 | 0.42                               | ...                                  | ...                           | 1.12                          | 2.36   | ... | ...  | ... | ...  | ... | ...  | ... | ...  | ...  |      |
| 21075551+4139252 | 84.613   | -4.009   | 1.216  | 1      | —      | —    | —    | —        | —    | —      | —     | D1                     | 10.902     | 0.45       | 1.54 | 1        | 32.2       | 0.66  | 3.93                               | 10.449                      | 0.25                        | 0.94                 | 0.38                               | 35.8                                 | 10.46                         | 0.27                          | 1.02   | ... | ...  | ... | ...  | ... | ...  | ... | ...  | ...  |      |
| 21081300+4403398 | 86.426   | -2.426   | 0.865  | 1      | —      | —    | —    | —        | —    | —      | —     | D1                     | 11.014     | 0.39       | 1.23 | 1        | 34.6       | 0.76  | 4.06                               | 10.692                      | 0.25                        | 0.80                 | 0.27                               | 37.1                                 | 10.70                         | 0.27                          | 0.86   | ... | ...  | ... | ...  | ... | ...  | ... | ...  | ...  |      |
| 21084767+4354039 | 86.378   | -2.610   | 0.863  | 1      | —      | —    | —    | t        | N    | —      | —     | D1                     | 10.835     | 0.45       | 1.34 | 1        | 52.4       | 0.36  | 4.02                               | 10.513                      | 0.31                        | 0.91                 | 0.27                               | 56.0                                 | 10.53                         | 0.32                          | 0.97   | ... | ...  | ... | ...  | ... | ...  | ... | ...  | ...  |      |
| 21084874+5229199 | 92.697   | 3.209    | 7.155  | 9      | —      | —    | —    | —        | —    | —      | —     | —                      | 13.428     | 0.39       | 1.58 | -1       | 18.8       | 0.58  | 3.93                               | 10.762                      | -0.79                       | -1.97                | 2.22                               | ...                                  | ...                           | -0.65                         | -1.50  | ... | ...  | ... | ...  | ... | ...  | ... | ...  | ...  |      |
| 21085630+4451164 | 87.097   | -1.983   | 1.296  | 1      | —      | —    | —    | t        | N    | —      | —     | D1                     | 10.442     | 0.44       | 1.51 | 1        | 59.8       | 0.34  | 4.06                               | 9.959                       | 0.22                        | 0.86                 | 0.40                               | 66.7                                 | 9.98                          | 0.25                          | 0.95   | ... | ...  | ... | ...  | ... | ...  | ... | ...  | ...  |      |
| 21085971+5222290 | 92.631   | 3.111    | 21.860 | 8      | —      | —    | —    | —        | —    | —      | —     | —                      | 12.845     | ...        | ...  | 1        | 17.2       | 1.00  | 4.04                               | 4.700                       | ...                         | ...                  | 6.77                               | ...                                  | ...                           | ...                           | ...    | ... | ...  | ... | ...  | ... | ...  | ... | ...  | ...  |      |
| 21090940+5001080 | 90.916   | 1.495    | 9.376  | 8      | —      | —    | —    | —        | —    | —      | —     | —                      | 10.971     | 0.80       | 2.47 | 1        | 59.2       | 0.82  | 4.15                               | 7.478                       | -0.75                       | -2.19                | 2.90                               | ...                                  | ...                           | -0.56                         | -1.57  | ... | ...  | ... | ...  | ... | ...  | ... | ...  | ...  |      |
| 21091056+5334310 | 93.535   | 3.904    | 2.861  | 9      | —      | —    | —    | —        | —    | —      | —     | —                      | 12.103     | 0.86       | 1.54 | -2       | 33.2       | 0.70  | 3.98                               | 11.037                      | 0.39                        | 0.12                 | 0.89                               | ...                                  | ...                           | 0.45                          | 0.31   | ... | ...  | ... | ...  | ... | ...  | ... | ...  | ...  |      |
| 21091402+5222590 | 92.662   | 3.090    | 31.319 | 9      | —      | —    | —    | —        | —    | —      | —     | —                      | 12.388     | 1.38       | ...  | 1        | 29.2       | 0.42  | 4.04                               | 0.719                       | -3.81                       | ...                  | 9.70                               | ...                                  | ...                           | -3.20                         | ...    | ... | ...  | ... | ...  | ... | ...  | ... | ...  |      |      |
| 21091708+5222280 | 92.661   | 3.078    | 31.113 | 9      | —      | —    | —    | —        | —    | —      | —     | —                      | 11.965     | 1.59       | ...  | 1        | 37.6       | 0.60  | 4.04                               | 0.372                       | -3.57                       | ...                  | 9.64                               | ...                                  | ...                           | -2.95                         | ...    | ... | ...  | ... | ...  | ... | ...  | ... | ...  |      |      |
| 21092185+5857595 | 97.550   | 7.525    | 0.635  | 1      | —      | —    | —    | —        | —    | —      | —     | D3                     | 10.853     | 0.43       | 1.30 | 1        | 34.6       | 0.76  | 3.76                               | 10.616                      | 0.33                        | 0.98                 | 0.20                               | 36.1                                 | 10.63                         | 0.34                          | 1.02   | ... | ...  | ... | ...  | ... | ...  | ... | ...  | ...  |      |
| 21092494+5222459 | 92.678   | 3.067    | 31.960 | 8      | —      | —    | —    | —        | —    | —      | —     | —                      | 9.091      | 1.30       | 3.02 | 1        | 88.4       | 0.76  | 4.04                               | -2.817                      | -3.99                       | -12.86               | 9.90                               | ...                                  | ...                           | -3.36                         | -10.75 | ... | ...  | ... | ...  | ... | ...  | ... | ...  | ...  |      |
| 21092756+5221489 | 92.671   | 3.051    | 29.816 | 9      | —      | —    | —    | —        | —    | —      | —     | —                      | 12.123     | 1.12       | ...  | 1        | 34.2       | 1.00  | 4.04                               | 1.014                       | -3.82                       | ...                  | 9.24                               | ...                                  | ...                           | -3.23                         | ...    | ... | ...  | ... | ...  | ... | ...  | ... | ...  |      |      |
| 21092871+4528414 | 87.620   | -1.630   | 1.136  | 1      | —      | —    | —    | —        | —    | —      | —     | D1                     | 9.447      | 0.39       | 1.39 | 1        | 75.6       | 0.62  | 4.14                               | 9.024                       | 0.20                        | 0.82                 | 0.35                               | 82.3                                 | 9.05                          | 0.22                          | 0.90   | ... | ...  | ... | ...  | ... | ...  | ... | ...  | ...  |      |
| 21092943+5222359 | 92.684   | 3.057    | 32.139 | 9      | —      | —    | —    | —        | —    | —      | —     | —                      | 10.049     | 1.20       | 2.56 | -2       | 69.0       | 0.50  | 3.99                               | -1.926                      | -4.12                       | -13.41               | 9.96                               | ...                                  | ...                           | -3.49                         | -11.29 | ... | ...  | ... | ...  | ... | ...  | ... | ...  | ...  |      |
| 21093062+5222229 | 92.684   | 3.052    | 31.116 | 9      | —      | —    | —    | —        | —    | —      | —     | —                      | 11.930     | 0.73       | 2.30 | -2       | 34.2       | 0.60  | 4.04                               | 0.336                       | -4.42                       | -13.15               | 9.64                               | ...                                  | ...                           | -3.81                         | -11.10 | ... | ...  | ... | ...  | ... | ...  | ... | ...  | ...  |      |
| 21093525+5013288 | 91.114   | 1.584    | 11.299 | 9      | —      | —    | —    | —        | —    | —      | —     | —                      | 11.408     | 0.68       | 1.85 | -1       | 50.2       | 0.58  | 4.15                               | 7.198                       | -1.20                       | -3.77                | 3.50                               | ...                                  | ...                           | -0.97                         | -3.02  | ... | ...  | ... | ...  | ... | ...  | ... | ...  | ...  |      |
| 21093561+5013190 | 91.113   | 1.581    | 11.274 | 9      | —      | —    | —    | —        | —    | —      | —     | —                      | 11.579     | 0.83       | ...  | 1        | 35.8       | 1.00  | 4.11                               | 7.378                       | -1.04                       | ...                  | 3.49                               | ...                                  | ...                           | -0.81                         | ...    | ... | ...  | ... | ...  | ... | ...  | ... | ...  |      |      |
| 21093749+5225300 | 92.734   | 3.074    | 21.029 | 8      | —      | —    | —    | —        | —    | —      | —     | —                      | 11.017     | 2.12       | ...  | 1        | 43.8       | 0.44  | 4.03                               | 3.182                       | -1.36                       | ...                  | 6.51                               | ...                                  | ...                           | -0.95                         | ...    | ... | ...  | ... | ...  | ... | ...  | ... | ...  |      |      |
| 21094611+4810591 | 89.637   | 0.173    | 5.058  | 7      | —      | —    | —    | —        | —    | —      | —     | —                      | 9.298      | 2.06       | ...  | 1        | 45.8       | 0.82  | 4.24                               | 7.413                       | 1.22                        | ...                  | 1.57                               | ...                                  | ...                           | 1.32                          | ...    | ... | ...  | ... | ...  | ... | ...  | ... | ...  |      |      |
| 21095816+5437431 | 94.390   | 4.533    | 1.968  | 1      | —      | —    | —    | t        | N    | —      | —     | D1                     | 11.749     | 0.66       | 1.73 | 1        | 32.8       | 0.48  | 3.94                               | 11.016                      | 0.34                        | 0.75                 | 0.61                               | 41.1                                 | 10.96                         | 0.37                          | 0.88   | ... | ...  | ... | ...  | ... | ...  | ... | ...  | ...  |      |
| 21101223+5129330 | 92.110   | 2.375    | 3.664  | 2      | o      | —    | —    | —        | —    | —      | —     | D2                     | 12.566     | 0.78       | 2.39 | 1        | 14.8       | 0.94  | 4.06                               | 11.201                      | 0.17                        | 0.57                 | 1.13                               | 24.5                                 | 11.03                         | 0.24                          | 0.82   | ... | ...  | ... | ...  | ... | ...  | ... | ...  | ...  |      |
| 21104814+4341173 | 86.468   | -3.021   | 0.850  | 1      | —      | —    | —    | —        | —    | —      | —     | D1                     | 10.818     | 0.38       | 1.29 | 1        | 41.2       | 0.90  | 4.01                               | 10.501                      | 0.24                        | 0.87                 | 0.26                               | 44.3                                 | 10.50                         | 0.26                          | 0.93   | ... | ...  | ... | ...  | ... | ...  | ... | ...  | ...  |      |
| 21111660+3753053 | 82.259   | -7.035   | 0.366  | 1      | —      | —    | —    | —        | —    | —      | —     | D1                     | 10.317     | 0.35       | 1.16 | 1        | 63.2       | 0.26  | 3.79                               | 10.181                      | 0.29                        | 0.98                 | 0.11                               | 64.6                                 | 10.19                         | 0.30                          | 1.00   | ... | ...  | ... | ...  | ... | ...  | ... | ...  | ...  |      |
| 21113874+5717065 | 91.608   | 6.166    | 0.943  | 1      | o      | —    | —    | —        | —    | —      | —     | D1                     | 11.420     | 0.62       | 1.56 | 1        | 29.4       | 0.74  | 3.79                               | 11.069                      | 0.47                        | 1.09                 | 0.29                               | 32.2                                 | 11.05                         | 0.49                          | 1.15   | ... | ...  | ... | ...  | ... | ...  | ... | ...  | ...  |      |
| 21114382+3731439 | 82.057   | -7.342   | 0.252  | 1      | —      | —    | —    | —        |      |        |       |                        |            |            |      |          |            |       |                                    |                             |                             |                      |                                    |                                      |                               |                               |        |     |      |     |      |     |      |     |      |      |      |

Table B1: a) continued.

| 2MASX J          | <i>l</i> | <i>b</i> | EBV    | Object | Sample | Disc | 2MRS | Velocity | NIR  | Photom | Ext  | <i>K</i> <sub>20</sub> | <i>H-K</i> | <i>J-K</i> | vc    | <i>a</i> | <i>b/a</i> | st.d. | <i>K</i> <sub>s</sub> <sup>o</sup> | ( <i>H-K</i> ) <sup>o</sup> | ( <i>J-K</i> ) <sup>o</sup> | <i>A<sub>K</sub></i> | <i>a</i> <sub>d</sub> <sup>o</sup> | <i>K</i> <sub>s</sub> <sup>o,d</sup> | ( <i>H-K</i> ) <sup>o,c</sup> | ( <i>J-K</i> ) <sup>o,c</sup> |       |       |      |       |       |       |       |
|------------------|----------|----------|--------|--------|--------|------|------|----------|------|--------|------|------------------------|------------|------------|-------|----------|------------|-------|------------------------------------|-----------------------------|-----------------------------|----------------------|------------------------------------|--------------------------------------|-------------------------------|-------------------------------|-------|-------|------|-------|-------|-------|-------|
| (1)              | deg      | deg      | mag    | class  | off    | gal  | TF   | (7b)     | (7c) | ext'd  | type | (9)                    | Opt        | HI         | (10b) | (11)     | flag       | flag  | flag                               | mag                         | mag                         | mag                  | mag                                | (25)                                 | mag                           | mag                           | mag   |       |      |       |       |       |       |
| (2a)             | (2b)     | (3)      | (4)    | (5)    | (6)    | (7a) | (7b) | (7c)     | (7d) | (8)    | (9)  | (10a)                  | (10b)      | (11)       | (12)  | (13)     | (14)       | (15)  | (16)                               | (17)                        | (18)                        | (19)                 | (20)                               | (21)                                 | (22)                          | (23)                          | (24)  | (25)  | (26) | (27)  | (28)  |       |       |
| 21181305+4526187 | 88.649   | -2.767   | 0.937  | 1      | -      | -    | -    | -        | -    | -      | D2   | -                      | -          | -          | -     | -        | -          | -     | 11.411                             | 0.40                        | 1.31                        | 1                    | 28.8                               | 0.78                                 | 4.02                          | 11.062                        | 0.25  | 0.85  | 0.29 | 31.2  | 11.07 | 0.26  | 0.91  |
| 21183139+5431287 | 95.171   | 3.563    | 1.925  | 1      | -      | -    | -    | -        | -    | -      | D1   | -                      | -          | -          | -     | -        | -          | -     | 10.491                             | 0.66                        | 1.90                        | 1                    | 59.4                               | 0.34                                 | 3.98                          | 9.774                         | 0.34  | 0.95  | 0.60 | 72.7  | 9.75  | 0.38  | 1.07  |
| 21183647+6047044 | 99.689   | 7.921    | 0.634  | 1      | -      | -    | -    | -        | -    | -      | D3   | c                      | o          | -          | -     | -        | -          | -     | 11.469                             | 0.33                        | 1.24                        | 1                    | 30.2                               | 0.76                                 | 3.66                          | 11.233                        | 0.23  | 0.93  | 0.20 | 31.7  | 11.24 | 0.24  | 0.97  |
| 21184034+5218497 | 93.607   | 1.998    | 4.005  | 1      | -      | -    | -    | -        | -    | -      | D3   | -                      | -          | -          | -     | -        | -          | -     | 12.181                             | 1.14                        | ...                         | 1                    | 22.0                               | 0.86                                 | 4.06                          | 10.689                        | 0.48  | ...   | 1.24 | 39.7  | 10.44 | 0.56  | ...   |
| 21185980+4401180 | 87.733   | -3.858   | 1.020  | 1      | -      | -    | -    | -        | -    | -      | D1   | -                      | -          | -          | -     | -        | -          | -     | 11.556                             | 0.41                        | 1.25                        | 1                    | 44.0                               | 0.64                                 | 3.95                          | 11.176                        | 0.24  | 0.75  | 0.32 | 49.5  | 11.12 | 0.26  | 0.81  |
| 21190736+4618471 | 89.384   | -2.266   | 1.818  | 8      | -      | p    | -    | -        | -    | -      | -    | -                      | -          | -          | -     | -        | -          | -     | 8.705                              | 0.94                        | 1.60                        | 1                    | 31.6                               | 0.94                                 | 4.01                          | 8.028                         | 0.64  | 0.70  | 0.56 | ...   | ...   | 0.67  | 0.82  |
| 21194132+4648489 | 89.809   | -1.984   | 2.663  | 8      | -      | -    | -    | -        | -    | -      | -    | -                      | -          | -          | -     | -        | -          | -     | 10.866                             | 1.10                        | 2.70                        | 1                    | 40.4                               | 0.42                                 | 4.00                          | 9.874                         | 0.66  | 1.38  | 0.82 | ...   | ...   | 0.72  | 1.56  |
| 21195557+4922432 | 91.658   | -0.206   | 3.581  | 1      | -      | -    | -    | -        | -    | -      | D1   | -                      | -          | -          | -     | -        | -          | -     | 11.594                             | 0.81                        | 2.39                        | 1                    | 37.4                               | 0.34                                 | 4.11                          | 10.260                        | 0.22  | 0.61  | 1.11 | 62.1  | 10.06 | 0.29  | 0.85  |
| 21195943+5519423 | 95.893   | 3.977    | 3.155  | 8      | -      | -    | -    | -        | -    | -      | -    | -                      | -          | -          | -     | -        | -          | -     | 10.937                             | 0.85                        | 1.59                        | 1                    | 52.2                               | 0.52                                 | 4.00                          | 9.761                         | 0.33  | 0.02  | 0.98 | ...   | ...   | 0.39  | 0.23  |
| 21201018+5911203 | 98.673   | 6.669    | 1.204  | 7      | -      | -    | -    | -        | -    | -      | -    | -                      | -          | -          | -     | -        | -          | -     | 11.117                             | 1.05                        | 2.62                        | 1                    | 33.4                               | 0.74                                 | 3.76                          | 10.668                        | 0.85  | 2.02  | 0.37 | ...   | ...   | 0.88  | 2.10  |
| 21202103+4519063 | 88.827   | -3.118   | 0.997  | 1      | o      | -    | -    | -        | -    | -      | D3   | -                      | -          | -          | -     | -        | -          | -     | 11.596                             | 0.40                        | 1.25                        | -2                   | 29.0                               | 0.54                                 | 3.96                          | 11.225                        | 0.24  | 0.76  | 0.31 | 31.5  | 11.23 | 0.26  | 0.82  |
| 21203006+3735002 | 83.305   | -8.566   | 0.175  | 1      | -      | -    | -    | -        | -    | -      | D1   | c                      | o          | -          | -     | -        | -          | -     | 10.611                             | 0.34                        | 1.13                        | 1                    | 61.8                               | 0.28                                 | 3.69                          | 10.546                        | 0.31  | 1.04  | 0.05 | 62.3  | 10.55 | 0.32  | 1.05  |
| 21204248+4423590 | 88.218   | -3.810   | 0.745  | 1      | -      | -    | -    | -        | -    | -      | D1   | -                      | -          | -          | -     | -        | -          | -     | 8.628                              | 0.34                        | 1.16                        | 1                    | 124.8                              | 0.44                                 | 3.93                          | 8.350                         | 0.21  | 0.79  | 0.23 | 130.7 | 8.38  | 0.23  | 0.84  |
| 21204397+5153170 | 93.527   | 1.474    | 6.997  | 8      | -      | o    | -    | -        | -    | -      | -    | -                      | -          | -          | -     | -        | -          | -     | 12.537                             | ...                         | ...                         | -2                   | 29.8                               | 0.42                                 | 4.13                          | 9.930                         | ...   | ...   | 2.17 | ...   | ...   | ...   |       |
| 21204618+4516221 | 88.846   | -3.202   | 0.999  | 1      | -      | -    | -    | -        | -    | -      | D1   | e                      | o          | -          | -     | -        | -          | -     | 10.087                             | 0.31                        | 1.22                        | 1                    | 70.8                               | 0.52                                 | 3.95                          | 9.715                         | 0.14  | 0.72  | 0.31 | 77.8  | 9.71  | 0.16  | 0.79  |
| 21205780+4828155 | 91.136   | -0.967   | 2.436  | 1      | -      | -    | -    | -        | -    | -      | D2   | -                      | -          | -          | -     | -        | -          | -     | 11.986                             | 0.76                        | ...                         | 1                    | 28.2                               | 0.72                                 | 4.15                          | 11.078                        | 0.36  | ...   | 0.75 | 39.0  | 10.94 | 0.41  | ...   |
| 21211139+4928526 | 91.876   | -0.279   | 4.076  | 9      | -      | -    | -    | -        | -    | -      | -    | -                      | -          | -          | -     | -        | -          | -     | 12.258                             | 1.02                        | ...                         | 1                    | 39.0                               | 0.40                                 | 4.13                          | 10.739                        | 0.35  | ...   | 1.26 | ...   | ...   | 0.43  | ...   |
| 21213904+4403499 | 88.099   | -4.167   | 0.815  | 1      | -      | -    | -    | -        | -    | -      | D2   | -                      | -          | -          | -     | -        | -          | -     | 8.912                              | 0.31                        | 1.16                        | 1                    | 91.2                               | 0.86                                 | 3.90                          | 8.608                         | 0.18  | 0.75  | 0.25 | 96.2  | 8.63  | 0.19  | 0.80  |
| 21214538+3736052 | 83.494   | -8.731   | 0.198  | 1      | -      | -    | -    | -        | -    | -      | D3   | c                      | o          | -          | -     | -        | -          | -     | 11.262                             | 0.26                        | 1.09                        | 1                    | 29.4                               | 0.66                                 | 3.67                          | 11.188                        | 0.23  | 0.99  | 0.06 | 29.7  | 11.20 | 0.23  | 1.00  |
| 21214731+4414419 | 88.245   | -4.056   | 0.882  | 1      | -      | -    | -    | -        | -    | -      | D1   | -                      | -          | -          | -     | -        | -          | -     | 10.326                             | 0.36                        | 1.26                        | 1                    | 55.8                               | 0.74                                 | 3.90                          | 9.997                         | 0.22  | 0.82  | 0.27 | 59.9  | 10.01 | 0.23  | 0.88  |
| 21214882+4313309 | 87.525   | -4.780   | 0.693  | 1      | -      | -    | -    | -        | -    | -      | D1   | e                      | o          | -          | -     | -        | -          | -     | 10.097                             | 0.39                        | 1.26                        | 1                    | 46.0                               | 0.82                                 | 3.86                          | 9.839                         | 0.27  | 0.91  | 0.21 | 48.2  | 9.86  | 0.28  | 0.96  |
| 21215188+4335429 | 87.794   | -4.525   | 0.799  | 1      | -      | -    | -    | -        | -    | -      | D1   | -                      | -          | -          | -     | -        | -          | -     | 11.064                             | 0.39                        | 1.36                        | 1                    | 35.4                               | 0.58                                 | 3.85                          | 10.766                        | 0.26  | 0.96  | 0.25 | 37.7  | 10.77 | 0.27  | 1.02  |
| 21215357+5210473 | 93.860   | 1.554    | 11.203 | 8      | -      | -    | -    | -        | -    | -      | -    | -                      | -          | -          | -     | -        | -          | -     | 8.676                              | 1.00                        | 2.19                        | 1                    | 93.8                               | 0.78                                 | 4.09                          | 4.502                         | -0.86 | -3.38 | 3.47 | ...   | ...   | -0.64 | -2.64 |
| 21215894+5219203 | 93.970   | 1.646    | 5.122  | 1      | -      | -    | -    | -        | -    | -      | D3   | -                      | -          | -          | -     | -        | -          | -     | 12.679                             | 0.88                        | ...                         | 1                    | 16.2                               | 0.82                                 | 4.09                          | 10.771                        | 0.03  | ...   | 1.59 | 35.1  | 10.46 | 0.13  | ...   |
| 21215917+4654296 | 90.153   | -2.195   | 2.591  | 8      | -      | -    | -    | -        | -    | -      | -    | -                      | -          | -          | -     | -        | -          | -     | 10.311                             | ...                         | 1.91                        | 1                    | 45.8                               | 1.00                                 | 3.98                          | 9.346                         | ...   | 0.62  | 0.80 | ...   | ...   | ...   | 0.79  |
| 21224661+5208343 | 93.930   | 1.433    | 4.463  | 2      | -      | -    | -    | -        | -    | -      | D4   | -                      | -          | -          | -     | -        | -          | -     | 12.904                             | ...                         | ...                         | -2                   | 19.0                               | 1.00                                 | 4.08                          | 11.241                        | ...   | ...   | 1.38 | 38.8  | 10.87 | ...   | ...   |
| 21231420+4850254 | 91.662   | -0.969   | 1.796  | 1      | -      | -    | -    | -        | -    | -      | D1   | -                      | -          | -          | -     | -        | -          | -     | 11.873                             | 0.60                        | 1.85                        | 1                    | 21.6                               | 0.68                                 | 4.08                          | 11.204                        | 0.31  | 0.95  | 0.56 | 26.2  | 11.17 | 0.34  | 1.07  |
| 21233995+6001261 | 99.584   | 6.943    | 0.605  | 1      | -      | -    | -    | -        | -    | -      | D1   | c                      | o          | -          | -     | -        | -          | -     | 10.866                             | 0.42                        | 1.27                        | 1                    | 36.2                               | 0.84                                 | 3.79                          | 10.641                        | 0.32  | 0.97  | 0.19 | 37.7  | 10.65 | 0.33  | 1.01  |
| 21240760+4943370 | 92.387   | -0.439   | 2.579  | 1      | -      | -    | -    | -        | -    | -      | D2   | -                      | -          | -          | -     | -        | -          | -     | 11.815                             | 0.73                        | ...                         | 1                    | 31.8                               | 0.34                                 | 4.16                          | 10.854                        | 0.30  | ...   | 0.80 | 43.6  | 10.77 | 0.35  | ...   |
| 21240771+5240380 | 94.452   | 1.669    | 3.187  | 8      | -      | -    | -    | -        | -    | -      | -    | -                      | -          | -          | -     | -        | -          | -     | 11.621                             | 0.51                        | 1.71                        | -2                   | 28.4                               | 0.90                                 | 4.13                          | 10.434                        | -0.02 | 0.13  | 0.99 | ...   | ...   | 0.04  | 0.34  |
| 21241922+4953140 | 92.522   | -0.346   | 2.312  | 2      | o      | -    | -    | -        | -    | -      | D1   | -                      | -          | -          | -     | -        | -          | -     | 11.628                             | 0.60                        | 1.49                        | -2                   | 50.4                               | 0.64                                 | 4.16                          | 10.767                        | 0.22  | 0.34  | 0.72 | 68.3  | 10.64 | 0.26  | 0.49  |
| 21242503+4933591 | 92.309   | -0.586   | 2.477  | 1      | -      | -    | -    | -        | -    | -      | D1   | -                      | -          | -          | -     | -        | -          | -     | 11.647                             | 0.58                        | 1.74                        | 1                    | 24.8                               | 0.52                                 | 4.16                          | 10.724                        | 0.17  | 0.51  | 0.77 | 32.9  | 10.68 | 0.22  | 0.67  |
| 21243845+5336450 | 95.162   | 2.284    | 3.307  | 8      | -      | -    | -    | -        | -    | -      | -    | -                      | -          | -          | -     | -        | -          | -     | 12.185                             | 1.13                        | ...                         | 1                    | 27.8                               | 0.30                                 | 4.08                          | 10.953                        | 0.58  | ...   | 1.02 | ...   | ...   | 0.65  | ...   |
| 21244081+5336510 | 95.167   | 2.281    | 3.296  | 8      | -      | -    | -    | -        | -    | -      | -    | -                      | -          | -          | -     | -        | -          | -     | 12.361                             | 0.93                        | 2.18                        | 1                    | 20.8                               | 0.72                                 | 4.08                          | 11.133                        | 0.39  | 0.54  | 1.02 | ...   | ...   | 0.45  | 0.76  |
| 21253828+4809267 | 91.469   | -1.736   | 1.420  | 1      | -      | -    | -    | -        | -    | -      | D2   | -                      | -          | -          | -     | -        | -          | -     | 11.084                             | 0.54                        | 1.69                        | 1                    | 32.0                               | 0.68                                 | 4.04                          | 10.555                        | 0.30  | 0.98  | 0.44 | 36.5  | 10.56 | 0.33  | 1.08  |
| 21255239+4423193 | 88.868   | -4.467   | 0.797  | 1      | -      | -    | -    | -        | -    | -      | D1   | -                      | -          | -          | -     | -        | -          | -     | 11.159                             | 0.35                        | 1.18                        | 1                    | 87.8                               | 0.40                                 | 3.90                          | 10.862                        | 0.22  | 0.79  | 0.25 | 95.4  | 10.83 | 0.24  | 0.84  |
| 21261821+4527133 | 89.667   | -3.756   | 0.947  | 1      | -      | -    | -    | -        | -    | -      | D4   | e                      | o          | -          | -     | -        | -          | -     | 10.418                             | 0.42                        | 1.32                        | 1                    | 42.4                               | 0.74                                 | 3.98                          | 10.065                        | 0.26  | 0.85  | 0.29 | 45.4  | 10.09 | 0.28  | 0.91  |
| 21262928+5344179 | 95.446   | 2.183    | 2.901  | 9      | -      | -    | -    | -        | -    | -      | -    | -                      | -          | -          | -     | -        | -          | -     | 12.224                             | ...                         | ...                         | -2                   | 26.0                               | 0.72                                 | 4.10                          | 11.143                        | ...   | ...   | 0.90 | ...   | ...   | ...   | ...   |
| 21263151+5755526 | 98.372   | 5.193    | 1.723  | 8      | -      | -    | -    | -        | -    | -      | -    | -                      | -          | -          | -     | -        | -          | -     | 10.636                             | 0.82                        | 2.42                        | 1                    | 26.6                               | 0.68                                 | 3.76                          | 9.994                         | 0.53  | 1.57  | 0.53 | ...   | ...   | 0.57  | 1.68  |
| 21263514+4541569 | 89.873   | -3.614   | 0.771  | 1      | -      | -    | -    | -        | -    | -      | D4   | -                      | -          | -          | -     | -        | -          | -     | 11.265                             | 0.43                        | 1.14                        | 1                    | 31.8                               | 0.82                                 | 4.02                          | 10.978                        | 0.31  | 0.76  | 0.24 | 33.8  | 10.99 | 0.32  | 0.81  |
| 21263766+5157260 | 94.224   | 0.886    | 4.921  | 8      | -      | -    | -    | -        | -    | -      | -    | -                      | -          | -          | -     | -        | -          | -     | 12.452                             | 0.57                        | 1.43                        | -2                   | 17.6                               | 0.68                                 | 4.08                          | 10.618                        | -0.24 | -1.02 | 1.52 | ...   | ...   | -0.15 | -0.69 |
| 21264513+5157390 | 94.241   | 0.876    | 4.769  | 8      | -      | -    | -    | -        | -    | -      | -    | -                      | -          | -          | -     | -        | -          | -     | 11.616                             | 0.69                        | 1.79                        | -2                   | 30.0                               | 0.66                                 | 4.08                          | 9.839                         | -0.10 | -0.58 | 1.48 | ...   | ...   | -0.01 | -0.26 |
| 21273041+4525157 | 89.796   | -3.926   | 0.694  | 1      | -      | -    | -    | -        | -    | -      | D1   | -                      | -          | -          | -     | -        | -          | -     | 11.018                             | 0.28                        | 1.18                        | 1                    | 55.6                               | 0.66                                 | 3.93                          | 10.759                        | 0.16  | 0.84  | 0.21 | 59.1  | 10.75 | 0.17  | 0.88  |
| 21273973+4528586 | 89.859   | -3.901   | 0.666  | 1      | -      | -    | -    | -        | -    | -      | D1   | e                      | o          | -          | -     | -        | -          | -     | 10.013                             | 0.33                        | 1.27                        | 1                    | 76.8                               | 0.36                                 | 3.93                          | 9.765                         | 0.22  | 0.93  |      |       |       |       |       |

Table B1: a) continued.

| 2MASX J          | <i>l</i> | <i>b</i> | EBV    | Object | Sample | Disc | 2MRS | Velocity | NIR  | Photom | Ext  | <i>K</i> <sub>20</sub> | <i>H-K</i> | <i>J-K</i> | vc    | <i>a</i> | <i>b/a</i> | st.d. | <i>K</i> <sub>s</sub> <sup>o</sup> | ( <i>H-K</i> ) <sup>o</sup> | ( <i>J-K</i> ) <sup>o</sup> | <i>A<sub>K</sub></i> | <i>a</i> <sub>d</sub> <sup>u</sup> | <i>K</i> <sub>s</sub> <sup>o,d</sup> | ( <i>H-K</i> ) <sup>o,c</sup> | ( <i>J-K</i> ) <sup>o,c</sup> |      |        |       |       |      |      |       |       |       |
|------------------|----------|----------|--------|--------|--------|------|------|----------|------|--------|------|------------------------|------------|------------|-------|----------|------------|-------|------------------------------------|-----------------------------|-----------------------------|----------------------|------------------------------------|--------------------------------------|-------------------------------|-------------------------------|------|--------|-------|-------|------|------|-------|-------|-------|
| (1)              | deg      | deg      | mag    | class  | off    | flg  | gal  | TF       | obs  | ext'd  | type | (14)                   | mag        | mag        | (17)  | "        | (19)       | (20)  | mag                                | mag                         | mag                         | mag                  | "                                  | mag                                  | mag                           | mag                           |      |        |       |       |      |      |       |       |       |
| (1)              | (2a)     | (2b)     | (3)    | (4)    | (5)    | (6)  | (7a) | (7b)     | (7c) | (7d)   | (8)  | (9)                    | Opt        | HI         | (10a) | (10b)    | (11)       | (12)  | (13)                               | (14)                        | (15)                        | (16)                 | (17)                               | (18)                                 | (19)                          | (20)                          | (21) | (22)   | (23)  | (24)  | (25) | (26) | (27)  | (28)  |       |
| 21335252+4151065 | 88.174   | -7.311   | 0.452  | 1      | -      | -    | g    | t        | -    | -      | D1   | c                      | o          | -          | -     | -        | -          | -     | -                                  | -                           | 10.568                      | 0.40                 | 1.23                               | 1                                    | 64.4                          | 0.40                          | 3.70 | 10.400 | 0.32  | 1.00  | 0.14 | 66.1 | 10.41 | 0.33  | 1.03  |
| 21335270+5123578 | 94.661   | -0.290   | 4.473  | 9      | -      | -    | -    | -        | -    | -      | -    | -                      | -          | -          | -     | -        | -          | -     | -                                  | -                           | 12.303                      | 0.93                 | 2.15                               | 1                                    | 27.2                          | 0.50                          | 4.10 | 10.636 | 0.19  | -0.07 | 1.39 | ...  | ...   | 0.28  | 0.23  |
| 21342433+5125353 | 94.740   | -0.325   | 6.796  | 9      | -      | -    | -    | -        | -    | -      | -    | -                      | -          | -          | -     | -        | -          | -     | -                                  | -                           | 11.625                      | 1.05                 | 2.41                               | 1                                    | 69.0                          | 0.28                          | 4.08 | 9.093  | -0.07 | -0.97 | 2.11 | ...  | ...   | 0.06  | -0.52 |
| 21345066+6322003 | 102.885  | 8.432    | 0.976  | 1      | -      | -    | g    | -        | -    | -      | -    | -                      | -          | -          | -     | -        | -          | -     | -                                  | -                           | 11.309                      | 0.44                 | 1.53                               | 1                                    | 28.8                          | 0.82                          | 3.66 | 10.945 | 0.28  | 1.04  | 0.30 | 31.2 | 10.96 | 0.30  | 1.11  |
| 21350281+5309074 | 95.975   | 0.884    | 2.271  | 1      | -      | -    | g    | t        | N    | -      | D1   | c                      | o          | -          | -     | -        | -          | -     | -                                  | -                           | 11.679                      | 0.49                 | 1.80                               | 1                                    | 22.2                          | 0.58                          | 4.07 | 10.833 | 0.11  | 0.67  | 0.70 | 28.4 | 10.81 | 0.16  | 0.82  |
| 21350891+5053115 | 94.463   | -0.803   | 5.001  | 8      | -      | -    | -    | -        | -    | -      | -    | -                      | -          | -          | -     | -        | -          | -     | -                                  | -                           | 9.002                       | 1.45                 | 2.99                               | 1                                    | 93.2                          | 0.58                          | 4.11 | 7.139  | 0.62  | 0.51  | 1.55 | ...  | ...   | 0.72  | 0.84  |
| 21351976+5708585 | 98.698   | 3.814    | 1.469  | 8      | -      | -    | -    | -        | -    | -      | -    | -                      | -          | -          | -     | -        | -          | -     | -                                  | -                           | 11.769                      | 0.65                 | 1.52                               | 1                                    | 24.2                          | 0.66                          | 3.96 | 11.222 | 0.40  | 0.79  | 0.46 | ...  | ...   | 0.43  | 0.89  |
| 21352062+5347115 | 96.435   | 1.324    | 7.192  | 8      | o      | -    | -    | -        | -    | -      | -    | -                      | -          | -          | -     | -        | o          | -     | -                                  | -                           | 8.979                       | 1.21                 | 2.39                               | 1                                    | 59.2                          | 0.86                          | 4.10 | 6.299  | 0.02  | -1.18 | 2.23 | ...  | ...   | 0.16  | -0.71 |
| 21354376+5353090 | 96.543   | 1.359    | 6.696  | 8      | -      | -    | -    | -        | -    | -      | -    | -                      | -          | -          | -     | -        | -          | -     | -                                  | -                           | 12.156                      | 1.41                 | ...                                | 1                                    | 18.8                          | 1.00                          | 4.11 | 9.661  | 0.31  | ...   | 2.07 | ...  | ...   | 0.44  | ...   |
| 21354605+5353155 | 96.549   | 1.357    | 6.560  | 8      | -      | -    | -    | -        | -    | -      | -    | -                      | -          | -          | -     | -        | -          | -     | -                                  | -                           | 11.855                      | ...                  | ...                                | 1                                    | 26.8                          | 0.74                          | 4.15 | 9.411  | ...   | ...   | 2.03 | ...  | ...   | ...   | ...   |
| 21354661+5352495 | 96.545   | 1.351    | 6.802  | 8      | -      | -    | -    | -        | -    | -      | -    | -                      | -          | -          | -     | -        | -          | -     | -                                  | -                           | 12.314                      | 1.04                 | 2.10                               | 1                                    | 21.0                          | 0.54                          | 4.15 | 9.780  | -0.08 | -1.28 | 2.11 | ...  | ...   | 0.05  | -0.83 |
| 21355259+4734217 | 92.322   | -3.337   | 0.643  | 1      | o      | -    | -    | -        | N    | -      | D1   | -                      | o          | -          | -     | -        | -          | o     | -                                  | -                           | 10.484                      | 0.32                 | 1.01                               | 1                                    | 63.6                          | 0.68                          | 3.95 | 10.244 | 0.21  | 0.69  | 0.20 | 67.1 | 10.24 | 0.23  | 0.73  |
| 21355399+4728217 | 92.258   | -3.414   | 0.635  | 1      | -      | -    | -    | -        | t    | N      | D1   | -                      | o          | -          | -     | -        | -          | -     | -                                  | -                           | 11.458                      | 0.53                 | 1.41                               | 1                                    | 26.2                          | 0.42                          | 3.97 | 11.221 | 0.42  | 1.10  | 0.20 | 27.4 | 11.24 | 0.44  | 1.14  |
| 21355419+5350566 | 96.538   | 1.315    | 5.665  | 8      | -      | -    | -    | -        | -    | -      | -    | -                      | -          | -          | -     | -        | -          | -     | -                                  | -                           | 10.418                      | 1.60                 | ...                                | 1                                    | 41.0                          | 0.44                          | 4.15 | 8.307  | 0.66  | ...   | 1.75 | ...  | ...   | 0.78  | ...   |
| 21362763+5936230 | 100.466  | 5.532    | 1.063  | 1      | -      | -    | -    | t        | N    | -      | D1   | e                      | o          | -          | -     | -        | -          | -     | -                                  | -                           | 11.616                      | 0.57                 | 1.55                               | 1                                    | 35.2                          | 0.30                          | 3.91 | 11.220 | 0.39  | 1.02  | 0.33 | 38.9 | 11.21 | 0.41  | 1.09  |
| 21371347+4700045 | 92.109   | -3.914   | 0.814  | 1      | -      | -    | -    | -        | -    | -      | D2   | e                      | o          | -          | -     | -        | -          | -     | -                                  | -                           | 11.358                      | 0.38                 | 1.25                               | 1                                    | 24.0                          | 0.74                          | 3.93 | 11.055 | 0.25  | 0.84  | 0.25 | 25.5 | 11.07 | 0.26  | 0.90  |
| 21371401+5129515 | 95.115   | -0.568   | 3.302  | 9      | -      | -    | -    | -        | -    | -      | -    | -                      | -          | -          | -     | -        | -          | -     | -                                  | -                           | 12.148                      | ...                  | ...                                | 1                                    | 23.0                          | 0.44                          | 4.09 | 10.918 | ...   | ...   | 1.02 | ...  | ...   | ...   | ...   |
| 21375000+5929172 | 100.516  | 5.327    | 1.055  | 1      | -      | -    | -    | -        | -    | -      | D4   | e                      | o          | -          | -     | -        | -          | -     | -                                  | -                           | 10.941                      | 0.57                 | 1.65                               | 1                                    | 48.0                          | 0.82                          | 3.84 | 10.548 | 0.39  | 1.13  | 0.33 | 52.8 | 10.55 | 0.41  | 1.20  |
| 21382248+5019142 | 94.465   | -1.566   | 3.774  | 8      | -      | -    | -    | -        | -    | -      | -    | -                      | -          | -          | -     | -        | -          | -     | -                                  | -                           | 11.070                      | 1.25                 | 2.32                               | 1                                    | 50.4                          | 0.38                          | 4.05 | 9.664  | 0.63  | 0.45  | 1.17 | ...  | ...   | 0.70  | 0.69  |
| 21382879+5510173 | 97.699   | 2.050    | 3.006  | 9      | -      | -    | -    | -        | -    | -      | -    | -                      | -          | -          | -     | -        | -          | -     | -                                  | -                           | 11.908                      | 0.68                 | 2.00                               | -2                                   | 36.8                          | 0.42                          | 4.08 | 10.788 | 0.19  | 0.51  | 0.93 | ...  | ...   | 0.25  | 0.71  |
| 21383365+4409322 | 90.377   | -6.185   | 0.579  | 1      | -      | -    | -    | -        | -    | -      | D3   | c                      | o          | -          | -     | -        | -          | -     | -                                  | -                           | 11.321                      | 0.38                 | 1.23                               | 1                                    | 25.6                          | 0.52                          | 3.80 | 11.105 | 0.28  | 0.94  | 0.18 | 26.5 | 11.12 | 0.29  | 0.98  |
| 21384081+4415442 | 90.463   | -6.123   | 0.525  | 1      | -      | -    | -    | -        | -    | -      | -    | -                      | -          | -          | -     | -        | -          | -     | -                                  | -                           | 10.385                      | 0.44                 | 1.32                               | 1                                    | 53.6                          | 0.66                          | 3.81 | 10.189 | 0.35  | 1.06  | 0.16 | 55.4 | 10.20 | 0.36  | 1.10  |
| 21390221+4414199 | 90.495   | -6.183   | 0.561  | 1      | -      | -    | -    | -        | -    | -      | D2   | c                      | o          | -          | -     | -        | -          | -     | -                                  | -                           | 9.353                       | 0.38                 | 1.18                               | 1                                    | 72.0                          | 0.78                          | 3.77 | 9.144  | 0.29  | 0.90  | 0.17 | 74.5 | 9.16  | 0.30  | 0.94  |
| 21393548+4147248 | 88.925   | -8.075   | 0.463  | 1      | -      | -    | -    | t        | -    | -      | D1   | c                      | o          | -          | -     | -        | -          | -     | -                                  | -                           | 11.305                      | 0.41                 | 1.21                               | 1                                    | 41.8                          | 0.26                          | 3.71 | 11.132 | 0.33  | 0.98  | 0.14 | 43.0 | 11.14 | 0.34  | 1.01  |
| 21394111+5120356 | 95.298   | -0.937   | 3.050  | 8      | -      | -    | -    | -        | -    | -      | -    | -                      | -          | -          | -     | -        | -          | -     | -                                  | -                           | 11.391                      | 1.49                 | ...                                | 1                                    | 51.6                          | 0.40                          | 4.05 | 10.255 | 0.99  | ...   | 0.94 | ...  | ...   | 1.05  | ...   |
| 21395357+5014175 | 94.592   | -1.788   | 4.133  | 9      | -      | -    | -    | -        | -    | -      | -    | -                      | -          | -          | -     | -        | -          | -     | -                                  | -                           | 12.271                      | 1.01                 | 1.96                               | 1                                    | 31.0                          | 0.26                          | 4.02 | 10.731 | 0.32  | -0.09 | 1.28 | ...  | ...   | 0.40  | 0.18  |
| 21401032+4130099 | 88.813   | -8.362   | 0.418  | 1      | -      | -    | -    | t        | N    | -      | D1   | c                      | o          | -          | -     | -        | -          | -     | -                                  | -                           | 11.340                      | 0.30                 | 1.16                               | 1                                    | 27.2                          | 0.46                          | 3.68 | 11.184 | 0.23  | 0.95  | 0.13 | 27.9 | 11.20 | 0.24  | 0.98  |
| 21402873+5636094 | 98.858   | 2.937    | 2.057  | 7      | -      | -    | -    | -        | -    | -      | -    | -                      | -          | -          | -     | -        | -          | -     | -                                  | -                           | 10.789                      | 0.83                 | 2.01                               | 1                                    | 50.4                          | 0.40                          | 4.03 | 10.023 | 0.49  | 0.99  | 0.64 | ...  | ...   | 0.53  | 1.13  |
| 21404554+5816024 | 99.986   | 4.164    | 3.537  | 9      | -      | -    | -    | -        | -    | -      | -    | -                      | -          | -          | -     | -        | -          | -     | -                                  | -                           | 10.080                      | ...                  | ...                                | 1                                    | 73.4                          | 1.00                          | 3.97 | 8.762  | ...   | ...   | 1.10 | ...  | ...   | ...   | ...   |
| 21405718+5039561 | 95.001   | -1.578   | 2.643  | 7      | -      | -    | -    | -        | -    | -      | -    | -                      | -          | -          | -     | -        | -          | -     | -                                  | -                           | 10.579                      | 1.34                 | 2.56                               | 1                                    | 44.6                          | 0.62                          | 4.11 | 9.594  | 0.90  | 1.25  | 0.82 | ...  | ...   | 0.95  | 1.42  |
| 21411938+5103170 | 95.301   | -1.323   | 1.924  | 1      | -      | -    | -    | t        | N    | -      | D3   | -                      | -          | -          | -     | -        | -          | -     | -                                  | -                           | 11.487                      | ...                  | 1.60                               | 1                                    | 29.4                          | 1.00                          | 4.06 | 10.770 | ...   | 0.65  | 0.60 | 36.0 | 10.75 | ...   | 0.78  |
| 21413756+5245302 | 96.454   | -0.068   | 3.157  | 1      | -      | -    | -    | -        | -    | -      | D1   | -                      | -          | -          | -     | -        | -          | -     | -                                  | -                           | 12.229                      | 0.63                 | 2.16                               | 1                                    | 22.8                          | 0.54                          | 4.09 | 11.053 | 0.11  | 0.59  | 0.98 | 33.8 | 10.96 | 0.17  | 0.80  |
| 21420185+5443285 | 97.788   | 1.378    | 3.229  | 8      | -      | -    | -    | -        | -    | -      | -    | -                      | -          | -          | -     | -        | -          | -     | -                                  | -                           | 12.148                      | 0.67                 | 1.70                               | 1                                    | 17.4                          | 0.68                          | 4.08 | 10.945 | 0.13  | 0.09  | 1.00 | ...  | ...   | 0.20  | 0.31  |
| 21420203+4416330 | 90.924   | -6.511   | 0.337  | 1      | -      | -    | -    | -        | -    | -      | D1   | c                      | o          | -          | -     | -        | -          | -     | -                                  | -                           | 11.338                      | 0.41                 | 1.15                               | 1                                    | 40.8                          | 0.54                          | 3.81 | 11.212 | 0.36  | 0.98  | 0.10 | 41.6 | 11.22 | 0.36  | 1.00  |
| 21421327+5442426 | 97.800   | 1.350    | 3.301  | 8      | -      | -    | -    | -        | -    | -      | -    | -                      | -          | -          | -     | -        | -          | -     | -                                  | -                           | 12.179                      | 0.96                 | ...                                | 1                                    | 26.6                          | 0.48                          | 4.08 | 10.949 | 0.41  | ...   | 1.02 | ...  | ...   | 0.48  | ...   |
| 21422368+5455056 | 97.954   | 1.490    | 12.345 | 8      | -      | -    | -    | -        | -    | -      | -    | -                      | -          | -          | -     | -        | -          | -     | -                                  | -                           | 9.731                       | 1.04                 | 2.04                               | 1                                    | 64.4                          | 0.86                          | 4.07 | 5.131  | -1.00 | -4.09 | 3.82 | ...  | ...   | -0.76 | -3.28 |
| 21422696+6604278 | 105.337  | 9.892    | 4.893  | 9      | -      | -    | -    | -        | -    | -      | -    | -                      | -          | -          | -     | -        | -          | -     | -                                  | -                           | 12.922                      | 1.37                 | ...                                | 1                                    | 18.6                          | 0.90                          | 3.58 | 11.099 | 0.56  | ...   | 1.52 | ...  | ...   | 0.66  | ...   |
| 21422809+5455586 | 97.972   | 1.494    | 14.765 | 9      | -      | -    | -    | -        | -    | -      | -    | -                      | -          | -          | -     | -        | -          | -     | -                                  | -                           | 9.400                       | 0.70                 | 1.83                               | 1                                    | 43.0                          | 0.54                          | 4.07 | 3.899  | -1.75 | -5.50 | 4.57 | ...  | ...   | -1.46 | -4.53 |
| 21423859+4330562 | 90.503   | -7.155   | 0.519  | 1      | o      | -    | -    | -        | -    | -      | D3   | c                      | o          | h          | -     | -        | o          | -     | -                                  | -                           | 10.201                      | 0.44                 | 1.27                               | 1                                    | 39.6                          | 0.90                          | 3.69 | 10.008 | 0.36  | 1.02  | 0.16 | 40.7 | 10.03 | 0.37  | 1.05  |
| 21424651+5450599 | 97.951   | 1.403    | 8.814  | 8      | -      | -    | -    | -        | -    | -      | -    | -                      | -          | -          | -     | -        | -          | -     | -                                  | -                           | 12.546                      | ...                  | ...                                | 1                                    | 14.0                          | 1.00                          | 4.12 | 9.262  | ...   | ...   | 2.73 | ...  | ...   | ...   | ...   |
| 21425014+4311456 | 90.317   | -7.419   | 0.450  | 1      | -      | -    | -    | -        | -    | -      | D1   | c                      | o          | -          | -     | -        | -          | -     | -                                  | -                           | 10.704                      | 0.35                 | 1.15                               | 1                                    | 45.8                          | 0.60                          | 3.73 | 10.536 | 0.28  | 0.92  | 0.14 | 47.0 | 10.55 | 0.29  | 0.95  |
| 21425451+6605200 | 105.382  | 9.872    | 8.206  | 9      | -      | -    | -    | -        | -    | -      | -    | -                      | -          | -          | -     | -        | -          | -     | -                                  | -                           | 11.465                      | 0.89                 | 1.71                               | 1                                    | 50.8                          | 0.10                          | 3.71 | 8.407  | -0.46 | -2.36 | 2.54 | ...  | ...   | -0.30 | -1.82 |
| 21425582+6605430 | 105.388  | 9.875    | 8.302  | 9      | -      | -    | -    | -        | -    | -      | -    | -                      | -          | -          | -     | -        | -          | -     | -                                  | -                           | 10.368                      | 1.04                 | 2.22                               | 1                                    | 64.8                          | 0.84                          |      |        |       |       |      |      |       |       |       |



Table B1: a) continued.

| 2MASX J          | $l$         | $b$         | EBV        | Object       | Sample     | Disc        | 2MRS        | Velocity   | NIR         | Photom        | Ext         | $K_{20}$ | $H-K$        | $J-K$       | vc           | $a$          | $b/a$        | st.d. | $K_s^o$     | $(H-K)^o$   | $(J-K)^o$ | $A_K$ | $a_d^d$ | $K_s^{o,d}$ | $(H-K)^{o,c}$ | $(J-K)^{o,c}$ |             |             |      |             |             |             |       |
|------------------|-------------|-------------|------------|--------------|------------|-------------|-------------|------------|-------------|---------------|-------------|----------|--------------|-------------|--------------|--------------|--------------|-------|-------------|-------------|-----------|-------|---------|-------------|---------------|---------------|-------------|-------------|------|-------------|-------------|-------------|-------|
| (1)              | deg<br>(2a) | deg<br>(2b) | mag<br>(3) | class<br>(4) | off<br>(5) | flag<br>(6) | gal<br>(7a) | TF<br>(7b) | obs<br>(7c) | ext'd<br>(7d) | type<br>(8) | (9)      | Opt<br>(10a) | HI<br>(10b) | flag<br>(11) | flag<br>(12) | flag<br>(13) | (14)  | mag<br>(15) | mag<br>(16) | (17)      | (18)  | (19)    | (20)        | mag<br>(21)   | mag<br>(22)   | mag<br>(23) | mag<br>(24) | (25) | mag<br>(26) | mag<br>(27) | mag<br>(28) |       |
| 21494160+5525121 | 99.075      | 1.203       | 2.934      | 7            | —          | —           | —           | —          | —           | —             | —           | —        | —            | —           | —            | —            | —            | —     | 11.498      | 1.08        | 3.07      | −2    | 23.4    | 0.68        | 4.06          | 10.405        | 0.59        | 1.61        | 0.91 | ...         | ...         | 0.65        | 1.81  |
| 21495878+5333509 | 97.931      | −0.259      | 2.620      | 9            | —          | —           | —           | —          | —           | —             | —           | —        | —            | —           | —            | —            | —            | —     | 12.166      | 1.43        | ...       | 1     | 22.0    | 0.66        | 4.09          | 11.190        | 0.99        | ...         | 0.81 | ...         | ...         | 1.04        | ...   |
| 21501202+5659240 | 100.125     | 2.372       | 2.155      | 9            | —          | —           | —           | —          | —           | —             | —           | —        | —            | —           | —            | —            | —            | —     | 11.775      | 1.02        | 2.13      | −2    | 31.6    | 0.50        | 4.05          | 10.972        | 0.67        | 1.06        | 0.67 | ...         | ...         | 0.71        | 1.20  |
| 21505636+4432319 | 92.318      | −7.337      | 0.365      | 1            | —          | —           | —           | —          | —           | —             | —           | —        | —            | —           | —            | —            | —            | —     | 9.944       | 0.31        | 1.15      | 1     | 65.0    | 0.56        | 3.73          | 9.808         | 0.25        | 0.97        | 0.11 | 66.3        | 9.82        | 0.26        | 0.99  |
| 21510146+4657059 | 93.869      | −5.485      | 0.389      | 1            | —          | —           | —           | —          | —           | —             | —           | —        | —            | —           | —            | —            | —            | —     | 11.184      | 0.35        | 1.19      | 1     | 32.4    | 0.88        | 3.80          | 11.039        | 0.29        | 1.00        | 0.12 | 33.2        | 11.05       | 0.30        | 1.02  |
| 21511366+6615441 | 106.144     | 9.457       | 0.799      | 1            | —          | —           | —           | —          | —           | —             | —           | —        | —            | —           | —            | —            | —            | —     | 11.220      | 0.55        | 1.52      | 1     | 30.2    | 0.76        | 3.49          | 10.922        | 0.42        | 1.12        | 0.25 | 32.3        | 10.93       | 0.44        | 1.17  |
| 21511496+5439031 | 98.762      | 0.466       | 2.716      | 1            | o          | —           | —           | —          | —           | —             | —           | —        | —            | —           | —            | —            | —            | —     | 11.246      | ...         | 2.02      | 1     | 47.8    | 1.00        | 3.99          | 10.234        | ...         | 0.67        | 0.84 | 69.4        | 10.08       | ...         | 0.85  |
| 21511714+5439331 | 98.771      | 0.469       | 2.722      | 1            | —          | —           | —           | —          | —           | —             | —           | —        | —            | —           | —            | —            | —            | —     | 11.252      | 0.70        | 2.01      | 1     | 40.6    | 0.70        | 3.99          | 10.238        | 0.25        | 0.65        | 0.84 | 56.4        | 10.16       | 0.31        | 0.83  |
| 21512406+4603029 | 93.346      | −6.223      | 0.388      | 1            | —          | —           | —           | —          | —           | —             | —           | —        | —            | —           | —            | —            | —            | —     | 10.336      | 0.32        | 1.19      | 1     | 66.6    | 0.24        | 3.76          | 10.191        | 0.26        | 1.00        | 0.12 | 68.1        | 10.20       | 0.27        | 1.03  |
| 21512814+5316383 | 97.922      | −0.622      | 1.409      | 1            | —          | —           | —           | —          | —           | —             | —           | —        | —            | —           | —            | —            | —            | —     | 11.060      | 0.51        | 1.58      | 1     | 35.2    | 0.60        | 4.11          | 10.535        | 0.27        | 0.88        | 0.44 | 39.8        | 10.55       | 0.30        | 0.97  |
| 21514071+5326542 | 98.054      | −0.509      | 1.431      | 1            | —          | —           | —           | —          | —           | —             | —           | —        | —            | —           | —            | —            | —            | —     | 10.338      | 0.50        | 1.61      | 1     | 56.0    | 0.54        | 4.12          | 9.805         | 0.26        | 0.90        | 0.44 | 64.5        | 9.79        | 0.29        | 0.99  |
| 21520223+5647489 | 100.198     | 2.064       | 5.858      | 8            | —          | —           | —           | —          | —           | —             | —           | —        | —            | —           | —            | —            | —            | —     | 9.728       | 0.85        | 2.04      | 1     | 49.4    | 0.88        | 4.07          | 7.545         | −0.12       | −0.87       | 1.81 | ...         | ...         | −0.00       | −0.49 |
| 21523166+5245290 | 97.720      | −1.126      | 1.327      | 1            | —          | —           | —           | —          | —           | —             | —           | —        | —            | —           | —            | —            | —            | —     | 11.253      | 0.39        | 1.51      | 1     | 30.4    | 0.76        | 4.06          | 10.759        | 0.17        | 0.85        | 0.41 | 34.2        | 10.77       | 0.20        | 0.93  |
| 21525720+5639548 | 100.213     | 1.883       | 4.049      | 7            | —          | —           | —           | —          | —           | —             | —           | —        | —            | —           | —            | —            | —            | —     | 9.912       | 1.30        | 2.61      | 1     | 47.8    | 0.94        | 4.07          | 8.403         | 0.63        | 0.60        | 1.25 | ...         | ...         | 0.71        | 0.87  |
| 21530361+4715302 | 94.333      | −5.465      | 6.475      | 9            | —          | —           | —           | —          | —           | —             | —           | —        | —            | —           | —            | —            | —            | —     | 12.789      | 0.65        | ...       | 1     | 24.0    | 1.00        | 3.81          | 10.376        | −0.42       | ...         | 2.01 | ...         | ...         | −0.30       | ...   |
| 21530635+4715052 | 94.335      | −5.475      | 6.555      | 9            | —          | —           | —           | —          | —           | —             | —           | —        | —            | —           | —            | —            | —            | —     | 13.542      | 0.86        | 1.95      | −1    | 13.6    | 1.00        | 3.81          | 11.100        | −0.23       | −1.30       | 2.03 | ...         | ...         | −0.10       | −0.87 |
| 21531600+4715587 | 94.365      | −5.481      | 8.500      | 8            | —          | —           | —           | —          | —           | —             | —           | —        | —            | —           | —            | —            | —            | —     | 13.140      | 0.66        | 1.68      | −2    | 18.0    | 0.60        | 3.98          | 9.973         | −0.74       | −2.54       | 2.63 | ...         | ...         | −0.58       | −1.98 |
| 21531776+4716197 | 94.373      | −5.479      | 9.057      | 8            | —          | —           | —           | —          | —           | —             | —           | —        | —            | —           | —            | —            | —            | —     | 12.224      | 0.69        | 1.51      | −2    | 35.2    | 0.58        | 3.98          | 8.849         | −0.81       | −2.99       | 2.81 | ...         | ...         | −0.63       | −2.39 |
| 21532427+4905535 | 95.353      | −4.067      | 0.424      | 1            | —          | —           | —           | —          | —           | —             | —           | —        | —            | —           | —            | —            | —            | —     | 10.963      | 0.38        | 1.22      | 1     | 31.8    | 0.84        | 3.96          | 10.805        | 0.31        | 1.01        | 0.13 | 32.6        | 10.82       | 0.32        | 1.03  |
| 21532906+4720147 | 94.439      | −5.449      | 8.956      | 8            | —          | —           | —           | —          | —           | —             | —           | —        | —            | —           | —            | —            | —            | —     | 12.910      | 0.80        | ...       | 1     | 23.0    | 0.70        | 3.98          | 9.573         | −0.69       | ...         | 2.77 | ...         | ...         | −0.51       | ...   |
| 21532956+4713467 | 94.372      | −5.533      | 8.217      | 9            | —          | —           | —           | —          | —           | —             | —           | —        | —            | —           | —            | —            | —            | —     | 13.038      | 0.42        | 1.23      | 2     | 12.0    | 1.00        | 3.98          | 9.976         | −0.94       | −2.85       | 2.55 | ...         | ...         | −0.78       | −2.30 |
| 21533319+4714397 | 94.390      | −5.528      | 8.801      | 9            | —          | —           | —           | —          | —           | —             | —           | —        | —            | —           | —            | —            | —            | —     | 10.898      | 0.91        | 2.06      | 1     | 64.4    | 0.50        | 3.98          | 7.619         | −0.55       | −2.31       | 2.73 | ...         | ...         | −0.37       | −1.73 |
| 21533339+4714177 | 94.386      | −5.534      | 8.523      | 8            | —          | —           | —           | —          | —           | —             | —           | —        | —            | —           | —            | —            | —            | —     | 10.732      | 0.83        | 1.81      | 1     | 73.4    | 0.70        | 3.98          | 7.556         | −0.58       | −2.43       | 2.64 | ...         | ...         | −0.41       | −1.86 |
| 21533418+4717267 | 94.421      | −5.494      | 9.870      | 9            | —          | —           | —           | —          | —           | —             | —           | —        | —            | —           | —            | —            | —            | —     | 12.386      | 1.06        | 2.27      | 1     | 30.0    | 0.72        | 3.98          | 8.708         | −0.58       | −2.64       | 3.06 | ...         | ...         | −0.38       | −1.99 |
| 21533448+4720347 | 94.455      | −5.454      | 8.626      | 8            | —          | —           | —           | —          | —           | —             | —           | —        | —            | —           | —            | —            | —            | —     | 13.090      | 0.66        | 1.69      | −1    | 20.8    | 0.60        | 3.98          | 9.876         | −0.77       | −2.59       | 2.67 | ...         | ...         | −0.60       | −2.02 |
| 21533869+5627509 | 100.162     | 1.666       | 2.837      | 8            | —          | —           | —           | —          | —           | —             | —           | —        | —            | —           | —            | —            | —            | —     | 10.705      | 1.32        | 2.98      | 1     | 48.8    | 0.56        | 4.08          | 9.648         | 0.85        | 1.57        | 0.88 | ...         | ...         | 0.90        | 1.76  |
| 21534890+4714036 | 94.418      | −5.564      | 7.170      | 9            | —          | —           | —           | —          | —           | —             | —           | —        | —            | —           | —            | —            | —            | —     | 13.011      | ...         | ...       | −1    | 19.0    | 1.00        | 3.98          | 10.339        | ...         | ...         | 2.22 | ...         | ...         | ...         | ...   |
| 21534978+4713506 | 94.418      | −5.568      | 6.949      | 8            | —          | —           | —           | —          | —           | —             | —           | —        | —            | —           | —            | —            | —            | —     | 12.711      | ...         | ...       | 1     | 26.4    | 0.50        | 3.98          | 10.122        | ...         | ...         | 2.15 | ...         | ...         | ...         | ...   |
| 21535436+4153584 | 91.048      | −9.724      | 0.327      | 1            | —          | —           | —           | —          | —           | —             | —           | —        | —            | —           | —            | —            | —            | —     | 11.078      | 0.31        | 1.10      | 1     | 42.4    | 0.32        | 3.54          | 10.956        | 0.26        | 0.94        | 0.10 | 43.2        | 10.97       | 0.27        | 0.96  |
| 21541046+5740409 | 100.975     | 2.571       | 4.191      | 8            | —          | —           | —           | —          | —           | —             | —           | —        | —            | —           | —            | —            | —            | —     | 12.596      | 0.66        | 1.95      | −2    | 21.6    | 0.50        | 4.01          | 11.034        | −0.03       | −0.13       | 1.30 | ...         | ...         | 0.05        | 0.14  |
| 21541934+5742569 | 101.014     | 2.588       | 4.516      | 8            | —          | —           | —           | —          | —           | —             | —           | —        | —            | —           | —            | —            | —            | —     | 10.063      | 0.86        | 1.95      | 1     | 50.2    | 0.44        | 4.01          | 8.380         | 0.12        | −0.30       | 1.40 | ...         | ...         | 0.20        | 0.00  |
| 21542119+5741039 | 100.998     | 2.561       | 4.319      | 9            | —          | —           | —           | —          | —           | —             | —           | —        | —            | —           | —            | —            | —            | —     | 10.348      | 0.91        | 2.06      | 1     | 52.4    | 0.48        | 4.01          | 8.739         | 0.19        | −0.09       | 1.34 | ...         | ...         | 0.28        | 0.20  |
| 21542207+5741204 | 101.002     | 2.564       | 4.367      | 8            | —          | —           | —           | —          | —           | —             | —           | —        | —            | —           | —            | —            | —            | —     | 11.280      | 1.16        | 2.93      | 1     | 33.6    | 0.60        | 4.09          | 9.653         | 0.43        | 0.76        | 1.35 | ...         | ...         | 0.52        | 1.05  |
| 21542556+4555386 | 93.678      | −6.449      | 0.351      | 1            | —          | —           | —           | —          | —           | —             | —           | —        | —            | —           | —            | —            | —            | —     | 10.508      | 0.39        | 1.18      | 1     | 59.4    | 0.22        | 3.77          | 10.377        | 0.33        | 1.00        | 0.11 | 60.5        | 10.39       | 0.34        | 1.02  |
| 21542613+4144038 | 91.020      | −9.915      | 0.310      | 1            | —          | —           | —           | —          | —           | —             | —           | —        | —            | —           | —            | —            | —            | —     | 10.712      | 0.36        | 1.28      | 1     | 76.4    | 0.22        | 3.55          | 10.596        | 0.31        | 1.13        | 0.10 | 77.8        | 10.60       | 0.32        | 1.15  |
| 21543095+4525535 | 93.378      | −7.046      | 0.343      | 1            | —          | —           | —           | —          | —           | —             | —           | —        | —            | —           | —            | —            | —            | —     | 10.986      | 0.33        | 1.11      | 1     | 47.0    | 0.36        | 3.76          | 10.858        | 0.28        | 0.94        | 0.11 | 48.1        | 10.86       | 0.28        | 0.97  |
| 21553252+4258052 | 91.967      | −9.083      | 0.307      | 1            | —          | —           | —           | —          | —           | —             | —           | —        | —            | —           | —            | —            | —            | —     | 11.173      | 0.40        | 1.20      | 1     | 43.4    | 0.36        | 3.61          | 11.059        | 0.35        | 1.05        | 0.10 | 44.2        | 11.07       | 0.35        | 1.07  |
| 21554184+5758309 | 101.319     | 2.679       | 2.509      | 8            | —          | —           | —           | —          | —           | —             | —           | —        | —            | —           | —            | —            | —            | —     | 11.844      | 1.22        | 2.99      | 1     | 17.0    | 0.82        | 4.03          | 10.909        | 0.80        | 1.75        | 0.78 | ...         | ...         | 0.85        | 1.91  |
| 21554456+5751079 | 101.247     | 2.578       | 2.966      | 9            | —          | —           | —           | —          | —           | —             | —           | —        | —            | —           | —            | —            | —            | —     | 12.091      | 0.62        | 1.64      | 1     | 29.0    | 0.58        | 4.03          | 10.986        | 0.13        | 0.16        | 0.92 | ...         | ...         | 0.19        | 0.36  |
| 21554534+5228186 | 97.925      | −1.655      | 1.143      | 1            | —          | —           | —           | —          | —           | —             | —           | —        | —            | —           | —            | —            | —            | —     | 11.475      | 0.45        | 1.28      | 1     | 44.0    | 0.80        | 4.02          | 11.049        | 0.26        | 0.72        | 0.35 | 49.8        | 11.01       | 0.28        | 0.79  |
| 21561508+5750419 | 101.296     | 2.531       | 2.939      | 8            | —          | —           | —           | —          | —           | —             | —           | —        | —            | —           | —            | —            | —            | —     | 11.256      | 1.13        | 2.72      | 1     | 17.6    | 0.74        | 4.01          | 10.161        | 0.65        | 1.26        | 0.91 | ...         | ...         | 0.70        | 1.45  |
| 21562089+5910210 | 102.126     | 3.568       | 2.947      | 9            | —          | —           | —           | —          | —           | —             | —           | —        | —            | —           | —            | —            | —            | —     | 11.398      | ...         | ...       | 1     | 42.0    | 0.30        | 3.98          | 10.300        | ...         | ...         | 0.91 | ...         | ...         | ...         | ...   |
| 21562725+5801500 | 101.432</   |             |            |              |            |             |             |            |             |               |             |          |              |             |              |              |              |       |             |             |           |       |         |             |               |               |             |             |      |             |             |             |       |

Table B1: a) continued.

| 2MASX J          | <i>l</i>    | <i>b</i>    | EBV        | Object       | Sample         | Disc        | 2MRS       | Velocity    | NIR           | Photom      | Ext | <i>K</i> <sub>20</sub> | <i>H-K</i>   | <i>J-K</i>  | vc          | <i>a</i>    | <i>b/a</i>  | st.d. | <i>K</i> <sub>s</sub> <sup>o</sup> | ( <i>H-K</i> ) <sup>o</sup> | ( <i>J-K</i> ) <sup>o</sup> | <i>A</i> <sub>K</sub> | <i>a</i> <sub>d</sub> <sup>o</sup> | <i>K</i> <sub>s</sub> <sup>o,d</sup> | ( <i>H-K</i> ) <sup>o,c</sup> | ( <i>J-K</i> ) <sup>o,c</sup> |       |       |      |       |       |       |       |
|------------------|-------------|-------------|------------|--------------|----------------|-------------|------------|-------------|---------------|-------------|-----|------------------------|--------------|-------------|-------------|-------------|-------------|-------|------------------------------------|-----------------------------|-----------------------------|-----------------------|------------------------------------|--------------------------------------|-------------------------------|-------------------------------|-------|-------|------|-------|-------|-------|-------|
| (1)              | deg<br>(2a) | deg<br>(2b) | mag<br>(3) | class<br>(4) | off flg<br>(5) | gal<br>(7a) | TF<br>(7b) | obs<br>(7c) | ext'd<br>(7d) | type<br>(8) |     | (9)                    | Opt<br>(10a) | HI<br>(10b) | flg<br>(11) | flg<br>(12) | flg<br>(13) |       | mag<br>(21)                        | mag<br>(22)                 | mag<br>(23)                 | mag<br>(24)           | (25)                               | mag<br>(26)                          | mag<br>(27)                   | mag<br>(28)                   |       |       |      |       |       |       |       |
| 22072093+4749348 | 96.605      | -6.480      | 0.267      | 1            | -              | -           | g          | -           | -             | D1          | c   | o                      | -            | *           | -           | -           | -           | -     | 11.046                             | 0.38                        | 1.14                        | 1                     | 29.6                               | 0.84                                 | 3.72                          | 10.947                        | 0.34  | 1.01  | 0.08 | 30.0  | 10.96 | 0.34  | 1.02  |
| 22074578+4843504 | 97.195      | -5.789      | 0.368      | 1            | o              | -           | g          | t           | N             | -           | D1  | cp                     | -            | *           | -           | po          | -           | -     | 11.142                             | 0.27                        | 0.94                        | 1                     | 32.0                               | 0.40                                 | 3.82                          | 11.005                        | 0.21  | 0.76  | 0.11 | 32.7  | 11.02 | 0.22  | 0.78  |
| 22080578+6741332 | 108.354     | 9.571       | 0.437      | 1            | -              | -           | g          | -           | -             | D3          | c   | -                      | o            | h           | -           | -           | -           | -     | 11.202                             | 0.29                        | 1.10                        | 1                     | 27.8                               | 0.80                                 | 3.59                          | 11.039                        | 0.22  | 0.88  | 0.14 | 28.5  | 11.05 | 0.23  | 0.91  |
| 22080795+4534167 | 95.377      | -8.383      | 0.347      | 1            | -              | -           | g          | t           | -             | D1          | c   | o                      | o            | -           | -           | -           | -           | -     | 11.361                             | 0.34                        | 1.19                        | 1                     | 40.0                               | 0.44                                 | 3.64                          | 11.232                        | 0.28  | 1.02  | 0.11 | 41.0  | 11.24 | 0.28  | 1.04  |
| 22081281+4800425 | 96.832      | -6.415      | 0.273      | 1            | -              | -           | g          | -           | -             | D3          | c   | o                      | o            | -           | -           | -           | -           | -     | 11.241                             | 0.41                        | 1.15                        | 1                     | 36.0                               | 0.62                                 | 3.71                          | 11.139                        | 0.36  | 1.02  | 0.08 | 36.5  | 11.15 | 0.37  | 1.03  |
| 22082737+4826268 | 97.118      | -6.091      | 0.291      | 1            | -              | -           | g          | -           | -             | D1          | c   | o                      | o            | h           | -           | -           | -           | -     | 8.117                              | 0.28                        | 1.02                        | 1                     | 145.2                              | 0.54                                 | 3.79                          | 8.009                         | 0.24  | 0.88  | 0.09 | 146.9 | 8.02  | 0.24  | 0.90  |
| 22095962+6659580 | 108.091     | 8.903       | 0.671      | 1            | -              | -           | g          | -           | -             | D1          | c   | o                      | o            | -           | -           | -           | -           | -     | 11.454                             | 0.58                        | 1.47                        | 1                     | 28.2                               | 0.76                                 | 3.58                          | 11.204                        | 0.47  | 1.14  | 0.21 | 29.7  | 11.21 | 0.48  | 1.18  |
| 22103166+5535087 | 101.524     | -0.450      | 2.493      | 8            | -              | -           | g          | -           | N             | -           | -   | -                      | -            | -           | -           | U           | -           | -     | 11.852                             | 0.78                        | 1.84                        | 1                     | 29.2                               | 0.64                                 | 4.06                          | 10.923                        | 0.37  | 0.60  | 0.77 | ...   | ...   | 0.42  | 0.76  |
| 22112302+5846598 | 103.453     | 2.103       | 2.143      | 9            | e              | -           | g          | -           | -             | -           | -   | -                      | -            | -           | -           | o           | -           | -     | 11.741                             | 0.56                        | 1.62                        | 1                     | 28.0                               | 0.60                                 | 3.97                          | 10.943                        | 0.20  | 0.56  | 0.66 | ...   | ...   | 0.25  | 0.70  |
| 22113897+4618346 | 96.314      | -8.140      | 0.254      | 1            | -              | -           | g          | -           | -             | D1          | c   | o                      | o            | h           | -           | -           | -           | -     | 10.534                             | 0.36                        | 1.08                        | 1                     | 59.6                               | 0.62                                 | 3.69                          | 10.439                        | 0.31  | 0.96  | 0.08 | 60.5  | 10.45 | 0.32  | 0.97  |
| 22120003+5842576 | 103.480     | 2.002       | 2.279      | 8            | -              | -           | g          | -           | -             | -           | -   | -                      | -            | -           | -           | U           | -           | -     | 10.012                             | 1.20                        | ...                         | 1                     | 67.2                               | 1.00                                 | 4.02                          | 9.163                         | 0.82  | ...   | 0.71 | ...   | ...   | 0.87  | ...   |
| 22123011+4519424 | 95.865      | -9.027      | 0.309      | 1            | -              | -           | g          | t           | -             | D1          | c   | o                      | o            | -           | -           | -           | -           | -     | 10.137                             | 0.31                        | 0.97                        | 1                     | 98.0                               | 0.40                                 | 3.64                          | 10.022                        | 0.26  | 0.82  | 0.10 | 100.0 | 10.03 | 0.26  | 0.84  |
| 22123357+6024561 | 104.509     | 3.358       | 1.479      | 1            | -              | -           | g          | -           | N             | D3          | c   | o                      | o            | h           | *           | -           | -           | -     | 11.302                             | 0.47                        | 1.64                        | 1                     | 31.2                               | 0.44                                 | 3.96                          | 10.751                        | 0.23  | 0.90  | 0.46 | 35.9  | 10.75 | 0.26  | 1.00  |
| 22123749+5858099 | 103.691     | 2.164       | 11.229     | 9            | -              | -           | g          | -           | -             | -           | -   | -                      | -            | -           | -           | -           | -           | -     | 13.187                             | ...                         | ...                         | -1                    | 14.4                               | 1.00                                 | 4.03                          | 9.003                         | ...   | ...   | 3.48 | ...   | ...   | ...   | ...   |
| 22125338+5901050 | 103.747     | 2.185       | 11.727     | 9            | -              | -           | g          | -           | -             | -           | -   | -                      | -            | -           | -           | -           | -           | -     | 9.765                              | 1.18                        | 2.59                        | 1                     | 82.4                               | 0.96                                 | 4.01                          | 5.396                         | -0.76 | -3.24 | 3.63 | ...   | ...   | -0.53 | -2.47 |
| 22125701+5900200 | 103.746     | 2.170       | 11.825     | 9            | -              | -           | g          | -           | -             | -           | -   | -                      | -            | -           | -           | -           | -           | -     | 13.911                             | 0.54                        | ...                         | -1                    | 12.6                               | 0.40                                 | 4.01                          | 9.505                         | -1.42 | ...   | 3.66 | ...   | ...   | -1.18 | ...   |
| 22125779+5858561 | 103.734     | 2.150       | 11.071     | 9            | -              | -           | g          | -           | -             | -           | -   | -                      | -            | -           | -           | -           | -           | -     | 13.395                             | 0.47                        | 1.43                        | 1                     | 17.0                               | 0.74                                 | 4.03                          | 9.270                         | -1.36 | -4.07 | 3.43 | ...   | ...   | -1.14 | -3.34 |
| 22131198+6153077 | 105.411     | 4.522       | 1.123      | 1            | -              | -           | g          | -           | N             | D1          | -   | -                      | -            | h?          | -           | -           | -           | -     | 11.076                             | 0.63                        | 1.68                        | 1                     | 39.4                               | 0.76                                 | 3.92                          | 10.658                        | 0.45  | 1.12  | 0.35 | 44.2  | 10.63 | 0.47  | 1.20  |
| 22131656+5612140 | 102.193     | -0.162      | 1.696      | 8            | -              | -           | g          | -           | -             | -           | -   | -                      | -            | -           | -           | U           | -           | -     | 11.804                             | 0.63                        | 1.76                        | -2                    | 23.4                               | 0.60                                 | 3.99                          | 11.172                        | 0.35  | 0.91  | 0.53 | ...   | ...   | 0.39  | 1.02  |
| 22132686+5030159 | 98.978      | -4.871      | 0.488      | 1            | -              | -           | g          | t           | -             | D1          | e   | o                      | h            | -           | -           | -           | -           | -     | 11.160                             | 0.40                        | 1.31                        | 1                     | 42.0                               | 0.34                                 | 3.84                          | 10.978                        | 0.32  | 1.07  | 0.15 | 43.5  | 10.99 | 0.33  | 1.10  |
| 22134060+6026059 | 104.633     | 3.295       | 1.946      | 1            | -              | -           | g          | -           | N             | D1          | -   | -                      | -            | -           | -           | -           | -           | -     | 11.833                             | 0.70                        | 2.06                        | 1                     | 31.8                               | 0.56                                 | 4.01                          | 11.108                        | 0.38  | 1.10  | 0.60 | 39.8  | 11.05 | 0.42  | 1.22  |
| 22141048+5949118 | 104.336     | 2.753       | 2.432      | 8            | -              | -           | g          | -           | -             | -           | -   | -                      | -            | -           | -           | U           | -           | -     | 9.536                              | 1.35                        | 2.84                        | 1                     | 48.6                               | 0.56                                 | 3.95                          | 8.630                         | 0.95  | 1.63  | 0.75 | ...   | ...   | 1.00  | 1.79  |
| 22143202+6126052 | 105.286     | 4.061       | 5.415      | 9            | -              | -           | g          | -           | -             | -           | -   | -                      | -            | -           | -           | U           | -           | -     | 12.311                             | 1.00                        | 2.16                        | 1                     | 24.2                               | 0.68                                 | 4.01                          | 10.293                        | 0.11  | -0.53 | 1.68 | ...   | ...   | 0.21  | -0.17 |
| 22143934+5902441 | 103.950     | 2.079       | 2.191      | 1            | -              | -           | g          | -           | N             | D3          | -   | -                      | -            | -           | -           | -           | -           | -     | 11.765                             | 0.63                        | 2.07                        | 1                     | 27.8                               | 0.76                                 | 4.00                          | 10.949                        | 0.27  | 0.98  | 0.68 | 36.1  | 10.88 | 0.32  | 1.13  |
| 22143941+6126172 | 105.300     | 4.056       | 5.439      | 9            | -              | -           | g          | -           | -             | -           | -   | -                      | -            | -           | -           | U           | -           | -     | 11.744                             | 0.59                        | 1.68                        | 1                     | 28.2                               | 0.30                                 | 4.01                          | 9.717                         | -0.31 | -1.03 | 1.68 | ...   | ...   | -0.20 | -0.67 |
| 22150528+5849311 | 103.872     | 1.865       | 6.675      | 9            | -              | -           | g          | -           | -             | -           | -   | -                      | -            | -           | -           | -           | -           | -     | 11.437                             | 0.91                        | 2.24                        | 1                     | 73.4                               | 0.24                                 | 4.01                          | 8.950                         | -0.20 | -1.08 | 2.07 | ...   | ...   | -0.07 | -0.64 |
| 22150865+5849157 | 103.876     | 1.858       | 6.605      | 9            | -              | -           | g          | -           | -             | -           | -   | -                      | -            | -           | -           | -           | -           | -     | 8.775                              | 1.45                        | 3.26                        | 1                     | 90.4                               | 0.74                                 | 4.04                          | 6.314                         | 0.36  | -0.03 | 2.05 | ...   | ...   | 0.49  | 0.41  |
| 22160172+5728311 | 103.219     | 0.677       | 1.792      | 9            | -              | -           | g          | -           | -             | -           | -   | -                      | -            | -           | -           | -           | -           | -     | 11.753                             | 1.20                        | 2.03                        | 1                     | 45.6                               | 0.42                                 | 4.08                          | 11.085                        | 0.91  | 1.14  | 0.56 | ...   | ...   | 0.94  | 1.26  |
| 22160870+6005457 | 104.696     | 2.843       | 5.095      | 7            | -              | -           | g          | -           | -             | -           | -   | -                      | -            | -           | -           | -           | -           | -     | 13.094                             | 0.35                        | 1.63                        | -1                    | 14.6                               | 0.84                                 | 3.95                          | 11.196                        | -0.49 | -0.90 | 1.58 | ...   | ...   | -0.39 | -0.56 |
| 22161026+5221220 | 100.376     | -3.581      | 1.463      | 7            | -              | -           | g          | -           | -             | -           | -   | -                      | -            | -           | -           | U           | -           | -     | 9.596                              | 1.30                        | 2.65                        | 1                     | 79.8                               | 0.46                                 | 3.94                          | 9.051                         | 1.06  | 1.93  | 0.45 | ...   | ...   | 1.09  | 2.02  |
| 22161031+5221345 | 100.378     | -3.578      | 1.429      | 8            | -              | -           | g          | -           | -             | -           | -   | -                      | -            | -           | -           | U           | -           | -     | 9.935                              | 1.61                        | 3.04                        | 1                     | 64.2                               | 0.60                                 | 3.90                          | 9.403                         | 1.37  | 2.34  | 0.44 | ...   | ...   | 1.40  | 2.43  |
| 22161783+5152106 | 100.119     | -3.995      | 0.634      | 1            | -              | -           | g          | -           | -             | D1          | e   | o                      | -            | -           | -           | -           | -           | -     | 11.241                             | 0.41                        | 1.41                        | 1                     | 49.6                               | 0.68                                 | 3.92                          | 11.005                        | 0.31  | 1.10  | 0.20 | 52.0  | 11.01 | 0.32  | 1.14  |
| 22162047+6006239 | 104.722     | 2.838       | 5.422      | 9            | -              | -           | g          | -           | -             | -           | -   | -                      | -            | -           | -           | -           | -           | -     | 12.025                             | ...                         | 1.66                        | -2                    | 36.2                               | 1.00                                 | 3.95                          | 10.005                        | ...   | -1.03 | 1.68 | ...   | ...   | ...   | -0.88 |
| 22162074+6006039 | 104.719     | 2.833       | 5.485      | 9            | -              | -           | g          | -           | -             | -           | -   | -                      | -            | -           | -           | -           | -           | -     | 11.308                             | 0.48                        | 1.42                        | -2                    | 40.8                               | 0.78                                 | 3.95                          | 9.264                         | -0.43 | -1.31 | 1.70 | ...   | ...   | -0.32 | -0.95 |
| 22163264+6004419 | 104.727     | 2.800       | 5.446      | 7            | -              | -           | g          | -           | -             | -           | -   | -                      | -            | -           | -           | -           | -           | -     | 10.737                             | 1.31                        | 2.97                        | 1                     | 38.8                               | 0.60                                 | 3.95                          | 8.708                         | 0.41  | 0.27  | 1.69 | ...   | ...   | 0.52  | 0.63  |
| 22165633+5802582 | 103.640     | 1.087       | 2.458      | 8            | -              | -           | g          | -           | -             | -           | -   | -                      | -            | -           | -           | U           | -           | -     | 11.831                             | 0.87                        | 1.55                        | -2                    | 36.8                               | 0.50                                 | 4.04                          | 10.915                        | 0.46  | 0.33  | 0.76 | ...   | ...   | 0.51  | 0.49  |
| 22174625+6155325 | 105.880     | 4.253       | 2.869      | 9            | -              | -           | g          | -           | -             | -           | -   | -                      | -            | -           | -           | -           | -           | -     | 12.075                             | 1.01                        | 2.23                        | 1                     | 59.0                               | 0.28                                 | 3.85                          | 11.006                        | 0.53  | 0.80  | 0.89 | ...   | ...   | 0.59  | 0.99  |
| 22175180+5605538 | 102.663     | -0.607      | 5.802      | 9            | -              | -           | g          | -           | -             | -           | -   | -                      | -            | -           | -           | -           | -           | -     | 10.370                             | 0.87                        | 1.95                        | 1                     | 68.6                               | 0.50                                 | 4.00                          | 8.208                         | -0.09 | -0.93 | 1.80 | ...   | ...   | 0.03  | -0.55 |
| 22180865+5605597 | 102.696     | -0.628      | 6.714      | 8            | -              | -           | g          | -           | -             | -           | -   | -                      | -            | -           | -           | U           | -           | -     | 12.354                             | 0.53                        | 1.42                        | -2                    | 31.0                               | 0.68                                 | 4.00                          | 9.852                         | -0.59 | -1.91 | 2.08 | ...   | ...   | -0.45 | -1.47 |
| 22181990+5610285 | 102.759     | -0.580      | 6.669      | 9            | -              | -           | g          | -           | -             | -           | -   | -                      | -            | -           | -           | -           | -           | -     | 11.465                             | 1.20                        | 2.43                        | 1                     | 34.0                               | 1.00                                 | 4.11                          | 8.980                         | 0.10  | -0.88 | 2.07 | ...   | ...   | 0.23  | -0.44 |
| 22183882+5610566 | 102.800     | -0.597      | 6.560      | 9            | -              | -           | g          | -           | -             | -           | -   | -                      | -            | -           | -           | -           | -           | -     | 10.696                             | 0.61                        | 1.50                        | 1                     | 83.2                               | 0.42                                 | 4.11                          | 8.252                         | -0.48 | -1.76 | 2.03 | ...   | ...   | -0.35 | -1.33 |
| 22185358+4458012 | 96.598      | -9.964      | 0.356      | 1            | -              | -           | g          | -           | -             | D3          | c   | o                      | -            | -           | -           | -           | -           | -     | 11.354                             | 0.35                        | 1.19                        | 1                     | 22.4                               | 0.64                                 | 3.50                          | 11.221                        | 0.29  | 1.02  | 0.11 | 22.8  | 11.23 | 0.30  | 1.04  |
| 22185689+5607386 | 102.805     | -0.666      | 6.632      | 9            | -              | -           | g          | -           | -             | -           | -   | -                      | -            | -           | -           | -           | -           | -     | 12.413                             | 0.35                        | 1.01                        | 1                     | 23.4                               | 0.12                                 | 4.11                          | 9.942                         | -0.75 | -2.29 | 2.05 | ...   | ...   | -0.62 | -1.85 |
| 22190240+6319150 | 106.776     | 5.335       | 5.159      | 9            | -              | -           | g          | -           | -             | -           | -   | -                      | -            | -           | -           | -           | -           | -     | 11.876                             | ...                         | ...                         | 1                     | 31.4                               | 1.00                                 | 3.93                          | 9.954                         | ...   | ...   | 1.60 | ...   | ...   | ...   | ...   |
| 22190403+6136110 | 105.829     | 3.900       | 2.450      | 8            | -              | -           | g          |             |               |             |     |                        |              |             |             |             |             |       |                                    |                             |                             |                       |                                    |                                      |                               |                               |       |       |      |       |       |       |       |

Table B1: a) continued.

| 2MSS J            | <i>l</i><br>deg<br>(2a) | <i>b</i><br>deg<br>(2b) | EBV<br>mag<br>(3) | Object<br>class<br>(4) | off<br>(5) | flg<br>(6) | gal<br>(7a) | TF<br>(7b) | obs<br>(7c) | ext'd<br>(7d) | Disc<br>type<br>(8) | 2MRS<br>(9) | Velocity<br>Opt<br>(10a) | HI<br>(10b) | NIR<br>flg<br>(11) | Photom<br>flg<br>(12) | Ext<br>flg<br>(13) | <i>K</i> <sub>20</sub><br>mag<br>(14) | <i>H-K</i><br>mag<br>(15) | <i>J-K</i><br>mag<br>(16) | vc<br>(17) | <i>a</i><br>" (18) | <i>b/a</i><br>(19) | std.d.<br>(20) | <i>K</i> <sub>S</sub> <sup>o</sup><br>mag<br>(21) | ( <i>H-K</i> ) <sup>o</sup><br>mag<br>(22) | ( <i>J-K</i> ) <sup>o</sup><br>mag<br>(23) | <i>A<sub>K</sub></i><br>mag<br>(24) | <i>a</i> <sup>d</sup><br>" (25) | <i>K</i> <sub>S</sub> <sup>d</sup><br>mag<br>(26) | ( <i>H-K</i> ) <sup>o,c</sup><br>mag<br>(27) | ( <i>J-K</i> ) <sup>o,c</sup><br>mag<br>(28) |       |
|-------------------|-------------------------|-------------------------|-------------------|------------------------|------------|------------|-------------|------------|-------------|---------------|---------------------|-------------|--------------------------|-------------|--------------------|-----------------------|--------------------|---------------------------------------|---------------------------|---------------------------|------------|--------------------|--------------------|----------------|---------------------------------------------------|--------------------------------------------|--------------------------------------------|-------------------------------------|---------------------------------|---------------------------------------------------|----------------------------------------------|----------------------------------------------|-------|
| 22282106+6414125  | 108.142                 | 5.555                   | 1.538             | 8                      | -          | -          | -           | -          | -           | -             | -                   | -           | g                        | -           | -                  | -                     | -                  | -                                     | 9.465                     | 1.38                      | 2.87       | 1                  | 34.6               | 0.72           | 3.83                                              | 8.892                                      | 1.13                                       | 2.10                                | 0.48                            | ...                                               | ...                                          | 1.16                                         | 2.21  |
| 22282804+6259265  | 107.500                 | 4.485                   | 3.166             | 9                      | -          | -          | -           | -          | -           | -             | -                   | -           | -                        | -           | -                  | -                     | -                  | -                                     | 9.244                     | 2.55                      | ...        | 1                  | 123.2              | 0.46           | 3.85                                              | 8.064                                      | 2.03                                       | ...                                 | 0.98                            | ...                                               | ...                                          | 2.09                                         | ...   |
| 22282952+6300105  | 107.509                 | 4.484                   | 3.256             | 9                      | -          | -          | -           | -          | -           | -             | -                   | -           | -                        | -           | -                  | -                     | -                  | -                                     | 10.905                    | ...                       | ...        | 1                  | 61.8               | 0.48           | 3.85                                              | 9.692                                      | ...                                        | ...                                 | 1.01                            | ...                                               | ...                                          | ...                                          | ...   |
| 22283401+6139086  | 106.811                 | 3.337                   | 2.623             | 8                      | -          | -          | -           | -          | -           | -             | -                   | -           | -                        | -           | -                  | -                     | -                  | -                                     | 11.311                    | 1.52                      | 3.22       | 1                  | 16.8               | 0.68           | 3.90                                              | 10.334                                     | 1.09                                       | 1.92                                | 0.81                            | ...                                               | ...                                          | 1.14                                         | 2.09  |
| 22284705+5102560  | 101.317                 | -5.736                  | 0.304             | 1                      | -          | -          | g           | -          | -           | -             | D2                  | c           | o                        | -           | -                  | -                     | -                  | -                                     | 10.430                    | 0.32                      | 1.09       | 1                  | 48.0               | 0.78           | 3.80                                              | 10.317                                     | 0.27                                       | 0.94                                | 0.09                            | 48.8                                              | 10.33                                        | 0.28                                         | 0.96  |
| 22285070+6413468  | 108.184                 | 5.521                   | 1.516             | 8                      | -          | -          | -           | -          | -           | -             | -                   | -           | -                        | -           | -                  | -                     | -                  | -                                     | 10.182                    | 2.01                      | ...        | 1                  | 104.2              | 0.28           | 3.80                                              | 9.617                                      | 1.76                                       | ...                                 | 0.47                            | ...                                               | ...                                          | 1.79                                         | ...   |
| 22285960+6413059  | 108.192                 | 5.503                   | 1.512             | 9                      | -          | -          | -           | -          | -           | -             | -                   | -           | -                        | -           | -                  | -                     | e                  | -                                     | 11.336                    | 0.91                      | 2.20       | 1                  | 61.8               | 0.22           | 3.80                                              | 10.773                                     | 0.66                                       | 1.45                                | 0.47                            | ...                                               | ...                                          | 0.69                                         | 1.55  |
| 22291029+6451069  | 108.540                 | 6.034                   | 2.430             | 6                      | -          | -          | -           | -          | -           | -             | -                   | -           | -                        | -           | -                  | -                     | -                  | -                                     | 11.099                    | 0.68                      | 2.24       | 1                  | 19.6               | 0.72           | 3.81                                              | 10.194                                     | 0.28                                       | 1.03                                | 0.75                            | ...                                               | ...                                          | 0.32                                         | 1.19  |
| 22293596+5051428  | 101.329                 | -5.963                  | 0.279             | 1                      | -          | -          | g           | -          | -           | -             | -                   | c           | o                        | -           | -                  | -                     | -                  | -                                     | 10.520                    | 0.33                      | 1.16       | 1                  | 42.4               | 0.84           | 3.83                                              | 10.416                                     | 0.29                                       | 1.02                                | 0.09                            | 43.0                                              | 10.43                                        | 0.29                                         | 1.04  |
| 22300095+5848477  | 105.494                 | 0.815                   | 1.861             | 1                      | -          | -          | -           | -          | N           | -             | n                   | -           | -                        | -           | -                  | U                     | -                  | -                                     | 11.857                    | 0.71                      | 2.10       | 1                  | 22.8               | 0.92           | 3.99                                              | 11.164                                     | 0.40                                       | 1.18                                | 0.58                            | 28.1                                              | 11.12                                        | 0.44                                         | 1.30  |
| 22301207+5105365  | 101.531                 | -5.814                  | 0.309             | 1                      | -          | -          | g           | -          | -           | -             | D1                  | c           | o                        | -           | -                  | -                     | -                  | -                                     | 11.119                    | 0.33                      | 1.17       | 1                  | 43.8               | 0.78           | 3.77                                              | 11.004                                     | 0.28                                       | 1.02                                | 0.10                            | 44.6                                              | 11.01                                        | 0.29                                         | 1.04  |
| 22303038+6152498  | 107.126                 | 3.414                   | 1.429             | 1                      | -          | -          | g           | t          | -           | -             | D1                  | e           | o                        | -           | h                  | -                     | -                  | -                                     | 9.661                     | 0.54                      | 1.62       | 1                  | 103.0              | 0.30           | 3.99                                              | 9.125                                      | 0.30                                       | 0.92                                | 0.44                            | 117.5                                             | 9.13                                         | 0.33                                         | 1.01  |
| 22305378+5248352  | 102.512                 | -4.308                  | 0.405             | 1                      | -          | -          | g           | -          | -           | -             | D1                  | e           | o                        | -           | -                  | U                     | -                  | -                                     | 11.033                    | 0.31                      | 1.05       | 1                  | 30.8               | 0.60           | 3.85                                              | 10.852                                     | 0.39                                       | 1.11                                | 0.13                            | 31.5                                              | 10.87                                        | 0.30                                         | 1.14  |
| 22311630+5206373  | 102.201                 | -5.028                  | 0.247             | 1                      | -          | -          | g           | -          | -           | -             | D1                  | c           | o                        | -           | -                  | U                     | -                  | -                                     | 10.800                    | 0.32                      | 1.12       | 1                  | 44.4               | 0.66           | 3.79                                              | 10.708                                     | 0.28                                       | 0.99                                | 0.08                            | 45.0                                              | 10.72                                        | 0.28                                         | 1.01  |
| 22312526+6541229  | 109.179                 | 6.629                   | 3.422             | 8                      | -          | -          | -           | -          | -           | -             | -                   | -           | -                        | -           | -                  | -                     | -                  | -                                     | 11.579                    | 1.06                      | 2.47       | 1                  | 32.8               | 0.64           | 3.67                                              | 10.304                                     | 0.49                                       | 0.77                                | 1.06                            | ...                                               | ...                                          | 0.56                                         | 1.00  |
| 22322397+5818579  | 105.507                 | 0.229                   | 2.883             | 7                      | -          | -          | -           | -          | -           | -             | -                   | -           | -                        | -           | -                  | U                     | -                  | -                                     | 9.463                     | 1.38                      | 2.84       | 1                  | 30.8               | 0.64           | 4.05                                              | 8.389                                      | 0.90                                       | 1.40                                | 0.89                            | ...                                               | ...                                          | 0.96                                         | 1.59  |
| 22322412+5819111  | 105.509                 | 0.232                   | 2.934             | 8                      | -          | -          | -           | -          | -           | -             | -                   | -           | -                        | -           | -                  | U                     | -                  | -                                     | 8.977                     | 1.15                      | 2.56       | 1                  | 107.8              | 0.38           | 4.07                                              | 7.884                                      | 0.67                                       | 1.10                                | 0.91                            | ...                                               | ...                                          | 0.72                                         | 1.29  |
| 22323008+5832162  | 105.631                 | 0.413                   | 7.175             | 7                      | -          | -          | -           | -          | -           | -             | -                   | -           | -                        | -           | -                  | U                     | -                  | -                                     | 11.124                    | 1.05                      | 2.67       | 1                  | 18.4               | 0.68           | 3.99                                              | 8.451                                      | -0.14                                      | -0.89                               | 2.22                            | ...                                               | ...                                          | 0.00                                         | -0.42 |
| 22323043+5822262  | 105.549                 | 0.271                   | 3.758             | 7                      | -          | -          | -           | -          | -           | -             | -                   | -           | -                        | -           | -                  | U                     | -                  | -                                     | 12.184                    | 0.88                      | ...        | 1                  | 19.2               | 0.44           | 4.07                                              | 10.784                                     | 0.26                                       | ...                                 | 1.16                            | ...                                               | ...                                          | 0.33                                         | ...   |
| 22324440+5828143  | 105.624                 | 0.339                   | 9.476             | 8                      | -          | -          | -           | -          | -           | -             | -                   | -           | -                        | -           | -                  | U                     | -                  | -                                     | 7.879                     | 1.42                      | 2.49       | 1                  | 125.4              | 0.76           | 3.99                                              | 4.348                                      | -0.15                                      | -2.21                               | 2.94                            | ...                                               | ...                                          | 0.03                                         | -1.59 |
| 22330362+5147457  | 102.278                 | -5.439                  | 0.273             | 1                      | -          | -          | g           | -          | -           | -             | D3                  | c           | o                        | -           | -                  | U                     | -                  | -                                     | 10.734                    | 0.29                      | 1.08       | 1                  | 36.4               | 0.76           | 3.78                                              | 10.632                                     | 0.24                                       | 0.95                                | 0.08                            | 36.9                                              | 10.64                                        | 0.25                                         | 0.96  |
| 22333889+5110463  | 102.043                 | -6.017                  | 0.240             | 1                      | -          | -          | g           | -          | N           | -             | D1                  | c           | o                        | -           | h?                 | -                     | U                  | -                                     | 10.884                    | 0.36                      | 1.09       | 1                  | 43.0               | 0.64           | 3.81                                              | 10.795                                     | 0.32                                       | 0.97                                | 0.07                            | 43.5                                              | 10.80                                        | 0.32                                         | 0.99  |
| 22333896+5831552  | 105.757                 | 0.332                   | 2.781             | 9                      | -          | -          | -           | -          | -           | -             | -                   | -           | -                        | -           | -                  | -                     | -                  | -                                     | 11.985                    | 0.75                      | 1.78       | 1                  | 25.6               | 0.86           | 3.98                                              | 10.949                                     | 0.29                                       | 0.40                                | 0.86                            | ...                                               | ...                                          | 0.35                                         | 0.58  |
| 22340404+6826298  | 110.821                 | 8.863                   | 0.709             | 1                      | -          | -          | g           | t          | -           | -             | D1                  | c           | o                        | -           | h                  | -                     | U                  | -                                     | 10.117                    | 0.39                      | 1.22       | 1                  | 78.6               | 0.40           | 3.56                                              | 9.853                                      | 0.27                                       | 0.86                                | 0.22                            | 82.5                                              | 9.87                                         | 0.28                                         | 0.91  |
| 22341089+5833513  | 105.834                 | 0.325                   | 2.307             | 8                      | -          | -          | -           | -          | -           | -             | -                   | -           | -                        | -           | -                  | U                     | -                  | -                                     | 11.239                    | 0.65                      | 1.85       | -2                 | 41.0               | 0.76           | 4.01                                              | 10.379                                     | 0.27                                       | 0.71                                | 0.71                            | ...                                               | ...                                          | 0.31                                         | 0.86  |
| 22342113+5759454  | 105.568                 | -0.178                  | 1.119             | 1                      | -          | -          | g           | -          | N           | -             | D2                  | c           | o                        | -           | -                  | U                     | -                  | -                                     | 9.452                     | 0.45                      | 1.52       | 1                  | 73.0               | 0.70           | 4.02                                              | 9.035                                      | 0.26                                       | 0.97                                | 0.35                            | 79.6                                              | 9.06                                         | 0.29                                         | 1.04  |
| 22342433+5026356  | 101.772                 | -6.713                  | 0.222             | 1                      | -          | -          | g           | -          | -           | -             | D4                  | c           | o                        | -           | -                  | U                     | -                  | -                                     | 9.837                     | 0.31                      | 1.06       | 1                  | 62.2               | 0.74           | 3.71                                              | 9.754                                      | 0.27                                       | 0.95                                | 0.07                            | 62.8                                              | 9.76                                         | 0.28                                         | 0.96  |
| 22342747+5919524  | 106.249                 | 0.971                   | 5.028             | 8                      | -          | -          | -           | -          | -           | -             | -                   | -           | -                        | -           | -                  | U                     | -                  | -                                     | 10.572                    | 0.60                      | 1.72       | -2                 | 38.4               | 0.98           | 3.98                                              | 8.699                                      | -0.23                                      | -0.78                               | 1.56                            | ...                                               | ...                                          | -0.14                                        | -0.45 |
| 22344034+5842443  | 105.963                 | 0.421                   | 2.271             | 9                      | -          | -          | -           | -          | -           | -             | -                   | -           | -                        | -           | -                  | U                     | -                  | -                                     | 11.111                    | 0.72                      | 1.60       | -2                 | 39.4               | 0.78           | 4.01                                              | 10.265                                     | 0.34                                       | 0.48                                | 0.70                            | ...                                               | ...                                          | 0.39                                         | 0.63  |
| 22344788+5010038  | 101.687                 | -6.982                  | 0.196             | 1                      | -          | -          | g           | t          | N           | -             | D1                  | c           | o                        | -           | -                  | U                     | -                  | -                                     | 11.085                    | 0.36                      | 1.11       | 1                  | 57.0               | 0.32           | 3.78                                              | 11.012                                     | 0.33                                       | 1.01                                | 0.06                            | 57.6                                              | 11.02                                        | 0.33                                         | 1.03  |
| 22350086+5824467  | 105.852                 | 0.140                   | 2.968             | 7                      | -          | -          | -           | -          | -           | -             | -                   | -           | -                        | -           | -                  | U                     | -                  | -                                     | 10.023                    | 0.93                      | 1.75       | 1                  | 44.0               | 0.98           | 3.98                                              | 8.917                                      | 0.44                                       | 0.28                                | 0.92                            | ...                                               | ...                                          | 0.50                                         | 0.48  |
| 22351757+5759528  | 105.677                 | -0.238                  | 1.487             | 8                      | -          | -          | -           | -          | -           | -             | -                   | -           | -                        | -           | -                  | U                     | -                  | -                                     | 10.894                    | 0.74                      | 1.86       | -2                 | 55.8               | 0.52           | 4.01                                              | 10.340                                     | 0.49                                       | 1.13                                | 0.46                            | ...                                               | ...                                          | 0.52                                         | 1.22  |
| 22352646+6048150  | 107.291                 | 2.186                   | 1.750             | 1                      | -          | -          | g           | t          | N           | -             | D1                  | c           | o                        | -           | *                  | -                     | U                  | -                                     | 10.840                    | 0.59                      | 1.72       | 1                  | 36.0               | 0.66           | 3.95                                              | 10.188                                     | 0.30                                       | 0.85                                | 0.54                            | 42.8                                              | 10.18                                        | 0.33                                         | 0.97  |
| 22353369+5103093  | 102.240                 | -6.278                  | 0.245             | 1                      | -          | -          | g           | -          | -           | -             | D1                  | c           | o                        | -           | -                  | U                     | -                  | -                                     | 11.111                    | 0.32                      | 1.06       | 1                  | 36.2               | 0.82           | 3.79                                              | 11.020                                     | 0.28                                       | 0.93                                | 0.08                            | 36.7                                              | 11.03                                        | 0.28                                         | 0.95  |
| 22355416+5919102  | 106.403                 | 0.869                   | 2.575             | 8                      | -          | -          | g           | -          | -           | -             | -                   | -           | -                        | -           | -                  | U                     | -                  | -                                     | 12.067                    | 1.07                      | 2.22       | 1                  | 31.6               | 0.60           | 3.89                                              | 11.108                                     | 0.65                                       | 0.94                                | 0.80                            | ...                                               | ...                                          | 0.70                                         | 1.11  |
| 22361232+5920192  | 106.446                 | 0.867                   | 2.837             | 7                      | -          | -          | -           | -          | -           | -             | -                   | -           | -                        | -           | -                  | U                     | -                  | -                                     | 10.932                    | ...                       | 2.81       | 1                  | 25.6               | 1.00           | 3.89                                              | 9.875                                      | ...                                        | 1.40                                | 0.88                            | ...                                               | ...                                          | ...                                          | 1.59  |
| 22362006+5924572  | 106.498                 | 0.925                   | 4.267             | 8                      | -          | -          | -           | -          | -           | -             | -                   | -           | -                        | -           | -                  | U                     | -                  | -                                     | 11.131                    | 1.31                      | 3.01       | 1                  | 49.2               | 0.76           | 3.89                                              | 9.541                                      | 0.61                                       | 0.89                                | 1.32                            | ...                                               | ...                                          | 0.69                                         | 1.17  |
| 22370933+5358339  | 103.909                 | -3.861                  | 0.681             | 1                      | -          | -          | g           | t          | -           | -             | D1                  | e           | o                        | -           | h                  | -                     | U                  | -                                     | 11.252                    | 0.41                      | 1.30       | 1                  | 45.2               | 0.52           | 3.88                                              | 10.998                                     | 0.29                                       | 0.96                                | 0.21                            | 48.0                                              | 10.99                                        | 0.31                                         | 1.01  |
| 22371234+5214386  | 103.057                 | -5.371                  | 0.310             | 1                      | -          | -          | o           | -          | N           | -             | D1                  | c           | o                        | -           | -                  | U                     | -                  | -                                     | 11.205                    | 0.29                      | 0.99       | 1                  | 48.2               | 0.48           | 3.80                                              | 11.089                                     | 0.24                                       | 0.84                                | 0.10                            | 49.1                                              | 11.10                                        | 0.24                                         | 0.86  |
| 22382102+5031104  | 102.359                 | -6.959                  | 0.225             | 1                      | -          | -          | g           | -          | -           | *             | D1                  | c           | o                        | -           | -                  | U                     | -                  | -                                     | 11.328                    | 0.51                      | 1.27       | 1                  | 33.6               | 0.72           | 3.66                                              | 11.244                                     | 0.47                                       | 1.15                                | 0.07                            | 34.0                                              | 11.25                                        | 0.48                                         | 1.17  |
| 22382576+56553037 | 105.495                 | -1.415                  | 1.040             | 9                      | -          | -          | -           | -          | -           | -             | -                   | -           | -                        | -           | -                  | -                     | -                  | -                                     | 11.314                    | ...                       | ...        | -2                 | 56.2               | 1.00           | 3.95                                              | 10.926                                     | ...                                        | ...                                 | 0.32                            | ...                                               | ...                                          | ...                                          | ...   |
| 22391220+6415330  | 109.175                 | 4.979                   | 1.750             | 8                      | -          | -          | -           | -          | -           | -             | -                   | -           | -                        | -           | -                  | -                     | -                  | -                                     | 10.750                    | 1.47                      | 2.85       | 1                  | 19.8               | 0.92           | 3.87                                              | 10.280                                     | 1.26                                       | 2.22                                | 0.39                            | ...                                               | ...                                          | 1.29                                         | 2.30  |
| 22402082+6117062  | 107.845                 | 2.314                   | 2.291             | 9                      | -          | -          | p           | -          | -           | -             | -                   | -           | -                        | -           | -                  | -                     | -                  | -                                     | 9.450                     | 0.91                      | 1.29       | 1                  | 55.0               | 0.78           | 3.94                                              | 8.596                                      | 0.53                                       | 0.15                                | 0.71                            | ...                                               | ...                                          | 0.57                                         | 0.30  |
| 22410583+5142164  | 103.319                 | -6.134                  | 0.281             | 1                      | -          | -          | g           | -          | -           | -             | D3                  | c           | o                        | -           | -                  | U                     | -                  | -                                     | 11.105                    | 0.35                      | 1.16       | 1                  | 28.4               | 0.64           | 3.75                                              | 11.000                                     | 0.30                                       | 1.02                                | 0.09                            | 28.8                                              | 11.01                                        | 0.31                                         | 1.04  |
| 22433663+5928141  | 107.335                 | 0.527                   | 2.276             | 8                      | -          | -          | -           | -          | -           | -             | -                   | -           | -                        | -           | -                  | U                     | -                  | -                                     | 11.914                    | 0.37                      | 1.27       | 1                  | 13.8               | 0.68           | 3.9                                               |                                            |                                            |                                     |                                 |                                                   |                                              |                                              |       |

2M-ZoA galaxy catalogue description and analysis 117

Table B1: a) continued.

| 2MASX J          | <i>l</i> | <i>b</i> | EBV    | Object | Sample | Disc | 2MRS | Velocity | NIR  | Photom | Ext  | <i>K</i> <sub>20</sub> | <i>H-K</i> | <i>J-K</i> | vc   | <i>a</i> | <i>b/a</i> | st.d. | <i>K</i> <sub>s</sub> <sup>o</sup> | ( <i>H-K</i> ) <sup>o</sup> | ( <i>J-K</i> ) <sup>o</sup> | <i>A<sub>K</sub></i> | <i>a</i> <sub>d</sub> <sup>o</sup> | <i>K</i> <sub>s</sub> <sup>o,d</sup> | ( <i>H-K</i> ) <sup>o,c</sup> | ( <i>J-K</i> ) <sup>o,c</sup> |        |        |       |      |       |        |        |     |
|------------------|----------|----------|--------|--------|--------|------|------|----------|------|--------|------|------------------------|------------|------------|------|----------|------------|-------|------------------------------------|-----------------------------|-----------------------------|----------------------|------------------------------------|--------------------------------------|-------------------------------|-------------------------------|--------|--------|-------|------|-------|--------|--------|-----|
| (1)              | deg      | deg      | mag    | class  | off    | flag | gal  | TF       | obs  | ext'd  | type | (9)                    | Opt        | HI         | flag | flag     | flag       | flag  | mag                                | mag                         | mag                         | mag                  | mag                                | mag                                  | mag                           | mag                           | mag    |        |       |      |       |        |        |     |
| (1)              | (2a)     | (2b)     | (3)    | (4)    | (5)    | (6)  | (7a) | (7b)     | (7c) | (7d)   | (8)  | (9)                    | (10a)      | (10b)      | (11) | (12)     | (13)       | (14)  | (15)                               | (16)                        | (17)                        | (18)                 | (19)                               | (20)                                 | (21)                          | (22)                          | (23)   | (24)   | (25)  | (26) | (27)  | (28)   |        |     |
| 22555978+5814424 | 108.212  | -1.288   | 3.079  | 8      | -      | -    | -    | -        | -    | -      | -    | -                      | -          | -          | -    | -        | -          | -     | 8.374                              | 1.27                        | 2.72                        | 1                    | 110.4                              | 0.60                                 | 3.94                          | 7.227                         | 0.76   | 1.19   | 0.95  | ...  | ...   | 0.82   | 1.39   |     |
| 22560350+6202554 | 109.853  | 2.143    | 46.527 | 9      | -      | -    | -    | -        | -    | -      | -    | -                      | -          | -          | -    | -        | -          | -     | 9.459                              | 1.12                        | 2.21                        | 1                    | 90.2                               | 0.78                                 | 4.01                          | -7.877                        | -6.58  | -20.91 | 14.41 | ...  | ...   | -5.67  | -17.84 |     |
| 22560422+6200184 | 109.836  | 2.103    | 39.749 | 9      | -      | -    | -    | -        | -    | -      | -    | -                      | -          | -          | -    | -        | -          | -     | 0.89                               | 2.59                        | 1                           | 97.0                 | 0.64                               | 3.89                                 | -7.735                        | -5.69                         | -17.16 | 12.31  | ...   | ...  | -4.91 | -14.54 |        |     |
| 22560492+6201264 | 109.845  | 2.120    | 47.128 | 9      | -      | -    | -    | -        | -    | -      | -    | -                      | -          | -          | -    | -        | -          | -     | 9.100                              | 0.68                        | 1.87                        | 1                    | 95.4                               | 0.28                                 | 4.01                          | -8.460                        | -7.13  | -21.54 | 14.60 | ...  | ...   | -6.20  | -18.43 |     |
| 22560522+6200384 | 109.840  | 2.107    | 42.818 | 9      | -      | -    | -    | -        | -    | -      | -    | -                      | -          | -          | -    | -        | -          | -     | 10.274                             | 1.25                        | ...                         | 1                    | 71.2                               | 0.40                                 | 4.01                          | -5.680                        | -5.84  | ...    | 13.26 | ...  | ...   | -5.00  | ...    |     |
| 22560592+6201554 | 109.850  | 2.126    | 47.634 | 9      | -      | -    | -    | -        | -    | -      | -    | -                      | -          | -          | -    | -        | -          | -     | 8.773                              | 1.05                        | 2.16                        | 1                    | 97.8                               | 0.90                                 | 4.01                          | -8.975                        | -6.84  | -21.51 | 14.75 | ...  | ...   | -5.90  | -18.37 |     |
| 22560891+6200444 | 109.847  | 2.106    | 45.696 | 8      | -      | -    | -    | -        | -    | -      | -    | -                      | -          | -          | -    | -        | -          | -     | 11.021                             | 1.47                        | 3.21                        | 1                    | 36.8                               | 0.66                                 | 4.01                          | -6.005                        | -6.10  | -19.49 | 14.15 | ...  | ...   | -5.20  | -16.48 |     |
| 22560905+6200514 | 109.848  | 2.107    | 46.521 | 8      | -      | -    | -    | -        | -    | -      | -    | -                      | -          | -          | -    | -        | -          | -     | 12.213                             | 1.54                        | ...                         | 1                    | 20.8                               | 1.00                                 | 3.89                          | -5.121                        | -6.16  | ...    | 14.41 | ...  | ...   | -5.25  | ...    |     |
| 22561275+5831223 | 108.357  | -1.050   | 7.480  | 9      | -      | -    | -    | -        | -    | -      | -    | -                      | -          | -          | -    | -        | -          | -     | 10.392                             | ...                         | 2.57                        | 1                    | 80.4                               | 1.00                                 | 3.99                          | 7.605                         | ...    | -1.15  | 2.32  | ...  | ...   | ...    | -0.65  | ... |
| 22561302+6202424 | 109.869  | 2.132    | 52.656 | 7      | -      | -    | -    | -        | -    | -      | -    | -                      | -          | -          | -    | -        | -          | -     | 11.145                             | 1.46                        | ...                         | 1                    | 40.2                               | 0.78                                 | 4.01                          | -8.475                        | -7.26  | ...    | 16.31 | ...  | ...   | -6.23  | ...    |     |
| 22561331+6201494 | 109.863  | 2.118    | 50.557 | 9      | -      | -    | -    | -        | -    | -      | -    | -                      | -          | -          | -    | -        | -          | -     | 7.968                              | 1.55                        | ...                         | 1                    | 166.0                              | 0.22                                 | 4.01                          | -10.870                       | -6.83  | ...    | 15.66 | ...  | ...   | -5.84  | ...    |     |
| 22561351+5915033 | 108.671  | -0.393   | 2.705  | 7      | -      | -    | -    | -        | -    | -      | -    | -                      | -          | -          | -    | -        | -          | -     | 11.975                             | 0.93                        | ...                         | 1                    | 28.2                               | 1.00                                 | 3.95                          | 10.967                        | 0.48   | ...    | 0.84  | ...  | ...   | 0.54   | ...    |     |
| 22561365+5915093 | 108.672  | -0.391   | 2.716  | 8      | -      | -    | -    | -        | -    | -      | -    | -                      | -          | -          | -    | -        | -          | -     | 11.681                             | 0.92                        | 2.54                        | 1                    | 35.6                               | 0.38                                 | 3.99                          | 10.669                        | 0.47   | 1.19   | 0.84  | ...  | ...   | 0.52   | 1.37   |     |
| 22561631+5830380 | 108.359  | -1.064   | 7.618  | 8      | -      | -    | -    | -        | -    | -      | -    | -                      | -          | -          | -    | -        | -          | -     | 12.428                             | 0.63                        | 1.45                        | 1                    | 30.4                               | 0.62                                 | 4.01                          | 9.590                         | -0.63  | -2.33  | 2.36  | ...  | ...   | -0.48  | -1.83  |     |
| 22561722+5831183 | 108.365  | -1.055   | 7.986  | 9      | -      | -    | -    | -        | -    | -      | -    | -                      | -          | -          | -    | -        | -          | -     | 8.598                              | 0.54                        | 1.17                        | 1                    | 44.0                               | 0.76                                 | 3.99                          | 5.622                         | -0.79  | -2.79  | 2.47  | ...  | ...   | -0.63  | -2.27  |     |
| 22562212+6202024 | 109.880  | 2.114    | 55.063 | 9      | -      | -    | -    | -        | -    | -      | -    | -                      | -          | -          | -    | -        | -          | -     | 5.794                              | 1.92                        | 4.28                        | 1                    | 192.2                              | 0.76                                 | 4.01                          | -14.722                       | -7.20  | -23.07 | 17.06 | ...  | ...   | -6.12  | -19.44 |     |
| 22562270+6202504 | 109.887  | 2.126    | 57.183 | 9      | -      | -    | -    | -        | -    | -      | -    | -                      | -          | -          | -    | -        | -          | -     | 7.426                              | 3.34                        | ...                         | 1                    | 151.0                              | 0.24                                 | 4.01                          | -13.880                       | -6.12  | ...    | 17.71 | ...  | ...   | -5.00  | ...    |     |
| 22562284+5831122 | 108.376  | -1.062   | 8.504  | 9      | -      | -    | -    | -        | -    | -      | -    | -                      | -          | -          | -    | -        | -          | -     | 11.899                             | 0.80                        | 1.86                        | 1                    | 49.2                               | 0.42                                 | 3.99                          | 8.730                         | -0.61  | -2.37  | 2.63  | ...  | ...   | -0.44  | -1.81  |     |
| 22562326+6201204 | 109.877  | 2.103    | 52.397 | 9      | -      | -    | -    | -        | -    | -      | -    | -                      | -          | -          | -    | -        | -          | -     | 10.205                             | 1.43                        | ...                         | 1                    | 77.6                               | 1.00                                 | 4.01                          | -9.318                        | -7.25  | ...    | 16.23 | ...  | ...   | -6.22  | ...    |     |
| 22562383+6201014 | 109.876  | 2.097    | 51.148 | 9      | -      | -    | -    | -        | -    | -      | -    | -                      | -          | -          | -    | -        | -          | -     | 11.029                             | 1.29                        | ...                         | 1                    | 62.0                               | 0.52                                 | 3.89                          | -8.029                        | -7.18  | ...    | 15.84 | ...  | ...   | -6.18  | ...    |     |
| 22563009+5831232 | 108.391  | -1.066   | 7.412  | 9      | -      | -    | -    | -        | -    | -      | -    | -                      | -          | -          | -    | -        | -          | -     | 13.322                             | 0.26                        | 1.08                        | 2                    | 13.0                               | 1.00                                 | 4.01                          | 10.560                        | -0.97  | -2.60  | 2.30  | ...  | ...   | -0.82  | -2.11  |     |
| 22563236+6202154 | 109.900  | 2.109    | 47.665 | 9      | -      | -    | -    | -        | -    | -      | -    | -                      | -          | -          | -    | -        | -          | -     | 6.423                              | 1.80                        | 3.88                        | 1                    | 202.2                              | 0.58                                 | 4.01                          | -11.337                       | -6.09  | -19.80 | 14.76 | ...  | ...   | -5.15  | -16.65 |     |
| 22563322+6203124 | 109.908  | 2.123    | 50.657 | 9      | -      | -    | -    | -        | -    | -      | -    | -                      | -          | -          | -    | -        | -          | -     | 8.095                              | 1.68                        | 3.15                        | 1                    | 109.8                              | 0.62                                 | 4.01                          | -10.780                       | -6.71  | -22.01 | 15.69 | ...  | ...   | -5.72  | -18.67 |     |
| 22564579+5830003 | 108.412  | -1.101   | 4.819  | 9      | -      | -    | -    | -        | -    | -      | -    | -                      | -          | -          | -    | -        | -          | -     | 10.770                             | 1.38                        | ...                         | 1                    | 63.2                               | 0.40                                 | 4.01                          | 8.974                         | 0.58   | ...    | 1.49  | ...  | ...   | 0.68   | ...    |     |
| 22565321+5352372 | 106.448  | -5.288   | 0.448  | 1      | -      | -    | g    | t        | -    | -      | D1   | c                      | o          | h          | U    | -        | -          | -     | 11.115                             | 0.44                        | 1.33                        | 1                    | 45.6                               | 0.32                                 | 3.76                          | 10.948                        | 0.37   | 1.11   | 0.14  | 47.0 | 10.96 | 0.38   | 1.14   |     |
| 22565704+6234018 | 110.169  | 2.567    | 11.506 | 7      | -      | -    | -    | -        | -    | -      | -    | -                      | -          | -          | -    | -        | -          | -     | 12.806                             | ...                         | ...                         | 1                    | 20.0                               | 1.00                                 | 4.17                          | 8.519                         | ...    | ...    | 3.56  | ...  | ...   | ...    | ...    |     |
| 22565724+6157468 | 109.912  | 2.021    | 13.324 | 9      | -      | -    | -    | -        | -    | -      | -    | -                      | -          | -          | -    | -        | -          | -     | 13.701                             | 0.43                        | ...                         | -1                   | 13.8                               | 0.56                                 | 3.91                          | 8.736                         | -1.78  | ...    | 4.13  | ...  | ...   | -1.52  | ...    |     |
| 22570049+6237398 | 110.201  | 2.619    | 17.264 | 9      | -      | -    | -    | -        | -    | -      | -    | -                      | -          | -          | -    | -        | -          | -     | 8.946                              | 1.10                        | 2.43                        | 1                    | 111.2                              | 0.62                                 | 4.17                          | 2.513                         | -1.76  | -6.15  | 5.35  | ...  | ...   | -1.42  | -5.01  |     |
| 22570222+6238248 | 110.209  | 2.629    | 17.238 | 9      | -      | -    | -    | -        | -    | -      | -    | -                      | -          | -          | -    | -        | -          | -     | 7.586                              | 1.09                        | 2.38                        | 1                    | 219.6                              | 0.22                                 | 4.17                          | 1.163                         | -1.76  | -6.18  | 5.34  | ...  | ...   | -1.43  | -5.05  |     |
| 22570324+6238468 | 110.214  | 2.634    | 16.942 | 9      | -      | -    | -    | -        | -    | -      | -    | -                      | -          | -          | -    | -        | -          | -     | 10.051                             | 0.99                        | 1.87                        | 1                    | 67.2                               | 0.56                                 | 4.17                          | 3.738                         | -1.81  | -6.54  | 5.25  | ...  | ...   | -1.48  | -5.42  |     |
| 22570944+6155368 | 109.918  | 1.978    | 7.085  | 9      | -      | -    | -    | -        | -    | -      | -    | -                      | -          | -          | -    | -        | -          | -     | 8.963                              | 1.23                        | 2.39                        | 1                    | 147.2                              | 0.46                                 | 3.88                          | 6.323                         | 0.06   | -1.13  | 2.19  | ...  | ...   | 0.20   | -0.67  |     |
| 22571100+6156388 | 109.928  | 1.992    | 7.935  | 9      | -      | -    | -    | -        | -    | -      | -    | -                      | -          | -          | -    | -        | -          | -     | 9.957                              | ...                         | 2.15                        | 1                    | 73.4                               | 1.00                                 | 3.88                          | 7.000                         | ...    | -1.79  | 2.46  | ...  | ...   | ...    | -1.27  | ... |
| 22571510+6156148 | 109.932  | 1.983    | 6.995  | 9      | -      | -    | -    | -        | -    | -      | -    | -                      | -          | -          | -    | -        | -          | -     | 7.570                              | 1.28                        | 2.52                        | 1                    | 214.4                              | 0.64                                 | 3.88                          | 4.964                         | 0.12   | -0.95  | 2.17  | ...  | ...   | 0.25   | -0.49  |     |
| 22571921+6155398 | 109.936  | 1.970    | 5.889  | 8      | -      | -    | -    | -        | -    | -      | -    | -                      | -          | -          | -    | -        | -          | -     | 10.372                             | 0.88                        | 1.86                        | 1                    | 79.4                               | 0.42                                 | 3.88                          | 8.178                         | -0.09  | -1.07  | 1.82  | ...  | ...   | 0.02   | -0.68  |     |
| 22572943+6230588 | 110.204  | 2.495    | 8.492  | 9      | -      | -    | -    | -        | -    | -      | -    | -                      | -          | -          | -    | -        | -          | -     | 12.921                             | ...                         | ...                         | 1                    | 15.4                               | 0.40                                 | 4.17                          | 9.757                         | ...    | ...    | 2.63  | ...  | ...   | ...    | ...    |     |
| 22572956+6229438 | 110.195  | 2.476    | 6.710  | 7      | -      | -    | -    | -        | -    | -      | -    | -                      | -          | -          | -    | -        | -          | -     | 11.873                             | ...                         | ...                         | 1                    | 24.8                               | 0.40                                 | 4.17                          | 9.373                         | ...    | ...    | 2.08  | ...  | ...   | ...    | ...    |     |
| 22580734+6233027 | 110.285  | 2.495    | 9.026  | 8      | -      | -    | -    | -        | -    | -      | -    | -                      | -          | -          | -    | -        | -          | -     | 12.307                             | 1.10                        | ...                         | 1                    | 51.0                               | 0.26                                 | 3.91                          | 8.944                         | -0.39  | ...    | 2.80  | ...  | ...   | -0.21  | ...    |     |
| 22580824+5928334 | 108.987  | -0.293   | 6.097  | 8      | -      | -    | -    | -        | -    | -      | -    | -                      | -          | -          | -    | -        | -          | -     | 12.435                             | ...                         | ...                         | 1                    | 23.0                               | 1.00                                 | 3.96                          | 10.163                        | ...    | ...    | 1.89  | ...  | ...   | ...    | ...    |     |
| 22580878+6232428 | 110.285  | 2.489    | 8.565  | 8      | -      | -    | -    | -        | -    | -      | -    | -                      | -          | -          | -    | -        | -          | -     | 10.648                             | 1.47                        | ...                         | 1                    | 55.6                               | 0.84                                 | 3.91                          | 7.457                         | 0.05   | ...    | 2.65  | ...  | ...   | 0.22   | ...    |     |
| 22583858+5855492 | 108.816  | -0.815   | 3.073  | 8      | -      | -    | -    | -        | -    | -      | -    | -                      | -          | -          | -    | -        | -          | -     | 11.188                             | 1.79                        | ...                         | 1                    | 28.2                               | 0.68                                 | 4.02                          | 10.043                        | 1.28   | ...    | 0.95  | ...  | ...   | 1.34   | ...    |     |
| 22584086+5846592 | 108.758  | -0.950   | 13.990 | 9      | -      | -    | -    | -        | -    | -      | -    | -                      | -          | -          | -    | -        | -          | -     | 7.244                              | 0.82                        | 1.55                        | 1                    | 143.6                              | 0.86                                 | 4.02                          | 2.031                         | -1.50  | -5.40  | 4.33  | ...  | ...   | -1.23  | -4.48  |     |
| 22584163+5929252 | 109.057  | -0.309   | 9.689  | 9      | -      | -    | -    | -        | -    | -      | -    | -                      | -          | -          | -    | -        | -          | -     | 12.991                             | 0.91                        | ...                         | 1                    | 16.8                               | 0.52                                 | 3.96                          | 9.381                         | -0.69  | ...    | 3.00  | ...  | ...   | -0.50  | ...    |     |
| 22584213+5845332 | 108.751  | -0.973   | 12.719 | 9      | -      | -    | -    | -        | -    | -      | -    | -                      | -          | -          | -    | -        | -          | -     | 9.782                              | 1.14                        | 2.32                        | 1                    | 79.6                               | 0.52                                 | 4.02                          | 5.043                         | -0.97  | -4.00  | 3.94  | ...  | ...   | -0.72  | -3.16  |     |
| 22584478+5847433 | 108.771  | -0.943   | 14.623 | 9      | -      | -    | -    | -        | -    | -      | -    | -                      | -          | -          | -    | -        | -          | -     | 9.763                              | 0.96                        | 1.83                        | 1                    | 220.2                              | 0.56                                 | 4.03                          | 4.314                         | -1.46  | -5.43  | 4.53  | ...  | ...   | -1.17  | -4.47  |     |
| 22584497+5847502 | 108.772  | -0.941   | 14.480 | 9      | -      | -    | -    | -        | -    | -      | -    | -                      | -          | -          | -    | -        | -          | -     | 10.078                             | 0.98                        | 1.90                        | 1                    | 120.2                              | 0.30                                 | 4.02                          | 4.683                         | -1.42  | -5.30  | 4.49  | ...  | ...   | -1.13  | -4.34  |     |
| 22584573+5846222 | 108.764  | -0.964   | 13.903 | 9      | -      | -    | -    |          |      |        |      |                        |            |            |      |          |            |       |                                    |                             |                             |                      |                                    |                                      |                               |                               |        |        |       |      |       |        |        |     |

Table B1: a) continued.

| 2MASX J          |         | <i>l</i>    | <i>b</i>    | EBV        | Object       | Sample     |             |             |            | Disc        | 2MRS          | Velocity    |     | NIR          | Photom      | Ext          | <i>K</i> <sub>20</sub> | <i>H-K</i>   | <i>J-K</i>  | <i>vc</i>   | <i>a</i>    | <i>b/a</i> | std.d. | <i>K</i> <sub>S</sub> <sup>o</sup> | ( <i>H-K</i> ) <sup>o</sup> | ( <i>J-K</i> ) <sup>o</sup> | <i>A<sub>K</sub></i> | <i>a</i> <sup>d</sup> | <i>K</i> <sub>S</sub> <sup>d</sup> | ( <i>H-K</i> ) <sup>o,c</sup> | ( <i>J-K</i> ) <sup>o,c</sup> |             |             |
|------------------|---------|-------------|-------------|------------|--------------|------------|-------------|-------------|------------|-------------|---------------|-------------|-----|--------------|-------------|--------------|------------------------|--------------|-------------|-------------|-------------|------------|--------|------------------------------------|-----------------------------|-----------------------------|----------------------|-----------------------|------------------------------------|-------------------------------|-------------------------------|-------------|-------------|
| (1)              |         | deg<br>(2a) | deg<br>(2b) | mag<br>(3) | class<br>(4) | off<br>(5) | flag<br>(6) | gal<br>(7a) | TF<br>(7b) | obs<br>(7c) | ext'd<br>(7d) | type<br>(8) | (9) | Opt<br>(10a) | HI<br>(10b) | flag<br>(11) | flag<br>(12)           | flag<br>(13) | mag<br>(14) | mag<br>(15) | mag<br>(16) | (17)       | (18)   | (19)                               | (20)                        | mag<br>(21)                 | mag<br>(22)          | mag<br>(23)           | mag<br>(24)                        | "<br>(25)                     | mag<br>(26)                   | mag<br>(27) | mag<br>(28) |
| 23051780+6004420 | 110.056 | -0.113      | 3.949       | 9          | -            | -          | -           | -           | -          | -           | -             | -           | -   | -            | -           | -            | -                      | -            | 11.526      | 0.70        | 1.92        | 1          | 21.6   | 0.66                               | 4.04                        | 10.055                      | 0.04                 | -0.04                 | 1.22                               | ...                           | ...                           | 0.12        | 0.22        |
| 23051883+6014099 | 110.120 | 0.031       | 12.576      | 9          | -            | -          | -           | -           | -          | -           | -             | -           | -   | -            | -           | -            | -                      | -            | 10.494      | 0.97        | 1.96        | 1          | 93.2   | 0.22                               | 4.05                        | 5.808                       | -1.11                | -4.29                 | 3.90                               | ...                           | ...                           | -0.86       | -3.46       |
| 23052587+6008149 | 110.095 | -0.065      | 5.841       | 8          | -            | -          | -           | -           | -          | -           | -             | -           | -   | -            | -           | -            | -                      | -            | 8.057       | 1.33        | 3.10        | 1          | 69.8   | 0.84                               | 4.05                        | 5.881                       | 0.36                 | 0.19                  | 1.81                               | ...                           | ...                           | 0.48        | 0.58        |
| 23053179+6015105 | 110.152 | 0.036       | 10.023      | 9          | -            | -          | -           | -           | -          | -           | -             | -           | -   | -            | -           | -            | -                      | -            | 13.719      | ...         | 1.63        | -1         | 10.2   | 1.00                               | 4.03                        | 9.984                       | ...                  | -3.35                 | 3.10                               | ...                           | ...                           | ...         | -2.69       |
| 23054004+6229166 | 111.053 | 2.081       | 3.298       | 7          | -            | -          | -           | -           | -          | -           | -             | -           | -   | -            | -           | -            | -                      | -            | 10.140      | 1.83        | 4.45        | 1          | 38.2   | 0.86                               | 3.86                        | 8.911                       | 1.28                 | 2.81                  | 1.02                               | ...                           | ...                           | 1.35        | 3.03        |
| 23054812+6230097 | 111.074 | 2.089       | 3.322       | 7          | -            | -          | -           | -           | -          | -           | -             | -           | -   | -            | -           | -            | -                      | -            | 9.209       | 1.23        | 2.84        | 1          | 94.6   | 0.64                               | 3.86                        | 7.971                       | 0.68                 | 1.19                  | 1.03                               | ...                           | ...                           | 0.75        | 1.41        |
| 23055649+6231517 | 111.100 | 2.108       | 3.369       | 8          | -            | -          | -           | -           | -          | -           | -             | -           | -   | -            | -           | -            | -                      | -            | 12.047      | 1.42        | 3.26        | 1          | 24.8   | 0.42                               | 3.86                        | 10.792                      | 0.87                 | 1.58                  | 1.04                               | ...                           | ...                           | 0.93        | 1.81        |
| 23060024+6232077 | 111.108 | 2.109       | 3.263       | 9          | -            | -          | -           | -           | -          | -           | -             | -           | -   | -            | -           | -            | -                      | -            | 11.979      | ...         | ...         | 1          | 31.4   | 0.68                               | 3.86                        | 10.763                      | ...                  | ...                   | 1.01                               | ...                           | ...                           | ...         |             |
| 23061748+6015487 | 110.243 | 0.008       | 7.965       | 9          | -            | -          | -           | -           | -          | -           | -             | -           | -   | -            | -           | -            | -                      | -            | 11.067      | 0.71        | 1.77        | 1          | 41.4   | 0.42                               | 4.03                        | 8.099                       | -0.61                | -2.19                 | 2.47                               | ...                           | ...                           | -0.45       | -1.66       |
| 23062219+6016176 | 110.255 | 0.012       | 7.580       | 9          | -            | -          | -           | -           | -          | -           | -             | -           | -   | -            | -           | -            | -                      | -            | 7.913       | 0.73        | 1.73        | 1          | 124.2  | 0.66                               | 4.03                        | 5.089                       | -0.52                | -2.03                 | 2.35                               | ...                           | ...                           | -0.38       | -1.53       |
| 23062652+6016037 | 110.261 | 0.005       | 7.429       | 9          | -            | -          | -           | -           | -          | -           | -             | -           | -   | -            | -           | -            | -                      | -            | 11.113      | 0.68        | 1.91        | 1          | 48.2   | 0.42                               | 3.95                        | 8.345                       | -0.55                | -1.78                 | 2.30                               | ...                           | ...                           | -0.41       | -1.29       |
| 23063325+6348588 | 111.671 | 3.262       | 2.037       | 8          | -            | -          | -           | -           | -          | -           | -             | -           | -   | -            | -           | -            | -                      | -            | 11.463      | 0.94        | 2.48        | 1          | 37.4   | 0.94                               | 3.88                        | 10.704                      | 0.60                 | 1.47                  | 0.63                               | ...                           | ...                           | 0.64        | 1.61        |
| 23073006+5850194 | 109.825 | -1.362      | 2.112       | 8          | -            | -          | -           | -           | -          | -           | -             | -           | -   | -            | -           | -            | -                      | -            | 11.169      | 1.25        | 2.76        | 1          | 26.2   | 0.48                               | 3.92                        | 10.382                      | 0.90                 | 1.71                  | 0.65                               | ...                           | ...                           | 0.94        | 1.85        |
| 23080278+6048543 | 110.657 | 0.432       | 1.988       | 7          | -            | -          | -           | -           | -          | -           | -             | -           | -   | -            | -           | -            | -                      | -            | 11.703      | 0.69        | 2.02        | 1          | 28.0   | 0.66                               | 4.05                        | 10.962                      | 0.36                 | 1.04                  | 0.62                               | ...                           | ...                           | 0.40        | 1.17        |
| 23085314+6133564 | 111.040 | 1.085       | 2.818       | 9          | -            | -          | -           | -           | -          | -           | -             | -           | -   | -            | -           | -            | -                      | -            | 11.143      | 0.91        | 1.93        | 1          | 74.6   | 0.32                               | 3.90                        | 10.093                      | 0.45                 | 0.53                  | 0.87                               | ...                           | ...                           | 0.50        | 0.71        |
| 23085734+6134204 | 111.051 | 1.088       | 2.770       | 9          | -            | -          | -           | -           | -          | -           | -             | -           | -   | -            | -           | -            | -                      | -            | 11.448      | 1.18        | 2.32        | 1          | 56.0   | 0.26                               | 3.90                        | 10.416                      | 0.72                 | 0.95                  | 0.86                               | ...                           | ...                           | 0.77        | 1.13        |
| 23094364+6723389 | 113.371 | 6.430       | 1.460       | 8          | -            | -          | -           | -           | -          | -           | -             | -           | -   | -            | -           | -            | -                      | -            | 10.608      | 1.18        | 2.07        | -2         | 16.0   | 0.84                               | 3.66                        | 10.064                      | 0.94                 | 1.35                  | 0.45                               | ...                           | ...                           | 0.96        | 1.45        |
| 23095920+5126055 | 107.275 | -8.326      | 0.327       | 1          | -            | -          | -           | g           | -          | -           | -             | D3          | c   | o            | -           | -            | -                      | -            | 10.976      | 0.41        | 1.21        | 1          | 40.2   | 0.68                               | 3.56                        | 10.854                      | 0.36                 | 1.05                  | 0.10                               | 40.9                          | 10.87                         | 0.37        | 1.07        |
| 23100249+5948289 | 110.498 | -0.593      | 4.504       | 9          | -            | -          | -           | -           | -          | -           | -             | -           | -   | -            | -           | -            | -                      | -            | 11.085      | 1.23        | 2.38        | 1          | 103.0  | 0.30                               | 3.88                        | 9.407                       | 0.49                 | 0.14                  | 1.40                               | ...                           | ...                           | 0.57        | 0.43        |
| 23103197+6739390 | 113.546 | 6.647       | 1.519       | 1          | -            | -          | -           | g           | t          | N           | -             | D1          | e   | o            | *           | -            | -                      | -            | 9.387       | 0.47        | 1.59        | 1          | 70.6   | 0.69                               | ...                         | 8.821                       | 0.22                 | 0.84                  | 0.47                               | ...                           | ...                           | 0.25        | 0.94        |
| 23125482+5944414 | 110.809 | -0.787      | 2.977       | 8          | -            | -          | -           | -           | -          | -           | -             | -           | -   | -            | -           | -            | -                      | -            | 11.526      | 0.98        | 2.38        | 1          | 42.2   | 0.46                               | 3.95                        | 10.417                      | 0.49                 | 0.90                  | 0.92                               | ...                           | ...                           | 0.55        | 1.10        |
| 23131683+6129075 | 111.495 | 0.813       | 45.485      | 8          | -            | -          | -           | -           | -          | -           | -             | -           | -   | -            | -           | -            | -                      | -            | 11.029      | 1.97        | ...         | 1          | 36.2   | 0.62                               | 3.94                        | -5.919                      | -5.56                | ...                   | 14.09                              | ...                           | ...                           | -4.67       | ...         |
| 23131962+6129285 | 111.503 | 0.816       | 48.900      | 9          | -            | -          | -           | -           | -          | -           | -             | -           | -   | -            | -           | -            | -                      | -            | 10.287      | 1.28        | 2.66        | 1          | 113.4  | 0.26                               | 3.94                        | -7.933                      | -6.81                | -21.64                | 15.15                              | ...                           | ...                           | -5.85       | -18.41      |
| 23132138+6125176 | 111.480 | 0.750       | 30.273      | 9          | -            | -          | -           | -           | -          | -           | -             | -           | -   | -            | -           | -            | -                      | -            | 12.521      | ...         | ...         | 1          | 39.6   | 1.0                                | 4.05                        | 1.241                       | ...                  | ...                   | 9.38                               | ...                           | ...                           | ...         | ...         |
| 23132200+6130436 | 111.515 | 0.834       | 51.998      | 9          | -            | -          | -           | -           | -          | -           | -             | -           | -   | -            | -           | -            | -                      | -            | 10.231      | 1.66        | 2.14        | 1          | 54.8   | 0.74                               | 4.08                        | -9.143                      | -6.95                | -23.69                | 16.11                              | ...                           | ...                           | -5.93       | -20.26      |
| 23133024+6130107 | 111.526 | 0.819       | 63.156      | 9          | -            | -          | -           | -           | -          | -           | -             | -           | -   | -            | -           | -            | -                      | -            | 6.326       | 1.10        | 1.77        | 1          | 165.8  | 0.92                               | 4.08                        | -17.206                     | -9.36                | -29.61                | 19.56                              | ...                           | ...                           | -8.12       | -25.44      |
| 23133389+6128537 | 111.525 | 0.797       | 60.661      | 9          | -            | -          | -           | -           | -          | -           | -             | -           | -   | -            | -           | -            | -                      | -            | 8.673       | 1.13        | 2.46        | 1          | 72.6   | 0.52                               | 4.05                        | -13.929                     | -8.92                | -27.68                | 18.79                              | ...                           | ...                           | -7.73       | -23.67      |
| 23133778+6131358 | 111.549 | 0.836       | 58.823      | 9          | -            | -          | -           | -           | -          | -           | -             | -           | -   | -            | -           | -            | -                      | -            | 8.052       | 1.37        | 2.00        | 1          | 219.6  | 0.32                               | 4.08                        | -13.865                     | -8.37                | -27.22                | 18.22                              | ...                           | ...                           | -7.22       | -23.34      |
| 23133780+6129188 | 111.535 | 0.800       | 68.305      | 9          | -            | -          | -           | -           | -          | -           | -             | -           | -   | -            | -           | -            | -                      | -            | 6.943       | 1.31        | 1.92        | 1          | 219.2  | 0.66                               | 4.08                        | -18.507                     | -10.00               | -32.01                | 21.16                              | ...                           | ...                           | -8.66       | -27.50      |
| 23133794+6128118 | 111.529 | 0.783       | 60.494      | 9          | -            | -          | -           | -           | -          | -           | -             | -           | -   | -            | -           | -            | -                      | -            | 10.592      | ...         | ...         | 1          | 88.4   | 0.20                               | 4.05                        | -11.948                     | ...                  | ...                   | 18.74                              | ...                           | ...                           | ...         | ...         |
| 23134396+6126588 | 111.532 | 0.760       | 52.993      | 8          | -            | -          | -           | -           | -          | -           | -             | -           | -   | -            | -           | -            | -                      | -            | 11.802      | 2.20        | ...         | 1          | 29.2   | 0.68                               | 4.05                        | -7.943                      | -6.58                | ...                   | 16.41                              | ...                           | ...                           | -5.54       | ...         |
| 23134423+6128378 | 111.543 | 0.785       | 62.678      | 9          | -            | -          | -           | -           | -          | -           | -             | -           | -   | -            | -           | -            | -                      | -            | 7.049       | 1.47        | 2.71        | 1          | 176.0  | 0.60                               | 4.08                        | -16.305                     | -8.91                | -28.43                | 19.41                              | ...                           | ...                           | -7.68       | -24.29      |
| 23134437+6128278 | 111.542 | 0.782       | 61.444      | 9          | -            | -          | -           | -           | -          | -           | -             | -           | -   | -            | -           | -            | -                      | -            | 7.265       | 1.61        | 3.27        | 1          | 160.0  | 0.58                               | 4.05                        | -15.629                     | -8.57                | -27.25                | 19.03                              | ...                           | ...                           | -7.36       | -23.20      |
| 23134574+5212063 | 108.113 | -7.837      | 0.220       | 1          | -            | o          | -           | g           | t          | -           | -             | D1          | c   | o            | -           | -            | o                      | -            | 11.171      | 0.26        | 0.93        | 1          | 43.8   | 0.40                               | 3.62                        | 11.089                      | 0.22                 | 0.82                  | 0.07                               | 44.2                          | 11.10                         | 0.22        | 0.83        |
| 23134743+6129198 | 111.553 | 0.793       | 66.425      | 9          | -            | -          | -           | -           | -          | -           | -             | -           | -   | -            | -           | -            | -                      | -            | 11.301      | 2.53        | 3.64        | 1          | 31.2   | 0.58                               | 4.08                        | -13.449                     | -8.47                | -29.36                | 20.58                              | ...                           | ...                           | -7.16       | -24.98      |
| 23134814+6127408 | 111.544 | 0.767       | 55.035      | 8          | -            | -          | -           | -           | -          | -           | -             | -           | -   | -            | -           | -            | -                      | -            | 10.428      | 1.80        | 3.18        | 1          | 50.6   | 0.86                               | 4.05                        | -10.078                     | -7.32                | -24.17                | 17.05                              | ...                           | ...                           | -6.24       | -20.53      |
| 23135623+6127058 | 111.556 | 0.752       | 47.758      | 9          | -            | -          | -           | -           | -          | -           | -             | -           | -   | -            | -           | -            | -                      | -            | 8.046       | 2.84        | 5.29        | 1          | 133.4  | 0.48                               | 4.05                        | -9.749                      | -5.07                | -18.44                | 14.79                              | ...                           | ...                           | -4.13       | -15.29      |
| 23135890+6130548 | 111.584 | 0.810       | 48.960      | 9          | -            | -          | -           | -           | -          | -           | -             | -           | -   | -            | -           | -            | -                      | -            | 9.540       | 1.15        | 2.21        | 1          | 113.2  | 0.52                               | 4.08                        | -8.702                      | -6.96                | -22.11                | 15.17                              | ...                           | ...                           | -6.00       | -18.88      |
| 23140169+6130178 | 111.585 | 0.798       | 49.033      | 8          | -            | -          | -           | -           | -          | -           | -             | -           | -   | -            | -           | -            | -                      | -            | 9.144       | 1.56        | 3.71        | 1          | 41.4   | 0.70                               | 4.08                        | -9.126                      | -6.56                | -20.65                | 15.19                              | ...                           | ...                           | -5.60       | -17.42      |
| 23140209+6127188 | 111.568 | 0.752       | 45.363      | 9          | -            | -          | -           | -           | -          | -           | -             | -           | -   | -            | -           | -            | -                      | -            | 7.664       | 2.11        | ...         | 1          | 219.8  | 0.58                               | 4.05                        | -9.238                      | -5.40                | ...                   | 14.05                              | ...                           | ...                           | -4.51       | ...         |
| 23140390+6126398 | 111.567 | 0.740       | 40.049      | 9          | -            | -          | -           | -           | -          | -           | -             | -           | -   | -            | -           | -            | -                      | -            | 11.307      | 2.28        | 3.12        | 1          | 46.4   | 0.32                               | 4.05                        | -3.615                      | -4.35                | -16.78                | 12.41                              | ...                           | ...                           | -3.57       | -14.13      |
| 23145710+5928024 | 110.947 | -1.140      | 2.725       | 1          | -            | -          | -           | g           | t          | N           | -             | D1          | -   | -            | -           | e            | -                      | -            | 12.165      | 0.49        | 1.67        | 1          | 28.0   | 0.46                               | 3.98                        | 11.150                      | 0.04                 | 0.31                  | 0.84                               | 41.6                          | 10.94                         | 0.10        | 0.49        |
| 23152630+6107544 | 111.607 | 0.389       | 13.056      | 9          | -            | -          | -           | -           | -          | -           | -             | -           | -   | -            | -           | -            | -                      | -            | 10.069      | 1.44        | 2.58        | 1          | 95.0   | 0.58                               | 3.98                        | 5.204                       | -0.72                | -3.91                 | 4.04                               | ...                           | ...                           | -0.46       | -3.05       |
| 23152744+5939586 | 111.079 | -0.978      | 3.688       | 8          | -            | o          | -           | -           | -          | -           | -             | -           | -   | -            | -           | -            | o                      | -            | 10.738      | 1.13        | 2.73        | 1          | 17.6   | 0.48                               | 3.95                        | 9.364                       | 0.52                 | 0.89                  | 1.14                               | ...                           | ...                           | 0.59        | 1.14        |
| 23153127+6107104 | 111.612 | 0.374       | 12.107      | 8          | -            | -          | -           | -           | -          | -           | -             | -           | -   | -            | -           | -            | -                      | -            | 7.206       | 1.09        | 2.47        | 1          | 130.0  | 0.78                               | 3.98                        | 2.695                       | -0.91                | -3.55                 | 3.75                               | ...                           | ...                           | -0.68       | -2.75       |
| 23154261+6147335 | 11      |             |             |            |              |            |             |             |            |             |               |             |     |              |             |              |                        |              |             |             |             |            |        |                                    |                             |                             |                      |                       |                                    |                               |                               |             |             |

© 2017 RAS, MNRAS 000, 1–133



11  
58  
06  
92  
00  
95  
83  
06  
95  
20  
82  
75  
23  
94  
42  
81  
75  
60  
89  
84  
79  
13  
88  
16  
99  
30  
73  
81  
59  
90  
72  
73  
75  
85

Table B1: b) continued.

| 2MASX J          | <i>l</i>    | <i>b</i>    | EBV        | Object       | Sample     | Disc       | 2MRS        | Velocity   | NIR         | Photom        | Ext         | <i>K</i> <sub>20</sub> | <i>H-K</i>   | <i>J-K</i>  | vc          | <i>a</i>    | <i>b/a</i>  | st.d.                                 | <i>K</i> <sub>s</sub> <sup>o</sup> | ( <i>H-K</i> ) <sup>o</sup> | ( <i>J-K</i> ) <sup>o</sup> | <i>A<sub>K</sub></i> | <i>a</i> <sup>d</sup> | <i>K</i> <sub>s</sub> <sup>o,d</sup> | ( <i>H-K</i> ) <sup>o,c</sup> | ( <i>J-K</i> ) <sup>o,c</sup> |             |             |             |             |             |             |
|------------------|-------------|-------------|------------|--------------|------------|------------|-------------|------------|-------------|---------------|-------------|------------------------|--------------|-------------|-------------|-------------|-------------|---------------------------------------|------------------------------------|-----------------------------|-----------------------------|----------------------|-----------------------|--------------------------------------|-------------------------------|-------------------------------|-------------|-------------|-------------|-------------|-------------|-------------|
| (1)              | deg<br>(2a) | deg<br>(2b) | mag<br>(3) | class<br>(4) | off<br>(5) | flg<br>(6) | gal<br>(7a) | TF<br>(7b) | Obs<br>(7c) | ext'd<br>(7d) | type<br>(8) | (9)                    | Opt<br>(10a) | HI<br>(10b) | flg<br>(11) | flg<br>(12) | flg<br>(13) | <i>K</i> <sub>20</sub><br>mag<br>(14) | <i>H-K</i><br>mag<br>(15)          | <i>J-K</i><br>mag<br>(16)   | (17)                        | (18)                 | (19)                  | (20)                                 | mag<br>(21)                   | mag<br>(22)                   | mag<br>(23) | mag<br>(24) | mag<br>(25) | mag<br>(26) | mag<br>(27) | mag<br>(28) |
| 04415132+2442501 | 175.176     | -14.034     | 1.426      | 1            | -          | -          | g           | t          | N           | -             | D1          | e                      | o            | *           | U           | -           | -           | 11.721                                | 0.45                               | 1.44                        | 1                           | 36.4                 | 0.50                  | 3.21                                 | 11.190                        | 0.21                          | 0.74        | 0.44        | 42.2        | 11.17       | 0.24        | 0.83        |
| 04455692+2508456 | 175.432     | -13.041     | 1.425      | 2            | -          | -          | g           | -          | -           | -             | D4          | e                      | o            | -           | U           | -           | -           | 11.414                                | 0.46                               | 1.42                        | 1                           | 25.4                 | 0.88                  | 3.23                                 | 10.883                        | 0.22                          | 0.72        | 0.44        | 29.1        | 10.88       | 0.25        | 0.81        |
| 04492734-6912056 | 280.734     | -35.919     | 1.588      | 6            | o          | -          | -           | -          | -           | -             | -           | -                      | -            | -           | -           | o           | e           | 10.722                                | 0.74                               | 1.09                        | 1                           | 40.4                 | 0.74                  | 3.67                                 | 10.130                        | 0.48                          | 0.31        | 0.49        | ...         | ...         | 0.51        | 0.41        |
| 04514956-6923045 | 280.866     | -35.662     | 2.507      | 9            | -          | -          | -           | -          | -           | -             | -           | -                      | -            | -           | -           | -           | -           | 12.119                                | 0.95                               | 1.00                        | 1                           | 30.2                 | 0.78                  | 3.77                                 | 11.185                        | 0.53                          | -0.24       | 0.78        | ...         | ...         | 0.58        | -0.08       |
| 04515204-6923318 | 280.874     | -35.656     | 2.419      | 7            | -          | -          | -           | -          | -           | -             | -           | -                      | -            | -           | -           | -           | -           | 9.468                                 | 0.91                               | 1.28                        | 1                           | 62.0                 | 0.74                  | 3.72                                 | 8.567                         | 0.51                          | 0.08        | 0.75        | ...         | ...         | 0.56        | 0.24        |
| 04515371-6923286 | 280.872     | -35.654     | 2.446      | 7            | -          | -          | -           | -          | -           | -             | -           | -                      | -            | -           | -           | -           | -           | 9.587                                 | 0.91                               | 1.31                        | 1                           | 58.8                 | 0.74                  | 3.77                                 | 8.676                         | 0.51                          | 0.10        | 0.76        | ...         | ...         | 0.55        | 0.26        |
| 04520886-6655238 | 277.951     | -36.369     | 1.407      | 7            | -          | -          | -           | -          | -           | -             | -           | -                      | -            | -           | -           | -           | -           | 9.717                                 | 0.73                               | 1.04                        | 1                           | 75.0                 | 0.74                  | 3.48                                 | 9.193                         | 0.50                          | 0.34        | 0.44        | ...         | ...         | 0.53        | 0.44        |
| 04524556-6911490 | 280.615     | -35.642     | 1.712      | 7            | -          | -          | -           | -          | -           | -             | -           | -                      | -            | -           | -           | -           | -           | 9.879                                 | 1.80                               | 3.46                        | 1                           | 24.0                 | 0.84                  | 3.79                                 | 9.241                         | 1.52                          | 2.61        | 0.53        | ...         | ...         | 1.55        | 2.73        |
| 04531656+2552432 | 175.891     | -11.290     | 1.000      | 1            | -          | -          | g           | -          | N           | -             | D2          | c                      | o            | -           | U           | -           | -           | 10.367                                | 0.40                               | 1.34                        | 1                           | 54.0                 | 0.66                  | 3.29                                 | 9.994                         | 0.23                          | 0.84        | 0.31        | 58.5        | 10.01       | 0.25        | 0.91        |
| 04540214-6911511 | 280.573     | -35.534     | 2.622      | 7            | -          | -          | -           | -          | -           | -             | -           | -                      | -            | -           | -           | -           | -           | 9.880                                 | 0.80                               | 1.12                        | 1                           | 79.6                 | 0.56                  | 3.79                                 | 8.903                         | 0.36                          | -0.18       | 0.81        | ...         | ...         | 0.41        | -0.01       |
| 04542617-6911025 | 280.544     | -35.504     | 2.592      | 7            | -          | -          | -           | -          | -           | -             | -           | -                      | -            | -           | -           | -           | -           | 10.958                                | 0.69                               | 0.94                        | 1                           | 36.4                 | 0.54                  | 3.86                                 | 9.992                         | 0.26                          | -0.35       | 0.80        | ...         | ...         | 0.31        | -0.18       |
| 04563813-6623543 | 277.175     | -36.083     | 3.125      | 9            | -          | -          | -           | -          | -           | -             | -           | -                      | -            | -           | -           | -           | -           | 11.367                                | 0.97                               | 1.04                        | 1                           | 55.6                 | 0.78                  | 3.52                                 | 10.203                        | 0.45                          | -0.51       | 0.97        | ...         | ...         | 0.51        | -0.30       |
| 04564692-6624309 | 277.183     | -36.066     | 3.341      | 8            | o          | -          | -           | -          | -           | -             | -           | -                      | -            | -           | -           | o           | -           | 10.482                                | 0.48                               | 0.73                        | 1                           | 72.2                 | 0.74                  | 3.62                                 | 9.237                         | -0.08                         | -0.93       | 1.03        | ...         | ...         | -0.01       | -0.71       |
| 04570259-6623211 | 277.151     | -36.046     | 3.746      | 8            | -          | -          | -           | -          | -           | -             | -           | -                      | -            | -           | -           | -           | -           | 12.483                                | 0.69                               | 0.86                        | 1                           | 32.2                 | 0.44                  | 3.43                                 | 11.087                        | 0.07                          | -1.00       | 1.16        | ...         | ...         | 0.14        | -0.75       |
| 04571529-6826292 | 279.581     | -35.476     | 1.386      | 8            | o          | -          | -           | -          | -           | -             | -           | -                      | -            | -           | -           | o           | -           | 10.984                                | 0.55                               | 1.07                        | 1                           | 53.8                 | 0.42                  | 3.82                                 | 10.468                        | 0.32                          | 0.38        | 0.43        | ...         | ...         | 0.35        | 0.47        |
| 04571624-6623202 | 277.144     | -36.024     | 3.612      | 7            | -          | p?         | -           | -          | -           | -             | -           | -                      | -            | -           | -           | -           | -           | 11.252                                | 0.71                               | 1.01                        | 1                           | 26.4                 | 0.66                  | 3.43                                 | 9.906                         | 0.12                          | -0.79       | 1.12        | ...         | ...         | 0.19        | -0.55       |
| 04581393+2536088 | 176.807     | -10.572     | 0.965      | 1            | -          | -          | g           | -          | N           | -             | D1          | c                      | o            | -           | U           | -           | -           | 11.357                                | 0.37                               | 1.28                        | 1                           | 35.0                 | 0.54                  | 3.39                                 | 10.997                        | 0.21                          | 0.80        | 0.30        | 38.2        | 10.99       | 0.23        | 0.87        |
| 05065477-0320348 | 203.519     | -24.702     | 2.351      | 8            | -          | -          | g           | -          | -           | -             | -           | -                      | -            | -           | U           | -           | -           | 8.874                                 | 0.97                               | 1.32                        | 1                           | 125.4                | 0.64                  | 3.14                                 | 7.998                         | 0.58                          | 0.15        | 0.73        | ...         | ...         | 0.62        | 0.31        |
| 05084823-6845390 | 279.626     | -34.375     | 1.321      | 9            | -          | -          | -           | -          | -           | -             | -           | -                      | -            | -           | -           | -           | -           | 8.696                                 | 0.06                               | 0.36                        | 1                           | 203.4                | 0.60                  | 4.22                                 | 8.204                         | -0.16                         | -0.30       | 0.41        | ...         | ...         | -0.13       | -0.21       |
| 05095025-6853490 | 279.760     | -34.253     | 3.728      | 9            | -          | -          | -           | -          | -           | -             | -           | -                      | -            | -           | -           | -           | -           | 11.097                                | 0.37                               | 0.94                        | 1                           | 46.8                 | 0.50                  | 4.25                                 | 9.708                         | -0.24                         | -0.91       | 1.15        | ...         | ...         | -0.17       | -0.66       |
| 05095278-6853007 | 279.743     | -34.252     | 3.762      | 7            | -          | -          | -           | -          | -           | -             | -           | -                      | -            | -           | -           | -           | -           | 9.349                                 | 0.82                               | 1.19                        | 1                           | 98.0                 | 0.56                  | 4.22                                 | 7.947                         | 0.19                          | -0.68       | 1.17        | ...         | ...         | 0.27        | -0.43       |
| 05131816-6922254 | 280.236     | -33.844     | 3.411      | 9            | -          | -          | -           | -          | -           | -             | -           | -                      | -            | -           | -           | -           | -           | 10.628                                | ...                                | ...                         | 1                           | 65.0                 | 1.00                  | 4.30                                 | 9.357                         | ...                           | ...         | 1.06        | ...         | ...         | ...         | ...         |
| 05132182-6922388 | 280.239     | -33.838     | 3.318      | 7            | -          | -          | -           | -          | -           | -             | -           | -                      | -            | -           | -           | -           | -           | 11.275                                | 0.88                               | 1.41                        | 1                           | 32.4                 | 0.82                  | 4.29                                 | 10.039                        | 0.33                          | -0.24       | 1.03        | ...         | ...         | 0.40        | -0.02       |
| 05181754+0710589 | 195.273     | -16.981     | 1.753      | 9            | -          | -          | -           | -          | -           | -             | -           | -                      | -            | -           | -           | -           | -           | 10.332                                | 2.24                               | ...                         | 1                           | 68.8                 | 0.34                  | 3.18                                 | 9.679                         | 1.95                          | ...         | 0.54        | ...         | ...         | 1.98        | ...         |
| 05184005-6924381 | 280.159     | -33.375     | 1.671      | 7            | -          | -          | -           | -          | -           | -             | -           | -                      | -            | -           | -           | -           | -           | 8.676                                 | 0.16                               | 0.54                        | -2                          | 139.0                | 0.52                  | 4.47                                 | 8.053                         | -0.12                         | -0.29       | 0.52        | ...         | ...         | -0.08       | -0.18       |
| 05191846-6947192 | 280.588     | -33.244     | 1.028      | 7            | -          | -          | -           | -          | -           | -             | -           | -                      | -            | -           | -           | -           | -           | 11.296                                | ...                                | 0.97                        | 1                           | 46.2                 | 0.54                  | 4.38                                 | 10.913                        | ...                           | 0.46        | 0.32        | ...         | ...         | ...         | 0.53        |
| 05195387-6911583 | 279.885     | -33.310     | 1.719      | 4            | -          | -          | g           | t          | +           | -             | n           | -                      | -            | -           | -           | -           | e?          | 11.847                                | 0.24                               | 0.95                        | 1                           | 27.4                 | 0.56                  | 4.30                                 | 11.207                        | -0.04                         | 0.10        | 0.53        | 32.8        | 11.18       | -0.01       | 0.21        |
| 05212671-6956472 | 280.729     | -33.032     | 1.077      | 7            | o          | -          | g           | -          | -           | -             | -           | -                      | -            | -           | -           | o           | -           | 10.271                                | 0.18                               | 0.63                        | 1                           | 87.2                 | 0.50                  | 4.30                                 | 9.870                         | -0.00                         | 0.09        | 0.33        | ...         | ...         | 0.02        | 0.16        |
| 05220415-6757547 | 278.390     | -33.340     | 4.506      | 8            | -          | -          | -           | -          | -           | -             | -           | -                      | -            | -           | -           | -           | -           | 10.202                                | 1.07                               | 1.43                        | 1                           | 184.8                | 0.24                  | 3.75                                 | 8.523                         | 0.32                          | -0.81       | 1.40        | ...         | ...         | 0.41        | -0.51       |
| 05220629-6757347 | 278.383     | -33.337     | 4.543      | 9            | -          | -          | -           | -          | -           | -             | -           | -                      | -            | -           | -           | -           | -           | 12.482                                | 0.75                               | 1.42                        | -2                          | 26.6                 | 1.00                  | 3.70                                 | 10.789                        | -0.01                         | -0.83       | 1.41        | ...         | ...         | 0.08        | -0.53       |
| 05221320-6758338 | 278.400     | -33.324     | 4.497      | 7            | -          | -          | -           | -          | -           | -             | -           | -                      | -            | -           | -           | -           | -           | 10.452                                | 1.07                               | 1.22                        | 1                           | 73.6                 | 0.56                  | 3.75                                 | 8.776                         | 0.32                          | -1.01       | 1.39        | ...         | ...         | 0.41        | -0.71       |
| 05221933-6804358 | 278.516     | -33.297     | 2.543      | 7            | -          | -          | -           | -          | -           | -             | -           | -                      | -            | -           | -           | -           | -           | 11.964                                | 0.60                               | 0.99                        | 1                           | 23.4                 | 0.78                  | 3.75                                 | 11.016                        | 0.18                          | -0.27       | 0.79        | ...         | ...         | 0.23        | -0.10       |
| 05223047-6754439 | 278.319     | -33.308     | 3.904      | 7            | -          | -          | -           | -          | -           | -             | -           | -                      | -            | -           | -           | -           | -           | 12.218                                | 0.93                               | 1.59                        | 1                           | 20.6                 | 0.98                  | 3.70                                 | 10.763                        | 0.28                          | -0.35       | 1.21        | ...         | ...         | 0.36        | -0.09       |
| 05225451-6804199 | 278.500     | -33.244     | 2.946      | 8            | -          | -          | -           | -          | -           | -             | -           | -                      | -            | -           | -           | -           | -           | 10.546                                | 1.02                               | 1.18                        | -2                          | 109.8                | 0.68                  | 3.75                                 | 9.448                         | 0.53                          | -0.28       | 0.91        | ...         | ...         | 0.59        | -0.09       |
| 05241342-6829583 | 278.979     | -33.052     | 1.162      | 8            | -          | -          | -           | -          | -           | -             | -           | -                      | -            | -           | -           | -           | -           | 10.776                                | 1.19                               | 2.31                        | 1                           | 32.4                 | 0.72                  | 3.76                                 | 10.343                        | 1.00                          | 1.73        | 0.36        | ...         | ...         | 1.02        | 1.81        |
| 05254927-6615093 | 276.298     | -33.242     | 2.082      | 7            | -          | -          | -           | -          | -           | -             | -           | -                      | -            | -           | -           | -           | -           | 12.009                                | 1.06                               | 1.45                        | 1                           | 16.8                 | 0.64                  | 3.59                                 | 11.233                        | 0.71                          | 0.41        | 0.64        | ...         | ...         | 0.75        | 0.55        |
| 05262734-6848421 | 279.306     | -32.801     | 2.250      | 8            | -          | -          | -           | -          | -           | -             | -           | -                      | -            | -           | -           | -           | -           | 11.777                                | 0.73                               | 1.15                        | 1                           | 51.8                 | 0.76                  | 3.95                                 | 10.939                        | 0.36                          | 0.03        | 0.70        | ...         | ...         | 0.41        | 0.18        |
| 05264745-6848474 | 279.302     | -32.771     | 2.083      | 8            | o          | -          | -           | -          | -           | -             | -           | -                      | -            | -           | -           | o           | -           | 11.179                                | 0.73                               | 1.04                        | 1                           | 39.8                 | 0.40                  | 3.95                                 | 10.403                        | 0.38                          | 0.01        | 0.65        | ...         | ...         | 0.42        | 0.15        |
| 05273778-6727305 | 277.694     | -32.898     | 1.562      | 8            | -          | -          | -           | -          | -           | -             | -           | -                      | -            | -           | -           | -           | -           | 11.536                                | 0.69                               | 1.05                        | -2                          | 22.4                 | 0.64                  | 3.73                                 | 10.954                        | 0.44                          | 0.28        | 0.48        | ...         | ...         | 0.47        | 0.38        |
| 05312290-7104136 | 281.863     | -32.014     | 2.492      | 8            | -          | -          | -           | -          | -           | -             | -           | -                      | -            | -           | -           | -           | -           | 10.747                                | 0.53                               | 1.05                        | 1                           | 34.6                 | 0.66                  | 3.89                                 | 9.818                         | 0.12                          | -0.19       | 0.77        | ...         | ...         | 0.17        | -0.03       |
| 05312551-7104173 | 281.864     | -32.011     | 2.468      | 9            | -          | -          | -           | -          | -           | -             | -           | -                      | -            | -           | -           | -           | -           | 10.168                                | 0.57                               | 1.01                        | 1                           | 121.0                | 0.28                  | 3.89                                 | 9.248                         | 0.16                          | -0.21       | 0.76        | ...         | ...         | 0.21        | -0.05       |
| 05313143+1256341 | 191.955     | -11.199     | 1.135      | 8            | -          | -          | -           | -          | -           | -             | -           | -                      | -            | -           | -           | -           | -           | 11.671                                | 1.32                               | ...                         | 1                           | 68.4                 | 0.20                  | 3.30                                 | 11.248                        | 1.13                          | ...         | 0.35        | ...         | ...         | 1.15        | ...         |
| 05322744-6741370 | 277.898     | -32.410     | 2.677      | 7            | -          | -          | -           | -          | -           | -             | -           | -                      | -            | -           | -           | -           | -           | 10.735                                | ...                                | ...                         | -2                          | 47.2                 | 1.00                  | 3.72                                 | 9.738                         | ...                           | ...         | 0.83        | ...         | ...         | ...         | ...         |
| 05323071-6627375 | 276.445     | -32.550     | 1.041      | 9            | -          | -          | -           | -          | -           | -             | -           | -                      | -            | -           | -           | -           | -           | 11.329                                | 0.62                               | 0.84                        | 1                           | 50.6                 | 0.44                  | 3.58                                 | 10.941                        | 0.45                          | 0.33        | 0.32        | ...         | ...         | 0.47        | 0.40        |
| 05325276-6946228 | 280.328     | -32.092     | 1.282      | 7            | -          | -          | -           | -          | -           | -             | -           | -                      | -            | -           | -           | -           | -           | 11.153                                | 0.73                               | 1.38                        | 1                           | 23.8                 | 0.74                  | 4.24                                 | 10.675                        | 0.52                          | 0.75        | 0.40        | ...         | ...         | 0.54        | 0.83        |
| 05334194-6845577 | 279.139     | -32.159     | 1.233      | 7            | -          | p          |             |            |             |               |             |                        |              |             |             |             |             |                                       |                                    |                             |                             |                      |                       |                                      |                               |                               |             |             |             |             |             |             |

Table B1: b) continued.

| 2MASX J          | <i>l</i> | <i>b</i> | EBV    | Object | Sample | Disc | 2MRS | Velocity | NIR | Photom | Ext  | <i>K</i> <sub>20</sub> | <i>H-K</i> | <i>J-K</i> | vc   | <i>a</i> | <i>b/a</i> | st.d. | <i>K</i> <sub>s</sub> <sup>o</sup> | ( <i>H-K</i> ) <sup>o</sup> | ( <i>J-K</i> ) <sup>o</sup> | <i>A<sub>K</sub></i> | <i>a</i> <sub>d</sub> <sup>o</sup> | <i>K</i> <sub>s</sub> <sup>o,d</sup> | ( <i>H-K</i> ) <sup>o,c</sup> | ( <i>J-K</i> ) <sup>o,c</sup> |        |      |      |      |      |      |      |
|------------------|----------|----------|--------|--------|--------|------|------|----------|-----|--------|------|------------------------|------------|------------|------|----------|------------|-------|------------------------------------|-----------------------------|-----------------------------|----------------------|------------------------------------|--------------------------------------|-------------------------------|-------------------------------|--------|------|------|------|------|------|------|
| (1)              | deg      | deg      | (mag)  | class  | off    | flag | gal  | TF       | obs | ext'd  | type | (9)                    | Opt        | HI         | (11) | flag     | flag       | flag  | (14)                               | (15)                        | (16)                        | (17)                 | (18)                               | (19)                                 | (20)                          | (21)                          | (22)   | (23) | (24) | (25) | (26) | (27) | (28) |
| 05350582–0523155 | 208.988  | –19.423  | 37.389 | 9      | –      | –    | –    | –        | –   | –      | –    | –                      | 7.032      | 1.66       | 1.34 | 1        | 219.4      | 0.38  | 3.85                               | –6.899                      | –4.54                       | –17.24               | 11.58                              | ...                                  | ...                           | –3.80                         | –14.77 |      |      |      |      |      |      |
| 05350615–0519555 | 208.936  | –19.396  | 36.634 | 9      | –      | –    | –    | –        | –   | –      | –    | –                      | 9.506      | 1.56       | 1.08 | 1        | 124.4      | 0.56  | 3.85                               | –4.144                      | –4.50                       | –17.12               | 11.35                              | ...                                  | ...                           | –3.79                         | –14.71 |      |      |      |      |      |      |
| 05350622–0527535 | 209.062  | –19.456  | 25.011 | 9      | –      | –    | –    | –        | –   | –      | –    | –                      | 11.287     | 1.05       | 3.29 | 1        | 69.4       | 0.32  | 3.85                               | –1.968                      | –3.09                       | –9.13                | 7.75                               | ...                                  | ...                           | –2.60                         | –7.48  |      |      |      |      |      |      |
| 05350648–0517225 | 208.896  | –19.376  | 30.292 | 9      | –      | –    | –    | –        | –   | –      | –    | –                      | 9.352      | 0.70       | 2.41 | 1        | 116.6      | 0.44  | 3.58                               | –1.935                      | –4.32                       | –12.64               | 9.38                               | ...                                  | ...                           | –3.72                         | –10.64 |      |      |      |      |      |      |
| 05350649–0521185 | 208.958  | –19.405  | 38.337 | 9      | –      | –    | –    | –        | –   | –      | –    | –                      | 6.881      | 1.52       | 1.22 | 1        | 219.2      | 0.90  | 3.85                               | –7.403                      | –4.83                       | –17.82               | 11.88                              | ...                                  | ...                           | –4.07                         | –15.29 |      |      |      |      |      |      |
| 05350810–0453318 | 208.524  | –19.189  | 8.286  | 9      | –      | –    | –    | –        | –   | –      | –    | –                      | 10.108     | 1.28       | ...  | 1        | 106.0      | 0.76  | 3.73                               | 7.021                       | –0.09                       | ...                  | 2.57                               | ...                                  | ...                           | 0.07                          | ...    |      |      |      |      |      |      |
| 05350857–0526188 | 209.041  | –19.435  | 33.849 | 9      | –      | –    | –    | –        | –   | –      | –    | –                      | 6.224      | 1.20       | 1.77 | 1        | 164.0      | 1.00  | 4.13                               | –6.388                      | –4.41                       | –15.05               | 10.48                              | ...                                  | ...                           | –3.75                         | –12.81 |      |      |      |      |      |      |
| 05350903–0520119 | 208.946  | –19.388  | 40.055 | 9      | –      | –    | –    | –        | –   | –      | –    | –                      | 6.134      | 1.17       | 1.52 | 1        | 221.0      | 0.28  | 4.17                               | –8.790                      | –5.46                       | –18.38               | 12.41                              | ...                                  | ...                           | –4.67                         | –15.74 |      |      |      |      |      |      |
| 05350950–0520588 | 208.959  | –19.392  | 42.004 | 9      | –      | –    | –    | –        | –   | –      | –    | –                      | 4.818      | 1.07       | 1.54 | 1        | 212.2      | 0.42  | 4.17                               | –10.833                     | –5.88                       | –19.33               | 13.01                              | ...                                  | ...                           | –5.06                         | –16.55 |      |      |      |      |      |      |
| 05351111–0455288 | 208.561  | –19.193  | 7.942  | 9      | –      | –    | –    | –        | –   | –      | –    | –                      | 12.378     | ...        | ...  | 1        | 48.0       | 0.22  | 3.73                               | 9.419                       | ...                         | ...                  | 2.46                               | ...                                  | ...                           | ...                           | ...    |      |      |      |      |      |      |
| 05351191–0520018 | 208.949  | –19.376  | 42.746 | 9      | –      | –    | –    | –        | –   | –      | –    | –                      | 7.947      | 1.62       | 0.78 | 1        | 82.4       | 0.72  | 4.17                               | –7.980                      | –5.46                       | –20.45               | 13.24                              | ...                                  | ...                           | –4.62                         | –17.63 |      |      |      |      |      |      |
| 05351251–0456029 | 208.573  | –19.192  | 7.882  | 9      | –      | –    | –    | –        | –   | –      | –    | –                      | 10.276     | 1.58       | ...  | 1        | 72.6       | 0.36  | 3.73                               | 7.339                       | 0.27                        | ...                  | 2.44                               | ...                                  | ...                           | 0.43                          | ...    |      |      |      |      |      |      |
| 05351272–0519359 | 208.944  | –19.369  | 42.939 | 9      | –      | –    | –    | –        | –   | –      | –    | –                      | 6.579      | 1.41       | 1.09 | 1        | 220.0      | 0.24  | 4.17                               | –9.420                      | –5.70                       | –20.24               | 13.30                              | ...                                  | ...                           | –4.85                         | –17.40 |      |      |      |      |      |      |
| 05351506–0500058 | 208.641  | –19.213  | 4.922  | 8      | –      | –    | –    | –        | –   | –      | –    | –                      | 12.997     | 1.43       | ...  | 1        | 25.8       | 0.20  | 3.73                               | 11.163                      | 0.61                        | ...                  | 1.52                               | ...                                  | ...                           | 0.71                          | ...    |      |      |      |      |      |      |
| 05351526–0520288 | 208.963  | –19.367  | 45.692 | 9      | –      | –    | –    | –        | –   | –      | –    | –                      | 4.777      | 1.04       | 1.80 | 1        | 141.0      | 0.90  | 4.17                               | –12.248                     | –6.53                       | –20.90               | 14.15                              | ...                                  | ...                           | –5.63                         | –17.88 |      |      |      |      |      |      |
| 05351532–0457458 | 208.605  | –19.195  | 6.432  | 8      | –      | –    | –    | –        | –   | –      | –    | –                      | 11.883     | 1.14       | ...  | 1        | 48.2       | 0.56  | 3.73                               | 9.486                       | 0.08                        | ...                  | 1.99                               | ...                                  | ...                           | 0.21                          | ...    |      |      |      |      |      |      |
| 05351647–0506008 | 208.737  | –19.253  | 6.083  | 8      | –      | –    | –    | –        | –   | –      | –    | –                      | 11.535     | 1.69       | 2.46 | 1        | 47.2       | 0.58  | 3.73                               | 9.268                       | 0.68                        | –0.56                | 1.88                               | ...                                  | ...                           | 0.80                          | –0.16  |      |      |      |      |      |      |
| 05351700–0520118 | 208.962  | –19.358  | 46.253 | 9      | –      | –    | –    | –        | –   | –      | –    | –                      | 6.021      | 1.08       | 1.41 | 1        | 220.0      | 0.36  | 4.17                               | –11.213                     | –6.58                       | –21.57               | 14.33                              | ...                                  | ...                           | –5.67                         | –18.52 |      |      |      |      |      |      |
| 05351746–0438588 | 208.315  | –19.044  | 2.567  | 8      | –      | –    | –    | –        | –   | –      | –    | –                      | 11.574     | 0.65       | 1.63 | 1        | 55.4       | 0.80  | 3.59                               | 10.618                      | 0.22                        | 0.36                 | 0.80                               | ...                                  | ...                           | 0.27                          | 0.53   |      |      |      |      |      |      |
| 05351820–0500338 | 208.655  | –19.205  | 4.818  | 8      | –      | –    | –    | –        | –   | –      | –    | –                      | 9.924      | 1.92       | 3.90 | 1        | 58.4       | 0.44  | 3.73                               | 8.129                       | 1.12                        | 1.51                 | 1.49                               | ...                                  | ...                           | 1.22                          | 1.83   |      |      |      |      |      |      |
| 05351854–0455098 | 208.571  | –19.163  | 7.662  | 9      | –      | –    | –    | –        | –   | –      | –    | –                      | 11.827     | ...        | ...  | 1        | 35.8       | 1.00  | 3.73                               | 8.972                       | ...                         | ...                  | 2.37                               | ...                                  | ...                           | ...                           | ...    |      |      |      |      |      |      |
| 05351855–0526248 | 209.063  | –19.399  | 38.564 | 9      | –      | –    | –    | –        | –   | –      | –    | –                      | 5.032      | 1.33       | 1.93 | 1        | 213.6      | 1.00  | 4.13                               | –9.337                      | –5.06                       | –17.23               | 11.95                              | ...                                  | ...                           | –4.30                         | –14.69 |      |      |      |      |      |      |
| 05351981–0515088 | 208.888  | –19.310  | 29.860 | 8      | –      | –    | –    | –        | –   | –      | –    | –                      | 9.500      | 1.62       | 4.24 | 1        | 79.2       | 1.00  | 4.17                               | –1.626                      | –3.33                       | –10.60               | 9.25                               | ...                                  | ...                           | –2.74                         | –8.63  |      |      |      |      |      |      |
| 05352068–0519268 | 208.957  | –19.339  | 46.614 | 9      | –      | –    | –    | –        | –   | –      | –    | –                      | 12.242     | ...        | 2.88 | 1        | 10.0       | 1.00  | 4.17                               | –5.126                      | ...                         | –20.28               | 14.44                              | ...                                  | ...                           | ...                           | –17.21 |      |      |      |      |      |      |
| 05352148–0501158 | 208.673  | –19.198  | 4.674  | 9      | –      | –    | –    | –        | –   | –      | –    | –                      | 12.359     | ...        | ...  | 1        | 19.6       | 0.50  | 3.73                               | 10.617                      | ...                         | ...                  | 1.45                               | ...                                  | ...                           | ...                           | ...    |      |      |      |      |      |      |
| 05352163–0526578 | 209.077  | –19.392  | 36.294 | 9      | –      | –    | –    | –        | –   | –      | –    | –                      | 9.283      | 0.92       | 1.18 | 1        | 53.6       | 0.14  | 4.13                               | –4.240                      | –5.09                       | –16.85               | 11.24                              | ...                                  | ...                           | –4.38                         | –14.45 |      |      |      |      |      |      |
| 05352177–6734329 | 277.721  | –32.150  | 3.259  | 9      | –      | –    | –    | –        | –   | –      | –    | –                      | 9.115      | 0.84       | 1.23 | 1        | 142.8      | 0.32  | 3.66                               | 7.901                       | 0.30                        | –0.39                | 1.01                               | ...                                  | ...                           | 0.37                          | –0.18  |      |      |      |      |      |      |
| 05352269–0519478 | 208.967  | –19.334  | 47.089 | 9      | –      | –    | –    | –        | –   | –      | –    | –                      | 6.763      | 1.34       | 1.84 | 1        | 126.4      | 0.50  | 4.17                               | –10.782                     | –6.46                       | –21.55               | 14.59                              | ...                                  | ...                           | –5.54                         | –18.45 |      |      |      |      |      |      |
| 05352329–0507078 | 208.769  | –19.236  | 8.141  | 7      | –      | –    | –    | –        | –   | –      | –    | –                      | 11.757     | 1.60       | ...  | 1        | 24.0       | 0.64  | 3.73                               | 8.724                       | 0.25                        | ...                  | 2.52                               | ...                                  | ...                           | 0.41                          | ...    |      |      |      |      |      |      |
| 05352416–0505518 | 208.750  | –19.223  | 7.075  | 8      | –      | –    | –    | –        | –   | –      | –    | –                      | 12.030     | 1.62       | 3.53 | 1        | 32.2       | 0.42  | 3.73                               | 9.394                       | 0.45                        | 0.01                 | 2.19                               | ...                                  | ...                           | 0.59                          | 0.48   |      |      |      |      |      |      |
| 05352423–0504068 | 208.723  | –19.210  | 5.489  | 9      | –      | –    | –    | –        | –   | –      | –    | –                      | 11.121     | 0.29       | 1.19 | 1        | 52.0       | 0.70  | 3.73                               | 9.076                       | –0.62                       | –1.53                | 1.70                               | ...                                  | ...                           | –0.51                         | –1.17  |      |      |      |      |      |      |
| 05352430–0526478 | 209.080  | –19.381  | 36.158 | 9      | –      | –    | –    | –        | –   | –      | –    | –                      | 6.021      | 1.77       | 1.67 | 1        | 219.2      | 0.38  | 4.13                               | –7.451                      | –4.21                       | –16.30               | 11.20                              | ...                                  | ...                           | –3.50                         | –13.97 |      |      |      |      |      |      |
| 05352443–0521068 | 208.991  | –19.337  | 47.530 | 9      | –      | –    | –    | –        | –   | –      | –    | –                      | 5.293      | 1.14       | 2.09 | 1        | 218.2      | 0.88  | 4.17                               | –12.417                     | –6.73                       | –21.53               | 14.72                              | ...                                  | ...                           | –5.80                         | –18.39 |      |      |      |      |      |      |
| 05352490–0510278 | 208.824  | –19.255  | 13.817 | 9      | –      | –    | –    | –        | –   | –      | –    | –                      | 6.531      | 1.88       | 3.68 | 1        | 232.8      | 0.64  | 4.17                               | 1.383                       | –0.41                       | –3.18                | 4.28                               | ...                                  | ...                           | –0.14                         | –2.27  |      |      |      |      |      |      |
| 05352577–0505578 | 208.755  | –19.218  | 7.184  | 9      | –      | –    | –    | –        | –   | –      | –    | –                      | 11.671     | 1.21       | 3.03 | 1        | 30.6       | 0.46  | 3.73                               | 8.994                       | 0.02                        | –0.53                | 2.23                               | ...                                  | ...                           | 0.16                          | –0.06  |      |      |      |      |      |      |
| 05352670–0503548 | 208.725  | –19.199  | 5.381  | 9      | –      | –    | –    | –        | –   | –      | –    | –                      | 7.906      | 0.81       | 2.04 | 1        | 194.0      | 0.28  | 3.73                               | 5.901                       | –0.08                       | –0.63                | 1.67                               | ...                                  | ...                           | 0.03                          | –0.28  |      |      |      |      |      |      |
| 05352818–0515508 | 208.915  | –19.284  | 32.164 | 9      | –      | –    | –    | –        | –   | –      | –    | –                      | 6.500      | 1.11       | 1.51 | 1        | 211.6      | 0.76  | 4.17                               | –5.484                      | –4.22                       | –14.47               | 9.96                               | ...                                  | ...                           | –3.59                         | –12.35 |      |      |      |      |      |      |
| 05352987–0626581 | 210.042  | –19.811  | 2.269  | 7      | –      | –    | –    | –        | –   | –      | –    | –                      | 11.521     | 1.04       | 2.45 | 1        | 38.4       | 0.44  | 3.37                               | 10.676                      | 0.66                        | 1.32                 | 0.70                               | ...                                  | ...                           | 0.70                          | 1.47   |      |      |      |      |      |      |
| 05353073–0521468 | 209.014  | –19.319  | 44.076 | 9      | –      | –    | –    | –        | –   | –      | –    | –                      | 7.313      | 1.79       | 2.22 | 1        | 110.2      | 0.44  | 4.17                               | –9.110                      | –5.51                       | –19.68               | 13.65                              | ...                                  | ...                           | –4.65                         | –16.77 |      |      |      |      |      |      |
| 05353094–0626321 | 210.037  | –19.804  | 2.237  | 8      | –      | –    | –    | –        | –   | –      | –    | –                      | 10.956     | 0.56       | 1.76 | 1        | 57.0       | 0.60  | 3.37                               | 10.122                      | 0.19                        | 0.65                 | 0.69                               | ...                                  | ...                           | 0.23                          | 0.80   |      |      |      |      |      |      |
| 05353100–0525438 | 209.077  | –19.348  | 37.147 | 9      | –      | –    | –    | –        | –   | –      | –    | –                      | 6.142      | 1.58       | 1.47 | 1        | 218.2      | 0.40  | 4.13                               | –7.699                      | –4.57                       | –16.98               | 11.51                              | ...                                  | ...                           | –3.84                         | –14.55 |      |      |      |      |      |      |
| 05353225–0521505 | 209.018  | –19.314  | 42.532 | 9      | –      | –    | –    | –        | –   | –      | –    | –                      | 8.708      | 1.60       | 2.65 | 1        | 64.6       | 0.80  | 3.59                               | –7.139                      | –5.45                       | –18.48               | 13.17                              | ...                                  | ...                           | –4.61                         | –15.67 |      |      |      |      |      |      |
| 05353360–0515228 | 208.919  | –19.260  | 26.210 | 9      | –      | –    | –    | –        | –   | –      | –    | –                      | 9.646      | 0.75       | 1.25 | 1        | 84.2       | 0.12  | 4.17                               | –0.120                      | –3.59                       | –11.77               | 8.12                               | ...                                  | ...                           | –3.07                         | –10.04 |      |      |      |      |      |      |
| 05353380–0504278 | 208.748  | –19.177  | 5.274  | 7      | –      | –    | –    | –        | –   | –      | –    | –                      | 10.381     | 1.25       | 3.21 | 1        | 17.4       | 0.76  | 3.73                               | 8.416                       | 0.37                        | 0.59                 | 1.63                               | ...                                  | ...                           | 0.48                          | 0.94   |      |      |      |      |      |      |
| 05353386–0517105 | 208.948  | –19.273  | 29.577 | 8      | –      | –    | –    | –        | –   | –      | –    | –                      | 12.561     | 0.57       | 1.13 | 1        | 16.6       | 0.66  | 3.70                               | 1.541                       | –4.33                       | –13.56               | 9.16                               | ...                                  | ...                           | –3.75                         | –11.61 |      |      |      |      |      |      |
| 05353406–0521265 | 209.015  | –19.304  | 40.449 | 9      | –      | –    | –    | –        | –   | –      | –    | –                      | 9.505      | ...        | ...  | 1        | 129.2      | 0.16  | 3.59                               | –5.566                      | ...                         | ...                  | 12.53                              | ...                                  | ...                           | ...                           | ...    |      |      |      |      |      |      |
| 05353417–6735319 | 277.738  | –32.128  | 3.330  | 9      | –      | –    | –    | –        | –   | –      | –    | –                      | 11.789     | 0.93       | 0.93 | –2       | 78.0       | 0.52  | 3.66                               | 10.548                      | 0.38                        | –0.73                | 1.03                               | ...                                  | ...                           | 0.44                          | –0.51  |      |      |      |      |      |      |
| 05353439–0518385 | 208.972  | –19.282  | 33.269 | 9      | –      | –    | –    | –        | –   | –      | –    | –                      | 9.913      | 1.02       | 3.88 | 1        | 70.6       | 0.32  | 3.70                               | –2.483                      | –4.49                       | –12.65               | 10.31                              | ...                                  | ...                           | –3.84                         | –10.46 |      |      |      |      |      |      |
| 05353446–0514045 | 208.900  | –19.247  | 21.638 | 9      | –      | –    | –    |          |     |        |      |                        |            |            |      |          |            |       |                                    |                             |                             |                      |                                    |                                      |                               |                               |        |      |      |      |      |      |      |

Table B1: b) continued.

| 2MASX J          | <i>l</i>    | <i>b</i>    | EBV        | Object       | Sample     | Disc        | 2MRS        | Velocity   | NIR         | Photom        | Ext         | <i>K</i> <sub>20</sub> | <i>H-K</i>   | <i>J-K</i>  | vc           | <i>a</i>     | <i>b/a</i>   | st.d.       | <i>K</i> <sub>s</sub> <sup>O</sup> | ( <i>H-K</i> ) <sup>O</sup> | ( <i>J-K</i> ) <sup>O</sup> | <i>A</i> <sub>K</sub> | <i>a</i> <sub>d</sub> | <i>K</i> <sub>s</sub> <sup>O,d</sup> | ( <i>H-K</i> ) <sup>O,c</sup> | ( <i>J-K</i> ) <sup>O,c</sup> |             |             |             |             |             |             |        |
|------------------|-------------|-------------|------------|--------------|------------|-------------|-------------|------------|-------------|---------------|-------------|------------------------|--------------|-------------|--------------|--------------|--------------|-------------|------------------------------------|-----------------------------|-----------------------------|-----------------------|-----------------------|--------------------------------------|-------------------------------|-------------------------------|-------------|-------------|-------------|-------------|-------------|-------------|--------|
| (1)              | deg<br>(2a) | deg<br>(2b) | mag<br>(3) | class<br>(4) | off<br>(5) | flag<br>(6) | gal<br>(7a) | TF<br>(7b) | obs<br>(7c) | ext'd<br>(7d) | type<br>(8) | (9)                    | Opt<br>(10a) | HI<br>(10b) | flag<br>(11) | flag<br>(12) | flag<br>(13) | mag<br>(14) | mag<br>(15)                        | mag<br>(16)                 | (17)                        | (18)                  | (19)                  | (20)                                 | mag<br>(21)                   | mag<br>(22)                   | mag<br>(23) | mag<br>(24) | mag<br>(25) | mag<br>(26) | mag<br>(27) | mag<br>(28) |        |
| 05360378–0525485 | 209.143     | −19.227     | 8.453      | 9            | –          | –           | –           | –          | –           | –             | –           | –                      | –            | –           | –            | –            | –            | –           | 12.662                             | 0.55                        | 1.58                        | 1                     | 49.6                  | 0.34                                 | 3.27                          | 9.512                         | −0.85       | −2.62       | 2.62        | ...         | ...         | −0.68       | −2.06  |
| 05360613–0525395 | 209.145     | −19.217     | 7.376      | 9            | –          | –           | –           | –          | –           | –             | –           | –                      | –            | –           | –            | –            | –            | –           | 12.755                             | 0.82                        | 1.59                        | −2                    | 29.2                  | 0.54                                 | 3.27                          | 10.007                        | −0.40       | −2.08       | 2.28        | ...         | ...         | −0.26       | −1.59  |
| 05361713–0638070 | 210.312     | −19.719     | 3.788      | 7            | –          | –           | –           | –          | –           | –             | –           | –                      | –            | –           | –            | –            | –            | –           | 12.305                             | 0.93                        | 2.77                        | 1                     | 26.2                  | 0.70                                 | 3.21                          | 10.894                        | 0.31        | 0.89        | 1.17        | ...         | ...         | 0.38        | 1.14   |
| 05361732–0622520 | 210.070     | −19.605     | 1.988      | 9            | –          | –           | –           | –          | –           | –             | –           | –                      | –            | –           | –            | –            | –            | –           | 11.699                             | ...                         | ...                         | 1                     | 36.4                  | 1.0                                  | 3.39                          | 10.958                        | ...         | ...         | 0.62        | ...         | ...         | ...         | ...    |
| 05361886–0622040 | 210.061     | −19.593     | 1.941      | 9            | –          | –           | –           | –          | –           | –             | –           | –                      | –            | –           | –            | –            | –            | –           | 10.098                             | 1.11                        | 2.23                        | 1                     | 80.8                  | 0.36                                 | 3.39                          | 9.375                         | 0.79        | 1.26        | 0.60        | ...         | ...         | 0.82        | 1.39   |
| 05362076–0645140 | 210.431     | −19.758     | 5.095      | 8            | –          | –           | –           | –          | –           | –             | –           | –                      | –            | –           | –            | –            | –            | –           | 12.777                             | 0.71                        | 1.30                        | 1                     | 31.4                  | 0.32                                 | 3.21                          | 10.879                        | −0.13       | −1.23       | 1.58        | ...         | ...         | −0.03       | −0.90  |
| 05362382–0623110 | 210.088     | −19.583     | 2.170      | 7            | –          | –           | –           | –          | –           | –             | –           | –                      | –            | –           | –            | –            | –            | –           | 10.720                             | 1.05                        | 2.24                        | 1                     | 29.2                  | 0.54                                 | 3.39                          | 9.911                         | 0.69        | 1.16        | 0.67        | ...         | ...         | 0.74        | 1.31   |
| 05362483–0625070 | 210.121     | −19.594     | 2.348      | 8            | –          | –           | –           | –          | –           | –             | –           | –                      | –            | –           | –            | –            | –            | –           | 10.291                             | 1.04                        | 2.45                        | 1                     | 70.4                  | 0.32                                 | 3.39                          | 9.416                         | 0.65        | 1.28        | 0.73        | ...         | ...         | 0.70        | 1.44   |
| 05362562–0647154 | 210.473     | −19.755     | 4.173      | 9            | –          | –           | –           | –          | –           | –             | –           | –                      | –            | –           | –            | –            | –            | –           | 12.183                             | 0.74                        | 1.26                        | 1                     | 29.2                  | 0.52                                 | 3.26                          | 10.628                        | 0.05        | −0.81       | 1.29        | ...         | ...         | 0.13        | −0.54  |
| 05362588–0624584 | 210.121     | −19.589     | 2.365      | 8            | –          | –           | –           | –          | –           | –             | –           | –                      | –            | –           | –            | –            | –            | –           | 10.239                             | 1.62                        | 4.14                        | 1                     | 47.4                  | 0.76                                 | 3.13                          | 9.358                         | 1.23        | 2.96        | 0.73        | ...         | ...         | 1.28        | 3.12   |
| 05362653–0647120 | 210.474     | −19.752     | 4.172      | 9            | –          | –           | –           | –          | –           | –             | –           | –                      | –            | –           | –            | –            | –            | –           | 11.980                             | 1.15                        | 1.81                        | 1                     | 47.6                  | 0.54                                 | 3.16                          | 10.426                        | 0.46        | −0.26       | 1.29        | ...         | ...         | 0.54        | 0.01   |
| 05364402–6734569 | 277.712     | −32.019     | 1.513      | 1            | –          | –           | g           | t          | –           | –             | D1          | c                      | o            | –           | –            | –            | e?           | 11.347      | 0.32                               | 1.20                        | 1                           | 49.0                  | 0.24                  | 3.62                                 | 10.783                        | 0.07                          | 0.45        | 0.47        | 57.3        | 10.76       | 0.10        | 0.55        |        |
| 05375004–6911075 | 279.574     | −31.739     | 12.931     | 9            | –          | –           | –           | –          | –           | –             | –           | –                      | –            | –           | –            | –            | –            | –           | 9.610                              | 0.86                        | 1.39                        | 1                     | 143.2                 | 0.64                                 | 4.03                          | 4.792                         | −1.28       | −5.03       | 4.01        | ...         | ...         | −1.03       | −4.18  |
| 05375082–0647161 | 210.640     | −19.440     | 3.048      | 9            | –          | –           | –           | –          | –           | –             | –           | –                      | –            | –           | –            | –            | –            | –           | 10.848                             | 1.25                        | 3.25                        | 1                     | 46.2                  | 0.54                                 | 3.15                          | 9.712                         | 0.74        | 1.74        | 0.94        | ...         | ...         | 0.80        | 1.94   |
| 05375737–6907505 | 279.509     | −31.735     | 20.140     | 9            | –          | –           | –           | –          | –           | –             | –           | –                      | –            | –           | –            | –            | –            | –           | 11.372                             | 0.75                        | 1.32                        | 1                     | 72.2                  | 0.36                                 | 4.03                          | 3.868                         | −2.58       | −8.69       | 6.24        | ...         | ...         | −2.19       | −7.36  |
| 05380749–0708290 | 211.008     | −19.535     | 3.599      | 9            | –          | –           | –           | –          | –           | –             | –           | –                      | –            | –           | –            | –            | –            | –           | 10.650                             | 1.50                        | 3.69                        | 1                     | 32.6                  | 0.70                                 | 3.13                          | 9.309                         | 0.90        | 1.90        | 1.11        | ...         | ...         | 0.97        | 2.14   |
| 05381098–0709260 | 211.030     | −19.529     | 3.642      | 9            | –          | –           | –           | –          | –           | –             | –           | –                      | –            | –           | –            | –            | –            | –           | 11.438                             | 2.19                        | 2.46                        | 1                     | 37.4                  | 0.58                                 | 3.13                          | 10.081                        | 1.58        | 0.65        | 1.13        | ...         | ...         | 1.65        | 0.89   |
| 05381473–6903295 | 279.421     | −31.717     | 24.188     | 8            | –          | –           | –           | –          | –           | –             | –           | –                      | –            | –           | –            | –            | –            | –           | 12.498                             | 0.42                        | 0.95                        | −2                    | 18.6                  | 0.16                                 | 4.03                          | 3.486                         | −3.59       | −11.07      | 7.49        | ...         | ...         | −3.11       | −9.47  |
| 05382530–6902435 | 279.404     | −31.703     | 24.082     | 9            | –          | –           | –           | –          | –           | –             | –           | –                      | –            | –           | –            | –            | –            | –           | 13.678                             | 0.43                        | 1.19                        | −1                    | 12.4                  | 0.48                                 | 3.97                          | 4.705                         | −3.56       | −10.77      | 7.49        | ...         | ...         | −3.09       | −9.19  |
| 05382659–6903116 | 279.413     | −31.700     | 25.424     | 9            | –          | –           | –           | –          | –           | –             | –           | –                      | –            | –           | –            | –            | –            | –           | 11.954                             | 0.65                        | 0.98                        | 1                     | 55.0                  | 0.34                                 | 3.97                          | 2.481                         | −3.56       | −11.65      | 7.88        | ...         | ...         | −3.06       | −9.97  |
| 05382928–6903414 | 279.422     | −31.696     | 26.851     | 8            | –          | –           | –           | –          | –           | –             | –           | –                      | –            | –           | –            | –            | –            | –           | 11.995                             | 0.77                        | 0.86                        | −2                    | 28.8                  | 0.48                                 | 4.03                          | 1.990                         | −3.68       | −12.48      | 8.32        | ...         | ...         | −3.15       | −10.71 |
| 05383165–6909373 | 279.537     | −31.681     | 20.204     | 9            | –          | –           | –           | –          | –           | –             | –           | –                      | –            | –           | –            | –            | –            | –           | 12.942                             | 0.41                        | ...                         | 1                     | 34.8                  | 0.14                                 | 4.03                          | 5.414                         | −2.94       | ...         | 6.26        | ...         | ...         | −2.54       | ...    |
| 05383167–6902143 | 279.393     | −31.695     | 22.562     | 7            | –          | –           | –           | –          | –           | –             | –           | –                      | –            | –           | –            | –            | –            | –           | 11.265                             | 1.02                        | 2.07                        | 1                     | 35.6                  | 0.56                                 | 4.03                          | 2.858                         | −2.71       | −9.14       | 6.99        | ...         | ...         | −2.27       | −7.65  |
| 05383184–6907417 | 279.499     | −31.684     | 26.273     | 9            | –          | –           | –           | –          | –           | –             | –           | –                      | –            | –           | –            | –            | –            | –           | 11.199                             | 0.86                        | 1.26                        | 1                     | 56.2                  | 0.44                                 | 3.99                          | 1.410                         | −3.49       | −11.79      | 8.14        | ...         | ...         | −2.97       | −10.05 |
| 05383269–6910197 | 279.550     | −31.678     | 17.987     | 9            | –          | –           | –           | –          | –           | –             | –           | –                      | –            | –           | –            | –            | –            | –           | 11.505                             | 0.81                        | 1.01                        | 1                     | 50.6                  | 0.38                                 | 3.99                          | 4.803                         | −2.17       | −7.93       | 5.57        | ...         | ...         | −1.82       | −6.74  |
| 05383290–6906553 | 279.484     | −31.684     | 28.681     | 9            | –          | –           | –           | –          | –           | –             | –           | –                      | –            | –           | –            | –            | –            | –           | 8.987                              | 0.74                        | 1.05                        | 1                     | 73.2                  | 0.74                                 | 4.03                          | −1.700                        | −4.01       | −13.20      | 8.88        | ...         | ...         | −3.45       | −11.30 |
| 05383396–6905457 | 279.461     | −31.685     | 29.524     | 9            | –          | –           | –           | –          | –           | –             | –           | cr                     | –            | –           | –            | –            | –            | –           | 7.490                              | 0.61                        | 0.80                        | 1                     | 140.4                 | 0.74                                 | 3.97                          | −3.511                        | −4.28       | −13.86      | 9.15        | ...         | ...         | −3.70       | −11.92 |
| 05383470–6905577 | 279.465     | −31.683     | 29.480     | 9            | –          | –           | –           | –          | –           | –             | –           | cr                     | –            | –           | –            | –            | –            | –           | 7.053                              | 0.75                        | 0.92                        | 1                     | 220.0                 | 0.76                                 | 3.99                          | −3.931                        | −4.13       | −13.73      | 9.13        | ...         | ...         | −3.55       | −11.78 |
| 05383549–6904437 | 279.441     | −31.684     | 30.164     | 9            | –          | –           | –           | –          | –           | –             | –           | cr                     | –            | –           | –            | –            | –            | –           | 10.056                             | 0.79                        | 0.67                        | 1                     | 67.4                  | 0.36                                 | 3.97                          | −1.183                        | −4.21       | −14.32      | 9.34        | ...         | ...         | −3.62       | −12.33 |
| 05383551–6910047 | 279.545     | −31.674     | 18.733     | 7            | –          | –           | –           | –          | –           | –             | –           | –                      | –            | –           | –            | –            | –            | –           | 13.481                             | 0.60                        | 1.01                        | 1                     | 19.4                  | 0.52                                 | 3.99                          | 6.501                         | −2.50       | −8.30       | 5.80        | ...         | ...         | −2.13       | −7.06  |
| 05383599–6906467 | 279.481     | −31.680     | 29.043     | 9            | –          | –           | –           | –          | –           | –             | –           | –                      | –            | –           | –            | –            | –            | –           | 8.136                              | 0.79                        | 1.01                        | 1                     | 113.4                 | 0.62                                 | 3.99                          | −2.685                        | −4.02       | −13.42      | 9.00        | ...         | ...         | −3.45       | −11.50 |
| 05383741–6900542 | 279.366     | −31.689     | 17.242     | 9            | –          | –           | –           | –          | –           | –             | –           | cr                     | –            | –           | –            | –            | –            | –           | 12.515                             | 0.79                        | 0.96                        | 1                     | 50.6                  | 0.24                                 | 3.88                          | 6.091                         | −2.07       | −7.61       | 5.34        | ...         | ...         | −1.73       | −6.47  |
| 05383796–6903297 | 279.416     | −31.683     | 27.224     | 8            | –          | –           | –           | –          | –           | –             | –           | cr                     | –            | –           | –            | –            | –            | –           | 10.043                             | 0.74                        | 0.70                        | −2                    | 80.8                  | 0.96                                 | 3.97                          | −0.101                        | −3.76       | −12.82      | 8.43        | ...         | ...         | −3.23       | −11.03 |
| 05384025–6908148 | 279.508     | −31.671     | 24.884     | 7            | –          | –           | –           | –          | –           | –             | –           | –                      | –            | –           | –            | –            | –            | –           | 11.726                             | ...                         | 1.24                        | 1                     | 38.0                  | 1.00                                 | 3.99                          | 2.454                         | ...         | −11.12      | 7.71        | ...         | ...         | ...         | −9.48  |
| 05384027–6907328 | 279.495     | −31.672     | 27.056     | 9            | –          | –           | –           | –          | –           | –             | –           | cr                     | –            | –           | –            | –            | –            | –           | 10.064                             | 1.07                        | 1.37                        | 1                     | 59.0                  | 0.54                                 | 3.99                          | −0.017                        | −3.41       | −12.07      | 8.38        | ...         | ...         | −2.88       | −10.28 |
| 05384066–6900218 | 279.355     | −31.685     | 15.426     | 9            | –          | –           | –           | –          | –           | –             | –           | cr                     | –            | –           | –            | –            | –            | –           | 10.696                             | 0.77                        | 0.98                        | 1                     | 117.8                 | 0.22                                 | 3.97                          | 4.948                         | −1.79       | −6.68       | 4.78        | ...         | ...         | −1.48       | −5.66  |
| 05384086–6859368 | 279.340     | −31.686     | 12.936     | 8            | –          | –           | –           | –          | –           | –             | –           | cr                     | –            | –           | –            | –            | –            | –           | 13.083                             | 0.40                        | 1.14                        | 2                     | 16.2                  | 0.58                                 | 3.97                          | 8.263                         | −1.74       | −5.29       | 4.01        | ...         | ...         | −1.48       | −4.43  |
| 05384402–6906598 | 279.483     | −31.668     | 29.183     | 9            | –          | –           | –           | –          | –           | –             | –           | –                      | –            | –           | –            | –            | –            | –           | 7.952                              | 0.71                        | 0.72                        | 1                     | 176.6                 | 0.60                                 | 3.99                          | −2.922                        | −4.13       | −13.78      | 9.04        | ...         | ...         | −3.56       | −11.85 |
| 05384519–6905088 | 279.447     | −31.669     | 30.974     | 9            | –          | –           | –           | –          | –           | –             | –           | –                      | –            | –           | –            | –            | –            | –           | 6.773                              | 0.64                        | 0.71                        | 1                     | 214.6                 | 0.80                                 | 3.97                          | −4.768                        | −4.49       | −14.68      | 9.59        | ...         | ...         | −3.88       | −12.64 |
| 05384652–0705371 | 211.039     | −19.369     | 4.113      | 7            | –          | –           | –           | –          | –           | –             | –           | –                      | –            | –           | –            | –            | –            | –           | 11.924                             | 1.20                        | 3.06                        | 1                     | 23.2                  | 0.54                                 | 3.35                          | 10.391                        | 0.52        | 1.01        | 1.27        | ...         | ...         | 0.60        | 1.28   |
| 05384895–6904109 | 279.427     | −31.666     | 29.995     | 9            | –          | –           | –           | –          | –           | –             | –           | –                      | –            | –           | –            | –            | –            | –           | 9.476                              | 1.16                        | 1.51                        | 1                     | 81.4                  | 0.42                                 | 3.97                          | −1.700                        | −3.81       | −13.40      | 9.29        | ...         | ...         | −3.22       | −11.42 |
| 05385200–6910149 | 279.545     | −31.650     | 18.214     | 9            | –          | –           | –           | –          | –           | –             | –           | –                      | –            | –           | –            | –            | –            | –           | 11.990                             | 0.80                        | 1.04                        | 1                     | 58.                   |                                      |                               |                               |             |             |             |             |             |             |        |

Table B1: b) continued.

| 2MASX J          | <i>l</i>    | <i>b</i>    | EBV        | Object       | Sample     | Disc        | 2MRS        | Velocity   | NIR         | Photom        | Ext         | K <sub>20</sub> | <i>H-K</i>   | <i>J-K</i>  | vc           | <i>a</i>     | <i>b/a</i>   | st.d.                          | K <sub>s</sub> <sup>o</sup> | ( <i>H-K</i> ) <sup>o</sup> | ( <i>J-K</i> ) <sup>o</sup> | A <sub>K</sub> | <i>a</i> <sup>d</sup> | K <sub>s</sub> <sup>o,d</sup> | ( <i>H-K</i> ) <sup>o,c</sup> | ( <i>J-K</i> ) <sup>o,c</sup> |             |             |             |             |             |             |        |     |
|------------------|-------------|-------------|------------|--------------|------------|-------------|-------------|------------|-------------|---------------|-------------|-----------------|--------------|-------------|--------------|--------------|--------------|--------------------------------|-----------------------------|-----------------------------|-----------------------------|----------------|-----------------------|-------------------------------|-------------------------------|-------------------------------|-------------|-------------|-------------|-------------|-------------|-------------|--------|-----|
| (1)              | deg<br>(2a) | deg<br>(2b) | mag<br>(3) | class<br>(4) | off<br>(5) | flag<br>(6) | gal<br>(7a) | TF<br>(7b) | obs<br>(7c) | ext'd<br>(7d) | type<br>(8) | (9)             | Opt<br>(10a) | HI<br>(10b) | flag<br>(11) | flag<br>(12) | flag<br>(13) | K <sub>20</sub><br>mag<br>(14) | <i>H-K</i><br>mag<br>(15)   | <i>J-K</i><br>mag<br>(16)   | (17)                        | (18)           | (19)                  | (20)                          | mag<br>(21)                   | mag<br>(22)                   | mag<br>(23) | mag<br>(24) | mag<br>(25) | mag<br>(26) | mag<br>(27) | mag<br>(28) |        |     |
| 05404982–0806084 | 212.236     | −19.357     | 3.857      | 8            | –          | –           | –           | –          | –           | –             | –           | –               | –            | –           | –            | –            | –            | –                              | 10.435                      | 1.49                        | 2.70                        | 1              | 41.2                  | 0.40                          | 2.95                          | 8.998                         | 0.85        | 0.78        | 1.19        | ...         | ...         | 0.93        | 1.04   |     |
| 05405886–0748034 | 211.967     | −19.191     | 4.455      | 8            | –          | –           | –           | –          | –           | –             | –           | –               | –            | –           | –            | –            | –            | –                              | 11.810                      | 1.02                        | 2.53                        | 1              | 11.8                  | 1.00                          | 3.01                          | 10.150                        | 0.28        | 0.32        | 1.38        | ...         | ...         | 0.37        | 0.61   |     |
| 05410201–0806024 | 212.258     | −19.311     | 4.072      | 7            | –          | –           | –           | –          | –           | –             | –           | –               | –            | –           | –            | –            | –            | –                              | 12.125                      | 1.40                        | ...                         | 1              | 23.4                  | 0.68                          | 2.95                          | 10.608                        | 0.73        | ...         | 1.26        | ...         | ...         | 0.81        | ...    |     |
| 05411245–0751255 | 212.046     | −19.165     | 4.144      | 6            | –          | –           | –           | –          | –           | –             | –           | –               | –            | –           | –            | –            | e            | 12.743                         | 0.83                        | 2.47                        | −2                          | 10.0           | 1.00                  | 3.01                          | 11.199                        | 0.14                          | 0.41        | 1.28        | ...         | ...         | 0.22        | 0.69        |        |     |
| 05411890–0755285 | 212.123     | −19.171     | 3.986      | 7            | –          | –           | –           | –          | –           | –             | –           | –               | –            | –           | –            | –            | –            | –                              | 11.689                      | 1.74                        | ...                         | 1              | 31.6                  | 0.58                          | 3.18                          | 10.204                        | 1.08        | ...         | 1.23        | ...         | ...         | 1.16        | ...    |     |
| 05412462–0754085 | 212.113     | −19.140     | 3.905      | 9            | –          | –           | –           | –          | –           | –             | –           | –               | –            | –           | –            | –            | –            | –                              | 11.558                      | 2.40                        | ...                         | 1              | 28.8                  | 0.40                          | 3.18                          | 10.103                        | 1.75        | ...         | 1.21        | ...         | ...         | 1.83        | ...    |     |
| 05413028–0153205 | 206.493     | −16.395     | 47.475     | 9            | –          | –           | –           | –          | –           | –             | –           | –               | –            | –           | –            | –            | –            | –                              | 12.873                      | 0.67                        | 1.80                        | 1              | 14.2                  | 1.00                          | 3.86                          | −4.816                        | −7.20       | −21.79      | 14.71       | ...         | ...         | −6.26       | −18.66 |     |
| 05413029–0840165 | 212.856     | −19.455     | 3.612      | 8            | –          | –           | –           | –          | –           | –             | –           | –               | –            | –           | –            | –            | –            | –                              | 11.651                      | 2.62                        | ...                         | 1              | 16.2                  | 0.56                          | 3.02                          | 10.305                        | 2.03        | ...         | 1.12        | ...         | ...         | 2.10        | ...    |     |
| 05413088–0153245 | 206.496     | −16.394     | 48.514     | 8            | –          | –           | –           | –          | –           | –             | –           | –               | –            | –           | –            | –            | –            | –                              | 12.143                      | 0.73                        | 1.71                        | 1              | 10.2                  | 1.00                          | 3.86                          | −5.933                        | −7.31       | −22.39      | 15.03       | ...         | ...         | −6.35       | −19.19 |     |
| 05413148–0157575 | 206.567     | −16.427     | 35.064     | 9            | –          | –           | –           | –          | –           | –             | –           | –               | –            | –           | –            | –            | –            | –                              | 13.516                      | 0.81                        | 1.16                        | −2             | 10.0                  | 1.00                          | 3.32                          | 0.451                         | −5.00       | −16.26      | 10.86       | ...         | ...         | −4.31       | −13.95 |     |
| 05413188–0154535 | 206.520     | −16.401     | 51.509     | 9            | –          | –           | –           | –          | –           | –             | –           | –               | –            | –           | –            | –            | –            | –                              | 8.205                       | 1.18                        | 1.97                        | 1              | 68.4                  | 1.00                          | 3.86                          | −10.987                       | −7.35       | −23.62      | 15.96       | ...         | ...         | −6.34       | −20.22 |     |
| 05413282–0152125 | 206.481     | −16.377     | 48.575     | 9            | –          | –           | –           | –          | –           | –             | –           | –               | –            | –           | –            | –            | –            | –                              | 11.232                      | 1.04                        | 2.39                        | 1              | 36.0                  | 1.00                          | 3.86                          | −6.867                        | −7.01       | −21.75      | 15.05       | ...         | ...         | −6.05       | −18.54 |     |
| 05413388–0153085 | 206.498     | −16.380     | 52.100     | 9            | –          | –           | –           | –          | –           | –             | –           | –               | –            | –           | –            | –            | –            | –                              | 9.555                       | 0.81                        | 1.19                        | 1              | 75.2                  | 0.58                          | 3.86                          | −9.857                        | −7.81       | −24.69      | 16.14       | ...         | ...         | −6.79       | −21.25 |     |
| 05413420–0835275 | 212.787     | −19.406     | 3.638      | 8            | –          | –           | –           | –          | –           | –             | –           | –               | –            | –           | –            | –            | –            | –                              | 9.814                       | 1.60                        | 4.22                        | 1              | 30.4                  | 0.48                          | 3.02                          | 8.458                         | 1.00        | 2.41        | 1.13        | ...         | ...         | 1.07        | 2.65   |     |
| 05413442–0155385 | 206.537     | −16.398     | 51.330     | 9            | –          | –           | –           | –          | –           | –             | –           | –               | –            | –           | –            | –            | –            | –                              | 6.354                       | 1.49                        | 2.86                        | 1              | 185.6                 | 0.40                          | 3.86                          | −12.772                       | −7.01       | −22.64      | 15.90       | ...         | ...         | −6.00       | −19.25 |     |
| 05413575–0216055 | 206.854     | −16.551     | 2.075      | 9            | –          | –           | –           | –          | –           | –             | –           | –               | –            | –           | –            | –            | –            | –                              | 7.796                       | 1.27                        | ...                         | 1              | 151.0                 | 1.00                          | 3.09                          | 7.023                         | 0.92        | ...         | 0.64        | ...         | ...         | 0.96        | ...    |     |
| 05413689–0217125 | 206.874     | −16.556     | 2.100      | 9            | –          | –           | –           | –          | –           | –             | –           | –               | –            | –           | –            | –            | –            | –                              | 9.142                       | 0.92                        | 1.62                        | 1              | 81.8                  | 0.22                          | 3.09                          | 8.360                         | 0.58        | 0.58        | 0.65        | ...         | ...         | 0.62        | 0.72   |     |
| 05413742–0152445 | 206.499     | −16.364     | 55.616     | 9            | –          | –           | –           | –          | –           | –             | –           | –               | –            | –           | –            | –            | –            | –                              | 10.344                      | 0.86                        | 1.53                        | 1              | 46.6                  | 0.68                          | 3.86                          | −10.379                       | −8.35       | −26.11      | 17.23       | ...         | ...         | −7.25       | −22.43 |     |
| 05413875–0150505 | 206.472     | −16.345     | 46.118     | 9            | –          | –           | –           | –          | –           | –             | –           | –               | –            | –           | –            | –            | –            | –                              | 8.563                       | 1.49                        | 3.60                        | 1              | 219.8                 | 0.30                          | 3.86                          | −8.621                        | −6.15       | −19.32      | 14.29       | ...         | ...         | −5.24       | −16.27 |     |
| 05413875–0156025 | 206.552     | −16.385     | 53.627     | 9            | –          | –           | –           | –          | –           | –             | –           | –               | –            | –           | –            | –            | –            | –                              | 9.325                       | 1.66                        | 4.07                        | 1              | 31.8                  | 0.16                          | 3.86                          | −10.656                       | −7.22       | −22.57      | 16.61       | ...         | ...         | −6.17       | −19.03 |     |
| 05413909–0156265 | 206.559     | −16.387     | 50.911     | 9            | –          | –           | –           | –          | –           | –             | –           | –               | –            | –           | –            | –            | –            | –                              | 8.709                       | 1.71                        | ...                         | 1              | 96.4                  | 0.28                          | 3.86                          | −10.260                       | −6.72       | ...         | 15.77       | ...         | ...         | −5.73       | ...    |     |
| 05413909–0213255 | 206.820     | −16.519     | 2.009      | 9            | –          | –           | –           | –          | –           | –             | –           | –               | –            | –           | –            | –            | –            | –                              | 10.395                      | 0.72                        | 1.63                        | 1              | 104.4                 | 0.38                          | 3.09                          | 9.646                         | 0.39        | 0.63        | 0.62        | ...         | ...         | 0.42        | 0.76   |     |
| 05413949–0153335 | 206.515     | −16.363     | 57.572     | 9            | –          | –           | –           | –          | –           | –             | –           | –               | –            | –           | –            | –            | –            | –                              | 8.923                       | ...                         | ...                         | 1              | 119.2                 | 1.00                          | 3.86                          | −12.528                       | ...         | ...         | 17.83       | ...         | ...         | ...         | ...    |     |
| 05414062–0140135 | 206.313     | −16.255     | 6.803      | 8            | –          | –           | –           | –          | –           | –             | –           | –               | –            | –           | –            | –            | –            | –                              | 13.734                      | 0.75                        | 1.52                        | −1             | 16.8                  | 1.00                          | 3.05                          | 11.199                        | −0.38       | −1.86       | 2.11        | ...         | ...         | −0.24       | −1.41  |     |
| 05414062–0155185 | 206.545     | −16.372     | 58.837     | 9            | –          | –           | –           | –          | –           | –             | –           | –               | –            | –           | –            | –            | –            | –                              | 6.441                       | 1.96                        | ...                         | 1              | 130.0                 | 0.68                          | 3.86                          | −15.482                       | −7.78       | ...         | 18.23       | ...         | ...         | −6.62       | ...    |     |
| 05414162–0150415 | 206.476     | −16.333     | 46.138     | 9            | –          | –           | –           | –          | –           | –             | –           | –               | –            | –           | –            | –            | –            | –                              | 8.970                       | 0.93                        | 2.26                        | 1              | 93.8                  | 1.00                          | 3.86                          | −8.221                        | −6.71       | −20.67      | 14.29       | ...         | ...         | −5.81       | −17.62 |     |
| 05414172–0144032 | 206.374     | −16.281     | 16.716     | 9            | –          | –           | –           | –          | –           | –             | –           | –               | –            | –           | –            | –            | –            | –                              | 9.937                       | ...                         | 2.06                        | 1              | 107.8                 | 1.00                          | 3.86                          | 3.709                         | ...         | −6.25       | 5.18        | ...         | ...         | ...         | −5.15  | ... |
| 05414196–0154245 | 206.533     | −16.361     | 59.673     | 9            | –          | –           | –           | –          | –           | –             | –           | –               | –            | –           | –            | –            | –            | –                              | 6.309                       | 2.94                        | ...                         | 1              | 163.2                 | 0.82                          | 3.86                          | −15.925                       | −6.94       | ...         | 18.48       | ...         | ...         | −5.77       | ...    |     |
| 05414209–0216255 | 206.872     | −16.531     | 2.069      | 8            | –          | –           | –           | –          | –           | –             | –           | –               | –            | –           | –            | –            | –            | –                              | 8.666                       | 0.93                        | 2.16                        | 1              | 95.6                  | 0.84                          | 3.09                          | 7.895                         | 0.59        | 1.13        | 0.64        | ...         | ...         | 0.63        | 1.26   |     |
| 05414442–0155235 | 206.553     | −16.359     | 57.963     | 9            | –          | –           | –           | –          | –           | –             | –           | –               | –            | –           | –            | –            | –            | –                              | 6.476                       | 2.27                        | 7.50                        | 1              | 142.6                 | 0.48                          | 3.86                          | −15.121                       | −7.33       | −21.29      | 17.95       | ...         | ...         | −6.20       | −17.47 |     |
| 05414476–0215555 | 206.870     | −16.517     | 2.051      | 8            | –          | –           | –           | –          | –           | –             | –           | –               | –            | –           | –            | –            | –            | –                              | 9.803                       | 1.14                        | 2.57                        | 1              | 29.6                  | 0.52                          | 3.09                          | 9.039                         | 0.80        | 1.55        | 0.64        | ...         | ...         | 0.84        | 1.68   |     |
| 05414482–0758155 | 212.217     | −19.095     | 3.720      | 7            | –          | –           | –           | –          | –           | –             | –           | –               | –            | –           | –            | –            | –            | –                              | 11.860                      | 1.15                        | 3.33                        | 1              | 18.0                  | 0.76                          | 3.03                          | 10.474                        | 0.53        | 1.48        | 1.15        | ...         | ...         | 0.61        | 1.73   |     |
| 05414762–0155435 | 206.565     | −16.350     | 56.496     | 9            | –          | –           | –           | –          | –           | –             | –           | –               | –            | –           | –            | –            | –            | –                              | 7.739                       | 1.40                        | 2.78                        | 1              | 77.8                  | 0.44                          | 3.86                          | −13.311                       | −7.96       | −25.29      | 17.50       | ...         | ...         | −6.85       | −21.56 |     |
| 05414808–0152201 | 206.514     | −16.322     | 54.286     | 9            | –          | –           | –           | –          | –           | –             | –           | –               | –            | –           | –            | –            | –            | –                              | 9.822                       | 1.35                        | 2.15                        | 1              | 87.6                  | 0.46                          | 3.72                          | −10.405                       | −7.64       | −24.82      | 16.82       | ...         | ...         | −6.57       | −21.24 |     |
| 05414855–0155221 | 206.561     | −16.344     | 56.169     | 9            | –          | –           | –           | –          | –           | –             | –           | –               | –            | –           | –            | –            | –            | –                              | 6.183                       | 1.61                        | 3.84                        | 1              | 165.0                 | 0.72                          | 3.72                          | −14.746                       | −7.69       | −24.07      | 17.40       | ...         | ...         | −6.59       | −20.36 |     |
| 05414968–0153271 | 206.534     | −16.325     | 58.688     | 9            | –          | –           | –           | –          | –           | –             | –           | –               | –            | –           | –            | –            | –            | –                              | 7.812                       | 1.32                        | 2.44                        | 1              | 219.8                 | 0.80                          | 3.72                          | −14.055                       | −8.40       | −26.71      | 18.18       | ...         | ...         | −7.25       | −22.84 |     |
| 05414975–0156271 | 206.581     | −16.348     | 51.575     | 9            | –          | –           | –           | –          | –           | –             | –           | –               | –            | –           | –            | –            | –            | –                              | 10.391                      | 1.07                        | 1.91                        | 1              | 63.2                  | 0.34                          | 3.72                          | −8.826                        | −7.47       | −23.71      | 15.98       | ...         | ...         | −6.46       | −20.31 |     |
| 05415015–0157451 | 206.601     | −16.356     | 38.990     | 8            | –          | –           | –           | –          | –           | –             | –           | –               | –            | –           | –            | –            | –            | –                              | 10.519                      | 1.08                        | 2.98                        | 1              | 16.6                  | 0.88                          | 3.72                          | −4.009                        | −5.38       | −16.39      | 12.08       | ...         | ...         | −4.61       | −13.87 |     |
| 05415095–0155071 | 206.562     | −16.333     | 54.745     | 9            | –          | –           | –           | –          | –           | –             | –           | –               | –            | –           | –            | –            | –            | –                              | 5.849                       | 1.40                        | 2.88                        | 1              | 233.2                 | 0.11                          | 3.72                          | −14.549                       | −7.66       | −24.32      | 16.96       | ...         | ...         | −6.59       | −20.70 |     |
| 05415148–0152471 | 206.528     | −16.313     | 53.910     | 9            | –          | –           | –           | –          | –           | –             | –           | –               | –            | –           | –            | –            | –            | –                              | 11.727                      | ...                         | ...                         | 1              | 45.2                  | 1.00                          | 3.72                          | −8.360                        | ...         | ...         | 16.70       | ...         | ...         | ...         | ...    |     |
| 05415162–0152161 | 206.520     | −16.308     | 51.820     | 9            | –          | –           | –           | –          | –           | –             | –           | –               | –            | –           | –            | –            | –            | –                              | 11.181                      | 0.92                        | 1.74                        | 1              | 46.2                  | 0.48                          | 3.72                          | −8.127                        | −7.66       | −24.01      | 16.05       | ...         | ...         | −6.65       | −20.59 |     |
| 05415208–0155181 | 206.568     | −16.330     | 52.580     | 9            | –          | –           | –           | –          | –           | –             | –           | –               | –            | –           | –            | –            | –            | –                              | 5.910                       | 1.38                        | 2.72                        | 1              | 184.4                 |                               |                               |                               |             |             |             |             |             |             |        |     |

© 2017 RAS, MNRAS 000, 1–133



Table B1: b) continued.

| 2MASX J          | <i>l</i>    | <i>b</i>    | EBV        | Object       | Sample         | Disc       | 2MRS        | Velocity   | NIR         | Photom        | Ext         | <i>K</i> <sub>20</sub> | <i>H-K</i>   | <i>J-K</i>  | vc          | <i>a</i>    | <i>b/a</i>  | st.d. | <i>K</i> <sub>s</sub> <sup>o</sup> | <i>(H-K)</i> <sup>o</sup> | <i>(J-K)</i> <sup>o</sup> | <i>A</i> <sub>K</sub> | <i>a</i> <sup>d</sup> | <i>K</i> <sub>s</sub> <sup>o,d</sup> | <i>(H-K)</i> <sup>o,c</sup> | <i>(J-K)</i> <sup>o,c</sup> |             |             |      |             |             |             |       |
|------------------|-------------|-------------|------------|--------------|----------------|------------|-------------|------------|-------------|---------------|-------------|------------------------|--------------|-------------|-------------|-------------|-------------|-------|------------------------------------|---------------------------|---------------------------|-----------------------|-----------------------|--------------------------------------|-----------------------------|-----------------------------|-------------|-------------|------|-------------|-------------|-------------|-------|
| (1)              | deg<br>(2a) | deg<br>(2b) | mag<br>(3) | class<br>(4) | off flg<br>(5) | flg<br>(6) | gal<br>(7a) | TF<br>(7b) | obs<br>(7c) | ext'd<br>(7d) | type<br>(8) | (9)                    | Opt<br>(10a) | HI<br>(10b) | flg<br>(11) | flg<br>(12) | flg<br>(13) | (14)  | mag<br>(15)                        | mag<br>(16)               | (17)                      | (18)                  | (19)                  | (20)                                 | mag<br>(21)                 | mag<br>(22)                 | mag<br>(23) | mag<br>(24) | (25) | mag<br>(26) | mag<br>(27) | mag<br>(28) |       |
| 16272842-2427203 | 353.191     | 16.697      | 4.959      | 9            | -              | -          | -           | -          | -           | -             | -           | -                      | -            | -           | -           | -           | -           | -     | 8.273                              | 1.22                      | 3.18                      | -2                    | 113.8                 | 0.80                                 | 3.11                        | 6.425                       | 0.40        | 0.71        | 1.54 | ...         | ...         | 0.50        | 1.04  |
| 16272936-2427407 | 353.189     | 16.691      | 4.906      | 9            | -              | -          | -           | -          | -           | -             | -           | -                      | -            | -           | -           | -           | -           | -     | 8.944                              | 1.34                      | ...                       | 1                     | 122.6                 | 0.50                                 | 3.32                        | 7.116                       | 0.53        | ...         | 1.52 | ...         | ...         | 0.62        | ...   |
| 16274579-2444536 | 353.006     | 16.455      | 2.287      | 7            | -              | -          | -           | -          | -           | -             | -           | -                      | -            | -           | -           | -           | -           | -     | 12.038                             | 1.64                      | ...                       | 1                     | 24.0                  | 0.62                                 | 3.26                        | 11.186                      | 1.26        | ...         | 0.71 | ...         | ...         | 1.31        | ...   |
| 16302859-2526003 | 352.890     | 15.541      | 1.763      | 2            | -              | -          | -           | -          | -           | N             | D2          | -                      | -            | -           | -           | -           | -           | e?    | 11.794                             | 0.55                      | 1.64                      | 1                     | 23.6                  | 0.72                                 | 3.58                        | 11.137                      | 0.25        | 0.76        | 0.55 | 28.3        | 11.12       | 0.29        | 0.88  |
| 16313280-2403504 | 354.133     | 16.252      | 1.222      | 9            | -              | -          | -           | -          | -           | -             | -           | -                      | -            | -           | -           | -           | -           | -     | 9.888                              | 0.88                      | 2.68                      | 1                     | 61.8                  | 0.34                                 | 3.34                        | 9.433                       | 0.68        | 2.07        | 0.38 | ...         | ...         | 0.70        | 2.15  |
| 16313457-1938009 | 357.698     | 19.097      | 1.293      | 2            | -              | -          | -           | -          | -           | -             | D4          | e                      | o            | -           | -           | -           | -           | e     | 11.655                             | 0.51                      | 1.60                      | 1                     | 22.0                  | 0.94                                 | 3.36                        | 11.173                      | 0.30        | 0.96        | 0.40 | 24.9        | 11.17       | 0.32        | 1.04  |
| 16315236-2455357 | 353.503     | 15.634      | 3.749      | 9            | -              | -          | -           | -          | -           | -             | -           | -                      | -            | -           | -           | -           | -           | -     | 9.980                              | 0.98                      | ...                       | 1                     | 112.4                 | 0.34                                 | 3.30                        | 8.583                       | 0.36        | ...         | 1.16 | ...         | ...         | 0.43        | ...   |
| 16322740-2419019 | 354.073     | 15.930      | 2.301      | 9            | -              | -          | -           | -          | -           | -             | -           | -                      | -            | -           | -           | -           | -           | -     | 10.689                             | ...                       | ...                       | 1                     | 63.8                  | 1.00                                 | 3.57                        | 9.832                       | ...         | ...         | 0.71 | ...         | ...         | ...         | ...   |
| 16352427-2433588 | 354.327     | 15.257      | 2.832      | 1            | -              | -          | -           | -          | -           | -             | D1          | -                      | -            | -           | -           | -           | -           | e     | 10.939                             | 0.69                      | 2.00                      | 1                     | 43.4                  | 0.54                                 | 3.51                        | 9.884                       | 0.22        | 0.59        | 0.88 | 58.9        | 9.87        | 0.28        | 0.78  |
| 16364636-1914400 | 358.833     | 18.392      | 1.011      | 2            | -              | -          | -           | -          | -           | -             | D2          | e                      | o            | -           | -           | -           | -           | -     | 11.518                             | 0.43                      | 1.38                      | 1                     | 29.0                  | 0.64                                 | 3.48                        | 11.141                      | 0.27        | 0.88        | 0.31 | 31.7        | 11.14       | 0.29        | 0.95  |
| 16400090-2223198 | 356.768     | 15.829      | 1.063      | 1            | -              | -          | -           | -          | -           | -             | D1          | e                      | o            | -           | -           | -           | -           | e     | 11.304                             | 0.59                      | 1.67                      | 1                     | 34.4                  | 0.80                                 | 3.49                        | 10.908                      | 0.42        | 1.14        | 0.33 | 38.5        | 10.87       | 0.44        | 1.22  |
| 16403760-2222099 | 356.876     | 15.731      | 1.133      | 2            | -              | -          | -           | -          | -           | -             | D3          | e                      | o            | -           | -           | -           | -           | e     | 11.135                             | 0.55                      | 1.83                      | 1                     | 41.8                  | 0.60                                 | 3.50                        | 10.713                      | 0.36        | 1.27        | 0.35 | 46.3        | 10.72       | 0.38        | 1.34  |
| 16465823-0935202 | 8.662       | 22.182      | 1.057      | 7            | -              | -          | -           | -          | -           | -             | -           | -                      | -            | -           | -           | -           | -           | -     | 10.779                             | 1.59                      | 3.54                      | 1                     | 24.2                  | 0.74                                 | 3.33                        | 10.385                      | 1.42        | 3.02        | 0.33 | ...         | ...         | 1.44        | 3.09  |
| 16480313-1414517 | 4.761       | 19.273      | 1.197      | 1            | -              | -          | -           | -          | -           | -             | D4          | e                      | o            | -           | -           | -           | -           | e     | 11.026                             | 0.36                      | 1.39                      | 1                     | 35.2                  | 0.82                                 | 3.36                        | 10.580                      | 0.16        | 0.80        | 0.37 | 39.1        | 10.59       | 0.18        | 0.88  |
| 16494036-1505105 | 4.287       | 18.463      | 1.074      | 1            | -              | -          | -           | -          | -           | -             | D1          | e                      | o            | -           | -           | -           | -           | -     | 10.985                             | 0.42                      | 1.36                      | 1                     | 43.8                  | 0.32                                 | 3.35                        | 10.585                      | 0.25        | 0.83        | 0.33 | 48.2        | 10.59       | 0.27        | 0.90  |
| 16495465-1417464 | 4.998       | 18.880      | 1.393      | 1            | -              | -          | -           | -          | -           | -             | D1          | e                      | o            | -           | -           | -           | -           | e     | 11.152                             | 0.44                      | 1.48                      | 1                     | 34.6                  | 0.36                                 | 3.38                        | 10.633                      | 0.21        | 0.79        | 0.43 | 39.3        | 10.64       | 0.24        | 0.88  |
| 16505342-1500143 | 4.539       | 18.274      | 0.964      | 1            | -              | -          | -           | -          | -           | -             | D4          | c                      | o            | -           | -           | -           | -           | -     | 10.050                             | 0.38                      | 1.30                      | 1                     | 49.0                  | 0.72                                 | 3.44                        | 9.691                       | 0.22        | 0.82        | 0.30 | 52.6        | 9.71        | 0.24        | 0.88  |
| 16521498-1536454 | 4.222       | 17.651      | 1.228      | 1            | -              | -          | -           | -          | -           | -             | D2          | e                      | o            | -           | -           | -           | -           | -     | 11.291                             | 0.40                      | 1.38                      | 1                     | 33.0                  | 0.74                                 | 3.52                        | 10.833                      | 0.20        | 0.77        | 0.38 | 37.0        | 10.83       | 0.22        | 0.85  |
| 16552395-1554306 | 4.434       | 16.863      | 1.025      | 1            | -              | -          | -           | -          | -           | -             | D1          | e                      | o            | -           | -           | -           | -           | -     | 11.555                             | 0.43                      | 1.34                      | 1                     | 37.0                  | 0.46                                 | 3.46                        | 11.173                      | 0.26        | 0.83        | 0.32 | 40.5        | 11.17       | 0.28        | 0.90  |
| 16554890-1553485 | 4.504       | 16.789      | 1.190      | 1            | -              | -          | -           | -          | -           | -             | D3          | e                      | o            | -           | -           | -           | -           | -     | 11.342                             | 0.62                      | 1.84                      | 1                     | 30.0                  | 0.80                                 | 3.52                        | 10.899                      | 0.43        | 1.24        | 0.37 | 33.3        | 10.91       | 0.45        | 1.32  |
| 17163319-0314237 | 18.605      | 19.371      | 1.029      | 1            | -              | -          | -           | -          | -           | -             | D1          | e                      | o            | -           | -           | -           | -           | e?    | 11.356                             | 0.48                      | 1.67                      | 1                     | 31.6                  | 0.50                                 | 3.28                        | 10.973                      | 0.30        | 1.16        | 0.32 | 34.4        | 10.98       | 0.32        | 1.23  |
| 17293594-0852282 | 15.268      | 13.711      | 1.028      | 1            | -              | -          | -           | -          | -           | -             | D2          | e                      | o            | -           | -           | -           | -           | -     | 11.467                             | 0.61                      | 1.74                      | 1                     | 30.0                  | 0.46                                 | 3.72                        | 11.084                      | 0.44        | 1.23        | 0.32 | 32.8        | 11.09       | 0.46        | 1.30  |
| 17303303-0855284 | 15.348      | 13.484      | 1.002      | 1            | -              | -          | -           | -          | -           | -             | D1          | e                      | o            | -           | -           | -           | -           | -     | 11.025                             | 0.44                      | 1.44                      | 1                     | 38.0                  | 0.58                                 | 3.66                        | 10.652                      | 0.28        | 0.95        | 0.31 | 41.3        | 10.66       | 0.29        | 1.01  |
| 17345703-0733015 | 17.133      | 13.244      | 1.004      | 1            | -              | -          | -           | -          | -           | -             | D1          | e                      | o            | -           | -           | -           | -           | -     | 11.440                             | 0.41                      | 1.44                      | 1                     | 35.6                  | 0.38                                 | 3.68                        | 11.066                      | 0.24        | 0.94        | 0.31 | 38.8        | 11.07       | 0.26        | 1.01  |
| 17353269-0504594 | 19.410      | 14.349      | 0.980      | 1            | -              | -          | -           | -          | -           | -             | D1          | c                      | o            | -           | -           | -           | -           | -     | 9.279                              | 0.36                      | 1.27                      | 1                     | 71.6                  | 0.64                                 | 3.59                        | 8.914                       | 0.20        | 0.78        | 0.30 | 76.5        | 8.95        | 0.22        | 0.84  |
| 17354023-0702097 | 17.682      | 13.348      | 0.968      | 1            | -              | -          | -           | -          | -           | -             | D1          | c                      | o            | -           | -           | -           | -           | -     | 11.366                             | 0.39                      | 1.32                      | 1                     | 36.2                  | 0.30                                 | 3.68                        | 11.005                      | 0.23        | 0.84        | 0.30 | 39.4        | 11.01       | 0.25        | 0.90  |
| 17354374-0720527 | 17.412      | 13.179      | 0.983      | 1            | -              | -          | -           | -          | -           | -             | D2          | c                      | o            | -           | -           | -           | -           | -     | 9.808                              | 0.40                      | 1.38                      | 1                     | 63.2                  | 0.72                                 | 3.68                        | 9.442                       | 0.23        | 0.89        | 0.30 | 69.0        | 9.44        | 0.25        | 0.96  |
| 17355885-0538149 | 18.969      | 13.979      | 0.962      | 1            | -              | -          | -           | -          | -           | -             | D3          | c                      | o            | -           | -           | -           | -           | -     | 10.662                             | 0.40                      | 1.39                      | 1                     | 36.8                  | 0.90                                 | 3.57                        | 10.304                      | 0.24        | 0.91        | 0.30 | 39.5        | 10.33       | 0.26        | 0.97  |
| 17360654-0657557 | 17.801      | 13.289      | 1.036      | 1            | -              | -          | -           | -          | -           | -             | D3          | e                      | o            | -           | -           | -           | -           | -     | 10.389                             | 0.38                      | 1.35                      | 1                     | 47.2                  | 0.70                                 | 3.62                        | 10.003                      | 0.21        | 0.84        | 0.32 | 51.2        | 10.02       | 0.23        | 0.91  |
| 17361220-0719287 | 17.494      | 13.089      | 1.042      | 1            | -              | -          | -           | -          | -           | -             | D2          | e                      | o            | -           | -           | -           | -           | -     | 10.191                             | 0.40                      | 1.40                      | 1                     | 51.8                  | 0.76                                 | 3.69                        | 9.803                       | 0.23        | 0.88        | 0.32 | 56.2        | 9.82        | 0.25        | 0.95  |
| 17363878-0637040 | 18.179      | 13.348      | 1.068      | 1            | -              | -          | -           | -          | -           | -             | D1          | e                      | o            | -           | -           | -           | *           | -     | 11.552                             | 0.59                      | 1.84                      | 1                     | 45.0                  | 0.32                                 | 3.65                        | 11.154                      | 0.41        | 1.31        | 0.33 | 50.0        | 11.14       | 0.43        | 1.38  |
| 17443087-0909036 | 16.930      | 10.395      | 1.140      | 1            | -              | -          | -           | -          | -           | -             | D1          | e                      | o            | -           | -           | -           | -           | -     | 10.738                             | 0.54                      | 1.45                      | 1                     | 49.4                  | 0.54                                 | 3.82                        | 10.313                      | 0.35        | 0.88        | 0.35 | 54.5        | 10.32       | 0.37        | 1.16  |
| 17554454-0324356 | 23.413      | 10.758      | 1.072      | 1            | -              | -          | -           | -          | -           | -             | D2          | e                      | o            | -           | -           | -           | -           | -     | 11.593                             | 0.68                      | 1.64                      | 1                     | 39.6                  | 0.52                                 | 3.79                        | 11.194                      | 0.50        | 1.11        | 0.33 | 44.2        | 11.17       | 0.32        | 0.98  |
| 17570553-0414033 | 22.840      | 10.069      | 1.098      | 1            | -              | -          | -           | -          | -           | -             | D1          | e                      | o            | -           | -           | -           | -           | -     | 11.026                             | 0.47                      | 1.38                      | 1                     | 48.8                  | 0.40                                 | 3.78                        | 10.617                      | 0.29        | 0.84        | 0.34 | 54.2        | 10.61       | 0.31        | 0.91  |
| 19015041-3658371 | 359.905     | -17.850     | 1.550      | 8            | -              | -          | -           | -          | -           | -             | -           | -                      | -            | -           | -           | -           | -           | -     | 8.999                              | 1.73                      | 3.68                      | 1                     | 137.0                 | 0.62                                 | 3.50                        | 8.421                       | 1.28        | 2.91        | 0.48 | ...         | ...         | 1.51        | 3.01  |
| 21001887+6813134 | 104.029     | 14.322      | 2.002      | 9            | -              | -          | -           | -          | -           | -             | -           | -                      | -            | -           | -           | -           | -           | -     | 11.962                             | 1.35                      | ...                       | 1                     | 33.2                  | 0.50                                 | 3.24                        | 11.216                      | 1.02        | ...         | 0.62 | ...         | ...         | 1.06        | ...   |
| 21013286+6808519 | 104.045     | 14.188      | 11.276     | 9            | -              | -          | -           | -          | -           | -             | -           | -                      | -            | -           | -           | -           | -           | -     | 9.282                              | ...                       | 1.40                      | 1                     | 118.4                 | 1.00                                 | 3.39                        | 5.081                       | ...         | -4.20       | 3.49 | ...         | ...         | ...         | -3.46 |
| 21013322+6811188 | 104.078     | 14.213      | 12.664     | 9            | -              | -          | -           | -          | -           | -             | -           | -                      | -            | -           | -           | -           | -           | -     | 9.302                              | 1.18                      | 1.78                      | 1                     | 162.4                 | 0.36                                 | 3.39                        | 4.583                       | -0.92       | -4.51       | 3.92 | ...         | ...         | ...         | -0.67 |
| 21015027+6811298 | 104.098     | 14.195      | 12.217     | 7            | -              | -          | -           | -          | -           | -             | -           | -                      | -            | -           | -           | -           | -           | -     | 12.319                             | 0.90                      | 1.90                      | 1                     | 27.6                  | 0.26                                 | 3.39                        | 7.767                       | -1.12       | -4.17       | 3.78 | ...         | ...         | ...         | -0.88 |
| 21021296+6807385 | 104.070     | 14.127      | 7.930      | 7            | -              | -          | -           | -          | -           | -             | -           | -                      | -            | -           | -           | -           | -           | -     | 13.505                             | 0.53                      | 1.72                      | -1                    | 16.0                  | 1.00                                 | 3.39                        | 10.550                      | -0.78       | -2.22       | 2.46 | ...         | ...         | ...         | -0.63 |
| 21022141+6804366 | 104.038     | 14.084      | 3.574      | 3            | -              | -          | -           | -          | -           | -             | D2          | -                      | -            | -           | -           | -           | -           | -     | 12.428                             | 0.70                      | 2.07                      | 1                     | 20.8                  | 0.36                                 | 3.39                        | 11.096                      | 0.11        | 0.30        | 1.11 | 34.8        | 10.88       | 0.18        | 0.53  |
| 21173843+6817340 | 105.166     | 13.157      | 1.124      | 8            | -              | -          | -           | -          | -           | -             | -           | -                      | -            | -           | -           | -           | -           | -     | 9.313                              | 0.81                      | 2.27                      | 1                     | 87.0                  | 0.50                                 | 3.38                        | 8.894                       | 0.62        | 1.71        | 0.35 | ...         | ...         | ...         | 0.64  |
| 21361828+6829375 | 106.552     | 12.079      | 1.177      | 1            | -              | -          | -           | -          | -           | -             | D1          | e                      | o            | -           | -           | -           | -           | -     | 10.660                             | 0.38                      | 1.33                      | 1                     | 55.2                  | 0.58                                 | 3.35                        | 10.221                      | 0.19        | 0.74        | 0.36 | 61.9        | 10.21       | 0.21        | 0.82  |
| 21409857+6635016 | 105.545     | 10.393      | 0.968      | 7            | -              | -          | -           | -          | -           | -             | -           | -                      | -            | -           | -           | -           | -           | -     | 10.915                             | 0.64                      | 1.73                      | 1                     | 32.8                  | 0.88                                 | 3.50                        | 10.554                      | 0.48        | 1.25        | 0.30 | ...         | ...         | ...         | 0.50  |
| 21511805+7113254 | 109.400     | 10.254      | 1.365      | 1</          |                |            |             |            |             |               |             |                        |              |             |             |             |             |       |                                    |                           |                           |                       |                       |                                      |                             |                             |             |             |      |             |             |             |       |

© 2017 RAS, MNRAS 000, 1–133

Table B2: a) continued.

| 2MASX J          | <i>l</i>    | <i>b</i>    | EBV        | Object       | Sample     | Disc        | 2MRS        | Velocity   | NIR         | Photom        | Ext         | <i>K</i> <sub>20</sub> | <i>H-K</i>   | <i>J-K</i>  | vc          | <i>a</i>    | <i>b/a</i>  | std.        | <i>K</i> <sub>s</sub> <sup>o</sup> | ( <i>H-K</i> ) <sup>o</sup> | ( <i>J-K</i> ) <sup>o</sup> | <i>A</i> <sub>K</sub> | <i>a</i> <sup>d</sup> | <i>K</i> <sub>s</sub> <sup>o,d</sup> | ( <i>H-K</i> ) <sup>o,c</sup> | ( <i>J-K</i> ) <sup>o,c</sup> |             |             |      |             |             |             |       |
|------------------|-------------|-------------|------------|--------------|------------|-------------|-------------|------------|-------------|---------------|-------------|------------------------|--------------|-------------|-------------|-------------|-------------|-------------|------------------------------------|-----------------------------|-----------------------------|-----------------------|-----------------------|--------------------------------------|-------------------------------|-------------------------------|-------------|-------------|------|-------------|-------------|-------------|-------|
| (1)              | deg<br>(2a) | deg<br>(2b) | mag<br>(3) | class<br>(4) | off<br>(5) | flag<br>(6) | gal<br>(7a) | TF<br>(7b) | obs<br>(7c) | ext'd<br>(7d) | type<br>(8) | (9)                    | Opt<br>(10a) | HI<br>(10b) | flg<br>(11) | flg<br>(12) | flg<br>(13) | mag<br>(14) | mag<br>(15)                        | mag<br>(16)                 | (17)                        | (18)                  | (19)                  | (20)                                 | mag<br>(21)                   | mag<br>(22)                   | mag<br>(23) | mag<br>(24) | (25) | mag<br>(26) | mag<br>(27) | mag<br>(28) |       |
| 06105134+2036167 | 190.076     | 0.787       | 6.072      | 8            | —          | —           | —           | —          | —           | —             | —           | —                      | —            | —           | U           | —           | —           | —           | 13.801                             | 0.86                        | 1.25                        | −1                    | 17.8                  | 1.00                                 | 3.75                          | 11.539                        | −0.14       | −1.77       | 1.88 | ...         | ...         | −0.03       | −1.37 |
| 06105697+2036417 | 190.080     | 0.809       | 6.201      | 9            | —          | —           | —           | —          | —           | —             | —           | —                      | —            | —           | —           | —           | —           | —           | 14.092                             | 0.38                        | 1.10                        | −1                    | 10.0                  | 1.00                                 | 3.75                          | 11.782                        | −0.64       | −1.98       | 1.92 | ...         | ...         | −0.52       | −1.57 |
| 06112657+1726350 | 192.913     | −0.615      | 4.280      | 8            | —          | —           | —           | —          | —           | —             | —           | —                      | —            | —           | —           | —           | —           | —           | 12.907                             | 0.70                        | 1.80                        | 1                     | 28.8                  | 0.48                                 | 3.64                          | 11.312                        | −0.01       | −0.33       | 1.33 | ...         | ...         | 0.07        | −0.04 |
| 06120964+1757519 | 192.538     | −0.214      | 6.821      | 8            | —          | —           | —           | —          | —           | —             | —           | —                      | —            | —           | —           | —           | —           | —           | 14.367                             | 0.12                        | 1.14                        | −1                    | 14.8                  | 0.48                                 | 3.71                          | 11.825                        | −1.01       | −2.25       | 2.11 | ...         | ...         | −0.87       | −1.80 |
| 06141005+1743518 | 192.972     | 0.093       | 3.860      | 8            | —          | —           | —           | —          | —           | —             | —           | —                      | —            | —           | —           | —           | —           | —           | 12.707                             | 1.06                        | 2.64                        | 1                     | 17.6                  | 0.72                                 | 3.76                          | 11.269                        | 0.42        | 0.73        | 1.20 | ...         | ...         | 0.50        | 0.98  |
| 06141957+1744578 | 192.974     | 0.135       | 5.438      | 9            | —          | —           | —           | —          | —           | —             | —           | —                      | —            | —           | —           | —           | —           | —           | 13.716                             | 0.54                        | 1.49                        | −1                    | 15.2                  | 0.56                                 | 3.76                          | 11.690                        | −0.36       | −1.21       | 1.68 | ...         | ...         | −0.26       | −0.85 |
| 06142097+1353238 | 196.367     | −1.704      | 6.742      | 9            | —          | —           | —           | —          | —           | —             | —           | —                      | —            | —           | —           | —           | —           | —           | 14.266                             | 0.54                        | 1.07                        | −2                    | 14.4                  | 0.58                                 | 3.73                          | 11.754                        | −0.58       | −2.28       | 2.09 | ...         | ...         | −0.45       | −1.83 |
| 06142097+1744138 | 192.987     | 0.134       | 5.245      | 8            | —          | —           | —           | —          | —           | —             | —           | —                      | —            | —           | —           | —           | —           | —           | 13.640                             | 0.77                        | 2.19                        | 1                     | 12.4                  | 0.58                                 | 3.76                          | 11.686                        | −0.10       | −0.42       | 1.62 | ...         | ...         | 0.00        | −0.07 |
| 06143262+1745271 | 192.991     | 0.184       | 5.460      | 8            | —          | —           | —           | —          | —           | —             | —           | —                      | —            | —           | —           | —           | —           | —           | 13.670                             | ...                         | ...                         | 1                     | 17.2                  | 0.46                                 | 3.66                          | 11.636                        | ...         | ...         | 1.69 | ...         | ...         | ...         | ...   |
| 06143273+1745408 | 192.988     | 0.186       | 5.556      | 8            | —          | —           | —           | —          | —           | —             | —           | —                      | —            | —           | —           | —           | —           | —           | 13.919                             | 0.99                        | ...                         | −1                    | 10.0                  | 1.00                                 | 3.76                          | 11.849                        | 0.07        | ...         | 1.72 | ...         | ...         | 0.18        | ...   |
| 06144064+1859504 | 191.917     | 0.804       | 4.813      | 8            | —          | —           | —           | —          | —           | —             | —           | —                      | —            | —           | —           | —           | —           | —           | 13.058                             | 1.06                        | 2.61                        | 1                     | 12.8                  | 0.42                                 | 3.87                          | 11.265                        | 0.26        | 0.22        | 1.49 | ...         | ...         | 0.36        | 0.54  |
| 06144135+1900064 | 191.915     | 0.809       | 5.070      | 8            | —          | —           | —           | —          | —           | —             | —           | —                      | —            | —           | —           | —           | —           | —           | 13.163                             | 0.56                        | 1.54                        | −2                    | 14.2                  | 0.72                                 | 3.87                          | 11.274                        | −0.27       | −0.97       | 1.57 | ...         | ...         | −0.18       | −0.64 |
| 06144234+1900174 | 191.914     | 0.814       | 5.296      | 8            | —          | —           | —           | —          | —           | —             | —           | —                      | —            | —           | —           | —           | —           | —           | 13.412                             | 0.95                        | ...                         | −1                    | 15.4                  | 0.62                                 | 3.87                          | 11.439                        | 0.07        | ...         | 1.64 | ...         | ...         | 0.18        | ...   |
| 06144962+1221240 | 197.772     | −2.333      | 5.482      | 9            | —          | —           | —           | —          | —           | —             | —           | —                      | —            | —           | —           | —           | —           | —           | 13.571                             | 0.68                        | 1.38                        | −2                    | 15.6                  | 0.42                                 | 3.70                          | 11.528                        | −0.23       | −1.35       | 1.70 | ...         | ...         | −0.12       | −0.99 |
| 06164120+2227536 | 189.089     | 2.867       | 2.058      | 9            | —          | —           | —           | —          | —           | —             | —           | —                      | —            | —           | —           | —           | —           | —           | 12.078                             | ...                         | ...                         | 1                     | 29.6                  | 1.0                                  | 3.78                          | 11.311                        | ...         | ...         | 0.64 | ...         | ...         | ...         | ...   |
| 06164552+2234586 | 188.993     | 2.937       | 2.069      | 9            | —          | —           | —           | —          | —           | —             | —           | —                      | —            | —           | —           | —           | —           | —           | 12.166                             | ...                         | ...                         | −2                    | 32.8                  | 1.00                                 | 3.78                          | 11.395                        | ...         | ...         | 0.64 | ...         | ...         | ...         | ...   |
| 06173854+2222304 | 189.273     | 3.019       | 2.110      | 9            | —          | —           | —           | —          | —           | —             | —           | —                      | —            | —           | —           | —           | —           | —           | 12.270                             | ...                         | ...                         | 1                     | 40.0                  | 0.40                                 | 3.70                          | 11.484                        | ...         | ...         | 0.65 | ...         | ...         | ...         | ...   |
| 06184012+1505100 | 195.812     | −0.216      | 1.835      | 8            | —          | —           | —           | —          | —           | —             | —           | —                      | —            | —           | —           | —           | —           | —           | 11.956                             | 0.59                        | 1.25                        | −2                    | 32.0                  | 0.56                                 | 3.71                          | 11.272                        | 0.29        | 0.33        | 0.57 | ...         | ...         | 0.32        | 0.46  |
| 06184648+1513240 | 195.703     | −0.128      | 4.862      | 8            | —          | —           | —           | —          | —           | —             | —           | —                      | —            | —           | —           | —           | —           | —           | 13.339                             | ...                         | ...                         | 1                     | 14.0                  | 1.00                                 | 3.71                          | 11.527                        | ...         | ...         | 1.51 | ...         | ...         | ...         | ...   |
| 06190061+1518092 | 195.660     | −0.041      | 4.929      | 8            | —          | —           | —           | —          | —           | —             | —           | —                      | —            | —           | —           | —           | —           | —           | 13.613                             | 0.75                        | 1.63                        | −2                    | 16.0                  | 0.66                                 | 3.69                          | 11.776                        | −0.07       | −0.82       | 1.53 | ...         | ...         | 0.03        | −0.50 |
| 06305755+0948266 | 201.880     | −0.034      | 5.363      | 8            | —          | —           | —           | —          | —           | —             | —           | —                      | —            | —           | —           | —           | —           | —           | 13.604                             | 0.66                        | 1.08                        | −1                    | 12.8                  | 1.00                                 | 3.80                          | 11.606                        | −0.23       | −1.58       | 1.66 | ...         | ...         | −0.12       | −1.23 |
| 06324107+1010227 | 201.753     | 0.512       | 4.693      | 8            | —          | —           | —           | —          | —           | —             | —           | —                      | —            | —           | —           | —           | —           | —           | 13.201                             | 0.79                        | 1.24                        | −2                    | 21.6                  | 0.28                                 | 3.70                          | 11.452                        | 0.01        | −1.09       | 1.45 | ...         | ...         | 0.10        | −0.78 |
| 06331478+0434532 | 206.779     | −1.944      | 5.183      | 8            | —          | —           | —           | —          | —           | —             | —           | —                      | —            | —           | —           | —           | —           | —           | 13.482                             | ...                         | ...                         | 1                     | 19.0                  | 0.22                                 | 3.81                          | 11.551                        | ...         | ...         | 1.61 | ...         | ...         | ...         | ...   |
| 06343124+0421054 | 207.129     | −1.768      | 5.493      | 8            | —          | —           | —           | —          | —           | —             | —           | —                      | —            | —           | —           | —           | —           | —           | 13.624                             | 0.52                        | 1.43                        | −1                    | 10.0                  | 0.66                                 | 3.80                          | 11.577                        | −0.39       | −1.30       | 1.70 | ...         | ...         | −0.29       | −0.94 |
| 06352735+0431158 | 207.086     | −1.483      | 2.019      | 1            | —          | —           | gal         | t          | —           | —             | D1          | —                      | —            | —           | —           | —           | e           | 12.004      | 0.56                               | 1.76                        | 1                           | 23.2                  | 0.44                  | 3.65                                 | 11.252                        | 0.22                          | 0.75        | 0.63        | 28.8 | 11.23       | 0.26        | 0.89        |       |
| 06360129+1046147 | 201.600     | 1.516       | 4.545      | 4            | —          | —           | gal         | —          | —           | —             | D1          | —                      | —            | —           | —           | —           | e           | 13.205      | 0.84                               | ...                         | −1                          | 16.0                  | 1.00                  | 3.68                                 | 11.512                        | 0.09                          | ...         | 1.41        | 35.3 | 11.00       | 0.18        | ...         |       |
| 06360204+1101457 | 201.371     | 1.637       | 3.236      | 8            | —          | —           | —           | —          | —           | —             | —           | —                      | —            | —           | —           | —           | —           | —           | 12.470                             | 1.02                        | 2.81                        | 1                     | 15.2                  | 0.64                                 | 3.69                          | 11.264                        | 0.49        | 1.20        | 1.00 | ...         | ...         | 0.55        | 1.42  |
| 06361473+1047157 | 201.610     | 1.572       | 6.010      | 4            | —          | —           | gal         | —          | —           | —             | n           | —                      | —            | —           | —           | —           | e           | 13.777      | 0.54                               | 1.57                        | −1                          | 10.0                  | 1.00                  | 3.68                                 | 11.538                        | −0.46                         | −1.42       | 1.86        | 27.0 | 11.05       | −0.34       | −1.02       |       |
| 06390417−0146157 | 213.100     | −3.559      | 2.147      | 8            | —          | —           | —           | —          | —           | —             | —           | —                      | —            | —           | —           | —           | —           | —           | 12.175                             | 0.79                        | 1.78                        | −2                    | 53.8                  | 0.34                                 | 3.54                          | 11.375                        | 0.44        | 0.71        | 0.67 | ...         | ...         | 0.48        | 0.85  |
| 06444931+0020162 | 211.877     | −1.318      | 2.915      | 8            | —          | —           | —           | —          | —           | —             | —           | —                      | —            | —           | —           | —           | —           | —           | 12.365                             | 0.94                        | 2.03                        | 1                     | 31.8                  | 0.58                                 | 3.78                          | 11.279                        | 0.46        | 0.59        | 0.90 | ...         | ...         | 0.51        | 0.78  |
| 06451485+0024261 | 211.864     | −1.191      | 4.378      | 8            | —          | —           | —           | —          | —           | —             | —           | —                      | —            | —           | —           | —           | —           | —           | 13.175                             | 1.03                        | ...                         | −1                    | 20.6                  | 0.60                                 | 3.78                          | 11.544                        | 0.31        | ...         | 1.36 | ...         | ...         | 0.39        | ...   |
| 06462319+0005414 | 212.272     | −1.081      | 2.755      | 8            | —          | —           | —           | —          | —           | —             | —           | —                      | —            | —           | —           | —           | —           | —           | 12.471                             | 1.31                        | ...                         | 1                     | 44.2                  | 0.22                                 | 3.74                          | 11.444                        | 0.85        | ...         | 0.85 | ...         | ...         | 0.91        | ...   |
| 06480324+0017337 | 212.286     | −0.619      | 1.293      | 8            | —          | —           | —           | —          | —           | —             | —           | —                      | —            | —           | —           | —           | —           | —           | 11.740                             | 0.62                        | 1.36                        | −2                    | 46.6                  | 0.86                                 | 3.75                          | 11.258                        | 0.40        | 0.71        | 0.40 | ...         | ...         | 0.43        | 0.80  |
| 06543022−0431390 | 217.311     | −1.382      | 5.059      | 9            | —          | —           | —           | —          | —           | —             | —           | —                      | —            | —           | —           | —           | —           | —           | 13.624                             | 0.64                        | 1.34                        | −1                    | 14.6                  | 1.00                                 | 3.70                          | 11.739                        | −0.20       | −1.18       | 1.57 | ...         | ...         | −0.10       | −0.84 |
| 06543109−0431460 | 217.314     | −1.380      | 5.080      | 9            | —          | —           | —           | —          | —           | —             | —           | —                      | —            | —           | —           | —           | —           | —           | 13.235                             | 0.64                        | 1.91                        | −2                    | 18.0                  | 0.32                                 | 3.70                          | 11.342                        | −0.21       | −0.62       | 1.57 | ...         | ...         | −0.11       | −0.28 |
| 06570202−0817246 | 220.950     | −2.536      | 7.469      | 9            | —          | —           | —           | —          | —           | —             | —           | —                      | —            | —           | —           | —           | —           | —           | 14.104                             | −0.05                       | 1.03                        | −1                    | 10.0                  | 1.00                                 | 3.75                          | 11.321                        | −1.28       | −2.68       | 2.31 | ...         | ...         | −1.14       | −2.19 |
| 06590581−0451591 | 218.135     | −0.519      | 3.601      | 8            | —          | —           | —           | —          | —           | —             | —           | —                      | —            | —           | —           | —           | —           | —           | 12.746                             | 1.55                        | ...                         | 1                     | 20.4                  | 0.54                                 | 3.78                          | 11.404                        | 0.96        | ...         | 1.12 | ...         | ...         | 1.03        | ...   |
| 06593819−0441480 | 218.045     | −0.322      | 4.614      | 7            | —          | o           | —           | —          | —           | —             | —           | —                      | —            | —           | —           | —           | —           | —           | 13.142                             | ...                         | ...                         | 1                     | 13.4                  | 1.00                                 | 3.87                          | 11.423                        | ...         | ...         | 1.43 | ...         | ...         | ...         | ...   |
| 06593962−0746575 | 220.794     | −1.726      | 6.083      | 8            | —          | —           | —           | —          | —           | —             | —           | —                      | —            | —           | —           | —           | —           | —           | 13.601                             | 0.48                        | 1.12                        | 1                     | 12.4                  | 1.00                                 | 3.81                          | 11.334                        | −0.52       | −1.90       | 1.88 | ...         | ...         | −0.40       | −1.50 |
| 07005247−0855534 | 221.954     | −1.983      | 6.139      | 8            | —          | —           | —           | —          | —           | —             | —           | —                      | —            | —           | —           | —           | —           | —           | 13.818                             | ...                         | ...                         | −1                    | 10.0                  | 1.00                                 | 3.80                          | 11.531                        | ...         | ...         | 1.90 | ...         | ...         | ...         | ...   |
| 07024224−1128114 | 224.420     | −2.741      | 4.619      | 9            | —          | —           | —           | —          | —           | —             | —           | —                      | —            | —           | —           | —           | —           | —           | 13.077                             | 0.62                        | 1.28                        | 2                     | 14.4                  | 0.78                                 | 3.80                          | 11.356                        | −0.15       | −1.02       | 1.43 | ...         | ...         | −0.06       | −0.71 |
| 07044772−1033400 | 223.846     | −1.869      | 4.125      | 8            | —          | —           | —           | —          | —           | —             | —           | —                      | —            | —           | —           | —           | —           | —           | 12.987                             | 1.37                        | ...                         | 1                     | 19.6                  | 0.46                                 | 3.64                          | 11.450                        | 0.69        | ...         | 1.28 | ...         | ...         | 0.77        | ...   |
| 07101111−1826388 | 231.463     | −4.317      | 5.886      | 9            | —          | —           | —           | —          | —           | —             | —           | —                      | —            | —           | —           | —           | —           | —           | 13.560                             | 0.20                        | 0.91                        | 2                     | 10.4                  | 1.00                                 | 3.78                          | 11.367                        | −0.78       | −2.02       |      |             |             |             |       |

Table B2: a) continued.

| 2MASX J          | <i>l</i>    | <i>b</i>    | EBV        | Object       |            |            | Sample      |            |             | Disc          | 2MRS        | Velocity     |             | NIR         | Photom      | Ext         | <i>K</i> <sub>20</sub> | <i>H-K</i>  | <i>J-K</i>  | vc   | <i>a</i> | <i>b/a</i> | std. | <i>K</i> <sub>s</sub> <sup>o</sup> | ( <i>H-K</i> ) <sup>o</sup> | ( <i>J-K</i> ) <sup>o</sup> | <i>A<sub>K</sub></i> | <i>a</i> <sup>d</sup> | <i>K</i> <sub>s</sub> <sup>o,d</sup> | ( <i>H-K</i> ) <sup>o,c</sup> | ( <i>J-K</i> ) <sup>o,c</sup> |
|------------------|-------------|-------------|------------|--------------|------------|------------|-------------|------------|-------------|---------------|-------------|--------------|-------------|-------------|-------------|-------------|------------------------|-------------|-------------|------|----------|------------|------|------------------------------------|-----------------------------|-----------------------------|----------------------|-----------------------|--------------------------------------|-------------------------------|-------------------------------|
| (1)              | deg<br>(2a) | deg<br>(2b) | mag<br>(3) | class<br>(4) | off<br>(5) | flg<br>(6) | gal<br>(7a) | TF<br>(7b) | obs<br>(7c) | ext'd<br>(7d) | type<br>(8) | Opt<br>(10a) | HI<br>(10b) | flg<br>(11) | flg<br>(12) | flg<br>(13) | mag<br>(14)            | mag<br>(15) | mag<br>(16) | (17) | (18)     | (19)       | (20) | mag<br>(21)                        | mag<br>(22)                 | mag<br>(23)                 | mag<br>(24)          | (25)                  | mag<br>(26)                          | mag<br>(27)                   | mag<br>(28)                   |
| 08463397−4243215 | 262.849     | 0.312       | 2.522      | 3            | −          | −          | g           | t          | −           | −             | D2          | −            | −           | −           | −           | e           | 12.250                 | 0.61        | 2.08        | 1    | 25.2     | 0.68       | 3.90 | 11.310                             | −0.19                       | 0.83                        | 0.78                 | 35.1                  | 11.19                                | 0.24                          | 0.99                          |
| 08483130−4333231 | 263.722     | 0.066       | 6.212      | 7            | −          | −          | −           | −          | −           | −             | −           | −            | −           | −           | −           | −           | 13.809                 | 0.51        | 1.72        | 1    | 10.0     | 1.00       | 3.90 | 11.494                             | −0.52                       | −1.36                       | 1.92                 | ...                   | ...                                  | −0.40                         | −0.95                         |
| 08490236−4529375 | 265.283     | −1.085      | 2.470      | 3            | −          | −          | g           | −          | −           | −             | D2          | −            | −           | −           | −           | e           | 12.271                 | 0.48        | 1.70        | 1    | 22.8     | 0.96       | 4.07 | 11.351                             | 0.08                        | 0.47                        | 0.77                 | 31.9                  | 11.20                                | 0.12                          | 0.63                          |
| 08505437−4342387 | 264.114     | 0.302       | 3.347      | 8            | o          | −          | −           | −          | −           | −             | −           | −            | −           | −           | −           | −           | 12.590                 | 1.18        | ...         | 1    | 17.8     | 0.70       | 3.97 | 11.343                             | 0.63                        | ...                         | 1.04                 | ...                   | ...                                  | 0.69                          | ...                           |
| 08513748−4627510 | 266.319     | −1.353      | 1.934      | 2            | −          | −          | g           | t          | −           | −             | n           | −            | −           | −           | −           | e?          | 12.006                 | 0.48        | 1.41        | 1    | 21.0     | 0.64       | 4.08 | 11.285                             | 0.16                        | 0.45                        | 0.60                 | 26.2                  | 11.24                                | 0.20                          | 0.57                          |
| 08524171−4337090 | 264.250     | 0.610       | 3.033      | 7            | −          | −          | −           | −          | −           | −             | −           | −            | −           | −           | −           | −           | 12.618                 | 1.42        | ...         | 1    | 21.4     | 0.66       | 3.94 | 11.488                             | 0.92                        | ...                         | 0.94                 | ...                   | ...                                  | 0.98                          | ...                           |
| 08572891−4641361 | 267.143     | −0.731      | 1.446      | 7            | −          | −          | −           | −          | −           | −             | −           | −            | −           | −           | −           | −           | 11.845                 | 0.56        | 1.85        | 0    | 50.4     | 0.48       | 4.02 | 11.306                             | 0.32                        | 1.14                        | 0.45                 | ...                   | ...                                  | 0.35                          | 1.23                          |
| 08575817−4246307 | 264.227     | 1.889       | 5.824      | 8            | −          | −          | −           | −          | −           | −             | −           | −            | −           | −           | −           | −           | 13.718                 | 1.17        | ...         | 1    | 10.0     | 1.00       | 3.78 | 11.548                             | 0.20                        | ...                         | 1.80                 | ...                   | ...                                  | 0.32                          | ...                           |
| 08595266−4650215 | 267.521     | −0.516      | 1.519      | 5            | o          | −          | g           | t          | −           | −             | D1          | −            | −           | −           | −           | o           | 11.887                 | 1.11        | ...         | 1    | 31.6     | 0.62       | 3.91 | 11.321                             | 0.86                        | ...                         | 0.47                 | 38.1                  | 11.24                                | 0.89                          | ...                           |
| 09011763−4835332 | 268.998     | −1.492      | 3.869      | 8            | −          | −          | −           | −          | −           | −             | −           | −            | −           | −           | −           | −           | 12.795                 | 1.17        | ...         | 0    | 26.6     | 0.44       | 4.00 | 11.353                             | 0.53                        | ...                         | 1.20                 | ...                   | ...                                  | 0.60                          | ...                           |
| 09055121−4828193 | 269.410     | −0.848      | 2.560      | 2            | −          | −          | g           | t          | −           | −             | D1          | −            | −           | −           | −           | e?          | 12.351                 | 0.95        | ...         | 0    | 34.2     | 0.30       | 3.91 | 11.397                             | 0.52                        | ...                         | 0.79                 | 49.7                  | 11.19                                | 0.57                          | ...                           |
| 09075056−4908057 | 270.121     | −1.052      | 5.193      | 7            | −          | −          | −           | −          | −           | −             | −           | −            | −           | −           | −           | −           | 13.382                 | 0.76        | ...         | 0    | 16.2     | 0.56       | 3.96 | 11.447                             | −0.10                       | ...                         | 1.61                 | ...                   | ...                                  | 0.00                          | ...                           |
| 09075279−4855597 | 269.977     | −0.912      | 4.578      | 9            | −          | −          | −           | −          | −           | −             | −           | −            | −           | −           | −           | −           | 13.145                 | 0.47        | 1.50        | 2    | 14.8     | 0.60       | 3.96 | 11.439                             | −0.29                       | −0.77                       | 1.42                 | ...                   | ...                                  | −0.20                         | −0.47                         |
| 09083414−4718333 | 268.859     | 0.272       | 4.580      | 9            | −          | −          | −           | −          | −           | −             | −           | −            | −           | −           | −           | −           | 13.239                 | ...         | ...         | 1    | 11.2     | 1.00       | 3.95 | 11.532                             | ...                         | ...                         | 1.42                 | ...                   | ...                                  | ...                           | ...                           |
| 09105720−4920578 | 270.624     | −0.826      | 4.037      | 9            | −          | −          | −           | −          | −           | −             | −           | −            | −           | −           | −           | −           | 13.002                 | ...         | ...         | 1    | 19.2     | 0.46       | 4.05 | 11.498                             | ...                         | ...                         | 1.25                 | ...                   | ...                                  | ...                           | ...                           |
| 09111001−5039373 | 271.604     | −1.697      | 4.141      | 8            | −          | −          | −           | −          | −           | −             | −           | −            | −           | −           | −           | −           | 13.062                 | 0.53        | 1.59        | 0    | 19.8     | 0.38       | 4.00 | 11.519                             | −0.16                       | −0.47                       | 1.28                 | ...                   | ...                                  | −0.08                         | −0.20                         |
| 09123061−5133119 | 272.400     | −2.155      | 2.912      | 8            | −          | −          | −           | −          | −           | −             | −           | −            | −           | −           | −           | −           | 12.392                 | 0.92        | 2.45        | 1    | 17.0     | 0.56       | 4.06 | 11.307                             | 0.44                        | 1.00                        | 0.90                 | ...                   | ...                                  | 0.50                          | 1.19                          |
| 09153010−4814354 | 270.337     | 0.479       | 3.319      | 4            | −          | −          | g           | −          | −           | −             | n           | −            | −           | −           | −           | e?          | 12.525                 | 1.14        | ...         | 0    | 29.2     | 1.00       | 3.92 | 11.288                             | 0.59                        | ...                         | 1.03                 | 46.9                  | 11.08                                | 0.66                          | ...                           |
| 09154186−4901334 | 270.923     | −0.041      | 3.614      | 4            | −          | −          | −           | −          | −           | −             | −           | −            | −           | −           | −           | e?          | 12.851                 | 0.59        | ...         | 1    | 17.0     | 0.90       | 3.92 | 11.504                             | −0.01                       | ...                         | 1.12                 | 29.4                  | 11.23                                | 0.06                          | ...                           |
| 09164479−4819394 | 270.542     | 0.569       | 3.685      | 3            | −          | −          | g           | t          | −           | −             | D2          | −            | −           | −           | −           | −           | 12.681                 | 0.79        | 2.36        | 0    | 20.0     | 0.52       | 3.90 | 11.308                             | 0.18                        | 0.53                        | 1.14                 | 33.3                  | 11.13                                | 0.26                          | 0.77                          |
| 09183041−4751367 | 270.413     | 1.106       | 3.342      | 8            | −          | −          | −           | −          | −           | −             | −           | −            | −           | −           | −           | −           | 12.591                 | 0.50        | 1.36        | 0    | 20.2     | 0.52       | 3.88 | 11.346                             | −0.05                       | −0.30                       | 1.04                 | ...                   | ...                                  | 0.01                          | −0.08                         |
| 09190122−4825337 | 270.877     | 0.770       | 4.391      | 4            | −          | −          | g           | −          | −           | −             | n           | −            | −           | −           | −           | e?          | 13.214                 | ...         | ...         | 1    | 15.4     | 1.00       | 3.92 | 11.578                             | ...                         | ...                         | 1.36                 | 31.8                  | 11.17                                | ...                           | ...                           |
| 09300115−4938090 | 273.012     | 1.165       | 1.918      | 2            | −          | −          | −           | −          | −           | −             | D3          | −            | −           | −           | −           | −           | 11.969                 | 0.64        | 1.93        | 1    | 15.6     | 0.84       | 4.05 | 11.254                             | 0.32                        | 0.97                        | 0.59                 | 26.9                  | 11.20                                | 0.36                          | 1.10                          |
| 09311408−5217133 | 274.964     | −0.639      | 1.644      | 9            | −          | −          | g           | −          | −           | −             | −           | −            | −           | −           | −           | −           | 11.920                 | 0.92        | 1.52        | 0    | 35.2     | 0.32       | 4.19 | 11.307                             | 0.65                        | 0.70                        | 0.51                 | ...                   | ...                                  | 0.68                          | 0.81                          |
| 09321559−5102501 | 274.236     | 0.377       | 1.529      | 2            | o          | −          | g           | t          | −           | −             | D2          | −            | *           | o           | −           | −           | 11.830                 | 0.58        | 1.26        | 0    | 36.8     | 0.34       | 4.09 | 11.260                             | 0.32                        | 0.50                        | 0.47                 | 43.2                  | 11.23                                | 0.35                          | 0.60                          |
| 09334665−5358154 | 276.388     | −1.616      | 3.274      | 8            | −          | −          | g           | −          | −           | −             | n           | −            | −           | −           | −           | −           | 12.663                 | 0.57        | 1.08        | 1    | 14.6     | 0.72       | 4.14 | 11.443                             | 0.03                        | −0.54                       | 1.01                 | ...                   | ...                                  | 0.09                          | −0.33                         |
| 09575803−5728314 | 281.250     | −2.098      | 3.159      | 3            | −          | −          | −           | −          | −           | −             | n           | −            | −           | −           | −           | −           | 12.561                 | 0.97        | ...         | 1    | 18.0     | 0.86       | 4.22 | 11.384                             | 0.44                        | ...                         | 0.98                 | 27.3                  | 11.25                                | 0.51                          | ...                           |
| 10013279−5842243 | 282.374     | −2.790      | 1.771      | 1            | −          | −          | g           | −          | −           | −             | D1          | −            | −           | −           | −           | −           | 11.977                 | 0.63        | 1.90        | 0    | 33.6     | 0.38       | 4.22 | 11.317                             | 0.33                        | 1.02                        | 0.55                 | 41.9                  | 11.23                                | 0.37                          | 1.13                          |
| 10014272−5710073 | 281.467     | −1.548      | 5.332      | 9            | −          | −          | g           | −          | −           | −             | n           | −            | −           | −           | −           | −           | 13.256                 | 0.32        | 1.05        | 2    | 12.4     | 0.72       | 4.14 | 11.269                             | −0.56                       | −1.60                       | 1.65                 | ...                   | ...                                  | −0.46                         | −1.25                         |
| 10061082−5551490 | 281.187     | −0.132      | 3.770      | 4            | −          | −          | g           | −          | −           | −             | n           | −            | −           | −           | −           | −           | 12.830                 | 0.71        | ...         | 1    | 12.2     | 1.00       | 4.27 | 11.425                             | 0.08                        | ...                         | 1.17                 | 20.8                  | 11.23                                | 0.16                          | ...                           |
| 10074793−5830509 | 282.917     | −2.152      | 2.791      | 3            | −          | −          | g           | t          | −           | −             | D3          | −            | −           | −           | −           | −           | 12.364                 | ...         | ...         | 0    | 23.2     | 0.56       | 4.29 | 11.324                             | ...                         | ...                         | 0.86                 | 33.3                  | 11.20                                | ...                           | ...                           |
| 13373272−5850056 | 308.879     | 3.503       | 1.089      | 1            | −          | −          | g           | −          | −           | −             | D1          | −            | −           | −           | −           | −           | 11.696                 | 0.32        | 1.13        | 1    | 29.4     | 0.62       | 4.31 | 11.290                             | 0.14                        | 0.59                        | 0.34                 | 33.1                  | 11.25                                | 0.16                          | 0.66                          |
| 14373109−5353249 | 318.269     | 5.793       | 0.776      | 1            | −          | −          | g           | −          | −           | −             | D1          | −            | *           | h           | −           | −           | 11.540                 | 0.25        | 1.12        | 1    | 38.8     | 0.62       | 4.06 | 11.251                             | 0.12                        | 0.73                        | 0.24                 | 42.0                  | 11.22                                | 0.14                          | 0.78                          |
| 17562216−0823304 | 19.063      | 8.221       | 1.381      | 1            | −          | −          | g           | −          | −           | −             | D1          | −            | −           | −           | −           | −           | 11.777                 | 0.45        | 1.51        | 1    | 32.4     | 0.40       | 3.96 | 11.262                             | 0.23                        | 0.82                        | 0.43                 | 37.4                  | 11.24                                | 0.25                          | 0.91                          |
| 18135080−0837571 | 20.939      | 4.315       | 1.487      | 1            | −          | −          | g           | −          | −           | −             | D1          | −            | −           | −           | −           | −           | 11.814                 | 0.54        | ...         | 1    | 25.8     | 0.40       | 4.41 | 11.260                             | 0.29                        | ...                         | 0.46                 | 30.2                  | 11.23                                | 0.32                          | ...                           |
| 18135365−0326344 | 25.545      | 6.748       | 2.215      | 1            | −          | −          | g           | −          | −           | −             | D2          | −            | −           | −           | −           | −           | 12.132                 | 0.63        | 1.81        | 1    | 22.2     | 0.84       | 3.97 | 11.307                             | 0.26                        | 0.71                        | 0.69                 | 28.9                  | 11.24                                | 0.30                          | 0.86                          |
| 18331560+0009318 | 30.998      | 4.116       | 2.203      | 1            | −          | −          | g           | −          | −           | −             | D2          | −            | −           | −           | −           | −           | 12.086                 | 0.61        | 2.04        | 1    | 18.4     | 0.78       | 4.28 | 11.265                             | 0.25                        | 0.94                        | 0.68                 | 23.7                  | 11.21                                | 0.29                          | 1.09                          |
| 19482638+2208369 | 59.013      | −1.779      | 2.142      | 8            | −          | p          | g           | −          | −           | −             | −           | −            | −           | −           | −           | −           | 12.102                 | ...         | 1.35        | 1    | 14.2     | 0.96       | 4.41 | 11.304                             | ...                         | 0.28                        | 0.66                 | ...                   | ...                                  | ...                           | 0.43                          |
| 20005349+2539031 | 63.488      | −2.409      | 2.259      | 1            | −          | −          | g           | t          | −           | −             | D3          | −            | −           | −           | −           | −           | 12.130                 | 0.70        | 1.94        | 1    | 18.6     | 0.68       | 4.27 | 11.288                             | 0.33                        | 0.82                        | 0.70                 | 24.1                  | 11.24                                | 0.37                          | 0.97                          |
| 20074349+2733377 | 65.920      | −2.684      | 4.975      | 9            | −          | −          | g           | −          | −           | −             | −           | −            | −           | −           | −           | −           | 13.253                 | 0.29        | 1.09        | 2    | 14.6     | 0.68       | 4.16 | 11.399                             | −0.53                       | −1.38                       | 1.54                 | ...                   | ...                                  | −0.44                         | −1.05                         |
| 20114967+2816542 | 67.019      | −3.053      | 4.681      | 8            | −          | −          | g           | −          | −           | −             | −           | −            | −           | −           | −           | −           | 13.180                 | ...         | ...         | −1   | 21.6     | 0.42       | 4.09 | 11.436                             | ...                         | ...                         | 1.45                 | ...                   | ...                                  | ...                           | ...                           |
| 20150411+3146118 | 70.319      | −1.715      | 3.860      | 1            | −          | −          | g           | −          | −           | −             | D2          | −            | −           | −           | −           | −           | 12.931                 | ...         | ...         | 1    | 21.4     | 0.54       | 4.16 | 11.493                             | ...                         | ...                         | 1.20                 | 39.2                  | 11.18                                | ...                           | ...                           |
| 20165199+4157372 | 78.988      | 3.662       | 4.741      | 9            | −          | −          | g           | t          | −           | −             | −           | −            | −           | −           | −           | −           | 13.112                 | 0.38        | 1.10        | 2    | 11.6     | 1.00       | 4.18 | 11.346                             | −0.40                       | −1.26                       | 1.47                 | ...                   | ...                                  | −0.31                         | −0.95                         |
| 20195373+4024125 | 78.017      | 2.317       | 5.234      | 8            | −          | −          | g           | −          | −           | −             | −           | −            | −           | −           | −           | −           | 13.220                 | ...         | ...         | −1   | 13.0     | 1.00       | 4.16 | 11.270                             | ...                         | ...                         | 1.62                 | ...                   | ...                                  | ...                           | ...                           |
| 20212329+4100192 | 78.674      | 2.424       | 4.461      | 8            | −          | −          | g           | −          | −           | −             |             |              |             |             |             |             |                        |             |             |      |          |            |      |                                    |                             |                             |                      |                       |                                      |                               |                               |

Table B2: a) continued.

| 2MASX J          | $l$         | $b$         | EBV        | Object       |            |            | Sample      |            |             | Disc          | 2MRS        | Velocity     |             | NIR         | Photom      | Ext         | $K_{20}$    | $H-K$       | $J-K$       | vc   | $a$  | $b/a$ | st.d. | $K_s^o$     | $(H-K)^o$   | $(J-K)^o$   | $A_K$       | $a''$ | $K_s^{o,d}$ | $(H-K)^{o,c}$ | $(J-K)^{o,c}$ |
|------------------|-------------|-------------|------------|--------------|------------|------------|-------------|------------|-------------|---------------|-------------|--------------|-------------|-------------|-------------|-------------|-------------|-------------|-------------|------|------|-------|-------|-------------|-------------|-------------|-------------|-------|-------------|---------------|---------------|
| (1)              | deg<br>(2a) | deg<br>(2b) | mag<br>(3) | class<br>(4) | off<br>(5) | flg<br>(6) | gal<br>(7a) | TF<br>(7b) | obs<br>(7c) | ext'd<br>(7d) | type<br>(8) | Opt<br>(10a) | HI<br>(10b) | flg<br>(11) | flg<br>(12) | flg<br>(13) | mag<br>(14) | mag<br>(15) | mag<br>(16) | (17) | (18) | (19)  | (20)  | mag<br>(21) | mag<br>(22) | mag<br>(23) | mag<br>(24) | (25)  | mag<br>(26) | mag<br>(27)   | mag<br>(28)   |
| 20571940+4832201 | 88.527      | 1.953       | 2.536      | 8            | —          | —          | g           | —          | —           | —             | n           | —            | —           | U           | —           | —           | 12.283      | ...         | ...         | 1    | 23.2 | 1.00  | 4.16  | 11.338      | ...         | ...         | 0.79        | ...   | ...         | ...           | ...           |
| 20575657+5016055 | 89.906      | 3.002       | 3.910      | 1            | —          | —          | g           | t          | —           | —             | —           | —            | —           | U           | —           | —           | 12.877      | 0.88        | ...         | 1    | 17.6 | 0.68  | 4.06  | 11.420      | 0.23        | ...         | 1.21        | 32.1  | 11.12       | 0.31          | ...           |
| 20585923+5346088 | 92.674      | 5.161       | 1.760      | 2            | —          | —          | —           | —          | —           | —             | D3          | —            | —           | —           | —           | —           | 11.914      | 0.52        | 1.61        | 1    | 24.6 | 0.88  | 3.87  | 11.258      | 0.22        | 0.73        | 0.55        | 30.0  | 11.21       | 0.26          | 0.85          |
| 21004012+5204289 | 91.555      | 3.860       | 4.236      | 8            | —          | —          | g           | —          | —           | —             | —           | —            | —           | U           | —           | —           | 13.111      | ...         | 1.62        | —    | 12.0 | 1.00  | 3.91  | 11.533      | ...         | −0.49       | 1.31        | ...   | ...         | ...           | −0.21         |
| 21013309+5211210 | 91.731      | 3.834       | 4.158      | 8            | —          | —          | —           | —          | —           | —             | —           | —            | —           | U           | —           | —           | 13.218      | ...         | 1.45        | —    | 18.6 | 1.00  | 3.73  | 11.669      | ...         | −0.62       | 1.29        | ...   | ...         | ...           | −0.35         |
| 21013606+5200199 | 91.598      | 3.707       | 4.389      | 9            | —          | —          | —           | —          | —           | —             | —           | —            | —           | U           | —           | —           | 13.050      | 0.38        | 1.14        | 2    | 15.0 | 0.68  | 3.89  | 11.415      | −0.35       | −1.04       | 1.36        | ...   | ...         | −0.26         | −0.75         |
| 21013667+5157530 | 91.568      | 3.679       | 4.395      | 8            | —          | —          | —           | —          | —           | —             | —           | —            | —           | U           | —           | —           | 13.020      | 0.44        | 1.53        | —    | 21.4 | 1.00  | 3.93  | 11.382      | −0.28       | −0.65       | 1.36        | ...   | ...         | −0.20         | −0.36         |
| 21021554+5129450 | 91.281      | 3.294       | 4.396      | 9            | —          | —          | —           | —          | —           | —             | —           | —            | —           | U           | —           | —           | 13.207      | 0.86        | 1.00        | 2    | 20.6 | 0.74  | 3.94  | 11.569      | 0.13        | −1.18       | 1.36        | ...   | ...         | 0.22          | −0.89         |
| 21024143+5128447 | 91.313      | 3.233       | 4.362      | 9            | —          | —          | —           | —          | —           | —             | —           | —            | —           | U           | —           | —           | 13.167      | 0.30        | 1.33        | 2    | 14.4 | 0.66  | 3.96  | 11.542      | −0.42       | −0.84       | 1.35        | ...   | ...         | −0.33         | −0.55         |
| 21024184+5101107 | 90.969      | 2.927       | 4.030      | 8            | —          | —          | —           | —          | —           | —             | —           | —            | —           | U           | —           | —           | 12.778      | 0.58        | 1.75        | 1    | 17.6 | 0.68  | 3.97  | 11.276      | −0.08       | −0.25       | 1.25        | ...   | ...         | −0.01         | 0.01          |
| 21045981+5205310 | 92.009      | 3.374       | 4.165      | 8            | —          | —          | —           | —          | —           | —             | —           | —            | —           | U           | —           | —           | 13.063      | 0.94        | 2.07        | —    | 17.6 | 0.50  | 3.91  | 11.511      | 0.25        | 0.01        | 1.29        | ...   | ...         | 0.34          | 0.28          |
| 21051672+5148399 | 91.829      | 3.154       | 4.168      | 9            | —          | —          | —           | —          | —           | —             | —           | —            | —           | U           | —           | —           | 13.077      | 0.70        | 1.89        | —    | 17.4 | 1.00  | 4.05  | 11.524      | 0.01        | −0.18       | 1.29        | ...   | ...         | 0.09          | 0.09          |
| 21061271+4934293 | 90.267      | 1.545       | 4.886      | 8            | —          | —          | —           | —          | —           | —             | —           | —            | —           | U           | —           | —           | 13.286      | ...         | 1.35        | —    | 12.0 | 1.00  | 4.16  | 11.465      | ...         | −1.08       | 1.51        | ...   | ...         | ...           | −0.75         |
| 21063958+5118322 | 91.600      | 2.658       | 5.395      | 8            | —          | —          | —           | —          | —           | —             | —           | —            | —           | U           | —           | —           | 13.415      | 0.51        | ...         | —    | 16.0 | 0.58  | 4.10  | 11.405      | −0.38       | ...         | 1.67        | ...   | ...         | −0.27         | ...           |
| 21083907+5133019 | 91.988      | 2.592       | 3.809      | 8            | —          | —          | —           | —          | —           | —             | —           | —            | —           | U           | —           | —           | 12.913      | 0.63        | 1.63        | −2   | 17.2 | 0.68  | 4.02  | 11.494      | 0.00        | −0.26       | 1.18        | ...   | ...         | 0.08          | −0.01         |
| 21100007+5156291 | 92.418      | 2.703       | 4.756      | 8            | —          | —          | —           | —          | —           | —             | —           | —            | —           | U           | —           | —           | 13.360      | ...         | ...         | —    | 14.6 | 1.00  | 4.03  | 11.588      | ...         | ...         | 1.47        | ...   | ...         | ...           | ...           |
| 21132201+5244357 | 93.355      | 2.877       | 4.717      | 8            | —          | —          | —           | —          | —           | —             | —           | —            | —           | U           | —           | —           | 13.158      | 0.44        | 1.95        | —    | 10.0 | 1.00  | 4.00  | 11.400      | −0.34       | −0.39       | 1.46        | ...   | ...         | −0.25         | −0.08         |
| 21150444+5014113 | 91.725      | 0.954       | 2.829      | 1            | —          | —          | g           | t          | —           | —             | D1          | —            | —           | U           | —           | —           | 12.336      | 0.91        | ...         | 1    | 32.8 | 0.30  | 4.16  | 11.282      | 0.44        | ...         | 0.88        | 49.0  | 11.09       | 0.49          | ...           |
| 21155544+5443301 | 95.053      | 3.973       | 2.417      | 7            | —          | —          | —           | —          | —           | —             | —           | —            | —           | U           | —           | —           | 12.211      | 1.22        | ...         | −2   | 22.4 | 1.00  | 3.97  | 11.310      | 0.82        | ...         | 0.75        | ...   | ...         | 0.87          | ...           |
| 21173550+5121513 | 92.812      | 1.453       | 2.594      | 1            | —          | —          | g           | —          | —           | —             | D2          | —            | —           | U           | —           | —           | 12.267      | 0.74        | 1.87        | 1    | 24.4 | 0.72  | 4.10  | 11.300      | 0.31        | 0.58        | 0.80        | 34.5  | 11.17       | 0.36          | 0.75          |
| 21174741+5138523 | 93.036      | 1.629       | 3.131      | 7            | o          | —          | —           | —          | —           | —             | —           | —            | —           | U           | o           | e?          | 12.606      | ...         | ...         | 1    | 19.6 | 1.0   | 4.13  | 11.439      | ...         | ...         | 0.97        | ...   | ...         | ...           | ...           |
| 21174968+5248294 | 93.871      | 2.436       | 3.007      | 1            | —          | —          | g           | —          | —           | —             | n           | —            | —           | U           | —           | —           | 12.425      | 0.75        | ...         | 1    | 20.4 | 0.86  | 4.05  | 11.305      | 0.25        | ...         | 0.93        | 31.2  | 11.12       | 0.31          | ...           |
| 21215277+5226477 | 94.047      | 1.745       | 4.215      | 8            | —          | —          | —           | —          | —           | —             | —           | —            | —           | U           | —           | —           | 13.015      | 0.80        | ...         | −2   | 15.4 | 0.54  | 4.07  | 11.444      | 0.10        | ...         | 1.31        | ...   | ...         | 0.18          | ...           |
| 21341021+5134177 | 94.811      | −0.193      | 4.161      | 9            | —          | —          | —           | —          | —           | —             | —           | —            | —           | U           | —           | —           | 13.068      | 0.75        | 1.55        | 2    | 17.8 | 1.00  | 4.10  | 11.518      | 0.06        | −0.52       | 1.29        | ...   | ...         | 0.14          | −0.25         |
| 21380138+5020132 | 94.434      | −1.516      | 3.871      | 9            | —          | —          | —           | —          | —           | —             | —           | —            | —           | U           | —           | —           | 13.028      | 0.57        | 1.16        | 2    | 29.0 | 0.64  | 4.05  | 11.586      | −0.07       | −0.76       | 1.20        | ...   | ...         | 0.01          | −0.50         |
| 21572904+5921414 | 102.357     | 3.628       | 3.259      | 9            | —          | —          | —           | —          | —           | —             | —           | —            | —           | U           | —           | —           | 12.475      | 0.80        | 1.87        | −2   | 42.4 | 0.54  | 4.00  | 11.261      | 0.26        | 0.25        | 1.01        | ...   | ...         | 0.33          | 0.47          |
| 21584713+5518145 | 100.015     | 0.309       | 2.077      | 1            | —          | —          | g           | —          | —           | —             | D2          | —            | —           | U           | —           | —           | 12.067      | 0.61        | 1.88        | 1    | 22.0 | 0.96  | 4.08  | 11.293      | 0.26        | 0.85        | 0.64        | 28.0  | 11.24       | 0.30          | 0.99          |
| 22094097+5834093 | 103.149     | 2.055       | 2.158      | 7            | —          | —          | —           | —          | —           | —             | —           | —            | —           | U           | —           | —           | 12.175      | 1.13        | ...         | 1    | 24.2 | 1.00  | 3.98  | 11.371      | 0.77        | ...         | 0.67        | ...   | ...         | 0.82          | ...           |
| 22140348+5953479 | 104.368     | 2.824       | 2.555      | 8            | o          | —          | —           | —          | —           | —             | —           | —            | —           | U           | o           | —           | 12.214      | 1.50        | ...         | 1    | 20.2 | 0.64  | 3.95  | 11.262      | 1.07        | ...         | 0.79        | ...   | ...         | 1.13          | ...           |
| 22144149+6126492 | 105.308     | 4.061       | 5.469      | 9            | —          | —          | —           | —          | —           | —             | —           | —            | —           | U           | —           | —           | 13.380      | 0.57        | 1.55        | −1   | 17.4 | 0.42  | 4.01  | 11.342      | −0.33       | −1.16       | 1.69        | ...   | ...         | −0.23         | −0.80         |
| 22185162+5813496 | 103.951     | 1.097       | 2.026      | 8            | —          | —          | —           | —          | —           | —             | —           | —            | —           | U           | —           | —           | 12.078      | 0.75        | 1.87        | 1    | 24.2 | 0.88  | 3.98  | 11.323      | 0.41        | 0.86        | 0.63        | ...   | ...         | 0.45          | 1.00          |
| 22203042+5736196 | 103.792     | 0.454       | 2.734      | 8            | —          | p          | —           | —          | —           | —             | —           | —            | —           | U           | —           | —           | 12.438      | ...         | ...         | −2   | 30.8 | 0.38  | 4.00  | 11.419      | ...         | ...         | 0.85        | ...   | ...         | ...           | ...           |
| 22214374+6357196 | 107.376     | 5.703       | 2.998      | 8            | —          | —          | —           | —          | —           | —             | —           | —            | —           | U           | —           | —           | 12.448      | 1.31        | ...         | 1    | 26.2 | 0.52  | 3.75  | 11.331      | 0.81        | ...         | 0.93        | ...   | ...         | 0.87          | ...           |
| 22220701+5842511 | 104.572     | 1.271       | 5.678      | 9            | —          | —          | —           | —          | —           | —             | —           | —            | —           | U           | —           | —           | 13.428      | 0.46        | 1.18        | −1   | 14.4 | 0.50  | 4.02  | 11.312      | −0.48       | −1.64       | 1.76        | ...   | ...         | −0.37         | −1.27         |
| 22283285+6255454 | 107.476     | 4.428       | 2.280      | 8            | —          | —          | —           | —          | —           | —             | —           | —            | —           | U           | —           | —           | 12.119      | 1.25        | 1.78        | −2   | 16.4 | 0.56  | 3.85  | 11.269      | 0.88        | 0.65        | 0.71        | ...   | ...         | 0.92          | 0.80          |
| 22422911+6212129 | 108.508     | 2.999       | 2.184      | 3            | —          | —          | g           | t          | —           | —             | D3          | —            | —           | U           | —           | —           | 12.131      | 0.64        | 1.83        | −2   | 25.2 | 0.60  | 3.95  | 11.317      | 0.28        | 0.74        | 0.68        | 32.8  | 11.24       | 0.32          | 0.89          |
| 22463421+5759472 | 106.987     | −0.956      | 3.315      | 7            | —          | —          | —           | —          | —           | —             | —           | —            | —           | U           | —           | —           | 12.674      | 1.15        | ...         | −2   | 20.0 | 0.62  | 4.04  | 11.439      | 0.60        | ...         | 1.03        | ...   | ...         | 0.67          | ...           |
| 22545807+6207283 | 109.771     | 2.267       | 5.089      | 7            | —          | —          | —           | —          | —           | —             | —           | —            | —           | U           | —           | —           | 113.195     | 0.50        | 1.46        | −2   | 10.8 | 0.60  | 3.91  | 11.299      | −0.34       | −1.07       | 1.58        | ...   | ...         | −0.24         | −0.74         |
| 22565926+6043008 | 109.384     | 0.892       | 2.263      | 5            | o          | —          | p           | —          | —           | —             | n           | —            | —           | U           | o           | —           | 12.150      | 0.67        | 1.73        | 1    | 19.2 | 0.80  | 3.93  | 11.307      | 0.30        | 0.60        | 0.70        | 25.0  | 11.25       | 0.34          | 0.75          |
| 23052373+6007539 | 110.088     | −0.069      | 5.653      | 9            | —          | —          | —           | —          | —           | —             | —           | —            | —           | U           | —           | —           | 13.529      | ...         | ...         | −2   | 20.4 | 0.26  | 4.05  | 11.423      | ...         | ...         | 1.75        | ...   | ...         | ...           | ...           |
| 23095557+5958289 | 110.548     | −0.433      | 3.430      | 8            | o          | —          | —           | —          | —           | —             | —           | —            | —           | U           | o           | —           | 12.754      | ...         | ...         | 1    | 34.2 | 0.40  | 3.88  | 11.476      | ...         | ...         | 1.06        | ...   | ...         | ...           | ...           |
| 23151265+6000055 | 111.171     | −0.654      | 5.264      | 6            | —          | —          | —           | —          | —           | —             | —           | —            | —           | U           | —           | e           | 13.358      | ...         | ...         | −1   | 11.2 | 1.00  | 4.07  | 11.397      | ...         | ...         | 1.63        | ...   | ...         | ...           | ...           |
| 23161302+6124141 | 111.792     | 0.609       | 4.278      | 7            | —          | —          | —           | —          | —           | —             | —           | —            | —           | U           | —           | —           | 12.887      | 1.07        | 2.78        | −2   | 10.2 | 1.00  | 3.93  | 11.293      | 0.36        | 0.66        | 1.33        | ...   | ...         | 0.45          | 0.94          |
| 23172479+5929296 | 111.247     | −1.230      | 4.637      | 9            | —          | —          | —           | —          | —           | —             | —           | —            | —           | U           | —           | —           | 13.196      | ...         | 1.44        | −1   | 15.2 | 1.00  | 3.92  | 11.468      | ...         | −0.87       | 1.44        | ...   | ...         | ...           | −0.56         |
| 23173430+6007042 | 111.488     | −0.651      | 5.106      | 7            | —          | —          | —           | —          | —           | —             | —           | —            | —           | U           | —           | —           | 13.164      | 0.87        | ...         | −1   | 12.6 | 1.00  | 3.98  | 11.262      | 0.03        | ...         | 1.58        | ...   | ...         | 0.13          | ...           |
| 23331774+60      |             |             |            |              |            |            |             |            |             |               |             |              |             |             |             |             |             |             |             |      |      |       |       |             |             |             |             |       |             |               |               |

Table B2: b) 2MASS EBV supplementary sample

| 2MASX J          | $l$<br>deg<br>(1) | $b$<br>deg<br>(2a) | EBV<br>mag<br>(2b) | Object<br>class<br>(3) | off<br>(4) | flg<br>(5) | gal<br>(6) | TF<br>(7a) | obs<br>(7b) | ext'd<br>(7c) | Disc<br>type<br>(7d) | 2MRS<br>(8) | Velocity<br>Opt<br>(9) | HI<br>(10a) | NIR<br>flg<br>(10b) | Photom<br>flg<br>(11) | Ext<br>flg<br>(12) | $K_{20}$<br>mag<br>(13) | $H-K$<br>mag<br>(14) | $J-K$<br>mag<br>(15) | vc<br>(16) | $a$<br>" (17) | $b/a$<br>(18) | st.d.<br>(19) | $K_s^O$<br>mag<br>(20) | $(H-K)^O$<br>mag<br>(21) | $(J-K)^O$<br>mag<br>(22) | $A_K$<br>mag<br>(23) | $a''$<br>mag<br>(24) | $K_s^{O,d}$<br>mag<br>(25) | $(H-K)^{O,c}$<br>mag<br>(26) | $(J-K)^{O,c}$<br>mag<br>(27) |
|------------------|-------------------|--------------------|--------------------|------------------------|------------|------------|------------|------------|-------------|---------------|----------------------|-------------|------------------------|-------------|---------------------|-----------------------|--------------------|-------------------------|----------------------|----------------------|------------|---------------|---------------|---------------|------------------------|--------------------------|--------------------------|----------------------|----------------------|----------------------------|------------------------------|------------------------------|
| 03435514+3201035 | 160.477           | -18.002            | 3.374              | 9                      | -          | -          | -          | -          | -           | -             | -                    | -           | -                      | -           | -                   | -                     | -                  | 12.545                  | 1.71                 | ...                  | 1          | 43.6          | 0.24          | 3.11          | 11.288                 | 1.15                     | ...                      | 1.05                 | ...                  | ...                        | 1.22                         | ...                          |
| 05213602-6754432 | 278.336           | -33.392            | 3.276              | 7                      | -          | -          | -          | -          | -           | -             | -                    | -           | -                      | -           | -                   | -                     | -                  | 12.502                  | 0.36                 | 0.49                 | -2         | 45.6          | 0.36          | 3.65          | 11.281                 | -0.18                    | -1.14                    | 1.01                 | ...                  | ...                        | -0.11                        | -0.92                        |
| 05215652-6757335 | 278.385           | -33.352            | 4.395              | 8                      | -          | -          | -          | -          | -           | -             | -                    | -           | -                      | -           | -                   | -                     | -                  | 13.349                  | ...                  | 0.78                 | 1          | 34.6          | 1.00          | 3.75          | 11.711                 | ...                      | -1.40                    | 1.36                 | ...                  | ...                        | ...                          | -1.11                        |
| 05340344-0520512 | 208.825           | -19.635            | 3.904              | 8                      | -          | -          | -          | -          | -           | -             | -                    | -           | -                      | -           | -                   | -                     | -                  | 13.174                  | 0.57                 | 1.24                 | -2         | 25.6          | 0.64          | 3.26          | 11.719                 | -0.07                    | -0.70                    | 1.21                 | ...                  | ...                        | 0.00                         | -0.44                        |
| 05341218-0525075 | 208.910           | -19.635            | 3.979              | 3                      | -          | -          | g          | t          | -           | -             | D1                   | -           | -                      | -           | -                   | -                     | e                  | 12.906                  | 0.53                 | 2.10                 | 1          | 18.6          | 0.44          | 3.42          | 11.423                 | -0.12                    | 0.12                     | 1.23                 | 34.0                 | 11.14                      | -0.05                        | 0.38                         |
| 05343294-0522144 | 208.906           | -19.536            | 6.071              | 9                      | -          | -          | -          | -          | -           | -             | -                    | -           | -                      | -           | -                   | -                     | -                  | 14.143                  | 0.45                 | 0.67                 | 0          | 26.4          | 0.18          | 3.33          | 11.881                 | -0.56                    | -2.34                    | 1.88                 | ...                  | ...                        | -0.44                        | -1.94                        |
| 05353259-0540125 | 209.308           | -19.451            | 3.558              | 9                      | -          | -          | -          | -          | -           | -             | -                    | -           | -                      | -           | -                   | -                     | -                  | 12.634                  | 0.61                 | 1.48                 | 1          | 38.8          | 0.42          | 3.36          | 11.308                 | 0.03                     | -0.29                    | 1.10                 | ...                  | ...                        | 0.10                         | -0.05                        |
| 05360847-0523395 | 209.118           | -19.194            | 6.819              | 8                      | -          | -          | -          | -          | -           | -             | -                    | -           | -                      | -           | -                   | -                     | -                  | 13.926                  | ...                  | ...                  | 1          | 12.8          | 1.00          | 3.27          | 11.385                 | ...                      | ...                      | 2.11                 | ...                  | ...                        | ...                          | ...                          |
| 05360947-0526535 | 209.171           | -19.214            | 5.606              | 8                      | -          | -          | -          | -          | -           | -             | -                    | -           | -                      | -           | -                   | -                     | -                  | 13.849                  | 0.46                 | 1.58                 | -2         | 12.8          | 0.68          | 3.27          | 11.760                 | -0.47                    | -1.20                    | 1.74                 | ...                  | ...                        | -0.36                        | -0.83                        |
| 05383994-0658291 | 210.913           | -19.341            | 4.241              | 8                      | -          | -          | -          | -          | -           | -             | -                    | -           | -                      | -           | -                   | -                     | -                  | 12.854                  | ...                  | ...                  | 1          | 25.4          | 1.00          | 3.35          | 11.274                 | ...                      | ...                      | 1.31                 | ...                  | ...                        | ...                          | ...                          |
| 05401277-6933048 | 279.973           | -31.489            | 5.717              | 9                      | -          | -          | -          | -          | -           | -             | -                    | -           | -                      | -           | -                   | -                     | -                  | 13.418                  | 0.23                 | 0.93                 | 2          | 12.0          | 1.00          | 3.95          | 11.288                 | -0.72                    | -1.91                    | 1.77                 | ...                  | ...                        | -0.60                        | -1.53                        |
| 16243864-2431456 | 352.687           | 17.131             | 3.791              | 8                      | -          | -          | -          | -          | -           | -             | -                    | -           | -                      | -           | -                   | -                     | -                  | 12.673                  | 2.18                 | ...                  | 1          | 23.2          | 1.00          | 3.34          | 11.260                 | 1.55                     | ...                      | 1.17                 | ...                  | ...                        | 1.62                         | ...                          |
| 16253068-2439384 | 352.722           | 16.896             | 6.194              | 8                      | -          | -          | -          | -          | -           | -             | -                    | -           | -                      | -           | -                   | -                     | -                  | 13.709                  | 0.46                 | 1.55                 | -1         | 10.0          | 1.00          | 3.41          | 11.401                 | -0.56                    | -1.53                    | 1.92                 | ...                  | ...                        | -0.44                        | -1.12                        |
| 21013880+6814468 | 104.130           | 14.243             | 6.119              | 7                      | -          | -          | -          | -          | -           | -             | -                    | -           | -                      | -           | -                   | -                     | -                  | 13.650                  | 0.60                 | 1.83                 | -1         | 12.6          | 1.00          | 3.30          | 11.370                 | -0.41                    | -1.20                    | 1.90                 | ...                  | ...                        | -0.29                        | -0.80                        |
